# Supplementary material for: Symmetry Restoration in the SMEFT: Finite Counterterms for a Non-Anticommuting $\gamma_5$
Source: arXiv:2507.19589 ancillary file (2026-02-13)
Supplement: Supplementary file 1 [file Suplemental.pdf]

# Symmetry-Restoring SMEFT Counterterms

|                                                               |          |
|---------------------------------------------------------------|----------|
| <b>Contents</b>                                               | <b>1</b> |
| 1 The SMEFT Lagrangian and Conventions . . . . .              | 1        |
| 2 Symmetry-restoring counterterms in the SMEFT . . . . .      | 2        |
| 2.1 Renormalizable operators . . . . .                        | 2        |
| 2.2 Dimension five: Weinberg operator . . . . .               | 3        |
| 2.3 Dimension six: bosonic operators . . . . .                | 3        |
| 2.4 Dimension six: semibosonic operators . . . . .            | 5        |
| 2.5 Dimension six: four-fermion operators . . . . .           | 41       |
| 3 Spurion-dependent symmetry-restoring counterterms . . . . . | 68       |
| 3.1 Renormalizable operators . . . . .                        | 68       |
| 3.2 Dimension five: Weinberg operator . . . . .               | 69       |
| 3.3 Dimension six: bosonic operators . . . . .                | 70       |
| 3.4 Dimension six: semibosonic operators . . . . .            | 72       |
| 3.5 Dimension six: four-fermion operators . . . . .           | 101      |

## 1 The SMEFT Lagrangian and Conventions

The four-dimensional SM Lagrangian is defined according to the following conventions:

$$\begin{aligned}
\mathcal{L}_{\text{SM}} = & -\frac{1}{4}G_{\mu\nu}^A G^{\mu\nu A} - \frac{1}{4}W_{\mu\nu}^I W^{\mu\nu I} - \frac{1}{4}B_{\mu\nu} B^{\mu\nu} + (D_\mu H)^\dagger (D^\mu H) + \mu^2 (H^\dagger H) - \frac{\lambda}{2} (H^\dagger H)^2 \\
& + \sum_{\psi=q,u,d,\ell,e} \bar{\psi} i \not{D} \psi - \left( y_u^{pr} \bar{q}_p \tilde{H} u_r + y_d^{pr} \bar{q}_p H d_r + y_e^{pr} \bar{\ell}_p H e_r + \text{h.c.} \right) + \mathcal{L}_{\text{gf}}, \quad (1.1)
\end{aligned}$$

where, as discussed in the main text, we employ the background-field gauge due to its technical advantages. We note, however, that ghost fields play no role in our computation, as they do not couple to chiral fermions. Their contributions must nevertheless be accounted for at higher-loop orders. The matter content follows standard conventions, with  $p$  and  $r$  denoting flavor indices. The conjugated Higgs doublet is defined by  $\tilde{H}^i = \varepsilon^{ij} H_j^*$ , where  $\varepsilon^{ij}$  is the antisymmetric SU(2) tensor with  $\varepsilon^{12} = +1$  and  $\varepsilon^{ij} = -\varepsilon^{ji}$ . The covariant derivative takes the form

$$D_\mu = \partial_\mu - ig_s T^A G_\mu^A - ig_L t^I W_\mu^I - ig_Y Y B_\mu, \quad (1.2)$$

where the SU(3)<sub>c</sub> and SU(2)<sub>L</sub> generators are  $T^A = \lambda^A/2$  and  $t^I = \tau^I/2$ , with  $\lambda^A$  and  $\tau^I$  the Gell-Mann and Pauli matrices, respectively. For the U(1)<sub>Y</sub> hypercharge  $Y$ , we follow the conventions of [1]. The associated gauge couplings are denoted by  $g_s$ ,  $g_L$ , and  $g_Y$ , respectively.

The field-strength tensors are

$$\begin{aligned}
G_{\mu\nu}^A &= \partial_\mu G_\nu^A - \partial_\nu G_\mu^A + g_s f_{ABC} G_\mu^B G_\nu^C, \\
W_{\mu\nu}^I &= \partial_\mu W_\nu^I - \partial_\nu W_\mu^I + g_L \varepsilon_{IJK} W_\mu^J W_\nu^K, \\
B_{\mu\nu} &= \partial_\mu B_\nu - \partial_\nu B_\mu,
\end{aligned} \tag{1.3}$$

where  $f_{ABC}$  and  $\varepsilon_{IJK}$  are the structure constants of  $SU(3)_c$  and  $SU(2)_L$ , respectively. For the SMEFT Lagrangian, we include only dimension-six operators in the Warsaw basis [1], where dual field strength tensors are defined by  $\tilde{X}^{\mu\nu} = \frac{1}{2} \varepsilon^{\mu\nu\rho\sigma} X_{\rho\sigma}$  with the convention  $\varepsilon^{0123} = +1$ .

The extension of the SMEFT Lagrangian to  $d$  dimensions in the BMHV scheme follows the conventions detailed in Section 2.2 of the main text. In particular, the gauge symmetry is kept strictly four-dimensional while the field content is extended with five spurion fields  $\Omega_\psi(x_{\bar{\mu}})$  (with  $\psi = q, u, d, \ell, e$ ), which enter in the evanescent fermionic kinetic terms as prescribed in (2.15) of the main text:

$$\begin{aligned}
\mathcal{L}_{(d)}^{\text{Fer}} &= i \bar{q}_{aip} \gamma^{\bar{\mu}} P_L D_{\bar{\mu}} q_p^{ai} + i \bar{q}_{ev,\hat{\alpha}p} \gamma^{\bar{\mu}} P_R \partial_{\bar{\mu}} q_{ev,p}^{\hat{\alpha}} + \left[ i \bar{q}_{aip} (\Omega_q)^{ai} \gamma^{\hat{\mu}} P_R \partial_{\bar{\mu}} q_{ev,p}^{\hat{\alpha}} + \text{h.c.} \right] \\
&+ i \bar{u}_{ap} \gamma^{\bar{\mu}} P_R D_{\bar{\mu}} u_p^a + i \bar{u}_{ev,\hat{\alpha}p} \gamma^{\bar{\mu}} P_L \partial_{\bar{\mu}} u_{ev,p}^{\hat{\alpha}} + \left[ i \bar{u}_{ap} (\Omega_u)^i \gamma^{\hat{\mu}} P_L \partial_{\bar{\mu}} u_{ev,p}^{\hat{\alpha}} + \text{h.c.} \right] \\
&+ i \bar{d}_{ap} \gamma^{\bar{\mu}} P_R D_{\bar{\mu}} d_p^a + i \bar{d}_{ev,\hat{\alpha}p} \gamma^{\bar{\mu}} P_L \partial_{\bar{\mu}} d_{ev,p}^{\hat{\alpha}} + \left[ i \bar{d}_{ap} (\Omega_d)^i \gamma^{\hat{\mu}} P_L \partial_{\bar{\mu}} d_{ev,p}^{\hat{\alpha}} + \text{h.c.} \right] \\
&+ i \bar{\ell}_{ip} \gamma^{\bar{\mu}} P_L D_{\bar{\mu}} \ell_p^i + i \bar{\ell}_{ev,\hat{\alpha}p} \gamma^{\bar{\mu}} P_R \partial_{\bar{\mu}} \ell_{ev,p}^{\hat{\alpha}} + \left[ i \bar{\ell}_{ip} (\Omega_\ell)^i \gamma^{\hat{\mu}} P_R \partial_{\bar{\mu}} \ell_{ev,p}^{\hat{\alpha}} + \text{h.c.} \right] \\
&+ i \bar{e}_p \gamma^{\bar{\mu}} P_R D_{\bar{\mu}} e_p + i \bar{e}_{ev,p} \gamma^{\bar{\mu}} P_L \partial_{\bar{\mu}} e_{ev,p} + \left( i \bar{e}_p \Omega_e \gamma^{\hat{\mu}} P_L \partial_{\bar{\mu}} e_{ev,p} + \text{h.c.} \right).
\end{aligned} \tag{1.4}$$

The indices  $a$  and  $i$  are fundamental  $SU(3)_c$  and  $SU(2)_L$  indices, respectively while  $p \in \{1, 2, 3\}$  denotes the flavor index. The  $\hat{\alpha}$  index is used for all spurion flavors, although they are not technically the same between different species.

We adopt a scheme in which all gamma matrices appearing in dimension-six operators are treated as strictly four-dimensional. This choice is fully general, since any evanescent contributions can be absorbed into finite renormalization of the physical couplings.

## 2 Symmetry-restoring counterterms in the SMEFT

Here, we present the finite restoring counterterms after performing the identity limit  $\Omega \rightarrow \mathbb{1}$  for the different spurions. Thus, the result is given in terms of the different gauge bosons, leading to gauge-variant terms. In the results below, we leave fundamental gauge indices implicit whenever possible. We also use the notation  $\overline{W}^I = W_{\bar{\mu}}^I \gamma^{\bar{\mu}}$ , and similarly for other gauge bosons, for compactness.

### 2.1 Renormalizable operators

We present here the results for the dimension-4 SMEFT operators, i.e. those of the SM. To the best of our knowledge, this is the first time these counterterms have been computed with the evanescent-partner scheme, defined by (1.4).

$$\begin{aligned}
\Delta S_{\text{SM}} = & \frac{1}{216} g_Y \left[ \left[ 119g_Y^2 - 27g_L^2 - 48g_s^2 \right] \delta^{rs} + 36y_d^{st} \bar{y}_d^{rt} - 72y_u^{st} \bar{y}_u^{rt} \right] (\bar{q}_s \bar{B} q_r) \\
& + \frac{1}{54} g_Y \left[ 2 \left[ 12g_s^2 - 29g_Y^2 \right] \delta^{rs} - 9y_d^{tr} \bar{y}_d^{ts} \right] (\bar{d}_s \bar{B} d_r) + \frac{1}{54} g_Y \left[ 8 \left[ 13g_Y^2 - 6g_s^2 \right] \delta^{rs} - 9y_u^{tr} \bar{y}_u^{ts} \right] (\bar{u}_s \bar{B} u_r) \\
& + \frac{1}{36} g_s \left[ - \left[ g_Y^2 + 27g_L^2 - 78g_s^2 \right] \delta^{rs} - 18y_d^{st} \bar{y}_d^{rt} - 18y_u^{st} \bar{y}_u^{rt} \right] (\bar{q}_s T^A \bar{G}^A q_r) + \frac{1}{36} g_L \left[ 81g_L^2 - g_Y^2 - 48g_s^2 \right] (\bar{q}_s t^I \bar{W}^I q_s) \\
& + \frac{1}{24} g_Y \left[ \left[ 9g_L^2 - 37g_Y^2 \right] \delta^{rs} + 12y_e^{st} \bar{y}_e^{rt} \right] (\bar{\ell}_s \bar{B} \ell_r) + \frac{1}{12} g_L^2 g_Y^2 B_\mu^2 W_\nu^{I2} \\
& + \frac{1}{12} g_Y^2 \left[ 20g_Y^2 - 7y_d^{rs} \bar{y}_d^{rs} - 9y_e^{rs} \bar{y}_e^{rs} - 13y_u^{rs} \bar{y}_u^{rs} \right] (H^\dagger H) B_\mu^2 + \frac{1}{8} g_L^2 g_s^2 G_\mu^{A2} W_\nu^{I2} + \frac{11}{72} g_s^2 g_Y^2 B_\mu^2 G_\nu^{A2} \\
& + \frac{1}{6} g_s^3 g_Y d^{ABC} B_\mu G_\mu^A G_\nu^B G_\nu^C + \frac{1}{6} g_L^2 g_Y^2 B_\mu B_\nu W_\mu^I W_\nu^I \\
& + \frac{i}{6} g_Y \left[ 10g_Y^2 - y_e^{rs} \bar{y}_e^{rs} - 3y_d^{rs} \bar{y}_d^{rs} - 3y_u^{rs} \bar{y}_u^{rs} \right] (H^\dagger \overset{\leftrightarrow}{\partial}_\mu H) B_\mu + \frac{1}{4} g_L^2 g_s^2 G_\mu^A G_\nu^A W_\mu^I W_\nu^I \\
& + \frac{1}{4} g_L^4 W_\mu^I W_\mu^J W_\nu^I W_\nu^J + \frac{1}{4} g_L^2 \left[ 4g_L^2 - y_e^{rs} \bar{y}_e^{rs} - 3y_d^{rs} \bar{y}_d^{rs} - 3y_u^{rs} \bar{y}_u^{rs} \right] (H^\dagger H) W_\mu^{I2} \\
& + \frac{1}{4} g_L \left[ 9g_L^2 - g_Y^2 \right] (\bar{\ell}_s t^I \bar{W}^I \ell_s) + \frac{11}{36} g_s^2 g_Y^2 B_\mu B_\nu G_\mu^A G_\nu^A \\
& + \frac{i}{3} g_L \left[ 6g_L^2 - y_e^{rs} \bar{y}_e^{rs} - 3y_d^{rs} \bar{y}_d^{rs} - 3y_u^{rs} \bar{y}_u^{rs} \right] (H^\dagger t^I \overset{\leftrightarrow}{\partial}_\mu H) W_\mu^I + \frac{95}{216} g_Y^4 B_\mu^2 B_\nu^2 \\
& + \frac{1}{2} g_s^2 \left[ - y_d^{rs} \bar{y}_d^{rs} - y_u^{rs} \bar{y}_u^{rs} \right] (H^\dagger H) G_\mu^{A2} + g_s^4 \text{tr}\{T^A T^B T^C T^D\} G_\mu^B G_\mu^D G_\nu^A G_\nu^C \\
& + g_L g_Y \left[ 2g_L^2 + \frac{10}{3} g_Y^2 - y_u^{rs} \bar{y}_u^{rs} - 2y_d^{rs} \bar{y}_d^{rs} \right] (H^\dagger t^I H) B_\mu W_\mu^I + g_s \left[ \frac{1}{18} \left[ 39g_s^2 - 2g_Y^2 \right] \delta^{rs} - y_d^{tr} \bar{y}_d^{ts} \right] (\bar{d}_s T^A \bar{G}^A d_r) \\
& + g_Y \left[ \frac{1}{2} y_e^{tr} \bar{y}_e^{ts} - \frac{7}{3} g_Y^2 \delta^{rs} \right] (\bar{e}_s \bar{B} e_r) + g_s \left[ \frac{1}{18} \left[ 39g_s^2 - 8g_Y^2 \right] \delta^{rs} - y_u^{tr} \bar{y}_u^{ts} \right] (\bar{u}_s T^A \bar{G}^A u_r) \\
& - \frac{1}{8} g_L^4 W_\mu^{I2} W_\nu^{J2} - g_s^2 \partial^\mu G_\mu^A \partial^\nu G_\nu^A - g_L^2 \partial^\mu W_\mu^I \partial^\nu W_\nu^I - \frac{5}{3} g_Y^2 \partial^\mu B_\mu \partial^\nu B_\nu \\
& - 2g_s^2 G_\mu^A \partial^2 G_\mu^A - 2g_L^2 W_\mu^I \partial^2 W_\mu^I - 2g_s^2 (\partial^\mu G_\mu^A)^2 - 2g_L^2 (\partial^\mu W_\mu^I)^2 - 2g_s^2 G_\mu^A \partial^\mu \partial^\nu G_\nu^A \\
& - 2g_L^2 W_\mu^I \partial^\mu \partial^\nu W_\nu^I - \frac{10}{3} g_Y^2 B_\mu \partial^2 B_\mu - \frac{10}{3} g_Y^2 (\partial^\mu B_\mu)^2 - \frac{10}{3} g_Y^2 B_\mu \partial^\mu \partial^\nu B_\nu. \tag{2.1}
\end{aligned}$$

## 2.2 Dimension five: Weinberg operator

$$\begin{aligned}
\Delta S_{\mathcal{O}_{\ell\ell HH}} = & -g_L^2 \bar{\mathcal{C}}_{\ell\ell HH}^{rs} \mathcal{C}_{\ell\ell HH}^{rs} (H^\dagger H)^2 W_\mu^{I2} - \frac{4i}{3} g_Y \bar{\mathcal{C}}_{\ell\ell HH}^{rs} \mathcal{C}_{\ell\ell HH}^{rs} (H^\dagger \overset{\leftrightarrow}{\partial}_\mu H) (H^\dagger H) B_\mu \\
& - \frac{4i}{3} g_L \bar{\mathcal{C}}_{\ell\ell HH}^{rs} \mathcal{C}_{\ell\ell HH}^{rs} (H^\dagger \overset{\leftrightarrow}{\partial}_\mu H) (H^\dagger t^I H) W_\mu^I - \frac{4i}{3} g_L \bar{\mathcal{C}}_{\ell\ell HH}^{rs} \mathcal{C}_{\ell\ell HH}^{rs} (H^\dagger t^I \overset{\leftrightarrow}{\partial}_\mu H) (H^\dagger H) W_\mu^I \\
& + 2g_L \bar{\mathcal{C}}_{\ell\ell HH}^{st} \mathcal{C}_{\ell\ell HH}^{rt} (H^\dagger H) (\bar{\ell}_s t^I \bar{W}^I \ell_r) + 4g_Y \bar{\mathcal{C}}_{\ell\ell HH}^{st} \mathcal{C}_{\ell\ell HH}^{rt} (\bar{\ell}_s H \bar{B} H^\dagger \ell_r) \\
& - \frac{3}{2} g_Y^2 \bar{\mathcal{C}}_{\ell\ell HH}^{rs} \mathcal{C}_{\ell\ell HH}^{rs} (H^\dagger H)^2 B_\mu^2 - 2g_L^2 \bar{\mathcal{C}}_{\ell\ell HH}^{rs} \mathcal{C}_{\ell\ell HH}^{rs} (H^\dagger t^I H) (H^\dagger t^J H) W_\mu^I W_\mu^J \\
& - 4g_L \bar{\mathcal{C}}_{\ell\ell HH}^{st} \mathcal{C}_{\ell\ell HH}^{rt} (H^\dagger t^I H) (\bar{\ell}_s \bar{W}^I \ell_r) - 5g_Y \bar{\mathcal{C}}_{\ell\ell HH}^{st} \mathcal{C}_{\ell\ell HH}^{rt} (H^\dagger H) (\bar{\ell}_s \bar{B} \ell_r) \\
& - 6g_L g_Y \bar{\mathcal{C}}_{\ell\ell HH}^{rs} \mathcal{C}_{\ell\ell HH}^{rs} (H^\dagger H) (H^\dagger t^I H) B_\mu W_\mu^I. \tag{2.2}
\end{aligned}$$

### 2.3 Dimension six: bosonic operators

$$\Delta S_{\mathcal{O}_H} = 0, \quad (2.3)$$

$$\Delta S_{\mathcal{O}_{H\Box}} = 0, \quad (2.4)$$

$$\Delta S_{\mathcal{O}_{HD}} = 0, \quad (2.5)$$

$$\begin{aligned} \Delta S_{\mathcal{O}_W} = & \frac{1}{2} g_L^3 \mathcal{C}_W W_{\bar{\mu}}^I \widetilde{W}^{\bar{\mu}\bar{\sigma}I} (\bar{\ell}_s \gamma^{\bar{\sigma}} \ell_s) + \frac{1}{2} g_L^3 \mathcal{C}_W W_{\bar{\mu}}^I \widetilde{W}^{\bar{\mu}\bar{\sigma}I} (\bar{q}_s \gamma^{\bar{\sigma}} q_s) \\ & + g_L^2 g_Y \mathcal{C}_W B_{\bar{\mu}} \widetilde{W}^{\bar{\mu}\bar{\sigma}I} (\bar{\ell}_s t^I \gamma^{\bar{\sigma}} \ell_s) - \frac{1}{3} g_L^2 g_Y \mathcal{C}_W B_{\bar{\mu}} \widetilde{W}^{\bar{\mu}\bar{\sigma}I} (\bar{q}_s t^I \gamma^{\bar{\sigma}} q_s) \\ & - 2 g_L^2 g_s \mathcal{C}_W G_{\bar{\mu}}^A \widetilde{W}^{\bar{\mu}\bar{\sigma}I} (\bar{q}_s t^I T^A \gamma^{\bar{\sigma}} q_s), \end{aligned} \quad (2.6)$$

$$\begin{aligned} \Delta S_{\mathcal{O}_{\bar{W}}} = & \frac{1}{6} g_L^3 \mathcal{C}_{\bar{W}} W_{\bar{\mu}}^I W^{\bar{\mu}\bar{\nu}I} (\bar{\ell}_s \gamma^{\bar{\nu}} \ell_s) + \frac{1}{6} g_L^3 \mathcal{C}_{\bar{W}} W_{\bar{\mu}}^I W^{\bar{\mu}\bar{\nu}I} (\bar{q}_s \gamma^{\bar{\nu}} q_s) \\ & + \frac{1}{3} g_L^2 g_Y \mathcal{C}_{\bar{W}} B_{\bar{\mu}} W^{\bar{\mu}\bar{\nu}I} (\bar{\ell}_s t^I \gamma^{\bar{\nu}} \ell_s) - \frac{1}{9} g_L^2 g_Y \mathcal{C}_{\bar{W}} B_{\bar{\mu}} W^{\bar{\mu}\bar{\nu}I} (\bar{q}_s t^I \gamma^{\bar{\nu}} q_s) \\ & - \frac{2}{3} g_L^2 g_s \mathcal{C}_{\bar{W}} G_{\bar{\mu}}^A W^{\bar{\mu}\bar{\nu}I} (\bar{q}_s t^I T^A \gamma^{\bar{\nu}} q_s), \end{aligned} \quad (2.7)$$

$$\begin{aligned} \Delta S_{\mathcal{O}_G} = & \frac{1}{2} g_s^3 \mathcal{C}_G G_{\bar{\mu}}^A \widetilde{G}^{\bar{\mu}\bar{\sigma}A} (\bar{q}_s \gamma^{\bar{\sigma}} q_s) + 2 g_s^2 g_Y \mathcal{C}_G B_{\bar{\mu}} \widetilde{G}^{\bar{\mu}\bar{\sigma}A} (\bar{u}_s T^A \gamma^{\bar{\sigma}} u_s) \\ & - \frac{1}{2} g_s^3 \mathcal{C}_G G_{\bar{\mu}}^A \widetilde{G}^{\bar{\mu}\bar{\sigma}A} (\bar{d}_s \gamma^{\bar{\sigma}} d_s) - \frac{1}{2} g_s^2 g_Y \mathcal{C}_G B_{\bar{\mu}} \widetilde{G}^{\bar{\mu}\bar{\sigma}A} (\bar{q}_s T^A \gamma^{\bar{\sigma}} q_s) \\ & - \frac{1}{2} g_s^3 \mathcal{C}_G G_{\bar{\mu}}^A \widetilde{G}^{\bar{\mu}\bar{\sigma}A} (\bar{u}_s \gamma^{\bar{\sigma}} u_s) - g_s^2 g_Y \mathcal{C}_G B_{\bar{\mu}} \widetilde{G}^{\bar{\mu}\bar{\sigma}A} (\bar{d}_s T^A \gamma^{\bar{\sigma}} d_s) \\ & - 3 g_L g_s^2 \mathcal{C}_G W_{\bar{\mu}}^I \widetilde{G}^{\bar{\mu}\bar{\sigma}A} (\bar{q}_s t^I T^A \gamma^{\bar{\sigma}} q_s), \end{aligned} \quad (2.8)$$

$$\begin{aligned} \Delta S_{\mathcal{O}_{\bar{G}}} = & \frac{1}{6} g_s^3 \mathcal{C}_{\bar{G}} G_{\bar{\mu}}^A G^{\bar{\mu}\bar{\nu}A} (\bar{q}_s \gamma^{\bar{\nu}} q_s) + \frac{2}{3} g_s^2 g_Y \mathcal{C}_{\bar{G}} B_{\bar{\mu}} G^{\bar{\mu}\bar{\nu}A} (\bar{u}_s T^A \gamma^{\bar{\nu}} u_s) \\ & - \frac{1}{6} g_s^3 \mathcal{C}_{\bar{G}} G_{\bar{\mu}}^A G^{\bar{\mu}\bar{\nu}A} (\bar{d}_s \gamma^{\bar{\nu}} d_s) - \frac{1}{6} g_s^2 g_Y \mathcal{C}_{\bar{G}} B_{\bar{\mu}} G^{\bar{\mu}\bar{\nu}A} (\bar{q}_s T^A \gamma^{\bar{\nu}} q_s) \\ & - \frac{1}{6} g_s^3 \mathcal{C}_{\bar{G}} G_{\bar{\mu}}^A G^{\bar{\mu}\bar{\nu}A} (\bar{u}_s \gamma^{\bar{\nu}} u_s) - \frac{1}{3} g_s^2 g_Y \mathcal{C}_{\bar{G}} B_{\bar{\mu}} G^{\bar{\mu}\bar{\nu}A} (\bar{d}_s T^A \gamma^{\bar{\nu}} d_s) \\ & - g_L g_s^2 \mathcal{C}_{\bar{G}} W_{\bar{\mu}}^I G^{\bar{\mu}\bar{\nu}A} (\bar{q}_s t^I T^A \gamma^{\bar{\nu}} q_s), \end{aligned} \quad (2.9)$$

$$\begin{aligned} \Delta S_{\mathcal{O}_{HB}} = & \frac{1}{324} g_Y^3 \mathcal{C}_{HB} (H^\dagger H) (\bar{q}_s \bar{B} q_s) + \frac{1}{54} g_s g_Y^2 \mathcal{C}_{HB} (H^\dagger H) (\bar{q}_s T^A \bar{G}^A q_s) + \frac{1}{54} g_L g_Y^2 \mathcal{C}_{HB} (H^\dagger H) (\bar{q}_s t^I \bar{W}^I q_s) \\ & + \frac{2}{27} g_s g_Y^2 \mathcal{C}_{HB} (H^\dagger H) (\bar{d}_s T^A \bar{G}^A d_s) + \frac{1}{6} g_L g_Y^2 \mathcal{C}_{HB} (H^\dagger H) (\bar{\ell}_s t^I \bar{W}^I \ell_s) + \frac{16}{81} g_Y^3 \mathcal{C}_{HB} (H^\dagger H) (\bar{u}_s \bar{B} u_s) \\ & + \frac{8}{27} g_s g_Y^2 \mathcal{C}_{HB} (H^\dagger H) (\bar{u}_s T^A \bar{G}^A u_s) - \frac{2}{81} g_Y^3 \mathcal{C}_{HB} (H^\dagger H) (\bar{d}_s \bar{B} d_s) - \frac{1}{12} g_Y^3 \mathcal{C}_{HB} (H^\dagger H) (\bar{\ell}_s \bar{B} \ell_s) \\ & - \frac{2}{3} g_Y^3 \mathcal{C}_{HB} (H^\dagger H) (\bar{e}_s \bar{B} e_s), \end{aligned} \quad (2.10)$$

$$\Delta S_{\mathcal{O}_{H\bar{B}}} = 0, \quad (2.11)$$

$$\begin{aligned} \Delta S_{\mathcal{O}_{HW}} &= \frac{1}{12} g_L^2 g_Y \mathcal{C}_{HW} (H^\dagger H) (\bar{q}_s \bar{\mathcal{B}} q_s) + \frac{1}{2} g_L^2 g_s \mathcal{C}_{HW} (H^\dagger H) (\bar{q}_s T^A \bar{\mathcal{G}}^A q_s) - \frac{1}{6} g_L^3 \mathcal{C}_{HW} (H^\dagger H) (\bar{\ell}_s t^I \bar{\mathcal{W}}^I \ell_s) \\ &\quad - \frac{1}{6} g_L^3 \mathcal{C}_{HW} (H^\dagger H) (\bar{q}_s t^I \bar{\mathcal{W}}^I q_s) - \frac{1}{4} g_L^2 g_Y \mathcal{C}_{HW} (H^\dagger H) (\bar{\ell}_s \bar{\mathcal{B}} \ell_s), \end{aligned} \quad (2.12)$$

$$\Delta S_{\mathcal{O}_{H\bar{W}}} = 0, \quad (2.13)$$

$$\begin{aligned} \Delta S_{\mathcal{O}_{HG}} &= \frac{4}{27} g_s^2 g_Y \mathcal{C}_{HG} (H^\dagger H) (\bar{q}_s \bar{\mathcal{B}} q_s) + \frac{16}{27} g_s^2 g_Y \mathcal{C}_{HG} (H^\dagger H) (\bar{u}_s \bar{\mathcal{B}} u_s) + \frac{8}{9} g_L g_s^2 \mathcal{C}_{HG} (H^\dagger H) (\bar{q}_s t^I \bar{\mathcal{W}}^I q_s) \\ &\quad - \frac{1}{9} g_s^3 \mathcal{C}_{HG} (H^\dagger H) (\bar{d}_s T^A \bar{\mathcal{G}}^A d_s) - \frac{1}{9} g_s^3 \mathcal{C}_{HG} (H^\dagger H) (\bar{q}_s T^A \bar{\mathcal{G}}^A q_s) - \frac{1}{9} g_s^3 \mathcal{C}_{HG} (H^\dagger H) (\bar{u}_s T^A \bar{\mathcal{G}}^A u_s) \\ &\quad - \frac{8}{27} g_s^2 g_Y \mathcal{C}_{HG} (H^\dagger H) (\bar{d}_s \bar{\mathcal{B}} d_s), \end{aligned} \quad (2.14)$$

$$\Delta S_{\mathcal{O}_{H\bar{G}}} = 0, \quad (2.15)$$

$$\begin{aligned} \Delta S_{\mathcal{O}_{HWB}} &= \frac{1}{54} g_L g_Y^2 \mathcal{C}_{HWB} (\bar{q}_s H \bar{\mathcal{B}} H^\dagger q_s) + \frac{1}{18} g_L^2 g_Y \mathcal{C}_{HWB} (H^\dagger t^I H) (\bar{q}_s \bar{\mathcal{W}}^I q_s) + \frac{1}{9} g_L g_s g_Y \mathcal{C}_{HWB} (\bar{q}_s T^A H \bar{\mathcal{G}}^A H^\dagger q_s) \\ &\quad + \frac{1}{6} g_L g_Y^2 \mathcal{C}_{HWB} (\bar{\ell}_s H \bar{\mathcal{B}} H^\dagger \ell_s) - \frac{1}{108} g_L g_Y^2 \mathcal{C}_{HWB} (H^\dagger H) (\bar{q}_s \bar{\mathcal{B}} q_s) - \frac{1}{18} g_L g_s g_Y \mathcal{C}_{HWB} (H^\dagger H) (\bar{q}_s T^A \bar{\mathcal{G}}^A q_s) \\ &\quad - \frac{1}{12} g_L g_Y^2 \mathcal{C}_{HWB} (H^\dagger H) (\bar{\ell}_s \bar{\mathcal{B}} \ell_s) - \frac{1}{6} g_L^2 g_Y \mathcal{C}_{HWB} (H^\dagger t^I H) (\bar{\ell}_s \bar{\mathcal{W}}^I \ell_s), \end{aligned} \quad (2.16)$$

$$\Delta S_{\mathcal{O}_{H\bar{W}B}} = 0, \quad (2.17)$$

## 2.4 Dimension six: semibosonic operators

$$\begin{aligned} \Delta S_{\mathcal{O}_{eH}} &= \frac{i}{6} \left[ \bar{y}_e^{rs} \mathcal{C}_{eH}^{rs} - y_e^{rs} \bar{\mathcal{C}}_{eH}^{rs} \right] \left[ g_Y (H^\dagger H) (H^\dagger \partial_{\bar{\mu}} H) B_{\bar{\mu}} + g_Y (H^\dagger H) (\partial_{\bar{\mu}} H^\dagger H) B_{\bar{\mu}} \right] \\ &\quad + \frac{i}{6} g_Y \left[ \bar{y}_e^{rs} \mathcal{C}_{eH}^{rs} + y_e^{rs} \bar{\mathcal{C}}_{eH}^{rs} \right] (H^\dagger \overset{\leftrightarrow}{\partial}_{\bar{\mu}} H) (H^\dagger H) B_{\bar{\mu}} + \frac{1}{4} g_L^2 \left[ \bar{y}_e^{rs} \mathcal{C}_{eH}^{rs} + y_e^{rs} \bar{\mathcal{C}}_{eH}^{rs} \right] (H^\dagger H)^2 W_{\bar{\mu}}^{I\,2} \\ &\quad + \frac{i}{3} \left[ \bar{y}_e^{rs} \mathcal{C}_{eH}^{rs} - y_e^{rs} \bar{\mathcal{C}}_{eH}^{rs} \right] \left[ g_L (H^\dagger \partial_{\bar{\mu}} H) (H^\dagger t^I H) W_{\bar{\mu}}^I + g_L (\partial_{\bar{\mu}} H^\dagger H) (H^\dagger t^I H) W_{\bar{\mu}}^I \right] \\ &\quad + \frac{i}{3} g_L \left[ \bar{y}_e^{rs} \mathcal{C}_{eH}^{rs} + y_e^{rs} \bar{\mathcal{C}}_{eH}^{rs} \right] (H^\dagger t^I \overset{\leftrightarrow}{\partial}_{\bar{\mu}} H) (H^\dagger H) W_{\bar{\mu}}^I + \frac{1}{2} g_L \left[ \bar{y}_e^{ts} \mathcal{C}_{eH}^{tr} + y_e^{tr} \bar{\mathcal{C}}_{eH}^{ts} \right] (H^\dagger t^I H) (\bar{e}_s \bar{\mathcal{W}}^I e_r) \\ &\quad + \frac{1}{2} g_Y \left[ -\bar{y}_e^{rt} \mathcal{C}_{eH}^{st} - y_e^{st} \bar{\mathcal{C}}_{eH}^{rt} \right] (H^\dagger H) (\bar{\ell}_s \bar{\mathcal{B}} \ell_r) + \frac{1}{2} g_Y \left[ -\bar{y}_e^{rt} \mathcal{C}_{eH}^{st} - y_e^{st} \bar{\mathcal{C}}_{eH}^{rt} \right] (\bar{\ell}_s H \bar{\mathcal{B}} H^\dagger \ell_r) \\ &\quad + \frac{3}{4} g_Y^2 \left[ \bar{y}_e^{rs} \mathcal{C}_{eH}^{rs} + y_e^{rs} \bar{\mathcal{C}}_{eH}^{rs} \right] (H^\dagger H)^2 B_{\bar{\mu}}^2 - \frac{3}{4} g_Y \left[ \bar{y}_e^{ts} \mathcal{C}_{eH}^{tr} + y_e^{tr} \bar{\mathcal{C}}_{eH}^{ts} \right] (H^\dagger H) (\bar{e}_s \bar{\mathcal{B}} e_r), \end{aligned} \quad (2.18)$$

$$\begin{aligned} \Delta S_{\mathcal{O}_{uH}} &= \frac{1}{4} g_Y \left[ \bar{y}_u^{ts} \mathcal{C}_{uH}^{tr} + y_u^{tr} \bar{\mathcal{C}}_{uH}^{ts} \right] (H^\dagger H) (\bar{u}_s \bar{\mathcal{B}} u_r) + \frac{1}{3} g_Y \left[ -\bar{y}_u^{rt} \mathcal{C}_{uH}^{st} - y_u^{st} \bar{\mathcal{C}}_{uH}^{rt} \right] (\bar{q}_s H \bar{\mathcal{B}} H^\dagger q_r) \\ &\quad + \frac{1}{2} g_s^2 \left[ \bar{y}_u^{rs} \mathcal{C}_{uH}^{rs} + y_u^{rs} \bar{\mathcal{C}}_{uH}^{rs} \right] (H^\dagger H)^2 G_{\bar{\mu}}^{A\,2} \\ &\quad - \frac{i}{2} \left[ \bar{y}_u^{rs} \mathcal{C}_{uH}^{rs} - y_u^{rs} \bar{\mathcal{C}}_{uH}^{rs} \right] \left[ g_Y (H^\dagger H) (H^\dagger \partial_{\bar{\mu}} H) B_{\bar{\mu}} + g_Y (H^\dagger H) (\partial_{\bar{\mu}} H^\dagger H) B_{\bar{\mu}} \right] + \frac{1}{2} g_L \bar{y}_d^{ts} \mathcal{C}_{uH}^{tr} t_k^{Ij} H_j^\dagger \tilde{H}_k (\bar{d}_s \bar{\mathcal{W}}^I u_r) \end{aligned}$$

$$\begin{aligned}
& + \frac{1}{2} g_s \left[ -\bar{y}_u^{rt} \mathcal{C}_{uH}^{st} - y_u^{st} \bar{\mathcal{C}}_{uH}^{rt} \right] (\bar{q}_s T^A H \bar{\mathcal{G}}^A H^\dagger q_r) + \frac{1}{2} g_L y_d^{tr} \bar{\mathcal{C}}_{uH}^{ts} t_k^{Ii} \tilde{H}^{\dagger i} H^k (\bar{u}_s \bar{W}^I d_r) \\
& + \frac{1}{2} g_L \left[ -\bar{y}_u^{ts} \mathcal{C}_{uH}^{tr} - y_u^{tr} \bar{\mathcal{C}}_{uH}^{ts} \right] (H^\dagger t^I H) (\bar{u}_s \bar{W}^I u_r) + \frac{i}{2} g_Y \left[ \bar{y}_u^{rs} \mathcal{C}_{uH}^{rs} + y_u^{rs} \bar{\mathcal{C}}_{uH}^{rs} \right] (H^\dagger \overleftrightarrow{\partial}_\mu H) (H^\dagger H) B_\mu \\
& + \frac{2}{3} g_Y \left[ \bar{y}_u^{rt} \mathcal{C}_{uH}^{st} + y_u^{st} \bar{\mathcal{C}}_{uH}^{rt} \right] (H^\dagger H) (\bar{q}_s \bar{\mathcal{B}} q_r) + \frac{3}{4} g_L^2 \left[ \bar{y}_u^{rs} \mathcal{C}_{uH}^{rs} + y_u^{rs} \bar{\mathcal{C}}_{uH}^{rs} \right] (H^\dagger H)^2 W_\mu^{I2} \\
& + g_L g_Y \left[ \bar{y}_u^{rs} \mathcal{C}_{uH}^{rs} + y_u^{rs} \bar{\mathcal{C}}_{uH}^{rs} \right] (H^\dagger H) (H^\dagger t^I H) B_\mu W_\mu^I \\
& - i \left[ \bar{y}_u^{rs} \mathcal{C}_{uH}^{rs} - y_u^{rs} \bar{\mathcal{C}}_{uH}^{rs} \right] \left[ g_L (H^\dagger \partial_\mu H) (H^\dagger t^I H) W_\mu^I + g_L (\partial_\mu H^\dagger H) (H^\dagger t^I H) W_\mu^I \right] \\
& + g_s \left[ \bar{y}_u^{rt} \mathcal{C}_{uH}^{st} + y_u^{st} \bar{\mathcal{C}}_{uH}^{rt} \right] (H^\dagger H) (\bar{q}_s T^A \bar{\mathcal{G}}^A q_r) + i g_L \left[ \bar{y}_u^{rs} \mathcal{C}_{uH}^{rs} + y_u^{rs} \bar{\mathcal{C}}_{uH}^{rs} \right] (H^\dagger t^I \overleftrightarrow{\partial}_\mu H) (H^\dagger H) W_\mu^I \\
& + \frac{13}{12} g_Y^2 \left[ \bar{y}_u^{rs} \mathcal{C}_{uH}^{rs} + y_u^{rs} \bar{\mathcal{C}}_{uH}^{rs} \right] (H^\dagger H)^2 B_\mu^2 + \frac{3}{2} g_s \left[ \bar{y}_u^{ts} \mathcal{C}_{uH}^{tr} + y_u^{tr} \bar{\mathcal{C}}_{uH}^{ts} \right] (H^\dagger H) (\bar{u}_s T^A \bar{\mathcal{G}}^A u_r), \tag{2.19}
\end{aligned}$$

$$\begin{aligned}
\Delta S_{\mathcal{O}_{dH}} &= \frac{1}{6} g_Y \left[ -\bar{y}_d^{rt} \mathcal{C}_{dH}^{st} - y_d^{st} \bar{\mathcal{C}}_{dH}^{rt} \right] (H^\dagger H) (\bar{q}_s \bar{\mathcal{B}} q_r) + \frac{1}{6} g_Y \left[ -\bar{y}_d^{rt} \mathcal{C}_{dH}^{st} - y_d^{st} \bar{\mathcal{C}}_{dH}^{rt} \right] (\bar{q}_s H \bar{\mathcal{B}} H^\dagger q_r) \\
& + \frac{1}{4} g_Y \left[ \bar{y}_d^{ts} \mathcal{C}_{dH}^{tr} + y_d^{tr} \bar{\mathcal{C}}_{dH}^{ts} \right] (H^\dagger H) (\bar{d}_s \bar{\mathcal{B}} d_r) + \frac{1}{2} g_s^2 \left[ \bar{y}_d^{rs} \mathcal{C}_{dH}^{rs} + y_d^{rs} \bar{\mathcal{C}}_{dH}^{rs} \right] (H^\dagger H)^2 G_\mu^{A2} \\
& + \frac{i}{2} \left[ \bar{y}_d^{rs} \mathcal{C}_{dH}^{rs} - y_d^{rs} \bar{\mathcal{C}}_{dH}^{rs} \right] \left[ g_Y (H^\dagger H) (H^\dagger \partial_\mu H) B_\mu + g_Y (H^\dagger H) (\partial_\mu H^\dagger H) B_\mu \right] \\
& + \frac{1}{2} g_L \left[ \bar{y}_d^{ts} \mathcal{C}_{dH}^{tr} + y_d^{tr} \bar{\mathcal{C}}_{dH}^{ts} \right] (H^\dagger t^I H) (\bar{d}_s \bar{W}^I d_r) + \frac{1}{2} g_L y_u^{tr} \bar{\mathcal{C}}_{dH}^{ts} t_k^{Ij} H_j^\dagger \tilde{H}^k (\bar{d}_s \bar{W}^I u_r) \\
& + \frac{1}{2} g_s \left[ \bar{y}_d^{rt} \mathcal{C}_{dH}^{st} + y_d^{st} \bar{\mathcal{C}}_{dH}^{rt} \right] (H^\dagger H) (\bar{q}_s T^A \bar{\mathcal{G}}^A q_r) + \frac{1}{2} g_s \left[ \bar{y}_d^{rt} \mathcal{C}_{dH}^{st} + y_d^{st} \bar{\mathcal{C}}_{dH}^{rt} \right] (\bar{q}_s T^A H \bar{\mathcal{G}}^A H^\dagger q_r) \\
& + \frac{1}{2} g_L \bar{y}_u^{ts} \mathcal{C}_{dH}^{tr} t_k^{Ii} \tilde{H}^{\dagger i} H^k (\bar{u}_s \bar{W}^I d_r) + \frac{i}{2} g_Y \left[ \bar{y}_d^{rs} \mathcal{C}_{dH}^{rs} + y_d^{rs} \bar{\mathcal{C}}_{dH}^{rs} \right] (H^\dagger \overleftrightarrow{\partial}_\mu H) (H^\dagger H) B_\mu \\
& + \frac{7}{12} g_Y^2 \left[ \bar{y}_d^{rs} \mathcal{C}_{dH}^{rs} + y_d^{rs} \bar{\mathcal{C}}_{dH}^{rs} \right] (H^\dagger H)^2 B_\mu^2 + \frac{3}{4} g_L^2 \left[ \bar{y}_d^{rs} \mathcal{C}_{dH}^{rs} + y_d^{rs} \bar{\mathcal{C}}_{dH}^{rs} \right] (H^\dagger H)^2 W_\mu^{I2} \\
& + i \left[ \bar{y}_d^{rs} \mathcal{C}_{dH}^{rs} - y_d^{rs} \bar{\mathcal{C}}_{dH}^{rs} \right] \left[ g_L (H^\dagger \partial_\mu H) (H^\dagger t^I H) W_\mu^I + g_L (\partial_\mu H^\dagger H) (H^\dagger t^I H) W_\mu^I \right] \\
& + i g_L \left[ \bar{y}_d^{rs} \mathcal{C}_{dH}^{rs} + y_d^{rs} \bar{\mathcal{C}}_{dH}^{rs} \right] (H^\dagger t^I \overleftrightarrow{\partial}_\mu H) (H^\dagger H) W_\mu^I + \frac{3}{2} g_s \left[ \bar{y}_d^{ts} \mathcal{C}_{dH}^{tr} + y_d^{tr} \bar{\mathcal{C}}_{dH}^{ts} \right] (H^\dagger H) (\bar{d}_s T^A \bar{\mathcal{G}}^A d_r) \\
& + 2 g_L g_Y \left[ \bar{y}_d^{rs} \mathcal{C}_{dH}^{rs} + y_d^{rs} \bar{\mathcal{C}}_{dH}^{rs} \right] (H^\dagger H) (H^\dagger t^I H) B_\mu W_\mu^I, \tag{2.20}
\end{aligned}$$

$$\begin{aligned}
\Delta S_{\mathcal{O}_{eB}} &= \frac{1}{6} g_L^2 g_Y \bar{\mathcal{C}}_{eB}^{rs} \varepsilon^{IJK} t_j^{Ki} H_i^\dagger W_\mu^J W_\nu^I (\bar{e}_s \sigma^{\mu\nu} \ell_r^j) + \frac{i}{6} g_L g_Y \mathcal{C}_{eB}^{sr} t_j^{Ii} H_j^\dagger W_\mu^I (\bar{\ell}_{is} \partial^\mu e_r) \\
& + \frac{1}{6} g_L^2 g_Y \mathcal{C}_{eB}^{sr} \varepsilon^{IJK} t_j^{Ki} H_j^\dagger W_\mu^J W_\nu^I (\bar{\ell}_{is} \sigma^{\mu\nu} e_r) - \frac{i}{6} g_L g_Y \bar{\mathcal{C}}_{eB}^{rs} t_j^{Ii} H_i^\dagger W_\mu^I (\partial^\mu \bar{e}_s \ell_r^j) \\
& + \frac{1}{4} g_L g_Y \left[ \bar{y}_e^{rt} \mathcal{C}_{eB}^{st} + y_e^{st} \bar{\mathcal{C}}_{eB}^{rt} \right] (H^\dagger t^I H) (\bar{\ell}_s \bar{W}^I \ell_r) + \frac{1}{4} g_L g_Y \left[ \bar{y}_e^{rt} \mathcal{C}_{eB}^{st} + y_e^{st} \bar{\mathcal{C}}_{eB}^{rt} \right] (H^\dagger H) (\bar{\ell}_s t^I \bar{W}^I \ell_r) \\
& + \frac{1}{4} g_Y \left[ \bar{y}_e^{rt} \mathcal{C}_{eB}^{st} - y_e^{st} \bar{\mathcal{C}}_{eB}^{rt} \right] \left[ g_L t_j^{Ii} H_i^\dagger (\bar{\ell}_s H \bar{W}^I \ell_r^j) - g_L t_k^{Ij} H^k (\bar{\ell}_{js} \bar{W}^I H^\dagger \ell_r) \right] \\
& - \frac{i}{3} \left[ \bar{y}_e^{rs} \mathcal{C}_{eB}^{rs} + y_e^{rs} \bar{\mathcal{C}}_{eB}^{rs} \right] \left[ 2 g_L W_\mu^I \tilde{B}^{\mu\sigma} (H^\dagger t^I \partial_\sigma H) - 2 g_L W_\mu^I \tilde{B}^{\mu\sigma} (\partial_\sigma H^\dagger t^I H) \right] \\
& + \frac{i}{3} \left[ \bar{y}_e^{rs} \mathcal{C}_{eB}^{rs} - y_e^{rs} \bar{\mathcal{C}}_{eB}^{rs} \right] \left[ 2 g_L W_\mu^I \tilde{B}^{\mu\sigma} (H^\dagger t^I \partial_\sigma H) + 2 g_L W_\mu^I \tilde{B}^{\mu\sigma} (\partial_\sigma H^\dagger t^I H) \right]
\end{aligned}$$

$$\begin{aligned}
& + \frac{3}{8} g_L^2 g_Y \bar{\mathcal{C}}_{eB}^{rs} W_{\bar{\mu}}^{I2} (\bar{e}_s H^\dagger \ell_r) + \frac{3}{8} g_L^2 g_Y \mathcal{C}_{eB}^{sr} W_{\bar{\mu}}^{I2} (\bar{\ell}_s H e_r) - \frac{1}{3} g_L g_Y \bar{\mathcal{C}}_{eB}^{rs} t_j^{Ii} W_{\bar{\mu}}^I (\bar{e}_s \sigma^{\bar{\mu}\bar{\nu}} \ell_r^j) \partial^{\bar{\nu}} H_i^\dagger \\
& + \frac{i}{2} \left[ \bar{y}_e^{rs} \mathcal{C}_{eB}^{rs} + y_e^{rs} \bar{\mathcal{C}}_{eB}^{rs} \right] \left[ 2g_Y B_{\bar{\mu}} \tilde{B}^{\bar{\mu}\bar{\sigma}} (H^\dagger \partial_{\bar{\sigma}} H) - 2g_Y B_{\bar{\mu}} \tilde{B}^{\bar{\mu}\bar{\sigma}} (\partial_{\bar{\sigma}} H^\dagger H) \right] \\
& - \frac{i}{2} \left[ \bar{y}_e^{rs} \mathcal{C}_{eB}^{rs} - y_e^{rs} \bar{\mathcal{C}}_{eB}^{rs} \right] \left[ 2g_Y B_{\bar{\mu}} \tilde{B}^{\bar{\mu}\bar{\sigma}} (H^\dagger \partial_{\bar{\sigma}} H) + 2g_Y B_{\bar{\mu}} \tilde{B}^{\bar{\mu}\bar{\sigma}} (\partial_{\bar{\sigma}} H^\dagger H) \right] \\
& + \frac{i}{2} g_L g_Y \bar{\mathcal{C}}_{eB}^{rs} t_j^{Ii} H_i^\dagger W_{\bar{\mu}}^I (\bar{e}_s \partial^{\bar{\mu}} \ell_r^j) - \frac{i}{2} g_L g_Y \mathcal{C}_{eB}^{sr} t_j^{Ii} H^j W_{\bar{\mu}}^I (\partial^{\bar{\mu}} \bar{\ell}_{is} e_r) \\
& - \frac{i}{2} g_L g_Y \bar{\mathcal{C}}_{eB}^{rs} t_j^{Ii} W_{\bar{\mu}}^I (\bar{e}_s \ell_r^j) \partial^{\bar{\mu}} H_i^\dagger + \frac{i}{2} g_L g_Y \mathcal{C}_{eB}^{sr} t_j^{Ii} W_{\bar{\mu}}^I (\bar{\ell}_{is} e_r) \partial^{\bar{\mu}} H^j - \frac{7i}{12} g_Y^2 \bar{\mathcal{C}}_{eB}^{rs} B_{\bar{\mu}} (\bar{e}_s H^\dagger \partial^{\bar{\mu}} \ell_r) \\
& + \frac{7i}{12} g_Y^2 \mathcal{C}_{eB}^{sr} B_{\bar{\mu}} (\partial^{\bar{\mu}} \bar{\ell}_s H e_r) \\
& + \frac{2}{3} \left[ \bar{y}_e^{rs} \mathcal{C}_{eB}^{rs} + y_e^{rs} \bar{\mathcal{C}}_{eB}^{rs} \right] \left[ g_L W_{\bar{\mu}}^I B^{\bar{\mu}\bar{\nu}} (H^\dagger t^I \partial_{\bar{\nu}} H) + g_L W_{\bar{\mu}}^I B^{\bar{\mu}\bar{\nu}} (\partial_{\bar{\nu}} H^\dagger t^I H) \right] \\
& + \frac{2}{3} g_L \left[ y_e^{rs} \bar{\mathcal{C}}_{eB}^{rs} - \bar{y}_e^{rs} \mathcal{C}_{eB}^{rs} \right] W_{\bar{\mu}}^I B^{\bar{\mu}\bar{\nu}} (H^\dagger t^I \overset{\leftrightarrow}{\partial}_{\bar{\nu}} H) - \frac{3i}{4} g_Y^2 \bar{\mathcal{C}}_{eB}^{rs} B_{\bar{\mu}} (\bar{e}_s \partial^{\bar{\mu}} H^\dagger \ell_r) \\
& + \frac{3i}{4} g_Y^2 \mathcal{C}_{eB}^{sr} B_{\bar{\mu}} (\bar{\ell}_s \partial^{\bar{\mu}} H e_r) + \frac{5}{6} g_Y^2 \bar{\mathcal{C}}_{eB}^{rs} B_{\bar{\mu}} (\bar{e}_s \sigma^{\bar{\mu}\bar{\nu}} \partial^{\bar{\nu}} H^\dagger \ell_r) + \frac{5}{6} g_Y^2 \mathcal{C}_{eB}^{sr} B_{\bar{\mu}} (\bar{\ell}_s \partial^{\bar{\nu}} H \sigma^{\bar{\mu}\bar{\nu}} e_r) \\
& + \left[ -\bar{y}_e^{rs} \mathcal{C}_{eB}^{rs} - y_e^{rs} \bar{\mathcal{C}}_{eB}^{rs} \right] \left[ g_Y B_{\bar{\mu}} B^{\bar{\mu}\bar{\nu}} (H^\dagger \partial_{\bar{\nu}} H) + g_Y B_{\bar{\mu}} B^{\bar{\mu}\bar{\nu}} (\partial_{\bar{\nu}} H^\dagger H) \right] \\
& + g_Y \left[ \bar{y}_e^{rt} \mathcal{C}_{eB}^{st} + y_e^{st} \bar{\mathcal{C}}_{eB}^{rt} \right] B_{\bar{\mu}} \tilde{B}^{\bar{\mu}\bar{\sigma}} (\bar{\ell}_s \gamma^{\bar{\sigma}} \ell_r) + g_Y \left[ \bar{y}_e^{rs} \mathcal{C}_{eB}^{rs} - y_e^{rs} \bar{\mathcal{C}}_{eB}^{rs} \right] B_{\bar{\mu}} B^{\bar{\mu}\bar{\nu}} (H^\dagger \overset{\leftrightarrow}{\partial}_{\bar{\nu}} H) \\
& - \frac{1}{4} g_Y^2 \left[ \bar{y}_e^{rt} \mathcal{C}_{eB}^{st} + y_e^{st} \bar{\mathcal{C}}_{eB}^{rt} \right] (\bar{\ell}_s H \tilde{B} H^\dagger \ell_r) - \frac{1}{3} g_L g_Y \mathcal{C}_{eB}^{sr} t_j^{Ii} W_{\bar{\mu}}^I (\bar{\ell}_{is} \sigma^{\bar{\mu}\bar{\nu}} e_r) \partial^{\bar{\nu}} H^j \\
& - \frac{1}{2} g_L g_Y^2 \bar{\mathcal{C}}_{eB}^{rs} t_j^{Ii} H_i^\dagger B_{\bar{\mu}} W_{\bar{\mu}}^I (\bar{e}_s \ell_r^j) - \frac{1}{2} g_L g_Y^2 \mathcal{C}_{eB}^{sr} t_j^{Ii} H^j B_{\bar{\mu}} W_{\bar{\mu}}^I (\bar{\ell}_{is} e_r) \\
& - \frac{2}{3} g_L^2 \left[ \bar{y}_e^{rs} \mathcal{C}_{eB}^{rs} + y_e^{rs} \bar{\mathcal{C}}_{eB}^{rs} \right] \varepsilon^{IJK} W_{\bar{\mu}}^J W_{\bar{\nu}}^I B^{\bar{\mu}\bar{\nu}} (H^\dagger t^K H) \\
& - \frac{2i}{3} g_L^2 \left[ \bar{y}_e^{rs} \mathcal{C}_{eB}^{rs} - y_e^{rs} \bar{\mathcal{C}}_{eB}^{rs} \right] \varepsilon^{IJK} W_{\bar{\mu}}^J W_{\bar{\nu}}^I \tilde{B}^{\bar{\mu}\bar{\nu}} (H^\dagger t^K H) \\
& - i g_Y \left[ \bar{y}_e^{ts} \mathcal{C}_{eB}^{tr} - y_e^{tr} \bar{\mathcal{C}}_{eB}^{ts} \right] B_{\bar{\mu}} B^{\bar{\mu}\bar{\nu}} (\bar{e}_s \gamma^{\bar{\nu}} e_r) + g_Y \left[ -\bar{y}_e^{ts} \mathcal{C}_{eB}^{tr} - y_e^{tr} \bar{\mathcal{C}}_{eB}^{ts} \right] B_{\bar{\mu}} \tilde{B}^{\bar{\mu}\bar{\sigma}} (\bar{e}_s \gamma^{\bar{\sigma}} e_r) \\
& + i g_L g_Y^2 \bar{\mathcal{C}}_{eB}^{rs} t_j^{Ii} H_i^\dagger B_{\bar{\mu}} W_{\bar{\nu}}^I (\bar{e}_s \sigma^{\bar{\mu}\bar{\nu}} \ell_r^j) - i g_L g_Y^2 \mathcal{C}_{eB}^{sr} t_j^{Ii} H^j B_{\bar{\mu}} W_{\bar{\nu}}^I (\bar{\ell}_{is} \sigma^{\bar{\mu}\bar{\nu}} e_r) \\
& - \frac{13i}{12} g_Y^2 \mathcal{C}_{eB}^{sr} B_{\bar{\mu}} (\bar{\ell}_s H \partial^{\bar{\mu}} e_r) + \frac{13i}{12} g_Y^2 \bar{\mathcal{C}}_{eB}^{rs} B_{\bar{\mu}} (\partial^{\bar{\mu}} \bar{e}_s H^\dagger \ell_r) \\
& - 2i g_L g_Y \left[ \bar{y}_e^{rs} \mathcal{C}_{eB}^{rs} - y_e^{rs} \bar{\mathcal{C}}_{eB}^{rs} \right] B_{\bar{\mu}} W_{\bar{\nu}}^I B^{\bar{\mu}\bar{\nu}} (H^\dagger t^I H) + 2g_L g_Y \left[ \bar{y}_e^{rs} \mathcal{C}_{eB}^{rs} + y_e^{rs} \bar{\mathcal{C}}_{eB}^{rs} \right] B_{\bar{\mu}} W_{\bar{\nu}}^I \tilde{B}^{\bar{\mu}\bar{\nu}} (H^\dagger t^I H) \\
& + \frac{23}{8} g_Y^3 \bar{\mathcal{C}}_{eB}^{rs} B_{\bar{\mu}}^2 (\bar{e}_s H^\dagger \ell_r) + \frac{23}{8} g_Y^3 \mathcal{C}_{eB}^{sr} B_{\bar{\mu}}^2 (\bar{\ell}_s H e_r) - g_Y^2 \left[ \bar{y}_e^{ts} \mathcal{C}_{eB}^{tr} + y_e^{tr} \bar{\mathcal{C}}_{eB}^{ts} \right] (H^\dagger H) (\bar{e}_s \tilde{B} e_r) \\
& + i g_Y \left[ \bar{y}_e^{rt} \mathcal{C}_{eB}^{st} - y_e^{st} \bar{\mathcal{C}}_{eB}^{rt} \right] B_{\bar{\mu}} B^{\bar{\mu}\bar{\nu}} (\bar{\ell}_s \gamma^{\bar{\nu}} \ell_r), \tag{2.21}
\end{aligned}$$

$$\begin{aligned}
\Delta S_{\mathcal{O}_{eW}} &= -\frac{i}{6} \left[ \bar{y}_e^{rs} \mathcal{C}_{eW}^{rs} + y_e^{rs} \bar{\mathcal{C}}_{eW}^{rs} \right] \left[ 2g_L W_{\bar{\mu}}^I \widetilde{W}^{\bar{\mu}\bar{\sigma}I} (H^\dagger \partial_{\bar{\sigma}} H) - 2g_L W_{\bar{\mu}}^I \widetilde{W}^{\bar{\mu}\bar{\sigma}I} (\partial_{\bar{\sigma}} H^\dagger H) \right] \\
&+ \frac{i}{6} \left[ \bar{y}_e^{rs} \mathcal{C}_{eW}^{rs} - y_e^{rs} \bar{\mathcal{C}}_{eW}^{rs} \right] \left[ 2g_L W_{\bar{\mu}}^I \widetilde{W}^{\bar{\mu}\bar{\sigma}I} (H^\dagger \partial_{\bar{\sigma}} H) + 2g_L W_{\bar{\mu}}^I \widetilde{W}^{\bar{\mu}\bar{\sigma}I} (\partial_{\bar{\sigma}} H^\dagger H) \right] \\
&+ \frac{1}{6} g_L^3 \bar{\mathcal{C}}_{eW}^{rs} \varepsilon^{IJK} t_j^{K^i} H_i^\dagger W_{\bar{\mu}}^J W_{\bar{\nu}}^I (\bar{e}_s \sigma^{\bar{\mu}\bar{\nu}} \ell_r^j) + \frac{1}{6} g_L^3 \mathcal{C}_{eW}^{sr} \varepsilon^{IJK} t_j^{K^i} H^j W_{\bar{\mu}}^J W_{\bar{\nu}}^I (\bar{\ell}_{is} \sigma^{\bar{\mu}\bar{\nu}} e_r)
\end{aligned}$$

$$\begin{aligned}
& + \frac{1}{3} g_L^2 \left[ -\bar{y}_e^{rs} \mathcal{C}_{eW}^{rs} - y_e^{rs} \bar{\mathcal{C}}_{eW}^{rs} \right] \varepsilon^{IJK} W_{\bar{\mu}}^K W_{\bar{\nu}}^J W^{\bar{\mu}\bar{\nu}I} (H^\dagger H) - \frac{1}{8} g_L^3 \mathcal{C}_{eW}^{sr} W_{\bar{\mu}}^I{}^2 (\bar{\ell}_s H e_r) \\
& + \frac{i}{6} g_L^2 \mathcal{C}_{eW}^{sr} t_j^{Ii} H^j W_{\bar{\mu}}^I (\bar{\ell}_{is} \partial^\mu e_r) - \frac{i}{6} g_L^2 \bar{\mathcal{C}}_{eW}^{rs} t_j^I H_i^\dagger W_{\bar{\mu}}^I (\partial^\mu \bar{e}_s \ell_r^j) + \frac{i}{4} g_L g_Y \mathcal{C}_{eW}^{sr} B_{\bar{\mu}} (\bar{\ell}_s H \partial^\mu e_r) \\
& + \frac{1}{4} g_L^2 \left[ \bar{y}_e^{rt} \mathcal{C}_{eW}^{st} + y_e^{st} \bar{\mathcal{C}}_{eW}^{rt} \right] (H^\dagger H) (\bar{\ell}_s t^I \bar{W}^I \ell_r) \\
& + \frac{1}{4} g_L \left[ \bar{y}_e^{rt} \mathcal{C}_{eW}^{st} - y_e^{st} \bar{\mathcal{C}}_{eW}^{rt} \right] \left[ g_L t_j^I H_i^\dagger (\bar{\ell}_s H \bar{W}^I \ell_r^j) - g_L t_k^{Ij} H^k (\bar{\ell}_{js} \bar{W}^I H^\dagger \ell_r) \right] \\
& - \frac{i}{4} g_L g_Y \bar{\mathcal{C}}_{eW}^{rs} B_{\bar{\mu}} (\partial^\mu \bar{e}_s H^\dagger \ell_r) - \frac{i}{3} g_L^2 \left[ \bar{y}_e^{rs} \mathcal{C}_{eW}^{rs} - y_e^{rs} \bar{\mathcal{C}}_{eW}^{rs} \right] \varepsilon^{IJK} W_{\bar{\mu}}^K W_{\bar{\nu}}^J \widetilde{W}^{\bar{\mu}\bar{\nu}I} (H^\dagger H) \\
& + \frac{1}{3} \left[ \bar{y}_e^{rs} \mathcal{C}_{eW}^{rs} + y_e^{rs} \bar{\mathcal{C}}_{eW}^{rs} \right] \left[ g_L W_{\bar{\mu}}^I W^{\bar{\mu}\bar{\nu}I} (H^\dagger \partial_{\bar{\nu}} H) + g_L W_{\bar{\mu}}^I W^{\bar{\mu}\bar{\nu}I} (\partial_{\bar{\nu}} H^\dagger H) \right] \\
& + \frac{1}{3} \left[ y_e^{rs} \bar{\mathcal{C}}_{eW}^{rs} - \bar{y}_e^{rs} \mathcal{C}_{eW}^{rs} \right] \left[ 2g_L \varepsilon^{IJK} W_{\bar{\mu}}^J \widetilde{W}^{\bar{\mu}\bar{\sigma}I} (H^\dagger t^K \partial_{\bar{\sigma}} H) - 2g_L \varepsilon^{IJK} W_{\bar{\mu}}^J \widetilde{W}^{\bar{\mu}\bar{\sigma}I} (\partial_{\bar{\sigma}} H^\dagger t^K H) \right] \\
& + \frac{1}{3} \left[ \bar{y}_e^{rs} \mathcal{C}_{eW}^{rs} + y_e^{rs} \bar{\mathcal{C}}_{eW}^{rs} \right] \left[ 2g_L \varepsilon^{IJK} W_{\bar{\mu}}^J \widetilde{W}^{\bar{\mu}\bar{\sigma}I} (H^\dagger t^K \partial_{\bar{\sigma}} H) + 2g_L \varepsilon^{IJK} W_{\bar{\mu}}^J \widetilde{W}^{\bar{\mu}\bar{\sigma}I} (\partial_{\bar{\sigma}} H^\dagger t^K H) \right] \\
& - \frac{1}{8} g_L^3 \bar{\mathcal{C}}_{eW}^{rs} W_{\bar{\mu}}^I{}^2 (\bar{e}_s H^\dagger \ell_r) - \frac{i}{3} g_L^2 g_Y \bar{\mathcal{C}}_{eW}^{rs} t_j^{Ii} H_i^\dagger B_{\bar{\mu}} W_{\bar{\nu}}^I (\bar{e}_s \sigma^{\bar{\mu}\bar{\nu}} \ell_r^j) \\
& + \frac{i}{3} g_L^2 g_Y \mathcal{C}_{eW}^{sr} t_j^{Ii} H^j B_{\bar{\mu}} W_{\bar{\nu}}^I (\bar{\ell}_{is} \sigma^{\bar{\mu}\bar{\nu}} e_r) + \frac{1}{3} g_L \left[ y_e^{rs} \bar{\mathcal{C}}_{eW}^{rs} - \bar{y}_e^{rs} \mathcal{C}_{eW}^{rs} \right] W_{\bar{\mu}}^I W^{\bar{\mu}\bar{\nu}I} (H^\dagger \partial_{\bar{\nu}} H) \\
& + \frac{i}{2} g_L^2 \bar{\mathcal{C}}_{eW}^{rs} t_j^{Ii} H_i^\dagger W_{\bar{\mu}}^I (\bar{e}_s \partial^\mu \ell_r^j) + \frac{1}{2} g_L g_Y \left[ \bar{y}_e^{rt} \mathcal{C}_{eW}^{st} + y_e^{st} \bar{\mathcal{C}}_{eW}^{rt} \right] (H^\dagger H) (\bar{\ell}_s \bar{B} \ell_r) \\
& - \frac{2i}{3} \left[ \bar{y}_e^{rs} \mathcal{C}_{eW}^{rs} - y_e^{rs} \bar{\mathcal{C}}_{eW}^{rs} \right] \left[ g_L \varepsilon^{IJK} W_{\bar{\mu}}^J W^{\bar{\mu}\bar{\nu}I} (H^\dagger t^K \partial_{\bar{\nu}} H) + g_L \varepsilon^{IJK} W_{\bar{\mu}}^J W^{\bar{\mu}\bar{\nu}I} (\partial_{\bar{\nu}} H^\dagger t^K H) \right] \\
& + \frac{3i}{4} g_L g_Y \bar{\mathcal{C}}_{eW}^{rs} B_{\bar{\mu}} (\bar{e}_s H^\dagger \partial^\mu \ell_r) - \frac{3i}{4} g_L g_Y \bar{\mathcal{C}}_{eW}^{rs} B_{\bar{\mu}} (\bar{e}_s \partial^\mu H^\dagger \ell_r) + \frac{5}{6} g_L^2 g_Y \bar{\mathcal{C}}_{eW}^{rs} t_j^{Ii} H_i^\dagger B_{\bar{\mu}} W_{\bar{\mu}}^I (\bar{e}_s \ell_r^j) \\
& + \frac{5}{6} g_L^2 g_Y \mathcal{C}_{eW}^{sr} t_j^{Ii} H^j B_{\bar{\mu}} W_{\bar{\mu}}^I (\bar{\ell}_{is} e_r) - \frac{1}{4} g_L g_Y \left[ \bar{y}_e^{rt} \mathcal{C}_{eW}^{st} + y_e^{st} \bar{\mathcal{C}}_{eW}^{rt} \right] (\bar{\ell}_s H \bar{B} H^\dagger \ell_r) \\
& - \frac{1}{3} g_L^2 \bar{\mathcal{C}}_{eW}^{rs} t_j^{Ii} W_{\bar{\mu}}^I (\bar{e}_s \sigma^{\bar{\mu}\bar{\nu}} \ell_r^j) \partial^{\bar{\nu}} H_i^\dagger - \frac{1}{3} g_L^2 \mathcal{C}_{eW}^{sr} t_j^I W_{\bar{\mu}}^I (\bar{\ell}_{is} \sigma^{\bar{\mu}\bar{\nu}} e_r) \partial^{\bar{\nu}} H^j \\
& - \frac{1}{2} g_L g_Y \bar{\mathcal{C}}_{eW}^{rs} B_{\bar{\mu}} (\bar{e}_s \sigma^{\bar{\mu}\bar{\nu}} \partial^{\bar{\nu}} H^\dagger \ell_r) - \frac{1}{2} g_L g_Y \mathcal{C}_{eW}^{sr} B_{\bar{\mu}} (\bar{\ell}_s \partial^{\bar{\nu}} H \sigma^{\bar{\mu}\bar{\nu}} e_r) \\
& - \frac{i}{2} g_L^2 \mathcal{C}_{eW}^{sr} t_j^{Ii} H^j W_{\bar{\mu}}^I (\partial^\mu \bar{\ell}_{is} e_r) - \frac{i}{2} g_L^2 \bar{\mathcal{C}}_{eW}^{rs} t_j^I W_{\bar{\mu}}^I (\bar{e}_s \ell_r^j) \partial^\mu H_i^\dagger \\
& + \frac{i}{2} g_L^2 \mathcal{C}_{eW}^{sr} t_j^{Ii} W_{\bar{\mu}}^I (\bar{\ell}_{is} e_r) \partial^\mu H^j - \frac{5}{8} g_L g_Y^2 \bar{\mathcal{C}}_{eW}^{rs} B_{\bar{\mu}}^2 (\bar{e}_s H^\dagger \ell_r) - \frac{5}{8} g_L g_Y^2 \mathcal{C}_{eW}^{sr} B_{\bar{\mu}}^2 (\bar{\ell}_s H e_r) \\
& + \frac{2i}{3} g_L \left[ \bar{y}_e^{rs} \mathcal{C}_{eW}^{rs} + y_e^{rs} \bar{\mathcal{C}}_{eW}^{rs} \right] \varepsilon^{IJK} W_{\bar{\mu}}^J W^{\bar{\mu}\bar{\nu}I} (H^\dagger t^K \partial_{\bar{\nu}} H) + \frac{3i}{4} g_L g_Y \mathcal{C}_{eW}^{sr} B_{\bar{\mu}} (\bar{\ell}_s \partial^\mu H e_r) \\
& - \frac{3}{4} g_L^2 \left[ \bar{y}_e^{rt} \mathcal{C}_{eW}^{st} + y_e^{st} \bar{\mathcal{C}}_{eW}^{rt} \right] (H^\dagger t^I H) (\bar{\ell}_s \bar{W}^I \ell_r) - \frac{3i}{4} g_L g_Y \mathcal{C}_{eW}^{sr} B_{\bar{\mu}} (\partial^\mu \bar{\ell}_s H e_r) \\
& - i g_L g_Y \left[ \bar{y}_e^{rs} \mathcal{C}_{eW}^{rs} - y_e^{rs} \bar{\mathcal{C}}_{eW}^{rs} \right] B_{\bar{\mu}} W_{\bar{\nu}}^I W^{\bar{\mu}\bar{\nu}I} (H^\dagger H) + g_L g_Y \left[ \bar{y}_e^{rs} \mathcal{C}_{eW}^{rs} + y_e^{rs} \bar{\mathcal{C}}_{eW}^{rs} \right] B_{\bar{\mu}} W_{\bar{\nu}}^I \widetilde{W}^{\bar{\mu}\bar{\nu}I} (H^\dagger H) \\
& + i \left[ \bar{y}_e^{rs} \mathcal{C}_{eW}^{rs} + y_e^{rs} \bar{\mathcal{C}}_{eW}^{rs} \right] \left[ 2g_Y B_{\bar{\mu}} \widetilde{W}^{\bar{\mu}\bar{\sigma}I} (H^\dagger t^I \partial_{\bar{\sigma}} H) - 2g_Y B_{\bar{\mu}} \widetilde{W}^{\bar{\mu}\bar{\sigma}I} (\partial_{\bar{\sigma}} H^\dagger t^I H) \right] \\
& - i \left[ \bar{y}_e^{rs} \mathcal{C}_{eW}^{rs} - y_e^{rs} \bar{\mathcal{C}}_{eW}^{rs} \right] \left[ 2g_Y B_{\bar{\mu}} \widetilde{W}^{\bar{\mu}\bar{\sigma}I} (H^\dagger t^I \partial_{\bar{\sigma}} H) + 2g_Y B_{\bar{\mu}} \widetilde{W}^{\bar{\mu}\bar{\sigma}I} (\partial_{\bar{\sigma}} H^\dagger t^I H) \right] \\
& + i g_L \left[ \bar{y}_e^{ts} \mathcal{C}_{eW}^{tr} - y_e^{tr} \bar{\mathcal{C}}_{eW}^{ts} \right] W_{\bar{\mu}}^I W^{\bar{\mu}\bar{\nu}I} (\bar{e}_s \gamma^{\bar{\nu}} e_r) + g_L \left[ \bar{y}_e^{ts} \mathcal{C}_{eW}^{tr} + y_e^{tr} \bar{\mathcal{C}}_{eW}^{ts} \right] W_{\bar{\mu}}^I \widetilde{W}^{\bar{\mu}\bar{\sigma}I} (\bar{e}_s \gamma^{\bar{\sigma}} e_r)
\end{aligned}$$

$$\begin{aligned}
& + g_Y \left[ 2\bar{y}_e^{rs} \mathcal{C}_{eW}^{rs} - 2y_e^{rs} \bar{\mathcal{C}}_{eW}^{rs} \right] B_{\bar{\mu}} W^{\bar{\mu}\bar{\nu}I} (H^\dagger t^I \bar{\partial}_{\bar{\nu}} H) \\
& - \frac{4i}{3} g_L^2 \left[ \bar{y}_e^{rs} \mathcal{C}_{eW}^{rs} - y_e^{rs} \bar{\mathcal{C}}_{eW}^{rs} \right] W_{\bar{\mu}}^I W_{\bar{\nu}}^J W^{\bar{\mu}\bar{\nu}J} (H^\dagger t^I H) \\
& + \frac{4}{3} g_L^2 \left[ \bar{y}_e^{rs} \mathcal{C}_{eW}^{rs} + y_e^{rs} \bar{\mathcal{C}}_{eW}^{rs} \right] W_{\bar{\mu}}^I W_{\bar{\nu}}^J \widetilde{W}^{\bar{\mu}\bar{\nu}J} (H^\dagger t^I H) \\
& - 2 \left[ \bar{y}_e^{rs} \mathcal{C}_{eW}^{rs} + y_e^{rs} \bar{\mathcal{C}}_{eW}^{rs} \right] \left[ g_Y B_{\bar{\mu}} W^{\bar{\mu}\bar{\nu}I} (H^\dagger t^I \partial_{\bar{\nu}} H) + g_Y B_{\bar{\mu}} W^{\bar{\mu}\bar{\nu}I} (\partial_{\bar{\nu}} H^\dagger t^I H) \right] \\
& - 2g_L g_Y \left[ \bar{y}_e^{rs} \mathcal{C}_{eW}^{rs} + y_e^{rs} \bar{\mathcal{C}}_{eW}^{rs} \right] \varepsilon^{IJK} B_{\bar{\mu}} W_{\bar{\nu}}^J W^{\bar{\mu}\bar{\nu}I} (H^\dagger t^K H) \\
& - 2ig_L g_Y \left[ \bar{y}_e^{rs} \mathcal{C}_{eW}^{rs} - y_e^{rs} \bar{\mathcal{C}}_{eW}^{rs} \right] \varepsilon^{IJK} B_{\bar{\mu}} W_{\bar{\nu}}^J \widetilde{W}^{\bar{\mu}\bar{\nu}I} (H^\dagger t^K H) \\
& + 2ig_Y \left[ \bar{y}_e^{rt} \mathcal{C}_{eW}^{st} - y_e^{st} \bar{\mathcal{C}}_{eW}^{rt} \right] B_{\bar{\mu}} W^{\bar{\mu}\bar{\nu}I} (\bar{\ell}_s t^I \gamma^{\bar{\nu}} \ell_r) \\
& + 2g_Y \left[ \bar{y}_e^{rt} \mathcal{C}_{eW}^{st} + y_e^{st} \bar{\mathcal{C}}_{eW}^{rt} \right] B_{\bar{\mu}} \widetilde{W}^{\bar{\mu}\bar{\sigma}I} (\bar{\ell}_s t^I \gamma^{\bar{\sigma}} \ell_r), \tag{2.22}
\end{aligned}$$

$$\begin{aligned}
\Delta S_{\mathcal{O}_{uB}} &= \frac{1}{36} g_Y^2 \left[ \bar{y}_u^{rt} \mathcal{C}_{uB}^{st} + y_u^{st} \bar{\mathcal{C}}_{uB}^{rt} \right] (\bar{q}_s H \bar{B} H^\dagger q_r) - \frac{i}{18} g_L g_Y \mathcal{C}_{uB}^{sr} \varepsilon^{jk} t_j^{Ii} H_i^\dagger W_{\bar{\mu}}^I (\bar{q}_{ks} \partial^{\bar{\mu}} u_r) \\
& + \frac{i}{18} g_L g_Y \bar{\mathcal{C}}_{uB}^{rs} \bar{\varepsilon}_{ij} t_k^{Ii} H^k W_{\bar{\mu}}^I (\partial^{\bar{\mu}} \bar{u}_s q_r^j) + \frac{1}{12} g_L^2 g_Y \mathcal{C}_{uB}^{sr} W_{\bar{\mu}}^{I2} (\bar{q}_s \tilde{H} u_r) \\
& + \frac{1}{12} g_L g_Y \left[ \bar{y}_u^{rt} \mathcal{C}_{uB}^{st} + y_u^{st} \bar{\mathcal{C}}_{uB}^{rt} \right] (H^\dagger t^I H) (\bar{q}_s \bar{W}^I q_r) \\
& + \frac{1}{12} g_Y \left[ \bar{y}_u^{rt} \mathcal{C}_{uB}^{st} - y_u^{st} \bar{\mathcal{C}}_{uB}^{rt} \right] \left[ g_L t_j^{Ii} H_i^\dagger (\bar{q}_s H \bar{W}^I q_r^j) - g_L t_k^{Ij} H^k (\bar{q}_{js} \bar{W}^I H^\dagger q_r) \right] \\
& + \frac{1}{12} g_L^2 g_Y \bar{\mathcal{C}}_{uB}^{rs} W_{\bar{\mu}}^{I2} (\bar{u}_s \tilde{H}^\dagger q_r) - \frac{1}{36} g_Y^2 \left[ \bar{y}_u^{rt} \mathcal{C}_{uB}^{st} + y_u^{st} \bar{\mathcal{C}}_{uB}^{rt} \right] (H^\dagger H) (\bar{q}_s \bar{B} q_r) \\
& - \frac{i}{9} g_L^2 g_Y \mathcal{C}_{uB}^{sr} t_l^{Ik} t_j^{Jl} \tilde{H}_j W_{\bar{\mu}}^I W_{\bar{\nu}}^J (\bar{q}_{ks} \sigma^{\bar{\mu}\bar{\nu}} u_r) + \frac{i}{9} g_L^2 g_Y \bar{\mathcal{C}}_{uB}^{rs} t_l^{Ik} t_k^{Ji} \tilde{H}^\dagger{}^i W_{\bar{\mu}}^I W_{\bar{\nu}}^J (\bar{u}_s \sigma^{\bar{\mu}\bar{\nu}} q_r^l) \\
& + \frac{1}{9} g_L g_Y \mathcal{C}_{uB}^{sr} \varepsilon^{ij} t_i^{Ik} W_{\bar{\mu}}^I (\bar{q}_{js} \sigma^{\bar{\mu}\bar{\nu}} u_r) \partial^{\bar{\nu}} H_k^\dagger + \frac{1}{9} g_L g_Y \bar{\mathcal{C}}_{uB}^{rs} \bar{\varepsilon}_{ij} t_k^{Ii} W_{\bar{\mu}}^I (\bar{u}_s \sigma^{\bar{\mu}\bar{\nu}} q_r^j) \partial^{\bar{\nu}} H^k \\
& + \frac{1}{6} g_s g_Y \left[ \bar{y}_u^{rt} \mathcal{C}_{uB}^{st} + y_u^{st} \bar{\mathcal{C}}_{uB}^{rt} \right] (\bar{q}_s T^A H \bar{G}^A H^\dagger q_r) + \frac{1}{6} g_L^2 g_Y \mathcal{C}_{uB}^{sr} \varepsilon^{jk} t_l^{Ii} t_j^{Jl} H_i^\dagger W_{\bar{\mu}}^I W_{\bar{\nu}}^J (\bar{q}_{ks} u_r) \\
& + \frac{1}{6} g_L^2 g_Y \bar{\mathcal{C}}_{uB}^{rs} \bar{\varepsilon}_{ij} t_l^{Ik} t_k^{Ji} H^l W_{\bar{\mu}}^I W_{\bar{\nu}}^J (\bar{u}_s q_r^j) - \frac{i}{6} g_L g_Y \bar{\mathcal{C}}_{uB}^{rs} \bar{\varepsilon}_{ij} t_k^{Ii} H^k W_{\bar{\mu}}^I (\bar{u}_s \partial^{\bar{\mu}} q_r^j) \\
& + \frac{i}{6} g_L g_Y \mathcal{C}_{uB}^{sr} \varepsilon^{jk} t_j^{Ii} H_i^\dagger W_{\bar{\mu}}^I (\partial^{\bar{\mu}} \bar{q}_{ks} u_r) - \frac{i}{6} g_L g_Y \mathcal{C}_{uB}^{sr} \varepsilon^{ij} t_i^{Ik} W_{\bar{\mu}}^I (\bar{q}_{js} u_r) \partial^{\bar{\mu}} H_k^\dagger \\
& + \frac{i}{6} g_L g_Y \bar{\mathcal{C}}_{uB}^{rs} \bar{\varepsilon}_{ij} t_k^{Ii} W_{\bar{\mu}}^I (\bar{u}_s q_r^j) \partial^{\bar{\mu}} H^k + \frac{19i}{108} g_Y^2 \bar{\mathcal{C}}_{uB}^{rs} B_{\bar{\mu}} (\bar{u}_s \tilde{H}^\dagger \partial^{\bar{\mu}} q_r) \\
& - \frac{19i}{108} g_Y^2 \mathcal{C}_{uB}^{sr} B_{\bar{\mu}} (\partial^{\bar{\mu}} \bar{q}_s \tilde{H} u_r) + \frac{11}{54} g_L g_Y^2 \mathcal{C}_{uB}^{sr} t_j^{Ik} \tilde{H}_j B_{\bar{\mu}} W_{\bar{\mu}}^I (\bar{q}_{ks} u_r) \\
& + \frac{11}{54} g_L g_Y^2 \bar{\mathcal{C}}_{uB}^{rs} t_k^{Ii} \tilde{H}^\dagger{}^i B_{\bar{\mu}} W_{\bar{\mu}}^I (\bar{u}_s q_r^k) + \frac{5i}{18} g_s g_Y^2 \mathcal{C}_{uB}^{sr} T_b^{Aa} B_{\bar{\mu}} G_{\bar{\nu}}^A (\bar{q}_{as} \tilde{H} \sigma^{\bar{\mu}\bar{\nu}} u_r^b) \\
& - \frac{5i}{18} g_s g_Y^2 \bar{\mathcal{C}}_{uB}^{rs} T_b^{Aa} B_{\bar{\mu}} G_{\bar{\nu}}^A (\bar{u}_{as} \sigma^{\bar{\mu}\bar{\nu}} \tilde{H}^\dagger q_r^b) + \frac{17}{54} g_Y^2 \mathcal{C}_{uB}^{sr} B_{\bar{\mu}} (\bar{q}_s \partial^{\bar{\nu}} \tilde{H} \sigma^{\bar{\mu}\bar{\nu}} u_r) \\
& + \frac{17}{54} g_Y^2 \bar{\mathcal{C}}_{uB}^{rs} B_{\bar{\mu}} (\bar{u}_s \sigma^{\bar{\mu}\bar{\nu}} \partial^{\bar{\nu}} \tilde{H} q_r) - \frac{1}{12} g_L g_Y \left[ \bar{y}_u^{rt} \mathcal{C}_{uB}^{st} + y_u^{st} \bar{\mathcal{C}}_{uB}^{rt} \right] (H^\dagger H) (\bar{q}_s t^I \bar{W}^I q_r)
\end{aligned}$$

$$\begin{aligned}
& + \frac{i}{3} g_Y \left[ \bar{y}_u^{ts} \mathcal{C}_{uB}^{tr} - y_u^{tr} \bar{\mathcal{C}}_{uB}^{ts} \right] B_{\bar{\mu}} B^{\bar{\mu}\bar{\nu}} (\bar{u}_s \gamma^{\bar{\nu}} u_r) + \frac{1}{3} g_Y \left[ \bar{y}_u^{ts} \mathcal{C}_{uB}^{tr} + y_u^{tr} \bar{\mathcal{C}}_{uB}^{ts} \right] B_{\bar{\mu}} \tilde{B}^{\bar{\mu}\bar{\sigma}} (\bar{u}_s \gamma^{\bar{\sigma}} u_r) \\
& - \frac{10i}{27} g_L g_Y^2 \mathcal{C}_{uB}^{sr} \varepsilon^{jk} t_j^I H_i^\dagger B_{\bar{\mu}} W_\nu^I (\bar{q}_{ks} \sigma^{\bar{\mu}\bar{\nu}} u_r) + \frac{10i}{27} g_L g_Y^2 \bar{\mathcal{C}}_{uB}^{rs} \bar{\varepsilon}_{ij} t_k^I H^k B_{\bar{\mu}} W_\nu^I (\bar{u}_s \sigma^{\bar{\mu}\bar{\nu}} q_r^j) \\
& + \frac{7i}{18} g_s g_Y \bar{\mathcal{C}}_{uB}^{rs} T_b^{Aa} G_\mu^A (\bar{u}_{as} \tilde{H}^\dagger \partial^{\bar{\mu}} q_r^b) - \frac{7i}{18} g_s g_Y \mathcal{C}_{uB}^{sr} T_b^{Aa} G_\mu^A (\partial^{\bar{\mu}} \bar{q}_{as} \tilde{H} u_r^b) \\
& + \frac{5i}{12} g_Y^2 \mathcal{C}_{uB}^{sr} B_{\bar{\mu}} (\bar{q}_s \partial^{\bar{\mu}} \tilde{H} u_r) - \frac{5i}{12} g_Y^2 \bar{\mathcal{C}}_{uB}^{rs} B_{\bar{\mu}} (\bar{u}_s \partial^{\bar{\mu}} \tilde{H} q_r) + \frac{49i}{108} g_Y^2 \mathcal{C}_{uB}^{sr} B_{\bar{\mu}} (\bar{q}_s \tilde{H} \partial^{\bar{\mu}} u_r) \\
& - \frac{49i}{108} g_Y^2 \bar{\mathcal{C}}_{uB}^{rs} B_{\bar{\mu}} (\partial^{\bar{\mu}} \bar{u}_s \tilde{H}^\dagger q_r) + \frac{i}{2} g_s g_Y \mathcal{C}_{uB}^{sr} T_b^{Aa} G_\mu^A (\bar{q}_{as} \partial^{\bar{\mu}} \tilde{H} u_r^b) \\
& - \frac{i}{2} g_s g_Y \bar{\mathcal{C}}_{uB}^{rs} T_b^{Aa} G_\mu^A (\bar{u}_{as} \partial^{\bar{\mu}} \tilde{H} q_r^b) + \frac{5i}{9} g_L g_s g_Y \bar{\mathcal{C}}_{uB}^{rs} \bar{\varepsilon}_{ij} t_k^I T_b^{Aa} H^k G_\mu^A W_\nu^I (\bar{u}_{as} \sigma^{\bar{\mu}\bar{\nu}} q_r^{bj}) \\
& - \frac{2i}{3} g_Y \left[ \bar{y}_u^{rt} \mathcal{C}_{uB}^{st} - y_u^{st} \bar{\mathcal{C}}_{uB}^{rt} \right] B_{\bar{\mu}} B^{\bar{\mu}\bar{\nu}} (\bar{q}_s \gamma^{\bar{\nu}} q_r) \\
& + \frac{2}{3} g_Y \left[ -\bar{y}_u^{rt} \mathcal{C}_{uB}^{st} - y_u^{st} \bar{\mathcal{C}}_{uB}^{rt} \right] B_{\bar{\mu}} \tilde{B}^{\bar{\mu}\bar{\sigma}} (\bar{q}_s \gamma^{\bar{\sigma}} q_r) + \frac{13i}{18} g_s g_Y \mathcal{C}_{uB}^{sr} T_b^{Aa} G_\mu^A (\bar{q}_{as} \tilde{H} \partial^{\bar{\mu}} u_r^b) \\
& - \frac{13i}{18} g_s g_Y \bar{\mathcal{C}}_{uB}^{rs} T_b^{Aa} G_\mu^A (\partial^{\bar{\mu}} \bar{u}_{as} \tilde{H}^\dagger q_r^b) \\
& + \frac{5i}{6} \left[ \bar{y}_u^{rs} \mathcal{C}_{uB}^{rs} + y_u^{rs} \bar{\mathcal{C}}_{uB}^{rs} \right] \left[ 2g_Y B_{\bar{\mu}} \tilde{B}^{\bar{\mu}\bar{\sigma}} (H^\dagger \partial_{\bar{\sigma}} H) - 2g_Y B_{\bar{\mu}} \tilde{B}^{\bar{\mu}\bar{\sigma}} (\partial_{\bar{\sigma}} H^\dagger H) \right] \\
& + \frac{5i}{6} \left[ \bar{y}_u^{rs} \mathcal{C}_{uB}^{rs} - y_u^{rs} \bar{\mathcal{C}}_{uB}^{rs} \right] \left[ 2g_Y B_{\bar{\mu}} \tilde{B}^{\bar{\mu}\bar{\sigma}} (H^\dagger \partial_{\bar{\sigma}} H) + 2g_Y B_{\bar{\mu}} \tilde{B}^{\bar{\mu}\bar{\sigma}} (\partial_{\bar{\sigma}} H^\dagger H) \right] \\
& + \frac{545}{648} g_Y^3 \mathcal{C}_{uB}^{sr} B_{\bar{\mu}}^2 (\bar{q}_s \tilde{H} u_r) + \frac{545}{648} g_Y^3 \bar{\mathcal{C}}_{uB}^{rs} B_{\bar{\mu}}^2 (\bar{u}_s \tilde{H}^\dagger q_r) \\
& - i \left[ \bar{y}_u^{rs} \mathcal{C}_{uB}^{rs} + y_u^{rs} \bar{\mathcal{C}}_{uB}^{rs} \right] \left[ 2g_L W_\mu^I \tilde{B}^{\bar{\mu}\bar{\sigma}} (H^\dagger t^I \partial_{\bar{\sigma}} H) - 2g_L W_\mu^I \tilde{B}^{\bar{\mu}\bar{\sigma}} (\partial_{\bar{\sigma}} H^\dagger t^I H) \right] \\
& - i \left[ \bar{y}_u^{rs} \mathcal{C}_{uB}^{rs} - y_u^{rs} \bar{\mathcal{C}}_{uB}^{rs} \right] \left[ 2g_L W_\mu^I \tilde{B}^{\bar{\mu}\bar{\sigma}} (H^\dagger t^I \partial_{\bar{\sigma}} H) + 2g_L W_\mu^I \tilde{B}^{\bar{\mu}\bar{\sigma}} (\partial_{\bar{\sigma}} H^\dagger t^I H) \right] \\
& - i g_s \left[ \bar{y}_u^{rt} \mathcal{C}_{uB}^{st} - y_u^{st} \bar{\mathcal{C}}_{uB}^{rt} \right] G_\mu^A B^{\bar{\mu}\bar{\nu}} (\bar{q}_s T^A \gamma^{\bar{\nu}} q_r) + g_s \left[ -\bar{y}_u^{rt} \mathcal{C}_{uB}^{st} - y_u^{st} \bar{\mathcal{C}}_{uB}^{rt} \right] G_\mu^A \tilde{B}^{\bar{\mu}\bar{\sigma}} (\bar{q}_s T^A \gamma^{\bar{\sigma}} q_r) \\
& + g_L \left[ 2y_u^{rs} \bar{\mathcal{C}}_{uB}^{rs} - 2\bar{y}_u^{rs} \mathcal{C}_{uB}^{rs} \right] W_\mu^I B^{\bar{\mu}\bar{\nu}} (H^\dagger t^I \partial_{\bar{\nu}} H) \\
& + \frac{5}{3} \left[ \bar{y}_u^{rs} \mathcal{C}_{uB}^{rs} + y_u^{rs} \bar{\mathcal{C}}_{uB}^{rs} \right] \left[ g_Y B_{\bar{\mu}} B^{\bar{\mu}\bar{\nu}} (H^\dagger \partial_{\bar{\nu}} H) + g_Y B_{\bar{\mu}} B^{\bar{\mu}\bar{\nu}} (\partial_{\bar{\nu}} H^\dagger H) \right] \\
& + \frac{5}{3} g_Y \left[ \bar{y}_u^{rs} \mathcal{C}_{uB}^{rs} - y_u^{rs} \bar{\mathcal{C}}_{uB}^{rs} \right] B_{\bar{\mu}} B^{\bar{\mu}\bar{\nu}} (H^\dagger \partial_{\bar{\nu}} H) + \frac{35}{18} g_s^2 g_Y \mathcal{C}_{uB}^{sr} T_b^{Aa} T_a^{Bc} G_\mu^A G_\mu^B (\bar{q}_{cs} \tilde{H} u_r^b) \\
& + \frac{35}{18} g_s^2 g_Y \bar{\mathcal{C}}_{uB}^{rs} T_b^{Aa} T_c^{Bb} G_\mu^A G_\mu^B (\bar{u}_{as} \tilde{H}^\dagger q_r^c) + 2g_L^2 \left[ \bar{y}_u^{rs} \mathcal{C}_{uB}^{rs} + y_u^{rs} \bar{\mathcal{C}}_{uB}^{rs} \right] \varepsilon^{IJK} W_\mu^J W_\nu^I B^{\bar{\mu}\bar{\nu}} (H^\dagger t^K H) \\
& + 2ig_L^2 \left[ \bar{y}_u^{rs} \mathcal{C}_{uB}^{rs} - y_u^{rs} \bar{\mathcal{C}}_{uB}^{rs} \right] \varepsilon^{IJK} W_\mu^J W_\nu^I \tilde{B}^{\bar{\mu}\bar{\nu}} (H^\dagger t^K H) + \frac{64}{27} g_s g_Y^2 \mathcal{C}_{uB}^{sr} T_b^{Aa} B_{\bar{\mu}} G_\mu^A (\bar{q}_{as} \tilde{H} u_r^b) \\
& + \frac{64}{27} g_s g_Y^2 \bar{\mathcal{C}}_{uB}^{rs} T_b^{Aa} B_{\bar{\mu}} G_\mu^A (\bar{u}_{as} \tilde{H}^\dagger q_r^b) - \frac{1}{6} g_s g_Y \left[ \bar{y}_u^{rt} \mathcal{C}_{uB}^{st} + y_u^{st} \bar{\mathcal{C}}_{uB}^{rt} \right] (H^\dagger H) (\bar{q}_s T^A \tilde{G}^A q_r) \\
& - \frac{4}{9} g_L g_s g_Y \mathcal{C}_{uB}^{sr} t_j^I T_b^{Aa} \tilde{H}_j G_\mu^A W_\mu^I (\bar{q}_{aks} u_r^b) - \frac{4}{9} g_Y^2 \left[ \bar{y}_u^{ts} \mathcal{C}_{uB}^{tr} + y_u^{tr} \bar{\mathcal{C}}_{uB}^{ts} \right] (H^\dagger H) (\bar{u}_s \tilde{B} u_r) \\
& - \frac{5}{9} g_s g_Y \mathcal{C}_{uB}^{sr} T_b^{Aa} G_\mu^A (\bar{q}_{as} \partial^{\bar{\nu}} \tilde{H} \sigma^{\bar{\mu}\bar{\nu}} u_r^b) - \frac{5i}{9} g_L g_s g_Y \mathcal{C}_{uB}^{sr} \varepsilon^{jk} t_j^I T_b^{Aa} H_i^\dagger G_\mu^A W_\nu^I (\bar{q}_{aks} \sigma^{\bar{\mu}\bar{\nu}} u_r^b) \\
& - \frac{5}{9} g_s g_Y \bar{\mathcal{C}}_{uB}^{rs} T_b^{Aa} G_\mu^A (\bar{u}_{as} \sigma^{\bar{\mu}\bar{\nu}} \partial^{\bar{\nu}} \tilde{H} q_r^b) + 2ig_s \left[ \bar{y}_u^{ts} \mathcal{C}_{uB}^{tr} - y_u^{tr} \bar{\mathcal{C}}_{uB}^{ts} \right] G_\mu^A B^{\bar{\mu}\bar{\nu}} (\bar{u}_s T^A \gamma^{\bar{\nu}} u_r)
\end{aligned}$$

$$\begin{aligned}
& + 2g_s \left[ \bar{y}_u^{ts} C_{uB}^{tr} + y_u^{tr} \bar{C}_{uB}^{ts} \right] G_{\bar{\mu}}^A \tilde{B}^{\bar{\mu}\bar{\sigma}} (\bar{u}_s T^A \gamma^{\bar{\sigma}} u_r) - \frac{4}{9} g_L g_s g_Y \bar{C}_{uB}^{rs} t_k^{Ii} T_b^{Aa} \tilde{H}^{\dagger i} G_{\bar{\mu}}^A W_{\bar{\mu}}^I (\bar{u}_{as} q_r^{bk}) \\
& - \frac{2}{3} g_s g_Y \left[ \bar{y}_u^{ts} C_{uB}^{tr} + y_u^{tr} \bar{C}_{uB}^{ts} \right] (H^\dagger H) (\bar{u}_s T^A \tilde{G}^A u_r) - 4i g_L g_Y \left[ \bar{y}_u^{rs} C_{uB}^{rs} - y_u^{rs} \bar{C}_{uB}^{rs} \right] B_{\bar{\mu}} W_{\bar{\nu}}^I B^{\bar{\mu}\bar{\nu}} (H^\dagger t^I H) \\
& + 4g_L g_Y \left[ \bar{y}_u^{rs} C_{uB}^{rs} + y_u^{rs} \bar{C}_{uB}^{rs} \right] B_{\bar{\mu}} W_{\bar{\nu}}^I \tilde{B}^{\bar{\mu}\bar{\nu}} (H^\dagger t^I H) \\
& - 2 \left[ \bar{y}_u^{rs} C_{uB}^{rs} + y_u^{rs} \bar{C}_{uB}^{rs} \right] \left[ g_L W_{\bar{\mu}}^I B^{\bar{\mu}\bar{\nu}} (H^\dagger t^I \partial_{\bar{\nu}} H) + g_L W_{\bar{\mu}}^I B^{\bar{\mu}\bar{\nu}} (\partial_{\bar{\nu}} H^\dagger t^I H) \right], \tag{2.23}
\end{aligned}$$

$$\begin{aligned}
\Delta S_{\mathcal{O}_{uW}} = & \frac{1}{72} g_L g_Y^2 C_{uW}^{sr} B_{\bar{\mu}}^2 (\bar{q}_s \tilde{H} u_r) + \frac{1}{72} g_L g_Y^2 \bar{C}_{uW}^{rs} B_{\bar{\mu}}^2 (\bar{u}_s \tilde{H}^\dagger q_r) + \frac{i}{12} g_L g_Y C_{uW}^{sr} B_{\bar{\mu}} (\bar{q}_s \tilde{H} \partial^{\bar{\mu}} u_r) \\
& - \frac{i}{12} g_L g_Y \bar{C}_{uW}^{rs} B_{\bar{\mu}} (\partial^{\bar{\mu}} \bar{u}_s \tilde{H}^\dagger q_r) + \frac{1}{6} g_L g_Y C_{uW}^{sr} B_{\bar{\mu}} (\bar{q}_s \partial^{\bar{\nu}} \tilde{H} \sigma^{\bar{\mu}\bar{\nu}} u_r) \\
& + \frac{i}{6} g_L^2 C_{uW}^{sr} \varepsilon^{jk} t_j^{Ii} H_i^\dagger W_{\bar{\mu}}^I (\bar{q}_{ks} \partial^{\bar{\mu}} u_r) + \frac{1}{6} g_L g_Y \bar{C}_{uW}^{rs} B_{\bar{\mu}} (\bar{u}_s \sigma^{\bar{\mu}\bar{\nu}} \partial^{\bar{\nu}} \tilde{H} q_r) \\
& - \frac{i}{6} g_L^2 \bar{C}_{uW}^{rs} \varepsilon_{ij} t_k^{Ii} H^k W_{\bar{\mu}}^I (\partial^{\bar{\mu}} \bar{u}_s q_r^j) + \frac{1}{4} g_L^3 C_{uW}^{sr} W_{\bar{\mu}}^{I2} (\bar{q}_s \tilde{H} u_r) - \frac{i}{4} g_L g_Y C_{uW}^{sr} B_{\bar{\mu}} (\bar{q}_s \partial^{\bar{\mu}} \tilde{H} u_r) \\
& + \frac{1}{4} g_L^2 \left[ \bar{y}_u^{rt} C_{uW}^{st} + y_u^{st} \bar{C}_{uW}^{rt} \right] (H^\dagger H) (\bar{q}_s t^I \bar{W}^I q_r) \\
& + \frac{1}{4} g_L \left[ y_u^{st} \bar{C}_{uW}^{rt} - \bar{y}_u^{rt} C_{uW}^{st} \right] \left[ g_L t_j^{Ii} H_i^\dagger (\bar{q}_s H \bar{W}^I q_r^j) - g_L t_k^{Ij} H^k (\bar{q}_{js} \bar{W}^I H^\dagger q_r) \right] \\
& + \frac{1}{4} g_L^3 \bar{C}_{uW}^{rs} W_{\bar{\mu}}^{I2} (\bar{u}_s \tilde{H}^\dagger q_r) + \frac{i}{4} g_L g_Y \bar{C}_{uW}^{rs} B_{\bar{\mu}} (\bar{u}_s \tilde{H}^\dagger \partial^{\bar{\mu}} q_r) + \frac{i}{4} g_L g_Y \bar{C}_{uW}^{rs} B_{\bar{\mu}} (\bar{u}_s \partial^{\bar{\mu}} \tilde{H} q_r) \\
& - \frac{i}{4} g_L g_Y C_{uW}^{sr} B_{\bar{\mu}} (\partial^{\bar{\mu}} \bar{q}_s \tilde{H} u_r) + \frac{i}{3} g_L^3 C_{uW}^{sr} t_l^{Ik} t_j^{Jl} \tilde{H}_j W_{\bar{\mu}}^I W_{\bar{\nu}}^J (\bar{q}_{ks} \sigma^{\bar{\mu}\bar{\nu}} u_r) \\
& - \frac{i}{3} g_L^3 \bar{C}_{uW}^{rs} t_l^{Ik} t_k^{Jl} \tilde{H}^{\dagger i} W_{\bar{\mu}}^I W_{\bar{\nu}}^J (\bar{u}_s \sigma^{\bar{\mu}\bar{\nu}} q_r^l) \\
& + \frac{i}{2} \left[ \bar{y}_u^{rs} C_{uW}^{rs} + y_u^{rs} \bar{C}_{uW}^{rs} \right] \left[ 2g_L W_{\bar{\mu}}^I \widetilde{W}^{\bar{\mu}\bar{\sigma}I} (H^\dagger \partial_{\bar{\sigma}} H) - 2g_L W_{\bar{\mu}}^I \widetilde{W}^{\bar{\mu}\bar{\sigma}I} (\partial_{\bar{\sigma}} H^\dagger H) \right] \\
& + \frac{i}{2} \left[ \bar{y}_u^{rs} C_{uW}^{rs} - y_u^{rs} \bar{C}_{uW}^{rs} \right] \left[ 2g_L W_{\bar{\mu}}^I \widetilde{W}^{\bar{\mu}\bar{\sigma}I} (H^\dagger \partial_{\bar{\sigma}} H) + 2g_L W_{\bar{\mu}}^I \widetilde{W}^{\bar{\mu}\bar{\sigma}I} (\partial_{\bar{\sigma}} H^\dagger H) \right] \\
& + \frac{i}{2} g_L g_s C_{uW}^{sr} T_b^{Aa} G_{\bar{\mu}}^A (\bar{q}_{as} \tilde{H} \partial^{\bar{\mu}} u_r^b) + \frac{i}{2} g_L g_s g_Y C_{uW}^{sr} T_b^{Aa} B_{\bar{\mu}} G_{\bar{\nu}}^A (\bar{q}_{as} \tilde{H} \sigma^{\bar{\mu}\bar{\nu}} u_r^b) \\
& + \frac{i}{2} g_L^2 \bar{C}_{uW}^{rs} \varepsilon_{ij} t_k^{Ii} H^k W_{\bar{\mu}}^I (\bar{u}_s \partial^{\bar{\mu}} q_r^j) - \frac{i}{2} g_L g_s g_Y \bar{C}_{uW}^{rs} T_b^{Aa} B_{\bar{\mu}} G_{\bar{\nu}}^A (\bar{u}_{as} \sigma^{\bar{\mu}\bar{\nu}} \tilde{H}^\dagger q_r^b) \\
& - \frac{i}{2} g_L^2 C_{uW}^{sr} \varepsilon^{jk} t_j^{Ii} H_i^\dagger W_{\bar{\mu}}^I (\partial^{\bar{\mu}} \bar{q}_{ks} u_r) - \frac{i}{2} g_L g_s \bar{C}_{uW}^{rs} T_b^{Aa} G_{\bar{\mu}}^A (\partial^{\bar{\mu}} \bar{u}_{as} \tilde{H}^\dagger q_r^b) \\
& + \frac{i}{2} g_L^2 C_{uW}^{sr} \varepsilon^{ij} t_i^{Ik} W_{\bar{\mu}}^I (\bar{q}_{js} u_r) \partial^{\bar{\mu}} H_k^\dagger - \frac{i}{2} g_L^2 \bar{C}_{uW}^{rs} \varepsilon_{ij} t_k^{Ii} W_{\bar{\mu}}^I (\bar{u}_s q_r^j) \partial^{\bar{\mu}} H^k \\
& + \frac{2}{3} g_L g_s g_Y C_{uW}^{sr} T_b^{Aa} B_{\bar{\mu}} G_{\bar{\mu}}^A (\bar{q}_{as} \tilde{H} u_r^b) + \frac{2}{3} g_L g_s g_Y \bar{C}_{uW}^{rs} T_b^{Aa} B_{\bar{\mu}} G_{\bar{\mu}}^A (\bar{u}_{as} \tilde{H}^\dagger q_r^b) \\
& + \frac{3}{4} g_L^2 \left[ \bar{y}_u^{rt} C_{uW}^{st} + y_u^{st} \bar{C}_{uW}^{rt} \right] (H^\dagger t^I H) (\bar{q}_s \bar{W}^I q_r) + g_L^2 \left[ -\bar{y}_u^{rs} C_{uW}^{rs} - y_u^{rs} \bar{C}_{uW}^{rs} \right] \varepsilon^{IJK} W_{\bar{\mu}}^K W_{\bar{\nu}}^J W^{\bar{\mu}\bar{\nu}I} (H^\dagger H) \\
& - i g_L^2 \left[ \bar{y}_u^{rs} C_{uW}^{rs} - y_u^{rs} \bar{C}_{uW}^{rs} \right] \varepsilon^{IJK} W_{\bar{\mu}}^K W_{\bar{\nu}}^J \widetilde{W}^{\bar{\mu}\bar{\nu}I} (H^\dagger H) \\
& + \left[ \bar{y}_u^{rs} C_{uW}^{rs} + y_u^{rs} \bar{C}_{uW}^{rs} \right] \left[ g_L W_{\bar{\mu}}^I W^{\bar{\mu}\bar{\nu}I} (H^\dagger \partial_{\bar{\nu}} H) + g_L W_{\bar{\mu}}^I W^{\bar{\mu}\bar{\nu}I} (\partial_{\bar{\nu}} H^\dagger H) \right]
\end{aligned}$$

$$\begin{aligned}
& + \left[ \bar{y}_u^{rs} \bar{C}_{uW}^{rs} - \bar{y}_u^{rs} C_{uW}^{rs} \right] \left[ 2g_L \varepsilon^{IJK} W_{\bar{\mu}}^J \widetilde{W}^{\bar{\mu}\bar{\sigma}I} (H^\dagger t^K \partial_{\bar{\sigma}} H) - 2g_L \varepsilon^{IJK} W_{\bar{\mu}}^J \widetilde{W}^{\bar{\mu}\bar{\sigma}I} (\partial_{\bar{\sigma}} H^\dagger t^K H) \right] \\
& + \left[ -\bar{y}_u^{rs} C_{uW}^{rs} - y_u^{rs} \bar{C}_{uW}^{rs} \right] \left[ 2g_L \varepsilon^{IJK} W_{\bar{\mu}}^J \widetilde{W}^{\bar{\mu}\bar{\sigma}I} (H^\dagger t^K \partial_{\bar{\sigma}} H) + 2g_L \varepsilon^{IJK} W_{\bar{\mu}}^J \widetilde{W}^{\bar{\mu}\bar{\sigma}I} (\partial_{\bar{\sigma}} H^\dagger t^K H) \right] \\
& + ig_L \left[ \bar{y}_u^{ts} C_{uW}^{tr} - y_u^{tr} \bar{C}_{uW}^{ts} \right] W_{\bar{\mu}}^I W^{\bar{\mu}\bar{\nu}I} (\bar{u}_s \gamma^{\bar{\nu}} u_r) + g_L \left[ \bar{y}_u^{ts} C_{uW}^{tr} + y_u^{tr} \bar{C}_{uW}^{ts} \right] W_{\bar{\mu}}^I \widetilde{W}^{\bar{\mu}\bar{\sigma}I} (\bar{u}_s \gamma^{\bar{\sigma}} u_r) \\
& + ig_L^2 \bar{C}_{uW}^{rs} \varepsilon_{ij} t_k^{Ii} T_b^{Aa} H^k G_{\bar{\mu}}^A W_{\bar{\nu}}^I (\bar{u}_{as} \sigma^{\bar{\mu}\bar{\nu}} q_r^{bj}) + g_L \left[ \bar{y}_u^{rs} C_{uW}^{rs} - y_u^{rs} \bar{C}_{uW}^{rs} \right] W_{\bar{\mu}}^I W^{\bar{\mu}\bar{\nu}I} (H^\dagger \overset{\leftrightarrow}{\partial}_{\bar{\nu}} H) \\
& - \frac{5i}{3} \left[ \bar{y}_u^{rs} C_{uW}^{rs} + y_u^{rs} \bar{C}_{uW}^{rs} \right] \left[ 2g_Y B_{\bar{\mu}} \widetilde{W}^{\bar{\mu}\bar{\sigma}I} (H^\dagger t^I \partial_{\bar{\sigma}} H) - 2g_Y B_{\bar{\mu}} \widetilde{W}^{\bar{\mu}\bar{\sigma}I} (\partial_{\bar{\sigma}} H^\dagger t^I H) \right] \\
& - \frac{5i}{3} \left[ \bar{y}_u^{rs} C_{uW}^{rs} - y_u^{rs} \bar{C}_{uW}^{rs} \right] \left[ 2g_Y B_{\bar{\mu}} \widetilde{W}^{\bar{\mu}\bar{\sigma}I} (H^\dagger t^I \partial_{\bar{\sigma}} H) + 2g_Y B_{\bar{\mu}} \widetilde{W}^{\bar{\mu}\bar{\sigma}I} (\partial_{\bar{\sigma}} H^\dagger t^I H) \right] \\
& + 2ig_L g_Y \left[ \bar{y}_u^{rs} C_{uW}^{rs} - y_u^{rs} \bar{C}_{uW}^{rs} \right] B_{\bar{\mu}} W_{\bar{\nu}}^I W^{\bar{\mu}\bar{\nu}I} (H^\dagger H) + 2g_L g_Y \left[ -\bar{y}_u^{rs} C_{uW}^{rs} - y_u^{rs} \bar{C}_{uW}^{rs} \right] B_{\bar{\mu}} W_{\bar{\nu}}^I \widetilde{W}^{\bar{\mu}\bar{\nu}I} (H^\dagger H) \\
& + 2i \left[ \bar{y}_u^{rs} C_{uW}^{rs} - y_u^{rs} \bar{C}_{uW}^{rs} \right] \left[ g_L \varepsilon^{IJK} W_{\bar{\mu}}^J W^{\bar{\mu}\bar{\nu}I} (H^\dagger t^K \partial_{\bar{\nu}} H) + g_L \varepsilon^{IJK} W_{\bar{\mu}}^J W^{\bar{\mu}\bar{\nu}I} (\partial_{\bar{\nu}} H^\dagger t^K H) \right] \\
& + 2g_s \left[ -\bar{y}_u^{rt} C_{uW}^{st} - y_u^{st} \bar{C}_{uW}^{rt} \right] G_{\bar{\mu}}^A \widetilde{W}^{\bar{\mu}\bar{\sigma}I} (\bar{q}_s t^I T^A \gamma^{\bar{\sigma}} q_r) + \frac{7}{2} g_L g_s^2 C_{uW}^{sr} T_b^{Aa} T_a^{Bc} G_{\bar{\mu}}^A G_{\bar{\mu}}^B (\bar{q}_{cs} \tilde{H} u_r^b) \\
& - \frac{1}{12} g_L g_Y \left[ \bar{y}_u^{rt} C_{uW}^{st} + y_u^{st} \bar{C}_{uW}^{rt} \right] (H^\dagger H) (\bar{q}_s \tilde{B} q_r) - \frac{1}{12} g_L g_Y \left[ \bar{y}_u^{rt} C_{uW}^{st} + y_u^{st} \bar{C}_{uW}^{rt} \right] (\bar{q}_s H \tilde{B} H^\dagger q_r) \\
& - \frac{1}{3} g_L^2 C_{uW}^{sr} \varepsilon^{ij} t_l^{Ii} W_{\bar{\mu}}^I (\bar{q}_{js} \sigma^{\bar{\mu}\bar{\nu}} u_r) \partial^{\bar{\nu}} H_k^\dagger - \frac{1}{3} g_L^2 \bar{C}_{uW}^{rs} \varepsilon_{ij} t_k^{Ii} W_{\bar{\mu}}^I (\bar{u}_s \sigma^{\bar{\mu}\bar{\nu}} q_r^j) \partial^{\bar{\nu}} H^k \\
& - \frac{7}{18} g_L^2 g_Y C_{uW}^{sr} t_j^{Ik} \tilde{H}_j B_{\bar{\mu}} W_{\bar{\mu}}^I (\bar{q}_{ks} u_r) - \frac{7}{18} g_L^2 g_Y \bar{C}_{uW}^{rs} t_k^{Ii} \tilde{H}^{\dagger i} B_{\bar{\mu}} W_{\bar{\mu}}^I (\bar{u}_s q_r^k) \\
& - \frac{1}{2} g_L g_s \left[ \bar{y}_u^{rt} C_{uW}^{st} + y_u^{st} \bar{C}_{uW}^{rt} \right] (H^\dagger H) (\bar{q}_s T^A \tilde{G}^A q_r) - \frac{1}{2} g_L g_s \left[ \bar{y}_u^{rt} C_{uW}^{st} + y_u^{st} \bar{C}_{uW}^{rt} \right] (\bar{q}_s T^A H \tilde{G}^A H^\dagger q_r) \\
& - \frac{1}{2} g_L^3 C_{uW}^{sr} \varepsilon^{jk} t_l^{Ii} t_j^{Jl} H_i^\dagger W_{\bar{\mu}}^I W_{\bar{\mu}}^J (\bar{q}_{ks} u_r) - \frac{1}{2} g_L^3 \bar{C}_{uW}^{rs} \varepsilon_{ij} t_l^{Ii} t_k^{Jl} H^l W_{\bar{\mu}}^I W_{\bar{\mu}}^J (\bar{u}_s q_r^j) \\
& - g_L g_s C_{uW}^{sr} T_b^{Aa} G_{\bar{\mu}}^A (\bar{q}_{as} \partial^{\bar{\nu}} \tilde{H} \sigma^{\bar{\mu}\bar{\nu}} u_r^b) - ig_L^2 g_s C_{uW}^{sr} \varepsilon^{jk} t_j^{Ii} T_b^{Aa} H_i^\dagger G_{\bar{\mu}}^A W_{\bar{\nu}}^I (\bar{q}_{aks} \sigma^{\bar{\mu}\bar{\nu}} u_r^b) \\
& - g_L g_s \bar{C}_{uW}^{rs} T_b^{Aa} G_{\bar{\mu}}^A (\bar{u}_{as} \sigma^{\bar{\mu}\bar{\nu}} \partial^{\bar{\nu}} \tilde{H} q_r^b) - \frac{4i}{3} g_Y \left[ \bar{y}_u^{rt} C_{uW}^{st} - y_u^{st} \bar{C}_{uW}^{rt} \right] B_{\bar{\mu}} W^{\bar{\mu}\bar{\nu}I} (\bar{q}_s t^I \gamma^{\bar{\nu}} q_r) \\
& - \frac{4}{3} g_Y \left[ \bar{y}_u^{rt} C_{uW}^{st} + y_u^{st} \bar{C}_{uW}^{rt} \right] B_{\bar{\mu}} \widetilde{W}^{\bar{\mu}\bar{\sigma}I} (\bar{q}_s t^I \gamma^{\bar{\sigma}} q_r) - \frac{4}{3} g_L^2 g_s C_{uW}^{sr} t_j^{Ik} T_b^{Aa} \tilde{H}_j G_{\bar{\mu}}^A W_{\bar{\mu}}^I (\bar{q}_{aks} u_r^b) \\
& - \frac{4}{3} g_L^2 g_s \bar{C}_{uW}^{rs} t_k^{Ii} T_b^{Aa} \tilde{H}^{\dagger i} G_{\bar{\mu}}^A W_{\bar{\mu}}^I (\bar{u}_{as} q_r^{bk}) - \frac{3i}{2} g_L g_s C_{uW}^{sr} T_b^{Aa} G_{\bar{\mu}}^A (\bar{q}_{as} \partial^{\bar{\mu}} \tilde{H} u_r^b) \\
& + \frac{3i}{2} g_L g_s \bar{C}_{uW}^{rs} T_b^{Aa} G_{\bar{\mu}}^A (\bar{u}_{as} \tilde{H}^\dagger \partial^{\bar{\mu}} q_r^b) + \frac{3i}{2} g_L g_s \bar{C}_{uW}^{rs} T_b^{Aa} G_{\bar{\mu}}^A (\bar{u}_{as} \partial^{\bar{\mu}} \tilde{H} q_r^b) \\
& - \frac{3i}{2} g_L g_s C_{uW}^{sr} T_b^{Aa} G_{\bar{\mu}}^A (\partial^{\bar{\mu}} \bar{q}_{as} \tilde{H} u_r^b) - 2ig_s \left[ \bar{y}_u^{rt} C_{uW}^{st} - y_u^{st} \bar{C}_{uW}^{rt} \right] G_{\bar{\mu}}^A W^{\bar{\mu}\bar{\nu}I} (\bar{q}_s t^I T^A \gamma^{\bar{\nu}} q_r) \\
& + 2ig_L \left[ \bar{y}_u^{rs} C_{uW}^{rs} + y_u^{rs} \bar{C}_{uW}^{rs} \right] \varepsilon^{IJK} W_{\bar{\mu}}^J W^{\bar{\mu}\bar{\nu}I} (H^\dagger t^K \overset{\leftrightarrow}{\partial}_{\bar{\nu}} H) + \frac{7}{2} g_L g_s^2 \bar{C}_{uW}^{rs} T_b^{Aa} T_c^{Bb} G_{\bar{\mu}}^A G_{\bar{\mu}}^B (\bar{u}_{as} \tilde{H}^\dagger q_r^c) \\
& - \frac{10}{3} \left[ \bar{y}_u^{rs} C_{uW}^{rs} + y_u^{rs} \bar{C}_{uW}^{rs} \right] \left[ g_Y B_{\bar{\mu}} W^{\bar{\mu}\bar{\nu}I} (H^\dagger t^I \partial_{\bar{\nu}} H) + g_Y B_{\bar{\mu}} W^{\bar{\mu}\bar{\nu}I} (\partial_{\bar{\nu}} H^\dagger t^I H) \right] \\
& - \frac{10}{3} g_Y \left[ \bar{y}_u^{rs} C_{uW}^{rs} - y_u^{rs} \bar{C}_{uW}^{rs} \right] B_{\bar{\mu}} W^{\bar{\mu}\bar{\nu}I} (H^\dagger t^I \overset{\leftrightarrow}{\partial}_{\bar{\nu}} H) \\
& + 4ig_L^2 \left[ \bar{y}_u^{rs} C_{uW}^{rs} - y_u^{rs} \bar{C}_{uW}^{rs} \right] W_{\bar{\mu}}^I W_{\bar{\nu}}^J W^{\bar{\mu}\bar{\nu}J} (H^\dagger t^I H) - 4g_L^2 \left[ \bar{y}_u^{rs} C_{uW}^{rs} + y_u^{rs} \bar{C}_{uW}^{rs} \right] W_{\bar{\mu}}^I W_{\bar{\nu}}^J \widetilde{W}^{\bar{\mu}\bar{\nu}J} (H^\dagger t^I H)
\end{aligned}$$

$$\begin{aligned}
& -4g_L g_Y \left[ \bar{y}_u^{rs} \mathcal{C}_{uW}^{rs} + y_u^{rs} \bar{\mathcal{C}}_{uW}^{rs} \right] \varepsilon^{IJK} B_{\bar{\mu}} W_{\bar{\nu}}^J W^{\bar{\mu}\bar{\nu}I} (H^\dagger t^K H) \\
& -4ig_L g_Y \left[ \bar{y}_u^{rs} \mathcal{C}_{uW}^{rs} - y_u^{rs} \bar{\mathcal{C}}_{uW}^{rs} \right] \varepsilon^{IJK} B_{\bar{\mu}} W_{\bar{\nu}}^J \widetilde{W}^{\bar{\mu}\bar{\nu}I} (H^\dagger t^K H),
\end{aligned} \tag{2.24}$$

$$\begin{aligned}
\Delta S_{\mathcal{O}_{uG}} = & -\frac{i}{9} g_s^2 g_Y \mathcal{C}_{uG}^{sr} T_b^{Aa} B_{\bar{\mu}} G_{\bar{\nu}}^A (\bar{q}_{as} \tilde{H} \sigma^{\bar{\mu}\bar{\nu}} u_r^b) + \frac{i}{9} g_s^2 g_Y \bar{\mathcal{C}}_{uG}^{rs} T_b^{Aa} B_{\bar{\mu}} G_{\bar{\nu}}^A (\bar{u}_{as} \sigma^{\bar{\mu}\bar{\nu}} \tilde{H}^\dagger q_r^b) \\
& + \frac{1}{6} g_s^2 \left[ \bar{y}_u^{rs} \mathcal{C}_{uG}^{rs} + y_u^{rs} \bar{\mathcal{C}}_{uG}^{rs} \right] f^{ABC} G_{\bar{\mu}}^B G_{\bar{\nu}}^C G^{\bar{\mu}\bar{\nu}A} (H^\dagger H) \\
& + \frac{i}{6} g_s^2 \left[ \bar{y}_u^{rs} \mathcal{C}_{uG}^{rs} - y_u^{rs} \bar{\mathcal{C}}_{uG}^{rs} \right] f^{ABC} G_{\bar{\mu}}^B G_{\bar{\nu}}^C \tilde{G}^{\bar{\mu}\bar{\nu}A} (H^\dagger H) + \frac{1}{6} g_s^2 \left[ \bar{y}_u^{rt} \mathcal{C}_{uG}^{st} + y_u^{st} \bar{\mathcal{C}}_{uG}^{rt} \right] (H^\dagger H) (\bar{q}_s T^A \overleftrightarrow{G}^A q_r) \\
& + \frac{1}{6} g_s^2 \left[ \bar{y}_u^{ts} \mathcal{C}_{uG}^{tr} + y_u^{tr} \bar{\mathcal{C}}_{uG}^{ts} \right] (H^\dagger H) (\bar{u}_s T^A \overleftrightarrow{G}^A u_r) + \frac{2}{9} g_s g_Y \left[ \bar{y}_u^{rt} \mathcal{C}_{uG}^{st} + y_u^{st} \bar{\mathcal{C}}_{uG}^{rt} \right] (\bar{q}_s H \overleftrightarrow{B} H^\dagger q_r) \\
& + \frac{2i}{9} g_L g_s^2 \mathcal{C}_{uG}^{sr} \varepsilon^{ijk} t_j^{Ii} t_k^{Ii} T_b^{Aa} H_i^\dagger G_{\bar{\mu}}^A W_{\bar{\nu}}^I (\bar{q}_{aks} \sigma^{\bar{\mu}\bar{\nu}} u_r^b) - \frac{2i}{9} g_s^2 \bar{\mathcal{C}}_{uG}^{rs} T_b^{Aa} G_{\bar{\mu}}^A (\bar{u}_{as} \tilde{H}^\dagger \partial^{\bar{\mu}} q_r^b) \\
& - \frac{2i}{9} g_L g_s^2 \bar{\mathcal{C}}_{uG}^{rs} \varepsilon_{ij} \bar{\varepsilon}_{ij} t_k^{Ii} T_b^{Aa} H^k G_{\bar{\mu}}^A W_{\bar{\nu}}^I (\bar{u}_{as} \sigma^{\bar{\mu}\bar{\nu}} q_r^{bj}) + \frac{2}{9} g_s^2 \bar{\mathcal{C}}_{uG}^{rs} T_b^{Aa} G_{\bar{\mu}}^A (\bar{u}_{as} \sigma^{\bar{\mu}\bar{\nu}} \partial^{\bar{\nu}} \tilde{H} q_r^b) \\
& + \frac{2i}{9} g_s^2 \mathcal{C}_{uG}^{sr} T_b^{Aa} G_{\bar{\mu}}^A (\partial^{\bar{\mu}} \bar{q}_{as} \tilde{H} u_r^b) + \frac{2i}{9} g_s^2 \bar{\mathcal{C}}_{uG}^{rs} T_b^{Aa} G_{\bar{\mu}}^A (\partial^{\bar{\mu}} \bar{u}_{as} \tilde{H}^\dagger q_r^b) \\
& + \frac{1}{4} \left[ y_u^{st} \bar{\mathcal{C}}_{uG}^{rt} - \bar{y}_u^{rt} \mathcal{C}_{uG}^{st} \right] \left[ 2g_s T_b^{Aa} T_c^{Bb} G_{\bar{\mu}}^B \tilde{G}^{\bar{\mu}\bar{\sigma}A} (\bar{q}_{as} \gamma^{\bar{\sigma}} q_r^c) - 2g_s T_b^{Aa} T_a^{Bc} G_{\bar{\mu}}^B \tilde{G}^{\bar{\mu}\bar{\sigma}A} (\bar{q}_{cs} \gamma^{\bar{\sigma}} q_r^b) \right] \\
& + \frac{1}{4} \left[ -\bar{y}_u^{rt} \mathcal{C}_{uG}^{st} - y_u^{st} \bar{\mathcal{C}}_{uG}^{rt} \right] \left[ 2g_s T_b^{Aa} T_c^{Bb} G_{\bar{\mu}}^B \tilde{G}^{\bar{\mu}\bar{\sigma}A} (\bar{q}_{as} \gamma^{\bar{\sigma}} q_r^c) + 2g_s T_b^{Aa} T_a^{Bc} G_{\bar{\mu}}^B \tilde{G}^{\bar{\mu}\bar{\sigma}A} (\bar{q}_{cs} \gamma^{\bar{\sigma}} q_r^b) \right] \\
& - \frac{1}{6} g_s^2 \left[ \bar{y}_u^{rt} \mathcal{C}_{uG}^{st} + y_u^{st} \bar{\mathcal{C}}_{uG}^{rt} \right] (\bar{q}_s T^A H \overleftrightarrow{G}^A H^\dagger q_r) - \frac{2i}{9} g_s^2 \mathcal{C}_{uG}^{sr} T_b^{Aa} G_{\bar{\mu}}^A (\bar{q}_{as} \tilde{H} \partial^{\bar{\mu}} u_r^b) \\
& + \frac{2}{9} g_s^2 \mathcal{C}_{uG}^{sr} T_b^{Aa} G_{\bar{\mu}}^A (\bar{q}_{as} \partial^{\bar{\nu}} \tilde{H} \sigma^{\bar{\mu}\bar{\nu}} u_r^b) \\
& + \frac{i}{3} \left[ \bar{y}_u^{rs} \mathcal{C}_{uG}^{rs} + y_u^{rs} \bar{\mathcal{C}}_{uG}^{rs} \right] \left[ 2g_s G_{\bar{\mu}}^A \tilde{G}^{\bar{\mu}\bar{\sigma}A} (H^\dagger \partial_{\bar{\sigma}} H) - 2g_s G_{\bar{\mu}}^A \tilde{G}^{\bar{\mu}\bar{\sigma}A} (\partial_{\bar{\sigma}} H^\dagger H) \right] \\
& + \frac{i}{3} \left[ \bar{y}_u^{rs} \mathcal{C}_{uG}^{rs} - y_u^{rs} \bar{\mathcal{C}}_{uG}^{rs} \right] \left[ 2g_s G_{\bar{\mu}}^A \tilde{G}^{\bar{\mu}\bar{\sigma}A} (H^\dagger \partial_{\bar{\sigma}} H) + 2g_s G_{\bar{\mu}}^A \tilde{G}^{\bar{\mu}\bar{\sigma}A} (\partial_{\bar{\sigma}} H^\dagger H) \right] \\
& + \frac{i}{3} g_Y \left[ \bar{y}_u^{ts} \mathcal{C}_{uG}^{tr} - y_u^{tr} \bar{\mathcal{C}}_{uG}^{ts} \right] B_{\bar{\mu}} G^{\bar{\mu}\bar{\nu}A} (\bar{u}_s T^A \gamma^{\bar{\nu}} u_r) \\
& + \frac{1}{3} g_Y \left[ \bar{y}_u^{ts} \mathcal{C}_{uG}^{tr} + y_u^{tr} \bar{\mathcal{C}}_{uG}^{ts} \right] B_{\bar{\mu}} \tilde{G}^{\bar{\mu}\bar{\sigma}A} (\bar{u}_s T^A \gamma^{\bar{\sigma}} u_r) + \frac{4i}{9} g_L g_s \bar{\mathcal{C}}_{uG}^{rs} \varepsilon_{ij} t_k^{Ii} H^k W_{\bar{\mu}}^I (\partial^{\bar{\mu}} \bar{u}_s q_r^j) \\
& + \frac{i}{2} g_s g_Y \left[ \bar{y}_u^{rs} \mathcal{C}_{uG}^{rs} - y_u^{rs} \bar{\mathcal{C}}_{uG}^{rs} \right] B_{\bar{\mu}} G_{\bar{\nu}}^A G^{\bar{\mu}\bar{\nu}A} (H^\dagger H) + \frac{1}{2} g_s g_Y \left[ -\bar{y}_u^{rs} \mathcal{C}_{uG}^{rs} - y_u^{rs} \bar{\mathcal{C}}_{uG}^{rs} \right] B_{\bar{\mu}} G_{\bar{\nu}}^A \tilde{G}^{\bar{\mu}\bar{\nu}A} (H^\dagger H) \\
& + \frac{1}{2} g_s^3 \mathcal{C}_{uG}^{sr} G_{\bar{\mu}}^{A2} (\bar{q}_s \tilde{H} u_r) \\
& - \frac{i}{2} \left[ \bar{y}_u^{rt} \mathcal{C}_{uG}^{st} + y_u^{st} \bar{\mathcal{C}}_{uG}^{rt} \right] \left[ g_s T_b^{Aa} T_c^{Bb} G_{\bar{\mu}}^B G^{\bar{\mu}\bar{\nu}A} (\bar{q}_{as} \gamma^{\bar{\nu}} q_r^c) - g_s T_b^{Aa} T_a^{Bc} G_{\bar{\mu}}^B G^{\bar{\mu}\bar{\nu}A} (\bar{q}_{cs} \gamma^{\bar{\nu}} q_r^b) \right] \\
& - \frac{i}{2} \left[ \bar{y}_u^{rt} \mathcal{C}_{uG}^{st} - y_u^{st} \bar{\mathcal{C}}_{uG}^{rt} \right] \left[ g_s T_b^{Aa} T_c^{Bb} G_{\bar{\mu}}^B G^{\bar{\mu}\bar{\nu}A} (\bar{q}_{as} \gamma^{\bar{\nu}} q_r^c) + g_s T_b^{Aa} T_a^{Bc} G_{\bar{\mu}}^B G^{\bar{\mu}\bar{\nu}A} (\bar{q}_{cs} \gamma^{\bar{\nu}} q_r^b) \right] \\
& + \frac{1}{2} g_s^3 \bar{\mathcal{C}}_{uG}^{rs} G_{\bar{\mu}}^{A2} (\bar{u}_s \tilde{H}^\dagger q_r) \\
& + \frac{1}{2} \left[ y_u^{tr} \bar{\mathcal{C}}_{uG}^{ts} - \bar{y}_u^{ts} \mathcal{C}_{uG}^{tr} \right] \left[ 2g_s T_b^{Aa} T_c^{Bb} G_{\bar{\mu}}^B \tilde{G}^{\bar{\mu}\bar{\sigma}A} (\bar{u}_{as} \gamma^{\bar{\sigma}} u_r^c) - 2g_s T_b^{Aa} T_a^{Bc} G_{\bar{\mu}}^B \tilde{G}^{\bar{\mu}\bar{\sigma}A} (\bar{u}_{cs} \gamma^{\bar{\sigma}} u_r^b) \right]
\end{aligned}$$

$$\begin{aligned}
& + \frac{1}{2} \left[ \bar{y}_u^{ts} C_{uG}^{tr} + y_u^{tr} \bar{C}_{uG}^{ts} \right] \left[ 2g_s T_b^{Aa} T_c^{Bb} G_{\bar{\mu}}^B \tilde{G}^{\bar{\mu}\bar{\sigma}A} (\bar{u}_{as} \gamma^{\bar{\sigma}} u_r^c) + 2g_s T_b^{Aa} T_a^{Bc} G_{\bar{\mu}}^B \tilde{G}^{\bar{\mu}\bar{\sigma}A} (\bar{u}_{cs} \gamma^{\bar{\sigma}} u_r^b) \right] \\
& + \frac{14i}{27} g_s g_Y \bar{C}_{uG}^{rs} B_{\bar{\mu}} (\bar{u}_s \tilde{H}^\dagger \partial^{\bar{\mu}} q_r) - \frac{14i}{27} g_s g_Y C_{uG}^{sr} B_{\bar{\mu}} (\partial^{\bar{\mu}} \bar{q}_s \tilde{H} u_r) \\
& + \frac{2}{3} \left[ \bar{y}_u^{rs} C_{uG}^{rs} + y_u^{rs} \bar{C}_{uG}^{rs} \right] \left[ g_s G_{\bar{\mu}}^A G^{\bar{\mu}\bar{\nu}A} (H^\dagger \partial_{\bar{\nu}} H) + g_s G_{\bar{\mu}}^A G^{\bar{\mu}\bar{\nu}A} (\partial_{\bar{\nu}} H^\dagger H) \right] + \frac{2}{3} g_L^2 g_s C_{uG}^{sr} W_{\bar{\mu}}^{I2} (\bar{q}_s \tilde{H} u_r) \\
& + \frac{2i}{3} g_s g_Y C_{uG}^{sr} B_{\bar{\mu}} (\bar{q}_s \partial^{\bar{\mu}} \tilde{H} u_r) + \frac{2}{3} g_L g_s \left[ \bar{y}_u^{rt} C_{uG}^{st} + y_u^{st} \bar{C}_{uG}^{rt} \right] (H^\dagger t^I H) (\bar{q}_s \bar{W}^I q_r) \\
& + \frac{2}{3} g_s \left[ \bar{y}_u^{rt} C_{uG}^{st} - y_u^{st} \bar{C}_{uG}^{rt} \right] \left[ g_L t_j^{Ii} H_i^\dagger (\bar{q}_s H \bar{W}^I q_r^j) - g_L t_k^{Ij} H^k (\bar{q}_j s \bar{W}^I H^\dagger q_r) \right] \\
& + \frac{2}{3} g_L^2 g_s \bar{C}_{uG}^{rs} W_{\bar{\mu}}^{I2} (\bar{u}_s \tilde{H}^\dagger q_r) - \frac{4}{27} g_L g_s g_Y C_{uG}^{sr} t_j^{Ik} \tilde{H}_j B_{\bar{\mu}} W_{\bar{\mu}}^I (\bar{q}_{ks} u_r) \\
& - \frac{2}{9} g_s g_Y \left[ \bar{y}_u^{rt} C_{uG}^{st} + y_u^{st} \bar{C}_{uG}^{rt} \right] (H^\dagger H) (\bar{q}_s \bar{B} q_r) - \frac{4i}{9} g_L g_s C_{uG}^{sr} \varepsilon^{jk} t_j^{Ii} H_i^\dagger W_{\bar{\mu}}^I (\bar{q}_{ks} \partial^{\bar{\mu}} u_r) \\
& - \frac{2i}{3} g_Y \left[ \bar{y}_u^{rt} C_{uG}^{st} - y_u^{st} \bar{C}_{uG}^{rt} \right] B_{\bar{\mu}} G^{\bar{\mu}\bar{\nu}A} (\bar{q}_s T^A \gamma^{\bar{\nu}} q_r) \\
& + \frac{2}{3} g_Y \left[ -\bar{y}_u^{rt} C_{uG}^{st} - y_u^{st} \bar{C}_{uG}^{rt} \right] B_{\bar{\mu}} \tilde{G}^{\bar{\mu}\bar{\sigma}A} (\bar{q}_s T^A \gamma^{\bar{\sigma}} q_r) - \frac{2i}{3} g_s g_Y \bar{C}_{uG}^{rs} B_{\bar{\mu}} (\bar{u}_s \partial^{\bar{\mu}} \tilde{H} q_r) \\
& + \frac{2}{3} g_s \left[ \bar{y}_u^{rs} C_{uG}^{rs} - y_u^{rs} \bar{C}_{uG}^{rs} \right] G_{\bar{\mu}}^A G^{\bar{\mu}\bar{\nu}A} (H^\dagger \partial_{\bar{\nu}} H) + \frac{20}{27} g_s g_Y C_{uG}^{sr} B_{\bar{\mu}} (\bar{q}_s \partial^{\bar{\nu}} \tilde{H} \sigma^{\bar{\mu}\bar{\nu}} u_r) \\
& + \frac{20}{27} g_s g_Y \bar{C}_{uG}^{rs} B_{\bar{\mu}} (\bar{u}_s \sigma^{\bar{\mu}\bar{\nu}} \partial^{\bar{\nu}} \tilde{H} q_r) - \frac{2}{3} g_L g_s \left[ \bar{y}_u^{rt} C_{uG}^{st} + y_u^{st} \bar{C}_{uG}^{rt} \right] (H^\dagger H) (\bar{q}_s t^I \bar{W}^I q_r) \\
& - \frac{7}{9} g_s^3 C_{uG}^{sr} T_b^{Aa} T_a^{Bc} G_{\bar{\mu}}^A G_{\bar{\mu}}^B (\bar{q}_{cs} \tilde{H} u_r^b) + \frac{8i}{9} g_L^2 g_s C_{uG}^{sr} \varepsilon^{jk} t_l^{Ii} t_k^{Jl} H_i^\dagger W_{\bar{\mu}}^I W_{\bar{\nu}}^J (\bar{q}_{js} \sigma^{\bar{\mu}\bar{\nu}} u_r) \\
& - \frac{8i}{9} g_L^2 g_s \bar{C}_{uG}^{rs} \varepsilon_{ij} t_l^{Ik} t_k^{Jj} H^l W_{\bar{\mu}}^I W_{\bar{\nu}}^J (\bar{u}_s \sigma^{\bar{\mu}\bar{\nu}} q_r^i) + \frac{8}{9} g_L g_s C_{uG}^{sr} \varepsilon^{ij} t_i^{Ik} W_{\bar{\mu}}^I (\bar{q}_{js} \sigma^{\bar{\mu}\bar{\nu}} u_r) \partial^{\bar{\nu}} H_k^\dagger \\
& + \frac{8}{9} g_L g_s \bar{C}_{uG}^{rs} \varepsilon_{ij} t_k^{Ii} W_{\bar{\mu}}^I (\bar{u}_s \sigma^{\bar{\mu}\bar{\nu}} q_r^j) \partial^{\bar{\nu}} H^k + \frac{26i}{27} g_s g_Y C_{uG}^{sr} B_{\bar{\mu}} (\bar{q}_s \tilde{H} \partial^{\bar{\mu}} u_r) \\
& - i g_L g_s \left[ \bar{y}_u^{rs} C_{uG}^{rs} - y_u^{rs} \bar{C}_{uG}^{rs} \right] G_{\bar{\mu}}^A W_{\bar{\nu}}^I G^{\bar{\mu}\bar{\nu}A} (H^\dagger t^I H) + g_L g_s \left[ \bar{y}_u^{rs} C_{uG}^{rs} + y_u^{rs} \bar{C}_{uG}^{rs} \right] G_{\bar{\mu}}^A W_{\bar{\nu}}^I \tilde{G}^{\bar{\mu}\bar{\nu}A} (H^\dagger t^I H) \\
& + \frac{55}{54} g_s^2 g_Y C_{uG}^{sr} T_b^{Aa} B_{\bar{\mu}} G_{\bar{\mu}}^A (\bar{q}_{as} \tilde{H} u_r^b) + \frac{55}{54} g_s^2 g_Y \bar{C}_{uG}^{rs} T_b^{Aa} B_{\bar{\mu}} G_{\bar{\mu}}^A (\bar{u}_{as} \tilde{H}^\dagger q_r^b) \\
& - \frac{32i}{27} g_L g_s g_Y C_{uG}^{sr} \varepsilon^{jk} t_j^{Ii} H_i^\dagger B_{\bar{\mu}} W_{\bar{\nu}}^I (\bar{q}_{ks} \sigma^{\bar{\mu}\bar{\nu}} u_r) + \frac{4}{3} g_L^2 g_s C_{uG}^{sr} t_l^{Ik} t_j^{Jl} \tilde{H}_j W_{\bar{\mu}}^I W_{\bar{\mu}}^J (\bar{q}_{ks} u_r) \\
& + \frac{4}{3} g_L^2 g_s \bar{C}_{uG}^{rs} t_l^{Ik} t_k^{Jj} \tilde{H}^\dagger{}^j W_{\bar{\mu}}^I W_{\bar{\mu}}^J (\bar{u}_s q_r^l) + \frac{137}{81} g_s g_Y^2 C_{uG}^{sr} B_{\bar{\mu}}^2 (\bar{q}_s \tilde{H} u_r) \\
& - \frac{4}{27} g_L g_s g_Y \bar{C}_{uG}^{rs} t_k^{Ii} \tilde{H}^\dagger{}^i B_{\bar{\mu}} W_{\bar{\mu}}^I (\bar{u}_s q_r^k) - \frac{7}{9} g_s^3 \bar{C}_{uG}^{rs} T_b^{Aa} T_c^{Bb} G_{\bar{\mu}}^A G_{\bar{\mu}}^B (\bar{u}_{as} \tilde{H}^\dagger q_r^c) \\
& - \frac{8}{9} g_s g_Y \left[ \bar{y}_u^{ts} C_{uG}^{tr} + y_u^{tr} \bar{C}_{uG}^{ts} \right] (H^\dagger H) (\bar{u}_s \bar{B} u_r) - \frac{26i}{27} g_s g_Y \bar{C}_{uG}^{rs} B_{\bar{\mu}} (\partial^{\bar{\mu}} \bar{u}_s \tilde{H}^\dagger q_r) \\
& - i \left[ \bar{y}_u^{ts} C_{uG}^{tr} + y_u^{tr} \bar{C}_{uG}^{ts} \right] \left[ g_s T_b^{Aa} T_c^{Bb} G_{\bar{\mu}}^B G^{\bar{\mu}\bar{\nu}A} (\bar{u}_{as} \gamma^{\bar{\nu}} u_r^c) - g_s T_b^{Aa} T_a^{Bc} G_{\bar{\mu}}^B G^{\bar{\mu}\bar{\nu}A} (\bar{u}_{cs} \gamma^{\bar{\nu}} u_r^b) \right] \\
& + i \left[ \bar{y}_u^{ts} C_{uG}^{tr} - y_u^{tr} \bar{C}_{uG}^{ts} \right] \left[ g_s T_b^{Aa} T_c^{Bb} G_{\bar{\mu}}^B G^{\bar{\mu}\bar{\nu}A} (\bar{u}_{as} \gamma^{\bar{\nu}} u_r^c) + g_s T_b^{Aa} T_a^{Bc} G_{\bar{\mu}}^B G^{\bar{\mu}\bar{\nu}A} (\bar{u}_{cs} \gamma^{\bar{\nu}} u_r^b) \right] \\
& + \frac{32i}{27} g_L g_s g_Y \bar{C}_{uG}^{rs} \varepsilon_{ij} t_k^{Ii} H^k B_{\bar{\mu}} W_{\bar{\nu}}^I (\bar{u}_s \sigma^{\bar{\mu}\bar{\nu}} q_r^j) - \frac{11}{9} g_L g_s^2 C_{uG}^{sr} t_j^{Ik} T_b^{Aa} \tilde{H}_j G_{\bar{\mu}}^A W_{\bar{\mu}}^I (\bar{q}_{aks} u_r^b) \\
& - \frac{11}{9} g_L g_s^2 \bar{C}_{uG}^{rs} t_k^{Ii} T_b^{Aa} \tilde{H}^\dagger{}^i G_{\bar{\mu}}^A W_{\bar{\mu}}^I (\bar{u}_{as} q_r^{bk}) - \frac{4i}{3} g_L g_s \bar{C}_{uG}^{rs} \varepsilon_{ij} t_k^{Ii} H^k W_{\bar{\mu}}^I (\bar{u}_s \partial^{\bar{\mu}} q_r^j)
\end{aligned}$$

$$\begin{aligned}
& + \frac{4i}{3} g_L g_s C_{uG}^{sr} \varepsilon^{jk} t_j^{Ii} H_i^\dagger W_\mu^I (\partial^{\bar{\mu}} \bar{q}_{ks} u_r) - \frac{4i}{3} g_L g_s C_{uG}^{sr} \varepsilon^{ij} t_i^{Ik} W_\mu^I (\bar{q}_{js} u_r) \partial^{\bar{\mu}} H_k^\dagger \\
& + \frac{4i}{3} g_L g_s \bar{C}_{uG}^{rs} \bar{\varepsilon}_{ij} t_k^{Ii} W_\mu^I (\bar{u}_s q_r^j) \partial^{\bar{\mu}} H^k + \frac{137}{81} g_s g_Y^2 \bar{C}_{uG}^{rs} B_\mu^2 (\bar{u}_s \tilde{H}^\dagger q_r), \tag{2.25}
\end{aligned}$$

$$\begin{aligned}
\Delta S_{\mathcal{O}_{dB}} = & -\frac{1}{36} g_Y^2 \left[ \bar{y}_d^{rt} C_{dB}^{st} + y_d^{st} \bar{C}_{dB}^{rt} \right] (\bar{q}_s H \bar{B} H^\dagger q_r) + \frac{i}{27} g_L g_Y^2 \bar{C}_{dB}^{rs} t_j^{Ii} H_i^\dagger B_\mu W_\nu^I (\bar{d}_s \sigma^{\bar{\mu}\bar{\nu}} q_r^j) \\
& - \frac{i}{27} g_L g_Y^2 C_{dB}^{sr} t_j^{Ii} H^j B_\mu W_\nu^I (\bar{q}_{is} \sigma^{\bar{\mu}\bar{\nu}} d_r) - \frac{i}{18} g_s g_Y \bar{C}_{dB}^{rs} T_b^{Aa} G_\mu^A (\bar{d}_{as} H^\dagger \partial^{\bar{\mu}} q_r^b) \\
& + \frac{i}{18} g_s g_Y^2 \bar{C}_{dB}^{rs} T_b^{Aa} B_\mu G_\nu^A (\bar{d}_{as} \sigma^{\bar{\mu}\bar{\nu}} H^\dagger q_r^b) - \frac{i}{18} g_L g_Y C_{dB}^{sr} t_j^{Ii} H^j W_\mu^I (\bar{q}_{is} \partial^{\bar{\mu}} d_r) \\
& - \frac{1}{18} g_L g_Y C_{dB}^{sr} \varepsilon^{IJK} t_j^{Ki} H^j W_\mu^J W_\nu^I (\bar{q}_{is} \sigma^{\bar{\mu}\bar{\nu}} d_r) - \frac{i}{18} g_s g_Y^2 C_{dB}^{sr} T_b^{Aa} B_\mu G_\nu^A (\bar{q}_{as} H \sigma^{\bar{\mu}\bar{\nu}} d_r^b) \\
& + \frac{i}{18} g_L g_Y \bar{C}_{dB}^{rs} t_j^{Ii} H_i^\dagger W_\mu^I (\partial^{\bar{\mu}} \bar{d}_s q_r^j) + \frac{i}{18} g_s g_Y C_{dB}^{sr} T_b^{Aa} G_\mu^A (\partial^{\bar{\mu}} \bar{q}_{as} H d_r^b) - \frac{7i}{108} g_Y^2 \bar{C}_{dB}^{rs} B_\mu (\bar{d}_s H^\dagger \partial^{\bar{\mu}} q_r) \\
& + \frac{7i}{108} g_Y^2 C_{dB}^{sr} B_\mu (\partial^{\bar{\mu}} \bar{q}_s H d_r) + \frac{i}{12} g_Y^2 C_{dB}^{sr} B_\mu (\bar{q}_s \partial^{\bar{\mu}} H d_r) \\
& + \frac{1}{12} g_Y \left[ y_d^{st} \bar{C}_{dB}^{rt} - \bar{y}_d^{rt} C_{dB}^{st} \right] \left[ g_L t_j^{Ii} H_i^\dagger (\bar{q}_s H \bar{W}^I q_r^j) - g_L t_k^{Ij} H^k (\bar{q}_{js} \bar{W}^I H^\dagger q_r) \right] \\
& + \frac{5}{54} g_Y^2 \bar{C}_{dB}^{rs} B_\mu (\bar{d}_s \sigma^{\bar{\mu}\bar{\nu}} \partial^{\bar{\nu}} H^\dagger q_r) + \frac{5}{54} g_Y^2 C_{dB}^{sr} B_\mu (\bar{q}_s \partial^{\bar{\nu}} H \sigma^{\bar{\mu}\bar{\nu}} d_r) + \frac{67}{648} g_Y^3 \bar{C}_{dB}^{rs} B_\mu^2 (\bar{d}_s H^\dagger q_r) \\
& + \frac{67}{648} g_Y^3 C_{dB}^{sr} B_\mu^2 (\bar{q}_s H d_r) - \frac{i}{9} g_L g_s g_Y \bar{C}_{dB}^{rs} t_j^{Ii} T_b^{Aa} H_i^\dagger G_\mu^A W_\nu^I (\bar{d}_{as} \sigma^{\bar{\mu}\bar{\nu}} q_r^{bj}) \\
& + \frac{1}{9} g_L g_Y \bar{C}_{dB}^{rs} t_j^{Ii} W_\mu^I (\bar{d}_s \sigma^{\bar{\mu}\bar{\nu}} q_r^j) \partial^{\bar{\nu}} H_i^\dagger + \frac{1}{9} g_L g_Y C_{dB}^{sr} t_j^{Ii} W_\mu^I (\bar{q}_{is} \sigma^{\bar{\mu}\bar{\nu}} d_r) \partial^{\bar{\nu}} H^j \\
& + \frac{1}{3} g_s g_Y \left[ \bar{y}_d^{ts} C_{dB}^{tr} + y_d^{tr} \bar{C}_{dB}^{ts} \right] (H^\dagger H) (\bar{d}_s T^A \bar{G}^A d_r) - \frac{1}{18} g_L^2 g_Y \bar{C}_{dB}^{rs} \varepsilon^{IJK} t_j^{Ki} H_i^\dagger W_\mu^J W_\nu^I (\bar{d}_s \sigma^{\bar{\mu}\bar{\nu}} q_r^j) \\
& - \frac{i}{12} g_Y^2 \bar{C}_{dB}^{rs} B_\mu (\bar{d}_s \partial^{\bar{\mu}} H^\dagger q_r) - \frac{1}{12} g_L g_Y \left[ \bar{y}_d^{rt} C_{dB}^{st} + y_d^{st} \bar{C}_{dB}^{rt} \right] (H^\dagger t^I H) (\bar{q}_s \bar{W}^I q_r) \\
& - \frac{1}{9} g_Y^2 \left[ \bar{y}_d^{ts} C_{dB}^{tr} + y_d^{tr} \bar{C}_{dB}^{ts} \right] (H^\dagger H) (\bar{d}_s \bar{B} d_r) - \frac{1}{9} g_s g_Y \bar{C}_{dB}^{rs} T_b^{Aa} G_\mu^A (\bar{d}_{as} \sigma^{\bar{\mu}\bar{\nu}} \partial^{\bar{\nu}} H^\dagger q_r^b) \\
& - \frac{1}{9} g_s g_Y C_{dB}^{sr} T_b^{Aa} G_\mu^A (\bar{q}_{as} \partial^{\bar{\nu}} H \sigma^{\bar{\mu}\bar{\nu}} d_r^b) + \frac{i}{9} g_L g_s g_Y C_{dB}^{sr} t_j^{Ii} T_b^{Aa} H^j G_\mu^A W_\nu^I (\bar{q}_{ais} \sigma^{\bar{\mu}\bar{\nu}} d_r^b) \\
& - \frac{13i}{108} g_Y^2 C_{dB}^{sr} B_\mu (\bar{q}_s H \partial^{\bar{\mu}} d_r) + \frac{13i}{108} g_Y^2 \bar{C}_{dB}^{rs} B_\mu (\partial^{\bar{\mu}} \bar{d}_s H^\dagger q_r) - \frac{1}{8} g_L^2 g_Y \bar{C}_{dB}^{rs} W_\mu^{I2} (\bar{d}_s H^\dagger q_r) \\
& - \frac{1}{8} g_L^2 g_Y C_{dB}^{sr} W_\mu^{I2} (\bar{q}_s H d_r) - \frac{7}{54} g_L g_Y^2 \bar{C}_{dB}^{rs} t_j^{Ii} H_i^\dagger B_\mu W_\mu^I (\bar{d}_s q_r^j) - \frac{7}{54} g_L g_Y^2 C_{dB}^{sr} t_j^{Ii} H^j B_\mu W_\mu^I (\bar{q}_{is} d_r) \\
& + \frac{i}{6} \left[ \bar{y}_d^{rs} C_{dB}^{rs} + y_d^{rs} \bar{C}_{dB}^{rs} \right] \left[ 2g_Y B_\mu \tilde{B}^{\bar{\mu}\bar{\sigma}} (H^\dagger \partial_{\bar{\sigma}} H) - 2g_Y B_\mu \tilde{B}^{\bar{\mu}\bar{\sigma}} (\partial_{\bar{\sigma}} H^\dagger H) \right] \\
& - \frac{i}{6} \left[ \bar{y}_d^{rs} C_{dB}^{rs} - y_d^{rs} \bar{C}_{dB}^{rs} \right] \left[ 2g_Y B_\mu \tilde{B}^{\bar{\mu}\bar{\sigma}} (H^\dagger \partial_{\bar{\sigma}} H) + 2g_Y B_\mu \tilde{B}^{\bar{\mu}\bar{\sigma}} (\partial_{\bar{\sigma}} H^\dagger H) \right] \\
& - \frac{i}{6} g_L g_Y \bar{C}_{dB}^{rs} t_j^{Ii} H_i^\dagger W_\mu^I (\bar{d}_s \partial^{\bar{\mu}} q_r^j) \\
& + \frac{1}{3} \left[ -\bar{y}_d^{rs} C_{dB}^{rs} - y_d^{rs} \bar{C}_{dB}^{rs} \right] \left[ g_Y B_\mu B^{\bar{\mu}\bar{\nu}} (H^\dagger \partial_{\bar{\nu}} H) + g_Y B_\mu B^{\bar{\mu}\bar{\nu}} (\partial_{\bar{\nu}} H^\dagger H) \right] \\
& - \frac{1}{6} g_s g_Y \left[ \bar{y}_d^{rt} C_{dB}^{st} + y_d^{st} \bar{C}_{dB}^{rt} \right] (\bar{q}_s T^A H \bar{G}^A H^\dagger q_r) + \frac{i}{6} g_L g_Y C_{dB}^{sr} t_j^{Ii} H^j W_\mu^I (\partial^{\bar{\mu}} \bar{q}_{is} d_r)
\end{aligned}$$

$$\begin{aligned}
& + \frac{i}{6} g_L g_Y \bar{C}_{dB}^{rs} t_j^{Ii} W_{\mu}^I (\bar{d}_s q_r^j) \partial^{\bar{\mu}} H_i^{\dagger} - \frac{i}{6} g_L g_Y C_{dB}^{sr} t_j^{Ii} W_{\mu}^I (\bar{q}_{is} d_r) \partial^{\bar{\mu}} H^j + \frac{5i}{18} g_s g_Y C_{dB}^{sr} T_b^{Aa} G_{\mu}^A (\bar{q}_{as} H \partial^{\bar{\mu}} d_r^b) \\
& - \frac{5i}{18} g_s g_Y \bar{C}_{dB}^{rs} T_b^{Aa} G_{\mu}^A (\partial^{\bar{\mu}} \bar{d}_{as} H^{\dagger} q_r^b) + \frac{i}{3} g_Y \left[ \bar{y}_d^{ts} C_{dB}^{tr} - y_d^{tr} \bar{C}_{dB}^{ts} \right] B_{\bar{\mu}} B^{\bar{\mu}\nu} (\bar{d}_s \gamma^{\bar{\nu}} d_r) \\
& + \frac{1}{3} g_Y \left[ \bar{y}_d^{ts} C_{dB}^{tr} + y_d^{tr} \bar{C}_{dB}^{ts} \right] B_{\bar{\mu}} \tilde{B}^{\bar{\mu}\bar{\sigma}} (\bar{d}_s \gamma^{\bar{\sigma}} d_r) + \frac{i}{3} g_Y \left[ \bar{y}_d^{rt} C_{dB}^{st} - y_d^{st} \bar{C}_{dB}^{rt} \right] B_{\bar{\mu}} B^{\bar{\mu}\bar{\nu}} (\bar{q}_s \gamma^{\bar{\nu}} q_r) \\
& + \frac{1}{3} g_Y \left[ \bar{y}_d^{rt} C_{dB}^{st} + y_d^{st} \bar{C}_{dB}^{rt} \right] B_{\bar{\mu}} \tilde{B}^{\bar{\mu}\bar{\sigma}} (\bar{q}_s \gamma^{\bar{\sigma}} q_r) \\
& + \frac{1}{3} g_Y \left[ \bar{y}_d^{rs} C_{dB}^{rs} - y_d^{rs} \bar{C}_{dB}^{rs} \right] B_{\bar{\mu}} B^{\bar{\mu}\bar{\nu}} (H^{\dagger} \overset{\leftrightarrow}{\partial}_{\bar{\nu}} H) + \frac{7}{18} g_s^2 g_Y \bar{C}_{dB}^{rs} T_b^{Aa} T_a^{Bc} G_{\mu}^A G_{\mu}^B (\bar{d}_{cs} H^{\dagger} q_r^b) \\
& + \frac{7}{18} g_s^2 g_Y C_{dB}^{sr} T_b^{Aa} T_c^{Bb} G_{\mu}^A G_{\mu}^B (\bar{q}_{as} H d_r^c) + \frac{i}{2} g_s g_Y \bar{C}_{dB}^{rs} T_b^{Aa} G_{\mu}^A (\bar{d}_{as} \partial^{\bar{\mu}} H^{\dagger} q_r^b) \\
& - \frac{i}{2} g_s g_Y C_{dB}^{sr} T_b^{Aa} G_{\mu}^A (\bar{q}_{as} \partial^{\bar{\mu}} H d_r^b) + g_L \left[ 2 \bar{y}_d^{rs} \bar{C}_{dB}^{rs} - 2 y_d^{rs} C_{dB}^{rs} \right] W_{\mu}^I B^{\bar{\mu}\bar{\nu}} (H^{\dagger} t^I \overset{\leftrightarrow}{\partial}_{\bar{\nu}} H) \\
& - \frac{22}{27} g_s g_Y^2 \bar{C}_{dB}^{rs} T_b^{Aa} B_{\bar{\mu}} G_{\mu}^A (\bar{d}_{as} H^{\dagger} q_r^b) - \frac{22}{27} g_s g_Y^2 C_{dB}^{sr} T_b^{Aa} B_{\bar{\mu}} G_{\mu}^A (\bar{q}_{as} H d_r^b) \\
& - i \left[ \bar{y}_d^{rs} C_{dB}^{rs} + y_d^{rs} \bar{C}_{dB}^{rs} \right] \left[ 2 g_L W_{\mu}^I \tilde{B}^{\bar{\mu}\bar{\sigma}} (H^{\dagger} t^I \partial_{\bar{\sigma}} H) - 2 g_L W_{\mu}^I \tilde{B}^{\bar{\mu}\bar{\sigma}} (\partial_{\bar{\sigma}} H^{\dagger} t^I H) \right] \\
& + i \left[ \bar{y}_d^{rs} C_{dB}^{rs} - y_d^{rs} \bar{C}_{dB}^{rs} \right] \left[ 2 g_L W_{\mu}^I \tilde{B}^{\bar{\mu}\bar{\sigma}} (H^{\dagger} t^I \partial_{\bar{\sigma}} H) + 2 g_L W_{\mu}^I \tilde{B}^{\bar{\mu}\bar{\sigma}} (\partial_{\bar{\sigma}} H^{\dagger} t^I H) \right] \\
& - i g_s \left[ \bar{y}_d^{rt} C_{dB}^{st} - y_d^{st} \bar{C}_{dB}^{rt} \right] G_{\mu}^A B^{\bar{\mu}\bar{\nu}} (\bar{q}_s T^A \gamma^{\bar{\nu}} q_r) + g_s \left[ - \bar{y}_d^{rt} C_{dB}^{st} - y_d^{st} \bar{C}_{dB}^{rt} \right] G_{\mu}^A \tilde{B}^{\bar{\mu}\bar{\sigma}} (\bar{q}_s T^A \gamma^{\bar{\sigma}} q_r) \\
& - \frac{1}{12} g_L g_Y \left[ \bar{y}_d^{rt} C_{dB}^{st} + y_d^{st} \bar{C}_{dB}^{rt} \right] (H^{\dagger} H) (\bar{q}_s t^I \bar{W}^I q_r) - \frac{10}{9} g_L g_s g_Y C_{dB}^{sr} t_j^{Ii} T_b^{Aa} H^j G_{\mu}^A W_{\mu}^I (\bar{q}_{ais} d_r^b) \\
& - 2 i g_L g_Y \left[ \bar{y}_d^{rs} C_{dB}^{rs} - y_d^{rs} \bar{C}_{dB}^{rs} \right] B_{\bar{\mu}} W_{\bar{\nu}}^I B^{\bar{\mu}\bar{\nu}} (H^{\dagger} t^I H) + 2 g_L g_Y \left[ \bar{y}_d^{rs} C_{dB}^{rs} + y_d^{rs} \bar{C}_{dB}^{rs} \right] B_{\bar{\mu}} W_{\bar{\nu}}^I \tilde{B}^{\bar{\mu}\bar{\nu}} (H^{\dagger} t^I H) \\
& + 2 \left[ \bar{y}_d^{rs} C_{dB}^{rs} + y_d^{rs} \bar{C}_{dB}^{rs} \right] \left[ g_L W_{\mu}^I B^{\bar{\mu}\bar{\nu}} (H^{\dagger} t^I \partial_{\bar{\nu}} H) + g_L W_{\mu}^I B^{\bar{\mu}\bar{\nu}} (\partial_{\bar{\nu}} H^{\dagger} t^I H) \right] \\
& - 2 g_L^2 \left[ \bar{y}_d^{rs} C_{dB}^{rs} + y_d^{rs} \bar{C}_{dB}^{rs} \right] \varepsilon^{IJK} W_{\mu}^J W_{\bar{\nu}}^I B^{\bar{\mu}\bar{\nu}} (H^{\dagger} t^K H) \\
& - 2 i g_L^2 \left[ \bar{y}_d^{rs} C_{dB}^{rs} - y_d^{rs} \bar{C}_{dB}^{rs} \right] \varepsilon^{IJK} W_{\mu}^J W_{\bar{\nu}}^I \tilde{B}^{\bar{\mu}\bar{\nu}} (H^{\dagger} t^K H) \\
& + 2 i g_s \left[ \bar{y}_d^{ts} C_{dB}^{tr} - y_d^{tr} \bar{C}_{dB}^{ts} \right] G_{\mu}^A B^{\bar{\mu}\bar{\nu}} (\bar{d}_s T^A \gamma^{\bar{\nu}} d_r) + 2 g_s \left[ \bar{y}_d^{ts} C_{dB}^{tr} + y_d^{tr} \bar{C}_{dB}^{ts} \right] G_{\mu}^A \tilde{B}^{\bar{\mu}\bar{\sigma}} (\bar{d}_s T^A \gamma^{\bar{\sigma}} d_r) \\
& - \frac{10}{9} g_L g_s g_Y \bar{C}_{dB}^{rs} t_j^{Ii} T_b^{Aa} H_i^{\dagger} G_{\mu}^A W_{\mu}^I (\bar{d}_{as} q_r^{bj}), \tag{2.26}
\end{aligned}$$

$$\begin{aligned}
\Delta S_{\mathcal{O}_{dW}} &= - \frac{i}{12} g_L g_Y C_{dW}^{sr} B_{\bar{\mu}} (\bar{q}_s H \partial^{\bar{\mu}} d_r) + \frac{1}{12} g_L g_Y \left[ \bar{y}_d^{rt} C_{dW}^{st} + y_d^{st} \bar{C}_{dW}^{rt} \right] (\bar{q}_s H \bar{B} H^{\dagger} q_r) + \frac{i}{12} g_L g_Y \bar{C}_{dW}^{rs} B_{\bar{\mu}} (\partial^{\bar{\mu}} \bar{d}_s H^{\dagger} q_r) \\
& + \frac{1}{6} g_L^3 \bar{C}_{dW}^{rs} \varepsilon^{IJK} t_j^{Ki} H_i^{\dagger} W_{\mu}^J W_{\bar{\nu}}^I (\bar{d}_s \sigma^{\bar{\mu}\bar{\nu}} q_r^j) + \frac{1}{6} g_L g_Y \bar{C}_{dW}^{rs} B_{\bar{\mu}} (\bar{d}_s \sigma^{\bar{\mu}\bar{\nu}} \partial^{\bar{\nu}} H^{\dagger} q_r) \\
& + \frac{1}{6} g_L g_Y C_{dW}^{sr} B_{\bar{\mu}} (\bar{q}_s \partial^{\bar{\nu}} H \sigma^{\bar{\mu}\bar{\nu}} d_r) - \frac{1}{8} g_L^3 \bar{C}_{dW}^{rs} W_{\mu}^{I2} (\bar{d}_s H^{\dagger} q_r) - \frac{i}{6} g_L^2 \bar{C}_{dW}^{rs} t_j^{Ii} H_i^{\dagger} W_{\mu}^I (\partial^{\bar{\mu}} \bar{d}_s q_r^j) \\
& + \frac{1}{4} g_L^2 \left[ \bar{y}_d^{rt} C_{dW}^{st} + y_d^{st} \bar{C}_{dW}^{rt} \right] (H^{\dagger} H) (\bar{q}_s t^I \bar{W}^I q_r) \\
& + \frac{1}{4} g_L \left[ \bar{y}_d^{rt} C_{dW}^{st} - y_d^{st} \bar{C}_{dW}^{rt} \right] \left[ g_L t_j^{Ii} H_i^{\dagger} (\bar{q}_s H \bar{W}^I q_r^j) - g_L t_k^{Ij} H^k (\bar{q}_{js} \bar{W}^I H^{\dagger} q_r) \right] - \frac{13}{72} g_L g_Y^2 \bar{C}_{dW}^{rs} B_{\bar{\mu}}^2 (\bar{d}_s H^{\dagger} q_r) \\
& - \frac{i}{4} g_L g_Y \bar{C}_{dW}^{rs} B_{\bar{\mu}} (\bar{d}_s H^{\dagger} \partial^{\bar{\mu}} q_r) + \frac{i}{4} g_L g_Y \bar{C}_{dW}^{rs} B_{\bar{\mu}} (\bar{d}_s \partial^{\bar{\mu}} H^{\dagger} q_r) + \frac{i}{4} g_L g_Y C_{dW}^{sr} B_{\bar{\mu}} (\partial^{\bar{\mu}} \bar{q}_s H d_r)
\end{aligned}$$

$$\begin{aligned}
& + \frac{i}{3} \left[ \bar{y}_d^{rs} \mathcal{C}_{dW}^{rs} + y_d^{rs} \bar{\mathcal{C}}_{dW}^{rs} \right] \left[ 2g_Y B_{\bar{\mu}} \widetilde{W}^{\bar{\mu}\bar{\sigma}I} (H^\dagger t^I \partial_{\bar{\sigma}} H) - 2g_Y B_{\bar{\mu}} \widetilde{W}^{\bar{\mu}\bar{\sigma}I} (\partial_{\bar{\sigma}} H^\dagger t^I H) \right] \\
& - \frac{i}{3} \left[ \bar{y}_d^{rs} \mathcal{C}_{dW}^{rs} - y_d^{rs} \bar{\mathcal{C}}_{dW}^{rs} \right] \left[ 2g_Y B_{\bar{\mu}} \widetilde{W}^{\bar{\mu}\bar{\sigma}I} (H^\dagger t^I \partial_{\bar{\sigma}} H) + 2g_Y B_{\bar{\mu}} \widetilde{W}^{\bar{\mu}\bar{\sigma}I} (\partial_{\bar{\sigma}} H^\dagger t^I H) \right] \\
& + \frac{i}{3} g_L^2 g_Y \bar{\mathcal{C}}_{dW}^{rs} t_j^{Ii} H_i^\dagger B_{\bar{\mu}} W_{\bar{\nu}}^I (\bar{d}_s \sigma^{\bar{\mu}\bar{\nu}} q_r^j) \\
& - \frac{i}{2} \left[ \bar{y}_d^{rs} \mathcal{C}_{dW}^{rs} + y_d^{rs} \bar{\mathcal{C}}_{dW}^{rs} \right] \left[ 2g_L W_{\bar{\mu}}^I \widetilde{W}^{\bar{\mu}\bar{\sigma}I} (H^\dagger \partial_{\bar{\sigma}} H) - 2g_L W_{\bar{\mu}}^I \widetilde{W}^{\bar{\mu}\bar{\sigma}I} (\partial_{\bar{\sigma}} H^\dagger H) \right] \\
& + \frac{i}{2} \left[ \bar{y}_d^{rs} \mathcal{C}_{dW}^{rs} - y_d^{rs} \bar{\mathcal{C}}_{dW}^{rs} \right] \left[ 2g_L W_{\bar{\mu}}^I \widetilde{W}^{\bar{\mu}\bar{\sigma}I} (H^\dagger \partial_{\bar{\sigma}} H) + 2g_L W_{\bar{\mu}}^I \widetilde{W}^{\bar{\mu}\bar{\sigma}I} (\partial_{\bar{\sigma}} H^\dagger H) \right] \\
& - \frac{i}{2} g_L g_s g_Y \bar{\mathcal{C}}_{dW}^{rs} T_b^{Aa} B_{\bar{\mu}} G_{\bar{\nu}}^A (\bar{d}_{as} \sigma^{\bar{\mu}\bar{\nu}} H^\dagger q_r^b) + \frac{1}{2} g_L g_s \left[ \bar{y}_d^{rt} \mathcal{C}_{dW}^{st} + y_d^{st} \bar{\mathcal{C}}_{dW}^{rt} \right] (\bar{q}_s T^A H \bar{G}^A H^\dagger q_r) \\
& - \frac{1}{6} g_L g_Y \left[ \bar{y}_d^{rt} \mathcal{C}_{dW}^{st} + y_d^{st} \bar{\mathcal{C}}_{dW}^{rt} \right] (H^\dagger H) (\bar{q}_s \bar{B} q_r) - \frac{i}{4} g_L g_Y \mathcal{C}_{dW}^{sr} B_{\bar{\mu}} (\bar{q}_s \partial^{\bar{\mu}} H d_r) - \frac{i}{2} g_L g_s \mathcal{C}_{dW}^{sr} T_b^{Aa} G_{\bar{\mu}}^A (\bar{q}_{as} H \partial^{\bar{\mu}} d_r^b) \\
& + \frac{i}{2} g_L g_s g_Y \mathcal{C}_{dW}^{sr} T_b^{Aa} B_{\bar{\mu}} G_{\bar{\nu}}^A (\bar{q}_{as} H \sigma^{\bar{\mu}\bar{\nu}} d_r^b) + \frac{i}{2} g_L g_s \bar{\mathcal{C}}_{dW}^{rs} T_b^{Aa} G_{\bar{\mu}}^A (\partial^{\bar{\mu}} \bar{d}_{as} H^\dagger q_r^b) \\
& - \frac{i}{2} g_L^2 \mathcal{C}_{dW}^{sr} t_j^{Ii} H^j W_{\bar{\mu}}^I (\partial^{\bar{\mu}} \bar{q}_{is} d_r) - \frac{i}{2} g_L^2 \bar{\mathcal{C}}_{dW}^{rs} t_j^{Ii} W_{\bar{\mu}}^I (\bar{d}_s q_r^j) \partial^{\bar{\mu}} H_i^\dagger + \frac{i}{2} g_L^2 \mathcal{C}_{dW}^{sr} t_j^{Ii} W_{\bar{\mu}}^I (\bar{q}_{is} d_r) \partial^{\bar{\mu}} H^j \\
& + \frac{2i}{3} g_Y \left[ \bar{y}_d^{rt} \mathcal{C}_{dW}^{st} - y_d^{st} \bar{\mathcal{C}}_{dW}^{rt} \right] B_{\bar{\mu}} W^{\bar{\mu}\bar{\nu}I} (\bar{q}_s t^I \gamma^{\bar{\nu}} q_r) \\
& + \frac{2}{3} g_Y \left[ \bar{y}_d^{rt} \mathcal{C}_{dW}^{st} + y_d^{st} \bar{\mathcal{C}}_{dW}^{rt} \right] B_{\bar{\mu}} \widetilde{W}^{\bar{\mu}\bar{\sigma}I} (\bar{q}_s t^I \gamma^{\bar{\sigma}} q_r) \\
& + \frac{2}{3} g_Y \left[ \bar{y}_d^{rs} \mathcal{C}_{dW}^{rs} - y_d^{rs} \bar{\mathcal{C}}_{dW}^{rs} \right] B_{\bar{\mu}} W^{\bar{\mu}\bar{\nu}I} (H^\dagger t^I \partial_{\bar{\nu}} H) - i g_L g_Y \left[ \bar{y}_d^{rs} \mathcal{C}_{dW}^{rs} - y_d^{rs} \bar{\mathcal{C}}_{dW}^{rs} \right] B_{\bar{\mu}} W_{\bar{\nu}}^I W^{\bar{\mu}\bar{\nu}I} (H^\dagger H) \\
& + g_L^2 \left[ -\bar{y}_d^{rs} \mathcal{C}_{dW}^{rs} - y_d^{rs} \bar{\mathcal{C}}_{dW}^{rs} \right] \varepsilon^{IJK} W_{\bar{\mu}}^K W_{\bar{\nu}}^J W^{\bar{\mu}\bar{\nu}I} (H^\dagger H) + g_L g_Y \left[ \bar{y}_d^{rs} \mathcal{C}_{dW}^{rs} + y_d^{rs} \bar{\mathcal{C}}_{dW}^{rs} \right] B_{\bar{\mu}} W_{\bar{\nu}}^I \widetilde{W}^{\bar{\mu}\bar{\nu}I} (H^\dagger H) \\
& - i g_L^2 \left[ \bar{y}_d^{rs} \mathcal{C}_{dW}^{rs} - y_d^{rs} \bar{\mathcal{C}}_{dW}^{rs} \right] \varepsilon^{IJK} W_{\bar{\mu}}^K W_{\bar{\nu}}^J \widetilde{W}^{\bar{\mu}\bar{\nu}I} (H^\dagger H) \\
& + \left[ \bar{y}_d^{rs} \mathcal{C}_{dW}^{rs} + y_d^{rs} \bar{\mathcal{C}}_{dW}^{rs} \right] \left[ g_L W_{\bar{\mu}}^I W^{\bar{\mu}\bar{\nu}I} (H^\dagger \partial_{\bar{\nu}} H) + g_L W_{\bar{\mu}}^I W^{\bar{\mu}\bar{\nu}I} (\partial_{\bar{\nu}} H^\dagger H) \right] \\
& + \left[ y_d^{rs} \bar{\mathcal{C}}_{dW}^{rs} - \bar{y}_d^{rs} \mathcal{C}_{dW}^{rs} \right] \left[ 2g_L \varepsilon^{IJK} W_{\bar{\mu}}^J \widetilde{W}^{\bar{\mu}\bar{\sigma}I} (H^\dagger t^K \partial_{\bar{\sigma}} H) - 2g_L \varepsilon^{IJK} W_{\bar{\mu}}^J \widetilde{W}^{\bar{\mu}\bar{\sigma}I} (\partial_{\bar{\sigma}} H^\dagger t^K H) \right] \\
& + \left[ \bar{y}_d^{rs} \mathcal{C}_{dW}^{rs} + y_d^{rs} \bar{\mathcal{C}}_{dW}^{rs} \right] \left[ 2g_L \varepsilon^{IJK} W_{\bar{\mu}}^J \widetilde{W}^{\bar{\mu}\bar{\sigma}I} (H^\dagger t^K \partial_{\bar{\sigma}} H) + 2g_L \varepsilon^{IJK} W_{\bar{\mu}}^J \widetilde{W}^{\bar{\mu}\bar{\sigma}I} (\partial_{\bar{\sigma}} H^\dagger t^K H) \right] \\
& + g_L g_s \mathcal{C}_{dW}^{sr} T_b^{Aa} G_{\bar{\mu}}^A (\bar{q}_{as} \partial^{\bar{\mu}} H \sigma^{\bar{\mu}\bar{\nu}} d_r^b) - \frac{1}{18} g_L^2 g_Y \bar{\mathcal{C}}_{dW}^{rs} t_j^{Ii} H_i^\dagger B_{\bar{\mu}} W_{\bar{\mu}}^I (\bar{d}_s q_r^j) \\
& + \frac{i}{2} g_L^2 \bar{\mathcal{C}}_{dW}^{rs} t_j^{Ii} H_i^\dagger W_{\bar{\mu}}^I (\bar{d}_s \partial^{\bar{\mu}} q_r^j) \\
& - \frac{2}{3} \left[ \bar{y}_d^{rs} \mathcal{C}_{dW}^{rs} + y_d^{rs} \bar{\mathcal{C}}_{dW}^{rs} \right] \left[ g_Y B_{\bar{\mu}} W^{\bar{\mu}\bar{\nu}I} (H^\dagger t^I \partial_{\bar{\nu}} H) + g_Y B_{\bar{\mu}} W^{\bar{\mu}\bar{\nu}I} (\partial_{\bar{\nu}} H^\dagger t^I H) \right] \\
& - \frac{3}{4} g_L^2 \left[ \bar{y}_d^{rt} \mathcal{C}_{dW}^{st} + y_d^{st} \bar{\mathcal{C}}_{dW}^{rt} \right] (H^\dagger t^I H) (\bar{q}_s \bar{W}^I q_r) + i g_L \left[ \bar{y}_d^{ts} \mathcal{C}_{dW}^{tr} - y_d^{tr} \bar{\mathcal{C}}_{dW}^{ts} \right] W_{\bar{\mu}}^I W^{\bar{\mu}\bar{\nu}I} (\bar{d}_s \gamma^{\bar{\nu}} d_r) \\
& + g_L \left[ \bar{y}_d^{ts} \mathcal{C}_{dW}^{tr} + y_d^{tr} \bar{\mathcal{C}}_{dW}^{ts} \right] W_{\bar{\mu}}^I \widetilde{W}^{\bar{\mu}\bar{\sigma}I} (\bar{d}_s \gamma^{\bar{\sigma}} d_r) + i g_L^2 g_s \bar{\mathcal{C}}_{dW}^{rs} t_j^{Ii} T_b^{Aa} H_i^\dagger G_{\bar{\mu}}^A W_{\bar{\nu}}^I (\bar{d}_{as} \sigma^{\bar{\mu}\bar{\nu}} q_r^{bj}) \\
& + g_L g_s \bar{\mathcal{C}}_{dW}^{rs} T_b^{Aa} G_{\bar{\mu}}^A (\bar{d}_{as} \sigma^{\bar{\mu}\bar{\nu}} \partial^{\bar{\nu}} H^\dagger q_r^b) - \frac{1}{8} g_L^3 \mathcal{C}_{dW}^{sr} W_{\bar{\mu}}^{I2} (\bar{q}_s H d_r) - \frac{13}{72} g_L g_Y^2 \mathcal{C}_{dW}^{sr} B_{\bar{\mu}}^2 (\bar{q}_s H d_r) \\
& - g_L g_s \left[ \bar{y}_d^{rt} \mathcal{C}_{dW}^{st} + y_d^{st} \bar{\mathcal{C}}_{dW}^{rt} \right] (H^\dagger H) (\bar{q}_s T^A \bar{G}^A q_r) - i g_L^2 g_s \mathcal{C}_{dW}^{sr} t_j^{Ii} T_b^{Aa} H^j G_{\bar{\mu}}^A W_{\bar{\nu}}^I (\bar{q}_{ais} \sigma^{\bar{\mu}\bar{\nu}} d_r^b)
\end{aligned}$$

$$\begin{aligned}
& + g_L \left[ y_d^{rs} \bar{\mathcal{C}}_{dW}^{rs} - \bar{y}_d^{rs} \mathcal{C}_{dW}^{rs} \right] W_\mu^I W^{\mu\nu I} (H^\dagger \partial_\nu H) - \frac{1}{3} g_L^2 \bar{\mathcal{C}}_{dW}^{rs} t_j^{Ii} W_\mu^I (\bar{d}_s \sigma^{\mu\nu} q_r^j) \partial^\nu H_i^\dagger \\
& - \frac{1}{3} g_L^2 \mathcal{C}_{dW}^{sr} t_j^{Ii} W_\mu^I (\bar{q}_{is} \sigma^{\mu\nu} d_r) \partial^\nu H^j - \frac{4}{3} g_L^2 \bar{\mathcal{C}}_{dW}^{rs} t_j^{Ii} T_b^{Aa} H_i^\dagger G_\mu^A W_\mu^I (\bar{d}_{as} q_r^{bj}) \\
& - \frac{4}{3} g_L^2 g_s \mathcal{C}_{dW}^{sr} t_j^{Ii} T_b^{Aa} H^j G_\mu^A W_\mu^I (\bar{q}_{ais} d_r^b) - \frac{3i}{2} g_L g_s \bar{\mathcal{C}}_{dW}^{rs} T_b^{Aa} G_\mu^A (\bar{d}_{as} H^\dagger \partial^\mu q_r^b) \\
& + \frac{3i}{2} g_L g_s \bar{\mathcal{C}}_{dW}^{rs} T_b^{Aa} G_\mu^A (\bar{d}_{as} \partial^\mu H^\dagger q_r^b) - \frac{3i}{2} g_L g_s \mathcal{C}_{dW}^{sr} T_b^{Aa} G_\mu^A (\bar{q}_{as} \partial^\mu H d_r^b) + \frac{3i}{2} g_L g_s \mathcal{C}_{dW}^{sr} T_b^{Aa} G_\mu^A (\partial^\mu \bar{q}_{as} H d_r^b) \\
& - \frac{5}{3} g_L g_s g_Y \bar{\mathcal{C}}_{dW}^{rs} T_b^{Aa} B_\mu G_\mu^A (\bar{d}_{as} H^\dagger q_r^b) - 2 g_L g_Y \left[ \bar{y}_d^{rs} \mathcal{C}_{dW}^{rs} + y_d^{rs} \bar{\mathcal{C}}_{dW}^{rs} \right] \varepsilon^{IJK} B_\mu W_\nu^J W^{\mu\nu I} (H^\dagger t^K H) \\
& - 2i g_L g_Y \left[ \bar{y}_d^{rs} \mathcal{C}_{dW}^{rs} - y_d^{rs} \bar{\mathcal{C}}_{dW}^{rs} \right] \varepsilon^{IJK} B_\mu W_\nu^J \widetilde{W}^{\mu\nu I} (H^\dagger t^K H) \\
& - 2i \left[ \bar{y}_d^{rs} \mathcal{C}_{dW}^{rs} - y_d^{rs} \bar{\mathcal{C}}_{dW}^{rs} \right] \left[ g_L \varepsilon^{IJK} W_\mu^J W^{\mu\nu I} (H^\dagger t^K \partial_\nu H) + g_L \varepsilon^{IJK} W_\mu^J W^{\mu\nu I} (\partial_\nu H^\dagger t^K H) \right] \\
& - 2i g_s \left[ \bar{y}_d^{rt} \mathcal{C}_{dW}^{st} - y_d^{st} \bar{\mathcal{C}}_{dW}^{rt} \right] G_\mu^A W^{\mu\nu I} (\bar{q}_s t^I T^A \gamma^\nu q_r) \\
& + 2g_s \left[ -\bar{y}_d^{rt} \mathcal{C}_{dW}^{st} - y_d^{st} \bar{\mathcal{C}}_{dW}^{rt} \right] G_\mu^A \widetilde{W}^{\mu\bar{\sigma} I} (\bar{q}_s t^I T^A \gamma^{\bar{\sigma}} q_r) - \frac{1}{18} g_L^2 g_Y \mathcal{C}_{dW}^{sr} t_j^{Ii} H^j B_\mu W_\mu^I (\bar{q}_{is} d_r) \\
& + \frac{i}{6} g_L^2 \mathcal{C}_{dW}^{sr} t_j^{Ii} H^j W_\mu^I (\bar{q}_{is} \partial^\mu d_r) + \frac{1}{6} g_L^3 \mathcal{C}_{dW}^{sr} \varepsilon^{IJK} t_j^{Ki} H^j W_\mu^J W_\nu^I (\bar{q}_{is} \sigma^{\mu\nu} d_r) \\
& - \frac{i}{3} g_L^2 g_Y \mathcal{C}_{dW}^{sr} t_j^{Ii} H^j B_\mu W_\nu^I (\bar{q}_{is} \sigma^{\mu\nu} d_r) - \frac{5}{3} g_L g_s g_Y \mathcal{C}_{dW}^{sr} T_b^{Aa} B_\mu G_\mu^A (\bar{q}_{as} H d_r^b) \\
& + 2i g_L \left[ \bar{y}_d^{rs} \mathcal{C}_{dW}^{rs} + y_d^{rs} \bar{\mathcal{C}}_{dW}^{rs} \right] \varepsilon^{IJK} W_\mu^J W^{\mu\nu I} (H^\dagger t^K \partial_\nu H) - \frac{7}{2} g_L g_s^2 \bar{\mathcal{C}}_{dW}^{rs} T_b^{Aa} T_a^{Bc} G_\mu^A G_\mu^B (\bar{d}_{cs} H^\dagger q_r^b) \\
& - \frac{7}{2} g_L g_s^2 \mathcal{C}_{dW}^{sr} T_b^{Aa} T_c^{Bb} G_\mu^A G_\mu^B (\bar{q}_{as} H d_r^c) - 4i g_L^2 \left[ \bar{y}_d^{rs} \mathcal{C}_{dW}^{rs} - y_d^{rs} \bar{\mathcal{C}}_{dW}^{rs} \right] W_\mu^I W_\nu^J W^{\mu\nu J} (H^\dagger t^I H) \\
& + 4g_L^2 \left[ \bar{y}_d^{rs} \mathcal{C}_{dW}^{rs} + y_d^{rs} \bar{\mathcal{C}}_{dW}^{rs} \right] W_\mu^I W_\nu^J \widetilde{W}^{\mu\nu J} (H^\dagger t^I H), \tag{2.27}
\end{aligned}$$

$$\begin{aligned}
\Delta S_{\mathcal{O}_{dG}} = & -\frac{2i}{27} g_s g_Y \bar{\mathcal{C}}_{dG}^{rs} B_\mu (\bar{d}_s H^\dagger \partial^\mu q_r) + \frac{2i}{27} g_s g_Y \mathcal{C}_{dG}^{sr} B_\mu (\partial^\mu \bar{q}_s H d_r) + \frac{i}{9} g_s^2 g_Y \bar{\mathcal{C}}_{dG}^{rs} T_b^{Aa} B_\mu G_\nu^A (\bar{d}_{as} \sigma^{\mu\nu} H^\dagger q_r^b) \\
& - \frac{i}{9} g_s^2 g_Y \mathcal{C}_{dG}^{sr} T_b^{Aa} B_\mu G_\nu^A (\bar{q}_{as} H \sigma^{\mu\nu} d_r^b) + \frac{1}{6} g_s^2 \left[ \bar{y}_d^{rs} \mathcal{C}_{dG}^{rs} + y_d^{rs} \bar{\mathcal{C}}_{dG}^{rs} \right] f^{ABC} G_\mu^B G_\nu^C G^{\mu\nu A} (H^\dagger H) \\
& + \frac{i}{6} g_s^2 \left[ \bar{y}_d^{rs} \mathcal{C}_{dG}^{rs} - y_d^{rs} \bar{\mathcal{C}}_{dG}^{rs} \right] f^{ABC} G_\mu^B G_\nu^C \widetilde{G}^{\mu\nu A} (H^\dagger H) + \frac{1}{6} g_s^2 \left[ \bar{y}_d^{ts} \mathcal{C}_{dG}^{tr} + y_d^{tr} \bar{\mathcal{C}}_{dG}^{ts} \right] (H^\dagger H) (\bar{d}_s T^A \bar{\mathcal{G}}^A d_r) \\
& + \frac{1}{6} g_s^2 \left[ \bar{y}_d^{rt} \mathcal{C}_{dG}^{st} + y_d^{st} \bar{\mathcal{C}}_{dG}^{rt} \right] (\bar{q}_s T^A H \bar{\mathcal{G}}^A H^\dagger q_r) + \frac{11}{54} g_s^2 g_Y \bar{\mathcal{C}}_{dG}^{rs} T_b^{Aa} B_\mu G_\mu^A (\bar{d}_{as} H^\dagger q_r^b) \\
& + \frac{11}{54} g_s^2 g_Y \mathcal{C}_{dG}^{sr} T_b^{Aa} B_\mu G_\mu^A (\bar{q}_{as} H d_r^b) - \frac{4}{27} g_s g_Y \mathcal{C}_{dG}^{sr} B_\mu (\bar{q}_s \partial^\nu H \sigma^{\mu\nu} d_r) \\
& + \frac{2i}{9} g_s^2 \bar{\mathcal{C}}_{dG}^{rs} T_b^{Aa} G_\mu^A (\bar{d}_{as} H^\dagger \partial^\mu q_r^b) - \frac{2i}{9} g_L g_s^2 \bar{\mathcal{C}}_{dG}^{rs} t_j^{Ii} T_b^{Aa} H_i^\dagger G_\mu^A W_\nu^I (\bar{d}_{as} \sigma^{\mu\nu} q_r^{bj}) \\
& + \frac{2i}{9} g_s^2 \mathcal{C}_{dG}^{sr} T_b^{Aa} G_\mu^A (\bar{q}_{as} H \partial^\mu d_r^b) + \frac{2i}{9} g_L g_s^2 \mathcal{C}_{dG}^{sr} t_j^{Ii} T_b^{Aa} H^j G_\mu^A W_\nu^I (\bar{q}_{ais} \sigma^{\mu\nu} d_r^b) \\
& - \frac{2i}{9} g_s^2 \bar{\mathcal{C}}_{dG}^{rs} T_b^{Aa} G_\mu^A (\partial^\mu \bar{d}_{as} H^\dagger q_r^b) - \frac{2i}{9} g_s^2 \mathcal{C}_{dG}^{sr} T_b^{Aa} G_\mu^A (\partial^\mu \bar{q}_{as} H d_r^b) \\
& + \frac{1}{4} \left[ \bar{y}_d^{st} \bar{\mathcal{C}}_{dG}^{rt} - \bar{y}_d^{rt} \mathcal{C}_{dG}^{st} \right] \left[ 2g_s T_b^{Aa} T_c^{Bb} G_\mu^B \widetilde{G}^{\mu\bar{\sigma} A} (\bar{q}_{as} \gamma^{\bar{\sigma}} q_r^c) - 2g_s T_b^{Aa} T_a^{Bc} G_\mu^B \widetilde{G}^{\mu\bar{\sigma} A} (\bar{q}_{cs} \gamma^{\bar{\sigma}} q_r^b) \right]
\end{aligned}$$

$$\begin{aligned}
& + \frac{1}{4} \left[ -\bar{y}_d^{rt} \mathcal{C}_{dG}^{st} - y_d^{st} \bar{\mathcal{C}}_{dG}^{rt} \right] \left[ 2g_s T_b^{Aa} T_c^{Bb} G_\mu^B \tilde{G}^{\mu\bar{\sigma}A} (\bar{q}_{as} \gamma^\sigma q_r^c) + 2g_s T_b^{Aa} T_a^{Bc} G_\mu^B \tilde{G}^{\mu\bar{\sigma}A} (\bar{q}_{cs} \gamma^\sigma q_r^b) \right] \\
& - \frac{i}{3} \left[ \bar{y}_d^{rs} \mathcal{C}_{dG}^{rs} + y_d^{rs} \bar{\mathcal{C}}_{dG}^{rs} \right] \left[ 2g_s G_\mu^A \tilde{G}^{\mu\bar{\sigma}A} (H^\dagger \partial_{\bar{\sigma}} H) - 2g_s G_\mu^A \tilde{G}^{\mu\bar{\sigma}A} (\partial_{\bar{\sigma}} H^\dagger H) \right] \\
& + \frac{i}{3} \left[ \bar{y}_d^{rs} \mathcal{C}_{dG}^{rs} - y_d^{rs} \bar{\mathcal{C}}_{dG}^{rs} \right] \left[ 2g_s G_\mu^A \tilde{G}^{\mu\bar{\sigma}A} (H^\dagger \partial_{\bar{\sigma}} H) + 2g_s G_\mu^A \tilde{G}^{\mu\bar{\sigma}A} (\partial_{\bar{\sigma}} H^\dagger H) \right] \\
& + \frac{i}{3} g_Y \left[ \bar{y}_d^{rt} \mathcal{C}_{dG}^{st} - y_d^{st} \bar{\mathcal{C}}_{dG}^{rt} \right] B_\mu G^{\mu\bar{\nu}A} (\bar{q}_s T^A \gamma^\nu q_r) \\
& + \frac{1}{3} g_Y \left[ \bar{y}_d^{rt} \mathcal{C}_{dG}^{st} + y_d^{st} \bar{\mathcal{C}}_{dG}^{rt} \right] B_\mu \tilde{G}^{\mu\bar{\sigma}A} (\bar{q}_s T^A \gamma^\sigma q_r) + \frac{4}{9} g_s g_Y \left[ \bar{y}_d^{ts} \mathcal{C}_{dG}^{tr} + y_d^{tr} \bar{\mathcal{C}}_{dG}^{ts} \right] (H^\dagger H) (\bar{d}_s \bar{B} d_r) \\
& + \frac{1}{2} \left[ \bar{y}_d^{tr} \bar{\mathcal{C}}_{dG}^{ts} - \bar{y}_d^{ts} \bar{\mathcal{C}}_{dG}^{tr} \right] \left[ 2g_s T_b^{Aa} T_c^{Bb} G_\mu^B \tilde{G}^{\mu\bar{\sigma}A} (\bar{d}_{as} \gamma^\sigma d_r^c) - 2g_s T_b^{Aa} T_a^{Bc} G_\mu^B \tilde{G}^{\mu\bar{\sigma}A} (\bar{d}_{cs} \gamma^\sigma d_r^b) \right] \\
& + \frac{1}{2} \left[ \bar{y}_d^{ts} \mathcal{C}_{dG}^{tr} + y_d^{tr} \bar{\mathcal{C}}_{dG}^{ts} \right] \left[ 2g_s T_b^{Aa} T_c^{Bb} G_\mu^B \tilde{G}^{\mu\bar{\sigma}A} (\bar{d}_{as} \gamma^\sigma d_r^c) + 2g_s T_b^{Aa} T_a^{Bc} G_\mu^B \tilde{G}^{\mu\bar{\sigma}A} (\bar{d}_{cs} \gamma^\sigma d_r^b) \right] \\
& + \frac{7}{9} g_s^3 \bar{\mathcal{C}}_{dG}^{rs} T_b^{Aa} T_a^{Bc} G_\mu^A G_\mu^B (\bar{d}_{cs} H^\dagger q_r^b) - \frac{4}{27} g_s g_Y \bar{\mathcal{C}}_{dG}^{rs} B_\mu (\bar{d}_s \sigma^{\mu\bar{\nu}} \partial^\nu H^\dagger q_r) \\
& - \frac{2}{9} g_s^2 \bar{\mathcal{C}}_{dG}^{rs} T_b^{Aa} G_\mu^A (\bar{d}_{as} \sigma^{\mu\bar{\nu}} \partial^\nu H^\dagger q_r^b) - \frac{2}{9} g_s g_Y \left[ \bar{y}_d^{rt} \mathcal{C}_{dG}^{st} + y_d^{st} \bar{\mathcal{C}}_{dG}^{rt} \right] (\bar{q}_s H \bar{B} H^\dagger q_r) \\
& + \frac{i}{3} g_Y \left[ \bar{y}_d^{ts} \mathcal{C}_{dG}^{tr} - y_d^{tr} \bar{\mathcal{C}}_{dG}^{ts} \right] B_\mu G^{\mu\bar{\nu}A} (\bar{d}_s T^A \gamma^\nu d_r) \\
& + \frac{1}{3} g_Y \left[ \bar{y}_d^{ts} \mathcal{C}_{dG}^{tr} + y_d^{tr} \bar{\mathcal{C}}_{dG}^{ts} \right] B_\mu \tilde{G}^{\mu\bar{\sigma}A} (\bar{d}_s T^A \gamma^\sigma d_r) + \frac{10i}{27} g_s g_Y \mathcal{C}_{dG}^{sr} B_\mu (\bar{q}_s H \partial^\mu d_r) \\
& - \frac{10i}{27} g_s g_Y \bar{\mathcal{C}}_{dG}^{rs} B_\mu (\partial^\mu \bar{d}_s H^\dagger q_r) - \frac{4}{9} g_L^2 g_s \bar{\mathcal{C}}_{dG}^{rs} \varepsilon^{IJK} t_j^{Ki} H_i^\dagger W_\mu^J W_\nu^I (\bar{d}_s \sigma^{\mu\bar{\nu}} q_r^j) \\
& - \frac{4i}{9} g_L g_s \mathcal{C}_{dG}^{sr} t_j^{Ii} H^j W_\mu^I (\bar{q}_{is} \partial^\mu d_r) + \frac{4i}{9} g_L g_s \bar{\mathcal{C}}_{dG}^{rs} t_j^{Ii} H_i^\dagger W_\mu^I (\partial^\mu \bar{d}_s q_r^j) \\
& - \frac{i}{2} g_s g_Y \left[ \bar{y}_d^{rs} \mathcal{C}_{dG}^{rs} - y_d^{rs} \bar{\mathcal{C}}_{dG}^{rs} \right] B_\mu G_\nu^A G^{\mu\bar{\nu}A} (H^\dagger H) + \frac{1}{2} g_s g_Y \left[ \bar{y}_d^{rs} \mathcal{C}_{dG}^{rs} + y_d^{rs} \bar{\mathcal{C}}_{dG}^{rs} \right] B_\mu G_\nu^A \tilde{G}^{\mu\bar{\nu}A} (H^\dagger H) \\
& + \frac{16i}{27} g_L g_s g_Y \mathcal{C}_{dG}^{sr} t_j^{Ii} H^j B_\mu W_\nu^I (\bar{q}_{is} \sigma^{\mu\bar{\nu}} d_r) \\
& + \frac{2}{3} \left[ \bar{y}_d^{rs} \mathcal{C}_{dG}^{rs} + y_d^{rs} \bar{\mathcal{C}}_{dG}^{rs} \right] \left[ g_s G_\mu^A G^{\mu\bar{\nu}A} (H^\dagger \partial_\nu H) + g_s G_\mu^A G^{\mu\bar{\nu}A} (\partial_\nu H^\dagger H) \right] - \frac{1}{2} g_s^3 \bar{\mathcal{C}}_{dG}^{rs} G_\mu^{A2} (\bar{d}_s H^\dagger q_r) \\
& - \frac{1}{2} g_s^3 \mathcal{C}_{dG}^{sr} G_\mu^{A2} (\bar{q}_s H d_r) - \frac{16i}{27} g_L g_s g_Y \bar{\mathcal{C}}_{dG}^{rs} t_j^{Ii} H_i^\dagger B_\mu W_\nu^I (\bar{d}_s \sigma^{\mu\bar{\nu}} q_r^j) - \frac{53}{81} g_s g_Y^2 \bar{\mathcal{C}}_{dG}^{rs} B_\mu^2 (\bar{d}_s H^\dagger q_r) \\
& - \frac{53}{81} g_s g_Y^2 \mathcal{C}_{dG}^{sr} B_\mu^2 (\bar{q}_s H d_r) + \frac{2i}{3} g_s g_Y \bar{\mathcal{C}}_{dG}^{rs} B_\mu (\bar{d}_s \partial^\mu H^\dagger q_r) - \frac{2i}{3} g_s g_Y \mathcal{C}_{dG}^{sr} B_\mu (\bar{q}_s \partial^\mu H d_r) \\
& + \frac{2}{3} g_s \left[ y_d^{st} \bar{\mathcal{C}}_{dG}^{rt} - \bar{y}_d^{rt} \mathcal{C}_{dG}^{st} \right] \left[ g_L t_j^{Ii} H_i^\dagger (\bar{q}_s H \bar{W}^I q_r^j) - g_L t_k^{Ij} H^k (\bar{q}_{js} \bar{W}^I H^\dagger q_r) \right] \\
& + \frac{2}{3} g_s \left[ y_d^{rs} \bar{\mathcal{C}}_{dG}^{rs} - \bar{y}_d^{rs} \mathcal{C}_{dG}^{rs} \right] G_\mu^A G^{\mu\bar{\nu}A} (H^\dagger \partial_\nu H) + \frac{7}{9} g_s^3 \mathcal{C}_{dG}^{sr} T_b^{Aa} T_c^{Bb} G_\mu^A G_\mu^B (\bar{q}_{as} H d_r^c) \\
& + \frac{8}{9} g_L g_s \bar{\mathcal{C}}_{dG}^{rs} t_j^{Ii} W_\mu^I (\bar{d}_s \sigma^{\mu\bar{\nu}} q_r^j) \partial^\nu H_i^\dagger + \frac{8}{9} g_L g_s \mathcal{C}_{dG}^{sr} t_j^{Ii} W_\mu^I (\bar{q}_{is} \sigma^{\mu\bar{\nu}} d_r) \partial^\nu H^j \\
& - \frac{2}{9} g_s^2 \mathcal{C}_{dG}^{sr} T_b^{Aa} G_\mu^A (\bar{q}_{as} \partial^\nu H \sigma^{\mu\bar{\nu}} d_r^b) - \frac{4}{9} g_L^2 g_s \mathcal{C}_{dG}^{sr} \varepsilon^{IJK} t_j^{Ki} H^j W_\mu^J W_\nu^I (\bar{q}_{is} \sigma^{\mu\bar{\nu}} d_r) \\
& - \frac{i}{2} \left[ \bar{y}_d^{rt} \mathcal{C}_{dG}^{st} + y_d^{st} \bar{\mathcal{C}}_{dG}^{rt} \right] \left[ g_s T_b^{Aa} T_c^{Bb} G_\mu^B G^{\mu\bar{\nu}A} (\bar{q}_{as} \gamma^\nu q_r^c) - g_s T_b^{Aa} T_a^{Bc} G_\mu^B G^{\mu\bar{\nu}A} (\bar{q}_{cs} \gamma^\nu q_r^b) \right]
\end{aligned}$$

$$\begin{aligned}
& -\frac{i}{2} \left[ \bar{y}_d^{rt} \mathcal{C}_{dG}^{st} - y_d^{st} \bar{\mathcal{C}}_{dG}^{rt} \right] \left[ g_s T_b^{Aa} T_c^{Bb} G_{\bar{\mu}}^B G^{\bar{\mu}\bar{\nu}A} (\bar{q}_{as} \gamma^{\bar{\nu}} q_r^c) + g_s T_b^{Aa} T_a^{Bc} G_{\bar{\mu}}^B G^{\bar{\mu}\bar{\nu}A} (\bar{q}_{cs} \gamma^{\bar{\nu}} q_r^b) \right] \\
& -\frac{2}{3} g_L g_s \left[ \bar{y}_d^{rt} \mathcal{C}_{dG}^{st} + y_d^{st} \bar{\mathcal{C}}_{dG}^{rt} \right] (H^\dagger t^I H) (\bar{q}_s \bar{W}^I q_r) - \frac{2}{3} g_L g_s \left[ \bar{y}_d^{rt} \mathcal{C}_{dG}^{st} + y_d^{st} \bar{\mathcal{C}}_{dG}^{rt} \right] (H^\dagger H) (\bar{q}_s t^I \bar{W}^I q_r) \\
& + i g_L g_s \left[ \bar{y}_d^{rs} \mathcal{C}_{dG}^{rs} - y_d^{rs} \bar{\mathcal{C}}_{dG}^{rs} \right] G_{\bar{\mu}}^A W_{\bar{\nu}}^I G^{\bar{\mu}\bar{\nu}A} (H^\dagger t^I H) + g_L g_s \left[ -\bar{y}_d^{rs} \mathcal{C}_{dG}^{rs} - y_d^{rs} \bar{\mathcal{C}}_{dG}^{rs} \right] G_{\bar{\mu}}^A W_{\bar{\nu}}^I \tilde{G}^{\bar{\mu}\bar{\nu}A} (H^\dagger t^I H) \\
& - g_L^2 g_s \bar{\mathcal{C}}_{dG}^{rs} W_{\bar{\mu}}^{I2} (\bar{d}_s H^\dagger q_r) \\
& - i \left[ \bar{y}_d^{ts} \mathcal{C}_{dG}^{tr} + y_d^{tr} \bar{\mathcal{C}}_{dG}^{ts} \right] \left[ g_s T_b^{Aa} T_c^{Bb} G_{\bar{\mu}}^B G^{\bar{\mu}\bar{\nu}A} (\bar{d}_{as} \gamma^{\bar{\nu}} d_r^c) - g_s T_b^{Aa} T_a^{Bc} G_{\bar{\mu}}^B G^{\bar{\mu}\bar{\nu}A} (\bar{d}_{cs} \gamma^{\bar{\nu}} d_r^b) \right] \\
& + i \left[ \bar{y}_d^{ts} \mathcal{C}_{dG}^{tr} - y_d^{tr} \bar{\mathcal{C}}_{dG}^{ts} \right] \left[ g_s T_b^{Aa} T_c^{Bb} G_{\bar{\mu}}^B G^{\bar{\mu}\bar{\nu}A} (\bar{d}_{as} \gamma^{\bar{\nu}} d_r^c) + g_s T_b^{Aa} T_a^{Bc} G_{\bar{\mu}}^B G^{\bar{\mu}\bar{\nu}A} (\bar{d}_{cs} \gamma^{\bar{\nu}} d_r^b) \right] \\
& - g_L^2 g_s \mathcal{C}_{dG}^{sr} W_{\bar{\mu}}^{I2} (\bar{q}_s H d_r) - \frac{11}{9} g_L g_s^2 \bar{\mathcal{C}}_{dG}^{rs} t_j^{Ii} T_b^{Aa} H_i^\dagger G_{\bar{\mu}}^A W_{\bar{\mu}}^I (\bar{d}_{as} q_r^{bj}) - \frac{11}{9} g_L g_s^2 \mathcal{C}_{dG}^{sr} t_j^{Ii} T_b^{Aa} H^j G_{\bar{\mu}}^A W_{\bar{\mu}}^I (\bar{q}_{ais} d_r^b) \\
& - \frac{4i}{3} g_L g_s \bar{\mathcal{C}}_{dG}^{rs} t_j^{Ii} H_i^\dagger W_{\bar{\mu}}^I (\bar{d}_s \partial^{\bar{\mu}} q_r^j) + \frac{4i}{3} g_L g_s \mathcal{C}_{dG}^{sr} t_j^{Ii} H^j W_{\bar{\mu}}^I (\partial^{\bar{\mu}} \bar{q}_{is} d_r) \\
& + \frac{4i}{3} g_L g_s \bar{\mathcal{C}}_{dG}^{rs} t_j^{Ii} W_{\bar{\mu}}^I (\bar{d}_s q_r^j) \partial^{\bar{\mu}} H_i^\dagger - \frac{4i}{3} g_L g_s \mathcal{C}_{dG}^{sr} t_j^{Ii} W_{\bar{\mu}}^I (\bar{q}_{is} d_r) \partial^{\bar{\mu}} H^j \\
& - \frac{52}{27} g_L g_s g_Y \bar{\mathcal{C}}_{dG}^{rs} t_j^{Ii} H_i^\dagger B_{\bar{\mu}} W_{\bar{\mu}}^I (\bar{d}_s q_r^j) - \frac{52}{27} g_L g_s g_Y \mathcal{C}_{dG}^{sr} t_j^{Ii} H^j B_{\bar{\mu}} W_{\bar{\mu}}^I (\bar{q}_{is} d_r), \tag{2.28}
\end{aligned}$$

$$\begin{aligned}
\Delta S_{\mathcal{O}_{He}} &= \frac{1}{12} g_Y \mathcal{C}_{He}^{tt} \left[ 3g_L^2 - g_Y^2 \right] (H^\dagger H) (\bar{q}_s \bar{\mathcal{B}} q_s) + \frac{1}{6} g_Y^3 \mathcal{C}_{He}^{tt} (H^\dagger H) (\bar{d}_s \bar{\mathcal{B}} d_s) - \frac{i}{6} g_Y \bar{y}_e^{rt} \mathcal{C}_{He}^{st} B_{\bar{\mu}} (\bar{e}_s H^\dagger \partial^{\bar{\mu}} \ell_r) \\
& + \frac{1}{6} g_Y^3 \left[ 3\mathcal{C}_{He}^{tt} \delta^{rs} - 10\mathcal{C}_{He}^{sr} \right] (H^\dagger H) (\bar{e}_s \bar{\mathcal{B}} e_r) + \frac{i}{6} g_Y y_e^{st} \mathcal{C}_{He}^{tr} B_{\bar{\mu}} (\bar{\ell}_s H \partial^{\bar{\mu}} e_r) \\
& - \frac{i}{6} g_Y \bar{y}_e^{rt} \mathcal{C}_{He}^{st} B_{\bar{\mu}} (\partial^{\bar{\mu}} \bar{e}_s H^\dagger \ell_r) + \frac{i}{6} g_Y y_e^{st} \mathcal{C}_{He}^{tr} B_{\bar{\mu}} (\partial^{\bar{\mu}} \bar{\ell}_s H e_r) + \frac{1}{4} g_Y \mathcal{C}_{He}^{tt} \left[ g_L^2 + g_Y^2 \right] (H^\dagger H) (\bar{\ell}_s \bar{\mathcal{B}} \ell_s) \\
& + \frac{i}{4} g_L^2 g_Y \mathcal{C}_{He}^{rr} (H^\dagger \bar{\partial}_{\bar{\mu}} H) B_{\bar{\mu}} W_{\bar{\mu}}^{I2} + \frac{1}{3} g_L^2 g_Y^2 \mathcal{C}_{He}^{rr} (H^\dagger H) B_{\bar{\mu}}^2 W_{\bar{\mu}}^{I2} \\
& + \frac{1}{3} g_L \left[ y_e^{tr} \bar{y}_e^{tu} \mathcal{C}_{He}^{su} + y_e^{tu} \bar{y}_e^{ts} \mathcal{C}_{He}^{ur} \right] (H^\dagger t^I H) (\bar{e}_s \bar{W}^I e_r) + \frac{1}{3} g_Y^2 \mathcal{C}_{He}^{rr} (H^\dagger \partial_{\bar{\mu}} H) B_{\bar{\mu}} \partial^{\bar{\nu}} B_{\bar{\nu}} \\
& + \frac{1}{3} g_Y^2 \mathcal{C}_{He}^{rr} (\partial_{\bar{\mu}} H^\dagger H) B_{\bar{\mu}} \partial^{\bar{\nu}} B_{\bar{\nu}} + \frac{1}{3} g_Y^2 \mathcal{C}_{He}^{rr} (H^\dagger H) B_{\bar{\mu}} \partial^{\bar{\mu}} \partial^{\bar{\nu}} B_{\bar{\nu}} + \frac{1}{2} g_L^2 g_Y^2 \mathcal{C}_{He}^{rr} (H^\dagger H) B_{\bar{\mu}} B_{\bar{\nu}} W_{\bar{\mu}}^I W_{\bar{\nu}}^I \\
& + \frac{2}{3} g_L^2 y_e^{rt} \bar{y}_e^{rs} \mathcal{C}_{He}^{ts} (H^\dagger t^I H) (H^\dagger t^J H) W_{\bar{\mu}}^I W_{\bar{\mu}}^J + g_Y^2 \left[ \frac{7}{6} y_e^{rt} \bar{y}_e^{rs} \mathcal{C}_{He}^{ts} - \frac{1}{4} \mathcal{C}_{He}^{rr} \left[ g_L^2 + g_Y^2 \right] \right] (H^\dagger H)^2 B_{\bar{\mu}}^2 \\
& + g_L g_Y \mathcal{C}_{He}^{rr} (\partial_{\bar{\mu}} H^\dagger t^I \partial_{\bar{\nu}} H) B_{\bar{\mu}} W_{\bar{\nu}}^I + g_L g_Y \mathcal{C}_{He}^{rr} (\partial_{\bar{\nu}} H^\dagger t^I \partial_{\bar{\mu}} H) B_{\bar{\mu}} W_{\bar{\nu}}^I + \frac{4}{3} g_Y^2 \mathcal{C}_{He}^{rr} (\partial_{\bar{\nu}} H^\dagger \partial_{\bar{\nu}} H) B_{\bar{\mu}}^2 \\
& + \frac{5}{3} g_Y^2 \mathcal{C}_{He}^{rr} (\partial_{\bar{\mu}} H^\dagger \partial_{\bar{\nu}} H) B_{\bar{\mu}} B_{\bar{\nu}} + 2g_L g_Y \mathcal{C}_{He}^{rr} (\partial_{\bar{\nu}} H^\dagger t^I \partial_{\bar{\nu}} H) B_{\bar{\mu}} W_{\bar{\mu}}^I - \frac{1}{6} g_Y^2 \mathcal{C}_{He}^{rr} (H^\dagger \partial_{\bar{\mu}} \partial_{\bar{\nu}} H) B_{\bar{\mu}} B_{\bar{\nu}} \\
& - \frac{1}{6} g_Y \mathcal{C}_{He}^{rr} \left[ g_Y B_{\bar{\mu}} B^{\bar{\mu}\bar{\nu}} (H^\dagger \partial_{\bar{\nu}} H) + g_Y B_{\bar{\mu}} B^{\bar{\mu}\bar{\nu}} (\partial_{\bar{\nu}} H^\dagger H) \right] - \frac{1}{6} g_Y^2 \mathcal{C}_{He}^{rr} (\partial_{\bar{\mu}} \partial_{\bar{\nu}} H^\dagger H) B_{\bar{\mu}} B_{\bar{\nu}} \\
& - \frac{1}{4} g_Y^2 \bar{y}_e^{rt} \mathcal{C}_{He}^{st} B_{\bar{\mu}}^2 (\bar{e}_s H^\dagger \ell_r) + \frac{i}{3} y_e^{rt} \bar{y}_e^{rs} \mathcal{C}_{He}^{ts} \left[ g_L (H^\dagger \partial_{\bar{\mu}} H) (H^\dagger t^I H) W_{\bar{\mu}}^I - g_L (\partial_{\bar{\mu}} H^\dagger H) (H^\dagger t^I H) W_{\bar{\mu}}^I \right] \\
& + \frac{1}{2} g_L^3 g_Y \mathcal{C}_{He}^{rr} (H^\dagger t^I H) B_{\bar{\mu}} W_{\bar{\mu}}^I W_{\bar{\mu}}^{I2} - \frac{1}{3} g_Y^3 \mathcal{C}_{He}^{tt} (H^\dagger H) (\bar{u}_s \bar{\mathcal{B}} u_s) + \frac{i}{3} g_Y \mathcal{C}_{He}^{rr} \partial^{\bar{\mu}} \partial^{\bar{\nu}} B_{\bar{\nu}} (H^\dagger \bar{\partial}_{\bar{\mu}} H) \\
& - \frac{1}{2} g_L^2 g_Y \mathcal{C}_{He}^{tt} (\bar{\ell}_s H \bar{\mathcal{B}} H^\dagger \ell_s) - \frac{1}{2} g_L^2 g_Y \mathcal{C}_{He}^{tt} (\bar{q}_s H \bar{\mathcal{B}} H^\dagger q_s) + \frac{i}{2} g_L^2 g_Y \mathcal{C}_{He}^{rr} (H^\dagger \bar{\partial}_{\bar{\nu}} H) B_{\bar{\mu}} W_{\bar{\mu}}^I W_{\bar{\nu}}^I
\end{aligned}$$

$$\begin{aligned}
& + \frac{7i}{12} g_Y^3 C_{He}^{rr} (H^\dagger \overset{\leftrightarrow}{\partial}_\mu H) B_\mu B_\mu^2 + \frac{2i}{3} g_Y C_{He}^{rr} \left[ 2g_Y B_\mu \tilde{B}^{\mu\sigma} (H^\dagger \partial_\sigma H) - 2g_Y B_\mu \tilde{B}^{\mu\sigma} (\partial_\sigma H^\dagger H) \right] \\
& + \frac{2i}{3} g_Y \bar{y}_e^{rt} C_{He}^{st} B_\mu (\bar{e}_s \partial^\mu H^\dagger \ell_r) - \frac{2i}{3} g_Y y_e^{st} C_{He}^{tr} B_\mu (\bar{\ell}_s \partial^\mu H e_r) + \frac{2}{3} g_L g_Y C_{He}^{rr} (H^\dagger t^I H) W_\mu^I \partial^\mu \partial^\nu B_\nu \\
& + \frac{5}{6} g_Y \bar{y}_e^{rt} C_{He}^{st} B_\mu (\bar{e}_s \sigma^{\mu\nu} \partial^\nu H^\dagger \ell_r) + \frac{5}{6} g_Y y_e^{st} C_{He}^{tr} B_\mu (\bar{\ell}_s \partial^\nu H \sigma^{\mu\nu} e_r) \\
& + g_L g_Y C_{He}^{rr} (H^\dagger t^I \partial_\nu H) B_\mu \partial^\nu W_\mu^I + g_L g_Y C_{He}^{rr} (\partial_\nu H^\dagger t^I H) B_\mu \partial^\nu W_\mu^I \\
& + g_Y \left[ -\frac{i}{4} C_{He}^{rr} [g_L^2 + g_Y^2] + \frac{7i}{6} y_e^{rt} \bar{y}_e^{rs} C_{He}^{ts} \right] (H^\dagger \overset{\leftrightarrow}{\partial}_\mu H) (H^\dagger H) B_\mu + \frac{7}{6} g_Y^2 C_{He}^{rr} (H^\dagger \partial_\nu H) B_\mu \partial^\nu B_\mu \\
& + \frac{7}{6} g_Y^2 C_{He}^{rr} (\partial_\nu H^\dagger H) B_\mu \partial^\nu B_\mu - \frac{1}{4} g_Y^2 y_e^{st} C_{He}^{tr} B_\mu^2 (\bar{\ell}_s H e_r) - \frac{5}{6} g_L g_Y \bar{y}_e^{rt} C_{He}^{st} t_j^{Ii} H_i^\dagger B_\mu W_\mu^I (\bar{e}_s \ell_r^j) \\
& + \frac{5i}{6} g_L g_Y \bar{y}_e^{rt} C_{He}^{st} t_j^{Ii} H_i^\dagger B_\mu W_\mu^I (\bar{e}_s \sigma^{\mu\nu} \ell_r^j) - \frac{5}{6} g_L g_Y y_e^{st} C_{He}^{tr} t_j^{Ii} H^j B_\mu W_\mu^I (\bar{\ell}_{is} e_r) \\
& - \frac{5i}{6} g_L g_Y y_e^{st} C_{He}^{tr} t_j^{Ii} H^j B_\mu W_\mu^I (\bar{\ell}_{is} \sigma^{\mu\nu} e_r) + i C_{He}^{rr} \left[ g_Y (\partial_\nu H^\dagger \partial_\mu \partial_\nu H) B_\mu - g_Y (\partial_\mu \partial_\nu H^\dagger \partial_\nu H) B_\mu \right] \\
& + g_L g_Y \left[ \frac{8}{3} y_e^{rt} \bar{y}_e^{rs} C_{He}^{ts} - \frac{1}{2} C_{He}^{rr} [g_L^2 + g_Y^2] \right] (H^\dagger H) (H^\dagger t^I H) B_\mu W_\mu^I + \frac{7}{6} g_L g_Y^3 C_{He}^{rr} (H^\dagger t^I H) B_\mu B_\mu^2 W_\mu^I \\
& + \frac{8}{3} g_L g_Y^2 C_{He}^{rr} B_\mu W_\nu^I \tilde{B}^{\mu\nu} (H^\dagger t^I H) - g_L g_Y C_{He}^{rr} (H^\dagger t^I \partial_\mu \partial_\nu H) B_\mu W_\nu^I \\
& - g_L C_{He}^{rr} \left[ g_Y B_\mu W^{\mu\nu I} (H^\dagger t^I \partial_\nu H) + g_Y B_\mu W^{\mu\nu I} (\partial_\nu H^\dagger t^I H) \right] - g_L g_Y C_{He}^{rr} (\partial_\mu \partial_\nu H^\dagger t^I H) B_\mu W_\nu^I \\
& - g_L^2 g_Y C_{He}^{rr} \varepsilon^{IJK} B_\mu W_\nu^J W^{\mu\nu I} (H^\dagger t^K H) - g_L^2 g_Y C_{He}^{rr} \varepsilon^{IJK} (H^\dagger t^K H) B_\mu W_\nu^I \partial^\nu W_\mu^J \\
& + \frac{4i}{3} g_L g_Y^2 C_{He}^{rr} (H^\dagger t^I \overset{\leftrightarrow}{\partial}_\nu H) B_\mu^2 W_\nu^I + 2i g_L g_Y^2 C_{He}^{rr} (H^\dagger t^I \overset{\leftrightarrow}{\partial}_\nu H) B_\mu B_\nu W_\mu^I, \tag{2.29}
\end{aligned}$$

$$\begin{aligned}
\Delta S_{\mathcal{O}_{He}^{(1)}} & = \frac{1}{24} g_L^4 (C_{He}^{(1)})^{rr} (H^\dagger H) W_\mu^I{}^2 W_\mu^I{}^2 - \frac{i}{12} g_Y \bar{y}_e^{ts} (C_{He}^{(1)})^{tr} B_\mu (\bar{e}_s H^\dagger \partial^\mu \ell_r) + \frac{i}{12} g_Y y_e^{tr} (C_{He}^{(1)})^{st} B_\mu (\bar{\ell}_s H \partial^\mu e_r) \\
& + \frac{1}{12} g_L \left[ y_e^{su} \bar{y}_e^{tu} (C_{He}^{(1)})^{tr} + y_e^{ut} \bar{y}_e^{rt} (C_{He}^{(1)})^{su} - 10 g_L^2 (C_{He}^{(1)})^{sr} \right] (H^\dagger t^I H) (\bar{\ell}_s \bar{W}^I \ell_r) \\
& + \frac{1}{12} g_L \left[ y_e^{su} \bar{y}_e^{tu} (C_{He}^{(1)})^{tr} + y_e^{ut} \bar{y}_e^{rt} (C_{He}^{(1)})^{su} + 10 g_Y^2 (C_{He}^{(1)})^{sr} \right] (H^\dagger H) (\bar{\ell}_s t^I \bar{W}^I \ell_r) \\
& + \frac{1}{12} g_Y \left[ 3 y_e^{su} \bar{y}_e^{tu} (C_{He}^{(1)})^{tr} + 3 y_e^{ut} \bar{y}_e^{rt} (C_{He}^{(1)})^{su} + 10 g_L^2 (C_{He}^{(1)})^{sr} - 6 g_L^2 (C_{He}^{(1)})^{tt} \delta^{rs} \right] (\bar{\ell}_s H \bar{B} H^\dagger \ell_r) \\
& + \frac{1}{12} \left[ y_e^{su} \bar{y}_e^{tu} (C_{He}^{(1)})^{tr} - y_e^{ut} \bar{y}_e^{rt} (C_{He}^{(1)})^{su} \right] \left[ g_L t_j^{Ii} H_i^\dagger (\bar{\ell}_s H \bar{W}^I \ell_r^j) - g_L t_k^{Ij} H^k (\bar{\ell}_{js} \bar{W}^I H^\dagger \ell_r) \right] \\
& + \frac{1}{12} g_Y (C_{He}^{(1)})^{tt} \left[ 3 g_L^2 - g_Y^2 \right] (H^\dagger H) (\bar{q}_s \bar{B} q_s) - \frac{i}{12} g_Y \bar{y}_e^{ts} (C_{He}^{(1)})^{tr} B_\mu (\partial^\mu \bar{e}_s H^\dagger \ell_r) \\
& + \frac{i}{12} g_Y y_e^{tr} (C_{He}^{(1)})^{st} B_\mu (\partial^\mu \bar{\ell}_s H e_r) - \frac{i}{12} g_Y \left[ 3 (C_{He}^{(1)})^{rr} [g_L^2 + g_Y^2] - 4 y_e^{ts} \bar{y}_e^{rs} (C_{He}^{(1)})^{rt} \right] (H^\dagger \overset{\leftrightarrow}{\partial}_\mu H) (H^\dagger H) B_\mu \\
& + \frac{i}{12} g_L^3 (C_{He}^{(1)})^{rr} \varepsilon^{IJK} W_\mu^I W_\nu^J W_\rho^K \varepsilon^{\mu\nu\rho\sigma} (H^\dagger \overset{\leftrightarrow}{\partial}_\sigma H) + \frac{1}{6} g_L^2 (C_{He}^{(1)})^{rr} (H^\dagger \partial_\mu \partial_\nu H) W_\mu^I W_\nu^I \\
& + \frac{1}{6} g_L (C_{He}^{(1)})^{rr} \left[ g_L W_\mu^I W^{\mu\nu I} (H^\dagger \partial_\nu H) + g_L W_\mu^I W^{\mu\nu I} (\partial_\nu H^\dagger H) \right] + \frac{1}{6} g_L^2 (C_{He}^{(1)})^{rr} (\partial_\nu H^\dagger \partial_\nu H) W_\mu^I{}^2 \\
& + \frac{1}{6} g_L^2 (C_{He}^{(1)})^{rr} (\partial_\mu \partial_\nu H^\dagger H) W_\mu^I W_\nu^I + \frac{1}{6} g_L g_Y \left[ -3 (C_{He}^{(1)})^{rr} [g_L^2 + g_Y^2] - 4 y_e^{ts} \bar{y}_e^{rs} (C_{He}^{(1)})^{rt} \right] (H^\dagger H) (H^\dagger t^I H) B_\mu W_\mu^I \\
& - \frac{i}{6} g_Y (C_{He}^{(1)})^{rr} \left[ 2 g_L W_\mu^I \tilde{B}^{\mu\sigma} (H^\dagger t^I \partial_\sigma H) - 2 g_L W_\mu^I \tilde{B}^{\mu\sigma} (\partial_\sigma H^\dagger t^I H) \right]
\end{aligned}$$

$$\begin{aligned}
& + \frac{i}{6} g_L (\mathcal{C}_{H\ell}^{(1)})^{rr} \left[ 2g_Y B_{\bar{\mu}} \widetilde{W}^{\bar{\mu}\bar{\sigma}I} (H^\dagger t^I \partial_{\bar{\sigma}} H) - 2g_Y B_{\bar{\mu}} \widetilde{W}^{\bar{\mu}\bar{\sigma}I} (\partial_{\bar{\sigma}} H^\dagger t^I H) \right] \\
& + \frac{1}{6} g_L (\mathcal{C}_{H\ell}^{(1)})^{rr} \left[ 2g_L \varepsilon^{IJK} W_{\bar{\mu}}^J \widetilde{W}^{\bar{\mu}\bar{\sigma}I} (H^\dagger t^K \partial_{\bar{\sigma}} H) + 2g_L \varepsilon^{IJK} W_{\bar{\mu}}^J \widetilde{W}^{\bar{\mu}\bar{\sigma}I} (\partial_{\bar{\sigma}} H^\dagger t^K H) \right] \\
& + \frac{1}{6} g_Y^3 (\mathcal{C}_{H\ell}^{(1)})^{tt} (H^\dagger H) (\bar{d}_s \bar{B} d_s) + \frac{1}{6} g_L g_Y \bar{y}_e^{ts} (\mathcal{C}_{H\ell}^{(1)})^{tr} t_j^{Ii} H_i^\dagger B_{\bar{\mu}} W_{\bar{\mu}}^I (\bar{e}_s \ell_r^j) + \frac{1}{6} g_L^2 \bar{y}_e^{ts} (\mathcal{C}_{H\ell}^{(1)})^{tr} W_{\bar{\mu}}^{I2} (\bar{e}_s H^\dagger \ell_r) \\
& + \frac{1}{6} g_L^2 y_e^{tr} (\mathcal{C}_{H\ell}^{(1)})^{st} W_{\bar{\mu}}^{I2} (\bar{\ell}_s H e_r) + \frac{1}{6} g_L g_Y y_e^{tr} (\mathcal{C}_{H\ell}^{(1)})^{st} t_j^{Ii} H^j B_{\bar{\mu}} W_{\bar{\mu}}^I (\bar{\ell}_{is} e_r) + \frac{1}{6} g_Y^2 (\mathcal{C}_{H\ell}^{(1)})^{rr} (H^\dagger \partial_{\bar{\mu}} H) B_{\bar{\mu}} \partial^{\bar{\nu}} B_{\bar{\nu}} \\
& + \frac{1}{6} g_Y^2 (\mathcal{C}_{H\ell}^{(1)})^{rr} (\partial_{\bar{\mu}} H^\dagger H) B_{\bar{\mu}} \partial^{\bar{\nu}} B_{\bar{\nu}} + \frac{1}{6} g_L^2 (\mathcal{C}_{H\ell}^{(1)})^{rr} (H^\dagger \partial_{\bar{\mu}} H) W_{\bar{\mu}}^I \partial^{\bar{\nu}} W_{\bar{\nu}}^I \\
& + \frac{1}{6} g_L^2 (\mathcal{C}_{H\ell}^{(1)})^{rr} (\partial_{\bar{\mu}} H^\dagger H) W_{\bar{\mu}}^I \partial^{\bar{\nu}} W_{\bar{\nu}}^I + \frac{5}{24} g_Y^4 (\mathcal{C}_{H\ell}^{(1)})^{rr} (H^\dagger H) B_{\bar{\mu}}^2 B_{\bar{\mu}}^2 + \frac{1}{4} g_L^2 g_Y^2 (\mathcal{C}_{H\ell}^{(1)})^{rr} (H^\dagger H) B_{\bar{\mu}}^2 W_{\bar{\mu}}^{I2} \\
& + \frac{1}{3} g_L^2 g_Y^2 (\mathcal{C}_{H\ell}^{(1)})^{rr} (H^\dagger H) B_{\bar{\mu}} B_{\bar{\nu}} W_{\bar{\mu}}^I W_{\bar{\nu}}^I + \frac{1}{3} g_L^2 (\mathcal{C}_{H\ell}^{(1)})^{rr} (\partial_{\bar{\mu}} H^\dagger \partial_{\bar{\nu}} H) W_{\bar{\mu}}^I W_{\bar{\nu}}^I \\
& - \frac{1}{12} g_Y \left[ g_L^2 + g_Y^2 \right] \left[ 5(\mathcal{C}_{H\ell}^{(1)})^{sr} - 3(\mathcal{C}_{H\ell}^{(1)})^{tt} \delta^{rs} \right] (H^\dagger H) (\bar{\ell}_s \bar{B} \ell_r) - \frac{i}{6} g_L y_e^{tr} (\mathcal{C}_{H\ell}^{(1)})^{st} t_j^{Ii} H^j W_{\bar{\mu}}^I (\bar{\ell}_{is} \partial^{\bar{\mu}} e_r) \\
& + \frac{i}{6} g_L \bar{y}_e^{ts} (\mathcal{C}_{H\ell}^{(1)})^{tr} t_j^{Ii} H_i^\dagger W_{\bar{\mu}}^I (\partial^{\bar{\mu}} \bar{e}_s \ell_r^j) - \frac{i}{6} g_L y_e^{tr} (\mathcal{C}_{H\ell}^{(1)})^{st} t_j^{Ii} H^j W_{\bar{\mu}}^I (\partial^{\bar{\mu}} \bar{\ell}_{is} e_r) \\
& + \frac{i}{6} g_L^3 (\mathcal{C}_{H\ell}^{(1)})^{rr} (H^\dagger t^I \partial_{\bar{\mu}}^{\leftrightarrow} H) W_{\bar{\mu}}^I W_{\bar{\mu}}^{I2} \\
& - \frac{i}{6} g_L^2 g_Y (\mathcal{C}_{H\ell}^{(1)})^{rr} \varepsilon^{IJK} B_{\bar{\mu}} W_{\bar{\nu}}^I W_{\bar{\rho}}^J \varepsilon^{\bar{\mu}\bar{\nu}\bar{\rho}\bar{\sigma}} (H^\dagger t^K \partial_{\bar{\sigma}}^{\leftrightarrow} H) - \frac{1}{4} g_Y^2 y_e^{tr} (\mathcal{C}_{H\ell}^{(1)})^{st} B_{\bar{\mu}}^2 (\bar{\ell}_s H e_r) \\
& + \frac{i}{4} g_L^2 g_Y (\mathcal{C}_{H\ell}^{(1)})^{rr} (H^\dagger \partial_{\bar{\mu}}^{\leftrightarrow} H) B_{\bar{\mu}} W_{\bar{\mu}}^{I2} \\
& - \frac{i}{3} g_Y (\mathcal{C}_{H\ell}^{(1)})^{rr} \left[ 2g_Y B_{\bar{\mu}} \widetilde{B}^{\bar{\mu}\bar{\sigma}} (H^\dagger \partial_{\bar{\sigma}} H) - 2g_Y B_{\bar{\mu}} \widetilde{B}^{\bar{\mu}\bar{\sigma}} (\partial_{\bar{\sigma}} H^\dagger H) \right] \\
& - \frac{i}{3} g_L (\mathcal{C}_{H\ell}^{(1)})^{rr} \left[ 2g_L W_{\bar{\mu}}^I \widetilde{W}^{\bar{\mu}\bar{\sigma}I} (H^\dagger \partial_{\bar{\sigma}} H) - 2g_L W_{\bar{\mu}}^I \widetilde{W}^{\bar{\mu}\bar{\sigma}I} (\partial_{\bar{\sigma}} H^\dagger H) \right] - \frac{i}{3} g_Y y_e^{tr} (\mathcal{C}_{H\ell}^{(1)})^{st} B_{\bar{\mu}} (\bar{\ell}_s \partial^{\bar{\mu}} H e_r) \\
& + \frac{1}{3} g_L^2 (\mathcal{C}_{H\ell}^{(1)})^{rr} (H^\dagger \partial_{\bar{\nu}} H) W_{\bar{\mu}}^I \partial^{\bar{\nu}} W_{\bar{\mu}}^I + \frac{1}{3} g_L^2 (\mathcal{C}_{H\ell}^{(1)})^{rr} (\partial_{\bar{\nu}} H^\dagger H) W_{\bar{\mu}}^I \partial^{\bar{\nu}} W_{\bar{\mu}}^I \\
& + \frac{1}{3} g_Y^2 (\mathcal{C}_{H\ell}^{(1)})^{rr} (H^\dagger H) B_{\bar{\mu}} \partial^{\bar{\mu}} \partial^{\bar{\nu}} B_{\bar{\nu}} + \frac{1}{2} g_L^3 g_Y (\mathcal{C}_{H\ell}^{(1)})^{rr} (H^\dagger t^I H) B_{\bar{\mu}} W_{\bar{\mu}}^I W_{\bar{\mu}}^{I2} \\
& + \frac{2}{3} g_L^2 g_Y (\mathcal{C}_{H\ell}^{(1)})^{rr} B_{\bar{\mu}} W_{\bar{\nu}}^I \widetilde{W}^{\bar{\mu}\bar{\nu}I} (H^\dagger H) + g_Y^2 \left[ \frac{1}{3} y_e^{ts} \bar{y}_e^{rs} (\mathcal{C}_{H\ell}^{(1)})^{rt} - \frac{1}{4} (\mathcal{C}_{H\ell}^{(1)})^{rr} \left[ g_L^2 + g_Y^2 \right] \right] (H^\dagger H)^2 B_{\bar{\mu}}^2 \\
& - \frac{1}{3} g_Y^3 (\mathcal{C}_{H\ell}^{(1)})^{tt} (H^\dagger H) (\bar{u}_s \bar{B} u_s) + \frac{i}{3} g_Y (\mathcal{C}_{H\ell}^{(1)})^{rr} \partial^{\bar{\mu}} \partial^{\bar{\nu}} B_{\bar{\nu}} (H^\dagger \partial_{\bar{\mu}}^{\leftrightarrow} H) \\
& + \frac{i}{3} g_L^2 g_Y (\mathcal{C}_{H\ell}^{(1)})^{rr} (H^\dagger \partial_{\bar{\nu}}^{\leftrightarrow} H) B_{\bar{\mu}} W_{\bar{\mu}}^I W_{\bar{\nu}}^I + \frac{2}{3} g_L g_Y (\mathcal{C}_{H\ell}^{(1)})^{rr} (H^\dagger t^I H) W_{\bar{\mu}}^I \partial^{\bar{\mu}} \partial^{\bar{\nu}} B_{\bar{\nu}} \\
& - \frac{5}{12} g_Y \bar{y}_e^{ts} (\mathcal{C}_{H\ell}^{(1)})^{tr} B_{\bar{\mu}} (\bar{e}_s \sigma^{\bar{\mu}\bar{\nu}} \partial^{\bar{\nu}} H^\dagger \ell_r) - \frac{5}{12} g_Y y_e^{tr} (\mathcal{C}_{H\ell}^{(1)})^{st} B_{\bar{\mu}} (\bar{\ell}_s \partial^{\bar{\nu}} H \sigma^{\bar{\mu}\bar{\nu}} e_r) \\
& - \frac{5}{12} g_L^2 y_e^{tr} (\mathcal{C}_{H\ell}^{(1)})^{st} \varepsilon^{IJK} t_j^{Ki} H^j W_{\bar{\mu}}^J W_{\bar{\nu}}^I (\bar{\ell}_{is} \sigma^{\bar{\mu}\bar{\nu}} e_r) - \frac{1}{2} g_L^2 g_Y (\mathcal{C}_{H\ell}^{(1)})^{tt} (\bar{q}_s H \bar{B} H^\dagger q_s) \\
& - \frac{2i}{3} g_L \bar{y}_e^{ts} (\mathcal{C}_{H\ell}^{(1)})^{tr} t_j^{Ii} W_{\bar{\mu}}^I (\bar{e}_s \ell_r^j) \partial^{\bar{\mu}} H_i^\dagger + \frac{2i}{3} g_L y_e^{tr} (\mathcal{C}_{H\ell}^{(1)})^{st} t_j^{Ii} W_{\bar{\mu}}^I (\bar{\ell}_{is} e_r) \partial^{\bar{\mu}} H^j \\
& + \frac{3i}{4} g_Y^3 (\mathcal{C}_{H\ell}^{(1)})^{rr} (H^\dagger \partial_{\bar{\mu}}^{\leftrightarrow} H) B_{\bar{\mu}} B_{\bar{\mu}}^2 + \frac{5i}{6} g_L g_Y y_e^{tr} (\mathcal{C}_{H\ell}^{(1)})^{st} t_j^{Ii} H^j B_{\bar{\mu}} W_{\bar{\nu}}^I (\bar{\ell}_{is} \sigma^{\bar{\mu}\bar{\nu}} e_r)
\end{aligned}$$

$$\begin{aligned}
& + \frac{5}{6} g_L \bar{y}_e^{ts} (\mathcal{C}_{H\ell}^{(1)})^{tr} t_j^I W_\mu^I (\bar{e}_s \sigma^{\bar{\mu}\bar{\nu}} \ell_r^j) \partial^{\bar{\nu}} H_i^\dagger + \frac{5}{6} g_Y^2 (\mathcal{C}_{H\ell}^{(1)})^{rr} (H^\dagger \partial_{\bar{\nu}} H) B_{\bar{\mu}} \partial^{\bar{\nu}} B_{\bar{\mu}} \\
& + \frac{5}{6} g_Y^2 (\mathcal{C}_{H\ell}^{(1)})^{rr} (\partial_{\bar{\nu}} H^\dagger H) B_{\bar{\mu}} \partial^{\bar{\nu}} B_{\bar{\mu}} + \frac{5}{6} g_L y_e^{tr} (\mathcal{C}_{H\ell}^{(1)})^{st} t_j^I W_\mu^I (\bar{\ell}_{is} \sigma^{\bar{\mu}\bar{\nu}} e_r) \partial^{\bar{\nu}} H^j \\
& + i (\mathcal{C}_{H\ell}^{(1)})^{rr} \left[ g_Y (\partial_{\bar{\nu}} H^\dagger \partial_{\bar{\mu}} \partial_{\bar{\nu}} H) B_{\bar{\mu}} - g_Y (\partial_{\bar{\mu}} \partial_{\bar{\nu}} H^\dagger \partial_{\bar{\nu}} H) B_{\bar{\mu}} \right] + g_L g_Y (\mathcal{C}_{H\ell}^{(1)})^{rr} (\partial_{\bar{\mu}} H^\dagger t^I \partial_{\bar{\nu}} H) B_{\bar{\mu}} W_\nu^I \\
& + g_L g_Y (\mathcal{C}_{H\ell}^{(1)})^{rr} (\partial_{\bar{\nu}} H^\dagger t^I \partial_{\bar{\mu}} H) B_{\bar{\mu}} W_\nu^I + g_L g_Y (\mathcal{C}_{H\ell}^{(1)})^{rr} (H^\dagger t^I \partial_{\bar{\nu}} H) B_{\bar{\mu}} \partial^{\bar{\nu}} W_\mu^I \\
& + g_L g_Y (\mathcal{C}_{H\ell}^{(1)})^{rr} (\partial_{\bar{\nu}} H^\dagger t^I H) B_{\bar{\mu}} \partial^{\bar{\nu}} W_\mu^I + \frac{7}{6} g_Y^2 (\mathcal{C}_{H\ell}^{(1)})^{rr} (\partial_{\bar{\nu}} H^\dagger \partial_{\bar{\nu}} H) B_{\bar{\mu}}^2 + \frac{4}{3} g_Y^2 (\mathcal{C}_{H\ell}^{(1)})^{rr} (\partial_{\bar{\mu}} H^\dagger \partial_{\bar{\nu}} H) B_{\bar{\mu}} B_{\bar{\nu}} \\
& + \frac{4}{3} g_L^3 (\mathcal{C}_{H\ell}^{(1)})^{rr} W_\mu^I W_\nu^J \widetilde{W}^{\bar{\mu}\bar{\nu}J} (H^\dagger t^I H) + \frac{3}{2} g_L g_Y^3 (\mathcal{C}_{H\ell}^{(1)})^{rr} (H^\dagger t^I H) B_{\bar{\mu}} B_{\bar{\mu}}^2 W_\mu^I \\
& + 2 g_L g_Y (\mathcal{C}_{H\ell}^{(1)})^{rr} (\partial_{\bar{\nu}} H^\dagger t^I \partial_{\bar{\nu}} H) B_{\bar{\mu}} W_\mu^I - \frac{1}{12} g_L^3 g_Y (\mathcal{C}_{H\ell}^{(1)})^{rr} \varepsilon^{IJK} (H^\dagger H) B_{\bar{\mu}} W_\nu^I W_\rho^J W_\sigma^K \varepsilon^{\bar{\mu}\bar{\nu}\bar{\rho}\bar{\sigma}} \\
& + \frac{i}{6} g_L \bar{y}_e^{ts} (\mathcal{C}_{H\ell}^{(1)})^{tr} t_j^I H_i^\dagger W_\mu^I (\bar{e}_s \partial^{\bar{\mu}} \ell_r^j) - \frac{1}{4} g_Y^2 \bar{y}_e^{ts} (\mathcal{C}_{H\ell}^{(1)})^{tr} B_{\bar{\mu}}^2 (\bar{e}_s H^\dagger \ell_r) \\
& - \frac{1}{3} g_Y^2 (\mathcal{C}_{H\ell}^{(1)})^{rr} (H^\dagger \partial_{\bar{\mu}} \partial_{\bar{\nu}} H) B_{\bar{\mu}} B_{\bar{\nu}} - \frac{1}{3} g_Y (\mathcal{C}_{H\ell}^{(1)})^{rr} \left[ g_Y B_{\bar{\mu}} B^{\bar{\mu}\bar{\nu}} (H^\dagger \partial_{\bar{\nu}} H) + g_Y B_{\bar{\mu}} B^{\bar{\mu}\bar{\nu}} (\partial_{\bar{\nu}} H^\dagger H) \right] \\
& - \frac{1}{3} g_Y^2 (\mathcal{C}_{H\ell}^{(1)})^{rr} (\partial_{\bar{\mu}} \partial_{\bar{\nu}} H^\dagger H) B_{\bar{\mu}} B_{\bar{\nu}} - \frac{1}{3} g_L^3 g_Y (\mathcal{C}_{H\ell}^{(1)})^{rr} (H^\dagger t^I H) B_{\bar{\mu}} W_\mu^J W_\nu^I W_\nu^J \\
& + \frac{i}{3} g_Y \bar{y}_e^{ts} (\mathcal{C}_{H\ell}^{(1)})^{tr} B_{\bar{\mu}} (\bar{e}_s \partial^{\bar{\mu}} H^\dagger \ell_r) + \frac{1}{2} g_Y^3 (\mathcal{C}_{H\ell}^{(1)})^{tt} (H^\dagger H) (\bar{e}_s \bar{B} e_s) \\
& - \frac{5}{12} g_L^2 \bar{y}_e^{ts} (\mathcal{C}_{H\ell}^{(1)})^{tr} \varepsilon^{IJK} t_j^K H_i^\dagger W_\mu^J W_\nu^I (\bar{e}_s \sigma^{\bar{\mu}\bar{\nu}} \ell_r^j) \\
& - \frac{2i}{3} g_L g_Y (\mathcal{C}_{H\ell}^{(1)})^{rr} (\partial_{\bar{\rho}} H^\dagger t^I \partial_{\bar{\sigma}} H) B_{\bar{\mu}} W_\nu^I \varepsilon^{\bar{\mu}\bar{\nu}\bar{\rho}\bar{\sigma}} - \frac{5i}{6} g_L g_Y \bar{y}_e^{ts} (\mathcal{C}_{H\ell}^{(1)})^{tr} t_j^I H_i^\dagger B_{\bar{\mu}} W_\nu^I (\bar{e}_s \sigma^{\bar{\mu}\bar{\nu}} \ell_r^j) \\
& - g_L g_Y (\mathcal{C}_{H\ell}^{(1)})^{rr} (H^\dagger t^I \partial_{\bar{\mu}} \partial_{\bar{\nu}} H) B_{\bar{\mu}} W_\nu^I - g_L (\mathcal{C}_{H\ell}^{(1)})^{rr} \left[ g_Y B_{\bar{\mu}} W^{\bar{\mu}\bar{\nu}I} (H^\dagger t^I \partial_{\bar{\nu}} H) + g_Y B_{\bar{\mu}} W^{\bar{\mu}\bar{\nu}I} (\partial_{\bar{\nu}} H^\dagger t^I H) \right] \\
& - g_L g_Y (\mathcal{C}_{H\ell}^{(1)})^{rr} (\partial_{\bar{\mu}} \partial_{\bar{\nu}} H^\dagger t^I H) B_{\bar{\mu}} W_\nu^I - g_L^2 g_Y (\mathcal{C}_{H\ell}^{(1)})^{rr} \varepsilon^{IJK} B_{\bar{\mu}} W_\nu^J W^{\bar{\mu}\bar{\nu}I} (H^\dagger t^K H) \\
& - g_L^2 g_Y (\mathcal{C}_{H\ell}^{(1)})^{rr} \varepsilon^{IJK} (H^\dagger t^K H) B_{\bar{\mu}} W_\nu^I \partial^{\bar{\nu}} W_\mu^J + \frac{7i}{6} g_L g_Y^2 (\mathcal{C}_{H\ell}^{(1)})^{rr} (H^\dagger t^I \overset{\leftrightarrow}{\partial}_{\bar{\nu}} H) B_{\bar{\mu}}^2 W_\nu^I \\
& - \frac{4}{3} g_L g_Y^2 (\mathcal{C}_{H\ell}^{(1)})^{rr} B_{\bar{\mu}} W_\nu^I \widetilde{B}^{\bar{\mu}\bar{\nu}} (H^\dagger t^I H) - \frac{4i}{3} y_e^{ts} \bar{y}_e^{rs} (\mathcal{C}_{H\ell}^{(1)})^{rt} \left[ g_L (H^\dagger \partial_{\bar{\mu}} H) (H^\dagger t^I H) W_\mu^I - g_L (\partial_{\bar{\mu}} H^\dagger H) (H^\dagger t^I H) W_\mu^I \right] \\
& + 2i g_L g_Y^2 (\mathcal{C}_{H\ell}^{(1)})^{rr} (H^\dagger t^I \overset{\leftrightarrow}{\partial}_{\bar{\nu}} H) B_{\bar{\mu}} B_{\bar{\nu}} W_\mu^I - \frac{8}{3} g_L^2 y_e^{ts} \bar{y}_e^{rs} (\mathcal{C}_{H\ell}^{(1)})^{rt} (H^\dagger t^I H) (H^\dagger t^J H) W_\mu^I W_\mu^J, \tag{2.30}
\end{aligned}$$

$$\begin{aligned}
\Delta S_{\mathcal{O}_{H\ell}^{(3)}} &= \frac{1}{24} g_L^4 (\mathcal{C}_{H\ell}^{(3)})^{rr} (H^\dagger H) W_\mu^I{}^2 W_\mu^I{}^2 \\
&+ \frac{1}{12} g_Y \left[ 5 (\mathcal{C}_{H\ell}^{(3)})^{sr} \left[ g_Y^2 + 3 g_L^2 \right] + 6 \left[ y_e^{su} \bar{y}_e^{tu} (\mathcal{C}_{H\ell}^{(3)})^{tr} + y_e^{ut} \bar{y}_e^{rt} (\mathcal{C}_{H\ell}^{(3)})^{su} \right] \right] (H^\dagger H) (\bar{\ell}_s \bar{B} \ell_r) \\
&+ \frac{1}{12} g_L \left[ 3 y_e^{su} \bar{y}_e^{tu} (\mathcal{C}_{H\ell}^{(3)})^{tr} + 3 y_e^{ut} \bar{y}_e^{rt} (\mathcal{C}_{H\ell}^{(3)})^{su} + 10 g_Y^2 (\mathcal{C}_{H\ell}^{(3)})^{sr} - 6 g_Y^2 (\mathcal{C}_{H\ell}^{(3)})^{tt} \delta^{rs} \right] (H^\dagger t^I H) (\bar{\ell}_s \bar{W}^I \ell_r) \\
&+ \frac{1}{12} g_L \left[ 6 g_L^2 (\mathcal{C}_{H\ell}^{(3)})^{tt} \delta^{rs} + 10 g_L^2 (\mathcal{C}_{H\ell}^{(3)})^{sr} - y_e^{su} \bar{y}_e^{tu} (\mathcal{C}_{H\ell}^{(3)})^{tr} - y_e^{ut} \bar{y}_e^{rt} (\mathcal{C}_{H\ell}^{(3)})^{su} \right] (H^\dagger H) (\bar{\ell}_s t^I \bar{W}^I \ell_r) \\
&+ \frac{1}{12} g_Y \left[ -3 \left[ y_e^{su} \bar{y}_e^{tu} (\mathcal{C}_{H\ell}^{(3)})^{tr} + y_e^{ut} \bar{y}_e^{rt} (\mathcal{C}_{H\ell}^{(3)})^{su} \right] - 10 g_Y^2 (\mathcal{C}_{H\ell}^{(3)})^{sr} \right] (\bar{\ell}_s H \bar{B} H^\dagger \ell_r) \\
&+ \frac{1}{12} \left[ y_e^{ut} \bar{y}_e^{rt} (\mathcal{C}_{H\ell}^{(3)})^{su} - y_e^{su} \bar{y}_e^{tu} (\mathcal{C}_{H\ell}^{(3)})^{tr} \right] \left[ g_L t_j^I H_i^\dagger (\bar{\ell}_s H \bar{W}^I \ell_r^j) - g_L t_k^I H^k (\bar{\ell}_{js} \bar{W}^I H^\dagger \ell_r) \right]
\end{aligned}$$

$$\begin{aligned}
& -\frac{i}{12}g_Y^3(\mathcal{C}_{H\ell}^{(3)})^{rr}(H^\dagger\overset{\leftrightarrow}{\partial}_\mu H)B_\mu B_\mu^2 + \frac{1}{6}g_Y^2(\mathcal{C}_{H\ell}^{(3)})^{rr}(H^\dagger\partial_\mu\partial_\nu H)B_\mu B_\nu \\
& + \frac{1}{6}g_Y(\mathcal{C}_{H\ell}^{(3)})^{rr}\left[g_Y B_\mu B^{\bar{\mu}\bar{\nu}}(H^\dagger\partial_\nu H) + g_Y B_\mu B^{\bar{\mu}\bar{\nu}}(\partial_\nu H^\dagger H)\right] + \frac{1}{6}g_Y^2(\mathcal{C}_{H\ell}^{(3)})^{rr}(\partial_\mu\partial_\nu H^\dagger H)B_\mu B_\nu \\
& + \frac{1}{6}g_L g_Y\left[3(\mathcal{C}_{H\ell}^{(3)})^{rr}\left[g_L^2 + g_Y^2\right] - 4y_e^{ts}\bar{y}_e^{rs}(\mathcal{C}_{H\ell}^{(3)})^{rt}\right](H^\dagger H)(H^\dagger t^I H)B_\mu W_\mu^I + \frac{i}{6}g_L y_e^{tr}(\mathcal{C}_{H\ell}^{(3)})^{st}t_j^{Ii}H^j W_\mu^I(\bar{\ell}_{is}\partial^\mu e_r) \\
& + \frac{1}{6}g_L g_Y^2(\mathcal{C}_{H\ell}^{(3)})^{tt}(H^\dagger t^I H)(\bar{q}_s\bar{W}^I q_s) - \frac{i}{6}g_L \bar{y}_e^{ts}(\mathcal{C}_{H\ell}^{(3)})^{tr}t_j^{Ii}H_i^\dagger W_\mu^I(\partial^\mu\bar{e}_s\ell_r^j) \\
& + \frac{i}{6}g_L y_e^{tr}(\mathcal{C}_{H\ell}^{(3)})^{st}t_j^{Ii}H^j W_\mu^I(\partial^\mu\bar{\ell}_{is}e_r) + \frac{1}{6}g_Y^2(\mathcal{C}_{H\ell}^{(3)})^{rr}(H^\dagger\partial_\mu H)B_\mu\partial^\nu B_\nu \\
& + \frac{1}{6}g_Y^2(\mathcal{C}_{H\ell}^{(3)})^{rr}(\partial_\mu H^\dagger H)B_\mu\partial^\nu B_\nu + \frac{1}{6}g_L^2(\mathcal{C}_{H\ell}^{(3)})^{rr}(H^\dagger\partial_\mu H)W_\mu^I\partial^\nu W_\nu^I \\
& + \frac{1}{6}g_L^2(\mathcal{C}_{H\ell}^{(3)})^{rr}(\partial_\mu H^\dagger H)W_\mu^I\partial^\nu W_\nu^I - \frac{i}{6}g_L^3(\mathcal{C}_{H\ell}^{(3)})^{rr}(H^\dagger t^I\overset{\leftrightarrow}{\partial}_\mu H)W_\mu^I W_\mu^{I2} \\
& + \frac{i}{6}g_L\left[3g_L^2(\mathcal{C}_{H\ell}^{(3)})^{rr} - 8y_e^{ts}\bar{y}_e^{rs}(\mathcal{C}_{H\ell}^{(3)})^{rt}\right](H^\dagger t^I\overset{\leftrightarrow}{\partial}_\mu H)(H^\dagger H)W_\mu^I + \frac{i}{4}g_Y y_e^{tr}(\mathcal{C}_{H\ell}^{(3)})^{st}B_\mu(\bar{\ell}_s H\partial^\mu e_r) \\
& - \frac{i}{4}g_Y \bar{y}_e^{ts}(\mathcal{C}_{H\ell}^{(3)})^{tr}B_\mu(\partial^\mu\bar{e}_s H^\dagger\ell_r) + \frac{i}{4}g_Y y_e^{tr}(\mathcal{C}_{H\ell}^{(3)})^{st}B_\mu(\partial^\mu\bar{\ell}_s H e_r) + \frac{1}{3}g_Y^2 y_e^{ts}\bar{y}_e^{rs}(\mathcal{C}_{H\ell}^{(3)})^{rt}(H^\dagger H)^2 B_\mu^2 \\
& + \frac{1}{3}g_Y^2(\mathcal{C}_{H\ell}^{(3)})^{rr}(\partial_\mu H^\dagger\partial_\nu H)B_\mu B_\nu + \frac{1}{3}g_Y(\mathcal{C}_{H\ell}^{(3)})^{rr}\left[g_L W_\mu^I B^{\bar{\mu}\bar{\nu}}(H^\dagger t^I\partial_\nu H) + g_L W_\mu^I B^{\bar{\mu}\bar{\nu}}(\partial_\nu H^\dagger t^I H)\right] \\
& + \frac{i}{3}g_Y y_e^{ts}\bar{y}_e^{rs}(\mathcal{C}_{H\ell}^{(3)})^{rt}(H^\dagger\overset{\leftrightarrow}{\partial}_\mu H)(H^\dagger H)B_\mu + \frac{5}{12}g_L^2 y_e^{tr}(\mathcal{C}_{H\ell}^{(3)})^{st}\varepsilon^{IJK}t_j^{Ki}H^j W_\mu^J W_\nu^I(\bar{\ell}_{is}\sigma^{\bar{\mu}\bar{\nu}}e_r) \\
& + \frac{1}{2}g_L^3(\mathcal{C}_{H\ell}^{(3)})^{tt}(H^\dagger H)(\bar{q}_s t^I\bar{W}^I q_s) + \frac{2}{3}g_L^2 g_Y(\mathcal{C}_{H\ell}^{(3)})^{rr}B_\mu W_\nu^I\widetilde{W}^{\bar{\mu}\bar{\nu}I}(H^\dagger H) \\
& + \frac{2}{3}g_L^2(\mathcal{C}_{H\ell}^{(3)})^{rr}(H^\dagger\partial_\mu\partial_\nu H)W_\mu^I W_\nu^I + \frac{2}{3}g_L(\mathcal{C}_{H\ell}^{(3)})^{rr}\left[g_L W_\mu^I W^{\bar{\mu}\bar{\nu}I}(H^\dagger\partial_\nu H) + g_L W_\mu^I W^{\bar{\mu}\bar{\nu}I}(\partial_\nu H^\dagger H)\right] \\
& + \frac{2}{3}g_L^2(\mathcal{C}_{H\ell}^{(3)})^{rr}(\partial_\mu\partial_\nu H^\dagger H)W_\mu^I W_\nu^I \\
& + \frac{2}{3}(\mathcal{C}_{H\ell}^{(3)})^{rr}\left[g_L^2 g_Y\varepsilon^{IJK}(H^\dagger t^K\partial_\nu H)B_\mu W_\mu^I W_\nu^J + g_L^2 g_Y\varepsilon^{IJK}(\partial_\nu H^\dagger t^K H)B_\mu W_\mu^I W_\nu^J\right] \\
& + \frac{2}{3}g_L g_Y^2(\mathcal{C}_{H\ell}^{(3)})^{tt}(H^\dagger t^I H)(\bar{u}_s\bar{W}^I u_s) + g_L^2\left[\frac{1}{4}g_L^2(\mathcal{C}_{H\ell}^{(3)})^{rr} - \frac{2}{3}y_e^{ts}\bar{y}_e^{rs}(\mathcal{C}_{H\ell}^{(3)})^{rt}\right](H^\dagger H)^2 W_\mu^{I2} \\
& + g_L^2 g_Y^2(\mathcal{C}_{H\ell}^{(3)})^{rr}(H^\dagger t^I H)(H^\dagger t^J H)W_\mu^I W_\mu^J - \frac{1}{24}g_Y^4(\mathcal{C}_{H\ell}^{(3)})^{rr}(H^\dagger H)B_\mu^2 B_\mu^2 \\
& - \frac{1}{12}g_L^3 g_Y(\mathcal{C}_{H\ell}^{(3)})^{rr}\varepsilon^{IJK}(H^\dagger H)B_\mu W_\nu^I W_\rho^J W_\sigma^K\varepsilon^{\bar{\mu}\bar{\nu}\bar{\rho}\bar{\sigma}} - \frac{1}{6}g_Y^2(\mathcal{C}_{H\ell}^{(3)})^{rr}(\partial_\nu H^\dagger\partial_\nu H)B_\mu^2 \\
& - \frac{1}{6}g_L g_Y^3(\mathcal{C}_{H\ell}^{(3)})^{rr}(H^\dagger t^I H)B_\mu B_\mu^2 W_\mu^I - \frac{1}{6}g_L^2 g_Y(\mathcal{C}_{H\ell}^{(3)})^{rr}\varepsilon^{IJK}W_\mu^J W_\nu^I B^{\bar{\mu}\bar{\nu}}(H^\dagger t^K H) \\
& - \frac{i}{6}g_L \bar{y}_e^{ts}(\mathcal{C}_{H\ell}^{(3)})^{tr}t_j^{Ii}H_i^\dagger W_\mu^I(\bar{e}_s\partial^\mu\ell_r^j) - \frac{1}{4}g_L^2 g_Y^2(\mathcal{C}_{H\ell}^{(3)})^{rr}(H^\dagger H)B_\mu^2 W_\mu^{I2} \\
& - \frac{1}{4}g_L^4(\mathcal{C}_{H\ell}^{(3)})^{rr}(H^\dagger H)W_\mu^I W_\mu^J W_\nu^I W_\nu^J - \frac{1}{4}g_L^3(\mathcal{C}_{H\ell}^{(3)})^{rr}\varepsilon^{IJK}W_\mu^K W_\nu^J W^{\bar{\mu}\bar{\nu}I}(H^\dagger H) \\
& - \frac{i}{4}g_Y \bar{y}_e^{ts}(\mathcal{C}_{H\ell}^{(3)})^{tr}B_\mu(\bar{e}_s H^\dagger\partial^\mu\ell_r) + \frac{5}{12}g_L^2 \bar{y}_e^{ts}(\mathcal{C}_{H\ell}^{(3)})^{tr}\varepsilon^{IJK}t_j^{Ki}H_i^\dagger W_\mu^J W_\nu^I(\bar{e}_s\sigma^{\bar{\mu}\bar{\nu}}\ell_r^j) \\
& - \frac{1}{3}g_L^2 g_Y^2(\mathcal{C}_{H\ell}^{(3)})^{rr}(H^\dagger H)B_\mu B_\nu W_\mu^I W_\nu^I - \frac{1}{3}g_L g_Y(\mathcal{C}_{H\ell}^{(3)})^{rr}(H^\dagger t^I\partial_\mu\partial_\nu H)B_\mu W_\nu^I
\end{aligned}$$

$$\begin{aligned}
& -\frac{1}{3}g_L g_Y (\mathcal{C}_{H\ell}^{(3)})^{rr} (\partial_{\bar{\mu}} \partial_{\bar{\nu}} H^\dagger t^I H) B_{\bar{\mu}} W_{\bar{\nu}}^I - \frac{1}{3}g_L g_Y^2 (\mathcal{C}_{H\ell}^{(3)})^{tt} (H^\dagger t^I H) (\bar{d}_s \bar{W}^I d_s) \\
& -\frac{1}{3}g_L^2 \bar{y}_e^{ts} (\mathcal{C}_{H\ell}^{(3)})^{tr} W_{\bar{\mu}}^{I2} (\bar{e}_s H^\dagger \ell_r) - \frac{1}{3}g_L^2 y_e^{tr} (\mathcal{C}_{H\ell}^{(3)})^{st} W_{\bar{\mu}}^{I2} (\bar{\ell}_s H e_r) \\
& -\frac{1}{3}g_L^2 g_Y (\mathcal{C}_{H\ell}^{(3)})^{rr} \varepsilon^{IJK} (H^\dagger t^K H) B_{\bar{\mu}} W_{\bar{\nu}}^J \partial^{\bar{\mu}} W_{\bar{\nu}}^I + \frac{i}{2}g_Y^2 (\mathcal{C}_{H\ell}^{(3)})^{rr} \left[ g_L (H^\dagger \partial_{\bar{\mu}} H) (H^\dagger t^I H) W_{\bar{\mu}}^I - g_L (\partial_{\bar{\mu}} H^\dagger H) (H^\dagger t^I H) W_{\bar{\mu}}^I \right] \\
& + \frac{i}{2}g_L (\mathcal{C}_{H\ell}^{(3)})^{rr} \left[ 2g_Y B_{\bar{\mu}} \widetilde{W}^{\bar{\mu}\bar{\sigma}I} (H^\dagger t^I \partial_{\bar{\sigma}} H) - 2g_Y B_{\bar{\mu}} \widetilde{W}^{\bar{\mu}\bar{\sigma}I} (\partial_{\bar{\sigma}} H^\dagger t^I H) \right] \\
& -\frac{1}{2}g_L^3 (\mathcal{C}_{H\ell}^{(3)})^{rr} \varepsilon^{IJK} (H^\dagger H) W_{\bar{\mu}}^J W_{\bar{\nu}}^I \partial^{\bar{\mu}} W_{\bar{\nu}}^K - \frac{1}{2}g_L^2 (\mathcal{C}_{H\ell}^{(3)})^{rr} (H^\dagger \partial_{\bar{\nu}} H) W_{\bar{\mu}}^I \partial^{\bar{\nu}} W_{\bar{\mu}}^I \\
& -\frac{1}{2}g_L^2 (\mathcal{C}_{H\ell}^{(3)})^{rr} (\partial_{\bar{\nu}} H^\dagger H) W_{\bar{\mu}}^I \partial^{\bar{\nu}} W_{\bar{\mu}}^I - \frac{i}{2}g_L g_Y^2 (\mathcal{C}_{H\ell}^{(3)})^{rr} (H^\dagger t^I \overset{\leftrightarrow}{\partial}_{\bar{\nu}} H) B_{\bar{\mu}}^2 W_{\bar{\nu}}^I \\
& -\frac{7i}{12}g_L^2 g_Y (\mathcal{C}_{H\ell}^{(3)})^{rr} (H^\dagger \overset{\leftrightarrow}{\partial}_{\bar{\mu}} H) B_{\bar{\mu}} W_{\bar{\mu}}^{I2} - \frac{2}{3}g_L^2 (\mathcal{C}_{H\ell}^{(3)})^{rr} (\partial_{\bar{\mu}} H^\dagger \partial_{\bar{\nu}} H) W_{\bar{\mu}}^I W_{\bar{\nu}}^I \\
& -\frac{2}{3}g_L^3 g_Y (\mathcal{C}_{H\ell}^{(3)})^{rr} (H^\dagger t^I H) B_{\bar{\mu}} W_{\bar{\mu}}^J W_{\bar{\nu}}^I W_{\bar{\nu}}^J - \frac{2}{3}g_L (\mathcal{C}_{H\ell}^{(3)})^{rr} \left[ g_Y B_{\bar{\mu}} W^{\bar{\mu}\bar{\nu}I} (H^\dagger t^I \partial_{\bar{\nu}} H) + g_Y B_{\bar{\mu}} W^{\bar{\mu}\bar{\nu}I} (\partial_{\bar{\nu}} H^\dagger t^I H) \right] \\
& + \frac{2i}{3}g_L g_Y (\mathcal{C}_{H\ell}^{(3)})^{rr} (\partial_{\bar{\rho}} H^\dagger t^I \partial_{\bar{\sigma}} H) B_{\bar{\mu}} W_{\bar{\nu}}^I \varepsilon^{\bar{\mu}\bar{\nu}\bar{\rho}\bar{\sigma}} + \frac{2i}{3}g_L \bar{y}_e^{ts} (\mathcal{C}_{H\ell}^{(3)})^{tr} t_j^{Ii} W_{\bar{\mu}}^I (\bar{e}_s \ell_r^j) \partial^{\bar{\mu}} H_i^\dagger \\
& -\frac{2i}{3}g_L y_e^{tr} (\mathcal{C}_{H\ell}^{(3)})^{st} t_j^{Ii} W_{\bar{\mu}}^I (\bar{\ell}_{is} e_r) \partial^{\bar{\mu}} H^j + \frac{2}{3}g_L^2 g_Y (\mathcal{C}_{H\ell}^{(3)})^{rr} \varepsilon^{IJK} (H^\dagger t^K H) B_{\bar{\mu}} W_{\bar{\mu}}^I \partial^{\bar{\nu}} W_{\bar{\nu}}^J \\
& -\frac{1}{3}g_L^2 (\mathcal{C}_{H\ell}^{(3)})^{rr} (H^\dagger H) W_{\bar{\mu}}^I \partial^{\bar{\mu}} \partial^{\bar{\nu}} W_{\bar{\nu}}^I - \frac{2}{3}g_L g_Y (\mathcal{C}_{H\ell}^{(3)})^{rr} (H^\dagger t^I \partial_{\bar{\mu}} H) W_{\bar{\mu}}^I \partial^{\bar{\nu}} B_{\bar{\nu}} \\
& -\frac{2}{3}g_L g_Y (\mathcal{C}_{H\ell}^{(3)})^{rr} (\partial_{\bar{\mu}} H^\dagger t^I H) W_{\bar{\mu}}^I \partial^{\bar{\nu}} B_{\bar{\nu}} - \frac{2}{3}g_L g_Y (\mathcal{C}_{H\ell}^{(3)})^{rr} (H^\dagger t^I \partial_{\bar{\nu}} H) B_{\bar{\mu}} \partial^{\bar{\nu}} W_{\bar{\mu}}^I \\
& -\frac{2}{3}g_L g_Y (\mathcal{C}_{H\ell}^{(3)})^{rr} (\partial_{\bar{\nu}} H^\dagger t^I H) B_{\bar{\mu}} \partial^{\bar{\nu}} W_{\bar{\mu}}^I - \frac{2}{3}g_L g_Y (\mathcal{C}_{H\ell}^{(3)})^{rr} (H^\dagger t^I \partial_{\bar{\mu}} H) B_{\bar{\mu}} \partial^{\bar{\nu}} W_{\bar{\nu}}^I \\
& -\frac{2}{3}g_L g_Y (\mathcal{C}_{H\ell}^{(3)})^{rr} (\partial_{\bar{\mu}} H^\dagger t^I H) B_{\bar{\mu}} \partial^{\bar{\nu}} W_{\bar{\nu}}^I - \frac{2}{3}g_L g_Y (\mathcal{C}_{H\ell}^{(3)})^{rr} (H^\dagger t^I H) B_{\bar{\mu}} \partial^{\bar{\mu}} \partial^{\bar{\nu}} W_{\bar{\nu}}^I \\
& -\frac{2i}{3}g_L (\mathcal{C}_{H\ell}^{(3)})^{rr} \partial^{\bar{\mu}} \partial^{\bar{\nu}} W_{\bar{\nu}}^I (H^\dagger t^I \overset{\leftrightarrow}{\partial}_{\bar{\mu}} H) - \frac{2i}{3}g_L g_Y^2 (\mathcal{C}_{H\ell}^{(3)})^{rr} (H^\dagger t^I \overset{\leftrightarrow}{\partial}_{\bar{\nu}} H) B_{\bar{\mu}} B_{\bar{\nu}} W_{\bar{\mu}}^I \\
& + \frac{2i}{3}g_L^2 (\mathcal{C}_{H\ell}^{(3)})^{rr} \varepsilon^{IJK} W_{\bar{\mu}}^J W^{\bar{\mu}\bar{\nu}I} (H^\dagger t^K \overset{\leftrightarrow}{\partial}_{\bar{\nu}} H) - \frac{3}{4}g_Y^2 \bar{y}_e^{ts} (\mathcal{C}_{H\ell}^{(3)})^{tr} B_{\bar{\mu}}^2 (\bar{e}_s H^\dagger \ell_r) \\
& -\frac{3}{4}g_Y^2 y_e^{tr} (\mathcal{C}_{H\ell}^{(3)})^{st} B_{\bar{\mu}}^2 (\bar{\ell}_s H e_r) - \frac{5}{6}g_L^3 g_Y (\mathcal{C}_{H\ell}^{(3)})^{rr} (H^\dagger t^I H) B_{\bar{\mu}} W_{\bar{\mu}}^I W_{\bar{\mu}}^{I2} \\
& + \frac{5i}{6}g_Y (\mathcal{C}_{H\ell}^{(3)})^{rr} \left[ 2g_L W_{\bar{\mu}}^I \widetilde{B}^{\bar{\mu}\bar{\sigma}} (H^\dagger t^I \partial_{\bar{\sigma}} H) - 2g_L W_{\bar{\mu}}^I \widetilde{B}^{\bar{\mu}\bar{\sigma}} (\partial_{\bar{\sigma}} H^\dagger t^I H) \right] \\
& -\frac{5i}{6}g_L g_Y \bar{y}_e^{ts} (\mathcal{C}_{H\ell}^{(3)})^{tr} t_j^{Ii} H_i^\dagger B_{\bar{\mu}} W_{\bar{\nu}}^I (\bar{e}_s \sigma^{\bar{\mu}\bar{\nu}} \ell_r^j) + \frac{5i}{6}g_L g_Y y_e^{tr} (\mathcal{C}_{H\ell}^{(3)})^{st} t_j^{Ii} H^j B_{\bar{\mu}} W_{\bar{\nu}}^I (\bar{\ell}_{is} \sigma^{\bar{\mu}\bar{\nu}} e_r) \\
& -\frac{5}{6}g_L \bar{y}_e^{ts} (\mathcal{C}_{H\ell}^{(3)})^{tr} t_j^{Ii} W_{\bar{\mu}}^I (\bar{e}_s \sigma^{\bar{\mu}\bar{\nu}} \ell_r^j) \partial^{\bar{\nu}} H_i^\dagger - \frac{5}{6}g_L y_e^{tr} (\mathcal{C}_{H\ell}^{(3)})^{st} t_j^{Ii} W_{\bar{\mu}}^I (\bar{\ell}_{is} \sigma^{\bar{\mu}\bar{\nu}} e_r) \partial^{\bar{\nu}} H^j \\
& + ig_L^2 (\mathcal{C}_{H\ell}^{(3)})^{rr} \varepsilon^{IJK} (H^\dagger t^K \partial_{\bar{\mu}} \partial_{\bar{\nu}} H) W_{\bar{\mu}}^I W_{\bar{\nu}}^J - ig_L^2 (\mathcal{C}_{H\ell}^{(3)})^{rr} \varepsilon^{IJK} (\partial_{\bar{\mu}} \partial_{\bar{\nu}} H^\dagger t^K H) W_{\bar{\mu}}^I W_{\bar{\nu}}^J \\
& + ig_Y \bar{y}_e^{ts} (\mathcal{C}_{H\ell}^{(3)})^{tr} B_{\bar{\mu}} (\bar{e}_s \partial^{\bar{\mu}} H^\dagger \ell_r) - g_L g_Y^2 (\mathcal{C}_{H\ell}^{(3)})^{tt} (H^\dagger t^I H) (\bar{e}_s \bar{W}^I e_s) - ig_Y y_e^{tr} (\mathcal{C}_{H\ell}^{(3)})^{st} B_{\bar{\mu}} (\bar{\ell}_s \partial^{\bar{\mu}} H e_r) \\
& + ig_L^2 (\mathcal{C}_{H\ell}^{(3)})^{rr} \varepsilon^{IJK} (H^\dagger t^K \partial_{\bar{\nu}} H) W_{\bar{\mu}}^I \partial^{\bar{\nu}} W_{\bar{\mu}}^J - ig_L^2 (\mathcal{C}_{H\ell}^{(3)})^{rr} \varepsilon^{IJK} (\partial_{\bar{\nu}} H^\dagger t^K H) W_{\bar{\mu}}^I \partial^{\bar{\nu}} W_{\bar{\mu}}^J \\
& - ig_L^2 g_Y (\mathcal{C}_{H\ell}^{(3)})^{rr} (H^\dagger \overset{\leftrightarrow}{\partial}_{\bar{\nu}} H) B_{\bar{\mu}} W_{\bar{\mu}}^I W_{\bar{\nu}}^I - \frac{7}{6}g_L^2 (\mathcal{C}_{H\ell}^{(3)})^{rr} (\partial_{\bar{\nu}} H^\dagger \partial_{\bar{\nu}} H) W_{\bar{\mu}}^{I2}
\end{aligned}$$

$$\begin{aligned}
& -\frac{5}{4}g_Y\bar{y}_e^{ts}(\mathcal{C}_{H\ell}^{(3)})^{tr}B_{\bar{\mu}}(\bar{e}_s\sigma^{\bar{\mu}\bar{\nu}}\partial^{\bar{\nu}}H^\dagger\ell_r)-\frac{5}{4}g_Yy_e^{tr}(\mathcal{C}_{H\ell}^{(3)})^{st}B_{\bar{\mu}}(\bar{\ell}_s\partial^{\bar{\nu}}H\sigma^{\bar{\mu}\bar{\nu}}e_r) \\
& -\frac{4}{3}g_Lg_Y^2(\mathcal{C}_{H\ell}^{(3)})^{rr}B_{\bar{\mu}}W_{\bar{\nu}}^I\tilde{B}^{\bar{\mu}\bar{\nu}}(H^\dagger t^I H)-\frac{4}{3}g_L^2g_Y(\mathcal{C}_{H\ell}^{(3)})^{rr}\varepsilon^{IJK}B_{\bar{\mu}}W_{\bar{\nu}}^JW^{\bar{\mu}\bar{\nu}I}(H^\dagger t^K H) \\
& +\frac{4i}{3}g_L^2(\mathcal{C}_{H\ell}^{(3)})^{rr}\varepsilon^{IJK}(\partial_{\bar{\mu}}H^\dagger t^K\partial_{\bar{\nu}}H)W_{\bar{\mu}}^IW_{\bar{\nu}}^J-\frac{4i}{3}g_L^3(\mathcal{C}_{H\ell}^{(3)})^{rr}(H^\dagger t^I\overset{\leftrightarrow}{\partial}_{\bar{\nu}}H)W_{\bar{\mu}}^IW_{\bar{\mu}}^JW_{\bar{\nu}}^J \\
& -\frac{5}{3}g_L^2g_Y(\mathcal{C}_{H\ell}^{(3)})^{rr}\varepsilon^{IJK}(H^\dagger t^K H)W_{\bar{\mu}}^JW_{\bar{\nu}}^I\partial^{\bar{\mu}}B_{\bar{\nu}}-\frac{5}{3}g_Lg_Y(\mathcal{C}_{H\ell}^{(3)})^{rr}(H^\dagger t^I\partial_{\bar{\nu}}H)W_{\bar{\mu}}^I\partial^{\bar{\nu}}B_{\bar{\mu}} \\
& -\frac{5}{3}g_Lg_Y(\mathcal{C}_{H\ell}^{(3)})^{rr}(\partial_{\bar{\nu}}H^\dagger t^I H)W_{\bar{\mu}}^I\partial^{\bar{\nu}}B_{\bar{\mu}}-\frac{11}{6}g_Lg_Y\bar{y}_e^{ts}(\mathcal{C}_{H\ell}^{(3)})^{tr}t_j^{Ii}H_i^\dagger B_{\bar{\mu}}W_{\bar{\mu}}^I(\bar{e}_s\ell_r^j) \\
& -\frac{11}{6}g_Lg_Yy_e^{tr}(\mathcal{C}_{H\ell}^{(3)})^{st}t_j^{Ii}H^jB_{\bar{\mu}}W_{\bar{\mu}}^I(\bar{\ell}_{is}e_r)-2g_Lg_Y(\mathcal{C}_{H\ell}^{(3)})^{rr}(\partial_{\bar{\nu}}H^\dagger t^I\partial_{\bar{\nu}}H)B_{\bar{\mu}}W_{\bar{\mu}}^I \\
& -2i(\mathcal{C}_{H\ell}^{(3)})^{rr}\left[g_L(\partial_{\bar{\nu}}H^\dagger t^I\partial_{\bar{\mu}}\partial_{\bar{\nu}}H)W_{\bar{\mu}}^I-g_L(\partial_{\bar{\mu}}\partial_{\bar{\nu}}H^\dagger t^I\partial_{\bar{\nu}}H)W_{\bar{\mu}}^I\right] \\
& -\frac{7}{3}g_Lg_Y(\mathcal{C}_{H\ell}^{(3)})^{rr}(\partial_{\bar{\mu}}H^\dagger t^I\partial_{\bar{\nu}}H)B_{\bar{\mu}}W_{\bar{\nu}}^I-\frac{7}{3}g_Lg_Y(\mathcal{C}_{H\ell}^{(3)})^{rr}(\partial_{\bar{\nu}}H^\dagger t^I\partial_{\bar{\mu}}H)B_{\bar{\mu}}W_{\bar{\nu}}^I, \tag{2.31}
\end{aligned}$$

$$\begin{aligned}
\Delta\mathcal{S}_{\mathcal{O}_{Hu}} &= \frac{1}{54}g_Y\left[3y_u^{tr}\bar{y}_u^{tu}\mathcal{C}_{Hu}^{su}+3y_u^{tu}\bar{y}_u^{ts}\mathcal{C}_{Hu}^{ur}+36g_Y^2\mathcal{C}_{Hu}^{tt}\delta^{rs}-40g_Y^2\mathcal{C}_{Hu}^{sr}\right](H^\dagger H)(\bar{u}_s\tilde{B}u_r) \\
& +\frac{1}{24}g_L^2g_s^2\mathcal{C}_{Hu}^{rr}(H^\dagger H)G_{\bar{\mu}}^A{}^2W_{\bar{\mu}}^I{}^2+\frac{1}{18}g_s\left[-3\left[y_u^{tr}\bar{y}_u^{tu}\mathcal{C}_{Hu}^{su}+y_u^{tu}\bar{y}_u^{ts}\mathcal{C}_{Hu}^{ur}\right]-20g_Y^2\mathcal{C}_{Hu}^{sr}\right](H^\dagger H)(\bar{u}_sT^A\tilde{G}^A u_r) \\
& +\frac{1}{12}g_s^3g_Y\mathcal{C}_{Hu}^{rr}d^{ABC}(H^\dagger H)B_{\bar{\mu}}G_{\bar{\mu}}^AG_{\bar{\nu}}^BG_{\bar{\nu}}^C+\frac{1}{12}g_s^3g_Y\mathcal{C}_{Hu}^{rr}f^{ABC}(H^\dagger H)B_{\bar{\mu}}G_{\bar{\nu}}^AG_{\bar{\rho}}^BG_{\bar{\sigma}}^C\varepsilon^{\bar{\mu}\bar{\nu}\bar{\rho}\bar{\sigma}} \\
& +\frac{i}{12}g_s^3\mathcal{C}_{Hu}^{rr}d^{ABC}(H^\dagger\overset{\leftrightarrow}{\partial}_{\bar{\mu}}H)G_{\bar{\mu}}^AG_{\bar{\nu}}^BG_{\bar{\nu}}^C \\
& -\frac{i}{12}g_s^3\mathcal{C}_{Hu}^{rr}f^{ABC}G_{\bar{\mu}}^AG_{\bar{\nu}}^BG_{\bar{\rho}}^C\varepsilon^{\bar{\mu}\bar{\nu}\bar{\rho}\bar{\sigma}}(H^\dagger\overset{\leftrightarrow}{\partial}_{\bar{\sigma}}H)-\frac{i}{9}g_Yy_u^{st}\mathcal{C}_{Hu}^{tr}B_{\bar{\mu}}(\bar{q}_s\tilde{H}\partial^{\bar{\mu}}u_r) \\
& +\frac{i}{9}g_Y\bar{y}_u^{rt}\mathcal{C}_{Hu}^{st}B_{\bar{\mu}}(\bar{u}_s\tilde{H}^\dagger\partial^{\bar{\mu}}q_r)-\frac{i}{9}g_Yy_u^{st}\mathcal{C}_{Hu}^{tr}B_{\bar{\mu}}(\partial^{\bar{\mu}}\bar{q}_s\tilde{H}u_r)+\frac{i}{9}g_Y\bar{y}_u^{rt}\mathcal{C}_{Hu}^{st}B_{\bar{\mu}}(\partial^{\bar{\mu}}\bar{u}_s\tilde{H}^\dagger q_r) \\
& +\frac{11}{72}g_s^2g_Y^2\mathcal{C}_{Hu}^{rr}(H^\dagger H)B_{\bar{\mu}}^2G_{\bar{\mu}}^A{}^2+\frac{1}{6}g_s^2\mathcal{C}_{Hu}^{rr}(H^\dagger\partial_{\bar{\mu}}\partial_{\bar{\nu}}H)G_{\bar{\mu}}^AG_{\bar{\nu}}^A \\
& +\frac{1}{6}g_s\mathcal{C}_{Hu}^{rr}\left[g_sG_{\bar{\mu}}^AG_{\bar{\nu}}^B{}^A(H^\dagger\partial_{\bar{\nu}}H)+g_sG_{\bar{\mu}}^AG_{\bar{\nu}}^B{}^A(\partial_{\bar{\nu}}H^\dagger H)\right]+\frac{1}{6}g_s^2\mathcal{C}_{Hu}^{rr}(\partial_{\bar{\nu}}H^\dagger\partial_{\bar{\nu}}H)G_{\bar{\mu}}^A{}^2 \\
& +\frac{1}{6}g_s^2\mathcal{C}_{Hu}^{rr}(\partial_{\bar{\mu}}\partial_{\bar{\nu}}H^\dagger H)G_{\bar{\mu}}^AG_{\bar{\nu}}^A+\frac{1}{6}g_Lg_s^3\mathcal{C}_{Hu}^{rr}d^{ABC}(H^\dagger t^I H)G_{\bar{\mu}}^AG_{\bar{\nu}}^BG_{\bar{\nu}}^CW_{\bar{\mu}}^I \\
& +\frac{1}{6}g_Y\mathcal{C}_{Hu}^{tt}\left[g_Y^2-3g_L^2\right](H^\dagger H)(\bar{q}_s\tilde{B}q_s)-\frac{i}{6}g_sy_u^{st}\mathcal{C}_{Hu}^{tr}T_b^{Aa}G_{\bar{\mu}}^A(\bar{q}_{as}\tilde{H}\partial^{\bar{\mu}}u_r^b) \\
& +\frac{1}{6}g_s^2y_u^{st}\mathcal{C}_{Hu}^{tr}T_b^{Aa}T_a^{Bc}G_{\bar{\mu}}^AG_{\bar{\mu}}^B(\bar{q}_{cs}\tilde{H}u_r^b)+\frac{1}{6}g_s^2\bar{y}_u^{rt}\mathcal{C}_{Hu}^{st}T_b^{Aa}T_c^{Bb}G_{\bar{\mu}}^AG_{\bar{\mu}}^B(\bar{u}_{as}\tilde{H}^\dagger q_r^c) \\
& +\frac{i}{6}g_s\bar{y}_u^{rt}\mathcal{C}_{Hu}^{st}T_b^{Aa}G_{\bar{\mu}}^A(\bar{u}_{as}\tilde{H}^\dagger\partial^{\bar{\mu}}q_r^b)-\frac{i}{6}g_sy_u^{st}\mathcal{C}_{Hu}^{tr}T_b^{Aa}G_{\bar{\mu}}^A(\partial^{\bar{\mu}}\bar{q}_{as}\tilde{H}u_r^b) \\
& +\frac{i}{6}g_s\bar{y}_u^{rt}\mathcal{C}_{Hu}^{st}T_b^{Aa}G_{\bar{\mu}}^A(\partial^{\bar{\mu}}\bar{u}_{as}\tilde{H}^\dagger q_r^b)+\frac{1}{6}g_s^2\mathcal{C}_{Hu}^{rr}(H^\dagger\partial_{\bar{\mu}}H)G_{\bar{\mu}}^A\partial^{\bar{\nu}}G_{\bar{\nu}}^A \\
& +\frac{1}{6}g_s^2\mathcal{C}_{Hu}^{rr}(\partial_{\bar{\mu}}H^\dagger H)G_{\bar{\mu}}^A\partial^{\bar{\nu}}G_{\bar{\nu}}^A+\frac{i}{6}g_Lg_s^2\mathcal{C}_{Hu}^{rr}(H^\dagger t^I\overset{\leftrightarrow}{\partial}_{\bar{\nu}}H)G_{\bar{\mu}}^A{}^2W_{\bar{\nu}}^I \\
& +\frac{7i}{36}g_s^2g_Y\mathcal{C}_{Hu}^{rr}(H^\dagger\overset{\leftrightarrow}{\partial}_{\bar{\mu}}H)B_{\bar{\mu}}G_{\bar{\mu}}^A{}^2+\frac{2}{9}g_s^2g_Y^2\mathcal{C}_{Hu}^{rr}(H^\dagger H)B_{\bar{\mu}}B_{\bar{\nu}}G_{\bar{\mu}}^AG_{\bar{\nu}}^A
\end{aligned}$$

$$\begin{aligned}
& + \frac{2i}{9} g_s^2 g_Y C_{Hu}^{rr} (H^\dagger \overset{\leftrightarrow}{\partial}_\nu H) B_{\bar{\mu}} G_{\bar{\mu}}^A G_\nu^A + \frac{1}{3} g_s^2 C_{Hu}^{rr} (\partial_{\bar{\mu}} H^\dagger \partial_\nu H) G_{\bar{\mu}}^A G_\nu^A \\
& + \frac{i}{3} g_s C_{Hu}^{rr} \left[ 2g_s G_{\bar{\mu}}^A \tilde{G}^{\bar{\mu}\sigma A} (H^\dagger \partial_{\bar{\sigma}} H) - 2g_s G_{\bar{\mu}}^A \tilde{G}^{\bar{\mu}\sigma A} (\partial_{\bar{\sigma}} H^\dagger H) \right] \\
& + \frac{1}{3} g_L y_u^{tu} \tilde{y}_d^{ts} C_{Hu}^{ur} t_k^{Ij} H_j^\dagger \tilde{H}_k (\bar{d}_s \bar{W}^I u_r) + \frac{1}{3} g_L y_d^{tr} \tilde{y}_u^{tu} C_{Hu}^{su} t_k^{Ii} \tilde{H}^{\dagger i} H^k (\bar{u}_s \bar{W}^I d_r) \\
& + \frac{1}{3} g_L \left[ y_u^{tr} \tilde{y}_u^{tu} C_{Hu}^{su} + y_u^{tu} \tilde{y}_u^{ts} C_{Hu}^{ur} \right] (H^\dagger t^I H) (\bar{u}_s \bar{W}^I u_r) + \frac{1}{3} g_s^2 C_{Hu}^{rr} (H^\dagger \partial_\nu H) G_{\bar{\mu}}^A \partial^\nu G_{\bar{\mu}}^A \\
& + \frac{1}{3} g_s^2 C_{Hu}^{rr} (\partial_\nu H^\dagger H) G_{\bar{\mu}}^A \partial^\nu G_{\bar{\mu}}^A + \frac{7}{18} g_L g_s^2 g_Y C_{Hu}^{rr} (H^\dagger t^I H) B_{\bar{\mu}} G_{\bar{\mu}}^A W_\mu^I \\
& + \frac{4}{9} g_L g_s^2 g_Y C_{Hu}^{rr} (H^\dagger t^I H) B_{\bar{\mu}} G_{\bar{\mu}}^A G_\nu^A W_\nu^I - \frac{4i}{9} g_Y y_u^{st} C_{Hu}^{tr} B_{\bar{\mu}} (\bar{q}_s \partial^\mu \tilde{H} u_r) + \frac{4}{9} g_Y^2 C_{Hu}^{rr} (H^\dagger \partial_\mu H) B_{\bar{\mu}} \partial^\nu B_\nu \\
& + \frac{4}{9} g_Y^2 C_{Hu}^{rr} (\partial_\mu H^\dagger H) B_{\bar{\mu}} \partial^\nu B_\nu + \frac{1}{2} g_Y^2 \left[ C_{Hu}^{rr} [g_L^2 + g_Y^2] - 5y_u^{rt} \tilde{y}_u^{rs} C_{Hu}^{ts} \right] (H^\dagger H)^2 B_\mu^2 \\
& + \frac{5}{9} g_Y y_u^{st} C_{Hu}^{tr} B_{\bar{\mu}} (\bar{q}_s \partial^\nu \tilde{H} \sigma^{\bar{\mu}\nu} u_r) - \frac{11}{54} g_Y^2 \tilde{y}_u^{rt} C_{Hu}^{st} B_{\bar{\mu}}^2 (\bar{u}_s \tilde{H}^\dagger q_r) \\
& + \frac{5i}{12} g_s g_Y y_u^{st} C_{Hu}^{tr} T_b^{Aa} B_{\bar{\mu}} G_\nu^A (\bar{q}_{as} \tilde{H} \sigma^{\bar{\mu}\nu} u_r^b) - \frac{5i}{12} g_s g_Y \tilde{y}_u^{rt} C_{Hu}^{st} T_b^{Aa} B_{\bar{\mu}} G_\nu^A (\bar{u}_{as} \sigma^{\bar{\mu}\nu} \tilde{H}^\dagger q_r^b) \\
& + \frac{4i}{9} g_Y \tilde{y}_u^{rt} C_{Hu}^{st} B_{\bar{\mu}} (\bar{u}_s \partial^\mu \tilde{H} q_r) - \frac{i}{2} g_L^2 g_Y C_{Hu}^{rr} (H^\dagger \overset{\leftrightarrow}{\partial}_\mu H) B_{\bar{\mu}} W_\mu^I{}^2 \\
& + \frac{i}{2} g_Y \left[ C_{Hu}^{rr} [g_L^2 + g_Y^2] - 5y_u^{rt} \tilde{y}_u^{rs} C_{Hu}^{ts} \right] (H^\dagger \overset{\leftrightarrow}{\partial}_\mu H) (H^\dagger H) B_{\bar{\mu}} + \frac{5}{9} g_Y \tilde{y}_u^{rt} C_{Hu}^{st} B_{\bar{\mu}} (\bar{u}_s \sigma^{\bar{\mu}\nu} \partial^\nu \tilde{H} q_r) \\
& + \frac{8i}{9} g_Y C_{Hu}^{rr} \left[ 2g_Y B_{\bar{\mu}} \tilde{B}^{\bar{\mu}\bar{\sigma}} (H^\dagger \partial_{\bar{\sigma}} H) - 2g_Y B_{\bar{\mu}} \tilde{B}^{\bar{\mu}\bar{\sigma}} (\partial_{\bar{\sigma}} H^\dagger H) \right] \\
& + g_L g_Y \left[ C_{Hu}^{rr} [g_L^2 + g_Y^2] - 6y_u^{rt} \tilde{y}_u^{rs} C_{Hu}^{ts} \right] (H^\dagger H) (H^\dagger t^I H) B_{\bar{\mu}} W_\mu^I \\
& - i y_u^{rt} \tilde{y}_u^{rs} C_{Hu}^{ts} \left[ g_L (H^\dagger \partial_\mu H) (H^\dagger t^I H) W_\mu^I - g_L (\partial_\mu H^\dagger H) (H^\dagger t^I H) W_\mu^I \right] + g_L^2 g_Y C_{Hu}^{tt} (\bar{\ell}_s H \bar{B} H^\dagger \ell_s) \\
& + g_L^2 g_Y C_{Hu}^{tt} (\bar{q}_s H \bar{B} H^\dagger q_s) + \frac{4}{3} g_L g_s^2 C_{Hu}^{rr} G_{\bar{\mu}}^A W_\nu^I \tilde{G}^{\bar{\mu}\nu A} (H^\dagger t^I H) + \frac{13}{9} g_Y^2 C_{Hu}^{rr} (H^\dagger \partial_\mu \partial_\nu H) B_{\bar{\mu}} B_\nu \\
& + \frac{13}{9} g_Y C_{Hu}^{rr} \left[ g_Y B_{\bar{\mu}} B^{\bar{\mu}\nu} (H^\dagger \partial_\nu H) + g_Y B_{\bar{\mu}} B^{\bar{\mu}\nu} (\partial_\nu H^\dagger H) \right] + \frac{13}{9} g_Y^2 C_{Hu}^{rr} (\partial_\mu \partial_\nu H^\dagger H) B_{\bar{\mu}} B_\nu \\
& + 2g_L g_Y C_{Hu}^{rr} (H^\dagger t^I \partial_\mu \partial_\nu H) B_{\bar{\mu}} W_\nu^I + 2g_L C_{Hu}^{rr} \left[ g_Y B_{\bar{\mu}} W^{\bar{\mu}\nu I} (H^\dagger t^I \partial_\nu H) + g_Y B_{\bar{\mu}} W^{\bar{\mu}\nu I} (\partial_\nu H^\dagger t^I H) \right] \\
& + 2g_L g_Y C_{Hu}^{rr} (\partial_\mu \partial_\nu H^\dagger t^I H) B_{\bar{\mu}} W_\nu^I + 2g_L^2 g_Y C_{Hu}^{rr} \varepsilon^{IJK} B_{\bar{\mu}} W_\nu^J W^{\bar{\mu}\nu I} (H^\dagger t^K H) \\
& + 2g_L^2 g_Y C_{Hu}^{rr} \varepsilon^{IJK} (H^\dagger t^K H) B_{\bar{\mu}} W_\nu^I \partial^\nu W_\mu^J + \frac{32}{9} g_L g_Y^2 C_{Hu}^{rr} B_{\bar{\mu}} W_\nu^I \tilde{B}^{\bar{\mu}\nu} (H^\dagger t^I H) - \frac{5}{54} g_Y^4 C_{Hu}^{rr} (H^\dagger H) B_{\bar{\mu}}^2 B_\mu^2 \\
& - \frac{1}{9} g_Y^2 C_{Hu}^{rr} (H^\dagger \partial_\nu H) B_{\bar{\mu}} \partial^\nu B_{\bar{\mu}} - \frac{1}{9} g_Y^2 C_{Hu}^{rr} (\partial_\nu H^\dagger H) B_{\bar{\mu}} \partial^\nu B_{\bar{\mu}} \\
& - \frac{1}{6} g_L g_s^3 C_{Hu}^{rr} f^{ABC} (H^\dagger t^I H) G_{\bar{\mu}}^A G_\nu^B G_\rho^C W_\sigma^I \varepsilon^{\bar{\mu}\nu\rho\sigma} - \frac{7}{36} g_s g_Y y_u^{st} C_{Hu}^{tr} T_b^{Aa} B_{\bar{\mu}} G_\mu^A (\bar{q}_{as} \tilde{H} u_r^b) \\
& - \frac{7}{36} g_s g_Y \tilde{y}_u^{rt} C_{Hu}^{st} T_b^{Aa} B_{\bar{\mu}} G_\mu^A (\bar{u}_{as} \tilde{H}^\dagger q_r^b) - \frac{11}{54} g_Y^2 y_u^{st} C_{Hu}^{tr} B_{\bar{\mu}}^2 (\bar{q}_s \tilde{H} u_r) - \frac{1}{3} g_Y^3 C_{Hu}^{tt} (H^\dagger H) (\bar{d}_s \bar{B} d_s) \\
& - \frac{7}{18} g_L^2 g_Y^2 C_{Hu}^{rr} (H^\dagger H) B_{\bar{\mu}}^2 W_\mu^I{}^2 - \frac{1}{2} g_Y C_{Hu}^{tt} [g_L^2 + g_Y^2] (H^\dagger H) (\bar{\ell}_s \bar{B} \ell_s) - \frac{5}{9} g_L g_Y y_u^{st} C_{Hu}^{tr} t_j^{Ik} \tilde{H}_j B_{\bar{\mu}} W_\mu^I (\bar{q}_{ks} u_r) \\
& - \frac{5i}{9} g_L g_Y y_u^{st} C_{Hu}^{tr} \varepsilon^{jk} t_j^{Ii} H_i^\dagger B_{\bar{\mu}} W_\nu^I (\bar{q}_{ks} \sigma^{\bar{\mu}\nu} u_r) - \frac{5}{9} g_L g_Y \tilde{y}_u^{rt} C_{Hu}^{st} t_k^{Ii} \tilde{H}^{\dagger i} B_{\bar{\mu}} W_\mu^I (\bar{u}_s q_r^k)
\end{aligned}$$

$$\begin{aligned}
& + \frac{5i}{9} g_L g_Y \bar{y}_u^{rt} C_{Hu}^{st} \bar{\varepsilon}_{ij} t_k^{Ii} H^k B_{\bar{\mu}} W_{\bar{\nu}}^I (\bar{u}_s \sigma^{\bar{\mu}\bar{\nu}} q_r^j) - \frac{2}{3} g_s^2 g_Y C_{Hu}^{rr} B_{\bar{\mu}} G_{\bar{\nu}}^A \tilde{G}^{\bar{\mu}\bar{\nu}A} (H^\dagger H) \\
& - \frac{2i}{3} g_s y_u^{st} C_{Hu}^{tr} T_b^{Aa} G_{\bar{\mu}}^A (\bar{q}_{as} \partial^{\bar{\mu}} \tilde{H} u_r^b) + \frac{2i}{3} g_s \bar{y}_u^{rt} C_{Hu}^{st} T_b^{Aa} G_{\bar{\mu}}^A (\bar{u}_{as} \partial^{\bar{\mu}} \tilde{H} q_r^b) \\
& - \frac{2}{3} g_Y^2 C_{Hu}^{rr} (H^\dagger H) B_{\bar{\mu}} \partial^{\bar{\mu}} \partial^{\bar{\nu}} B_{\bar{\nu}} - \frac{2i}{3} g_Y C_{Hu}^{rr} \partial^{\bar{\mu}} \partial^{\bar{\nu}} B_{\bar{\nu}} (H^\dagger \overset{\leftrightarrow}{\partial}_{\bar{\mu}} H) \\
& - \frac{5}{6} g_s y_u^{st} C_{Hu}^{tr} T_b^{Aa} G_{\bar{\mu}}^A (\bar{q}_{as} \partial^{\bar{\mu}} \tilde{H} \sigma^{\bar{\mu}\bar{\nu}} u_r^b) - \frac{5}{6} g_L g_s y_u^{st} C_{Hu}^{tr} t_j^{Ik} T_b^{Aa} \tilde{H}_j G_{\bar{\mu}}^A W_{\bar{\mu}}^I (\bar{q}_{aks} u_r^b) \\
& - \frac{5i}{6} g_L g_s y_u^{st} C_{Hu}^{tr} \varepsilon^{jk} t_j^{Ii} T_b^{Aa} H_i^\dagger G_{\bar{\mu}}^A W_{\bar{\nu}}^I (\bar{q}_{aks} \sigma^{\bar{\mu}\bar{\nu}} u_r^b) - \frac{5}{6} g_L g_s \bar{y}_u^{rt} C_{Hu}^{st} t_k^{Ii} T_b^{Aa} \tilde{H}^{\dagger i} G_{\bar{\mu}}^A W_{\bar{\mu}}^I (\bar{u}_{as} q_r^{bk}) \\
& + \frac{5i}{6} g_L g_s \bar{y}_u^{rt} C_{Hu}^{st} \bar{\varepsilon}_{ij} t_k^{Ii} T_b^{Aa} H^k G_{\bar{\mu}}^A W_{\bar{\nu}}^I (\bar{u}_{as} \sigma^{\bar{\mu}\bar{\nu}} q_r^{bj}) - \frac{5}{6} g_s \bar{y}_u^{rt} C_{Hu}^{st} T_b^{Aa} G_{\bar{\mu}}^A (\bar{u}_{as} \sigma^{\bar{\mu}\bar{\nu}} \partial^{\bar{\nu}} \tilde{H} q_r^b) \\
& - \frac{53i}{54} g_Y^3 C_{Hu}^{rr} (H^\dagger \overset{\leftrightarrow}{\partial}_{\bar{\mu}} H) B_{\bar{\mu}} B_{\bar{\mu}}^2 - g_L^2 g_Y^2 C_{Hu}^{rr} (H^\dagger H) B_{\bar{\mu}} B_{\bar{\nu}} W_{\bar{\mu}}^I W_{\bar{\nu}}^I - g_L^3 g_Y C_{Hu}^{rr} (H^\dagger t^I H) B_{\bar{\mu}} W_{\bar{\mu}}^I W_{\bar{\mu}}^{I^2} \\
& - g_Y^3 C_{Hu}^{tt} (H^\dagger H) (\bar{e}_s \bar{B} e_s) - i g_L^2 g_Y C_{Hu}^{rr} (H^\dagger \overset{\leftrightarrow}{\partial}_{\bar{\nu}} H) B_{\bar{\mu}} W_{\bar{\mu}}^I W_{\bar{\nu}}^I - \frac{10}{9} g_Y^2 C_{Hu}^{rr} (\partial_{\bar{\mu}} H^\dagger \partial_{\bar{\nu}} H) B_{\bar{\mu}} B_{\bar{\nu}} \\
& - \frac{4}{3} g_L g_Y C_{Hu}^{rr} (H^\dagger t^I H) W_{\bar{\mu}}^I \partial^{\bar{\mu}} \partial^{\bar{\nu}} B_{\bar{\nu}} - \frac{14}{9} g_Y^2 C_{Hu}^{rr} (\partial_{\bar{\nu}} H^\dagger \partial_{\bar{\nu}} H) B_{\bar{\mu}}^2 \\
& - \frac{14i}{9} g_L g_Y^2 C_{Hu}^{rr} (H^\dagger t^I \overset{\leftrightarrow}{\partial}_{\bar{\nu}} H) B_{\bar{\mu}}^2 W_{\bar{\nu}}^I - \frac{53}{27} g_L g_Y^3 C_{Hu}^{rr} (H^\dagger t^I H) B_{\bar{\mu}} B_{\bar{\mu}}^2 W_{\bar{\mu}}^I \\
& - 2i C_{Hu}^{rr} \left[ g_Y (\partial_{\bar{\nu}} H^\dagger \partial_{\bar{\mu}} \partial_{\bar{\nu}} H) B_{\bar{\mu}} - g_Y (\partial_{\bar{\mu}} \partial_{\bar{\nu}} H^\dagger \partial_{\bar{\nu}} H) B_{\bar{\mu}} \right] - 2 g_L g_Y C_{Hu}^{rr} (\partial_{\bar{\mu}} H^\dagger t^I \partial_{\bar{\nu}} H) B_{\bar{\mu}} W_{\bar{\nu}}^I \\
& - 2 g_L g_Y C_{Hu}^{rr} (\partial_{\bar{\nu}} H^\dagger t^I \partial_{\bar{\mu}} H) B_{\bar{\mu}} W_{\bar{\nu}}^I - 2 g_L^2 y_u^{rt} \bar{y}_u^{rs} C_{Hu}^{ts} (H^\dagger t^I H) (H^\dagger t^J H) W_{\bar{\mu}}^I W_{\bar{\mu}}^J - 2 g_L g_Y C_{Hu}^{rr} (H^\dagger t^I \partial_{\bar{\nu}} H) B_{\bar{\mu}} \partial^{\bar{\nu}} W_{\bar{\mu}}^I \\
& - 2 g_L g_Y C_{Hu}^{rr} (\partial_{\bar{\nu}} H^\dagger t^I H) B_{\bar{\mu}} \partial^{\bar{\nu}} W_{\bar{\mu}}^I - 4 g_L g_Y C_{Hu}^{rr} (\partial_{\bar{\nu}} H^\dagger t^I \partial_{\bar{\nu}} H) B_{\bar{\mu}} W_{\bar{\mu}}^I \\
& - 4 i g_L g_Y^2 C_{Hu}^{rr} (H^\dagger t^I \overset{\leftrightarrow}{\partial}_{\bar{\nu}} H) B_{\bar{\mu}} B_{\bar{\nu}} W_{\bar{\mu}}^I, \tag{2.32}
\end{aligned}$$

$$\begin{aligned}
\Delta S_{\mathcal{O}_{Hd}} &= \frac{1}{54} g_Y \left[ 6 y_d^{tr} \bar{y}_d^{tu} C_{Hd}^{su} + 6 y_d^{tu} \bar{y}_d^{ts} C_{Hd}^{ur} + 9 g_Y^2 C_{Hd}^{tt} \delta^{rs} - 10 g_Y^2 C_{Hd}^{sr} \right] (H^\dagger H) (\bar{d}_s \bar{B} d_r) \\
& + \frac{i}{36} g_s^2 g_Y C_{Hd}^{rr} (H^\dagger \overset{\leftrightarrow}{\partial}_{\bar{\mu}} H) B_{\bar{\mu}} G_{\bar{\mu}}^{A^2} + \frac{1}{24} g_L^2 g_s^2 C_{Hd}^{rr} (H^\dagger H) G_{\bar{\mu}}^{A^2} W_{\bar{\mu}}^{I^2} + \frac{1}{18} g_L g_s^2 g_Y C_{Hd}^{rr} (H^\dagger t^I H) B_{\bar{\mu}} G_{\bar{\mu}}^{A^2} W_{\bar{\mu}}^I \\
& - \frac{i}{18} g_Y \bar{y}_d^{rt} C_{Hd}^{st} B_{\bar{\mu}} (\bar{d}_s H^\dagger \partial^{\bar{\mu}} q_r) + \frac{1}{18} g_s \left[ 3 y_d^{tr} \bar{y}_d^{tu} C_{Hd}^{su} + 3 y_d^{tu} \bar{y}_d^{ts} C_{Hd}^{ur} + 10 g_Y^2 C_{Hd}^{sr} \right] (H^\dagger H) (\bar{d}_s T^A \bar{G}^A d_r) \\
& + \frac{i}{18} g_Y y_d^{st} C_{Hd}^{tr} B_{\bar{\mu}} (\bar{q}_s H \partial^{\bar{\mu}} d_r) - \frac{i}{18} g_Y \bar{y}_d^{rt} C_{Hd}^{st} B_{\bar{\mu}} (\partial^{\bar{\mu}} \bar{d}_s H^\dagger q_r) + \frac{i}{18} g_Y y_d^{st} C_{Hd}^{tr} B_{\bar{\mu}} (\partial^{\bar{\mu}} \bar{q}_s H d_r) \\
& + \frac{1}{12} g_s^3 g_Y C_{Hd}^{rr} d^{ABC} (H^\dagger H) B_{\bar{\mu}} G_{\bar{\mu}}^A G_{\bar{\nu}}^B G_{\bar{\nu}}^C + \frac{1}{12} g_s^3 g_Y C_{Hd}^{rr} f^{ABC} (H^\dagger H) B_{\bar{\mu}} G_{\bar{\nu}}^A G_{\bar{\rho}}^B G_{\bar{\sigma}}^C \varepsilon^{\bar{\mu}\bar{\nu}\bar{\rho}\bar{\sigma}} \\
& + \frac{1}{12} g_Y C_{Hd}^{tt} \left[ 3 g_L^2 - g_Y^2 \right] (H^\dagger H) (\bar{q}_s \bar{B} q_s) + \frac{i}{12} g_s^3 C_{Hd}^{rr} d^{ABC} (H^\dagger \overset{\leftrightarrow}{\partial}_{\bar{\mu}} H) G_{\bar{\mu}}^A G_{\bar{\nu}}^B G_{\bar{\nu}}^C \\
& - \frac{i}{12} g_s^3 C_{Hd}^{rr} f^{ABC} G_{\bar{\mu}}^A G_{\bar{\nu}}^B G_{\bar{\rho}}^C \varepsilon^{\bar{\mu}\bar{\nu}\bar{\rho}\bar{\sigma}} (H^\dagger \overset{\leftrightarrow}{\partial}_{\bar{\sigma}} H) + \frac{1}{9} g_Y^2 C_{Hd}^{rr} (H^\dagger \partial_{\bar{\mu}} H) B_{\bar{\mu}} \partial^{\bar{\nu}} B_{\bar{\nu}} \\
& + \frac{1}{9} g_Y^2 C_{Hd}^{rr} (\partial_{\bar{\mu}} H^\dagger H) B_{\bar{\mu}} \partial^{\bar{\nu}} B_{\bar{\nu}} - \frac{i}{9} g_s^2 g_Y C_{Hd}^{rr} (H^\dagger \overset{\leftrightarrow}{\partial}_{\bar{\nu}} H) B_{\bar{\mu}} G_{\bar{\mu}}^A G_{\bar{\nu}}^A \\
& + \frac{1}{6} g_s^2 C_{Hd}^{rr} (H^\dagger \partial_{\bar{\mu}} \partial_{\bar{\nu}} H) G_{\bar{\mu}}^A G_{\bar{\nu}}^A + \frac{1}{6} g_s C_{Hd}^{rr} \left[ g_s G_{\bar{\mu}}^A G^{\bar{\mu}\bar{\nu}A} (H^\dagger \partial_{\bar{\nu}} H) + g_s G_{\bar{\mu}}^A G^{\bar{\mu}\bar{\nu}A} (\partial_{\bar{\nu}} H^\dagger H) \right] \\
& + \frac{1}{6} g_s^2 C_{Hd}^{rr} (\partial_{\bar{\nu}} H^\dagger \partial_{\bar{\nu}} H) G_{\bar{\mu}}^{A^2} + \frac{1}{6} g_s^2 C_{Hd}^{rr} (\partial_{\bar{\mu}} \partial_{\bar{\nu}} H^\dagger H) G_{\bar{\mu}}^A G_{\bar{\nu}}^A
\end{aligned}$$

$$\begin{aligned}
& + \frac{1}{6} g_L g_s^3 \mathcal{C}_{Hd}^{rr} d^{ABC} (H^\dagger t^I H) G_\mu^A G_\nu^B G_\nu^C W_\mu^I + \frac{1}{6} g_s^2 \bar{y}_d^{rt} \mathcal{C}_{Hd}^{st} T_b^{Aa} T_a^{Bc} G_\mu^A G_\mu^B (\bar{d}_{cs} H^\dagger q_r^b) \\
& + \frac{1}{6} g_s^2 y_d^{st} \mathcal{C}_{Hd}^{tr} T_b^{Aa} T_c^{Bb} G_\mu^A G_\mu^B (\bar{q}_{as} H d_r^c) - \frac{i}{6} g_s y_d^{st} \mathcal{C}_{Hd}^{tr} T_b^{Aa} G_\mu^A (\bar{q}_{as} H \partial^\mu d_r^b) \\
& + \frac{i}{6} g_s \bar{y}_d^{rt} \mathcal{C}_{Hd}^{st} T_b^{Aa} G_\mu^A (\partial^\mu \bar{d}_{as} H^\dagger q_r^b) - \frac{i}{6} g_s y_d^{st} \mathcal{C}_{Hd}^{tr} T_b^{Aa} G_\mu^A (\partial^\mu \bar{q}_{as} H d_r^b) \\
& + \frac{1}{6} g_s^2 \mathcal{C}_{Hd}^{rr} (H^\dagger \partial_\mu H) G_\mu^A \partial^\nu G_\nu^A + \frac{1}{6} g_s^2 \mathcal{C}_{Hd}^{rr} (\partial_\mu H^\dagger H) G_\mu^A \partial^\nu G_\nu^A \\
& + \frac{i}{6} g_L g_s^2 \mathcal{C}_{Hd}^{rr} (H^\dagger t^I \overleftrightarrow{\partial}_\nu H) G_\mu^A {}^2 W_\nu^I \\
& + \frac{2i}{9} g_Y \mathcal{C}_{Hd}^{rr} \left[ 2g_Y B_\mu \tilde{B}^{\mu\bar{\sigma}} (H^\dagger \partial_\sigma H) - 2g_Y B_\mu \tilde{B}^{\mu\bar{\sigma}} (\partial_\sigma H^\dagger H) \right] - \frac{2i}{9} g_Y y_d^{st} \mathcal{C}_{Hd}^{tr} B_\mu (\bar{q}_s \partial^\mu H d_r) \\
& + \frac{13}{54} g_Y^4 \mathcal{C}_{Hd}^{rr} (H^\dagger H) B_\mu^2 B_\mu^2 + \frac{1}{4} g_Y^2 \left[ 6y_d^{rt} \bar{y}_d^{rs} \mathcal{C}_{Hd}^{ts} - \mathcal{C}_{Hd}^{rr} [g_L^2 + g_Y^2] \right] (H^\dagger H)^2 B_\mu^2 \\
& + \frac{1}{4} g_Y \mathcal{C}_{Hd}^{tt} [g_L^2 + g_Y^2] (H^\dagger H) (\bar{\ell}_s \bar{B} \ell_s) + \frac{i}{4} g_L^2 g_Y \mathcal{C}_{Hd}^{rr} (H^\dagger \overleftrightarrow{\partial}_\mu H) B_\mu W_\mu^{I\,2} \\
& - \frac{i}{4} g_Y \left[ \mathcal{C}_{Hd}^{rr} [g_L^2 + g_Y^2] - 6y_d^{rt} \bar{y}_d^{rs} \mathcal{C}_{Hd}^{ts} \right] (H^\dagger \overleftrightarrow{\partial}_\mu H) (H^\dagger H) B_\mu + \frac{5}{18} g_L^2 g_Y^2 \mathcal{C}_{Hd}^{rr} (H^\dagger H) B_\mu^2 W_\mu^{I\,2} \\
& + \frac{5}{18} g_Y y_d^{st} \mathcal{C}_{Hd}^{tr} B_\mu (\bar{q}_s \partial^\nu H \sigma^{\mu\nu} d_r) + \frac{11}{36} g_s g_Y y_d^{st} \mathcal{C}_{Hd}^{tr} T_b^{Aa} B_\mu G_\mu^A (\bar{q}_{as} H d_r^b) \\
& + \frac{1}{3} g_s^2 \mathcal{C}_{Hd}^{rr} (\partial_\mu H^\dagger \partial_\nu H) G_\mu^A G_\nu^A \\
& + \frac{i}{3} g_s \mathcal{C}_{Hd}^{rr} \left[ 2g_s G_\mu^A \tilde{G}^{\mu\bar{\sigma}A} (H^\dagger \partial_\sigma H) - 2g_s G_\mu^A \tilde{G}^{\mu\bar{\sigma}A} (\partial_\sigma H^\dagger H) \right] \\
& + \frac{1}{3} g_s^2 \mathcal{C}_{Hd}^{rr} (H^\dagger \partial_\nu H) G_\mu^A \partial^\nu G_\mu^A + \frac{1}{3} g_s^2 \mathcal{C}_{Hd}^{rr} (\partial_\nu H^\dagger H) G_\mu^A \partial^\nu G_\mu^A \\
& + \frac{1}{3} g_Y^2 \mathcal{C}_{Hd}^{rr} (H^\dagger H) B_\mu \partial^\mu \partial^\nu B_\nu + \frac{1}{2} g_L^2 g_Y^2 \mathcal{C}_{Hd}^{rr} (H^\dagger H) B_\mu B_\nu W_\mu^I W_\nu^I + \frac{1}{2} g_L^3 g_Y \mathcal{C}_{Hd}^{rr} (H^\dagger t^I H) B_\mu W_\mu^I W_\mu^{I\,2} \\
& + \frac{8}{9} g_L g_Y^2 \mathcal{C}_{Hd}^{rr} B_\mu W_\nu^I \tilde{B}^{\mu\nu} (H^\dagger t^I H) + g_L g_Y \left[ 4y_d^{rt} \bar{y}_d^{rs} \mathcal{C}_{Hd}^{ts} - \frac{1}{2} \mathcal{C}_{Hd}^{rr} [g_L^2 + g_Y^2] \right] (H^\dagger H) (H^\dagger t^I H) B_\mu W_\mu^I \\
& + \frac{10}{9} g_Y^2 \mathcal{C}_{Hd}^{rr} (\partial_\nu H^\dagger \partial_\nu H) B_\mu^2 + \frac{11}{9} g_Y^2 \mathcal{C}_{Hd}^{rr} (\partial_\mu H^\dagger \partial_\nu H) B_\mu B_\nu - \frac{1}{72} g_s^2 g_Y^2 \mathcal{C}_{Hd}^{rr} (H^\dagger H) B_\mu^2 G_\mu^{A\,2} \\
& - \frac{1}{9} g_s^2 g_Y^2 \mathcal{C}_{Hd}^{rr} (H^\dagger H) B_\mu B_\nu G_\mu^A G_\nu^A - \frac{13}{108} g_Y^2 \bar{y}_d^{rt} \mathcal{C}_{Hd}^{st} B_\mu^2 (\bar{d}_s H^\dagger q_r) - \frac{13}{108} g_Y^2 y_d^{st} \mathcal{C}_{Hd}^{tr} B_\mu^2 (\bar{q}_s H d_r) \\
& - \frac{1}{6} g_L g_s^3 \mathcal{C}_{Hd}^{rr} f^{ABC} (H^\dagger t^I H) G_\mu^A G_\nu^B G_\rho^C W_\sigma^I \varepsilon^{\mu\nu\rho\sigma} + \frac{i}{6} g_s \bar{y}_d^{rt} \mathcal{C}_{Hd}^{st} T_b^{Aa} G_\mu^A (\bar{d}_{as} H^\dagger \partial^\mu q_r^b) \\
& - \frac{2}{9} g_L g_s^2 g_Y \mathcal{C}_{Hd}^{rr} (H^\dagger t^I H) B_\mu G_\mu^A G_\nu^A W_\nu^I + \frac{2i}{9} g_Y \bar{y}_d^{rt} \mathcal{C}_{Hd}^{st} B_\mu (\bar{d}_s \partial^\mu H^\dagger q_r) \\
& + \frac{5}{18} g_Y \bar{y}_d^{rt} \mathcal{C}_{Hd}^{st} B_\mu (\bar{d}_s \sigma^{\mu\nu} \partial^\nu H^\dagger q_r) + \frac{11}{36} g_s g_Y \bar{y}_d^{rt} \mathcal{C}_{Hd}^{st} T_b^{Aa} B_\mu G_\mu^A (\bar{d}_{as} H^\dagger q_r^b) \\
& + \frac{1}{3} g_L \left[ y_d^{tr} \bar{y}_d^{tu} \mathcal{C}_{Hd}^{su} + y_d^{tu} \bar{y}_d^{ts} \mathcal{C}_{Hd}^{ur} \right] (H^\dagger t^I H) (\bar{d}_s \bar{W}^I d_r) + \frac{5}{6} g_L g_s \bar{y}_d^{rt} \mathcal{C}_{Hd}^{st} t_j^{Ii} T_b^{Aa} H_i^\dagger G_\mu^A W_\mu^I (\bar{d}_{as} q_r^{bj}) \\
& - \frac{5}{18} g_L g_Y \bar{y}_d^{rt} \mathcal{C}_{Hd}^{st} t_j^{Ii} H_i^\dagger B_\mu W_\mu^I (\bar{d}_s q_r^j) + \frac{5i}{18} g_L g_Y \bar{y}_d^{rt} \mathcal{C}_{Hd}^{st} t_j^{Ii} H_i^\dagger B_\mu W_\nu^I (\bar{d}_s \sigma^{\mu\nu} q_r^j) \\
& - \frac{5}{18} g_L g_Y y_d^{st} \mathcal{C}_{Hd}^{tr} t_j^{Ii} H^j B_\mu W_\mu^I (\bar{q}_{is} d_r) - \frac{5i}{18} g_L g_Y y_d^{st} \mathcal{C}_{Hd}^{tr} t_j^{Ii} H^j B_\mu W_\nu^I (\bar{q}_{is} \sigma^{\mu\nu} d_r)
\end{aligned}$$

$$\begin{aligned}
& -\frac{1}{3}g_L y_u^{tr} \bar{y}_d^{tu} \mathcal{C}_{Hd}^{su} t_k^{Ij} H_j^\dagger \tilde{H}_k (\bar{d}_s \bar{W}^I u_r) - \frac{1}{3}g_Y^3 \mathcal{C}_{Hd}^{tt} (H^\dagger H) (\bar{u}_s \bar{B} u_s) \\
& -\frac{1}{3}g_L y_d^{tu} \bar{y}_u^{ts} \mathcal{C}_{Hd}^{ur} t_k^{Ii} \tilde{H}^\dagger{}^i H^k (\bar{u}_s \bar{W}^I d_r) + \frac{i}{3}g_Y \mathcal{C}_{Hd}^{rr} \partial^{\bar{\mu}} \partial^{\bar{\nu}} B_{\bar{\nu}} (H^\dagger \overset{\leftrightarrow}{\partial}_{\bar{\mu}} H) \\
& -\frac{7}{18}g_Y^2 \mathcal{C}_{Hd}^{rr} (H^\dagger \partial_{\bar{\mu}} \partial_{\bar{\nu}} H) B_{\bar{\mu}} B_{\bar{\nu}} - \frac{7}{18}g_Y \mathcal{C}_{Hd}^{rr} \left[ g_Y B_{\bar{\mu}} B^{\bar{\mu}\bar{\nu}} (H^\dagger \partial_{\bar{\nu}} H) + g_Y B_{\bar{\mu}} B^{\bar{\mu}\bar{\nu}} (\partial_{\bar{\nu}} H^\dagger H) \right] \\
& -\frac{7}{18}g_Y^2 \mathcal{C}_{Hd}^{rr} (\partial_{\bar{\mu}} \partial_{\bar{\nu}} H^\dagger H) B_{\bar{\mu}} B_{\bar{\nu}} + \frac{5i}{12}g_s g_Y \bar{y}_d^{rt} \mathcal{C}_{Hd}^{st} T_b^{Aa} B_{\bar{\mu}} G_{\bar{\nu}}^A (\bar{d}_{as} \sigma^{\bar{\mu}\bar{\nu}} H^\dagger q_r^b) \\
& -\frac{5i}{12}g_s g_Y y_d^{st} \mathcal{C}_{Hd}^{tr} T_b^{Aa} B_{\bar{\mu}} G_{\bar{\nu}}^A (\bar{q}_{as} H \sigma^{\bar{\mu}\bar{\nu}} d_r^b) + \frac{1}{2}g_Y^3 \mathcal{C}_{Hd}^{tt} (H^\dagger H) (\bar{e}_s \bar{B} e_s) \\
& +\frac{i}{2}g_L^2 g_Y \mathcal{C}_{Hd}^{rr} (H^\dagger \overset{\leftrightarrow}{\partial}_{\bar{\nu}} H) B_{\bar{\mu}} W_{\bar{\mu}}^I W_{\bar{\nu}}^I + \frac{2}{3}g_L g_Y \mathcal{C}_{Hd}^{rr} (H^\dagger t^I H) W_{\bar{\mu}}^I \partial^{\bar{\mu}} \partial^{\bar{\nu}} B_{\bar{\nu}} \\
& +\frac{13}{18}g_Y^2 \mathcal{C}_{Hd}^{rr} (H^\dagger \partial_{\bar{\nu}} H) B_{\bar{\mu}} \partial^{\bar{\nu}} B_{\bar{\mu}} + \frac{13}{18}g_Y^2 \mathcal{C}_{Hd}^{rr} (\partial_{\bar{\nu}} H^\dagger H) B_{\bar{\mu}} \partial^{\bar{\nu}} B_{\bar{\mu}} - \frac{2}{3}g_s^2 g_Y \mathcal{C}_{Hd}^{rr} B_{\bar{\mu}} G_{\bar{\nu}}^A \tilde{G}^{\bar{\mu}\bar{\nu}A} (H^\dagger H) \\
& +\frac{83i}{108}g_Y^3 \mathcal{C}_{Hd}^{rr} (H^\dagger \overset{\leftrightarrow}{\partial}_{\bar{\mu}} H) B_{\bar{\mu}} B_{\bar{\mu}}^2 + \frac{5}{6}g_L g_s y_d^{st} \mathcal{C}_{Hd}^{tr} t_j^{Ii} T_b^{Aa} H^j G_{\bar{\mu}}^A W_{\bar{\mu}}^I (\bar{q}_{ais} d_r^b) \\
& +i\mathcal{C}_{Hd}^{rr} \left[ g_Y (\partial_{\bar{\nu}} H^\dagger \partial_{\bar{\mu}} \partial_{\bar{\nu}} H) B_{\bar{\mu}} - g_Y (\partial_{\bar{\mu}} \partial_{\bar{\nu}} H^\dagger \partial_{\bar{\nu}} H) B_{\bar{\mu}} \right] \\
& +iy_d^{rt} \bar{y}_d^{rs} \mathcal{C}_{Hd}^{ts} \left[ g_L (H^\dagger \partial_{\bar{\mu}} H) (H^\dagger t^I H) W_{\bar{\mu}}^I - g_L (\partial_{\bar{\mu}} H^\dagger H) (H^\dagger t^I H) W_{\bar{\mu}}^I \right] + g_L g_Y \mathcal{C}_{Hd}^{rr} (\partial_{\bar{\mu}} H^\dagger t^I \partial_{\bar{\nu}} H) B_{\bar{\mu}} W_{\bar{\nu}}^I \\
& +g_L g_Y \mathcal{C}_{Hd}^{rr} (\partial_{\bar{\nu}} H^\dagger t^I \partial_{\bar{\mu}} H) B_{\bar{\mu}} W_{\bar{\nu}}^I + g_L g_Y \mathcal{C}_{Hd}^{rr} (H^\dagger t^I \partial_{\bar{\nu}} H) B_{\bar{\mu}} \partial^{\bar{\nu}} W_{\bar{\mu}}^I + g_L g_Y \mathcal{C}_{Hd}^{rr} (\partial_{\bar{\nu}} H^\dagger t^I H) B_{\bar{\mu}} \partial^{\bar{\nu}} W_{\bar{\mu}}^I \\
& +\frac{4}{3}g_L g_s^2 \mathcal{C}_{Hd}^{rr} G_{\bar{\mu}}^A W_{\bar{\nu}}^I \tilde{G}^{\bar{\mu}\bar{\nu}A} (H^\dagger t^I H) + \frac{83}{54}g_L g_Y^3 \mathcal{C}_{Hd}^{rr} (H^\dagger t^I H) B_{\bar{\mu}} B_{\bar{\mu}}^2 W_{\bar{\mu}}^I + 2g_L g_Y \mathcal{C}_{Hd}^{rr} (\partial_{\bar{\nu}} H^\dagger t^I \partial_{\bar{\nu}} H) B_{\bar{\mu}} W_{\bar{\mu}}^I \\
& +2g_L^2 y_d^{rt} \bar{y}_d^{rs} \mathcal{C}_{Hd}^{ts} (H^\dagger t^I H) (H^\dagger t^J H) W_{\bar{\mu}}^I W_{\bar{\mu}}^J - \frac{1}{2}g_L^2 g_Y \mathcal{C}_{Hd}^{tt} (\bar{\ell}_s H \bar{B} H^\dagger \ell_s) - \frac{1}{2}g_L^2 g_Y \mathcal{C}_{Hd}^{tt} (\bar{q}_s H \bar{B} H^\dagger q_s) \\
& -\frac{2i}{3}g_s \bar{y}_d^{rt} \mathcal{C}_{Hd}^{st} T_b^{Aa} G_{\bar{\mu}}^A (\bar{d}_{as} \partial^{\bar{\mu}} H^\dagger q_r^b) + \frac{2i}{3}g_s y_d^{st} \mathcal{C}_{Hd}^{tr} T_b^{Aa} G_{\bar{\mu}}^A (\bar{q}_{as} \partial^{\bar{\mu}} H d_r^b) \\
& -\frac{5i}{6}g_L g_s \bar{y}_d^{rt} \mathcal{C}_{Hd}^{st} t_j^{Ii} T_b^{Aa} H_i^\dagger G_{\bar{\mu}}^A W_{\bar{\nu}}^I (\bar{d}_{as} \sigma^{\bar{\mu}\bar{\nu}} q_r^{bj}) - \frac{5}{6}g_s \bar{y}_d^{rt} \mathcal{C}_{Hd}^{st} T_b^{Aa} G_{\bar{\mu}}^A (\bar{d}_{as} \sigma^{\bar{\mu}\bar{\nu}} \partial^{\bar{\nu}} H^\dagger q_r^b) \\
& -\frac{5}{6}g_s y_d^{st} \mathcal{C}_{Hd}^{tr} T_b^{Aa} G_{\bar{\mu}}^A (\bar{q}_{as} \partial^{\bar{\nu}} H \sigma^{\bar{\mu}\bar{\nu}} d_r^b) + \frac{5i}{6}g_L g_s y_d^{st} \mathcal{C}_{Hd}^{tr} t_j^{Ii} T_b^{Aa} H^j G_{\bar{\mu}}^A W_{\bar{\nu}}^I (\bar{q}_{ais} \sigma^{\bar{\mu}\bar{\nu}} d_r^b) \\
& -g_L g_Y \mathcal{C}_{Hd}^{rr} (H^\dagger t^I \partial_{\bar{\mu}} \partial_{\bar{\nu}} H) B_{\bar{\mu}} W_{\bar{\nu}}^I - g_L \mathcal{C}_{Hd}^{rr} \left[ g_Y B_{\bar{\mu}} W^{\bar{\mu}\bar{\nu}I} (H^\dagger t^I \partial_{\bar{\nu}} H) + g_Y B_{\bar{\mu}} W^{\bar{\mu}\bar{\nu}I} (\partial_{\bar{\nu}} H^\dagger t^I H) \right] \\
& -g_L g_Y \mathcal{C}_{Hd}^{rr} (\partial_{\bar{\mu}} \partial_{\bar{\nu}} H^\dagger t^I H) B_{\bar{\mu}} W_{\bar{\nu}}^I - g_L^2 g_Y \mathcal{C}_{Hd}^{rr} \varepsilon^{IJK} B_{\bar{\mu}} W_{\bar{\nu}}^J W^{\bar{\mu}\bar{\nu}I} (H^\dagger t^K H) \\
& -g_L^2 g_Y \mathcal{C}_{Hd}^{rr} \varepsilon^{IJK} (H^\dagger t^K H) B_{\bar{\mu}} W_{\bar{\nu}}^I \partial^{\bar{\nu}} W_{\bar{\mu}}^J + \frac{10i}{9}g_L g_Y^2 \mathcal{C}_{Hd}^{rr} (H^\dagger t^I \overset{\leftrightarrow}{\partial}_{\bar{\nu}} H) B_{\bar{\mu}}^2 W_{\bar{\nu}}^I \\
& +2ig_L g_Y^2 \mathcal{C}_{Hd}^{rr} (H^\dagger t^I \overset{\leftrightarrow}{\partial}_{\bar{\nu}} H) B_{\bar{\mu}} B_{\bar{\nu}} W_{\bar{\mu}}^I, \tag{2.33}
\end{aligned}$$

$$\begin{aligned}
\Delta S_{\mathcal{O}_{Hud}} &= \frac{1}{18}g_Y \left[ -y_d^{ur} \bar{y}_u^{ut} \bar{\mathcal{C}}_{Hud}^{ts} - y_u^{tu} \bar{y}_d^{ts} \mathcal{C}_{Hud}^{ur} \right] (H^\dagger H) (\bar{d}_s \bar{B} d_r) - \frac{i}{18}g_Y y_d^{st} \bar{\mathcal{C}}_{Hud}^{rt} B_{\bar{\mu}} (\bar{q}_s \tilde{H} \partial^{\bar{\mu}} u_r) \\
& +\frac{i}{18}g_Y \bar{y}_d^{rt} \mathcal{C}_{Hud}^{st} B_{\bar{\mu}} (\bar{u}_s \tilde{H}^\dagger \partial^{\bar{\mu}} q_r) - \frac{i}{18}g_Y y_d^{st} \bar{\mathcal{C}}_{Hud}^{rt} B_{\bar{\mu}} (\partial^{\bar{\mu}} \bar{q}_s \tilde{H} u_r) + \frac{i}{18}g_Y \bar{y}_d^{rt} \mathcal{C}_{Hud}^{st} B_{\bar{\mu}} (\partial^{\bar{\mu}} \bar{u}_s \tilde{H}^\dagger q_r) \\
& +\frac{i}{9}g_Y \bar{y}_u^{rt} \bar{\mathcal{C}}_{Hud}^{ts} B_{\bar{\mu}} (\bar{d}_s H^\dagger \partial^{\bar{\mu}} q_r) - \frac{i}{9}g_Y y_u^{st} \mathcal{C}_{Hud}^{tr} B_{\bar{\mu}} (\bar{q}_s H \partial^{\bar{\mu}} d_r) \\
& +\frac{1}{9}g_Y \left[ y_d^{ut} \bar{y}_u^{us} \bar{\mathcal{C}}_{Hud}^{rt} + y_u^{tr} \bar{y}_d^{tu} \mathcal{C}_{Hud}^{su} \right] (H^\dagger H) (\bar{u}_s \bar{B} u_r) + \frac{i}{9}g_Y \bar{y}_u^{rt} \bar{\mathcal{C}}_{Hud}^{ts} B_{\bar{\mu}} (\partial^{\bar{\mu}} \bar{d}_s H^\dagger q_r)
\end{aligned}$$

$$\begin{aligned}
& -\frac{i}{9}g_Y y_u^{st} \mathcal{C}_{Hud}^{tr} B_{\bar{\mu}} (\partial^{\bar{\mu}} \bar{q}_s H d_r) + \frac{1}{6}g_s \left[ y_d^{ur} \bar{y}_u^{ut} \bar{\mathcal{C}}_{Hud}^{ts} + y_u^{tu} \bar{y}_d^{ts} \mathcal{C}_{Hud}^{ur} \right] (H^\dagger H) (\bar{d}_s T^A \bar{\mathcal{G}}^A d_r) \\
& + \frac{i}{6}g_s \bar{y}_u^{rt} \bar{\mathcal{C}}_{Hud}^{ts} T_b^{Aa} G_{\bar{\mu}}^A (\bar{d}_{as} H^\dagger \partial^{\bar{\mu}} q_r^b) + \frac{1}{6}g_s^2 \bar{y}_u^{rt} \bar{\mathcal{C}}_{Hud}^{ts} T_b^{Aa} T_a^{Bc} G_{\bar{\mu}}^A G_{\bar{\mu}}^B (\bar{d}_{cs} H^\dagger q_r^b) \\
& + \frac{1}{6}g_s^2 y_u^{st} \mathcal{C}_{Hud}^{tr} T_b^{Aa} T_c^{Bb} G_{\bar{\mu}}^A G_{\bar{\mu}}^B (\bar{q}_{as} H d_r^c) - \frac{i}{6}g_s y_u^{st} \mathcal{C}_{Hud}^{tr} T_b^{Aa} G_{\bar{\mu}}^A (\bar{q}_{as} H \partial^{\bar{\mu}} d_r^b) \\
& + \frac{i}{6}g_s y_d^{st} \bar{\mathcal{C}}_{Hud}^{rt} T_b^{Aa} G_{\bar{\mu}}^A (\bar{q}_{as} \tilde{H} \partial^{\bar{\mu}} u_r^b) + \frac{1}{6}g_s \left[ y_d^{ut} \bar{y}_u^{us} \bar{\mathcal{C}}_{Hud}^{rt} + y_u^{tr} \bar{y}_d^{tu} \mathcal{C}_{Hud}^{su} \right] (H^\dagger H) (\bar{u}_s T^A \bar{\mathcal{G}}^A u_r) \\
& + \frac{i}{6}g_s \bar{y}_u^{rt} \bar{\mathcal{C}}_{Hud}^{ts} T_b^{Aa} G_{\bar{\mu}}^A (\partial^{\bar{\mu}} \bar{d}_{as} H^\dagger q_r^b) - \frac{i}{6}g_s y_u^{st} \mathcal{C}_{Hud}^{tr} T_b^{Aa} G_{\bar{\mu}}^A (\partial^{\bar{\mu}} \bar{q}_{as} H d_r^b) \\
& + \frac{i}{6}g_s y_d^{st} \bar{\mathcal{C}}_{Hud}^{rt} T_b^{Aa} G_{\bar{\mu}}^A (\partial^{\bar{\mu}} \bar{q}_{as} \tilde{H} u_r^b) - \frac{i}{6}g_s \bar{y}_d^{rt} \mathcal{C}_{Hud}^{st} T_b^{Aa} G_{\bar{\mu}}^A (\partial^{\bar{\mu}} \bar{u}_{as} \tilde{H}^\dagger q_r^b) \\
& + \frac{2i}{9}g_Y \bar{y}_d^{rt} \mathcal{C}_{Hud}^{st} B_{\bar{\mu}} (\bar{u}_s \partial^{\bar{\mu}} \tilde{H} q_r) + \frac{1}{4}g_L^2 \left[ y_d^{ts} \bar{y}_u^{tr} \bar{\mathcal{C}}_{Hud}^{rs} + y_u^{rt} \bar{y}_d^{rs} \mathcal{C}_{Hud}^{ts} \right] (H^\dagger H)^2 W_{\bar{\mu}}^{I2} \\
& + \frac{5}{18}g_Y y_d^{st} \bar{\mathcal{C}}_{Hud}^{rt} B_{\bar{\mu}} (\bar{q}_s \partial^{\bar{\nu}} \tilde{H} \sigma^{\bar{\mu}\bar{\nu}} u_r) + \frac{5i}{18}g_L g_Y \bar{y}_d^{rt} \mathcal{C}_{Hud}^{st} \bar{\epsilon}_{ij} t_k^{Ii} H^k B_{\bar{\mu}} W_{\bar{\nu}}^I (\bar{u}_s \sigma^{\bar{\mu}\bar{\nu}} q_r^j) \\
& + \frac{5}{18}g_Y \bar{y}_d^{rt} \mathcal{C}_{Hud}^{st} B_{\bar{\mu}} (\bar{u}_s \sigma^{\bar{\mu}\bar{\nu}} \partial^{\bar{\nu}} \tilde{H} q_r) + \frac{1}{3}g_L \left[ -y_d^{ur} \bar{y}_u^{ut} \bar{\mathcal{C}}_{Hud}^{ts} - y_u^{tu} \bar{y}_d^{ts} \mathcal{C}_{Hud}^{ur} \right] (H^\dagger t^I H) (\bar{d}_s \bar{W}^I d_r) \\
& + \frac{1}{3}g_L \left[ y_d^{ut} \bar{y}_u^{us} \bar{\mathcal{C}}_{Hud}^{rt} + y_u^{tr} \bar{y}_d^{tu} \mathcal{C}_{Hud}^{su} \right] (H^\dagger t^I H) (\bar{u}_s \bar{W}^I u_r) + \frac{19}{54}g_Y^2 \bar{y}_u^{rt} \bar{\mathcal{C}}_{Hud}^{ts} B_{\bar{\mu}}^2 (\bar{d}_s H^\dagger q_r) \\
& + \frac{19}{54}g_Y^2 y_u^{st} \mathcal{C}_{Hud}^{tr} B_{\bar{\mu}}^2 (\bar{q}_s H d_r) - \frac{5i}{12}g_s g_Y y_u^{st} \mathcal{C}_{Hud}^{tr} T_b^{Aa} B_{\bar{\mu}} G_{\bar{\nu}}^A (\bar{q}_{as} H \sigma^{\bar{\mu}\bar{\nu}} d_r^b) \\
& - \frac{5i}{12}g_s g_Y y_d^{st} \bar{\mathcal{C}}_{Hud}^{rt} T_b^{Aa} B_{\bar{\mu}} G_{\bar{\nu}}^A (\bar{q}_{as} \tilde{H} \sigma^{\bar{\mu}\bar{\nu}} u_r^b) - \frac{4i}{9}g_Y \bar{y}_u^{rt} \bar{\mathcal{C}}_{Hud}^{ts} B_{\bar{\mu}} (\bar{d}_s \partial^{\bar{\mu}} H^\dagger q_r) \\
& - \frac{i}{2} \left[ y_d^{ts} \bar{y}_u^{tr} \bar{\mathcal{C}}_{Hud}^{rs} + y_u^{rt} \bar{y}_d^{rs} \mathcal{C}_{Hud}^{ts} \right] \left[ g_L (H^\dagger \partial_{\bar{\mu}} H) (H^\dagger t^I H) W_{\bar{\mu}}^I - g_L (\partial_{\bar{\mu}} H^\dagger H) (H^\dagger t^I H) W_{\bar{\mu}}^I \right] \\
& + \frac{i}{2} \left[ y_d^{ts} \bar{y}_u^{tr} \bar{\mathcal{C}}_{Hud}^{rs} - y_u^{rt} \bar{y}_d^{rs} \mathcal{C}_{Hud}^{ts} \right] \left[ g_L (H^\dagger \partial_{\bar{\mu}} H) (H^\dagger t^I H) W_{\bar{\mu}}^I + g_L (\partial_{\bar{\mu}} H^\dagger H) (H^\dagger t^I H) W_{\bar{\mu}}^I \right] \\
& - \frac{i}{2} \left[ y_d^{ts} \bar{y}_u^{tr} \bar{\mathcal{C}}_{Hud}^{rs} - y_u^{rt} \bar{y}_d^{rs} \mathcal{C}_{Hud}^{ts} \right] \left[ g_L (H^\dagger H) (H^\dagger t^I \partial_{\bar{\mu}} H) W_{\bar{\mu}}^I + g_L (H^\dagger H) (\partial_{\bar{\mu}} H^\dagger t^I H) W_{\bar{\mu}}^I \right] \\
& + \frac{i}{2}g_L \left[ y_d^{ts} \bar{y}_u^{tr} \bar{\mathcal{C}}_{Hud}^{rs} + y_u^{rt} \bar{y}_d^{rs} \mathcal{C}_{Hud}^{ts} \right] (H^\dagger t^I \partial_{\bar{\mu}} H) (H^\dagger H) W_{\bar{\mu}}^I + \frac{19}{36}g_s g_Y y_d^{st} \bar{\mathcal{C}}_{Hud}^{rt} T_b^{Aa} B_{\bar{\mu}} G_{\bar{\mu}}^A (\bar{q}_{as} \tilde{H} u_r^b) \\
& + \frac{19}{36}g_s g_Y \bar{y}_d^{rt} \mathcal{C}_{Hud}^{st} T_b^{Aa} B_{\bar{\mu}} G_{\bar{\mu}}^A (\bar{u}_{as} \tilde{H}^\dagger q_r^b) + \frac{5}{9}g_L g_Y \bar{y}_u^{rt} \bar{\mathcal{C}}_{Hud}^{ts} t_j^{Ii} H_i^\dagger B_{\bar{\mu}} W_{\bar{\mu}}^I (\bar{d}_s q_r^j) \\
& - \frac{5i}{9}g_L g_Y \bar{y}_u^{rt} \bar{\mathcal{C}}_{Hud}^{ts} t_j^{Ii} H_i^\dagger B_{\bar{\mu}} W_{\bar{\nu}}^I (\bar{d}_s \sigma^{\bar{\mu}\bar{\nu}} q_r^j) + \frac{5}{9}g_L g_Y y_u^{st} \mathcal{C}_{Hud}^{tr} t_j^{Ii} H^j B_{\bar{\mu}} W_{\bar{\mu}}^I (\bar{q}_{is} d_r) \\
& + \frac{23}{36}g_s g_Y \bar{y}_u^{rt} \bar{\mathcal{C}}_{Hud}^{ts} T_b^{Aa} B_{\bar{\mu}} G_{\bar{\mu}}^A (\bar{d}_{as} H^\dagger q_r^b) + \frac{2i}{3}g_s y_d^{st} \bar{\mathcal{C}}_{Hud}^{rt} T_b^{Aa} G_{\bar{\mu}}^A (\bar{q}_{as} \partial^{\bar{\mu}} \tilde{H} u_r^b) \\
& + \frac{5}{6}g_s y_d^{st} \bar{\mathcal{C}}_{Hud}^{rt} T_b^{Aa} G_{\bar{\mu}}^A (\bar{q}_{as} \partial^{\bar{\nu}} \tilde{H} \sigma^{\bar{\mu}\bar{\nu}} u_r^b) + \frac{5}{6}g_L g_s \bar{y}_d^{rt} \mathcal{C}_{Hud}^{st} t_k^{Ii} T_b^{Aa} \tilde{H}^{\dagger i} G_{\bar{\mu}}^A W_{\bar{\mu}}^I (\bar{u}_{as} q_r^{bk}) \\
& + \frac{5}{6}g_s \bar{y}_d^{rt} \mathcal{C}_{Hud}^{st} T_b^{Aa} G_{\bar{\mu}}^A (\bar{u}_{as} \sigma^{\bar{\mu}\bar{\nu}} \partial^{\bar{\nu}} \tilde{H} q_r^b) + g_L^2 \left[ -y_d^{ts} \bar{y}_u^{tr} \bar{\mathcal{C}}_{Hud}^{rs} - y_u^{rt} \bar{y}_d^{rs} \mathcal{C}_{Hud}^{ts} \right] (H^\dagger t^I H) (H^\dagger t^J H) W_{\bar{\mu}}^I W_{\bar{\mu}}^J \\
& - \frac{17}{108}g_Y^2 y_d^{st} \bar{\mathcal{C}}_{Hud}^{rt} B_{\bar{\mu}}^2 (\bar{q}_s \tilde{H} u_r) - \frac{1}{6}g_s^2 y_d^{st} \bar{\mathcal{C}}_{Hud}^{rt} T_b^{Aa} T_a^{Bc} G_{\bar{\mu}}^A G_{\bar{\mu}}^B (\bar{q}_{cs} \tilde{H} u_r^b) \\
& - \frac{1}{6}g_s^2 \bar{y}_d^{rt} \mathcal{C}_{Hud}^{st} T_b^{Aa} T_c^{Bb} G_{\bar{\mu}}^A G_{\bar{\mu}}^B (\bar{u}_{as} \tilde{H}^\dagger q_r^c) - \frac{i}{6}g_s \bar{y}_d^{rt} \mathcal{C}_{Hud}^{st} T_b^{Aa} G_{\bar{\mu}}^A (\bar{u}_{as} \tilde{H}^\dagger \partial^{\bar{\mu}} q_r^b)
\end{aligned}$$

$$\begin{aligned}
& -\frac{2i}{9}g_Y y_d^{st} \bar{C}_{Hud}^{rt} B_{\bar{\mu}} (\bar{q}_s \partial^{\bar{\mu}} \tilde{H} u_r) - \frac{5}{18} g_L g_Y y_d^{st} \bar{C}_{Hud}^{rt} t_j^{Ik} \tilde{H}_j B_{\bar{\mu}} W_{\bar{\mu}}^I (\bar{q}_{ks} u_r) \\
& - \frac{5i}{18} g_L g_Y y_d^{st} \bar{C}_{Hud}^{rt} \varepsilon^{jk} t_j^{Ii} H_i^\dagger B_{\bar{\mu}} W_{\bar{\nu}}^I (\bar{q}_{ks} \sigma^{\bar{\mu}\bar{\nu}} u_r) + \frac{5i}{12} g_s g_Y \bar{y}_u^{rt} \bar{C}_{Hud}^{ts} T_b^{Aa} B_{\bar{\mu}} G_{\bar{\nu}}^A (\bar{d}_{as} \sigma^{\bar{\mu}\bar{\nu}} H^\dagger q_r^b) \\
& + \frac{5i}{12} g_s g_Y \bar{y}_d^{rt} \bar{C}_{Hud}^{st} T_b^{Aa} B_{\bar{\mu}} G_{\bar{\nu}}^A (\bar{u}_{as} \sigma^{\bar{\mu}\bar{\nu}} \tilde{H}^\dagger q_r^b) + \frac{4i}{9} g_Y y_u^{st} C_{Hud}^{tr} B_{\bar{\mu}} (\bar{q}_s \partial^{\bar{\mu}} H d_r) \\
& - \frac{5}{9} g_Y \bar{y}_u^{rt} \bar{C}_{Hud}^{ts} B_{\bar{\mu}} (\bar{d}_s \sigma^{\bar{\mu}\bar{\nu}} \partial^{\bar{\nu}} H^\dagger q_r) - \frac{5}{9} g_Y y_u^{st} C_{Hud}^{tr} B_{\bar{\mu}} (\bar{q}_s \partial^{\bar{\nu}} H \sigma^{\bar{\mu}\bar{\nu}} d_r) \\
& + \frac{5i}{9} g_L g_Y y_u^{st} C_{Hud}^{tr} t_j^{Ii} H^j B_{\bar{\mu}} W_{\bar{\nu}}^I (\bar{q}_{is} \sigma^{\bar{\mu}\bar{\nu}} d_r) + \frac{23}{36} g_s g_Y y_u^{st} C_{Hud}^{tr} T_b^{Aa} B_{\bar{\mu}} G_{\bar{\mu}}^A (\bar{q}_{as} H d_r^b) \\
& - \frac{2i}{3} g_s \bar{y}_u^{rt} \bar{C}_{Hud}^{ts} T_b^{Aa} G_{\bar{\mu}}^A (\bar{d}_{as} \partial^{\bar{\mu}} H^\dagger q_r^b) + \frac{2i}{3} g_s y_u^{st} C_{Hud}^{tr} T_b^{Aa} G_{\bar{\mu}}^A (\bar{q}_{as} \partial^{\bar{\mu}} H d_r^b) \\
& - \frac{2i}{3} g_s \bar{y}_d^{rt} \bar{C}_{Hud}^{st} T_b^{Aa} G_{\bar{\mu}}^A (\bar{u}_{as} \partial^{\bar{\mu}} \tilde{H} q_r^b) + \frac{5}{6} g_L g_s \bar{y}_u^{rt} \bar{C}_{Hud}^{ts} t_j^{Ii} T_b^{Aa} H_i^\dagger G_{\bar{\mu}}^A W_{\bar{\mu}}^I (\bar{d}_{as} q_r^{bj}) \\
& - \frac{5i}{6} g_L g_s \bar{y}_u^{rt} \bar{C}_{Hud}^{ts} t_j^{Ii} T_b^{Aa} H_i^\dagger G_{\bar{\mu}}^A W_{\bar{\nu}}^I (\bar{d}_{as} \sigma^{\bar{\mu}\bar{\nu}} q_r^{bj}) + \frac{5}{6} g_L g_s y_u^{st} C_{Hud}^{tr} t_j^{Ii} T_b^{Aa} H^j G_{\bar{\mu}}^A W_{\bar{\mu}}^I (\bar{q}_{ais} d_r^b) \\
& - \frac{5}{6} g_s \bar{y}_u^{rt} \bar{C}_{Hud}^{ts} T_b^{Aa} G_{\bar{\mu}}^A (\bar{d}_{as} \sigma^{\bar{\mu}\bar{\nu}} \partial^{\bar{\nu}} H^\dagger q_r^b) - \frac{5}{6} g_s y_u^{st} C_{Hud}^{tr} T_b^{Aa} G_{\bar{\mu}}^A (\bar{q}_{as} \partial^{\bar{\nu}} H \sigma^{\bar{\mu}\bar{\nu}} d_r^b) \\
& + \frac{5i}{6} g_L g_s y_u^{st} C_{Hud}^{tr} t_j^{Ii} T_b^{Aa} H^j G_{\bar{\mu}}^A W_{\bar{\nu}}^I (\bar{q}_{ais} \sigma^{\bar{\mu}\bar{\nu}} d_r^b) + \frac{5}{6} g_L g_s y_d^{st} \bar{C}_{Hud}^{rt} t_j^{Ik} T_b^{Aa} \tilde{H}_j G_{\bar{\mu}}^A W_{\bar{\mu}}^I (\bar{q}_{aks} u_r^b) \\
& - \frac{17}{108} g_Y^2 \bar{y}_d^{rt} \bar{C}_{Hud}^{st} B_{\bar{\mu}}^2 (\bar{u}_s \tilde{H}^\dagger q_r) - \frac{5}{18} g_L g_Y \bar{y}_d^{rt} \bar{C}_{Hud}^{st} t_k^{Ii} \tilde{H}^{\dagger i} B_{\bar{\mu}} W_{\bar{\mu}}^I (\bar{u}_s q_r^k) \\
& + \frac{5i}{6} g_L g_s y_d^{st} \bar{C}_{Hud}^{rt} \varepsilon^{jk} t_j^{Ii} T_b^{Aa} H_i^\dagger G_{\bar{\mu}}^A W_{\bar{\nu}}^I (\bar{q}_{aks} \sigma^{\bar{\mu}\bar{\nu}} u_r^b) \\
& - \frac{5i}{6} g_L g_s \bar{y}_d^{rt} \bar{C}_{Hud}^{st} \varepsilon_{ij} t_k^{Ii} T_b^{Aa} H^k G_{\bar{\mu}}^A W_{\bar{\nu}}^I (\bar{u}_{as} \sigma^{\bar{\mu}\bar{\nu}} q_r^{bj}), \tag{2.34}
\end{aligned}$$

$$\begin{aligned}
\Delta S_{\mathcal{O}_{Hq}^{(1)}} &= \frac{1}{108} g_Y \left[ 5(\mathcal{C}_{Hq}^{(1)})^{sr} \left[ 3g_L^2 - g_Y^2 \right] + 9(\mathcal{C}_{Hq}^{(1)})^{tt} \left[ g_Y^2 - 3g_L^2 \right] \delta^{rs} \right. \\
&\quad \left. + 21y_u^{su} \bar{y}_u^{tu} (\mathcal{C}_{Hq}^{(1)})^{tr} + 21y_u^{ut} \bar{y}_u^{rt} (\mathcal{C}_{Hq}^{(1)})^{su} \right] (H^\dagger H) (\bar{q}_s \bar{B} q_r) \\
&+ \frac{i}{36} g_Y \bar{y}_d^{ts} (\mathcal{C}_{Hq}^{(1)})^{tr} B_{\bar{\mu}} (\bar{d}_s H^\dagger \partial^{\bar{\mu}} q_r) - \frac{i}{36} g_Y y_d^{tr} (\mathcal{C}_{Hq}^{(1)})^{st} B_{\bar{\mu}} (\bar{q}_s H \partial^{\bar{\mu}} d_r) - \frac{i}{36} g_Y y_u^{tr} (\mathcal{C}_{Hq}^{(1)})^{st} B_{\bar{\mu}} (\bar{q}_s \tilde{H} \partial^{\bar{\mu}} u_r) \\
&+ \frac{1}{36} g_L \left[ 3y_d^{su} \bar{y}_d^{tu} (\mathcal{C}_{Hq}^{(1)})^{tr} + 3y_d^{ut} \bar{y}_d^{rt} (\mathcal{C}_{Hq}^{(1)})^{su} - 3y_u^{su} \bar{y}_u^{tu} (\mathcal{C}_{Hq}^{(1)})^{tr} - 3y_u^{ut} \bar{y}_u^{rt} (\mathcal{C}_{Hq}^{(1)})^{su} - 10g_Y^2 (\mathcal{C}_{Hq}^{(1)})^{sr} \right] (H^\dagger H) (\bar{q}_s t^I \bar{W}^I q_r) \\
&+ \frac{1}{36} g_Y \left[ 5y_d^{su} \bar{y}_d^{tu} (\mathcal{C}_{Hq}^{(1)})^{tr} + 5y_d^{ut} \bar{y}_d^{rt} (\mathcal{C}_{Hq}^{(1)})^{su} + 18g_L^2 (\mathcal{C}_{Hq}^{(1)})^{tt} \delta^{rs} \right. \\
&\quad \left. - 7y_u^{su} \bar{y}_u^{tu} (\mathcal{C}_{Hq}^{(1)})^{tr} - 7y_u^{ut} \bar{y}_u^{rt} (\mathcal{C}_{Hq}^{(1)})^{su} - 10g_L^2 (\mathcal{C}_{Hq}^{(1)})^{sr} \right] (\bar{q}_s H \bar{B} H^\dagger q_r) \\
&+ \frac{i}{36} g_Y \bar{y}_u^{ts} (\mathcal{C}_{Hq}^{(1)})^{tr} B_{\bar{\mu}} (\bar{u}_s \tilde{H}^\dagger \partial^{\bar{\mu}} q_r) + \frac{i}{36} g_Y \bar{y}_d^{ts} (\mathcal{C}_{Hq}^{(1)})^{tr} B_{\bar{\mu}} (\partial^{\bar{\mu}} \bar{d}_s H^\dagger q_r) - \frac{i}{36} g_Y y_d^{tr} (\mathcal{C}_{Hq}^{(1)})^{st} B_{\bar{\mu}} (\partial^{\bar{\mu}} \bar{q}_s H d_r) \\
&- \frac{i}{36} g_Y y_u^{tr} (\mathcal{C}_{Hq}^{(1)})^{st} B_{\bar{\mu}} (\partial^{\bar{\mu}} \bar{q}_s \tilde{H} u_r) + \frac{i}{36} g_Y \bar{y}_u^{ts} (\mathcal{C}_{Hq}^{(1)})^{tr} B_{\bar{\mu}} (\partial^{\bar{\mu}} \bar{u}_s \tilde{H}^\dagger q_r) \\
&+ \frac{1}{18} g_s \left[ 3 \left[ y_u^{su} \bar{y}_u^{tu} (\mathcal{C}_{Hq}^{(1)})^{tr} + y_u^{ut} \bar{y}_u^{rt} (\mathcal{C}_{Hq}^{(1)})^{su} \right] + 5(\mathcal{C}_{Hq}^{(1)})^{sr} \left[ 3g_L^2 - g_Y^2 \right] \right] (H^\dagger H) (\bar{q}_s T^A \bar{G}^A q_r) \\
&+ \frac{1}{18} g_Y^2 (\mathcal{C}_{Hq}^{(1)})^{rr} (H^\dagger \partial_{\bar{\mu}} H) B_{\bar{\mu}} \partial^{\bar{\nu}} B_{\bar{\nu}} + \frac{1}{18} g_Y^2 (\mathcal{C}_{Hq}^{(1)})^{rr} (\partial_{\bar{\mu}} H^\dagger H) B_{\bar{\mu}} \partial^{\bar{\nu}} B_{\bar{\nu}} + \frac{7}{108} g_Y^2 \bar{y}_d^{ts} (\mathcal{C}_{Hq}^{(1)})^{tr} B_{\bar{\mu}}^2 (\bar{d}_s H^\dagger q_r)
\end{aligned}$$

$$\begin{aligned}
& + \frac{7}{108} g_Y^2 y_d^{tr} (\mathcal{C}_{Hq}^{(1)})^{st} B_{\bar{\mu}}^2 (\bar{q}_s H d_r) + \frac{1}{12} g_L^2 g_s^2 (\mathcal{C}_{Hq}^{(1)})^{rr} (H^\dagger H) G_{\bar{\mu}}^{A2} W_{\bar{\mu}}^{I2} \\
& + \frac{1}{12} g_L \left[ y_d^{su} \bar{y}_d^{tu} (\mathcal{C}_{Hq}^{(1)})^{tr} + y_d^{ut} \bar{y}_d^{rt} (\mathcal{C}_{Hq}^{(1)})^{su} + y_u^{su} \bar{y}_u^{tu} (\mathcal{C}_{Hq}^{(1)})^{tr} + y_u^{ut} \bar{y}_u^{rt} (\mathcal{C}_{Hq}^{(1)})^{su} - 10 g_L^2 (\mathcal{C}_{Hq}^{(1)})^{sr} \right] (H^\dagger t^I H) (\bar{q}_s \bar{W}^I q_r) \\
& + \frac{1}{12} \left[ y_d^{su} \bar{y}_d^{tu} (\mathcal{C}_{Hq}^{(1)})^{tr} + y_u^{su} \bar{y}_u^{tu} (\mathcal{C}_{Hq}^{(1)})^{tr} - y_d^{ut} \bar{y}_d^{rt} (\mathcal{C}_{Hq}^{(1)})^{su} - y_u^{ut} \bar{y}_u^{rt} (\mathcal{C}_{Hq}^{(1)})^{su} \right] \\
& \quad \left[ g_L t_j^{Ii} H_i^\dagger (\bar{q}_s H \bar{W}^I q_r^j) - g_L t_k^{Ij} H^k (\bar{q}_{js} \bar{W}^I H^\dagger q_r) \right] \\
& + \frac{i}{12} g_L^2 g_Y (\mathcal{C}_{Hq}^{(1)})^{rr} (H^\dagger \overset{\leftrightarrow}{\partial}_{\bar{\mu}} H) B_{\bar{\mu}} W_{\bar{\mu}}^{I2} + \frac{1}{9} g_s^2 g_Y^2 (\mathcal{C}_{Hq}^{(1)})^{rr} (H^\dagger H) B_{\bar{\mu}} B_{\bar{\nu}} G_{\bar{\mu}}^A G_{\bar{\nu}}^A \\
& - \frac{i}{9} g_Y (\mathcal{C}_{Hq}^{(1)})^{rr} \left[ 2 g_Y B_{\bar{\mu}} \tilde{B}^{\bar{\mu}\bar{\sigma}} (H^\dagger \partial_{\bar{\sigma}} H) - 2 g_Y B_{\bar{\mu}} \tilde{B}^{\bar{\mu}\bar{\sigma}} (\partial_{\bar{\sigma}} H^\dagger H) \right] - \frac{i}{9} g_Y \bar{y}_d^{ts} (\mathcal{C}_{Hq}^{(1)})^{tr} B_{\bar{\mu}} (\bar{d}_s \partial^{\bar{\mu}} H^\dagger q_r) \\
& + \frac{i}{9} g_Y y_d^{tr} (\mathcal{C}_{Hq}^{(1)})^{st} B_{\bar{\mu}} (\bar{q}_s \partial^{\bar{\mu}} H d_r) - \frac{i}{9} g_Y y_u^{tr} (\mathcal{C}_{Hq}^{(1)})^{st} B_{\bar{\mu}} (\bar{q}_s \partial^{\bar{\mu}} \tilde{H} u_r) + \frac{i}{9} g_Y \bar{y}_u^{ts} (\mathcal{C}_{Hq}^{(1)})^{tr} B_{\bar{\mu}} (\bar{u}_s \partial^{\bar{\mu}} \tilde{H} q_r) \\
& + \frac{i}{9} g_s^2 g_Y (\mathcal{C}_{Hq}^{(1)})^{rr} (H^\dagger \overset{\leftrightarrow}{\partial}_{\bar{\nu}} H) B_{\bar{\mu}} G_{\bar{\mu}}^A G_{\bar{\nu}}^A + \frac{1}{8} g_L^4 (\mathcal{C}_{Hq}^{(1)})^{rr} (H^\dagger H) W_{\bar{\mu}}^{I2} W_{\bar{\mu}}^{I2} + \frac{5}{36} g_s^2 g_Y^2 (\mathcal{C}_{Hq}^{(1)})^{rr} (H^\dagger H) B_{\bar{\mu}}^2 G_{\bar{\mu}}^{A2} \\
& + \frac{5}{36} g_Y \bar{y}_d^{ts} (\mathcal{C}_{Hq}^{(1)})^{tr} B_{\bar{\mu}} (\bar{d}_s \sigma^{\bar{\mu}\bar{\nu}} \partial^{\bar{\nu}} H^\dagger q_r) + \frac{5}{36} g_Y y_d^{tr} (\mathcal{C}_{Hq}^{(1)})^{st} B_{\bar{\mu}} (\bar{q}_s \partial^{\bar{\nu}} H \sigma^{\bar{\mu}\bar{\nu}} d_r) \\
& + \frac{1}{6} g_s^3 g_Y (\mathcal{C}_{Hq}^{(1)})^{rr} d^{ABC} (H^\dagger H) B_{\bar{\mu}} G_{\bar{\mu}}^A G_{\bar{\nu}}^B G_{\bar{\nu}}^C + \frac{1}{6} g_L^3 g_Y (\mathcal{C}_{Hq}^{(1)})^{rr} (H^\dagger t^I H) B_{\bar{\mu}} W_{\bar{\mu}}^I W_{\bar{\mu}}^{I2} \\
& - \frac{i}{6} g_Y (\mathcal{C}_{Hq}^{(1)})^{rr} \left[ 2 g_L W_{\bar{\mu}}^I \tilde{B}^{\bar{\mu}\bar{\sigma}} (H^\dagger t^I \partial_{\bar{\sigma}} H) - 2 g_L W_{\bar{\mu}}^I \tilde{B}^{\bar{\mu}\bar{\sigma}} (\partial_{\bar{\sigma}} H^\dagger t^I H) \right] \\
& + \frac{i}{6} g_L (\mathcal{C}_{Hq}^{(1)})^{rr} \left[ 2 g_Y B_{\bar{\mu}} \tilde{W}^{\bar{\mu}\bar{\sigma}I} (H^\dagger t^I \partial_{\bar{\sigma}} H) - 2 g_Y B_{\bar{\mu}} \tilde{W}^{\bar{\mu}\bar{\sigma}I} (\partial_{\bar{\sigma}} H^\dagger t^I H) \right] \\
& + \frac{i}{6} g_L \bar{y}_d^{ts} (\mathcal{C}_{Hq}^{(1)})^{tr} t_j^{Ii} H_i^\dagger W_{\bar{\mu}}^I (\bar{d}_s \partial^{\bar{\mu}} q_r^j) + \frac{1}{6} g_L^2 \bar{y}_d^{ts} (\mathcal{C}_{Hq}^{(1)})^{tr} W_{\bar{\mu}}^{I2} (\bar{d}_s H^\dagger q_r) + \frac{1}{6} g_L^2 y_d^{tr} (\mathcal{C}_{Hq}^{(1)})^{st} W_{\bar{\mu}}^{I2} (\bar{q}_s H d_r) \\
& + \frac{1}{6} g_s \left[ - y_d^{su} \bar{y}_d^{tu} (\mathcal{C}_{Hq}^{(1)})^{tr} - y_d^{ut} \bar{y}_d^{rt} (\mathcal{C}_{Hq}^{(1)})^{su} - y_u^{su} \bar{y}_u^{tu} (\mathcal{C}_{Hq}^{(1)})^{tr} - y_u^{ut} \bar{y}_u^{rt} (\mathcal{C}_{Hq}^{(1)})^{su} - 10 g_L^2 (\mathcal{C}_{Hq}^{(1)})^{sr} \right] (\bar{q}_s T^A H \bar{G}^A H^\dagger q_r) \\
& - \frac{i}{6} g_s y_u^{tr} (\mathcal{C}_{Hq}^{(1)})^{st} T_b^{Aa} G_{\bar{\mu}}^A (\bar{q}_{as} \tilde{H} \partial^{\bar{\mu}} u_r^b) + \frac{i}{6} g_L y_u^{tr} (\mathcal{C}_{Hq}^{(1)})^{st} \varepsilon^{jk} t_j^{Ii} H_i^\dagger W_{\bar{\mu}}^I (\bar{q}_{ks} \partial^{\bar{\mu}} u_r) \\
& - \frac{i}{6} g_L y_d^{tr} (\mathcal{C}_{Hq}^{(1)})^{st} t_j^{Ii} H^j W_{\bar{\mu}}^I (\partial^{\bar{\mu}} \bar{q}_{is} d_r) - \frac{i}{6} g_s y_d^{tr} (\mathcal{C}_{Hq}^{(1)})^{st} T_b^{Aa} G_{\bar{\mu}}^A (\partial^{\bar{\mu}} \bar{q}_{as} H d_r^b) \\
& - \frac{i}{6} g_s y_u^{tr} (\mathcal{C}_{Hq}^{(1)})^{st} T_b^{Aa} G_{\bar{\mu}}^A (\partial^{\bar{\mu}} \bar{q}_{as} \tilde{H} u_r^b) + \frac{i}{6} g_L y_u^{tr} (\mathcal{C}_{Hq}^{(1)})^{st} \varepsilon^{jk} t_j^{Ii} H_i^\dagger W_{\bar{\mu}}^I (\partial^{\bar{\mu}} \bar{q}_{ks} u_r) \\
& - \frac{i}{6} g_L \bar{y}_u^{ts} (\mathcal{C}_{Hq}^{(1)})^{tr} \bar{\varepsilon}_{ij} t_k^{Ii} H^k W_{\bar{\mu}}^I (\partial^{\bar{\mu}} \bar{u}_s q_r^j) + \frac{i}{6} g_s \bar{y}_u^{ts} (\mathcal{C}_{Hq}^{(1)})^{tr} T_b^{Aa} G_{\bar{\mu}}^A (\partial^{\bar{\mu}} \bar{u}_{as} \tilde{H}^\dagger q_r^b) \\
& + \frac{i}{6} g_s^3 (\mathcal{C}_{Hq}^{(1)})^{rr} d^{ABC} (H^\dagger \overset{\leftrightarrow}{\partial}_{\bar{\mu}} H) G_{\bar{\mu}}^A G_{\bar{\nu}}^B G_{\bar{\nu}}^C \\
& + \frac{i}{6} g_s^3 (\mathcal{C}_{Hq}^{(1)})^{rr} f^{ABC} G_{\bar{\mu}}^A G_{\bar{\nu}}^B G_{\bar{\rho}}^C \varepsilon^{\bar{\mu}\bar{\nu}\bar{\rho}\bar{\sigma}} (H^\dagger \overset{\leftrightarrow}{\partial}_{\bar{\sigma}} H) \\
& - \frac{i}{6} g_L^2 g_Y (\mathcal{C}_{Hq}^{(1)})^{rr} \varepsilon^{IJK} B_{\bar{\mu}} W_{\bar{\nu}}^I W_{\bar{\rho}}^J \varepsilon^{\bar{\mu}\bar{\nu}\bar{\rho}\bar{\sigma}} (H^\dagger t^K \overset{\leftrightarrow}{\partial}_{\bar{\sigma}} H) \\
& + \frac{2}{9} g_L g_s^2 g_Y (\mathcal{C}_{Hq}^{(1)})^{rr} (H^\dagger t^I H) B_{\bar{\mu}} G_{\bar{\mu}}^A G_{\bar{\nu}}^A W_{\bar{\nu}}^I + \frac{2i}{9} g_s^2 g_Y (\mathcal{C}_{Hq}^{(1)})^{rr} (H^\dagger \overset{\leftrightarrow}{\partial}_{\bar{\mu}} H) B_{\bar{\mu}} G_{\bar{\mu}}^{A2} \\
& + \frac{i}{4} g_Y \left[ (\mathcal{C}_{Hq}^{(1)})^{rr} \left[ g_L^2 + g_Y^2 \right] - 4 y_d^{ts} \bar{y}_d^{rs} (\mathcal{C}_{Hq}^{(1)})^{rt} \right] (H^\dagger \overset{\leftrightarrow}{\partial}_{\bar{\mu}} H) (H^\dagger H) B_{\bar{\mu}}
\end{aligned}$$

$$\begin{aligned}
& + \frac{i}{4} g_L^3 (\mathcal{C}_{Hq}^{(1)})^{rr} \varepsilon^{IJK} W_{\bar{\mu}}^I W_{\bar{\nu}}^J W_{\bar{\rho}}^K \varepsilon^{\bar{\mu}\bar{\nu}\bar{\rho}\bar{\sigma}} (H^\dagger \overset{\leftrightarrow}{\partial}_{\bar{\sigma}} H) \\
& + \frac{5i}{18} g_L g_Y y_d^{tr} (\mathcal{C}_{Hq}^{(1)})^{st} t_j^{Ii} H^j B_{\bar{\mu}} W_{\bar{\nu}}^I (\bar{q}_{is} \sigma^{\bar{\mu}\bar{\nu}} d_r) + \frac{1}{3} g_s^2 (\mathcal{C}_{Hq}^{(1)})^{rr} (H^\dagger \partial_{\bar{\mu}} \partial_{\bar{\nu}} H) G_{\bar{\mu}}^A G_{\bar{\nu}}^A \\
& + \frac{1}{3} g_s (\mathcal{C}_{Hq}^{(1)})^{rr} \left[ g_s G_{\bar{\mu}}^A G^{\bar{\mu}\bar{\nu}A} (H^\dagger \partial_{\bar{\nu}} H) + g_s G_{\bar{\mu}}^A G^{\bar{\mu}\bar{\nu}A} (\partial_{\bar{\nu}} H^\dagger H) \right] + \frac{1}{3} g_s^2 (\mathcal{C}_{Hq}^{(1)})^{rr} (\partial_{\bar{\nu}} H^\dagger \partial_{\bar{\nu}} H) G_{\bar{\mu}}^{A^2} \\
& + \frac{1}{3} g_s^2 (\mathcal{C}_{Hq}^{(1)})^{rr} (\partial_{\bar{\mu}} \partial_{\bar{\nu}} H^\dagger H) G_{\bar{\mu}}^A G_{\bar{\nu}}^A + \frac{1}{3} g_L g_s^3 (\mathcal{C}_{Hq}^{(1)})^{rr} d^{ABC} (H^\dagger t^I H) G_{\bar{\mu}}^A G_{\bar{\nu}}^B G_{\bar{\rho}}^C W_{\bar{\sigma}}^I \\
& + \frac{1}{3} g_L^3 g_Y (\mathcal{C}_{Hq}^{(1)})^{rr} (H^\dagger t^I H) B_{\bar{\mu}} W_{\bar{\mu}}^J W_{\bar{\nu}}^I W_{\bar{\nu}}^J + \frac{1}{3} g_L g_s^3 (\mathcal{C}_{Hq}^{(1)})^{rr} f^{ABC} (H^\dagger t^I H) G_{\bar{\mu}}^A G_{\bar{\nu}}^B G_{\bar{\rho}}^C W_{\bar{\sigma}}^I \varepsilon^{\bar{\mu}\bar{\nu}\bar{\rho}\bar{\sigma}} \\
& + \frac{1}{3} g_L g_Y y_u^{tr} (\mathcal{C}_{Hq}^{(1)})^{st} t_j^{Ii} \tilde{H}_j B_{\bar{\mu}} W_{\bar{\mu}}^I (\bar{q}_{ks} u_r) + \frac{1}{3} g_L g_Y \bar{y}_u^{ts} (\mathcal{C}_{Hq}^{(1)})^{tr} t_k^{Ii} \tilde{H}^{\dagger i} B_{\bar{\mu}} W_{\bar{\mu}}^I (\bar{u}_s q_r^k) \\
& + \frac{1}{3} g_Y^3 (\mathcal{C}_{Hq}^{(1)})^{tt} (H^\dagger H) (\bar{u}_s \tilde{B} u_s) + \frac{1}{3} g_s^2 (\mathcal{C}_{Hq}^{(1)})^{rr} (H^\dagger \partial_{\bar{\mu}} H) G_{\bar{\mu}}^A \partial^{\bar{\nu}} G_{\bar{\nu}}^A \\
& + \frac{1}{3} g_s^2 (\mathcal{C}_{Hq}^{(1)})^{rr} (\partial_{\bar{\mu}} H^\dagger H) G_{\bar{\mu}}^A \partial^{\bar{\nu}} G_{\bar{\nu}}^A - \frac{i}{3} g_Y (\mathcal{C}_{Hq}^{(1)})^{rr} \partial^{\bar{\mu}} \partial^{\bar{\nu}} B_{\bar{\nu}} (H^\dagger \overset{\leftrightarrow}{\partial}_{\bar{\mu}} H) \\
& - \frac{i}{3} g_L^2 g_Y (\mathcal{C}_{Hq}^{(1)})^{rr} (H^\dagger \overset{\leftrightarrow}{\partial}_{\bar{\nu}} H) B_{\bar{\mu}} W_{\bar{\mu}}^I W_{\bar{\nu}}^I + \frac{i}{3} g_L g_s^2 (\mathcal{C}_{Hq}^{(1)})^{rr} (H^\dagger t^I \overset{\leftrightarrow}{\partial}_{\bar{\nu}} H) G_{\bar{\mu}}^{A^2} W_{\bar{\nu}}^I \\
& + \frac{13}{36} g_s g_Y y_d^{tr} (\mathcal{C}_{Hq}^{(1)})^{st} T_b^{Aa} B_{\bar{\mu}} G_{\bar{\mu}}^A (\bar{q}_{as} H d_r^b) + \frac{4}{9} g_L g_s^2 g_Y (\mathcal{C}_{Hq}^{(1)})^{rr} (H^\dagger t^I H) B_{\bar{\mu}} G_{\bar{\mu}}^{A^2} W_{\bar{\mu}}^I \\
& + \frac{1}{2} g_L^2 (\mathcal{C}_{Hq}^{(1)})^{rr} (H^\dagger \partial_{\bar{\mu}} \partial_{\bar{\nu}} H) W_{\bar{\mu}}^I W_{\bar{\nu}}^I + \frac{1}{2} g_L (\mathcal{C}_{Hq}^{(1)})^{rr} \left[ g_L W_{\bar{\mu}}^I W^{\bar{\mu}\bar{\nu}I} (H^\dagger \partial_{\bar{\nu}} H) + g_L W_{\bar{\mu}}^I W^{\bar{\mu}\bar{\nu}I} (\partial_{\bar{\nu}} H^\dagger H) \right] \\
& + \frac{1}{2} g_L^2 (\mathcal{C}_{Hq}^{(1)})^{rr} (\partial_{\bar{\nu}} H^\dagger \partial_{\bar{\nu}} H) W_{\bar{\mu}}^{I^2} + \frac{1}{2} g_L^2 (\mathcal{C}_{Hq}^{(1)})^{rr} (\partial_{\bar{\mu}} \partial_{\bar{\nu}} H^\dagger H) W_{\bar{\mu}}^I W_{\bar{\nu}}^I \\
& + \frac{1}{2} g_L g_Y \bar{y}_d^{ts} (\mathcal{C}_{Hq}^{(1)})^{tr} t_j^{Ii} H_i^\dagger B_{\bar{\mu}} W_{\bar{\mu}}^I (\bar{d}_s q_r^j) + \frac{1}{2} g_L g_s y_d^{tr} (\mathcal{C}_{Hq}^{(1)})^{st} t_j^{Ii} T_b^{Aa} H^j G_{\bar{\mu}}^A W_{\bar{\mu}}^I (\bar{q}_{ais} d_r^b) \\
& + \frac{1}{2} g_L^2 (\mathcal{C}_{Hq}^{(1)})^{rr} (H^\dagger \partial_{\bar{\mu}} H) W_{\bar{\mu}}^I \partial^{\bar{\nu}} W_{\bar{\nu}}^I + \frac{1}{2} g_L^2 (\mathcal{C}_{Hq}^{(1)})^{rr} (\partial_{\bar{\mu}} H^\dagger H) W_{\bar{\mu}}^I \partial^{\bar{\nu}} W_{\bar{\nu}}^I \\
& + \frac{i}{2} g_L^3 (\mathcal{C}_{Hq}^{(1)})^{rr} (H^\dagger t^I \overset{\leftrightarrow}{\partial}_{\bar{\mu}} H) W_{\bar{\mu}}^I W_{\bar{\mu}}^{I^2} + \frac{5}{9} g_Y^2 (\mathcal{C}_{Hq}^{(1)})^{rr} (H^\dagger \partial_{\bar{\mu}} \partial_{\bar{\nu}} H) B_{\bar{\mu}} B_{\bar{\nu}} \\
& + \frac{5}{9} g_Y (\mathcal{C}_{Hq}^{(1)})^{rr} \left[ g_Y B_{\bar{\mu}} B^{\bar{\mu}\bar{\nu}} (H^\dagger \partial_{\bar{\nu}} H) + g_Y B_{\bar{\mu}} B^{\bar{\mu}\bar{\nu}} (\partial_{\bar{\nu}} H^\dagger H) \right] + \frac{5}{9} g_Y^2 (\mathcal{C}_{Hq}^{(1)})^{rr} (\partial_{\bar{\mu}} \partial_{\bar{\nu}} H^\dagger H) B_{\bar{\mu}} B_{\bar{\nu}} \\
& + \frac{2}{3} g_s^2 (\mathcal{C}_{Hq}^{(1)})^{rr} (\partial_{\bar{\mu}} H^\dagger \partial_{\bar{\nu}} H) G_{\bar{\mu}}^A G_{\bar{\nu}}^A \\
& - \frac{2i}{3} g_s (\mathcal{C}_{Hq}^{(1)})^{rr} \left[ 2g_s G_{\bar{\mu}}^A \tilde{G}^{\bar{\mu}\bar{\sigma}A} (H^\dagger \partial_{\bar{\sigma}} H) - 2g_s G_{\bar{\mu}}^A \tilde{G}^{\bar{\mu}\bar{\sigma}A} (\partial_{\bar{\sigma}} H^\dagger H) \right] \\
& - \frac{2i}{3} g_L \bar{y}_d^{ts} (\mathcal{C}_{Hq}^{(1)})^{tr} t_j^{Ii} W_{\bar{\mu}}^I (\bar{d}_s q_r^j) \partial^{\bar{\mu}} H_i^\dagger - \frac{2i}{3} g_L y_u^{tr} (\mathcal{C}_{Hq}^{(1)})^{st} \varepsilon^{ij} t_i^{Ik} W_{\bar{\mu}}^I (\bar{q}_{js} u_r) \partial^{\bar{\mu}} H_k^\dagger \\
& + \frac{2i}{3} g_L y_d^{tr} (\mathcal{C}_{Hq}^{(1)})^{st} t_j^{Ii} W_{\bar{\mu}}^I (\bar{q}_{is} d_r) \partial^{\bar{\mu}} H^j + \frac{2i}{3} g_L \bar{y}_u^{ts} (\mathcal{C}_{Hq}^{(1)})^{tr} \bar{\varepsilon}_{ij} t_k^{Ii} W_{\bar{\mu}}^I (\bar{u}_s q_r^j) \partial^{\bar{\mu}} H^k \\
& + \frac{2}{3} g_s^2 (\mathcal{C}_{Hq}^{(1)})^{rr} (H^\dagger \partial_{\bar{\nu}} H) G_{\bar{\mu}}^A \partial^{\bar{\nu}} G_{\bar{\mu}}^A + \frac{2}{3} g_s^2 (\mathcal{C}_{Hq}^{(1)})^{rr} (\partial_{\bar{\nu}} H^\dagger H) G_{\bar{\mu}}^A \partial^{\bar{\nu}} G_{\bar{\mu}}^A \\
& + \frac{5}{6} g_s y_d^{tr} (\mathcal{C}_{Hq}^{(1)})^{st} T_b^{Aa} G_{\bar{\mu}}^A (\bar{q}_{as} \partial^{\bar{\nu}} H \sigma^{\bar{\mu}\bar{\nu}} d_r^b) + \frac{5}{6} g_s y_u^{tr} (\mathcal{C}_{Hq}^{(1)})^{st} T_b^{Aa} G_{\bar{\mu}}^A (\bar{q}_{as} \partial^{\bar{\nu}} \tilde{H} \sigma^{\bar{\mu}\bar{\nu}} u_r^b) \\
& + \frac{5}{6} g_L \bar{y}_d^{ts} (\mathcal{C}_{Hq}^{(1)})^{tr} t_j^{Ii} W_{\bar{\mu}}^I (\bar{d}_s \sigma^{\bar{\mu}\bar{\nu}} q_r^j) \partial^{\bar{\nu}} H_i^\dagger + \frac{5}{6} g_L y_d^{tr} (\mathcal{C}_{Hq}^{(1)})^{st} t_j^{Ii} W_{\bar{\mu}}^I (\bar{q}_{is} \sigma^{\bar{\mu}\bar{\nu}} d_r) \partial^{\bar{\nu}} H^j
\end{aligned}$$

$$\begin{aligned}
& + g_Y^2 \left[ \frac{1}{4} (\mathcal{C}_{Hq}^{(1)})^{rr} \left[ g_L^2 + g_Y^2 \right] - y_d^{ts} \bar{y}_d^{rs} (\mathcal{C}_{Hq}^{(1)})^{rt} \right] (H^\dagger H)^2 B_\mu^2 + g_L^2 (\mathcal{C}_{Hq}^{(1)})^{rr} (\partial_\mu H^\dagger \partial_\nu H) W_\mu^I W_\nu^I \\
& - i g_L (\mathcal{C}_{Hq}^{(1)})^{rr} \left[ 2 g_L W_\mu^I \widetilde{W}^{\mu\bar{\sigma}I} (H^\dagger \partial_\sigma H) - 2 g_L W_\mu^I \widetilde{W}^{\mu\bar{\sigma}I} (\partial_\sigma H^\dagger H) \right] \\
& - i (\mathcal{C}_{Hq}^{(1)})^{rr} \left[ g_Y (\partial_\nu H^\dagger \partial_\mu \partial_\nu H) B_\mu - g_Y (\partial_\mu \partial_\nu H^\dagger \partial_\nu H) B_\mu \right] \\
& + g_L g_Y \left[ \frac{1}{2} (\mathcal{C}_{Hq}^{(1)})^{rr} \left[ g_L^2 + g_Y^2 \right] + 2 (\mathcal{C}_{Hq}^{(1)})^{rt} \left[ 2 y_u^{ts} \bar{y}_u^{rs} - 3 y_d^{ts} \bar{y}_d^{rs} \right] \right] \\
& \quad (H^\dagger H) (H^\dagger t^I H) B_\mu W_\mu^I + g_L g_Y (\mathcal{C}_{Hq}^{(1)})^{rr} (H^\dagger t^I \partial_\mu \partial_\nu H) B_\mu W_\nu^I \\
& + g_L (\mathcal{C}_{Hq}^{(1)})^{rr} \left[ g_Y B_\mu W^{\mu\bar{\nu}I} (H^\dagger t^I \partial_\nu H) + g_Y B_\mu W^{\mu\bar{\nu}I} (\partial_\nu H^\dagger t^I H) \right] + g_L g_Y (\mathcal{C}_{Hq}^{(1)})^{rr} (\partial_\mu \partial_\nu H^\dagger t^I H) B_\mu W_\nu^I \\
& + g_L^2 g_Y (\mathcal{C}_{Hq}^{(1)})^{rr} \varepsilon^{IJK} B_\mu W_\nu^J W^{\mu\bar{\nu}I} (H^\dagger t^K H) + g_L^2 y_u^{tr} (\mathcal{C}_{Hq}^{(1)})^{st} \varepsilon^{jk} t_l^{Ii} t_j^{Jl} H_i^\dagger W_\mu^I W_\mu^J (\bar{q}_{ks} u_r) \\
& + \frac{4}{3} g_s^2 g_Y (\mathcal{C}_{Hq}^{(1)})^{rr} B_\mu G_\nu^A \widetilde{G}^{\mu\bar{\nu}A} (H^\dagger H) + 2 g_L^2 g_Y (\mathcal{C}_{Hq}^{(1)})^{rr} B_\mu W_\nu^I \widetilde{W}^{\mu\bar{\nu}I} (H^\dagger H) \\
& + 4 g_L^3 (\mathcal{C}_{Hq}^{(1)})^{rr} W_\mu^I W_\nu^J \widetilde{W}^{\mu\bar{\nu}J} (H^\dagger t^I H) + 8 g_L^2 (\mathcal{C}_{Hq}^{(1)})^{rt} \left[ y_u^{ts} \bar{y}_u^{rs} - y_d^{ts} \bar{y}_d^{rs} \right] (H^\dagger t^I H) (H^\dagger t^J H) W_\mu^I W_\mu^J \\
& - \frac{1}{36} g_L^2 g_Y^2 (\mathcal{C}_{Hq}^{(1)})^{rr} (H^\dagger H) B_\mu^2 W_\mu^{I2} - \frac{2}{27} g_Y^2 y_u^{tr} (\mathcal{C}_{Hq}^{(1)})^{st} B_\mu^2 (\bar{q}_s \tilde{H} u_r) - \frac{1}{12} g_L^2 y_u^{tr} (\mathcal{C}_{Hq}^{(1)})^{st} W_\mu^{I2} (\bar{q}_s \tilde{H} u_r) \\
& - \frac{5}{36} g_Y y_u^{tr} (\mathcal{C}_{Hq}^{(1)})^{st} B_\mu (\bar{q}_s \partial^\nu \tilde{H} \sigma^{\mu\bar{\nu}} u_r) - \frac{5}{36} g_Y \bar{y}_u^{ts} (\mathcal{C}_{Hq}^{(1)})^{tr} B_\mu (\bar{u}_s \sigma^{\mu\bar{\nu}} \partial^\nu \tilde{H} q_r) \\
& - \frac{1}{6} g_s^3 g_Y (\mathcal{C}_{Hq}^{(1)})^{rr} f^{ABC} (H^\dagger H) B_\mu G_\nu^A G_\rho^B G_\sigma^C \varepsilon^{\mu\bar{\nu}\rho\bar{\sigma}} - \frac{1}{6} g_Y^3 (\mathcal{C}_{Hq}^{(1)})^{tt} (H^\dagger H) (\bar{d}_s \tilde{B} d_s) \\
& + \frac{i}{6} g_s \bar{y}_d^{ts} (\mathcal{C}_{Hq}^{(1)})^{tr} T_b^{Aa} G_\mu^A (\bar{d}_{as} H^\dagger \partial^\mu q_r^b) - \frac{i}{6} g_L y_d^{tr} (\mathcal{C}_{Hq}^{(1)})^{st} t_j^{Ii} H^j W_\mu^I (\bar{q}_{is} \partial^\mu d_r) \\
& - \frac{1}{6} g_s^2 y_d^{tr} (\mathcal{C}_{Hq}^{(1)})^{st} T_b^{Aa} T_c^{Bb} G_\mu^A G_\mu^B (\bar{q}_{as} H d_r^c) - \frac{i}{6} g_s y_d^{tr} (\mathcal{C}_{Hq}^{(1)})^{st} T_b^{Aa} G_\mu^A (\bar{q}_{as} H \partial^\mu d_r^b) \\
& - \frac{1}{6} g_s^2 y_u^{tr} (\mathcal{C}_{Hq}^{(1)})^{st} T_b^{Aa} T_a^{Bc} G_\mu^A G_\mu^B (\bar{q}_{cs} \tilde{H} u_r^b) - \frac{1}{6} g_s^2 \bar{y}_u^{ts} (\mathcal{C}_{Hq}^{(1)})^{tr} T_b^{Aa} T_c^{Bb} G_\mu^A G_\mu^B (\bar{u}_{as} \tilde{H}^\dagger q_r^c) \\
& + \frac{i}{6} g_s \bar{y}_u^{ts} (\mathcal{C}_{Hq}^{(1)})^{tr} T_b^{Aa} G_\mu^A (\bar{u}_{as} \tilde{H}^\dagger \partial^\mu q_r^b) + \frac{i}{6} g_L \bar{y}_d^{ts} (\mathcal{C}_{Hq}^{(1)})^{tr} t_j^{Ii} H_i^\dagger W_\mu^I (\partial^\mu \bar{d}_s q_r^j) \\
& + \frac{i}{6} g_s \bar{y}_d^{ts} (\mathcal{C}_{Hq}^{(1)})^{tr} T_b^{Aa} G_\mu^A (\partial^\mu \bar{d}_{as} H^\dagger q_r^b) - \frac{49}{216} g_Y^4 (\mathcal{C}_{Hq}^{(1)})^{rr} (H^\dagger H) B_\mu^2 B_\mu^2 \\
& - \frac{1}{4} g_L^3 g_Y (\mathcal{C}_{Hq}^{(1)})^{rr} \varepsilon^{IJK} (H^\dagger H) B_\mu W_\nu^I W_\rho^J W_\sigma^K \varepsilon^{\mu\bar{\nu}\rho\bar{\sigma}} \\
& - \frac{5i}{18} g_L g_Y \bar{y}_d^{ts} (\mathcal{C}_{Hq}^{(1)})^{tr} t_j^{Ii} H_i^\dagger B_\mu W_\nu^I (\bar{d}_s \sigma^{\mu\bar{\nu}} q_r^j) + \frac{13}{36} g_s g_Y \bar{y}_d^{ts} (\mathcal{C}_{Hq}^{(1)})^{tr} T_b^{Aa} B_\mu G_\mu^A (\bar{d}_{as} H^\dagger q_r^b) \\
& - \frac{1}{3} g_L^2 g_Y^2 (\mathcal{C}_{Hq}^{(1)})^{rr} (H^\dagger H) B_\mu B_\nu W_\mu^I W_\nu^I - \frac{7}{18} g_Y^2 (\mathcal{C}_{Hq}^{(1)})^{rr} (H^\dagger \partial_\nu H) B_\mu \partial^\nu B_\mu \\
& - \frac{7}{18} g_Y^2 (\mathcal{C}_{Hq}^{(1)})^{rr} (\partial_\nu H^\dagger H) B_\mu \partial^\nu B_\mu - \frac{5i}{12} g_s g_Y \bar{y}_d^{ts} (\mathcal{C}_{Hq}^{(1)})^{tr} T_b^{Aa} B_\mu G_\nu^A (\bar{d}_{as} \sigma^{\mu\bar{\nu}} H^\dagger q_r^b) \\
& + \frac{1}{2} g_L g_s \bar{y}_d^{ts} (\mathcal{C}_{Hq}^{(1)})^{tr} t_j^{Ii} T_b^{Aa} H_i^\dagger G_\mu^A W_\mu^I (\bar{d}_{as} q_r^{bj}) + \frac{1}{2} g_L^2 g_Y (\mathcal{C}_{Hq}^{(1)})^{tt} (\bar{\ell}_s H \tilde{B} H^\dagger \ell_s) \\
& + \frac{1}{2} g_L g_Y y_d^{tr} (\mathcal{C}_{Hq}^{(1)})^{st} t_j^{Ii} H^j B_\mu W_\mu^I (\bar{q}_{is} d_r) + \frac{5}{6} g_s \bar{y}_d^{ts} (\mathcal{C}_{Hq}^{(1)})^{tr} T_b^{Aa} G_\mu^A (\bar{d}_{as} \sigma^{\mu\bar{\nu}} \partial^\nu H^\dagger q_r^b) \\
& - \frac{1}{6} g_s^2 \bar{y}_d^{ts} (\mathcal{C}_{Hq}^{(1)})^{tr} T_b^{Aa} T_a^{Bc} G_\mu^A G_\mu^B (\bar{d}_{cs} H^\dagger q_r^b) - \frac{1}{4} g_Y (\mathcal{C}_{Hq}^{(1)})^{tt} \left[ g_L^2 + g_Y^2 \right] (H^\dagger H) (\bar{\ell}_s \tilde{B} \ell_s)
\end{aligned}$$

$$\begin{aligned}
& -\frac{5}{12}g_L^2\bar{y}_d^{ts}(\mathcal{C}_{Hq}^{(1)})^{tr}\varepsilon^{IJK}t_j^{Ki}H_i^\dagger W_\mu^J W_\nu^I(\bar{d}_s\sigma^{\bar{\mu}\bar{\nu}}q_r^j) - \frac{5}{12}g_L^2y_d^{tr}(\mathcal{C}_{Hq}^{(1)})^{st}\varepsilon^{IJK}t_j^{Ki}H^j W_\mu^J W_\nu^I(\bar{q}_{is}\sigma^{\bar{\mu}\bar{\nu}}d_r) \\
& + \frac{5i}{12}g_s g_Y y_d^{tr}(\mathcal{C}_{Hq}^{(1)})^{st}T_b^{Aa}B_\mu G_\nu^A(\bar{q}_{as}H\sigma^{\bar{\mu}\bar{\nu}}d_r^b) - \frac{5i}{12}g_s g_Y y_u^{tr}(\mathcal{C}_{Hq}^{(1)})^{st}T_b^{Aa}B_\mu G_\nu^A(\bar{q}_{as}\tilde{H}\sigma^{\bar{\mu}\bar{\nu}}u_r^b) \\
& + \frac{5i}{12}g_s g_Y \bar{y}_u^{ts}(\mathcal{C}_{Hq}^{(1)})^{tr}T_b^{Aa}B_\mu G_\nu^A(\bar{u}_{as}\sigma^{\bar{\mu}\bar{\nu}}\tilde{H}^\dagger q_r^b) - \frac{4}{9}g_L g_Y^2(\mathcal{C}_{Hq}^{(1)})^{rr}B_\mu W_\nu^I \tilde{B}^{\bar{\mu}\bar{\nu}}(H^\dagger t^I H) \\
& - \frac{17}{36}g_s g_Y y_u^{tr}(\mathcal{C}_{Hq}^{(1)})^{st}T_b^{Aa}B_\mu G_\mu^A(\bar{q}_{as}\tilde{H}u_r^b) \\
& - \frac{1}{2}g_L(\mathcal{C}_{Hq}^{(1)})^{rr}\left[2g_L\varepsilon^{IJK}W_\mu^J \tilde{W}^{\bar{\mu}\bar{\sigma}I}(H^\dagger t^K \partial_{\bar{\sigma}}H) + 2g_L\varepsilon^{IJK}W_\mu^J \tilde{W}^{\bar{\mu}\bar{\sigma}I}(\partial_{\bar{\sigma}}H^\dagger t^K H)\right] \\
& - \frac{1}{2}g_Y^3(\mathcal{C}_{Hq}^{(1)})^{tt}(H^\dagger H)(\bar{e}_s\tilde{B}e_s) - \frac{1}{2}g_L g_s y_u^{tr}(\mathcal{C}_{Hq}^{(1)})^{st}t_j^{Ik}T_b^{Aa}\tilde{H}_j G_\mu^A W_\mu^I(\bar{q}_{aks}u_r^b) \\
& + \frac{5i}{9}g_L g_Y y_u^{tr}(\mathcal{C}_{Hq}^{(1)})^{st}\varepsilon^{jk}t_j^{Ii}H_i^\dagger B_\mu W_\nu^I(\bar{q}_{ks}\sigma^{\bar{\mu}\bar{\nu}}u_r) - \frac{5i}{9}g_L g_Y \bar{y}_u^{ts}(\mathcal{C}_{Hq}^{(1)})^{tr}\varepsilon_{ij}t_k^{Ii}H^k B_\mu W_\nu^I(\bar{u}_s\sigma^{\bar{\mu}\bar{\nu}}q_r^j) \\
& - \frac{2i}{3}g_L g_Y(\mathcal{C}_{Hq}^{(1)})^{rr}(\partial_{\bar{\rho}}H^\dagger t^I \partial_{\bar{\sigma}}H)B_\mu W_\nu^I \varepsilon^{\bar{\mu}\bar{\nu}\bar{\rho}\bar{\sigma}} - \frac{2i}{3}g_s \bar{y}_d^{ts}(\mathcal{C}_{Hq}^{(1)})^{tr}T_b^{Aa}G_\mu^A(\bar{d}_{as}\partial^{\bar{\mu}}H^\dagger q_r^b) \\
& + \frac{2i}{3}g_s y_d^{tr}(\mathcal{C}_{Hq}^{(1)})^{st}T_b^{Aa}G_\mu^A(\bar{q}_{as}\partial^{\bar{\mu}}H d_r^b) - \frac{2i}{3}g_s y_u^{tr}(\mathcal{C}_{Hq}^{(1)})^{st}T_b^{Aa}G_\mu^A(\bar{q}_{as}\partial^{\bar{\mu}}\tilde{H}u_r^b) \\
& + \frac{5i}{6}g_L g_s \bar{y}_d^{ts}(\mathcal{C}_{Hq}^{(1)})^{tr}t_j^{Ii}T_b^{Aa}H_i^\dagger G_\mu^A W_\nu^I(\bar{d}_{as}\sigma^{\bar{\mu}\bar{\nu}}q_r^{bj}) + \frac{5i}{6}g_L^2 y_u^{tr}(\mathcal{C}_{Hq}^{(1)})^{st}t_l^{Ik}t_j^{Jl}\tilde{H}_j W_\mu^I W_\nu^J(\bar{q}_{ks}\sigma^{\bar{\mu}\bar{\nu}}u_r) \\
& - \frac{5i}{6}g_L g_s y_d^{tr}(\mathcal{C}_{Hq}^{(1)})^{st}t_j^{Ii}T_b^{Aa}H^j G_\mu^A W_\nu^I(\bar{q}_{ais}\sigma^{\bar{\mu}\bar{\nu}}d_r^b) + \frac{5i}{6}g_L g_s y_u^{tr}(\mathcal{C}_{Hq}^{(1)})^{st}\varepsilon^{jk}t_j^{Ii}T_b^{Aa}H_i^\dagger G_\mu^A W_\nu^I(\bar{q}_{aks}\sigma^{\bar{\mu}\bar{\nu}}u_r^b) \\
& - \frac{5i}{6}g_L^2 \bar{y}_u^{ts}(\mathcal{C}_{Hq}^{(1)})^{tr}t_l^{Ik}t_k^{Ji}\tilde{H}^\dagger{}^i W_\mu^I W_\nu^J(\bar{u}_s\sigma^{\bar{\mu}\bar{\nu}}q_r^l) + \frac{5}{6}g_s \bar{y}_u^{ts}(\mathcal{C}_{Hq}^{(1)})^{tr}T_b^{Aa}G_\mu^A(\bar{u}_{as}\sigma^{\bar{\mu}\bar{\nu}}\partial^{\bar{\nu}}\tilde{H}q_r^b) \\
& + g_L^2 \bar{y}_u^{ts}(\mathcal{C}_{Hq}^{(1)})^{tr}\varepsilon_{ij}t_l^{Ik}t_k^{Ji}H^l W_\mu^I W_\mu^J(\bar{u}_s q_r^j) - \frac{2}{27}g_Y^2 \bar{y}_u^{ts}(\mathcal{C}_{Hq}^{(1)})^{tr}B_\mu^2(\bar{u}_s\tilde{H}^\dagger q_r) \\
& - \frac{1}{12}g_L^2 \bar{y}_u^{ts}(\mathcal{C}_{Hq}^{(1)})^{tr}W_\mu^I{}^2(\bar{u}_s\tilde{H}^\dagger q_r) - \frac{i}{6}g_L \bar{y}_u^{ts}(\mathcal{C}_{Hq}^{(1)})^{tr}\varepsilon_{ij}t_k^{Ii}H^k W_\mu^I(\bar{u}_s\partial^{\bar{\mu}}q_r^j) \\
& - \frac{17}{36}g_s g_Y \bar{y}_u^{ts}(\mathcal{C}_{Hq}^{(1)})^{tr}T_b^{Aa}B_\mu G_\mu^A(\bar{u}_{as}\tilde{H}^\dagger q_r^b) - \frac{1}{2}g_L g_s \bar{y}_u^{ts}(\mathcal{C}_{Hq}^{(1)})^{tr}t_k^{Ii}T_b^{Aa}\tilde{H}^\dagger{}^i G_\mu^A W_\mu^I(\bar{u}_{as}q_r^{bk}) \\
& + \frac{2i}{3}g_s \bar{y}_u^{ts}(\mathcal{C}_{Hq}^{(1)})^{tr}T_b^{Aa}G_\mu^A(\bar{u}_{as}\partial^{\bar{\mu}}\tilde{H}q_r^b) - \frac{5i}{6}g_L g_s \bar{y}_u^{ts}(\mathcal{C}_{Hq}^{(1)})^{tr}\varepsilon_{ij}t_k^{Ii}T_b^{Aa}H^k G_\mu^A W_\nu^I(\bar{u}_{as}\sigma^{\bar{\mu}\bar{\nu}}q_r^{bj}) \\
& - \frac{5}{6}g_L y_u^{tr}(\mathcal{C}_{Hq}^{(1)})^{st}\varepsilon^{ij}t_i^{Ik}W_\mu^I(\bar{q}_{js}\sigma^{\bar{\mu}\bar{\nu}}u_r)\partial^{\bar{\nu}}H_k^\dagger - \frac{5}{6}g_L \bar{y}_u^{ts}(\mathcal{C}_{Hq}^{(1)})^{tr}\varepsilon_{ij}t_k^{Ii}W_\mu^I(\bar{u}_s\sigma^{\bar{\mu}\bar{\nu}}q_r^j)\partial^{\bar{\nu}}H^k \\
& - \frac{8}{9}g_Y^2(\mathcal{C}_{Hq}^{(1)})^{rr}(\partial_{\bar{\mu}}H^\dagger \partial_{\bar{\nu}}H)B_\mu B_\nu - \frac{17}{18}g_Y^2(\mathcal{C}_{Hq}^{(1)})^{rr}(\partial_{\bar{\nu}}H^\dagger \partial_{\bar{\nu}}H)B_\mu^2 \\
& - \frac{17i}{18}g_L g_Y^2(\mathcal{C}_{Hq}^{(1)})^{rr}(H^\dagger t^I \partial_{\bar{\nu}}H)B_\mu^2 W_\nu^I + g_L^2(\mathcal{C}_{Hq}^{(1)})^{rr}(H^\dagger \partial_{\bar{\nu}}H)W_\mu^I \partial^{\bar{\nu}}W_\mu^I \\
& + g_L^2(\mathcal{C}_{Hq}^{(1)})^{rr}(\partial_{\bar{\nu}}H^\dagger H)W_\mu^I \partial^{\bar{\nu}}W_\mu^I + g_L^2 g_Y(\mathcal{C}_{Hq}^{(1)})^{rr}\varepsilon^{IJK}(H^\dagger t^K H)B_\mu W_\nu^I \partial^{\bar{\nu}}W_\mu^J \\
& - \frac{1}{3}g_Y^2(\mathcal{C}_{Hq}^{(1)})^{rr}(H^\dagger H)B_\mu \partial^{\bar{\mu}}\partial^{\bar{\nu}}B_\nu - \frac{2}{3}g_L g_Y(\mathcal{C}_{Hq}^{(1)})^{rr}(H^\dagger t^I H)W_\mu^I \partial^{\bar{\mu}}\partial^{\bar{\nu}}B_\nu \\
& - \frac{77i}{108}g_Y^3(\mathcal{C}_{Hq}^{(1)})^{rr}(H^\dagger \partial_{\bar{\mu}}H)B_\mu B_\mu^2 - g_L g_Y(\mathcal{C}_{Hq}^{(1)})^{rr}(\partial_{\bar{\mu}}H^\dagger t^I \partial_{\bar{\nu}}H)B_\mu W_\nu^I \\
& - g_L g_Y(\mathcal{C}_{Hq}^{(1)})^{rr}(\partial_{\bar{\nu}}H^\dagger t^I \partial_{\bar{\mu}}H)B_\mu W_\nu^I - g_L g_Y(\mathcal{C}_{Hq}^{(1)})^{rr}(H^\dagger t^I \partial_{\bar{\nu}}H)B_\mu \partial^{\bar{\nu}}W_\mu^I - g_L g_Y(\mathcal{C}_{Hq}^{(1)})^{rr}(\partial_{\bar{\nu}}H^\dagger t^I H)B_\mu \partial^{\bar{\nu}}W_\mu^I \\
& - \frac{77}{54}g_L g_Y^3(\mathcal{C}_{Hq}^{(1)})^{rr}(H^\dagger t^I H)B_\mu B_\mu^2 W_\mu^I - 2g_L g_Y(\mathcal{C}_{Hq}^{(1)})^{rr}(\partial_{\bar{\nu}}H^\dagger t^I \partial_{\bar{\nu}}H)B_\mu W_\mu^I
\end{aligned}$$

$$\begin{aligned}
& -2ig_L g_Y^2 (\mathcal{C}_{Hq}^{(1)})^{rr} (H^\dagger t^I \overleftrightarrow{\partial}_\nu H) B_{\bar{\mu}} B_{\bar{\nu}} W_{\bar{\mu}}^I - \frac{8}{3} g_L g_s^2 (\mathcal{C}_{Hq}^{(1)})^{rr} G_{\bar{\mu}}^A W_{\bar{\nu}}^I \tilde{G}^{\bar{\mu}\bar{\nu}A} (H^\dagger t^I H) \\
& -4i(\mathcal{C}_{Hq}^{(1)})^{rt} \left[ y_d^{ts} \bar{y}_d^{rs} - y_u^{ts} \bar{y}_u^{rs} \right] \left[ g_L (H^\dagger \partial_{\bar{\mu}} H) (H^\dagger t^I H) W_{\bar{\mu}}^I - g_L (\partial_{\bar{\mu}} H^\dagger H) (H^\dagger t^I H) W_{\bar{\mu}}^I \right], \tag{2.35}
\end{aligned}$$

$$\begin{aligned}
\Delta S_{\mathcal{O}_{Hq}^{(3)}} = & \frac{1}{108} g_Y \left[ 5(\mathcal{C}_{Hq}^{(3)})^{sr} \left[ g_Y^2 - 9g_L^2 \right] + 30y_d^{su} \bar{y}_d^{tu} (\mathcal{C}_{Hq}^{(3)})^{tr} \right. \\
& \left. + 30y_d^{ut} \bar{y}_d^{rt} (\mathcal{C}_{Hq}^{(3)})^{su} - 21 \left[ y_u^{su} \bar{y}_u^{tu} (\mathcal{C}_{Hq}^{(3)})^{tr} + y_u^{ut} \bar{y}_u^{rt} (\mathcal{C}_{Hq}^{(3)})^{su} \right] \right] (H^\dagger H) (\bar{q}_s \bar{B}_{q_r}) \\
& + \frac{1}{108} g_Y \left[ -3 \left[ 5y_d^{su} \bar{y}_d^{tu} (\mathcal{C}_{Hq}^{(3)})^{tr} + 5y_d^{ut} \bar{y}_d^{rt} (\mathcal{C}_{Hq}^{(3)})^{su} + 7y_u^{su} \bar{y}_u^{tu} (\mathcal{C}_{Hq}^{(3)})^{tr} + 7y_u^{ut} \bar{y}_u^{rt} (\mathcal{C}_{Hq}^{(3)})^{su} \right] - 10g_Y^2 (\mathcal{C}_{Hq}^{(3)})^{sr} \right] (\bar{q}_s H \bar{B} H^\dagger q_r) \\
& + \frac{1}{72} g_Y^4 (\mathcal{C}_{Hq}^{(3)})^{rr} (H^\dagger H) B_{\bar{\mu}}^2 B_{\bar{\mu}}^2 + \frac{i}{36} g_Y^3 (\mathcal{C}_{Hq}^{(3)})^{rr} (H^\dagger \overleftrightarrow{\partial}_{\bar{\mu}} H) B_{\bar{\mu}} B_{\bar{\mu}}^2 + \frac{1}{18} g_Y^2 (\mathcal{C}_{Hq}^{(3)})^{rr} (\partial_\nu H^\dagger \partial_\nu H) B_{\bar{\mu}}^2 \\
& + \frac{1}{18} g_L g_Y \bar{y}_d^{ts} (\mathcal{C}_{Hq}^{(3)})^{tr} t_j^{Ii} H_i^\dagger B_{\bar{\mu}} W_{\bar{\mu}}^I (\bar{d}_s q_r^j) \\
& + \frac{1}{18} g_s \left[ 5(\mathcal{C}_{Hq}^{(3)})^{sr} \left[ g_Y^2 - 9g_L^2 \right] - 3 \left[ y_u^{su} \bar{y}_u^{tu} (\mathcal{C}_{Hq}^{(3)})^{tr} + y_u^{ut} \bar{y}_u^{rt} (\mathcal{C}_{Hq}^{(3)})^{su} + 2y_d^{su} \bar{y}_d^{tu} (\mathcal{C}_{Hq}^{(3)})^{tr} + 2y_d^{ut} \bar{y}_d^{rt} (\mathcal{C}_{Hq}^{(3)})^{su} \right] \right] \\
& (H^\dagger H) (\bar{q}_s T^A \bar{G}^A q_r) \\
& + \frac{1}{18} g_s \left[ 3y_d^{su} \bar{y}_d^{tu} (\mathcal{C}_{Hq}^{(3)})^{tr} + 3y_d^{ut} \bar{y}_d^{rt} (\mathcal{C}_{Hq}^{(3)})^{su} - 3y_u^{su} \bar{y}_u^{tu} (\mathcal{C}_{Hq}^{(3)})^{tr} - 3y_u^{ut} \bar{y}_u^{rt} (\mathcal{C}_{Hq}^{(3)})^{su} - 10g_Y^2 (\mathcal{C}_{Hq}^{(3)})^{sr} \right] (\bar{q}_s T^A H \bar{G}^A H^\dagger q_r) \\
& + \frac{1}{18} g_L g_Y y_d^{tr} (\mathcal{C}_{Hq}^{(3)})^{st} t_j^{Ii} H^j B_{\bar{\mu}} W_{\bar{\mu}}^I (\bar{q}_{is} d_r) + \frac{1}{12} g_s^2 g_Y^2 (\mathcal{C}_{Hq}^{(3)})^{rr} (H^\dagger H) B_{\bar{\mu}}^2 G_{\bar{\mu}}^A{}^2 \\
& + \frac{1}{12} g_L^3 g_Y (\mathcal{C}_{Hq}^{(3)})^{rr} \varepsilon^{IJK} (H^\dagger H) B_{\bar{\mu}} W_{\bar{\nu}}^I W_{\bar{\rho}}^J W_{\bar{\sigma}}^K \varepsilon^{\bar{\mu}\bar{\nu}\bar{\rho}\bar{\sigma}} + \frac{i}{12} g_Y \bar{y}_d^{ts} (\mathcal{C}_{Hq}^{(3)})^{tr} B_{\bar{\mu}} (\bar{d}_s H^\dagger \partial^{\bar{\mu}} q_r) \\
& - \frac{i}{12} g_Y y_d^{tr} (\mathcal{C}_{Hq}^{(3)})^{st} B_{\bar{\mu}} (\bar{q}_s H \partial^{\bar{\mu}} d_r) + \frac{1}{12} g_L^2 y_u^{tr} (\mathcal{C}_{Hq}^{(3)})^{st} W_{\bar{\mu}}^I{}^2 (\bar{q}_s \tilde{H} u_r) + \frac{i}{12} g_Y y_u^{tr} (\mathcal{C}_{Hq}^{(3)})^{st} B_{\bar{\mu}} (\bar{q}_s \tilde{H} \partial^{\bar{\mu}} u_r) \\
& + \frac{1}{12} g_L \left[ 10g_L^2 (\mathcal{C}_{Hq}^{(3)})^{sr} + 18g_L^2 (\mathcal{C}_{Hq}^{(3)})^{tt} \delta^{rs} - y_d^{su} \bar{y}_d^{tu} (\mathcal{C}_{Hq}^{(3)})^{tr} - y_d^{ut} \bar{y}_d^{rt} (\mathcal{C}_{Hq}^{(3)})^{su} - y_u^{su} \bar{y}_u^{tu} (\mathcal{C}_{Hq}^{(3)})^{tr} - y_u^{ut} \bar{y}_u^{rt} (\mathcal{C}_{Hq}^{(3)})^{su} \right] \\
& (H^\dagger H) (\bar{q}_s t^I \bar{W}^I q_r) \\
& + \frac{1}{12} \left[ y_d^{ut} \bar{y}_d^{rt} (\mathcal{C}_{Hq}^{(3)})^{su} + y_u^{su} \bar{y}_u^{tu} (\mathcal{C}_{Hq}^{(3)})^{tr} - y_d^{su} \bar{y}_d^{tu} (\mathcal{C}_{Hq}^{(3)})^{tr} - y_u^{ut} \bar{y}_u^{rt} (\mathcal{C}_{Hq}^{(3)})^{su} \right] \\
& \left[ g_L t_j^{Ii} H_i^\dagger (\bar{q}_s H \bar{W}^I q_r^j) - g_L t_k^{Ij} H^k (\bar{q}_{js} \bar{W}^I H^\dagger q_r) \right] \\
& + \frac{1}{12} g_L^2 \bar{y}_u^{ts} (\mathcal{C}_{Hq}^{(3)})^{tr} W_{\bar{\mu}}^I{}^2 (\bar{u}_s \tilde{H}^\dagger q_r) - \frac{1}{18} g_Y^2 (\mathcal{C}_{Hq}^{(3)})^{rr} (H^\dagger \partial_{\bar{\mu}} H) B_{\bar{\mu}} \partial^{\bar{\nu}} B_{\bar{\nu}} \\
& - \frac{1}{18} g_Y^2 (\mathcal{C}_{Hq}^{(3)})^{rr} (\partial_{\bar{\mu}} H^\dagger H) B_{\bar{\mu}} \partial^{\bar{\nu}} B_{\bar{\nu}} - \frac{i}{12} g_Y \bar{y}_u^{ts} (\mathcal{C}_{Hq}^{(3)})^{tr} B_{\bar{\mu}} (\bar{u}_s \tilde{H}^\dagger \partial^{\bar{\mu}} q_r) \\
& + \frac{i}{12} g_Y \bar{y}_d^{ts} (\mathcal{C}_{Hq}^{(3)})^{tr} B_{\bar{\mu}} (\partial^{\bar{\mu}} \bar{d}_s H^\dagger q_r) - \frac{i}{12} g_Y y_d^{tr} (\mathcal{C}_{Hq}^{(3)})^{st} B_{\bar{\mu}} (\partial^{\bar{\mu}} \bar{q}_s H d_r) + \frac{i}{12} g_Y y_u^{tr} (\mathcal{C}_{Hq}^{(3)})^{st} B_{\bar{\mu}} (\partial^{\bar{\mu}} \bar{q}_s \tilde{H} u_r) \\
& - \frac{i}{12} g_Y \bar{y}_u^{ts} (\mathcal{C}_{Hq}^{(3)})^{tr} B_{\bar{\mu}} (\partial^{\bar{\mu}} \bar{u}_s \tilde{H}^\dagger q_r) - \frac{i}{6} g_L \bar{y}_d^{ts} (\mathcal{C}_{Hq}^{(3)})^{tr} t_j^{Ii} H_i^\dagger W_{\bar{\mu}}^I (\bar{d}_s \partial^{\bar{\mu}} q_r^j) \\
& + \frac{i}{6} g_L y_d^{tr} (\mathcal{C}_{Hq}^{(3)})^{st} t_j^{Ii} H^j W_{\bar{\mu}}^I (\bar{q}_{is} \partial^{\bar{\mu}} d_r) + \frac{i}{6} g_L y_u^{tr} (\mathcal{C}_{Hq}^{(3)})^{st} \varepsilon^{jk} t_j^{Ii} H_i^\dagger W_{\bar{\mu}}^I (\bar{q}_{ks} \partial^{\bar{\mu}} u_r) \\
& - \frac{i}{6} g_L \bar{y}_u^{ts} (\mathcal{C}_{Hq}^{(3)})^{tr} \bar{\varepsilon}_{ij} t_k^{Ii} H^k W_{\bar{\mu}}^I (\bar{u}_s \partial^{\bar{\mu}} q_r^j) - \frac{i}{6} g_L \bar{y}_d^{ts} (\mathcal{C}_{Hq}^{(3)})^{tr} t_j^{Ii} H_i^\dagger W_{\bar{\mu}}^I (\partial^{\bar{\mu}} \bar{d}_s q_r^j) \\
& + \frac{i}{6} g_L y_d^{tr} (\mathcal{C}_{Hq}^{(3)})^{st} t_j^{Ii} H^j W_{\bar{\mu}}^I (\partial^{\bar{\mu}} \bar{q}_{is} d_r) + \frac{i}{6} g_L y_u^{tr} (\mathcal{C}_{Hq}^{(3)})^{st} \varepsilon^{jk} t_j^{Ii} H_i^\dagger W_{\bar{\mu}}^I (\partial^{\bar{\mu}} \bar{q}_{ks} u_r)
\end{aligned}$$

$$\begin{aligned}
& -\frac{i}{6}g_L\bar{y}_u^{ts}(\mathcal{C}_{Hq}^{(3)})^{tr}\bar{\varepsilon}_{ij}t_k^{Ii}H^kW_\mu^I(\partial^\mu\bar{u}_sq_r^j)+\frac{i}{6}g_s^2g_Y(\mathcal{C}_{Hq}^{(3)})^{rr}(H^\dagger\overset{\leftrightarrow}{\partial}_\mu H)B_\mu G_\mu^{A^2} \\
& +\frac{7}{36}g_Y^2\bar{y}_d^{ts}(\mathcal{C}_{Hq}^{(3)})^{tr}B_\mu^2(\bar{d}_sH^\dagger q_r)+\frac{7}{36}g_Y^2y_d^{tr}(\mathcal{C}_{Hq}^{(3)})^{st}B_\mu^2(\bar{q}_sHd_r)+\frac{2}{9}g_Y^2y_u^{tr}(\mathcal{C}_{Hq}^{(3)})^{st}B_\mu^2(\bar{q}_s\tilde{H}u_r) \\
& +\frac{2}{9}g_Y^2\bar{y}_u^{ts}(\mathcal{C}_{Hq}^{(3)})^{tr}B_\mu^2(\bar{u}_s\tilde{H}^\dagger q_r)+\frac{1}{4}g_L^2g_s^2(\mathcal{C}_{Hq}^{(3)})^{rr}(H^\dagger H)G_\mu^{A^2}W_\mu^{I^2}+\frac{1}{3}g_L^2g_s^2(\mathcal{C}_{Hq}^{(3)})^{rr}(H^\dagger H)G_\mu^AG_\nu^AW_\mu^IW_\nu^I \\
& +\frac{1}{3}g_s^2(\mathcal{C}_{Hq}^{(3)})^{rr}(\partial_\nu H^\dagger\partial_\nu H)G_\mu^{A^2}-\frac{1}{3}g_L^2\bar{y}_d^{ts}(\mathcal{C}_{Hq}^{(3)})^{tr}W_\mu^{I^2}(\bar{d}_sH^\dagger q_r)-\frac{i}{3}g_Y\bar{y}_d^{ts}(\mathcal{C}_{Hq}^{(3)})^{tr}B_\mu(\bar{d}_s\partial^\mu H^\dagger q_r) \\
& +\frac{i}{3}g_Yy_d^{tr}(\mathcal{C}_{Hq}^{(3)})^{st}B_\mu(\bar{q}_s\partial^\mu Hd_r)+\frac{i}{3}g_Yy_u^{tr}(\mathcal{C}_{Hq}^{(3)})^{st}B_\mu(\bar{q}_s\partial^\mu\tilde{H}u_r)-\frac{i}{3}g_Y\bar{y}_u^{ts}(\mathcal{C}_{Hq}^{(3)})^{tr}B_\mu(\bar{u}_s\partial^\mu\tilde{H}q_r) \\
& +\frac{5}{12}g_L^2\bar{y}_d^{ts}(\mathcal{C}_{Hq}^{(3)})^{tr}\varepsilon^{IJK}t_j^{Ki}H_i^W_\mu^JW_\nu^I(\bar{d}_s\sigma^{\mu\nu}q_r^j)+\frac{5}{12}g_Y\bar{y}_d^{ts}(\mathcal{C}_{Hq}^{(3)})^{tr}B_\mu(\bar{d}_s\sigma^{\mu\nu}\partial^\nu H^\dagger q_r) \\
& +\frac{5}{12}g_Yy_d^{tr}(\mathcal{C}_{Hq}^{(3)})^{st}B_\mu(\bar{q}_s\partial^\nu H\sigma^{\mu\nu}d_r)+\frac{5}{12}g_Yy_u^{tr}(\mathcal{C}_{Hq}^{(3)})^{st}B_\mu(\bar{q}_s\partial^\nu\tilde{H}\sigma^{\mu\nu}u_r) \\
& +\frac{5}{12}g_L^2y_d^{tr}(\mathcal{C}_{Hq}^{(3)})^{st}\varepsilon^{IJK}t_j^{Ki}H^jW_\mu^JW_\nu^I(\bar{q}_{is}\sigma^{\mu\nu}d_r)+\frac{5}{12}g_Y\bar{y}_u^{ts}(\mathcal{C}_{Hq}^{(3)})^{tr}B_\mu(\bar{u}_s\sigma^{\mu\nu}\partial^\nu\tilde{H}q_r) \\
& -\frac{i}{2}g_Y(\mathcal{C}_{Hq}^{(3)})^{rr}\left[2g_LW_\mu^I\tilde{B}^{\mu\bar{\sigma}}(H^\dagger t^I\partial_{\bar{\sigma}}H)-2g_LW_\mu^I\tilde{B}^{\mu\bar{\sigma}}(\partial_{\bar{\sigma}}H^\dagger t^IH)\right] \\
& +\frac{i}{2}g_s\bar{y}_d^{ts}(\mathcal{C}_{Hq}^{(3)})^{tr}T_b^{Aa}G_\mu^A(\bar{d}_{as}H^\dagger\partial^\mu q_r^b)+\frac{1}{2}g_s^2y_u^{tr}(\mathcal{C}_{Hq}^{(3)})^{st}T_b^{Aa}T_a^{Bc}G_\mu^AG_\mu^B(\bar{q}_{cs}\tilde{H}u_r^b) \\
& +\frac{1}{2}g_s^2\bar{y}_u^{ts}(\mathcal{C}_{Hq}^{(3)})^{tr}T_b^{Aa}T_c^{Bb}G_\mu^AG_\mu^B(\bar{u}_{as}\tilde{H}^\dagger q_r^c)+\frac{2}{3}g_Lg_s^2g_Y(\mathcal{C}_{Hq}^{(3)})^{rr}(H^\dagger t^IH)B_\mu G_\mu^{A^2}W_\mu^I \\
& +\frac{2}{3}g_Lg_s^2g_Y(\mathcal{C}_{Hq}^{(3)})^{rr}(H^\dagger t^IH)B_\mu G_\mu^AG_\nu^AW_\nu^I-\frac{1}{3}g_L^2g_Y(\mathcal{C}_{Hq}^{(3)})^{rr}\varepsilon^{IJK}(H^\dagger t^KH)W_\mu^JW_\nu^I\partial^\mu B_\nu \\
& -\frac{1}{3}g_s^2(\mathcal{C}_{Hq}^{(3)})^{rr}(H^\dagger\partial_\mu H)G_\mu^A\partial^\nu G_\nu^A-\frac{1}{3}g_s^2(\mathcal{C}_{Hq}^{(3)})^{rr}(\partial_\mu H^\dagger H)G_\mu^A\partial^\nu G_\nu^A \\
& +\frac{i}{3}g_L^2g_Y(\mathcal{C}_{Hq}^{(3)})^{rr}\varepsilon^{IJK}B_\mu W_\nu^IW_\rho^J\varepsilon^{\mu\nu\rho\bar{\sigma}}(H^\dagger t^K\overset{\leftrightarrow}{\partial}_{\bar{\sigma}}H) \\
& -\frac{i}{2}g_s\bar{y}_u^{ts}(\mathcal{C}_{Hq}^{(3)})^{tr}T_b^{Aa}G_\mu^A(\bar{u}_{as}\tilde{H}^\dagger\partial^\mu q_r^b)+\frac{i}{2}g_s\bar{y}_d^{ts}(\mathcal{C}_{Hq}^{(3)})^{tr}T_b^{Aa}G_\mu^A(\partial^\mu\bar{d}_{as}H^\dagger q_r^b) \\
& -\frac{i}{2}g_sy_d^{tr}(\mathcal{C}_{Hq}^{(3)})^{st}T_b^{Aa}G_\mu^A(\partial^\mu\bar{q}_{as}Hd_r^b)+\frac{i}{2}g_sy_u^{tr}(\mathcal{C}_{Hq}^{(3)})^{st}T_b^{Aa}G_\mu^A(\partial^\mu\bar{q}_{as}\tilde{H}u_r^b) \\
& -\frac{i}{2}g_s\bar{y}_u^{ts}(\mathcal{C}_{Hq}^{(3)})^{tr}T_b^{Aa}G_\mu^A(\partial^\mu\bar{u}_{as}\tilde{H}^\dagger q_r^b)-\frac{1}{2}g_L^3(\mathcal{C}_{Hq}^{(3)})^{rr}\varepsilon^{IJK}(H^\dagger H)W_\mu^JW_\nu^I\partial^\mu W_\nu^K \\
& +\frac{i}{2}g_L^3(\mathcal{C}_{Hq}^{(3)})^{rr}(H^\dagger t^I\overset{\leftrightarrow}{\partial}_\mu H)W_\mu^IW_\mu^{I^2} \\
& +\frac{i}{2}g_L\left[3g_L^2(\mathcal{C}_{Hq}^{(3)})^{rr}-8(\mathcal{C}_{Hq}^{(3)})^{rt}\left[y_d^{ts}\bar{y}_d^{rs}+y_u^{ts}\bar{y}_u^{rs}\right]\right](H^\dagger t^I\overset{\leftrightarrow}{\partial}_\mu H)(H^\dagger H)W_\mu^I \\
& +\frac{2i}{3}g_Lg_Y(\mathcal{C}_{Hq}^{(3)})^{rr}(\partial_\rho H^\dagger t^I\partial_{\bar{\sigma}}H)B_\mu W_\nu^I\varepsilon^{\mu\nu\rho\bar{\sigma}}+\frac{2i}{3}g_L\bar{y}_d^{ts}(\mathcal{C}_{Hq}^{(3)})^{tr}t_j^{Ii}W_\mu^I(\bar{d}_sq_r^j)\partial^\mu H_i^\dagger \\
& -\frac{2i}{3}g_Ly_u^{tr}(\mathcal{C}_{Hq}^{(3)})^{st}\varepsilon^{ij}t_i^{Ik}W_\mu^I(\bar{q}_{js}u_r)\partial^\mu H_k^\dagger-\frac{2i}{3}g_Ly_d^{tr}(\mathcal{C}_{Hq}^{(3)})^{st}t_j^{Ii}W_\mu^I(\bar{q}_{is}d_r)\partial^\mu H^j \\
& +\frac{2i}{3}g_L\bar{y}_u^{ts}(\mathcal{C}_{Hq}^{(3)})^{tr}\bar{\varepsilon}_{ij}t_k^{Ii}W_\mu^I(\bar{u}_sq_r^j)\partial^\mu H^k+\frac{2}{3}g_Lg_Y(\mathcal{C}_{Hq}^{(3)})^{rr}(H^\dagger t^I\partial_\nu H)B_\mu\partial^\nu W_\mu^I \\
& +\frac{2}{3}g_Lg_Y(\mathcal{C}_{Hq}^{(3)})^{rr}(\partial_\nu H^\dagger t^IH)B_\mu\partial^\nu W_\mu^I+\frac{5}{6}g_L^3g_Y(\mathcal{C}_{Hq}^{(3)})^{rr}(H^\dagger t^IH)B_\mu W_\mu^IW_\mu^{I^2}
\end{aligned}$$

$$\begin{aligned}
& -\frac{1}{2}g_L^2(\mathcal{C}_{Hq}^{(3)})^{rr}(H^\dagger\partial_\mu H)W_\mu^I\partial^\nu W_\nu^I - \frac{1}{2}g_L^2(\mathcal{C}_{Hq}^{(3)})^{rr}(\partial_\mu H^\dagger H)W_\mu^I\partial^\nu W_\nu^I \\
& -\frac{2}{3}g_L^2g_Y(\mathcal{C}_{Hq}^{(3)})^{rr}\varepsilon^{IJK}(H^\dagger t^K H)B_\mu W_\nu^I\partial^\nu W_\mu^J + \frac{2i}{3}g_Lg_s^2(\mathcal{C}_{Hq}^{(3)})^{rr}(H^\dagger t^I\overleftrightarrow{\partial}_\nu H)G_\mu^AG_\nu^AW_\mu^I \\
& +\frac{2i}{3}g_Lg_s^2(\mathcal{C}_{Hq}^{(3)})^{rr}(H^\dagger t^I\overleftrightarrow{\partial}_\nu H)G_\mu^A{}^2W_\nu^I \\
& -\frac{5i}{6}g_L(\mathcal{C}_{Hq}^{(3)})^{rr}\left[2g_YB_\mu\widetilde{W}^{\mu\bar{\sigma}I}(H^\dagger t^I\partial_\sigma H) - 2g_YB_\mu\widetilde{W}^{\mu\bar{\sigma}I}(\partial_\sigma H^\dagger t^I H)\right] \\
& +\frac{5i}{6}g_Lg_Y\bar{y}_d^{ts}(\mathcal{C}_{Hq}^{(3)})^{tr}t_j^{Ii}H_i^\dagger B_\mu W_\nu^I(\bar{d}_s\sigma^{\mu\bar{\nu}}q_r^j) - \frac{5i}{6}g_Lg_Yy_d^{tr}(\mathcal{C}_{Hq}^{(3)})^{st}t_j^{Ii}H^j B_\mu W_\nu^I(\bar{q}_{is}\sigma^{\mu\bar{\nu}}d_r) \\
& +\frac{5i}{6}g_L^2y_u^{tr}(\mathcal{C}_{Hq}^{(3)})^{st}t_l^{Ik}t_j^{Jl}\tilde{H}_jW_\mu^IW_\nu^J(\bar{q}_{ks}\sigma^{\mu\bar{\nu}}u_r) - \frac{5i}{6}g_L^2\bar{y}_u^{ts}(\mathcal{C}_{Hq}^{(3)})^{tr}t_l^{Ik}t_k^{Ji}\tilde{H}^\dagger{}^iW_\mu^IW_\nu^J(\bar{u}_s\sigma^{\mu\bar{\nu}}q_r^l) \\
& +\frac{8}{9}g_Lg_Yy_u^{tr}(\mathcal{C}_{Hq}^{(3)})^{st}t_j^{Ik}\tilde{H}_jB_\mu W_\mu^I(\bar{q}_{ks}u_r) + \frac{8}{9}g_Lg_Y\bar{y}_u^{ts}(\mathcal{C}_{Hq}^{(3)})^{tr}t_k^{Ii}\tilde{H}^\dagger{}^iB_\mu W_\mu^I(\bar{u}_sq_r^k) \\
& +g_L^2\left[\frac{3}{4}g_L^2(\mathcal{C}_{Hq}^{(3)})^{rr} - 2(\mathcal{C}_{Hq}^{(3)})^{rt}\left[y_d^{ts}\bar{y}_d^{rs} + y_u^{ts}\bar{y}_u^{rs}\right]\right](H^\dagger H)^2W_\mu^I{}^2 + g_L^2(\mathcal{C}_{Hq}^{(3)})^{rr}(H^\dagger\partial_\mu\partial_\nu H)W_\mu^IW_\nu^I \\
& +g_L(\mathcal{C}_{Hq}^{(3)})^{rr}\left[g_LW_\mu^IW^{\mu\bar{\nu}I}(H^\dagger\partial_\nu H) + g_LW_\mu^IW^{\mu\bar{\nu}I}(\partial_\nu H^\dagger H)\right] + g_L^2(\mathcal{C}_{Hq}^{(3)})^{rr}(\partial_\mu\partial_\nu H^\dagger H)W_\mu^IW_\nu^I \\
& +g_Lg_Y\left[\frac{3}{2}(\mathcal{C}_{Hq}^{(3)})^{rr}\left[g_L^2 + g_Y^2\right] - 2(\mathcal{C}_{Hq}^{(3)})^{rt}\left[2y_u^{ts}\bar{y}_u^{rs} + 3y_d^{ts}\bar{y}_d^{rs}\right]\right](H^\dagger H)(H^\dagger t^I H)B_\mu W_\mu^I \\
& +ig_L^2(\mathcal{C}_{Hq}^{(3)})^{rr}\varepsilon^{IJK}(H^\dagger t^K\partial_\mu\partial_\nu H)W_\mu^IW_\nu^J - ig_L^2(\mathcal{C}_{Hq}^{(3)})^{rr}\varepsilon^{IJK}(\partial_\mu\partial_\nu H^\dagger t^K H)W_\mu^IW_\nu^J \\
& +g_L\left[\frac{1}{4}\left[y_d^{su}\bar{y}_d^{tu}(\mathcal{C}_{Hq}^{(3)})^{tr} + y_d^{ut}\bar{y}_d^{rt}(\mathcal{C}_{Hq}^{(3)})^{su} + 2g_Y^2(\mathcal{C}_{Hq}^{(3)})^{tt}\delta^{rs} - y_u^{su}\bar{y}_u^{tu}(\mathcal{C}_{Hq}^{(3)})^{tr} - y_u^{ut}\bar{y}_u^{rt}(\mathcal{C}_{Hq}^{(3)})^{su}\right] \right. \\
& \quad \left. - \frac{5}{18}g_Y^2(\mathcal{C}_{Hq}^{(3)})^{sr}\right](H^\dagger t^I H)(\bar{q}_s\overline{W}^I q_r) \\
& +g_L^2y_u^{tr}(\mathcal{C}_{Hq}^{(3)})^{st}\varepsilon^{jk}t_l^i t_j^{Jl}H_i^\dagger W_\mu^IW_\mu^J(\bar{q}_{ks}u_r) + g_L^2\bar{y}_u^{ts}(\mathcal{C}_{Hq}^{(3)})^{tr}\bar{\varepsilon}_{ij}t_l^{Ik}t_k^{Ji}H^l W_\mu^IW_\mu^J(\bar{u}_sq_r^j) \\
& +\frac{13}{12}g_s g_Y\bar{y}_d^{ts}(\mathcal{C}_{Hq}^{(3)})^{tr}T_b^{Aa}B_\mu G_\mu^A(\bar{d}_{as}H^\dagger q_r^b) + \frac{13}{12}g_s g_Y y_d^{tr}(\mathcal{C}_{Hq}^{(3)})^{st}T_b^{Aa}B_\mu G_\mu^A(\bar{q}_{as}H d_r^b) \\
& -\frac{1}{2}g_s^2y_d^{tr}(\mathcal{C}_{Hq}^{(3)})^{st}T_b^{Aa}T_c^{Bb}G_\mu^AG_\mu^B(\bar{q}_{as}H d_r^c) - \frac{i}{2}g_s y_d^{tr}(\mathcal{C}_{Hq}^{(3)})^{st}T_b^{Aa}G_\mu^A(\bar{q}_{as}H\partial^\mu d_r^b) \\
& +\frac{i}{2}g_s y_u^{tr}(\mathcal{C}_{Hq}^{(3)})^{st}T_b^{Aa}G_\mu^A(\bar{q}_{as}\tilde{H}\partial^\mu u_r^b) - \frac{5}{6}g_L\bar{y}_d^{ts}(\mathcal{C}_{Hq}^{(3)})^{tr}t_j^{Ii}W_\mu^I(\bar{d}_s\sigma^{\mu\bar{\nu}}q_r^j)\partial^\nu H_i^\dagger \\
& -\frac{5}{6}g_L y_u^{tr}(\mathcal{C}_{Hq}^{(3)})^{st}\varepsilon^{ij}t_i^{Ik}W_\mu^I(\bar{q}_{js}\sigma^{\mu\bar{\nu}}u_r)\partial^\nu H_k^\dagger - \frac{5}{6}g_L y_d^{tr}(\mathcal{C}_{Hq}^{(3)})^{st}t_j^{Ii}W_\mu^I(\bar{q}_{is}\sigma^{\mu\bar{\nu}}d_r)\partial^\nu H^j \\
& -\frac{5}{6}g_L\bar{y}_u^{ts}(\mathcal{C}_{Hq}^{(3)})^{tr}\bar{\varepsilon}_{ij}t_k^{Ii}W_\mu^I(\bar{u}_s\sigma^{\mu\bar{\nu}}q_r^j)\partial^\nu H^k - g_L^2(\mathcal{C}_{Hq}^{(3)})^{rr}(H^\dagger H)W_\mu^I\partial^\mu\partial^\nu W_\nu^I \\
& -ig_Y y_d^{ts}\bar{y}_d^{rs}(\mathcal{C}_{Hq}^{(3)})^{rt}(H^\dagger\overleftrightarrow{\partial}_\mu H)(H^\dagger H)B_\mu - \frac{5i}{4}g_s g_Y\bar{y}_d^{ts}(\mathcal{C}_{Hq}^{(3)})^{tr}T_b^{Aa}B_\mu G_\nu^A(\bar{d}_{as}\sigma^{\mu\bar{\nu}}H^\dagger q_r^b) \\
& +\frac{5i}{4}g_s g_Y y_d^{tr}(\mathcal{C}_{Hq}^{(3)})^{st}T_b^{Aa}B_\mu G_\nu^A(\bar{q}_{as}H\sigma^{\mu\bar{\nu}}d_r^b) + \frac{5i}{4}g_s g_Y y_u^{tr}(\mathcal{C}_{Hq}^{(3)})^{st}T_b^{Aa}B_\mu G_\nu^A(\bar{q}_{as}\tilde{H}\sigma^{\mu\bar{\nu}}u_r^b) \\
& -\frac{5i}{4}g_s g_Y\bar{y}_u^{ts}(\mathcal{C}_{Hq}^{(3)})^{tr}T_b^{Aa}B_\mu G_\nu^A(\bar{u}_{as}\sigma^{\mu\bar{\nu}}\tilde{H}^\dagger q_r^b) - \frac{5i}{4}g_L^2g_Y(\mathcal{C}_{Hq}^{(3)})^{rr}(H^\dagger\overleftrightarrow{\partial}_\mu H)B_\mu W_\mu^I{}^2 \\
& +\frac{4}{3}g_Lg_Y^2(\mathcal{C}_{Hq}^{(3)})^{rr}B_\mu W_\nu^I\tilde{B}^{\mu\bar{\nu}}(H^\dagger t^I H) - \frac{25i}{18}g_Lg_Y^2(\mathcal{C}_{Hq}^{(3)})^{rr}(H^\dagger t^I\overleftrightarrow{\partial}_\nu H)B_\mu^2W_\nu^I \\
& +\frac{17}{12}g_s g_Y y_u^{tr}(\mathcal{C}_{Hq}^{(3)})^{st}T_b^{Aa}B_\mu G_\mu^A(\bar{q}_{as}\tilde{H}u_r^b) + \frac{17}{12}g_s g_Y\bar{y}_u^{ts}(\mathcal{C}_{Hq}^{(3)})^{tr}T_b^{Aa}B_\mu G_\mu^A(\bar{u}_{as}\tilde{H}^\dagger q_r^b)
\end{aligned}$$

$$\begin{aligned}
& + \frac{3}{2} g_L^3 (\mathcal{C}_{Hq}^{(3)})^{tt} (H^\dagger H) (\bar{\ell}_s t^I \bar{W}^I \ell_s) + 3 g_L g_Y (\mathcal{C}_{Hq}^{(3)})^{rr} (H^\dagger t^I \partial_{\bar{\nu}} \partial_{\bar{\nu}} H) B_{\bar{\mu}} W_{\bar{\nu}}^I \\
& + 3 g_Y (\mathcal{C}_{Hq}^{(3)})^{rr} \left[ g_L W_{\bar{\mu}}^I B^{\bar{\mu}\bar{\nu}} (H^\dagger t^I \partial_{\bar{\nu}} H) + g_L W_{\bar{\mu}}^I B^{\bar{\mu}\bar{\nu}} (\partial_{\bar{\nu}} H^\dagger t^I H) \right] + 3 g_L g_Y (\mathcal{C}_{Hq}^{(3)})^{rr} (\partial_{\bar{\mu}} \partial_{\bar{\nu}} H^\dagger t^I H) B_{\bar{\mu}} W_{\bar{\nu}}^I \\
& + 3 g_L^2 g_Y^2 (\mathcal{C}_{Hq}^{(3)})^{rr} (H^\dagger t^I H) (H^\dagger t^J H) W_{\bar{\mu}}^I W_{\bar{\mu}}^J - \frac{1}{18} g_Y^2 (\mathcal{C}_{Hq}^{(3)})^{rr} (H^\dagger \partial_{\bar{\mu}} \partial_{\bar{\nu}} H) B_{\bar{\mu}} B_{\bar{\nu}} \\
& - \frac{1}{18} g_Y (\mathcal{C}_{Hq}^{(3)})^{rr} \left[ g_Y B_{\bar{\mu}} B^{\bar{\mu}\bar{\nu}} (H^\dagger \partial_{\bar{\nu}} H) + g_Y B_{\bar{\mu}} B^{\bar{\mu}\bar{\nu}} (\partial_{\bar{\nu}} H^\dagger H) \right] - \frac{1}{18} g_Y^2 (\mathcal{C}_{Hq}^{(3)})^{rr} (\partial_{\bar{\mu}} \partial_{\bar{\nu}} H^\dagger H) B_{\bar{\mu}} B_{\bar{\nu}} \\
& - \frac{1}{9} g_Y^2 (\mathcal{C}_{Hq}^{(3)})^{rr} (\partial_{\bar{\mu}} H^\dagger \partial_{\bar{\nu}} H) B_{\bar{\mu}} B_{\bar{\nu}} - \frac{1}{8} g_L^4 (\mathcal{C}_{Hq}^{(3)})^{rr} (H^\dagger H) W_{\bar{\mu}}^{I2} W_{\bar{\mu}}^{I2} - \frac{1}{4} g_L^4 (\mathcal{C}_{Hq}^{(3)})^{rr} (H^\dagger H) W_{\bar{\mu}}^I W_{\bar{\mu}}^J W_{\bar{\nu}}^I W_{\bar{\nu}}^J \\
& - \frac{1}{3} g_s^2 (\mathcal{C}_{Hq}^{(3)})^{rr} (H^\dagger \partial_{\bar{\mu}} \partial_{\bar{\nu}} H) G_{\bar{\mu}}^A G_{\bar{\nu}}^A - \frac{1}{3} g_s (\mathcal{C}_{Hq}^{(3)})^{rr} \left[ g_s G_{\bar{\mu}}^A G^{\bar{\mu}\bar{\nu}A} (H^\dagger \partial_{\bar{\nu}} H) + g_s G_{\bar{\mu}}^A G^{\bar{\mu}\bar{\nu}A} (\partial_{\bar{\nu}} H^\dagger H) \right] \\
& - \frac{1}{3} g_s^2 (\mathcal{C}_{Hq}^{(3)})^{rr} (\partial_{\bar{\mu}} \partial_{\bar{\nu}} H^\dagger H) G_{\bar{\mu}}^A G_{\bar{\nu}}^A - \frac{1}{3} g_L^2 y_d^{tr} (\mathcal{C}_{Hq}^{(3)})^{st} W_{\bar{\mu}}^{I2} (\bar{q}_s H d_r) \\
& - \frac{1}{2} g_s^2 \bar{y}_d^{ts} (\mathcal{C}_{Hq}^{(3)})^{tr} T_b^{Aa} T_a^{Bc} G_{\bar{\mu}}^A G_{\bar{\mu}}^B (\bar{d}_{cs} H^\dagger q_r^b) - \frac{7}{12} g_L^2 g_Y^2 (\mathcal{C}_{Hq}^{(3)})^{rr} (H^\dagger H) B_{\bar{\mu}}^2 W_{\bar{\mu}}^{I2} \\
& - \frac{2}{3} g_L^2 g_Y (\mathcal{C}_{Hq}^{(3)})^{rr} B_{\bar{\mu}} W_{\bar{\nu}}^I \widetilde{W}^{\bar{\mu}\bar{\nu}I} (H^\dagger H) - \frac{2}{3} g_s^2 (\mathcal{C}_{Hq}^{(3)})^{rr} (\partial_{\bar{\mu}} H^\dagger \partial_{\bar{\nu}} H) G_{\bar{\mu}}^A G_{\bar{\nu}}^A \\
& - \frac{17}{18} g_L g_Y^3 (\mathcal{C}_{Hq}^{(3)})^{rr} (H^\dagger t^I H) B_{\bar{\mu}} B_{\bar{\mu}}^2 W_{\bar{\mu}}^I - g_Y^2 y_d^{ts} \bar{y}_d^{rs} (\mathcal{C}_{Hq}^{(3)})^{rt} (H^\dagger H)^2 B_{\bar{\mu}}^2 - \frac{10}{9} g_L^2 g_Y^2 (\mathcal{C}_{Hq}^{(3)})^{rr} (H^\dagger H) B_{\bar{\mu}} B_{\bar{\nu}} W_{\bar{\mu}}^I W_{\bar{\nu}}^I \\
& - \frac{5}{4} g_L^3 (\mathcal{C}_{Hq}^{(3)})^{rr} \varepsilon^{IJK} W_{\bar{\mu}}^K W_{\bar{\nu}}^J W^{\bar{\mu}\bar{\nu}I} (H^\dagger H) + \frac{3i}{2} g_Y^2 (\mathcal{C}_{Hq}^{(3)})^{rr} \left[ g_L (H^\dagger \partial_{\bar{\mu}} H) (H^\dagger t^I H) W_{\bar{\mu}}^I - g_L (\partial_{\bar{\mu}} H^\dagger H) (H^\dagger t^I H) W_{\bar{\mu}}^I \right] \\
& - \frac{3}{2} g_L g_Y^2 (\mathcal{C}_{Hq}^{(3)})^{tt} (H^\dagger t^I H) (\bar{\ell}_s \bar{W}^I \ell_s) - \frac{3}{2} g_L^2 (\mathcal{C}_{Hq}^{(3)})^{rr} (H^\dagger \partial_{\bar{\nu}} H) W_{\bar{\mu}}^I \partial^{\bar{\nu}} W_{\bar{\mu}}^I \\
& - \frac{3}{2} g_L^2 (\mathcal{C}_{Hq}^{(3)})^{rr} (\partial_{\bar{\nu}} H^\dagger H) W_{\bar{\mu}}^I \partial^{\bar{\nu}} W_{\bar{\mu}}^I - 2 g_L^2 g_Y (\mathcal{C}_{Hq}^{(3)})^{rr} \varepsilon^{IJK} B_{\bar{\mu}} W_{\bar{\nu}}^J W^{\bar{\mu}\bar{\nu}I} (H^\dagger t^K H) \\
& - 2 (\mathcal{C}_{Hq}^{(3)})^{rr} \left[ g_L^2 g_Y \varepsilon^{IJK} (H^\dagger t^K \partial_{\bar{\nu}} H) B_{\bar{\mu}} W_{\bar{\nu}}^I W_{\bar{\nu}}^J + g_L^2 g_Y \varepsilon^{IJK} (\partial_{\bar{\nu}} H^\dagger t^K H) B_{\bar{\mu}} W_{\bar{\nu}}^I W_{\bar{\nu}}^J \right] \\
& - 2 i g_s \bar{y}_d^{ts} (\mathcal{C}_{Hq}^{(3)})^{tr} T_b^{Aa} G_{\bar{\mu}}^A (\bar{d}_{as} \partial^{\bar{\mu}} H^\dagger q_r^b) + 2 i g_s y_d^{tr} (\mathcal{C}_{Hq}^{(3)})^{st} T_b^{Aa} G_{\bar{\mu}}^A (\bar{q}_{as} \partial^{\bar{\mu}} H d_r^b) \\
& + 2 i g_s y_u^{tr} (\mathcal{C}_{Hq}^{(3)})^{st} T_b^{Aa} G_{\bar{\mu}}^A (\bar{q}_{as} \partial^{\bar{\mu}} \tilde{H} u_r^b) + 2 g_L g_Y^2 (\mathcal{C}_{Hq}^{(3)})^{tt} (H^\dagger t^I H) (\bar{u}_s \bar{W}^I u_s) \\
& - 2 i g_s \bar{y}_u^{ts} (\mathcal{C}_{Hq}^{(3)})^{tr} T_b^{Aa} G_{\bar{\mu}}^A (\bar{u}_{as} \partial^{\bar{\mu}} \tilde{H} q_r^b) + \frac{5}{2} g_s y_d^{tr} (\mathcal{C}_{Hq}^{(3)})^{st} T_b^{Aa} G_{\bar{\mu}}^A (\bar{q}_{as} \partial^{\bar{\nu}} H \sigma^{\bar{\mu}\bar{\nu}} d_r^b) \\
& - 2 g_L g_Y (\mathcal{C}_{Hq}^{(3)})^{rr} (H^\dagger t^I H) B_{\bar{\mu}} \partial^{\bar{\mu}} \partial^{\bar{\nu}} W_{\bar{\nu}}^I - 2 i g_L (\mathcal{C}_{Hq}^{(3)})^{rr} \partial^{\bar{\mu}} \partial^{\bar{\nu}} W_{\bar{\nu}}^I (H^\dagger t^I \partial_{\bar{\mu}} H) \\
& + 2 i g_L^2 (\mathcal{C}_{Hq}^{(3)})^{rr} \varepsilon^{IJK} W_{\bar{\mu}}^J W^{\bar{\mu}\bar{\nu}I} (H^\dagger t^K \partial_{\bar{\nu}} H) - \frac{20i}{9} g_L g_Y^2 (\mathcal{C}_{Hq}^{(3)})^{rr} (H^\dagger t^I \partial_{\bar{\nu}} H) B_{\bar{\mu}} B_{\bar{\nu}} W_{\bar{\mu}}^I \\
& - \frac{7}{3} g_L g_Y (\mathcal{C}_{Hq}^{(3)})^{rr} (H^\dagger t^I \partial_{\bar{\nu}} H) W_{\bar{\mu}}^I \partial^{\bar{\nu}} B_{\bar{\mu}} - \frac{7}{3} g_L g_Y (\mathcal{C}_{Hq}^{(3)})^{rr} (\partial_{\bar{\nu}} H^\dagger t^I H) W_{\bar{\mu}}^I \partial^{\bar{\nu}} B_{\bar{\mu}} \\
& - \frac{5}{2} g_L^2 (\mathcal{C}_{Hq}^{(3)})^{rr} (\partial_{\bar{\nu}} H^\dagger \partial_{\bar{\nu}} H) W_{\bar{\mu}}^{I2} + \frac{5i}{2} g_L g_s \bar{y}_d^{ts} (\mathcal{C}_{Hq}^{(3)})^{tr} t_j^{Ii} T_b^{Aa} H_i^\dagger G_{\bar{\mu}}^A W_{\bar{\nu}}^I (\bar{d}_{as} \sigma^{\bar{\mu}\bar{\nu}} q_r^{bj}) \\
& + \frac{5}{2} g_s \bar{y}_d^{ts} (\mathcal{C}_{Hq}^{(3)})^{tr} T_b^{Aa} G_{\bar{\mu}}^A (\bar{d}_{as} \sigma^{\bar{\mu}\bar{\nu}} \partial^{\bar{\nu}} H^\dagger q_r^b) + \frac{17}{6} g_L g_s \bar{y}_d^{ts} (\mathcal{C}_{Hq}^{(3)})^{tr} t_j^{Ii} T_b^{Aa} H_i^\dagger G_{\bar{\mu}}^A W_{\bar{\mu}}^I (\bar{d}_{as} q_r^{bj}) \\
& - g_L g_Y^2 (\mathcal{C}_{Hq}^{(3)})^{tt} (H^\dagger t^I H) (\bar{d}_s \bar{W}^I d_s) - \frac{5}{2} g_s y_u^{tr} (\mathcal{C}_{Hq}^{(3)})^{st} T_b^{Aa} G_{\bar{\mu}}^A (\bar{q}_{as} \partial^{\bar{\nu}} \tilde{H} \sigma^{\bar{\mu}\bar{\nu}} u_r^b) \\
& - \frac{5i}{2} g_L g_s y_d^{tr} (\mathcal{C}_{Hq}^{(3)})^{st} t_j^{Ii} T_b^{Aa} H_j^\dagger G_{\bar{\mu}}^A W_{\bar{\nu}}^I (\bar{q}_{ais} \sigma^{\bar{\mu}\bar{\nu}} d_r^b) - \frac{5i}{2} g_L g_s y_u^{tr} (\mathcal{C}_{Hq}^{(3)})^{st} \varepsilon^{jk} t_j^{Ii} T_b^{Aa} H_i^\dagger G_{\bar{\mu}}^A W_{\bar{\nu}}^I (\bar{q}_{aks} \sigma^{\bar{\mu}\bar{\nu}} u_r^b)
\end{aligned}$$

$$\begin{aligned}
& + \frac{5i}{2} g_L g_s \bar{y}_u^{ts} (\mathcal{C}_{Hq}^{(3)})^{tr} \bar{\varepsilon}_{ij} t_k^{Ii} T_b^{Aa} H^k G_{\bar{\mu}}^A W_{\bar{\nu}}^I (\bar{u}_{as} \sigma^{\bar{\mu}\bar{\nu}} q_r^{bj}) - \frac{8i}{3} g_L^2 g_Y (\mathcal{C}_{Hq}^{(3)})^{rr} (H^\dagger \overset{\leftrightarrow}{\partial}_{\bar{\nu}} H) B_{\bar{\mu}} W_{\bar{\mu}}^I W_{\bar{\nu}}^I \\
& + \frac{17}{6} g_L g_s y_d^{tr} (\mathcal{C}_{Hq}^{(3)})^{st} t_j^{Ii} T_b^{Aa} H^j G_{\bar{\mu}}^A W_{\bar{\mu}}^I (\bar{q}_{ais} d_r^b) + \frac{17}{6} g_L g_s y_u^{tr} (\mathcal{C}_{Hq}^{(3)})^{st} t_j^{Ik} T_b^{Aa} \tilde{H}_j G_{\bar{\mu}}^A W_{\bar{\mu}}^I (\bar{q}_{aks} u_r^b) \\
& + \frac{17}{6} g_L g_s \bar{y}_u^{ts} (\mathcal{C}_{Hq}^{(3)})^{tr} t_k^{Ii} T_b^{Aa} \tilde{H}^{\dagger i} G_{\bar{\mu}}^A W_{\bar{\mu}}^I (\bar{u}_{as} q_r^{bk}) - \frac{5}{2} g_s \bar{y}_u^{ts} (\mathcal{C}_{Hq}^{(3)})^{tr} T_b^{Aa} G_{\bar{\mu}}^A (\bar{u}_{as} \sigma^{\bar{\mu}\bar{\nu}} \partial^{\bar{\nu}} \tilde{H} q_r^b) \\
& - 3g_L g_Y (\mathcal{C}_{Hq}^{(3)})^{rr} (\partial_{\bar{\mu}} H^\dagger t^I \partial_{\bar{\nu}} H) B_{\bar{\mu}} W_{\bar{\nu}}^I - 3g_L g_Y (\mathcal{C}_{Hq}^{(3)})^{rr} (\partial_{\bar{\nu}} H^\dagger t^I \partial_{\bar{\mu}} H) B_{\bar{\mu}} W_{\bar{\nu}}^I - 3g_L g_Y^2 (\mathcal{C}_{Hq}^{(3)})^{tt} (H^\dagger t^I H) (\bar{e}_s \bar{W}^I e_s) \\
& - 3g_L^2 g_Y (\mathcal{C}_{Hq}^{(3)})^{rr} \varepsilon^{IJK} (H^\dagger t^K H) B_{\bar{\mu}} W_{\bar{\nu}}^J \partial^{\bar{\mu}} W_{\bar{\nu}}^I + 3ig_L^2 (\mathcal{C}_{Hq}^{(3)})^{rr} \varepsilon^{IJK} (H^\dagger t^K \partial_{\bar{\nu}} H) W_{\bar{\mu}}^I \partial^{\bar{\nu}} W_{\bar{\mu}}^J \\
& - 3ig_L^2 (\mathcal{C}_{Hq}^{(3)})^{rr} \varepsilon^{IJK} (\partial_{\bar{\nu}} H^\dagger t^K H) W_{\bar{\mu}}^I \partial^{\bar{\nu}} W_{\bar{\mu}}^J - \frac{7}{2} g_L^2 g_Y (\mathcal{C}_{Hq}^{(3)})^{rr} \varepsilon^{IJK} W_{\bar{\mu}}^J W_{\bar{\nu}}^I B^{\bar{\mu}\bar{\nu}} (H^\dagger t^K H) \\
& - 4g_L^2 (\mathcal{C}_{Hq}^{(3)})^{rr} (\partial_{\bar{\mu}} H^\dagger \partial_{\bar{\nu}} H) W_{\bar{\mu}}^I W_{\bar{\nu}}^I - 4g_L^3 g_Y (\mathcal{C}_{Hq}^{(3)})^{rr} (H^\dagger t^I H) B_{\bar{\mu}} W_{\bar{\mu}}^J W_{\bar{\nu}}^I W_{\bar{\nu}}^J \\
& + 4ig_L^2 (\mathcal{C}_{Hq}^{(3)})^{rr} \varepsilon^{IJK} (\partial_{\bar{\mu}} H^\dagger t^K \partial_{\bar{\nu}} H) W_{\bar{\mu}}^I W_{\bar{\nu}}^J - 4ig_L^3 (\mathcal{C}_{Hq}^{(3)})^{rr} (H^\dagger t^I \overset{\leftrightarrow}{\partial}_{\bar{\nu}} H) W_{\bar{\mu}}^I W_{\bar{\mu}}^J W_{\bar{\nu}}^J \\
& - \frac{14}{3} g_L g_Y (\mathcal{C}_{Hq}^{(3)})^{rr} (\partial_{\bar{\nu}} H^\dagger t^I \partial_{\bar{\nu}} H) B_{\bar{\mu}} W_{\bar{\mu}}^I \\
& - 6i(\mathcal{C}_{Hq}^{(3)})^{rr} \left[ g_L (\partial_{\bar{\nu}} H^\dagger t^I \partial_{\bar{\mu}} \partial_{\bar{\nu}} H) W_{\bar{\mu}}^I - g_L (\partial_{\bar{\mu}} \partial_{\bar{\nu}} H^\dagger t^I \partial_{\bar{\nu}} H) W_{\bar{\mu}}^I \right].
\end{aligned} \tag{2.36}$$

## 2.5 Dimension six: four-fermion operators

$$\begin{aligned}
\Delta S_{\mathcal{O}_{ee}} &= \frac{4}{3} g_Y \mathcal{C}_{ee}^{srtt} (\bar{e}_s \bar{B} \partial^2 e_r) + \frac{4}{3} g_L y_e^{tv} \bar{y}_e^{tu} \mathcal{C}_{ee}^{srvu} (H^\dagger t^I H) (\bar{e}_s \bar{W}^I e_r) + \frac{4}{3} g_Y \mathcal{C}_{ee}^{srtt} (\partial^2 \bar{e}_s \bar{B} e_r) \\
&+ \frac{4}{3} g_Y \mathcal{C}_{ee}^{srtt} (\bar{e}_s \gamma^{\bar{\mu}} e_r) \partial^2 B_{\bar{\mu}} + \frac{8}{3} g_Y \mathcal{C}_{ee}^{srtt} (\partial^{\bar{\nu}} \bar{e}_s \bar{B} \partial^{\bar{\nu}} e_r) + \frac{14}{3} g_Y y_e^{tv} \bar{y}_e^{tu} \mathcal{C}_{ee}^{srvu} (H^\dagger H) (\bar{e}_s \bar{B} e_r) \\
&- \frac{4}{3} g_Y^3 \mathcal{C}_{ee}^{srtt} B_{\bar{\mu}}^2 (\bar{e}_s \bar{B} e_r),
\end{aligned} \tag{2.37}$$

$$\begin{aligned}
\Delta S_{\mathcal{O}_{\ell\ell}} &= \frac{1}{12} g_L^3 \left[ \mathcal{C}_{\ell\ell}^{sttr} - 2\mathcal{C}_{\ell\ell}^{srtt} \right] \varepsilon^{IJK} W_{\bar{\mu}}^I W_{\bar{\nu}}^K W_{\bar{\rho}}^J \varepsilon^{\bar{\mu}\bar{\nu}\bar{\rho}\bar{\sigma}} (\bar{\ell}_s \gamma^{\bar{\sigma}} \ell_r) \\
&+ \frac{1}{12} g_Y^3 \left[ -\mathcal{C}_{\ell\ell}^{sttr} - 2\mathcal{C}_{\ell\ell}^{srtt} \right] B_{\bar{\mu}}^2 (\bar{\ell}_s \bar{B} \ell_r) + \frac{1}{12} g_L^2 g_Y \left[ -\mathcal{C}_{\ell\ell}^{sttr} - 2\mathcal{C}_{\ell\ell}^{srtt} \right] W_{\bar{\mu}}^I{}^2 (\bar{\ell}_s \bar{B} \ell_r) \\
&+ \frac{1}{6} g_L^2 g_Y \left[ -\mathcal{C}_{\ell\ell}^{sttr} - 2\mathcal{C}_{\ell\ell}^{srtt} \right] B_{\bar{\mu}} W_{\bar{\mu}}^I (\bar{\ell}_s \bar{W}^I \ell_r) + \frac{1}{6} g_L g_Y^2 \mathcal{C}_{\ell\ell}^{sttr} B_{\bar{\mu}}^2 (\bar{\ell}_s t^I \bar{W}^I \ell_r) \\
&+ \frac{1}{6} g_L^2 g_Y \left[ \mathcal{C}_{\ell\ell}^{sttr} + 2\mathcal{C}_{\ell\ell}^{srtt} \right] \varepsilon^{IJK} B_{\bar{\mu}} W_{\bar{\nu}}^I W_{\bar{\rho}}^J \varepsilon^{\bar{\mu}\bar{\nu}\bar{\rho}\bar{\sigma}} (\bar{\ell}_s t^K \gamma^{\bar{\sigma}} \ell_r) \\
&+ \frac{1}{3} g_Y \left[ \mathcal{C}_{\ell\ell}^{sttr} + 2\mathcal{C}_{\ell\ell}^{srtt} \right] (\bar{\ell}_s \bar{B} \partial^2 \ell_r) + \frac{1}{3} g_L g_Y^2 \mathcal{C}_{\ell\ell}^{sttr} B_{\bar{\mu}} W_{\bar{\mu}}^I (\bar{\ell}_s t^I \bar{B} \ell_r) \\
&+ \frac{1}{3} g_Y \left[ \mathcal{C}_{\ell\ell}^{sttr} + 2\mathcal{C}_{\ell\ell}^{srtt} \right] (\partial^2 \bar{\ell}_s \bar{B} \ell_r) + \frac{1}{3} g_Y \left[ \mathcal{C}_{\ell\ell}^{sttr} + 2\mathcal{C}_{\ell\ell}^{srtt} \right] (\bar{\ell}_s \gamma^{\bar{\mu}} \ell_r) \partial^2 B_{\bar{\mu}} \\
&+ \frac{1}{3} g_L^2 \mathcal{C}_{\ell\ell}^{sttr} \varepsilon^{IJK} W_{\bar{\mu}}^J (\bar{\ell}_s t^K \gamma^{\bar{\nu}} \ell_r) \partial^{\bar{\mu}} W_{\bar{\nu}}^I + \frac{1}{2} g_L^3 \mathcal{C}_{\ell\ell}^{sttr} W_{\bar{\mu}}^I{}^2 (\bar{\ell}_s t^I \bar{W}^I \ell_r) \\
&+ \frac{2}{3} g_Y^2 \left[ \mathcal{C}_{\ell\ell}^{sttr} - 2\mathcal{C}_{\ell\ell}^{srtt} \right] B_{\bar{\mu}} \tilde{B}^{\bar{\mu}\bar{\sigma}} (\bar{\ell}_s \gamma^{\bar{\sigma}} \ell_r) \\
&+ \frac{2}{3} g_L^2 \left[ \mathcal{C}_{\ell\ell}^{sttr} - 2\mathcal{C}_{\ell\ell}^{srtt} \right] W_{\bar{\mu}}^I \tilde{W}^{\bar{\mu}\bar{\sigma}I} (\bar{\ell}_s \gamma^{\bar{\sigma}} \ell_r) + \frac{2}{3} g_Y y_e^{vu} \bar{y}_e^{tu} \mathcal{C}_{\ell\ell}^{srtv} (H^\dagger H) (\bar{\ell}_s \bar{B} \ell_r) \\
&+ \frac{2}{3} g_L g_Y \left[ \mathcal{C}_{\ell\ell}^{srtt} - 2\mathcal{C}_{\ell\ell}^{sttr} \right] W_{\bar{\mu}}^I \tilde{B}^{\bar{\mu}\bar{\sigma}} (\bar{\ell}_s t^I \gamma^{\bar{\sigma}} \ell_r) + \frac{2}{3} g_Y y_e^{vu} \bar{y}_e^{tu} \mathcal{C}_{\ell\ell}^{svtr} (\bar{\ell}_s H \bar{B} H^\dagger \ell_r)
\end{aligned}$$

$$\begin{aligned}
& + \frac{2}{3} g_Y \left[ \mathcal{C}_{\ell\ell}^{sttr} + 2\mathcal{C}_{\ell\ell}^{srtt} \right] (\partial^{\bar{\nu}} \bar{\ell}_s \bar{\mathcal{B}} \partial^{\bar{\nu}} \ell_r) + 2g_L^2 \mathcal{C}_{\ell\ell}^{sttr} \varepsilon^{IJK} W_{\bar{\mu}}^J W^{\bar{\mu}\bar{\nu}I} (\bar{\ell}_s t^K \gamma^{\bar{\nu}} \ell_r) \\
& - \frac{1}{3} g_L^3 \mathcal{C}_{\ell\ell}^{sttr} W_{\bar{\mu}}^I W_{\bar{\mu}}^J (\bar{\ell}_s t^I \bar{W}^J \ell_r) - \frac{1}{3} g_L^2 \mathcal{C}_{\ell\ell}^{sttr} \varepsilon^{IJK} (\bar{\ell}_s t^K \bar{W}^I \ell_r) \partial^{\bar{\nu}} W_{\bar{\nu}}^J \\
& - \frac{2}{3} g_L g_Y \left[ \mathcal{C}_{\ell\ell}^{srtt} + 2\mathcal{C}_{\ell\ell}^{sttr} \right] B_{\bar{\mu}} \widetilde{W}^{\bar{\mu}\bar{\sigma}I} (\bar{\ell}_s t^I \gamma^{\bar{\sigma}} \ell_r) - \frac{2}{3} g_L \mathcal{C}_{\ell\ell}^{sttr} (\bar{\ell}_s t^I \bar{W}^I \partial^2 \ell_r) \\
& - \frac{2}{3} g_L \mathcal{C}_{\ell\ell}^{sttr} (\partial^2 \bar{\ell}_s t^I \bar{W}^I \ell_r) \\
& - \frac{2}{3} \mathcal{C}_{\ell\ell}^{srtt} \left[ g_L g_Y B_{\bar{\mu}} W_{\bar{\nu}}^I \varepsilon^{\bar{\mu}\bar{\nu}\bar{\rho}\bar{\sigma}} (\bar{\ell}_s t^I \gamma^{\bar{\rho}} \partial^{\bar{\sigma}} \ell_r) + g_L g_Y B_{\bar{\mu}} W_{\bar{\nu}}^I \varepsilon^{\bar{\mu}\bar{\nu}\bar{\rho}\bar{\sigma}} (\partial^{\bar{\sigma}} \bar{\ell}_s t^I \gamma^{\bar{\rho}} \ell_r) \right] \\
& - \frac{2}{3} g_L \mathcal{C}_{\ell\ell}^{sttr} (\bar{\ell}_s t^I \gamma^{\bar{\mu}} \ell_r) \partial^2 W_{\bar{\mu}}^I - \frac{4}{3} g_L y_e^{vu} \bar{y}_e^{tu} \left[ \mathcal{C}_{\ell\ell}^{svtr} + 2\mathcal{C}_{\ell\ell}^{srtv} \right] (H^\dagger t^I H) (\bar{\ell}_s \bar{W}^I \ell_r) \\
& - \frac{4}{3} g_L y_e^{vu} \bar{y}_e^{tu} \mathcal{C}_{\ell\ell}^{svtr} (H^\dagger H) (\bar{\ell}_s t^I \bar{W}^I \ell_r) - \frac{4}{3} g_L \mathcal{C}_{\ell\ell}^{sttr} (\partial^{\bar{\nu}} \bar{\ell}_s t^I \bar{W}^I \partial^{\bar{\nu}} \ell_r) \\
& - \frac{5}{3} \mathcal{C}_{\ell\ell}^{sttr} \left[ g_L^2 \varepsilon^{IJK} W_{\bar{\nu}}^J (\bar{\ell}_s t^K \bar{W}^I \partial^{\bar{\nu}} \ell_r) + g_L^2 \varepsilon^{IJK} W_{\bar{\nu}}^J (\partial^{\bar{\nu}} \bar{\ell}_s t^K \bar{W}^I \ell_r) \right], \tag{2.38}
\end{aligned}$$

$$\begin{aligned}
\Delta S_{\mathcal{O}_{\ell e}} = & \frac{1}{12} g_L^3 \mathcal{C}_{\ell e}^{ttsr} \varepsilon^{IJK} W_{\bar{\mu}}^I W_{\bar{\nu}}^J W_{\bar{\rho}}^K \varepsilon^{\bar{\mu}\bar{\nu}\bar{\rho}\bar{\sigma}} (\bar{e}_s \gamma^{\bar{\sigma}} e_r) + \frac{1}{3} g_Y y_e^{vu} \bar{y}_e^{tu} \mathcal{C}_{\ell e}^{tvsr} (H^\dagger H) (\bar{e}_s \bar{\mathcal{B}} e_r) \\
& + \frac{1}{3} g_Y \mathcal{C}_{\ell e}^{ttsr} (\bar{e}_s \bar{\mathcal{B}} \partial^2 e_r) - \frac{1}{12} g_Y^3 \mathcal{C}_{\ell e}^{ttsr} B_{\bar{\mu}}^2 (\bar{e}_s \bar{\mathcal{B}} e_r) - \frac{1}{12} g_L^2 g_Y \mathcal{C}_{\ell e}^{ttsr} W_{\bar{\mu}}^{I2} (\bar{e}_s \bar{\mathcal{B}} e_r) \\
& - \frac{1}{6} g_L^2 g_Y \mathcal{C}_{\ell e}^{ttsr} B_{\bar{\mu}} W_{\bar{\mu}}^I (\bar{e}_s \bar{W}^I e_r) - \frac{i}{3} g_Y \bar{y}_e^{tu} \mathcal{C}_{\ell e}^{trsu} B_{\bar{\mu}} (\bar{e}_s H^\dagger \partial^{\bar{\mu}} \ell_r) \\
& + \frac{i}{3} g_Y \bar{y}_e^{tu} \mathcal{C}_{\ell e}^{trsu} B_{\bar{\mu}} (\bar{e}_s \partial^{\bar{\mu}} H^\dagger \ell_r) + \frac{i}{3} g_Y y_e^{tu} \mathcal{C}_{\ell e}^{stur} B_{\bar{\mu}} (\bar{\ell}_s H \partial^{\bar{\mu}} e_r) - \frac{i}{3} g_Y y_e^{tu} \mathcal{C}_{\ell e}^{stur} B_{\bar{\mu}} (\bar{\ell}_s \partial^{\bar{\mu}} H e_r) \\
& + \frac{1}{3} g_Y \mathcal{C}_{\ell e}^{srtt} (\bar{\ell}_s \bar{\mathcal{B}} \partial^2 \ell_r) + \frac{1}{3} g_L y_e^{tv} \bar{y}_e^{tu} \mathcal{C}_{\ell e}^{srvu} (H^\dagger t^I H) (\bar{\ell}_s \bar{W}^I \ell_r) + \frac{1}{3} g_Y \mathcal{C}_{\ell e}^{ttsr} (\partial^2 \bar{e}_s \bar{\mathcal{B}} e_r) \\
& + \frac{1}{3} g_Y \mathcal{C}_{\ell e}^{srtt} (\partial^2 \bar{\ell}_s \bar{\mathcal{B}} \ell_r) + \frac{2i}{3} g_L y_e^{tu} \mathcal{C}_{\ell e}^{stur} t_j^{Ii} H^j W_{\bar{\mu}}^I (\bar{\ell}_{is} \partial^{\bar{\mu}} e_r) \\
& - \frac{2i}{3} g_L \bar{y}_e^{tu} \mathcal{C}_{\ell e}^{trsu} t_j^{Ii} H_i^\dagger W_{\bar{\mu}}^I (\partial^{\bar{\mu}} \bar{e}_s \ell_r^j) + \frac{7}{6} g_Y y_e^{tv} \bar{y}_e^{tu} \mathcal{C}_{\ell e}^{srvu} (H^\dagger H) (\bar{\ell}_s \bar{\mathcal{B}} \ell_r) \\
& + \frac{4}{3} g_Y \mathcal{C}_{\ell e}^{srtt} B_{\bar{\mu}} \widetilde{B}^{\bar{\mu}\bar{\sigma}} (\bar{\ell}_s \gamma^{\bar{\sigma}} \ell_r) - \frac{1}{3} g_Y \mathcal{C}_{\ell e}^{srtt} B_{\bar{\mu}}^2 (\bar{\ell}_s \bar{\mathcal{B}} \ell_r) \\
& - \frac{i}{3} g_Y \bar{y}_e^{tu} \mathcal{C}_{\ell e}^{trsu} B_{\bar{\mu}} (\partial^{\bar{\mu}} \bar{e}_s H^\dagger \ell_r) + \frac{i}{3} g_Y y_e^{tu} \mathcal{C}_{\ell e}^{stur} B_{\bar{\mu}} (\partial^{\bar{\mu}} \bar{\ell}_s H e_r) + \frac{1}{3} g_Y \mathcal{C}_{\ell e}^{ttsr} (\bar{e}_s \gamma^{\bar{\mu}} e_r) \partial^2 B_{\bar{\mu}} \\
& + \frac{1}{3} g_Y \mathcal{C}_{\ell e}^{srtt} (\bar{\ell}_s \gamma^{\bar{\mu}} \ell_r) \partial^2 B_{\bar{\mu}} - \frac{1}{2} g_L^2 \bar{y}_e^{tu} \mathcal{C}_{\ell e}^{trsu} W_{\bar{\mu}}^{I2} (\bar{e}_s H^\dagger \ell_r) - \frac{1}{2} g_L^2 y_e^{tu} \mathcal{C}_{\ell e}^{stur} W_{\bar{\mu}}^{I2} (\bar{\ell}_s H e_r) \\
& - \frac{2i}{3} g_L \bar{y}_e^{tu} \mathcal{C}_{\ell e}^{trsu} t_j^{Ii} H_i^\dagger W_{\bar{\mu}}^I (\bar{e}_s \partial^{\bar{\mu}} \ell_r^j) - \frac{2}{3} g_Y^2 \mathcal{C}_{\ell e}^{ttsr} B_{\bar{\mu}} \widetilde{B}^{\bar{\mu}\bar{\sigma}} (\bar{e}_s \gamma^{\bar{\sigma}} e_r) \\
& - \frac{2}{3} g_L^2 \mathcal{C}_{\ell e}^{ttsr} W_{\bar{\mu}}^I \widetilde{W}^{\bar{\mu}\bar{\sigma}I} (\bar{e}_s \gamma^{\bar{\sigma}} e_r) + \frac{2i}{3} g_L y_e^{tu} \mathcal{C}_{\ell e}^{stur} t_j^{Ii} H^j W_{\bar{\mu}}^I (\partial^{\bar{\mu}} \bar{\ell}_{is} e_r) \\
& + \frac{2}{3} g_Y \mathcal{C}_{\ell e}^{ttsr} (\partial^{\bar{\nu}} \bar{e}_s \bar{\mathcal{B}} \partial^{\bar{\nu}} e_r) + \frac{2}{3} g_Y \mathcal{C}_{\ell e}^{srtt} (\partial^{\bar{\nu}} \bar{\ell}_s \bar{\mathcal{B}} \partial^{\bar{\nu}} \ell_r) \\
& + \frac{2i}{3} g_L \bar{y}_e^{tu} \mathcal{C}_{\ell e}^{trsu} t_j^{Ii} W_{\bar{\mu}}^I (\bar{e}_s \ell_r^j) \partial^{\bar{\mu}} H_i^\dagger - \frac{2i}{3} g_L y_e^{tu} \mathcal{C}_{\ell e}^{stur} t_j^{Ii} W_{\bar{\mu}}^I (\bar{\ell}_{is} e_r) \partial^{\bar{\mu}} H^j \\
& - \frac{4}{3} g_L y_e^{vu} \bar{y}_e^{tu} \mathcal{C}_{\ell e}^{tvsr} (H^\dagger t^I H) (\bar{e}_s \bar{W}^I e_r) - \frac{3}{2} g_Y^2 \bar{y}_e^{tu} \mathcal{C}_{\ell e}^{trsu} B_{\bar{\mu}}^2 (\bar{e}_s H^\dagger \ell_r) - \frac{3}{2} g_Y^2 y_e^{tu} \mathcal{C}_{\ell e}^{stur} B_{\bar{\mu}}^2 (\bar{\ell}_s H e_r), \tag{2.39}
\end{aligned}$$

$$\begin{aligned}
\Delta S_{\mathcal{O}_{uu}} = & \frac{1}{6} g_s^3 \mathcal{C}_{uu}^{sr\bar{t}t} d^{ABC} G_{\bar{\nu}}^B G_{\bar{\nu}}^C (\bar{u}_s \bar{\mathcal{G}}^A u_r) + \frac{16}{81} g_Y^3 \left[ \mathcal{C}_{uu}^{st\bar{t}r} + 3\mathcal{C}_{uu}^{sr\bar{t}t} \right] B_{\bar{\mu}}^2 (\bar{u}_s \bar{\mathcal{B}} u_r) \\
& + \frac{2}{9} g_s^2 g_Y \mathcal{C}_{uu}^{sr\bar{t}t} G_{\bar{\mu}}^{A2} (\bar{u}_s \bar{\mathcal{B}} u_r) + \frac{8}{27} g_s g_Y^2 \mathcal{C}_{uu}^{st\bar{t}r} B_{\bar{\mu}}^2 (\bar{u}_s T^A \bar{\mathcal{G}}^A u_r) \\
& - \frac{i}{3} \mathcal{C}_{uu}^{st\bar{t}r} \left[ g_s^2 T_b^{Aa} T_c^{Bb} G_{\bar{\mu}}^B (\bar{u}_{as} \gamma^{\bar{\nu}} u_r^c) \partial^{\bar{\mu}} G_{\bar{\nu}}^A - g_s^2 T_b^{Aa} T_a^{Bc} G_{\bar{\mu}}^B (\bar{u}_{cs} \gamma^{\bar{\nu}} u_r^b) \partial^{\bar{\mu}} G_{\bar{\nu}}^A \right] \\
& - \frac{i}{3} \mathcal{C}_{uu}^{st\bar{t}r} \left[ g_s^2 T_b^{Aa} T_c^{Bb} (\bar{u}_{as} \bar{\mathcal{G}}^B u_r^c) \partial^{\bar{\nu}} G_{\bar{\nu}}^A - g_s^2 T_b^{Aa} T_a^{Bc} (\bar{u}_{cs} \bar{\mathcal{G}}^B u_r^b) \partial^{\bar{\nu}} G_{\bar{\nu}}^A \right] \\
& + \frac{4}{9} g_s^2 g_Y \mathcal{C}_{uu}^{sr\bar{t}t} B_{\bar{\mu}} G_{\bar{\mu}}^A (\bar{u}_s \bar{\mathcal{G}}^A u_r) - \frac{4i}{9} g_s^2 g_Y \mathcal{C}_{uu}^{st\bar{t}r} T_b^{Aa} T_a^{Bc} B_{\bar{\mu}} G_{\bar{\nu}}^B G_{\bar{\rho}}^A \varepsilon^{\bar{\mu}\bar{\nu}\bar{\rho}\bar{\sigma}} (\bar{u}_{cs} \gamma^{\bar{\sigma}} u_r^b) \\
& + \frac{4}{9} g_s^2 g_Y \mathcal{C}_{uu}^{st\bar{t}r} T_b^{Aa} T_a^{Bc} G_{\bar{\nu}}^A G_{\bar{\nu}}^B (\bar{u}_{cs} \bar{\mathcal{B}} u_r^b) \\
& + \frac{4}{9} \mathcal{C}_{uu}^{st\bar{t}r} \left[ g_s^2 g_Y T_b^{Aa} T_c^{Bb} B_{\bar{\mu}} G_{\bar{\mu}}^B (\bar{u}_{as} \bar{\mathcal{G}}^A u_r^c) + g_s^2 g_Y T_b^{Aa} T_a^{Bc} B_{\bar{\mu}} G_{\bar{\mu}}^B (\bar{u}_{cs} \bar{\mathcal{G}}^A u_r^b) \right] \\
& + \frac{16}{27} g_s g_Y^2 \mathcal{C}_{uu}^{st\bar{t}r} B_{\bar{\mu}} G_{\bar{\mu}}^A (\bar{u}_s T^A \bar{\mathcal{B}} u_r) + \frac{32}{27} g_Y^2 \left[ 3\mathcal{C}_{uu}^{sr\bar{t}t} - \mathcal{C}_{uu}^{st\bar{t}r} \right] B_{\bar{\mu}} \tilde{B}^{\bar{\mu}\bar{\sigma}} (\bar{u}_s \gamma^{\bar{\sigma}} u_r) \\
& + \frac{4}{3} g_s^2 \mathcal{C}_{uu}^{sr\bar{t}t} G_{\bar{\mu}}^A \tilde{G}^{\bar{\mu}\bar{\sigma}A} (\bar{u}_s \gamma^{\bar{\sigma}} u_r) - \frac{1}{6} g_s^3 \mathcal{C}_{uu}^{sr\bar{t}t} f^{ABC} G_{\bar{\mu}}^A G_{\bar{\nu}}^B G_{\bar{\rho}}^C \varepsilon^{\bar{\mu}\bar{\nu}\bar{\rho}\bar{\sigma}} (\bar{u}_s \gamma^{\bar{\sigma}} u_r) \\
& - \frac{4}{9} g_Y \left[ \mathcal{C}_{uu}^{st\bar{t}r} + 3\mathcal{C}_{uu}^{sr\bar{t}t} \right] (\bar{u}_s \bar{\mathcal{B}} \partial^2 u_r) - \frac{4}{9} g_Y \left[ \mathcal{C}_{uu}^{st\bar{t}r} + 3\mathcal{C}_{uu}^{sr\bar{t}t} \right] (\bar{u}_s \gamma^{\bar{\mu}} u_r) \partial^2 B_{\bar{\mu}} \\
& - \frac{2}{3} g_L y_u^{t\bar{v}} \bar{y}_u^{t\bar{u}} \left[ \mathcal{C}_{uu}^{su\bar{v}r} + 3\mathcal{C}_{uu}^{sr\bar{v}u} \right] (H^\dagger t^I H) (\bar{u}_s \bar{W}^I u_r) - \frac{2}{3} g_s \mathcal{C}_{uu}^{st\bar{t}r} (\bar{u}_s T^A \bar{\mathcal{G}}^A \partial^2 u_r) \\
& - \frac{2}{3} g_s \mathcal{C}_{uu}^{st\bar{t}r} \left[ 2g_s T_b^{Aa} T_c^{Bb} G_{\bar{\mu}}^B \tilde{G}^{\bar{\mu}\bar{\sigma}A} (\bar{u}_{as} \gamma^{\bar{\sigma}} u_r^c) + 2g_s T_b^{Aa} T_a^{Bc} G_{\bar{\mu}}^B \tilde{G}^{\bar{\mu}\bar{\sigma}A} (\bar{u}_{cs} \gamma^{\bar{\sigma}} u_r^b) \right] \\
& - \frac{2i}{3} g_s^3 \mathcal{C}_{uu}^{st\bar{t}r} T_b^{Aa} T_a^{Bc} T_c^{Cd} G_{\bar{\mu}}^A G_{\bar{\nu}}^C G_{\bar{\rho}}^B \varepsilon^{\bar{\mu}\bar{\nu}\bar{\rho}\bar{\sigma}} (\bar{u}_{ds} \gamma^{\bar{\sigma}} u_r^b) \\
& + \frac{2}{3} \mathcal{C}_{uu}^{st\bar{t}r} \left[ g_s^3 T_b^{Aa} T_c^{Bb} T_d^{Cc} G_{\bar{\mu}}^B G_{\bar{\mu}}^C (\bar{u}_{as} \bar{\mathcal{G}}^A u_r^d) + g_s^3 T_b^{Aa} T_a^{Bc} T_c^{Cd} G_{\bar{\mu}}^B G_{\bar{\mu}}^C (\bar{u}_{ds} \bar{\mathcal{G}}^A u_r^b) \right] \\
& - \frac{4}{9} g_Y \left[ \mathcal{C}_{uu}^{st\bar{t}r} + 3\mathcal{C}_{uu}^{sr\bar{t}t} \right] (\partial^2 \bar{u}_s \bar{\mathcal{B}} u_r) - \frac{2}{3} g_s^3 \mathcal{C}_{uu}^{st\bar{t}r} T_b^{Aa} T_a^{Bc} T_c^{Cd} G_{\bar{\mu}}^A G_{\bar{\mu}}^C (\bar{u}_{ds} \bar{\mathcal{G}}^B u_r^b) \\
& - \frac{2}{3} g_s \mathcal{C}_{uu}^{st\bar{t}r} (\partial^2 \bar{u}_s T^A \bar{\mathcal{G}}^A u_r) - \frac{2}{3} g_s \mathcal{C}_{uu}^{st\bar{t}r} (\bar{u}_s T^A \gamma^{\bar{\mu}} u_r) \partial^2 G_{\bar{\mu}}^A - \frac{8}{9} g_Y \left[ \mathcal{C}_{uu}^{st\bar{t}r} + 3\mathcal{C}_{uu}^{sr\bar{t}t} \right] (\partial^{\bar{\nu}} \bar{u}_s \bar{\mathcal{B}} \partial^{\bar{\nu}} u_r) \\
& - \frac{4}{3} g_s \mathcal{C}_{uu}^{st\bar{t}r} (\partial^{\bar{\nu}} \bar{u}_s T^A \bar{\mathcal{G}}^A \partial^{\bar{\nu}} u_r) - \frac{5}{3} g_Y y_u^{t\bar{v}} \bar{y}_u^{t\bar{u}} \left[ \mathcal{C}_{uu}^{su\bar{v}r} + 3\mathcal{C}_{uu}^{sr\bar{v}u} \right] (H^\dagger H) (\bar{u}_s \bar{\mathcal{B}} u_r) \\
& - \frac{5i}{3} \mathcal{C}_{uu}^{st\bar{t}r} \left[ g_s^2 T_b^{Aa} T_a^{Bc} G_{\bar{\nu}}^B (\bar{u}_{cs} \bar{\mathcal{G}}^A \partial^{\bar{\nu}} u_r^b) - g_s^2 T_b^{Aa} T_c^{Bb} G_{\bar{\nu}}^B (\partial^{\bar{\nu}} \bar{u}_{as} \bar{\mathcal{G}}^A u_r^c) \right] \\
& - \frac{5i}{3} \mathcal{C}_{uu}^{st\bar{t}r} \left[ g_s^2 T_b^{Aa} T_c^{Bb} G_{\bar{\nu}}^A (\partial^{\bar{\nu}} \bar{u}_{as} \bar{\mathcal{G}}^B u_r^c) - g_s^2 T_b^{Aa} T_a^{Bc} G_{\bar{\nu}}^A (\bar{u}_{cs} \bar{\mathcal{G}}^B \partial^{\bar{\nu}} u_r^b) \right] \\
& - \frac{16}{9} g_s g_Y \mathcal{C}_{uu}^{st\bar{t}r} G_{\bar{\mu}}^A \tilde{B}^{\bar{\mu}\bar{\sigma}} (\bar{u}_s T^A \gamma^{\bar{\sigma}} u_r) - \frac{16}{9} g_s g_Y \mathcal{C}_{uu}^{st\bar{t}r} B_{\bar{\mu}} \tilde{G}^{\bar{\mu}\bar{\sigma}A} (\bar{u}_s T^A \gamma^{\bar{\sigma}} u_r) \\
& - 2g_s y_u^{t\bar{v}} \bar{y}_u^{t\bar{u}} \mathcal{C}_{uu}^{su\bar{v}r} (H^\dagger H) (\bar{u}_s T^A \bar{\mathcal{G}}^A u_r) \\
& - 2ig_s \mathcal{C}_{uu}^{st\bar{t}r} \left[ g_s T_b^{Aa} T_c^{Bb} G_{\bar{\mu}}^B G^{\bar{\mu}\bar{\nu}A} (\bar{u}_{as} \gamma^{\bar{\nu}} u_r^c) - g_s T_b^{Aa} T_a^{Bc} G_{\bar{\mu}}^B G^{\bar{\mu}\bar{\nu}A} (\bar{u}_{cs} \gamma^{\bar{\nu}} u_r^b) \right], \tag{2.40}
\end{aligned}$$

$$\Delta S_{\mathcal{O}_{dd}} = \frac{2}{27} g_s g_Y^2 \mathcal{C}_{dd}^{st\bar{t}r} B_{\bar{\mu}}^2 (\bar{d}_s T^A \bar{\mathcal{G}}^A d_r) + \frac{4}{27} g_s g_Y^2 \mathcal{C}_{dd}^{st\bar{t}r} B_{\bar{\mu}} G_{\bar{\mu}}^A (\bar{d}_s T^A \bar{\mathcal{B}} d_r)$$

$$\begin{aligned}
& + \frac{1}{6} g_s^3 \mathcal{C}_{dd}^{srtt} d^{ABC} G_\nu^B G_\nu^C (\bar{d}_s \overleftrightarrow{\mathcal{G}}^A d_r) + \frac{2}{9} g_Y \left[ \mathcal{C}_{dd}^{sttr} + 3\mathcal{C}_{dd}^{srtt} \right] (\bar{d}_s \overleftrightarrow{\mathcal{B}} \partial^2 d_r) \\
& + \frac{2i}{9} g_s^2 g_Y \mathcal{C}_{dd}^{sttr} T_b^{Aa} T_a^{Bc} B_\mu G_\nu^B G_\rho^A \varepsilon^{\mu\nu\rho\sigma} (\bar{d}_{cs} \gamma^\sigma d_r^b) + \frac{2}{9} g_Y \left[ \mathcal{C}_{dd}^{sttr} + 3\mathcal{C}_{dd}^{srtt} \right] (\partial^2 \bar{d}_s \overleftrightarrow{\mathcal{B}} d_r) \\
& + \frac{2}{9} g_Y \left[ \mathcal{C}_{dd}^{sttr} + 3\mathcal{C}_{dd}^{srtt} \right] (\bar{d}_s \gamma^\mu d_r) \partial^2 B_\mu + \frac{8}{27} g_Y^2 \left[ 3\mathcal{C}_{dd}^{srtt} - \mathcal{C}_{dd}^{sttr} \right] B_\mu \tilde{B}^{\mu\sigma} (\bar{d}_s \gamma^\sigma d_r) \\
& + \frac{2}{3} g_L g_d^{tv} \bar{y}_d^{tu} \left[ \mathcal{C}_{dd}^{suuv} + 3\mathcal{C}_{dd}^{srvu} \right] (H^\dagger t^I H) (\bar{d}_s \overleftrightarrow{W}^I d_r) + \frac{8}{9} g_s g_Y \mathcal{C}_{dd}^{sttr} G_\mu^A \tilde{B}^{\mu\sigma} (\bar{d}_s T^A \gamma^\sigma d_r) \\
& + \frac{8}{9} g_s g_Y \mathcal{C}_{dd}^{sttr} B_\mu \tilde{G}^{\mu\sigma A} (\bar{d}_s T^A \gamma^\sigma d_r) + g_Y y_d^{tv} \bar{y}_d^{tu} \left[ \mathcal{C}_{dd}^{suuv} + 3\mathcal{C}_{dd}^{srvu} \right] (H^\dagger H) (\bar{d}_s \overleftrightarrow{\mathcal{B}} d_r) \\
& + \frac{4}{3} g_s^2 \mathcal{C}_{dd}^{srtt} G_\mu^A \tilde{G}^{\mu\sigma A} (\bar{d}_s \gamma^\sigma d_r) - \frac{2}{81} g_Y^3 \left[ \mathcal{C}_{dd}^{sttr} + 3\mathcal{C}_{dd}^{srtt} \right] B_\mu^2 (\bar{d}_s \overleftrightarrow{\mathcal{B}} d_r) \\
& - \frac{1}{9} g_s^2 g_Y \mathcal{C}_{dd}^{srtt} G_\mu^A{}^2 (\bar{d}_s \overleftrightarrow{\mathcal{B}} d_r) - \frac{1}{6} g_s^3 \mathcal{C}_{dd}^{srtt} f^{ABC} G_\mu^A G_\nu^B G_\rho^C \varepsilon^{\mu\nu\rho\sigma} (\bar{d}_s \gamma^\sigma d_r) \\
& - \frac{2}{9} g_s^2 g_Y \mathcal{C}_{dd}^{srtt} B_\mu G_\mu^A (\bar{d}_s \overleftrightarrow{\mathcal{G}}^A d_r) - \frac{2}{9} g_s^2 g_Y \mathcal{C}_{dd}^{sttr} T_b^{Aa} T_a^{Bc} G_\nu^A G_\nu^B (\bar{d}_{cs} \overleftrightarrow{\mathcal{B}} d_r^b) \\
& - \frac{2}{9} \mathcal{C}_{dd}^{sttr} \left[ g_s^2 g_Y T_b^{Aa} T_c^{Bb} B_\mu G_\mu^B (\bar{d}_{as} \overleftrightarrow{\mathcal{G}}^A d_r^c) + g_s^2 g_Y T_b^{Aa} T_a^{Bc} B_\mu G_\mu^B (\bar{d}_{cs} \overleftrightarrow{\mathcal{G}}^A d_r^b) \right] \\
& - \frac{i}{3} \mathcal{C}_{dd}^{sttr} \left[ g_s^2 T_b^{Aa} T_c^{Bb} G_\mu^B (\bar{d}_{as} \gamma^\nu d_r^c) \partial^\mu G_\nu^A - g_s^2 T_b^{Aa} T_a^{Bc} G_\mu^B (\bar{d}_{cs} \gamma^\nu d_r^b) \partial^\mu G_\nu^A \right] \\
& - \frac{i}{3} \mathcal{C}_{dd}^{sttr} \left[ g_s^2 T_b^{Aa} T_c^{Bb} (\bar{d}_{as} \overleftrightarrow{\mathcal{G}}^B d_r^c) \partial^\nu G_\nu^A - g_s^2 T_b^{Aa} T_a^{Bc} (\bar{d}_{cs} \overleftrightarrow{\mathcal{G}}^B d_r^b) \partial^\nu G_\nu^A \right] \\
& + \frac{4}{9} g_Y \left[ \mathcal{C}_{dd}^{sttr} + 3\mathcal{C}_{dd}^{srtt} \right] (\partial^\nu \bar{d}_s \overleftrightarrow{\mathcal{B}} \partial^\nu d_r) - \frac{2}{3} g_s \mathcal{C}_{dd}^{sttr} (\bar{d}_s T^A \overleftrightarrow{\mathcal{G}}^A \partial^2 d_r) \\
& - \frac{2}{3} g_s \mathcal{C}_{dd}^{sttr} \left[ 2g_s T_b^{Aa} T_c^{Bb} G_\mu^B \tilde{G}^{\mu\sigma A} (\bar{d}_{as} \gamma^\sigma d_r^c) + 2g_s T_b^{Aa} T_a^{Bc} G_\mu^B \tilde{G}^{\mu\sigma A} (\bar{d}_{cs} \gamma^\sigma d_r^b) \right] \\
& - \frac{2i}{3} g_s^3 \mathcal{C}_{dd}^{sttr} T_b^{Aa} T_a^{Bc} T_c^{Cd} G_\mu^A G_\nu^C G_\rho^B \varepsilon^{\mu\nu\rho\sigma} (\bar{d}_{ds} \gamma^\sigma d_r^b) \\
& + \frac{2}{3} \mathcal{C}_{dd}^{sttr} \left[ g_s^3 T_b^{Aa} T_c^{Bb} T_d^{Cd} G_\mu^B G_\mu^C (\bar{d}_{as} \overleftrightarrow{\mathcal{G}}^A d_r^d) + g_s^3 T_b^{Aa} T_a^{Bc} T_c^{Cd} G_\mu^B G_\mu^C (\bar{d}_{ds} \overleftrightarrow{\mathcal{G}}^A d_r^b) \right] \\
& - \frac{2}{3} g_s^3 \mathcal{C}_{dd}^{sttr} T_b^{Aa} T_a^{Bc} T_c^{Cd} G_\mu^A G_\mu^C (\bar{d}_{ds} \overleftrightarrow{\mathcal{G}}^B d_r^b) - \frac{2}{3} g_s \mathcal{C}_{dd}^{sttr} (\partial^2 \bar{d}_s T^A \overleftrightarrow{\mathcal{G}}^A d_r) \\
& - \frac{2}{3} g_s \mathcal{C}_{dd}^{sttr} (\bar{d}_s T^A \gamma^\mu d_r) \partial^2 G_\mu^A - \frac{4}{3} g_s \mathcal{C}_{dd}^{sttr} (\partial^\nu \bar{d}_s T^A \overleftrightarrow{\mathcal{G}}^A \partial^\nu d_r) \\
& - \frac{5i}{3} \mathcal{C}_{dd}^{sttr} \left[ g_s^2 T_b^{Aa} T_a^{Bc} G_\nu^B (\bar{d}_{cs} \overleftrightarrow{\mathcal{G}}^A \partial^\nu d_r^b) - g_s^2 T_b^{Aa} T_c^{Bb} G_\nu^B (\partial^\nu \bar{d}_{as} \overleftrightarrow{\mathcal{G}}^A d_r^c) \right] \\
& - \frac{5i}{3} \mathcal{C}_{dd}^{sttr} \left[ g_s^2 T_b^{Aa} T_c^{Bb} G_\nu^A (\partial^\nu \bar{d}_{as} \overleftrightarrow{\mathcal{G}}^B d_r^c) - g_s^2 T_b^{Aa} T_a^{Bc} G_\nu^A (\bar{d}_{cs} \overleftrightarrow{\mathcal{G}}^B \partial^\nu d_r^b) \right] \\
& - 2g_s y_d^{tv} \bar{y}_d^{tu} \mathcal{C}_{dd}^{suuv} (H^\dagger H) (\bar{d}_s T^A \overleftrightarrow{\mathcal{G}}^A d_r) \\
& - 2ig_s \mathcal{C}_{dd}^{sttr} \left[ g_s T_b^{Aa} T_c^{Bb} G_\mu^B G^{\mu\nu A} (\bar{d}_{as} \gamma^\nu d_r^c) - g_s T_b^{Aa} T_a^{Bc} G_\mu^B G^{\mu\nu A} (\bar{d}_{cs} \gamma^\nu d_r^b) \right], \tag{2.41}
\end{aligned}$$

$$\begin{aligned}
\Delta S_{\mathcal{O}_{qq}^{(1)}} &= \frac{1}{324} g_Y^3 \left[ (\mathcal{C}_{qq}^{(1)})^{sttr} + 6(\mathcal{C}_{qq}^{(1)})^{srtt} \right] B_\mu^2 (\bar{q}_s \overleftrightarrow{\mathcal{B}} q_r) + \frac{1}{54} g_s g_Y^2 (\mathcal{C}_{qq}^{(1)})^{rsst} B_\mu^2 (\bar{q}_r T^A \overleftrightarrow{\mathcal{G}}^A q_t) \\
&+ \frac{1}{54} g_L g_Y^2 (\mathcal{C}_{qq}^{(1)})^{rsst} B_\mu^2 (\bar{q}_r t^I \overleftrightarrow{W}^I q_t) + \frac{1}{36} g_L^2 g_Y \left[ (\mathcal{C}_{qq}^{(1)})^{sttr} + 6(\mathcal{C}_{qq}^{(1)})^{srtt} \right] W_\mu^{I2} (\bar{q}_s \overleftrightarrow{\mathcal{B}} q_r)
\end{aligned}$$

$$\begin{aligned}
& + \frac{1}{27} g_s g_Y^2 (\mathcal{C}_{qq}^{(1)})^{rsst} B_{\bar{\mu}} G_{\bar{\mu}}^A (\bar{q}_r T^A \bar{\mathcal{B}}_{qt}) + \frac{1}{27} g_L g_Y^2 (\mathcal{C}_{qq}^{(1)})^{rsst} B_{\bar{\mu}} W_{\bar{\mu}}^I (\bar{q}_r t^I \bar{\mathcal{B}}_{qt}) \\
& + \frac{1}{18} g_L^2 g_Y (\mathcal{C}_{qq}^{(1)})^{rsst} \varepsilon^{IJK} B_{\bar{\mu}} W_{\bar{\nu}}^I W_{\bar{\rho}}^J \varepsilon^{\bar{\mu}\bar{\nu}\bar{\rho}\bar{\sigma}} (\bar{q}_r t^K \gamma^{\bar{\sigma}} q_t) \\
& + \frac{1}{18} g_L^2 g_Y \left[ (\mathcal{C}_{qq}^{(1)})^{sttr} + 6(\mathcal{C}_{qq}^{(1)})^{srtt} \right] B_{\bar{\mu}} W_{\bar{\mu}}^I (\bar{q}_s \bar{\mathcal{W}}^I q_r) + \frac{2}{27} g_Y^2 \left[ (\mathcal{C}_{qq}^{(1)})^{sttr} - 6(\mathcal{C}_{qq}^{(1)})^{srtt} \right] B_{\bar{\mu}} \tilde{B}^{\bar{\mu}\bar{\sigma}} (\bar{q}_s \gamma^{\bar{\sigma}} q_r) \\
& + \frac{1}{9} g_s^2 g_Y (\mathcal{C}_{qq}^{(1)})^{srtt} G_{\bar{\mu}}^{A2} (\bar{q}_s \bar{\mathcal{B}}_{qr}) + \frac{1}{9} g_Y \left[ -(\mathcal{C}_{qq}^{(1)})^{sttr} - 6(\mathcal{C}_{qq}^{(1)})^{srtt} \right] (\bar{q}_s \bar{\mathcal{B}} \partial^2 q_r) \\
& + \frac{i}{9} g_s^2 g_Y (\mathcal{C}_{qq}^{(1)})^{rsst} T_b^{Aa} T_a^{Bc} B_{\bar{\mu}} G_{\bar{\nu}}^B G_{\bar{\rho}}^A \varepsilon^{\bar{\mu}\bar{\nu}\bar{\rho}\bar{\sigma}} (\bar{q}_{cr} \gamma^{\bar{\sigma}} q_t^b) \\
& + \frac{1}{9} g_s^2 g_Y (\mathcal{C}_{qq}^{(1)})^{rsst} T_b^{Aa} T_a^{Bc} G_{\bar{\nu}}^A G_{\bar{\rho}}^B (\bar{q}_{cr} \bar{\mathcal{B}}_{qt}^b) \\
& + \frac{1}{9} (\mathcal{C}_{qq}^{(1)})^{sttr} \left[ g_s^2 g_Y T_b^{Aa} T_c^{Bb} B_{\bar{\mu}} G_{\bar{\mu}}^B (\bar{q}_{as} \bar{\mathcal{G}}^A q_r^c) + g_s^2 g_Y T_b^{Aa} T_a^{Bc} B_{\bar{\mu}} G_{\bar{\mu}}^B (\bar{q}_{cs} \bar{\mathcal{G}}^A q_r^b) \right] \\
& + \frac{1}{9} g_Y \left[ -(\mathcal{C}_{qq}^{(1)})^{sttr} - 6(\mathcal{C}_{qq}^{(1)})^{srtt} \right] (\partial^2 \bar{q}_s \bar{\mathcal{B}}_{qr}) + \frac{1}{9} g_Y \left[ -(\mathcal{C}_{qq}^{(1)})^{sttr} - 6(\mathcal{C}_{qq}^{(1)})^{srtt} \right] (\bar{q}_s \gamma^{\bar{\mu}} q_r) \partial^2 B_{\bar{\mu}} \\
& + \frac{1}{6} g_L^2 g_s (\mathcal{C}_{qq}^{(1)})^{rsst} W_{\bar{\mu}}^{I2} (\bar{q}_r T^A \bar{\mathcal{G}}^A q_t) + \frac{2}{9} g_L g_Y (\mathcal{C}_{qq}^{(1)})^{rsst} B_{\bar{\mu}} \widetilde{W}^{\bar{\mu}\bar{\sigma}I} (\bar{q}_r t^I \gamma^{\bar{\sigma}} q_t) \\
& + \frac{2}{9} g_L g_s g_Y (\mathcal{C}_{qq}^{(1)})^{rsst} G_{\bar{\nu}}^A W_{\bar{\nu}}^I (\bar{q}_r t^I T^A \bar{\mathcal{B}}_{qt}) + \frac{2}{9} g_L g_s g_Y (\mathcal{C}_{qq}^{(1)})^{rsst} B_{\bar{\mu}} W_{\bar{\mu}}^I (\bar{q}_r t^I T^A \bar{\mathcal{G}}^A q_t) \\
& + \frac{2}{9} g_L g_s g_Y (\mathcal{C}_{qq}^{(1)})^{rsst} B_{\bar{\mu}} G_{\bar{\mu}}^A (\bar{q}_r t^I T^A \bar{\mathcal{W}}^I q_t) + \frac{2}{9} g_s^2 g_Y (\mathcal{C}_{qq}^{(1)})^{srtt} B_{\bar{\mu}} G_{\bar{\mu}}^A (\bar{q}_s \bar{\mathcal{G}}^A q_r) \\
& + \frac{2}{9} \left[ 3(\mathcal{C}_{qq}^{(1)})^{srtt} - (\mathcal{C}_{qq}^{(1)})^{sttr} \right] \left[ g_L g_Y B_{\bar{\mu}} W_{\bar{\nu}}^I \varepsilon^{\bar{\mu}\bar{\nu}\bar{\rho}\bar{\sigma}} (\bar{q}_s t^I \gamma^{\bar{\rho}} \partial^{\bar{\sigma}} q_r) + g_L g_Y B_{\bar{\mu}} W_{\bar{\nu}}^I \varepsilon^{\bar{\mu}\bar{\nu}\bar{\rho}\bar{\sigma}} (\partial^{\bar{\sigma}} \bar{q}_s t^I \gamma^{\bar{\rho}} q_r) \right] \\
& + \frac{1}{3} g_s^3 (\mathcal{C}_{qq}^{(1)})^{rslt} f^{ABC} G_{\bar{\mu}}^A G_{\bar{\nu}}^B G_{\bar{\rho}}^C \varepsilon^{\bar{\mu}\bar{\nu}\bar{\rho}\bar{\sigma}} (\bar{q}_r \gamma^{\bar{\sigma}} q_s) + \frac{1}{3} g_s^3 (\mathcal{C}_{qq}^{(1)})^{rslt} d^{ABC} G_{\bar{\nu}}^B G_{\bar{\rho}}^C (\bar{q}_r \bar{\mathcal{G}}^A q_s) \\
& + \frac{1}{3} g_L^2 g_s (\mathcal{C}_{qq}^{(1)})^{rsst} G_{\bar{\mu}}^A W_{\bar{\mu}}^I (\bar{q}_r T^A \bar{\mathcal{W}}^I q_t) + \frac{1}{3} g_L^2 g_s (\mathcal{C}_{qq}^{(1)})^{rsst} \varepsilon^{IJK} G_{\bar{\mu}}^A W_{\bar{\nu}}^I W_{\bar{\rho}}^J \varepsilon^{\bar{\mu}\bar{\nu}\bar{\rho}\bar{\sigma}} (\bar{q}_r t^K T^A \gamma^{\bar{\sigma}} q_t) \\
& + \frac{1}{3} g_L^2 (\mathcal{C}_{qq}^{(1)})^{rsst} \varepsilon^{IJK} W_{\bar{\mu}}^J (\bar{q}_r t^K \gamma^{\bar{\nu}} q_t) \partial^{\bar{\mu}} W_{\bar{\nu}}^I \\
& - \frac{i}{3} (\mathcal{C}_{qq}^{(1)})^{sttr} \left[ g_s^2 T_b^{Aa} T_c^{Bb} (\bar{q}_{as} \bar{\mathcal{G}}^B q_r^c) \partial^{\bar{\nu}} G_{\bar{\nu}}^A - g_s^2 T_b^{Aa} T_a^{Bc} (\bar{q}_{cs} \bar{\mathcal{G}}^B q_r^b) \partial^{\bar{\nu}} G_{\bar{\nu}}^A \right] \\
& + \frac{4}{9} g_s g_Y (\mathcal{C}_{qq}^{(1)})^{rsst} G_{\bar{\mu}}^A \tilde{B}^{\bar{\mu}\bar{\sigma}} (\bar{q}_r T^A \gamma^{\bar{\sigma}} q_t) + \frac{4}{9} g_s g_Y (\mathcal{C}_{qq}^{(1)})^{rsst} B_{\bar{\mu}} \tilde{G}^{\bar{\mu}\bar{\sigma}A} (\bar{q}_r T^A \gamma^{\bar{\sigma}} q_t) \\
& + \frac{1}{2} g_L^3 (\mathcal{C}_{qq}^{(1)})^{rslt} \varepsilon^{IJK} W_{\bar{\mu}}^I W_{\bar{\nu}}^J W_{\bar{\rho}}^K \varepsilon^{\bar{\mu}\bar{\nu}\bar{\rho}\bar{\sigma}} (\bar{q}_r \gamma^{\bar{\sigma}} q_s) + \frac{1}{2} g_L^3 (\mathcal{C}_{qq}^{(1)})^{rsst} W_{\bar{\mu}}^{I2} (\bar{q}_r t^I \bar{\mathcal{W}}^I q_t) \\
& + \frac{2}{3} g_L g_Y (\mathcal{C}_{qq}^{(1)})^{rslt} B_{\bar{\mu}} \widetilde{W}^{\bar{\mu}\bar{\sigma}I} (\bar{q}_r t^I \gamma^{\bar{\sigma}} q_s) + \frac{2}{3} g_L g_Y (\mathcal{C}_{qq}^{(1)})^{rsst} W_{\bar{\mu}}^I \tilde{B}^{\bar{\mu}\bar{\sigma}} (\bar{q}_r t^I \gamma^{\bar{\sigma}} q_t) \\
& + \frac{2}{3} g_L^2 \left[ (\mathcal{C}_{qq}^{(1)})^{sttr} - 6(\mathcal{C}_{qq}^{(1)})^{srtt} \right] W_{\bar{\mu}}^I \widetilde{W}^{\bar{\mu}\bar{\sigma}I} (\bar{q}_s \gamma^{\bar{\sigma}} q_r) + \frac{2}{3} g_L g_s^2 (\mathcal{C}_{qq}^{(1)})^{rsst} T_b^{Aa} T_a^{Bc} G_{\bar{\mu}}^A G_{\bar{\mu}}^B (\bar{q}_{cr} t^I \bar{\mathcal{W}}^I q_t^b) \\
& - \frac{2i}{3} g_s (\mathcal{C}_{qq}^{(1)})^{sttr} \left[ g_s T_b^{Aa} T_c^{Bb} G_{\bar{\mu}}^B G^{\bar{\mu}\bar{\nu}A} (\bar{q}_{as} \gamma^{\bar{\nu}} q_r^c) - g_s T_b^{Aa} T_a^{Bc} G_{\bar{\mu}}^B G^{\bar{\mu}\bar{\nu}A} (\bar{q}_{cs} \gamma^{\bar{\nu}} q_r^b) \right] \\
& + \frac{2}{3} g_s (\mathcal{C}_{qq}^{(1)})^{sttr} \left[ 2g_s T_b^{Aa} T_c^{Bb} G_{\bar{\mu}}^B \tilde{G}^{\bar{\mu}\bar{\sigma}A} (\bar{q}_{as} \gamma^{\bar{\sigma}} q_r^c) + 2g_s T_b^{Aa} T_a^{Bc} G_{\bar{\mu}}^B \tilde{G}^{\bar{\mu}\bar{\sigma}A} (\bar{q}_{cs} \gamma^{\bar{\sigma}} q_r^b) \right] \\
& + \frac{2}{3} (\mathcal{C}_{qq}^{(1)})^{sttr} \left[ g_L g_s^2 T_b^{Aa} T_c^{Bb} G_{\bar{\mu}}^B W_{\bar{\mu}}^I (\bar{q}_{as} t^I \bar{\mathcal{G}}^A q_r^c) + g_L g_s^2 T_b^{Aa} T_a^{Bc} G_{\bar{\mu}}^B W_{\bar{\mu}}^I (\bar{q}_{cs} t^I \bar{\mathcal{G}}^A q_r^b) \right]
\end{aligned}$$

$$\begin{aligned}
& + \frac{2i}{3} g_s^3 (\mathcal{C}_{qq}^{(1)})^{rsst} T_b^{Aa} T_a^{Bc} T_c^{Cd} G_{\bar{\mu}}^A G_{\bar{\nu}}^C G_{\bar{\rho}}^B \varepsilon^{\bar{\mu}\bar{\nu}\bar{\rho}\bar{\sigma}} (\bar{q}_{dr} \gamma^{\bar{\sigma}} q_t^b) \\
& + \frac{4}{3} g_L g_s (\mathcal{C}_{qq}^{(1)})^{rsst} G_{\bar{\mu}}^A \widetilde{W}^{\bar{\mu}\bar{\sigma}I} (\bar{q}_r t^I T^A \gamma^{\bar{\sigma}} q_t) + \frac{4}{3} g_L y_u^{us} \bar{y}_u^{rs} (\mathcal{C}_{qq}^{(1)})^{turv} (H^\dagger t^I H) (\bar{q}_t \bar{W}^I q_v) \\
& + \frac{4}{3} (\mathcal{C}_{qq}^{(1)})^{sttr} \left[ g_L g_s G_{\bar{\mu}}^A W_{\bar{\nu}}^I \varepsilon^{\bar{\mu}\bar{\nu}\bar{\rho}\bar{\sigma}} (\bar{q}_s t^I T^A \gamma^{\bar{\sigma}} \partial^{\bar{\rho}} q_r) + g_L g_s G_{\bar{\mu}}^A W_{\bar{\nu}}^I \varepsilon^{\bar{\mu}\bar{\nu}\bar{\rho}\bar{\sigma}} (\partial^{\bar{\rho}} \bar{q}_s t^I T^A \gamma^{\bar{\sigma}} q_r) \right] \\
& + 2g_L^2 (\mathcal{C}_{qq}^{(1)})^{rsst} \varepsilon^{IJK} W_{\bar{\mu}}^J W_{\bar{\nu}}^{\bar{\mu}\bar{\nu}I} (\bar{q}_r t^K \gamma^{\bar{\nu}} q_t) + 2g_s y_u^{us} \bar{y}_u^{rs} (\mathcal{C}_{qq}^{(1)})^{turv} (\bar{q}_t T^A H \bar{G}^A H^\dagger q_v) \\
& - 2ig_L g_s^2 (\mathcal{C}_{qq}^{(1)})^{rsst} T_b^{Aa} T_a^{Bc} G_{\bar{\mu}}^A G_{\bar{\nu}}^B W_{\bar{\rho}}^I \varepsilon^{\bar{\mu}\bar{\nu}\bar{\rho}\bar{\sigma}} (\bar{q}_{cr} t^I \gamma^{\bar{\sigma}} q_t^b) \\
& + 2(\mathcal{C}_{qq}^{(1)})^{sttr} \left[ g_s^3 T_b^{Aa} T_c^{Bb} T_d^{Cc} G_{\bar{\mu}}^B G_{\bar{\nu}}^C (\bar{q}_{as} \bar{G}^A q_r^d) + g_s^3 T_b^{Aa} T_a^{Bc} T_c^{Cd} G_{\bar{\mu}}^B G_{\bar{\nu}}^C (\bar{q}_{ds} \bar{G}^A q_r^b) \right] \\
& + 4g_L g_s (\mathcal{C}_{qq}^{(1)})^{rsst} W_{\bar{\mu}}^I \widetilde{G}^{\bar{\mu}\bar{\sigma}A} (\bar{q}_r t^I T^A \gamma^{\bar{\sigma}} q_t) + 8g_L y_u^{us} \bar{y}_u^{rs} (\mathcal{C}_{qq}^{(1)})^{turv} (H^\dagger t^I H) (\bar{q}_t \bar{W}^I q_v) \\
& - \frac{1}{12} g_L^3 (\mathcal{C}_{qq}^{(1)})^{rsst} \varepsilon^{IJK} W_{\bar{\mu}}^I W_{\bar{\nu}}^J W_{\bar{\rho}}^K \varepsilon^{\bar{\mu}\bar{\nu}\bar{\rho}\bar{\sigma}} (\bar{q}_r \gamma^{\bar{\sigma}} q_t) \\
& - \frac{2}{9} g_Y \left[ (\mathcal{C}_{qq}^{(1)})^{sttr} + 6(\mathcal{C}_{qq}^{(1)})^{srtt} \right] (\partial^{\bar{\nu}} \bar{q}_s \bar{B} \partial^{\bar{\nu}} q_r) - \frac{1}{3} g_L^3 (\mathcal{C}_{qq}^{(1)})^{rsst} W_{\bar{\mu}}^I W_{\bar{\nu}}^J (\bar{q}_r t^I \bar{W}^J q_t) \\
& - \frac{1}{3} g_L^2 g_Y (\mathcal{C}_{qq}^{(1)})^{rstt} \varepsilon^{IJK} B_{\bar{\mu}} W_{\bar{\nu}}^I W_{\bar{\rho}}^J \varepsilon^{\bar{\mu}\bar{\nu}\bar{\rho}\bar{\sigma}} (\bar{q}_r t^K \gamma^{\bar{\sigma}} q_s) \\
& - \frac{1}{3} g_L^2 (\mathcal{C}_{qq}^{(1)})^{rsst} \varepsilon^{IJK} (\bar{q}_r t^K \bar{W}^I q_t) \partial^{\bar{\nu}} W_{\bar{\nu}}^J - \frac{2}{3} g_s (\mathcal{C}_{qq}^{(1)})^{rsst} (\bar{q}_r T^A \bar{G}^A \partial^2 q_t) \\
& - \frac{2}{3} g_L g_Y (\mathcal{C}_{qq}^{(1)})^{rstt} W_{\bar{\mu}}^I \widetilde{B}^{\bar{\mu}\bar{\sigma}} (\bar{q}_r t^I \gamma^{\bar{\sigma}} q_s) - \frac{2}{3} g_L (\mathcal{C}_{qq}^{(1)})^{rsst} (\bar{q}_r t^I \bar{W}^I \partial^2 q_t) \\
& - \frac{2}{3} g_Y y_d^{vu} \bar{y}_d^{tu} (\mathcal{C}_{qq}^{(1)})^{svtr} (\bar{q}_s H \bar{B} H^\dagger q_r) - \frac{2}{3} g_s (\mathcal{C}_{qq}^{(1)})^{rsst} (\partial^2 \bar{q}_r T^A \bar{G}^A q_t) - \frac{2}{3} g_L (\mathcal{C}_{qq}^{(1)})^{rsst} (\partial^2 \bar{q}_r t^I \bar{W}^I q_t) \\
& - \frac{2}{3} g_s (\mathcal{C}_{qq}^{(1)})^{rsst} (\bar{q}_r T^A \gamma^{\bar{\mu}} q_t) \partial^2 G_{\bar{\mu}}^A - \frac{2}{3} g_L (\mathcal{C}_{qq}^{(1)})^{rsst} (\bar{q}_r t^I \gamma^{\bar{\mu}} q_t) \partial^2 W_{\bar{\mu}}^I - \frac{4}{3} g_L y_d^{us} \bar{y}_d^{rs} (\mathcal{C}_{qq}^{(1)})^{turv} (H^\dagger t^I H) (\bar{q}_t \bar{W}^I q_v) \\
& - \frac{4}{3} g_L y_d^{us} \bar{y}_d^{rs} (\mathcal{C}_{qq}^{(1)})^{turv} (H^\dagger H) (\bar{q}_t t^I \bar{W}^I q_v) - \frac{4}{3} g_L y_u^{us} \bar{y}_u^{rs} (\mathcal{C}_{qq}^{(1)})^{turv} (H^\dagger H) (\bar{q}_t t^I \bar{W}^I q_v) \\
& - \frac{4}{3} g_s (\mathcal{C}_{qq}^{(1)})^{rsst} (\partial^{\bar{\nu}} \bar{q}_r T^A \bar{G}^A \partial^{\bar{\nu}} q_t) - \frac{4}{3} g_L (\mathcal{C}_{qq}^{(1)})^{rsst} (\partial^{\bar{\nu}} \bar{q}_r t^I \bar{W}^I \partial^{\bar{\nu}} q_t) \\
& + \frac{4i}{3} (\mathcal{C}_{qq}^{(1)})^{sttr} \left[ g_s^2 T_b^{Aa} T_c^{Bb} G_{\bar{\mu}}^B (\bar{q}_{as} \gamma^{\bar{\nu}} q_r^c) \partial^{\bar{\nu}} G_{\bar{\mu}}^A - g_s^2 T_b^{Aa} T_a^{Bc} G_{\bar{\mu}}^B (\bar{q}_{cs} \gamma^{\bar{\nu}} q_r^b) \partial^{\bar{\nu}} G_{\bar{\mu}}^A \right] \\
& - \frac{5}{3} (\mathcal{C}_{qq}^{(1)})^{sttr} \left[ g_L^2 \varepsilon^{IJK} W_{\bar{\nu}}^J (\bar{q}_s t^K \bar{W}^I \partial^{\bar{\nu}} q_r) + g_L^2 \varepsilon^{IJK} W_{\bar{\nu}}^J (\partial^{\bar{\nu}} \bar{q}_s t^K \bar{W}^I q_r) \right] \\
& - \frac{5i}{3} (\mathcal{C}_{qq}^{(1)})^{sttr} \left[ g_s^2 T_b^{Aa} T_a^{Bc} G_{\bar{\nu}}^B (\bar{q}_{cs} \bar{G}^A \partial^{\bar{\nu}} q_r^b) - g_s^2 T_b^{Aa} T_c^{Bb} G_{\bar{\nu}}^B (\partial^{\bar{\nu}} \bar{q}_{as} \bar{G}^A q_r^c) \right] \\
& - \frac{5i}{3} (\mathcal{C}_{qq}^{(1)})^{sttr} \left[ g_s^2 T_b^{Aa} T_c^{Bb} G_{\bar{\nu}}^A (\partial^{\bar{\nu}} \bar{q}_{as} \bar{G}^B q_r^c) - g_s^2 T_b^{Aa} T_a^{Bc} G_{\bar{\nu}}^A (\bar{q}_{cs} \bar{G}^B \partial^{\bar{\nu}} q_r^b) \right] \\
& - \frac{5i}{3} (\mathcal{C}_{qq}^{(1)})^{sttr} \left[ g_s^2 T_b^{Aa} T_c^{Bb} G_{\bar{\mu}}^B (\bar{q}_{as} \gamma^{\bar{\nu}} q_r^c) \partial^{\bar{\mu}} G_{\bar{\nu}}^A - g_s^2 T_b^{Aa} T_a^{Bc} G_{\bar{\mu}}^B (\bar{q}_{cs} \gamma^{\bar{\nu}} q_r^b) \partial^{\bar{\mu}} G_{\bar{\nu}}^A \right] \\
& - 2g_Y y_d^{vu} \bar{y}_d^{tu} (\mathcal{C}_{qq}^{(1)})^{srtv} (H^\dagger H) (\bar{q}_s \bar{B} q_r) - 2g_s y_u^{us} \bar{y}_u^{rs} (\mathcal{C}_{qq}^{(1)})^{turv} (H^\dagger H) (\bar{q}_t T^A \bar{G}^A q_v) \\
& - 2g_s y_d^{us} \bar{y}_d^{rs} (\mathcal{C}_{qq}^{(1)})^{turv} (\bar{q}_t T^A H \bar{G}^A H^\dagger q_v) \\
& - \frac{8}{3} g_s^2 (\mathcal{C}_{qq}^{(1)})^{srtt} G_{\bar{\mu}}^A \widetilde{G}^{\bar{\mu}\bar{\sigma}A} (\bar{q}_s \gamma^{\bar{\sigma}} q_r) - \frac{10}{3} g_s^3 (\mathcal{C}_{qq}^{(1)})^{rsst} T_b^{Aa} T_a^{Bc} T_c^{Cd} G_{\bar{\mu}}^A G_{\bar{\nu}}^C (\bar{q}_{dr} \bar{G}^B q_t^b)
\end{aligned}$$

$$-8g_L y_d^{vs} \bar{y}_d^{rs} (\mathcal{C}_{qq}^{(1)})^{turv} (H^\dagger t^I H) (\bar{q}_t \bar{W}^I q_u), \quad (2.42)$$

$$\begin{aligned} \Delta S_{\mathcal{O}_{qq}^{(3)}} = & \frac{1}{108} g_Y^3 (\mathcal{C}_{qq}^{(3)})^{sttr} B_\mu^2 (\bar{q}_s \bar{\mathcal{B}} q_r) + \frac{1}{18} g_s g_Y^2 (\mathcal{C}_{qq}^{(3)})^{rsst} B_\mu^2 (\bar{q}_r T^A \bar{\mathcal{G}}^A q_t) + \frac{1}{12} g_L^2 g_Y (\mathcal{C}_{qq}^{(3)})^{sttr} W_\mu^{I2} (\bar{q}_s \bar{\mathcal{B}} q_r) \\ & + \frac{1}{9} g_s g_Y^2 (\mathcal{C}_{qq}^{(3)})^{rsst} B_\mu G_\mu^A (\bar{q}_r T^A \bar{\mathcal{B}} q_t) + \frac{1}{9} g_L g_Y^2 (\mathcal{C}_{qq}^{(3)})^{rstt} B_\mu^2 (\bar{q}_r t^I \bar{W}^I q_s) \\ & + \frac{1}{6} g_L^2 g_Y (\mathcal{C}_{qq}^{(3)})^{sttr} B_\mu W_\mu^I (\bar{q}_s \bar{W}^I q_r) + \frac{2}{9} g_L g_Y^2 (\mathcal{C}_{qq}^{(3)})^{rstt} B_\mu W_\mu^I (\bar{q}_r t^I \bar{\mathcal{B}} q_s) \\ & + \frac{2}{9} g_Y^2 (\mathcal{C}_{qq}^{(3)})^{sttr} B_\mu \tilde{B}^{\bar{\mu}\bar{\sigma}} (\bar{q}_s \gamma^{\bar{\sigma}} q_r) \\ & + \frac{2}{9} \left[ (\mathcal{C}_{qq}^{(3)})^{sttr} - 3(\mathcal{C}_{qq}^{(3)})^{srtt} \right] \left[ g_L g_Y B_\mu W_\nu^I \varepsilon^{\bar{\mu}\bar{\nu}\bar{\rho}\bar{\sigma}} (\bar{q}_s t^I \gamma^{\bar{\rho}} \partial^{\bar{\sigma}} q_r) + g_L g_Y B_\mu W_\nu^I \varepsilon^{\bar{\mu}\bar{\nu}\bar{\rho}\bar{\sigma}} (\partial^{\bar{\sigma}} \bar{q}_s t^I \gamma^{\bar{\rho}} q_r) \right] \\ & + \frac{1}{3} g_L^3 (\mathcal{C}_{qq}^{(3)})^{rsst} W_\mu^I W_\mu^J (\bar{q}_r t^I \bar{W}^J q_t) + \frac{i}{3} g_s^2 g_Y (\mathcal{C}_{qq}^{(3)})^{rsst} T_b^{Aa} T_a^{Bc} B_\mu G_\nu^B G_\rho^A \varepsilon^{\bar{\mu}\bar{\nu}\bar{\rho}\bar{\sigma}} (\bar{q}_{cr} \gamma^{\bar{\sigma}} q_t^b) \\ & + \frac{1}{3} g_s^2 g_Y (\mathcal{C}_{qq}^{(3)})^{rsst} T_b^{Aa} T_a^{Bc} G_\nu^A G_\nu^B (\bar{q}_{cr} \bar{\mathcal{B}} q_t^b) \\ & + \frac{1}{3} (\mathcal{C}_{qq}^{(3)})^{sttr} \left[ g_s^2 g_Y T_b^{Aa} T_c^{Bb} B_\mu G_\mu^B (\bar{q}_{as} \bar{\mathcal{G}}^A q_r^c) + g_s^2 g_Y T_b^{Aa} T_a^{Bc} B_\mu G_\mu^B (\bar{q}_{cs} \bar{\mathcal{G}}^A q_r^b) \right] \\ & + \frac{1}{3} g_L^2 (\mathcal{C}_{qq}^{(3)})^{rsst} \varepsilon^{IJK} (\bar{q}_r t^K \bar{W}^I q_t) \partial^{\bar{\nu}} W_\nu^J + \frac{1}{2} g_L^2 g_s (\mathcal{C}_{qq}^{(3)})^{rsst} W_\mu^{I2} (\bar{q}_r T^A \bar{\mathcal{G}}^A q_t) \\ & + \frac{2}{3} g_L g_s^2 (\mathcal{C}_{qq}^{(3)})^{rstt} G_\mu^A (\bar{q}_r t^I \bar{W}^I q_s) + \frac{2}{3} g_L (\mathcal{C}_{qq}^{(3)})^{rsst} (\bar{q}_r t^I \bar{W}^I \partial^2 q_t) \\ & + \frac{2}{3} g_L g_Y (\mathcal{C}_{qq}^{(3)})^{rstt} \varepsilon^{IJK} B_\mu W_\nu^I W_\rho^J \varepsilon^{\bar{\mu}\bar{\nu}\bar{\rho}\bar{\sigma}} (\bar{q}_r t^K \gamma^{\bar{\sigma}} q_s) \\ & + \frac{2}{3} g_Y y_d^{vu} \bar{y}_d^{tu} \left[ 3(\mathcal{C}_{qq}^{(3)})^{srtv} - 2(\mathcal{C}_{qq}^{(3)})^{svtr} \right] (H^\dagger H) (\bar{q}_s \bar{\mathcal{B}} q_r) + \frac{2}{3} g_Y y_d^{vu} \bar{y}_d^{tu} \left[ (\mathcal{C}_{qq}^{(3)})^{svtr} - 6(\mathcal{C}_{qq}^{(3)})^{srtv} \right] (\bar{q}_s H \bar{\mathcal{B}} H^\dagger q_r) \\ & + \frac{2}{3} g_s^3 (\mathcal{C}_{qq}^{(3)})^{rsst} T_b^{Aa} T_a^{Bc} T_c^{Cd} G_\mu^A G_\mu^C (\bar{q}_{dr} \bar{\mathcal{G}}^B q_t^b) \\ & + \frac{2}{3} (\mathcal{C}_{qq}^{(3)})^{sttr} \left[ g_s^3 T_b^{Aa} T_c^{Bb} T_d^{Cc} G_\mu^B G_\mu^C (\bar{q}_{as} \bar{\mathcal{G}}^A q_r^d) + g_s^3 T_b^{Aa} T_a^{Bc} T_c^{Cd} G_\mu^B G_\mu^C (\bar{q}_{ds} \bar{\mathcal{G}}^A q_r^b) \right] \\ & + \frac{2}{3} g_L (\mathcal{C}_{qq}^{(3)})^{rsst} (\partial^2 \bar{q}_r t^I \bar{W}^I q_t) + g_L^2 g_s (\mathcal{C}_{qq}^{(3)})^{rsst} G_\mu^A W_\mu^I (\bar{q}_r T^A \bar{W}^I q_t) \\ & + \frac{4}{3} g_s g_Y (\mathcal{C}_{qq}^{(3)})^{rsst} G_\mu^A \tilde{B}^{\bar{\mu}\bar{\sigma}} (\bar{q}_r T^A \gamma^{\bar{\sigma}} q_t) + \frac{4}{3} g_s g_Y (\mathcal{C}_{qq}^{(3)})^{rsst} B_\mu \tilde{G}^{\bar{\mu}\bar{\sigma}A} (\bar{q}_r T^A \gamma^{\bar{\sigma}} q_t) \\ & + \frac{4}{3} g_L g_s^2 (\mathcal{C}_{qq}^{(3)})^{rstt} G_\mu^A W_\mu^I (\bar{q}_r t^I \bar{\mathcal{G}}^A q_s) + \frac{4}{3} g_L y_d^{us} \bar{y}_d^{rs} (\mathcal{C}_{qq}^{(3)})^{turv} (H^\dagger H) (\bar{q}_t t^I \bar{W}^I q_v) \\ & + \frac{4}{3} g_L y_u^{us} \bar{y}_u^{rs} (\mathcal{C}_{qq}^{(3)})^{turv} (H^\dagger H) (\bar{q}_t t^I \bar{W}^I q_v) + \frac{4}{3} g_L (\mathcal{C}_{qq}^{(3)})^{rsst} (\partial^{\bar{\nu}} \bar{q}_r t^I \bar{W}^I \partial^{\bar{\nu}} q_t) \\ & + \frac{5}{3} \left[ (\mathcal{C}_{qq}^{(3)})^{sttr} - 6(\mathcal{C}_{qq}^{(3)})^{srtt} \right] \left[ g_L^2 \varepsilon^{IJK} W_\nu^J (\bar{q}_s t^K \bar{W}^I \partial^{\bar{\nu}} q_r) + g_L^2 \varepsilon^{IJK} W_\nu^J (\partial^{\bar{\nu}} \bar{q}_s t^K \bar{W}^I q_r) \right] \\ & + 2g_L^2 (\mathcal{C}_{qq}^{(3)})^{sttr} W_\mu^I \tilde{W}^{\bar{\mu}\bar{\sigma}I} (\bar{q}_s \gamma^{\bar{\sigma}} q_r) + 2g_s y_d^{us} \bar{y}_d^{rs} (\mathcal{C}_{qq}^{(3)})^{turv} (\bar{q}_t T^A H \bar{\mathcal{G}}^A H^\dagger q_v) \\ & + 2g_s (\mathcal{C}_{qq}^{(3)})^{sttr} \left[ 2g_s T_b^{Aa} T_c^{Bb} G_\mu^B \tilde{G}^{\bar{\mu}\bar{\sigma}A} (\bar{q}_{as} \gamma^{\bar{\sigma}} q_r^c) + 2g_s T_b^{Aa} T_a^{Bc} G_\mu^B \tilde{G}^{\bar{\mu}\bar{\sigma}A} (\bar{q}_{cs} \gamma^{\bar{\sigma}} q_r^b) \right] \\ & + 3g_L^3 (\mathcal{C}_{qq}^{(3)})^{rstt} W_\mu^{I2} (\bar{q}_r t^I \bar{W}^I q_s) + 4g_L y_u^{us} \bar{y}_u^{rs} (\mathcal{C}_{qq}^{(3)})^{turv} (H^\dagger t^I H) (\bar{q}_t \bar{W}^I q_v) \\ & + 12g_L^2 (\mathcal{C}_{qq}^{(3)})^{rstt} \varepsilon^{IJK} W_\mu^J W^{\bar{\mu}\bar{\nu}I} (\bar{q}_r t^K \gamma^{\bar{\nu}} q_s) - \frac{1}{54} g_L g_Y^2 (\mathcal{C}_{qq}^{(3)})^{rsst} B_\mu^2 (\bar{q}_r t^I \bar{W}^I q_t) \end{aligned}$$

$$\begin{aligned}
& -\frac{1}{27}g_L g_Y^2 (\mathcal{C}_{qq}^{(3)})^{rsst} B_{\bar{\mu}} W_{\bar{\mu}}^I (\bar{q}_r t^I \bar{B}_{qt}) - \frac{1}{18}g_L^2 g_Y (\mathcal{C}_{qq}^{(3)})^{rsst} \varepsilon^{IJK} B_{\bar{\mu}} W_{\bar{\nu}}^I W_{\bar{\rho}}^J \varepsilon^{\bar{\mu}\bar{\nu}\bar{\rho}\bar{\sigma}} (\bar{q}_r t^K \gamma^{\bar{\sigma}} q_t) \\
& -\frac{2}{9}g_L g_Y (\mathcal{C}_{qq}^{(3)})^{rsst} B_{\bar{\mu}} \widetilde{W}^{\bar{\mu}\bar{\sigma}I} (\bar{q}_r t^I \gamma^{\bar{\sigma}} q_t) - \frac{2}{9}g_L g_s g_Y (\mathcal{C}_{qq}^{(3)})^{rsst} G_{\bar{\nu}}^A W_{\bar{\nu}}^I (\bar{q}_r t^I T^A \bar{B}_{qt}) \\
& -\frac{2}{9}g_L g_s g_Y (\mathcal{C}_{qq}^{(3)})^{rsst} B_{\bar{\mu}} W_{\bar{\mu}}^I (\bar{q}_r t^I T^A \bar{G}^A q_t) - \frac{2}{9}g_L g_s g_Y (\mathcal{C}_{qq}^{(3)})^{rsst} B_{\bar{\mu}} G_{\bar{\mu}}^A (\bar{q}_r t^I T^A \bar{W}^I q_t) \\
& -\frac{1}{4}g_L^3 (\mathcal{C}_{qq}^{(3)})^{rsst} \varepsilon^{IJK} W_{\bar{\mu}}^I W_{\bar{\nu}}^J W_{\bar{\rho}}^K \varepsilon^{\bar{\mu}\bar{\nu}\bar{\rho}\bar{\sigma}} (\bar{q}_r \gamma^{\bar{\sigma}} q_t) \\
& -\frac{1}{3}g_L^2 g_s (\mathcal{C}_{qq}^{(3)})^{rsst} \varepsilon^{IJK} G_{\bar{\mu}}^A W_{\bar{\nu}}^I W_{\bar{\rho}}^J \varepsilon^{\bar{\mu}\bar{\nu}\bar{\rho}\bar{\sigma}} (\bar{q}_r t^K T^A \gamma^{\bar{\sigma}} q_t) - \frac{1}{3}g_Y (\mathcal{C}_{qq}^{(3)})^{sttr} (\bar{q}_s \bar{B} \partial^2 q_r) \\
& -\frac{1}{3}g_Y (\mathcal{C}_{qq}^{(3)})^{sttr} (\partial^2 \bar{q}_s \bar{B} q_r) - \frac{1}{3}g_Y (\mathcal{C}_{qq}^{(3)})^{sttr} (\bar{q}_s \gamma^{\bar{\mu}} q_r) \partial^2 B_{\bar{\mu}} \\
& +\frac{i}{3}(\mathcal{C}_{qq}^{(3)})^{sttr} \left[ g_s^2 T_b^{Aa} T_c^{Bb} G_{\bar{\mu}}^B (\bar{q}_{as} \gamma^{\bar{\nu}} q_r^c) \partial^{\bar{\mu}} G_{\bar{\nu}}^A - g_s^2 T_b^{Aa} T_a^{Bc} G_{\bar{\mu}}^B (\bar{q}_{cs} \gamma^{\bar{\nu}} q_r^b) \partial^{\bar{\mu}} G_{\bar{\nu}}^A \right] \\
& +\frac{2}{3}g_L (\mathcal{C}_{qq}^{(3)})^{rsst} (\bar{q}_r t^I \gamma^{\bar{\mu}} q_t) \partial^2 W_{\bar{\mu}}^I - \frac{1}{2}g_L^3 (\mathcal{C}_{qq}^{(3)})^{rsst} W_{\bar{\mu}}^{I2} (\bar{q}_r t^I \bar{W}^I q_t) \\
& -\frac{2}{3}g_L g_Y (\mathcal{C}_{qq}^{(3)})^{rsst} W_{\bar{\mu}}^I \widetilde{B}^{\bar{\mu}\bar{\sigma}} (\bar{q}_r t^I \gamma^{\bar{\sigma}} q_t) - \frac{2}{3}g_L g_s^2 (\mathcal{C}_{qq}^{(3)})^{rsst} T_b^{Aa} T_a^{Bc} G_{\bar{\mu}}^A G_{\bar{\mu}}^B (\bar{q}_{cr} t^I \bar{W}^I q_t^b) \\
& -\frac{2}{3}(\mathcal{C}_{qq}^{(3)})^{sttr} \left[ g_L g_s^2 T_b^{Aa} T_c^{Bb} G_{\bar{\mu}}^B W_{\bar{\mu}}^I (\bar{q}_{as} t^I \bar{G}^A q_r^c) + g_L g_s^2 T_b^{Aa} T_a^{Bc} G_{\bar{\mu}}^B W_{\bar{\mu}}^I (\bar{q}_{cs} t^I \bar{G}^A q_r^b) \right] \\
& -\frac{2}{3}g_Y (\mathcal{C}_{qq}^{(3)})^{sttr} (\partial^{\bar{\nu}} \bar{q}_s \bar{B} \partial^{\bar{\nu}} q_r) \\
& -i(\mathcal{C}_{qq}^{(3)})^{sttr} \left[ g_s^2 T_b^{Aa} T_c^{Bb} (\bar{q}_{as} \bar{G}^B q_r^c) \partial^{\bar{\nu}} G_{\bar{\nu}}^A - g_s^2 T_b^{Aa} T_a^{Bc} (\bar{q}_{cs} \bar{G}^B q_r^b) \partial^{\bar{\nu}} G_{\bar{\nu}}^A \right] \\
& +2g_L^2 (\mathcal{C}_{qq}^{(3)})^{rstt} \varepsilon^{IJK} W_{\bar{\mu}}^J (\bar{q}_r t^K \gamma^{\bar{\nu}} q_s) \partial^{\bar{\mu}} W_{\bar{\nu}}^I - \frac{1}{3}g_L^2 (\mathcal{C}_{qq}^{(3)})^{rsst} \varepsilon^{IJK} W_{\bar{\mu}}^J (\bar{q}_r t^K \gamma^{\bar{\nu}} q_t) \partial^{\bar{\mu}} W_{\bar{\nu}}^I \\
& -\frac{4}{3}g_L g_s (\mathcal{C}_{qq}^{(3)})^{rsst} G_{\bar{\mu}}^A \widetilde{W}^{\bar{\mu}\bar{\sigma}I} (\bar{q}_r t^I T^A \gamma^{\bar{\sigma}} q_t) \\
& -\frac{4}{3}(\mathcal{C}_{qq}^{(3)})^{sttr} \left[ g_L g_s G_{\bar{\mu}}^A W_{\bar{\nu}}^I \varepsilon^{\bar{\mu}\bar{\nu}\bar{\rho}\bar{\sigma}} (\bar{q}_s t^I T^A \gamma^{\bar{\sigma}} \partial^{\bar{\rho}} q_r) + g_L g_s G_{\bar{\mu}}^A W_{\bar{\nu}}^I \varepsilon^{\bar{\mu}\bar{\nu}\bar{\rho}\bar{\sigma}} (\partial^{\bar{\rho}} \bar{q}_s t^I T^A \gamma^{\bar{\sigma}} q_r) \right] \\
& -\frac{4i}{3}(\mathcal{C}_{qq}^{(3)})^{sttr} \left[ g_s^2 T_b^{Aa} T_c^{Bb} G_{\bar{\mu}}^B (\bar{q}_{as} \gamma^{\bar{\nu}} q_r^c) \partial^{\bar{\nu}} G_{\bar{\mu}}^A - g_s^2 T_b^{Aa} T_a^{Bc} G_{\bar{\mu}}^B (\bar{q}_{cs} \gamma^{\bar{\nu}} q_r^b) \partial^{\bar{\nu}} G_{\bar{\mu}}^A \right] \\
& -2g_s (\mathcal{C}_{qq}^{(3)})^{rstt} (\bar{q}_r T^A \bar{G}^A \partial^2 q_t) - 2g_L g_Y (\mathcal{C}_{qq}^{(3)})^{rstt} W_{\bar{\mu}}^I \widetilde{B}^{\bar{\mu}\bar{\sigma}} (\bar{q}_r t^I \gamma^{\bar{\sigma}} q_s) - 2g_L^3 (\mathcal{C}_{qq}^{(3)})^{rstt} W_{\bar{\mu}}^I W_{\bar{\mu}}^J (\bar{q}_r t^I \bar{W}^J q_s) \\
& -2g_L^2 (\mathcal{C}_{qq}^{(3)})^{rsst} \varepsilon^{IJK} W_{\bar{\mu}}^J W_{\bar{\nu}}^I \varepsilon^{\bar{\mu}\bar{\nu}I} (\bar{q}_r t^K \gamma^{\bar{\nu}} q_t) - 2g_s y_u^{us} \bar{y}_u^{rs} (\mathcal{C}_{qq}^{(3)})^{turv} (H^\dagger H) (\bar{q}_t T^A \bar{G}^A q_v) \\
& -2g_s y_u^{us} \bar{y}_u^{rs} (\mathcal{C}_{qq}^{(3)})^{turv} (\bar{q}_t T^A H \bar{G}^A H^\dagger q_v) + 2ig_L g_s^2 (\mathcal{C}_{qq}^{(3)})^{rsst} T_b^{Aa} T_a^{Bc} G_{\bar{\mu}}^A G_{\bar{\nu}}^B W_{\bar{\rho}}^I \varepsilon^{\bar{\mu}\bar{\nu}\bar{\rho}\bar{\sigma}} (\bar{q}_{cr} t^I \gamma^{\bar{\sigma}} q_t^b) \\
& +2ig_s^3 (\mathcal{C}_{qq}^{(3)})^{rsst} T_b^{Aa} T_a^{Bc} T_c^{Cd} G_{\bar{\mu}}^A G_{\bar{\nu}}^C G_{\bar{\rho}}^B \varepsilon^{\bar{\mu}\bar{\nu}\bar{\rho}\bar{\sigma}} (\bar{q}_{dr} \gamma^{\bar{\sigma}} q_t^b) - 2g_s (\mathcal{C}_{qq}^{(3)})^{rsst} (\partial^2 \bar{q}_r T^A \bar{G}^A q_t) \\
& -2g_s (\mathcal{C}_{qq}^{(3)})^{rsst} (\bar{q}_r T^A \gamma^{\bar{\mu}} q_t) \partial^2 G_{\bar{\mu}}^A - 2g_L^2 (\mathcal{C}_{qq}^{(3)})^{rstt} \varepsilon^{IJK} (\bar{q}_r t^K \bar{W}^I q_s) \partial^{\bar{\nu}} W_{\bar{\nu}}^J \\
& -\frac{10}{3}g_L g_Y (\mathcal{C}_{qq}^{(3)})^{rstt} B_{\bar{\mu}} \widetilde{W}^{\bar{\mu}\bar{\sigma}I} (\bar{q}_r t^I \gamma^{\bar{\sigma}} q_s) - 4g_L (\mathcal{C}_{qq}^{(3)})^{rstt} (\bar{q}_r t^I \bar{W}^I \partial^2 q_s) \\
& -4g_L g_s (\mathcal{C}_{qq}^{(3)})^{rsst} W_{\bar{\mu}}^I \widetilde{G}^{\bar{\mu}\bar{\sigma}A} (\bar{q}_r t^I T^A \gamma^{\bar{\sigma}} q_t) - 4g_L y_d^{us} \bar{y}_d^{rs} (\mathcal{C}_{qq}^{(3)})^{turv} (H^\dagger t^I H) (\bar{q}_t \bar{W}^I q_v) \\
& -4g_s y_d^{us} \bar{y}_d^{rs} (\mathcal{C}_{qq}^{(3)})^{turv} (H^\dagger H) (\bar{q}_t T^A \bar{G}^A q_v) - 4g_L (\mathcal{C}_{qq}^{(3)})^{rstt} (\partial^2 \bar{q}_r t^I \bar{W}^I q_s) - 4g_s (\mathcal{C}_{qq}^{(3)})^{rsst} (\partial^{\bar{\nu}} \bar{q}_r T^A \bar{G}^A \partial^{\bar{\nu}} q_t) \\
& -4g_L (\mathcal{C}_{qq}^{(3)})^{rstt} (\bar{q}_r t^I \gamma^{\bar{\mu}} q_s) \partial^2 W_{\bar{\mu}}^I
\end{aligned}$$

$$\begin{aligned}
& -5i(C_{qq}^{(3)})^{sttr} \left[ g_s^2 T_b^{Aa} T_a^{Bc} G_\nu^B (\bar{q}_{cs} \bar{G}^A \partial^\nu q_r^b) - g_s^2 T_b^{Aa} T_c^{Bb} G_\nu^B (\partial^\nu \bar{q}_{as} \bar{G}^A q_r^c) \right] \\
& -5i(C_{qq}^{(3)})^{sttr} \left[ g_s^2 T_b^{Aa} T_c^{Bb} G_\nu^A (\partial^\nu \bar{q}_{as} \bar{G}^B q_r^c) - g_s^2 T_b^{Aa} T_a^{Bc} G_\nu^A (\bar{q}_{cs} \bar{G}^B \partial^\nu q_r^b) \right] \\
& -\frac{22i}{3} g_s (C_{qq}^{(3)})^{sttr} \left[ g_s T_b^{Aa} T_c^{Bb} G_\mu^B G^{\mu\nu A} (\bar{q}_{as} \gamma^\nu q_r^c) - g_s T_b^{Aa} T_a^{Bc} G_\mu^B G^{\mu\nu A} (\bar{q}_{cs} \gamma^\nu q_r^b) \right] \\
& -8g_L y_d^{vs} \bar{y}_d^{rs} (C_{qq}^{(3)})^{turv} (H^\dagger H) (\bar{q}_t t^I \bar{W}^I q_u) - 8g_L y_u^{vs} \bar{y}_u^{rs} (C_{qq}^{(3)})^{turv} (H^\dagger H) (\bar{q}_t t^I \bar{W}^I q_u) \\
& -8g_L (C_{qq}^{(3)})^{rstt} (\partial^\nu \bar{q}_r t^I \bar{W}^I \partial^\nu q_s), \tag{2.43}
\end{aligned}$$

$$\begin{aligned}
\Delta S_{\mathcal{O}_{eu}} &= \frac{1}{12} g_s^3 C_{eu}^{srtt} d^{ABC} G_\nu^B G_\nu^C (\bar{e}_s \bar{G}^A e_r) + \frac{1}{9} g_s^2 g_Y C_{eu}^{srtt} G_\mu^{A2} (\bar{e}_s \bar{B} e_r) + \frac{2}{9} g_s^2 g_Y C_{eu}^{srtt} B_\mu G_\mu^A (\bar{e}_s \bar{G}^A e_r) \\
&+ \frac{8}{27} g_Y^3 C_{eu}^{srtt} B_\mu^2 (\bar{e}_s \bar{B} e_r) + \frac{1}{3} g_Y C_{eu}^{ttsr} (\bar{u}_s \bar{B} \partial^2 u_r) + \frac{1}{3} g_L y_e^{tv} \bar{y}_e^{tu} C_{eu}^{vusr} (H^\dagger t^I H) (\bar{u}_s \bar{W}^I u_r) \\
&+ \frac{1}{3} g_Y C_{eu}^{ttsr} (\partial^2 \bar{u}_s \bar{B} u_r) + \frac{1}{3} g_Y C_{eu}^{ttsr} (\bar{u}_s \gamma^\mu u_r) \partial^2 B_\mu + \frac{2}{3} g_s^2 C_{eu}^{srtt} G_\mu^A \tilde{G}^{\mu\bar{\sigma} A} (\bar{e}_s \gamma^\sigma e_r) \\
&+ \frac{2}{3} g_Y C_{eu}^{ttsr} (\partial^\nu \bar{u}_s \bar{B} \partial^\nu u_r) + \frac{7}{6} g_Y y_e^{tv} \bar{y}_e^{tu} C_{eu}^{vusr} (H^\dagger H) (\bar{u}_s \bar{B} u_r) + \frac{4}{3} g_Y^2 C_{eu}^{ttsr} B_\mu \tilde{B}^{\mu\bar{\sigma}} (\bar{u}_s \gamma^\sigma u_r) \\
&+ \frac{16}{9} g_Y^2 C_{eu}^{srtt} B_\mu \tilde{B}^{\mu\bar{\sigma}} (\bar{e}_s \gamma^\sigma e_r) - \frac{1}{12} g_s^3 C_{eu}^{srtt} f^{ABC} G_\mu^A G_\nu^B G_\rho^C \varepsilon^{\mu\nu\rho\bar{\sigma}} (\bar{e}_s \gamma^\sigma e_r) \\
&- \frac{1}{3} g_Y^3 C_{eu}^{ttsr} B_\mu^2 (\bar{u}_s \bar{B} u_r) - \frac{2}{3} g_Y C_{eu}^{srtt} (\bar{e}_s \bar{B} \partial^2 e_r) - \frac{2}{3} g_Y C_{eu}^{srtt} (\partial^2 \bar{e}_s \bar{B} e_r) \\
&- \frac{2}{3} g_Y C_{eu}^{srtt} (\bar{e}_s \gamma^\mu e_r) \partial^2 B_\mu - g_L y_u^{tv} \bar{y}_u^{tu} C_{eu}^{srvu} (H^\dagger t^I H) (\bar{e}_s \bar{W}^I e_r) - \frac{4}{3} g_Y C_{eu}^{srtt} (\partial^\nu \bar{e}_s \bar{B} \partial^\nu e_r) \\
&- \frac{5}{2} g_Y y_u^{tv} \bar{y}_u^{tu} C_{eu}^{srvu} (H^\dagger H) (\bar{e}_s \bar{B} e_r), \tag{2.44}
\end{aligned}$$

$$\begin{aligned}
\Delta S_{\mathcal{O}_{ed}} &= \frac{1}{12} g_s^3 C_{ed}^{srtt} d^{ABC} G_\nu^B G_\nu^C (\bar{e}_s \bar{G}^A e_r) + \frac{1}{3} g_Y C_{ed}^{ttsr} (\bar{d}_s \bar{B} \partial^2 d_r) + \frac{1}{3} g_L y_e^{tv} \bar{y}_e^{tu} C_{ed}^{vusr} (H^\dagger t^I H) (\bar{d}_s \bar{W}^I d_r) \\
&+ \frac{1}{3} g_Y C_{ed}^{srtt} (\bar{e}_s \bar{B} \partial^2 e_r) + \frac{1}{3} g_Y C_{ed}^{ttsr} (\partial^2 \bar{d}_s \bar{B} d_r) + \frac{1}{3} g_Y C_{ed}^{srtt} (\partial^2 \bar{e}_s \bar{B} e_r) \\
&+ \frac{1}{3} g_Y C_{ed}^{ttsr} (\bar{d}_s \gamma^\mu d_r) \partial^2 B_\mu + \frac{1}{3} g_Y C_{ed}^{srtt} (\bar{e}_s \gamma^\mu e_r) \partial^2 B_\mu + \frac{4}{9} g_Y^2 C_{ed}^{srtt} B_\mu \tilde{B}^{\mu\bar{\sigma}} (\bar{e}_s \gamma^\sigma e_r) \\
&+ \frac{2}{3} g_s^2 C_{ed}^{srtt} G_\mu^A \tilde{G}^{\mu\bar{\sigma} A} (\bar{e}_s \gamma^\sigma e_r) + \frac{2}{3} g_Y C_{ed}^{ttsr} (\partial^\nu \bar{d}_s \bar{B} \partial^\nu d_r) \\
&+ \frac{2}{3} g_Y C_{ed}^{srtt} (\partial^\nu \bar{e}_s \bar{B} \partial^\nu e_r) + g_L y_d^{tv} \bar{y}_d^{tu} C_{ed}^{srvu} (H^\dagger t^I H) (\bar{e}_s \bar{W}^I e_r) + \frac{7}{6} g_Y y_e^{tv} \bar{y}_e^{tu} C_{ed}^{vusr} (H^\dagger H) (\bar{d}_s \bar{B} d_r) \\
&+ \frac{4}{3} g_Y^2 C_{ed}^{ttsr} B_\mu \tilde{B}^{\mu\bar{\sigma}} (\bar{d}_s \gamma^\sigma d_r) + \frac{3}{2} g_Y y_d^{tv} \bar{y}_d^{tu} C_{ed}^{srvu} (H^\dagger H) (\bar{e}_s \bar{B} e_r) - \frac{1}{27} g_Y^3 C_{ed}^{srtt} B_\mu^2 (\bar{e}_s \bar{B} e_r) \\
&- \frac{1}{18} g_s^2 g_Y C_{ed}^{srtt} G_\mu^{A2} (\bar{e}_s \bar{B} e_r) - \frac{1}{12} g_s^3 C_{ed}^{srtt} f^{ABC} G_\mu^A G_\nu^B G_\rho^C \varepsilon^{\mu\nu\rho\bar{\sigma}} (\bar{e}_s \gamma^\sigma e_r) \\
&- \frac{1}{9} g_s^2 g_Y C_{ed}^{srtt} B_\mu G_\mu^A (\bar{e}_s \bar{G}^A e_r) - \frac{1}{3} g_Y^3 C_{ed}^{ttsr} B_\mu^2 (\bar{d}_s \bar{B} d_r), \tag{2.45}
\end{aligned}$$

$$\begin{aligned}
\Delta S_{\mathcal{O}_{qe}} &= \frac{1}{108} g_Y^3 C_{qe}^{ttsr} B_\mu^2 (\bar{e}_s \bar{B} e_r) + \frac{1}{18} g_s^2 g_Y C_{qe}^{ttsr} G_\mu^{A2} (\bar{e}_s \bar{B} e_r) + \frac{1}{12} g_L^2 g_Y C_{qe}^{ttsr} W_\mu^{I2} (\bar{e}_s \bar{B} e_r) \\
&+ \frac{1}{9} g_s^2 g_Y C_{qe}^{ttsr} B_\mu G_\mu^A (\bar{e}_s \bar{G}^A e_r) + \frac{1}{6} g_s^3 C_{qe}^{ttsr} f^{ABC} G_\mu^A G_\nu^B G_\rho^C \varepsilon^{\mu\nu\rho\bar{\sigma}} (\bar{e}_s \gamma^\sigma e_r)
\end{aligned}$$

$$\begin{aligned}
& + \frac{1}{6} g_s^3 \mathcal{C}_{qe}^{ttsr} d^{ABC} G_{\bar{\nu}}^B G_{\bar{\nu}}^C (\bar{e}_s \bar{G}^A e_r) + \frac{1}{6} g_L^2 g_Y \mathcal{C}_{qe}^{ttsr} B_{\bar{\mu}} W_{\bar{\mu}}^I (\bar{e}_s \bar{W}^I e_r) \\
& + \frac{1}{4} g_L^3 \mathcal{C}_{qe}^{ttsr} \varepsilon^{IJK} W_{\bar{\mu}}^I W_{\bar{\nu}}^J W_{\bar{\rho}}^K \varepsilon^{\bar{\mu}\bar{\nu}\bar{\rho}\bar{\sigma}} (\bar{e}_s \gamma^{\bar{\sigma}} e_r) + \frac{1}{3} g_Y \mathcal{C}_{qe}^{srtt} (\bar{q}_s \bar{B} \partial^2 q_r) \\
& + \frac{1}{3} g_L y_e^{tv} \bar{y}_e^{tu} \mathcal{C}_{qe}^{srvu} (H^\dagger t^I H) (\bar{q}_s \bar{W}^I q_r) + \frac{1}{3} g_Y \mathcal{C}_{qe}^{srtt} (\partial^2 \bar{q}_s \bar{B} q_r) + \frac{1}{3} g_Y \mathcal{C}_{qe}^{srtt} (\bar{q}_s \gamma^{\bar{\mu}} q_r) \partial^2 B_{\bar{\mu}} \\
& + \frac{2}{3} g_Y \mathcal{C}_{qe}^{srtt} (\partial^{\bar{\nu}} \bar{q}_s \bar{B} \partial^{\bar{\nu}} q_r) + \frac{7}{6} g_Y y_e^{tv} \bar{y}_e^{tu} \mathcal{C}_{qe}^{srvu} (H^\dagger H) (\bar{q}_s \bar{B} q_r) + \frac{4}{3} g_Y^2 \mathcal{C}_{qe}^{srtt} B_{\bar{\mu}} \tilde{B}^{\bar{\mu}\bar{\sigma}} (\bar{q}_s \gamma^{\bar{\sigma}} q_r) \\
& + 4 g_L \mathcal{C}_{qe}^{tvsr} \left[ y_u^{vu} \bar{y}_u^{tu} - y_d^{vu} \bar{y}_d^{tu} \right] (H^\dagger t^I H) (\bar{e}_s \bar{W}^I e_r) - \frac{2}{9} g_Y^2 \mathcal{C}_{qe}^{ttsr} B_{\bar{\mu}} \tilde{B}^{\bar{\mu}\bar{\sigma}} (\bar{e}_s \gamma^{\bar{\sigma}} e_r) \\
& - \frac{1}{3} g_Y \mathcal{C}_{qe}^{ttsr} (\bar{e}_s \bar{B} \partial^2 e_r) - \frac{1}{3} g_Y^3 \mathcal{C}_{qe}^{srtt} B_{\bar{\mu}}^2 (\bar{q}_s \bar{B} q_r) - \frac{1}{3} g_Y \mathcal{C}_{qe}^{ttsr} (\partial^2 \bar{e}_s \bar{B} e_r) \\
& - \frac{1}{3} g_Y \mathcal{C}_{qe}^{ttsr} (\bar{e}_s \gamma^{\bar{\mu}} e_r) \partial^2 B_{\bar{\mu}} - \frac{2}{3} g_Y \mathcal{C}_{qe}^{ttsr} (\partial^{\bar{\nu}} \bar{e}_s \bar{B} \partial^{\bar{\nu}} e_r) - g_Y y_d^{vu} \bar{y}_d^{tu} \mathcal{C}_{qe}^{tvsr} (H^\dagger H) (\bar{e}_s \bar{B} e_r) \\
& - \frac{4}{3} g_s^2 \mathcal{C}_{qe}^{ttsr} G_{\bar{\mu}}^A \tilde{G}^{\bar{\mu}\bar{\sigma} A} (\bar{e}_s \gamma^{\bar{\sigma}} e_r) - 2 g_L^2 \mathcal{C}_{qe}^{ttsr} W_{\bar{\mu}}^I \tilde{W}^{\bar{\mu}\bar{\sigma} I} (\bar{e}_s \gamma^{\bar{\sigma}} e_r), \tag{2.46}
\end{aligned}$$

$$\begin{aligned}
\Delta S_{\mathcal{O}_{\ell u}} &= \frac{1}{12} g_s^3 \mathcal{C}_{\ell u}^{srtt} d^{ABC} G_{\bar{\nu}}^B G_{\bar{\nu}}^C (\bar{\ell}_s \bar{G}^A \ell_r) + \frac{1}{12} g_L^3 \mathcal{C}_{\ell u}^{ttsr} \varepsilon^{IJK} W_{\bar{\mu}}^I W_{\bar{\nu}}^J W_{\bar{\rho}}^K \varepsilon^{\bar{\mu}\bar{\nu}\bar{\rho}\bar{\sigma}} (\bar{u}_s \gamma^{\bar{\sigma}} u_r) \\
& + \frac{1}{9} g_s^2 g_Y \mathcal{C}_{\ell u}^{srtt} G_{\bar{\mu}}^A{}^2 (\bar{\ell}_s \bar{B} \ell_r) + \frac{2}{9} g_s^2 g_Y \mathcal{C}_{\ell u}^{srtt} B_{\bar{\mu}} G_{\bar{\mu}}^A (\bar{\ell}_s \bar{G}^A \ell_r) + \frac{8}{27} g_Y^3 \mathcal{C}_{\ell u}^{srtt} B_{\bar{\mu}}^2 (\bar{\ell}_s \bar{B} \ell_r) \\
& + \frac{1}{3} g_Y y_e^{vu} \bar{y}_e^{tu} \mathcal{C}_{\ell u}^{tvsr} (H^\dagger H) (\bar{u}_s \bar{B} u_r) + \frac{1}{3} g_Y \mathcal{C}_{\ell u}^{ttsr} (\bar{u}_s \bar{B} \partial^2 u_r) + \frac{1}{3} g_Y \mathcal{C}_{\ell u}^{ttsr} (\partial^2 \bar{u}_s \bar{B} u_r) \\
& + \frac{1}{3} g_Y \mathcal{C}_{\ell u}^{ttsr} (\bar{u}_s \gamma^{\bar{\mu}} u_r) \partial^2 B_{\bar{\mu}} + \frac{2}{3} g_s^2 \mathcal{C}_{\ell u}^{srtt} G_{\bar{\mu}}^A \tilde{G}^{\bar{\mu}\bar{\sigma} A} (\bar{\ell}_s \gamma^{\bar{\sigma}} \ell_r) \\
& + \frac{2}{3} g_Y \mathcal{C}_{\ell u}^{ttsr} (\partial^{\bar{\nu}} \bar{u}_s \bar{B} \partial^{\bar{\nu}} u_r) + \frac{16}{9} g_Y^2 \mathcal{C}_{\ell u}^{srtt} B_{\bar{\mu}} \tilde{B}^{\bar{\mu}\bar{\sigma}} (\bar{\ell}_s \gamma^{\bar{\sigma}} \ell_r) \\
& - \frac{1}{12} g_s^3 \mathcal{C}_{\ell u}^{srtt} f^{ABC} G_{\bar{\mu}}^A G_{\bar{\nu}}^B G_{\bar{\rho}}^C \varepsilon^{\bar{\mu}\bar{\nu}\bar{\rho}\bar{\sigma}} (\bar{\ell}_s \gamma^{\bar{\sigma}} \ell_r) - \frac{1}{12} g_Y^3 \mathcal{C}_{\ell u}^{ttsr} B_{\bar{\mu}}^2 (\bar{u}_s \bar{B} u_r) \\
& - \frac{1}{12} g_L^2 g_Y \mathcal{C}_{\ell u}^{ttsr} W_{\bar{\mu}}^I{}^2 (\bar{u}_s \bar{B} u_r) - \frac{1}{6} g_L^2 g_Y \mathcal{C}_{\ell u}^{ttsr} B_{\bar{\mu}} W_{\bar{\mu}}^I (\bar{u}_s \bar{W}^I u_r) - \frac{2}{3} g_Y \mathcal{C}_{\ell u}^{srtt} (\bar{\ell}_s \bar{B} \partial^2 \ell_r) \\
& - \frac{2}{3} g_Y^2 \mathcal{C}_{\ell u}^{ttsr} B_{\bar{\mu}} \tilde{B}^{\bar{\mu}\bar{\sigma}} (\bar{u}_s \gamma^{\bar{\sigma}} u_r) - \frac{2}{3} g_L^2 \mathcal{C}_{\ell u}^{ttsr} W_{\bar{\mu}}^I \tilde{W}^{\bar{\mu}\bar{\sigma} I} (\bar{u}_s \gamma^{\bar{\sigma}} u_r) \\
& - \frac{2}{3} g_Y \mathcal{C}_{\ell u}^{srtt} (\partial^2 \bar{\ell}_s \bar{B} \ell_r) - \frac{2}{3} g_Y \mathcal{C}_{\ell u}^{srtt} (\bar{\ell}_s \gamma^{\bar{\mu}} \ell_r) \partial^2 B_{\bar{\mu}} - g_L y_u^{tv} \bar{y}_u^{tu} \mathcal{C}_{\ell u}^{srvu} (H^\dagger t^I H) (\bar{\ell}_s \bar{W}^I \ell_r) \\
& - \frac{4}{3} g_L y_e^{vu} \bar{y}_e^{tu} \mathcal{C}_{\ell u}^{tvsr} (H^\dagger t^I H) (\bar{u}_s \bar{W}^I u_r) - \frac{4}{3} g_Y \mathcal{C}_{\ell u}^{srtt} (\partial^{\bar{\nu}} \bar{\ell}_s \bar{B} \partial^{\bar{\nu}} \ell_r) \\
& - \frac{5}{2} g_Y y_u^{tv} \bar{y}_u^{tu} \mathcal{C}_{\ell u}^{srvu} (H^\dagger H) (\bar{\ell}_s \bar{B} \ell_r), \tag{2.47}
\end{aligned}$$

$$\begin{aligned}
\Delta S_{\mathcal{O}_{\ell d}} &= \frac{1}{12} g_L^3 \mathcal{C}_{\ell d}^{ttsr} \varepsilon^{IJK} W_{\bar{\mu}}^I W_{\bar{\nu}}^J W_{\bar{\rho}}^K \varepsilon^{\bar{\mu}\bar{\nu}\bar{\rho}\bar{\sigma}} (\bar{d}_s \gamma^{\bar{\sigma}} d_r) + \frac{1}{12} g_s^3 \mathcal{C}_{\ell d}^{srtt} d^{ABC} G_{\bar{\nu}}^B G_{\bar{\nu}}^C (\bar{\ell}_s \bar{G}^A \ell_r) \\
& + \frac{1}{3} g_Y y_e^{vu} \bar{y}_e^{tu} \mathcal{C}_{\ell d}^{tvsr} (H^\dagger H) (\bar{d}_s \bar{B} d_r) + \frac{1}{3} g_Y \mathcal{C}_{\ell d}^{ttsr} (\bar{d}_s \bar{B} \partial^2 d_r) + \frac{1}{3} g_Y \mathcal{C}_{\ell d}^{srtt} (\bar{\ell}_s \bar{B} \partial^2 \ell_r) \\
& + \frac{1}{3} g_Y \mathcal{C}_{\ell d}^{ttsr} (\partial^2 \bar{d}_s \bar{B} d_r) + \frac{1}{3} g_Y \mathcal{C}_{\ell d}^{srtt} (\partial^2 \bar{\ell}_s \bar{B} \ell_r) + \frac{1}{3} g_Y \mathcal{C}_{\ell d}^{ttsr} (\bar{d}_s \gamma^{\bar{\mu}} d_r) \partial^2 B_{\bar{\mu}} \\
& + \frac{1}{3} g_Y \mathcal{C}_{\ell d}^{srtt} (\bar{\ell}_s \gamma^{\bar{\mu}} \ell_r) \partial^2 B_{\bar{\mu}} + \frac{4}{9} g_Y^2 \mathcal{C}_{\ell d}^{srtt} B_{\bar{\mu}} \tilde{B}^{\bar{\mu}\bar{\sigma}} (\bar{\ell}_s \gamma^{\bar{\sigma}} \ell_r)
\end{aligned}$$

$$\begin{aligned}
& + \frac{2}{3} g_s^2 \mathcal{C}_{\ell d}^{srtt} G_{\bar{\mu}}^A \tilde{G}^{\bar{\mu}\bar{\sigma} A} (\bar{\ell}_s \gamma^{\bar{\sigma}} \ell_r) + \frac{2}{3} g_Y \mathcal{C}_{\ell d}^{ttsr} (\partial^{\bar{\nu}} \bar{d}_s \bar{\mathcal{B}} \partial^{\bar{\nu}} d_r) \\
& + \frac{2}{3} g_Y \mathcal{C}_{\ell d}^{srtt} (\partial^{\bar{\nu}} \bar{\ell}_s \bar{\mathcal{B}} \partial^{\bar{\nu}} \ell_r) + g_L y_d^{tv} \bar{y}_d^{tu} \mathcal{C}_{\ell d}^{srvu} (H^\dagger t^I H) (\bar{\ell}_s \bar{W}^I \ell_r) \\
& + \frac{3}{2} g_Y y_d^{tv} \bar{y}_d^{tu} \mathcal{C}_{\ell d}^{srvu} (H^\dagger H) (\bar{\ell}_s \bar{\mathcal{B}} \ell_r) - \frac{1}{27} g_Y^3 \mathcal{C}_{\ell d}^{srtt} B_{\bar{\mu}}^2 (\bar{\ell}_s \bar{\mathcal{B}} \ell_r) - \frac{1}{18} g_s^2 g_Y \mathcal{C}_{\ell d}^{srtt} G_{\bar{\mu}}^{A2} (\bar{\ell}_s \bar{\mathcal{B}} \ell_r) \\
& - \frac{1}{12} g_Y^3 \mathcal{C}_{\ell d}^{ttsr} B_{\bar{\mu}}^2 (\bar{d}_s \bar{\mathcal{B}} d_r) - \frac{1}{12} g_L^2 g_Y \mathcal{C}_{\ell d}^{ttsr} W_{\bar{\mu}}^{I2} (\bar{d}_s \bar{\mathcal{B}} d_r) \\
& - \frac{1}{12} g_s^3 \mathcal{C}_{\ell d}^{srtt} f^{ABC} G_{\bar{\mu}}^A G_{\bar{\nu}}^B G_{\bar{\rho}}^C \varepsilon^{\bar{\mu}\bar{\nu}\bar{\rho}\bar{\sigma}} (\bar{\ell}_s \gamma^{\bar{\sigma}} \ell_r) - \frac{1}{9} g_s^2 g_Y \mathcal{C}_{\ell d}^{srtt} B_{\bar{\mu}} G_{\bar{\mu}}^A (\bar{\ell}_s \bar{\mathcal{G}}^A \ell_r) \\
& - \frac{1}{6} g_L^2 g_Y \mathcal{C}_{\ell d}^{ttsr} B_{\bar{\mu}} W_{\bar{\mu}}^I (\bar{d}_s \bar{W}^I d_r) - \frac{2}{3} g_Y^2 \mathcal{C}_{\ell d}^{ttsr} B_{\bar{\mu}} \tilde{B}^{\bar{\mu}\bar{\sigma}} (\bar{d}_s \gamma^{\bar{\sigma}} d_r) \\
& - \frac{2}{3} g_L^2 \mathcal{C}_{\ell d}^{ttsr} W_{\bar{\mu}}^I \tilde{W}^{\bar{\mu}\bar{\sigma} I} (\bar{d}_s \gamma^{\bar{\sigma}} d_r) - \frac{4}{3} g_L y_e^{vu} \bar{y}_e^{tu} \mathcal{C}_{\ell d}^{tvsr} (H^\dagger t^I H) (\bar{d}_s \bar{W}^I d_r), \tag{2.48}
\end{aligned}$$

$$\begin{aligned}
\Delta S_{\mathcal{O}_{\ell q}^{(1)}} &= \frac{1}{108} g_Y^3 (\mathcal{C}_{\ell q}^{(1)})^{srtt} B_{\bar{\mu}}^2 (\bar{\ell}_s \bar{\mathcal{B}} \ell_r) + \frac{1}{18} g_s^2 g_Y (\mathcal{C}_{\ell q}^{(1)})^{srtt} G_{\bar{\mu}}^{A2} (\bar{\ell}_s \bar{\mathcal{B}} \ell_r) + \frac{1}{12} g_L^2 g_Y (\mathcal{C}_{\ell q}^{(1)})^{srtt} W_{\bar{\mu}}^{I2} (\bar{\ell}_s \bar{\mathcal{B}} \ell_r) \\
& + \frac{1}{12} g_L^3 (\mathcal{C}_{\ell q}^{(1)})^{ttsr} \varepsilon^{IJK} W_{\bar{\mu}}^I W_{\bar{\nu}}^J W_{\bar{\rho}}^K \varepsilon^{\bar{\mu}\bar{\nu}\bar{\rho}\bar{\sigma}} (\bar{q}_s \gamma^{\bar{\sigma}} q_r) + \frac{1}{9} g_s^2 g_Y (\mathcal{C}_{\ell q}^{(1)})^{srtt} B_{\bar{\mu}} G_{\bar{\mu}}^A (\bar{\ell}_s \bar{\mathcal{G}}^A \ell_r) \\
& + \frac{1}{6} g_s^3 (\mathcal{C}_{\ell q}^{(1)})^{srtt} f^{ABC} G_{\bar{\mu}}^A G_{\bar{\nu}}^B G_{\bar{\rho}}^C \varepsilon^{\bar{\mu}\bar{\nu}\bar{\rho}\bar{\sigma}} (\bar{\ell}_s \gamma^{\bar{\sigma}} \ell_r) + \frac{1}{6} g_s^3 (\mathcal{C}_{\ell q}^{(1)})^{srtt} d^{ABC} G_{\bar{\nu}}^B G_{\bar{\rho}}^C (\bar{\ell}_s \bar{\mathcal{G}}^A \ell_r) \\
& + \frac{1}{6} g_L^2 g_Y (\mathcal{C}_{\ell q}^{(1)})^{srtt} B_{\bar{\mu}} W_{\bar{\mu}}^I (\bar{\ell}_s \bar{W}^I \ell_r) + \frac{1}{6} g_L^2 g_Y (\mathcal{C}_{\ell q}^{(1)})^{ttsr} \varepsilon^{IJK} B_{\bar{\mu}} W_{\bar{\nu}}^I W_{\bar{\rho}}^J \varepsilon^{\bar{\mu}\bar{\nu}\bar{\rho}\bar{\sigma}} (\bar{q}_s t^K \gamma^{\bar{\sigma}} q_r) \\
& + \frac{1}{3} g_L g_Y (\mathcal{C}_{\ell q}^{(1)})^{srtt} B_{\bar{\mu}} \tilde{W}^{\bar{\mu}\bar{\sigma} I} (\bar{\ell}_s t^I \gamma^{\bar{\sigma}} \ell_r) + \frac{1}{3} g_Y y_e^{vu} \bar{y}_e^{tu} (\mathcal{C}_{\ell q}^{(1)})^{tvsr} (H^\dagger H) (\bar{q}_s \bar{\mathcal{B}} q_r) \\
& + \frac{1}{3} g_Y (\mathcal{C}_{\ell q}^{(1)})^{ttsr} (\bar{q}_s \bar{\mathcal{B}} \partial^2 q_r) + \frac{1}{3} g_L g_Y (\mathcal{C}_{\ell q}^{(1)})^{ttsr} W_{\bar{\mu}}^I \tilde{B}^{\bar{\mu}\bar{\sigma}} (\bar{q}_s t^I \gamma^{\bar{\sigma}} q_r) + \frac{1}{3} g_Y (\mathcal{C}_{\ell q}^{(1)})^{ttsr} (\partial^2 \bar{q}_s \bar{\mathcal{B}} q_r) \\
& + \frac{1}{3} (\mathcal{C}_{\ell q}^{(1)})^{rstt} \left[ g_L g_Y B_{\bar{\mu}} W_{\bar{\nu}}^I \varepsilon^{\bar{\mu}\bar{\nu}\bar{\rho}\bar{\sigma}} (\bar{\ell}_r t^I \gamma^{\bar{\rho}} \partial^{\bar{\sigma}} \ell_s) + g_L g_Y B_{\bar{\mu}} W_{\bar{\nu}}^I \varepsilon^{\bar{\mu}\bar{\nu}\bar{\rho}\bar{\sigma}} (\partial^{\bar{\sigma}} \bar{\ell}_r t^I \gamma^{\bar{\rho}} \ell_s) \right] \\
& + \frac{1}{3} g_Y (\mathcal{C}_{\ell q}^{(1)})^{ttsr} (\bar{q}_s \gamma^{\bar{\mu}} q_r) \partial^2 B_{\bar{\mu}} + \frac{2}{3} g_Y (\mathcal{C}_{\ell q}^{(1)})^{ttsr} (\partial^{\bar{\nu}} \bar{q}_s \bar{\mathcal{B}} \partial^{\bar{\nu}} q_r) \\
& + 4 g_L (\mathcal{C}_{\ell q}^{(1)})^{srtv} \left[ y_u^{vu} \bar{y}_u^{tu} - y_d^{vu} \bar{y}_d^{tu} \right] (H^\dagger t^I H) (\bar{\ell}_s \bar{W}^I \ell_r) - \frac{1}{12} g_Y^3 (\mathcal{C}_{\ell q}^{(1)})^{ttsr} B_{\bar{\mu}}^2 (\bar{q}_s \bar{\mathcal{B}} q_r) \\
& - \frac{1}{12} g_L^2 g_Y (\mathcal{C}_{\ell q}^{(1)})^{ttsr} W_{\bar{\mu}}^{I2} (\bar{q}_s \bar{\mathcal{B}} q_r) - \frac{1}{6} g_L^2 g_Y (\mathcal{C}_{\ell q}^{(1)})^{srtt} \varepsilon^{IJK} B_{\bar{\mu}} W_{\bar{\nu}}^I W_{\bar{\rho}}^J \varepsilon^{\bar{\mu}\bar{\nu}\bar{\rho}\bar{\sigma}} (\bar{\ell}_s t^K \gamma^{\bar{\sigma}} \ell_r) \\
& - \frac{1}{6} g_L^2 g_Y (\mathcal{C}_{\ell q}^{(1)})^{ttsr} B_{\bar{\mu}} W_{\bar{\mu}}^I (\bar{q}_s \bar{W}^I q_r) - \frac{2}{9} g_Y^2 (\mathcal{C}_{\ell q}^{(1)})^{srtt} B_{\bar{\mu}} \tilde{B}^{\bar{\mu}\bar{\sigma}} (\bar{\ell}_s \gamma^{\bar{\sigma}} \ell_r) \\
& - \frac{1}{4} g_L^3 (\mathcal{C}_{\ell q}^{(1)})^{srtt} \varepsilon^{IJK} W_{\bar{\mu}}^I W_{\bar{\nu}}^J W_{\bar{\rho}}^K \varepsilon^{\bar{\mu}\bar{\nu}\bar{\rho}\bar{\sigma}} (\bar{\ell}_s \gamma^{\bar{\sigma}} \ell_r) - \frac{1}{3} g_Y (\mathcal{C}_{\ell q}^{(1)})^{srtt} (\bar{\ell}_s \bar{\mathcal{B}} \partial^2 \ell_r) \\
& - \frac{1}{3} g_L g_Y (\mathcal{C}_{\ell q}^{(1)})^{srtt} W_{\bar{\mu}}^I \tilde{B}^{\bar{\mu}\bar{\sigma}} (\bar{\ell}_s t^I \gamma^{\bar{\sigma}} \ell_r) - \frac{1}{3} g_L g_Y (\mathcal{C}_{\ell q}^{(1)})^{ttsr} B_{\bar{\mu}} \tilde{W}^{\bar{\mu}\bar{\sigma} I} (\bar{q}_s t^I \gamma^{\bar{\sigma}} q_r) \\
& - \frac{1}{3} g_Y (\mathcal{C}_{\ell q}^{(1)})^{srtt} (\partial^2 \bar{\ell}_s \bar{\mathcal{B}} \ell_r) \\
& - \frac{1}{3} (\mathcal{C}_{\ell q}^{(1)})^{rrst} \left[ g_L g_Y B_{\bar{\mu}} W_{\bar{\nu}}^I \varepsilon^{\bar{\mu}\bar{\nu}\bar{\rho}\bar{\sigma}} (\bar{q}_s t^I \gamma^{\bar{\rho}} \partial^{\bar{\sigma}} q_t) + g_L g_Y B_{\bar{\mu}} W_{\bar{\nu}}^I \varepsilon^{\bar{\mu}\bar{\nu}\bar{\rho}\bar{\sigma}} (\partial^{\bar{\sigma}} \bar{q}_s t^I \gamma^{\bar{\rho}} q_t) \right] \\
& - \frac{1}{3} g_Y (\mathcal{C}_{\ell q}^{(1)})^{srtt} (\bar{\ell}_s \gamma^{\bar{\mu}} \ell_r) \partial^2 B_{\bar{\mu}} - \frac{2}{3} g_Y^2 (\mathcal{C}_{\ell q}^{(1)})^{ttsr} B_{\bar{\mu}} \tilde{B}^{\bar{\mu}\bar{\sigma}} (\bar{q}_s \gamma^{\bar{\sigma}} q_r)
\end{aligned}$$

$$\begin{aligned}
& -\frac{2}{3}g_L^2(\mathcal{C}_{\ell q}^{(1)})^{ttsr}W_{\bar{\mu}}^I\widetilde{W}^{\bar{\mu}\bar{\sigma}I}(\bar{q}_s\gamma^{\bar{\sigma}}q_r) - \frac{2}{3}g_Y(\mathcal{C}_{\ell q}^{(1)})^{srtt}(\partial^{\bar{\nu}}\bar{\ell}_s\bar{B}\partial^{\bar{\nu}}\ell_r) \\
& - g_Y y_d^{vu}\bar{y}_d^{tu}(\mathcal{C}_{\ell q}^{(1)})^{srtv}(H^\dagger H)(\bar{\ell}_s\bar{B}\ell_r) - \frac{4}{3}g_s^2(\mathcal{C}_{\ell q}^{(1)})^{srtt}G_{\bar{\mu}}^A\widetilde{G}^{\bar{\mu}\bar{\sigma}A}(\bar{\ell}_s\gamma^{\bar{\sigma}}\ell_r) \\
& - \frac{4}{3}g_L y_e^{vu}\bar{y}_e^{tu}(\mathcal{C}_{\ell q}^{(1)})^{tvsr}(H^\dagger t^I H)(\bar{q}_s\bar{W}^I q_r) - 2g_L^2(\mathcal{C}_{\ell q}^{(1)})^{srtt}W_{\bar{\mu}}^I\widetilde{W}^{\bar{\mu}\bar{\sigma}I}(\bar{\ell}_s\gamma^{\bar{\sigma}}\ell_r), \tag{2.49}
\end{aligned}$$

$$\begin{aligned}
\Delta S_{\mathcal{O}_{\ell q}^{(3)}} = & \frac{1}{18}g_L g_Y^2(\mathcal{C}_{\ell q}^{(3)})^{srtt}B_{\bar{\mu}}^2(\bar{\ell}_s t^I \bar{W}^I \ell_r) + \frac{1}{9}g_L g_Y^2(\mathcal{C}_{\ell q}^{(3)})^{srtt}B_{\bar{\mu}}W_{\bar{\mu}}^I(\bar{\ell}_s t^I \bar{B}\ell_r) \\
& + \frac{1}{6}g_L g_Y^2(\mathcal{C}_{\ell q}^{(3)})^{ttsr}B_{\bar{\mu}}^2(\bar{q}_s t^I \bar{W}^I q_r) + \frac{1}{3}g_L g_s^2(\mathcal{C}_{\ell q}^{(3)})^{srtt}G_{\bar{\mu}}^{A2}(\bar{\ell}_s t^I \bar{W}^I \ell_r) \\
& + \frac{1}{3}g_L g_Y(\mathcal{C}_{\ell q}^{(3)})^{srtt}\varepsilon^{IJK}B_{\bar{\mu}}W_{\bar{\nu}}^I W_{\bar{\rho}}^J \varepsilon^{\bar{\mu}\bar{\nu}\bar{\rho}\bar{\sigma}}(\bar{\ell}_s t^K \gamma^{\bar{\sigma}}\ell_r) + \frac{1}{3}g_L g_Y^2(\mathcal{C}_{\ell q}^{(3)})^{ttsr}B_{\bar{\mu}}W_{\bar{\mu}}^I(\bar{q}_s t^I \bar{B}q_r) \\
& + \frac{1}{3}(\mathcal{C}_{\ell q}^{(3)})^{ttsr}\left[g_L g_Y B_{\bar{\mu}}W_{\bar{\nu}}^I \varepsilon^{\bar{\mu}\bar{\nu}\bar{\rho}\bar{\sigma}}(\bar{q}_s t^I \gamma^{\bar{\rho}}\partial^{\bar{\sigma}}q_r) + g_L g_Y B_{\bar{\mu}}W_{\bar{\nu}}^I \varepsilon^{\bar{\mu}\bar{\nu}\bar{\rho}\bar{\sigma}}(\partial^{\bar{\sigma}}\bar{q}_s t^I \gamma^{\bar{\rho}}q_r)\right] \\
& + \frac{1}{3}g_L^2(\mathcal{C}_{\ell q}^{(3)})^{ttsr}\varepsilon^{IJK}W_{\bar{\mu}}^J(\bar{q}_s t^K \gamma^{\bar{\nu}}q_r)\partial^{\bar{\mu}}W_{\bar{\nu}}^I + \frac{1}{2}g_L^3(\mathcal{C}_{\ell q}^{(3)})^{ttsr}W_{\bar{\mu}}^{I2}(\bar{q}_s t^I \bar{W}^I q_r) \\
& + \frac{2}{3}g_L g_s^2(\mathcal{C}_{\ell q}^{(3)})^{srtt}G_{\bar{\mu}}^A W_{\bar{\mu}}^I(\bar{\ell}_s t^I \bar{G}^A \ell_r) + \frac{2}{3}g_Y y_e^{vu}\bar{y}_e^{tu}(\mathcal{C}_{\ell q}^{(3)})^{tvsr}(\bar{q}_s H \bar{B}H^\dagger q_r) \\
& + g_Y y_d^{vu}\bar{y}_d^{tu}(\mathcal{C}_{\ell q}^{(3)})^{srtv}(H^\dagger H)(\bar{\ell}_s\bar{B}\ell_r) + g_L g_Y(\mathcal{C}_{\ell q}^{(3)})^{ttsr}W_{\bar{\mu}}^I\widetilde{B}^{\bar{\mu}\bar{\sigma}}(\bar{q}_s t^I \gamma^{\bar{\sigma}}q_r) \\
& + g_L^2(\mathcal{C}_{\ell q}^{(3)})^{srtt}\varepsilon^{IJK}W_{\bar{\mu}}^J(\bar{\ell}_s t^K \gamma^{\bar{\nu}}\ell_r)\partial^{\bar{\mu}}W_{\bar{\nu}}^I + \frac{3}{2}g_L^3(\mathcal{C}_{\ell q}^{(3)})^{srtt}W_{\bar{\mu}}^{I2}(\bar{\ell}_s t^I \bar{W}^I \ell_r) \\
& + \frac{5}{3}g_L g_Y(\mathcal{C}_{\ell q}^{(3)})^{ttsr}B_{\bar{\mu}}\widetilde{W}^{\bar{\mu}\bar{\sigma}I}(\bar{q}_s t^I \gamma^{\bar{\sigma}}q_r) + 2g_L^2(\mathcal{C}_{\ell q}^{(3)})^{ttsr}\varepsilon^{IJK}W_{\bar{\mu}}^J W^{\bar{\mu}\bar{\nu}I}(\bar{q}_s t^K \gamma^{\bar{\nu}}q_r) \\
& + 6g_L^2(\mathcal{C}_{\ell q}^{(3)})^{srtt}\varepsilon^{IJK}W_{\bar{\mu}}^J W^{\bar{\mu}\bar{\nu}I}(\bar{\ell}_s t^K \gamma^{\bar{\nu}}\ell_r) - \frac{1}{3}g_Y y_e^{vu}\bar{y}_e^{tu}(\mathcal{C}_{\ell q}^{(3)})^{tvsr}(H^\dagger H)(\bar{q}_s\bar{B}q_r) \\
& - \frac{1}{3}g_L^3(\mathcal{C}_{\ell q}^{(3)})^{ttsr}W_{\bar{\mu}}^I W_{\bar{\mu}}^J(\bar{q}_s t^I \bar{W}^J q_r) - \frac{1}{3}g_L^2 g_Y(\mathcal{C}_{\ell q}^{(3)})^{ttsr}\varepsilon^{IJK}B_{\bar{\mu}}W_{\bar{\nu}}^I W_{\bar{\rho}}^J \varepsilon^{\bar{\mu}\bar{\nu}\bar{\rho}\bar{\sigma}}(\bar{q}_s t^K \gamma^{\bar{\sigma}}q_r) \\
& - \frac{1}{3}(\mathcal{C}_{\ell q}^{(3)})^{srtt}\left[g_L g_Y B_{\bar{\mu}}W_{\bar{\nu}}^I \varepsilon^{\bar{\mu}\bar{\nu}\bar{\rho}\bar{\sigma}}(\bar{\ell}_s t^I \gamma^{\bar{\rho}}\partial^{\bar{\sigma}}\ell_r) + g_L g_Y B_{\bar{\mu}}W_{\bar{\nu}}^I \varepsilon^{\bar{\mu}\bar{\nu}\bar{\rho}\bar{\sigma}}(\partial^{\bar{\sigma}}\bar{\ell}_s t^I \gamma^{\bar{\rho}}\ell_r)\right] \\
& - \frac{1}{3}g_L^2(\mathcal{C}_{\ell q}^{(3)})^{ttsr}\varepsilon^{IJK}(\bar{q}_s t^K \bar{W}^I q_r)\partial^{\bar{\nu}}W_{\bar{\nu}}^J - \frac{2}{3}g_L(\mathcal{C}_{\ell q}^{(3)})^{ttsr}(\bar{q}_s t^I \bar{W}^I \partial^2 q_r) \\
& - \frac{2}{3}g_L(\mathcal{C}_{\ell q}^{(3)})^{ttsr}(\partial^2 \bar{q}_s t^I \bar{W}^I q_r) - \frac{2}{3}g_L(\mathcal{C}_{\ell q}^{(3)})^{ttsr}(\bar{q}_s t^I \gamma^{\bar{\mu}}q_r)\partial^2 W_{\bar{\mu}}^I \\
& - g_L g_Y(\mathcal{C}_{\ell q}^{(3)})^{srtt}W_{\bar{\mu}}^I\widetilde{B}^{\bar{\mu}\bar{\sigma}}(\bar{\ell}_s t^I \gamma^{\bar{\sigma}}\ell_r) - g_L^3(\mathcal{C}_{\ell q}^{(3)})^{srtt}W_{\bar{\mu}}^I W_{\bar{\mu}}^J(\bar{\ell}_s t^I \bar{W}^J \ell_r) \\
& - g_L^2(\mathcal{C}_{\ell q}^{(3)})^{srtt}\varepsilon^{IJK}(\bar{\ell}_s t^K \bar{W}^I \ell_r)\partial^{\bar{\nu}}W_{\bar{\nu}}^J - \frac{4}{3}g_L y_e^{vu}\bar{y}_e^{tu}(\mathcal{C}_{\ell q}^{(3)})^{tvsr}(H^\dagger H)(\bar{q}_s t^I \bar{W}^I q_r) \\
& - \frac{4}{3}g_L(\mathcal{C}_{\ell q}^{(3)})^{ttsr}(\partial^{\bar{\nu}}\bar{q}_s t^I \bar{W}^I \partial^{\bar{\nu}}q_r) - \frac{5}{3}g_L g_Y(\mathcal{C}_{\ell q}^{(3)})^{srtt}B_{\bar{\mu}}\widetilde{W}^{\bar{\mu}\bar{\sigma}I}(\bar{\ell}_s t^I \gamma^{\bar{\sigma}}\ell_r) \\
& - \frac{5}{3}(\mathcal{C}_{\ell q}^{(3)})^{ttsr}\left[g_L^2\varepsilon^{IJK}W_{\bar{\nu}}^J(\bar{q}_s t^K \bar{W}^I \partial^{\bar{\nu}}q_r) + g_L^2\varepsilon^{IJK}W_{\bar{\nu}}^J(\partial^{\bar{\nu}}\bar{q}_s t^K \bar{W}^I q_r)\right] \\
& - 2g_L(\mathcal{C}_{\ell q}^{(3)})^{srtt}(\bar{\ell}_s t^I \bar{W}^I \partial^2 \ell_r) - 2g_Y y_d^{vu}\bar{y}_d^{tu}(\mathcal{C}_{\ell q}^{(3)})^{srtv}(\bar{\ell}_s H \bar{B}H^\dagger \ell_r) - 2g_L(\mathcal{C}_{\ell q}^{(3)})^{srtt}(\partial^2 \bar{\ell}_s t^I \bar{W}^I \ell_r) \\
& - 2g_L(\mathcal{C}_{\ell q}^{(3)})^{srtt}(\bar{\ell}_s t^I \gamma^{\bar{\mu}}\ell_r)\partial^2 W_{\bar{\mu}}^I - 4g_L(\mathcal{C}_{\ell q}^{(3)})^{srtv}\left[y_d^{vu}\bar{y}_d^{tu} + y_u^{vu}\bar{y}_u^{tu}\right](H^\dagger H)(\bar{\ell}_s t^I \bar{W}^I \ell_r) \\
& - 4g_L(\mathcal{C}_{\ell q}^{(3)})^{srtt}(\partial^{\bar{\nu}}\bar{\ell}_s t^I \bar{W}^I \partial^{\bar{\nu}}\ell_r)
\end{aligned}$$

$$-5(\mathcal{C}_{\ell_q}^{(3)})^{srtt} \left[ g_L^2 \varepsilon^{IJK} W_{\bar{\nu}}^J (\bar{\ell}_s t^K \bar{W}^I \partial^{\bar{\nu}} \ell_r) + g_L^2 \varepsilon^{IJK} W_{\bar{\nu}}^J (\partial^{\bar{\nu}} \bar{\ell}_s t^K \bar{W}^I \ell_r) \right], \quad (2.50)$$

$$\begin{aligned} \Delta S_{\mathcal{O}_{ud}^{(1)}} = & \frac{1}{12} g_s^3 (\mathcal{C}_{ud}^{(1)})^{ttsr} d^{ABC} G_{\bar{\nu}}^B G_{\bar{\nu}}^C (\bar{d}_s \bar{\mathcal{G}}^A d_r) + \frac{1}{12} g_s^3 (\mathcal{C}_{ud}^{(1)})^{srtt} d^{ABC} G_{\bar{\nu}}^B G_{\bar{\nu}}^C (\bar{u}_s \bar{\mathcal{G}}^A u_r) \\ & + \frac{1}{9} g_s^2 g_Y (\mathcal{C}_{ud}^{(1)})^{ttsr} G_{\bar{\mu}}^{A2} (\bar{d}_s \bar{\mathcal{B}} d_r) + \frac{2}{9} g_s^2 g_Y (\mathcal{C}_{ud}^{(1)})^{ttsr} B_{\bar{\mu}} G_{\bar{\mu}}^A (\bar{d}_s \bar{\mathcal{G}}^A d_r) + \frac{8}{27} g_Y^3 (\mathcal{C}_{ud}^{(1)})^{ttsr} B_{\bar{\mu}}^2 (\bar{d}_s \bar{\mathcal{B}} d_r) \\ & + \frac{1}{3} g_L y_u^{tv} \bar{y}_d^{tu} (\mathcal{C}_{ud}^{(1)})^{vrsu} t_k^{Ij} H_j^\dagger \tilde{H}_k (\bar{d}_s \bar{W}^I u_r) + \frac{1}{3} g_Y (\mathcal{C}_{ud}^{(1)})^{srtt} (\bar{u}_s \bar{\mathcal{B}} \partial^2 u_r) \\ & + \frac{1}{3} g_L y_d^{tv} \bar{y}_u^{tu} (\mathcal{C}_{ud}^{(1)})^{suvs} t_k^{Ii} \tilde{H}^{\dagger i} H^k (\bar{u}_s \bar{W}^I d_r) + \frac{1}{3} g_Y (\mathcal{C}_{ud}^{(1)})^{srtt} (\partial^2 \bar{u}_s \bar{\mathcal{B}} u_r) + \frac{1}{3} g_Y (\mathcal{C}_{ud}^{(1)})^{srtt} (\bar{u}_s \gamma^{\bar{\mu}} u_r) \partial^2 B_{\bar{\mu}} \\ & + \frac{4}{9} g_Y^2 (\mathcal{C}_{ud}^{(1)})^{srtt} B_{\bar{\mu}} \tilde{B}^{\bar{\mu}\bar{\sigma}} (\bar{u}_s \gamma^{\bar{\sigma}} u_r) + \frac{2}{3} g_s^2 (\mathcal{C}_{ud}^{(1)})^{ttsr} G_{\bar{\mu}}^A \tilde{G}^{\bar{\mu}\bar{\sigma}A} (\bar{d}_s \gamma^{\bar{\sigma}} d_r) \\ & + \frac{2}{3} g_s^2 (\mathcal{C}_{ud}^{(1)})^{srtt} G_{\bar{\mu}}^A \tilde{G}^{\bar{\mu}\bar{\sigma}A} (\bar{u}_s \gamma^{\bar{\sigma}} u_r) + \frac{2}{3} g_Y (\mathcal{C}_{ud}^{(1)})^{srtt} (\partial^{\bar{\nu}} \bar{u}_s \bar{\mathcal{B}} \partial^{\bar{\nu}} u_r) \\ & + g_L y_d^{tv} \bar{y}_u^{tu} (\mathcal{C}_{ud}^{(1)})^{srvu} (H^\dagger t^I H) (\bar{u}_s \bar{W}^I u_r) + \frac{3}{2} g_Y y_d^{tv} \bar{y}_u^{tu} (\mathcal{C}_{ud}^{(1)})^{srvu} (H^\dagger H) (\bar{u}_s \bar{\mathcal{B}} u_r) \\ & + \frac{16}{9} g_Y^2 (\mathcal{C}_{ud}^{(1)})^{ttsr} B_{\bar{\mu}} \tilde{B}^{\bar{\mu}\bar{\sigma}} (\bar{d}_s \gamma^{\bar{\sigma}} d_r) - \frac{1}{27} g_Y^3 (\mathcal{C}_{ud}^{(1)})^{srtt} B_{\bar{\mu}}^2 (\bar{u}_s \bar{\mathcal{B}} u_r) - \frac{1}{18} g_s^2 g_Y (\mathcal{C}_{ud}^{(1)})^{srtt} G_{\bar{\mu}}^{A2} (\bar{u}_s \bar{\mathcal{B}} u_r) \\ & - \frac{1}{12} g_s^3 (\mathcal{C}_{ud}^{(1)})^{ttsr} f^{ABC} G_{\bar{\mu}}^A G_{\bar{\nu}}^B G_{\bar{\rho}}^C \varepsilon^{\bar{\mu}\bar{\nu}\bar{\rho}\bar{\sigma}} (\bar{d}_s \gamma^{\bar{\sigma}} d_r) \\ & - \frac{1}{12} g_s^3 (\mathcal{C}_{ud}^{(1)})^{srtt} f^{ABC} G_{\bar{\mu}}^A G_{\bar{\nu}}^B G_{\bar{\rho}}^C \varepsilon^{\bar{\mu}\bar{\nu}\bar{\rho}\bar{\sigma}} (\bar{u}_s \gamma^{\bar{\sigma}} u_r) - \frac{1}{9} g_s^2 g_Y (\mathcal{C}_{ud}^{(1)})^{srtt} B_{\bar{\mu}} G_{\bar{\mu}}^A (\bar{u}_s \bar{\mathcal{G}}^A u_r) \\ & - \frac{2}{3} g_Y (\mathcal{C}_{ud}^{(1)})^{ttsr} (\bar{d}_s \bar{\mathcal{B}} \partial^2 d_r) - \frac{2}{3} g_Y (\mathcal{C}_{ud}^{(1)})^{ttsr} (\partial^2 \bar{d}_s \bar{\mathcal{B}} d_r) - \frac{2}{3} g_Y (\mathcal{C}_{ud}^{(1)})^{ttsr} (\bar{d}_s \gamma^{\bar{\mu}} d_r) \partial^2 B_{\bar{\mu}} \\ & - g_L y_u^{tv} \bar{y}_d^{tu} (\mathcal{C}_{ud}^{(1)})^{vusr} (H^\dagger t^I H) (\bar{d}_s \bar{W}^I d_r) - \frac{4}{3} g_Y (\mathcal{C}_{ud}^{(1)})^{ttsr} (\partial^{\bar{\nu}} \bar{d}_s \bar{\mathcal{B}} \partial^{\bar{\nu}} d_r) - \frac{5}{2} g_Y y_u^{tv} \bar{y}_d^{tu} (\mathcal{C}_{ud}^{(1)})^{vusr} (H^\dagger H) (\bar{d}_s \bar{\mathcal{B}} d_r), \end{aligned} \quad (2.51)$$

$$\begin{aligned} \Delta S_{\mathcal{O}_{ud}^{(8)}} = & \frac{1}{108} g_s^2 g_Y (\mathcal{C}_{ud}^{(8)})^{srtt} G_{\bar{\mu}}^{A2} (\bar{u}_s \bar{\mathcal{B}} u_r) + \frac{1}{72} g_s^3 (\mathcal{C}_{ud}^{(8)})^{ttsr} f^{ABC} G_{\bar{\mu}}^A G_{\bar{\nu}}^B G_{\bar{\rho}}^C \varepsilon^{\bar{\mu}\bar{\nu}\bar{\rho}\bar{\sigma}} (\bar{d}_s \gamma^{\bar{\sigma}} d_r) \\ & + \frac{1}{72} g_s^3 (\mathcal{C}_{ud}^{(8)})^{srtt} f^{ABC} G_{\bar{\mu}}^A G_{\bar{\nu}}^B G_{\bar{\rho}}^C \varepsilon^{\bar{\mu}\bar{\nu}\bar{\rho}\bar{\sigma}} (\bar{u}_s \gamma^{\bar{\sigma}} u_r) + \frac{1}{54} g_s^2 g_Y (\mathcal{C}_{ud}^{(8)})^{srtt} B_{\bar{\mu}} G_{\bar{\mu}}^A (\bar{u}_s \bar{\mathcal{G}}^A u_r) \\ & + \frac{1}{54} g_s g_Y^2 (\mathcal{C}_{ud}^{(8)})^{srtt} B_{\bar{\mu}}^2 (\bar{u}_s T^A \bar{\mathcal{G}}^A u_r) + \frac{1}{27} g_s g_Y^2 (\mathcal{C}_{ud}^{(8)})^{srtt} B_{\bar{\mu}} G_{\bar{\mu}}^A (\bar{u}_s T^A \bar{\mathcal{B}} u_r) \\ & - \frac{i}{18} g_s^2 g_Y (\mathcal{C}_{ud}^{(8)})^{srtt} T_b^{Aa} T_a^{Bc} B_{\bar{\mu}} G_{\bar{\nu}}^B G_{\bar{\rho}}^A \varepsilon^{\bar{\mu}\bar{\nu}\bar{\rho}\bar{\sigma}} (\bar{u}_{cs} \gamma^{\bar{\sigma}} u_r^b) + \frac{2}{27} g_s g_Y^2 (\mathcal{C}_{ud}^{(8)})^{ttsr} B_{\bar{\mu}}^2 (\bar{d}_s T^A \bar{\mathcal{G}}^A d_r) \\ & - \frac{i}{12} (\mathcal{C}_{ud}^{(8)})^{ttsr} \left[ g_s^2 T_b^{Aa} T_c^{Bb} G_{\bar{\mu}}^B (\bar{d}_{as} \gamma^{\bar{\nu}} d_r^c) \partial^{\bar{\mu}} G_{\bar{\nu}}^A - g_s^2 T_b^{Aa} T_a^{Bc} G_{\bar{\mu}}^B (\bar{d}_{cs} \gamma^{\bar{\nu}} d_r^b) \partial^{\bar{\mu}} G_{\bar{\nu}}^A \right] \\ & - \frac{i}{12} (\mathcal{C}_{ud}^{(8)})^{srtt} \left[ g_s^2 T_b^{Aa} T_c^{Bb} G_{\bar{\mu}}^B (\bar{u}_{as} \gamma^{\bar{\nu}} u_r^c) \partial^{\bar{\mu}} G_{\bar{\nu}}^A - g_s^2 T_b^{Aa} T_a^{Bc} G_{\bar{\mu}}^B (\bar{u}_{cs} \gamma^{\bar{\nu}} u_r^b) \partial^{\bar{\mu}} G_{\bar{\nu}}^A \right] \\ & - \frac{i}{12} (\mathcal{C}_{ud}^{(8)})^{ttsr} \left[ g_s^2 T_b^{Aa} T_c^{Bb} (\bar{d}_{as} \bar{\mathcal{G}}^B d_r^c) \partial^{\bar{\nu}} G_{\bar{\nu}}^A - g_s^2 T_b^{Aa} T_a^{Bc} (\bar{d}_{cs} \bar{\mathcal{G}}^B d_r^b) \partial^{\bar{\nu}} G_{\bar{\nu}}^A \right] \\ & - \frac{i}{12} (\mathcal{C}_{ud}^{(8)})^{srtt} \left[ g_s^2 T_b^{Aa} T_c^{Bb} (\bar{u}_{as} \bar{\mathcal{G}}^B u_r^c) \partial^{\bar{\nu}} G_{\bar{\nu}}^A - g_s^2 T_b^{Aa} T_a^{Bc} (\bar{u}_{cs} \bar{\mathcal{G}}^B u_r^b) \partial^{\bar{\nu}} G_{\bar{\nu}}^A \right] \\ & + \frac{i}{9} g_s^2 g_Y (\mathcal{C}_{ud}^{(8)})^{ttsr} T_b^{Aa} T_a^{Bc} B_{\bar{\mu}} G_{\bar{\nu}}^B G_{\bar{\rho}}^A \varepsilon^{\bar{\mu}\bar{\nu}\bar{\rho}\bar{\sigma}} (\bar{d}_{cs} \gamma^{\bar{\sigma}} d_r^b) \end{aligned}$$

$$\begin{aligned}
& + \frac{1}{9} g_s^2 g_Y (\mathcal{C}_{ud}^{(8)})^{ttsr} T_b^{Aa} T_a^{Bc} G_{\bar{\nu}}^A G_{\bar{\nu}}^B (\bar{d}_{cs} \bar{B} d_r^b) \\
& + \frac{1}{9} (\mathcal{C}_{ud}^{(8)})^{ttsr} \left[ g_s^2 g_Y T_b^{Aa} T_c^{Bb} B_{\bar{\mu}} G_{\bar{\mu}}^B (\bar{d}_{as} \bar{G}^A d_r^c) + g_s^2 g_Y T_b^{Aa} T_a^{Bc} B_{\bar{\mu}} G_{\bar{\mu}}^B (\bar{d}_{cs} \bar{G}^A d_r^b) \right] \\
& + \frac{4}{27} g_s g_Y^2 (\mathcal{C}_{ud}^{(8)})^{ttsr} B_{\bar{\mu}} G_{\bar{\mu}}^A (\bar{d}_s T^A \bar{B} d_r) \\
& + \frac{1}{6} g_s (\mathcal{C}_{ud}^{(8)})^{ttsr} \left[ 2g_s T_b^{Aa} T_c^{Bb} G_{\bar{\mu}}^B \tilde{G}^{\bar{\mu}\bar{\sigma}A} (\bar{d}_{as} \gamma^{\bar{\sigma}} d_r^c) + 2g_s T_b^{Aa} T_a^{Bc} G_{\bar{\mu}}^B \tilde{G}^{\bar{\mu}\bar{\sigma}A} (\bar{d}_{cs} \gamma^{\bar{\sigma}} d_r^b) \right] \\
& + \frac{i}{6} g_s^3 (\mathcal{C}_{ud}^{(8)})^{ttsr} T_b^{Aa} T_a^{Bc} T_c^{Cd} G_{\bar{\mu}}^A G_{\bar{\nu}}^C G_{\bar{\rho}}^B \varepsilon^{\bar{\mu}\bar{\nu}\bar{\rho}\bar{\sigma}} (\bar{d}_{ds} \gamma^{\bar{\sigma}} d_r^b) \\
& + \frac{1}{6} (\mathcal{C}_{ud}^{(8)})^{ttsr} \left[ g_s^3 T_b^{Aa} T_c^{Bb} T_d^{Cd} G_{\bar{\mu}}^B G_{\bar{\mu}}^C (\bar{d}_{as} \bar{G}^A d_r^d) + g_s^3 T_b^{Aa} T_a^{Bc} T_c^{Cd} G_{\bar{\mu}}^B G_{\bar{\mu}}^C (\bar{d}_{ds} \bar{G}^A d_r^b) \right] \\
& + \frac{1}{6} g_s (\mathcal{C}_{ud}^{(8)})^{srtt} \left[ 2g_s T_b^{Aa} T_c^{Bb} G_{\bar{\mu}}^B \tilde{G}^{\bar{\mu}\bar{\sigma}A} (\bar{u}_{as} \gamma^{\bar{\sigma}} u_r^c) + 2g_s T_b^{Aa} T_a^{Bc} G_{\bar{\mu}}^B \tilde{G}^{\bar{\mu}\bar{\sigma}A} (\bar{u}_{cs} \gamma^{\bar{\sigma}} u_r^b) \right] \\
& + \frac{4}{9} g_L y_u^{tu} \bar{y}_d^{tu} (\mathcal{C}_{ud}^{(8)})^{vrsu} t_k^{Ij} H_j^\dagger \tilde{H}_k (\bar{d}_s \bar{W}^I u_r) + \frac{4}{9} g_s g_Y (\mathcal{C}_{ud}^{(8)})^{ttsr} G_{\bar{\mu}}^A \tilde{B}^{\bar{\mu}\bar{\sigma}} (\bar{d}_s T^A \gamma^{\bar{\sigma}} d_r) \\
& + \frac{4}{9} g_s g_Y (\mathcal{C}_{ud}^{(8)})^{ttsr} B_{\bar{\mu}} \tilde{G}^{\bar{\mu}\bar{\sigma}A} (\bar{d}_s T^A \gamma^{\bar{\sigma}} d_r) + \frac{4}{9} g_L y_d^{tu} \bar{y}_u^{tu} (\mathcal{C}_{ud}^{(8)})^{suvr} t_k^{Ii} \tilde{H}^{\dagger i} H^k (\bar{u}_s \bar{W}^I d_r) \\
& - \frac{1}{72} g_s^3 (\mathcal{C}_{ud}^{(8)})^{ttsr} d^{ABC} G_{\bar{\nu}}^B G_{\bar{\nu}}^C (\bar{d}_s \bar{G}^A d_r) - \frac{1}{72} g_s^3 (\mathcal{C}_{ud}^{(8)})^{srtt} d^{ABC} G_{\bar{\nu}}^B G_{\bar{\nu}}^C (\bar{u}_s \bar{G}^A u_r) \\
& - \frac{1}{54} g_s^2 g_Y (\mathcal{C}_{ud}^{(8)})^{ttsr} G_{\bar{\mu}}^{A2} (\bar{d}_s \bar{B} d_r) - \frac{1}{27} g_s^2 g_Y (\mathcal{C}_{ud}^{(8)})^{ttsr} B_{\bar{\mu}} G_{\bar{\mu}}^A (\bar{d}_s \bar{G}^A d_r) \\
& - \frac{1}{18} g_s^2 g_Y (\mathcal{C}_{ud}^{(8)})^{srtt} T_b^{Aa} T_a^{Bc} G_{\bar{\nu}}^A G_{\bar{\nu}}^B (\bar{u}_{cs} \bar{B} u_r^b) \\
& - \frac{1}{18} (\mathcal{C}_{ud}^{(8)})^{srtt} \left[ g_s^2 g_Y T_b^{Aa} T_c^{Bb} B_{\bar{\mu}} G_{\bar{\mu}}^B (\bar{u}_{as} \bar{G}^A u_r^c) + g_s^2 g_Y T_b^{Aa} T_a^{Bc} B_{\bar{\mu}} G_{\bar{\mu}}^B (\bar{u}_{cs} \bar{G}^A u_r^b) \right] \\
& - \frac{1}{9} g_s^2 (\mathcal{C}_{ud}^{(8)})^{ttsr} G_{\bar{\mu}}^A \tilde{G}^{\bar{\mu}\bar{\sigma}A} (\bar{d}_s \gamma^{\bar{\sigma}} d_r) - \frac{1}{9} g_s^2 (\mathcal{C}_{ud}^{(8)})^{srtt} G_{\bar{\mu}}^A \tilde{G}^{\bar{\mu}\bar{\sigma}A} (\bar{u}_s \gamma^{\bar{\sigma}} u_r) \\
& - \frac{1}{6} g_s (\mathcal{C}_{ud}^{(8)})^{ttsr} (\bar{d}_s T^A \bar{G}^A \partial^2 d_r) - \frac{1}{6} g_s^3 (\mathcal{C}_{ud}^{(8)})^{ttsr} T_b^{Aa} T_a^{Bc} T_c^{Cd} G_{\bar{\mu}}^A G_{\bar{\mu}}^C (\bar{d}_{ds} \bar{G}^B d_r^b) \\
& - \frac{1}{6} g_s (\mathcal{C}_{ud}^{(8)})^{srtt} (\bar{u}_s T^A \bar{G}^A \partial^2 u_r) + \frac{i}{6} g_s^3 (\mathcal{C}_{ud}^{(8)})^{srtt} T_b^{Aa} T_a^{Bc} T_c^{Cd} G_{\bar{\mu}}^A G_{\bar{\nu}}^C G_{\bar{\rho}}^B \varepsilon^{\bar{\mu}\bar{\nu}\bar{\rho}\bar{\sigma}} (\bar{u}_{ds} \gamma^{\bar{\sigma}} u_r^b) \\
& + \frac{1}{6} (\mathcal{C}_{ud}^{(8)})^{srtt} \left[ g_s^3 T_b^{Aa} T_c^{Bb} T_d^{Cd} G_{\bar{\mu}}^B G_{\bar{\mu}}^C (\bar{u}_{as} \bar{G}^A u_r^d) + g_s^3 T_b^{Aa} T_a^{Bc} T_c^{Cd} G_{\bar{\mu}}^B G_{\bar{\mu}}^C (\bar{u}_{ds} \bar{G}^A u_r^b) \right] \\
& - \frac{1}{6} g_s^3 (\mathcal{C}_{ud}^{(8)})^{srtt} T_b^{Aa} T_a^{Bc} T_c^{Cd} G_{\bar{\mu}}^A G_{\bar{\mu}}^C (\bar{u}_{ds} \bar{G}^B u_r^b) - \frac{1}{6} g_s (\mathcal{C}_{ud}^{(8)})^{ttsr} (\partial^2 \bar{d}_s T^A \bar{G}^A d_r) \\
& - \frac{1}{6} g_s (\mathcal{C}_{ud}^{(8)})^{srtt} (\partial^2 \bar{u}_s T^A \bar{G}^A u_r) - \frac{1}{6} g_s (\mathcal{C}_{ud}^{(8)})^{ttsr} (\bar{d}_s T^A \gamma^{\bar{\mu}} d_r) \partial^2 G_{\bar{\mu}}^A - \frac{1}{6} g_s (\mathcal{C}_{ud}^{(8)})^{srtt} (\bar{u}_s T^A \gamma^{\bar{\mu}} u_r) \partial^2 G_{\bar{\mu}}^A \\
& - \frac{2}{9} g_s g_Y (\mathcal{C}_{ud}^{(8)})^{srtt} G_{\bar{\mu}}^A \tilde{B}^{\bar{\mu}\bar{\sigma}} (\bar{u}_s T^A \gamma^{\bar{\sigma}} u_r) - \frac{2}{9} g_s g_Y (\mathcal{C}_{ud}^{(8)})^{srtt} B_{\bar{\mu}} \tilde{G}^{\bar{\mu}\bar{\sigma}A} (\bar{u}_s T^A \gamma^{\bar{\sigma}} u_r) \\
& - \frac{1}{3} g_s (\mathcal{C}_{ud}^{(8)})^{ttsr} (\partial^{\bar{\nu}} \bar{d}_s T^A \bar{G}^A \partial^{\bar{\nu}} d_r) - \frac{1}{3} g_s (\mathcal{C}_{ud}^{(8)})^{srtt} (\partial^{\bar{\nu}} \bar{u}_s T^A \bar{G}^A \partial^{\bar{\nu}} u_r) \\
& - \frac{5i}{12} (\mathcal{C}_{ud}^{(8)})^{ttsr} \left[ g_s^2 T_b^{Aa} T_a^{Bc} G_{\bar{\nu}}^B (\bar{d}_{cs} \bar{G}^A \partial^{\bar{\nu}} d_r^b) - g_s^2 T_b^{Aa} T_c^{Bb} G_{\bar{\nu}}^B (\partial^{\bar{\nu}} \bar{d}_{as} \bar{G}^A d_r^c) \right] \\
& - \frac{5i}{12} (\mathcal{C}_{ud}^{(8)})^{ttsr} \left[ g_s^2 T_b^{Aa} T_c^{Bb} G_{\bar{\nu}}^A (\partial^{\bar{\nu}} \bar{d}_{as} \bar{G}^B d_r^c) - g_s^2 T_b^{Aa} T_a^{Bc} G_{\bar{\nu}}^A (\bar{d}_{cs} \bar{G}^B \partial^{\bar{\nu}} d_r^b) \right]
\end{aligned}$$

$$\begin{aligned}
& -\frac{5i}{12}(\mathcal{C}_{ud}^{(8)})^{srtt} \left[ g_s^2 T_b^{Aa} T_a^{Bc} G_\nu^B (\bar{u}_{cs} \bar{\mathcal{G}}^A \partial^\nu u_r^b) - g_s^2 T_b^{Aa} T_c^{Bb} G_\nu^B (\partial^\nu \bar{u}_{as} \bar{\mathcal{G}}^A u_r^c) \right] \\
& -\frac{5i}{12}(\mathcal{C}_{ud}^{(8)})^{srtt} \left[ g_s^2 T_b^{Aa} T_c^{Bb} G_\nu^A (\partial^\nu \bar{u}_{as} \bar{\mathcal{G}}^B u_r^c) - g_s^2 T_b^{Aa} T_a^{Bc} G_\nu^A (\bar{u}_{cs} \bar{\mathcal{G}}^B \partial^\nu u_r^b) \right] \\
& -\frac{1}{2} g_s y_u^{tv} \bar{y}_u^{tu} (\mathcal{C}_{ud}^{(8)})^{vusr} (H^\dagger H) (\bar{d}_s T^A \bar{\mathcal{G}}^A d_r) \\
& -\frac{i}{2} g_s (\mathcal{C}_{ud}^{(8)})^{ttsr} \left[ g_s T_b^{Aa} T_c^{Bb} G_\mu^B G^{\mu\nu A} (\bar{d}_{as} \gamma^\nu d_r^c) - g_s T_b^{Aa} T_a^{Bc} G_\mu^B G^{\mu\nu A} (\bar{d}_{cs} \gamma^\nu d_r^b) \right] \\
& -\frac{1}{2} g_s y_d^{tv} \bar{y}_d^{tu} (\mathcal{C}_{ud}^{(8)})^{srvu} (H^\dagger H) (\bar{u}_s T^A \bar{\mathcal{G}}^A u_r) \\
& -\frac{i}{2} g_s (\mathcal{C}_{ud}^{(8)})^{srtt} \left[ g_s T_b^{Aa} T_c^{Bb} G_\mu^B G^{\mu\nu A} (\bar{u}_{as} \gamma^\nu u_r^c) - g_s T_b^{Aa} T_a^{Bc} G_\mu^B G^{\mu\nu A} (\bar{u}_{cs} \gamma^\nu u_r^b) \right], \tag{2.52}
\end{aligned}$$

$$\begin{aligned}
\Delta S_{\mathcal{O}_{qu}^{(1)}} &= \frac{1}{108} g_Y^3 (\mathcal{C}_{qu}^{(1)})^{ttsr} B_\mu^2 (\bar{u}_s \bar{\mathcal{B}} u_r) + \frac{1}{18} g_s^2 g_Y (\mathcal{C}_{qu}^{(1)})^{ttsr} G_\mu^A{}^2 (\bar{u}_s \bar{\mathcal{B}} u_r) + \frac{1}{12} g_s^3 (\mathcal{C}_{qu}^{(1)})^{srtt} d^{ABC} G_\nu^B G_\nu^C (\bar{q}_s \bar{\mathcal{G}}^A q_r) \\
&+ \frac{1}{12} g_L^2 g_Y (\mathcal{C}_{qu}^{(1)})^{ttsr} W_\mu^I{}^2 (\bar{u}_s \bar{\mathcal{B}} u_r) + \frac{1}{9} g_s^2 g_Y (\mathcal{C}_{qu}^{(1)})^{srtt} G_\mu^A{}^2 (\bar{q}_s \bar{\mathcal{B}} q_r) + \frac{1}{9} g_s^2 g_Y (\mathcal{C}_{qu}^{(1)})^{ttsr} B_\mu G_\mu^A (\bar{u}_s \bar{\mathcal{G}}^A u_r) \\
&+ \frac{1}{6} g_s^3 (\mathcal{C}_{qu}^{(1)})^{ttsr} f^{ABC} G_\mu^A G_\nu^B G_\rho^C \varepsilon^{\mu\nu\rho\sigma} (\bar{u}_s \gamma^\sigma u_r) + \frac{1}{6} g_s^3 (\mathcal{C}_{qu}^{(1)})^{ttsr} d^{ABC} G_\nu^B G_\nu^C (\bar{u}_s \bar{\mathcal{G}}^A u_r) \\
&+ \frac{1}{6} g_L^2 g_Y (\mathcal{C}_{qu}^{(1)})^{ttsr} B_\mu W_\mu^I (\bar{u}_s \bar{W}^I u_r) + \frac{2}{9} g_s^2 g_Y (\mathcal{C}_{qu}^{(1)})^{srtt} B_\mu G_\mu^A (\bar{q}_s \bar{\mathcal{G}}^A q_r) \\
&+ \frac{1}{4} g_L^3 (\mathcal{C}_{qu}^{(1)})^{ttsr} \varepsilon^{IJK} W_\mu^I W_\nu^J W_\rho^K \varepsilon^{\mu\nu\rho\sigma} (\bar{u}_s \gamma^\sigma u_r) + \frac{8}{27} g_Y^3 (\mathcal{C}_{qu}^{(1)})^{srtt} B_\mu^2 (\bar{q}_s \bar{\mathcal{B}} q_r) \\
&+ \frac{1}{3} g_L^2 y_u^{tu} (\mathcal{C}_{qu}^{(1)})^{stur} W_\mu^I{}^2 (\bar{q}_s \tilde{H} u_r) + \frac{i}{3} g_Y y_u^{tu} (\mathcal{C}_{qu}^{(1)})^{stur} B_\mu (\bar{q}_s \tilde{H} \partial^\mu u_r) + \frac{i}{3} g_Y y_u^{tu} (\mathcal{C}_{qu}^{(1)})^{stur} B_\mu (\bar{q}_s \partial^\mu \tilde{H} u_r) \\
&+ \frac{1}{3} g_L^2 \bar{y}_u^{tu} (\mathcal{C}_{qu}^{(1)})^{trsu} W_\mu^I{}^2 (\bar{u}_s \tilde{H}^\dagger q_r) - \frac{i}{3} g_Y \bar{y}_u^{tu} (\mathcal{C}_{qu}^{(1)})^{trsu} B_\mu (\bar{u}_s \partial^\mu \tilde{H} q_r) \\
&- \frac{i}{3} g_Y \bar{y}_u^{tu} (\mathcal{C}_{qu}^{(1)})^{trsu} B_\mu (\partial^\mu \bar{u}_s \tilde{H}^\dagger q_r) + \frac{2}{3} g_s^2 (\mathcal{C}_{qu}^{(1)})^{srtt} G_\mu^A \tilde{G}^{\mu\sigma A} (\bar{q}_s \gamma^\sigma q_r) \\
&+ \frac{2}{3} g_L^2 y_u^{tu} (\mathcal{C}_{qu}^{(1)})^{stur} \varepsilon^{jk} t_l^i t_j^{Il} H_i^\dagger W_\mu^I W_\mu^J (\bar{q}_{ks} u_r) + \frac{2}{3} g_L g_Y y_u^{tu} (\mathcal{C}_{qu}^{(1)})^{stur} t_j^{Ik} \tilde{H}_j B_\mu W_\mu^I (\bar{q}_{ks} u_r) \\
&+ \frac{2i}{3} g_L y_u^{tu} (\mathcal{C}_{qu}^{(1)})^{stur} \varepsilon^{jk} t_j^{Ii} H_i^\dagger W_\mu^I (\bar{q}_{ks} \partial^\mu u_r) + \frac{2}{3} g_L^2 \bar{y}_u^{tu} (\mathcal{C}_{qu}^{(1)})^{trsu} \varepsilon_{ij} t_l^{Ik} t_k^{Ji} H^l W_\mu^I W_\mu^J (\bar{u}_s q_r^j) \\
&+ \frac{2}{3} g_L g_Y y_u^{tu} (\mathcal{C}_{qu}^{(1)})^{trsu} t_k^{Ii} \tilde{H}^\dagger{}^i B_\mu W_\mu^I (\bar{u}_s q_r^k) + \frac{13}{18} g_Y^2 y_u^{tu} (\mathcal{C}_{qu}^{(1)})^{stur} B_\mu^2 (\bar{q}_s \tilde{H} u_r) \\
&+ \frac{5}{3} g_s g_Y y_u^{tu} (\mathcal{C}_{qu}^{(1)})^{stur} T_b^{Aa} B_\mu G_\mu^A (\bar{q}_{as} \tilde{H} u_r^b) + \frac{5}{3} g_s g_Y \bar{y}_u^{tu} (\mathcal{C}_{qu}^{(1)})^{trsu} T_b^{Aa} B_\mu G_\mu^A (\bar{u}_{as} \tilde{H}^\dagger q_r^b) \\
&+ \frac{16}{9} g_Y^2 (\mathcal{C}_{qu}^{(1)})^{srtt} B_\mu \tilde{B}^{\mu\sigma} (\bar{q}_s \gamma^\sigma q_r) + 2 g_s^2 y_u^{tu} (\mathcal{C}_{qu}^{(1)})^{stur} T_b^{Aa} T_a^{Bc} G_\mu^A G_\mu^B (\bar{q}_{cs} \tilde{H} u_r^b) \\
&+ 2 g_s^2 \bar{y}_u^{tu} (\mathcal{C}_{qu}^{(1)})^{trsu} T_b^{Aa} T_c^{Bb} G_\mu^A G_\mu^B (\bar{u}_{as} \tilde{H}^\dagger q_r^c) + 4 g_L (\mathcal{C}_{qu}^{(1)})^{tvsr} \left[ y_u^{vu} \bar{y}_u^{tu} - y_d^{vu} \bar{y}_d^{tu} \right] (H^\dagger t^I H) (\bar{u}_s \bar{W}^I u_r) \\
&- \frac{1}{12} g_s^3 (\mathcal{C}_{qu}^{(1)})^{srtt} f^{ABC} G_\mu^A G_\nu^B G_\rho^C \varepsilon^{\mu\nu\rho\sigma} (\bar{q}_s \gamma^\sigma q_r) - \frac{2}{9} g_Y^2 (\mathcal{C}_{qu}^{(1)})^{ttsr} B_\mu \tilde{B}^{\mu\sigma} (\bar{u}_s \gamma^\sigma u_r) \\
&- \frac{i}{3} g_Y \bar{y}_u^{tu} (\mathcal{C}_{qu}^{(1)})^{trsu} B_\mu (\bar{u}_s \tilde{H}^\dagger \partial^\mu q_r) - \frac{1}{3} g_Y (\mathcal{C}_{qu}^{(1)})^{ttsr} (\bar{u}_s \bar{\mathcal{B}} \partial^2 u_r) - \frac{1}{3} g_Y (\mathcal{C}_{qu}^{(1)})^{ttsr} (\partial^2 \bar{u}_s \bar{\mathcal{B}} u_r) \\
&+ \frac{i}{3} g_Y y_u^{tu} (\mathcal{C}_{qu}^{(1)})^{stur} B_\mu (\partial^\mu \bar{q}_s \tilde{H} u_r) - \frac{1}{3} g_Y (\mathcal{C}_{qu}^{(1)})^{ttsr} (\bar{u}_s \gamma^\mu u_r) \partial^2 B_\mu - \frac{2}{3} g_Y (\mathcal{C}_{qu}^{(1)})^{srtt} (\bar{q}_s \bar{\mathcal{B}} \partial^2 q_r)
\end{aligned}$$

$$\begin{aligned}
& -\frac{2i}{3}g_L\bar{y}_u^{tu}(\mathcal{C}_{qu}^{(1)})^{trsu}\bar{\varepsilon}_{ij}t_k^{Ii}H^kW_{\bar{\mu}}^I(\bar{u}_s\partial^{\bar{\mu}}q_r^j)+\frac{13}{18}g_Y^2\bar{y}_u^{tu}(\mathcal{C}_{qu}^{(1)})^{trsu}B_{\bar{\mu}}^2(\bar{u}_s\tilde{H}^\dagger q_r) \\
& -\frac{2}{3}g_Y(\mathcal{C}_{qu}^{(1)})^{srtt}(\partial^2\bar{q}_s\bar{\mathcal{B}}q_r)+\frac{2i}{3}g_Ly_u^{tu}(\mathcal{C}_{qu}^{(1)})^{stur}\varepsilon^{jk}t_j^{Ii}H_i^\dagger W_{\bar{\mu}}^I(\partial^{\bar{\mu}}\bar{q}_{ks}u_r) \\
& -\frac{2i}{3}g_L\bar{y}_u^{tu}(\mathcal{C}_{qu}^{(1)})^{trsu}\bar{\varepsilon}_{ij}t_k^{Ii}H^kW_{\bar{\mu}}^I(\partial^{\bar{\mu}}\bar{u}_sq_r^j)-\frac{2}{3}g_Y(\mathcal{C}_{qu}^{(1)})^{ttsr}(\partial^{\bar{\nu}}\bar{u}_s\bar{\mathcal{B}}\partial^{\bar{\nu}}u_r) \\
& -\frac{2}{3}g_Y(\mathcal{C}_{qu}^{(1)})^{srtt}(\bar{q}_s\gamma^{\bar{\mu}}q_r)\partial^2B_{\bar{\mu}}-\frac{2i}{3}g_Ly_u^{tu}(\mathcal{C}_{qu}^{(1)})^{stur}\varepsilon^{ij}t_i^{Ik}W_{\bar{\mu}}^I(\bar{q}_{js}u_r)\partial^{\bar{\mu}}H_k^\dagger \\
& +\frac{2i}{3}g_L\bar{y}_u^{tu}(\mathcal{C}_{qu}^{(1)})^{trsu}\bar{\varepsilon}_{ij}t_k^{Ii}W_{\bar{\mu}}^I(\bar{u}_sq_r^j)\partial^{\bar{\mu}}H^k-g_Ly_u^{tv}\bar{y}_u^{tu}(\mathcal{C}_{qu}^{(1)})^{srvu}(H^\dagger t^IH)(\bar{q}_s\bar{W}^Iq_r) \\
& -g_Yy_d^{vu}\bar{y}_d^{tu}(\mathcal{C}_{qu}^{(1)})^{tvsr}(H^\dagger H)(\bar{u}_s\bar{\mathcal{B}}u_r)-\frac{4}{3}g_s^2(\mathcal{C}_{qu}^{(1)})^{ttsr}G_{\bar{\mu}}^A\tilde{G}^{\bar{\mu}\bar{\sigma}A}(\bar{u}_s\gamma^{\bar{\sigma}}u_r) \\
& -\frac{4}{3}g_Y(\mathcal{C}_{qu}^{(1)})^{srtt}(\partial^{\bar{\nu}}\bar{q}_s\bar{\mathcal{B}}\partial^{\bar{\nu}}q_r)-2g_Lg_sy_u^{tu}(\mathcal{C}_{qu}^{(1)})^{stur}t_j^{Ik}T_b^{Aa}\tilde{H}_jG_{\bar{\mu}}^AW_{\bar{\mu}}^I(\bar{q}_{aks}u_r^b) \\
& -2g_L^2(\mathcal{C}_{qu}^{(1)})^{ttsr}W_{\bar{\mu}}^I\tilde{W}^{\bar{\mu}\bar{\sigma}I}(\bar{u}_s\gamma^{\bar{\sigma}}u_r)-2g_Lg_s\bar{y}_u^{tu}(\mathcal{C}_{qu}^{(1)})^{trsu}t_k^{Ii}T_b^{Aa}\tilde{H}^{\dagger i}G_{\bar{\mu}}^AW_{\bar{\mu}}^I(\bar{u}_{as}q_r^{bk}) \\
& -\frac{5}{2}g_Yy_u^{tv}\bar{y}_u^{tu}(\mathcal{C}_{qu}^{(1)})^{srvu}(H^\dagger H)(\bar{q}_s\bar{\mathcal{B}}q_r), \tag{2.53}
\end{aligned}$$

$$\begin{aligned}
\Delta S_{\mathcal{O}_{qu}^{(8)}} &= \frac{1}{108}g_s g_Y^2(\mathcal{C}_{qu}^{(8)})^{ttsr}B_{\bar{\mu}}^2(\bar{u}_sT^A\bar{\mathcal{G}}^A u_r)+\frac{1}{72}g_s^3(\mathcal{C}_{qu}^{(8)})^{srtt}f^{ABC}G_{\bar{\mu}}^AG_{\bar{\nu}}^BG_{\bar{\rho}}^C\varepsilon^{\bar{\mu}\bar{\nu}\bar{\rho}\bar{\sigma}}(\bar{q}_s\gamma^{\bar{\sigma}}q_r) \\
& +\frac{1}{54}g_s g_Y^2(\mathcal{C}_{qu}^{(8)})^{ttsr}B_{\bar{\mu}}G_{\bar{\mu}}^A(\bar{u}_sT^A\bar{\mathcal{B}}u_r)-\frac{i}{18}g_s^2g_Y(\mathcal{C}_{qu}^{(8)})^{ttsr}T_b^{Aa}T_a^{Bc}B_{\bar{\mu}}G_{\bar{\nu}}^BG_{\bar{\rho}}^A\varepsilon^{\bar{\mu}\bar{\nu}\bar{\rho}\bar{\sigma}}(\bar{u}_{cs}\gamma^{\bar{\sigma}}u_r^b) \\
& +\frac{1}{18}g_s^2g_Y(\mathcal{C}_{qu}^{(8)})^{ttsr}T_b^{Aa}T_a^{Bc}G_{\bar{\nu}}^AG_{\bar{\nu}}^B(\bar{u}_{cs}\bar{\mathcal{B}}u_r^b) \\
& +\frac{1}{18}(\mathcal{C}_{qu}^{(8)})^{ttsr}\left[g_s^2g_YT_b^{Aa}T_c^{Bb}B_{\bar{\mu}}G_{\bar{\mu}}^B(\bar{u}_{as}\bar{\mathcal{G}}^A u_r^c)+g_s^2g_YT_b^{Aa}T_a^{Bc}B_{\bar{\mu}}G_{\bar{\mu}}^B(\bar{u}_{cs}\bar{\mathcal{G}}^A u_r^b)\right] \\
& +\frac{2}{27}g_s g_Y^2(\mathcal{C}_{qu}^{(8)})^{srtt}B_{\bar{\mu}}^2(\bar{q}_sT^A\bar{\mathcal{G}}^A q_r)+\frac{1}{12}g_L^2g_s(\mathcal{C}_{qu}^{(8)})^{ttsr}W_{\bar{\mu}}^{I2}(\bar{u}_sT^A\bar{\mathcal{G}}^A u_r) \\
& -\frac{i}{12}(\mathcal{C}_{qu}^{(8)})^{srtt}\left[g_s^2T_b^{Aa}T_c^{Bb}G_{\bar{\mu}}^B(\bar{q}_{as}\gamma^{\bar{\nu}}q_r^c)\partial^{\bar{\mu}}G_{\bar{\nu}}^A-g_s^2T_b^{Aa}T_a^{Bc}G_{\bar{\mu}}^B(\bar{q}_{cs}\gamma^{\bar{\nu}}q_r^b)\partial^{\bar{\mu}}G_{\bar{\nu}}^A\right] \\
& -\frac{i}{12}(\mathcal{C}_{qu}^{(8)})^{srtt}\left[g_s^2T_b^{Aa}T_c^{Bb}(\bar{q}_{as}\bar{\mathcal{G}}^B q_r^c)\partial^{\bar{\nu}}G_{\bar{\nu}}^A-g_s^2T_b^{Aa}T_a^{Bc}(\bar{q}_{cs}\bar{\mathcal{G}}^B q_r^b)\partial^{\bar{\nu}}G_{\bar{\nu}}^A\right] \\
& +\frac{i}{9}g_s^2g_Y(\mathcal{C}_{qu}^{(8)})^{srtt}T_b^{Aa}T_a^{Bc}B_{\bar{\mu}}G_{\bar{\nu}}^BG_{\bar{\rho}}^A\varepsilon^{\bar{\mu}\bar{\nu}\bar{\rho}\bar{\sigma}}(\bar{q}_{cs}\gamma^{\bar{\sigma}}q_r^b) \\
& +\frac{1}{9}g_s^2g_Y(\mathcal{C}_{qu}^{(8)})^{srtt}T_b^{Aa}T_a^{Bc}G_{\bar{\nu}}^AG_{\bar{\nu}}^B(\bar{q}_{cs}\bar{\mathcal{B}}q_r^b) \\
& +\frac{1}{9}(\mathcal{C}_{qu}^{(8)})^{srtt}\left[g_s^2g_YT_b^{Aa}T_c^{Bb}B_{\bar{\mu}}G_{\bar{\mu}}^B(\bar{q}_{as}\bar{\mathcal{G}}^A q_r^c)+g_s^2g_YT_b^{Aa}T_a^{Bc}B_{\bar{\mu}}G_{\bar{\mu}}^B(\bar{q}_{cs}\bar{\mathcal{G}}^A q_r^b)\right] \\
& +\frac{4}{27}g_s g_Y^2(\mathcal{C}_{qu}^{(8)})^{srtt}B_{\bar{\mu}}G_{\bar{\mu}}^A(\bar{q}_sT^A\bar{\mathcal{B}}q_r) \\
& +\frac{1}{6}g_s(\mathcal{C}_{qu}^{(8)})^{srtt}\left[2g_sT_b^{Aa}T_c^{Bb}G_{\bar{\mu}}^B\tilde{G}^{\bar{\mu}\bar{\sigma}A}(\bar{q}_{as}\gamma^{\bar{\sigma}}q_r^c)+2g_sT_b^{Aa}T_a^{Bc}G_{\bar{\mu}}^B\tilde{G}^{\bar{\mu}\bar{\sigma}A}(\bar{q}_{cs}\gamma^{\bar{\sigma}}q_r^b)\right] \\
& +\frac{i}{6}g_s^3(\mathcal{C}_{qu}^{(8)})^{srtt}T_b^{Aa}T_a^{Bc}T_c^{Cd}G_{\bar{\mu}}^AG_{\bar{\nu}}^CG_{\bar{\rho}}^B\varepsilon^{\bar{\mu}\bar{\nu}\bar{\rho}\bar{\sigma}}(\bar{q}_{ds}\gamma^{\bar{\sigma}}q_r^b) \\
& +\frac{1}{6}(\mathcal{C}_{qu}^{(8)})^{srtt}\left[g_s^3T_b^{Aa}T_c^{Bb}T_d^{Cd}G_{\bar{\mu}}^BG_{\bar{\mu}}^C(\bar{q}_{as}\bar{\mathcal{G}}^A q_r^d)+g_s^3T_b^{Aa}T_a^{Bc}T_c^{Cd}G_{\bar{\mu}}^BG_{\bar{\mu}}^C(\bar{q}_{ds}\bar{\mathcal{G}}^A q_r^b)\right]
\end{aligned}$$

$$\begin{aligned}
& + \frac{1}{6} g_L^2 g_s (\mathcal{C}_{qu}^{(8)})^{ttsr} G_{\bar{\mu}}^A W_{\bar{\mu}}^I (\bar{u}_s T^A \bar{W}^I u_r) + \frac{2}{9} g_s^2 (\mathcal{C}_{qu}^{(8)})^{ttsr} G_{\bar{\mu}}^A \tilde{G}^{\bar{\mu}\bar{\sigma}A} (\bar{u}_s \gamma^{\bar{\sigma}} u_r) \\
& + \frac{1}{3} g_L g_s y_u^{tu} (\mathcal{C}_{qu}^{(8)})^{stur} t_j^{Ik} T_b^{Aa} \tilde{H}_j G_{\bar{\mu}}^A W_{\bar{\mu}}^I (\bar{q}_{aks} u_r^b) + \frac{1}{3} g_L g_s \bar{y}_u^{tu} (\mathcal{C}_{qu}^{(8)})^{trsu} t_k^{Ii} T_b^{Aa} \tilde{H}^{\dagger i} G_{\bar{\mu}}^A W_{\bar{\mu}}^I (\bar{u}_{as} q_r^{bk}) \\
& + \frac{4}{9} g_L^2 y_u^{tu} (\mathcal{C}_{qu}^{(8)})^{stur} W_{\bar{\mu}}^{I2} (\bar{q}_s \tilde{H} u_r) + \frac{4}{9} g_s g_Y (\mathcal{C}_{qu}^{(8)})^{srtt} G_{\bar{\mu}}^A \tilde{B}^{\bar{\mu}\bar{\sigma}} (\bar{q}_s T^A \gamma^{\bar{\sigma}} q_r) \\
& + \frac{4}{9} g_s g_Y (\mathcal{C}_{qu}^{(8)})^{srtt} B_{\bar{\mu}} \tilde{G}^{\bar{\mu}\bar{\sigma}A} (\bar{q}_s T^A \gamma^{\bar{\sigma}} q_r) + \frac{4}{9} g_L^2 \bar{y}_u^{tu} (\mathcal{C}_{qu}^{(8)})^{trsu} W_{\bar{\mu}}^{I2} (\bar{u}_s \tilde{H}^{\dagger} q_r) \\
& + \frac{1}{2} g_s^2 y_u^{tu} (\mathcal{C}_{qu}^{(8)})^{stur} G_{\bar{\mu}}^{A2} (\bar{q}_s \tilde{H} u_r) + \frac{1}{2} g_s^2 \bar{y}_u^{tu} (\mathcal{C}_{qu}^{(8)})^{trsu} G_{\bar{\mu}}^{A2} (\bar{u}_s \tilde{H}^{\dagger} q_r) \\
& + \frac{8}{9} g_L^2 y_u^{tu} (\mathcal{C}_{qu}^{(8)})^{stur} \varepsilon^{jk} t_l^{Ii} t_j^{Il} H_i^{\dagger} W_{\bar{\mu}}^I W_{\bar{\mu}}^J (\bar{q}_{ks} u_r) + \frac{8}{9} g_L g_Y y_u^{tu} (\mathcal{C}_{qu}^{(8)})^{stur} t_j^{Ik} \tilde{H}_j B_{\bar{\mu}} W_{\bar{\mu}}^I (\bar{q}_{ks} u_r) \\
& + \frac{8}{9} g_L^2 \bar{y}_u^{tu} (\mathcal{C}_{qu}^{(8)})^{trsu} \bar{\varepsilon}_{ij} t_l^{Ik} t_k^{Ji} H^l W_{\bar{\mu}}^I W_{\bar{\mu}}^J (\bar{u}_{s} q_r^j) + \frac{8}{9} g_L g_Y \bar{y}_u^{tu} (\mathcal{C}_{qu}^{(8)})^{trsu} t_k^{Ii} \tilde{H}^{\dagger i} B_{\bar{\mu}} W_{\bar{\mu}}^I (\bar{u}_s q_r^k) \\
& + \frac{26}{27} g_Y^2 y_u^{tu} (\mathcal{C}_{qu}^{(8)})^{stur} B_{\bar{\mu}}^2 (\bar{q}_s \tilde{H} u_r) - \frac{1}{108} g_s^2 g_Y (\mathcal{C}_{qu}^{(8)})^{ttsr} G_{\bar{\mu}}^{A2} (\bar{u}_s \bar{B} u_r) - \frac{1}{72} g_s^3 (\mathcal{C}_{qu}^{(8)})^{srtt} d^{ABC} G_{\bar{\nu}}^B G_{\bar{\nu}}^C (\bar{q}_s \bar{G}^A q_r) \\
& - \frac{1}{54} g_s^2 g_Y (\mathcal{C}_{qu}^{(8)})^{srtt} G_{\bar{\mu}}^{A2} (\bar{q}_s \bar{B} q_r) - \frac{1}{54} g_s^2 g_Y (\mathcal{C}_{qu}^{(8)})^{ttsr} B_{\bar{\mu}} G_{\bar{\mu}}^A (\bar{u}_s \bar{G}^A u_r) \\
& - \frac{1}{36} g_s^3 (\mathcal{C}_{qu}^{(8)})^{ttsr} f^{ABC} G_{\bar{\mu}}^A G_{\bar{\nu}}^B G_{\bar{\rho}}^C \varepsilon^{\bar{\mu}\bar{\nu}\bar{\rho}\bar{\sigma}} (\bar{u}_s \gamma^{\bar{\sigma}} u_r) - \frac{1}{36} g_s^3 (\mathcal{C}_{qu}^{(8)})^{ttsr} d^{ABC} G_{\bar{\nu}}^B G_{\bar{\nu}}^C (\bar{u}_s \bar{G}^A u_r) \\
& - \frac{1}{27} g_s^2 g_Y (\mathcal{C}_{qu}^{(8)})^{srtt} B_{\bar{\mu}} G_{\bar{\mu}}^A (\bar{q}_s \bar{G}^A q_r) - \frac{1}{9} g_s^2 (\mathcal{C}_{qu}^{(8)})^{srtt} G_{\bar{\mu}}^A \tilde{G}^{\bar{\mu}\bar{\sigma}A} (\bar{q}_s \gamma^{\bar{\sigma}} q_r) \\
& - \frac{1}{6} g_s (\mathcal{C}_{qu}^{(8)})^{srtt} (\bar{q}_s T^A \bar{G}^A \partial^2 q_r) - \frac{1}{6} g_s^3 (\mathcal{C}_{qu}^{(8)})^{srtt} T_b^{Aa} T_a^{Bc} T_c^{Cd} G_{\bar{\mu}}^A G_{\bar{\mu}}^C (\bar{q}_{ds} \bar{G}^B q_r^b) \\
& - \frac{1}{6} g_s (\mathcal{C}_{qu}^{(8)})^{srtt} (\partial^2 \bar{q}_s T^A \bar{G}^A q_r) - \frac{1}{6} g_s (\mathcal{C}_{qu}^{(8)})^{srtt} (\bar{q}_s T^A \gamma^{\bar{\mu}} q_r) \partial^2 G_{\bar{\mu}}^A \\
& - \frac{i}{6} (\mathcal{C}_{qu}^{(8)})^{ttsr} \left[ g_s^2 T_b^{Aa} T_c^{Bb} G_{\bar{\mu}}^B (\bar{u}_{as} \gamma^{\bar{\nu}} u_r^c) \partial^{\bar{\mu}} G_{\bar{\nu}}^A - g_s^2 T_b^{Aa} T_a^{Bc} G_{\bar{\mu}}^B (\bar{u}_{cs} \gamma^{\bar{\nu}} u_r^b) \partial^{\bar{\mu}} G_{\bar{\nu}}^A \right] \\
& - \frac{i}{6} (\mathcal{C}_{qu}^{(8)})^{ttsr} \left[ g_s^2 T_b^{Aa} T_c^{Bb} (\bar{u}_{as} \bar{G}^B u_r^c) \partial^{\bar{\nu}} G_{\bar{\nu}}^A - g_s^2 T_b^{Aa} T_a^{Bc} (\bar{u}_{cs} \bar{G}^B u_r^b) \partial^{\bar{\nu}} G_{\bar{\nu}}^A \right] \\
& - \frac{2}{9} g_s g_Y (\mathcal{C}_{qu}^{(8)})^{ttsr} G_{\bar{\mu}}^A \tilde{B}^{\bar{\mu}\bar{\sigma}} (\bar{u}_s T^A \gamma^{\bar{\sigma}} u_r) - \frac{2}{9} g_s g_Y (\mathcal{C}_{qu}^{(8)})^{ttsr} B_{\bar{\mu}} \tilde{G}^{\bar{\mu}\bar{\sigma}A} (\bar{u}_s T^A \gamma^{\bar{\sigma}} u_r) \\
& - \frac{5}{18} g_s g_Y y_u^{tu} (\mathcal{C}_{qu}^{(8)})^{stur} T_b^{Aa} B_{\bar{\mu}} G_{\bar{\mu}}^A (\bar{q}_{as} \tilde{H} u_r^b) - \frac{5}{18} g_s g_Y \bar{y}_u^{tu} (\mathcal{C}_{qu}^{(8)})^{trsu} T_b^{Aa} B_{\bar{\mu}} G_{\bar{\mu}}^A (\bar{u}_{as} \tilde{H}^{\dagger} q_r^b) \\
& - \frac{1}{3} g_s^2 y_u^{tu} (\mathcal{C}_{qu}^{(8)})^{stur} T_b^{Aa} T_a^{Bc} G_{\bar{\mu}}^A G_{\bar{\mu}}^B (\bar{q}_{cs} \tilde{H} u_r^b) - \frac{1}{3} g_s (\mathcal{C}_{qu}^{(8)})^{ttsr} (\bar{u}_s T^A \bar{G}^A \partial^2 u_r) \\
& - \frac{1}{3} g_s^2 \bar{y}_u^{tu} (\mathcal{C}_{qu}^{(8)})^{trsu} T_b^{Aa} T_c^{Bb} G_{\bar{\mu}}^A G_{\bar{\mu}}^B (\bar{u}_{as} \tilde{H}^{\dagger} q_r^c) \\
& - \frac{1}{3} g_s (\mathcal{C}_{qu}^{(8)})^{ttsr} \left[ 2g_s T_b^{Aa} T_c^{Bb} G_{\bar{\mu}}^B \tilde{G}^{\bar{\mu}\bar{\sigma}A} (\bar{u}_{as} \gamma^{\bar{\sigma}} u_r^c) + 2g_s T_b^{Aa} T_a^{Bc} G_{\bar{\mu}}^B \tilde{G}^{\bar{\mu}\bar{\sigma}A} (\bar{u}_{cs} \gamma^{\bar{\sigma}} u_r^b) \right] \\
& - \frac{i}{3} g_s^3 (\mathcal{C}_{qu}^{(8)})^{ttsr} T_b^{Aa} T_a^{Bc} T_c^{Cd} G_{\bar{\mu}}^A G_{\bar{\nu}}^C G_{\bar{\rho}}^B \varepsilon^{\bar{\mu}\bar{\nu}\bar{\rho}\bar{\sigma}} (\bar{u}_{ds} \gamma^{\bar{\sigma}} u_r^b) \\
& + \frac{1}{3} (\mathcal{C}_{qu}^{(8)})^{ttsr} \left[ g_s^3 T_b^{Aa} T_c^{Bb} T_d^{Cd} G_{\bar{\mu}}^B G_{\bar{\mu}}^C (\bar{u}_{as} \bar{G}^A u_r^d) + g_s^3 T_b^{Aa} T_a^{Bc} T_c^{Cd} G_{\bar{\mu}}^B G_{\bar{\mu}}^C (\bar{u}_{ds} \bar{G}^A u_r^b) \right] \\
& - \frac{1}{3} g_s^3 (\mathcal{C}_{qu}^{(8)})^{ttsr} T_b^{Aa} T_a^{Bc} T_c^{Cd} G_{\bar{\mu}}^A G_{\bar{\mu}}^C (\bar{u}_{ds} \bar{G}^B u_r^b) - \frac{1}{3} g_s (\mathcal{C}_{qu}^{(8)})^{ttsr} (\partial^2 \bar{u}_s T^A \bar{G}^A u_r)
\end{aligned}$$

$$\begin{aligned}
& -\frac{1}{3}g_s(\mathcal{C}_{qu}^{(8)})^{srtt}(\partial^{\bar{\nu}}\bar{q}_s T^A \bar{\mathcal{G}}^A \partial^{\bar{\nu}} q_r) - \frac{1}{3}g_s(\mathcal{C}_{qu}^{(8)})^{ttsr}(\bar{u}_s T^A \gamma^{\bar{\mu}} u_r) \partial^2 G_{\bar{\mu}}^A \\
& -\frac{5i}{12}(\mathcal{C}_{qu}^{(8)})^{srtt} \left[ g_s^2 T_b^{Aa} T_a^{Bc} G_{\bar{\nu}}^B (\bar{q}_{cs} \bar{\mathcal{G}}^A \partial^{\bar{\nu}} q_r^b) - g_s^2 T_b^{Aa} T_c^{Bb} G_{\bar{\nu}}^B (\partial^{\bar{\nu}} \bar{q}_{as} \bar{\mathcal{G}}^A q_r^c) \right] \\
& -\frac{5i}{12}(\mathcal{C}_{qu}^{(8)})^{srtt} \left[ g_s^2 T_b^{Aa} T_c^{Bb} G_{\bar{\nu}}^A (\partial^{\bar{\nu}} \bar{q}_{as} \bar{\mathcal{G}}^B q_r^c) - g_s^2 T_b^{Aa} T_a^{Bc} G_{\bar{\nu}}^A (\bar{q}_{cs} \bar{\mathcal{G}}^B \partial^{\bar{\nu}} q_r^b) \right] \\
& +\frac{4i}{9}g_Y y_u^{tu}(\mathcal{C}_{qu}^{(8)})^{stur} B_{\bar{\mu}}(\bar{q}_s \tilde{H} \partial^{\bar{\mu}} u_r) + \frac{4i}{9}g_Y y_u^{tu}(\mathcal{C}_{qu}^{(8)})^{stur} B_{\bar{\mu}}(\bar{q}_s \partial^{\bar{\mu}} \tilde{H} u_r) \\
& -\frac{4i}{9}g_Y \bar{y}_u^{tu}(\mathcal{C}_{qu}^{(8)})^{trsu} B_{\bar{\mu}}(\bar{u}_s \tilde{H}^\dagger \partial^{\bar{\mu}} q_r) - \frac{4i}{9}g_Y \bar{y}_u^{tu}(\mathcal{C}_{qu}^{(8)})^{trsu} B_{\bar{\mu}}(\bar{u}_s \partial^{\bar{\mu}} \tilde{H} q_r) \\
& +\frac{4i}{9}g_Y y_u^{tu}(\mathcal{C}_{qu}^{(8)})^{stur} B_{\bar{\mu}}(\partial^{\bar{\mu}} \bar{q}_s \tilde{H} u_r) - \frac{4i}{9}g_Y \bar{y}_u^{tu}(\mathcal{C}_{qu}^{(8)})^{trsu} B_{\bar{\mu}}(\partial^{\bar{\mu}} \bar{u}_s \tilde{H}^\dagger q_r) \\
& -\frac{1}{2}g_s y_u^{tv} \bar{y}_u^{tu}(\mathcal{C}_{qu}^{(8)})^{srvu} (H^\dagger H) (\bar{q}_s T^A \bar{\mathcal{G}}^A q_r) \\
& -\frac{i}{2}g_s(\mathcal{C}_{qu}^{(8)})^{srtt} \left[ g_s T_b^{Aa} T_c^{Bb} G_{\bar{\mu}}^B G^{\bar{\mu}\bar{\nu}A} (\bar{q}_{as} \gamma^{\bar{\nu}} q_r^c) - g_s T_b^{Aa} T_a^{Bc} G_{\bar{\mu}}^B G^{\bar{\mu}\bar{\nu}A} (\bar{q}_{cs} \gamma^{\bar{\nu}} q_r^b) \right] \\
& -\frac{1}{2}g_s(\mathcal{C}_{qu}^{(8)})^{tvsr} \left[ y_d^{vu} \bar{y}_d^{tu} + y_u^{vu} \bar{y}_u^{tu} \right] (H^\dagger H) (\bar{u}_s T^A \bar{\mathcal{G}}^A u_r) - \frac{2}{3}g_s(\mathcal{C}_{qu}^{(8)})^{ttsr} (\partial^{\bar{\nu}} \bar{u}_s T^A \bar{\mathcal{G}}^A \partial^{\bar{\nu}} u_r) \\
& -\frac{5i}{6}(\mathcal{C}_{qu}^{(8)})^{ttsr} \left[ g_s^2 T_b^{Aa} T_a^{Bc} G_{\bar{\nu}}^B (\bar{u}_{cs} \bar{\mathcal{G}}^A \partial^{\bar{\nu}} u_r^b) - g_s^2 T_b^{Aa} T_c^{Bb} G_{\bar{\nu}}^B (\partial^{\bar{\nu}} \bar{u}_{as} \bar{\mathcal{G}}^A u_r^c) \right] \\
& -\frac{5i}{6}(\mathcal{C}_{qu}^{(8)})^{ttsr} \left[ g_s^2 T_b^{Aa} T_c^{Bb} G_{\bar{\nu}}^A (\partial^{\bar{\nu}} \bar{u}_{as} \bar{\mathcal{G}}^B u_r^c) - g_s^2 T_b^{Aa} T_a^{Bc} G_{\bar{\nu}}^A (\bar{u}_{cs} \bar{\mathcal{G}}^B \partial^{\bar{\nu}} u_r^b) \right] \\
& +\frac{8i}{9}g_L y_u^{tu}(\mathcal{C}_{qu}^{(8)})^{stur} \varepsilon^{jk} t_j^{Ii} H_i^\dagger W_{\bar{\mu}}^I (\bar{q}_{ks} \partial^{\bar{\mu}} u_r) - \frac{8i}{9}g_L \bar{y}_u^{tu}(\mathcal{C}_{qu}^{(8)})^{trsu} \bar{\varepsilon}_{ij} t_k^{Ii} H^k W_{\bar{\mu}}^I (\bar{u}_s \partial^{\bar{\mu}} q_r^j) \\
& +\frac{8i}{9}g_L y_u^{tu}(\mathcal{C}_{qu}^{(8)})^{stur} \varepsilon^{jk} t_j^{Ii} H_i^\dagger W_{\bar{\mu}}^I (\partial^{\bar{\mu}} \bar{q}_{ks} u_r) - \frac{8i}{9}g_L \bar{y}_u^{tu}(\mathcal{C}_{qu}^{(8)})^{trsu} \bar{\varepsilon}_{ij} t_k^{Ii} H^k W_{\bar{\mu}}^I (\partial^{\bar{\mu}} \bar{u}_s q_r^j) \\
& -\frac{8i}{9}g_L y_u^{tu}(\mathcal{C}_{qu}^{(8)})^{stur} \varepsilon^{ij} t_i^{Ik} W_{\bar{\mu}}^I (\bar{q}_{js} u_r) \partial^{\bar{\mu}} H_k^\dagger + \frac{8i}{9}g_L \bar{y}_u^{tu}(\mathcal{C}_{qu}^{(8)})^{trsu} \bar{\varepsilon}_{ij} t_k^{Ii} W_{\bar{\mu}}^I (\bar{u}_s q_r^j) \partial^{\bar{\mu}} H^k \\
& +\frac{26}{27}g_Y^2 \bar{y}_u^{tu}(\mathcal{C}_{qu}^{(8)})^{trsu} B_{\bar{\mu}}^2 (\bar{u}_s \tilde{H}^\dagger q_r) \\
& -ig_s(\mathcal{C}_{qu}^{(8)})^{ttsr} \left[ g_s T_b^{Aa} T_c^{Bb} G_{\bar{\mu}}^B G^{\bar{\mu}\bar{\nu}A} (\bar{u}_{as} \gamma^{\bar{\nu}} u_r^c) - g_s T_b^{Aa} T_a^{Bc} G_{\bar{\mu}}^B G^{\bar{\mu}\bar{\nu}A} (\bar{u}_{cs} \gamma^{\bar{\nu}} u_r^b) \right], \tag{2.54}
\end{aligned}$$

$$\begin{aligned}
\Delta S_{\mathcal{O}_{qd}^{(1)}} &= \frac{1}{108}g_Y^3(\mathcal{C}_{qd}^{(1)})^{ttsr} B_{\bar{\mu}}^2(\bar{d}_s \bar{\mathcal{B}} d_r) + \frac{1}{18}g_s^2 g_Y(\mathcal{C}_{qd}^{(1)})^{ttsr} G_{\bar{\mu}}^{A2}(\bar{d}_s \bar{\mathcal{B}} d_r) + \frac{1}{12}g_L^2 g_Y(\mathcal{C}_{qd}^{(1)})^{ttsr} W_{\bar{\mu}}^{I2}(\bar{d}_s \bar{\mathcal{B}} d_r) \\
&+ \frac{1}{12}g_s^3(\mathcal{C}_{qd}^{(1)})^{srtt} d^{ABC} G_{\bar{\nu}}^B G_{\bar{\nu}}^C (\bar{q}_s \bar{\mathcal{G}}^A q_r) + \frac{1}{9}g_s^2 g_Y(\mathcal{C}_{qd}^{(1)})^{ttsr} B_{\bar{\mu}} G_{\bar{\mu}}^A (\bar{d}_s \bar{\mathcal{G}}^A d_r) \\
&+ \frac{1}{6}g_s^3(\mathcal{C}_{qd}^{(1)})^{ttsr} f^{ABC} G_{\bar{\mu}}^A G_{\bar{\nu}}^B G_{\bar{\rho}}^C \varepsilon^{\bar{\mu}\bar{\nu}\bar{\rho}\bar{\sigma}} (\bar{d}_s \gamma^{\bar{\sigma}} d_r) + \frac{1}{6}g_s^3(\mathcal{C}_{qd}^{(1)})^{ttsr} d^{ABC} G_{\bar{\nu}}^B G_{\bar{\nu}}^C (\bar{d}_s \bar{\mathcal{G}}^A d_r) \\
&+ \frac{1}{6}g_L^2 g_Y(\mathcal{C}_{qd}^{(1)})^{ttsr} B_{\bar{\mu}} W_{\bar{\mu}}^I (\bar{d}_s \bar{W}^I d_r) + \frac{1}{4}g_L^3(\mathcal{C}_{qd}^{(1)})^{ttsr} \varepsilon^{IJK} W_{\bar{\mu}}^I W_{\bar{\nu}}^J W_{\bar{\rho}}^K \varepsilon^{\bar{\mu}\bar{\nu}\bar{\rho}\bar{\sigma}} (\bar{d}_s \gamma^{\bar{\sigma}} d_r) \\
&+ \frac{1}{3}g_s g_Y \bar{y}_d^{tu}(\mathcal{C}_{qd}^{(1)})^{trsu} T_b^{Aa} B_{\bar{\mu}} G_{\bar{\mu}}^A (\bar{d}_{as} H^\dagger q_r^b) + \frac{i}{3}g_Y y_d^{tu}(\mathcal{C}_{qd}^{(1)})^{stur} B_{\bar{\mu}}(\bar{q}_s H \partial^{\bar{\mu}} d_r) - \frac{i}{3}g_Y y_d^{tu}(\mathcal{C}_{qd}^{(1)})^{stur} B_{\bar{\mu}}(\bar{q}_s \partial^{\bar{\mu}} H d_r) \\
&+ \frac{1}{3}g_Y(\mathcal{C}_{qd}^{(1)})^{srtt} (\bar{q}_s \bar{\mathcal{B}} \partial^2 q_r) + \frac{1}{3}g_s g_Y y_d^{tu}(\mathcal{C}_{qd}^{(1)})^{stur} T_b^{Aa} B_{\bar{\mu}} G_{\bar{\mu}}^A (\bar{q}_{as} H d_r^b) + \frac{1}{3}g_Y(\mathcal{C}_{qd}^{(1)})^{srtt} (\partial^2 \bar{q}_s \bar{\mathcal{B}} q_r) \\
&+ \frac{1}{3}g_Y(\mathcal{C}_{qd}^{(1)})^{srtt} (\bar{q}_s \gamma^{\bar{\mu}} q_r) \partial^2 B_{\bar{\mu}} + \frac{4}{9}g_Y^2(\mathcal{C}_{qd}^{(1)})^{srtt} B_{\bar{\mu}} \tilde{B}^{\bar{\mu}\bar{\sigma}} (\bar{q}_s \gamma^{\bar{\sigma}} q_r)
\end{aligned}$$

$$\begin{aligned}
& + \frac{2}{3} g_s^2 (\mathcal{C}_{qd}^{(1)})^{srtt} G_{\bar{\mu}}^A \tilde{G}^{\bar{\mu}\bar{\sigma} A} (\bar{q}_s \gamma^{\bar{\sigma}} q_r) + \frac{3}{2} g_Y y_d^{tv} \bar{y}_d^{tu} (\mathcal{C}_{qd}^{(1)})^{srvu} (H^\dagger H) (\bar{q}_s \bar{\mathcal{B}} q_r) \\
& + 4 g_L (\mathcal{C}_{qd}^{(1)})^{tvsr} \left[ y_u^{vu} \bar{y}_u^{tu} - y_u^{vu} \bar{y}_d^{tu} \right] (H^\dagger t^I H) (\bar{d}_s \bar{\mathcal{W}}^I d_r) - \frac{1}{27} g_Y^3 (\mathcal{C}_{qd}^{(1)})^{srtt} B_{\bar{\mu}}^2 (\bar{q}_s \bar{\mathcal{B}} q_r) \\
& - \frac{1}{18} g_s^2 g_Y (\mathcal{C}_{qd}^{(1)})^{srtt} G_{\bar{\mu}}^A {}^2 (\bar{q}_s \bar{\mathcal{B}} q_r) - \frac{1}{12} g_s^3 (\mathcal{C}_{qd}^{(1)})^{srtt} f^{ABC} G_{\bar{\mu}}^A G_{\bar{\nu}}^B G_{\bar{\rho}}^C \varepsilon^{\bar{\mu}\bar{\nu}\bar{\rho}\bar{\sigma}} (\bar{q}_s \gamma^{\bar{\sigma}} q_r) \\
& - \frac{1}{9} g_s^2 g_Y (\mathcal{C}_{qd}^{(1)})^{srtt} B_{\bar{\mu}} G_{\bar{\mu}}^A (\bar{q}_s \bar{\mathcal{G}}^A q_r) - \frac{2}{9} g_Y^2 (\mathcal{C}_{qd}^{(1)})^{ttsr} B_{\bar{\mu}} \tilde{B}^{\bar{\mu}\bar{\sigma}} (\bar{d}_s \gamma^{\bar{\sigma}} d_r) \\
& - \frac{i}{3} g_Y \bar{y}_d^{tu} (\mathcal{C}_{qd}^{(1)})^{trsu} B_{\bar{\mu}} (\bar{d}_s H^\dagger \partial^{\bar{\mu}} q_r) + \frac{i}{3} g_Y \bar{y}_d^{tu} (\mathcal{C}_{qd}^{(1)})^{trsu} B_{\bar{\mu}} (\bar{d}_s \partial^{\bar{\mu}} H^\dagger q_r) - \frac{1}{3} g_Y (\mathcal{C}_{qd}^{(1)})^{ttsr} (\bar{d}_s \bar{\mathcal{B}} \partial^2 d_r) \\
& - \frac{1}{3} g_Y (\mathcal{C}_{qd}^{(1)})^{ttsr} (\partial^2 \bar{d}_s \bar{\mathcal{B}} d_r) - \frac{i}{3} g_Y \bar{y}_d^{tu} (\mathcal{C}_{qd}^{(1)})^{trsu} B_{\bar{\mu}} (\partial^{\bar{\mu}} \bar{d}_s H^\dagger q_r) + \frac{i}{3} g_Y y_d^{tu} (\mathcal{C}_{qd}^{(1)})^{stur} B_{\bar{\mu}} (\partial^{\bar{\mu}} \bar{q}_s H d_r) \\
& - \frac{1}{3} g_Y (\mathcal{C}_{qd}^{(1)})^{ttsr} (\bar{d}_s \gamma^{\bar{\mu}} d_r) \partial^2 B_{\bar{\mu}} - \frac{7}{18} g_Y^2 \bar{y}_d^{tu} (\mathcal{C}_{qd}^{(1)})^{trsu} B_{\bar{\mu}}^2 (\bar{d}_s H^\dagger q_r) - \frac{7}{18} g_Y^2 y_d^{tu} (\mathcal{C}_{qd}^{(1)})^{stur} B_{\bar{\mu}}^2 (\bar{q}_s H d_r) \\
& - \frac{1}{2} g_L \bar{y}_d^{tu} (\mathcal{C}_{qd}^{(1)})^{trsu} W_{\bar{\mu}}^I {}^2 (\bar{d}_s H^\dagger q_r) - \frac{1}{2} g_L y_d^{tu} (\mathcal{C}_{qd}^{(1)})^{stur} W_{\bar{\mu}}^I {}^2 (\bar{q}_s H d_r) - \frac{2i}{3} g_L \bar{y}_d^{tu} (\mathcal{C}_{qd}^{(1)})^{trsu} t_j^I H_i^\dagger W_{\bar{\mu}}^I (\bar{d}_s \partial^{\bar{\mu}} q_r^j) \\
& + \frac{2i}{3} g_L y_d^{tu} (\mathcal{C}_{qd}^{(1)})^{stur} t_j^I H^j W_{\bar{\mu}}^I (\bar{q}_{is} \partial^{\bar{\mu}} d_r) - \frac{2i}{3} g_L \bar{y}_d^{tu} (\mathcal{C}_{qd}^{(1)})^{trsu} t_j^I H_i^\dagger W_{\bar{\mu}}^I (\partial^{\bar{\mu}} \bar{d}_s q_r^j) \\
& + \frac{2i}{3} g_L y_d^{tu} (\mathcal{C}_{qd}^{(1)})^{stur} t_j^I H^j W_{\bar{\mu}}^I (\partial^{\bar{\mu}} \bar{q}_{is} d_r) + \frac{2}{3} g_Y (\mathcal{C}_{qd}^{(1)})^{srtt} (\partial^{\bar{\nu}} \bar{q}_s \bar{\mathcal{B}} \partial^{\bar{\nu}} q_r) \\
& + g_L y_d^{tv} \bar{y}_d^{tu} (\mathcal{C}_{qd}^{(1)})^{srvu} (H^\dagger t^I H) (\bar{q}_s \bar{\mathcal{W}}^I q_r) - \frac{2}{3} g_Y (\mathcal{C}_{qd}^{(1)})^{ttsr} (\partial^{\bar{\nu}} \bar{d}_s \bar{\mathcal{B}} \partial^{\bar{\nu}} d_r) \\
& + \frac{2i}{3} g_L \bar{y}_d^{tu} (\mathcal{C}_{qd}^{(1)})^{trsu} t_j^I W_{\bar{\mu}}^I (\bar{d}_s q_r^j) \partial^{\bar{\mu}} H_i^\dagger - \frac{2i}{3} g_L y_d^{tu} (\mathcal{C}_{qd}^{(1)})^{stur} t_j^I W_{\bar{\mu}}^I (\bar{q}_{is} d_r) \partial^{\bar{\mu}} H^j \\
& - g_Y y_d^{vu} \bar{y}_d^{tu} (\mathcal{C}_{qd}^{(1)})^{tvsr} (H^\dagger H) (\bar{d}_s \bar{\mathcal{B}} d_r) - \frac{4}{3} g_L g_Y \bar{y}_d^{tu} (\mathcal{C}_{qd}^{(1)})^{trsu} t_j^I H_i^\dagger B_{\bar{\mu}} W_{\bar{\mu}}^I (\bar{d}_s q_r^j) \\
& - \frac{4}{3} g_s^2 (\mathcal{C}_{qd}^{(1)})^{ttsr} G_{\bar{\mu}}^A \tilde{G}^{\bar{\mu}\bar{\sigma} A} (\bar{d}_s \gamma^{\bar{\sigma}} d_r) - \frac{4}{3} g_L g_Y y_d^{tu} (\mathcal{C}_{qd}^{(1)})^{stur} t_j^I H^j B_{\bar{\mu}} W_{\bar{\mu}}^I (\bar{q}_{is} d_r) \\
& - 2 g_L^2 (\mathcal{C}_{qd}^{(1)})^{ttsr} W_{\bar{\mu}}^I \tilde{W}^{\bar{\mu}\bar{\sigma} I} (\bar{d}_s \gamma^{\bar{\sigma}} d_r) - 2 g_L g_s \bar{y}_d^{tu} (\mathcal{C}_{qd}^{(1)})^{trsu} t_j^I T_b^{Aa} H_i^\dagger G_{\bar{\mu}}^A W_{\bar{\mu}}^I (\bar{d}_{as} q_r^{bj}) \\
& - 2 g_s^2 \bar{y}_d^{tu} (\mathcal{C}_{qd}^{(1)})^{trsu} T_b^{Aa} T_a^{Bc} G_{\bar{\mu}}^A G_{\bar{\mu}}^B (\bar{d}_{cs} H^\dagger q_r^b) - 2 g_s^2 y_d^{tu} (\mathcal{C}_{qd}^{(1)})^{stur} T_b^{Aa} T_c^{Bb} G_{\bar{\mu}}^A G_{\bar{\mu}}^B (\bar{q}_{as} H d_r^c) \\
& - 2 g_L g_s y_d^{tu} (\mathcal{C}_{qd}^{(1)})^{stur} t_j^I T_b^{Aa} H^j G_{\bar{\mu}}^A W_{\bar{\mu}}^I (\bar{q}_{ais} d_r^b), \tag{2.55}
\end{aligned}$$

$$\begin{aligned}
\Delta S_{\mathcal{O}_{qd}^{(8)}} &= \frac{1}{108} g_s g_Y^2 (\mathcal{C}_{qd}^{(8)})^{ttsr} B_{\bar{\mu}}^2 (\bar{d}_s T^A \bar{\mathcal{G}}^A d_r) + \frac{1}{108} g_s^2 g_Y (\mathcal{C}_{qd}^{(8)})^{srtt} G_{\bar{\mu}}^A {}^2 (\bar{q}_s \bar{\mathcal{B}} q_r) \\
& + \frac{1}{72} g_s^3 (\mathcal{C}_{qd}^{(8)})^{srtt} f^{ABC} G_{\bar{\mu}}^A G_{\bar{\nu}}^B G_{\bar{\rho}}^C \varepsilon^{\bar{\mu}\bar{\nu}\bar{\rho}\bar{\sigma}} (\bar{q}_s \gamma^{\bar{\sigma}} q_r) + \frac{1}{54} g_s g_Y^2 (\mathcal{C}_{qd}^{(8)})^{ttsr} B_{\bar{\mu}} G_{\bar{\mu}}^A (\bar{d}_s T^A \bar{\mathcal{B}} d_r) \\
& + \frac{1}{54} g_s^2 g_Y (\mathcal{C}_{qd}^{(8)})^{srtt} B_{\bar{\mu}} G_{\bar{\mu}}^A (\bar{q}_s \bar{\mathcal{G}}^A q_r) + \frac{1}{54} g_s g_Y^2 (\mathcal{C}_{qd}^{(8)})^{srtt} B_{\bar{\mu}}^2 (\bar{q}_s T^A \bar{\mathcal{G}}^A q_r) \\
& + \frac{1}{27} g_s g_Y^2 (\mathcal{C}_{qd}^{(8)})^{srtt} B_{\bar{\mu}} G_{\bar{\mu}}^A (\bar{q}_s T^A \bar{\mathcal{B}} q_r) + \frac{1}{18} g_s^2 g_Y (\mathcal{C}_{qd}^{(8)})^{ttsr} T_b^{Aa} T_a^{Bc} G_{\bar{\nu}}^A G_{\bar{\nu}}^B (\bar{d}_{cs} \bar{\mathcal{B}} d_r^b) \\
& + \frac{1}{18} (\mathcal{C}_{qd}^{(8)})^{ttsr} \left[ g_s^2 g_Y T_b^{Aa} T_c^{Bb} B_{\bar{\mu}} G_{\bar{\mu}}^B (\bar{d}_{as} \bar{\mathcal{G}}^A d_r^c) + g_s^2 g_Y T_b^{Aa} T_a^{Bc} B_{\bar{\mu}} G_{\bar{\mu}}^B (\bar{d}_{cs} \bar{\mathcal{G}}^A d_r^b) \right] \\
& + \frac{1}{12} g_L^2 g_s (\mathcal{C}_{qd}^{(8)})^{ttsr} W_{\bar{\mu}}^I {}^2 (\bar{d}_s T^A \bar{\mathcal{G}}^A d_r) + \frac{1}{6} g_L^2 g_s (\mathcal{C}_{qd}^{(8)})^{ttsr} G_{\bar{\mu}}^A W_{\bar{\mu}}^I (\bar{d}_s T^A \bar{\mathcal{W}}^I d_r) \\
& + \frac{2}{9} g_s^2 (\mathcal{C}_{qd}^{(8)})^{ttsr} G_{\bar{\mu}}^A \tilde{G}^{\bar{\mu}\bar{\sigma} A} (\bar{d}_s \gamma^{\bar{\sigma}} d_r) + \frac{1}{3} g_L g_s \bar{y}_d^{tu} (\mathcal{C}_{qd}^{(8)})^{trsu} t_j^I T_b^{Aa} H_i^\dagger G_{\bar{\mu}}^A W_{\bar{\mu}}^I (\bar{d}_{as} q_r^{bj})
\end{aligned}$$

$$\begin{aligned}
& -\frac{1}{108}g_s^2g_Y(\mathcal{C}_{qd}^{(8)})^{ttsr}G_{\bar{\mu}}^{A^2}(\bar{d}_s\bar{B}d_r) - \frac{1}{72}g_s^3(\mathcal{C}_{qd}^{(8)})^{srtt}d^{ABC}G_{\bar{\nu}}^BG_{\bar{\nu}}^C(\bar{q}_s\bar{G}^Aq_r) \\
& -\frac{1}{54}g_s^2g_Y(\mathcal{C}_{qd}^{(8)})^{ttsr}B_{\bar{\mu}}G_{\bar{\mu}}^A(\bar{d}_s\bar{G}^Ad_r) - \frac{1}{36}g_s^3(\mathcal{C}_{qd}^{(8)})^{ttsr}f^{ABC}G_{\bar{\mu}}^AG_{\bar{\nu}}^BG_{\bar{\rho}}^C\varepsilon^{\bar{\mu}\bar{\nu}\bar{\rho}\bar{\sigma}}(\bar{d}_s\gamma^{\bar{\sigma}}d_r) \\
& -\frac{1}{36}g_s^3(\mathcal{C}_{qd}^{(8)})^{ttsr}d^{ABC}G_{\bar{\nu}}^BG_{\bar{\nu}}^C(\bar{d}_s\bar{G}^Ad_r) - \frac{1}{18}g_s g_Y \bar{y}_d^{tu}(\mathcal{C}_{qd}^{(8)})^{trsu}T_b^{Aa}B_{\bar{\mu}}G_{\bar{\mu}}^A(\bar{d}_{as}H^\dagger q_r^b) \\
& -\frac{i}{18}g_s^2g_Y(\mathcal{C}_{qd}^{(8)})^{ttsr}T_b^{Aa}T_a^{Bc}B_{\bar{\mu}}G_{\bar{\nu}}^BG_{\bar{\rho}}^A\varepsilon^{\bar{\mu}\bar{\nu}\bar{\rho}\bar{\sigma}}(\bar{d}_{cs}\gamma^{\bar{\sigma}}d_r^b) \\
& +\frac{1}{3}g_s^2\bar{y}_d^{tu}(\mathcal{C}_{qd}^{(8)})^{trsu}T_b^{Aa}T_a^{Bc}G_{\bar{\mu}}^AG_{\bar{\mu}}^B(\bar{d}_{cs}H^\dagger q_r^b) - \frac{1}{18}g_s g_Y \bar{y}_d^{tu}(\mathcal{C}_{qd}^{(8)})^{stur}T_b^{Aa}B_{\bar{\mu}}G_{\bar{\mu}}^A(\bar{q}_{as}Hd_r^b) \\
& -\frac{i}{18}g_s^2g_Y(\mathcal{C}_{qd}^{(8)})^{srtt}T_b^{Aa}T_a^{Bc}B_{\bar{\mu}}G_{\bar{\nu}}^BG_{\bar{\rho}}^A\varepsilon^{\bar{\mu}\bar{\nu}\bar{\rho}\bar{\sigma}}(\bar{q}_{cs}\gamma^{\bar{\sigma}}q_r^b) \\
& -\frac{i}{12}(\mathcal{C}_{qd}^{(8)})^{srtt}\left[g_s^2T_b^{Aa}T_c^{Bb}G_{\bar{\mu}}^B(\bar{q}_{as}\gamma^{\bar{\nu}}q_r^c)\partial^{\bar{\mu}}G_{\bar{\nu}}^A - g_s^2T_b^{Aa}T_a^{Bc}G_{\bar{\mu}}^B(\bar{q}_{cs}\gamma^{\bar{\nu}}q_r^b)\partial^{\bar{\mu}}G_{\bar{\nu}}^A\right] \\
& -\frac{i}{12}(\mathcal{C}_{qd}^{(8)})^{srtt}\left[g_s^2T_b^{Aa}T_c^{Bb}(\bar{q}_{as}\bar{G}^Bq_r^c)\partial^{\bar{\nu}}G_{\bar{\nu}}^A - g_s^2T_b^{Aa}T_a^{Bc}(\bar{q}_{cs}\bar{G}^Bq_r^b)\partial^{\bar{\nu}}G_{\bar{\nu}}^A\right] \\
& +\frac{1}{6}g_s(\mathcal{C}_{qd}^{(8)})^{srtt}\left[2g_sT_b^{Aa}T_c^{Bb}G_{\bar{\mu}}^B\tilde{G}^{\bar{\mu}\bar{\sigma}A}(\bar{q}_{as}\gamma^{\bar{\sigma}}q_r^c) + 2g_sT_b^{Aa}T_a^{Bc}G_{\bar{\mu}}^B\tilde{G}^{\bar{\mu}\bar{\sigma}A}(\bar{q}_{cs}\gamma^{\bar{\sigma}}q_r^b)\right] \\
& +\frac{1}{3}g_s^2\bar{y}_d^{tu}(\mathcal{C}_{qd}^{(8)})^{stur}T_b^{Aa}T_c^{Bb}G_{\bar{\mu}}^AG_{\bar{\mu}}^B(\bar{q}_{as}Hd_r^c) - \frac{1}{18}g_s^2g_Y(\mathcal{C}_{qd}^{(8)})^{srtt}T_b^{Aa}T_a^{Bc}G_{\bar{\nu}}^AG_{\bar{\nu}}^B(\bar{q}_{cs}\bar{B}q_r^b) \\
& -\frac{1}{18}(\mathcal{C}_{qd}^{(8)})^{srtt}\left[g_s^2g_YT_b^{Aa}T_c^{Bb}B_{\bar{\mu}}G_{\bar{\mu}}^B(\bar{q}_{as}\bar{G}^Aq_r^c) + g_s^2g_YT_b^{Aa}T_a^{Bc}B_{\bar{\mu}}G_{\bar{\mu}}^B(\bar{q}_{cs}\bar{G}^Aq_r^b)\right] \\
& -\frac{1}{9}g_s^2(\mathcal{C}_{qd}^{(8)})^{srtt}G_{\bar{\mu}}^A\tilde{G}^{\bar{\mu}\bar{\sigma}A}(\bar{q}_s\gamma^{\bar{\sigma}}q_r) - \frac{1}{6}g_s(\mathcal{C}_{qd}^{(8)})^{srtt}(\bar{q}_sT^A\bar{G}^A\partial^2q_r) \\
& +\frac{i}{6}g_s^3(\mathcal{C}_{qd}^{(8)})^{srtt}T_b^{Aa}T_a^{Bc}T_c^{Cd}G_{\bar{\mu}}^AG_{\bar{\nu}}^CG_{\bar{\rho}}^B\varepsilon^{\bar{\mu}\bar{\nu}\bar{\rho}\bar{\sigma}}(\bar{q}_{ds}\gamma^{\bar{\sigma}}q_r^b) \\
& +\frac{1}{6}(\mathcal{C}_{qd}^{(8)})^{srtt}\left[g_s^3T_b^{Aa}T_c^{Bb}T_d^{Cc}G_{\bar{\mu}}^BG_{\bar{\mu}}^C(\bar{q}_{as}\bar{G}^Aq_r^d) + g_s^3T_b^{Aa}T_a^{Bc}T_c^{Cd}G_{\bar{\mu}}^BG_{\bar{\mu}}^C(\bar{q}_{ds}\bar{G}^Aq_r^b)\right] \\
& +\frac{1}{3}g_Lg_s\bar{y}_d^{tu}(\mathcal{C}_{qd}^{(8)})^{stur}t_j^{Ii}T_b^{Aa}H^jG_{\bar{\mu}}^AW_{\bar{\mu}}^I(\bar{q}_{ais}d_r^b) - \frac{1}{6}g_s^3(\mathcal{C}_{qd}^{(8)})^{srtt}T_b^{Aa}T_a^{Bc}T_c^{Cd}G_{\bar{\mu}}^AG_{\bar{\mu}}^C(\bar{q}_{ds}\bar{G}^Bq_r^b) \\
& -\frac{1}{6}g_s(\mathcal{C}_{qd}^{(8)})^{srtt}(\partial^2\bar{q}_sT^A\bar{G}^Aq_r) - \frac{1}{6}g_s(\mathcal{C}_{qd}^{(8)})^{srtt}(\bar{q}_sT^A\gamma^{\bar{\mu}}q_r)\partial^2G_{\bar{\mu}}^A \\
& -\frac{i}{6}(\mathcal{C}_{qd}^{(8)})^{ttsr}\left[g_s^2T_b^{Aa}T_c^{Bb}G_{\bar{\mu}}^B(\bar{d}_{as}\gamma^{\bar{\nu}}d_r^c)\partial^{\bar{\mu}}G_{\bar{\nu}}^A - g_s^2T_b^{Aa}T_a^{Bc}G_{\bar{\mu}}^B(\bar{d}_{cs}\gamma^{\bar{\nu}}d_r^b)\partial^{\bar{\mu}}G_{\bar{\nu}}^A\right] \\
& -\frac{i}{6}(\mathcal{C}_{qd}^{(8)})^{ttsr}\left[g_s^2T_b^{Aa}T_c^{Bb}(\bar{d}_{as}\bar{G}^Bd_r^c)\partial^{\bar{\nu}}G_{\bar{\nu}}^A - g_s^2T_b^{Aa}T_a^{Bc}(\bar{d}_{cs}\bar{G}^Bd_r^b)\partial^{\bar{\nu}}G_{\bar{\nu}}^A\right] \\
& -\frac{2}{9}g_s g_Y (\mathcal{C}_{qd}^{(8)})^{ttsr}G_{\bar{\mu}}^A\tilde{B}^{\bar{\mu}\bar{\sigma}}(\bar{d}_sT^A\gamma^{\bar{\sigma}}d_r) - \frac{2}{9}g_s g_Y (\mathcal{C}_{qd}^{(8)})^{ttsr}B_{\bar{\mu}}\tilde{G}^{\bar{\mu}\bar{\sigma}A}(\bar{d}_sT^A\gamma^{\bar{\sigma}}d_r) \\
& -\frac{2}{9}g_s g_Y (\mathcal{C}_{qd}^{(8)})^{srtt}G_{\bar{\mu}}^A\tilde{B}^{\bar{\mu}\bar{\sigma}}(\bar{q}_sT^A\gamma^{\bar{\sigma}}q_r) - \frac{2}{9}g_s g_Y (\mathcal{C}_{qd}^{(8)})^{srtt}B_{\bar{\mu}}\tilde{G}^{\bar{\mu}\bar{\sigma}A}(\bar{q}_sT^A\gamma^{\bar{\sigma}}q_r) \\
& -\frac{1}{3}g_s(\mathcal{C}_{qd}^{(8)})^{ttsr}(\bar{d}_sT^A\bar{G}^A\partial^2d_r) \\
& -\frac{1}{3}g_s(\mathcal{C}_{qd}^{(8)})^{ttsr}\left[2g_sT_b^{Aa}T_c^{Bb}G_{\bar{\mu}}^B\tilde{G}^{\bar{\mu}\bar{\sigma}A}(\bar{d}_{as}\gamma^{\bar{\sigma}}d_r^c) + 2g_sT_b^{Aa}T_a^{Bc}G_{\bar{\mu}}^B\tilde{G}^{\bar{\mu}\bar{\sigma}A}(\bar{d}_{cs}\gamma^{\bar{\sigma}}d_r^b)\right] \\
& -\frac{i}{3}g_s^3(\mathcal{C}_{qd}^{(8)})^{ttsr}T_b^{Aa}T_a^{Bc}T_c^{Cd}G_{\bar{\mu}}^AG_{\bar{\nu}}^CG_{\bar{\rho}}^B\varepsilon^{\bar{\mu}\bar{\nu}\bar{\rho}\bar{\sigma}}(\bar{d}_{ds}\gamma^{\bar{\sigma}}d_r^b)
\end{aligned}$$

$$\begin{aligned}
& + \frac{1}{3}(\mathcal{C}_{qd}^{(8)})^{ttsr} \left[ g_s^3 T_b^{Aa} T_c^{Bb} T_d^{Cc} G_{\bar{\mu}}^B G_{\bar{\mu}}^C (\bar{d}_{as} \bar{\mathcal{G}}^A d_r^d) + g_s^3 T_b^{Aa} T_a^{Bc} T_c^{Cd} G_{\bar{\mu}}^B G_{\bar{\mu}}^C (\bar{d}_{ds} \bar{\mathcal{G}}^A d_r^b) \right] \\
& - \frac{1}{3} g_s^3 (\mathcal{C}_{qd}^{(8)})^{ttsr} T_b^{Aa} T_a^{Bc} T_c^{Cd} G_{\bar{\mu}}^A G_{\bar{\mu}}^C (\bar{d}_{ds} \bar{\mathcal{G}}^B d_r^b) - \frac{1}{3} g_s (\mathcal{C}_{qd}^{(8)})^{ttsr} (\partial^2 \bar{d}_s T^A \bar{\mathcal{G}}^A d_r) \\
& - \frac{1}{3} g_s (\mathcal{C}_{qd}^{(8)})^{srtt} (\partial^{\bar{\nu}} \bar{q}_s T^A \bar{\mathcal{G}}^A \partial^{\bar{\nu}} q_r) - \frac{1}{3} g_s (\mathcal{C}_{qd}^{(8)})^{ttsr} (\bar{d}_s T^A \gamma^{\bar{\mu}} d_r) \partial^2 G_{\bar{\mu}}^A \\
& - \frac{5i}{12} (\mathcal{C}_{qd}^{(8)})^{srtt} \left[ g_s^2 T_b^{Aa} T_a^{Bc} G_{\bar{\nu}}^B (\bar{q}_{cs} \bar{\mathcal{G}}^A \partial^{\bar{\nu}} q_r^b) - g_s^2 T_b^{Aa} T_c^{Bb} G_{\bar{\nu}}^B (\partial^{\bar{\nu}} \bar{q}_{as} \bar{\mathcal{G}}^A q_r^c) \right] \\
& - \frac{5i}{12} (\mathcal{C}_{qd}^{(8)})^{srtt} \left[ g_s^2 T_b^{Aa} T_c^{Bb} G_{\bar{\nu}}^A (\partial^{\bar{\nu}} \bar{q}_{as} \bar{\mathcal{G}}^B q_r^c) - g_s^2 T_b^{Aa} T_a^{Bc} G_{\bar{\nu}}^A (\bar{q}_{cs} \bar{\mathcal{G}}^B \partial^{\bar{\nu}} q_r^b) \right] \\
& - \frac{4i}{9} g_Y \bar{y}_d^{tu} (\mathcal{C}_{qd}^{(8)})^{trsu} B_{\bar{\mu}} (\bar{d}_s H^\dagger \partial^{\bar{\mu}} q_r) + \frac{4i}{9} g_Y \bar{y}_d^{tu} (\mathcal{C}_{qd}^{(8)})^{trsu} B_{\bar{\mu}} (\bar{d}_s \partial^{\bar{\mu}} H^\dagger q_r) + \frac{4i}{9} g_Y y_d^{tu} (\mathcal{C}_{qd}^{(8)})^{stur} B_{\bar{\mu}} (\bar{q}_s H \partial^{\bar{\mu}} d_r) \\
& - \frac{4i}{9} g_Y y_d^{tu} (\mathcal{C}_{qd}^{(8)})^{stur} B_{\bar{\mu}} (\bar{q}_s \partial^{\bar{\mu}} H d_r) - \frac{4i}{9} g_Y \bar{y}_d^{tu} (\mathcal{C}_{qd}^{(8)})^{trsu} B_{\bar{\mu}} (\partial^{\bar{\mu}} \bar{d}_s H^\dagger q_r) + \frac{4i}{9} g_Y y_d^{tu} (\mathcal{C}_{qd}^{(8)})^{stur} B_{\bar{\mu}} (\partial^{\bar{\mu}} \bar{q}_s H d_r) \\
& - \frac{1}{2} g_s^2 \bar{y}_d^{tu} (\mathcal{C}_{qd}^{(8)})^{trsu} G_{\bar{\mu}}^{A2} (\bar{d}_s H^\dagger q_r) - \frac{1}{2} g_s (\mathcal{C}_{qd}^{(8)})^{tv sr} \left[ y_d^{vu} \bar{y}_d^{tu} + y_u^{vu} \bar{y}_u^{tu} \right] (H^\dagger H) (\bar{d}_s T^A \bar{\mathcal{G}}^A d_r) \\
& - \frac{1}{2} g_s^2 y_d^{tu} (\mathcal{C}_{qd}^{(8)})^{stur} G_{\bar{\mu}}^{A2} (\bar{q}_s H d_r) - \frac{1}{2} g_s y_d^{tv} \bar{y}_d^{tu} (\mathcal{C}_{qd}^{(8)})^{sr vu} (H^\dagger H) (\bar{q}_s T^A \bar{\mathcal{G}}^A q_r) \\
& - \frac{i}{2} g_s (\mathcal{C}_{qd}^{(8)})^{srtt} \left[ g_s T_b^{Aa} T_c^{Bb} G_{\bar{\mu}}^B G^{\bar{\mu}\bar{\nu}A} (\bar{q}_{as} \gamma^{\bar{\nu}} q_r^c) - g_s T_b^{Aa} T_a^{Bc} G_{\bar{\mu}}^B G^{\bar{\mu}\bar{\nu}A} (\bar{q}_{cs} \gamma^{\bar{\nu}} q_r^b) \right] \\
& - \frac{14}{27} g_Y^2 \bar{y}_d^{tu} (\mathcal{C}_{qd}^{(8)})^{trsu} B_{\bar{\mu}}^2 (\bar{d}_s H^\dagger q_r) - \frac{14}{27} g_Y^2 y_d^{tu} (\mathcal{C}_{qd}^{(8)})^{stur} B_{\bar{\mu}}^2 (\bar{q}_s H d_r) - \frac{2}{3} g_L^2 \bar{y}_d^{tu} (\mathcal{C}_{qd}^{(8)})^{trsu} W_{\bar{\mu}}^{I2} (\bar{d}_s H^\dagger q_r) \\
& - \frac{2}{3} g_L^2 y_d^{tu} (\mathcal{C}_{qd}^{(8)})^{stur} W_{\bar{\mu}}^{I2} (\bar{q}_s H d_r) - \frac{2}{3} g_s (\mathcal{C}_{qd}^{(8)})^{ttsr} (\partial^{\bar{\nu}} \bar{d}_s T^A \bar{\mathcal{G}}^A \partial^{\bar{\nu}} d_r) \\
& - \frac{5i}{6} (\mathcal{C}_{qd}^{(8)})^{ttsr} \left[ g_s^2 T_b^{Aa} T_a^{Bc} G_{\bar{\nu}}^B (\bar{d}_{cs} \bar{\mathcal{G}}^A \partial^{\bar{\nu}} d_r^b) - g_s^2 T_b^{Aa} T_c^{Bb} G_{\bar{\nu}}^B (\partial^{\bar{\nu}} \bar{d}_{as} \bar{\mathcal{G}}^A d_r^c) \right] \\
& - \frac{5i}{6} (\mathcal{C}_{qd}^{(8)})^{ttsr} \left[ g_s^2 T_b^{Aa} T_c^{Bb} G_{\bar{\nu}}^A (\partial^{\bar{\nu}} \bar{d}_{as} \bar{\mathcal{G}}^B d_r^c) - g_s^2 T_b^{Aa} T_a^{Bc} G_{\bar{\nu}}^A (\bar{d}_{cs} \bar{\mathcal{G}}^B \partial^{\bar{\nu}} d_r^b) \right] \\
& - \frac{8i}{9} g_L \bar{y}_d^{tu} (\mathcal{C}_{qd}^{(8)})^{trsu} t_j^{Ii} H_i^\dagger W_{\bar{\mu}}^I (\bar{d}_s \partial^{\bar{\mu}} q_r^j) + \frac{8i}{9} g_L y_d^{tu} (\mathcal{C}_{qd}^{(8)})^{stur} t_j^{Ii} H^j W_{\bar{\mu}}^I (\bar{q}_{is} \partial^{\bar{\mu}} d_r) \\
& - \frac{8i}{9} g_L \bar{y}_d^{tu} (\mathcal{C}_{qd}^{(8)})^{trsu} t_j^{Ii} H_i^\dagger W_{\bar{\mu}}^I (\partial^{\bar{\mu}} \bar{d}_s q_r^j) + \frac{8i}{9} g_L y_d^{tu} (\mathcal{C}_{qd}^{(8)})^{stur} t_j^{Ii} H^j W_{\bar{\mu}}^I (\partial^{\bar{\mu}} \bar{q}_{is} d_r) \\
& + \frac{8i}{9} g_L \bar{y}_d^{tu} (\mathcal{C}_{qd}^{(8)})^{trsu} t_j^{Ii} W_{\bar{\mu}}^I (\bar{d}_s q_r^j) \partial^{\bar{\mu}} H_i^\dagger - \frac{8i}{9} g_L y_d^{tu} (\mathcal{C}_{qd}^{(8)})^{stur} t_j^{Ii} W_{\bar{\mu}}^I (\bar{q}_{is} d_r) \partial^{\bar{\mu}} H^j \\
& - i g_s (\mathcal{C}_{qd}^{(8)})^{ttsr} \left[ g_s T_b^{Aa} T_c^{Bb} G_{\bar{\mu}}^B G^{\bar{\mu}\bar{\nu}A} (\bar{d}_{as} \gamma^{\bar{\nu}} d_r^c) - g_s T_b^{Aa} T_a^{Bc} G_{\bar{\mu}}^B G^{\bar{\mu}\bar{\nu}A} (\bar{d}_{cs} \gamma^{\bar{\nu}} d_r^b) \right] \\
& - \frac{16}{9} g_L g_Y \bar{y}_d^{tu} (\mathcal{C}_{qd}^{(8)})^{trsu} t_j^{Ii} H_i^\dagger B_{\bar{\mu}} W_{\bar{\mu}}^I (\bar{d}_s q_r^j) - \frac{16}{9} g_L g_Y y_d^{tu} (\mathcal{C}_{qd}^{(8)})^{stur} t_j^{Ii} H^j B_{\bar{\mu}} W_{\bar{\mu}}^I (\bar{q}_{is} d_r), \tag{2.56}
\end{aligned}$$

$$\begin{aligned}
\Delta S_{\mathcal{O}_{\ell edq}} &= \frac{i}{6} g_Y \bar{y}_e^{tu} \mathcal{C}_{\ell edq}^{tusr} B_{\bar{\mu}} (\bar{d}_s H^\dagger \partial^{\bar{\mu}} q_r) - \frac{i}{6} g_Y \bar{y}_e^{tu} \mathcal{C}_{\ell edq}^{tusr} B_{\bar{\mu}} (\bar{d}_s \partial^{\bar{\mu}} H^\dagger q_r) - \frac{i}{6} g_Y y_e^{tu} \bar{\mathcal{C}}_{\ell edq}^{turs} B_{\bar{\mu}} (\bar{q}_s H \partial^{\bar{\mu}} d_r) \\
& + \frac{i}{6} g_Y y_e^{tu} \bar{\mathcal{C}}_{\ell edq}^{turs} B_{\bar{\mu}} (\bar{q}_s \partial^{\bar{\mu}} H d_r) + \frac{i}{6} g_Y \bar{y}_e^{tu} \mathcal{C}_{\ell edq}^{tusr} B_{\bar{\mu}} (\partial^{\bar{\mu}} \bar{d}_s H^\dagger q_r) - \frac{i}{6} g_Y y_e^{tu} \bar{\mathcal{C}}_{\ell edq}^{turs} B_{\bar{\mu}} (\partial^{\bar{\mu}} \bar{q}_s H d_r) \\
& + \frac{1}{4} g_L^2 \bar{y}_e^{tu} \mathcal{C}_{\ell edq}^{tusr} W_{\bar{\mu}}^{I2} (\bar{d}_s H^\dagger q_r) + \frac{1}{4} g_L^2 y_e^{tu} \bar{\mathcal{C}}_{\ell edq}^{turs} W_{\bar{\mu}}^{I2} (\bar{q}_s H d_r) + \frac{i}{3} g_L \bar{y}_e^{tu} \mathcal{C}_{\ell edq}^{tusr} t_j^{Ii} H_i^\dagger W_{\bar{\mu}}^I (\bar{d}_s \partial^{\bar{\mu}} q_r^j) \\
& - \frac{i}{3} g_L y_e^{tu} \bar{\mathcal{C}}_{\ell edq}^{turs} t_j^{Ii} H^j W_{\bar{\mu}}^I (\bar{q}_{is} \partial^{\bar{\mu}} d_r) + \frac{i}{3} g_L \bar{y}_e^{tu} \mathcal{C}_{\ell edq}^{tusr} t_j^{Ii} H_i^\dagger W_{\bar{\mu}}^I (\partial^{\bar{\mu}} \bar{d}_s q_r^j)
\end{aligned}$$

$$\begin{aligned}
& -\frac{i}{3}g_L\bar{y}_e^{tu}\bar{C}_{ledq}^{Ii}t_j^{Ii}H^jW_\mu^I(\partial^\mu\bar{q}_{is}d_r)-\frac{i}{3}g_L\bar{y}_e^{tu}C_{ledq}^{tusr}t_j^{Ii}W_\mu^I(\bar{d}_sq_r^j)\partial^\mu H_i^\dagger \\
& +\frac{i}{3}g_L\bar{y}_e^{tu}\bar{C}_{ledq}^{Ii}W_\mu^I(\bar{q}_{is}d_r)\partial^\mu H^j+\frac{1}{2}g_s^2\bar{y}_d^{ut}\bar{C}_{ledq}^{rstu}G_\mu^{A2}(\bar{e}_sH^\dagger\ell_r) \\
& +\frac{i}{2}g_Y\bar{y}_d^{ut}\bar{C}_{ledq}^{rstu}B_\mu(\bar{e}_sH^\dagger\partial^\mu\ell_r)-\frac{i}{2}g_Y\bar{y}_d^{ut}\bar{C}_{ledq}^{rstu}B_\mu(\bar{e}_s\partial^\mu H^\dagger\ell_r)+\frac{1}{2}g_s^2\bar{y}_d^{ut}C_{ledq}^{srtu}G_\mu^{A2}(\bar{\ell}_sHe_r) \\
& -\frac{i}{2}g_Y\bar{y}_d^{ut}C_{ledq}^{srtu}B_\mu(\bar{\ell}_sH\partial^\mu e_r)+\frac{i}{2}g_Y\bar{y}_d^{ut}C_{ledq}^{srtu}B_\mu(\bar{\ell}_s\partial^\mu He_r)+\frac{i}{2}g_Y\bar{y}_d^{ut}\bar{C}_{ledq}^{rstu}B_\mu(\partial^\mu\bar{e}_sH^\dagger\ell_r) \\
& -\frac{i}{2}g_Y\bar{y}_d^{ut}C_{ledq}^{srtu}B_\mu(\partial^\mu\bar{\ell}_sHe_r)+\frac{7}{12}g_Y^2\bar{y}_d^{ut}\bar{C}_{ledq}^{rstu}B_\mu^2(\bar{e}_sH^\dagger\ell_r)+\frac{7}{12}g_Y^2\bar{y}_d^{ut}C_{ledq}^{srtu}B_\mu^2(\bar{\ell}_sHe_r) \\
& +\frac{3}{4}g_Y^2\bar{y}_e^{tu}C_{ledq}^{tusr}B_\mu^2(\bar{d}_sH^\dagger q_r)+\frac{3}{4}g_L^2\bar{y}_d^{ut}\bar{C}_{ledq}^{rstu}W_\mu^{I2}(\bar{e}_sH^\dagger\ell_r)+\frac{3}{4}g_L^2\bar{y}_d^{ut}C_{ledq}^{srtu}W_\mu^{I2}(\bar{\ell}_sHe_r) \\
& +\frac{3}{4}g_Y^2\bar{y}_e^{tu}\bar{C}_{ledq}^{Ii}t_j^{Ii}H_i^\dagger W_\mu^I(\partial^\mu\bar{e}_s\ell_r^j)-ig_L\bar{y}_d^{ut}\bar{C}_{ledq}^{rstu}t_j^{Ii}H_i^\dagger W_\mu^I(\bar{e}_s\partial^\mu\ell_r^j)-ig_L\bar{y}_d^{ut}C_{ledq}^{srtu}t_j^{Ii}H^jW_\mu^I(\bar{\ell}_{is}\partial^\mu e_r) \\
& +ig_L\bar{y}_d^{ut}\bar{C}_{ledq}^{rstu}t_j^{Ii}H_i^\dagger W_\mu^I(\partial^\mu\bar{e}_s\ell_r^j)-ig_L\bar{y}_d^{ut}C_{ledq}^{srtu}t_j^{Ii}H^jW_\mu^I(\partial^\mu\bar{\ell}_{is}e_r) \\
& -ig_L\bar{y}_d^{ut}\bar{C}_{ledq}^{Ii}t_j^{Ii}W_\mu^I(\bar{e}_s\ell_r^j)\partial^\mu H_i^\dagger+ig_L\bar{y}_d^{ut}C_{ledq}^{srtu}t_j^{Ii}W_\mu^I(\bar{\ell}_{is}e_r)\partial^\mu H^j \\
& +2g_Lg_Y\bar{y}_d^{ut}\bar{C}_{ledq}^{rstu}t_j^{Ii}H_i^\dagger B_\mu W_\mu^I(\bar{e}_s\ell_r^j)+2g_Lg_Y\bar{y}_d^{ut}C_{ledq}^{srtu}t_j^{Ii}H^j B_\mu W_\mu^I(\bar{\ell}_{is}e_r), \tag{2.57}
\end{aligned}$$

$$\begin{aligned}
\Delta S_{\mathcal{O}_{lequ}^{(1)}} &= \frac{1}{6}g_L^2\bar{y}_e^{tu}(C_{lequ}^{(1)})^{tusr}W_\mu^{I2}(\bar{q}_s\tilde{H}u_r)+\frac{i}{6}g_Y\bar{y}_e^{tu}(C_{lequ}^{(1)})^{tusr}B_\mu(\bar{q}_s\tilde{H}\partial^\mu u_r) \\
& +\frac{i}{6}g_Y\bar{y}_e^{tu}(C_{lequ}^{(1)})^{tusr}B_\mu(\bar{q}_s\partial^\mu\tilde{H}u_r)+\frac{1}{6}g_L^2\bar{y}_e^{tu}(\bar{C}_{lequ}^{(1)})^{turs}W_\mu^{I2}(\bar{u}_s\tilde{H}^\dagger q_r) \\
& -\frac{i}{6}g_Y\bar{y}_e^{tu}(\bar{C}_{lequ}^{(1)})^{turs}B_\mu(\bar{u}_s\tilde{H}^\dagger\partial^\mu q_r)-\frac{i}{6}g_Y\bar{y}_e^{tu}(\bar{C}_{lequ}^{(1)})^{turs}B_\mu(\bar{u}_s\partial^\mu\tilde{H}q_r) \\
& +\frac{i}{6}g_Y\bar{y}_e^{tu}(C_{lequ}^{(1)})^{tusr}B_\mu(\partial^\mu\bar{q}_s\tilde{H}u_r)-\frac{i}{6}g_Y\bar{y}_e^{tu}(\bar{C}_{lequ}^{(1)})^{turs}B_\mu(\partial^\mu\bar{u}_s\tilde{H}^\dagger q_r) \\
& +\frac{1}{3}g_L^2\bar{y}_e^{tu}(C_{lequ}^{(1)})^{tusr}\varepsilon^{jk}t_l^{Ii}t_j^{Jl}H_i^\dagger W_\mu^IW_\mu^J(\bar{q}_{ks}u_r)+\frac{i}{3}g_L\bar{y}_e^{tu}(C_{lequ}^{(1)})^{tusr}\varepsilon^{jk}t_j^{Ii}H_i^\dagger W_\mu^I(\bar{q}_{ks}\partial^\mu u_r) \\
& +\frac{1}{3}g_L^2\bar{y}_e^{tu}(\bar{C}_{lequ}^{(1)})^{turs}\bar{\varepsilon}_{ij}t_l^{Ik}t_k^{Jl}H^lW_\mu^IW_\mu^J(\bar{u}_sq_r^j)-\frac{i}{3}g_L\bar{y}_e^{tu}(\bar{C}_{lequ}^{(1)})^{turs}\bar{\varepsilon}_{ij}t_k^{Ii}H^k W_\mu^I(\bar{u}_s\partial^\mu q_r^j) \\
& +\frac{i}{3}g_L\bar{y}_e^{tu}(C_{lequ}^{(1)})^{tusr}\varepsilon^{jk}t_j^{Ii}H_i^\dagger W_\mu^I(\partial^\mu\bar{q}_{ks}u_r)-\frac{i}{3}g_L\bar{y}_e^{tu}(\bar{C}_{lequ}^{(1)})^{turs}\bar{\varepsilon}_{ij}t_k^{Ii}H^k W_\mu^I(\partial^\mu\bar{u}_sq_r^j) \\
& -\frac{i}{3}g_L\bar{y}_e^{tu}(C_{lequ}^{(1)})^{tusr}\varepsilon^{ij}t_i^{Ik}W_\mu^I(\bar{q}_{js}u_r)\partial^\mu H_k^\dagger+\frac{i}{3}g_L\bar{y}_e^{tu}(\bar{C}_{lequ}^{(1)})^{turs}\bar{\varepsilon}_{ij}t_k^{Ii}W_\mu^I(\bar{u}_sq_r^j)\partial^\mu H^k \\
& -\frac{1}{2}g_s^2\bar{y}_u^{tu}(\bar{C}_{lequ}^{(1)})^{rstu}G_\mu^{A2}(\bar{e}_sH^\dagger\ell_r)-\frac{i}{2}g_Y\bar{y}_u^{tu}(\bar{C}_{lequ}^{(1)})^{rstu}B_\mu(\bar{e}_sH^\dagger\partial^\mu\ell_r) \\
& +\frac{i}{2}g_Y\bar{y}_u^{tu}(\bar{C}_{lequ}^{(1)})^{rstu}B_\mu(\bar{e}_s\partial^\mu H^\dagger\ell_r)-\frac{1}{2}g_s^2\bar{y}_u^{tu}(C_{lequ}^{(1)})^{srtu}G_\mu^{A2}(\bar{\ell}_sHe_r) \\
& +\frac{i}{2}g_Y\bar{y}_u^{tu}(C_{lequ}^{(1)})^{srtu}B_\mu(\bar{\ell}_sH\partial^\mu e_r)-\frac{i}{2}g_Y\bar{y}_u^{tu}(C_{lequ}^{(1)})^{srtu}B_\mu(\bar{\ell}_s\partial^\mu He_r) \\
& -\frac{i}{2}g_Y\bar{y}_u^{tu}(\bar{C}_{lequ}^{(1)})^{rstu}B_\mu(\partial^\mu\bar{e}_sH^\dagger\ell_r)+\frac{i}{2}g_Y\bar{y}_u^{tu}(C_{lequ}^{(1)})^{srtu}B_\mu(\partial^\mu\bar{\ell}_sHe_r) \\
& +\frac{3}{4}g_Y^2\bar{y}_e^{tu}(C_{lequ}^{(1)})^{tusr}B_\mu^2(\bar{q}_s\tilde{H}u_r)+\frac{3}{4}g_Y^2\bar{y}_e^{tu}(\bar{C}_{lequ}^{(1)})^{turs}B_\mu^2(\bar{u}_s\tilde{H}^\dagger q_r)-\frac{3}{4}g_L^2\bar{y}_u^{tu}(\bar{C}_{lequ}^{(1)})^{rstu}W_\mu^{I2}(\bar{e}_sH^\dagger\ell_r) \\
& -\frac{3}{4}g_L^2\bar{y}_u^{tu}(C_{lequ}^{(1)})^{srtu}W_\mu^{I2}(\bar{\ell}_sHe_r)-g_Lg_Y\bar{y}_u^{tu}(\bar{C}_{lequ}^{(1)})^{rstu}t_j^{Ii}H_i^\dagger B_\mu W_\mu^I(\bar{e}_s\ell_r^j)
\end{aligned}$$

$$\begin{aligned}
& -ig_L y_u^{tu} (\bar{\mathcal{C}}_{\ell equ}^{(1)})^{rstu} t_j^{Ii} H_i^\dagger W_\mu^I (\bar{e}_s \partial^\mu \ell_r^j) - g_L g_Y \bar{y}_u^{tu} (\mathcal{C}_{\ell equ}^{(1)})^{srtu} t_j^{Ii} H^j B_\mu W_\mu^I (\bar{\ell}_{is} e_r) \\
& + ig_L \bar{y}_u^{tu} (\mathcal{C}_{\ell equ}^{(1)})^{srtu} t_j^{Ii} H^j W_\mu^I (\bar{\ell}_{is} \partial^\mu e_r) - ig_L y_u^{tu} (\bar{\mathcal{C}}_{\ell equ}^{(1)})^{rstu} t_j^{Ii} H_i^\dagger W_\mu^I (\partial^\mu \bar{e}_s \ell_r^j) \\
& + ig_L \bar{y}_u^{tu} (\mathcal{C}_{\ell equ}^{(1)})^{srtu} t_j^{Ii} H^j W_\mu^I (\partial^\mu \bar{\ell}_{is} e_r) + ig_L y_u^{tu} (\bar{\mathcal{C}}_{\ell equ}^{(1)})^{rstu} t_j^{Ii} W_\mu^I (\bar{e}_s \ell_r^j) \partial^\mu H_i^\dagger \\
& - ig_L \bar{y}_u^{tu} (\mathcal{C}_{\ell equ}^{(1)})^{srtu} t_j^{Ii} W_\mu^I (\bar{\ell}_{is} e_r) \partial^\mu H^j - \frac{13}{12} g_Y^2 y_u^{tu} (\bar{\mathcal{C}}_{\ell equ}^{(1)})^{rstu} B_\mu^2 (\bar{e}_s H^\dagger \ell_r) - \frac{13}{12} g_Y^2 \bar{y}_u^{tu} (\mathcal{C}_{\ell equ}^{(1)})^{srtu} B_\mu^2 (\bar{\ell}_s H e_r),
\end{aligned} \tag{2.58}$$

$$\begin{aligned}
\Delta S_{\mathcal{O}_{\ell equ}^{(3)}} &= \frac{8i}{3} g_L^2 \bar{y}_e^{tu} (\mathcal{C}_{\ell equ}^{(3)})^{tusr} t_l^{Ik} t_j^{Jl} \tilde{H}_j W_\mu^I W_\nu^J (\bar{q}_{ks} \sigma^{\mu\nu} u_r) \\
& - \frac{8i}{3} g_L^2 y_e^{tu} (\bar{\mathcal{C}}_{\ell equ}^{(3)})^{turs} t_l^{Ik} t_k^{Ji} \tilde{H}^\dagger{}^i W_\mu^I W_\nu^J (\bar{u}_s \sigma^{\mu\nu} q_r^l) \\
& + 4g_L^2 y_u^{tu} (\bar{\mathcal{C}}_{\ell equ}^{(3)})^{rstu} \varepsilon^{IJK} t_j^{Ki} H_i^\dagger W_\mu^J W_\nu^I (\bar{e}_s \sigma^{\mu\nu} \ell_r^j) \\
& + 4g_L^2 \bar{y}_u^{tu} (\mathcal{C}_{\ell equ}^{(3)})^{srtu} \varepsilon^{IJK} t_j^{Ki} H^j W_\mu^J W_\nu^I (\bar{\ell}_{is} \sigma^{\mu\nu} e_r) + \frac{20}{3} g_Y y_u^{tu} (\bar{\mathcal{C}}_{\ell equ}^{(3)})^{rstu} B_\mu (\bar{e}_s \sigma^{\mu\nu} \partial^\nu H^\dagger \ell_r) \\
& + \frac{20}{3} g_Y \bar{y}_u^{tu} (\mathcal{C}_{\ell equ}^{(3)})^{srtu} B_\mu (\bar{\ell}_s \partial^\nu H \sigma^{\mu\nu} e_r) - \frac{8}{3} g_L \bar{y}_e^{tu} (\mathcal{C}_{\ell equ}^{(3)})^{tusr} \varepsilon^{ij} t_i^{Ik} W_\mu^I (\bar{q}_{js} \sigma^{\mu\nu} u_r) \partial^\nu H_k^\dagger \\
& - \frac{8}{3} g_L y_e^{tu} (\bar{\mathcal{C}}_{\ell equ}^{(3)})^{turs} \bar{\varepsilon}_{ij} t_k^{Ii} W_\mu^I (\bar{u}_s \sigma^{\mu\nu} q_r^j) \partial^\nu H^k - 4g_Y \bar{y}_e^{tu} (\mathcal{C}_{\ell equ}^{(3)})^{tusr} B_\mu (\bar{q}_s \partial^\nu \tilde{H} \sigma^{\mu\nu} u_r) \\
& + 4ig_L g_Y \bar{y}_e^{tu} (\mathcal{C}_{\ell equ}^{(3)})^{tusr} \varepsilon^{jk} t_j^{Ii} H_i^\dagger B_\mu W_\nu^I (\bar{q}_{ks} \sigma^{\mu\nu} u_r) - 4ig_L g_Y y_e^{tu} (\bar{\mathcal{C}}_{\ell equ}^{(3)})^{turs} \bar{\varepsilon}_{ij} t_k^{Ii} H^k B_\mu W_\nu^I (\bar{u}_s \sigma^{\mu\nu} q_r^j) \\
& - 4g_Y y_e^{tu} (\bar{\mathcal{C}}_{\ell equ}^{(3)})^{turs} B_\mu (\bar{u}_s \sigma^{\mu\nu} \partial^\nu \tilde{H} q_r) + 8ig_L g_Y y_u^{tu} (\bar{\mathcal{C}}_{\ell equ}^{(3)})^{rstu} t_j^{Ii} H_i^\dagger B_\mu W_\nu^I (\bar{e}_s \sigma^{\mu\nu} \ell_r^j) \\
& - 8ig_L g_Y \bar{y}_u^{tu} (\mathcal{C}_{\ell equ}^{(3)})^{srtu} t_j^{Ii} H^j B_\mu W_\nu^I (\bar{\ell}_{is} \sigma^{\mu\nu} e_r) - 8g_L y_u^{tu} (\bar{\mathcal{C}}_{\ell equ}^{(3)})^{rstu} t_j^{Ii} W_\mu^I (\bar{e}_s \sigma^{\mu\nu} \ell_r^j) \partial^\nu H_i^\dagger \\
& - 8g_L \bar{y}_u^{tu} (\mathcal{C}_{\ell equ}^{(3)})^{srtu} t_j^{Ii} W_\mu^I (\bar{\ell}_{is} \sigma^{\mu\nu} e_r) \partial^\nu H^j,
\end{aligned} \tag{2.59}$$

$$\begin{aligned}
\Delta S_{\mathcal{O}_{quqd}^{(1)}} &= \frac{1}{18} g_Y \bar{y}_d^{tu} (\mathcal{C}_{quqd}^{(1)})^{trsu} B_\mu (\bar{q}_s \partial^\nu \tilde{H} \sigma^{\mu\nu} u_r) + \frac{1}{18} g_Y y_d^{tu} (\bar{\mathcal{C}}_{quqd}^{(1)})^{tsru} B_\mu (\bar{u}_s \sigma^{\mu\nu} \partial^\nu \tilde{H} q_r) \\
& + \frac{i}{12} g_Y \left[ y_u^{ut} (\bar{\mathcal{C}}_{quqd}^{(1)})^{rtus} + 6y_u^{tu} (\bar{\mathcal{C}}_{quqd}^{(1)})^{turs} \right] B_\mu (\bar{d}_s H^\dagger \partial^\mu q_r) \\
& - \frac{i}{12} g_Y \left[ y_u^{ut} (\bar{\mathcal{C}}_{quqd}^{(1)})^{rtus} + 6y_u^{tu} (\bar{\mathcal{C}}_{quqd}^{(1)})^{turs} \right] B_\mu (\bar{d}_s \partial^\mu H^\dagger q_r) - \frac{i}{12} g_Y \bar{y}_u^{tu} \left[ (\mathcal{C}_{quqd}^{(1)})^{sutr} + 6(\mathcal{C}_{quqd}^{(1)})^{tusr} \right] B_\mu (\bar{q}_s H \partial^\mu d_r) \\
& - \frac{i}{12} g_Y \bar{y}_d^{tu} \left[ (\mathcal{C}_{quqd}^{(1)})^{trsu} + 6(\mathcal{C}_{quqd}^{(1)})^{srtu} \right] B_\mu (\bar{q}_s \tilde{H} \partial^\mu u_r) + \frac{i}{12} g_Y \bar{y}_u^{tu} \left[ (\mathcal{C}_{quqd}^{(1)})^{sutr} + 6(\mathcal{C}_{quqd}^{(1)})^{tusr} \right] B_\mu (\bar{q}_s \partial^\mu H d_r) \\
& - \frac{i}{12} g_Y \bar{y}_d^{tu} \left[ (\mathcal{C}_{quqd}^{(1)})^{trsu} + 6(\mathcal{C}_{quqd}^{(1)})^{srtu} \right] B_\mu (\bar{q}_s \partial^\mu \tilde{H} u_r) + \frac{1}{12} g_s g_Y \bar{y}_d^{tu} (\mathcal{C}_{quqd}^{(1)})^{trsu} T_b^{Aa} B_\mu G_\mu^A (\bar{q}_{as} \tilde{H} u_r^b) \\
& + \frac{i}{12} g_Y \bar{y}_d^{tu} \left[ (\bar{\mathcal{C}}_{quqd}^{(1)})^{tsru} + 6(\bar{\mathcal{C}}_{quqd}^{(1)})^{rstu} \right] B_\mu (\bar{u}_s \tilde{H}^\dagger \partial^\mu q_r) + \frac{i}{12} g_Y y_d^{tu} \left[ (\bar{\mathcal{C}}_{quqd}^{(1)})^{tsru} + 6(\bar{\mathcal{C}}_{quqd}^{(1)})^{rstu} \right] B_\mu (\bar{u}_s \partial^\mu \tilde{H} q_r) \\
& + \frac{1}{12} g_s g_Y y_d^{tu} (\bar{\mathcal{C}}_{quqd}^{(1)})^{tsru} T_b^{Aa} B_\mu G_\mu^A (\bar{u}_{as} \tilde{H}^\dagger q_r^b) + \frac{i}{12} g_Y \left[ y_u^{ut} (\bar{\mathcal{C}}_{quqd}^{(1)})^{rtus} + 6y_u^{tu} (\bar{\mathcal{C}}_{quqd}^{(1)})^{turs} \right] B_\mu (\partial^\mu \bar{d}_s H^\dagger q_r) \\
& - \frac{i}{12} g_Y \bar{y}_u^{tu} \left[ (\mathcal{C}_{quqd}^{(1)})^{sutr} + 6(\mathcal{C}_{quqd}^{(1)})^{tusr} \right] B_\mu (\partial^\mu \bar{q}_s H d_r) - \frac{i}{12} g_Y \bar{y}_d^{tu} \left[ (\mathcal{C}_{quqd}^{(1)})^{trsu} + 6(\mathcal{C}_{quqd}^{(1)})^{srtu} \right] B_\mu (\partial^\mu \bar{q}_s \tilde{H} u_r) \\
& + \frac{i}{12} g_Y y_d^{tu} \left[ (\bar{\mathcal{C}}_{quqd}^{(1)})^{tsru} + 6(\bar{\mathcal{C}}_{quqd}^{(1)})^{rstu} \right] B_\mu (\partial^\mu \bar{u}_s \tilde{H}^\dagger q_r) + \frac{1}{8} g_L^2 \left[ y_u^{ut} (\bar{\mathcal{C}}_{quqd}^{(1)})^{rtus} + 6y_u^{tu} (\bar{\mathcal{C}}_{quqd}^{(1)})^{turs} \right] W_\mu^{I2} (\bar{d}_s H^\dagger q_r) \\
& + \frac{1}{8} g_L^2 \bar{y}_u^{tu} \left[ (\mathcal{C}_{quqd}^{(1)})^{sutr} + 6(\mathcal{C}_{quqd}^{(1)})^{tusr} \right] W_\mu^{I2} (\bar{q}_s H d_r) - \frac{7}{72} g_Y^2 y_d^{tu} \left[ (\bar{\mathcal{C}}_{quqd}^{(1)})^{tsru} + 6(\bar{\mathcal{C}}_{quqd}^{(1)})^{rstu} \right] B_\mu^2 (\bar{u}_s \tilde{H}^\dagger q_r)
\end{aligned}$$

$$\begin{aligned}
& + \frac{i}{6} g_L \left[ y_u^{ut} (\bar{\mathcal{C}}_{quqd}^{(1)})^{rtus} + 6 y_u^{tu} (\bar{\mathcal{C}}_{quqd}^{(1)})^{turs} \right] t_j^{Ii} H_i^\dagger W_\mu^I (\bar{d}_s \partial^\mu q_r^j) \\
& + \frac{i}{6} g_s^2 y_u^{ut} (\bar{\mathcal{C}}_{quqd}^{(1)})^{rtus} T_b^{Aa} T_a^{Bc} G_\mu^B G_\nu^A (\bar{d}_{cs} \sigma^{\mu\nu} H^\dagger q_r^b) + \frac{1}{6} g_L g_Y \bar{y}_u^{tu} \left[ (\mathcal{C}_{quqd}^{(1)})^{sutr} + 6 (\mathcal{C}_{quqd}^{(1)})^{tusr} \right] t_j^{Ii} H^j B_\mu W_\mu^I (\bar{q}_{is} d_r) \\
& - \frac{i}{6} g_L \bar{y}_d^{tu} \left[ (\mathcal{C}_{quqd}^{(1)})^{trsu} + 6 (\mathcal{C}_{quqd}^{(1)})^{srtu} \right] \varepsilon^{jk} t_j^{Ii} H_i^\dagger W_\mu^I (\bar{q}_{ks} \partial^\mu u_r) \\
& - \frac{i}{6} g_L g_Y \bar{y}_d^{tu} (\mathcal{C}_{quqd}^{(1)})^{trsu} \varepsilon^{jk} t_j^{Ii} H_i^\dagger B_\mu W_\nu^I (\bar{q}_{ks} \sigma^{\mu\nu} u_r) - \frac{i}{6} g_s^2 \bar{y}_d^{tu} (\mathcal{C}_{quqd}^{(1)})^{trsu} T_b^{Aa} T_a^{Bc} G_\mu^B G_\nu^A (\bar{q}_{cs} \tilde{H} \sigma^{\mu\nu} u_r^b) \\
& + \frac{i}{6} g_L \bar{y}_d^{tu} \left[ (\bar{\mathcal{C}}_{quqd}^{(1)})^{tsru} + 6 (\bar{\mathcal{C}}_{quqd}^{(1)})^{rstu} \right] \bar{\varepsilon}_{ij} t_k^{Ii} H^k W_\mu^I (\bar{u}_s \partial^\mu q_r^j) \\
& + \frac{i}{6} g_L g_Y \bar{y}_d^{tu} (\bar{\mathcal{C}}_{quqd}^{(1)})^{tsru} \bar{\varepsilon}_{ij} t_k^{Ii} H^k B_\mu W_\nu^I (\bar{u}_s \sigma^{\mu\nu} q_r^j) \\
& + \frac{i}{6} g_s^2 \bar{y}_d^{tu} (\bar{\mathcal{C}}_{quqd}^{(1)})^{tsru} T_b^{Aa} T_c^{Bb} G_\mu^B G_\nu^A (\bar{u}_{as} \sigma^{\mu\nu} \tilde{H}^\dagger q_r^c) \\
& + \frac{i}{6} g_L \left[ y_u^{ut} (\bar{\mathcal{C}}_{quqd}^{(1)})^{rtus} + 6 y_u^{tu} (\bar{\mathcal{C}}_{quqd}^{(1)})^{turs} \right] t_j^{Ii} H_i^\dagger W_\mu^I (\partial^\mu \bar{d}_s q_r^j) \\
& - \frac{i}{6} g_L \bar{y}_u^{tu} \left[ (\mathcal{C}_{quqd}^{(1)})^{sutr} + 6 (\mathcal{C}_{quqd}^{(1)})^{tusr} \right] t_j^{Ii} H^j W_\mu^I (\partial^\mu \bar{q}_{is} d_r) \\
& - \frac{i}{6} g_L \bar{y}_d^{tu} \left[ (\mathcal{C}_{quqd}^{(1)})^{trsu} + 6 (\mathcal{C}_{quqd}^{(1)})^{srtu} \right] \varepsilon^{jk} t_j^{Ii} H_i^\dagger W_\mu^I (\partial^\mu \bar{q}_{ks} u_r) \\
& + \frac{i}{6} g_L \bar{y}_d^{tu} \left[ (\bar{\mathcal{C}}_{quqd}^{(1)})^{tsru} + 6 (\bar{\mathcal{C}}_{quqd}^{(1)})^{rstu} \right] \bar{\varepsilon}_{ij} t_k^{Ii} H^k W_\mu^I (\partial^\mu \bar{u}_s q_r^j) \\
& - \frac{i}{6} g_L \left[ y_u^{ut} (\bar{\mathcal{C}}_{quqd}^{(1)})^{rtus} + 6 y_u^{tu} (\bar{\mathcal{C}}_{quqd}^{(1)})^{turs} \right] t_j^{Ii} W_\mu^I (\bar{d}_s q_r^j) \partial^\mu H_i^\dagger \\
& + \frac{i}{6} g_L \bar{y}_d^{tu} \left[ (\mathcal{C}_{quqd}^{(1)})^{trsu} + 6 (\mathcal{C}_{quqd}^{(1)})^{srtu} \right] \varepsilon^{ij} t_i^{Ik} W_\mu^I (\bar{q}_{js} u_r) \partial^\mu H_k^\dagger \\
& + \frac{i}{6} g_L \bar{y}_u^{tu} \left[ (\mathcal{C}_{quqd}^{(1)})^{sutr} + 6 (\mathcal{C}_{quqd}^{(1)})^{tusr} \right] t_j^{Ii} W_\mu^I (\bar{q}_{is} d_r) \partial^\mu H^j \\
& - \frac{i}{6} g_L \bar{y}_d^{tu} \left[ (\bar{\mathcal{C}}_{quqd}^{(1)})^{tsru} + 6 (\bar{\mathcal{C}}_{quqd}^{(1)})^{rstu} \right] \bar{\varepsilon}_{ij} t_k^{Ii} W_\mu^I (\bar{u}_s q_r^j) \partial^\mu H^k \\
& + \frac{13}{72} g_Y^2 \left[ y_u^{ut} (\bar{\mathcal{C}}_{quqd}^{(1)})^{rtus} + 6 y_u^{tu} (\bar{\mathcal{C}}_{quqd}^{(1)})^{turs} \right] B_\mu^2 (\bar{d}_s H^\dagger q_r) + \frac{13}{72} g_Y^2 \bar{y}_u^{tu} \left[ (\mathcal{C}_{quqd}^{(1)})^{sutr} + 6 (\mathcal{C}_{quqd}^{(1)})^{tusr} \right] B_\mu^2 (\bar{q}_s H d_r) \\
& - \frac{7}{72} g_Y^2 \bar{y}_d^{tu} \left[ (\mathcal{C}_{quqd}^{(1)})^{trsu} + 6 (\mathcal{C}_{quqd}^{(1)})^{srtu} \right] B_\mu^2 (\bar{q}_s \tilde{H} u_r) - \frac{i}{6} g_L \bar{y}_u^{tu} \left[ (\mathcal{C}_{quqd}^{(1)})^{sutr} + 6 (\mathcal{C}_{quqd}^{(1)})^{tusr} \right] t_j^{Ii} H^j W_\mu^I (\bar{q}_{is} \partial^\mu d_r) \\
& + \frac{i}{4} g_s g_Y y_u^{ut} (\bar{\mathcal{C}}_{quqd}^{(1)})^{rtus} T_b^{Aa} B_\mu G_\nu^A (\bar{d}_{as} \sigma^{\mu\nu} H^\dagger q_r^b) - \frac{i}{4} g_s g_Y \bar{y}_u^{tu} (\mathcal{C}_{quqd}^{(1)})^{sutr} T_b^{Aa} B_\mu G_\nu^A (\bar{q}_{as} H \sigma^{\mu\nu} d_r^b) \\
& + \frac{i}{4} g_s g_Y \bar{y}_d^{tu} (\bar{\mathcal{C}}_{quqd}^{(1)})^{tsru} T_b^{Aa} B_\mu G_\nu^A (\bar{u}_{as} \sigma^{\mu\nu} \tilde{H}^\dagger q_r^b) - \frac{i}{3} g_L^2 \bar{y}_d^{tu} (\mathcal{C}_{quqd}^{(1)})^{trsu} t_l^{Ik} t_j^{Jl} \tilde{H}_j W_\mu^I W_\nu^J (\bar{q}_{ks} \sigma^{\mu\nu} u_r) \\
& + \frac{1}{3} g_L y_u^{ut} (\bar{\mathcal{C}}_{quqd}^{(1)})^{rtus} t_j^{Ii} W_\mu^I (\bar{d}_s \sigma^{\mu\nu} q_r^j) \partial^\nu H_i^\dagger + \frac{1}{3} g_L \bar{y}_d^{tu} (\mathcal{C}_{quqd}^{(1)})^{trsu} \varepsilon^{ij} t_i^{Ik} W_\mu^I (\bar{q}_{js} \sigma^{\mu\nu} u_r) \partial^\nu H_k^\dagger \\
& + \frac{1}{3} g_L \bar{y}_u^{tu} (\mathcal{C}_{quqd}^{(1)})^{sutr} t_j^{Ii} W_\mu^I (\bar{q}_{is} \sigma^{\mu\nu} d_r) \partial^\nu H^j + \frac{1}{3} g_L \bar{y}_d^{tu} (\bar{\mathcal{C}}_{quqd}^{(1)})^{tsru} \bar{\varepsilon}_{ij} t_k^{Ii} W_\mu^I (\bar{u}_s \sigma^{\mu\nu} q_r^j) \partial^\nu H^k \\
& + \frac{5}{12} g_s g_Y y_u^{ut} (\bar{\mathcal{C}}_{quqd}^{(1)})^{rtus} T_b^{Aa} B_\mu G_\mu^A (\bar{d}_{as} H^\dagger q_r^b) + \frac{5}{12} g_s g_Y \bar{y}_u^{tu} (\mathcal{C}_{quqd}^{(1)})^{sutr} T_b^{Aa} B_\mu G_\mu^A (\bar{q}_{as} H d_r^b) \\
& + \frac{1}{2} g_s^2 y_u^{tu} (\bar{\mathcal{C}}_{quqd}^{(1)})^{turs} G_\mu^A{}^2 (\bar{d}_s H^\dagger q_r) + \frac{1}{2} g_s^2 y_u^{ut} (\bar{\mathcal{C}}_{quqd}^{(1)})^{rtus} T_b^{Aa} T_a^{Bc} G_\mu^A G_\mu^B (\bar{d}_{cs} H^\dagger q_r^b)
\end{aligned}$$

$$\begin{aligned}
& + \frac{1}{2} g_s^2 \bar{y}_u^{tu} (\mathcal{C}_{quqd}^{(1)})^{tusr} G_{\bar{\mu}}^{A2} (\bar{q}_s H d_r) + \frac{1}{2} g_s^2 \bar{y}_u^{tu} (\mathcal{C}_{quqd}^{(1)})^{sutr} T_b^{Aa} T_c^{Bb} G_{\bar{\mu}}^A G_{\bar{\mu}}^B (\bar{q}_{as} H d_r^c) \\
& + \frac{2}{3} g_s y_d^{tu} (\bar{\mathcal{C}}_{quqd}^{(1)})^{tsru} T_b^{Aa} G_{\bar{\mu}}^A (\bar{u}_{as} \sigma^{\bar{\mu}\bar{\nu}} \partial^{\bar{\nu}} \tilde{H} q_r^b) \\
& + g_L g_Y \left[ \frac{1}{6} y_u^{ut} (\bar{\mathcal{C}}_{quqd}^{(1)})^{rtus} + y_u^{tu} (\bar{\mathcal{C}}_{quqd}^{(1)})^{turs} \right] t_j^{Ii} H_i^\dagger B_{\bar{\mu}} W_{\bar{\mu}}^I (\bar{d}_s q_r^j) \\
& - \frac{1}{6} g_L^2 y_u^{ut} (\bar{\mathcal{C}}_{quqd}^{(1)})^{rtus} \varepsilon^{IJK} t_j^{Ki} H_i^\dagger W_{\bar{\mu}}^J W_{\bar{\nu}}^I (\bar{d}_s \sigma^{\bar{\mu}\bar{\nu}} q_r^j) \\
& - \frac{1}{6} g_L^2 \bar{y}_u^{tu} (\mathcal{C}_{quqd}^{(1)})^{sutr} \varepsilon^{IJK} t_j^{Ki} H^j W_{\bar{\mu}}^J W_{\bar{\nu}}^I (\bar{q}_{is} \sigma^{\bar{\mu}\bar{\nu}} d_r) - \frac{i}{6} g_s^2 \bar{y}_u^{tu} (\mathcal{C}_{quqd}^{(1)})^{sutr} T_b^{Aa} T_c^{Bb} G_{\bar{\mu}}^B G_{\bar{\nu}}^A (\bar{q}_{as} H \sigma^{\bar{\mu}\bar{\nu}} d_r^c) \\
& - \frac{i}{4} g_s g_Y \bar{y}_d^{tu} (\mathcal{C}_{quqd}^{(1)})^{trsu} T_b^{Aa} B_{\bar{\mu}} G_{\bar{\nu}}^A (\bar{q}_{as} \tilde{H} \sigma^{\bar{\mu}\bar{\nu}} u_r^b) + \frac{2}{3} g_s \bar{y}_d^{tu} (\mathcal{C}_{quqd}^{(1)})^{trsu} T_b^{Aa} G_{\bar{\mu}}^A (\bar{q}_{as} \partial^{\bar{\nu}} \tilde{H} \sigma^{\bar{\mu}\bar{\nu}} u_r^b) \\
& - \frac{5}{18} g_Y y_u^{ut} (\bar{\mathcal{C}}_{quqd}^{(1)})^{rtus} B_{\bar{\mu}} (\bar{d}_s \sigma^{\bar{\mu}\bar{\nu}} \partial^{\bar{\nu}} H^\dagger q_r) - \frac{5}{18} g_Y \bar{y}_u^{tu} (\mathcal{C}_{quqd}^{(1)})^{sutr} B_{\bar{\mu}} (\bar{q}_s \partial^{\bar{\nu}} H \sigma^{\bar{\mu}\bar{\nu}} d_r) \\
& - \frac{i}{3} g_L g_Y y_u^{ut} (\bar{\mathcal{C}}_{quqd}^{(1)})^{rtus} t_j^{Ii} H_i^\dagger B_{\bar{\mu}} W_{\bar{\nu}}^I (\bar{d}_s \sigma^{\bar{\mu}\bar{\nu}} q_r^j) + \frac{i}{3} g_L g_Y \bar{y}_u^{tu} (\mathcal{C}_{quqd}^{(1)})^{sutr} t_j^{Ii} H^j B_{\bar{\mu}} W_{\bar{\nu}}^I (\bar{q}_{is} \sigma^{\bar{\mu}\bar{\nu}} d_r) \\
& - \frac{1}{3} g_L g_Y \bar{y}_d^{tu} \left[ (\mathcal{C}_{quqd}^{(1)})^{trsu} + 6(\mathcal{C}_{quqd}^{(1)})^{srtu} \right] t_j^{Ik} \tilde{H}_j B_{\bar{\mu}} W_{\bar{\mu}}^I (\bar{q}_{ks} u_r) \\
& - \frac{1}{3} g_L g_Y y_d^{tu} \left[ (\bar{\mathcal{C}}_{quqd}^{(1)})^{tsru} + 6(\bar{\mathcal{C}}_{quqd}^{(1)})^{rstu} \right] t_k^{Ii} \tilde{H}^\dagger{}^i B_{\bar{\mu}} W_{\bar{\mu}}^I (\bar{u}_s q_r^k) \\
& + \frac{i}{3} g_L^2 y_d^{tu} (\bar{\mathcal{C}}_{quqd}^{(1)})^{tsru} t_l^{Ik} t_k^{Ji} \tilde{H}^\dagger{}^i W_{\bar{\mu}}^I W_{\bar{\nu}}^J (\bar{u}_s \sigma^{\bar{\mu}\bar{\nu}} q_r^l) - \frac{1}{2} g_L g_s y_u^{ut} (\bar{\mathcal{C}}_{quqd}^{(1)})^{rtus} t_j^{Ii} T_b^{Aa} H_i^\dagger G_{\bar{\mu}}^A W_{\bar{\mu}}^I (\bar{d}_{as} q_r^{bj}) \\
& - \frac{i}{2} g_L g_s y_u^{ut} (\bar{\mathcal{C}}_{quqd}^{(1)})^{rtus} t_j^{Ii} T_b^{Aa} H_i^\dagger G_{\bar{\mu}}^A W_{\bar{\nu}}^I (\bar{d}_{as} \sigma^{\bar{\mu}\bar{\nu}} q_r^{bj}) - \frac{1}{2} g_s^2 \bar{y}_d^{tu} (\mathcal{C}_{quqd}^{(1)})^{srtu} G_{\bar{\mu}}^{A2} (\bar{q}_s \tilde{H} u_r) \\
& - \frac{1}{2} g_L^2 \bar{y}_d^{tu} \left[ (\mathcal{C}_{quqd}^{(1)})^{trsu} + 6(\mathcal{C}_{quqd}^{(1)})^{srtu} \right] \varepsilon^{jk} t_l^{Ii} t_j^{Jl} H_i^\dagger W_{\bar{\mu}}^I W_{\bar{\mu}}^J (\bar{q}_{ks} u_r) \\
& - \frac{1}{2} g_s^2 \bar{y}_d^{tu} (\mathcal{C}_{quqd}^{(1)})^{trsu} T_b^{Aa} T_a^{Bc} G_{\bar{\mu}}^A G_{\bar{\mu}}^B (\bar{q}_{cs} \tilde{H} u_r^b) - \frac{1}{2} g_L g_s \bar{y}_u^{tu} (\mathcal{C}_{quqd}^{(1)})^{sutr} t_j^{Ii} T_b^{Aa} H^j G_{\bar{\mu}}^A W_{\bar{\mu}}^I (\bar{q}_{ais} d_r^b) \\
& + \frac{i}{2} g_L g_s \bar{y}_u^{tu} (\mathcal{C}_{quqd}^{(1)})^{sutr} t_j^{Ii} T_b^{Aa} H^j G_{\bar{\mu}}^A W_{\bar{\nu}}^I (\bar{q}_{ais} \sigma^{\bar{\mu}\bar{\nu}} d_r^b) - \frac{1}{2} g_L g_s \bar{y}_d^{tu} (\mathcal{C}_{quqd}^{(1)})^{trsu} t_j^{Ik} T_b^{Aa} \tilde{H}_j G_{\bar{\mu}}^A W_{\bar{\mu}}^I (\bar{q}_{aks} u_r^b) \\
& + \frac{i}{2} g_L g_s \bar{y}_d^{tu} (\mathcal{C}_{quqd}^{(1)})^{trsu} \varepsilon^{jk} t_j^{Ii} T_b^{Aa} H_i^\dagger G_{\bar{\mu}}^A W_{\bar{\nu}}^I (\bar{q}_{aks} \sigma^{\bar{\mu}\bar{\nu}} u_r^b) \\
& - \frac{1}{2} g_L^2 y_d^{tu} \left[ (\bar{\mathcal{C}}_{quqd}^{(1)})^{tsru} + 6(\bar{\mathcal{C}}_{quqd}^{(1)})^{rstu} \right] \bar{\varepsilon}_{ij} t_l^{Ik} t_k^{Ji} H^l W_{\bar{\mu}}^I W_{\bar{\mu}}^J (\bar{u}_s q_r^j) - \frac{1}{2} g_s^2 y_d^{tu} (\bar{\mathcal{C}}_{quqd}^{(1)})^{rstu} G_{\bar{\mu}}^{A2} (\bar{u}_s \tilde{H}^\dagger q_r) \\
& - \frac{1}{2} g_L g_s y_d^{tu} (\bar{\mathcal{C}}_{quqd}^{(1)})^{tsru} t_k^{Ii} T_b^{Aa} \tilde{H}^\dagger{}^i G_{\bar{\mu}}^A W_{\bar{\mu}}^I (\bar{u}_{as} q_r^{bk}) - \frac{1}{2} g_s^2 y_d^{tu} (\bar{\mathcal{C}}_{quqd}^{(1)})^{tsru} T_b^{Aa} T_c^{Bb} G_{\bar{\mu}}^A G_{\bar{\mu}}^B (\bar{u}_{as} \tilde{H}^\dagger q_r^c) \\
& - \frac{i}{2} g_L g_s y_d^{tu} (\bar{\mathcal{C}}_{quqd}^{(1)})^{tsru} \bar{\varepsilon}_{ij} t_k^{Ii} T_b^{Aa} H^k G_{\bar{\mu}}^A W_{\bar{\nu}}^I (\bar{u}_{as} \sigma^{\bar{\mu}\bar{\nu}} q_r^{bj}) \\
& - \frac{2}{3} g_s y_u^{ut} (\bar{\mathcal{C}}_{quqd}^{(1)})^{rtus} T_b^{Aa} G_{\bar{\mu}}^A (\bar{d}_{as} \sigma^{\bar{\mu}\bar{\nu}} \partial^{\bar{\nu}} H^\dagger q_r^b) - \frac{2}{3} g_s \bar{y}_u^{tu} (\mathcal{C}_{quqd}^{(1)})^{sutr} T_b^{Aa} G_{\bar{\mu}}^A (\bar{q}_{as} \partial^{\bar{\nu}} H \sigma^{\bar{\mu}\bar{\nu}} d_r^b), \quad (2.60)
\end{aligned}$$

$$\begin{aligned}
\Delta S_{\mathcal{O}_{quqd}^{(8)}} & = \frac{1}{72} g_s g_Y \bar{y}_d^{tu} \left[ 6(\mathcal{C}_{quqd}^{(8)})^{srtu} - (\mathcal{C}_{quqd}^{(8)})^{trsu} \right] T_b^{Aa} B_{\bar{\mu}} G_{\bar{\mu}}^A (\bar{q}_{as} \tilde{H} u_r^b) \\
& + \frac{1}{72} g_s g_Y y_d^{tu} \left[ 6(\bar{\mathcal{C}}_{quqd}^{(8)})^{rstu} - (\bar{\mathcal{C}}_{quqd}^{(8)})^{tsru} \right] T_b^{Aa} B_{\bar{\mu}} G_{\bar{\mu}}^A (\bar{u}_{as} \tilde{H}^\dagger q_r^b) \\
& - \frac{i}{36} g_s^2 y_u^{ut} (\bar{\mathcal{C}}_{quqd}^{(8)})^{rtus} T_b^{Aa} T_a^{Bc} G_{\bar{\mu}}^B G_{\bar{\nu}}^A (\bar{d}_{cs} \sigma^{\bar{\mu}\bar{\nu}} H^\dagger q_r^b) + \frac{i}{36} g_s^2 \bar{y}_u^{tu} (\mathcal{C}_{quqd}^{(8)})^{sutr} T_b^{Aa} T_c^{Bb} G_{\bar{\mu}}^B G_{\bar{\nu}}^A (\bar{q}_{as} H \sigma^{\bar{\mu}\bar{\nu}} d_r^c)
\end{aligned}$$

$$\begin{aligned}
& + \frac{i}{36} g_s^2 \bar{y}_d^{tu} (\mathcal{C}_{quqd}^{(8)})^{trsu} T_b^{Aa} T_a^{Bc} G_{\bar{\mu}}^B G_{\bar{\nu}}^A (\bar{q}_{cs} \tilde{H} \sigma^{\bar{\mu}\bar{\nu}} u_r^b) \\
& - \frac{i}{36} g_s^2 \bar{y}_d^{tu} (\bar{\mathcal{C}}_{quqd}^{(8)})^{tsru} T_b^{Aa} T_c^{Bb} G_{\bar{\mu}}^B G_{\bar{\nu}}^A (\bar{u}_{as} \sigma^{\bar{\mu}\bar{\nu}} \tilde{H}^\dagger q_r^c) \\
& + \frac{1}{24} g_s^2 \left[ 3 y_u^{ut} (\bar{\mathcal{C}}_{quqd}^{(8)})^{rtus} - 2 y_u^{tu} (\bar{\mathcal{C}}_{quqd}^{(8)})^{turs} \right] G_{\bar{\mu}}^{A2} (\bar{d}_s H^\dagger q_r) - \frac{i}{24} g_s g_Y y_u^{ut} (\bar{\mathcal{C}}_{quqd}^{(8)})^{rtus} T_b^{Aa} B_{\bar{\mu}} G_{\bar{\nu}}^A (\bar{d}_{as} \sigma^{\bar{\mu}\bar{\nu}} H^\dagger q_r^b) \\
& + \frac{1}{24} g_s^2 \bar{y}_u^{tu} \left[ 3 (\mathcal{C}_{quqd}^{(8)})^{sutr} - 2 (\mathcal{C}_{quqd}^{(8)})^{tusr} \right] G_{\bar{\mu}}^{A2} (\bar{q}_s H d_r) + \frac{1}{24} g_s^2 \bar{y}_d^{tu} \left[ 2 (\mathcal{C}_{quqd}^{(8)})^{srtu} - 3 (\mathcal{C}_{quqd}^{(8)})^{trsu} \right] G_{\bar{\mu}}^{A2} (\bar{q}_s \tilde{H} u_r) \\
& + \frac{i}{24} g_s g_Y \bar{y}_u^{tu} (\mathcal{C}_{quqd}^{(8)})^{sutr} T_b^{Aa} B_{\bar{\mu}} G_{\bar{\nu}}^A (\bar{q}_{as} H \sigma^{\bar{\mu}\bar{\nu}} d_r^b) + \frac{i}{24} g_s g_Y \bar{y}_d^{tu} (\mathcal{C}_{quqd}^{(8)})^{trsu} T_b^{Aa} B_{\bar{\mu}} G_{\bar{\nu}}^A (\bar{q}_{as} \tilde{H} \sigma^{\bar{\mu}\bar{\nu}} u_r^b) \\
& + \frac{1}{24} g_s^2 y_d^{tu} \left[ 2 (\bar{\mathcal{C}}_{quqd}^{(8)})^{rstu} - 3 (\bar{\mathcal{C}}_{quqd}^{(8)})^{tsru} \right] G_{\bar{\mu}}^{A2} (\bar{u}_s \tilde{H}^\dagger q_r) - \frac{i}{24} g_s g_Y y_d^{tu} (\bar{\mathcal{C}}_{quqd}^{(8)})^{tsru} T_b^{Aa} B_{\bar{\mu}} G_{\bar{\nu}}^A (\bar{u}_{as} \sigma^{\bar{\mu}\bar{\nu}} \tilde{H}^\dagger q_r^b) \\
& + \frac{5}{72} g_s g_Y \left[ 6 y_u^{tu} (\bar{\mathcal{C}}_{quqd}^{(8)})^{turs} - y_u^{ut} (\bar{\mathcal{C}}_{quqd}^{(8)})^{rtus} \right] T_b^{Aa} B_{\bar{\mu}} G_{\bar{\mu}}^A (\bar{d}_{as} H^\dagger q_r^b) + \frac{2}{27} g_Y \bar{y}_d^{tu} (\mathcal{C}_{quqd}^{(8)})^{trsu} B_{\bar{\mu}} (\bar{q}_s \partial^{\bar{\nu}} \tilde{H} \sigma^{\bar{\mu}\bar{\nu}} u_r) \\
& + \frac{2}{27} g_Y y_d^{tu} (\bar{\mathcal{C}}_{quqd}^{(8)})^{tsru} B_{\bar{\mu}} (\bar{u}_s \sigma^{\bar{\mu}\bar{\nu}} \partial^{\bar{\nu}} \tilde{H} q_r) \\
& + \frac{1}{12} g_L g_s \left[ y_u^{ut} (\bar{\mathcal{C}}_{quqd}^{(8)})^{rtus} - 6 y_u^{tu} (\bar{\mathcal{C}}_{quqd}^{(8)})^{turs} \right] t_j^{Ii} T_b^{Aa} H_i^\dagger G_{\bar{\mu}}^A W_{\bar{\mu}}^I (\bar{d}_{as} q_r^{bj}) \\
& + \frac{i}{12} g_L g_s y_u^{ut} (\bar{\mathcal{C}}_{quqd}^{(8)})^{rtus} t_j^{Ii} T_b^{Aa} H_i^\dagger G_{\bar{\mu}}^A W_{\bar{\nu}}^I (\bar{d}_{as} \sigma^{\bar{\mu}\bar{\nu}} q_r^{bj}) \\
& + \frac{1}{12} g_s^2 \left[ 6 y_u^{tu} (\bar{\mathcal{C}}_{quqd}^{(8)})^{turs} - y_u^{ut} (\bar{\mathcal{C}}_{quqd}^{(8)})^{rtus} \right] T_b^{Aa} T_a^{Bc} G_{\bar{\mu}}^A G_{\bar{\mu}}^B (\bar{d}_{cs} H^\dagger q_r^b) \\
& + \frac{1}{12} g_s^2 \bar{y}_d^{tu} \left[ (\mathcal{C}_{quqd}^{(8)})^{trsu} - 6 (\mathcal{C}_{quqd}^{(8)})^{srtu} \right] T_b^{Aa} T_a^{Bc} G_{\bar{\mu}}^A G_{\bar{\mu}}^B (\bar{q}_{cs} \tilde{H} u_r^b) \\
& + \frac{1}{12} g_L g_s \bar{y}_u^{tu} \left[ (\mathcal{C}_{quqd}^{(8)})^{sutr} - 6 (\mathcal{C}_{quqd}^{(8)})^{tusr} \right] t_j^{Ii} T_b^{Aa} H^j G_{\bar{\mu}}^A W_{\bar{\mu}}^I (\bar{q}_{ais} d_r^b) \\
& - \frac{i}{12} g_L g_s \bar{y}_u^{tu} (\mathcal{C}_{quqd}^{(8)})^{sutr} t_j^{Ii} T_b^{Aa} H^j G_{\bar{\mu}}^A W_{\bar{\nu}}^I (\bar{q}_{ais} \sigma^{\bar{\mu}\bar{\nu}} d_r^b) \\
& + \frac{1}{12} g_L g_s \bar{y}_d^{tu} \left[ (\mathcal{C}_{quqd}^{(8)})^{trsu} - 6 (\mathcal{C}_{quqd}^{(8)})^{srtu} \right] t_j^{Ik} T_b^{Aa} \tilde{H}_j G_{\bar{\mu}}^A W_{\bar{\mu}}^I (\bar{q}_{aks} u_r^b) \\
& - \frac{i}{12} g_L g_s \bar{y}_d^{tu} (\mathcal{C}_{quqd}^{(8)})^{trsu} \varepsilon^{jk} t_j^{Ii} T_b^{Aa} H_i^\dagger G_{\bar{\mu}}^A W_{\bar{\nu}}^I (\bar{q}_{aks} \sigma^{\bar{\mu}\bar{\nu}} u_r^b) \\
& + \frac{1}{12} g_L g_s y_d^{tu} \left[ (\bar{\mathcal{C}}_{quqd}^{(8)})^{tsru} - 6 (\bar{\mathcal{C}}_{quqd}^{(8)})^{rstu} \right] t_k^{Ii} T_b^{Aa} \tilde{H}^\dagger i G_{\bar{\mu}}^A W_{\bar{\mu}}^I (\bar{u}_{as} q_r^{bk}) \\
& + \frac{1}{12} g_s^2 \bar{y}_d^{tu} \left[ (\bar{\mathcal{C}}_{quqd}^{(8)})^{tsru} - 6 (\bar{\mathcal{C}}_{quqd}^{(8)})^{rstu} \right] T_b^{Aa} T_c^{Bb} G_{\bar{\mu}}^A G_{\bar{\mu}}^B (\bar{u}_{as} \tilde{H}^\dagger q_r^c) \\
& + \frac{i}{12} g_L g_s y_d^{tu} (\bar{\mathcal{C}}_{quqd}^{(8)})^{tsru} \bar{\varepsilon}_{ij} t_k^{Ii} T_b^{Aa} H^k G_{\bar{\mu}}^A W_{\bar{\nu}}^I (\bar{u}_{as} \sigma^{\bar{\mu}\bar{\nu}} q_r^{bj}) + \frac{i}{9} g_Y y_u^{ut} (\bar{\mathcal{C}}_{quqd}^{(8)})^{rtus} B_{\bar{\mu}} (\bar{d}_s H^\dagger \partial^{\bar{\mu}} q_r) \\
& - \frac{i}{9} g_Y y_u^{ut} (\bar{\mathcal{C}}_{quqd}^{(8)})^{rtus} B_{\bar{\mu}} (\bar{d}_s \partial^{\bar{\mu}} H^\dagger q_r) + \frac{1}{9} g_s y_u^{ut} (\bar{\mathcal{C}}_{quqd}^{(8)})^{rtus} T_b^{Aa} G_{\bar{\mu}}^A (\bar{d}_{as} \sigma^{\bar{\mu}\bar{\nu}} \partial^{\bar{\nu}} H^\dagger q_r^b) \\
& - \frac{i}{9} g_Y \bar{y}_u^{tu} (\mathcal{C}_{quqd}^{(8)})^{sutr} B_{\bar{\mu}} (\bar{q}_s H \partial^{\bar{\mu}} d_r) - \frac{i}{9} g_Y \bar{y}_d^{tu} (\mathcal{C}_{quqd}^{(8)})^{trsu} B_{\bar{\mu}} (\bar{q}_s \tilde{H} \partial^{\bar{\mu}} u_r) + \frac{i}{9} g_Y \bar{y}_u^{tu} (\mathcal{C}_{quqd}^{(8)})^{sutr} B_{\bar{\mu}} (\bar{q}_s \partial^{\bar{\mu}} H d_r) \\
& - \frac{i}{9} g_Y \bar{y}_d^{tu} (\mathcal{C}_{quqd}^{(8)})^{trsu} B_{\bar{\mu}} (\bar{q}_s \partial^{\bar{\mu}} \tilde{H} u_r) + \frac{1}{9} g_s \bar{y}_u^{tu} (\mathcal{C}_{quqd}^{(8)})^{sutr} T_b^{Aa} G_{\bar{\mu}}^A (\bar{q}_{as} \partial^{\bar{\nu}} H \sigma^{\bar{\mu}\bar{\nu}} d_r^b) \\
& + \frac{i}{9} g_Y y_d^{tu} (\bar{\mathcal{C}}_{quqd}^{(8)})^{tsru} B_{\bar{\mu}} (\bar{u}_s \tilde{H}^\dagger \partial^{\bar{\mu}} q_r) + \frac{i}{9} g_Y y_d^{tu} (\bar{\mathcal{C}}_{quqd}^{(8)})^{tsru} B_{\bar{\mu}} (\bar{u}_s \partial^{\bar{\mu}} \tilde{H} q_r)
\end{aligned}$$

$$\begin{aligned}
& + \frac{1}{6} g_L^2 y_u^{ut} (\bar{\mathcal{C}}_{quqd}^{(8)})^{rtus} W_{\bar{\mu}}^I{}^2 (\bar{d}_s H^\dagger q_r) + \frac{1}{6} g_L^2 \bar{y}_u^{tu} (\mathcal{C}_{quqd}^{(8)})^{sutr} W_{\bar{\mu}}^I{}^2 (\bar{q}_s H d_r) + \frac{2}{9} g_L g_Y y_u^{ut} (\bar{\mathcal{C}}_{quqd}^{(8)})^{rtus} t_j^{Ii} H_i^\dagger B_{\bar{\mu}} W_{\bar{\mu}}^I (\bar{d}_s q_r^j) \\
& - \frac{1}{9} g_s y_d^{tu} (\bar{\mathcal{C}}_{quqd}^{(8)})^{tsru} T_b^{Aa} G_{\bar{\mu}}^A (\bar{u}_{as} \sigma^{\bar{\mu}\bar{\nu}} \partial^{\bar{\nu}} \tilde{H} q_r^b) + \frac{i}{9} g_Y y_u^{ut} (\bar{\mathcal{C}}_{quqd}^{(8)})^{rtus} B_{\bar{\mu}} (\partial^{\bar{\mu}} \bar{d}_s H^\dagger q_r) \\
& - \frac{i}{9} g_Y \bar{y}_u^{tu} (\mathcal{C}_{quqd}^{(8)})^{sutr} B_{\bar{\mu}} (\partial^{\bar{\mu}} \bar{q}_s H d_r) - \frac{i}{9} g_Y \bar{y}_d^{tu} (\mathcal{C}_{quqd}^{(8)})^{trsu} B_{\bar{\mu}} (\partial^{\bar{\mu}} \bar{q}_s \tilde{H} u_r) \\
& + \frac{i}{9} g_Y y_d^{tu} (\bar{\mathcal{C}}_{quqd}^{(8)})^{tsru} B_{\bar{\mu}} (\partial^{\bar{\mu}} \bar{u}_s \tilde{H}^\dagger q_r) - \frac{7}{54} g_Y^2 y_d^{tu} (\bar{\mathcal{C}}_{quqd}^{(8)})^{tsru} B_{\bar{\mu}}^2 (\bar{u}_s \tilde{H}^\dagger q_r) \\
& + \frac{2i}{9} g_L y_u^{ut} (\bar{\mathcal{C}}_{quqd}^{(8)})^{rtus} t_j^{Ii} H_i^\dagger W_{\bar{\mu}}^I (\bar{d}_s \partial^{\bar{\mu}} q_r^j) + \frac{2}{9} g_L g_Y \bar{y}_u^{tu} (\mathcal{C}_{quqd}^{(8)})^{sutr} t_j^{Ii} H^j B_{\bar{\mu}} W_{\bar{\mu}}^I (\bar{q}_{is} d_r) \\
& - \frac{2i}{9} g_L \bar{y}_d^{tu} (\mathcal{C}_{quqd}^{(8)})^{trsu} \varepsilon^{jk} t_j^{Ii} H_i^\dagger W_{\bar{\mu}}^I (\bar{q}_{ks} \partial^{\bar{\mu}} u_r) - \frac{2i}{9} g_L g_Y \bar{y}_d^{tu} (\mathcal{C}_{quqd}^{(8)})^{trsu} \varepsilon^{jk} t_j^{Ii} H_i^\dagger B_{\bar{\mu}} W_{\bar{\nu}}^I (\bar{q}_{ks} \sigma^{\bar{\mu}\bar{\nu}} u_r) \\
& + \frac{2i}{9} g_L y_d^{tu} (\bar{\mathcal{C}}_{quqd}^{(8)})^{tsru} \bar{\varepsilon}_{ij} t_k^{Ii} H^k W_{\bar{\mu}}^I (\bar{u}_s \partial^{\bar{\mu}} q_r^j) + \frac{2i}{9} g_L g_Y y_d^{tu} (\bar{\mathcal{C}}_{quqd}^{(8)})^{tsru} \bar{\varepsilon}_{ij} t_k^{Ii} H^k B_{\bar{\mu}} W_{\bar{\nu}}^I (\bar{u}_s \sigma^{\bar{\mu}\bar{\nu}} q_r^j) \\
& + \frac{2i}{9} g_L y_u^{ut} (\bar{\mathcal{C}}_{quqd}^{(8)})^{rtus} t_j^{Ii} H_i^\dagger W_{\bar{\mu}}^I (\partial^{\bar{\mu}} \bar{d}_s q_r^j) - \frac{2i}{9} g_L \bar{y}_u^{tu} (\mathcal{C}_{quqd}^{(8)})^{sutr} t_j^{Ii} H^j W_{\bar{\mu}}^I (\partial^{\bar{\mu}} \bar{q}_{is} d_r) \\
& - \frac{2i}{9} g_L \bar{y}_d^{tu} (\mathcal{C}_{quqd}^{(8)})^{trsu} \varepsilon^{jk} t_j^{Ii} H_i^\dagger W_{\bar{\mu}}^I (\partial^{\bar{\mu}} \bar{q}_{ks} u_r) + \frac{2i}{9} g_L y_d^{tu} (\bar{\mathcal{C}}_{quqd}^{(8)})^{tsru} \bar{\varepsilon}_{ij} t_k^{Ii} H^k W_{\bar{\mu}}^I (\partial^{\bar{\mu}} \bar{u}_s q_r^j) \\
& - \frac{2i}{9} g_L y_u^{ut} (\bar{\mathcal{C}}_{quqd}^{(8)})^{rtus} t_j^{Ii} W_{\bar{\mu}}^I (\bar{d}_s q_r^j) \partial^{\bar{\mu}} H_i^\dagger + \frac{2i}{9} g_L \bar{y}_d^{tu} (\mathcal{C}_{quqd}^{(8)})^{trsu} \varepsilon^{ij} t_i^{Ik} W_{\bar{\mu}}^I (\bar{q}_{js} u_r) \partial^{\bar{\mu}} H_k^\dagger \\
& + \frac{2i}{9} g_L \bar{y}_u^{tu} (\mathcal{C}_{quqd}^{(8)})^{sutr} t_j^{Ii} W_{\bar{\mu}}^I (\bar{q}_{is} d_r) \partial^{\bar{\mu}} H^j - \frac{2i}{9} g_L y_d^{tu} (\bar{\mathcal{C}}_{quqd}^{(8)})^{tsru} \bar{\varepsilon}_{ij} t_k^{Ii} W_{\bar{\mu}}^I (\bar{u}_s q_r^j) \partial^{\bar{\mu}} H^k \\
& + \frac{13}{54} g_Y^2 y_u^{ut} (\bar{\mathcal{C}}_{quqd}^{(8)})^{rtus} B_{\bar{\mu}}^2 (\bar{d}_s H^\dagger q_r) + \frac{13}{54} g_Y^2 \bar{y}_u^{tu} (\mathcal{C}_{quqd}^{(8)})^{sutr} B_{\bar{\mu}}^2 (\bar{q}_s H d_r) \\
& - \frac{5}{72} g_s g_Y \bar{y}_u^{tu} \left[ (\mathcal{C}_{quqd}^{(8)})^{sutr} - 6(\mathcal{C}_{quqd}^{(8)})^{tusr} \right] T_b^{Aa} B_{\bar{\mu}} G_{\bar{\mu}}^A (\bar{q}_{as} H d_r^b) \\
& - \frac{1}{12} g_s^2 \bar{y}_u^{tu} \left[ (\mathcal{C}_{quqd}^{(8)})^{sutr} - 6(\mathcal{C}_{quqd}^{(8)})^{tusr} \right] T_b^{Aa} T_c^{Bb} G_{\bar{\mu}}^A G_{\bar{\mu}}^B (\bar{q}_{as} H d_r^c) \\
& - \frac{1}{9} g_s \bar{y}_d^{tu} (\mathcal{C}_{quqd}^{(8)})^{trsu} T_b^{Aa} G_{\bar{\mu}}^A (\bar{q}_{as} \partial^{\bar{\nu}} \tilde{H} \sigma^{\bar{\mu}\bar{\nu}} u_r^b) - \frac{7}{54} g_Y^2 \bar{y}_d^{tu} (\mathcal{C}_{quqd}^{(8)})^{trsu} B_{\bar{\mu}}^2 (\bar{q}_s \tilde{H} u_r) \\
& - \frac{2}{9} g_L^2 y_u^{ut} (\bar{\mathcal{C}}_{quqd}^{(8)})^{rtus} \varepsilon^{IJK} t_j^{Ki} H_i^\dagger W_{\bar{\mu}}^J W_{\bar{\nu}}^I (\bar{d}_s \sigma^{\bar{\mu}\bar{\nu}} q_r^j) - \frac{2i}{9} g_L \bar{y}_u^{tu} (\mathcal{C}_{quqd}^{(8)})^{sutr} t_j^{Ii} H^j W_{\bar{\mu}}^I (\bar{q}_{is} \partial^{\bar{\mu}} d_r) \\
& - \frac{2}{9} g_L^2 \bar{y}_u^{tu} (\mathcal{C}_{quqd}^{(8)})^{sutr} \varepsilon^{IJK} t_j^{Ki} H^j W_{\bar{\mu}}^J W_{\bar{\nu}}^I (\bar{q}_{is} \sigma^{\bar{\mu}\bar{\nu}} d_r) - \frac{10}{27} g_Y y_u^{ut} (\bar{\mathcal{C}}_{quqd}^{(8)})^{rtus} B_{\bar{\mu}} (\bar{d}_s \sigma^{\bar{\mu}\bar{\nu}} \partial^{\bar{\nu}} H^\dagger q_r) \\
& - \frac{10}{27} g_Y \bar{y}_u^{tu} (\mathcal{C}_{quqd}^{(8)})^{sutr} B_{\bar{\mu}} (\bar{q}_s \partial^{\bar{\nu}} H \sigma^{\bar{\mu}\bar{\nu}} d_r) - \frac{4i}{9} g_L g_Y y_u^{ut} (\bar{\mathcal{C}}_{quqd}^{(8)})^{rtus} t_j^{Ii} H_i^\dagger B_{\bar{\mu}} W_{\bar{\nu}}^I (\bar{d}_s \sigma^{\bar{\mu}\bar{\nu}} q_r^j) \\
& + \frac{4i}{9} g_L g_Y \bar{y}_u^{tu} (\mathcal{C}_{quqd}^{(8)})^{sutr} t_j^{Ii} H^j B_{\bar{\mu}} W_{\bar{\nu}}^I (\bar{q}_{is} \sigma^{\bar{\mu}\bar{\nu}} d_r) - \frac{4}{9} g_L g_Y \bar{y}_d^{tu} (\mathcal{C}_{quqd}^{(8)})^{trsu} t_j^{Ik} \tilde{H}_j B_{\bar{\mu}} W_{\bar{\mu}}^I (\bar{q}_{ks} u_r) \\
& - \frac{4i}{9} g_L \bar{y}_d^{tu} (\mathcal{C}_{quqd}^{(8)})^{trsu} t_l^{Ik} t_j^{Jl} \tilde{H}_j W_{\bar{\mu}}^I W_{\bar{\nu}}^J (\bar{q}_{ks} \sigma^{\bar{\mu}\bar{\nu}} u_r) + \frac{4}{9} g_L y_u^{ut} (\bar{\mathcal{C}}_{quqd}^{(8)})^{rtus} t_j^{Ii} W_{\bar{\mu}}^I (\bar{d}_s \sigma^{\bar{\mu}\bar{\nu}} q_r^j) \partial^{\bar{\nu}} H_i^\dagger \\
& + \frac{4}{9} g_L \bar{y}_d^{tu} (\mathcal{C}_{quqd}^{(8)})^{trsu} \varepsilon^{ij} t_i^{Ik} W_{\bar{\mu}}^I (\bar{q}_{js} \sigma^{\bar{\mu}\bar{\nu}} u_r) \partial^{\bar{\nu}} H_k^\dagger + \frac{4}{9} g_L \bar{y}_u^{tu} (\mathcal{C}_{quqd}^{(8)})^{sutr} t_j^{Ii} W_{\bar{\mu}}^I (\bar{q}_{is} \sigma^{\bar{\mu}\bar{\nu}} d_r) \partial^{\bar{\nu}} H^j \\
& + \frac{4}{9} g_L y_d^{tu} (\bar{\mathcal{C}}_{quqd}^{(8)})^{tsru} \bar{\varepsilon}_{ij} t_k^{Ii} W_{\bar{\mu}}^I (\bar{u}_s \sigma^{\bar{\mu}\bar{\nu}} q_r^j) \partial^{\bar{\nu}} H^k - \frac{4}{9} g_L g_Y y_d^{tu} (\bar{\mathcal{C}}_{quqd}^{(8)})^{tsru} t_k^{Ii} \tilde{H}^{\dagger i} B_{\bar{\mu}} W_{\bar{\mu}}^I (\bar{u}_s q_r^k) \\
& + \frac{4i}{9} g_L^2 y_d^{tu} (\bar{\mathcal{C}}_{quqd}^{(8)})^{tsru} t_l^{Ik} t_k^{Ji} \tilde{H}^{\dagger i} W_{\bar{\mu}}^I W_{\bar{\nu}}^J (\bar{u}_s \sigma^{\bar{\mu}\bar{\nu}} q_r^l) - \frac{2}{3} g_L^2 \bar{y}_d^{tu} (\mathcal{C}_{quqd}^{(8)})^{trsu} \varepsilon^{jk} t_l^{Ii} t_j^{Jl} H_i^\dagger W_{\bar{\mu}}^I W_{\bar{\mu}}^J (\bar{q}_{ks} u_r)
\end{aligned}$$

$$-\frac{2}{3}g_L^2y_d^{tu}(\bar{C}_{quqd}^{(8)})^{tsru}\bar{\varepsilon}_{ij}t_l^{Ik}t_k^{Ji}H^lW_{\bar{\mu}}^IW_{\bar{\mu}}^J(\bar{u}_sq_r^j). \quad (2.61)$$

### 3 Spurion-dependent symmetry-restoring counterterms

We now present the symmetry-restoring counterterms keeping the explicit spurion dependence.

#### 3.1 Renormalizable operators

$$\begin{aligned}
\Gamma_{\Omega}^{(1)}[\text{SM}] = & \frac{i}{72} [6g_s^2 + 9g_L^2 - g_Y^2] (\Omega_q^\dagger \overleftrightarrow{D}_{\bar{\mu}} \Omega_q) (\bar{q}_s \gamma^{\bar{\mu}} q_s) - \frac{i}{72} [6g_s^2 + 9g_L^2 - g_Y^2] (\Omega_{q,at}^\dagger \overleftrightarrow{D}_{\bar{\mu}} \Omega_q^{bj}) (\bar{q}_{bjs} \gamma^{\bar{\mu}} q_s^{ai}) \\
& + \frac{i}{36} [g_Y^2 + 3g_s^2] (\Omega_d^\dagger \overleftrightarrow{D}_{\bar{\mu}} \Omega_d) (\bar{q}_s \gamma^{\bar{\mu}} q_s) + \frac{i}{36} [3g_s^2 + 4g_Y^2] (\Omega_d^\dagger \overleftrightarrow{D}_{\bar{\mu}} \Omega_d) (\bar{u}_s \gamma^{\bar{\mu}} u_s) \\
& + \frac{i}{36} [g_Y^2 + 3g_s^2] (\Omega_q^\dagger \overleftrightarrow{D}_{\bar{\mu}} \Omega_q) (\bar{d}_s \gamma^{\bar{\mu}} d_s) + \frac{i}{36} [3g_s^2 - 2g_Y^2] (\Omega_q^\dagger \overleftrightarrow{D}_{\bar{\mu}} \Omega_q) (\bar{u}_s \gamma^{\bar{\mu}} u_s) \\
& + \frac{i}{36} [3g_s^2 + 4g_Y^2] (\Omega_u^\dagger \overleftrightarrow{D}_{\bar{\mu}} \Omega_u) (\bar{d}_s \gamma^{\bar{\mu}} d_s) + \frac{i}{36} [3g_s^2 - 2g_Y^2] (\Omega_u^\dagger \overleftrightarrow{D}_{\bar{\mu}} \Omega_u) (\bar{q}_s \gamma^{\bar{\mu}} q_s) \\
& + \frac{i}{24} [g_Y^2 + 3g_L^2] (\Omega_\ell^\dagger \overleftrightarrow{D}_{\bar{\mu}} \Omega_\ell) (\bar{q}_s \gamma^{\bar{\mu}} q_s) + \frac{i}{24} [g_Y^2 + 3g_L^2] (\Omega_q^\dagger \overleftrightarrow{D}_{\bar{\mu}} \Omega_q) (\bar{\ell}_s \gamma^{\bar{\mu}} \ell_s) \\
& + \frac{i}{18} [6g_s^2 - g_Y^2] (\Omega_d^\dagger \overleftrightarrow{D}_{\bar{\mu}} \Omega_d) (\bar{d}_s \gamma^{\bar{\mu}} d_s) - \frac{i}{18} [6g_s^2 - g_Y^2] (\Omega_{d,a}^\dagger \overleftrightarrow{D}_{\bar{\mu}} \Omega_d^b) (\bar{d}_{bs} \gamma^{\bar{\mu}} d_s^a) \\
& + \frac{1}{12} [g_Y^2 + 4y_u^{rs} \bar{y}_u^{rs} - 3g_L^2] \left[ (\Omega_q^\dagger D_{\bar{\mu}} \Omega_q) (H^\dagger D_{\bar{\mu}} H) + (D_{\bar{\mu}} \Omega_q^\dagger \Omega_q) (D_{\bar{\mu}} H^\dagger H) \right] - \frac{i}{12} g_Y^2 (\Omega_d^\dagger \overleftrightarrow{D}_{\bar{\mu}} \Omega_d) (\bar{\ell}_s \gamma^{\bar{\mu}} \ell_s) \\
& + \frac{i}{12} g_Y^2 (\Omega_e^\dagger \overleftrightarrow{D}_{\bar{\mu}} \Omega_e) (\bar{q}_s \gamma^{\bar{\mu}} q_s) - \frac{i}{12} g_Y^2 (\Omega_\ell^\dagger \overleftrightarrow{D}_{\bar{\mu}} \Omega_\ell) (\bar{d}_s \gamma^{\bar{\mu}} d_s) + \frac{i}{12} g_Y^2 (\Omega_q^\dagger \overleftrightarrow{D}_{\bar{\mu}} \Omega_q) (\bar{e}_s \gamma^{\bar{\mu}} e_s) \\
& + \frac{i}{9} [3g_s^2 - 2g_Y^2] (\Omega_u^\dagger \overleftrightarrow{D}_{\bar{\mu}} \Omega_u) (\bar{u}_s \gamma^{\bar{\mu}} u_s) - \frac{i}{9} [3g_s^2 - 2g_Y^2] (\Omega_{u,a}^\dagger \overleftrightarrow{D}_{\bar{\mu}} \Omega_u^b) (\bar{u}_{bs} \gamma^{\bar{\mu}} u_s^a) \\
& + \frac{i}{8} [3g_L^2 - g_Y^2] (\Omega_\ell^\dagger \overleftrightarrow{D}_{\bar{\mu}} \Omega_\ell) (\bar{\ell}_s \gamma^{\bar{\mu}} \ell_s) - \frac{i}{8} [3g_L^2 - g_Y^2] (\Omega_{\ell,i}^\dagger \overleftrightarrow{D}_{\bar{\mu}} \Omega_\ell^j) (\bar{\ell}_{js} \gamma^{\bar{\mu}} \ell_s^i) \\
& + \frac{1}{6} y_u^{rs} \bar{y}_u^{rs} \left[ (\Omega_{q,aj}^* D_{\bar{\mu}} \Omega_q^{bi}) (\Omega_{u,b}^* D_{\bar{\mu}} \Omega_u^a) H_i^\dagger H^j + (D_{\bar{\mu}} \Omega_{q,aj}^* \Omega_q^{bi}) (D_{\bar{\mu}} \Omega_{u,b}^* \Omega_u^a) H_i^\dagger H^j \right] \\
& + \frac{1}{6} [3g_L^2 - 2y_e^{rs} \bar{y}_e^{rs}] \left[ (D_{\bar{\mu}} \Omega_{\ell,j}^* \Omega_\ell^i) D^{\bar{\mu}} H_i^\dagger H^j + (\Omega_{\ell,j}^* D_{\bar{\mu}} \Omega_\ell^i) H_i^\dagger D^{\bar{\mu}} H^j \right] \\
& + \frac{1}{6} [3g_L^2 - 2[y_d^{rs} \bar{y}_d^{rs} + y_u^{rs} \bar{y}_u^{rs}]] \left[ (D_{\bar{\mu}} \Omega_{q,j}^* \Omega_q^i) D^{\bar{\mu}} H_i^\dagger H^j + (\Omega_{q,j}^* D_{\bar{\mu}} \Omega_q^i) H_i^\dagger D^{\bar{\mu}} H^j \right] \\
& + \frac{1}{6} [2y_d^{rs} \bar{y}_d^{rs} - g_Y^2] \left[ (\Omega_d^\dagger D_{\bar{\mu}} \Omega_d) (H^\dagger D_{\bar{\mu}} H) + (D_{\bar{\mu}} \Omega_d^\dagger \Omega_d) (D_{\bar{\mu}} H^\dagger H) \right] \\
& + \frac{1}{6} [2y_e^{rs} \bar{y}_e^{rs} - 3g_Y^2] \left[ (\Omega_e^\dagger D_{\bar{\mu}} \Omega_e) (H^\dagger D_{\bar{\mu}} H) + (D_{\bar{\mu}} \Omega_e^\dagger \Omega_e) (D_{\bar{\mu}} H^\dagger H) \right] - \frac{i}{6} g_Y^2 (\Omega_d^\dagger \overleftrightarrow{D}_{\bar{\mu}} \Omega_d) (\bar{e}_s \gamma^{\bar{\mu}} e_s) \\
& - \frac{i}{6} g_Y^2 (\Omega_e^\dagger \overleftrightarrow{D}_{\bar{\mu}} \Omega_e) (\bar{d}_s \gamma^{\bar{\mu}} d_s) + \frac{i}{6} g_Y^2 (\Omega_\ell^\dagger \overleftrightarrow{D}_{\bar{\mu}} \Omega_\ell) (\bar{u}_s \gamma^{\bar{\mu}} u_s) + \frac{i}{6} g_Y^2 (\Omega_u^\dagger \overleftrightarrow{D}_{\bar{\mu}} \Omega_u) (\bar{\ell}_s \gamma^{\bar{\mu}} \ell_s) \\
& + \frac{1}{4} (D_{\bar{\mu}} \Omega_{d,a}^* D_{\bar{\nu}} \Omega_d^b) (D_{\bar{\nu}} \Omega_{d,b}^* D_{\bar{\mu}} \Omega_d^a) + \frac{1}{4} (D_{\bar{\mu}} \Omega_{d,a}^* D_{\bar{\mu}} \Omega_d^b) (D_{\bar{\nu}} \Omega_{d,b}^* D_{\bar{\nu}} \Omega_d^a) + \frac{1}{4} (D_{\bar{\mu}} \Omega_e^\dagger D_{\bar{\nu}} \Omega_e) (D_{\bar{\nu}} \Omega_e^\dagger D_{\bar{\mu}} \Omega_e) \\
& + \frac{1}{4} (D_{\bar{\mu}} \Omega_e^\dagger D_{\bar{\mu}} \Omega_e) (D_{\bar{\nu}} \Omega_e^\dagger D_{\bar{\nu}} \Omega_e) + \frac{1}{4} (D_{\bar{\mu}} \Omega_{\ell,i}^* D_{\bar{\nu}} \Omega_\ell^j) (D_{\bar{\nu}} \Omega_{\ell,j}^* D_{\bar{\mu}} \Omega_\ell^i) + \frac{1}{4} (D_{\bar{\mu}} \Omega_{\ell,i}^* D_{\bar{\mu}} \Omega_\ell^j) (D_{\bar{\nu}} \Omega_{\ell,j}^* D_{\bar{\nu}} \Omega_\ell^i) \\
& + \frac{1}{4} (D_{\bar{\mu}} \Omega_{q,ai}^* D_{\bar{\nu}} \Omega_q^{bj}) (D_{\bar{\nu}} \Omega_{q,bj}^* D_{\bar{\mu}} \Omega_q^{ai}) + \frac{1}{4} (D_{\bar{\mu}} \Omega_{q,ai}^* D_{\bar{\mu}} \Omega_q^{bj}) (D_{\bar{\nu}} \Omega_{q,bj}^* D_{\bar{\nu}} \Omega_q^{ai}) + \frac{1}{4} (D_{\bar{\mu}} \Omega_{u,a}^* D_{\bar{\nu}} \Omega_u^b) (D_{\bar{\nu}} \Omega_{u,b}^* D_{\bar{\mu}} \Omega_u^a) \\
& + \frac{1}{4} (D_{\bar{\mu}} \Omega_{u,a}^* D_{\bar{\mu}} \Omega_u^b) (D_{\bar{\nu}} \Omega_{u,b}^* D_{\bar{\nu}} \Omega_u^a) + \frac{1}{4} \left[ -g_L^2 - g_Y^2 \right] \left[ (\Omega_\ell^\dagger D_{\bar{\mu}} \Omega_\ell) (H^\dagger D_{\bar{\mu}} H) + (D_{\bar{\mu}} \Omega_\ell^\dagger \Omega_\ell) (D_{\bar{\mu}} H^\dagger H) \right] \\
& + \frac{i}{4} [y_d^{st} \bar{y}_d^{rt} - g_s^2 \delta^{rs}] (\Omega_{d,a}^\dagger \overleftrightarrow{D}_{\bar{\mu}} \Omega_d^b) (\bar{q}_{bs} \gamma^{\bar{\mu}} q_r^a) - \frac{i}{4} g_s^2 (\Omega_{d,a}^\dagger \overleftrightarrow{D}_{\bar{\mu}} \Omega_d^b) (\bar{u}_{bs} \gamma^{\bar{\mu}} u_s^a)
\end{aligned}$$

$$\begin{aligned}
& + \frac{i}{4} \left[ y_e^{st} \bar{y}_e^{rt} - g_Y^2 \delta^{rs} \right] (\Omega_e^\dagger \overleftrightarrow{D}_\mu \Omega_e) (\bar{\ell}_s \gamma^\mu \ell_r) + \frac{i}{4} \left[ y_e^{tr} \bar{y}_e^{ts} - g_Y^2 \delta^{rs} \right] (\Omega_\ell^\dagger \overleftrightarrow{D}_\mu \Omega_\ell) (\bar{e}_s \gamma^\mu e_r) \\
& - \frac{i}{4} g_L^2 (\Omega_{\ell,i}^\dagger \overleftrightarrow{D}_\mu \Omega_\ell^j) (\bar{q}_{js} \gamma^\mu q_s^i) - \frac{i}{4} g_L^2 (\Omega_{q,i}^\dagger \overleftrightarrow{D}_\mu \Omega_q^j) (\bar{\ell}_{js} \gamma^\mu \ell_s^i) \\
& - \frac{i}{4} \left[ g_L^2 - g_s^2 \right] (\Omega_{q,i}^\dagger \overleftrightarrow{D}_\mu \Omega_q^j) (\bar{q}_{js} \gamma^\mu q_s^i) + \frac{i}{4} \left[ y_d^{tr} \bar{y}_d^{ts} - g_s^2 \delta^{rs} \right] (\Omega_{q,a}^\dagger \overleftrightarrow{D}_\mu \Omega_q^b) (\bar{d}_{bs} \gamma^\mu d_r^a) \\
& + \frac{i}{4} \left[ g_L^2 - g_s^2 \right] (\Omega_{q,a}^\dagger \overleftrightarrow{D}_\mu \Omega_q^b) (\bar{q}_{bs} \gamma^\mu q_s^a) + \frac{i}{4} \left[ y_u^{tr} \bar{y}_u^{ts} - g_s^2 \delta^{rs} \right] (\Omega_{q,a}^\dagger \overleftrightarrow{D}_\mu \Omega_q^b) (\bar{u}_{bs} \gamma^\mu u_r^a) \\
& - \frac{i}{4} g_s^2 (\Omega_{u,a}^\dagger \overleftrightarrow{D}_\mu \Omega_u^b) (\bar{d}_{bs} \gamma^\mu d_s^a) + \frac{i}{4} \left[ y_u^{st} \bar{y}_u^{rt} - g_s^2 \delta^{rs} \right] (\Omega_{u,a}^\dagger \overleftrightarrow{D}_\mu \Omega_u^b) (\bar{q}_{bs} \gamma^\mu q_r^a) \\
& + \frac{1}{3} y_e^{rs} \bar{y}_e^{rs} (D_\mu \Omega_{\ell,j}^* D_\mu \Omega_\ell^i) H_i^\dagger H^j + \frac{1}{3} \left[ y_d^{rs} \bar{y}_d^{rs} - y_u^{rs} \bar{y}_u^{rs} \right] (D_\mu \Omega_{q,j}^* D_\mu \Omega_q^i) H_i^\dagger H^j + \frac{1}{3} y_d^{rs} \bar{y}_d^{rs} (D_\mu \Omega_d^\dagger D_\mu \Omega_d) (H^\dagger H) \\
& + \frac{1}{3} y_e^{rs} \bar{y}_e^{rs} (D_\mu \Omega_e^\dagger D_\mu \Omega_e) (H^\dagger H) + \frac{1}{3} y_u^{rs} \bar{y}_u^{rs} (D_\mu \Omega_q^\dagger D_\mu \Omega_q) (H^\dagger H) + \frac{1}{3} y_u^{rs} \bar{y}_u^{rs} (D_\mu \Omega_u^\dagger D_\mu \Omega_u) (H^\dagger H) \\
& + \frac{1}{3} \left[ g_Y^2 - y_u^{rs} \bar{y}_u^{rs} \right] \left[ (\Omega_u^\dagger D_\mu \Omega_u) (H^\dagger D_\mu H) + (D_\mu \Omega_u^\dagger \Omega_u) (D_\mu H^\dagger H) \right] \\
& - \frac{1}{6} y_e^{rs} \bar{y}_e^{rs} \left[ (\Omega_e^\dagger D_\mu \Omega_e) (\Omega_{\ell,j}^* D_\mu \Omega_\ell^i) H_i^\dagger H^j + (D_\mu \Omega_e^\dagger \Omega_e) (D_\mu \Omega_{\ell,j}^* \Omega_\ell^i) H_i^\dagger H^j \right] \\
& - \frac{1}{6} y_d^{rs} \bar{y}_d^{rs} \left[ (\Omega_{d,a}^* D_\mu \Omega_d^b) (\Omega_{q,bj}^* D_\mu \Omega_q^{ai}) H_i^\dagger H^j + (D_\mu \Omega_{d,a}^* \Omega_d^b) (D_\mu \Omega_{q,bj}^* \Omega_q^{ai}) H_i^\dagger H^j \right] \\
& - \frac{1}{6} y_u^{rs} \bar{y}_u^{rs} \left[ (\Omega_{q,a}^* D_\mu \Omega_q^b) (\Omega_{u,b}^* D_\mu \Omega_u^a) (H^\dagger H) + (D_\mu \Omega_{q,a}^* \Omega_q^b) (D_\mu \Omega_{u,b}^* \Omega_u^a) (H^\dagger H) \right] - \frac{1}{4} \left[ (\Omega_d^\dagger D_2 \Omega_d) + (D_2 \Omega_d^\dagger \Omega_d) \right] \\
& - \frac{1}{4} (D_\mu \Omega_{d,a}^* D_\mu \Omega_d^b) (D_\mu \Omega_{d,b}^* D_\mu \Omega_d^a) - \frac{1}{4} \left[ (\Omega_e^\dagger D_2 \Omega_e) + (D_2 \Omega_e^\dagger \Omega_e) \right] - \frac{1}{4} (D_\mu \Omega_e^\dagger D_\mu \Omega_e)^2 \\
& - \frac{1}{4} \left[ (\Omega_\ell^\dagger D_2 \Omega_\ell) + (D_2 \Omega_\ell^\dagger \Omega_\ell) \right] - \frac{1}{4} (D_\mu \Omega_{\ell,i}^* D_\mu \Omega_\ell^j) (D_\mu \Omega_{\ell,j}^* D_\mu \Omega_\ell^i) - \frac{1}{4} \left[ (\Omega_q^\dagger D_2 \Omega_q) + (D_2 \Omega_q^\dagger \Omega_q) \right] \\
& - \frac{1}{4} (D_\mu \Omega_{q,ai}^* D_\mu \Omega_q^{bj}) (D_\mu \Omega_{q,bj}^* D_\mu \Omega_q^{ai}) - \frac{1}{4} \left[ (\Omega_u^\dagger D_2 \Omega_u) + (D_2 \Omega_u^\dagger \Omega_u) \right] - \frac{1}{4} (D_\mu \Omega_{u,a}^* D_\mu \Omega_u^b) (D_\mu \Omega_{u,b}^* D_\mu \Omega_u^a) \\
& + \frac{i}{3} g_Y^2 (\Omega_e^\dagger \overleftrightarrow{D}_\mu \Omega_e) (\bar{u}_s \gamma^\mu u_s) + \frac{i}{3} g_Y^2 (\Omega_u^\dagger \overleftrightarrow{D}_\mu \Omega_u) (\bar{e}_s \gamma^\mu e_s). \tag{3.1}
\end{aligned}$$

### 3.2 Dimension five: Weinberg operator

$$\begin{aligned}
\Gamma_\Omega^{(1)} [\mathcal{O}_{\ell HH}] &= \frac{4}{3} \bar{\mathcal{C}}_{\ell HH}^{rs} \mathcal{C}_{\ell HH}^{rs} (D_\mu \Omega_{\ell,k}^* \Omega_\ell^l) (\Omega_{\ell,l}^* D_\mu \Omega_\ell^i) (H^\dagger H) H_i^\dagger H^k + \frac{4}{3} \bar{\mathcal{C}}_{\ell HH}^{rs} \mathcal{C}_{\ell HH}^{rs} (D_\mu \Omega_\ell^\dagger D_\mu \Omega_\ell) (H^\dagger H)^2 \\
& + \frac{8}{3} \bar{\mathcal{C}}_{\ell HH}^{rs} \mathcal{C}_{\ell HH}^{rs} \left[ (\Omega_\ell^\dagger D_\mu \Omega_\ell) (H^\dagger H) (H^\dagger D_\mu H) + (D_\mu \Omega_\ell^\dagger \Omega_\ell) (H^\dagger H) (D_\mu H^\dagger H) \right] \\
& - \frac{2}{3} \bar{\mathcal{C}}_{\ell HH}^{rs} \mathcal{C}_{\ell HH}^{rs} (\Omega_{\ell,k}^* D_\mu \Omega_\ell^i) (D_\mu \Omega_{\ell,l}^* \Omega_\ell^j) H_i^\dagger H_j^\dagger H^k H^l - \frac{2}{3} \bar{\mathcal{C}}_{\ell HH}^{rs} \mathcal{C}_{\ell HH}^{rs} (\Omega_{\ell,k}^* D_\mu \Omega_\ell^l) (D_\mu \Omega_{\ell,l}^* \Omega_\ell^k) (H^\dagger H)^2 \\
& - \frac{4}{3} \bar{\mathcal{C}}_{\ell HH}^{rs} \mathcal{C}_{\ell HH}^{rs} (D_\mu \Omega_{\ell,k}^* D_\mu \Omega_\ell^j) (H^\dagger H) H_j^\dagger H^k \\
& - \frac{4}{3} \bar{\mathcal{C}}_{\ell HH}^{rs} \mathcal{C}_{\ell HH}^{rs} \left[ (D_\mu \Omega_{\ell,k}^* \Omega_\ell^j) (H^\dagger H) D_\mu H_j^\dagger H^k + (\Omega_{\ell,k}^* D_\mu \Omega_\ell^j) (H^\dagger H) H_j^\dagger D_\mu H^k \right] \\
& - \frac{4}{3} \bar{\mathcal{C}}_{\ell HH}^{rs} \mathcal{C}_{\ell HH}^{rs} \left[ (\Omega_{\ell,k}^* D_\mu \Omega_\ell^j) (H^\dagger D_\mu H) H_j^\dagger H^k + (D_\mu \Omega_{\ell,k}^* \Omega_\ell^j) (D_\mu H^\dagger H) H_j^\dagger H^k \right] \\
& - 2i \bar{\mathcal{C}}_{\ell HH}^{st} \mathcal{C}_{\ell HH}^{rt} \left[ (\Omega_{\ell,j}^* D_\mu \Omega_\ell^i) H_i^\dagger (\bar{\ell}_s H \gamma^\mu \ell_r^j) - (D_\mu \Omega_{\ell,j}^* \Omega_\ell^k) H^j (\bar{\ell}_{ks} \gamma^\mu H^\dagger \ell_r) \right] \\
& + 3i \bar{\mathcal{C}}_{\ell HH}^{st} \mathcal{C}_{\ell HH}^{rt} (\Omega_\ell^\dagger \overleftrightarrow{D}_\mu \Omega_\ell) (\bar{\ell}_s H \gamma^\mu H^\dagger \ell_r)
\end{aligned}$$

$$\begin{aligned}
& + 3i\bar{\mathcal{C}}_{\ell\ell HH}^{st}\mathcal{C}_{\ell\ell HH}^{rt}(\Omega_{\ell,j}^\dagger\overset{\leftrightarrow}{D}_\mu\Omega_\ell^i)H_i^\dagger H^j(\bar{\ell}_s\gamma^\mu\ell_r) \\
& - 4i\bar{\mathcal{C}}_{\ell\ell HH}^{st}\mathcal{C}_{\ell\ell HH}^{rt}(\Omega_\ell^\dagger\overset{\leftrightarrow}{D}_\mu\Omega_\ell)(H^\dagger H)(\bar{\ell}_s\gamma^\mu\ell_r).
\end{aligned} \tag{3.2}$$

### 3.3 Dimension six: bosonic operators

$$\Gamma_\Omega^{(1)}[\mathcal{O}_H] = 0, \tag{3.3}$$

$$\Gamma_\Omega^{(1)}[\mathcal{O}_{H\Box}] = 0, \tag{3.4}$$

$$\Gamma_\Omega^{(1)}[\mathcal{O}_{HD}] = 0, \tag{3.5}$$

$$\begin{aligned}
\Gamma_\Omega^{(1)}[\mathcal{O}_W] = & \frac{i}{2}g_L^2\mathcal{C}_W\left[2(\Omega_\ell^\dagger D_\rho\Omega_\ell)\widetilde{W}^{\rho\bar{\sigma}I}(\bar{\ell}_r t^I\gamma^{\bar{\sigma}}\ell_r) - 2(D_\mu\Omega_\ell^\dagger\Omega_\ell)\widetilde{W}^{\mu\bar{\sigma}I}(\bar{\ell}_r t^I\gamma^{\bar{\sigma}}\ell_r)\right] \\
& - \frac{i}{2}g_L^2\mathcal{C}_W\left[2t_j^{Ii}(\Omega_{\ell,i}^*D_\rho\Omega_\ell^k)\widetilde{W}^{\rho\bar{\sigma}I}(\bar{\ell}_{kr}\gamma^{\bar{\sigma}}\ell_r^j) - 2t_k^{Ij}(D_\mu\Omega_{\ell,i}^*\Omega_\ell^k)\widetilde{W}^{\mu\bar{\sigma}I}(\bar{\ell}_{jr}\gamma^{\bar{\sigma}}\ell_r^i)\right] \\
& + \frac{i}{2}g_L^2\mathcal{C}_W\left[2(\Omega_{q,a}^*D_\rho\Omega_q^b)\widetilde{W}^{\rho\bar{\sigma}I}(\bar{q}_{br}t^I\gamma^{\bar{\sigma}}q_r^a) - 2(D_\mu\Omega_{q,a}^*\Omega_q^b)\widetilde{W}^{\mu\bar{\sigma}I}(\bar{q}_{br}t^I\gamma^{\bar{\sigma}}q_r^a)\right] \\
& - \frac{i}{2}g_L^2\mathcal{C}_W\left[2t_j^{Ii}(\Omega_{q,ai}^*D_\rho\Omega_q^{bk})\widetilde{W}^{\rho\bar{\sigma}I}(\bar{q}_{bkr}\gamma^{\bar{\sigma}}q_r^{aj}) - 2t_k^{Ij}(D_\mu\Omega_{q,ai}^*\Omega_q^{bk})\widetilde{W}^{\mu\bar{\sigma}I}(\bar{q}_{bjr}\gamma^{\bar{\sigma}}q_r^{ai})\right],
\end{aligned} \tag{3.6}$$

$$\begin{aligned}
\Gamma_\Omega^{(1)}[\mathcal{O}_{\bar{W}}] = & -\frac{i}{3}g_L^2\mathcal{C}_{\bar{W}}\left[t_j^{Ii}(\Omega_{\ell,i}^*D_\mu\Omega_\ell^k)W^{\mu\bar{\nu}I}(\bar{\ell}_{kr}\gamma^{\bar{\nu}}\ell_r^j) - t_k^{Ij}(D_\mu\Omega_{\ell,i}^*\Omega_\ell^k)W^{\mu\bar{\nu}I}(\bar{\ell}_{jr}\gamma^{\bar{\nu}}\ell_r^i)\right] \\
& - \frac{i}{3}g_L^2\mathcal{C}_{\bar{W}}\left[t_j^{Ii}(\Omega_{q,ai}^*D_\mu\Omega_q^{bk})W^{\mu\bar{\nu}I}(\bar{q}_{bkr}\gamma^{\bar{\nu}}q_r^{aj}) - t_k^{Ij}(D_\mu\Omega_{q,ai}^*\Omega_q^{bk})W^{\mu\bar{\nu}I}(\bar{q}_{bjr}\gamma^{\bar{\nu}}q_r^{ai})\right] \\
& + \frac{i}{3}g_L^2\mathcal{C}_{\bar{W}}W^{\mu\bar{\nu}I}(\Omega_\ell^\dagger\overset{\leftrightarrow}{D}_\mu\Omega_\ell)(\bar{\ell}_r t^I\gamma^{\bar{\nu}}\ell_r) + \frac{i}{3}g_L^2\mathcal{C}_{\bar{W}}W^{\mu\bar{\nu}I}(\Omega_{q,a}^\dagger\overset{\leftrightarrow}{D}_\mu\Omega_q^b)(\bar{q}_{br}t^I\gamma^{\bar{\nu}}q_r^a),
\end{aligned} \tag{3.7}$$

$$\begin{aligned}
\Gamma_\Omega^{(1)}[\mathcal{O}_G] = & \frac{i}{4}g_s^2\mathcal{C}_G\left[2T_b^{Aa}(\Omega_{d,a}^*D_\rho\Omega_d^b)\widetilde{G}^{\rho\bar{\sigma}A}(\bar{d}_r\gamma^{\bar{\sigma}}d_r) - 2T_b^{Aa}(D_\mu\Omega_{d,a}^*\Omega_d^b)\widetilde{G}^{\mu\bar{\sigma}A}(\bar{d}_r\gamma^{\bar{\sigma}}d_r)\right] \\
& - \frac{i}{4}g_s^2\mathcal{C}_G\left[2(\Omega_d^\dagger D_\rho\Omega_d)\widetilde{G}^{\rho\bar{\sigma}A}(\bar{d}_r T^A\gamma^{\bar{\sigma}}d_r) - 2(D_\mu\Omega_d^\dagger\Omega_d)\widetilde{G}^{\mu\bar{\sigma}A}(\bar{d}_r T^A\gamma^{\bar{\sigma}}d_r)\right] \\
& - \frac{i}{4}g_s^2\mathcal{C}_G\left[2T_b^{Aa}(\Omega_{q,ai}^*D_\rho\Omega_q^{bj})\widetilde{G}^{\rho\bar{\sigma}A}(\bar{q}_{jr}\gamma^{\bar{\sigma}}q_r^i) - 2T_b^{Aa}(D_\mu\Omega_{q,ai}^*\Omega_q^{bj})\widetilde{G}^{\mu\bar{\sigma}A}(\bar{q}_{jr}\gamma^{\bar{\sigma}}q_r^i)\right] \\
& + \frac{i}{4}g_s^2\mathcal{C}_G\left[2(\Omega_{q,i}^*D_\rho\Omega_q^j)\widetilde{G}^{\rho\bar{\sigma}A}(\bar{q}_{jr}T^A\gamma^{\bar{\sigma}}q_r^i) - 2(D_\mu\Omega_{q,i}^*\Omega_q^j)\widetilde{G}^{\mu\bar{\sigma}A}(\bar{q}_{jr}T^A\gamma^{\bar{\sigma}}q_r^i)\right] \\
& + \frac{i}{4}g_s^2\mathcal{C}_G\left[2T_b^{Aa}(\Omega_{u,a}^*D_\rho\Omega_u^b)\widetilde{G}^{\rho\bar{\sigma}A}(\bar{u}_r\gamma^{\bar{\sigma}}u_r) - 2T_b^{Aa}(D_\mu\Omega_{u,a}^*\Omega_u^b)\widetilde{G}^{\mu\bar{\sigma}A}(\bar{u}_r\gamma^{\bar{\sigma}}u_r)\right] \\
& - \frac{i}{4}g_s^2\mathcal{C}_G\left[2(\Omega_u^\dagger D_\rho\Omega_u)\widetilde{G}^{\rho\bar{\sigma}A}(\bar{u}_r T^A\gamma^{\bar{\sigma}}u_r) - 2(D_\mu\Omega_u^\dagger\Omega_u)\widetilde{G}^{\mu\bar{\sigma}A}(\bar{u}_r T^A\gamma^{\bar{\sigma}}u_r)\right],
\end{aligned} \tag{3.8}$$

$$\begin{aligned}
\Gamma_\Omega^{(1)}[\mathcal{O}_{\bar{G}}] = & -\frac{i}{6}g_s^2\mathcal{C}_{\bar{G}}G^{\mu\bar{\nu}A}(\Omega_d^\dagger\overset{\leftrightarrow}{D}_\mu\Omega_d)(\bar{d}_r T^A\gamma^{\bar{\nu}}d_r) + \frac{i}{6}g_s^2\mathcal{C}_{\bar{G}}T_b^{Aa}G^{\mu\bar{\nu}A}(\Omega_{d,a}^\dagger\overset{\leftrightarrow}{D}_\mu\Omega_d^b)(\bar{d}_r\gamma^{\bar{\nu}}d_r) \\
& + \frac{i}{6}g_s^2\mathcal{C}_{\bar{G}}G^{\mu\bar{\nu}A}(\Omega_{q,i}^\dagger\overset{\leftrightarrow}{D}_\mu\Omega_q^j)(\bar{q}_{jr}T^A\gamma^{\bar{\nu}}q_r^i) - \frac{i}{6}g_s^2\mathcal{C}_{\bar{G}}T_b^{Aa}G^{\mu\bar{\nu}A}(\Omega_{q,ai}^\dagger\overset{\leftrightarrow}{D}_\mu\Omega_q^{bj})(\bar{q}_{jr}\gamma^{\bar{\nu}}q_r^i) \\
& - \frac{i}{6}g_s^2\mathcal{C}_{\bar{G}}G^{\mu\bar{\nu}A}(\Omega_u^\dagger\overset{\leftrightarrow}{D}_\mu\Omega_u)(\bar{u}_r T^A\gamma^{\bar{\nu}}u_r) + \frac{i}{6}g_s^2\mathcal{C}_{\bar{G}}T_b^{Aa}G^{\mu\bar{\nu}A}(\Omega_{u,a}^\dagger\overset{\leftrightarrow}{D}_\mu\Omega_u^b)(\bar{u}_r\gamma^{\bar{\nu}}u_r),
\end{aligned} \tag{3.9}$$

$$\begin{aligned}
\Gamma_{\Omega}^{(1)} [\mathcal{O}_{HB}] = & -\frac{i}{108} g_Y^2 \mathcal{C}_{HB} (\Omega_{q,a}^\dagger \overleftrightarrow{D}_{\bar{\mu}} \Omega_q^b) (H^\dagger H) (\bar{q}_{bs} \gamma^{\bar{\mu}} q_s^a) + \frac{i}{108} g_Y^2 \mathcal{C}_{HB} (\Omega_{q,a}^\dagger \overleftrightarrow{D}_{\bar{\mu}} \Omega_q^b) (\bar{q}_{bs} H \gamma^{\bar{\mu}} H^\dagger q_s^a) \\
& + \frac{i}{108} g_Y^2 \mathcal{C}_{HB} (\Omega_{q,aj}^\dagger \overleftrightarrow{D}_{\bar{\mu}} \Omega_q^{bi}) H_i^\dagger H^j (\bar{q}_{bs} \gamma^{\bar{\mu}} q_s^a) \\
& - \frac{i}{54} g_Y^2 \mathcal{C}_{HB} \left[ (\Omega_{q,aj}^* D_{\bar{\mu}} \Omega_q^{bi}) H_i^\dagger (\bar{q}_{bs} H \gamma^{\bar{\mu}} q_s^{aj}) - (D_{\bar{\mu}} \Omega_{q,aj}^* \Omega_q^{bk}) H^j (\bar{q}_{bks} \gamma^{\bar{\mu}} H^\dagger q_s^a) \right] \\
& - \frac{i}{27} g_Y^2 \mathcal{C}_{HB} (\Omega_{d,a}^\dagger \overleftrightarrow{D}_{\bar{\mu}} \Omega_d^b) (H^\dagger H) (\bar{d}_{bs} \gamma^{\bar{\mu}} d_s^a) - \frac{i}{12} g_Y^2 \mathcal{C}_{HB} (\Omega_\ell^\dagger \overleftrightarrow{D}_{\bar{\mu}} \Omega_\ell) (H^\dagger H) (\bar{\ell}_s \gamma^{\bar{\mu}} \ell_s) \\
& + \frac{i}{12} g_Y^2 \mathcal{C}_{HB} (\Omega_\ell^\dagger \overleftrightarrow{D}_{\bar{\mu}} \Omega_\ell) (\bar{\ell}_s H \gamma^{\bar{\mu}} H^\dagger \ell_s) + \frac{i}{12} g_Y^2 \mathcal{C}_{HB} (\Omega_{\ell,j}^\dagger \overleftrightarrow{D}_{\bar{\mu}} \Omega_\ell^i) H_i^\dagger H^j (\bar{\ell}_s \gamma^{\bar{\mu}} \ell_s) \\
& - \frac{4i}{27} g_Y^2 \mathcal{C}_{HB} (\Omega_{u,a}^\dagger \overleftrightarrow{D}_{\bar{\mu}} \Omega_u^b) (H^\dagger H) (\bar{u}_{bs} \gamma^{\bar{\mu}} u_s^a) \\
& - \frac{i}{6} g_Y^2 \mathcal{C}_{HB} \left[ (\Omega_{\ell,j}^* D_{\bar{\mu}} \Omega_\ell^i) H_i^\dagger (\bar{\ell}_s H \gamma^{\bar{\mu}} \ell_s^j) - (D_{\bar{\mu}} \Omega_{\ell,j}^* \Omega_\ell^k) H^j (\bar{\ell}_{ks} \gamma^{\bar{\mu}} H^\dagger \ell_s) \right] \\
& - \frac{i}{3} g_Y^2 \mathcal{C}_{HB} (\Omega_e^\dagger \overleftrightarrow{D}_{\bar{\mu}} \Omega_e) (H^\dagger H) (\bar{e}_s \gamma^{\bar{\mu}} e_s), \tag{3.10}
\end{aligned}$$

$$\Gamma_{\Omega}^{(1)} [\mathcal{O}_{H\hat{B}}] = 0, \tag{3.11}$$

$$\begin{aligned}
\Gamma_{\Omega}^{(1)} [\mathcal{O}_{HW}] = & -\frac{i}{12} g_L^2 \mathcal{C}_{HW} (\Omega_\ell^\dagger \overleftrightarrow{D}_{\bar{\mu}} \Omega_\ell) (H^\dagger H) (\bar{\ell}_s \gamma^{\bar{\mu}} \ell_s) - \frac{i}{12} g_L^2 \mathcal{C}_{HW} (\Omega_\ell^\dagger \overleftrightarrow{D}_{\bar{\mu}} \Omega_\ell) (\bar{\ell}_s H \gamma^{\bar{\mu}} H^\dagger \ell_s) \\
& - \frac{i}{12} g_L^2 \mathcal{C}_{HW} (\Omega_{\ell,j}^\dagger \overleftrightarrow{D}_{\bar{\mu}} \Omega_\ell^i) H_i^\dagger H^j (\bar{\ell}_s \gamma^{\bar{\mu}} \ell_s) - \frac{i}{12} g_L^2 \mathcal{C}_{HW} (\Omega_{q,a}^\dagger \overleftrightarrow{D}_{\bar{\mu}} \Omega_q^b) (H^\dagger H) (\bar{q}_{bs} \gamma^{\bar{\mu}} q_s^a) \\
& - \frac{i}{12} g_L^2 \mathcal{C}_{HW} (\Omega_{q,a}^\dagger \overleftrightarrow{D}_{\bar{\mu}} \Omega_q^b) (\bar{q}_{bs} H \gamma^{\bar{\mu}} H^\dagger q_s^a) - \frac{i}{12} g_L^2 \mathcal{C}_{HW} (\Omega_{q,aj}^\dagger \overleftrightarrow{D}_{\bar{\mu}} \Omega_q^{bi}) H_i^\dagger H^j (\bar{q}_{bs} \gamma^{\bar{\mu}} q_s^a) \\
& + \frac{i}{6} g_L^2 \mathcal{C}_{HW} \left[ (\Omega_{\ell,j}^* D_{\bar{\mu}} \Omega_\ell^i) H_i^\dagger (\bar{\ell}_s H \gamma^{\bar{\mu}} \ell_s^j) - (D_{\bar{\mu}} \Omega_{\ell,j}^* \Omega_\ell^k) H^j (\bar{\ell}_{ks} \gamma^{\bar{\mu}} H^\dagger \ell_s) \right] \\
& + \frac{i}{6} g_L^2 \mathcal{C}_{HW} \left[ (\Omega_{q,aj}^* D_{\bar{\mu}} \Omega_q^{bi}) H_i^\dagger (\bar{q}_{bs} H \gamma^{\bar{\mu}} q_s^{aj}) - (D_{\bar{\mu}} \Omega_{q,aj}^* \Omega_q^{bk}) H^j (\bar{q}_{bks} \gamma^{\bar{\mu}} H^\dagger q_s^a) \right], \tag{3.12}
\end{aligned}$$

$$\Gamma_{\Omega}^{(1)} [\mathcal{O}_{H\bar{W}}] = 0, \tag{3.13}$$

$$\begin{aligned}
\Gamma_{\Omega}^{(1)} [\mathcal{O}_{HG}] = & \frac{i}{18} g_s^2 \mathcal{C}_{HG} (\Omega_{d,a}^\dagger \overleftrightarrow{D}_{\bar{\mu}} \Omega_d^b) (H^\dagger H) (\bar{d}_{bs} \gamma^{\bar{\mu}} d_s^a) + \frac{i}{18} g_s^2 \mathcal{C}_{HG} (\Omega_{q,a}^\dagger \overleftrightarrow{D}_{\bar{\mu}} \Omega_q^b) (H^\dagger H) (\bar{q}_{bs} \gamma^{\bar{\mu}} q_s^a) \\
& - \frac{i}{18} g_s^2 \mathcal{C}_{HG} (\Omega_{q,a}^\dagger \overleftrightarrow{D}_{\bar{\mu}} \Omega_q^b) (\bar{q}_{bs} H \gamma^{\bar{\mu}} H^\dagger q_s^a) - \frac{i}{18} g_s^2 \mathcal{C}_{HG} (\Omega_{q,aj}^\dagger \overleftrightarrow{D}_{\bar{\mu}} \Omega_q^{bi}) H_i^\dagger H^j (\bar{q}_{bs} \gamma^{\bar{\mu}} q_s^a) \\
& + \frac{i}{18} g_s^2 \mathcal{C}_{HG} (\Omega_{u,a}^\dagger \overleftrightarrow{D}_{\bar{\mu}} \Omega_u^b) (H^\dagger H) (\bar{u}_{bs} \gamma^{\bar{\mu}} u_s^a) \\
& + \frac{i}{9} g_s^2 \mathcal{C}_{HG} \left[ (\Omega_{q,aj}^* D_{\bar{\mu}} \Omega_q^{bi}) H_i^\dagger (\bar{q}_{bs} H \gamma^{\bar{\mu}} q_s^{aj}) - (D_{\bar{\mu}} \Omega_{q,aj}^* \Omega_q^{bk}) H^j (\bar{q}_{bks} \gamma^{\bar{\mu}} H^\dagger q_s^a) \right] \\
& - \frac{i}{6} g_s^2 \mathcal{C}_{HG} (\Omega_d^\dagger \overleftrightarrow{D}_{\bar{\mu}} \Omega_d) (H^\dagger H) (\bar{d}_s \gamma^{\bar{\mu}} d_s) - \frac{i}{6} g_s^2 \mathcal{C}_{HG} (\Omega_q^\dagger \overleftrightarrow{D}_{\bar{\mu}} \Omega_q) (H^\dagger H) (\bar{q}_s \gamma^{\bar{\mu}} q_s) \\
& + \frac{i}{6} g_s^2 \mathcal{C}_{HG} (\Omega_q^\dagger \overleftrightarrow{D}_{\bar{\mu}} \Omega_q) (\bar{q}_s H \gamma^{\bar{\mu}} H^\dagger q_s) + \frac{i}{6} g_s^2 \mathcal{C}_{HG} (\Omega_{q,j}^\dagger \overleftrightarrow{D}_{\bar{\mu}} \Omega_q^i) H_i^\dagger H^j (\bar{q}_s \gamma^{\bar{\mu}} q_s) \\
& - \frac{i}{6} g_s^2 \mathcal{C}_{HG} (\Omega_u^\dagger \overleftrightarrow{D}_{\bar{\mu}} \Omega_u) (H^\dagger H) (\bar{u}_s \gamma^{\bar{\mu}} u_s)
\end{aligned}$$

$$-\frac{i}{3}g_s^2\mathcal{C}_{HG}\left[(\Omega_{q,j}^*D_{\bar{\mu}}\Omega_q^i)H_i^\dagger(\bar{q}_sH\gamma^{\bar{\mu}}q_s^j)-(D_{\bar{\mu}}\Omega_{q,j}^*\Omega_q^k)H^j(\bar{q}_{ks}\gamma^{\bar{\mu}}H^\dagger q_s)\right], \quad (3.14)$$

$$\Gamma_\Omega^{(1)}[\mathcal{O}_{H\tilde{G}}]=0, \quad (3.15)$$

$$\begin{aligned} \Gamma_\Omega^{(1)}[\mathcal{O}_{HWB}] &= \frac{i}{36}g_Lg_Y\mathcal{C}_{HWB}(\Omega_{q,a}^\dagger\overset{\leftrightarrow}{D}_{\bar{\mu}}\Omega_q^b)(H^\dagger H)(\bar{q}_{bs}\gamma^{\bar{\mu}}q_s^a)-\frac{i}{36}g_Lg_Y\mathcal{C}_{HWB}(\Omega_{q,a}^\dagger\overset{\leftrightarrow}{D}_{\bar{\mu}}\Omega_q^b)(\bar{q}_{bs}H\gamma^{\bar{\mu}}H^\dagger q_s^a) \\ &- \frac{i}{36}g_Lg_Y\mathcal{C}_{HWB}(\Omega_{q,a}^\dagger\overset{\leftrightarrow}{D}_{\bar{\mu}}\Omega_q^{bi})H_i^\dagger H^j(\bar{q}_{bs}\gamma^{\bar{\mu}}q_s^a)-\frac{i}{12}g_Lg_Y\mathcal{C}_{HWB}(\Omega_\ell^\dagger\overset{\leftrightarrow}{D}_{\bar{\mu}}\Omega_\ell)(H^\dagger H)(\bar{\ell}_s\gamma^{\bar{\mu}}\ell_s) \\ &+ \frac{i}{12}g_Lg_Y\mathcal{C}_{HWB}(\Omega_\ell^\dagger\overset{\leftrightarrow}{D}_{\bar{\mu}}\Omega_\ell)(\bar{\ell}_sH\gamma^{\bar{\mu}}H^\dagger\ell_s)+\frac{i}{12}g_Lg_Y\mathcal{C}_{HWB}(\Omega_{\ell,j}^\dagger\overset{\leftrightarrow}{D}_{\bar{\mu}}\Omega_\ell^i)H_i^\dagger H^j(\bar{\ell}_s\gamma^{\bar{\mu}}\ell_s), \end{aligned} \quad (3.16)$$

$$\Gamma_\Omega^{(1)}[\mathcal{O}_{H\bar{W}B}]=0. \quad (3.17)$$

### 3.4 Dimension six: semibosonic operators

$$\begin{aligned} \Gamma_\Omega^{(1)}[\mathcal{O}_{eH}] &= \frac{1}{6}\left[\bar{y}_e^{rs}\mathcal{C}_{eH}^{rs}+y_e^{rs}\bar{\mathcal{C}}_{eH}^{rs}\right]\left[(\Omega_e^\dagger D_{\bar{\mu}}\Omega_e)(\Omega_{\ell,k}^*D_{\bar{\mu}}\Omega_\ell^j)(H^\dagger H)H_j^\dagger H^k+(D_{\bar{\mu}}\Omega_e^\dagger\Omega_e)(D_{\bar{\mu}}\Omega_{\ell,k}^*\Omega_\ell^j)(H^\dagger H)H_j^\dagger H^k\right] \\ &- \frac{i}{4}\left[\bar{y}_e^{rt}\mathcal{C}_{eH}^{st}+y_e^{st}\bar{\mathcal{C}}_{eH}^{rt}\right](\Omega_e^\dagger\overset{\leftrightarrow}{D}_{\bar{\mu}}\Omega_e)(H^\dagger H)(\bar{\ell}_s\gamma^{\bar{\mu}}\ell_r) \\ &- \frac{i}{4}\left[\bar{y}_e^{rt}\mathcal{C}_{eH}^{st}+y_e^{st}\bar{\mathcal{C}}_{eH}^{rt}\right](\Omega_e^\dagger\overset{\leftrightarrow}{D}_{\bar{\mu}}\Omega_e)(\bar{\ell}_sH\gamma^{\bar{\mu}}H^\dagger\ell_r) \\ &- \frac{i}{4}\left[\bar{y}_e^{ts}\mathcal{C}_{eH}^{tr}+y_e^{tr}\bar{\mathcal{C}}_{eH}^{ts}\right](\Omega_\ell^\dagger\overset{\leftrightarrow}{D}_{\bar{\mu}}\Omega_\ell)(H^\dagger H)(\bar{e}_s\gamma^{\bar{\mu}}e_r) \\ &- \frac{i}{4}\left[\bar{y}_e^{ts}\mathcal{C}_{eH}^{tr}+y_e^{tr}\bar{\mathcal{C}}_{eH}^{ts}\right](\Omega_{\ell,j}^\dagger\overset{\leftrightarrow}{D}_{\bar{\mu}}\Omega_\ell^i)H_i^\dagger H^j(\bar{e}_s\gamma^{\bar{\mu}}e_r) \\ &+ \frac{1}{3}\left[-\bar{y}_e^{rs}\mathcal{C}_{eH}^{rs}-y_e^{rs}\bar{\mathcal{C}}_{eH}^{rs}\right](D_{\bar{\mu}}\Omega_{\ell,k}^*D_{\bar{\mu}}\Omega_\ell^j)(H^\dagger H)H_j^\dagger H^k+\frac{1}{3}\left[-\bar{y}_e^{rs}\mathcal{C}_{eH}^{rs}-y_e^{rs}\bar{\mathcal{C}}_{eH}^{rs}\right](D_{\bar{\mu}}\Omega_e^\dagger D_{\bar{\mu}}\Omega_e)(H^\dagger H)^2 \\ &+ \frac{1}{3}\left[\bar{y}_e^{rs}\mathcal{C}_{eH}^{rs}+y_e^{rs}\bar{\mathcal{C}}_{eH}^{rs}\right]\left[(D_{\bar{\mu}}\Omega_{\ell,k}^*\Omega_\ell^j)(H^\dagger H)D_{\bar{\mu}}H_j^\dagger H^k+(\Omega_{\ell,k}^*D_{\bar{\mu}}\Omega_\ell^j)(H^\dagger H)H_j^\dagger D_{\bar{\mu}}H^k\right] \\ &+ \frac{1}{3}\left[\bar{y}_e^{rs}\mathcal{C}_{eH}^{rs}-y_e^{rs}\bar{\mathcal{C}}_{eH}^{rs}\right]\left[(\Omega_{\ell,k}^*D_{\bar{\mu}}\Omega_\ell^j)(H^\dagger D_{\bar{\mu}}H)H_j^\dagger H^k-(D_{\bar{\mu}}\Omega_{\ell,k}^*\Omega_\ell^j)(D_{\bar{\mu}}H^\dagger H)H_j^\dagger H^k\right] \\ &+ \frac{1}{3}\left[y_e^{rs}\bar{\mathcal{C}}_{eH}^{rs}-\bar{y}_e^{rs}\mathcal{C}_{eH}^{rs}\right]\left[(\Omega_e^\dagger D_{\bar{\mu}}\Omega_e)(H^\dagger H)(H^\dagger D_{\bar{\mu}}H)-(D_{\bar{\mu}}\Omega_e^\dagger\Omega_e)(H^\dagger H)(D_{\bar{\mu}}H^\dagger H)\right] \\ &+ \frac{1}{3}\left[-\bar{y}_e^{rs}\mathcal{C}_{eH}^{rs}-y_e^{rs}\bar{\mathcal{C}}_{eH}^{rs}\right]\left[(\Omega_e^\dagger D_{\bar{\mu}}\Omega_e)(H^\dagger H)(H^\dagger D_{\bar{\mu}}H)+(D_{\bar{\mu}}\Omega_e^\dagger\Omega_e)(H^\dagger H)(D_{\bar{\mu}}H^\dagger H)\right], \end{aligned} \quad (3.18)$$

$$\begin{aligned} \Gamma_\Omega^{(1)}[\mathcal{O}_{uH}] &= \frac{1}{6}\left[-\bar{y}_u^{rs}\mathcal{C}_{uH}^{rs}-y_u^{rs}\bar{\mathcal{C}}_{uH}^{rs}\right]\left[(\Omega_{q,ak}^*D_{\bar{\mu}}\Omega_q^{bj})(\Omega_{u,b}^*D_{\bar{\mu}}\Omega_u^a)(H^\dagger H)H_j^\dagger H^k+ \right. \\ &\quad \left. (D_{\bar{\mu}}\Omega_{q,ak}^*\Omega_q^{bj})(D_{\bar{\mu}}\Omega_{u,b}^*\Omega_u^a)(H^\dagger H)H_j^\dagger H^k\right] \\ &+ \frac{1}{6}\left[\bar{y}_u^{rs}\mathcal{C}_{uH}^{rs}+y_u^{rs}\bar{\mathcal{C}}_{uH}^{rs}\right]\left[(\Omega_{q,a}^*D_{\bar{\mu}}\Omega_q^b)(\Omega_{u,b}^*D_{\bar{\mu}}\Omega_u^a)(H^\dagger H)^2+(D_{\bar{\mu}}\Omega_{q,a}^*\Omega_q^b)(D_{\bar{\mu}}\Omega_{u,b}^*\Omega_u^a)(H^\dagger H)^2\right] \\ &+ \frac{i}{4}\left[\bar{y}_u^{ts}\mathcal{C}_{uH}^{tr}+y_u^{tr}\bar{\mathcal{C}}_{uH}^{ts}\right](\Omega_{q,aj}^\dagger\overset{\leftrightarrow}{D}_{\bar{\mu}}\Omega_q^{bi})H_i^\dagger H^j(\bar{u}_{bs}\gamma^{\bar{\mu}}u_r^a) \\ &+ \frac{i}{4}\left[\bar{y}_u^{rt}\mathcal{C}_{uH}^{st}+y_u^{st}\bar{\mathcal{C}}_{uH}^{rt}\right](\Omega_{u,a}^*\overset{\leftrightarrow}{D}_{\bar{\mu}}\Omega_u^b)(\bar{q}_{bs}H\gamma^{\bar{\mu}}H^\dagger q_r^a) \\ &+ \frac{1}{3}\left[\bar{y}_u^{rs}\mathcal{C}_{uH}^{rs}+y_u^{rs}\bar{\mathcal{C}}_{uH}^{rs}\right](D_{\bar{\mu}}\Omega_{q,k}^*D_{\bar{\mu}}\Omega_q^j)(H^\dagger H)H_j^\dagger H^k+\frac{1}{3}\left[-\bar{y}_u^{rs}\mathcal{C}_{uH}^{rs}-y_u^{rs}\bar{\mathcal{C}}_{uH}^{rs}\right](D_{\bar{\mu}}\Omega_q^\dagger D_{\bar{\mu}}\Omega_q)(H^\dagger H)^2 \end{aligned}$$

$$\begin{aligned}
& + \frac{1}{3} \left[ -\bar{y}_u^{rs} \mathcal{C}_{uH}^{rs} - y_u^{rs} \bar{\mathcal{C}}_{uH}^{rs} \right] (D_{\bar{\mu}} \Omega_u^\dagger D_{\bar{\mu}} \Omega_u) (H^\dagger H)^2 \\
& + \frac{1}{3} \left[ \bar{y}_u^{rs} \mathcal{C}_{uH}^{rs} + y_u^{rs} \bar{\mathcal{C}}_{uH}^{rs} \right] \left[ (D_{\bar{\mu}} \Omega_{q,k}^* \Omega_q^j) (H^\dagger H) D_{\bar{\mu}} H_j^\dagger H^k + (\Omega_{q,k}^* D_{\bar{\mu}} \Omega_q^j) (H^\dagger H) H_j^\dagger D_{\bar{\mu}} H^k \right] \\
& + \frac{1}{3} \left[ y_u^{rs} \mathcal{C}_{uH}^{rs} - \bar{y}_u^{rs} \mathcal{C}_{uH}^{rs} \right] \left[ (\Omega_{q,k}^* D_{\bar{\mu}} \Omega_q^j) (H^\dagger D_{\bar{\mu}} H) H_j^\dagger H^k - (D_{\bar{\mu}} \Omega_{q,k}^* \Omega_q^j) (D_{\bar{\mu}} H^\dagger H) H_j^\dagger H^k \right] \\
& + \frac{1}{3} \left[ \bar{y}_u^{rs} \mathcal{C}_{uH}^{rs} - y_u^{rs} \bar{\mathcal{C}}_{uH}^{rs} \right] \left[ (\Omega_q^\dagger D_{\bar{\mu}} \Omega_q) (H^\dagger H) (H^\dagger D_{\bar{\mu}} H) - (D_{\bar{\mu}} \Omega_q^\dagger \Omega_q) (H^\dagger H) (D_{\bar{\mu}} H^\dagger H) \right] \\
& + \frac{1}{3} \left[ -\bar{y}_u^{rs} \mathcal{C}_{uH}^{rs} - y_u^{rs} \bar{\mathcal{C}}_{uH}^{rs} \right] \left[ (\Omega_q^\dagger D_{\bar{\mu}} \Omega_q) (H^\dagger H) (H^\dagger D_{\bar{\mu}} H) + (D_{\bar{\mu}} \Omega_q^\dagger \Omega_q) (H^\dagger H) (D_{\bar{\mu}} H^\dagger H) \right] \\
& + \frac{1}{3} \left[ y_u^{rs} \mathcal{C}_{uH}^{rs} - \bar{y}_u^{rs} \mathcal{C}_{uH}^{rs} \right] \left[ (\Omega_u^\dagger D_{\bar{\mu}} \Omega_u) (H^\dagger H) (H^\dagger D_{\bar{\mu}} H) - (D_{\bar{\mu}} \Omega_u^\dagger \Omega_u) (H^\dagger H) (D_{\bar{\mu}} H^\dagger H) \right] \\
& + \frac{1}{3} \left[ \bar{y}_u^{rs} \mathcal{C}_{uH}^{rs} + y_u^{rs} \bar{\mathcal{C}}_{uH}^{rs} \right] \left[ (\Omega_u^\dagger D_{\bar{\mu}} \Omega_u) (H^\dagger H) (H^\dagger D_{\bar{\mu}} H) + (D_{\bar{\mu}} \Omega_u^\dagger \Omega_u) (H^\dagger H) (D_{\bar{\mu}} H^\dagger H) \right] \\
& + \frac{i}{2} \bar{y}_d^{rs} \mathcal{C}_{uH}^{rt} (D_{\bar{\mu}} \Omega_{q,ak}^* \Omega_q^{bj}) H_j^\dagger \tilde{H}_k (\bar{d}_{bs} \gamma^\mu u_t^a) - \frac{i}{2} y_d^{rt} \bar{\mathcal{C}}_{uH}^{rs} (\Omega_{q,ai}^* D_{\bar{\mu}} \Omega_q^{bj}) \tilde{H}^{\dagger j} H^i (\bar{u}_{bs} \gamma^\mu d_t^a) \\
& - \frac{i}{2} \left[ \bar{y}_u^{ts} \mathcal{C}_{uH}^{tr} + y_u^{tr} \bar{\mathcal{C}}_{uH}^{ts} \right] (\Omega_{q,a}^* \overleftrightarrow{D}_{\bar{\mu}} \Omega_q^b) (H^\dagger H) (\bar{u}_{bs} \gamma^\mu u_r^a) \\
& - \frac{i}{2} \left[ \bar{y}_u^{rt} \mathcal{C}_{uH}^{st} + y_u^{st} \bar{\mathcal{C}}_{uH}^{rt} \right] (\Omega_{u,a}^* \overleftrightarrow{D}_{\bar{\mu}} \Omega_u^b) (H^\dagger H) (\bar{q}_{bs} \gamma^\mu q_r^a), \tag{3.19}
\end{aligned}$$

$$\begin{aligned}
\Gamma_\Omega^{(1)} [\mathcal{O}_{dH}] &= \frac{1}{6} \left[ \bar{y}_d^{rs} \mathcal{C}_{dH}^{rs} + y_d^{rs} \bar{\mathcal{C}}_{dH}^{rs} \right] \left[ (\Omega_{d,a}^* D_{\bar{\mu}} \Omega_d^b) (\Omega_{q,bk}^* D_{\bar{\mu}} \Omega_q^{aj}) (H^\dagger H) H_j^\dagger H^k + (D_{\bar{\mu}} \Omega_{d,a}^* \Omega_d^b) (D_{\bar{\mu}} \Omega_{q,bk}^* \Omega_q^{aj}) (H^\dagger H) H_j^\dagger H^k \right] \\
& - \frac{i}{4} \left[ \bar{y}_d^{rt} \mathcal{C}_{dH}^{st} + y_d^{st} \bar{\mathcal{C}}_{dH}^{rt} \right] (\Omega_{d,a}^* \overleftrightarrow{D}_{\bar{\mu}} \Omega_d^b) (H^\dagger H) (\bar{q}_{bs} \gamma^\mu q_r^a) \\
& - \frac{i}{4} \left[ \bar{y}_d^{rt} \mathcal{C}_{dH}^{st} + y_d^{st} \bar{\mathcal{C}}_{dH}^{rt} \right] (\Omega_{d,a}^* \overleftrightarrow{D}_{\bar{\mu}} \Omega_d^b) (\bar{q}_{bs} H \gamma^\mu H^\dagger q_r^a) \\
& - \frac{i}{4} \left[ \bar{y}_d^{ts} \mathcal{C}_{dH}^{tr} + y_d^{tr} \bar{\mathcal{C}}_{dH}^{ts} \right] (\Omega_{q,a}^* \overleftrightarrow{D}_{\bar{\mu}} \Omega_q^b) (H^\dagger H) (\bar{d}_{bs} \gamma^\mu d_r^a) \\
& - \frac{i}{4} \left[ \bar{y}_d^{ts} \mathcal{C}_{dH}^{tr} + y_d^{tr} \bar{\mathcal{C}}_{dH}^{ts} \right] (\Omega_{q,aj}^* \overleftrightarrow{D}_{\bar{\mu}} \Omega_q^{bi}) H_i^\dagger H^j (\bar{d}_{bs} \gamma^\mu d_r^a) \\
& + \frac{1}{3} \left[ -\bar{y}_d^{rs} \mathcal{C}_{dH}^{rs} - y_d^{rs} \bar{\mathcal{C}}_{dH}^{rs} \right] (D_{\bar{\mu}} \Omega_{q,k}^* D_{\bar{\mu}} \Omega_q^j) (H^\dagger H) H_j^\dagger H^k + \frac{1}{3} \left[ -\bar{y}_d^{rs} \mathcal{C}_{dH}^{rs} - y_d^{rs} \bar{\mathcal{C}}_{dH}^{rs} \right] (D_{\bar{\mu}} \Omega_d^\dagger D_{\bar{\mu}} \Omega_d) (H^\dagger H)^2 \\
& + \frac{1}{3} \left[ \bar{y}_d^{rs} \mathcal{C}_{dH}^{rs} + y_d^{rs} \bar{\mathcal{C}}_{dH}^{rs} \right] \left[ (D_{\bar{\mu}} \Omega_{q,k}^* \Omega_q^j) (H^\dagger H) D_{\bar{\mu}} H_j^\dagger H^k + (\Omega_{q,k}^* D_{\bar{\mu}} \Omega_q^j) (H^\dagger H) H_j^\dagger D_{\bar{\mu}} H^k \right] \\
& + \frac{1}{3} \left[ \bar{y}_d^{rs} \mathcal{C}_{dH}^{rs} - y_d^{rs} \bar{\mathcal{C}}_{dH}^{rs} \right] \left[ (\Omega_{q,k}^* D_{\bar{\mu}} \Omega_q^j) (H^\dagger D_{\bar{\mu}} H) H_j^\dagger H^k - (D_{\bar{\mu}} \Omega_{q,k}^* \Omega_q^j) (D_{\bar{\mu}} H^\dagger H) H_j^\dagger H^k \right] \\
& + \frac{1}{3} \left[ y_d^{rs} \mathcal{C}_{dH}^{rs} - \bar{y}_d^{rs} \mathcal{C}_{dH}^{rs} \right] \left[ (\Omega_d^\dagger D_{\bar{\mu}} \Omega_d) (H^\dagger H) (H^\dagger D_{\bar{\mu}} H) - (D_{\bar{\mu}} \Omega_d^\dagger \Omega_d) (H^\dagger H) (D_{\bar{\mu}} H^\dagger H) \right] \\
& + \frac{1}{3} \left[ -\bar{y}_d^{rs} \mathcal{C}_{dH}^{rs} - y_d^{rs} \bar{\mathcal{C}}_{dH}^{rs} \right] \left[ (\Omega_d^\dagger D_{\bar{\mu}} \Omega_d) (H^\dagger H) (H^\dagger D_{\bar{\mu}} H) + (D_{\bar{\mu}} \Omega_d^\dagger \Omega_d) (H^\dagger H) (D_{\bar{\mu}} H^\dagger H) \right] \\
& + \frac{i}{2} \bar{y}_u^{rt} \bar{\mathcal{C}}_{dH}^{rs} (D_{\bar{\mu}} \Omega_{q,ak}^* \Omega_q^{bj}) H_j^\dagger \tilde{H}_k (\bar{d}_{bs} \gamma^\mu u_t^a) - \frac{i}{2} \bar{y}_u^{rs} \mathcal{C}_{dH}^{rt} (\Omega_{q,ai}^* D_{\bar{\mu}} \Omega_q^{bj}) \tilde{H}^{\dagger j} H^i (\bar{u}_{bs} \gamma^\mu d_t^a), \tag{3.20}
\end{aligned}$$

$$\begin{aligned}
\Gamma_\Omega^{(1)} [\mathcal{O}_{eB}] &= \frac{1}{6} \left[ -\bar{y}_e^{rs} \mathcal{C}_{eB}^{rs} - y_e^{rs} \bar{\mathcal{C}}_{eB}^{rs} \right] \left[ 2(\Omega_e^\dagger D_{\bar{\sigma}} \Omega_e) (\Omega_{\ell,j}^* D_{\bar{\rho}} \Omega_\ell^i) H_i^\dagger H^j \tilde{B}^{\bar{\rho}\bar{\sigma}} - 2(D_{\bar{\mu}} \Omega_e^\dagger \Omega_e) (D_{\bar{\nu}} \Omega_{\ell,j}^* \Omega_\ell^i) H_i^\dagger H^j \tilde{B}^{\bar{\mu}\bar{\nu}} \right] \\
& + \frac{1}{6} g_Y \bar{\mathcal{C}}_{eB}^{rs} (D_{\bar{\mu}} \Omega_{\ell,j}^* \Omega_\ell^i) H_i^\dagger (D^{\bar{\mu}} \bar{e}_s \ell_r^j) + \frac{1}{6} g_Y \mathcal{C}_{eB}^{sr} (\Omega_{\ell,i}^* D_{\bar{\mu}} \Omega_\ell^j) H^i (\bar{\ell}_{js} D^{\bar{\mu}} e_r)
\end{aligned}$$

$$\begin{aligned}
& -\frac{i}{4} \left[ \bar{y}_e^{ts} \mathcal{C}_{eB}^{tr} + y_e^{tr} \bar{\mathcal{C}}_{eB}^{ts} \right] \left[ 2(\Omega_\ell^\dagger D_{\bar{\rho}} \Omega_\ell) \tilde{B}^{\bar{\rho}\bar{\sigma}} (\bar{e}_s \gamma^{\bar{\sigma}} e_r) - 2(D_{\bar{\mu}} \Omega_\ell^\dagger \Omega_\ell) \tilde{B}^{\bar{\mu}\bar{\sigma}} (\bar{e}_s \gamma^{\bar{\sigma}} e_r) \right] \\
& + \frac{i}{4} \left[ \bar{y}_e^{rt} \mathcal{C}_{eB}^{st} + y_e^{st} \bar{\mathcal{C}}_{eB}^{rt} \right] \left[ 2(\Omega_e^\dagger D_{\bar{\rho}} \Omega_e) \tilde{B}^{\bar{\rho}\bar{\sigma}} (\bar{\ell}_s \gamma^{\bar{\sigma}} \ell_r) - 2(D_{\bar{\mu}} \Omega_e^\dagger \Omega_e) \tilde{B}^{\bar{\mu}\bar{\sigma}} (\bar{\ell}_s \gamma^{\bar{\sigma}} \ell_r) \right] \\
& - \frac{i}{4} g_Y \left[ \bar{y}_e^{rt} \mathcal{C}_{eB}^{st} + y_e^{st} \bar{\mathcal{C}}_{eB}^{rt} \right] \left[ (\Omega_{\ell,j}^* D_{\bar{\mu}} \Omega_\ell^i) H_i^\dagger (\bar{\ell}_s H \gamma^{\bar{\mu}} \ell_r^j) - (D_{\bar{\mu}} \Omega_{\ell,j}^* \Omega_\ell^k) H^j (\bar{\ell}_{ks} \gamma^{\bar{\mu}} H^\dagger \ell_r) \right] \\
& - \frac{i}{4} g_Y \left[ \bar{y}_e^{rt} \mathcal{C}_{eB}^{st} - y_e^{st} \bar{\mathcal{C}}_{eB}^{rt} \right] \left[ (\Omega_{\ell,j}^* D_{\bar{\mu}} \Omega_\ell^i) H_i^\dagger (\bar{\ell}_s H \gamma^{\bar{\mu}} \ell_r^j) + (D_{\bar{\mu}} \Omega_{\ell,j}^* \Omega_\ell^k) H^j (\bar{\ell}_{ks} \gamma^{\bar{\mu}} H^\dagger \ell_r) \right] \\
& + \frac{i}{3} \left[ \bar{y}_e^{rs} \mathcal{C}_{eB}^{rs} - y_e^{rs} \bar{\mathcal{C}}_{eB}^{rs} \right] \left[ (\Omega_e^\dagger D_{\bar{\nu}} \Omega_e) (\Omega_{\ell,j}^* D_{\bar{\mu}} \Omega_\ell^i) H_i^\dagger H^j B^{\bar{\mu}\bar{\nu}} - (D_{\bar{\mu}} \Omega_e^\dagger \Omega_e) (D_{\bar{\nu}} \Omega_{\ell,j}^* \Omega_\ell^i) H_i^\dagger H^j B^{\bar{\mu}\bar{\nu}} \right] \\
& + \frac{1}{3} \left[ y_e^{rs} \bar{\mathcal{C}}_{eB}^{rs} - \bar{y}_e^{rs} \mathcal{C}_{eB}^{rs} \right] \left[ 2(\Omega_{\ell,j}^* D_{\bar{\sigma}} \Omega_\ell^i) H_i^\dagger D^{\bar{\mu}} H^j \tilde{B}^{\bar{\mu}\bar{\sigma}} - 2(D_{\bar{\nu}} \Omega_{\ell,j}^* \Omega_\ell^i) D^{\bar{\mu}} H_i^\dagger H^j \tilde{B}^{\bar{\mu}\bar{\nu}} \right] \\
& + \frac{1}{3} \left[ \bar{y}_e^{rs} \mathcal{C}_{eB}^{rs} + y_e^{rs} \bar{\mathcal{C}}_{eB}^{rs} \right] \left[ 2(D_{\bar{\nu}} \Omega_{\ell,j}^* \Omega_\ell^i) D^{\bar{\mu}} H_i^\dagger H^j \tilde{B}^{\bar{\mu}\bar{\nu}} + 2(\Omega_{\ell,j}^* D_{\bar{\sigma}} \Omega_\ell^i) H_i^\dagger D^{\bar{\mu}} H^j \tilde{B}^{\bar{\mu}\bar{\sigma}} \right] \\
& + \frac{1}{3} \left[ y_e^{rs} \bar{\mathcal{C}}_{eB}^{rs} - \bar{y}_e^{rs} \mathcal{C}_{eB}^{rs} \right] \left[ 2(\Omega_e^\dagger D_{\bar{\sigma}} \Omega_e) \tilde{B}^{\bar{\mu}\bar{\sigma}} (H^\dagger D_{\bar{\mu}} H) - 2(D_{\bar{\nu}} \Omega_e^\dagger \Omega_e) \tilde{B}^{\bar{\mu}\bar{\nu}} (D_{\bar{\mu}} H^\dagger H) \right] \\
& + \frac{1}{3} \left[ \bar{y}_e^{rs} \mathcal{C}_{eB}^{rs} + y_e^{rs} \bar{\mathcal{C}}_{eB}^{rs} \right] \left[ 2(\Omega_e^\dagger D_{\bar{\sigma}} \Omega_e) \tilde{B}^{\bar{\mu}\bar{\sigma}} (H^\dagger D_{\bar{\mu}} H) + 2(D_{\bar{\nu}} \Omega_e^\dagger \Omega_e) \tilde{B}^{\bar{\mu}\bar{\nu}} (D_{\bar{\mu}} H^\dagger H) \right] \\
& + \frac{i}{3} g_Y \bar{\mathcal{C}}_{eB}^{rs} (D_{\bar{\nu}} \Omega_{\ell,j}^* \Omega_\ell^i) D^{\bar{\mu}} H_i^\dagger (\bar{e}_s \sigma^{\bar{\mu}\bar{\nu}} \ell_r^j) - \frac{i}{3} g_Y \mathcal{C}_{eB}^{sr} (\Omega_{\ell,i}^* D_{\bar{\nu}} \Omega_\ell^j) D^{\bar{\mu}} H^i (\bar{\ell}_{js} \sigma^{\bar{\mu}\bar{\nu}} e_r) \\
& + \frac{1}{2} g_Y \bar{\mathcal{C}}_{eB}^{rs} (D_{\bar{\mu}} \Omega_{\ell,j}^* \Omega_\ell^i) D^{\bar{\mu}} H_i^\dagger (\bar{e}_s \ell_r^j) \\
& + \frac{1}{2} \left[ y_e^{tr} \bar{\mathcal{C}}_{eB}^{ts} - \bar{y}_e^{ts} \mathcal{C}_{eB}^{tr} \right] \left[ (\Omega_\ell^\dagger D_{\bar{\nu}} \Omega_\ell) B^{\bar{\mu}\bar{\nu}} (\bar{e}_s \gamma^{\bar{\mu}} e_r) + (D_{\bar{\mu}} \Omega_\ell^\dagger \Omega_\ell) B^{\bar{\mu}\bar{\nu}} (\bar{e}_s \gamma^{\bar{\nu}} e_r) \right] \\
& + \frac{1}{2} \left[ \bar{y}_e^{rt} \mathcal{C}_{eB}^{st} - y_e^{st} \bar{\mathcal{C}}_{eB}^{rt} \right] \left[ (\Omega_e^\dagger D_{\bar{\nu}} \Omega_e) B^{\bar{\mu}\bar{\nu}} (\bar{\ell}_s \gamma^{\bar{\mu}} \ell_r) + (D_{\bar{\mu}} \Omega_e^\dagger \Omega_e) B^{\bar{\mu}\bar{\nu}} (\bar{\ell}_s \gamma^{\bar{\nu}} \ell_r) \right] \\
& + \frac{1}{2} g_Y \mathcal{C}_{eB}^{sr} (\Omega_{\ell,i}^* D_{\bar{\mu}} \Omega_\ell^j) D^{\bar{\mu}} H^i (\bar{\ell}_{js} e_r) - \frac{1}{3} g_Y \bar{\mathcal{C}}_{eB}^{rs} (D_{\bar{\mu}} \Omega_e^\dagger \Omega_e) (\bar{e}_s H^\dagger D^{\bar{\mu}} \ell_r) - \frac{1}{3} g_Y \mathcal{C}_{eB}^{sr} (\Omega_e^\dagger D_{\bar{\mu}} \Omega_e) (D^{\bar{\mu}} \bar{\ell}_s H e_r) \\
& - \frac{1}{2} g_Y \bar{\mathcal{C}}_{eB}^{rs} (D_{\bar{\mu}} \Omega_{\ell,j}^* D_{\bar{\mu}} \Omega_\ell^i) H_i^\dagger (\bar{e}_s \ell_r^j) - \frac{1}{2} g_Y \bar{\mathcal{C}}_{eB}^{rs} (D_{\bar{\mu}} \Omega_{\ell,j}^* \Omega_\ell^i) H_i^\dagger (\bar{e}_s D^{\bar{\mu}} \ell_r^j) \\
& - \frac{1}{2} g_Y \mathcal{C}_{eB}^{sr} (D_{\bar{\mu}} \Omega_{\ell,i}^* D_{\bar{\mu}} \Omega_\ell^j) H^i (\bar{\ell}_{js} e_r) - \frac{1}{2} g_Y \mathcal{C}_{eB}^{sr} (\Omega_{\ell,i}^* D_{\bar{\mu}} \Omega_\ell^j) H^i (D^{\bar{\mu}} \bar{\ell}_{js} e_r) \\
& - \frac{i}{2} g_Y \left[ \bar{y}_e^{ts} \mathcal{C}_{eB}^{tr} + y_e^{tr} \bar{\mathcal{C}}_{eB}^{ts} \right] (\Omega_e^\dagger \bar{D}_{\bar{\mu}} \Omega_e) (H^\dagger H) (\bar{e}_s \gamma^{\bar{\mu}} e_r) \\
& + \frac{2i}{3} \left[ \bar{y}_e^{rs} \mathcal{C}_{eB}^{rs} + y_e^{rs} \bar{\mathcal{C}}_{eB}^{rs} \right] \left[ (\Omega_{\ell,j}^* D_{\bar{\nu}} \Omega_\ell^i) H_i^\dagger D^{\bar{\mu}} H^j B^{\bar{\mu}\bar{\nu}} - (D_{\bar{\nu}} \Omega_{\ell,j}^* \Omega_\ell^i) D^{\bar{\mu}} H_i^\dagger H^j B^{\bar{\mu}\bar{\nu}} \right] \\
& - \frac{2i}{3} \left[ \bar{y}_e^{rs} \mathcal{C}_{eB}^{rs} - y_e^{rs} \bar{\mathcal{C}}_{eB}^{rs} \right] \left[ (D_{\bar{\nu}} \Omega_{\ell,j}^* \Omega_\ell^i) D^{\bar{\mu}} H_i^\dagger H^j B^{\bar{\mu}\bar{\nu}} + (\Omega_{\ell,j}^* D_{\bar{\nu}} \Omega_\ell^i) H_i^\dagger D^{\bar{\mu}} H^j B^{\bar{\mu}\bar{\nu}} \right] \\
& + \frac{2i}{3} \left[ \bar{y}_e^{rs} \mathcal{C}_{eB}^{rs} + y_e^{rs} \bar{\mathcal{C}}_{eB}^{rs} \right] \left[ (\Omega_e^\dagger D_{\bar{\nu}} \Omega_e) B^{\bar{\mu}\bar{\nu}} (H^\dagger D_{\bar{\mu}} H) - (D_{\bar{\nu}} \Omega_e^\dagger \Omega_e) B^{\bar{\mu}\bar{\nu}} (D_{\bar{\mu}} H^\dagger H) \right] \\
& - \frac{2i}{3} \left[ \bar{y}_e^{rs} \mathcal{C}_{eB}^{rs} - y_e^{rs} \bar{\mathcal{C}}_{eB}^{rs} \right] \left[ (\Omega_e^\dagger D_{\bar{\nu}} \Omega_e) B^{\bar{\mu}\bar{\nu}} (H^\dagger D_{\bar{\mu}} H) + (D_{\bar{\nu}} \Omega_e^\dagger \Omega_e) B^{\bar{\mu}\bar{\nu}} (D_{\bar{\mu}} H^\dagger H) \right] \\
& + \frac{2i}{3} g_Y \bar{\mathcal{C}}_{eB}^{rs} (D_{\bar{\nu}} \Omega_e^\dagger \Omega_e) (\bar{e}_s \sigma^{\bar{\mu}\bar{\nu}} D_{\bar{\mu}} H^\dagger \ell_r) - \frac{2i}{3} g_Y \mathcal{C}_{eB}^{sr} (\Omega_e^\dagger D_{\bar{\nu}} \Omega_e) (\bar{\ell}_s D_{\bar{\mu}} H \sigma^{\bar{\mu}\bar{\nu}} e_r) \\
& + g_Y \bar{\mathcal{C}}_{eB}^{rs} (D_{\bar{\mu}} \Omega_e^\dagger \Omega_e) (D^{\bar{\mu}} \bar{e}_s H^\dagger \ell_r) + g_Y \mathcal{C}_{eB}^{sr} (\Omega_e^\dagger D_{\bar{\mu}} \Omega_e) (\bar{\ell}_s H D^{\bar{\mu}} e_r) - g_Y \bar{\mathcal{C}}_{eB}^{rs} (D_{\bar{\mu}} \Omega_e^\dagger D_{\bar{\mu}} \Omega_e) (\bar{e}_s H^\dagger \ell_r)
\end{aligned}$$

$$-g_Y \bar{\mathcal{C}}_{eB}^{rs} (D_{\bar{\mu}} \Omega_e^\dagger \Omega_e) (\bar{e}_s D_{\bar{\mu}} H^\dagger \ell_r) - g_Y \mathcal{C}_{eB}^{sr} (D_{\bar{\mu}} \Omega_e^\dagger D_{\bar{\mu}} \Omega_e) (\bar{\ell}_s H e_r) - g_Y \mathcal{C}_{eB}^{sr} (\Omega_e^\dagger D_{\bar{\mu}} \Omega_e) (\bar{\ell}_s D_{\bar{\mu}} H e_r), \quad (3.21)$$

$$\begin{aligned} \Gamma_\Omega^{(1)} [\mathcal{O}_{eW}] = & \frac{1}{6} g_L \bar{\mathcal{C}}_{eW}^{rs} (D_{\bar{\mu}} \Omega_{\ell,j}^* \Omega_\ell^i) H_i^\dagger (D^\mu \bar{e}_s \ell_r^j) + \frac{1}{6} g_L \mathcal{C}_{eW}^{sr} (\Omega_{\ell,i}^* D_{\bar{\mu}} \Omega_\ell^j) H^i (\bar{\ell}_{js} D^\mu e_r) \\ & - \frac{i}{4} g_L \left[ \bar{y}_e^{rt} \mathcal{C}_{eW}^{st} + y_e^{st} \bar{\mathcal{C}}_{eW}^{rt} \right] \left[ (\Omega_{\ell,j}^* D_{\bar{\mu}} \Omega_\ell^i) H_i^\dagger (\bar{\ell}_s H \gamma^\mu \ell_r^j) - (D_{\bar{\mu}} \Omega_{\ell,j}^* \Omega_\ell^k) H^j (\bar{\ell}_{ks} \gamma^\mu H^\dagger \ell_r) \right] \\ & - \frac{i}{4} g_L \left[ \bar{y}_e^{rt} \mathcal{C}_{eW}^{st} - y_e^{st} \bar{\mathcal{C}}_{eW}^{rt} \right] \left[ (\Omega_{\ell,j}^* D_{\bar{\mu}} \Omega_\ell^i) H_i^\dagger (\bar{\ell}_s H \gamma^\mu \ell_r^j) + (D_{\bar{\mu}} \Omega_{\ell,j}^* \Omega_\ell^k) H^j (\bar{\ell}_{ks} \gamma^\mu H^\dagger \ell_r) \right] \\ & + \frac{1}{3} \left[ -\bar{y}_e^{rs} \mathcal{C}_{eW}^{rs} - y_e^{rs} \bar{\mathcal{C}}_{eW}^{rs} \right] \left[ 2t_k^{Ij} (\Omega_e^\dagger D_{\bar{\sigma}} \Omega_e) (\Omega_{\ell,j}^* D_{\bar{\rho}} \Omega_\ell^i) H_i^\dagger H^k \widetilde{W}^{\bar{\rho}\bar{\sigma}I} - 2t_k^{Ii} (D_{\bar{\mu}} \Omega_e^\dagger \Omega_e) (D_{\bar{\nu}} \Omega_{\ell,j}^* \Omega_\ell^k) H_i^\dagger H^j \widetilde{W}^{\bar{\mu}\bar{\nu}I} \right] \\ & + \frac{1}{3} \left[ y_e^{rs} \bar{\mathcal{C}}_{eW}^{rs} - \bar{y}_e^{rs} \mathcal{C}_{eW}^{rs} \right] \left[ 2t_k^{Ii} (D_{\bar{\mu}} \Omega_e^\dagger \Omega_e) (D_{\bar{\nu}} \Omega_{\ell,j}^* \Omega_\ell^k) H_i^\dagger H^j \widetilde{W}^{\bar{\mu}\bar{\nu}I} + 2t_k^{Ij} (\Omega_e^\dagger D_{\bar{\sigma}} \Omega_e) (\Omega_{\ell,j}^* D_{\bar{\rho}} \Omega_\ell^i) H_i^\dagger H^k \widetilde{W}^{\bar{\rho}\bar{\sigma}I} \right] \\ & + \frac{i}{3} g_L \bar{\mathcal{C}}_{eW}^{rs} (D_{\bar{\nu}} \Omega_{\ell,j}^* \Omega_\ell^i) D_{\bar{\mu}} H_i^\dagger (\bar{e}_s \sigma^{\bar{\mu}\bar{\nu}} \ell_r^j) + \frac{1}{2} g_L \bar{\mathcal{C}}_{eW}^{rs} (D_{\bar{\mu}} \Omega_{\ell,j}^* \Omega_\ell^i) D_{\bar{\mu}} H_i^\dagger (\bar{e}_s \ell_r^j) \\ & - \frac{1}{3} g_L \bar{\mathcal{C}}_{eW}^{rs} (D_{\bar{\mu}} \Omega_\ell^\dagger \Omega_\ell) (D^\mu \bar{e}_s H^\dagger \ell_r) - \frac{i}{3} g_L \mathcal{C}_{eW}^{sr} (\Omega_{\ell,i}^* D_{\bar{\nu}} \Omega_\ell^j) D_{\bar{\mu}} H^i (\bar{\ell}_{js} \sigma^{\bar{\mu}\bar{\nu}} e_r) \\ & - \frac{i}{2} \left[ \bar{y}_e^{ts} \mathcal{C}_{eW}^{tr} + y_e^{tr} \bar{\mathcal{C}}_{eW}^{ts} \right] \left[ 2t_j^{Ii} (\Omega_{\ell,i}^* D_{\bar{\rho}} \Omega_\ell^j) \widetilde{W}^{\bar{\rho}\bar{\sigma}I} (\bar{e}_s \gamma^{\bar{\sigma}} e_r) - 2t_j^{Ii} (D_{\bar{\mu}} \Omega_{\ell,i}^* \Omega_\ell^j) \widetilde{W}^{\bar{\mu}\bar{\sigma}I} (\bar{e}_s \gamma^{\bar{\sigma}} e_r) \right] \\ & + \frac{i}{2} \left[ \bar{y}_e^{rt} \mathcal{C}_{eW}^{st} + y_e^{st} \bar{\mathcal{C}}_{eW}^{rt} \right] \left[ 2(\Omega_e^\dagger D_{\bar{\rho}} \Omega_e) \widetilde{W}^{\bar{\rho}\bar{\sigma}I} (\bar{\ell}_s t^I \gamma^{\bar{\sigma}} \ell_r) - 2(D_{\bar{\mu}} \Omega_e^\dagger \Omega_e) \widetilde{W}^{\bar{\mu}\bar{\sigma}I} (\bar{\ell}_s t^I \gamma^{\bar{\sigma}} \ell_r) \right] \\ & + \frac{1}{2} g_L \mathcal{C}_{eW}^{sr} (\Omega_{\ell,i}^* D_{\bar{\mu}} \Omega_\ell^j) D_{\bar{\mu}} H^i (\bar{\ell}_{js} e_r) \\ & + \frac{2i}{3} \left[ \bar{y}_e^{rs} \mathcal{C}_{eW}^{rs} - y_e^{rs} \bar{\mathcal{C}}_{eW}^{rs} \right] \left[ t_k^{Ij} (\Omega_e^\dagger D_{\bar{\nu}} \Omega_e) (\Omega_{\ell,j}^* D_{\bar{\mu}} \Omega_\ell^i) H_i^\dagger H^k W^{\bar{\mu}\bar{\nu}I} - t_k^{Ii} (D_{\bar{\mu}} \Omega_e^\dagger \Omega_e) (D_{\bar{\nu}} \Omega_{\ell,j}^* \Omega_\ell^k) H_i^\dagger H^j W^{\bar{\mu}\bar{\nu}I} \right] \\ & + \frac{2i}{3} \left[ \bar{y}_e^{rs} \mathcal{C}_{eW}^{rs} + y_e^{rs} \bar{\mathcal{C}}_{eW}^{rs} \right] \left[ t_k^{Ii} (D_{\bar{\mu}} \Omega_e^\dagger \Omega_e) (D_{\bar{\nu}} \Omega_{\ell,j}^* \Omega_\ell^k) H_i^\dagger H^j W^{\bar{\mu}\bar{\nu}I} + t_k^{Ij} (\Omega_e^\dagger D_{\bar{\nu}} \Omega_e) (\Omega_{\ell,j}^* D_{\bar{\mu}} \Omega_\ell^i) H_i^\dagger H^k W^{\bar{\mu}\bar{\nu}I} \right] \\ & + \frac{2}{3} \left[ y_e^{rs} \bar{\mathcal{C}}_{eW}^{rs} - \bar{y}_e^{rs} \mathcal{C}_{eW}^{rs} \right] \left[ 2t_k^{Ii} (\Omega_{\ell,j}^* D_{\bar{\sigma}} \Omega_\ell^k) H_i^\dagger D_{\bar{\mu}} H^j \widetilde{W}^{\bar{\mu}\bar{\sigma}I} - 2t_k^{Ij} (D_{\bar{\nu}} \Omega_{\ell,j}^* \Omega_\ell^i) D_{\bar{\mu}} H_i^\dagger H^k \widetilde{W}^{\bar{\mu}\bar{\nu}I} \right] \\ & + \frac{2}{3} \left[ \bar{y}_e^{rs} \mathcal{C}_{eW}^{rs} + y_e^{rs} \bar{\mathcal{C}}_{eW}^{rs} \right] \left[ 2t_k^{Ij} (D_{\bar{\nu}} \Omega_{\ell,j}^* \Omega_\ell^i) D_{\bar{\mu}} H_i^\dagger H^k \widetilde{W}^{\bar{\mu}\bar{\nu}I} + 2t_k^{Ii} (\Omega_{\ell,j}^* D_{\bar{\sigma}} \Omega_\ell^k) H_i^\dagger D_{\bar{\mu}} H^j \widetilde{W}^{\bar{\mu}\bar{\sigma}I} \right] \\ & + \frac{2}{3} \left[ y_e^{rs} \bar{\mathcal{C}}_{eW}^{rs} - \bar{y}_e^{rs} \mathcal{C}_{eW}^{rs} \right] \left[ 2(\Omega_e^\dagger D_{\bar{\sigma}} \Omega_e) \widetilde{W}^{\bar{\mu}\bar{\sigma}I} (H^\dagger t^I D_{\bar{\mu}} H) - 2(D_{\bar{\nu}} \Omega_e^\dagger \Omega_e) \widetilde{W}^{\bar{\mu}\bar{\nu}I} (D_{\bar{\mu}} H^\dagger t^I H) \right] \\ & + \frac{2}{3} \left[ \bar{y}_e^{rs} \mathcal{C}_{eW}^{rs} + y_e^{rs} \bar{\mathcal{C}}_{eW}^{rs} \right] \left[ 2t_k^{Ij} (D_{\bar{\nu}} \Omega_{\ell,j}^* \Omega_\ell^i) D_{\bar{\mu}} H_i^\dagger H^k \widetilde{W}^{\bar{\mu}\bar{\nu}I} + 2t_k^{Ii} (\Omega_{\ell,j}^* D_{\bar{\sigma}} \Omega_\ell^k) H_i^\dagger D_{\bar{\mu}} H^j \widetilde{W}^{\bar{\mu}\bar{\sigma}I} \right] \\ & + \frac{2}{3} \left[ y_e^{rs} \bar{\mathcal{C}}_{eW}^{rs} - \bar{y}_e^{rs} \mathcal{C}_{eW}^{rs} \right] \left[ 2(\Omega_e^\dagger D_{\bar{\sigma}} \Omega_e) \widetilde{W}^{\bar{\mu}\bar{\sigma}I} (H^\dagger t^I D_{\bar{\mu}} H) - 2(D_{\bar{\nu}} \Omega_e^\dagger \Omega_e) \widetilde{W}^{\bar{\mu}\bar{\nu}I} (D_{\bar{\mu}} H^\dagger t^I H) \right] \\ & + \frac{2}{3} \left[ \bar{y}_e^{rs} \mathcal{C}_{eW}^{rs} + y_e^{rs} \bar{\mathcal{C}}_{eW}^{rs} \right] \left[ 2(\Omega_e^\dagger D_{\bar{\sigma}} \Omega_e) \widetilde{W}^{\bar{\mu}\bar{\sigma}I} (H^\dagger t^I D_{\bar{\mu}} H) + 2(D_{\bar{\nu}} \Omega_e^\dagger \Omega_e) \widetilde{W}^{\bar{\mu}\bar{\nu}I} (D_{\bar{\mu}} H^\dagger t^I H) \right] \\ & - \frac{2i}{3} g_L \bar{\mathcal{C}}_{eW}^{rs} (D_{\bar{\nu}} \Omega_\ell^\dagger \Omega_\ell) (\bar{e}_s \sigma^{\bar{\mu}\bar{\nu}} D_{\bar{\mu}} H^\dagger \ell_r) + g_L \bar{\mathcal{C}}_{eW}^{rs} (D_{\bar{\mu}} \Omega_\ell^\dagger D_{\bar{\mu}} \Omega_\ell) (\bar{e}_s H^\dagger \ell_r) \\ & + g_L \bar{\mathcal{C}}_{eW}^{rs} (D_{\bar{\mu}} \Omega_\ell^\dagger \Omega_\ell) (\bar{e}_s H^\dagger D_{\bar{\mu}} \ell_r) \\ & + \left[ y_e^{tr} \bar{\mathcal{C}}_{eW}^{ts} - \bar{y}_e^{ts} \mathcal{C}_{eW}^{tr} \right] \left[ t_j^{Ii} (\Omega_{\ell,i}^* D_{\bar{\nu}} \Omega_\ell^j) W^{\bar{\mu}\bar{\nu}I} (\bar{e}_s \gamma^{\bar{\mu}} e_r) + t_j^{Ii} (D_{\bar{\mu}} \Omega_{\ell,i}^* \Omega_\ell^j) W^{\bar{\mu}\bar{\nu}I} (\bar{e}_s \gamma^{\bar{\nu}} e_r) \right] \\ & + g_L \mathcal{C}_{eW}^{sr} (D_{\bar{\mu}} \Omega_\ell^\dagger D_{\bar{\mu}} \Omega_\ell) (\bar{\ell}_s H e_r) + g_L \mathcal{C}_{eW}^{sr} (\Omega_\ell^\dagger D_{\bar{\mu}} \Omega_\ell) (D_{\bar{\mu}} \bar{\ell}_s H e_r) - \frac{1}{3} g_L \mathcal{C}_{eW}^{sr} (\Omega_\ell^\dagger D_{\bar{\mu}} \Omega_\ell) (\bar{\ell}_s H D_{\bar{\mu}} e_r) \\ & - \frac{1}{2} g_L \bar{\mathcal{C}}_{eW}^{rs} (D_{\bar{\mu}} \Omega_{\ell,j}^* D_{\bar{\mu}} \Omega_\ell^i) H_i^\dagger (\bar{e}_s \ell_r^j) - \frac{1}{2} g_L \bar{\mathcal{C}}_{eW}^{rs} (D_{\bar{\mu}} \Omega_{\ell,j}^* \Omega_\ell^i) H_i^\dagger (\bar{e}_s D_{\bar{\mu}} \ell_r^j) \\ & - \frac{1}{2} g_L \mathcal{C}_{eW}^{sr} (D_{\bar{\mu}} \Omega_{\ell,i}^* D_{\bar{\mu}} \Omega_\ell^j) H^i (\bar{\ell}_{js} e_r) - \frac{1}{2} g_L \mathcal{C}_{eW}^{sr} (\Omega_{\ell,i}^* D_{\bar{\mu}} \Omega_\ell^j) H^i (D_{\bar{\mu}} \bar{\ell}_{js} e_r) \end{aligned}$$

$$\begin{aligned}
& + \frac{i}{2} g_L \left[ \bar{y}_e^{rt} \mathcal{C}_{eW}^{st} + y_e^{st} \bar{\mathcal{C}}_{eW}^{rt} \right] (\Omega_{\ell,j}^* \overset{\leftrightarrow}{D}_{\bar{\mu}} \Omega_{\ell}^i) H_i^{\dagger} H^j (\bar{\ell}_s \gamma^{\bar{\mu}} \ell_r) + \frac{2i}{3} g_L \mathcal{C}_{eW}^{sr} (\Omega_{\ell}^{\dagger} D_{\bar{\nu}} \Omega_{\ell}) (\bar{\ell}_s D_{\bar{\mu}} H \sigma^{\bar{\mu}\bar{\nu}} e_r) \\
& + \left[ \bar{y}_e^{rt} \mathcal{C}_{eW}^{st} - y_e^{st} \bar{\mathcal{C}}_{eW}^{rt} \right] \left[ (\Omega_{\ell}^{\dagger} D_{\bar{\nu}} \Omega_{\ell}) W^{\bar{\mu}\bar{\nu}I} (\bar{\ell}_s t^I \gamma^{\bar{\mu}} \ell_r) + (D_{\bar{\mu}} \Omega_{\ell}^{\dagger} \Omega_{\ell}) W^{\bar{\mu}\bar{\nu}I} (\bar{\ell}_s t^I \gamma^{\bar{\nu}} \ell_r) \right] \\
& - g_L \bar{\mathcal{C}}_{eW}^{rs} (D_{\bar{\mu}} \Omega_{\ell}^{\dagger} \Omega_{\ell}) (\bar{e}_s D_{\bar{\mu}} H^{\dagger} \ell_r) - g_L \mathcal{C}_{eW}^{sr} (\Omega_{\ell}^{\dagger} D_{\bar{\mu}} \Omega_{\ell}) (\bar{\ell}_s D_{\bar{\mu}} H e_r) \\
& + \frac{4i}{3} \left[ \bar{y}_e^{rs} \mathcal{C}_{eW}^{rs} + y_e^{rs} \bar{\mathcal{C}}_{eW}^{rs} \right] \left[ t_k^{Ii} (\Omega_{\ell,j}^* D_{\bar{\nu}} \Omega_{\ell}^k) H_i^{\dagger} D^{\bar{\mu}} H^j W^{\bar{\mu}\bar{\nu}I} - t_k^{Ij} (D_{\bar{\nu}} \Omega_{\ell,j}^* \Omega_{\ell}^i) D^{\bar{\mu}} H_i^{\dagger} H^k W^{\bar{\mu}\bar{\nu}I} \right] \\
& - \frac{4i}{3} \left[ \bar{y}_e^{rs} \mathcal{C}_{eW}^{rs} - y_e^{rs} \bar{\mathcal{C}}_{eW}^{rs} \right] \left[ t_k^{Ii} (\Omega_{\ell,j}^* D_{\bar{\nu}} \Omega_{\ell}^k) H_i^{\dagger} D^{\bar{\mu}} H^j W^{\bar{\mu}\bar{\nu}I} + t_k^{Ij} (D_{\bar{\nu}} \Omega_{\ell,j}^* \Omega_{\ell}^i) D^{\bar{\mu}} H_i^{\dagger} H^k W^{\bar{\mu}\bar{\nu}I} \right] \\
& + \frac{4i}{3} \left[ \bar{y}_e^{rs} \mathcal{C}_{eW}^{rs} + y_e^{rs} \bar{\mathcal{C}}_{eW}^{rs} \right] \left[ (\Omega_{\ell}^{\dagger} D_{\bar{\nu}} \Omega_{\ell}) W^{\bar{\mu}\bar{\nu}I} (H^{\dagger} t^I D_{\bar{\mu}} H) - (D_{\bar{\nu}} \Omega_{\ell}^{\dagger} \Omega_{\ell}) W^{\bar{\mu}\bar{\nu}I} (D_{\bar{\mu}} H^{\dagger} t^I H) \right] \\
& - \frac{4i}{3} \left[ \bar{y}_e^{rs} \mathcal{C}_{eW}^{rs} - y_e^{rs} \bar{\mathcal{C}}_{eW}^{rs} \right] \left[ (\Omega_{\ell}^{\dagger} D_{\bar{\nu}} \Omega_{\ell}) W^{\bar{\mu}\bar{\nu}I} (H^{\dagger} t^I D_{\bar{\mu}} H) + (D_{\bar{\nu}} \Omega_{\ell}^{\dagger} \Omega_{\ell}) W^{\bar{\mu}\bar{\nu}I} (D_{\bar{\mu}} H^{\dagger} t^I H) \right], \tag{3.22}
\end{aligned}$$

$$\begin{aligned}
\Gamma_{\Omega}^{(1)} [\mathcal{O}_{uB}] &= \frac{i}{9} g_Y \mathcal{C}_{uB}^{rs} (D_{\bar{\nu}} \Omega_{q,a}^* \Omega_q^b) (\bar{q}_{br} D_{\bar{\mu}} \tilde{H} \sigma^{\bar{\mu}\bar{\nu}} u_s^a) - \frac{i}{9} g_Y \bar{\mathcal{C}}_{uB}^{rs} \bar{\varepsilon}_{jk} (\Omega_{q,ai}^* D_{\bar{\nu}} \Omega_q^{bk}) D^{\bar{\mu}} H^i (\bar{u}_{bs} \sigma^{\bar{\mu}\bar{\nu}} q_r^{aj}) \\
& - \frac{i}{9} g_Y \bar{\mathcal{C}}_{uB}^{rs} (\Omega_{q,a}^* D_{\bar{\nu}} \Omega_q^b) (\bar{u}_{bs} \sigma^{\bar{\mu}\bar{\nu}} D_{\bar{\mu}} \tilde{H}^{\dagger} q_r^a) \\
& + \frac{1}{6} \left[ -\bar{y}_u^{rs} \mathcal{C}_{uB}^{rs} - y_u^{rs} \bar{\mathcal{C}}_{uB}^{rs} \right] \left[ 2(\Omega_{q,aj}^* D_{\bar{\sigma}} \Omega_q^{bi}) (\Omega_{u,b}^* D_{\bar{\rho}} \Omega_u^a) H_i^{\dagger} H^j \tilde{B}^{\bar{\rho}\bar{\sigma}} - 2(D_{\bar{\mu}} \Omega_{q,aj}^* \Omega_q^{bi}) (D_{\bar{\nu}} \Omega_{u,b}^* \Omega_u^a) H_i^{\dagger} H^j \tilde{B}^{\bar{\mu}\bar{\nu}} \right] \\
& + \frac{1}{6} \left[ \bar{y}_u^{rs} \mathcal{C}_{uB}^{rs} + y_u^{rs} \bar{\mathcal{C}}_{uB}^{rs} \right] \left[ 2(\Omega_{q,a}^* D_{\bar{\sigma}} \Omega_q^b) (\Omega_{u,b}^* D_{\bar{\rho}} \Omega_u^a) \tilde{B}^{\bar{\rho}\bar{\sigma}} (H^{\dagger} H) - 2(D_{\bar{\mu}} \Omega_{q,a}^* \Omega_q^b) (D_{\bar{\nu}} \Omega_{u,b}^* \Omega_u^a) \tilde{B}^{\bar{\mu}\bar{\nu}} (H^{\dagger} H) \right] \\
& + \frac{1}{6} g_Y \mathcal{C}_{uB}^{rs} (D_{\bar{\mu}} \Omega_{q,a}^* \Omega_q^b) (D^{\bar{\mu}} \bar{q}_{br} \tilde{H} u_s^a) + \frac{1}{6} g_Y \bar{\mathcal{C}}_{uB}^{rs} \bar{\varepsilon}_{jk} (\Omega_{q,ai}^* D_{\bar{\mu}} \Omega_q^{bk}) H^i (\bar{u}_{bs} D^{\bar{\mu}} q_r^{aj}) \\
& + \frac{1}{6} g_Y \bar{\mathcal{C}}_{uB}^{rs} (\Omega_{q,a}^* D_{\bar{\mu}} \Omega_q^b) (\bar{u}_{bs} \tilde{H}^{\dagger} D^{\bar{\mu}} q_r^a) \\
& - \frac{i}{4} \left[ \bar{y}_u^{ts} \mathcal{C}_{uB}^{tr} + y_u^{tr} \bar{\mathcal{C}}_{uB}^{ts} \right] \left[ 2(\Omega_{q,a}^* D_{\bar{\rho}} \Omega_q^b) \tilde{B}^{\bar{\rho}\bar{\sigma}} (\bar{u}_{bs} \gamma^{\bar{\sigma}} u_r^a) - 2(D_{\bar{\mu}} \Omega_{q,a}^* \Omega_q^b) \tilde{B}^{\bar{\mu}\bar{\sigma}} (\bar{u}_{bs} \gamma^{\bar{\sigma}} u_r^a) \right] \\
& + \frac{i}{3} \left[ \bar{y}_u^{rs} \mathcal{C}_{uB}^{rs} - y_u^{rs} \bar{\mathcal{C}}_{uB}^{rs} \right] \left[ (\Omega_{q,aj}^* D_{\bar{\nu}} \Omega_q^{bi}) (\Omega_{u,b}^* D_{\bar{\mu}} \Omega_u^a) H_i^{\dagger} H^j B^{\bar{\mu}\bar{\nu}} - (D_{\bar{\mu}} \Omega_{q,aj}^* \Omega_q^{bi}) (D_{\bar{\nu}} \Omega_{u,b}^* \Omega_u^a) H_i^{\dagger} H^j B^{\bar{\mu}\bar{\nu}} \right] \\
& + \frac{1}{3} \left[ \bar{y}_u^{rs} \mathcal{C}_{uB}^{rs} - y_u^{rs} \bar{\mathcal{C}}_{uB}^{rs} \right] \left[ 2(\Omega_{q,j}^* D_{\bar{\sigma}} \Omega_q^i) H_i^{\dagger} D^{\bar{\mu}} H^j \tilde{B}^{\bar{\mu}\bar{\sigma}} - 2(D_{\bar{\nu}} \Omega_{q,j}^* \Omega_q^i) D^{\bar{\mu}} H_i^{\dagger} H^j \tilde{B}^{\bar{\mu}\bar{\nu}} \right] \\
& + \frac{1}{3} \left[ \bar{y}_u^{rs} \mathcal{C}_{uB}^{rs} + y_u^{rs} \bar{\mathcal{C}}_{uB}^{rs} \right] \left[ 2(D_{\bar{\nu}} \Omega_{q,j}^* \Omega_q^i) D^{\bar{\mu}} H_i^{\dagger} H^j \tilde{B}^{\bar{\mu}\bar{\nu}} + 2(\Omega_{q,j}^* D_{\bar{\sigma}} \Omega_q^i) H_i^{\dagger} D^{\bar{\mu}} H^j \tilde{B}^{\bar{\mu}\bar{\sigma}} \right] \\
& - \frac{i}{3} \left[ \bar{y}_u^{rs} \mathcal{C}_{uB}^{rs} - y_u^{rs} \bar{\mathcal{C}}_{uB}^{rs} \right] \left[ (\Omega_{q,a}^* D_{\bar{\nu}} \Omega_q^b) (\Omega_{u,b}^* D_{\bar{\mu}} \Omega_u^a) B^{\bar{\mu}\bar{\nu}} (H^{\dagger} H) - (D_{\bar{\mu}} \Omega_{q,a}^* \Omega_q^b) (D_{\bar{\nu}} \Omega_{u,b}^* \Omega_u^a) B^{\bar{\mu}\bar{\nu}} (H^{\dagger} H) \right] \\
& + \frac{1}{3} \left[ y_u^{rs} \bar{\mathcal{C}}_{uB}^{rs} - \bar{y}_u^{rs} \mathcal{C}_{uB}^{rs} \right] \left[ 2(\Omega_q^{\dagger} D_{\bar{\sigma}} \Omega_q) \tilde{B}^{\bar{\mu}\bar{\sigma}} (H^{\dagger} D_{\bar{\mu}} H) - 2(D_{\bar{\nu}} \Omega_q^{\dagger} \Omega_q) \tilde{B}^{\bar{\mu}\bar{\nu}} (D_{\bar{\mu}} H^{\dagger} H) \right] \\
& + \frac{1}{3} \left[ -\bar{y}_u^{rs} \mathcal{C}_{uB}^{rs} - y_u^{rs} \bar{\mathcal{C}}_{uB}^{rs} \right] \left[ 2(\Omega_q^{\dagger} D_{\bar{\sigma}} \Omega_q) \tilde{B}^{\bar{\mu}\bar{\sigma}} (H^{\dagger} D_{\bar{\mu}} H) + 2(D_{\bar{\nu}} \Omega_q^{\dagger} \Omega_q) \tilde{B}^{\bar{\mu}\bar{\nu}} (D_{\bar{\mu}} H^{\dagger} H) \right] \\
& + \frac{1}{3} \left[ y_u^{rs} \bar{\mathcal{C}}_{uB}^{rs} - \bar{y}_u^{rs} \mathcal{C}_{uB}^{rs} \right] \left[ 2(\Omega_u^{\dagger} D_{\bar{\sigma}} \Omega_u) \tilde{B}^{\bar{\mu}\bar{\sigma}} (H^{\dagger} D_{\bar{\mu}} H) - 2(D_{\bar{\nu}} \Omega_u^{\dagger} \Omega_u) \tilde{B}^{\bar{\mu}\bar{\nu}} (D_{\bar{\mu}} H^{\dagger} H) \right] \\
& + \frac{1}{3} \left[ -\bar{y}_u^{rs} \mathcal{C}_{uB}^{rs} - y_u^{rs} \bar{\mathcal{C}}_{uB}^{rs} \right] \left[ 2(\Omega_u^{\dagger} D_{\bar{\sigma}} \Omega_u) \tilde{B}^{\bar{\mu}\bar{\sigma}} (H^{\dagger} D_{\bar{\mu}} H) + 2(D_{\bar{\nu}} \Omega_u^{\dagger} \Omega_u) \tilde{B}^{\bar{\mu}\bar{\nu}} (D_{\bar{\mu}} H^{\dagger} H) \right] \\
& + \frac{4i}{9} g_Y \bar{\mathcal{C}}_{uB}^{rs} (\Omega_{u,a}^* D_{\bar{\nu}} \Omega_u^b) (\bar{u}_{bs} \sigma^{\bar{\mu}\bar{\nu}} D_{\bar{\mu}} \tilde{H}^{\dagger} q_r^a)
\end{aligned}$$

$$\begin{aligned}
& + \frac{1}{2} \left[ y_u^{tr} \bar{\mathcal{C}}_{uB}^{ts} - \bar{y}_u^{ts} \mathcal{C}_{uB}^{tr} \right] \left[ (\Omega_{q,a}^* D_{\bar{\nu}} \Omega_q^b) B^{\bar{\mu}\bar{\nu}} (\bar{u}_{bs} \gamma^{\bar{\mu}} u_r^a) + (D_{\bar{\mu}} \Omega_{q,a}^* \Omega_q^b) B^{\bar{\mu}\bar{\nu}} (\bar{u}_{bs} \gamma^{\bar{\nu}} u_r^a) \right] \\
& - \frac{2i}{3} \left[ \bar{y}_u^{rs} \mathcal{C}_{uB}^{rs} + y_u^{rs} \bar{\mathcal{C}}_{uB}^{rs} \right] \left[ (\Omega_{q,j}^* D_{\bar{\nu}} \Omega_q^i) H_i^\dagger D^{\bar{\mu}} H^j B^{\bar{\mu}\bar{\nu}} - (D_{\bar{\nu}} \Omega_{q,j}^* \Omega_q^i) D^{\bar{\mu}} H_i^\dagger H^j B^{\bar{\mu}\bar{\nu}} \right] \\
& - \frac{2i}{3} \left[ \bar{y}_u^{rs} \mathcal{C}_{uB}^{rs} - y_u^{rs} \bar{\mathcal{C}}_{uB}^{rs} \right] \left[ (D_{\bar{\nu}} \Omega_{q,j}^* \Omega_q^i) D^{\bar{\mu}} H_i^\dagger H^j B^{\bar{\mu}\bar{\nu}} + (\Omega_{q,j}^* D_{\bar{\nu}} \Omega_q^i) H_i^\dagger D^{\bar{\mu}} H^j B^{\bar{\mu}\bar{\nu}} \right] \\
& + \frac{2i}{3} \left[ \bar{y}_u^{rs} \mathcal{C}_{uB}^{rs} + y_u^{rs} \bar{\mathcal{C}}_{uB}^{rs} \right] \left[ (\Omega_q^\dagger D_{\bar{\nu}} \Omega_q) B^{\bar{\mu}\bar{\nu}} (H^\dagger D_{\bar{\mu}} H) - (D_{\bar{\nu}} \Omega_q^\dagger \Omega_q) B^{\bar{\mu}\bar{\nu}} (D_{\bar{\mu}} H^\dagger H) \right] \\
& + \frac{2i}{3} \left[ \bar{y}_u^{rs} \mathcal{C}_{uB}^{rs} - y_u^{rs} \bar{\mathcal{C}}_{uB}^{rs} \right] \left[ (\Omega_q^\dagger D_{\bar{\nu}} \Omega_q) B^{\bar{\mu}\bar{\nu}} (H^\dagger D_{\bar{\mu}} H) + (D_{\bar{\nu}} \Omega_q^\dagger \Omega_q) B^{\bar{\mu}\bar{\nu}} (D_{\bar{\mu}} H^\dagger H) \right] \\
& + \frac{2i}{3} \left[ \bar{y}_u^{rs} \mathcal{C}_{uB}^{rs} + y_u^{rs} \bar{\mathcal{C}}_{uB}^{rs} \right] \left[ (\Omega_u^\dagger D_{\bar{\nu}} \Omega_u) B^{\bar{\mu}\bar{\nu}} (H^\dagger D_{\bar{\mu}} H) - (D_{\bar{\nu}} \Omega_u^\dagger \Omega_u) B^{\bar{\mu}\bar{\nu}} (D_{\bar{\mu}} H^\dagger H) \right] \\
& + \frac{2i}{3} \left[ \bar{y}_u^{rs} \mathcal{C}_{uB}^{rs} - y_u^{rs} \bar{\mathcal{C}}_{uB}^{rs} \right] \left[ (\Omega_u^\dagger D_{\bar{\nu}} \Omega_u) B^{\bar{\mu}\bar{\nu}} (H^\dagger D_{\bar{\mu}} H) + (D_{\bar{\nu}} \Omega_u^\dagger \Omega_u) B^{\bar{\mu}\bar{\nu}} (D_{\bar{\mu}} H^\dagger H) \right] \\
& + \frac{2}{3} g_Y \mathcal{C}_{uB}^{rs} (D_{\bar{\mu}} \Omega_{u,a}^* D_{\bar{\mu}} \Omega_u^b) (\bar{q}_{br} \tilde{H} u_s^a) + \frac{2}{3} g_Y \mathcal{C}_{uB}^{rs} (D_{\bar{\mu}} \Omega_{u,a}^* \Omega_u^b) (\bar{q}_{br} \tilde{H} D^{\bar{\mu}} u_s^a) + \frac{2}{3} g_Y \bar{\mathcal{C}}_{uB}^{rs} (D_{\bar{\mu}} \Omega_{u,a}^* D_{\bar{\mu}} \Omega_u^b) (\bar{u}_{bs} \tilde{H}^\dagger q_r^a) \\
& + \frac{2}{3} g_Y \bar{\mathcal{C}}_{uB}^{rs} (\Omega_{u,a}^* D_{\bar{\mu}} \Omega_u^b) (D^{\bar{\mu}} \bar{u}_{bs} \tilde{H}^\dagger q_r^a) - \frac{1}{18} g_Y \mathcal{C}_{uB}^{rs} (D_{\bar{\mu}} \Omega_{q,a}^* \Omega_q^b) (\bar{q}_{br} \tilde{H} D^{\bar{\mu}} u_s^a) \\
& - \frac{1}{18} g_Y \mathcal{C}_{uB}^{rs} \varepsilon^{kj} (D_{\bar{\mu}} \Omega_{q,aj}^* \Omega_q^{bi}) H_i^\dagger (\bar{q}_{bkr} D^{\bar{\mu}} u_s^a) - \frac{1}{18} g_Y \bar{\mathcal{C}}_{uB}^{rs} \bar{\varepsilon}_{jk} (\Omega_{q,ai}^* D_{\bar{\mu}} \Omega_q^{bk}) H^i (D^{\bar{\mu}} \bar{u}_{bs} q_r^{aj}) \\
& - \frac{1}{18} g_Y \bar{\mathcal{C}}_{uB}^{rs} (\Omega_{q,a}^* D_{\bar{\mu}} \Omega_q^b) (D^{\bar{\mu}} \bar{u}_{bs} \tilde{H}^\dagger q_r^a) \\
& + \frac{i}{12} g_Y \left[ \bar{y}_u^{rt} \mathcal{C}_{uB}^{st} + y_u^{st} \bar{\mathcal{C}}_{uB}^{rt} \right] \left[ (\Omega_{q,aj}^* D_{\bar{\mu}} \Omega_q^{bi}) H_i^\dagger (\bar{q}_{bs} H \gamma^{\bar{\mu}} q_r^{aj}) - (D_{\bar{\mu}} \Omega_{q,aj}^* \Omega_q^{bk}) H^j (\bar{q}_{bks} \gamma^{\bar{\mu}} H^\dagger q_r^a) \right] \\
& - \frac{i}{12} g_Y \left[ \bar{y}_u^{rt} \mathcal{C}_{uB}^{st} - y_u^{st} \bar{\mathcal{C}}_{uB}^{rt} \right] \left[ (\Omega_{q,aj}^* D_{\bar{\mu}} \Omega_q^{bi}) H_i^\dagger (\bar{q}_{bs} H \gamma^{\bar{\mu}} q_r^{aj}) + (D_{\bar{\mu}} \Omega_{q,aj}^* \Omega_q^{bk}) H^j (\bar{q}_{bks} \gamma^{\bar{\mu}} H^\dagger q_r^a) \right] \\
& + \frac{i}{12} g_Y \left[ \bar{y}_u^{rt} \mathcal{C}_{uB}^{st} + y_u^{st} \bar{\mathcal{C}}_{uB}^{rt} \right] (\Omega_{q,a}^* \overleftrightarrow{D}_{\bar{\mu}} \Omega_q^b) (H^\dagger H) (\bar{q}_{bs} \gamma^{\bar{\mu}} q_r^a) \\
& - \frac{i}{12} g_Y \left[ \bar{y}_u^{rt} \mathcal{C}_{uB}^{st} + y_u^{st} \bar{\mathcal{C}}_{uB}^{rt} \right] (\Omega_{q,a}^* \overleftrightarrow{D}_{\bar{\mu}} \Omega_q^b) (\bar{q}_{bs} H \gamma^{\bar{\mu}} H^\dagger q_r^a) \\
& - \frac{i}{12} g_Y \left[ \bar{y}_u^{rt} \mathcal{C}_{uB}^{st} + y_u^{st} \bar{\mathcal{C}}_{uB}^{rt} \right] (\Omega_{q,aj}^* \overleftrightarrow{D}_{\bar{\mu}} \Omega_q^{bi}) H_i^\dagger H^j (\bar{q}_{bs} \gamma^{\bar{\mu}} q_r^a) \\
& + \frac{i}{9} g_Y \mathcal{C}_{uB}^{rs} \varepsilon^{kj} (D_{\bar{\nu}} \Omega_{q,aj}^* \Omega_q^{bi}) D^{\bar{\mu}} H_i^\dagger (\bar{q}_{bkr} \sigma^{\bar{\mu}\bar{\nu}} u_s^a) + \frac{1}{6} g_Y \mathcal{C}_{uB}^{rs} \varepsilon^{kj} (D_{\bar{\mu}} \Omega_{q,aj}^* \Omega_q^{bi}) H_i^\dagger (D^{\bar{\mu}} \bar{q}_{bkr} u_s^a) \\
& - \frac{1}{6} g_Y \mathcal{C}_{uB}^{rs} (D_{\bar{\mu}} \Omega_{q,a}^* D_{\bar{\mu}} \Omega_q^b) (\bar{q}_{br} \tilde{H} u_s^a) - \frac{1}{6} g_Y \mathcal{C}_{uB}^{rs} (D_{\bar{\mu}} \Omega_{q,a}^* \Omega_q^b) (\bar{q}_{br} D_{\bar{\mu}} \tilde{H} u_s^a) \\
& - \frac{1}{6} g_Y \mathcal{C}_{uB}^{rs} \varepsilon^{kj} (D_{\bar{\mu}} \Omega_{q,aj}^* \Omega_q^{bi}) D^{\bar{\mu}} H_i^\dagger (\bar{q}_{bkr} u_s^a) - \frac{1}{6} g_Y \mathcal{C}_{uB}^{rs} \varepsilon^{kj} (D_{\bar{\mu}} \Omega_{q,aj}^* D_{\bar{\mu}} \Omega_q^{bi}) H_i^\dagger (\bar{q}_{bkr} u_s^a) \\
& - \frac{1}{6} g_Y \bar{\mathcal{C}}_{uB}^{rs} \bar{\varepsilon}_{jk} (D_{\bar{\mu}} \Omega_{q,ai}^* D_{\bar{\mu}} \Omega_q^{bk}) H^i (\bar{u}_{bs} q_r^{aj}) - \frac{1}{6} g_Y \bar{\mathcal{C}}_{uB}^{rs} \bar{\varepsilon}_{jk} (\Omega_{q,ai}^* D_{\bar{\mu}} \Omega_q^{bk}) D^{\bar{\mu}} H^i (\bar{u}_{bs} q_r^{aj}) \\
& - \frac{1}{6} g_Y \bar{\mathcal{C}}_{uB}^{rs} (D_{\bar{\mu}} \Omega_{q,a}^* D_{\bar{\mu}} \Omega_q^b) (\bar{u}_{bs} \tilde{H}^\dagger q_r^a) - \frac{1}{6} g_Y \bar{\mathcal{C}}_{uB}^{rs} (\Omega_{q,a}^* D_{\bar{\mu}} \Omega_q^b) (\bar{u}_{bs} D_{\bar{\mu}} \tilde{H}^\dagger q_r^a) \\
& - \frac{2}{9} g_Y \mathcal{C}_{uB}^{rs} (D_{\bar{\mu}} \Omega_{u,a}^* \Omega_u^b) (D^{\bar{\mu}} \bar{q}_{br} \tilde{H} u_s^a) - \frac{2}{9} g_Y \bar{\mathcal{C}}_{uB}^{rs} (\Omega_{u,a}^* D_{\bar{\mu}} \Omega_u^b) (\bar{u}_{bs} \tilde{H}^\dagger D^{\bar{\mu}} q_r^a) \\
& + \frac{i}{4} \left[ \bar{y}_u^{rt} \mathcal{C}_{uB}^{st} + y_u^{st} \bar{\mathcal{C}}_{uB}^{rt} \right] \left[ 2(\Omega_{u,a}^* D_{\bar{\rho}} \Omega_u^b) \tilde{B}^{\bar{\rho}\bar{\sigma}} (\bar{q}_{bs} \gamma^{\bar{\sigma}} q_r^a) - 2(D_{\bar{\mu}} \Omega_{u,a}^* \Omega_u^b) \tilde{B}^{\bar{\mu}\bar{\sigma}} (\bar{q}_{bs} \gamma^{\bar{\sigma}} q_r^a) \right]
\end{aligned}$$

$$\begin{aligned}
& + \frac{i}{3} g_Y \left[ \bar{y}_u^{ts} \mathcal{C}_{uB}^{tr} + y_u^{tr} \bar{\mathcal{C}}_{uB}^{ts} \right] (\Omega_{u,a}^* \overset{\leftrightarrow}{D}_{\bar{\mu}} \Omega_u^b) (H^\dagger H) (\bar{u}_{bs} \gamma^{\bar{\mu}} u_r^a) - \frac{4i}{9} g_Y \mathcal{C}_{uB}^{rs} (D_{\bar{\nu}} \Omega_{u,a}^* \Omega_u^b) (\bar{q}_{br} D_{\bar{\mu}} \tilde{H} \sigma^{\bar{\mu}\bar{\nu}} u_s^a) \\
& + \frac{1}{2} \left[ \bar{y}_u^{rt} \mathcal{C}_{uB}^{st} - y_u^{st} \bar{\mathcal{C}}_{uB}^{rt} \right] \left[ (\Omega_{u,a}^* D_{\bar{\nu}} \Omega_u^b) B^{\bar{\mu}\bar{\nu}} (\bar{q}_{bs} \gamma^{\bar{\mu}} q_r^a) + (D_{\bar{\mu}} \Omega_{u,a}^* \Omega_u^b) B^{\bar{\mu}\bar{\nu}} (\bar{q}_{bs} \gamma^{\bar{\nu}} q_r^a) \right] \\
& - \frac{2}{3} g_Y \mathcal{C}_{uB}^{rs} (D_{\bar{\mu}} \Omega_{u,a}^* \Omega_u^b) (\bar{q}_{br} D_{\bar{\mu}} \tilde{H} u_s^a) - \frac{2}{3} g_Y \bar{\mathcal{C}}_{uB}^{rs} (\Omega_{u,a}^* D_{\bar{\mu}} \Omega_u^b) (\bar{u}_{bs} D_{\bar{\mu}} \tilde{H}^\dagger q_r^a), \tag{3.23}
\end{aligned}$$

$$\begin{aligned}
\Gamma_\Omega^{(1)} [\mathcal{O}_{uW}] &= \frac{1}{6} g_L \mathcal{C}_{uW}^{rs} \varepsilon^{kj} (D_{\bar{\mu}} \Omega_{q,a,j}^* \Omega_q^{bi}) H_i^\dagger (\bar{q}_{bkr} D_{\bar{\mu}} u_s^a) + \frac{1}{6} g_L \bar{\mathcal{C}}_{uW}^{rs} \bar{\varepsilon}_{jk} (\Omega_{q,ai}^* D_{\bar{\mu}} \Omega_q^{bk}) H^i (D_{\bar{\nu}} \bar{u}_{bs} q_r^{aj}) \\
& + \frac{1}{3} \left[ \bar{y}_u^{rs} \mathcal{C}_{uW}^{rs} + y_u^{rs} \bar{\mathcal{C}}_{uW}^{rs} \right] \left[ 2t_k^{Ij} (\Omega_{q,aj}^* D_{\bar{\sigma}} \Omega_q^{bi}) (\Omega_{u,b}^* D_{\bar{\rho}} \Omega_u^a) H_i^\dagger H^k \widetilde{W}^{\bar{\rho}\bar{\sigma}I} - 2t_k^{Ii} (D_{\bar{\mu}} \Omega_{q,aj}^* \Omega_q^{bk}) (D_{\bar{\nu}} \Omega_{u,b}^* \Omega_u^a) H_i^\dagger H^j \widetilde{W}^{\bar{\mu}\bar{\nu}I} \right] \\
& + \frac{1}{3} \left[ y_u^{rs} \bar{\mathcal{C}}_{uW}^{rs} - \bar{y}_u^{rs} \mathcal{C}_{uW}^{rs} \right] \left[ 2t_k^{Ii} (D_{\bar{\mu}} \Omega_{q,aj}^* \Omega_q^{bk}) (D_{\bar{\nu}} \Omega_{u,b}^* \Omega_u^a) H_i^\dagger H^j \widetilde{W}^{\bar{\mu}\bar{\nu}I} + 2t_k^{Ij} (\Omega_{q,aj}^* D_{\bar{\sigma}} \Omega_q^{bi}) (\Omega_{u,b}^* D_{\bar{\rho}} \Omega_u^a) H_i^\dagger H^k \widetilde{W}^{\bar{\rho}\bar{\sigma}I} \right] \\
& + \frac{1}{3} \left[ -\bar{y}_u^{rs} \mathcal{C}_{uW}^{rs} - y_u^{rs} \bar{\mathcal{C}}_{uW}^{rs} \right] \left[ 2(\Omega_{q,a}^* D_{\bar{\sigma}} \Omega_q^b) (\Omega_{u,b}^* D_{\bar{\rho}} \Omega_u^a) \widetilde{W}^{\bar{\rho}\bar{\sigma}I} (H^\dagger t^I H) - 2(D_{\bar{\mu}} \Omega_{q,a}^* \Omega_q^b) (D_{\bar{\nu}} \Omega_{u,b}^* \Omega_u^a) \widetilde{W}^{\bar{\mu}\bar{\nu}I} (H^\dagger t^I H) \right] \\
& - \frac{1}{6} g_L \bar{\mathcal{C}}_{uW}^{rs} (\Omega_{q,a}^* D_{\bar{\mu}} \Omega_q^b) (D_{\bar{\mu}} \bar{u}_{bs} \tilde{H}^\dagger q_r^a) \\
& - \frac{i}{4} g_L \left[ \bar{y}_u^{rt} \mathcal{C}_{uW}^{st} + y_u^{st} \bar{\mathcal{C}}_{uW}^{rt} \right] \left[ (\Omega_{q,aj}^* D_{\bar{\mu}} \Omega_q^{bi}) H_i^\dagger (\bar{q}_{bs} H \gamma^{\bar{\mu}} q_r^{aj}) - (D_{\bar{\mu}} \Omega_{q,aj}^* \Omega_q^{bk}) H^j (\bar{q}_{bks} \gamma^{\bar{\mu}} H^\dagger q_r^a) \right] \\
& + \frac{i}{4} g_L \left[ \bar{y}_u^{rt} \mathcal{C}_{uW}^{st} - y_u^{st} \bar{\mathcal{C}}_{uW}^{rt} \right] \left[ (\Omega_{q,aj}^* D_{\bar{\mu}} \Omega_q^{bi}) H_i^\dagger (\bar{q}_{bs} H \gamma^{\bar{\mu}} q_r^{aj}) + (D_{\bar{\mu}} \Omega_{q,aj}^* \Omega_q^{bk}) H^j (\bar{q}_{bks} \gamma^{\bar{\mu}} H^\dagger q_r^a) \right] \\
& + \frac{i}{4} g_L \left[ \bar{y}_u^{rt} \mathcal{C}_{uW}^{st} + y_u^{st} \bar{\mathcal{C}}_{uW}^{rt} \right] (\Omega_{q,a}^* \overset{\leftrightarrow}{D}_{\bar{\mu}} \Omega_q^b) (H^\dagger H) (\bar{q}_{bs} \gamma^{\bar{\mu}} q_r^a) \\
& + \frac{i}{4} g_L \left[ \bar{y}_u^{rt} \mathcal{C}_{uW}^{st} + y_u^{st} \bar{\mathcal{C}}_{uW}^{rt} \right] (\Omega_{q,a}^* \overset{\leftrightarrow}{D}_{\bar{\mu}} \Omega_q^b) (\bar{q}_{bs} H \gamma^{\bar{\mu}} H^\dagger q_r^a) \\
& - \frac{i}{4} g_L \left[ \bar{y}_u^{rt} \mathcal{C}_{uW}^{st} + y_u^{st} \bar{\mathcal{C}}_{uW}^{rt} \right] (\Omega_{q,aj}^* \overset{\leftrightarrow}{D}_{\bar{\mu}} \Omega_q^{bi}) H_i^\dagger H^j (\bar{q}_{bs} \gamma^{\bar{\mu}} q_r^a) + \frac{i}{3} g_L \mathcal{C}_{uW}^{rs} (D_{\bar{\nu}} \Omega_{q,a}^* \Omega_q^b) (\bar{q}_{br} D_{\bar{\mu}} \tilde{H} \sigma^{\bar{\mu}\bar{\nu}} u_s^a) \\
& - \frac{i}{3} g_L \mathcal{C}_{uW}^{rs} \varepsilon^{kj} (D_{\bar{\nu}} \Omega_{q,aj}^* \Omega_q^{bi}) D_{\bar{\mu}} H_i^\dagger (\bar{q}_{bkr} \sigma^{\bar{\mu}\bar{\nu}} u_s^a) + \frac{i}{3} g_L \bar{\mathcal{C}}_{uW}^{rs} \bar{\varepsilon}_{jk} (\Omega_{q,ai}^* D_{\bar{\nu}} \Omega_q^{bk}) D_{\bar{\mu}} H^i (\bar{u}_{bs} \sigma^{\bar{\mu}\bar{\nu}} q_r^{aj}) \\
& - \frac{i}{3} g_L \bar{\mathcal{C}}_{uW}^{rs} (\Omega_{q,a}^* D_{\bar{\nu}} \Omega_q^b) (\bar{u}_{bs} \sigma^{\bar{\mu}\bar{\nu}} D_{\bar{\mu}} \tilde{H}^\dagger q_r^a) + \frac{1}{2} g_L \mathcal{C}_{uW}^{rs} (D_{\bar{\mu}} \Omega_{q,a}^* \Omega_q^b) (D_{\bar{\mu}} \bar{q}_{br} \tilde{H} u_s^a) \\
& + \frac{i}{2} \left[ \bar{y}_u^{rt} \mathcal{C}_{uW}^{st} + y_u^{st} \bar{\mathcal{C}}_{uW}^{rt} \right] \left[ 2(\Omega_{u,a}^* D_{\bar{\rho}} \Omega_u^b) \widetilde{W}^{\bar{\rho}\bar{\sigma}I} (\bar{q}_{bs} t^I \gamma^{\bar{\sigma}} q_r^a) - 2(D_{\bar{\mu}} \Omega_{u,a}^* \Omega_u^b) \widetilde{W}^{\bar{\mu}\bar{\sigma}I} (\bar{q}_{bs} t^I \gamma^{\bar{\sigma}} q_r^a) \right] \\
& + \frac{1}{2} g_L \mathcal{C}_{uW}^{rs} \varepsilon^{kj} (D_{\bar{\mu}} \Omega_{q,aj}^* \Omega_q^{bi}) D_{\bar{\mu}} H_i^\dagger (\bar{q}_{bkr} u_s^a) + \frac{1}{2} g_L \mathcal{C}_{uW}^{rs} \varepsilon^{kj} (D_{\bar{\mu}} \Omega_{q,aj}^* D_{\bar{\mu}} \Omega_q^{bi}) H_i^\dagger (\bar{q}_{bkr} u_s^a) \\
& + \frac{1}{2} g_L \bar{\mathcal{C}}_{uW}^{rs} \bar{\varepsilon}_{jk} (D_{\bar{\mu}} \Omega_{q,ai}^* D_{\bar{\mu}} \Omega_q^{bk}) H^i (\bar{u}_{bs} q_r^{aj}) + \frac{1}{2} g_L \bar{\mathcal{C}}_{uW}^{rs} \bar{\varepsilon}_{jk} (\Omega_{q,ai}^* D_{\bar{\mu}} \Omega_q^{bk}) D_{\bar{\mu}} H^i (\bar{u}_{bs} q_r^{aj}) \\
& + \frac{1}{2} g_L \bar{\mathcal{C}}_{uW}^{rs} (\Omega_{q,a}^* D_{\bar{\mu}} \Omega_q^b) (\bar{u}_{bs} \tilde{H}^\dagger D_{\bar{\mu}} q_r^a) \\
& - \frac{2i}{3} \left[ \bar{y}_u^{rs} \mathcal{C}_{uW}^{rs} - y_u^{rs} \bar{\mathcal{C}}_{uW}^{rs} \right] \left[ t_k^{Ii} (D_{\bar{\mu}} \Omega_{q,aj}^* \Omega_q^{bk}) (\Omega_{u,b}^* D_{\bar{\nu}} \Omega_u^a) H_i^\dagger H^j W^{\bar{\mu}\bar{\nu}I} - t_k^{Ij} (\Omega_{q,aj}^* D_{\bar{\nu}} \Omega_q^{bi}) (D_{\bar{\mu}} \Omega_{u,b}^* \Omega_u^a) H_i^\dagger H^k W^{\bar{\mu}\bar{\nu}I} \right] \\
& - \frac{2i}{3} \left[ \bar{y}_u^{rs} \mathcal{C}_{uW}^{rs} + y_u^{rs} \bar{\mathcal{C}}_{uW}^{rs} \right] \left[ t_k^{Ii} (D_{\bar{\mu}} \Omega_{q,aj}^* \Omega_q^{bk}) (\Omega_{u,b}^* D_{\bar{\nu}} \Omega_u^a) H_i^\dagger H^j W^{\bar{\mu}\bar{\nu}I} + t_k^{Ij} (\Omega_{q,aj}^* D_{\bar{\nu}} \Omega_q^{bi}) (D_{\bar{\mu}} \Omega_{u,b}^* \Omega_u^a) H_i^\dagger H^k W^{\bar{\mu}\bar{\nu}I} \right] \\
& + \frac{2}{3} \left[ \bar{y}_u^{rs} \mathcal{C}_{uW}^{rs} - y_u^{rs} \bar{\mathcal{C}}_{uW}^{rs} \right] \left[ 2t_k^{Ij} (\Omega_{q,j}^* D_{\bar{\sigma}} \Omega_q^i) H_i^\dagger D_{\bar{\mu}} H^k \widetilde{W}^{\bar{\mu}\bar{\sigma}I} - 2t_k^{Ii} (D_{\bar{\nu}} \Omega_{q,j}^* \Omega_q^k) D_{\bar{\mu}} H_i^\dagger H^j \widetilde{W}^{\bar{\mu}\bar{\sigma}I} \right] \\
& + \frac{2}{3} \left[ \bar{y}_u^{rs} \mathcal{C}_{uW}^{rs} + y_u^{rs} \bar{\mathcal{C}}_{uW}^{rs} \right] \left[ 2t_k^{Ii} (D_{\bar{\nu}} \Omega_{q,j}^* \Omega_q^k) D_{\bar{\mu}} H_i^\dagger H^j \widetilde{W}^{\bar{\mu}\bar{\nu}I} + 2t_k^{Ij} (\Omega_{q,j}^* D_{\bar{\sigma}} \Omega_q^i) H_i^\dagger D_{\bar{\mu}} H^k \widetilde{W}^{\bar{\mu}\bar{\sigma}I} \right]
\end{aligned}$$

$$\begin{aligned}
& + \frac{2}{3} [\bar{y}_u^{rs} \mathcal{C}_{uW}^{rs} + y_u^{rs} \bar{\mathcal{C}}_{uW}^{rs}] \left[ 2t_k^{Ij} (\Omega_{q,j}^* D_{\bar{\sigma}} \Omega_q^k) \widetilde{W}^{\bar{\mu}\bar{\sigma}I} (D_{\bar{\mu}} H^\dagger H) - 2t_k^{Ij} (D_{\bar{\mu}} \Omega_{q,j}^* \Omega_q^k) \widetilde{W}^{\bar{\mu}\bar{\nu}I} (H^\dagger D_{\bar{\nu}} H) \right] \\
& + \frac{2}{3} [\bar{y}_u^{rs} \bar{\mathcal{C}}_{uW}^{rs} - y_u^{rs} \mathcal{C}_{uW}^{rs}] \left[ 2t_k^{Ij} (D_{\bar{\mu}} \Omega_{q,j}^* \Omega_q^k) \widetilde{W}^{\bar{\mu}\bar{\nu}I} (H^\dagger D_{\bar{\nu}} H) + 2t_k^{Ij} (\Omega_{q,j}^* D_{\bar{\sigma}} \Omega_q^k) \widetilde{W}^{\bar{\mu}\bar{\sigma}I} (D_{\bar{\mu}} H^\dagger H) \right] \\
& - \frac{2i}{3} [\bar{y}_u^{rs} \mathcal{C}_{uW}^{rs} - y_u^{rs} \bar{\mathcal{C}}_{uW}^{rs}] \left[ (\Omega_{q,a}^* D_{\bar{\nu}} \Omega_q^b) (D_{\bar{\mu}} \Omega_{u,b}^* \Omega_u^a) W^{\bar{\mu}\bar{\nu}I} (H^\dagger t^I H) - (D_{\bar{\mu}} \Omega_{q,a}^* \Omega_q^b) (\Omega_{u,b}^* D_{\bar{\nu}} \Omega_u^a) W^{\bar{\mu}\bar{\nu}I} (H^\dagger t^I H) \right] \\
& + \frac{2}{3} [\bar{y}_u^{rs} \mathcal{C}_{uW}^{rs} - y_u^{rs} \bar{\mathcal{C}}_{uW}^{rs}] \left[ 2(\Omega_u^\dagger D_{\bar{\sigma}} \Omega_u) \widetilde{W}^{\bar{\mu}\bar{\sigma}I} (H^\dagger t^I D_{\bar{\mu}} H) - 2(D_{\bar{\nu}} \Omega_u^\dagger \Omega_u) \widetilde{W}^{\bar{\mu}\bar{\nu}I} (D_{\bar{\mu}} H^\dagger t^I H) \right] \\
& + \frac{2}{3} [\bar{y}_u^{rs} \mathcal{C}_{uW}^{rs} + y_u^{rs} \bar{\mathcal{C}}_{uW}^{rs}] \left[ 2(\Omega_u^\dagger D_{\bar{\sigma}} \Omega_u) \widetilde{W}^{\bar{\mu}\bar{\sigma}I} (H^\dagger t^I D_{\bar{\mu}} H) + 2(D_{\bar{\nu}} \Omega_u^\dagger \Omega_u) \widetilde{W}^{\bar{\mu}\bar{\nu}I} (D_{\bar{\mu}} H^\dagger t^I H) \right] \\
& + [\bar{y}_u^{rt} \mathcal{C}_{uW}^{st} - y_u^{st} \bar{\mathcal{C}}_{uW}^{rt}] \left[ (\Omega_{u,a}^* D_{\bar{\nu}} \Omega_u^b) W^{\bar{\mu}\bar{\nu}I} (\bar{q}_{bs} t^I \gamma^{\bar{\mu}} q_r^a) + (D_{\bar{\mu}} \Omega_{u,a}^* \Omega_u^b) W^{\bar{\mu}\bar{\nu}I} (\bar{q}_{bs} t^I \gamma^{\bar{\nu}} q_r^a) \right] \\
& - \frac{1}{6} g_L \mathcal{C}_{uW}^{rs} (D_{\bar{\mu}} \Omega_{q,a}^* \Omega_q^b) (\bar{q}_{br} \tilde{H} D_{\bar{\mu}} u_s^a) - \frac{1}{2} g_L \mathcal{C}_{uW}^{rs} (D_{\bar{\mu}} \Omega_{q,a}^* D_{\bar{\mu}} \Omega_q^b) (\bar{q}_{br} \tilde{H} u_s^a) - \frac{1}{2} g_L \mathcal{C}_{uW}^{rs} (D_{\bar{\mu}} \Omega_{q,a}^* \Omega_q^b) (\bar{q}_{br} D_{\bar{\mu}} \tilde{H} u_s^a) \\
& - \frac{1}{2} g_L \mathcal{C}_{uW}^{rs} \varepsilon^{kj} (D_{\bar{\mu}} \Omega_{q,a,j}^* \Omega_q^{bi}) H_i^\dagger (D^{\bar{\mu}} \bar{q}_{bkr} u_s^a) - \frac{1}{2} g_L \bar{\mathcal{C}}_{uW}^{rs} \bar{\varepsilon}_{jk} (\Omega_{q,ai}^* D_{\bar{\mu}} \Omega_q^{bk}) H^i (\bar{u}_{bs} D^{\bar{\mu}} q_r^{aj}) \\
& - \frac{1}{2} g_L \bar{\mathcal{C}}_{uW}^{rs} (D_{\bar{\mu}} \Omega_{q,a}^* D_{\bar{\mu}} \Omega_q^b) (\bar{u}_{bs} \tilde{H}^\dagger q_r^a) - \frac{1}{2} g_L \bar{\mathcal{C}}_{uW}^{rs} (\Omega_{q,a}^* D_{\bar{\mu}} \Omega_q^b) (\bar{u}_{bs} D_{\bar{\mu}} \tilde{H}^\dagger q_r^a) \\
& - \frac{i}{2} [\bar{y}_u^{ts} \mathcal{C}_{uW}^{tr} + y_u^{tr} \bar{\mathcal{C}}_{uW}^{ts}] \left[ 2t_j^{Ii} (\Omega_{q,ai}^* D_{\bar{\rho}} \Omega_q^{bj}) \widetilde{W}^{\bar{\rho}\bar{\sigma}I} (\bar{u}_{bs} \gamma^{\bar{\sigma}} u_r^a) - 2t_j^{Ii} (D_{\bar{\mu}} \Omega_{q,ai}^* \Omega_q^{bj}) \widetilde{W}^{\bar{\mu}\bar{\sigma}I} (\bar{u}_{bs} \gamma^{\bar{\sigma}} u_r^a) \right] \\
& + [\bar{y}_u^{tr} \bar{\mathcal{C}}_{uW}^{ts} - \bar{y}_u^{ts} \mathcal{C}_{uW}^{tr}] \left[ t_j^{Ii} (\Omega_{q,ai}^* D_{\bar{\nu}} \Omega_q^{bj}) W^{\bar{\mu}\bar{\nu}I} (\bar{u}_{bs} \gamma^{\bar{\mu}} u_r^a) + t_j^{Ii} (D_{\bar{\mu}} \Omega_{q,ai}^* \Omega_q^{bj}) W^{\bar{\mu}\bar{\nu}I} (\bar{u}_{bs} \gamma^{\bar{\nu}} u_r^a) \right] \\
& - \frac{4i}{3} [\bar{y}_u^{rs} \mathcal{C}_{uW}^{rs} + y_u^{rs} \bar{\mathcal{C}}_{uW}^{rs}] \left[ t_k^{Ij} (\Omega_{q,j}^* D_{\bar{\nu}} \Omega_q^i) H_i^\dagger D^{\bar{\mu}} H^k W^{\bar{\mu}\bar{\nu}I} - t_k^{Ii} (D_{\bar{\nu}} \Omega_{q,j}^* \Omega_q^k) D^{\bar{\mu}} H_i^\dagger H^j W^{\bar{\mu}\bar{\nu}I} \right] \\
& - \frac{4i}{3} [\bar{y}_u^{rs} \mathcal{C}_{uW}^{rs} - y_u^{rs} \bar{\mathcal{C}}_{uW}^{rs}] \left[ t_k^{Ii} (D_{\bar{\nu}} \Omega_{q,j}^* \Omega_q^k) D^{\bar{\mu}} H_i^\dagger H^j W^{\bar{\mu}\bar{\nu}I} + t_k^{Ij} (\Omega_{q,j}^* D_{\bar{\nu}} \Omega_q^i) H_i^\dagger D^{\bar{\mu}} H^k W^{\bar{\mu}\bar{\nu}I} \right] \\
& - \frac{4i}{3} [\bar{y}_u^{rs} \mathcal{C}_{uW}^{rs} - y_u^{rs} \bar{\mathcal{C}}_{uW}^{rs}] \left[ t_k^{Ij} (\Omega_{q,j}^* D_{\bar{\nu}} \Omega_q^k) W^{\bar{\mu}\bar{\nu}I} (D_{\bar{\mu}} H^\dagger H) - t_k^{Ij} (D_{\bar{\mu}} \Omega_{q,j}^* \Omega_q^k) W^{\bar{\mu}\bar{\nu}I} (H^\dagger D_{\bar{\nu}} H) \right] \\
& + \frac{4i}{3} [\bar{y}_u^{rs} \mathcal{C}_{uW}^{rs} + y_u^{rs} \bar{\mathcal{C}}_{uW}^{rs}] \left[ t_k^{Ij} (D_{\bar{\mu}} \Omega_{q,j}^* \Omega_q^k) W^{\bar{\mu}\bar{\nu}I} (H^\dagger D_{\bar{\nu}} H) + t_k^{Ij} (\Omega_{q,j}^* D_{\bar{\nu}} \Omega_q^k) W^{\bar{\mu}\bar{\nu}I} (D_{\bar{\mu}} H^\dagger H) \right] \\
& - \frac{4i}{3} [\bar{y}_u^{rs} \mathcal{C}_{uW}^{rs} + y_u^{rs} \bar{\mathcal{C}}_{uW}^{rs}] \left[ (\Omega_u^\dagger D_{\bar{\nu}} \Omega_u) W^{\bar{\mu}\bar{\nu}I} (H^\dagger t^I D_{\bar{\mu}} H) - (D_{\bar{\nu}} \Omega_u^\dagger \Omega_u) W^{\bar{\mu}\bar{\nu}I} (D_{\bar{\mu}} H^\dagger t^I H) \right] \\
& - \frac{4i}{3} [\bar{y}_u^{rs} \mathcal{C}_{uW}^{rs} - y_u^{rs} \bar{\mathcal{C}}_{uW}^{rs}] \left[ (\Omega_u^\dagger D_{\bar{\nu}} \Omega_u) W^{\bar{\mu}\bar{\nu}I} (H^\dagger t^I D_{\bar{\mu}} H) + (D_{\bar{\nu}} \Omega_u^\dagger \Omega_u) W^{\bar{\mu}\bar{\nu}I} (D_{\bar{\mu}} H^\dagger t^I H) \right], \tag{3.24}
\end{aligned}$$

$$\begin{aligned}
\Gamma_\Omega^{(1)} [\mathcal{O}_{uG}] &= \frac{1}{18} g_s \mathcal{C}_{uG}^{rs} (D_{\bar{\mu}} \Omega_{q,a}^* \Omega_q^b) (\bar{q}_{br} \tilde{H} D_{\bar{\mu}} u_s^a) + \frac{1}{18} g_s \mathcal{C}_{uG}^{rs} (D_{\bar{\mu}} \Omega_{u,a}^* \Omega_u^b) (D^{\bar{\mu}} \bar{q}_{br} \tilde{H} u_s^a) \\
& + \frac{1}{18} g_s \mathcal{C}_{uG}^{rs} \varepsilon^{kj} (D_{\bar{\mu}} \Omega_{q,a,j}^* \Omega_q^{bi}) H_i^\dagger (\bar{q}_{bkr} D^{\bar{\mu}} u_s^a) + \frac{1}{18} g_s \bar{\mathcal{C}}_{uG}^{rs} (\Omega_{u,a}^* D_{\bar{\mu}} \Omega_u^b) (\bar{u}_{bs} \tilde{H}^\dagger D^{\bar{\mu}} q_r^a) \\
& + \frac{1}{18} g_s \bar{\mathcal{C}}_{uG}^{rs} \bar{\varepsilon}_{jk} (\Omega_{q,ai}^* D_{\bar{\mu}} \Omega_q^{bk}) H^i (D^{\bar{\mu}} \bar{u}_{bs} q_r^{aj}) + \frac{1}{18} g_s \bar{\mathcal{C}}_{uG}^{rs} (\Omega_{q,a}^* D_{\bar{\mu}} \Omega_q^b) (D^{\bar{\mu}} \bar{u}_{bs} \tilde{H}^\dagger q_r^a) \\
& - \frac{i}{12} g_s [\bar{y}_u^{rt} \mathcal{C}_{uG}^{st} + y_u^{st} \bar{\mathcal{C}}_{uG}^{rt}] \left[ (\Omega_{q,aj}^* D_{\bar{\mu}} \Omega_q^{bi}) H_i^\dagger (\bar{q}_{bs} H \gamma^{\bar{\mu}} q_r^{aj}) - (D_{\bar{\mu}} \Omega_{q,aj}^* \Omega_q^{bk}) H^j (\bar{q}_{bks} \gamma^{\bar{\mu}} H^\dagger q_r^a) \right] \\
& + \frac{i}{12} g_s [\bar{y}_u^{rt} \mathcal{C}_{uG}^{st} - y_u^{st} \bar{\mathcal{C}}_{uG}^{rt}] \left[ (\Omega_{q,aj}^* D_{\bar{\mu}} \Omega_q^{bi}) H_i^\dagger (\bar{q}_{bs} H \gamma^{\bar{\mu}} q_r^{aj}) + (D_{\bar{\mu}} \Omega_{q,aj}^* \Omega_q^{bk}) H^j (\bar{q}_{bks} \gamma^{\bar{\mu}} H^\dagger q_r^a) \right] \\
& - \frac{i}{12} g_s [\bar{y}_u^{rt} \mathcal{C}_{uG}^{st} + y_u^{st} \bar{\mathcal{C}}_{uG}^{rt}] \left[ (\Omega_{q,a}^* \overleftrightarrow{D}_{\bar{\mu}} \Omega_q^b) (H^\dagger H) (\bar{q}_{bs} \gamma^{\bar{\mu}} q_r^a) \right]
\end{aligned}$$

$$\begin{aligned}
& + \frac{i}{12} g_s \left[ \bar{y}_u^{rt} \mathcal{C}_{uG}^{st} + y_u^{st} \bar{\mathcal{C}}_{uG}^{rt} \right] (\Omega_{q,a}^* \overleftrightarrow{D}_{\bar{\mu}} \Omega_q^b) (\bar{q}_{bs} H \gamma^{\bar{\mu}} H^\dagger q_r^a) \\
& + \frac{i}{12} g_s \left[ \bar{y}_u^{rt} \mathcal{C}_{uG}^{st} + y_u^{st} \bar{\mathcal{C}}_{uG}^{rt} \right] (\Omega_{q,aj}^* \overleftrightarrow{D}_{\bar{\mu}} \Omega_q^{bi}) H_i^\dagger H^j (\bar{q}_{bs} \gamma^{\bar{\mu}} q_r^a) \\
& - \frac{i}{12} g_s \left[ \bar{y}_u^{tr} \mathcal{C}_{uG}^{tr} + y_u^{tr} \bar{\mathcal{C}}_{uG}^{ts} \right] (\Omega_{u,a}^* \overleftrightarrow{D}_{\bar{\mu}} \Omega_u^b) (H^\dagger H) (\bar{u}_{bs} \gamma^{\bar{\mu}} u_r^a) - \frac{i}{9} g_s \mathcal{C}_{uG}^{rs} (D_{\bar{\nu}} \Omega_{q,a}^* \Omega_q^b) (\bar{q}_{br} D_{\bar{\mu}} \tilde{H} \sigma^{\bar{\mu}\bar{\nu}} u_s^a) \\
& + \frac{i}{9} g_s \mathcal{C}_{uG}^{rs} (D_{\bar{\nu}} \Omega_{u,a}^* \Omega_u^b) (\bar{q}_{br} D_{\bar{\mu}} \tilde{H} \sigma^{\bar{\mu}\bar{\nu}} u_s^a) - \frac{i}{9} g_s \mathcal{C}_{uG}^{rs} \varepsilon^{kj} (D_{\bar{\nu}} \Omega_{q,aj}^* \Omega_q^{bi}) D_{\bar{\mu}} H_i^\dagger (\bar{q}_{bkr} \sigma^{\bar{\mu}\bar{\nu}} u_s^a) \\
& + \frac{i}{9} g_s \bar{\mathcal{C}}_{uG}^{rs} \bar{\varepsilon}_{jk} (\Omega_{q,ai}^* D_{\bar{\nu}} \Omega_q^{bk}) D_{\bar{\mu}} H^i (\bar{u}_{bs} \sigma^{\bar{\mu}\bar{\nu}} q_r^{aj}) + \frac{i}{9} g_s \bar{\mathcal{C}}_{uG}^{rs} (\Omega_{q,a}^* D_{\bar{\nu}} \Omega_q^b) (\bar{u}_{bs} \sigma^{\bar{\mu}\bar{\nu}} D_{\bar{\mu}} \tilde{H}^\dagger q_r^a) \\
& - \frac{i}{9} g_s \bar{\mathcal{C}}_{uG}^{rs} (\Omega_{u,a}^* D_{\bar{\nu}} \Omega_u^b) (\bar{u}_{bs} \sigma^{\bar{\mu}\bar{\nu}} D_{\bar{\mu}} \tilde{H}^\dagger q_r^a) \\
& + \frac{1}{6} \left[ -\bar{y}_u^{rs} \mathcal{C}_{uG}^{rs} - y_u^{rs} \bar{\mathcal{C}}_{uG}^{rs} \right] \left[ 2T_c^{Ab} (D_{\bar{\mu}} \Omega_{q,aj}^* \Omega_q^{ci}) (\Omega_{u,b}^* D_{\bar{\sigma}} \Omega_u^a) H_i^\dagger H^j \tilde{G}^{\bar{\mu}\bar{\sigma}A} - 2T_c^{Aa} (\Omega_{q,aj}^* D_{\bar{\sigma}} \Omega_q^{bi}) (D_{\bar{\mu}} \Omega_{u,b}^* \Omega_u^c) H_i^\dagger H^j \tilde{G}^{\bar{\mu}\bar{\sigma}A} \right] \\
& + \frac{1}{6} \left[ \bar{y}_u^{rs} \mathcal{C}_{uG}^{rs} - y_u^{rs} \bar{\mathcal{C}}_{uG}^{rs} \right] \left[ 2T_c^{Aa} (\Omega_{q,aj}^* D_{\bar{\sigma}} \Omega_q^{bi}) (D_{\bar{\mu}} \Omega_{u,b}^* \Omega_u^c) H_i^\dagger H^j \tilde{G}^{\bar{\mu}\bar{\sigma}A} + 2T_c^{Ab} (D_{\bar{\mu}} \Omega_{q,aj}^* \Omega_q^{ci}) (\Omega_{u,b}^* D_{\bar{\sigma}} \Omega_u^a) H_i^\dagger H^j \tilde{G}^{\bar{\mu}\bar{\sigma}A} \right] \\
& + \frac{1}{6} \left[ \bar{y}_u^{rs} \mathcal{C}_{uG}^{rs} + y_u^{rs} \bar{\mathcal{C}}_{uG}^{rs} \right] \left[ 2T_c^{Ab} (D_{\bar{\mu}} \Omega_{q,a}^* \Omega_q^c) (\Omega_{u,b}^* D_{\bar{\sigma}} \Omega_u^a) \tilde{G}^{\bar{\mu}\bar{\sigma}A} (H^\dagger H) - 2T_c^{Aa} (\Omega_{q,a}^* D_{\bar{\sigma}} \Omega_q^b) (D_{\bar{\mu}} \Omega_{u,b}^* \Omega_u^c) \tilde{G}^{\bar{\mu}\bar{\sigma}A} (H^\dagger H) \right] \\
& + \frac{1}{6} \left[ y_u^{rs} \bar{\mathcal{C}}_{uG}^{rs} - \bar{y}_u^{rs} \mathcal{C}_{uG}^{rs} \right] \left[ 2T_c^{Aa} (\Omega_{q,a}^* D_{\bar{\sigma}} \Omega_q^b) (D_{\bar{\mu}} \Omega_{u,b}^* \Omega_u^c) \tilde{G}^{\bar{\mu}\bar{\sigma}A} (H^\dagger H) + 2T_c^{Ab} (D_{\bar{\mu}} \Omega_{q,a}^* \Omega_q^c) (\Omega_{u,b}^* D_{\bar{\sigma}} \Omega_u^a) \tilde{G}^{\bar{\mu}\bar{\sigma}A} (H^\dagger H) \right] \\
& + \frac{1}{6} g_s \mathcal{C}_{uG}^{rs} (D_{\bar{\mu}} \Omega_{q,a}^* D_{\bar{\mu}} \Omega_q^b) (\bar{q}_{br} \tilde{H} u_s^a) + \frac{1}{6} g_s \mathcal{C}_{uG}^{rs} (D_{\bar{\mu}} \Omega_{q,a}^* \Omega_q^b) (\bar{q}_{br} D_{\bar{\mu}} \tilde{H} u_s^a) + \frac{1}{6} g_s \mathcal{C}_{uG}^{rs} (D_{\bar{\mu}} \Omega_{u,a}^* \Omega_u^b) (\bar{q}_{br} D_{\bar{\mu}} \tilde{H} u_s^a) \\
& + \frac{1}{6} g_s \mathcal{C}_{uG}^{rs} \varepsilon^{kj} (D_{\bar{\mu}} \Omega_{q,aj}^* \Omega_q^{bi}) D_{\bar{\mu}} H_i^\dagger (\bar{q}_{bkr} u_s^a) + \frac{1}{6} g_s \mathcal{C}_{uG}^{rs} \varepsilon^{kj} (D_{\bar{\mu}} \Omega_{q,aj}^* D_{\bar{\mu}} \Omega_q^{bi}) H_i^\dagger (\bar{q}_{bkr} u_s^a) \\
& + \frac{1}{6} g_s \bar{\mathcal{C}}_{uG}^{rs} \bar{\varepsilon}_{jk} (D_{\bar{\mu}} \Omega_{q,ai}^* D_{\bar{\mu}} \Omega_q^{bk}) H^i (\bar{u}_{bs} q_r^{aj}) + \frac{1}{6} g_s \bar{\mathcal{C}}_{uG}^{rs} \bar{\varepsilon}_{jk} (\Omega_{q,ai}^* D_{\bar{\mu}} \Omega_q^{bk}) D_{\bar{\mu}} H^i (\bar{u}_{bs} q_r^{aj}) \\
& + \frac{1}{6} g_s \bar{\mathcal{C}}_{uG}^{rs} (D_{\bar{\mu}} \Omega_{q,a}^* D_{\bar{\mu}} \Omega_q^b) (\bar{u}_{bs} \tilde{H}^\dagger q_r^a) + \frac{1}{6} g_s \bar{\mathcal{C}}_{uG}^{rs} (\Omega_{q,a}^* D_{\bar{\mu}} \Omega_q^b) (\bar{u}_{bs} D_{\bar{\mu}} \tilde{H}^\dagger q_r^a) \\
& + \frac{1}{6} g_s \bar{\mathcal{C}}_{uG}^{rs} (\Omega_{u,a}^* D_{\bar{\mu}} \Omega_u^b) (\bar{u}_{bs} D_{\bar{\mu}} \tilde{H}^\dagger q_r^a) + \frac{1}{2} g_s \bar{\mathcal{C}}_{uG}^{rs} \bar{\varepsilon}_{jk} (\Omega_{q,i}^* D_{\bar{\mu}} \Omega_q^k) H^i (\bar{u}_s D^{\bar{\mu}} q_r^j) \\
& + \frac{1}{2} g_s \bar{\mathcal{C}}_{uG}^{rs} (D_{\bar{\mu}} \Omega_u^\dagger D_{\bar{\mu}} \Omega_u) (\bar{u}_s \tilde{H}^\dagger q_r) + \frac{1}{2} g_s \bar{\mathcal{C}}_{uG}^{rs} (\Omega_q^\dagger D_{\bar{\mu}} \Omega_q) (\bar{u}_s \tilde{H}^\dagger D^{\bar{\mu}} q_r) \\
& + \frac{1}{2} g_s \bar{\mathcal{C}}_{uG}^{rs} (\Omega_u^\dagger D_{\bar{\mu}} \Omega_u) (D^{\bar{\mu}} \bar{u}_s \tilde{H}^\dagger q_r) - \frac{1}{6} g_s \mathcal{C}_{uG}^{rs} (D_{\bar{\mu}} \Omega_{u,a}^* D_{\bar{\mu}} \Omega_u^b) (\bar{q}_{br} \tilde{H} u_s^a) - \frac{1}{6} g_s \mathcal{C}_{uG}^{rs} (D_{\bar{\mu}} \Omega_{u,a}^* \Omega_u^b) (\bar{q}_{br} \tilde{H} D^{\bar{\mu}} u_s^a) \\
& - \frac{1}{6} g_s \mathcal{C}_{uG}^{rs} (D_{\bar{\mu}} \Omega_{q,a}^* \Omega_q^b) (D^{\bar{\mu}} \bar{q}_{br} \tilde{H} u_s^a) - \frac{1}{6} g_s \mathcal{C}_{uG}^{rs} \varepsilon^{kj} (D_{\bar{\mu}} \Omega_{q,j}^* \Omega_q^i) H_i^\dagger (\bar{q}_{kr} D^{\bar{\mu}} u_s) \\
& - \frac{1}{6} g_s \mathcal{C}_{uG}^{rs} \varepsilon^{kj} (D_{\bar{\mu}} \Omega_{q,aj}^* \Omega_q^{bi}) H_i^\dagger (D^{\bar{\mu}} \bar{q}_{bkr} u_s^a) - \frac{1}{6} g_s \bar{\mathcal{C}}_{uG}^{rs} (\Omega_u^\dagger D_{\bar{\mu}} \Omega_u) (\bar{u}_s \tilde{H}^\dagger D^{\bar{\mu}} q_r) \\
& - \frac{1}{6} g_s \bar{\mathcal{C}}_{uG}^{rs} \bar{\varepsilon}_{jk} (\Omega_{q,i}^* D_{\bar{\mu}} \Omega_q^k) H^i (D^{\bar{\mu}} \bar{u}_s q_r^j) - \frac{1}{6} g_s \bar{\mathcal{C}}_{uG}^{rs} (\Omega_q^\dagger D_{\bar{\mu}} \Omega_q) (D^{\bar{\mu}} \bar{u}_s \tilde{H}^\dagger q_r) \\
& - \frac{1}{6} g_s \bar{\mathcal{C}}_{uG}^{rs} \bar{\varepsilon}_{jk} (\Omega_{q,ai}^* D_{\bar{\mu}} \Omega_q^{bk}) H^i (\bar{u}_{bs} D^{\bar{\mu}} q_r^{aj}) - \frac{1}{6} g_s \bar{\mathcal{C}}_{uG}^{rs} (D_{\bar{\mu}} \Omega_{u,a}^* D_{\bar{\mu}} \Omega_u^b) (\bar{u}_{bs} \tilde{H}^\dagger q_r^a) \\
& - \frac{1}{6} g_s \bar{\mathcal{C}}_{uG}^{rs} (\Omega_{q,a}^* D_{\bar{\mu}} \Omega_q^b) (\bar{u}_{bs} \tilde{H}^\dagger D^{\bar{\mu}} q_r^a) \\
& + \frac{i}{4} g_s \left[ \bar{y}_u^{rt} \mathcal{C}_{uG}^{st} + y_u^{st} \bar{\mathcal{C}}_{uG}^{rt} \right] \left[ (\Omega_{q,j}^* D_{\bar{\mu}} \Omega_q^i) H_i^\dagger (\bar{q}_s H \gamma^{\bar{\mu}} q_r^j) - (D_{\bar{\mu}} \Omega_{q,j}^* \Omega_q^k) H^j (\bar{q}_{ks} \gamma^{\bar{\mu}} H^\dagger q_r) \right]
\end{aligned}$$

$$\begin{aligned}
& -\frac{i}{4}g_s\left[\bar{y}_u^{rt}C_{uG}^{st}-y_u^{st}\bar{C}_{uG}^{rt}\right]\left[(\Omega_{q,j}^*D_{\bar{\mu}}\Omega_q^i)H_i^\dagger(\bar{q}_sH\gamma^{\bar{\mu}}q_r^j)+(D_{\bar{\mu}}\Omega_{q,j}^*\Omega_q^k)H^j(\bar{q}_{ks}\gamma^{\bar{\mu}}H^\dagger q_r)\right] \\
& +\frac{i}{4}\left[\bar{y}_u^{rt}C_{uG}^{st}+y_u^{st}\bar{C}_{uG}^{rt}\right]\left[2T_b^{Aa}(\Omega_{u,a}^*D_{\bar{\rho}}\Omega_u^c)\tilde{G}^{\bar{\rho}\bar{\sigma}A}(\bar{q}_{cs}\gamma^{\bar{\sigma}}q_r^b)-2T_c^{Ab}(D_{\bar{\mu}}\Omega_{u,a}^*\Omega_u^c)\tilde{G}^{\bar{\mu}\bar{\sigma}A}(\bar{q}_{bs}\gamma^{\bar{\sigma}}q_r^a)\right] \\
& -\frac{i}{4}\left[\bar{y}_u^{rt}C_{uG}^{st}-y_u^{st}\bar{C}_{uG}^{rt}\right]\left[2T_c^{Ab}(D_{\bar{\mu}}\Omega_{u,a}^*\Omega_u^c)\tilde{G}^{\bar{\mu}\bar{\sigma}A}(\bar{q}_{bs}\gamma^{\bar{\sigma}}q_r^a)+2T_b^{Aa}(\Omega_{u,a}^*D_{\bar{\rho}}\Omega_u^c)\tilde{G}^{\bar{\rho}\bar{\sigma}A}(\bar{q}_{cs}\gamma^{\bar{\sigma}}q_r^b)\right] \\
& -\frac{i}{4}g_s\left[\bar{y}_u^{rt}C_{uG}^{st}+y_u^{st}\bar{C}_{uG}^{rt}\right](\Omega_q^\dagger\overset{\leftrightarrow}{D}_{\bar{\mu}}\Omega_q)(\bar{q}_sH\gamma^{\bar{\mu}}H^\dagger q_r) \\
& -\frac{i}{4}g_s\left[\bar{y}_u^{rt}C_{uG}^{st}+y_u^{st}\bar{C}_{uG}^{rt}\right](\Omega_{q,j}^*\overset{\leftrightarrow}{D}_{\bar{\mu}}\Omega_q^i)H_i^\dagger H^j(\bar{q}_s\gamma^{\bar{\mu}}q_r) \\
& +\frac{i}{4}g_s\left[\bar{y}_u^{ts}C_{uG}^{tr}+y_u^{tr}\bar{C}_{uG}^{ts}\right](\Omega_u^\dagger\overset{\leftrightarrow}{D}_{\bar{\mu}}\Omega_u)(H^\dagger H)(\bar{u}_s\gamma^{\bar{\mu}}u_r) \\
& +\frac{i}{3}\left[\bar{y}_u^{rs}C_{uG}^{rs}-y_u^{rs}\bar{C}_{uG}^{rs}\right]\left[T_c^{Ab}(D_{\bar{\mu}}\Omega_{q,aj}^*\Omega_q^{ci})(\Omega_{u,b}^*D_{\bar{\nu}}\Omega_u^a)H_i^\dagger H^jG^{\bar{\mu}\bar{\nu}A}-T_c^{Aa}(\Omega_{q,aj}^*D_{\bar{\nu}}\Omega_q^{bi})(D_{\bar{\mu}}\Omega_{u,b}^*\Omega_u^c)H_i^\dagger H^jG^{\bar{\mu}\bar{\nu}A}\right] \\
& -\frac{i}{3}\left[\bar{y}_u^{rs}C_{uG}^{rs}+y_u^{rs}\bar{C}_{uG}^{rs}\right]\left[T_c^{Aa}(\Omega_{q,aj}^*D_{\bar{\nu}}\Omega_q^{bi})(D_{\bar{\mu}}\Omega_{u,b}^*\Omega_u^c)H_i^\dagger H^jG^{\bar{\mu}\bar{\nu}A}+T_c^{Ab}(D_{\bar{\mu}}\Omega_{q,aj}^*\Omega_q^{ci})(\Omega_{u,b}^*D_{\bar{\nu}}\Omega_u^a)H_i^\dagger H^jG^{\bar{\mu}\bar{\nu}A}\right] \\
& +\frac{1}{3}\left[\bar{y}_u^{rs}C_{uG}^{rs}-y_u^{rs}\bar{C}_{uG}^{rs}\right]\left[2T_b^{Aa}(\Omega_{q,aj}^*D_{\bar{\sigma}}\Omega_q^{bi})H_i^\dagger D^{\bar{\mu}}H^j\tilde{G}^{\bar{\mu}\bar{\sigma}A}-2T_b^{Aa}(D_{\bar{\nu}}\Omega_{q,aj}^*\Omega_q^{bi})D^{\bar{\mu}}H_i^\dagger H^j\tilde{G}^{\bar{\mu}\bar{\nu}A}\right] \\
& +\frac{1}{3}\left[\bar{y}_u^{rs}C_{uG}^{rs}+y_u^{rs}\bar{C}_{uG}^{rs}\right]\left[2T_b^{Aa}(D_{\bar{\nu}}\Omega_{q,aj}^*\Omega_q^{bi})D^{\bar{\mu}}H_i^\dagger H^j\tilde{G}^{\bar{\mu}\bar{\nu}A}+2T_b^{Aa}(\Omega_{q,aj}^*D_{\bar{\sigma}}\Omega_q^{bi})H_i^\dagger D^{\bar{\mu}}H^j\tilde{G}^{\bar{\mu}\bar{\sigma}A}\right] \\
& -\frac{i}{3}\left[\bar{y}_u^{rs}C_{uG}^{rs}-y_u^{rs}\bar{C}_{uG}^{rs}\right]\left[T_c^{Ab}(D_{\bar{\mu}}\Omega_{q,a}^*\Omega_q^c)(\Omega_{u,b}^*D_{\bar{\nu}}\Omega_u^a)G^{\bar{\mu}\bar{\nu}A}(H^\dagger H)-T_c^{Aa}(\Omega_{q,a}^*D_{\bar{\nu}}\Omega_q^b)(D_{\bar{\mu}}\Omega_{u,b}^*\Omega_u^c)G^{\bar{\mu}\bar{\nu}A}(H^\dagger H)\right] \\
& +\frac{i}{3}\left[\bar{y}_u^{rs}C_{uG}^{rs}+y_u^{rs}\bar{C}_{uG}^{rs}\right]\left[T_c^{Aa}(\Omega_{q,a}^*D_{\bar{\nu}}\Omega_q^b)(D_{\bar{\mu}}\Omega_{u,b}^*\Omega_u^c)G^{\bar{\mu}\bar{\nu}A}(H^\dagger H)+T_c^{Ab}(D_{\bar{\mu}}\Omega_{q,a}^*\Omega_q^c)(\Omega_{u,b}^*D_{\bar{\nu}}\Omega_u^a)G^{\bar{\mu}\bar{\nu}A}(H^\dagger H)\right] \\
& +\frac{1}{3}\left[\bar{y}_u^{rs}\bar{C}_{uG}^{rs}-\bar{y}_u^{rs}C_{uG}^{rs}\right]\left[2T_b^{Aa}(\Omega_{q,a}^*D_{\bar{\sigma}}\Omega_q^b)\tilde{G}^{\bar{\mu}\bar{\sigma}A}(H^\dagger D_{\bar{\mu}}H)-2T_b^{Aa}(D_{\bar{\nu}}\Omega_{q,a}^*\Omega_q^b)\tilde{G}^{\bar{\mu}\bar{\nu}A}(D_{\bar{\mu}}H^\dagger H)\right] \\
& +\frac{1}{3}\left[-\bar{y}_u^{rs}C_{uG}^{rs}-y_u^{rs}\bar{C}_{uG}^{rs}\right]\left[2T_b^{Aa}(\Omega_{q,a}^*D_{\bar{\sigma}}\Omega_q^b)\tilde{G}^{\bar{\mu}\bar{\sigma}A}(H^\dagger D_{\bar{\mu}}H)+2T_b^{Aa}(D_{\bar{\nu}}\Omega_{q,a}^*\Omega_q^b)\tilde{G}^{\bar{\mu}\bar{\nu}A}(D_{\bar{\mu}}H^\dagger H)\right] \\
& +\frac{1}{3}\left[\bar{y}_u^{rs}\bar{C}_{uG}^{rs}-\bar{y}_u^{rs}C_{uG}^{rs}\right]\left[2T_b^{Aa}(\Omega_{u,a}^*D_{\bar{\sigma}}\Omega_u^b)\tilde{G}^{\bar{\mu}\bar{\sigma}A}(H^\dagger D_{\bar{\mu}}H)-2T_b^{Aa}(D_{\bar{\nu}}\Omega_{u,a}^*\Omega_u^b)\tilde{G}^{\bar{\mu}\bar{\nu}A}(D_{\bar{\mu}}H^\dagger H)\right] \\
& +\frac{1}{3}\left[-\bar{y}_u^{rs}C_{uG}^{rs}-y_u^{rs}\bar{C}_{uG}^{rs}\right]\left[2T_b^{Aa}(\Omega_{u,a}^*D_{\bar{\sigma}}\Omega_u^b)\tilde{G}^{\bar{\mu}\bar{\sigma}A}(H^\dagger D_{\bar{\mu}}H)+2T_b^{Aa}(D_{\bar{\nu}}\Omega_{u,a}^*\Omega_u^b)\tilde{G}^{\bar{\mu}\bar{\nu}A}(D_{\bar{\mu}}H^\dagger H)\right] \\
& +\frac{i}{3}g_sC_{uG}^{rs}(D_{\bar{\nu}}\Omega_q^\dagger\Omega_q)(\bar{q}_rD_{\bar{\mu}}\tilde{H}\sigma^{\bar{\mu}\bar{\nu}}u_s)-\frac{i}{3}g_sC_{uG}^{rs}(D_{\bar{\nu}}\Omega_u^\dagger\Omega_u)(\bar{q}_rD_{\bar{\mu}}\tilde{H}\sigma^{\bar{\mu}\bar{\nu}}u_s) \\
& +\frac{i}{3}g_sC_{uG}^{rs}\varepsilon^{kj}(D_{\bar{\nu}}\Omega_{q,j}^*\Omega_q^i)D^{\bar{\mu}}H_i^\dagger(\bar{q}_{kr}\sigma^{\bar{\mu}\bar{\nu}}u_s)-\frac{i}{3}g_s\bar{C}_{uG}^{rs}\varepsilon_{jk}(\Omega_{q,i}^*D_{\bar{\nu}}\Omega_q^k)D^{\bar{\mu}}H^i(\bar{u}_s\sigma^{\bar{\mu}\bar{\nu}}q_r^j) \\
& -\frac{i}{3}g_s\bar{C}_{uG}^{rs}(\Omega_q^\dagger D_{\bar{\nu}}\Omega_q)(\bar{u}_s\sigma^{\bar{\mu}\bar{\nu}}D_{\bar{\mu}}\tilde{H}^\dagger q_r)+\frac{i}{3}g_s\bar{C}_{uG}^{rs}(\Omega_u^\dagger D_{\bar{\nu}}\Omega_u)(\bar{u}_s\sigma^{\bar{\mu}\bar{\nu}}D_{\bar{\mu}}\tilde{H}^\dagger q_r) \\
& +\frac{1}{2}g_sC_{uG}^{rs}(D_{\bar{\mu}}\Omega_u^\dagger D_{\bar{\mu}}\Omega_u)(\bar{q}_r\tilde{H}u_s)+\frac{1}{2}g_sC_{uG}^{rs}(D_{\bar{\mu}}\Omega_u^\dagger\Omega_u)(\bar{q}_r\tilde{H}D^{\bar{\mu}}u_s)+\frac{1}{2}g_sC_{uG}^{rs}(D_{\bar{\mu}}\Omega_q^\dagger\Omega_q)(D^{\bar{\mu}}\bar{q}_r\tilde{H}u_s) \\
& +\frac{1}{2}g_sC_{uG}^{rs}\varepsilon^{kj}(D_{\bar{\mu}}\Omega_{q,j}^*\Omega_q^i)H_i^\dagger(D^{\bar{\mu}}\bar{q}_{kr}u_s) \\
& +\frac{1}{2}\left[-\bar{y}_u^{rt}C_{uG}^{st}-y_u^{st}\bar{C}_{uG}^{rt}\right]\left[T_b^{Aa}(\Omega_{u,a}^*D_{\bar{\nu}}\Omega_u^c)G^{\bar{\mu}\bar{\nu}A}(\bar{q}_{cs}\gamma^{\bar{\mu}}q_r^b)-T_c^{Ab}(D_{\bar{\mu}}\Omega_{u,a}^*\Omega_u^c)G^{\bar{\mu}\bar{\nu}A}(\bar{q}_{bs}\gamma^{\bar{\nu}}q_r^a)\right] \\
& +\frac{1}{2}\left[\bar{y}_u^{rt}C_{uG}^{st}-y_u^{st}\bar{C}_{uG}^{rt}\right]\left[T_c^{Ab}(D_{\bar{\mu}}\Omega_{u,a}^*\Omega_u^c)G^{\bar{\mu}\bar{\nu}A}(\bar{q}_{bs}\gamma^{\bar{\nu}}q_r^a)+T_b^{Aa}(\Omega_{u,a}^*D_{\bar{\nu}}\Omega_u^c)G^{\bar{\mu}\bar{\nu}A}(\bar{q}_{cs}\gamma^{\bar{\mu}}q_r^b)\right]
\end{aligned}$$

$$\begin{aligned}
& + \frac{1}{2} \left[ -\bar{y}_u^{ts} \mathcal{C}_{uG}^{tr} - y_u^{tr} \bar{\mathcal{C}}_{uG}^{ts} \right] \left[ T_b^{Aa} (\Omega_{q,a}^* D_{\bar{\nu}} \Omega_q^c) G^{\bar{\mu}\bar{\nu}A} (\bar{u}_{cs} \gamma^{\bar{\mu}} u_r^b) - T_c^{Ab} (D_{\bar{\mu}} \Omega_{q,a}^* \Omega_q^c) G^{\bar{\mu}\bar{\nu}A} (\bar{u}_{bs} \gamma^{\bar{\nu}} u_r^a) \right] \\
& + \frac{1}{2} \left[ y_u^{tr} \bar{\mathcal{C}}_{uG}^{ts} - \bar{y}_u^{ts} \mathcal{C}_{uG}^{tr} \right] \left[ T_c^{Ab} (D_{\bar{\mu}} \Omega_{q,a}^* \Omega_q^c) G^{\bar{\mu}\bar{\nu}A} (\bar{u}_{bs} \gamma^{\bar{\nu}} u_r^a) + T_b^{Aa} (\Omega_{q,a}^* D_{\bar{\nu}} \Omega_q^c) G^{\bar{\mu}\bar{\nu}A} (\bar{u}_{cs} \gamma^{\bar{\mu}} u_r^b) \right] \\
& - \frac{1}{6} g_s \mathcal{C}_{uG}^{rs} (D_{\bar{\mu}} \Omega_q^\dagger \Omega_q) (\bar{q}_r \tilde{H} D_{\bar{\mu}} u_s) - \frac{1}{6} g_s \mathcal{C}_{uG}^{rs} (D_{\bar{\mu}} \Omega_u^\dagger \Omega_u) (D_{\bar{\mu}} \bar{q}_r \tilde{H} u_s) - \frac{1}{6} g_s \bar{\mathcal{C}}_{uG}^{rs} (\Omega_{u,a}^* D_{\bar{\mu}} \Omega_u^b) (D_{\bar{\mu}} \bar{u}_{bs} \tilde{H}^\dagger q_r^a) \\
& - \frac{i}{4} \left[ \bar{y}_u^{ts} \mathcal{C}_{uG}^{tr} + y_u^{tr} \bar{\mathcal{C}}_{uG}^{ts} \right] \left[ 2T_b^{Aa} (\Omega_{q,a}^* D_{\bar{\rho}} \Omega_q^c) \tilde{G}^{\bar{\rho}\bar{\sigma}A} (\bar{u}_{cs} \gamma^{\bar{\sigma}} u_r^b) - 2T_c^{Ab} (D_{\bar{\mu}} \Omega_{q,a}^* \Omega_q^c) \tilde{G}^{\bar{\mu}\bar{\sigma}A} (\bar{u}_{bs} \gamma^{\bar{\sigma}} u_r^a) \right] \\
& - \frac{i}{4} \left[ \bar{y}_u^{ts} \mathcal{C}_{uG}^{tr} - y_u^{tr} \bar{\mathcal{C}}_{uG}^{ts} \right] \left[ 2T_c^{Ab} (D_{\bar{\mu}} \Omega_{q,a}^* \Omega_q^c) \tilde{G}^{\bar{\mu}\bar{\sigma}A} (\bar{u}_{bs} \gamma^{\bar{\sigma}} u_r^a) + 2T_b^{Aa} (\Omega_{q,a}^* D_{\bar{\rho}} \Omega_q^c) \tilde{G}^{\bar{\rho}\bar{\sigma}A} (\bar{u}_{cs} \gamma^{\bar{\sigma}} u_r^b) \right] \\
& + \frac{i}{4} g_s \left[ \bar{y}_u^{rt} \mathcal{C}_{uG}^{st} + y_u^{st} \bar{\mathcal{C}}_{uG}^{rt} \right] (\Omega_q^\dagger D_{\bar{\mu}} \Omega_q) (H^\dagger H) (\bar{q}_s \gamma^{\bar{\mu}} q_r) - \frac{1}{2} g_s \mathcal{C}_{uG}^{rs} (D_{\bar{\mu}} \Omega_q^\dagger D_{\bar{\mu}} \Omega_q) (\bar{q}_r \tilde{H} u_s) \\
& - \frac{1}{2} g_s \mathcal{C}_{uG}^{rs} (D_{\bar{\mu}} \Omega_q^\dagger \Omega_q) (\bar{q}_r D_{\bar{\mu}} \tilde{H} u_s) - \frac{1}{2} g_s \mathcal{C}_{uG}^{rs} (D_{\bar{\mu}} \Omega_u^\dagger \Omega_u) (\bar{q}_r D_{\bar{\mu}} \tilde{H} u_s) - \frac{1}{2} g_s \mathcal{C}_{uG}^{rs} \varepsilon^{kj} (D_{\bar{\mu}} \Omega_{q,j}^* \Omega_q^i) D_{\bar{\mu}} H_i^\dagger (\bar{q}_{kr} u_s) \\
& - \frac{1}{2} g_s \mathcal{C}_{uG}^{rs} \varepsilon^{kj} (D_{\bar{\mu}} \Omega_{q,j}^* D_{\bar{\mu}} \Omega_q^i) H_i^\dagger (\bar{q}_{kr} u_s) - \frac{1}{2} g_s \bar{\mathcal{C}}_{uG}^{rs} \bar{\varepsilon}_{jk} (D_{\bar{\mu}} \Omega_{q,i}^* D_{\bar{\mu}} \Omega_q^k) H^i (\bar{u}_s q_r^j) \\
& - \frac{1}{2} g_s \bar{\mathcal{C}}_{uG}^{rs} \bar{\varepsilon}_{jk} (\Omega_{q,i}^* D_{\bar{\mu}} \Omega_q^k) D_{\bar{\mu}} H^i (\bar{u}_s q_r^j) - \frac{1}{2} g_s \bar{\mathcal{C}}_{uG}^{rs} (D_{\bar{\mu}} \Omega_q^\dagger D_{\bar{\mu}} \Omega_q) (\bar{u}_s \tilde{H}^\dagger q_r) \\
& - \frac{1}{2} g_s \bar{\mathcal{C}}_{uG}^{rs} (\Omega_q^\dagger D_{\bar{\mu}} \Omega_q) (\bar{u}_s D_{\bar{\mu}} \tilde{H}^\dagger q_r) - \frac{1}{2} g_s \bar{\mathcal{C}}_{uG}^{rs} (\Omega_u^\dagger D_{\bar{\mu}} \Omega_u) (\bar{u}_s D_{\bar{\mu}} \tilde{H}^\dagger q_r) \\
& - \frac{2i}{3} \left[ \bar{y}_u^{rs} \mathcal{C}_{uG}^{rs} + y_u^{rs} \bar{\mathcal{C}}_{uG}^{rs} \right] \left[ T_b^{Aa} (\Omega_{q,aj}^* D_{\bar{\nu}} \Omega_q^{bi}) H_i^\dagger D_{\bar{\mu}} H^j G^{\bar{\mu}\bar{\nu}A} - T_b^{Aa} (D_{\bar{\nu}} \Omega_{q,aj}^* \Omega_q^{bi}) D_{\bar{\mu}} H_i^\dagger H^j G^{\bar{\mu}\bar{\nu}A} \right] \\
& - \frac{2i}{3} \left[ \bar{y}_u^{rs} \mathcal{C}_{uG}^{rs} - y_u^{rs} \bar{\mathcal{C}}_{uG}^{rs} \right] \left[ T_b^{Aa} (D_{\bar{\nu}} \Omega_{q,aj}^* \Omega_q^{bi}) D_{\bar{\mu}} H_i^\dagger H^j G^{\bar{\mu}\bar{\nu}A} + T_b^{Aa} (\Omega_{q,aj}^* D_{\bar{\nu}} \Omega_q^{bi}) H_i^\dagger D_{\bar{\mu}} H^j G^{\bar{\mu}\bar{\nu}A} \right] \\
& + \frac{2i}{3} \left[ \bar{y}_u^{rs} \mathcal{C}_{uG}^{rs} + y_u^{rs} \bar{\mathcal{C}}_{uG}^{rs} \right] \left[ T_b^{Aa} (\Omega_{q,a}^* D_{\bar{\nu}} \Omega_q^b) G^{\bar{\mu}\bar{\nu}A} (H^\dagger D_{\bar{\mu}} H) - T_b^{Aa} (D_{\bar{\nu}} \Omega_{q,a}^* \Omega_q^b) G^{\bar{\mu}\bar{\nu}A} (D_{\bar{\mu}} H^\dagger H) \right] \\
& + \frac{2i}{3} \left[ \bar{y}_u^{rs} \mathcal{C}_{uG}^{rs} - y_u^{rs} \bar{\mathcal{C}}_{uG}^{rs} \right] \left[ T_b^{Aa} (\Omega_{q,a}^* D_{\bar{\nu}} \Omega_q^b) G^{\bar{\mu}\bar{\nu}A} (H^\dagger D_{\bar{\mu}} H) + T_b^{Aa} (D_{\bar{\nu}} \Omega_{q,a}^* \Omega_q^b) G^{\bar{\mu}\bar{\nu}A} (D_{\bar{\mu}} H^\dagger H) \right] \\
& + \frac{2i}{3} \left[ \bar{y}_u^{rs} \mathcal{C}_{uG}^{rs} + y_u^{rs} \bar{\mathcal{C}}_{uG}^{rs} \right] \left[ T_b^{Aa} (\Omega_{u,a}^* D_{\bar{\nu}} \Omega_u^b) G^{\bar{\mu}\bar{\nu}A} (H^\dagger D_{\bar{\mu}} H) - T_b^{Aa} (D_{\bar{\nu}} \Omega_{u,a}^* \Omega_u^b) G^{\bar{\mu}\bar{\nu}A} (D_{\bar{\mu}} H^\dagger H) \right] \\
& + \frac{2i}{3} \left[ \bar{y}_u^{rs} \mathcal{C}_{uG}^{rs} - y_u^{rs} \bar{\mathcal{C}}_{uG}^{rs} \right] \left[ T_b^{Aa} (\Omega_{u,a}^* D_{\bar{\nu}} \Omega_u^b) G^{\bar{\mu}\bar{\nu}A} (H^\dagger D_{\bar{\mu}} H) + T_b^{Aa} (D_{\bar{\nu}} \Omega_{u,a}^* \Omega_u^b) G^{\bar{\mu}\bar{\nu}A} (D_{\bar{\mu}} H^\dagger H) \right], \\
\end{aligned} \tag{3.25}$$

$$\begin{aligned}
\Gamma_\Omega^{(1)} [\mathcal{O}_{dB}] &= \frac{i}{12} g_Y \left[ \bar{y}_d^{rt} \mathcal{C}_{dB}^{st} + y_d^{st} \bar{\mathcal{C}}_{dB}^{rt} \right] \left[ (\Omega_{q,aj}^* D_{\bar{\mu}} \Omega_q^{bi}) H_i^\dagger (\bar{q}_{bs} H \gamma^{\bar{\mu}} q_r^{aj}) - (D_{\bar{\mu}} \Omega_{q,aj}^* \Omega_q^{bk}) H^j (\bar{q}_{bks} \gamma^{\bar{\mu}} H^\dagger q_r^a) \right] \\
& + \frac{i}{12} g_Y \left[ \bar{y}_d^{rt} \mathcal{C}_{dB}^{st} - y_d^{st} \bar{\mathcal{C}}_{dB}^{rt} \right] \left[ (\Omega_{q,aj}^* D_{\bar{\mu}} \Omega_q^{bi}) H_i^\dagger (\bar{q}_{bs} H \gamma^{\bar{\mu}} q_r^{aj}) + (D_{\bar{\mu}} \Omega_{q,aj}^* \Omega_q^{bk}) H^j (\bar{q}_{bks} \gamma^{\bar{\mu}} H^\dagger q_r^a) \right] \\
& - \frac{i}{9} g_Y \bar{\mathcal{C}}_{dB}^{rs} (D_{\bar{\nu}} \Omega_{q,aj}^* \Omega_q^{bi}) D_{\bar{\mu}} H_i^\dagger (\bar{d}_{bs} \sigma^{\bar{\mu}\bar{\nu}} q_r^{aj}) + \frac{i}{9} g_Y \mathcal{C}_{dB}^{sr} (\Omega_{q,ai}^* D_{\bar{\nu}} \Omega_q^{bj}) D_{\bar{\mu}} H^i (\bar{q}_{bjs} \sigma^{\bar{\mu}\bar{\nu}} d_r^a) \\
& + \frac{1}{6} \left[ -\bar{y}_d^{rs} \mathcal{C}_{dB}^{rs} - y_d^{rs} \bar{\mathcal{C}}_{dB}^{rs} \right] \left[ 2(\Omega_{d,a}^* D_{\bar{\sigma}} \Omega_d^b) (\Omega_{q,bj}^* D_{\bar{\rho}} \Omega_q^{ai}) H_i^\dagger H^j \tilde{B}^{\bar{\rho}\bar{\sigma}} - 2(D_{\bar{\mu}} \Omega_{d,a}^* \Omega_d^b) (D_{\bar{\nu}} \Omega_{q,bj}^* \Omega_q^{ai}) H_i^\dagger H^j \tilde{B}^{\bar{\mu}\bar{\nu}} \right] \\
& + \frac{1}{6} g_Y \bar{\mathcal{C}}_{dB}^{rs} (D_{\bar{\mu}} \Omega_{q,aj}^* D_{\bar{\mu}} \Omega_q^{bi}) H_i^\dagger (\bar{d}_{bs} q_r^{aj}) + \frac{1}{6} g_Y \bar{\mathcal{C}}_{dB}^{rs} (D_{\bar{\mu}} \Omega_{q,aj}^* \Omega_q^{bi}) H_i^\dagger (\bar{d}_{bs} D_{\bar{\mu}} q_r^{aj}) \\
& + \frac{1}{6} g_Y \mathcal{C}_{dB}^{sr} (D_{\bar{\mu}} \Omega_{q,ai}^* D_{\bar{\mu}} \Omega_q^{bj}) H^i (\bar{q}_{bjs} d_r^a) + \frac{1}{6} g_Y \mathcal{C}_{dB}^{sr} (\Omega_{q,ai}^* D_{\bar{\mu}} \Omega_q^{bj}) H^i (D_{\bar{\mu}} \bar{q}_{bjs} d_r^a) - \frac{1}{18} g_Y \mathcal{C}_{dB}^{sr} (\Omega_{q,ai}^* D_{\bar{\mu}} \Omega_q^{bj}) H^i (\bar{q}_{bjs} D_{\bar{\mu}} d_r^a)
\end{aligned}$$

$$\begin{aligned}
& -\frac{1}{9}g_Y\mathcal{C}_{dB}^{sr}(\Omega_{d,a}^*D_{\bar{\mu}}\Omega_d^b)(D^{\bar{\mu}}\bar{q}_{bs}Hd_r^a) - \frac{1}{6}g_Y\mathcal{C}_{dB}^{sr}(\Omega_{q,ai}^*D_{\bar{\mu}}\Omega_q^{bj})D^{\bar{\mu}}H^i(\bar{q}_{bj}s d_r^a) \\
& -\frac{i}{6}g_Y\left[\bar{y}_d^{ts}\mathcal{C}_{dB}^{tr} + y_d^{tr}\bar{\mathcal{C}}_{dB}^{ts}\right](\Omega_{d,a}^*\overleftrightarrow{D}_{\bar{\mu}}\Omega_d^b)(H^\dagger H)(\bar{d}_{bs}\gamma^{\bar{\mu}}d_r^a) + \frac{2i}{9}g_Y\bar{\mathcal{C}}_{dB}^{rs}(D_{\bar{\nu}}\Omega_{d,a}^*\Omega_d^b)(\bar{d}_{bs}\sigma^{\bar{\mu}\bar{\nu}}D_{\bar{\mu}}H^\dagger q_r^a) \\
& -\frac{2i}{9}g_Y\mathcal{C}_{dB}^{sr}(\Omega_{d,a}^*D_{\bar{\nu}}\Omega_d^b)(\bar{q}_{bs}D_{\bar{\mu}}H\sigma^{\bar{\mu}\bar{\nu}}d_r^a) \\
& +\frac{i}{3}\left[\bar{y}_d^{rs}\mathcal{C}_{dB}^{rs} - y_d^{rs}\bar{\mathcal{C}}_{dB}^{rs}\right]\left[(\Omega_{d,a}^*D_{\bar{\nu}}\Omega_d^b)(\Omega_{q,bj}^*D_{\bar{\mu}}\Omega_q^{ai})H_i^\dagger H^j B^{\bar{\mu}\bar{\nu}} - (D_{\bar{\mu}}\Omega_{d,a}^*\Omega_d^b)(D_{\bar{\nu}}\Omega_{q,bj}^*\Omega_q^{ai})H_i^\dagger H^j B^{\bar{\mu}\bar{\nu}}\right] \\
& +\frac{1}{3}\left[y_d^{rs}\bar{\mathcal{C}}_{dB}^{rs} - \bar{y}_d^{rs}\mathcal{C}_{dB}^{rs}\right]\left[2(\Omega_{q,j}^*D_{\bar{\sigma}}\Omega_q^i)H_i^\dagger D^{\bar{\mu}}H^j\tilde{B}^{\bar{\mu}\bar{\sigma}} - 2(D_{\bar{\nu}}\Omega_{q,j}^*\Omega_q^i)D^{\bar{\mu}}H_i^\dagger H^j\tilde{B}^{\bar{\mu}\bar{\nu}}\right] \\
& +\frac{1}{3}\left[\bar{y}_d^{rs}\mathcal{C}_{dB}^{rs} + y_d^{rs}\bar{\mathcal{C}}_{dB}^{rs}\right]\left[2(D_{\bar{\nu}}\Omega_{q,j}^*\Omega_q^i)D^{\bar{\mu}}H_i^\dagger H^j\tilde{B}^{\bar{\mu}\bar{\nu}} + 2(\Omega_{q,j}^*D_{\bar{\sigma}}\Omega_q^i)H_i^\dagger D^{\bar{\mu}}H^j\tilde{B}^{\bar{\mu}\bar{\sigma}}\right] \\
& +\frac{1}{3}\left[y_d^{rs}\bar{\mathcal{C}}_{dB}^{rs} - \bar{y}_d^{rs}\mathcal{C}_{dB}^{rs}\right]\left[2(\Omega_d^\dagger D_{\bar{\sigma}}\Omega_d)\tilde{B}^{\bar{\mu}\bar{\sigma}}(H^\dagger D_{\bar{\mu}}H) - 2(D_{\bar{\nu}}\Omega_d^\dagger\Omega_d)\tilde{B}^{\bar{\mu}\bar{\nu}}(D_{\bar{\mu}}H^\dagger H)\right] \\
& +\frac{1}{3}\left[\bar{y}_d^{rs}\mathcal{C}_{dB}^{rs} + y_d^{rs}\bar{\mathcal{C}}_{dB}^{rs}\right]\left[2(\Omega_d^\dagger D_{\bar{\sigma}}\Omega_d)\tilde{B}^{\bar{\mu}\bar{\sigma}}(H^\dagger D_{\bar{\mu}}H) + 2(D_{\bar{\nu}}\Omega_d^\dagger\Omega_d)\tilde{B}^{\bar{\mu}\bar{\nu}}(D_{\bar{\mu}}H^\dagger H)\right] \\
& +\frac{1}{3}g_Y\bar{\mathcal{C}}_{dB}^{rs}(D_{\bar{\mu}}\Omega_{d,a}^*\Omega_d^b)(D^{\bar{\mu}}\bar{d}_{bs}H^\dagger q_r^a) - \frac{1}{18}g_Y\bar{\mathcal{C}}_{dB}^{rs}(D_{\bar{\mu}}\Omega_{q,aj}^*\Omega_q^{bi})H_i^\dagger(D^{\bar{\mu}}\bar{d}_{bs}q_r^{aj}) \\
& -\frac{1}{9}g_Y\bar{\mathcal{C}}_{dB}^{rs}(D_{\bar{\mu}}\Omega_{d,a}^*\Omega_d^b)(\bar{d}_{bs}H^\dagger D^{\bar{\mu}}q_r^a) - \frac{1}{6}g_Y\bar{\mathcal{C}}_{dB}^{rs}(D_{\bar{\mu}}\Omega_{q,aj}^*\Omega_q^{bi})D^{\bar{\mu}}H_i^\dagger(\bar{d}_{bs}q_r^{aj}) \\
& -\frac{i}{4}\left[\bar{y}_d^{ts}\mathcal{C}_{dB}^{tr} + y_d^{tr}\bar{\mathcal{C}}_{dB}^{ts}\right]\left[2(\Omega_{q,a}^*D_{\bar{\rho}}\Omega_q^b)\tilde{B}^{\bar{\rho}\bar{\sigma}}(\bar{d}_{bs}\gamma^{\bar{\sigma}}d_r^a) - 2(D_{\bar{\mu}}\Omega_{q,a}^*\Omega_q^b)\tilde{B}^{\bar{\mu}\bar{\sigma}}(\bar{d}_{bs}\gamma^{\bar{\sigma}}d_r^a)\right] \\
& +\frac{i}{4}\left[\bar{y}_d^{rt}\mathcal{C}_{dB}^{st} + y_d^{st}\bar{\mathcal{C}}_{dB}^{rt}\right]\left[2(\Omega_{d,a}^*D_{\bar{\rho}}\Omega_d^b)\tilde{B}^{\bar{\rho}\bar{\sigma}}(\bar{q}_{bs}\gamma^{\bar{\sigma}}q_r^a) - 2(D_{\bar{\mu}}\Omega_{d,a}^*\Omega_d^b)\tilde{B}^{\bar{\mu}\bar{\sigma}}(\bar{q}_{bs}\gamma^{\bar{\sigma}}q_r^a)\right] \\
& +\frac{1}{3}g_Y\mathcal{C}_{dB}^{sr}(\Omega_{d,a}^*D_{\bar{\mu}}\Omega_d^b)(\bar{q}_{bs}H D^{\bar{\mu}}d_r^a) \\
& +\frac{1}{2}\left[y_d^{tr}\bar{\mathcal{C}}_{dB}^{ts} - \bar{y}_d^{ts}\mathcal{C}_{dB}^{tr}\right]\left[(\Omega_{q,a}^*D_{\bar{\nu}}\Omega_q^b)B^{\bar{\mu}\bar{\nu}}(\bar{d}_{bs}\gamma^{\bar{\mu}}d_r^a) + (D_{\bar{\mu}}\Omega_{q,a}^*\Omega_q^b)B^{\bar{\mu}\bar{\nu}}(\bar{d}_{bs}\gamma^{\bar{\nu}}d_r^a)\right] \\
& +\frac{1}{2}\left[\bar{y}_d^{rt}\mathcal{C}_{dB}^{st} - y_d^{st}\bar{\mathcal{C}}_{dB}^{rt}\right]\left[(\Omega_{d,a}^*D_{\bar{\nu}}\Omega_d^b)B^{\bar{\mu}\bar{\nu}}(\bar{q}_{bs}\gamma^{\bar{\mu}}q_r^a) + (D_{\bar{\mu}}\Omega_{d,a}^*\Omega_d^b)B^{\bar{\mu}\bar{\nu}}(\bar{q}_{bs}\gamma^{\bar{\nu}}q_r^a)\right] \\
& -\frac{1}{3}g_Y\bar{\mathcal{C}}_{dB}^{rs}(D_{\bar{\mu}}\Omega_{d,a}^*D_{\bar{\mu}}\Omega_d^b)(\bar{d}_{bs}H^\dagger q_r^a) - \frac{1}{3}g_Y\bar{\mathcal{C}}_{dB}^{rs}(D_{\bar{\mu}}\Omega_{d,a}^*\Omega_d^b)(\bar{d}_{bs}D_{\bar{\mu}}H^\dagger q_r^a) - \frac{1}{3}g_Y\mathcal{C}_{dB}^{sr}(D_{\bar{\mu}}\Omega_{d,a}^*D_{\bar{\mu}}\Omega_d^b)(\bar{q}_{bs}H d_r^a) \\
& -\frac{1}{3}g_Y\mathcal{C}_{dB}^{sr}(\Omega_{d,a}^*D_{\bar{\mu}}\Omega_d^b)(\bar{q}_{bs}D_{\bar{\mu}}H d_r^a) \\
& +\frac{2i}{3}\left[\bar{y}_d^{rs}\mathcal{C}_{dB}^{rs} + y_d^{rs}\bar{\mathcal{C}}_{dB}^{rs}\right]\left[(\Omega_{q,j}^*D_{\bar{\nu}}\Omega_q^i)H_i^\dagger D^{\bar{\mu}}H^j B^{\bar{\mu}\bar{\nu}} - (D_{\bar{\nu}}\Omega_{q,j}^*\Omega_q^i)D^{\bar{\mu}}H_i^\dagger H^j B^{\bar{\mu}\bar{\nu}}\right] \\
& -\frac{2i}{3}\left[\bar{y}_d^{rs}\mathcal{C}_{dB}^{rs} - y_d^{rs}\bar{\mathcal{C}}_{dB}^{rs}\right]\left[(D_{\bar{\nu}}\Omega_{q,j}^*\Omega_q^i)D^{\bar{\mu}}H_i^\dagger H^j B^{\bar{\mu}\bar{\nu}} + (\Omega_{q,j}^*D_{\bar{\nu}}\Omega_q^i)H_i^\dagger D^{\bar{\mu}}H^j B^{\bar{\mu}\bar{\nu}}\right] \\
& +\frac{2i}{3}\left[\bar{y}_d^{rs}\mathcal{C}_{dB}^{rs} + y_d^{rs}\bar{\mathcal{C}}_{dB}^{rs}\right]\left[(\Omega_d^\dagger D_{\bar{\nu}}\Omega_d)B^{\bar{\mu}\bar{\nu}}(H^\dagger D_{\bar{\mu}}H) - (D_{\bar{\nu}}\Omega_d^\dagger\Omega_d)B^{\bar{\mu}\bar{\nu}}(D_{\bar{\mu}}H^\dagger H)\right] \\
& -\frac{2i}{3}\left[\bar{y}_d^{rs}\mathcal{C}_{dB}^{rs} - y_d^{rs}\bar{\mathcal{C}}_{dB}^{rs}\right]\left[(\Omega_d^\dagger D_{\bar{\nu}}\Omega_d)B^{\bar{\mu}\bar{\nu}}(H^\dagger D_{\bar{\mu}}H) + (D_{\bar{\nu}}\Omega_d^\dagger\Omega_d)B^{\bar{\mu}\bar{\nu}}(D_{\bar{\mu}}H^\dagger H)\right], \tag{3.26}
\end{aligned}$$

$$\begin{aligned}
\Gamma_\Omega^{(1)}[\mathcal{O}_{dW}] &= \frac{1}{6}g_L\bar{\mathcal{C}}_{dW}^{rs}(D_{\bar{\mu}}\Omega_{q,aj}^*\Omega_q^{bi})H_i^\dagger(D^{\bar{\mu}}\bar{d}_{bs}q_r^{aj}) + \frac{1}{6}g_L\mathcal{C}_{dW}^{sr}(\Omega_{q,ai}^*D_{\bar{\mu}}\Omega_q^{bj})H^i(\bar{q}_{bj}s D^{\bar{\mu}}d_r^a) \\
& -\frac{i}{4}g_L\left[\bar{y}_d^{rt}\mathcal{C}_{dW}^{st} + y_d^{st}\bar{\mathcal{C}}_{dW}^{rt}\right]\left[(\Omega_{q,aj}^*D_{\bar{\mu}}\Omega_q^{bi})H_i^\dagger(\bar{q}_{bs}H\gamma^{\bar{\mu}}q_r^{aj}) - (D_{\bar{\mu}}\Omega_{q,aj}^*\Omega_q^{bk})H^j(\bar{q}_{bks}\gamma^{\bar{\mu}}H^\dagger q_r^a)\right]
\end{aligned}$$

$$\begin{aligned}
& -\frac{i}{4}g_L \left[ \bar{y}_d^{rt} \mathcal{C}_{dW}^{st} - y_d^{st} \bar{\mathcal{C}}_{dW}^{rt} \right] \left[ (\Omega_{q,aj}^* D_{\bar{\mu}} \Omega_q^{bi}) H_i^\dagger (\bar{q}_{bs} H \gamma^{\bar{\mu}} q_r^{aj}) + (D_{\bar{\mu}} \Omega_{q,aj}^* \Omega_q^{bk}) H^j (\bar{q}_{bks} \gamma^{\bar{\mu}} H^\dagger q_r^a) \right] \\
& + \frac{1}{3} \left[ -\bar{y}_d^{rs} \mathcal{C}_{dW}^{rs} - y_d^{rs} \bar{\mathcal{C}}_{dW}^{rs} \right] \left[ 2t_k^{Ij} (\Omega_{d,a}^* D_{\bar{\sigma}} \Omega_d^b) (\Omega_{q,bj}^* D_{\bar{\rho}} \Omega_q^{ai}) H_i^\dagger H^k \widetilde{W}^{\bar{\rho}\bar{\sigma}I} - 2t_k^{Ii} (D_{\bar{\mu}} \Omega_{d,a}^* \Omega_d^b) (D_{\bar{\nu}} \Omega_{q,bj}^* \Omega_q^{ak}) H_i^\dagger H^j \widetilde{W}^{\bar{\mu}\bar{\nu}I} \right] \\
& + \frac{1}{3} \left[ y_d^{rs} \bar{\mathcal{C}}_{dW}^{rs} - \bar{y}_d^{rs} \mathcal{C}_{dW}^{rs} \right] \left[ 2t_k^{Ii} (D_{\bar{\mu}} \Omega_{d,a}^* \Omega_d^b) (D_{\bar{\nu}} \Omega_{q,bj}^* \Omega_q^{ak}) H_i^\dagger H^j \widetilde{W}^{\bar{\mu}\bar{\nu}I} + 2t_k^{Ij} (\Omega_{d,a}^* D_{\bar{\sigma}} \Omega_d^b) (\Omega_{q,bj}^* D_{\bar{\rho}} \Omega_q^{ai}) H_i^\dagger H^k \widetilde{W}^{\bar{\rho}\bar{\sigma}I} \right] \\
& + \frac{i}{3} g_L \bar{\mathcal{C}}_{dW}^{rs} (D_{\bar{\nu}} \Omega_{q,aj}^* \Omega_q^{bi}) D_{\bar{\mu}} H_i^\dagger (\bar{d}_{bs} \sigma^{\bar{\mu}\bar{\nu}} q_r^{aj}) + \frac{1}{2} g_L \bar{\mathcal{C}}_{dW}^{rs} (D_{\bar{\mu}} \Omega_{q,aj}^* \Omega_q^{bi}) D_{\bar{\mu}} H_i^\dagger (\bar{d}_{bs} q_r^{aj}) \\
& - \frac{1}{3} g_L \bar{\mathcal{C}}_{dW}^{rs} (D_{\bar{\mu}} \Omega_{q,a}^* \Omega_q^b) (D_{\bar{\mu}} \bar{d}_{bs} H^\dagger q_r^a) - \frac{i}{3} g_L \mathcal{C}_{dW}^{sr} (\Omega_{q,ai}^* D_{\bar{\nu}} \Omega_q^{bj}) D_{\bar{\mu}} H^i (\bar{q}_{bjs} \sigma^{\bar{\mu}\bar{\nu}} d_r^a) \\
& - \frac{i}{2} \left[ \bar{y}_d^{ts} \mathcal{C}_{dW}^{tr} + y_d^{tr} \bar{\mathcal{C}}_{dW}^{ts} \right] \left[ 2t_j^{Ii} (\Omega_{q,ai}^* D_{\bar{\rho}} \Omega_q^{bj}) \widetilde{W}^{\bar{\rho}\bar{\sigma}I} (\bar{d}_{bs} \gamma^{\bar{\sigma}} d_r^a) - 2t_j^{Ii} (D_{\bar{\mu}} \Omega_{q,ai}^* \Omega_q^{bj}) \widetilde{W}^{\bar{\mu}\bar{\sigma}I} (\bar{d}_{bs} \gamma^{\bar{\sigma}} d_r^a) \right] \\
& + \frac{i}{2} \left[ \bar{y}_d^{rt} \mathcal{C}_{dW}^{st} + y_d^{st} \bar{\mathcal{C}}_{dW}^{rt} \right] \left[ 2(\Omega_{d,a}^* D_{\bar{\rho}} \Omega_d^b) \widetilde{W}^{\bar{\rho}\bar{\sigma}I} (\bar{q}_{bs} t^I \gamma^{\bar{\sigma}} q_r^a) - 2(D_{\bar{\mu}} \Omega_{d,a}^* \Omega_d^b) \widetilde{W}^{\bar{\mu}\bar{\sigma}I} (\bar{q}_{bs} t^I \gamma^{\bar{\sigma}} q_r^a) \right] \\
& + \frac{1}{2} g_L \mathcal{C}_{dW}^{sr} (\Omega_{q,ai}^* D_{\bar{\mu}} \Omega_q^{bj}) D_{\bar{\mu}} H^i (\bar{q}_{bjs} d_r^a) \\
& + \frac{2i}{3} \left[ \bar{y}_d^{rs} \mathcal{C}_{dW}^{rs} - y_d^{rs} \bar{\mathcal{C}}_{dW}^{rs} \right] \left[ t_k^{Ij} (\Omega_{d,a}^* D_{\bar{\nu}} \Omega_d^b) (\Omega_{q,bj}^* D_{\bar{\mu}} \Omega_q^{ai}) H_i^\dagger H^k W^{\bar{\mu}\bar{\nu}I} - t_k^{Ii} (D_{\bar{\mu}} \Omega_{d,a}^* \Omega_d^b) (D_{\bar{\nu}} \Omega_{q,bj}^* \Omega_q^{ak}) H_i^\dagger H^j W^{\bar{\mu}\bar{\nu}I} \right] \\
& + \frac{2i}{3} \left[ \bar{y}_d^{rs} \mathcal{C}_{dW}^{rs} + y_d^{rs} \bar{\mathcal{C}}_{dW}^{rs} \right] \left[ t_k^{Ii} (D_{\bar{\mu}} \Omega_{d,a}^* \Omega_d^b) (D_{\bar{\nu}} \Omega_{q,bj}^* \Omega_q^{ak}) H_i^\dagger H^j W^{\bar{\mu}\bar{\nu}I} + t_k^{Ij} (\Omega_{d,a}^* D_{\bar{\nu}} \Omega_d^b) (\Omega_{q,bj}^* D_{\bar{\mu}} \Omega_q^{ai}) H_i^\dagger H^k W^{\bar{\mu}\bar{\nu}I} \right] \\
& + \frac{2}{3} \left[ y_d^{rs} \bar{\mathcal{C}}_{dW}^{rs} - \bar{y}_d^{rs} \mathcal{C}_{dW}^{rs} \right] \left[ 2t_k^{Ii} (D_{\bar{\mu}} \Omega_{q,j}^* \Omega_q^k) H_i^\dagger D_{\bar{\nu}} H^j \widetilde{W}^{\bar{\mu}\bar{\nu}I} + 2t_k^{Ij} (\Omega_{q,j}^* D_{\bar{\sigma}} \Omega_q^i) D_{\bar{\mu}} H_i^\dagger H^k \widetilde{W}^{\bar{\mu}\bar{\sigma}I} \right] \\
& + \frac{2}{3} \left[ y_d^{rs} \bar{\mathcal{C}}_{dW}^{rs} - \bar{y}_d^{rs} \mathcal{C}_{dW}^{rs} \right] \left[ 2(\Omega_d^\dagger D_{\bar{\sigma}} \Omega_d) \widetilde{W}^{\bar{\mu}\bar{\sigma}I} (H^\dagger t^I D_{\bar{\mu}} H) - 2(D_{\bar{\nu}} \Omega_d^\dagger \Omega_d) \widetilde{W}^{\bar{\mu}\bar{\nu}I} (D_{\bar{\mu}} H^\dagger t^I H) \right] \\
& + \frac{2}{3} \left[ \bar{y}_d^{rs} \mathcal{C}_{dW}^{rs} + y_d^{rs} \bar{\mathcal{C}}_{dW}^{rs} \right] \left[ 2(\Omega_d^\dagger D_{\bar{\sigma}} \Omega_d) \widetilde{W}^{\bar{\mu}\bar{\sigma}I} (H^\dagger t^I D_{\bar{\mu}} H) + 2(D_{\bar{\nu}} \Omega_d^\dagger \Omega_d) \widetilde{W}^{\bar{\mu}\bar{\nu}I} (D_{\bar{\mu}} H^\dagger t^I H) \right] \\
& - \frac{2i}{3} g_L \bar{\mathcal{C}}_{dW}^{rs} (D_{\bar{\nu}} \Omega_{q,a}^* \Omega_q^b) (\bar{d}_{bs} \sigma^{\bar{\mu}\bar{\nu}} D_{\bar{\mu}} H^\dagger q_r^a) + g_L \bar{\mathcal{C}}_{dW}^{rs} (D_{\bar{\mu}} \Omega_{q,a}^* D_{\bar{\mu}} \Omega_q^b) (\bar{d}_{bs} H^\dagger q_r^a) \\
& + g_L \bar{\mathcal{C}}_{dW}^{rs} (D_{\bar{\mu}} \Omega_{q,a}^* \Omega_q^b) (\bar{d}_{bs} H^\dagger D_{\bar{\mu}} q_r^a) \\
& + \left[ y_d^{tr} \bar{\mathcal{C}}_{dW}^{ts} - \bar{y}_d^{ts} \mathcal{C}_{dW}^{tr} \right] \left[ t_j^{Ii} (\Omega_{q,ai}^* D_{\bar{\nu}} \Omega_q^{bj}) W^{\bar{\mu}\bar{\nu}I} (\bar{d}_{bs} \gamma^{\bar{\mu}} d_r^a) + t_j^{Ii} (D_{\bar{\mu}} \Omega_{q,ai}^* \Omega_q^{bj}) W^{\bar{\mu}\bar{\nu}I} (\bar{d}_{bs} \gamma^{\bar{\nu}} d_r^a) \right] \\
& + g_L \mathcal{C}_{dW}^{sr} (D_{\bar{\mu}} \Omega_{q,a}^* D_{\bar{\mu}} \Omega_q^b) (\bar{q}_{bs} H d_r^a) + g_L \mathcal{C}_{dW}^{sr} (\Omega_{q,a}^* D_{\bar{\mu}} \Omega_q^b) (D_{\bar{\mu}} \bar{q}_{bs} H d_r^a) - \frac{1}{3} g_L \mathcal{C}_{dW}^{sr} (\Omega_{q,a}^* D_{\bar{\mu}} \Omega_q^b) (\bar{q}_{bs} H D_{\bar{\mu}} d_r^a) \\
& - \frac{1}{2} g_L \bar{\mathcal{C}}_{dW}^{rs} (D_{\bar{\mu}} \Omega_{q,aj}^* D_{\bar{\mu}} \Omega_q^{bi}) H_i^\dagger (\bar{d}_{bs} q_r^{aj}) - \frac{1}{2} g_L \bar{\mathcal{C}}_{dW}^{rs} (D_{\bar{\mu}} \Omega_{q,aj}^* \Omega_q^{bi}) H_i^\dagger (\bar{d}_{bs} D_{\bar{\mu}} q_r^{aj}) \\
& - \frac{1}{2} g_L \mathcal{C}_{dW}^{sr} (D_{\bar{\mu}} \Omega_{q,ai}^* D_{\bar{\mu}} \Omega_q^{bj}) H^i (\bar{q}_{bjs} d_r^a) - \frac{1}{2} g_L \mathcal{C}_{dW}^{sr} (\Omega_{q,ai}^* D_{\bar{\mu}} \Omega_q^{bj}) H^i (D_{\bar{\mu}} \bar{q}_{bjs} d_r^a) \\
& + \frac{i}{2} g_L \left[ \bar{y}_d^{rt} \mathcal{C}_{dW}^{st} + y_d^{st} \bar{\mathcal{C}}_{dW}^{rt} \right] (\Omega_{q,aj}^* \overset{\leftrightarrow}{D}_{\bar{\mu}} \Omega_q^{bi}) H_i^\dagger H^j (\bar{q}_{bs} \gamma^{\bar{\mu}} q_r^a) \\
& - \frac{2}{3} \left[ \bar{y}_d^{rs} \mathcal{C}_{dW}^{rs} + y_d^{rs} \bar{\mathcal{C}}_{dW}^{rs} \right] \left[ 2t_k^{Ij} (\Omega_{q,j}^* D_{\bar{\sigma}} \Omega_q^i) D_{\bar{\mu}} H_i^\dagger H^k \widetilde{W}^{\bar{\mu}\bar{\sigma}I} - 2t_k^{Ii} (D_{\bar{\mu}} \Omega_{q,j}^* \Omega_q^k) H_i^\dagger D_{\bar{\nu}} H^j \widetilde{W}^{\bar{\mu}\bar{\nu}I} \right] \\
& + \frac{2i}{3} g_L \mathcal{C}_{dW}^{sr} (\Omega_{q,a}^* D_{\bar{\nu}} \Omega_q^b) (\bar{q}_{bs} D_{\bar{\mu}} H \sigma^{\bar{\mu}\bar{\nu}} d_r^a) \\
& + \left[ \bar{y}_d^{rt} \mathcal{C}_{dW}^{st} - y_d^{st} \bar{\mathcal{C}}_{dW}^{rt} \right] \left[ (\Omega_{d,a}^* D_{\bar{\nu}} \Omega_d^b) W^{\bar{\mu}\bar{\nu}I} (\bar{q}_{bs} t^I \gamma^{\bar{\mu}} q_r^a) + (D_{\bar{\mu}} \Omega_{d,a}^* \Omega_d^b) W^{\bar{\mu}\bar{\nu}I} (\bar{q}_{bs} t^I \gamma^{\bar{\nu}} q_r^a) \right] \\
& - g_L \bar{\mathcal{C}}_{dW}^{rs} (D_{\bar{\mu}} \Omega_{q,a}^* \Omega_q^b) (\bar{d}_{bs} D_{\bar{\mu}} H^\dagger q_r^a) - g_L \mathcal{C}_{dW}^{sr} (\Omega_{q,a}^* D_{\bar{\mu}} \Omega_q^b) (\bar{q}_{bs} D_{\bar{\mu}} H d_r^a)
\end{aligned}$$

$$\begin{aligned}
& + \frac{4i}{3} \left[ \bar{y}_d^{rs} \mathcal{C}_{dW}^{rs} - y_d^{rs} \bar{\mathcal{C}}_{dW}^{rs} \right] \left[ t_k^{Ij} (\Omega_{q,j}^* D_{\bar{\nu}} \Omega_q^i) D^{\bar{\mu}} H_i^\dagger H^k W^{\bar{\mu}\bar{\nu}I} - t_k^{Ii} (D_{\bar{\mu}} \Omega_{q,j}^* \Omega_q^k) H_i^\dagger D^{\bar{\nu}} H^j W^{\bar{\mu}\bar{\nu}I} \right] \\
& + \frac{4i}{3} \left[ \bar{y}_d^{rs} \mathcal{C}_{dW}^{rs} + y_d^{rs} \bar{\mathcal{C}}_{dW}^{rs} \right] \left[ t_k^{Ii} (D_{\bar{\mu}} \Omega_{q,j}^* \Omega_q^k) H_i^\dagger D^{\bar{\nu}} H^j W^{\bar{\mu}\bar{\nu}I} + t_k^{Ij} (\Omega_{q,j}^* D_{\bar{\nu}} \Omega_q^i) D^{\bar{\mu}} H_i^\dagger H^k W^{\bar{\mu}\bar{\nu}I} \right] \\
& + \frac{4i}{3} \left[ \bar{y}_d^{rs} \mathcal{C}_{dW}^{rs} + y_d^{rs} \bar{\mathcal{C}}_{dW}^{rs} \right] \left[ (\Omega_d^\dagger D_{\bar{\nu}} \Omega_d) W^{\bar{\mu}\bar{\nu}I} (H^\dagger t^I D_{\bar{\mu}} H) - (D_{\bar{\nu}} \Omega_d^\dagger \Omega_d) W^{\bar{\mu}\bar{\nu}I} (D_{\bar{\mu}} H^\dagger t^I H) \right] \\
& - \frac{4i}{3} \left[ \bar{y}_d^{rs} \mathcal{C}_{dW}^{rs} - y_d^{rs} \bar{\mathcal{C}}_{dW}^{rs} \right] \left[ (\Omega_d^\dagger D_{\bar{\nu}} \Omega_d) W^{\bar{\mu}\bar{\nu}I} (H^\dagger t^I D_{\bar{\mu}} H) + (D_{\bar{\nu}} \Omega_d^\dagger \Omega_d) W^{\bar{\mu}\bar{\nu}I} (D_{\bar{\mu}} H^\dagger t^I H) \right], \tag{3.27}
\end{aligned}$$

$$\begin{aligned}
\Gamma_\Omega^{(1)} [\mathcal{O}_{dG}] &= \frac{1}{18} g_s \bar{\mathcal{C}}_{dG}^{rs} (D_{\bar{\mu}} \Omega_{q,aj}^* \Omega_q^{bi}) H_i^\dagger (D^{\bar{\mu}} \bar{d}_{bs} q_r^{aj}) + \frac{1}{18} g_s \mathcal{C}_{dG}^{sr} (\Omega_{q,ai}^* D_{\bar{\mu}} \Omega_q^{bj}) H^i (\bar{q}_{bjs} D^{\bar{\mu}} d_r^a) \\
& + \frac{1}{6} \left[ -\bar{y}_d^{rs} \mathcal{C}_{dG}^{rs} - y_d^{rs} \bar{\mathcal{C}}_{dG}^{rs} \right] \left[ 2T_c^{Ab} (D_{\bar{\mu}} \Omega_{d,a}^* \Omega_d^c) (\Omega_{q,bj}^* D_{\bar{\sigma}} \Omega_q^{ai}) H_i^\dagger H^j \tilde{G}^{\bar{\mu}\bar{\sigma}A} - 2T_c^{Aa} (\Omega_{d,a}^* D_{\bar{\sigma}} \Omega_d^b) (D_{\bar{\mu}} \Omega_{q,bj}^* \Omega_q^{ci}) H_i^\dagger H^j \tilde{G}^{\bar{\mu}\bar{\sigma}A} \right] \\
& + \frac{1}{6} \left[ y_d^{rs} \bar{\mathcal{C}}_{dG}^{rs} - \bar{y}_d^{rs} \mathcal{C}_{dG}^{rs} \right] \left[ 2T_c^{Aa} (\Omega_{d,a}^* D_{\bar{\sigma}} \Omega_d^b) (D_{\bar{\mu}} \Omega_{q,bj}^* \Omega_q^{ci}) H_i^\dagger H^j \tilde{G}^{\bar{\mu}\bar{\sigma}A} + 2T_c^{Ab} (D_{\bar{\mu}} \Omega_{d,a}^* \Omega_d^c) (\Omega_{q,bj}^* D_{\bar{\sigma}} \Omega_q^{ai}) H_i^\dagger H^j \tilde{G}^{\bar{\mu}\bar{\sigma}A} \right] \\
& + \frac{1}{6} g_s \bar{\mathcal{C}}_{dG}^{rs} (D_{\bar{\mu}} \Omega_d^\dagger \Omega_d) (\bar{d}_s H^\dagger D^{\bar{\mu}} q_r) + \frac{1}{6} g_s \bar{\mathcal{C}}_{dG}^{rs} (D_{\bar{\mu}} \Omega_{q,aj}^* \Omega_q^{bi}) D^{\bar{\mu}} H_i^\dagger (\bar{d}_{bs} q_r^{aj}) + \frac{1}{6} g_s \mathcal{C}_{dG}^{sr} (\Omega_d^\dagger D_{\bar{\mu}} \Omega_d) (D^{\bar{\mu}} \bar{q}_{bs} H d_r^a) \\
& + \frac{1}{6} g_s \mathcal{C}_{dG}^{sr} (\Omega_{d,a}^* D_{\bar{\mu}} \Omega_d^b) (\bar{q}_{bs} H D^{\bar{\mu}} d_r^a) - \frac{1}{18} g_s \bar{\mathcal{C}}_{dG}^{rs} (D_{\bar{\mu}} \Omega_{d,a}^* \Omega_d^b) (\bar{d}_{bs} H^\dagger D^{\bar{\mu}} q_r^a) - \frac{1}{18} g_s \mathcal{C}_{dG}^{sr} (\Omega_{d,a}^* D_{\bar{\mu}} \Omega_d^b) (D^{\bar{\mu}} \bar{q}_{bs} H d_r^a) \\
& - \frac{i}{12} g_s \left[ \bar{y}_d^{rt} \mathcal{C}_{dG}^{st} + y_d^{st} \bar{\mathcal{C}}_{dG}^{rt} \right] \left[ (\Omega_{q,aj}^* D_{\bar{\mu}} \Omega_q^{bi}) H_i^\dagger (\bar{q}_{bs} H \gamma^{\bar{\mu}} q_r^{aj}) - (D_{\bar{\mu}} \Omega_{q,aj}^* \Omega_q^{bk}) H^j (\bar{q}_{bks} \gamma^{\bar{\mu}} H^\dagger q_r^a) \right] \\
& - \frac{i}{12} g_s \left[ \bar{y}_d^{rt} \mathcal{C}_{dG}^{st} - y_d^{st} \bar{\mathcal{C}}_{dG}^{rt} \right] \left[ (\Omega_{q,aj}^* D_{\bar{\mu}} \Omega_q^{bi}) H_i^\dagger (\bar{q}_{bs} H \gamma^{\bar{\mu}} q_r^{aj}) + (D_{\bar{\mu}} \Omega_{q,aj}^* \Omega_q^{bk}) H^j (\bar{q}_{bks} \gamma^{\bar{\mu}} H^\dagger q_r^a) \right] \\
& - \frac{i}{12} g_s \left[ \bar{y}_d^{ts} \mathcal{C}_{dG}^{tr} + y_d^{tr} \bar{\mathcal{C}}_{dG}^{ts} \right] \left[ (\Omega_{d,a}^* \overleftrightarrow{D}_{\bar{\mu}} \Omega_d^b) (H^\dagger H) (\bar{d}_{bs} \gamma^{\bar{\mu}} d_r^a) + \frac{i}{9} g_s \bar{\mathcal{C}}_{dG}^{rs} (D_{\bar{\nu}} \Omega_{q,aj}^* \Omega_q^{bi}) D^{\bar{\mu}} H_i^\dagger (\bar{d}_{bs} \sigma^{\bar{\mu}\bar{\nu}} q_r^{aj}) \right. \\
& + \frac{i}{9} g_s \bar{\mathcal{C}}_{dG}^{rs} (D_{\bar{\nu}} \Omega_{d,a}^* \Omega_d^b) (\bar{d}_{bs} \sigma^{\bar{\mu}\bar{\nu}} D_{\bar{\mu}} H^\dagger q_r^a) - \frac{i}{9} g_s \mathcal{C}_{dG}^{sr} (\Omega_{d,a}^* D_{\bar{\nu}} \Omega_d^b) (\bar{q}_{bs} D_{\bar{\mu}} H \sigma^{\bar{\mu}\bar{\nu}} d_r^a) \\
& \left. - \frac{i}{9} g_s \mathcal{C}_{dG}^{sr} (\Omega_{q,ai}^* D_{\bar{\nu}} \Omega_q^{bj}) D^{\bar{\mu}} H^i (\bar{q}_{bjs} \sigma^{\bar{\mu}\bar{\nu}} d_r^a) + \frac{1}{6} g_s \bar{\mathcal{C}}_{dG}^{rs} (D_{\bar{\mu}} \Omega_{d,a}^* \Omega_d^b) (D^{\bar{\mu}} \bar{d}_{bs} H^\dagger q_r^a) \right] \\
& + \frac{1}{6} g_s \mathcal{C}_{dG}^{sr} (\Omega_{q,ai}^* D_{\bar{\mu}} \Omega_q^{bj}) D^{\bar{\mu}} H^i (\bar{q}_{bjs} d_r^a) - \frac{1}{6} g_s \mathcal{C}_{dG}^{sr} (D_{\bar{\mu}} \Omega_{q,ai}^* D_{\bar{\mu}} \Omega_q^{bj}) H^i (\bar{q}_{bjs} d_r^a) - \frac{1}{6} g_s \mathcal{C}_{dG}^{sr} (\Omega_{q,ai}^* D_{\bar{\mu}} \Omega_q^{bj}) H^i (D^{\bar{\mu}} \bar{q}_{bjs} d_r^a) \\
& - \frac{i}{4} \left[ \bar{y}_d^{ts} \mathcal{C}_{dG}^{tr} + y_d^{tr} \bar{\mathcal{C}}_{dG}^{ts} \right] \left[ 2T_b^{Aa} (\Omega_{q,a}^* D_{\bar{\rho}} \Omega_q^c) \tilde{G}^{\bar{\rho}\bar{\sigma}A} (\bar{d}_{cs} \gamma^{\bar{\sigma}} d_r^b) - 2T_c^{Ab} (D_{\bar{\mu}} \Omega_{q,a}^* \Omega_q^c) \tilde{G}^{\bar{\mu}\bar{\sigma}A} (\bar{d}_{bs} \gamma^{\bar{\sigma}} d_r^a) \right] \\
& - \frac{i}{4} \left[ \bar{y}_d^{ts} \mathcal{C}_{dG}^{tr} - y_d^{tr} \bar{\mathcal{C}}_{dG}^{ts} \right] \left[ 2T_c^{Ab} (D_{\bar{\mu}} \Omega_{q,a}^* \Omega_q^c) \tilde{G}^{\bar{\mu}\bar{\sigma}A} (\bar{d}_{bs} \gamma^{\bar{\sigma}} d_r^a) + 2T_b^{Aa} (\Omega_{q,a}^* D_{\bar{\rho}} \Omega_q^c) \tilde{G}^{\bar{\rho}\bar{\sigma}A} (\bar{d}_{cs} \gamma^{\bar{\sigma}} d_r^b) \right] \\
& + \frac{i}{4} g_s \left[ \bar{y}_d^{rt} \mathcal{C}_{dG}^{st} + y_d^{st} \bar{\mathcal{C}}_{dG}^{rt} \right] \left[ (\Omega_{q,j}^* D_{\bar{\mu}} \Omega_q^i) H_i^\dagger (\bar{q}_s H \gamma^{\bar{\mu}} q_r^j) - (D_{\bar{\mu}} \Omega_{q,j}^* \Omega_q^k) H^j (\bar{q}_{ks} \gamma^{\bar{\mu}} H^\dagger q_r) \right] \\
& + \frac{i}{4} g_s \left[ \bar{y}_d^{rt} \mathcal{C}_{dG}^{st} - y_d^{st} \bar{\mathcal{C}}_{dG}^{rt} \right] \left[ (\Omega_{q,j}^* D_{\bar{\mu}} \Omega_q^i) H_i^\dagger (\bar{q}_s H \gamma^{\bar{\mu}} q_r^j) + (D_{\bar{\mu}} \Omega_{q,j}^* \Omega_q^k) H^j (\bar{q}_{ks} \gamma^{\bar{\mu}} H^\dagger q_r) \right] \\
& + \frac{i}{4} \left[ \bar{y}_d^{rt} \mathcal{C}_{dG}^{st} + y_d^{st} \bar{\mathcal{C}}_{dG}^{rt} \right] \left[ 2T_b^{Aa} (\Omega_{d,a}^* D_{\bar{\rho}} \Omega_d^c) \tilde{G}^{\bar{\rho}\bar{\sigma}A} (\bar{q}_{cs} \gamma^{\bar{\sigma}} q_r^b) - 2T_c^{Ab} (D_{\bar{\mu}} \Omega_{d,a}^* \Omega_d^c) \tilde{G}^{\bar{\mu}\bar{\sigma}A} (\bar{q}_{bs} \gamma^{\bar{\sigma}} q_r^a) \right] \\
& - \frac{i}{4} \left[ \bar{y}_d^{rt} \mathcal{C}_{dG}^{st} - y_d^{st} \bar{\mathcal{C}}_{dG}^{rt} \right] \left[ 2T_c^{Ab} (D_{\bar{\mu}} \Omega_{d,a}^* \Omega_d^c) \tilde{G}^{\bar{\mu}\bar{\sigma}A} (\bar{q}_{bs} \gamma^{\bar{\sigma}} q_r^a) + 2T_b^{Aa} (\Omega_{d,a}^* D_{\bar{\rho}} \Omega_d^c) \tilde{G}^{\bar{\rho}\bar{\sigma}A} (\bar{q}_{cs} \gamma^{\bar{\sigma}} q_r^b) \right] \\
& + \frac{i}{4} g_s \left[ \bar{y}_d^{ts} \mathcal{C}_{dG}^{tr} + y_d^{tr} \bar{\mathcal{C}}_{dG}^{ts} \right] \left[ (\Omega_d^\dagger \overleftrightarrow{D}_{\bar{\mu}} \Omega_d) (H^\dagger H) (\bar{d}_s \gamma^{\bar{\mu}} d_r) \right] \\
& + \frac{i}{3} \left[ \bar{y}_d^{rs} \mathcal{C}_{dG}^{rs} - y_d^{rs} \bar{\mathcal{C}}_{dG}^{rs} \right] \left[ T_c^{Ab} (D_{\bar{\mu}} \Omega_{d,a}^* \Omega_d^c) (\Omega_{q,bj}^* D_{\bar{\nu}} \Omega_q^{ai}) H_i^\dagger H^j G^{\bar{\mu}\bar{\nu}A} - T_c^{Aa} (\Omega_{d,a}^* D_{\bar{\nu}} \Omega_d^b) (D_{\bar{\mu}} \Omega_{q,bj}^* \Omega_q^{ci}) H_i^\dagger H^j G^{\bar{\mu}\bar{\nu}A} \right]
\end{aligned}$$

$$\begin{aligned}
& + \frac{i}{3} \left[ \bar{y}_d^{rs} \mathcal{C}_{dG}^{rs} + y_d^{rs} \bar{\mathcal{C}}_{dG}^{rs} \right] \left[ T_c^{Aa} (\Omega_{d,a}^* D_{\bar{\nu}} \Omega_d^b) (D_{\bar{\mu}} \Omega_{q,bj}^* \Omega_q^{ci}) H_i^\dagger H^j G^{\bar{\mu}\bar{\nu}A} + T_c^{Ab} (D_{\bar{\mu}} \Omega_{d,a}^* \Omega_d^c) (\Omega_{q,bj}^* D_{\bar{\nu}} \Omega_q^{ai}) H_i^\dagger H^j G^{\bar{\mu}\bar{\nu}A} \right] \\
& + \frac{1}{3} \left[ y_d^{rs} \bar{\mathcal{C}}_{dG}^{rs} - \bar{y}_d^{rs} \mathcal{C}_{dG}^{rs} \right] \left[ 2T_b^{Aa} (\Omega_{q,aj}^* D_{\bar{\sigma}} \Omega_q^{bi}) H_i^\dagger D^{\bar{\mu}} H^j \tilde{G}^{\bar{\mu}\bar{\sigma}A} - 2T_b^{Aa} (D_{\bar{\nu}} \Omega_{q,aj}^* \Omega_q^{bi}) D^{\bar{\mu}} H_i^\dagger H^j \tilde{G}^{\bar{\mu}\bar{\sigma}A} \right] \\
& + \frac{1}{3} \left[ \bar{y}_d^{rs} \mathcal{C}_{dG}^{rs} + y_d^{rs} \bar{\mathcal{C}}_{dG}^{rs} \right] \left[ 2T_b^{Aa} (D_{\bar{\nu}} \Omega_{q,aj}^* \Omega_q^{bi}) D^{\bar{\mu}} H_i^\dagger H^j \tilde{G}^{\bar{\mu}\bar{\sigma}A} + 2T_b^{Aa} (\Omega_{q,aj}^* D_{\bar{\sigma}} \Omega_q^{bi}) H_i^\dagger D^{\bar{\mu}} H^j \tilde{G}^{\bar{\mu}\bar{\sigma}A} \right] \\
& + \frac{1}{3} \left[ y_d^{rs} \bar{\mathcal{C}}_{dG}^{rs} - \bar{y}_d^{rs} \mathcal{C}_{dG}^{rs} \right] \left[ 2T_b^{Aa} (\Omega_{d,a}^* D_{\bar{\sigma}} \Omega_d^b) \tilde{G}^{\bar{\mu}\bar{\sigma}A} (H^\dagger D_{\bar{\mu}} H) - 2T_b^{Aa} (D_{\bar{\nu}} \Omega_{d,a}^* \Omega_d^b) \tilde{G}^{\bar{\mu}\bar{\sigma}A} (D_{\bar{\mu}} H^\dagger H) \right] \\
& + \frac{1}{3} \left[ \bar{y}_d^{rs} \mathcal{C}_{dG}^{rs} + y_d^{rs} \bar{\mathcal{C}}_{dG}^{rs} \right] \left[ 2T_b^{Aa} (\Omega_{d,a}^* D_{\bar{\sigma}} \Omega_d^b) \tilde{G}^{\bar{\mu}\bar{\sigma}A} (H^\dagger D_{\bar{\mu}} H) + 2T_b^{Aa} (D_{\bar{\nu}} \Omega_{d,a}^* \Omega_d^b) \tilde{G}^{\bar{\mu}\bar{\sigma}A} (D_{\bar{\mu}} H^\dagger H) \right] \\
& + \frac{i}{3} g_s \mathcal{C}_{dG}^{sr} (\Omega_d^\dagger D_{\bar{\nu}} \Omega_d) (\bar{q}_s D_{\bar{\mu}} H \sigma^{\bar{\mu}\bar{\nu}} d_r) + \frac{1}{2} g_s \bar{\mathcal{C}}_{dG}^{rs} (D_{\bar{\mu}} \Omega_{q,j}^* D_{\bar{\mu}} \Omega_q^i) H_i^\dagger (\bar{d}_s q_r^j) \\
& + \frac{1}{2} g_s \bar{\mathcal{C}}_{dG}^{rs} (D_{\bar{\mu}} \Omega_{q,j}^* \Omega_q^i) H_i^\dagger (\bar{d}_s D^{\bar{\mu}} q_r^j) + \frac{1}{2} g_s \bar{\mathcal{C}}_{dG}^{rs} (D_{\bar{\mu}} \Omega_d^\dagger D_{\bar{\mu}} \Omega_d) (\bar{d}_s H^\dagger q_r) \\
& + \frac{1}{2} \left[ -\bar{y}_d^{tr} \mathcal{C}_{dG}^{tr} - y_d^{tr} \bar{\mathcal{C}}_{dG}^{ts} \right] \left[ T_b^{Aa} (\Omega_{q,a}^* D_{\bar{\nu}} \Omega_q^c) G^{\bar{\mu}\bar{\nu}A} (\bar{d}_{cs} \gamma^{\bar{\mu}} d_r^b) - T_c^{Ab} (D_{\bar{\mu}} \Omega_{q,a}^* \Omega_q^c) G^{\bar{\mu}\bar{\nu}A} (\bar{d}_{bs} \gamma^{\bar{\nu}} d_r^a) \right] \\
& + \frac{1}{2} \left[ y_d^{tr} \bar{\mathcal{C}}_{dG}^{ts} - \bar{y}_d^{ts} \mathcal{C}_{dG}^{tr} \right] \left[ T_c^{Ab} (D_{\bar{\mu}} \Omega_{q,a}^* \Omega_q^c) G^{\bar{\mu}\bar{\nu}A} (\bar{d}_{bs} \gamma^{\bar{\nu}} d_r^a) + T_b^{Aa} (\Omega_{q,a}^* D_{\bar{\nu}} \Omega_q^c) G^{\bar{\mu}\bar{\nu}A} (\bar{d}_{cs} \gamma^{\bar{\mu}} d_r^b) \right] \\
& + \frac{1}{2} g_s \mathcal{C}_{dG}^{sr} (D_{\bar{\mu}} \Omega_d^\dagger D_{\bar{\mu}} \Omega_d) (\bar{q}_s H d_r) + \frac{1}{2} g_s \mathcal{C}_{dG}^{sr} (\Omega_d^\dagger D_{\bar{\mu}} \Omega_d) (\bar{q}_s D_{\bar{\mu}} H d_r) + \frac{1}{2} g_s \mathcal{C}_{dG}^{sr} (D_{\bar{\mu}} \Omega_{q,i}^* D_{\bar{\mu}} \Omega_q^j) H^i (\bar{q}_{js} d_r) \\
& + \frac{1}{2} g_s \mathcal{C}_{dG}^{sr} (\Omega_{q,i}^* D_{\bar{\mu}} \Omega_q^j) H^i (D^{\bar{\mu}} \bar{q}_{js} d_r) \\
& + \frac{1}{2} \left[ -\bar{y}_d^{rt} \mathcal{C}_{dG}^{st} - y_d^{st} \bar{\mathcal{C}}_{dG}^{rt} \right] \left[ T_b^{Aa} (\Omega_{d,a}^* D_{\bar{\nu}} \Omega_d^c) G^{\bar{\mu}\bar{\nu}A} (\bar{q}_{bs} \gamma^{\bar{\mu}} q_r^b) - T_c^{Ab} (D_{\bar{\mu}} \Omega_{d,a}^* \Omega_d^c) G^{\bar{\mu}\bar{\nu}A} (\bar{q}_{bs} \gamma^{\bar{\nu}} q_r^a) \right] \\
& + \frac{1}{2} \left[ \bar{y}_d^{rt} \mathcal{C}_{dG}^{st} - y_d^{st} \bar{\mathcal{C}}_{dG}^{rt} \right] \left[ T_c^{Ab} (D_{\bar{\mu}} \Omega_{d,a}^* \Omega_d^c) G^{\bar{\mu}\bar{\nu}A} (\bar{q}_{bs} \gamma^{\bar{\nu}} q_r^a) + T_b^{Aa} (\Omega_{d,a}^* D_{\bar{\nu}} \Omega_d^c) G^{\bar{\mu}\bar{\nu}A} (\bar{q}_{cs} \gamma^{\bar{\mu}} q_r^b) \right] \\
& - \frac{1}{6} g_s \bar{\mathcal{C}}_{dG}^{rs} (D_{\bar{\mu}} \Omega_{q,j}^* \Omega_q^i) H_i^\dagger (D^{\bar{\mu}} \bar{d}_s q_r^j) - \frac{1}{6} g_s \bar{\mathcal{C}}_{dG}^{rs} (D_{\bar{\mu}} \Omega_{q,aj}^* D_{\bar{\mu}} \Omega_q^{bi}) H_i^\dagger (\bar{d}_{bs} q_r^{aj}) \\
& - \frac{1}{6} g_s \bar{\mathcal{C}}_{dG}^{rs} (D_{\bar{\mu}} \Omega_{q,aj}^* \Omega_q^{bi}) H_i^\dagger (\bar{d}_{bs} D^{\bar{\mu}} q_r^{aj}) - \frac{1}{6} g_s \bar{\mathcal{C}}_{dG}^{rs} (D_{\bar{\mu}} \Omega_{d,a}^* D_{\bar{\mu}} \Omega_d^b) (\bar{d}_{bs} H^\dagger q_r^a) \\
& - \frac{1}{6} g_s \bar{\mathcal{C}}_{dG}^{rs} (D_{\bar{\mu}} \Omega_{d,a}^* \Omega_d^b) (\bar{d}_{bs} D_{\bar{\mu}} H^\dagger q_r^a) - \frac{1}{6} g_s \mathcal{C}_{dG}^{sr} (\Omega_{q,i}^* D_{\bar{\mu}} \Omega_q^j) H^i (\bar{q}_{js} D^{\bar{\mu}} d_r) - \frac{1}{6} g_s \mathcal{C}_{dG}^{sr} (D_{\bar{\mu}} \Omega_{d,a}^* D_{\bar{\mu}} \Omega_d^b) (\bar{q}_{bs} H d_r^a) \\
& - \frac{1}{6} g_s \mathcal{C}_{dG}^{sr} (\Omega_{d,a}^* D_{\bar{\mu}} \Omega_d^b) (\bar{q}_{bs} D_{\bar{\mu}} H d_r^a) - \frac{i}{3} g_s \bar{\mathcal{C}}_{dG}^{rs} (D_{\bar{\nu}} \Omega_{q,j}^* \Omega_q^i) D^{\bar{\mu}} H_i^\dagger (\bar{d}_s \sigma^{\bar{\mu}\bar{\nu}} q_r^j) \\
& - \frac{i}{3} g_s \bar{\mathcal{C}}_{dG}^{rs} (D_{\bar{\nu}} \Omega_d^\dagger \Omega_d) (\bar{d}_s \sigma^{\bar{\mu}\bar{\nu}} D_{\bar{\mu}} H^\dagger q_r) + \frac{i}{3} g_s \mathcal{C}_{dG}^{sr} (\Omega_{q,i}^* D_{\bar{\nu}} \Omega_q^j) D^{\bar{\mu}} H^i (\bar{q}_{js} \sigma^{\bar{\mu}\bar{\nu}} d_r) \\
& + \frac{1}{2} g_s \bar{\mathcal{C}}_{dG}^{rs} (D_{\bar{\mu}} \Omega_d^\dagger \Omega_d) (\bar{d}_s D_{\bar{\mu}} H^\dagger q_r) - \frac{1}{2} g_s \bar{\mathcal{C}}_{dG}^{rs} (D_{\bar{\mu}} \Omega_{q,j}^* \Omega_q^i) D^{\bar{\mu}} H_i^\dagger (\bar{d}_s q_r^j) \\
& - \frac{1}{2} g_s \bar{\mathcal{C}}_{dG}^{rs} (D_{\bar{\mu}} \Omega_d^\dagger \Omega_d) (D^{\bar{\mu}} \bar{d}_s H^\dagger q_r) - \frac{1}{2} g_s \mathcal{C}_{dG}^{sr} (\Omega_d^\dagger D_{\bar{\mu}} \Omega_d) (\bar{q}_s H D^{\bar{\mu}} d_r) - \frac{1}{2} g_s \mathcal{C}_{dG}^{sr} (\Omega_{q,i}^* D_{\bar{\mu}} \Omega_q^j) D^{\bar{\mu}} H^i (\bar{q}_{js} d_r) \\
& + \frac{2i}{3} \left[ \bar{y}_d^{rs} \mathcal{C}_{dG}^{rs} + y_d^{rs} \bar{\mathcal{C}}_{dG}^{rs} \right] \left[ T_b^{Aa} (\Omega_{q,aj}^* D_{\bar{\nu}} \Omega_q^{bi}) H_i^\dagger D^{\bar{\mu}} H^j G^{\bar{\mu}\bar{\nu}A} - T_b^{Aa} (D_{\bar{\nu}} \Omega_{q,aj}^* \Omega_q^{bi}) D^{\bar{\mu}} H_i^\dagger H^j G^{\bar{\mu}\bar{\nu}A} \right] \\
& - \frac{2i}{3} \left[ \bar{y}_d^{rs} \mathcal{C}_{dG}^{rs} - y_d^{rs} \bar{\mathcal{C}}_{dG}^{rs} \right] \left[ T_b^{Aa} (D_{\bar{\nu}} \Omega_{q,aj}^* \Omega_q^{bi}) D^{\bar{\mu}} H_i^\dagger H^j G^{\bar{\mu}\bar{\nu}A} + T_b^{Aa} (\Omega_{q,aj}^* D_{\bar{\nu}} \Omega_q^{bi}) H_i^\dagger D^{\bar{\mu}} H^j G^{\bar{\mu}\bar{\nu}A} \right] \\
& + \frac{2i}{3} \left[ \bar{y}_d^{rs} \mathcal{C}_{dG}^{rs} + y_d^{rs} \bar{\mathcal{C}}_{dG}^{rs} \right] \left[ T_b^{Aa} (\Omega_{d,a}^* D_{\bar{\nu}} \Omega_d^b) G^{\bar{\mu}\bar{\nu}A} (H^\dagger D_{\bar{\mu}} H) - T_b^{Aa} (D_{\bar{\nu}} \Omega_{d,a}^* \Omega_d^b) G^{\bar{\mu}\bar{\nu}A} (D_{\bar{\mu}} H^\dagger H) \right]
\end{aligned}$$

$$- \frac{2i}{3} \left[ \bar{y}_d^{rs} \mathcal{C}_{dG}^{rs} - y_d^{rs} \bar{\mathcal{C}}_{dG}^{rs} \right] \left[ T_b^{Aa} (\Omega_{d,a}^* D_{\bar{\nu}} \Omega_d^b) G^{\bar{\mu}\bar{\nu}A} (H^\dagger D_{\bar{\mu}} H) + T_b^{Aa} (D_{\bar{\nu}} \Omega_{d,a}^* \Omega_d^b) G^{\bar{\mu}\bar{\nu}A} (D_{\bar{\mu}} H^\dagger H) \right], \quad (3.28)$$

$$\begin{aligned} \Gamma_\Omega^{(1)} [\mathcal{O}_{He}] = & \frac{i}{24} \mathcal{C}_{He}^{tt} \left[ 3g_L^2 - g_Y^2 \right] (\Omega_e^\dagger \overset{\leftrightarrow}{D}_{\bar{\mu}} \Omega_e) (H^\dagger H) (\bar{q}_s \gamma^{\bar{\mu}} q_s) + \frac{i}{12} g_Y^2 \mathcal{C}_{He}^{tt} (\Omega_e^\dagger \overset{\leftrightarrow}{D}_{\bar{\mu}} \Omega_e) (H^\dagger H) (\bar{d}_s \gamma^{\bar{\mu}} d_s) \\ & - \frac{i}{12} \left[ 10g_Y^2 \mathcal{C}_{He}^{sr} - y_e^{tr} \bar{y}_e^{tu} \mathcal{C}_{He}^{su} - y_e^{tu} \bar{y}_e^{ts} \mathcal{C}_{He}^{ur} - 3g_Y^2 \mathcal{C}_{He}^{tt} \delta^{rs} \right] (\Omega_e^\dagger \overset{\leftrightarrow}{D}_{\bar{\mu}} \Omega_e) (H^\dagger H) (\bar{e}_s \gamma^{\bar{\mu}} e_r) \\ & + \frac{i}{8} \mathcal{C}_{He}^{tt} \left[ g_L^2 + g_Y^2 \right] (\Omega_e^\dagger \overset{\leftrightarrow}{D}_{\bar{\mu}} \Omega_e) (H^\dagger H) (\bar{\ell}_s \gamma^{\bar{\mu}} \ell_s) \\ & + \frac{i}{6} g_Y \mathcal{C}_{He}^{rr} \left[ (\Omega_e^\dagger D_{\bar{\nu}} \Omega_e) B^{\bar{\mu}\bar{\nu}} (H^\dagger D_{\bar{\mu}} H) - (D_{\bar{\nu}} \Omega_e^\dagger \Omega_e) B^{\bar{\mu}\bar{\nu}} (D_{\bar{\mu}} H^\dagger H) \right] - \frac{i}{6} g_Y^2 \mathcal{C}_{He}^{tt} (\Omega_e^\dagger \overset{\leftrightarrow}{D}_{\bar{\mu}} \Omega_e) (H^\dagger H) (\bar{u}_s \gamma^{\bar{\mu}} u_s) \\ & - \frac{i}{6} \left[ y_e^{tr} \bar{y}_e^{tu} \mathcal{C}_{He}^{su} + y_e^{tu} \bar{y}_e^{ts} \mathcal{C}_{He}^{ur} \right] (\Omega_{\ell,j}^* \overset{\leftrightarrow}{D}_{\bar{\mu}} \Omega_\ell^i) H_i^\dagger H^j (\bar{e}_s \gamma^{\bar{\mu}} e_r) \\ & - \frac{i}{4} g_L^2 \mathcal{C}_{He}^{tt} (\Omega_e^\dagger \overset{\leftrightarrow}{D}_{\bar{\mu}} \Omega_e) (\bar{\ell}_s H \gamma^{\bar{\mu}} H^\dagger \ell_s) - \frac{i}{4} g_L^2 \mathcal{C}_{He}^{tt} (\Omega_e^\dagger \overset{\leftrightarrow}{D}_{\bar{\mu}} \Omega_e) (\bar{q}_s H \gamma^{\bar{\mu}} H^\dagger q_s) \\ & + \frac{1}{3} \mathcal{C}_{He}^{rr} \left[ (D_{\bar{\mu}} D_2 \Omega_e^\dagger \Omega_e) (H^\dagger D_{\bar{\mu}} H) + (\Omega_e^\dagger D_{\bar{\mu}} D_2 \Omega_e) (D_{\bar{\mu}} H^\dagger H) \right] \\ & + \frac{1}{3} y_e^{rt} \bar{y}_e^{rs} \mathcal{C}_{He}^{ts} \left[ (\Omega_{\ell,k}^* D_{\bar{\mu}} \Omega_\ell^j) (H^\dagger D_{\bar{\mu}} H) H_j^\dagger H^k + (D_{\bar{\mu}} \Omega_{\ell,k}^* \Omega_\ell^j) (D_{\bar{\mu}} H^\dagger H) H_j^\dagger H^k \right] \\ & + \frac{2}{3} g_Y \mathcal{C}_{He}^{rr} \left[ 2(\Omega_e^\dagger D_{\bar{\sigma}} \Omega_e) \tilde{B}^{\bar{\mu}\bar{\sigma}} (H^\dagger D_{\bar{\mu}} H) + 2(D_{\bar{\nu}} \Omega_e^\dagger \Omega_e) \tilde{B}^{\bar{\mu}\bar{\nu}} (D_{\bar{\mu}} H^\dagger H) \right] + \frac{2}{3} y_e^{st} \mathcal{C}_{He}^{tr} (\Omega_e^\dagger D_{\bar{\mu}} \Omega_e) (\bar{\ell}_s D_{\bar{\mu}} H e_r) \\ & + \left[ \frac{1}{4} \mathcal{C}_{He}^{rr} \left[ g_L^2 + g_Y^2 \right] - \frac{4}{3} y_e^{rt} \bar{y}_e^{rs} \mathcal{C}_{He}^{ts} \right] \left[ (\Omega_e^\dagger D_{\bar{\mu}} \Omega_e) (H^\dagger H) (H^\dagger D_{\bar{\mu}} H) + (D_{\bar{\mu}} \Omega_e^\dagger \Omega_e) (H^\dagger H) (D_{\bar{\mu}} H^\dagger H) \right] \\ & - \frac{1}{6} \bar{y}_e^{rt} \mathcal{C}_{He}^{st} (D_{\bar{\mu}} \Omega_e^\dagger D_{\bar{\mu}} \Omega_e) (\bar{e}_s H^\dagger \ell_r) - \frac{1}{6} \bar{y}_e^{rt} \mathcal{C}_{He}^{st} (D_{\bar{\mu}} \Omega_e^\dagger \Omega_e) (D_{\bar{\mu}} \bar{e}_s H^\dagger \ell_r) \\ & - \frac{1}{6} y_e^{st} \mathcal{C}_{He}^{tr} (D_{\bar{\mu}} \Omega_e^\dagger D_{\bar{\mu}} \Omega_e) (\bar{\ell}_s H e_r) - \frac{1}{6} y_e^{st} \mathcal{C}_{He}^{tr} (\Omega_e^\dagger D_{\bar{\mu}} \Omega_e) (\bar{\ell}_s H D_{\bar{\mu}} e_r) - \frac{1}{6} y_e^{st} \mathcal{C}_{He}^{tr} (\Omega_e^\dagger D_{\bar{\mu}} \Omega_e) (D_{\bar{\mu}} \bar{\ell}_s H e_r) \\ & - \frac{1}{3} \mathcal{C}_{He}^{rr} (D_{\bar{\nu}} \Omega_e^\dagger D_{\bar{\nu}} \Omega_e) (D_{\bar{\mu}} H^\dagger D_{\bar{\mu}} H) - \frac{1}{3} \mathcal{C}_{He}^{rr} \left[ (D_{\bar{\mu}} \Omega_e^\dagger D_{\bar{\nu}} \Omega_e) (H^\dagger D_{\bar{\mu}} D_{\bar{\nu}} H) + (D_{\bar{\nu}} \Omega_e^\dagger D_{\bar{\mu}} \Omega_e) (D_{\bar{\mu}} D_{\bar{\nu}} H^\dagger H) \right] \\ & - \frac{i}{3} \mathcal{C}_{He}^{rr} \left[ (\Omega_e^\dagger D_{\bar{\sigma}} \Omega_e) (D_{\bar{\mu}} \Omega_e^\dagger D_{\bar{\rho}} \Omega_e) (H^\dagger D_{\bar{\nu}} H) \varepsilon^{\bar{\mu}\bar{\nu}\bar{\rho}\bar{\sigma}} + (D_{\bar{\nu}} \Omega_e^\dagger D_{\bar{\sigma}} \Omega_e) (D_{\bar{\rho}} \Omega_e^\dagger \Omega_e) (D_{\bar{\mu}} H^\dagger H) \varepsilon^{\bar{\mu}\bar{\nu}\bar{\rho}\bar{\sigma}} \right] \\ & + \frac{2}{3} \bar{y}_e^{rt} \mathcal{C}_{He}^{st} (D_{\bar{\mu}} \Omega_e^\dagger \Omega_e) (\bar{e}_s D_{\bar{\mu}} H^\dagger \ell_r) - \frac{1}{6} \bar{y}_e^{rt} \mathcal{C}_{He}^{st} (D_{\bar{\mu}} \Omega_e^\dagger \Omega_e) (\bar{e}_s H^\dagger D_{\bar{\mu}} \ell_r) \\ & - \frac{2}{3} \mathcal{C}_{He}^{rr} (D_{\bar{\mu}} \Omega_e^\dagger D_{\bar{\nu}} \Omega_e) (D_{\bar{\mu}} H^\dagger D_{\bar{\nu}} H) + \frac{5i}{6} \bar{y}_e^{rt} \mathcal{C}_{He}^{st} (D_{\bar{\nu}} \Omega_e^\dagger \Omega_e) (\bar{e}_s \sigma^{\bar{\mu}\bar{\nu}} D_{\bar{\mu}} H^\dagger \ell_r) \\ & - \frac{5i}{6} y_e^{st} \mathcal{C}_{He}^{tr} (\Omega_e^\dagger D_{\bar{\nu}} \Omega_e) (\bar{\ell}_s D_{\bar{\mu}} H \sigma^{\bar{\mu}\bar{\nu}} e_r) - \mathcal{C}_{He}^{rr} \left[ (\Omega_e^\dagger D_{\bar{\nu}} \Omega_e) (D_{\bar{\mu}} H^\dagger D_{\bar{\mu}} D_{\bar{\nu}} H) + (D_{\bar{\nu}} \Omega_e^\dagger \Omega_e) (D_{\bar{\mu}} D_{\bar{\nu}} H^\dagger D_{\bar{\mu}} H) \right] \\ & + i g_L \mathcal{C}_{He}^{rr} \left[ (\Omega_e^\dagger D_{\bar{\nu}} \Omega_e) W^{\bar{\mu}\bar{\nu}I} (H^\dagger t^I D_{\bar{\mu}} H) - (D_{\bar{\nu}} \Omega_e^\dagger \Omega_e) W^{\bar{\mu}\bar{\nu}I} (D_{\bar{\mu}} H^\dagger t^I H) \right], \quad (3.29) \end{aligned}$$

$$\begin{aligned} \Gamma_\Omega^{(1)} [\mathcal{O}_{H\ell}] = & - \frac{i}{24} \left[ g_L^2 + g_Y^2 \right] \left[ 10(\mathcal{C}_{H\ell}^{(1)})^{sr} - 3(\mathcal{C}_{H\ell}^{(1)})^{tt} \delta^{rs} \right] (\Omega_\ell^\dagger \overset{\leftrightarrow}{D}_{\bar{\mu}} \Omega_\ell) (H^\dagger H) (\bar{\ell}_s \gamma^{\bar{\mu}} \ell_r) \\ & - \frac{i}{24} (\mathcal{C}_{H\ell}^{(1)})^{tt} \left[ g_Y^2 + 3g_L^2 \right] (\Omega_\ell^\dagger \overset{\leftrightarrow}{D}_{\bar{\mu}} \Omega_\ell) (H^\dagger H) (\bar{q}_s \gamma^{\bar{\mu}} q_s) \\ & + \frac{1}{12} g_Y (\mathcal{C}_{H\ell}^{(1)})^{rr} \left[ 2(\Omega_\ell^\dagger D_{\bar{\rho}} \Omega_\ell) (\Omega_{\ell,j}^* D_{\bar{\sigma}} \Omega_\ell^i) H_i^\dagger H^j \tilde{B}^{\bar{\rho}\bar{\sigma}} - 2(D_{\bar{\nu}} \Omega_\ell^\dagger \Omega_\ell) (D_{\bar{\mu}} \Omega_{\ell,j}^* \Omega_\ell^i) H_i^\dagger H^j \tilde{B}^{\bar{\mu}\bar{\nu}} \right] \end{aligned}$$

$$\begin{aligned}
& -\frac{i}{12} \left[ y_e^{su} \bar{y}_e^{tu} (\mathcal{C}_{H\ell}^{(1)})^{tr} + y_e^{ut} \bar{y}_e^{rt} (\mathcal{C}_{H\ell}^{(1)})^{su} + 10g_Y^2 (\mathcal{C}_{H\ell}^{(1)})^{sr} \right] \left[ (\Omega_{\ell,j}^* D_{\bar{\mu}} \Omega_{\ell}^i) H_i^{\dagger} (\bar{\ell}_s H \gamma^{\bar{\mu}} \ell_r^j) - (D_{\bar{\mu}} \Omega_{\ell,j}^* \Omega_{\ell}^k) H^j (\bar{\ell}_{ks} \gamma^{\bar{\mu}} H^{\dagger} \ell_r) \right] \\
& -\frac{i}{12} \left[ y_e^{su} \bar{y}_e^{tu} (\mathcal{C}_{H\ell}^{(1)})^{tr} - y_e^{ut} \bar{y}_e^{rt} (\mathcal{C}_{H\ell}^{(1)})^{su} \right] \left[ (\Omega_{\ell,j}^* D_{\bar{\mu}} \Omega_{\ell}^i) H_i^{\dagger} (\bar{\ell}_s H \gamma^{\bar{\mu}} \ell_r^j) + (D_{\bar{\mu}} \Omega_{\ell,j}^* \Omega_{\ell}^k) H^j (\bar{\ell}_{ks} \gamma^{\bar{\mu}} H^{\dagger} \ell_r) \right] \\
& +\frac{i}{12} g_Y^2 (\mathcal{C}_{H\ell}^{(1)})^{tt} (\Omega_{\ell}^{\dagger} \overleftrightarrow{D}_{\bar{\mu}} \Omega_{\ell}) (H^{\dagger} H) (\bar{d}_s \gamma^{\bar{\mu}} d_s) \\
& +\frac{i}{12} \left[ 5(\mathcal{C}_{H\ell}^{(1)})^{sr} \left[ g_L^2 + g_Y^2 \right] - 3g_L^2 (\mathcal{C}_{H\ell}^{(1)})^{tt} \delta^{rs} \right] (\Omega_{\ell}^{\dagger} \overleftrightarrow{D}_{\bar{\mu}} \Omega_{\ell}) (\bar{\ell}_s H \gamma^{\bar{\mu}} H^{\dagger} \ell_r) \\
& +\frac{1}{6} g_Y (\mathcal{C}_{H\ell}^{(1)})^{rr} \left[ 2(D_{\bar{\nu}} \Omega_{\ell,j}^* \Omega_{\ell}^i) D_{\bar{\mu}} H_i^{\dagger} H^j \widetilde{B}^{\bar{\mu}\bar{\nu}} + 2(\Omega_{\ell,j}^* D_{\bar{\sigma}} \Omega_{\ell}^i) H_i^{\dagger} D_{\bar{\mu}} H^j \widetilde{B}^{\bar{\mu}\bar{\sigma}} \right] \\
& +\frac{1}{6} g_L (\mathcal{C}_{H\ell}^{(1)})^{rr} \left[ 2t_l^{Ij} (\Omega_{\ell}^{\dagger} D_{\bar{\rho}} \Omega_{\ell}) (\Omega_{\ell,j}^* D_{\bar{\sigma}} \Omega_{\ell}^i) H_i^{\dagger} H^l \widetilde{W}^{\bar{\rho}\bar{\sigma}I} - 2t_l^{Ii} (D_{\bar{\nu}} \Omega_{\ell}^{\dagger} \Omega_{\ell}) (D_{\bar{\mu}} \Omega_{\ell,j}^* \Omega_{\ell}^l) H_i^{\dagger} H^j \widetilde{W}^{\bar{\mu}\bar{\nu}I} \right] \\
& +\frac{1}{6} \bar{y}_e^{ts} (\mathcal{C}_{H\ell}^{(1)})^{tr} (D_{\bar{\mu}} \Omega_{\ell,j}^* D_{\bar{\mu}} \Omega_{\ell}^i) H_i^{\dagger} (\bar{e}_s \ell_r^j) + \frac{1}{6} y_e^{tr} (\mathcal{C}_{H\ell}^{(1)})^{st} (D_{\bar{\mu}} \Omega_{\ell,i}^* D_{\bar{\mu}} \Omega_{\ell}^j) H^i (\bar{\ell}_{js} e_r) \\
& +\frac{i}{6} \left[ y_e^{su} \bar{y}_e^{tu} (\mathcal{C}_{H\ell}^{(1)})^{tr} + y_e^{ut} \bar{y}_e^{rt} (\mathcal{C}_{H\ell}^{(1)})^{su} \right] (\Omega_e^{\dagger} \overleftrightarrow{D}_{\bar{\mu}} \Omega_e) (\bar{\ell}_s H \gamma^{\bar{\mu}} H^{\dagger} \ell_r) \\
& -\frac{i}{6} g_Y^2 (\mathcal{C}_{H\ell}^{(1)})^{tt} (\Omega_{\ell}^{\dagger} \overleftrightarrow{D}_{\bar{\mu}} \Omega_{\ell}) (H^{\dagger} H) (\bar{u}_s \gamma^{\bar{\mu}} u_s) \\
& +\frac{1}{4} (\mathcal{C}_{H\ell}^{(1)})^{rr} \left[ g_L^2 + g_Y^2 \right] \left[ (\Omega_{\ell}^{\dagger} D_{\bar{\mu}} \Omega_{\ell}) (H^{\dagger} H) (H^{\dagger} D_{\bar{\mu}} H) + (D_{\bar{\mu}} \Omega_{\ell}^{\dagger} \Omega_{\ell}) (H^{\dagger} H) (D_{\bar{\mu}} H^{\dagger} H) \right] \\
& +\frac{i}{4} g_Y^2 (\mathcal{C}_{H\ell}^{(1)})^{tt} (\Omega_{\ell}^{\dagger} \overleftrightarrow{D}_{\bar{\mu}} \Omega_{\ell}) (H^{\dagger} H) (\bar{e}_s \gamma^{\bar{\mu}} e_s) + \frac{i}{4} g_L^2 (\mathcal{C}_{H\ell}^{(1)})^{tt} (\Omega_{\ell,j}^* \overleftrightarrow{D}_{\bar{\mu}} \Omega_{\ell}^i) H_i^{\dagger} H^j (\bar{q}_s \gamma^{\bar{\mu}} q_s) \\
& +\frac{i}{4} g_L^2 (\mathcal{C}_{H\ell}^{(1)})^{tt} (\Omega_{\ell,j}^* \overleftrightarrow{D}_{\bar{\mu}} \Omega_{\ell}^k) (H^{\dagger} H) (\bar{q}_{ks} \gamma^{\bar{\mu}} q_s^j) \\
& +\frac{1}{3} g_L (\mathcal{C}_{H\ell}^{(1)})^{rr} \left[ 2t_k^{Ij} (D_{\bar{\nu}} \Omega_{\ell,j}^* \Omega_{\ell}^i) D_{\bar{\mu}} H_i^{\dagger} H^k \widetilde{W}^{\bar{\mu}\bar{\nu}I} + 2t_k^{Ii} (\Omega_{\ell,j}^* D_{\bar{\sigma}} \Omega_{\ell}^k) H_i^{\dagger} D_{\bar{\mu}} H^j \widetilde{W}^{\bar{\mu}\bar{\sigma}I} \right] \\
& +\frac{1}{3} (\mathcal{C}_{H\ell}^{(1)})^{rr} \left[ (D_{\bar{\mu}} D_2 \Omega_{\ell}^{\dagger} \Omega_{\ell}) (H^{\dagger} D_{\bar{\mu}} H) + (\Omega_{\ell}^{\dagger} D_{\bar{\mu}} D_2 \Omega_{\ell}) (D_{\bar{\mu}} H^{\dagger} H) \right] \\
& +\frac{1}{3} y_e^{ts} \bar{y}_e^{rs} (\mathcal{C}_{H\ell}^{(1)})^{rt} \left[ (\Omega_e^{\dagger} D_{\bar{\mu}} \Omega_e) (H^{\dagger} H) (H^{\dagger} D_{\bar{\mu}} H) + (D_{\bar{\mu}} \Omega_e^{\dagger} \Omega_e) (H^{\dagger} H) (D_{\bar{\mu}} H^{\dagger} H) \right] \\
& -\frac{1}{6} g_L (\mathcal{C}_{H\ell}^{(1)})^{rr} \left[ 2t_l^{Ii} (D_{\bar{\mu}} \Omega_{\ell,j}^* \Omega_{\ell}^k) (D_{\bar{\nu}} \Omega_{\ell,k}^* \Omega_{\ell}^l) H_i^{\dagger} H^j \widetilde{W}^{\bar{\mu}\bar{\nu}I} + 2t_l^{Ik} (\Omega_{\ell,j}^* D_{\bar{\rho}} \Omega_{\ell}^i) (\Omega_{\ell,k}^* D_{\bar{\sigma}} \Omega_{\ell}^j) H_i^{\dagger} H^l \widetilde{W}^{\bar{\rho}\bar{\sigma}I} \right] \\
& +\frac{i}{3} g_Y (\mathcal{C}_{H\ell}^{(1)})^{rr} \left[ (\Omega_{\ell}^{\dagger} D_{\bar{\nu}} \Omega_{\ell}) B^{\bar{\mu}\bar{\nu}} (H^{\dagger} D_{\bar{\mu}} H) - (D_{\bar{\nu}} \Omega_{\ell}^{\dagger} \Omega_{\ell}) B^{\bar{\mu}\bar{\nu}} (D_{\bar{\mu}} H^{\dagger} H) \right] \\
& +\frac{i}{3} g_L (\mathcal{C}_{H\ell}^{(1)})^{rr} \left[ t_k^{Ij} (\Omega_{\ell,j}^* D_{\bar{\nu}} \Omega_{\ell}^k) W^{\bar{\mu}\bar{\nu}I} (H^{\dagger} D_{\bar{\mu}} H) - t_k^{Ij} (D_{\bar{\nu}} \Omega_{\ell,j}^* \Omega_{\ell}^k) W^{\bar{\mu}\bar{\nu}I} (D_{\bar{\mu}} H^{\dagger} H) \right] \\
& +\frac{5i}{12} (\mathcal{C}_{H\ell}^{(1)})^{sr} \left[ g_L^2 + g_Y^2 \right] (\Omega_{\ell,j}^* \overleftrightarrow{D}_{\bar{\mu}} \Omega_{\ell}^i) H_i^{\dagger} H^j (\bar{\ell}_s \gamma^{\bar{\mu}} \ell_r) \\
& +\frac{1}{2} g_L (\mathcal{C}_{H\ell}^{(1)})^{rr} \left[ 2t_k^{Ij} (\Omega_{\ell,j}^* D_{\bar{\sigma}} \Omega_{\ell}^k) \widetilde{W}^{\bar{\mu}\bar{\sigma}I} (H^{\dagger} D_{\bar{\mu}} H) + 2t_k^{Ij} (D_{\bar{\nu}} \Omega_{\ell,j}^* \Omega_{\ell}^k) \widetilde{W}^{\bar{\mu}\bar{\nu}I} (D_{\bar{\mu}} H^{\dagger} H) \right] \\
& -\frac{1}{3} (\mathcal{C}_{H\ell}^{(1)})^{rr} (D_{\bar{\nu}} \Omega_{\ell}^{\dagger} D_{\bar{\nu}} \Omega_{\ell}) (D_{\bar{\mu}} H^{\dagger} D_{\bar{\mu}} H) \\
& -\frac{1}{3} (\mathcal{C}_{H\ell}^{(1)})^{rr} \left[ (D_{\bar{\mu}} \Omega_{\ell}^{\dagger} D_{\bar{\nu}} \Omega_{\ell}) (H^{\dagger} D_{\bar{\mu}} D_{\bar{\nu}} H) + (D_{\bar{\nu}} \Omega_{\ell}^{\dagger} D_{\bar{\mu}} \Omega_{\ell}) (D_{\bar{\mu}} D_{\bar{\nu}} H^{\dagger} H) \right] \\
& +\frac{i}{3} (\mathcal{C}_{H\ell}^{(1)})^{rr} \left[ (\Omega_{\ell}^{\dagger} D_{\bar{\rho}} \Omega_{\ell}) (\Omega_{\ell,j}^* D_{\bar{\sigma}} \Omega_{\ell}^i) D_{\bar{\mu}} H_i^{\dagger} D^{\bar{\nu}} H^j \varepsilon^{\bar{\mu}\bar{\nu}\bar{\rho}\bar{\sigma}} - (D_{\bar{\rho}} \Omega_{\ell}^{\dagger} \Omega_{\ell}) (D_{\bar{\nu}} \Omega_{\ell,j}^* \Omega_{\ell}^i) D_{\bar{\mu}} H_i^{\dagger} D^{\bar{\sigma}} H^j \varepsilon^{\bar{\mu}\bar{\nu}\bar{\rho}\bar{\sigma}} \right]
\end{aligned}$$

$$\begin{aligned}
& + \frac{i}{3}(\mathcal{C}_{H\ell}^{(1)})^{rr} \left[ (\Omega_\ell^\dagger D_{\bar{\sigma}} \Omega_\ell) (D_{\bar{\mu}} \Omega_\ell^\dagger D_{\bar{\rho}} \Omega_\ell) (H^\dagger D_{\bar{\nu}} H) \varepsilon^{\bar{\mu}\bar{\nu}\bar{\rho}\bar{\sigma}} - (D_{\bar{\nu}} \Omega_\ell^\dagger \Omega_\ell) (D_{\bar{\rho}} \Omega_\ell^\dagger D_{\bar{\sigma}} \Omega_\ell) (D_{\bar{\mu}} H^\dagger H) \varepsilon^{\bar{\mu}\bar{\nu}\bar{\rho}\bar{\sigma}} \right] \\
& - \frac{5}{12} g_Y (\mathcal{C}_{H\ell}^{(1)})^{rr} \left[ 2(\Omega_\ell^\dagger D_{\bar{\sigma}} \Omega_\ell) \tilde{B}^{\bar{\mu}\bar{\sigma}} (H^\dagger D_{\bar{\mu}} H) + 2(D_{\bar{\nu}} \Omega_\ell^\dagger \Omega_\ell) \tilde{B}^{\bar{\mu}\bar{\nu}} (D_{\bar{\mu}} H^\dagger H) \right] \\
& - \frac{i}{2} g_L^2 (\mathcal{C}_{H\ell}^{(1)})^{tt} \left[ (\Omega_{\ell,j}^* D_{\bar{\mu}} \Omega_\ell^i) H_i^\dagger (\bar{q}_s H \gamma^{\bar{\mu}} q_s^j) - (D_{\bar{\mu}} \Omega_{\ell,j}^* \Omega_\ell^k) H^j (\bar{q}_{ks} \gamma^{\bar{\mu}} H^\dagger q_s) \right] \\
& + \frac{2}{3} \bar{y}_e^{ts} (\mathcal{C}_{H\ell}^{(1)})^{tr} (D_{\bar{\mu}} \Omega_{\ell,j}^* \Omega_\ell^i) D_{\bar{\mu}} H_i^\dagger (\bar{e}_s \ell_r^j) + \frac{2}{3} y_e^{tr} (\mathcal{C}_{H\ell}^{(1)})^{st} (\Omega_{\ell,i}^* D_{\bar{\mu}} \Omega_\ell^j) D_{\bar{\mu}} H^i (\bar{\ell}_{js} e_r) \\
& - \frac{1}{6} \bar{y}_e^{ts} (\mathcal{C}_{H\ell}^{(1)})^{tr} (D_{\bar{\mu}} \Omega_{\ell,j}^* \Omega_\ell^i) H_i^\dagger (\bar{e}_s D_{\bar{\mu}} \ell_r^j) - \frac{1}{6} \bar{y}_e^{ts} (\mathcal{C}_{H\ell}^{(1)})^{tr} (D_{\bar{\mu}} \Omega_{\ell,j}^* \Omega_\ell^i) H_i^\dagger (D_{\bar{\mu}} \bar{e}_s \ell_r^j) \\
& - \frac{1}{6} y_e^{tr} (\mathcal{C}_{H\ell}^{(1)})^{st} (\Omega_{\ell,i}^* D_{\bar{\mu}} \Omega_\ell^j) H^i (\bar{\ell}_{js} D_{\bar{\mu}} e_r) - \frac{1}{6} y_e^{tr} (\mathcal{C}_{H\ell}^{(1)})^{st} (\Omega_{\ell,i}^* D_{\bar{\mu}} \Omega_\ell^j) H^i (D_{\bar{\mu}} \bar{\ell}_{js} e_r) \\
& - \frac{2}{3} (\mathcal{C}_{H\ell}^{(1)})^{rr} (D_{\bar{\mu}} \Omega_\ell^\dagger D_{\bar{\nu}} \Omega_\ell) (D_{\bar{\mu}} H^\dagger D_{\bar{\nu}} H) \\
& - \frac{2i}{3} (\mathcal{C}_{H\ell}^{(1)})^{rr} \left[ (D_{\bar{\rho}} \Omega_\ell^\dagger \Omega_\ell) (D_{\bar{\nu}} \Omega_{\ell,j}^* D_{\bar{\sigma}} \Omega_\ell^i) D_{\bar{\mu}} H_i^\dagger H^j \varepsilon^{\bar{\mu}\bar{\nu}\bar{\rho}\bar{\sigma}} + (\Omega_\ell^\dagger D_{\bar{\sigma}} \Omega_\ell) (D_{\bar{\mu}} \Omega_{\ell,j}^* D_{\bar{\rho}} \Omega_\ell^i) H_i^\dagger D_{\bar{\nu}} H^j \varepsilon^{\bar{\mu}\bar{\nu}\bar{\rho}\bar{\sigma}} \right] \\
& + \frac{2i}{3} (\mathcal{C}_{H\ell}^{(1)})^{rr} \left[ (D_{\bar{\mu}} \Omega_{\ell,j}^* D_{\bar{\rho}} \Omega_\ell^k) (\Omega_{\ell,k}^* D_{\bar{\sigma}} \Omega_\ell^i) H_i^\dagger D_{\bar{\nu}} H^j \varepsilon^{\bar{\mu}\bar{\nu}\bar{\rho}\bar{\sigma}} - (D_{\bar{\nu}} \Omega_{\ell,j}^* \Omega_\ell^k) (D_{\bar{\rho}} \Omega_{\ell,k}^* D_{\bar{\sigma}} \Omega_\ell^i) D_{\bar{\mu}} H_i^\dagger H^j \varepsilon^{\bar{\mu}\bar{\nu}\bar{\rho}\bar{\sigma}} \right] \\
& - \frac{5i}{6} \bar{y}_e^{ts} (\mathcal{C}_{H\ell}^{(1)})^{tr} (D_{\bar{\nu}} \Omega_{\ell,j}^* \Omega_\ell^i) D_{\bar{\mu}} H_i^\dagger (\bar{e}_s \sigma^{\bar{\mu}\bar{\nu}} \ell_r^j) + \frac{5i}{6} y_e^{tr} (\mathcal{C}_{H\ell}^{(1)})^{st} (\Omega_{\ell,i}^* D_{\bar{\nu}} \Omega_\ell^j) D_{\bar{\mu}} H^i (\bar{\ell}_{js} \sigma^{\bar{\mu}\bar{\nu}} e_r) \\
& - (\mathcal{C}_{H\ell}^{(1)})^{rr} \left[ (\Omega_\ell^\dagger D_{\bar{\nu}} \Omega_\ell) (D_{\bar{\mu}} H^\dagger D_{\bar{\mu}} D_{\bar{\nu}} H) + (D_{\bar{\nu}} \Omega_\ell^\dagger \Omega_\ell) (D_{\bar{\mu}} D_{\bar{\nu}} H^\dagger D_{\bar{\mu}} H) \right] \\
& + i g_L (\mathcal{C}_{H\ell}^{(1)})^{rr} \left[ (\Omega_\ell^\dagger D_{\bar{\nu}} \Omega_\ell) W^{\bar{\mu}\bar{\nu}I} (H^\dagger t^I D_{\bar{\mu}} H) - (D_{\bar{\nu}} \Omega_\ell^\dagger \Omega_\ell) W^{\bar{\mu}\bar{\nu}I} (D_{\bar{\mu}} H^\dagger t^I H) \right] \\
& - \frac{4}{3} y_e^{ts} \bar{y}_e^{rs} (\mathcal{C}_{H\ell}^{(1)})^{rt} \left[ (\Omega_{\ell,k}^* D_{\bar{\mu}} \Omega_\ell^j) (H^\dagger D_{\bar{\mu}} H) H_j^\dagger H^k + (D_{\bar{\mu}} \Omega_{\ell,k}^* \Omega_\ell^j) (D_{\bar{\mu}} H^\dagger H) H_j^\dagger H^k \right], \tag{3.30}
\end{aligned}$$

$$\begin{aligned}
\Gamma_\Omega^{(1)} [\mathcal{O}_{H\ell}^{(3)}] &= \frac{i}{24} \left[ g_L^2 + g_Y^2 \right] \left[ 10(\mathcal{C}_{H\ell}^{(3)})^{sr} - 3(\mathcal{C}_{H\ell}^{(3)})^{tt} \delta^{rs} \right] (\Omega_\ell^\dagger \overset{\leftrightarrow}{D}_{\bar{\mu}} \Omega_\ell) (H^\dagger H) (\bar{\ell}_s \gamma^{\bar{\mu}} \ell_r) \\
& + \frac{i}{24} (\mathcal{C}_{H\ell}^{(3)})^{tt} \left[ g_Y^2 + 3g_L^2 \right] (\Omega_\ell^\dagger \overset{\leftrightarrow}{D}_{\bar{\mu}} \Omega_\ell) (H^\dagger H) (\bar{q}_s \gamma^{\bar{\mu}} q_s) \\
& - \frac{i}{12} \left[ 6g_L^2 (\mathcal{C}_{H\ell}^{(3)})^{tt} \delta^{rs} + 10g_L^2 (\mathcal{C}_{H\ell}^{(3)})^{sr} - y_e^{su} \bar{y}_e^{tu} (\mathcal{C}_{H\ell}^{(3)})^{tr} - y_e^{ut} \bar{y}_e^{rt} (\mathcal{C}_{H\ell}^{(3)})^{su} \right] \\
& \quad \left[ (\Omega_{\ell,j}^* D_{\bar{\mu}} \Omega_\ell^i) H_i^\dagger (\bar{\ell}_s H \gamma^{\bar{\mu}} \ell_r^j) - (D_{\bar{\mu}} \Omega_{\ell,j}^* \Omega_\ell^k) H^j (\bar{\ell}_{ks} \gamma^{\bar{\mu}} H^\dagger \ell_r) \right] \\
& + \frac{i}{12} \left[ y_e^{su} \bar{y}_e^{tu} (\mathcal{C}_{H\ell}^{(3)})^{tr} - y_e^{ut} \bar{y}_e^{rt} (\mathcal{C}_{H\ell}^{(3)})^{su} \right] \left[ (\Omega_{\ell,j}^* D_{\bar{\mu}} \Omega_\ell^i) H_i^\dagger (\bar{\ell}_s H \gamma^{\bar{\mu}} \ell_r^j) + (D_{\bar{\mu}} \Omega_{\ell,j}^* \Omega_\ell^k) H^j (\bar{\ell}_{ks} \gamma^{\bar{\mu}} H^\dagger \ell_r) \right] \\
& - \frac{i}{12} g_Y^2 (\mathcal{C}_{H\ell}^{(3)})^{tt} (\Omega_\ell^\dagger \overset{\leftrightarrow}{D}_{\bar{\mu}} \Omega_\ell) (H^\dagger H) (\bar{d}_s \gamma^{\bar{\mu}} d_s) \\
& + \frac{i}{12} \left[ 3g_L^2 (\mathcal{C}_{H\ell}^{(3)})^{tt} \delta^{rs} + 5(\mathcal{C}_{H\ell}^{(3)})^{sr} \left[ g_L^2 - g_Y^2 \right] \right] (\Omega_\ell^\dagger \overset{\leftrightarrow}{D}_{\bar{\mu}} \Omega_\ell) (\bar{\ell}_s H \gamma^{\bar{\mu}} H^\dagger \ell_r) \\
& + \frac{i}{12} \left[ 3g_L^2 (\mathcal{C}_{H\ell}^{(3)})^{tt} \delta^{rs} + 3g_Y^2 (\mathcal{C}_{H\ell}^{(3)})^{tt} \delta^{rs} + 5(\mathcal{C}_{H\ell}^{(3)})^{sr} \left[ g_L^2 - g_Y^2 \right] - 2y_e^{su} \bar{y}_e^{tu} (\mathcal{C}_{H\ell}^{(3)})^{tr} - 2y_e^{ut} \bar{y}_e^{rt} (\mathcal{C}_{H\ell}^{(3)})^{su} \right] \\
& \quad (\Omega_{\ell,j}^* \overset{\leftrightarrow}{D}_{\bar{\mu}} \Omega_\ell^i) H_i^\dagger H^j (\bar{\ell}_s \gamma^{\bar{\mu}} \ell_r) \\
& - \frac{i}{12} g_Y^2 (\mathcal{C}_{H\ell}^{(3)})^{tt} (\Omega_{\ell,j}^* \overset{\leftrightarrow}{D}_{\bar{\mu}} \Omega_\ell^i) H_i^\dagger H^j (\bar{q}_s \gamma^{\bar{\mu}} q_s) \tag{3.31}
\end{aligned}$$

$$\begin{aligned}
& + \frac{1}{6} \left[ 3g_L^2 (\mathcal{C}_{H\ell}^{(3)})^{rr} - 8y_e^{ts} \bar{y}_e^{rs} (\mathcal{C}_{H\ell}^{(3)})^{rt} \right] \left[ (D_{\bar{\mu}} \Omega_{\ell,k}^* \Omega_{\ell}^j) (H^\dagger H) D^{\bar{\mu}} H_j^\dagger H^k + (\Omega_{\ell,k}^* D_{\bar{\mu}} \Omega_{\ell}^j) (H^\dagger H) H_j^\dagger D^{\bar{\mu}} H^k \right] \\
& + \frac{1}{6} \bar{y}_e^{ts} (\mathcal{C}_{H\ell}^{(3)})^{tr} (D_{\bar{\mu}} \Omega_{\ell,j}^* \Omega_{\ell}^i) H_i^\dagger (\bar{e}_s D^{\bar{\mu}} \ell_r^j) + \frac{1}{6} \bar{y}_e^{ts} (\mathcal{C}_{H\ell}^{(3)})^{tr} (D_{\bar{\mu}} \Omega_{\ell,j}^* \Omega_{\ell}^i) H_i^\dagger (D^{\bar{\mu}} \bar{e}_s \ell_r^j) \\
& + \frac{1}{6} y_e^{tr} (\mathcal{C}_{H\ell}^{(3)})^{st} (\Omega_{\ell,i}^* D_{\bar{\mu}} \Omega_{\ell}^j) H^i (\bar{\ell}_{js} D^{\bar{\mu}} e_r) + \frac{1}{6} y_e^{tr} (\mathcal{C}_{H\ell}^{(3)})^{st} (\Omega_{\ell,i}^* D_{\bar{\mu}} \Omega_{\ell}^j) H^i (D^{\bar{\mu}} \bar{\ell}_{js} e_r) \\
& - \frac{i}{6} \left[ y_e^{su} \bar{y}_e^{tu} (\mathcal{C}_{H\ell}^{(3)})^{tr} + y_e^{ut} \bar{y}_e^{rt} (\mathcal{C}_{H\ell}^{(3)})^{su} \right] (\Omega_{\ell}^\dagger \overleftrightarrow{D}_{\bar{\mu}} \Omega_e) (\bar{\ell}_s H \gamma^{\bar{\mu}} H^\dagger \ell_r) \\
& + \frac{i}{6} g_Y^2 (\mathcal{C}_{H\ell}^{(3)})^{tt} (\Omega_{\ell}^\dagger \overleftrightarrow{D}_{\bar{\mu}} \Omega_{\ell}) (H^\dagger H) (\bar{u}_s \gamma^{\bar{\mu}} u_s) + \frac{i}{6} g_Y^2 (\mathcal{C}_{H\ell}^{(3)})^{tt} (\Omega_{\ell,j}^* \overleftrightarrow{D}_{\bar{\mu}} \Omega_{\ell}^i) H_i^\dagger H^j (\bar{d}_s \gamma^{\bar{\mu}} d_s) \\
& - \frac{i}{4} g_Y^2 (\mathcal{C}_{H\ell}^{(3)})^{tt} (\Omega_{\ell}^\dagger \overleftrightarrow{D}_{\bar{\mu}} \Omega_{\ell}) (H^\dagger H) (\bar{e}_s \gamma^{\bar{\mu}} e_s) - \frac{i}{4} g_L^2 (\mathcal{C}_{H\ell}^{(3)})^{tt} (\Omega_{\ell,j}^* \overleftrightarrow{D}_{\bar{\mu}} \Omega_{\ell}^k) (H^\dagger H) (\bar{q}_{ks} \gamma^{\bar{\mu}} q_s^j) \\
& + \frac{1}{3} (\mathcal{C}_{H\ell}^{(3)})^{rr} (D_{\bar{\nu}} \Omega_{\ell}^\dagger D_{\bar{\nu}} \Omega_{\ell}) (D_{\bar{\mu}} H^\dagger D_{\bar{\mu}} H) \\
& + \frac{1}{3} (\mathcal{C}_{H\ell}^{(3)})^{rr} \left[ (D_{\bar{\mu}} \Omega_{\ell}^\dagger D_{\bar{\nu}} \Omega_{\ell}) (H^\dagger D_{\bar{\mu}} D_{\bar{\nu}} H) + (D_{\bar{\nu}} \Omega_{\ell}^\dagger D_{\bar{\mu}} \Omega_{\ell}) (D_{\bar{\mu}} D_{\bar{\nu}} H^\dagger H) \right] \\
& + \frac{1}{3} \bar{y}_e^{ts} (\mathcal{C}_{H\ell}^{(3)})^{tr} (D_{\bar{\mu}} \Omega_{\ell}^\dagger D_{\bar{\mu}} \Omega_{\ell}) (\bar{e}_s H^\dagger \ell_r) + \frac{1}{3} y_e^{tr} (\mathcal{C}_{H\ell}^{(3)})^{st} (D_{\bar{\mu}} \Omega_{\ell}^\dagger D_{\bar{\mu}} \Omega_{\ell}) (\bar{\ell}_s H e_r) \\
& + \frac{i}{3} \left[ y_e^{su} \bar{y}_e^{tu} (\mathcal{C}_{H\ell}^{(3)})^{tr} + y_e^{ut} \bar{y}_e^{rt} (\mathcal{C}_{H\ell}^{(3)})^{su} \right] (\Omega_{\ell}^\dagger \overleftrightarrow{D}_{\bar{\mu}} \Omega_e) (H^\dagger H) (\bar{\ell}_s \gamma^{\bar{\mu}} \ell_r) \\
& - \frac{i}{3} g_Y^2 (\mathcal{C}_{H\ell}^{(3)})^{tt} (\Omega_{\ell,j}^* \overleftrightarrow{D}_{\bar{\mu}} \Omega_{\ell}^i) H_i^\dagger H^j (\bar{u}_s \gamma^{\bar{\mu}} u_s) + \frac{i}{2} g_Y^2 (\mathcal{C}_{H\ell}^{(3)})^{tt} (\Omega_{\ell,j}^* \overleftrightarrow{D}_{\bar{\mu}} \Omega_{\ell}^i) H_i^\dagger H^j (\bar{e}_s \gamma^{\bar{\mu}} e_s) \\
& + \frac{2}{3} (\mathcal{C}_{H\ell}^{(3)})^{rr} (D_{\bar{\nu}} \Omega_{\ell,j}^* \Omega_{\ell}^k) (\Omega_{\ell,k}^* D_{\bar{\nu}} \Omega_{\ell}^i) D^{\bar{\mu}} H_i^\dagger D^{\bar{\mu}} H^j \\
& + \frac{2}{3} (\mathcal{C}_{H\ell}^{(3)})^{rr} \left[ (\Omega_{\ell,j}^* D_{\bar{\mu}} D_2 \Omega_{\ell}^i) D^{\bar{\mu}} H_i^\dagger H^j + (D_{\bar{\mu}} D_2 \Omega_{\ell,j}^* \Omega_{\ell}^i) H_i^\dagger D^{\bar{\mu}} H^j \right] \\
& + \frac{2}{3} (\mathcal{C}_{H\ell}^{(3)})^{rr} \left[ (D_{\bar{\nu}} \Omega_{\ell,j}^* \Omega_{\ell}^k) (D_{\bar{\mu}} \Omega_{\ell,k}^* D_{\bar{\nu}} \Omega_{\ell}^i) D^{\bar{\mu}} H_i^\dagger H^j + (D_{\bar{\mu}} \Omega_{\ell,j}^* D_{\bar{\nu}} \Omega_{\ell}^k) (\Omega_{\ell,k}^* D_{\bar{\mu}} \Omega_{\ell}^i) H_i^\dagger D^{\bar{\nu}} H^j \right] \\
& + \frac{2}{3} (\mathcal{C}_{H\ell}^{(3)})^{rr} \left[ (D_{\bar{\mu}} \Omega_{\ell,j}^* \Omega_{\ell}^k) (D_{\bar{\nu}} \Omega_{\ell,k}^* \Omega_{\ell}^i) D^{\bar{\mu}} D^{\bar{\nu}} H_i^\dagger H^j + (\Omega_{\ell,j}^* D_{\bar{\nu}} \Omega_{\ell}^k) (\Omega_{\ell,k}^* D_{\bar{\mu}} \Omega_{\ell}^i) H_i^\dagger D^{\bar{\mu}} D^{\bar{\nu}} H^j \right] \\
& + \frac{2}{3} (\mathcal{C}_{H\ell}^{(3)})^{rr} (D_{\bar{\mu}} \Omega_{\ell}^\dagger D_{\bar{\nu}} \Omega_{\ell}) (D_{\bar{\mu}} H^\dagger D_{\bar{\nu}} H) \\
& - \frac{1}{12} g_Y (\mathcal{C}_{H\ell}^{(3)})^{rr} \left[ 2(\Omega_{\ell}^\dagger D_{\bar{\rho}} \Omega_{\ell}) (\Omega_{\ell,j}^* D_{\bar{\sigma}} \Omega_{\ell}^i) H_i^\dagger H^j \widetilde{B}^{\bar{\rho}\bar{\sigma}} - 2(D_{\bar{\nu}} \Omega_{\ell}^\dagger \Omega_{\ell}) (D_{\bar{\mu}} \Omega_{\ell,j}^* \Omega_{\ell}^i) H_i^\dagger H^j \widetilde{B}^{\bar{\mu}\bar{\nu}} \right] \\
& - \frac{1}{6} g_L (\mathcal{C}_{H\ell}^{(3)})^{rr} \left[ 2t_l^{Ij} (\Omega_{\ell}^\dagger D_{\bar{\rho}} \Omega_{\ell}) (\Omega_{\ell,j}^* D_{\bar{\sigma}} \Omega_{\ell}^i) H_i^\dagger H^l \widetilde{W}^{\bar{\rho}\bar{\sigma}I} - 2t_l^{Ii} (D_{\bar{\nu}} \Omega_{\ell}^\dagger \Omega_{\ell}) (D_{\bar{\mu}} \Omega_{\ell,j}^* \Omega_{\ell}^l) H_i^\dagger H^j \widetilde{W}^{\bar{\mu}\bar{\nu}I} \right] \\
& - \frac{1}{4} (\mathcal{C}_{H\ell}^{(3)})^{rr} \left[ g_L^2 + g_Y^2 \right] \left[ (\Omega_{\ell}^\dagger D_{\bar{\mu}} \Omega_{\ell}) (H^\dagger H) (H^\dagger D_{\bar{\mu}} H) + (D_{\bar{\mu}} \Omega_{\ell}^\dagger \Omega_{\ell}) (H^\dagger H) (D_{\bar{\mu}} H^\dagger H) \right] \\
& - \frac{i}{3} g_Y (\mathcal{C}_{H\ell}^{(3)})^{rr} (\Omega_{\ell,j}^* D_{\bar{\nu}} \Omega_{\ell}^k) (D_{\bar{\mu}} \Omega_{\ell,k}^* \Omega_{\ell}^i) H_i^\dagger H^j B^{\bar{\mu}\bar{\nu}} \\
& + \frac{i}{3} g_Y (\mathcal{C}_{H\ell}^{(3)})^{rr} \left[ (\Omega_{\ell,j}^* D_{\bar{\nu}} \Omega_{\ell}^i) H_i^\dagger D^{\bar{\mu}} H^j B^{\bar{\mu}\bar{\nu}} - (D_{\bar{\nu}} \Omega_{\ell,j}^* \Omega_{\ell}^i) D^{\bar{\mu}} H_i^\dagger H^j B^{\bar{\mu}\bar{\nu}} \right] \\
& - \frac{i}{3} g_L (\mathcal{C}_{H\ell}^{(3)})^{rr} t_l^{Ik} (D_{\bar{\mu}} \Omega_{\ell,j}^* \Omega_{\ell}^l) (\Omega_{\ell,k}^* D_{\bar{\nu}} \Omega_{\ell}^j) W^{\bar{\mu}\bar{\nu}I} (H^\dagger H) \\
& - \frac{1}{3} (\mathcal{C}_{H\ell}^{(3)})^{rr} \left[ (D_{\bar{\mu}} D_2 \Omega_{\ell}^\dagger \Omega_{\ell}) (H^\dagger D_{\bar{\mu}} H) + (\Omega_{\ell}^\dagger D_{\bar{\mu}} D_2 \Omega_{\ell}) (D_{\bar{\mu}} H^\dagger H) \right]
\end{aligned}$$

$$\begin{aligned}
& -\frac{i}{3}g_Y(\mathcal{C}_{H\ell}^{(3)})^{rr}\left[(\Omega_\ell^\dagger D_{\bar{\nu}}\Omega_\ell)B^{\bar{\mu}\bar{\nu}}(H^\dagger D_{\bar{\mu}}H) - (D_{\bar{\nu}}\Omega_\ell^\dagger\Omega_\ell)B^{\bar{\mu}\bar{\nu}}(D_{\bar{\mu}}H^\dagger H)\right] \\
& +\frac{1}{3}y_e^{ts}\bar{y}_e^{rs}(\mathcal{C}_{H\ell}^{(3)})^{rt}\left[(\Omega_e^\dagger D_{\bar{\mu}}\Omega_e)(H^\dagger H)(H^\dagger D_{\bar{\mu}}H) + (D_{\bar{\mu}}\Omega_e^\dagger\Omega_e)(H^\dagger H)(D_{\bar{\mu}}H^\dagger H)\right] \\
& -\frac{i}{3}(\mathcal{C}_{H\ell}^{(3)})^{rr}\left[(\Omega_\ell^\dagger D_{\bar{\rho}}\Omega_\ell)(\Omega_{\ell,j}^* D_{\bar{\sigma}}\Omega_\ell^i)D^{\bar{\mu}}H_i^\dagger D^{\bar{\nu}}H^j\varepsilon^{\bar{\mu}\bar{\nu}\bar{\rho}\bar{\sigma}} - (D_{\bar{\rho}}\Omega_\ell^\dagger\Omega_\ell)(D_{\bar{\nu}}\Omega_{\ell,j}^*\Omega_\ell^i)D^{\bar{\mu}}H_i^\dagger D^{\bar{\sigma}}H^j\varepsilon^{\bar{\mu}\bar{\nu}\bar{\rho}\bar{\sigma}}\right] \\
& -\frac{i}{3}(\mathcal{C}_{H\ell}^{(3)})^{rr}\left[(\Omega_\ell^\dagger D_{\bar{\sigma}}\Omega_\ell)(D_{\bar{\mu}}\Omega_\ell^\dagger D_{\bar{\rho}}\Omega_\ell)(H^\dagger D_{\bar{\nu}}H)\varepsilon^{\bar{\mu}\bar{\nu}\bar{\rho}\bar{\sigma}} - (D_{\bar{\nu}}\Omega_\ell^\dagger\Omega_\ell)(D_{\bar{\rho}}\Omega_\ell^\dagger D_{\bar{\sigma}}\Omega_\ell)(D_{\bar{\mu}}H^\dagger H)\varepsilon^{\bar{\mu}\bar{\nu}\bar{\rho}\bar{\sigma}}\right] \\
& +\frac{5}{12}g_Y(\mathcal{C}_{H\ell}^{(3)})^{rr}\left[2(\Omega_\ell^\dagger D_{\bar{\sigma}}\Omega_\ell)\tilde{B}^{\bar{\mu}\bar{\sigma}}(H^\dagger D_{\bar{\mu}}H) + 2(D_{\bar{\nu}}\Omega_\ell^\dagger\Omega_\ell)\tilde{B}^{\bar{\mu}\bar{\nu}}(D_{\bar{\mu}}H^\dagger H)\right] \\
& +\frac{1}{2}g_Y^2(\mathcal{C}_{H\ell}^{(3)})^{rr}\left[(\Omega_{\ell,k}^* D_{\bar{\mu}}\Omega_\ell^j)(H^\dagger D_{\bar{\mu}}H)H_j^\dagger H^k + (D_{\bar{\mu}}\Omega_{\ell,k}^*\Omega_\ell^j)(D_{\bar{\mu}}H^\dagger H)H_j^\dagger H^k\right] \\
& +\frac{1}{2}g_L(\mathcal{C}_{H\ell}^{(3)})^{rr}\left[2(\Omega_\ell^\dagger D_{\bar{\sigma}}\Omega_\ell)\tilde{W}^{\bar{\mu}\bar{\sigma}I}(H^\dagger t^I D_{\bar{\mu}}H) + 2(D_{\bar{\nu}}\Omega_\ell^\dagger\Omega_\ell)\tilde{W}^{\bar{\mu}\bar{\nu}I}(D_{\bar{\mu}}H^\dagger t^I H)\right] \\
& -\frac{2}{3}(\mathcal{C}_{H\ell}^{(3)})^{rr}(D_{\bar{\nu}}\Omega_{\ell,j}^* D_{\bar{\nu}}\Omega_\ell^i)D^{\bar{\mu}}H_i^\dagger D^{\bar{\mu}}H^j \\
& -\frac{2}{3}(\mathcal{C}_{H\ell}^{(3)})^{rr}\left[(D_{\bar{\nu}}\Omega_{\ell,j}^*\Omega_\ell^k)(D_{\bar{\nu}}\Omega_{\ell,k}^* D_{\bar{\mu}}\Omega_\ell^i)D^{\bar{\mu}}H_i^\dagger H^j + (D_{\bar{\mu}}\Omega_{\ell,j}^* D_{\bar{\nu}}\Omega_\ell^k)(\Omega_{\ell,k}^* D_{\bar{\nu}}\Omega_\ell^i)H_i^\dagger D^{\bar{\mu}}H^j\right] \\
& -\frac{2}{3}(\mathcal{C}_{H\ell}^{(3)})^{rr}(D_{\bar{\mu}}\Omega_{\ell,j}^*\Omega_\ell^k)(\Omega_{\ell,k}^* D_{\bar{\nu}}\Omega_\ell^i)D^{\bar{\mu}}H_i^\dagger D^{\bar{\nu}}H^j - \frac{2}{3}(\mathcal{C}_{H\ell}^{(3)})^{rr}(\Omega_{\ell,j}^* D_{\bar{\nu}}\Omega_\ell^k)(D_{\bar{\mu}}\Omega_{\ell,k}^*\Omega_\ell^i)D^{\bar{\mu}}H_i^\dagger D^{\bar{\nu}}H^j \\
& -\frac{2}{3}(\mathcal{C}_{H\ell}^{(3)})^{rr}\left[(D_{\bar{\mu}}\Omega_{\ell,j}^*\Omega_\ell^k)(\Omega_{\ell,k}^* D_{\bar{2}}\Omega_\ell^i)D^{\bar{\mu}}H_i^\dagger H^j + (D_{\bar{2}}\Omega_{\ell,j}^*\Omega_\ell^k)(\Omega_{\ell,k}^* D_{\bar{\nu}}\Omega_\ell^i)H_i^\dagger D^{\bar{\nu}}H^j\right] \\
& -\frac{2}{3}(\mathcal{C}_{H\ell}^{(3)})^{rr}\left[(D_{\bar{\mu}}\Omega_{\ell,j}^*\Omega_\ell^k)(D_{\bar{\nu}}\Omega_{\ell,k}^* D_{\bar{\nu}}\Omega_\ell^i)D^{\bar{\mu}}H_i^\dagger H^j + (D_{\bar{\mu}}\Omega_{\ell,j}^* D_{\bar{\mu}}\Omega_\ell^k)(\Omega_{\ell,k}^* D_{\bar{\nu}}\Omega_\ell^i)H_i^\dagger D^{\bar{\nu}}H^j\right] \\
& -\frac{2}{3}(\mathcal{C}_{H\ell}^{(3)})^{rr}\left[(D_{\bar{\nu}}\Omega_{\ell,j}^* D_{\bar{\mu}}\Omega_\ell^i)D^{\bar{\mu}}D^{\bar{\nu}}H_i^\dagger H^j + (D_{\bar{\mu}}\Omega_{\ell,j}^* D_{\bar{\nu}}\Omega_\ell^i)H_i^\dagger D^{\bar{\mu}}D^{\bar{\nu}}H^j\right] \\
& +\frac{2i}{3}g_L(\mathcal{C}_{H\ell}^{(3)})^{rr}\left[t_k^{Ij}(\Omega_{\ell,j}^* D_{\bar{\nu}}\Omega_\ell^k)W^{\bar{\mu}\bar{\nu}I}(H^\dagger D_{\bar{\mu}}H) - t_k^{Ij}(D_{\bar{\nu}}\Omega_{\ell,j}^*\Omega_\ell^k)W^{\bar{\mu}\bar{\nu}I}(D_{\bar{\mu}}H^\dagger H)\right] \\
& +\frac{2i}{3}(\mathcal{C}_{H\ell}^{(3)})^{rr}\left[(D_{\bar{\rho}}\Omega_\ell^\dagger\Omega_\ell)(D_{\bar{\nu}}\Omega_{\ell,j}^* D_{\bar{\sigma}}\Omega_\ell^i)D^{\bar{\mu}}H_i^\dagger H^j\varepsilon^{\bar{\mu}\bar{\nu}\bar{\rho}\bar{\sigma}} + (\Omega_\ell^\dagger D_{\bar{\sigma}}\Omega_\ell)(D_{\bar{\mu}}\Omega_{\ell,j}^* D_{\bar{\rho}}\Omega_\ell^i)H_i^\dagger D^{\bar{\nu}}H^j\varepsilon^{\bar{\mu}\bar{\nu}\bar{\rho}\bar{\sigma}}\right] \\
& -\frac{5i}{6}y_e^{tr}(\mathcal{C}_{H\ell}^{(3)})^{st}(\Omega_{\ell,i}^* D_{\bar{\nu}}\Omega_\ell^j)D^{\bar{\mu}}H^i(\bar{\ell}_{js}\sigma^{\bar{\mu}\bar{\nu}}e_r) \\
& +(\mathcal{C}_{H\ell}^{(3)})^{rr}\left[(\Omega_\ell^\dagger D_{\bar{\nu}}\Omega_\ell)(D_{\bar{\mu}}H^\dagger D_{\bar{\mu}}D_{\bar{\nu}}H) + (D_{\bar{\nu}}\Omega_\ell^\dagger\Omega_\ell)(D_{\bar{\mu}}D_{\bar{\nu}}H^\dagger D_{\bar{\mu}}H)\right] + \frac{4}{3}y_e^{tr}(\mathcal{C}_{H\ell}^{(3)})^{st}(\Omega_\ell^\dagger D_{\bar{\mu}}\Omega_\ell)(\bar{\ell}_s D_{\bar{\mu}}H e_r) \\
& -\frac{1}{6}\bar{y}_e^{ts}(\mathcal{C}_{H\ell}^{(3)})^{tr}(D_{\bar{\mu}}\Omega_{\ell,j}^* D_{\bar{\mu}}\Omega_\ell^i)H_i^\dagger(\bar{e}_s\ell_r^j) - \frac{1}{6}y_e^{tr}(\mathcal{C}_{H\ell}^{(3)})^{st}(D_{\bar{\mu}}\Omega_{\ell,i}^* D_{\bar{\mu}}\Omega_\ell^j)H^i(\bar{\ell}_{js}e_r) \\
& -\frac{1}{3}\bar{y}_e^{ts}(\mathcal{C}_{H\ell}^{(3)})^{tr}(D_{\bar{\mu}}\Omega_\ell^\dagger\Omega_\ell)(D_{\bar{\mu}}\bar{e}_s H^\dagger\ell_r) - \frac{1}{3}y_e^{tr}(\mathcal{C}_{H\ell}^{(3)})^{st}(\Omega_\ell^\dagger D_{\bar{\mu}}\Omega_\ell)(\bar{\ell}_s H D_{\bar{\mu}}e_r) \\
& -\frac{1}{3}y_e^{tr}(\mathcal{C}_{H\ell}^{(3)})^{st}(\Omega_\ell^\dagger D_{\bar{\mu}}\Omega_\ell)(D_{\bar{\mu}}\bar{\ell}_s H e_r) - \frac{2}{3}\bar{y}_e^{ts}(\mathcal{C}_{H\ell}^{(3)})^{tr}(D_{\bar{\mu}}\Omega_{\ell,j}^*\Omega_\ell^i)D^{\bar{\mu}}H_i^\dagger(\bar{e}_s\ell_r^j) \\
& -\frac{2}{3}y_e^{tr}(\mathcal{C}_{H\ell}^{(3)})^{st}(\Omega_{\ell,i}^* D_{\bar{\mu}}\Omega_\ell^j)D^{\bar{\mu}}H^i(\bar{\ell}_{js}e_r) \\
& -\frac{5}{6}g_Y(\mathcal{C}_{H\ell}^{(3)})^{rr}\left[2(D_{\bar{\nu}}\Omega_{\ell,j}^*\Omega_\ell^i)D^{\bar{\mu}}H_i^\dagger H^j\tilde{B}^{\bar{\mu}\bar{\nu}} + 2(\Omega_{\ell,j}^* D_{\bar{\sigma}}\Omega_\ell^i)H_i^\dagger D^{\bar{\mu}}H^j\tilde{B}^{\bar{\mu}\bar{\sigma}}\right] \\
& +\frac{5i}{6}\bar{y}_e^{ts}(\mathcal{C}_{H\ell}^{(3)})^{tr}(D_{\bar{\nu}}\Omega_{\ell,j}^*\Omega_\ell^i)D^{\bar{\mu}}H_i^\dagger(\bar{e}_s\sigma^{\bar{\mu}\bar{\nu}}\ell_r^j) + \frac{4}{3}\bar{y}_e^{ts}(\mathcal{C}_{H\ell}^{(3)})^{tr}(D_{\bar{\mu}}\Omega_\ell^\dagger\Omega_\ell)(\bar{e}_s D_{\bar{\mu}}H^\dagger\ell_r)
\end{aligned}$$

$$\begin{aligned}
& -\frac{1}{3}\bar{y}_e^{ts}(\mathcal{C}_{H\ell}^{(3)})^{tr}(D_{\bar{\mu}}\Omega_{\ell}^{\dagger}\Omega_{\ell})(\bar{e}_s H^{\dagger} D^{\bar{\mu}}\ell_r) - \frac{4}{3}(\mathcal{C}_{H\ell}^{(3)})^{rr}(D_{\bar{\mu}}\Omega_{\ell,j}^* D_{\bar{\nu}}\Omega_{\ell}^i) D^{\bar{\mu}} H_i^{\dagger} D^{\bar{\nu}} H^j \\
& + \frac{4i}{3}g_L(\mathcal{C}_{H\ell}^{(3)})^{rr}\left[t_k^{Ii}(\Omega_{\ell,j}^* D_{\bar{\nu}}\Omega_{\ell}^k) H_i^{\dagger} D^{\bar{\mu}} H^j W^{\bar{\mu}\bar{\nu}I} - t_k^{Ij}(D_{\bar{\nu}}\Omega_{\ell,j}^* \Omega_{\ell}^i) D^{\bar{\mu}} H_i^{\dagger} H^k W^{\bar{\mu}\bar{\nu}I}\right] \\
& - \frac{5i}{3}\bar{y}_e^{ts}(\mathcal{C}_{H\ell}^{(3)})^{tr}(D_{\bar{\nu}}\Omega_{\ell}^{\dagger}\Omega_{\ell})(\bar{e}_s \sigma^{\bar{\mu}\bar{\nu}} D_{\bar{\mu}} H^{\dagger} \ell_r) + \frac{5i}{3}y_e^{tr}(\mathcal{C}_{H\ell}^{(3)})^{st}(\Omega_{\ell}^{\dagger} D_{\bar{\nu}}\Omega_{\ell})(\bar{\ell}_s D_{\bar{\mu}} H \sigma^{\bar{\mu}\bar{\nu}} e_r) \\
& - 2(\mathcal{C}_{H\ell}^{(3)})^{rr}\left[(D_{\bar{\nu}}\Omega_{\ell,j}^* \Omega_{\ell}^i) D^{\bar{\mu}} D^{\bar{\nu}} H_i^{\dagger} D^{\bar{\mu}} H^j + (\Omega_{\ell,j}^* D_{\bar{\nu}}\Omega_{\ell}^i) D^{\bar{\mu}} H_i^{\dagger} D^{\bar{\mu}} D^{\bar{\nu}} H^j\right], \tag{3.32}
\end{aligned}$$

$$\begin{aligned}
\Gamma_{\Omega}^{(1)}[\mathcal{O}_{Hu}] &= \frac{i}{36}\left[20g_Y^2\mathcal{C}_{Hu}^{sr} - 3\left[y_u^{tr}\bar{y}_u^{tu}\mathcal{C}_{Hu}^{su} + y_u^{tu}\bar{y}_u^{ts}\mathcal{C}_{Hu}^{ur}\right]\right](\Omega_{u,a}^* \overleftrightarrow{D}_{\bar{\mu}}\Omega_u^b)(H^{\dagger}H)(\bar{u}_{bs}\gamma^{\bar{\mu}}u_r^a) \\
& + \frac{i}{24}\mathcal{C}_{Hu}^{tt}\left[3g_L^2 - g_Y^2\right](\Omega_u^{\dagger}\overleftrightarrow{D}_{\bar{\mu}}\Omega_u)(H^{\dagger}H)(\bar{q}_s\gamma^{\bar{\mu}}q_s) + \frac{i}{12}g_Y^2\mathcal{C}_{Hu}^{tt}(\Omega_u^{\dagger}\overleftrightarrow{D}_{\bar{\mu}}\Omega_u)(H^{\dagger}H)(\bar{d}_s\gamma^{\bar{\mu}}d_s) \\
& + \frac{i}{8}\mathcal{C}_{Hu}^{tt}\left[g_L^2 + g_Y^2\right](\Omega_u^{\dagger}\overleftrightarrow{D}_{\bar{\mu}}\Omega_u)(H^{\dagger}H)(\bar{\ell}_s\gamma^{\bar{\mu}}\ell_s) + \frac{1}{6}y_u^{tr}\mathcal{C}_{Hu}^{rs}(D_{\bar{\mu}}\Omega_{u,a}^* D_{\bar{\mu}}\Omega_u^b)(\bar{q}_{bt}\tilde{H}u_s^a) \\
& + \frac{1}{6}\bar{y}_u^{rs}\mathcal{C}_{Hu}^{ts}(D_{\bar{\mu}}\Omega_{u,a}^* D_{\bar{\mu}}\Omega_u^b)(\bar{u}_{bt}\tilde{H}^{\dagger}q_r^a) + \frac{1}{3}\mathcal{C}_{Hu}^{rr}\left[(D_{\bar{\mu}}D_2\Omega_u^{\dagger}\Omega_u)(H^{\dagger}D_{\bar{\mu}}H) + (\Omega_u^{\dagger}D_{\bar{\mu}}D_2\Omega_u)(D_{\bar{\mu}}H^{\dagger}H)\right] \\
& + \frac{1}{3}y_u^{rt}\bar{y}_u^{rs}\mathcal{C}_{Hu}^{ts}\left[(\Omega_q^{\dagger}D_{\bar{\mu}}\Omega_q)(H^{\dagger}H)(H^{\dagger}D_{\bar{\mu}}H) + (D_{\bar{\mu}}\Omega_q^{\dagger}\Omega_q)(H^{\dagger}H)(D_{\bar{\mu}}H^{\dagger}H)\right] \\
& + \left[\frac{1}{4}\mathcal{C}_{Hu}^{rr}\left[g_L^2 + g_Y^2\right] - \frac{4}{3}y_u^{rt}\bar{y}_u^{rs}\mathcal{C}_{Hu}^{ts}\right]\left[(\Omega_u^{\dagger}D_{\bar{\mu}}\Omega_u)(H^{\dagger}H)(H^{\dagger}D_{\bar{\mu}}H) + (D_{\bar{\mu}}\Omega_u^{\dagger}\Omega_u)(H^{\dagger}H)(D_{\bar{\mu}}H^{\dagger}H)\right] \\
& - \frac{1}{6}y_u^{tr}\mathcal{C}_{Hu}^{rs}(D_{\bar{\mu}}\Omega_{u,a}^* \Omega_u^b)(D^{\bar{\mu}}\bar{q}_{bt}\tilde{H}u_s^a) - \frac{1}{6}\bar{y}_u^{rs}\mathcal{C}_{Hu}^{ts}(\Omega_{u,a}^* D_{\bar{\mu}}\Omega_u^b)(\bar{u}_{bt}\tilde{H}^{\dagger}D^{\bar{\mu}}q_r^a) \\
& - \frac{i}{6}\left[y_u^{tr}\bar{y}_u^{tu}\mathcal{C}_{Hu}^{su} + y_u^{tu}\bar{y}_u^{ts}\mathcal{C}_{Hu}^{ur}\right](\Omega_{q,a,j}^* \overleftrightarrow{D}_{\bar{\mu}}\Omega_q^{bj})H_i^{\dagger}H^j(\bar{u}_{bs}\gamma^{\bar{\mu}}u_r^a) \\
& - \frac{i}{6}g_Y^2\mathcal{C}_{Hu}^{tt}(\Omega_u^{\dagger}\overleftrightarrow{D}_{\bar{\mu}}\Omega_u)(H^{\dagger}H)(\bar{u}_s\gamma^{\bar{\mu}}u_s) + \frac{i}{4}g_Y^2\mathcal{C}_{Hu}^{tt}(\Omega_u^{\dagger}\overleftrightarrow{D}_{\bar{\mu}}\Omega_u)(H^{\dagger}H)(\bar{e}_s\gamma^{\bar{\mu}}e_s) \\
& - \frac{i}{4}g_L^2\mathcal{C}_{Hu}^{tt}(\Omega_u^{\dagger}\overleftrightarrow{D}_{\bar{\mu}}\Omega_u)(\bar{\ell}_s H\gamma^{\bar{\mu}}H^{\dagger}\ell_s) - \frac{i}{4}g_L^2\mathcal{C}_{Hu}^{tt}(\Omega_u^{\dagger}\overleftrightarrow{D}_{\bar{\mu}}\Omega_u)(\bar{q}_s H\gamma^{\bar{\mu}}H^{\dagger}q_s) \\
& - \frac{1}{3}y_u^{rt}\bar{y}_u^{rs}\mathcal{C}_{Hu}^{ts}\left[(\Omega_{q,k}^* D_{\bar{\mu}}\Omega_q^j)(H^{\dagger}D_{\bar{\mu}}H)H_j^{\dagger}H^k + (D_{\bar{\mu}}\Omega_{q,k}^* \Omega_q^j)(D_{\bar{\mu}}H^{\dagger}H)H_j^{\dagger}H^k\right] \\
& + \frac{i}{3}g_s\mathcal{C}_{Hu}^{rr}\left[T_b^{Aa}(\Omega_{u,a}^* D_{\bar{\nu}}\Omega_u^b)G^{\bar{\mu}\bar{\nu}A}(H^{\dagger}D_{\bar{\mu}}H) - T_b^{Aa}(D_{\bar{\nu}}\Omega_{u,a}^* \Omega_u^b)G^{\bar{\mu}\bar{\nu}A}(D_{\bar{\mu}}H^{\dagger}H)\right] \\
& - \frac{1}{3}\mathcal{C}_{Hu}^{rr}(D_{\bar{\nu}}\Omega_u^{\dagger}D_{\bar{\nu}}\Omega_u)(D_{\bar{\mu}}H^{\dagger}D_{\bar{\mu}}H) \\
& - \frac{1}{3}\mathcal{C}_{Hu}^{rr}\left[(D_{\bar{\mu}}\Omega_u^{\dagger}D_{\bar{\nu}}\Omega_u)(H^{\dagger}D_{\bar{\mu}}D_{\bar{\nu}}H) + (D_{\bar{\nu}}\Omega_u^{\dagger}D_{\bar{\mu}}\Omega_u)(D_{\bar{\mu}}D_{\bar{\nu}}H^{\dagger}H)\right] \\
& - \frac{i}{3}\mathcal{C}_{Hu}^{rr}\left[(D_{\bar{\mu}}\Omega_{u,a}^* D_{\bar{\rho}}\Omega_u^b)(\Omega_{u,b}^* D_{\bar{\sigma}}\Omega_u^a)(H^{\dagger}D_{\bar{\nu}}H)\varepsilon^{\bar{\mu}\bar{\nu}\bar{\rho}\bar{\sigma}} - (D_{\bar{\nu}}\Omega_{u,a}^* \Omega_u^b)(D_{\bar{\rho}}\Omega_{u,b}^* D_{\bar{\sigma}}\Omega_u^a)(D_{\bar{\mu}}H^{\dagger}H)\varepsilon^{\bar{\mu}\bar{\nu}\bar{\rho}\bar{\sigma}}\right] \\
& + \frac{i}{3}y_u^{rt}\bar{y}_u^{rs}\mathcal{C}_{Hu}^{tu}(D_{\bar{\mu}}\Omega_{q,ak}^* \Omega_q^{bj})H_j^{\dagger}\tilde{H}_k(\bar{d}_{bs}\gamma^{\bar{\mu}}u_u^a) - \frac{i}{3}y_d^{ru}\bar{y}_u^{rs}\mathcal{C}_{Hu}^{ts}(\Omega_{q,ai}^* D_{\bar{\mu}}\Omega_q^{bj})\tilde{H}^{\dagger j}H^i(\bar{u}_{bt}\gamma^{\bar{\mu}}d_u^a) \\
& + \frac{2}{3}y_u^{tr}\mathcal{C}_{Hu}^{rs}(D_{\bar{\mu}}\Omega_{u,a}^* \Omega_u^b)(\bar{q}_{bt}D_{\bar{\mu}}\tilde{H}u_s^a) + \frac{2}{3}\bar{y}_u^{rs}\mathcal{C}_{Hu}^{ts}(\Omega_{u,a}^* D_{\bar{\mu}}\Omega_u^b)(\bar{u}_{bt}D_{\bar{\mu}}\tilde{H}^{\dagger}q_r^a) \\
& - \frac{1}{6}y_u^{tr}\mathcal{C}_{Hu}^{rs}(D_{\bar{\mu}}\Omega_{u,a}^* \Omega_u^b)(\bar{q}_{bt}\tilde{H}D^{\bar{\mu}}u_s^a) - \frac{1}{6}\bar{y}_u^{rs}\mathcal{C}_{Hu}^{ts}(\Omega_{u,a}^* D_{\bar{\mu}}\Omega_u^b)(D^{\bar{\mu}}\bar{u}_{bt}\tilde{H}^{\dagger}q_r^a) \\
& + \frac{i}{6}\left[y_u^{tr}\bar{y}_u^{tu}\mathcal{C}_{Hu}^{su} + y_u^{tu}\bar{y}_u^{ts}\mathcal{C}_{Hu}^{ur}\right](\Omega_{q,a}^* \overleftrightarrow{D}_{\bar{\mu}}\Omega_q^b)(H^{\dagger}H)(\bar{u}_{bs}\gamma^{\bar{\mu}}u_r^a)
\end{aligned}$$

$$\begin{aligned}
& -\frac{4}{9}g_Y\mathcal{C}_{Hu}^{rr}\left[2(\Omega_u^\dagger D_\sigma\Omega_u)\tilde{B}^{\bar{\mu}\bar{\sigma}}(H^\dagger D_\mu H)+2(D_\nu\Omega_u^\dagger\Omega_u)\tilde{B}^{\bar{\mu}\bar{\nu}}(D_\mu H^\dagger H)\right] \\
& -\frac{2}{3}g_s\mathcal{C}_{Hu}^{rr}\left[2T_b^{Aa}(\Omega_{u,a}^*D_\sigma\Omega_u^b)\tilde{G}^{\bar{\mu}\bar{\sigma}A}(H^\dagger D_\mu H)+2T_b^{Aa}(D_\nu\Omega_{u,a}^*\Omega_u^b)\tilde{G}^{\bar{\mu}\bar{\nu}A}(D_\mu H^\dagger H)\right] \\
& -\frac{2}{3}\mathcal{C}_{Hu}^{rr}(D_\mu\Omega_u^\dagger D_\nu\Omega_u)(D_\mu H^\dagger D_\nu H)+\frac{13i}{18}g_Y\mathcal{C}_{Hu}^{rr}\left[(\Omega_u^\dagger D_\nu\Omega_u)B^{\bar{\mu}\bar{\nu}}(H^\dagger D_\mu H)-(D_\nu\Omega_u^\dagger\Omega_u)B^{\bar{\mu}\bar{\nu}}(D_\mu H^\dagger H)\right] \\
& -\frac{5i}{6}y_u^{tr}\mathcal{C}_{Hu}^{rs}(D_\nu\Omega_{u,a}^*\Omega_u^b)(\bar{q}_{bt}D_\mu\tilde{H}\sigma^{\bar{\mu}\bar{\nu}}u_s^a)+\frac{5i}{6}\bar{y}_u^{rs}\mathcal{C}_{Hu}^{ts}(\Omega_{u,a}^*D_\nu\Omega_u^b)(\bar{u}_{bt}\sigma^{\bar{\mu}\bar{\nu}}D_\mu\tilde{H}^\dagger q_r^a) \\
& -\mathcal{C}_{Hu}^{rr}\left[(\Omega_u^\dagger D_\nu\Omega_u)(D_\mu H^\dagger D_\mu D_\nu H)+(D_\nu\Omega_u^\dagger\Omega_u)(D_\mu D_\nu H^\dagger D_\mu H)\right] \\
& +ig_L\mathcal{C}_{Hu}^{rr}\left[(\Omega_u^\dagger D_\nu\Omega_u)W^{\bar{\mu}\bar{\nu}I}(H^\dagger t^I D_\mu H)-(D_\nu\Omega_u^\dagger\Omega_u)W^{\bar{\mu}\bar{\nu}I}(D_\mu H^\dagger t^I H)\right], \tag{3.33}
\end{aligned}$$

$$\begin{aligned}
\Gamma_\Omega^{(1)}[\mathcal{O}_{Hd}] &= -\frac{i}{36}\left[10g_Y^2\mathcal{C}_{Hd}^{sr}-3\left[y_d^{tr}\bar{y}_d^{tu}\mathcal{C}_{Hd}^{su}+y_d^{tu}\bar{y}_d^{ts}\mathcal{C}_{Hd}^{ur}\right]\right](\Omega_{d,a}^*\overset{\leftrightarrow}{D}_\mu\Omega_d^b)(H^\dagger H)(\bar{d}_{bs}\gamma^\mu d_r^a) \\
& +\frac{i}{24}\mathcal{C}_{Hd}^{tt}\left[3g_L^2-g_Y^2\right](\Omega_d^\dagger\overset{\leftrightarrow}{D}_\mu\Omega_d)(H^\dagger H)(\bar{q}_s\gamma^\mu q_s)+\frac{i}{12}g_Y^2\mathcal{C}_{Hd}^{tt}(\Omega_d^\dagger\overset{\leftrightarrow}{D}_\mu\Omega_d)(H^\dagger H)(\bar{d}_s\gamma^\mu d_s) \\
& +\frac{i}{8}\mathcal{C}_{Hd}^{tt}\left[g_L^2+g_Y^2\right](\Omega_d^\dagger\overset{\leftrightarrow}{D}_\mu\Omega_d)(H^\dagger H)(\bar{\ell}_s\gamma^\mu \ell_s) \\
& +\frac{2}{9}g_Y\mathcal{C}_{Hd}^{rr}\left[2(\Omega_d^\dagger D_\sigma\Omega_d)\tilde{B}^{\bar{\mu}\bar{\sigma}}(H^\dagger D_\mu H)+2(D_\nu\Omega_d^\dagger\Omega_d)\tilde{B}^{\bar{\mu}\bar{\nu}}(D_\mu H^\dagger H)\right] \\
& +\frac{1}{3}\mathcal{C}_{Hd}^{rr}\left[(D_\mu D_2\Omega_d^\dagger\Omega_d)(H^\dagger D_\mu H)+(\Omega_d^\dagger D_\mu D_2\Omega_d)(D_\mu H^\dagger H)\right] \\
& +\frac{1}{3}y_d^{rt}\bar{y}_d^{rs}\mathcal{C}_{Hd}^{ts}\left[(\Omega_{q,k}^*D_\mu\Omega_q^j)(H^\dagger D_\mu H)H_j^\dagger H^k+(D_\mu\Omega_{q,k}^*\Omega_q^j)(D_\mu H^\dagger H)H_j^\dagger H^k\right]-\frac{1}{6}\bar{y}_d^{rt}\mathcal{C}_{Hd}^{st}(D_\mu\Omega_{d,a}^*D_\mu\Omega_d^b)(\bar{d}_{bs}H^\dagger q_r^a) \\
& -\frac{1}{6}\bar{y}_d^{rt}\mathcal{C}_{Hd}^{st}(D_\mu\Omega_{d,a}^*\Omega_d^b)(D^\mu\bar{d}_{bs}H^\dagger q_r^a)-\frac{1}{6}y_d^{st}\mathcal{C}_{Hd}^{tr}(D_\mu\Omega_{d,a}^*D_\mu\Omega_d^b)(\bar{q}_{bs}Hd_r^a)-\frac{1}{6}y_d^{st}\mathcal{C}_{Hd}^{tr}(\Omega_{d,a}^*D_\mu\Omega_d^b)(\bar{q}_{bs}HD^\mu d_r^a) \\
& -\frac{i}{6}g_Y^2\mathcal{C}_{Hd}^{tt}(\Omega_d^\dagger\overset{\leftrightarrow}{D}_\mu\Omega_d)(H^\dagger H)(\bar{u}_s\gamma^\mu u_s) \\
& -\frac{i}{6}\left[y_d^{tr}\bar{y}_d^{tu}\mathcal{C}_{Hd}^{su}+y_d^{tu}\bar{y}_d^{ts}\mathcal{C}_{Hd}^{ur}\right](\Omega_{q,a,j}^*\overset{\leftrightarrow}{D}_\mu\Omega_q^{bi})H_i^\dagger H^j(\bar{d}_{bs}\gamma^\mu d_r^a) \\
& +\frac{i}{4}g_Y^2\mathcal{C}_{Hd}^{tt}(\Omega_d^\dagger\overset{\leftrightarrow}{D}_\mu\Omega_d)(H^\dagger H)(\bar{e}_s\gamma^\mu e_s)-\frac{i}{4}g_L^2\mathcal{C}_{Hd}^{tt}(\Omega_d^\dagger\overset{\leftrightarrow}{D}_\mu\Omega_d)(\bar{\ell}_sH\gamma^\mu H^\dagger \ell_s) \\
& -\frac{i}{4}g_L^2\mathcal{C}_{Hd}^{tt}(\Omega_d^\dagger\overset{\leftrightarrow}{D}_\mu\Omega_d)(\bar{q}_sH\gamma^\mu H^\dagger q_s) \\
& +\frac{i}{3}g_s\mathcal{C}_{Hd}^{rr}\left[T_b^{Aa}(\Omega_{d,a}^*D_\nu\Omega_d^b)G^{\bar{\mu}\bar{\nu}A}(H^\dagger D_\mu H)-T_b^{Aa}(D_\nu\Omega_{d,a}^*\Omega_d^b)G^{\bar{\mu}\bar{\nu}A}(D_\mu H^\dagger H)\right] \\
& -\frac{1}{3}\mathcal{C}_{Hd}^{rr}\left[(D_\mu\Omega_d^\dagger D_\nu\Omega_d)(H^\dagger D_\mu D_\nu H)+(D_\nu\Omega_d^\dagger D_\mu\Omega_d)(D_\mu D_\nu H^\dagger H)\right] \\
& -\frac{i}{3}\mathcal{C}_{Hd}^{rr}\left[(D_\mu\Omega_{d,a}^*D_\rho\Omega_d^b)(\Omega_{d,b}^*D_\sigma\Omega_d^a)(H^\dagger D_\nu H)\varepsilon^{\bar{\mu}\bar{\nu}\bar{\rho}\bar{\sigma}}-(D_\nu\Omega_{d,a}^*\Omega_d^b)(D_\rho\Omega_{d,b}^*D_\sigma\Omega_d^a)(D_\mu H^\dagger H)\varepsilon^{\bar{\mu}\bar{\nu}\bar{\rho}\bar{\sigma}}\right] \\
& -\frac{i}{3}y_u^{ru}\bar{y}_d^{rs}\mathcal{C}_{Hd}^{ts}(D_\mu\Omega_{q,ak}^*\Omega_q^{bj})H_j^\dagger \tilde{H}_k(\bar{d}_{bt}\gamma^\mu u_u^a) \\
& +\frac{7i}{18}g_Y\mathcal{C}_{Hd}^{rr}\left[(\Omega_d^\dagger D_\nu\Omega_d)B^{\bar{\mu}\bar{\nu}}(H^\dagger D_\mu H)-(D_\nu\Omega_d^\dagger\Omega_d)B^{\bar{\mu}\bar{\nu}}(D_\mu H^\dagger H)\right]+\frac{2}{3}\bar{y}_d^{rt}\mathcal{C}_{Hd}^{st}(D_\mu\Omega_{d,a}^*\Omega_d^b)(\bar{d}_{bs}D_\mu H^\dagger q_r^a) \\
& +\frac{2}{3}y_d^{st}\mathcal{C}_{Hd}^{tr}(\Omega_{d,a}^*D_\mu\Omega_d^b)(\bar{q}_{bs}D_\mu Hd_r^a)
\end{aligned}$$

$$\begin{aligned}
& + \left[ \frac{1}{4} \mathcal{C}_{Hd}^{rr} [g_L^2 + g_Y^2] - \frac{4}{3} y_d^{rt} \bar{y}_d^{rs} \mathcal{C}_{Hd}^{ts} \right] \left[ (\Omega_d^\dagger D_{\bar{\mu}} \Omega_d) (H^\dagger H) (H^\dagger D_{\bar{\mu}} H) + (D_{\bar{\mu}} \Omega_d^\dagger \Omega_d) (H^\dagger H) (D_{\bar{\mu}} H^\dagger H) \right] \\
& - \frac{1}{6} \bar{y}_d^{rt} \mathcal{C}_{Hd}^{st} (D_{\bar{\mu}} \Omega_{d,a}^* \Omega_d^b) (\bar{d}_{bs} H^\dagger D^{\bar{\mu}} q_r^a) - \frac{1}{6} y_d^{st} \mathcal{C}_{Hd}^{tr} (\Omega_{d,a}^* D_{\bar{\mu}} \Omega_d^b) (D^{\bar{\mu}} \bar{q}_{bs} H d_r^a) - \frac{1}{3} \mathcal{C}_{Hd}^{rr} (D_{\bar{\nu}} \Omega_d^\dagger D_{\bar{\nu}} \Omega_d) (D_{\bar{\mu}} H^\dagger D_{\bar{\mu}} H) \\
& + \frac{i}{3} y_d^{rt} \bar{y}_u^{rs} \mathcal{C}_{Hd}^{tu} (\Omega_{q,ai}^* D_{\bar{\mu}} \Omega_q^{bj}) \tilde{H}^{\dagger j} H^i (\bar{u}_{bs} \gamma^{\bar{\mu}} d_u^a) \\
& - \frac{2}{3} g_s \mathcal{C}_{Hd}^{rr} \left[ 2 T_b^{Aa} (\Omega_{d,a}^* D_{\bar{\sigma}} \Omega_d^b) \tilde{G}^{\bar{\mu}\bar{\sigma} A} (H^\dagger D_{\bar{\mu}} H) + 2 T_b^{Aa} (D_{\bar{\nu}} \Omega_{d,a}^* \Omega_d^b) \tilde{G}^{\bar{\mu}\bar{\nu} A} (D_{\bar{\mu}} H^\dagger H) \right] \\
& - \frac{2}{3} \mathcal{C}_{Hd}^{rr} (D_{\bar{\mu}} \Omega_d^\dagger D_{\bar{\nu}} \Omega_d) (D_{\bar{\mu}} H^\dagger D_{\bar{\nu}} H) + \frac{5i}{6} \bar{y}_d^{rt} \mathcal{C}_{Hd}^{st} (D_{\bar{\nu}} \Omega_{d,a}^* \Omega_d^b) (\bar{d}_{bs} \sigma^{\bar{\mu}\bar{\nu}} D_{\bar{\mu}} H^\dagger q_r^a) \\
& - \frac{5i}{6} y_d^{st} \mathcal{C}_{Hd}^{tr} (\Omega_{d,a}^* D_{\bar{\nu}} \Omega_d^b) (\bar{q}_{bs} D_{\bar{\mu}} H \sigma^{\bar{\mu}\bar{\nu}} d_r^a) - \mathcal{C}_{Hd}^{rr} \left[ (\Omega_d^\dagger D_{\bar{\nu}} \Omega_d) (D_{\bar{\mu}} H^\dagger D_{\bar{\mu}} D_{\bar{\nu}} H) + (D_{\bar{\nu}} \Omega_d^\dagger \Omega_d) (D_{\bar{\mu}} D_{\bar{\nu}} H^\dagger D_{\bar{\mu}} H) \right] \\
& + i g_L \mathcal{C}_{Hd}^{rr} \left[ (\Omega_d^\dagger D_{\bar{\nu}} \Omega_d) W^{\bar{\mu}\bar{\nu} I} (H^\dagger t^I D_{\bar{\mu}} H) - (D_{\bar{\nu}} \Omega_d^\dagger \Omega_d) W^{\bar{\mu}\bar{\nu} I} (D_{\bar{\mu}} H^\dagger t^I H) \right], \tag{3.34}
\end{aligned}$$

$$\begin{aligned}
\Gamma_\Omega^{(1)} [\mathcal{O}_{Hud}] &= \frac{i}{12} \left[ y_d^{ut} \bar{y}_u^{us} \bar{\mathcal{C}}_{Hud}^{rt} + y_u^{tr} \bar{y}_d^{tu} \mathcal{C}_{Hud}^{su} \right] (\Omega_{d,a}^* \overset{\leftrightarrow}{D}_{\bar{\mu}} \Omega_d^b) (H^\dagger H) (\bar{u}_{bs} \gamma^{\bar{\mu}} u_r^a) \\
& + \frac{i}{12} \left[ y_d^{ur} \bar{y}_u^{ut} \bar{\mathcal{C}}_{Hud}^{ts} + y_u^{tu} \bar{y}_d^{ts} \mathcal{C}_{Hud}^{ur} \right] (\Omega_{u,a}^* \overset{\leftrightarrow}{D}_{\bar{\mu}} \Omega_u^b) (H^\dagger H) (\bar{d}_{bs} \gamma^{\bar{\mu}} d_r^a) \\
& + \frac{1}{6} \left[ y_u^{rt} \bar{y}_d^{rs} \mathcal{C}_{Hud}^{ts} - y_d^{ts} \bar{y}_u^{tr} \bar{\mathcal{C}}_{Hud}^{rs} \right] \left[ (\Omega_{q,k}^* D_{\bar{\mu}} \Omega_q^j) (H^\dagger H) H_j^\dagger D^{\bar{\mu}} H^k - (D_{\bar{\mu}} \Omega_{q,k}^* \Omega_q^j) (H^\dagger H) D^{\bar{\mu}} H_j^\dagger H^k \right] \\
& + \frac{1}{6} \left[ y_d^{ts} \bar{y}_u^{tr} \bar{\mathcal{C}}_{Hud}^{rs} + y_u^{rt} \bar{y}_d^{rs} \mathcal{C}_{Hud}^{ts} \right] \left[ (D_{\bar{\mu}} \Omega_{q,k}^* \Omega_q^j) (H^\dagger H) D^{\bar{\mu}} H_j^\dagger H^k + (\Omega_{q,k}^* D_{\bar{\mu}} \Omega_q^j) (H^\dagger H) H_j^\dagger D^{\bar{\mu}} H^k \right] \\
& + \frac{1}{6} \left[ y_d^{ts} \bar{y}_u^{tr} \bar{\mathcal{C}}_{Hud}^{rs} - y_u^{rt} \bar{y}_d^{rs} \mathcal{C}_{Hud}^{ts} \right] \left[ (\Omega_{q,k}^* D_{\bar{\mu}} \Omega_q^j) (H^\dagger D_{\bar{\mu}} H) H_j^\dagger H^k - (D_{\bar{\mu}} \Omega_{q,k}^* \Omega_q^j) (D_{\bar{\mu}} H^\dagger H) H_j^\dagger H^k \right] \\
& + \frac{1}{6} \left[ - y_d^{ts} \bar{y}_u^{tr} \bar{\mathcal{C}}_{Hud}^{rs} - y_u^{rt} \bar{y}_d^{rs} \mathcal{C}_{Hud}^{ts} \right] \left[ (\Omega_{q,k}^* D_{\bar{\mu}} \Omega_q^j) (H^\dagger D_{\bar{\mu}} H) H_j^\dagger H^k + (D_{\bar{\mu}} \Omega_{q,k}^* \Omega_q^j) (D_{\bar{\mu}} H^\dagger H) H_j^\dagger H^k \right] \\
& + \frac{1}{6} y_d^{ts} \bar{\mathcal{C}}_{Hud}^{rs} (D_{\bar{\mu}} \Omega_{d,a}^* \Omega_d^b) (\bar{q}_{bt} \tilde{H} D^{\bar{\mu}} u_r^a) + \frac{1}{6} y_d^{ts} \bar{\mathcal{C}}_{Hud}^{rs} (D_{\bar{\mu}} \Omega_{d,a}^* \Omega_d^b) (D^{\bar{\mu}} \bar{q}_{bt} \tilde{H} u_r^a) \\
& + \frac{1}{6} \bar{y}_d^{rs} \mathcal{C}_{Hud}^{ts} (\Omega_{d,a}^* D_{\bar{\mu}} \Omega_d^b) (\bar{u}_{bt} \tilde{H}^\dagger D^{\bar{\mu}} q_r^a) + \frac{1}{6} \bar{y}_d^{rs} \mathcal{C}_{Hud}^{ts} (\Omega_{d,a}^* D_{\bar{\mu}} \Omega_d^b) (D^{\bar{\mu}} \bar{u}_{bt} \tilde{H}^\dagger q_r^a) \\
& - \frac{i}{6} \left[ y_d^{ur} \bar{y}_u^{ut} \bar{\mathcal{C}}_{Hud}^{ts} + y_u^{tu} \bar{y}_d^{ts} \mathcal{C}_{Hud}^{ur} \right] (\Omega_{q,a}^* \overset{\leftrightarrow}{D}_{\bar{\mu}} \Omega_q^b) (H^\dagger H) (\bar{d}_{bs} \gamma^{\bar{\mu}} d_r^a) \\
& + \frac{i}{6} \left[ y_d^{ur} \bar{y}_u^{ut} \bar{\mathcal{C}}_{Hud}^{ts} + y_u^{tu} \bar{y}_d^{ts} \mathcal{C}_{Hud}^{ur} \right] (\Omega_{q,aj}^* \overset{\leftrightarrow}{D}_{\bar{\mu}} \Omega_q^{bi}) H_i^\dagger H^j (\bar{d}_{bs} \gamma^{\bar{\mu}} d_r^a) \\
& - \frac{i}{6} \left[ y_d^{ut} \bar{y}_u^{us} \bar{\mathcal{C}}_{Hud}^{rt} + y_u^{tr} \bar{y}_d^{tu} \mathcal{C}_{Hud}^{su} \right] (\Omega_{q,aj}^* \overset{\leftrightarrow}{D}_{\bar{\mu}} \Omega_q^{bi}) H_i^\dagger H^j (\bar{u}_{bs} \gamma^{\bar{\mu}} u_r^a) + \frac{2}{3} \bar{y}_u^{rt} \bar{\mathcal{C}}_{Hud}^{ts} (D_{\bar{\mu}} \Omega_{u,a}^* \Omega_u^b) (\bar{d}_{bs} D_{\bar{\mu}} H^\dagger q_r^a) \\
& + \frac{2}{3} y_u^{st} \mathcal{C}_{Hud}^{tr} (\Omega_{u,a}^* D_{\bar{\mu}} \Omega_u^b) (\bar{q}_{bs} D_{\bar{\mu}} H d_r^a) + \frac{2}{3} y_d^{ts} \bar{\mathcal{C}}_{Hud}^{rs} (D_{\bar{\mu}} \Omega_{d,a}^* \Omega_d^b) (\bar{q}_{bt} D_{\bar{\mu}} \tilde{H} u_r^a) \\
& + \frac{2}{3} \bar{y}_d^{rs} \mathcal{C}_{Hud}^{ts} (\Omega_{d,a}^* D_{\bar{\mu}} \Omega_d^b) (\bar{u}_{bt} D_{\bar{\mu}} \tilde{H}^\dagger q_r^a) - \frac{1}{6} \bar{y}_u^{rt} \bar{\mathcal{C}}_{Hud}^{ts} (D_{\bar{\mu}} \Omega_{u,a}^* D_{\bar{\mu}} \Omega_u^b) (\bar{d}_{bs} H^\dagger q_r^a) \\
& - \frac{1}{6} \bar{y}_u^{rt} \bar{\mathcal{C}}_{Hud}^{ts} (D_{\bar{\mu}} \Omega_{u,a}^* \Omega_u^b) (\bar{d}_{bs} H^\dagger D^{\bar{\mu}} q_r^a) - \frac{1}{6} \bar{y}_u^{rt} \bar{\mathcal{C}}_{Hud}^{ts} (D_{\bar{\mu}} \Omega_{u,a}^* \Omega_u^b) (D^{\bar{\mu}} \bar{d}_{bs} H^\dagger q_r^a) \\
& - \frac{1}{6} y_u^{st} \mathcal{C}_{Hud}^{tr} (D_{\bar{\mu}} \Omega_{u,a}^* D_{\bar{\mu}} \Omega_u^b) (\bar{q}_{bs} H d_r^a) - \frac{1}{6} y_u^{st} \mathcal{C}_{Hud}^{tr} (\Omega_{u,a}^* D_{\bar{\mu}} \Omega_u^b) (\bar{q}_{bs} H D^{\bar{\mu}} d_r^a) - \frac{1}{6} y_u^{st} \mathcal{C}_{Hud}^{tr} (\Omega_{u,a}^* D_{\bar{\mu}} \Omega_u^b) (D^{\bar{\mu}} \bar{q}_{bs} H d_r^a) \\
& - \frac{1}{6} y_d^{ts} \bar{\mathcal{C}}_{Hud}^{rs} (D_{\bar{\mu}} \Omega_{d,a}^* D_{\bar{\mu}} \Omega_d^b) (\bar{q}_{bt} \tilde{H} u_r^a) - \frac{1}{6} \bar{y}_d^{rs} \mathcal{C}_{Hud}^{ts} (D_{\bar{\mu}} \Omega_{d,a}^* D_{\bar{\mu}} \Omega_d^b) (\bar{u}_{bt} \tilde{H}^\dagger q_r^a)
\end{aligned}$$

$$\begin{aligned}
& + \frac{5i}{6} \bar{y}_u^{rt} \bar{C}_{Hud}^{ts} (D_{\bar{\nu}} \Omega_{u,a}^* \Omega_u^b) (\bar{d}_{bs} \sigma^{\bar{\mu}\bar{\nu}} D_{\bar{\mu}} H^\dagger q_r^a) - \frac{5i}{6} y_u^{st} C_{Hud}^{tr} (\Omega_{u,a}^* D_{\bar{\nu}} \Omega_u^b) (\bar{q}_{bs} D_{\bar{\mu}} H \sigma^{\bar{\mu}\bar{\nu}} d_r^a) \\
& - \frac{5i}{6} y_d^{ts} \bar{C}_{Hud}^{rs} (D_{\bar{\nu}} \Omega_{d,a}^* \Omega_d^b) (\bar{q}_{bt} D_{\bar{\mu}} \tilde{H} \sigma^{\bar{\mu}\bar{\nu}} u_r^a) + \frac{5i}{6} \bar{y}_d^{rs} C_{Hud}^{ts} (\Omega_{d,a}^* D_{\bar{\nu}} \Omega_d^b) (\bar{u}_{bt} \sigma^{\bar{\mu}\bar{\nu}} D_{\bar{\mu}} \tilde{H}^\dagger q_r^a), \tag{3.35}
\end{aligned}$$

$$\begin{aligned}
\Gamma_\Omega^{(1)} [\mathcal{O}_{Hq}^{(1)}] &= \frac{i}{36} \left[ 3y_u^{su} \bar{y}_u^{tu} (\mathcal{C}_{Hq}^{(1)})^{tr} + 3y_u^{ut} \bar{y}_u^{rt} (\mathcal{C}_{Hq}^{(1)})^{su} + 10g_Y^2 (\mathcal{C}_{Hq}^{(1)})^{sr} - 3y_d^{su} \bar{y}_d^{tu} (\mathcal{C}_{Hq}^{(1)})^{tr} - 3y_d^{ut} \bar{y}_d^{rt} (\mathcal{C}_{Hq}^{(1)})^{su} \right] \\
&\quad \left[ (\Omega_{q,aj}^* D_{\bar{\mu}} \Omega_q^{bi}) H_i^\dagger (\bar{q}_{bs} H \gamma^{\bar{\mu}} q_r^{aj}) - (D_{\bar{\mu}} \Omega_{q,aj}^* \Omega_q^{bk}) H^j (\bar{q}_{bks} \gamma^{\bar{\mu}} H^\dagger q_r^a) \right] \\
&- \frac{i}{36} \left[ 5(\mathcal{C}_{Hq}^{(1)})^{sr} [3g_L^2 - g_Y^2] - 3[y_u^{su} \bar{y}_u^{tu} (\mathcal{C}_{Hq}^{(1)})^{tr} + y_u^{ut} \bar{y}_u^{rt} (\mathcal{C}_{Hq}^{(1)})^{su}] \right] (\Omega_{q,a}^* \overleftrightarrow{D}_{\bar{\mu}} \Omega_q^b) (H^\dagger H) (\bar{q}_{bs} \gamma^{\bar{\mu}} q_r^a) \\
&+ \frac{i}{36} \left[ 5(\mathcal{C}_{Hq}^{(1)})^{sr} [3g_L^2 - g_Y^2] - 3[y_u^{su} \bar{y}_u^{tu} (\mathcal{C}_{Hq}^{(1)})^{tr} + y_u^{ut} \bar{y}_u^{rt} (\mathcal{C}_{Hq}^{(1)})^{su}] \right] (\Omega_{q,a}^* \overleftrightarrow{D}_{\bar{\mu}} \Omega_q^b) (\bar{q}_{bs} H \gamma^{\bar{\mu}} H^\dagger q_r^a) \\
&+ \frac{i}{36} \left[ 5(\mathcal{C}_{Hq}^{(1)})^{sr} [3g_L^2 - g_Y^2] - 3[y_u^{su} \bar{y}_u^{tu} (\mathcal{C}_{Hq}^{(1)})^{tr} + y_u^{ut} \bar{y}_u^{rt} (\mathcal{C}_{Hq}^{(1)})^{su}] \right] (\Omega_{q,aj}^* \overleftrightarrow{D}_{\bar{\mu}} \Omega_q^{bi}) H_i^\dagger H^j (\bar{q}_{bs} \gamma^{\bar{\mu}} q_r^a) \\
&+ \frac{i}{24} (\mathcal{C}_{Hq}^{(1)})^{tt} [3g_L^2 - g_Y^2] (\Omega_q^\dagger \overleftrightarrow{D}_{\bar{\mu}} \Omega_q) (H^\dagger H) (\bar{q}_s \gamma^{\bar{\mu}} q_s) \\
&+ \frac{1}{18} g_Y (\mathcal{C}_{Hq}^{(1)})^{rr} \left[ 2(D_{\bar{\nu}} \Omega_{q,j}^* \Omega_q^i) D^{\bar{\mu}} H_i^\dagger H^j \tilde{B}^{\bar{\mu}\bar{\nu}} + 2(\Omega_{q,j}^* D_{\bar{\sigma}} \Omega_q^i) H_i^\dagger D^{\bar{\mu}} H^j \tilde{B}^{\bar{\mu}\bar{\sigma}} \right] \\
&+ \frac{1}{12} g_Y (\mathcal{C}_{Hq}^{(1)})^{rr} \left[ 2(\Omega_{q,b}^* D_{\bar{\sigma}} \Omega_q^a) (\Omega_{q,aj}^* D_{\bar{\rho}} \Omega_q^{bi}) H_i^\dagger H^j \tilde{B}^{\bar{\rho}\bar{\sigma}} - 2(D_{\bar{\mu}} \Omega_{q,a}^* \Omega_q^b) (D_{\bar{\nu}} \Omega_{q,bk}^* \Omega_q^{ai}) H_i^\dagger H^k \tilde{B}^{\bar{\mu}\bar{\nu}} \right] \\
&+ \frac{1}{12} g_Y (\mathcal{C}_{Hq}^{(1)})^{rr} \left[ 2(\Omega_q^\dagger D_{\bar{\sigma}} \Omega_q) \tilde{B}^{\bar{\mu}\bar{\sigma}} (H^\dagger D_{\bar{\mu}} H) + 2(D_{\bar{\nu}} \Omega_q^\dagger \Omega_q) \tilde{B}^{\bar{\mu}\bar{\nu}} (D_{\bar{\mu}} H^\dagger H) \right] \\
&- \frac{i}{12} \left[ y_d^{su} \bar{y}_d^{tu} (\mathcal{C}_{Hq}^{(1)})^{tr} + y_u^{su} \bar{y}_u^{tu} (\mathcal{C}_{Hq}^{(1)})^{tr} - y_d^{ut} \bar{y}_d^{rt} (\mathcal{C}_{Hq}^{(1)})^{su} - y_u^{ut} \bar{y}_u^{rt} (\mathcal{C}_{Hq}^{(1)})^{su} \right] \\
&\quad \left[ (\Omega_{q,aj}^* D_{\bar{\mu}} \Omega_q^{bi}) H_i^\dagger (\bar{q}_{bs} H \gamma^{\bar{\mu}} q_r^{aj}) + (D_{\bar{\mu}} \Omega_{q,aj}^* \Omega_q^{bk}) H^j (\bar{q}_{bks} \gamma^{\bar{\mu}} H^\dagger q_r^a) \right] \\
&+ \frac{i}{12} g_Y^2 (\mathcal{C}_{Hq}^{(1)})^{tt} (\Omega_q^\dagger \overleftrightarrow{D}_{\bar{\mu}} \Omega_q) (H^\dagger H) (\bar{d}_s \gamma^{\bar{\mu}} d_s) - \frac{i}{8} (\mathcal{C}_{Hq}^{(1)})^{tt} [g_L^2 - g_Y^2] (\Omega_q^\dagger \overleftrightarrow{D}_{\bar{\mu}} \Omega_q) (H^\dagger H) (\bar{\ell}_s \gamma^{\bar{\mu}} \ell_s) \\
&+ \frac{1}{6} g_L (\mathcal{C}_{Hq}^{(1)})^{rr} \left[ 2t_l^{Ik} (\Omega_{q,aj}^* D_{\bar{\rho}} \Omega_q^{bi}) (\Omega_{q,bk}^* D_{\bar{\sigma}} \Omega_q^{aj}) H_i^\dagger H^l \widetilde{W}^{\bar{\rho}\bar{\sigma}I} - 2t_l^{Ii} (D_{\bar{\mu}} \Omega_{q,aj}^* \Omega_q^{bl}) (D_{\bar{\nu}} \Omega_{q,bk}^* \Omega_q^{aj}) H_i^\dagger H^k \widetilde{W}^{\bar{\mu}\bar{\nu}I} \right] \\
&+ \frac{1}{6} \bar{y}_d^{ts} (\mathcal{C}_{Hq}^{(1)})^{tr} (D_{\bar{\mu}} \Omega_{q,aj}^* D_{\bar{\mu}} \Omega_q^{bi}) H_i^\dagger (\bar{d}_{bs} q_r^{aj}) + \frac{1}{6} y_u^{st} (\mathcal{C}_{Hq}^{(1)})^{rs} (D_{\bar{\mu}} \Omega_{q,a}^* D_{\bar{\mu}} \Omega_q^b) (\bar{q}_{br} \tilde{H} u_t^a) \\
&+ \frac{1}{6} y_u^{st} (\mathcal{C}_{Hq}^{(1)})^{rs} (D_{\bar{\mu}} \Omega_{q,a}^* \Omega_q^b) (\bar{q}_{br} \tilde{H} D^{\bar{\mu}} u_t^a) + \frac{1}{6} y_u^{st} (\mathcal{C}_{Hq}^{(1)})^{rs} (D_{\bar{\mu}} \Omega_{q,a}^* \Omega_q^b) (D^{\bar{\mu}} \bar{q}_{br} \tilde{H} u_t^a) \\
&+ \frac{1}{6} y_d^{tr} (\mathcal{C}_{Hq}^{(1)})^{st} (D_{\bar{\mu}} \Omega_{q,ai}^* D_{\bar{\mu}} \Omega_q^{bj}) H_i^\dagger (\bar{q}_{bjs} d_r^a) + \frac{1}{6} y_u^{st} (\mathcal{C}_{Hq}^{(1)})^{rs} \varepsilon^{kj} (D_{\bar{\mu}} \Omega_{q,aj}^* D_{\bar{\mu}} \Omega_q^{bi}) H_i^\dagger (\bar{q}_{bkr} u_t^a) \\
&+ \frac{1}{6} y_u^{st} (\mathcal{C}_{Hq}^{(1)})^{rs} \varepsilon^{kj} (D_{\bar{\mu}} \Omega_{q,aj}^* \Omega_q^{bi}) H_i^\dagger (\bar{q}_{bkr} D^{\bar{\mu}} u_t^a) + \frac{1}{6} y_u^{st} (\mathcal{C}_{Hq}^{(1)})^{rs} \varepsilon^{kj} (D_{\bar{\mu}} \Omega_{q,aj}^* \Omega_q^{bi}) H_i^\dagger (D^{\bar{\mu}} \bar{q}_{bkr} u_t^a) \\
&+ \frac{1}{6} \bar{y}_u^{rs} (\mathcal{C}_{Hq}^{(1)})^{rt} \bar{\varepsilon}_{jk} (D_{\bar{\mu}} \Omega_{q,ai}^* D_{\bar{\mu}} \Omega_q^{bk}) H_i^\dagger (\bar{u}_{bs} q_t^{aj}) + \frac{1}{6} \bar{y}_u^{rs} (\mathcal{C}_{Hq}^{(1)})^{rt} \bar{\varepsilon}_{jk} (\Omega_{q,ai}^* D_{\bar{\mu}} \Omega_q^{bk}) H_i^\dagger (\bar{u}_{bs} D^{\bar{\mu}} q_t^{aj}) \\
&+ \frac{1}{6} \bar{y}_u^{rs} (\mathcal{C}_{Hq}^{(1)})^{rt} (D_{\bar{\mu}} \Omega_{q,a}^* D_{\bar{\mu}} \Omega_q^b) (\bar{u}_{bs} \tilde{H}^\dagger q_t^a) + \frac{1}{6} \bar{y}_u^{rs} (\mathcal{C}_{Hq}^{(1)})^{rt} (\Omega_{q,a}^* D_{\bar{\mu}} \Omega_q^b) (\bar{u}_{bs} \tilde{H}^\dagger D^{\bar{\mu}} q_t^a) \\
&+ \frac{1}{6} \bar{y}_u^{rs} (\mathcal{C}_{Hq}^{(1)})^{rt} \bar{\varepsilon}_{jk} (\Omega_{q,ai}^* D_{\bar{\mu}} \Omega_q^{bk}) H_i^\dagger (D^{\bar{\mu}} \bar{u}_{bs} q_t^{aj}) + \frac{1}{6} \bar{y}_u^{rs} (\mathcal{C}_{Hq}^{(1)})^{rt} (\Omega_{q,a}^* D_{\bar{\mu}} \Omega_q^b) (D^{\bar{\mu}} \bar{u}_{bs} \tilde{H}^\dagger q_t^a) \\
&+ \frac{i}{6} \left[ y_d^{su} \bar{y}_d^{tu} (\mathcal{C}_{Hq}^{(1)})^{tr} + y_d^{ut} \bar{y}_d^{rt} (\mathcal{C}_{Hq}^{(1)})^{su} \right] (\Omega_{d,a}^* \overleftrightarrow{D}_{\bar{\mu}} \Omega_d^b) (\bar{q}_{bs} H \gamma^{\bar{\mu}} H^\dagger q_r^a)
\end{aligned}$$

$$\begin{aligned}
& -\frac{i}{6}g_Y^2(\mathcal{C}_{Hq}^{(1)})^{tt}(\Omega_q^\dagger \overleftrightarrow{D}_{\bar{\mu}}\Omega_q)(H^\dagger H)(\bar{u}_s\gamma^{\bar{\mu}}u_s) \\
& -\frac{i}{6}\left[y_u^{su}\bar{y}_u^{tu}(\mathcal{C}_{Hq}^{(1)})^{tr}+y_u^{ut}\bar{y}_u^{rt}(\mathcal{C}_{Hq}^{(1)})^{su}\right](\Omega_{u,a}^*\overleftrightarrow{D}_{\bar{\mu}}\Omega_u^b)(H^\dagger H)(\bar{q}_{bs}\gamma^{\bar{\mu}}q_r^a) \\
& +\frac{i}{6}\left[y_u^{su}\bar{y}_u^{tu}(\mathcal{C}_{Hq}^{(1)})^{tr}+y_u^{ut}\bar{y}_u^{rt}(\mathcal{C}_{Hq}^{(1)})^{su}\right](\Omega_{u,a}^*\overleftrightarrow{D}_{\bar{\mu}}\Omega_u^b)(\bar{q}_{bs}H\gamma^{\bar{\mu}}H^\dagger q_r^a) \\
& +\frac{i}{4}g_Y^2(\mathcal{C}_{Hq}^{(1)})^{tt}(\Omega_q^\dagger \overleftrightarrow{D}_{\bar{\mu}}\Omega_q)(H^\dagger H)(\bar{e}_s\gamma^{\bar{\mu}}e_s)-\frac{i}{4}g_L^2(\mathcal{C}_{Hq}^{(1)})^{tt}(\Omega_q^\dagger \overleftrightarrow{D}_{\bar{\mu}}\Omega_q)(\bar{q}_sH\gamma^{\bar{\mu}}H^\dagger q_s) \\
& +\frac{i}{4}g_L^2(\mathcal{C}_{Hq}^{(1)})^{tt}(\Omega_{q,j}^*\overleftrightarrow{D}_{\bar{\mu}}\Omega_q^i)H_i^\dagger H^j(\bar{\ell}_s\gamma^{\bar{\mu}}\ell_s)+\frac{i}{4}g_L^2(\mathcal{C}_{Hq}^{(1)})^{tt}(\Omega_{q,j}^*\overleftrightarrow{D}_{\bar{\mu}}\Omega_q^k)(H^\dagger H)(\bar{\ell}_{ks}\gamma^{\bar{\mu}}\ell_s^j) \\
& +\frac{1}{3}g_s(\mathcal{C}_{Hq}^{(1)})^{rr}\left[2T_b^{Aa}(D_{\bar{\nu}}\Omega_{q,aj}^*\Omega_q^{bi})D^{\bar{\mu}}H_i^\dagger H^j\widetilde{G}^{\bar{\mu}\bar{\nu}A}+2T_b^{Aa}(\Omega_{q,aj}^*D_{\bar{\sigma}}\Omega_q^{bi})H_i^\dagger D^{\bar{\mu}}H^j\widetilde{G}^{\bar{\mu}\bar{\sigma}A}\right] \\
& +\frac{1}{3}g_L(\mathcal{C}_{Hq}^{(1)})^{rr}\left[2t_k^{Ij}(\Omega_{q,j}^*D_{\bar{\sigma}}\Omega_q^i)D^{\bar{\mu}}H_i^\dagger H^k\widetilde{W}^{\bar{\mu}\bar{\sigma}I}-2t_k^{Ii}(D_{\bar{\mu}}\Omega_{q,j}^*\Omega_q^k)H_i^\dagger D^{\bar{\nu}}H^j\widetilde{W}^{\bar{\mu}\bar{\nu}I}\right] \\
& +\frac{1}{3}(\mathcal{C}_{Hq}^{(1)})^{rr}\left[(D_{\bar{\mu}}D_2\Omega_q^\dagger\Omega_q)(H^\dagger D_{\bar{\mu}}H)+(\Omega_q^\dagger D_{\bar{\mu}}D_2\Omega_q)(D_{\bar{\mu}}H^\dagger H)\right] \\
& +\frac{1}{3}y_u^{ts}\bar{y}_u^{rs}(\mathcal{C}_{Hq}^{(1)})^{rt}\left[(\Omega_u^\dagger D_{\bar{\mu}}\Omega_u)(H^\dagger H)(H^\dagger D_{\bar{\mu}}H)+(D_{\bar{\mu}}\Omega_u^\dagger\Omega_u)(H^\dagger H)(D_{\bar{\mu}}H^\dagger H)\right] \\
& +\frac{2}{3}y_d^{tr}(\mathcal{C}_{Hq}^{(1)})^{st}(\Omega_{q,ai}^*D_{\bar{\mu}}\Omega_q^{bj})D^{\bar{\mu}}H^i(\bar{q}_{bjs}d_r^a) \\
& -\frac{1}{6}g_L(\mathcal{C}_{Hq}^{(1)})^{rr}\left[2t_l^{Ik}(\Omega_{q,a}^*D_{\bar{\rho}}\Omega_q^b)(\Omega_{q,bk}^*D_{\bar{\sigma}}\Omega_q^{ai})H_i^\dagger H^l\widetilde{W}^{\bar{\rho}\bar{\sigma}I}-2t_l^{Ii}(D_{\bar{\nu}}\Omega_{q,b}^*\Omega_q^a)(D_{\bar{\mu}}\Omega_{q,aj}^*\Omega_q^{bl})H_i^\dagger H^j\widetilde{W}^{\bar{\mu}\bar{\nu}I}\right] \\
& -\frac{1}{6}y_d^{tr}(\mathcal{C}_{Hq}^{(1)})^{st}(\Omega_{q,ai}^*D_{\bar{\mu}}\Omega_q^{bj})H^i(\bar{q}_{bjs}D^{\bar{\mu}}d_r^a)-\frac{1}{6}y_d^{tr}(\mathcal{C}_{Hq}^{(1)})^{st}(\Omega_{q,ai}^*D_{\bar{\mu}}\Omega_q^{bj})H^i(D^{\bar{\mu}}\bar{q}_{bjs}d_r^a) \\
& +\frac{i}{3}g_s(\mathcal{C}_{Hq}^{(1)})^{rr}\left[T_b^{Aa}(\Omega_{q,a}^*D_{\bar{\nu}}\Omega_q^b)G^{\bar{\mu}\bar{\nu}A}(H^\dagger D_{\bar{\mu}}H)-T_b^{Aa}(D_{\bar{\nu}}\Omega_{q,a}^*\Omega_q^b)G^{\bar{\mu}\bar{\nu}A}(D_{\bar{\mu}}H^\dagger H)\right] \\
& +\frac{1}{3}y_d^{ts}\bar{y}_d^{rs}(\mathcal{C}_{Hq}^{(1)})^{rt}\left[(\Omega_d^\dagger D_{\bar{\mu}}\Omega_d)(H^\dagger H)(H^\dagger D_{\bar{\mu}}H)+(D_{\bar{\mu}}\Omega_d^\dagger\Omega_d)(H^\dagger H)(D_{\bar{\mu}}H^\dagger H)\right] \\
& +\frac{1}{2}g_s(\mathcal{C}_{Hq}^{(1)})^{rr}\left[2T_b^{Aa}(\Omega_{q,a}^*D_{\bar{\sigma}}\Omega_q^b)\widetilde{G}^{\bar{\mu}\bar{\sigma}A}(H^\dagger D_{\bar{\mu}}H)+2T_b^{Aa}(D_{\bar{\nu}}\Omega_{q,a}^*\Omega_q^b)\widetilde{G}^{\bar{\mu}\bar{\nu}A}(D_{\bar{\mu}}H^\dagger H)\right] \\
& -\frac{1}{3}(\mathcal{C}_{Hq}^{(1)})^{rr}(D_{\bar{\nu}}\Omega_q^\dagger D_{\bar{\nu}}\Omega_q)(D_{\bar{\mu}}H^\dagger D_{\bar{\mu}}H)-\frac{1}{3}(\mathcal{C}_{Hq}^{(1)})^{rr}\left[(D_{\bar{\mu}}\Omega_q^\dagger D_{\bar{\nu}}\Omega_q)(H^\dagger D_{\bar{\mu}}D_{\bar{\nu}}H)+(D_{\bar{\nu}}\Omega_q^\dagger D_{\bar{\mu}}\Omega_q)(D_{\bar{\mu}}D_{\bar{\nu}}H^\dagger H)\right] \\
& +\frac{i}{3}(\mathcal{C}_{Hq}^{(1)})^{rr}\left[(\Omega_{q,b}^*D_{\bar{\sigma}}\Omega_q^a)(\Omega_{q,aj}^*D_{\bar{\rho}}\Omega_q^{bi})D^{\bar{\mu}}H_i^\dagger D^{\bar{\nu}}H^j\varepsilon^{\bar{\mu}\bar{\nu}\bar{\rho}\bar{\sigma}}-(D_{\bar{\nu}}\Omega_{q,a}^*\Omega_q^b)(D_{\bar{\rho}}\Omega_{q,bk}^*\Omega_q^{ai})D^{\bar{\mu}}H_i^\dagger D^{\bar{\sigma}}H^k\varepsilon^{\bar{\mu}\bar{\nu}\bar{\rho}\bar{\sigma}}\right] \\
& +\frac{i}{3}(\mathcal{C}_{Hq}^{(1)})^{rr}\left[(D_{\bar{\mu}}\Omega_{q,a}^*D_{\bar{\rho}}\Omega_q^b)(\Omega_{q,b}^*D_{\bar{\sigma}}\Omega_q^a)(H^\dagger D_{\bar{\nu}}H)\varepsilon^{\bar{\mu}\bar{\nu}\bar{\rho}\bar{\sigma}}-(D_{\bar{\nu}}\Omega_{q,a}^*\Omega_q^b)(D_{\bar{\rho}}\Omega_{q,b}^*D_{\bar{\sigma}}\Omega_q^a)(D_{\bar{\mu}}H^\dagger H)\varepsilon^{\bar{\mu}\bar{\nu}\bar{\rho}\bar{\sigma}}\right] \\
& -\frac{i}{2}g_L^2(\mathcal{C}_{Hq}^{(1)})^{tt}\left[(\Omega_{q,j}^*D_{\bar{\mu}}\Omega_q^i)H_i^\dagger(\bar{\ell}_sH\gamma^{\bar{\mu}}\ell_s^j)-(D_{\bar{\mu}}\Omega_{q,j}^*\Omega_q^k)H^j(\bar{\ell}_{ks}\gamma^{\bar{\mu}}H^\dagger\ell_s)\right] \\
& +\frac{5i}{9}g_Y(\mathcal{C}_{Hq}^{(1)})^{rr}\left[(\Omega_q^\dagger D_{\bar{\nu}}\Omega_q)B^{\bar{\mu}\bar{\nu}}(H^\dagger D_{\bar{\mu}}H)-(D_{\bar{\nu}}\Omega_q^\dagger\Omega_q)B^{\bar{\mu}\bar{\nu}}(D_{\bar{\mu}}H^\dagger H)\right] \\
& -\frac{2i}{3}g_L(\mathcal{C}_{Hq}^{(1)})^{rr}\left[t_k^{Ij}(D_{\bar{\mu}}\Omega_{q,j}^*\Omega_q^k)W^{\bar{\mu}\bar{\nu}I}(H^\dagger D_{\bar{\nu}}H)+t_k^{Ij}(\Omega_{q,j}^*D_{\bar{\nu}}\Omega_q^k)W^{\bar{\mu}\bar{\nu}I}(D_{\bar{\mu}}H^\dagger H)\right] \\
& +\frac{2}{3}\bar{y}_d^{ts}(\mathcal{C}_{Hq}^{(1)})^{tr}(D_{\bar{\mu}}\Omega_{q,aj}^*\Omega_q^{bi})D^{\bar{\mu}}H_i^\dagger(\bar{d}_{bs}q_r^{aj})-\frac{1}{6}\bar{y}_d^{ts}(\mathcal{C}_{Hq}^{(1)})^{tr}(D_{\bar{\mu}}\Omega_{q,aj}^*\Omega_q^{bi})H_i^\dagger(\bar{d}_{bs}D^{\bar{\mu}}q_r^{aj}) \\
& -\frac{1}{6}\bar{y}_d^{ts}(\mathcal{C}_{Hq}^{(1)})^{tr}(D_{\bar{\mu}}\Omega_{q,aj}^*\Omega_q^{bi})H_i^\dagger(D^{\bar{\mu}}\bar{d}_{bs}q_r^{aj})-\frac{2}{3}(\mathcal{C}_{Hq}^{(1)})^{rr}(D_{\bar{\mu}}\Omega_q^\dagger D_{\bar{\nu}}\Omega_q)(D_{\bar{\mu}}H^\dagger D_{\bar{\nu}}H)
\end{aligned}$$

$$\begin{aligned}
& -\frac{2i}{3}(\mathcal{C}_{Hq}^{(1)})^{rr} \left[ (D_{\bar{\mu}}\Omega_{q,a}^* D_{\bar{\rho}}\Omega_q^b)(\Omega_{q,bk}^* D_{\bar{\sigma}}\Omega_q^{ai}) H_i^\dagger D^{\bar{\nu}} H^k \varepsilon^{\bar{\mu}\bar{\nu}\bar{\rho}\bar{\sigma}} - (D_{\bar{\rho}}\Omega_{q,b}^* D_{\bar{\sigma}}\Omega_q^a)(D_{\bar{\nu}}\Omega_{q,aj}^* \Omega_q^{bi}) D^{\bar{\mu}} H_i^\dagger H^j \varepsilon^{\bar{\mu}\bar{\nu}\bar{\rho}\bar{\sigma}} \right] \\
& +\frac{2i}{3}(\mathcal{C}_{Hq}^{(1)})^{rr} \left[ (D_{\bar{\mu}}\Omega_{q,aj}^* D_{\bar{\rho}}\Omega_q^{bi})(\Omega_{q,bk}^* D_{\bar{\sigma}}\Omega_q^{aj}) H_i^\dagger D^{\bar{\nu}} H^k \varepsilon^{\bar{\mu}\bar{\nu}\bar{\rho}\bar{\sigma}} - (D_{\bar{\nu}}\Omega_{q,aj}^* \Omega_q^{bi})(D_{\bar{\rho}}\Omega_{q,bk}^* D_{\bar{\sigma}}\Omega_q^{aj}) D^{\bar{\mu}} H_i^\dagger H^k \varepsilon^{\bar{\mu}\bar{\nu}\bar{\rho}\bar{\sigma}} \right] \\
& -\frac{2}{3}y_u^{st}(\mathcal{C}_{Hq}^{(1)})^{rs} (D_{\bar{\mu}}\Omega_{q,a}^* \Omega_q^b)(\bar{q}_{br} D_{\bar{\mu}} \tilde{H} u_t^a) - \frac{2}{3}y_u^{st}(\mathcal{C}_{Hq}^{(1)})^{rs} \varepsilon^{kj} (D_{\bar{\mu}}\Omega_{q,aj}^* \Omega_q^{bi}) D^{\bar{\mu}} H_i^\dagger (\bar{q}_{bkr} u_t^a) \\
& -\frac{2}{3}\bar{y}_u^{rs}(\mathcal{C}_{Hq}^{(1)})^{rt} \bar{\varepsilon}_{jk} (\Omega_{q,ai}^* D_{\bar{\mu}}\Omega_q^{bk}) D^{\bar{\mu}} H^i (\bar{u}_{bs} q_t^{aj}) - \frac{2}{3}\bar{y}_u^{rs}(\mathcal{C}_{Hq}^{(1)})^{rt} (\Omega_{q,a}^* D_{\bar{\mu}}\Omega_q^b)(\bar{u}_{bs} D_{\bar{\mu}} \tilde{H}^\dagger q_t^a) \\
& -\frac{5i}{6}\bar{y}_d^{ts}(\mathcal{C}_{Hq}^{(1)})^{tr} (D_{\bar{\nu}}\Omega_{q,aj}^* \Omega_q^{bi}) D^{\bar{\mu}} H_i^\dagger (\bar{d}_{bs} \sigma^{\bar{\mu}\bar{\nu}} q_r^{aj}) - \frac{5i}{6}y_u^{st}(\mathcal{C}_{Hq}^{(1)})^{rs} (D_{\bar{\nu}}\Omega_{q,a}^* \Omega_q^b)(\bar{q}_{br} D_{\bar{\mu}} \tilde{H} \sigma^{\bar{\mu}\bar{\nu}} u_t^a) \\
& +\frac{5i}{6}y_d^{tr}(\mathcal{C}_{Hq}^{(1)})^{st} (\Omega_{q,ai}^* D_{\bar{\nu}}\Omega_q^{bj}) D^{\bar{\mu}} H^i (\bar{q}_{bjs} \sigma^{\bar{\mu}\bar{\nu}} d_r^a) - \frac{5i}{6}y_u^{st}(\mathcal{C}_{Hq}^{(1)})^{rs} \varepsilon^{kj} (D_{\bar{\nu}}\Omega_{q,aj}^* \Omega_q^{bi}) D^{\bar{\mu}} H_i^\dagger (\bar{q}_{bkr} \sigma^{\bar{\mu}\bar{\nu}} u_t^a) \\
& +\frac{5i}{6}\bar{y}_u^{rs}(\mathcal{C}_{Hq}^{(1)})^{rt} \bar{\varepsilon}_{jk} (\Omega_{q,ai}^* D_{\bar{\nu}}\Omega_q^{bk}) D^{\bar{\mu}} H^i (\bar{u}_{bs} \sigma^{\bar{\mu}\bar{\nu}} q_t^{aj}) + \frac{5i}{6}\bar{y}_u^{rs}(\mathcal{C}_{Hq}^{(1)})^{rt} (\Omega_{q,a}^* D_{\bar{\nu}}\Omega_q^b)(\bar{u}_{bs} \sigma^{\bar{\mu}\bar{\nu}} D_{\bar{\mu}} \tilde{H}^\dagger q_t^a) \\
& +ig_L(\mathcal{C}_{Hq}^{(1)})^{rr} \left[ t_k^{Ii} (D_{\bar{\mu}}\Omega_{q,j}^* \Omega_q^k) H_i^\dagger D^{\bar{\nu}} H^j W^{\bar{\mu}\bar{\nu}I} + t_k^{Ij} (\Omega_{q,j}^* D_{\bar{\nu}}\Omega_q^i) D^{\bar{\mu}} H_i^\dagger H^k W^{\bar{\mu}\bar{\nu}I} \right] \\
& +ig_L(\mathcal{C}_{Hq}^{(1)})^{rr} \left[ t_k^{Ij} (\Omega_{q,j}^* D_{\bar{\nu}}\Omega_q^i) H_i^\dagger D^{\bar{\mu}} H^k W^{\bar{\mu}\bar{\nu}I} - t_k^{Ii} (D_{\bar{\nu}}\Omega_{q,j}^* \Omega_q^k) D^{\bar{\mu}} H_i^\dagger H^j W^{\bar{\mu}\bar{\nu}I} \right] \\
& +\left[ \frac{1}{4}(\mathcal{C}_{Hq}^{(1)})^{rr} \left[ g_L^2 + g_Y^2 \right] - \frac{4}{3}y_u^{ts}\bar{y}_u^{rs}(\mathcal{C}_{Hq}^{(1)})^{rt} \right] \left[ (\Omega_q^\dagger D_{\bar{\mu}}\Omega_q)(H^\dagger H)(H^\dagger D_{\bar{\mu}}H) + (D_{\bar{\mu}}\Omega_q^\dagger\Omega_q)(H^\dagger H)(D_{\bar{\mu}}H^\dagger H) \right] \\
& +\frac{4}{3}(\mathcal{C}_{Hq}^{(1)})^{rt} \left[ y_u^{ts}\bar{y}_u^{rs} - y_d^{ts}\bar{y}_d^{rs} \right] \left[ (\Omega_{q,k}^* D_{\bar{\mu}}\Omega_q^j)(H^\dagger D_{\bar{\mu}}H) H_j^\dagger H^k + (D_{\bar{\mu}}\Omega_{q,k}^* \Omega_q^j)(D_{\bar{\mu}}H^\dagger H) H_j^\dagger H^k \right] \\
& -\frac{5}{6}g_L(\mathcal{C}_{Hq}^{(1)})^{rr} \left[ 2t_k^{Ij} (\Omega_{q,j}^* D_{\bar{\sigma}}\Omega_q^k) \widetilde{W}^{\bar{\mu}\bar{\sigma}I} (D_{\bar{\mu}}H^\dagger H) - 2t_k^{Ij} (D_{\bar{\mu}}\Omega_{q,j}^* \Omega_q^k) \widetilde{W}^{\bar{\mu}\bar{\nu}I} (H^\dagger D_{\bar{\nu}}H) \right] \\
& -(\mathcal{C}_{Hq}^{(1)})^{rr} \left[ (\Omega_q^\dagger D_{\bar{\nu}}\Omega_q)(D_{\bar{\mu}}H^\dagger D_{\bar{\mu}}D_{\bar{\nu}}H) + (D_{\bar{\nu}}\Omega_q^\dagger\Omega_q)(D_{\bar{\mu}}D_{\bar{\nu}}H^\dagger D_{\bar{\mu}}H) \right], \tag{3.36}
\end{aligned}$$

$$\begin{aligned}
\Gamma_\Omega^{(1)}[\mathcal{O}_{Hq}^{(3)}] &= \frac{i}{36} \left[ 5(\mathcal{C}_{Hq}^{(3)})^{sr} \left[ 3g_L^2 - g_Y^2 \right] - 3 \left[ y_u^{su}\bar{y}_u^{tu}(\mathcal{C}_{Hq}^{(3)})^{tr} + y_u^{ut}\bar{y}_u^{rt}(\mathcal{C}_{Hq}^{(3)})^{su} \right] \right] (\Omega_{q,a}^* \overset{\leftrightarrow}{D}_{\bar{\mu}}\Omega_q^b)(H^\dagger H)(\bar{q}_{bs}\gamma^{\bar{\mu}}q_r^a) \\
& +\frac{i}{36} \left[ 5(\mathcal{C}_{Hq}^{(3)})^{sr} \left[ g_Y^2 + 3g_L^2 \right] - 3 \left[ y_u^{su}\bar{y}_u^{tu}(\mathcal{C}_{Hq}^{(3)})^{tr} + y_u^{ut}\bar{y}_u^{rt}(\mathcal{C}_{Hq}^{(3)})^{su} \right] \right] (\Omega_{q,a}^* \overset{\leftrightarrow}{D}_{\bar{\mu}}\Omega_q^b)(\bar{q}_{bs}H\gamma^{\bar{\mu}}H^\dagger q_r^a) \\
& +\frac{i}{36} \left[ 3y_u^{su}\bar{y}_u^{tu}(\mathcal{C}_{Hq}^{(3)})^{tr} + 3y_u^{ut}\bar{y}_u^{rt}(\mathcal{C}_{Hq}^{(3)})^{su} + 5(\mathcal{C}_{Hq}^{(3)})^{sr} \left[ g_Y^2 + 3g_L^2 \right] - 6y_d^{su}\bar{y}_d^{tu}(\mathcal{C}_{Hq}^{(3)})^{tr} - 6y_d^{ut}\bar{y}_d^{rt}(\mathcal{C}_{Hq}^{(3)})^{su} \right] \\
& \quad (\Omega_{q,aj}^* \overset{\leftrightarrow}{D}_{\bar{\mu}}\Omega_q^{bi}) H_i^\dagger H^j (\bar{q}_{bs}\gamma^{\bar{\mu}}q_r^a) \\
& -\frac{i}{24}(\mathcal{C}_{Hq}^{(3)})^{tt} \left[ 3g_L^2 - g_Y^2 \right] (\Omega_q^\dagger \overset{\leftrightarrow}{D}_{\bar{\mu}}\Omega_q)(H^\dagger H)(\bar{q}_s\gamma^{\bar{\mu}}q_s) \\
& -\frac{i}{12} \left[ 10g_L^2(\mathcal{C}_{Hq}^{(3)})^{sr} - y_d^{su}\bar{y}_d^{tu}(\mathcal{C}_{Hq}^{(3)})^{tr} - y_d^{ut}\bar{y}_d^{rt}(\mathcal{C}_{Hq}^{(3)})^{su} - y_u^{su}\bar{y}_u^{tu}(\mathcal{C}_{Hq}^{(3)})^{tr} - y_u^{ut}\bar{y}_u^{rt}(\mathcal{C}_{Hq}^{(3)})^{su} \right] \\
& \quad \left[ (\Omega_{q,aj}^* D_{\bar{\mu}}\Omega_q^{bi}) H_i^\dagger (\bar{q}_{bs}H\gamma^{\bar{\mu}}q_r^{aj}) - (D_{\bar{\mu}}\Omega_{q,aj}^* \Omega_q^{bk}) H^j (\bar{q}_{bks}\gamma^{\bar{\mu}}H^\dagger q_r^a) \right] \\
& +\frac{i}{12} \left[ y_d^{su}\bar{y}_d^{tu}(\mathcal{C}_{Hq}^{(3)})^{tr} + y_u^{ut}\bar{y}_u^{rt}(\mathcal{C}_{Hq}^{(3)})^{su} - y_d^{ut}\bar{y}_d^{rt}(\mathcal{C}_{Hq}^{(3)})^{su} - y_u^{su}\bar{y}_u^{tu}(\mathcal{C}_{Hq}^{(3)})^{tr} \right] \\
& \quad \left[ (\Omega_{q,aj}^* D_{\bar{\mu}}\Omega_q^{bi}) H_i^\dagger (\bar{q}_{bs}H\gamma^{\bar{\mu}}q_r^{aj}) + (D_{\bar{\mu}}\Omega_{q,aj}^* \Omega_q^{bk}) H^j (\bar{q}_{bks}\gamma^{\bar{\mu}}H^\dagger q_r^a) \right] \\
& -\frac{i}{12}g_Y^2(\mathcal{C}_{Hq}^{(3)})^{tt} (\Omega_q^\dagger \overset{\leftrightarrow}{D}_{\bar{\mu}}\Omega_q)(H^\dagger H)(\bar{d}_s\gamma^{\bar{\mu}}d_s) + \frac{i}{12}(\mathcal{C}_{Hq}^{(3)})^{tt} \left[ 3g_L^2 - g_Y^2 \right] (\Omega_{q,j}^* \overset{\leftrightarrow}{D}_{\bar{\mu}}\Omega_q^i) H_i^\dagger H^j (\bar{q}_s\gamma^{\bar{\mu}}q_s) \\
& +\frac{i}{8}(\mathcal{C}_{Hq}^{(3)})^{tt} \left[ g_L^2 - g_Y^2 \right] (\Omega_q^\dagger \overset{\leftrightarrow}{D}_{\bar{\mu}}\Omega_q)(H^\dagger H)(\bar{\ell}_s\gamma^{\bar{\mu}}\ell_s)
\end{aligned}$$

$$\begin{aligned}
& + \frac{1}{6} g_Y (\mathcal{C}_{Hq}^{(3)})^{rr} \left[ 2(D_{\bar{\nu}} \Omega_{q,j}^* \Omega_q^i) D^{\bar{\mu}} H_i^\dagger H^j \widetilde{B}^{\bar{\mu}\bar{\nu}} + 2(\Omega_{q,j}^* D_{\bar{\sigma}} \Omega_q^i) H_i^\dagger D^{\bar{\mu}} H^j \widetilde{B}^{\bar{\mu}\bar{\sigma}} \right] \\
& + \frac{1}{6} g_L (\mathcal{C}_{Hq}^{(3)})^{rr} \left[ 2t_l^{Ik} (\Omega_{q,a}^* D_{\bar{\rho}} \Omega_q^b) (\Omega_{q,bk}^* D_{\bar{\sigma}} \Omega_q^{ai}) H_i^\dagger H^l \widetilde{W}^{\bar{\rho}\bar{\sigma}I} - 2t_l^{Ii} (D_{\bar{\nu}} \Omega_{q,b}^* \Omega_q^a) (D_{\bar{\mu}} \Omega_{q,a,j}^* \Omega_q^{bl}) H_i^\dagger H^j \widetilde{W}^{\bar{\mu}\bar{\nu}I} \right] \\
& + \frac{1}{6} \left[ 3g_L^2 (\mathcal{C}_{Hq}^{(3)})^{rr} - 8(\mathcal{C}_{Hq}^{(3)})^{rt} \left[ y_d^{ts} \bar{y}_d^{rs} + y_u^{ts} \bar{y}_u^{rs} \right] \right] \left[ (D_{\bar{\mu}} \Omega_{q,k}^* \Omega_q^j) (H^\dagger H) D^{\bar{\mu}} H_j^\dagger H^k + (\Omega_{q,k}^* D_{\bar{\mu}} \Omega_q^j) (H^\dagger H) H_j^\dagger D^{\bar{\mu}} H^k \right] \\
& + \frac{1}{6} \bar{y}_d^{ts} (\mathcal{C}_{Hq}^{(3)})^{tr} (D_{\bar{\mu}} \Omega_{q,a,j}^* \Omega_q^{bi}) H_i^\dagger (\bar{d}_{bs} D^{\bar{\mu}} q_r^{aj}) + \frac{1}{6} \bar{y}_d^{ts} (\mathcal{C}_{Hq}^{(3)})^{tr} (D_{\bar{\mu}} \Omega_{q,a,j}^* \Omega_q^{bi}) H_i^\dagger (D^{\bar{\mu}} \bar{d}_{bs} q_r^{aj}) \\
& + \frac{1}{6} y_d^{tr} (\mathcal{C}_{Hq}^{(3)})^{st} (\Omega_{q,ai}^* D_{\bar{\mu}} \Omega_q^{bj}) H^i (\bar{q}_{bjs} D^{\bar{\mu}} d_r^a) + \frac{1}{6} y_d^{tr} (\mathcal{C}_{Hq}^{(3)})^{st} (\Omega_{q,ai}^* D_{\bar{\mu}} \Omega_q^{bj}) H^i (D^{\bar{\mu}} \bar{q}_{bjs} d_r^a) \\
& + \frac{1}{6} y_u^{st} (\mathcal{C}_{Hq}^{(3)})^{rs} \varepsilon^{kj} (D_{\bar{\mu}} \Omega_{q,a,j}^* D_{\bar{\mu}} \Omega_q^{bi}) H_i^\dagger (\bar{q}_{bkr} u_t^a) + \frac{1}{6} y_u^{st} (\mathcal{C}_{Hq}^{(3)})^{rs} \varepsilon^{kj} (D_{\bar{\mu}} \Omega_{q,a,j}^* \Omega_q^{bi}) H_i^\dagger (\bar{q}_{bkr} D^{\bar{\mu}} u_t^a) \\
& + \frac{1}{6} y_u^{st} (\mathcal{C}_{Hq}^{(3)})^{rs} \varepsilon^{kj} (D_{\bar{\mu}} \Omega_{q,a,j}^* \Omega_q^{bi}) H_i^\dagger (D^{\bar{\mu}} \bar{q}_{bkr} u_t^a) + \frac{1}{6} \bar{y}_u^{rs} (\mathcal{C}_{Hq}^{(3)})^{rt} \bar{\varepsilon}_{jk} (D_{\bar{\mu}} \Omega_{q,ai}^* D_{\bar{\mu}} \Omega_q^{bk}) H^i (\bar{u}_{bs} q_t^{aj}) \\
& + \frac{1}{6} \bar{y}_u^{rs} (\mathcal{C}_{Hq}^{(3)})^{rt} \bar{\varepsilon}_{jk} (\Omega_{q,ai}^* D_{\bar{\mu}} \Omega_q^{bk}) H^i (\bar{u}_{bs} D^{\bar{\mu}} q_t^{aj}) + \frac{1}{6} \bar{y}_u^{rs} (\mathcal{C}_{Hq}^{(3)})^{rt} \bar{\varepsilon}_{jk} (\Omega_{q,ai}^* D_{\bar{\mu}} \Omega_q^{bk}) H^i (D^{\bar{\mu}} \bar{u}_{bs} q_t^{aj}) \\
& + \frac{i}{6} g_Y^2 (\mathcal{C}_{Hq}^{(3)})^{tt} (\Omega_q^\dagger \overleftrightarrow{D}_{\bar{\mu}} \Omega_q) (H^\dagger H) (\bar{u}_s \gamma^{\bar{\mu}} u_s) + \frac{i}{6} g_Y^2 (\mathcal{C}_{Hq}^{(3)})^{tt} (\Omega_{q,j}^* \overleftrightarrow{D}_{\bar{\mu}} \Omega_q^i) H_i^\dagger H^j (\bar{d}_s \gamma^{\bar{\mu}} d_s) \\
& + \frac{i}{6} \left[ y_u^{su} \bar{y}_u^{tu} (\mathcal{C}_{Hq}^{(3)})^{tr} + y_u^{ut} \bar{y}_u^{rt} (\mathcal{C}_{Hq}^{(3)})^{su} \right] (\Omega_{u,a}^* \overleftrightarrow{D}_{\bar{\mu}} \Omega_u^b) (H^\dagger H) (\bar{q}_{bs} \gamma^{\bar{\mu}} q_r^a) \\
& + \frac{i}{6} \left[ y_u^{su} \bar{y}_u^{tu} (\mathcal{C}_{Hq}^{(3)})^{tr} + y_u^{ut} \bar{y}_u^{rt} (\mathcal{C}_{Hq}^{(3)})^{su} \right] (\Omega_{u,a}^* \overleftrightarrow{D}_{\bar{\mu}} \Omega_u^b) (\bar{q}_{bs} H \gamma^{\bar{\mu}} H^\dagger q_r^a) \\
& + \frac{i}{4} g_L^2 (\mathcal{C}_{Hq}^{(3)})^{tt} (\Omega_q^\dagger \overleftrightarrow{D}_{\bar{\mu}} \Omega_q) (\bar{q}_s H \gamma^{\bar{\mu}} H^\dagger q_s) + \frac{i}{4} g_Y^2 (\mathcal{C}_{Hq}^{(3)})^{tt} (\Omega_{q,j}^* \overleftrightarrow{D}_{\bar{\mu}} \Omega_q^i) H_i^\dagger H^j (\bar{\ell}_s \gamma^{\bar{\mu}} \ell_s) \\
& - \frac{i}{4} g_L^2 (\mathcal{C}_{Hq}^{(3)})^{tt} (\Omega_{q,j}^* \overleftrightarrow{D}_{\bar{\mu}} \Omega_q^k) (H^\dagger H) (\bar{\ell}_{ks} \gamma^{\bar{\mu}} \ell_s^j) \\
& + \frac{1}{3} y_d^{ts} \bar{y}_d^{rs} (\mathcal{C}_{Hq}^{(3)})^{rt} \left[ (\Omega_d^\dagger D_{\bar{\mu}} \Omega_d) (H^\dagger H) (H^\dagger D_{\bar{\mu}} H) \right. \\
& + (D_{\bar{\mu}} \Omega_d^\dagger \Omega_d) (H^\dagger H) (D_{\bar{\mu}} H^\dagger H) \left. \right] + \frac{1}{3} (\mathcal{C}_{Hq}^{(3)})^{rr} (D_{\bar{\nu}} \Omega_q^\dagger D_{\bar{\nu}} \Omega_q) (D_{\bar{\mu}} H^\dagger D_{\bar{\mu}} H) \\
& + \frac{1}{3} (\mathcal{C}_{Hq}^{(3)})^{rr} \left[ (D_{\bar{\mu}} \Omega_q^\dagger D_{\bar{\nu}} \Omega_q) (H^\dagger D_{\bar{\mu}} D_{\bar{\nu}} H) + (D_{\bar{\nu}} \Omega_q^\dagger D_{\bar{\mu}} \Omega_q) (D_{\bar{\mu}} D_{\bar{\nu}} H^\dagger H) \right] \\
& - \frac{i}{3} (\mathcal{C}_{Hq}^{(3)})^{rr} \left[ (\Omega_{q,b}^* D_{\bar{\sigma}} \Omega_q^a) (\Omega_{q,aj}^* D_{\bar{\rho}} \Omega_q^{bi}) D^{\bar{\mu}} H_i^\dagger D^{\bar{\nu}} H^j \varepsilon^{\bar{\mu}\bar{\nu}\bar{\rho}\bar{\sigma}} - (D_{\bar{\nu}} \Omega_{q,a}^* \Omega_q^b) (D_{\bar{\rho}} \Omega_{q,bk}^* \Omega_q^{ai}) D^{\bar{\mu}} H_i^\dagger D^{\bar{\sigma}} H^k \varepsilon^{\bar{\mu}\bar{\nu}\bar{\rho}\bar{\sigma}} \right] \\
& + \frac{1}{3} \bar{y}_d^{ts} (\mathcal{C}_{Hq}^{(3)})^{tr} (D_{\bar{\mu}} \Omega_{q,a}^* D_{\bar{\mu}} \Omega_q^b) (\bar{d}_{bs} H^\dagger q_r^a) + \frac{1}{3} y_d^{tr} (\mathcal{C}_{Hq}^{(3)})^{st} (D_{\bar{\mu}} \Omega_{q,a}^* D_{\bar{\mu}} \Omega_q^b) (\bar{q}_{bs} H d_r^a) \\
& - \frac{i}{3} g_Y^2 (\mathcal{C}_{Hq}^{(3)})^{tt} (\Omega_{q,j}^* \overleftrightarrow{D}_{\bar{\mu}} \Omega_q^i) H_i^\dagger H^j (\bar{u}_s \gamma^{\bar{\mu}} u_s) + \frac{i}{2} g_Y^2 (\mathcal{C}_{Hq}^{(3)})^{tt} (\Omega_{q,j}^* \overleftrightarrow{D}_{\bar{\mu}} \Omega_q^i) H_i^\dagger H^j (\bar{e}_s \gamma^{\bar{\mu}} e_s) \\
& + \frac{2}{3} (\mathcal{C}_{Hq}^{(3)})^{rr} \left[ (\Omega_{q,j}^* D_{\bar{\mu}} D_2 \Omega_q^i) D^{\bar{\mu}} H_i^\dagger H^j + (D_{\bar{\mu}} D_2 \Omega_{q,j}^* \Omega_q^i) H_i^\dagger D^{\bar{\mu}} H^j \right] \\
& + \frac{2}{3} (\mathcal{C}_{Hq}^{(3)})^{rr} (D_{\bar{\mu}} \Omega_{q,aj}^* \Omega_q^{bk}) (\Omega_{q,bk}^* D_{\bar{\nu}} \Omega_q^{ai}) D^{\bar{\mu}} H_i^\dagger D^{\bar{\nu}} H^j \\
& + \frac{2}{3} (\mathcal{C}_{Hq}^{(3)})^{rr} \left[ (D_{\bar{\nu}} \Omega_{q,aj}^* \Omega_q^{bi}) (D_{\bar{\nu}} \Omega_{q,bk}^* D_{\bar{\mu}} \Omega_q^{aj}) D^{\bar{\mu}} H_i^\dagger H^k + (D_{\bar{\mu}} \Omega_{q,aj}^* D_{\bar{\nu}} \Omega_q^{bi}) (\Omega_{q,bk}^* D_{\bar{\nu}} \Omega_q^{aj}) H_i^\dagger D^{\bar{\mu}} H^k \right] \\
& + \frac{2}{3} (\mathcal{C}_{Hq}^{(3)})^{rr} (D_{\bar{\mu}} \Omega_{q,aj}^* \Omega_q^{bi}) (\Omega_{q,bk}^* D_{\bar{\nu}} \Omega_q^{aj}) D^{\bar{\mu}} H_i^\dagger D^{\bar{\nu}} H^k
\end{aligned}$$

$$\begin{aligned}
& + \frac{2}{3}(\mathcal{C}_{Hq}^{(3)})^{rr} \left[ (D_{\bar{\mu}}\Omega_{q,aj}^*\Omega_q^{bi})(\Omega_{q,bk}^*D_2\Omega_q^{aj})D^{\bar{\mu}}H_i^\dagger H^k + (D_2\Omega_{q,aj}^*\Omega_q^{bi})(\Omega_{q,bk}^*D_{\bar{\nu}}\Omega_q^{aj})H_i^\dagger D^{\bar{\nu}}H^k \right] \\
& + \frac{2}{3}(\mathcal{C}_{Hq}^{(3)})^{rr} \left[ (D_{\bar{\mu}}\Omega_{q,aj}^*\Omega_q^{bi})(D_{\bar{\nu}}\Omega_{q,bk}^*D_{\bar{\nu}}\Omega_q^{aj})D^{\bar{\mu}}H_i^\dagger H^k + (D_{\bar{\mu}}\Omega_{q,aj}^*D_{\bar{\mu}}\Omega_q^{bi})(\Omega_{q,bk}^*D_{\bar{\nu}}\Omega_q^{aj})H_i^\dagger D^{\bar{\nu}}H^k \right] \\
& + \frac{2}{3}(\mathcal{C}_{Hq}^{(3)})^{rr}(D_{\bar{\mu}}\Omega_q^\dagger D_{\bar{\nu}}\Omega_q)(D_{\bar{\mu}}H^\dagger D_{\bar{\nu}}H) + \frac{2}{3}y_u^{st}(\mathcal{C}_{Hq}^{(3)})^{rs}(D_{\bar{\mu}}\Omega_{q,a}^*\Omega_q^b)(\bar{q}_{br}D_{\bar{\mu}}\tilde{H}u_t^a) \\
& + \frac{2}{3}\bar{g}_u^{rs}(\mathcal{C}_{Hq}^{(3)})^{rt}(\Omega_{q,a}^*D_{\bar{\mu}}\Omega_q^b)(\bar{u}_{bs}D_{\bar{\mu}}\tilde{H}^\dagger q_t^a) \\
& + \frac{5}{6}g_L(\mathcal{C}_{Hq}^{(3)})^{rr} \left[ 2t_k^{Ij}(\Omega_{q,j}^*D_{\bar{\sigma}}\Omega_q^k)\widetilde{W}^{\bar{\mu}\bar{\sigma}I}(D_{\bar{\mu}}H^\dagger H) - 2t_k^{Ij}(D_{\bar{\mu}}\Omega_{q,j}^*\Omega_q^k)\widetilde{W}^{\bar{\mu}\bar{\nu}I}(H^\dagger D_{\bar{\nu}}H) \right] \\
& + \left[ \frac{4}{3}y_u^{ts}\bar{g}_u^{rs}(\mathcal{C}_{Hq}^{(3)})^{rt} - \frac{1}{4}(\mathcal{C}_{Hq}^{(3)})^{rr} \left[ g_L^2 + g_Y^2 \right] \right] \left[ (\Omega_q^\dagger D_{\bar{\mu}}\Omega_q)(H^\dagger H)(H^\dagger D_{\bar{\mu}}H) + (D_{\bar{\mu}}\Omega_q^\dagger\Omega_q)(H^\dagger H)(D_{\bar{\mu}}H^\dagger H) \right] \\
& + \frac{4}{3}y_d^{tr}(\mathcal{C}_{Hq}^{(3)})^{st}(\Omega_{q,a}^*D_{\bar{\mu}}\Omega_q^b)(\bar{q}_{bs}D_{\bar{\mu}}Hd_r^a) \\
& - \frac{1}{12}g_Y(\mathcal{C}_{Hq}^{(3)})^{rr} \left[ 2(\Omega_{q,b}^*D_{\bar{\sigma}}\Omega_q^a)(\Omega_{q,aj}^*D_{\bar{\rho}}\Omega_q^{bi})H_i^\dagger H^j\tilde{B}^{\bar{\rho}\bar{\sigma}} - 2(D_{\bar{\mu}}\Omega_{q,a}^*\Omega_q^b)(D_{\bar{\nu}}\Omega_{q,bk}^*\Omega_q^{ai})H_i^\dagger H^k\tilde{B}^{\bar{\mu}\bar{\nu}} \right] \\
& - \frac{1}{12}g_Y(\mathcal{C}_{Hq}^{(3)})^{rr} \left[ 2(\Omega_q^\dagger D_{\bar{\sigma}}\Omega_q)\tilde{B}^{\bar{\mu}\bar{\sigma}}(H^\dagger D_{\bar{\mu}}H) + 2(D_{\bar{\nu}}\Omega_q^\dagger\Omega_q)\tilde{B}^{\bar{\mu}\bar{\nu}}(D_{\bar{\mu}}H^\dagger H) \right] \\
& - \frac{1}{6}y_u^{st}(\mathcal{C}_{Hq}^{(3)})^{rs}(D_{\bar{\mu}}\Omega_{q,a}^*D_{\bar{\mu}}\Omega_q^b)(\bar{q}_{br}\tilde{H}u_t^a) - \frac{1}{6}y_u^{st}(\mathcal{C}_{Hq}^{(3)})^{rs}(D_{\bar{\mu}}\Omega_{q,a}^*\Omega_q^b)(\bar{q}_{br}\tilde{H}D^{\bar{\mu}}u_t^a) \\
& - \frac{1}{6}y_u^{st}(\mathcal{C}_{Hq}^{(3)})^{rs}(D_{\bar{\mu}}\Omega_{q,a}^*\Omega_q^b)(D^{\bar{\mu}}\bar{q}_{br}\tilde{H}u_t^a) - \frac{1}{6}y_d^{tr}(\mathcal{C}_{Hq}^{(3)})^{st}(D_{\bar{\mu}}\Omega_{q,ai}^*D_{\bar{\mu}}\Omega_q^{bj})H^i(\bar{q}_{bj}s d_r^a) \\
& - \frac{1}{6}\bar{g}_u^{rs}(\mathcal{C}_{Hq}^{(3)})^{rt}(D_{\bar{\mu}}\Omega_{q,a}^*D_{\bar{\mu}}\Omega_q^b)(\bar{u}_{bs}\tilde{H}^\dagger q_t^a) - \frac{1}{6}\bar{g}_u^{rs}(\mathcal{C}_{Hq}^{(3)})^{rt}(\Omega_{q,a}^*D_{\bar{\mu}}\Omega_q^b)(\bar{u}_{bs}\tilde{H}^\dagger D^{\bar{\mu}}q_t^a) \\
& - \frac{1}{6}\bar{g}_u^{rs}(\mathcal{C}_{Hq}^{(3)})^{rt}(\Omega_{q,a}^*D_{\bar{\mu}}\Omega_q^b)(D^{\bar{\mu}}\bar{u}_{bs}\tilde{H}^\dagger q_t^a) - \frac{i}{6} \left[ y_d^{su}\bar{y}_d^{tu}(\mathcal{C}_{Hq}^{(3)})^{tr} + y_d^{ut}\bar{y}_d^{rt}(\mathcal{C}_{Hq}^{(3)})^{su} \right] (\Omega_{d,a}^*\overset{\leftrightarrow}{D}_{\bar{\mu}}\Omega_d^b)(\bar{q}_{bs}H\gamma^{\bar{\mu}}H^\dagger q_r^a) \\
& - \frac{i}{4}g_Y^2(\mathcal{C}_{Hq}^{(3)})^{tt}(\Omega_q^\dagger\overset{\leftrightarrow}{D}_{\bar{\mu}}\Omega_q)(H^\dagger H)(\bar{e}_s\gamma^{\bar{\mu}}e_s) + \frac{i}{3}g_Y(\mathcal{C}_{Hq}^{(3)})^{rr}(D_{\bar{\mu}}\Omega_{q,aj}^*\Omega_q^{bi})(\Omega_{q,bk}^*D_{\bar{\nu}}\Omega_q^{aj})H_i^\dagger H^k B^{\bar{\mu}\bar{\nu}} \\
& + \frac{i}{3}g_L(\mathcal{C}_{Hq}^{(3)})^{rr}t_l^{Ik}(D_{\bar{\mu}}\Omega_{q,aj}^*\Omega_q^{bl})(\Omega_{q,bk}^*D_{\bar{\nu}}\Omega_q^{aj})W^{\bar{\mu}\bar{\nu}I}(H^\dagger H) \\
& - \frac{i}{3}g_s(\mathcal{C}_{Hq}^{(3)})^{rr} \left[ T_b^{Aa}(\Omega_{q,a}^*D_{\bar{\nu}}\Omega_q^b)G^{\bar{\mu}\bar{\nu}A}(H^\dagger D_{\bar{\mu}}H) - T_b^{Aa}(D_{\bar{\nu}}\Omega_{q,a}^*\Omega_q^b)G^{\bar{\mu}\bar{\nu}A}(D_{\bar{\mu}}H^\dagger H) \right] \\
& + \frac{1}{2}g_Y^2(\mathcal{C}_{Hq}^{(3)})^{rr} \left[ (\Omega_{q,k}^*D_{\bar{\mu}}\Omega_q^j)(H^\dagger D_{\bar{\mu}}H)H_j^\dagger H^k + (D_{\bar{\mu}}\Omega_{q,k}^*\Omega_q^j)(D_{\bar{\mu}}H^\dagger H)H_j^\dagger H^k \right] \\
& - \frac{1}{3}y_u^{ts}\bar{g}_u^{rs}(\mathcal{C}_{Hq}^{(3)})^{rt} \left[ (\Omega_u^\dagger D_{\bar{\mu}}\Omega_u)(H^\dagger H)(H^\dagger D_{\bar{\mu}}H) + (D_{\bar{\mu}}\Omega_u^\dagger\Omega_u)(H^\dagger H)(D_{\bar{\mu}}H^\dagger H) \right] \\
& - \frac{1}{3}\bar{y}_d^{ts}(\mathcal{C}_{Hq}^{(3)})^{tr}(D_{\bar{\mu}}\Omega_{q,a}^*\Omega_q^b)(\bar{d}_{bs}H^\dagger D^{\bar{\mu}}q_r^a) \\
& - \frac{1}{3}\bar{y}_d^{ts}(\mathcal{C}_{Hq}^{(3)})^{tr}(D_{\bar{\mu}}\Omega_{q,a}^*\Omega_q^b)(D^{\bar{\mu}}\bar{d}_{bs}H^\dagger q_r^a) - \frac{1}{3}y_d^{tr}(\mathcal{C}_{Hq}^{(3)})^{st}(\Omega_{q,a}^*D_{\bar{\mu}}\Omega_q^b)(\bar{q}_{bs}HD^{\bar{\mu}}d_r^a) \\
& - \frac{1}{3}y_d^{tr}(\mathcal{C}_{Hq}^{(3)})^{st}(\Omega_{q,a}^*D_{\bar{\mu}}\Omega_q^b)(D^{\bar{\mu}}\bar{q}_{bs}HD^{\bar{\mu}}d_r^a) + \frac{i}{3} \left[ y_d^{su}\bar{y}_d^{tu}(\mathcal{C}_{Hq}^{(3)})^{tr} + y_d^{ut}\bar{y}_d^{rt}(\mathcal{C}_{Hq}^{(3)})^{su} \right] (\Omega_{d,a}^*\overset{\leftrightarrow}{D}_{\bar{\mu}}\Omega_d^b)(H^\dagger H)(\bar{q}_{bs}\gamma^{\bar{\mu}}q_r^a) \\
& - \frac{1}{2}g_s(\mathcal{C}_{Hq}^{(3)})^{rr} \left[ 2T_b^{Aa}(\Omega_{q,a}^*D_{\bar{\sigma}}\Omega_q^b)\tilde{G}^{\bar{\mu}\bar{\sigma}A}(H^\dagger D_{\bar{\mu}}H) + 2T_b^{Aa}(D_{\bar{\nu}}\Omega_{q,a}^*\Omega_q^b)\tilde{G}^{\bar{\mu}\bar{\nu}A}(D_{\bar{\mu}}H^\dagger H) \right] \\
& - \frac{i}{2}g_L^2(\mathcal{C}_{Hq}^{(3)})^{tt} \left[ (\Omega_{q,j}^*D_{\bar{\mu}}\Omega_q^i)H_i^\dagger(\bar{q}_sH\gamma^{\bar{\mu}}q_s^j) - (D_{\bar{\mu}}\Omega_{q,j}^*\Omega_q^k)H^j(\bar{q}_{ks}\gamma^{\bar{\mu}}H^\dagger q_s) \right]
\end{aligned}$$

$$\begin{aligned}
& -\frac{5i}{9}g_Y(\mathcal{C}_{Hq}^{(3)})^{rr}\left[(\Omega_q^\dagger D_{\bar{\nu}}\Omega_q)B^{\bar{\mu}\bar{\nu}}(H^\dagger D_{\bar{\mu}}H) - (D_{\bar{\nu}}\Omega_q^\dagger\Omega_q)B^{\bar{\mu}\bar{\nu}}(D_{\bar{\mu}}H^\dagger H)\right] - \frac{2}{3}(\mathcal{C}_{Hq}^{(3)})^{rr}(D_{\bar{\nu}}\Omega_{q,j}^*D_{\bar{\nu}}\Omega_q^i)D^{\bar{\mu}}H_i^\dagger D^{\bar{\mu}}H^j \\
& - \frac{2}{3}(\mathcal{C}_{Hq}^{(3)})^{rr}\left[(D_{\bar{\nu}}\Omega_{q,j}^*D_{\bar{\mu}}\Omega_q^i)D^{\bar{\mu}}D^{\bar{\nu}}H_i^\dagger H^j + (D_{\bar{\mu}}\Omega_{q,j}^*D_{\bar{\nu}}\Omega_q^i)H_i^\dagger D^{\bar{\mu}}D^{\bar{\nu}}H^j\right] \\
& - \frac{2}{3}(\mathcal{C}_{Hq}^{(3)})^{rr}(D_{\bar{\nu}}\Omega_{q,aj}^*\Omega_q^{bi})(\Omega_{q,bk}^*D_{\bar{\nu}}\Omega_q^{aj})D^{\bar{\mu}}H_i^\dagger D^{\bar{\mu}}H^k \\
& - \frac{2}{3}(\mathcal{C}_{Hq}^{(3)})^{rr}\left[(D_{\bar{\nu}}\Omega_{q,aj}^*\Omega_q^{bi})(D_{\bar{\mu}}\Omega_{q,bk}^*D_{\bar{\nu}}\Omega_q^{aj})D^{\bar{\mu}}H_i^\dagger H^k + (D_{\bar{\mu}}\Omega_{q,aj}^*D_{\bar{\nu}}\Omega_q^{bi})(\Omega_{q,bk}^*D_{\bar{\mu}}\Omega_q^{aj})H_i^\dagger D^{\bar{\nu}}H^k\right] \\
& - \frac{2}{3}(\mathcal{C}_{Hq}^{(3)})^{rr}\left[(D_{\bar{\nu}}\Omega_{q,aj}^*\Omega_q^{bi})(D_{\bar{\mu}}\Omega_{q,bk}^*\Omega_q^{aj})D^{\bar{\mu}}D^{\bar{\nu}}H_i^\dagger H^k + (\Omega_{q,aj}^*D_{\bar{\mu}}\Omega_q^{bi})(\Omega_{q,bk}^*D_{\bar{\nu}}\Omega_q^{aj})H_i^\dagger D^{\bar{\mu}}D^{\bar{\nu}}H^k\right] \\
& + \frac{2i}{3}g_L(\mathcal{C}_{Hq}^{(3)})^{rr}\left[t_k^{Ii}(D_{\bar{\mu}}\Omega_{q,j}^*\Omega_q^k)H_i^\dagger D^{\bar{\nu}}H^j W^{\bar{\mu}\bar{\nu}I} + t_k^{Ij}(\Omega_{q,j}^*D_{\bar{\nu}}\Omega_q^i)D^{\bar{\mu}}H_i^\dagger H^k W^{\bar{\mu}\bar{\nu}I}\right] \\
& - \frac{2i}{3}g_L(\mathcal{C}_{Hq}^{(3)})^{rr}\left[t_k^{Ij}(\Omega_{q,j}^*D_{\bar{\nu}}\Omega_q^i)H_i^\dagger D^{\bar{\mu}}H^k W^{\bar{\mu}\bar{\nu}I} - t_k^{Ii}(D_{\bar{\nu}}\Omega_{q,j}^*\Omega_q^k)D^{\bar{\mu}}H_i^\dagger H^j W^{\bar{\mu}\bar{\nu}I}\right] \\
& + \frac{2i}{3}g_L(\mathcal{C}_{Hq}^{(3)})^{rr}\left[t_k^{Ij}(D_{\bar{\mu}}\Omega_{q,j}^*\Omega_q^k)W^{\bar{\mu}\bar{\nu}I}(H^\dagger D_{\bar{\nu}}H) + t_k^{Ij}(\Omega_{q,j}^*D_{\bar{\nu}}\Omega_q^k)W^{\bar{\mu}\bar{\nu}I}(D_{\bar{\mu}}H^\dagger H)\right] \\
& + \frac{2i}{3}(\mathcal{C}_{Hq}^{(3)})^{rr}\left[(D_{\bar{\mu}}\Omega_{q,a}^*D_{\bar{\rho}}\Omega_q^b)(\Omega_{q,bk}^*D_{\bar{\sigma}}\Omega_q^a)H_i^\dagger D^{\bar{\nu}}H^k \varepsilon^{\bar{\mu}\bar{\nu}\bar{\rho}\bar{\sigma}} - (D_{\bar{\rho}}\Omega_{q,b}^*D_{\bar{\sigma}}\Omega_q^a)(D_{\bar{\nu}}\Omega_{q,aj}^*\Omega_q^{bi})D^{\bar{\mu}}H_i^\dagger H^j \varepsilon^{\bar{\mu}\bar{\nu}\bar{\rho}\bar{\sigma}}\right] \\
& + \frac{5}{6}g_L(\mathcal{C}_{Hq}^{(3)})^{rr}\left[2t_k^{Ii}(D_{\bar{\nu}}\Omega_{q,j}^*\Omega_q^k)D^{\bar{\mu}}H_i^\dagger H^j \widetilde{W}^{\bar{\mu}\bar{\nu}I} + 2t_k^{Ij}(\Omega_{q,j}^*D_{\bar{\sigma}}\Omega_q^i)H_i^\dagger D^{\bar{\mu}}H^k \widetilde{W}^{\bar{\mu}\bar{\sigma}I}\right] \\
& - \frac{2}{3}y_d^{tr}(\mathcal{C}_{Hq}^{(3)})^{st}(\Omega_{q,ai}^*D_{\bar{\mu}}\Omega_q^{bj})D^{\bar{\mu}}H^i(\bar{q}_{bjs}d_r^a) - \frac{2}{3}y_u^{st}(\mathcal{C}_{Hq}^{(3)})^{rs}\varepsilon^{kj}(D_{\bar{\mu}}\Omega_{q,aj}^*\Omega_q^{bi})D^{\bar{\mu}}H_i^\dagger(\bar{q}_{bkr}u_t^a) \\
& - \frac{2}{3}\bar{y}_u^{rs}(\mathcal{C}_{Hq}^{(3)})^{rt}\bar{\varepsilon}_{jk}(\Omega_{q,ai}^*D_{\bar{\mu}}\Omega_q^{bk})D^{\bar{\mu}}H^i(\bar{u}_{bs}q_t^{aj}) + \frac{5i}{6}\bar{y}_d^{ts}(\mathcal{C}_{Hq}^{(3)})^{tr}(D_{\bar{\nu}}\Omega_{q,aj}^*\Omega_q^{bi})D^{\bar{\mu}}H_i^\dagger(\bar{d}_{bs}\sigma^{\bar{\mu}\bar{\nu}}q_r^{aj}) \\
& + \frac{5i}{6}y_u^{st}(\mathcal{C}_{Hq}^{(3)})^{rs}(D_{\bar{\nu}}\Omega_{q,a}^*\Omega_q^b)(\bar{q}_{br}D_{\bar{\mu}}\tilde{H}\sigma^{\bar{\mu}\bar{\nu}}u_t^a) - \frac{5i}{6}y_d^{tr}(\mathcal{C}_{Hq}^{(3)})^{st}(\Omega_{q,ai}^*D_{\bar{\nu}}\Omega_q^{bj})D^{\bar{\mu}}H^i(\bar{q}_{bjs}\sigma^{\bar{\mu}\bar{\nu}}d_r^a) \\
& - \frac{5i}{6}\bar{y}_u^{st}(\mathcal{C}_{Hq}^{(3)})^{rs}\varepsilon^{kj}(D_{\bar{\nu}}\Omega_{q,aj}^*\Omega_q^{bi})D^{\bar{\mu}}H_i^\dagger(\bar{q}_{bkr}\sigma^{\bar{\mu}\bar{\nu}}u_t^a) + \frac{5i}{6}\bar{y}_u^{rs}(\mathcal{C}_{Hq}^{(3)})^{rt}\bar{\varepsilon}_{jk}(\Omega_{q,ai}^*D_{\bar{\nu}}\Omega_q^{bk})D^{\bar{\mu}}H^i(\bar{u}_{bs}\sigma^{\bar{\mu}\bar{\nu}}q_t^{aj}) \\
& - \frac{5i}{6}\bar{y}_u^{rs}(\mathcal{C}_{Hq}^{(3)})^{rt}(\Omega_{q,a}^*D_{\bar{\nu}}\Omega_q^b)(\bar{u}_{bs}\sigma^{\bar{\mu}\bar{\nu}}D_{\bar{\mu}}\tilde{H}^\dagger q_t^a) \\
& + ig_Y(\mathcal{C}_{Hq}^{(3)})^{rr}\left[(\Omega_{q,j}^*D_{\bar{\nu}}\Omega_q^i)H_i^\dagger D^{\bar{\mu}}H^j B^{\bar{\mu}\bar{\nu}} - (D_{\bar{\nu}}\Omega_{q,j}^*\Omega_q^i)D^{\bar{\mu}}H_i^\dagger H^j B^{\bar{\mu}\bar{\nu}}\right] \\
& + g_s(\mathcal{C}_{Hq}^{(3)})^{rr}\left[2T_b^{Aa}(D_{\bar{\nu}}\Omega_{q,aj}^*\Omega_q^{bi})D^{\bar{\mu}}H_i^\dagger H^j \tilde{G}^{\bar{\mu}\bar{\nu}A} + 2T_b^{Aa}(\Omega_{q,aj}^*D_{\bar{\sigma}}\Omega_q^{bi})H_i^\dagger D^{\bar{\mu}}H^j \tilde{G}^{\bar{\mu}\bar{\sigma}A}\right] \\
& + (\mathcal{C}_{Hq}^{(3)})^{rr}\left[(\Omega_q^\dagger D_{\bar{\nu}}\Omega_q)(D_{\bar{\mu}}H^\dagger D_{\bar{\mu}}D_{\bar{\nu}}H) + (D_{\bar{\nu}}\Omega_q^\dagger\Omega_q)(D_{\bar{\mu}}D_{\bar{\nu}}H^\dagger D_{\bar{\mu}}H)\right] + \frac{4}{3}\bar{y}_d^{ts}(\mathcal{C}_{Hq}^{(3)})^{tr}(D_{\bar{\mu}}\Omega_{q,a}^*\Omega_q^b)(\bar{d}_{bs}D_{\bar{\mu}}H^\dagger q_r^a) \\
& - \frac{1}{6}\bar{y}_d^{ts}(\mathcal{C}_{Hq}^{(3)})^{tr}(D_{\bar{\mu}}\Omega_{q,aj}^*D_{\bar{\mu}}\Omega_q^{bi})H_i^\dagger(\bar{d}_{bs}q_r^{aj}) - \frac{1}{3}(\mathcal{C}_{Hq}^{(3)})^{rr}\left[(D_{\bar{\mu}}D_2\Omega_q^\dagger\Omega_q)(H^\dagger D_{\bar{\mu}}H) + (\Omega_q^\dagger D_{\bar{\mu}}D_2\Omega_q)(D_{\bar{\mu}}H^\dagger H)\right] \\
& - \frac{i}{3}(\mathcal{C}_{Hq}^{(3)})^{rr}\left[(D_{\bar{\mu}}\Omega_{q,a}^*D_{\bar{\rho}}\Omega_q^b)(\Omega_{q,b}^*D_{\bar{\sigma}}\Omega_q^a)(H^\dagger D_{\bar{\nu}}H)\varepsilon^{\bar{\mu}\bar{\nu}\bar{\rho}\bar{\sigma}} - (D_{\bar{\nu}}\Omega_{q,a}^*\Omega_q^b)(D_{\bar{\rho}}\Omega_{q,b}^*D_{\bar{\sigma}}\Omega_q^a)(D_{\bar{\mu}}H^\dagger H)\varepsilon^{\bar{\mu}\bar{\nu}\bar{\rho}\bar{\sigma}}\right] \\
& - \frac{2}{3}\bar{y}_d^{ts}(\mathcal{C}_{Hq}^{(3)})^{tr}(D_{\bar{\mu}}\Omega_{q,aj}^*\Omega_q^{bi})D^{\bar{\mu}}H_i^\dagger(\bar{d}_{bs}q_r^{aj}) \\
& - \frac{5}{6}g_L(\mathcal{C}_{Hq}^{(3)})^{rr}\left[2t_k^{Ij}(\Omega_{q,j}^*D_{\bar{\sigma}}\Omega_q^i)D^{\bar{\mu}}H_i^\dagger H^k \widetilde{W}^{\bar{\mu}\bar{\sigma}I} - 2t_k^{Ii}(D_{\bar{\mu}}\Omega_{q,j}^*\Omega_q^k)H_i^\dagger D^{\bar{\nu}}H^j \widetilde{W}^{\bar{\mu}\bar{\nu}I}\right] \\
& - \frac{4}{3}(\mathcal{C}_{Hq}^{(3)})^{rr}(D_{\bar{\mu}}\Omega_{q,j}^*D_{\bar{\nu}}\Omega_q^i)D^{\bar{\mu}}H_i^\dagger D^{\bar{\nu}}H^j - \frac{5i}{3}\bar{y}_d^{ts}(\mathcal{C}_{Hq}^{(3)})^{tr}(D_{\bar{\nu}}\Omega_{q,a}^*\Omega_q^b)(\bar{d}_{bs}\sigma^{\bar{\mu}\bar{\nu}}D_{\bar{\mu}}H^\dagger q_r^a) \\
& + \frac{5i}{3}y_d^{tr}(\mathcal{C}_{Hq}^{(3)})^{st}(\Omega_{q,a}^*D_{\bar{\nu}}\Omega_q^b)(\bar{q}_{bs}D_{\bar{\mu}}H\sigma^{\bar{\mu}\bar{\nu}}d_r^a)
\end{aligned}$$

$$- 2(\mathcal{C}_{Hq}^{(3)})^{rr} \left[ (D_{\bar{\nu}} \Omega_{q,j}^* \Omega_q^i) D^{\bar{\mu}} D^{\bar{\nu}} H_i^{\dagger} D^{\bar{\mu}} H^j + (\Omega_{q,j}^* D_{\bar{\nu}} \Omega_q^i) D^{\bar{\mu}} H_i^{\dagger} D^{\bar{\mu}} D^{\bar{\nu}} H^j \right]. \quad (3.37)$$

### 3.5 Dimension six: four-fermion operators

$$\begin{aligned} \Gamma_{\Omega}^{(1)} [\mathcal{O}_{ee}] &= \frac{2i}{3} \mathcal{C}_{ee}^{srtt} \left[ (\Omega_e^{\dagger} D_2 D_{\bar{\mu}} \Omega_e) (\bar{e}_s \gamma^{\bar{\mu}} e_r) - (D_2 D_{\bar{\nu}} \Omega_e^{\dagger} \Omega_e) (\bar{e}_s \gamma^{\bar{\nu}} e_r) \right] \\ &\quad - \frac{2i}{3} y_e^{tv} \bar{y}_e^{tu} \mathcal{C}_{ee}^{srvu} (\Omega_{\ell,j}^* \overset{\leftrightarrow}{D}_{\bar{\mu}} \Omega_{\ell}^i) H_i^{\dagger} H^j (\bar{e}_s \gamma^{\bar{\mu}} e_r) \\ &\quad + \frac{4i}{3} \mathcal{C}_{ee}^{srtt} \left[ (\Omega_e^{\dagger} D_{\bar{\nu}} \Omega_e) (D^{\bar{\mu}} \bar{e}_s \gamma^{\bar{\nu}} D^{\bar{\mu}} e_r) - (D_{\bar{\mu}} \Omega_e^{\dagger} \Omega_e) (D^{\bar{\nu}} \bar{e}_s \gamma^{\bar{\mu}} D^{\bar{\nu}} e_r) \right] \\ &\quad + \frac{4i}{3} \mathcal{C}_{ee}^{srtt} \left[ (\Omega_e^{\dagger} D_{\bar{\nu}} \Omega_e) (D^{\bar{\mu}} D^{\bar{\mu}} \bar{e}_s \gamma^{\bar{\nu}} e_r) - (D_{\bar{\mu}} \Omega_e^{\dagger} \Omega_e) (\bar{e}_s \gamma^{\bar{\mu}} D^{\bar{\nu}} D^{\bar{\nu}} e_r) \right] \\ &\quad + \frac{8i}{3} y_e^{tv} \bar{y}_e^{tu} \mathcal{C}_{ee}^{srvu} (\Omega_e^{\dagger} \overset{\leftrightarrow}{D}_{\bar{\mu}} \Omega_e) (H^{\dagger} H) (\bar{e}_s \gamma^{\bar{\mu}} e_r), \end{aligned} \quad (3.38)$$

$$\begin{aligned} \Gamma_{\Omega}^{(1)} [\mathcal{O}_{\ell\ell}] &= -\frac{i}{6} g_Y \left[ \mathcal{C}_{\ell\ell}^{srtt} - 2\mathcal{C}_{\ell\ell}^{sttr} \right] \left[ 2(\Omega_{\ell,i}^* D_{\bar{\rho}} \Omega_{\ell}^j) \tilde{B}^{\bar{\rho}\bar{\sigma}} (\bar{\ell}_{js} \gamma^{\bar{\sigma}} \ell_r^i) - 2(D_{\bar{\mu}} \Omega_{\ell,i}^* \Omega_{\ell}^j) \tilde{B}^{\bar{\mu}\bar{\sigma}} (\bar{\ell}_{js} \gamma^{\bar{\sigma}} \ell_r^i) \right] \\ &\quad + \frac{i}{4} g_Y \mathcal{C}_{\ell\ell}^{srtt} \left[ 2(\Omega_{\ell}^{\dagger} D_{\bar{\sigma}} \Omega_{\ell}) \tilde{B}^{\bar{\rho}\bar{\sigma}} (\bar{\ell}_s \gamma^{\bar{\rho}} \ell_r) + 2(D_{\bar{\mu}} \Omega_{\ell}^{\dagger} \Omega_{\ell}) \tilde{B}^{\bar{\mu}\bar{\sigma}} (\bar{\ell}_s \gamma^{\bar{\sigma}} \ell_r) \right] \\ &\quad + \frac{i}{3} \mathcal{C}_{\ell\ell}^{srtt} \left[ (\Omega_{\ell}^{\dagger} D_2 D_{\bar{\mu}} \Omega_{\ell}) (\bar{\ell}_s \gamma^{\bar{\mu}} \ell_r) - (D_2 D_{\bar{\nu}} \Omega_{\ell}^{\dagger} \Omega_{\ell}) (\bar{\ell}_s \gamma^{\bar{\nu}} \ell_r) \right] \\ &\quad + \frac{1}{3} \mathcal{C}_{\ell\ell}^{srtt} \left[ (\Omega_{\ell}^{\dagger} D_{\bar{\sigma}} \Omega_{\ell}) (D_{\bar{\mu}} \Omega_{\ell}^{\dagger} D_{\bar{\rho}} \Omega_{\ell}) \varepsilon^{\bar{\mu}\bar{\nu}\bar{\rho}\bar{\sigma}} (\bar{\ell}_s \gamma^{\bar{\nu}} \ell_r) - (D_{\bar{\mu}} \Omega_{\ell}^{\dagger} \Omega_{\ell}) (D_{\bar{\nu}} \Omega_{\ell}^{\dagger} D_{\bar{\rho}} \Omega_{\ell}) \varepsilon^{\bar{\mu}\bar{\nu}\bar{\rho}\bar{\sigma}} (\bar{\ell}_s \gamma^{\bar{\sigma}} \ell_r) \right] \\ &\quad + \frac{i}{3} \mathcal{C}_{\ell\ell}^{sttr} \left[ (\Omega_{\ell}^{\dagger} D_{\bar{\mu}} \Omega_{\ell}) (\Omega_{\ell}^{\dagger} D_{\bar{\nu}} \Omega_{\ell}) (D^{\bar{\mu}} \bar{\ell}_s \gamma^{\bar{\nu}} \ell_r) - (D_{\bar{\mu}} \Omega_{\ell}^{\dagger} \Omega_{\ell}) (D_{\bar{\nu}} \Omega_{\ell}^{\dagger} \Omega_{\ell}) (\bar{\ell}_s \gamma^{\bar{\mu}} D^{\bar{\nu}} \ell_r) \right] \\ &\quad - \frac{i}{3} \mathcal{C}_{\ell\ell}^{sttr} \left[ (\Omega_{\ell,i}^* D_{\bar{\mu}} \Omega_{\ell}^j) (\Omega_{\ell,j}^* D_{\bar{\nu}} \Omega_{\ell}^i) (D^{\bar{\mu}} \bar{\ell}_s \gamma^{\bar{\nu}} \ell_r) - (D_{\bar{\mu}} \Omega_{\ell,i}^* \Omega_{\ell}^j) (D_{\bar{\nu}} \Omega_{\ell,j}^* \Omega_{\ell}^i) (\bar{\ell}_s \gamma^{\bar{\mu}} D^{\bar{\nu}} \ell_r) \right] \\ &\quad + \frac{i}{3} \mathcal{C}_{\ell\ell}^{sttr} \left[ (\Omega_{\ell,i}^* D_2 D_{\bar{\mu}} \Omega_{\ell}^j) (\bar{\ell}_{js} \gamma^{\bar{\mu}} \ell_r^i) - (D_2 D_{\bar{\nu}} \Omega_{\ell,i}^* \Omega_{\ell}^j) (\bar{\ell}_{js} \gamma^{\bar{\nu}} \ell_r^i) \right] \\ &\quad - \frac{i}{3} \mathcal{C}_{\ell\ell}^{sttr} \left[ (D_{\bar{\mu}} D_{\bar{\nu}} \Omega_{\ell,i}^* \Omega_{\ell}^k) (\Omega_{\ell,j}^* D_{\bar{\mu}} \Omega_{\ell}^i) (\bar{\ell}_{ks} \gamma^{\bar{\nu}} \ell_r^j) - (D_{\bar{\mu}} \Omega_{\ell,i}^* \Omega_{\ell}^k) (\Omega_{\ell,j}^* D_{\bar{\mu}} D_{\bar{\nu}} \Omega_{\ell}^i) (\bar{\ell}_{ks} \gamma^{\bar{\nu}} \ell_r^j) \right] \\ &\quad + \frac{i}{3} \mathcal{C}_{\ell\ell}^{sttr} \left[ (\Omega_{\ell,i}^* D_{\bar{\nu}} \Omega_{\ell}^k) (D_{\bar{\mu}} \Omega_{\ell,j}^* D_{\bar{\nu}} \Omega_{\ell}^i) (\bar{\ell}_{ks} \gamma^{\bar{\mu}} \ell_r^j) - (D_{\bar{\mu}} \Omega_{\ell,i}^* D_{\bar{\nu}} \Omega_{\ell}^k) (D_{\bar{\mu}} \Omega_{\ell,j}^* \Omega_{\ell}^i) (\bar{\ell}_{ks} \gamma^{\bar{\nu}} \ell_r^j) \right] \\ &\quad + \frac{1}{3} \left[ \mathcal{C}_{\ell\ell}^{sttr} - 2\mathcal{C}_{\ell\ell}^{srtt} \right] \left[ (\Omega_{\ell,i}^* D_{\bar{\nu}} \Omega_{\ell}^k) (D_{\bar{\mu}} \Omega_{\ell,j}^* D_{\bar{\rho}} \Omega_{\ell}^i) \varepsilon^{\bar{\mu}\bar{\nu}\bar{\rho}\bar{\sigma}} (\bar{\ell}_{ks} \gamma^{\bar{\sigma}} \ell_r^j) - (D_{\bar{\mu}} \Omega_{\ell,i}^* D_{\bar{\rho}} \Omega_{\ell}^k) (D_{\bar{\nu}} \Omega_{\ell,j}^* \Omega_{\ell}^i) \varepsilon^{\bar{\mu}\bar{\nu}\bar{\rho}\bar{\sigma}} (\bar{\ell}_{ks} \gamma^{\bar{\sigma}} \ell_r^j) \right] \\ &\quad - \frac{i}{3} \mathcal{C}_{\ell\ell}^{sttr} \left[ (\Omega_{\ell}^{\dagger} D_{\bar{\mu}} \Omega_{\ell}) (\Omega_{\ell,i}^* D_{\bar{\nu}} \Omega_{\ell}^k) (D^{\bar{\mu}} \bar{\ell}_{ks} \gamma^{\bar{\nu}} \ell_r^i) - (D_{\bar{\mu}} \Omega_{\ell}^{\dagger} \Omega_{\ell}) (D_{\bar{\nu}} \Omega_{\ell,i}^* \Omega_{\ell}^k) (\bar{\ell}_{ks} \gamma^{\bar{\nu}} D^{\bar{\mu}} \ell_r^i) \right] \\ &\quad - \frac{i}{3} \mathcal{C}_{\ell\ell}^{sttr} \left[ (\Omega_{\ell}^{\dagger} D_{\bar{\nu}} \Omega_{\ell}) (\Omega_{\ell,j}^* D_{\bar{\mu}} \Omega_{\ell}^k) (D^{\bar{\mu}} \bar{\ell}_{ks} \gamma^{\bar{\nu}} \ell_r^j) - (D_{\bar{\mu}} \Omega_{\ell}^{\dagger} \Omega_{\ell}) (D_{\bar{\nu}} \Omega_{\ell,j}^* \Omega_{\ell}^k) (\bar{\ell}_{ks} \gamma^{\bar{\mu}} D^{\bar{\nu}} \ell_r^j) \right] \\ &\quad - \frac{i}{3} y_e^{vu} \bar{y}_e^{tu} \mathcal{C}_{\ell\ell}^{srtv} (\Omega_e^{\dagger} \overset{\leftrightarrow}{D}_{\bar{\mu}} \Omega_e) (H^{\dagger} H) (\bar{\ell}_s \gamma^{\bar{\mu}} \ell_r) - \frac{i}{3} y_e^{vu} \bar{y}_e^{tu} \mathcal{C}_{\ell\ell}^{svtr} (\Omega_e^{\dagger} \overset{\leftrightarrow}{D}_{\bar{\mu}} \Omega_e) (\bar{\ell}_s H \gamma^{\bar{\mu}} H^{\dagger} \ell_r) \\ &\quad + \frac{2i}{3} \mathcal{C}_{\ell\ell}^{srtt} \left[ (\Omega_{\ell}^{\dagger} D_{\bar{\nu}} \Omega_{\ell}) (D^{\bar{\mu}} \bar{\ell}_s \gamma^{\bar{\nu}} D^{\bar{\mu}} \ell_r) - (D_{\bar{\mu}} \Omega_{\ell}^{\dagger} \Omega_{\ell}) (D^{\bar{\nu}} \bar{\ell}_s \gamma^{\bar{\mu}} D^{\bar{\nu}} \ell_r) \right] \\ &\quad + \frac{2i}{3} \mathcal{C}_{\ell\ell}^{srtt} \left[ (\Omega_{\ell}^{\dagger} D_{\bar{\nu}} \Omega_{\ell}) (D^{\bar{\mu}} D^{\bar{\mu}} \bar{\ell}_s \gamma^{\bar{\nu}} \ell_r) - (D_{\bar{\mu}} \Omega_{\ell}^{\dagger} \Omega_{\ell}) (\bar{\ell}_s \gamma^{\bar{\mu}} D^{\bar{\nu}} D^{\bar{\nu}} \ell_r) \right] \\ &\quad + \frac{2i}{3} \mathcal{C}_{\ell\ell}^{sttr} \left[ (\Omega_{\ell,i}^* D_{\bar{\nu}} \Omega_{\ell}^j) (D^{\bar{\mu}} \bar{\ell}_{js} \gamma^{\bar{\nu}} D^{\bar{\mu}} \ell_r^i) - (D_{\bar{\mu}} \Omega_{\ell,i}^* \Omega_{\ell}^j) (D^{\bar{\nu}} \bar{\ell}_{js} \gamma^{\bar{\mu}} D^{\bar{\nu}} \ell_r^i) \right] \end{aligned}$$

$$\begin{aligned}
& + \frac{2i}{3} \mathcal{C}_{\ell\ell}^{sttr} \left[ (\Omega_{\ell,i}^* D_{\bar{\nu}} \Omega_{\ell}^j) (D^{\bar{\mu}} D^{\bar{\mu}} \bar{\ell}_{js} \gamma^{\bar{\nu}} \ell_r^i) - (D_{\bar{\mu}} \Omega_{\ell,i}^* \Omega_{\ell}^j) (\bar{\ell}_{js} \gamma^{\bar{\mu}} D^{\bar{\nu}} D^{\bar{\nu}} \ell_r^i) \right] \\
& - \frac{2i}{3} \mathcal{C}_{\ell\ell}^{sttr} \left[ (\Omega_{\ell,i}^* D_{\bar{\mu}} \Omega_{\ell}^k) (D_{\bar{\nu}} \Omega_{\ell,j}^* D_{\bar{\nu}} \Omega_{\ell}^i) (\bar{\ell}_{ks} \gamma^{\bar{\nu}} \ell_r^j) - (D_{\bar{\mu}} \Omega_{\ell,i}^* D_{\bar{\nu}} \Omega_{\ell}^k) (D_{\bar{\nu}} \Omega_{\ell,j}^* \Omega_{\ell}^i) (\bar{\ell}_{ks} \gamma^{\bar{\mu}} \ell_r^j) \right] \\
& + \frac{2i}{3} g_L \left[ 2\mathcal{C}_{\ell\ell}^{srtt} - \mathcal{C}_{\ell\ell}^{sttr} \right] \left[ 2t_j^{Ii} (\Omega_{\ell,i}^* D_{\bar{\rho}} \Omega_{\ell}^k) \widetilde{W}^{\bar{\rho}\bar{\sigma}I} (\bar{\ell}_{ks} \gamma^{\bar{\sigma}} \ell_r^j) - 2t_k^{Ij} (D_{\bar{\mu}} \Omega_{\ell,i}^* \Omega_{\ell}^k) \widetilde{W}^{\bar{\mu}\bar{\sigma}I} (\bar{\ell}_{js} \gamma^{\bar{\sigma}} \ell_r^i) \right] \\
& + \frac{2i}{3} \mathcal{C}_{\ell\ell}^{sttr} \left[ (\Omega_{\ell,i}^* D_{\bar{\nu}} \Omega_{\ell}^k) (\Omega_{\ell,j}^* D_{\bar{\mu}} \Omega_{\ell}^i) (D^{\bar{\mu}} \bar{\ell}_{ks} \gamma^{\bar{\nu}} \ell_r^j) - (D_{\bar{\mu}} \Omega_{\ell,i}^* \Omega_{\ell}^k) (D_{\bar{\nu}} \Omega_{\ell,j}^* \Omega_{\ell}^i) (\bar{\ell}_{ks} \gamma^{\bar{\nu}} D^{\bar{\mu}} \ell_r^j) \right] \\
& + \frac{2}{3} \mathcal{C}_{\ell\ell}^{srtt} \left[ (D_{\bar{\mu}} \Omega_{\ell}^{\dagger} \Omega_{\ell}) (D_{\bar{\nu}} \Omega_{\ell,j}^* \Omega_{\ell}^k) \varepsilon^{\bar{\mu}\bar{\nu}\bar{\rho}\bar{\sigma}} (\bar{\ell}_{ks} \gamma^{\bar{\rho}} D^{\bar{\sigma}} \ell_r^j) + (\Omega_{\ell}^{\dagger} D_{\bar{\sigma}} \Omega_{\ell}) (\Omega_{\ell,j}^* D_{\bar{\nu}} \Omega_{\ell}^k) \varepsilon^{\bar{\mu}\bar{\nu}\bar{\rho}\bar{\sigma}} (D^{\bar{\rho}} \bar{\ell}_{ks} \gamma^{\bar{\mu}} \ell_r^j) \right] \\
& - \frac{5i}{6} g_L \mathcal{C}_{\ell\ell}^{srtt} \left[ 2(\Omega_{\ell}^{\dagger} D_{\bar{\rho}} \Omega_{\ell}) \widetilde{W}^{\bar{\rho}\bar{\sigma}I} (\bar{\ell}_s t^I \gamma^{\bar{\sigma}} \ell_r) - 2(D_{\bar{\mu}} \Omega_{\ell}^{\dagger} \Omega_{\ell}) \widetilde{W}^{\bar{\mu}\bar{\sigma}I} (\bar{\ell}_s t^I \gamma^{\bar{\sigma}} \ell_r) \right] \\
& + \frac{4i}{3} y_e^{vu} \bar{y}_e^{tu} \mathcal{C}_{\ell\ell}^{srtv} (\Omega_{\ell,j}^* \overleftrightarrow{D}_{\bar{\mu}} \Omega_{\ell}^i) H_i^{\dagger} H^j (\bar{\ell}_s \gamma^{\bar{\mu}} \ell_r) \\
& + 2g_L \mathcal{C}_{\ell\ell}^{sttr} \left[ t_k^{Ij} (D_{\bar{\mu}} \Omega_{\ell,i}^* \Omega_{\ell}^k) W^{\bar{\mu}\bar{\nu}I} (\bar{\ell}_{js} \gamma^{\bar{\nu}} \ell_r^i) + t_j^{Ii} (\Omega_{\ell,i}^* D_{\bar{\mu}} \Omega_{\ell}^k) W^{\bar{\mu}\bar{\nu}I} (\bar{\ell}_{ks} \gamma^{\bar{\nu}} \ell_r^j) \right] \\
& - \frac{2}{3} \mathcal{C}_{\ell\ell}^{srtt} \left[ (D_{\bar{\mu}} \Omega_{\ell}^{\dagger} D_{\bar{\rho}} \Omega_{\ell}) (\Omega_{\ell,j}^* D_{\bar{\sigma}} \Omega_{\ell}^k) \varepsilon^{\bar{\mu}\bar{\nu}\bar{\rho}\bar{\sigma}} (\bar{\ell}_{ks} \gamma^{\bar{\nu}} \ell_r^j) + (D_{\bar{\mu}} \Omega_{\ell}^{\dagger} D_{\bar{\rho}} \Omega_{\ell}) (D_{\bar{\nu}} \Omega_{\ell,j}^* \Omega_{\ell}^k) \varepsilon^{\bar{\mu}\bar{\nu}\bar{\rho}\bar{\sigma}} (\bar{\ell}_{ks} \gamma^{\bar{\sigma}} \ell_r^j) \right] \\
& + \frac{4i}{3} y_e^{vu} \bar{y}_e^{tu} \mathcal{C}_{\ell\ell}^{svtr} \left[ (\Omega_{\ell,j}^* D_{\bar{\mu}} \Omega_{\ell}^i) H_i^{\dagger} (\bar{\ell}_s H \gamma^{\bar{\mu}} \ell_r^j) - (D_{\bar{\mu}} \Omega_{\ell,j}^* \Omega_{\ell}^k) H^j (\bar{\ell}_{ks} \gamma^{\bar{\mu}} H^{\dagger} \ell_r) \right], \tag{3.39}
\end{aligned}$$

$$\begin{aligned}
\Gamma_{\Omega}^{(1)} [\mathcal{O}_{\ell e}] &= \frac{i}{6} \mathcal{C}_{\ell e}^{ttsr} \left[ (\Omega_{\ell}^{\dagger} D_2 D_{\bar{\mu}} \Omega_{\ell}) (\bar{e}_s \gamma^{\bar{\mu}} e_r) - (D_2 D_{\bar{\nu}} \Omega_{\ell}^{\dagger} \Omega_{\ell}) (\bar{e}_s \gamma^{\bar{\nu}} e_r) \right] \\
& - \frac{i}{6} g_Y \mathcal{C}_{\ell e}^{ttsr} \left[ 2(\Omega_{\ell}^{\dagger} D_{\bar{\rho}} \Omega_{\ell}) \widetilde{B}^{\bar{\rho}\bar{\sigma}} (\bar{e}_s \gamma^{\bar{\sigma}} e_r) - 2(D_{\bar{\mu}} \Omega_{\ell}^{\dagger} \Omega_{\ell}) \widetilde{B}^{\bar{\mu}\bar{\sigma}} (\bar{e}_s \gamma^{\bar{\sigma}} e_r) \right] \\
& + \frac{1}{6} \mathcal{C}_{\ell e}^{ttsr} \left[ (D_{\bar{\mu}} \Omega_{\ell,i}^* D_{\bar{\rho}} \Omega_{\ell}^j) (\Omega_{\ell,j}^* D_{\bar{\sigma}} \Omega_{\ell}^i) \varepsilon^{\bar{\mu}\bar{\nu}\bar{\rho}\bar{\sigma}} (\bar{e}_s \gamma^{\bar{\nu}} e_r) - (D_{\bar{\mu}} \Omega_{\ell,i}^* \Omega_{\ell}^j) (D_{\bar{\nu}} \Omega_{\ell,j}^* D_{\bar{\rho}} \Omega_{\ell}^i) \varepsilon^{\bar{\mu}\bar{\nu}\bar{\rho}\bar{\sigma}} (\bar{e}_s \gamma^{\bar{\sigma}} e_r) \right] \\
& + \frac{i}{6} \mathcal{C}_{\ell e}^{srtt} \left[ (\Omega_{\ell}^{\dagger} D_2 D_{\bar{\mu}} \Omega_e) (\bar{\ell}_s \gamma^{\bar{\mu}} \ell_r) - (D_2 D_{\bar{\nu}} \Omega_e^{\dagger} \Omega_e) (\bar{\ell}_s \gamma^{\bar{\nu}} \ell_r) \right] \\
& - \frac{1}{6} \mathcal{C}_{\ell e}^{srtt} \left[ (\Omega_{\ell}^{\dagger} D_{\bar{\sigma}} \Omega_e) (D_{\bar{\mu}} \Omega_e^{\dagger} D_{\bar{\rho}} \Omega_e) \varepsilon^{\bar{\mu}\bar{\nu}\bar{\rho}\bar{\sigma}} (\bar{\ell}_s \gamma^{\bar{\nu}} \ell_r) + (D_{\bar{\mu}} \Omega_e^{\dagger} D_{\bar{\rho}} \Omega_e) (D_{\bar{\nu}} \Omega_e^{\dagger} \Omega_e) \varepsilon^{\bar{\mu}\bar{\nu}\bar{\rho}\bar{\sigma}} (\bar{\ell}_s \gamma^{\bar{\sigma}} \ell_r) \right] \\
& - \frac{i}{6} y_e^{vu} \bar{y}_e^{tu} \mathcal{C}_{\ell e}^{tvsr} (\Omega_e^{\dagger} \overleftrightarrow{D}_{\bar{\mu}} \Omega_e) (H^{\dagger} H) (\bar{e}_s \gamma^{\bar{\mu}} e_r) - \frac{i}{6} y_e^{tv} \bar{y}_e^{tu} \mathcal{C}_{\ell e}^{srvu} (\Omega_{\ell,j}^* \overleftrightarrow{D}_{\bar{\mu}} \Omega_{\ell}^i) H_i^{\dagger} H^j (\bar{\ell}_s \gamma^{\bar{\mu}} \ell_r) \\
& + \frac{i}{3} g_L \mathcal{C}_{\ell e}^{ttsr} \left[ 2t_j^{Ii} (\Omega_{\ell,i}^* D_{\bar{\rho}} \Omega_{\ell}^j) \widetilde{W}^{\bar{\rho}\bar{\sigma}I} (\bar{e}_s \gamma^{\bar{\sigma}} e_r) - 2t_k^{Ii} (D_{\bar{\mu}} \Omega_{\ell,i}^* \Omega_{\ell}^j) \widetilde{W}^{\bar{\mu}\bar{\sigma}I} (\bar{e}_s \gamma^{\bar{\sigma}} e_r) \right] \\
& + \frac{i}{3} \mathcal{C}_{\ell e}^{ttsr} \left[ (\Omega_{\ell}^{\dagger} D_{\bar{\nu}} \Omega_{\ell}) (D^{\bar{\mu}} \bar{e}_s \gamma^{\bar{\nu}} D^{\bar{\mu}} e_r) - (D_{\bar{\mu}} \Omega_{\ell}^{\dagger} \Omega_{\ell}) (D^{\bar{\nu}} \bar{e}_s \gamma^{\bar{\mu}} D^{\bar{\nu}} e_r) \right] \\
& + \frac{i}{3} \mathcal{C}_{\ell e}^{ttsr} \left[ (\Omega_{\ell}^{\dagger} D_{\bar{\nu}} \Omega_{\ell}) (D^{\bar{\mu}} D^{\bar{\mu}} \bar{e}_s \gamma^{\bar{\nu}} e_r) - (D_{\bar{\mu}} \Omega_{\ell}^{\dagger} \Omega_{\ell}) (\bar{e}_s \gamma^{\bar{\mu}} D^{\bar{\nu}} D^{\bar{\nu}} e_r) \right] \\
& + \frac{i}{3} g_Y \mathcal{C}_{\ell e}^{srtt} \left[ 2(\Omega_e^{\dagger} D_{\bar{\rho}} \Omega_e) \widetilde{B}^{\bar{\rho}\bar{\sigma}} (\bar{\ell}_s \gamma^{\bar{\sigma}} \ell_r) - 2(D_{\bar{\mu}} \Omega_e^{\dagger} \Omega_e) \widetilde{B}^{\bar{\mu}\bar{\sigma}} (\bar{\ell}_s \gamma^{\bar{\sigma}} \ell_r) \right] \\
& + \frac{i}{3} \mathcal{C}_{\ell e}^{srtt} \left[ (\Omega_e^{\dagger} D_{\bar{\nu}} \Omega_e) (D^{\bar{\mu}} \bar{\ell}_s \gamma^{\bar{\nu}} D^{\bar{\mu}} \ell_r) - (D_{\bar{\mu}} \Omega_e^{\dagger} \Omega_e) (D^{\bar{\nu}} \bar{\ell}_s \gamma^{\bar{\mu}} D^{\bar{\nu}} \ell_r) \right] \\
& + \frac{i}{3} \mathcal{C}_{\ell e}^{srtt} \left[ (\Omega_e^{\dagger} D_{\bar{\nu}} \Omega_e) (D^{\bar{\mu}} D^{\bar{\mu}} \bar{\ell}_s \gamma^{\bar{\nu}} \ell_r) - (D_{\bar{\mu}} \Omega_e^{\dagger} \Omega_e) (\bar{\ell}_s \gamma^{\bar{\mu}} D^{\bar{\nu}} D^{\bar{\nu}} \ell_r) \right] \\
& + \frac{2}{3} \bar{y}_e^{tu} \mathcal{C}_{\ell e}^{trsu} (D_{\bar{\mu}} \Omega_{\ell,j}^* D_{\bar{\mu}} \Omega_{\ell}^i) H_i^{\dagger} (\bar{e}_s \ell_r^j) + \frac{2}{3} \bar{y}_e^{tu} \mathcal{C}_{\ell e}^{trsu} (D_{\bar{\mu}} \Omega_{\ell,j}^* \Omega_{\ell}^i) H_i^{\dagger} (\bar{e}_s D^{\bar{\mu}} \ell_r^j)
\end{aligned}$$

$$\begin{aligned}
& + \frac{2}{3} \bar{y}_e^{tu} \mathcal{C}_{\ell e}^{trsu} (D_{\bar{\mu}} \Omega_e^\dagger D_{\bar{\mu}} \Omega_e) (\bar{e}_s H^\dagger \ell_r) + \frac{2}{3} \bar{y}_e^{tu} \mathcal{C}_{\ell e}^{trsu} (D_{\bar{\mu}} \Omega_e^\dagger \Omega_e) (\bar{e}_s D_{\bar{\mu}} H^\dagger \ell_r) \\
& + \frac{2}{3} \bar{y}_e^{tu} \mathcal{C}_{\ell e}^{trsu} (D_{\bar{\mu}} \Omega_{\ell,j}^* \Omega_\ell^i) H_i^\dagger (D^{\bar{\mu}} \bar{e}_s \ell_r^j) + \frac{2}{3} y_e^{tu} \mathcal{C}_{\ell e}^{stur} (D_{\bar{\mu}} \Omega_e^\dagger D_{\bar{\mu}} \Omega_e) (\bar{\ell}_s H e_r) \\
& + \frac{2}{3} y_e^{tu} \mathcal{C}_{\ell e}^{stur} (\Omega_e^\dagger D_{\bar{\mu}} \Omega_e) (\bar{\ell}_s D_{\bar{\mu}} H e_r) + \frac{2}{3} y_e^{tu} \mathcal{C}_{\ell e}^{stur} (D_{\bar{\mu}} \Omega_{\ell,i}^* D_{\bar{\mu}} \Omega_\ell^j) H^i (\bar{\ell}_{js} e_r) \\
& + \frac{2}{3} y_e^{tu} \mathcal{C}_{\ell e}^{stur} (\Omega_{\ell,i}^* D_{\bar{\mu}} \Omega_\ell^j) H^i (\bar{\ell}_{js} D^{\bar{\mu}} e_r) + \frac{2}{3} y_e^{tu} \mathcal{C}_{\ell e}^{stur} (\Omega_{\ell,i}^* D_{\bar{\mu}} \Omega_\ell^j) H^i (D^{\bar{\mu}} \bar{\ell}_{js} e_r) \\
& - \frac{2}{3} \bar{y}_e^{tu} \mathcal{C}_{\ell e}^{trsu} (D_{\bar{\mu}} \Omega_{\ell,j}^* \Omega_\ell^i) D^{\bar{\mu}} H_i^\dagger (\bar{e}_s \ell_r^j) - \frac{2}{3} \bar{y}_e^{tu} \mathcal{C}_{\ell e}^{trsu} (D_{\bar{\mu}} \Omega_e^\dagger \Omega_e) (D_{\bar{\mu}} \Omega_{\ell,j}^* \Omega_\ell^i) H_i^\dagger (\bar{e}_s \ell_r^j) \\
& - \frac{2}{3} \bar{y}_e^{tu} \mathcal{C}_{\ell e}^{trsu} (D_{\bar{\mu}} \Omega_e^\dagger \Omega_e) (\bar{e}_s H^\dagger D^{\bar{\mu}} \ell_r) - \frac{2}{3} \bar{y}_e^{tu} \mathcal{C}_{\ell e}^{trsu} (D_{\bar{\mu}} \Omega_e^\dagger \Omega_e) (D^{\bar{\mu}} \bar{e}_s H^\dagger \ell_r) \\
& - \frac{2}{3} y_e^{tu} \mathcal{C}_{\ell e}^{stur} (\Omega_e^\dagger D_{\bar{\mu}} \Omega_e) (\bar{\ell}_s H D^{\bar{\mu}} e_r) - \frac{2}{3} y_e^{tu} \mathcal{C}_{\ell e}^{stur} (\Omega_e^\dagger D_{\bar{\mu}} \Omega_e) (D^{\bar{\mu}} \bar{\ell}_s H e_r) \\
& - \frac{2}{3} y_e^{tu} \mathcal{C}_{\ell e}^{stur} (\Omega_e^\dagger D_{\bar{\mu}} \Omega_e) (\Omega_{\ell,i}^* D_{\bar{\mu}} \Omega_\ell^j) H^i (\bar{\ell}_{js} e_r) - \frac{2}{3} y_e^{tu} \mathcal{C}_{\ell e}^{stur} (\Omega_{\ell,i}^* D_{\bar{\mu}} \Omega_\ell^j) D^{\bar{\mu}} H^i (\bar{\ell}_{js} e_r) \\
& + \frac{2i}{3} y_e^{tv} \bar{y}_e^{tu} \mathcal{C}_{\ell e}^{srvu} (\Omega_e^\dagger \overleftrightarrow{D}_{\bar{\mu}} \Omega_e) (H^\dagger H) (\bar{\ell}_s \gamma^{\bar{\mu}} \ell_r) + \frac{2i}{3} y_e^{vu} \bar{y}_e^{tu} \mathcal{C}_{\ell e}^{tvsr} (\Omega_{\ell,j}^* \overleftrightarrow{D}_{\bar{\mu}} \Omega_\ell^i) H_i^\dagger H^j (\bar{e}_s \gamma^{\bar{\mu}} e_r), \quad (3.40)
\end{aligned}$$

$$\begin{aligned}
\Gamma_\Omega^{(1)} [\mathcal{O}_{uu}] &= \frac{i}{3} \mathcal{C}_{uu}^{srtt} \left[ (\Omega_u^\dagger D_2 D_{\bar{\mu}} \Omega_u) (\bar{u}_s \gamma^{\bar{\mu}} u_r) - (D_2 D_{\bar{\nu}} \Omega_u^\dagger \Omega_u) (\bar{u}_s \gamma^{\bar{\nu}} u_r) \right] \\
& - \frac{1}{3} \mathcal{C}_{uu}^{srtt} \left[ (D_{\bar{\mu}} \Omega_{u,a}^* D_{\bar{\rho}} \Omega_u^b) (\Omega_{u,b}^* D_{\bar{\sigma}} \Omega_u^a) \varepsilon^{\bar{\mu}\bar{\nu}\bar{\rho}\bar{\sigma}} (\bar{u}_s \gamma^{\bar{\nu}} u_r) - (D_{\bar{\mu}} \Omega_{u,a}^* \Omega_u^b) (D_{\bar{\nu}} \Omega_{u,b}^* D_{\bar{\rho}} \Omega_u^a) \varepsilon^{\bar{\mu}\bar{\nu}\bar{\rho}\bar{\sigma}} (\bar{u}_s \gamma^{\bar{\sigma}} u_r) \right] \\
& + \frac{i}{3} \mathcal{C}_{uu}^{sttr} \left[ (\Omega_{u,a}^* D_2 D_{\bar{\mu}} \Omega_u^b) (\bar{u}_{bs} \gamma^{\bar{\mu}} u_r^a) - (D_2 D_{\bar{\nu}} \Omega_{u,a}^* \Omega_u^b) (\bar{u}_{bs} \gamma^{\bar{\nu}} u_r^a) \right] \\
& - \frac{i}{3} \mathcal{C}_{uu}^{sttr} \left[ (D_{\bar{\mu}} D_{\bar{\nu}} \Omega_{u,a}^* \Omega_u^c) (\Omega_{u,b}^* D_{\bar{\mu}} \Omega_u^a) (\bar{u}_{cs} \gamma^{\bar{\nu}} u_r^b) - (D_{\bar{\mu}} \Omega_{u,a}^* \Omega_u^c) (\Omega_{u,b}^* D_{\bar{\mu}} D_{\bar{\nu}} \Omega_u^a) (\bar{u}_{cs} \gamma^{\bar{\nu}} u_r^b) \right] \\
& + \frac{i}{3} \mathcal{C}_{uu}^{sttr} \left[ (\Omega_{u,a}^* D_{\bar{\nu}} \Omega_u^c) (D_{\bar{\mu}} \Omega_{u,b}^* D_{\bar{\nu}} \Omega_u^a) (\bar{u}_{cs} \gamma^{\bar{\mu}} u_r^b) - (D_{\bar{\mu}} \Omega_{u,a}^* D_{\bar{\nu}} \Omega_u^c) (D_{\bar{\mu}} \Omega_{u,b}^* \Omega_u^a) (\bar{u}_{cs} \gamma^{\bar{\nu}} u_r^b) \right] \\
& - \frac{1}{3} \mathcal{C}_{uu}^{sttr} \left[ (\Omega_{u,a}^* D_{\bar{\nu}} \Omega_u^c) (D_{\bar{\mu}} \Omega_{u,b}^* D_{\bar{\rho}} \Omega_u^a) \varepsilon^{\bar{\mu}\bar{\nu}\bar{\rho}\bar{\sigma}} (\bar{u}_{cs} \gamma^{\bar{\sigma}} u_r^b) - (D_{\bar{\mu}} \Omega_{u,a}^* D_{\bar{\rho}} \Omega_u^c) (D_{\bar{\nu}} \Omega_{u,b}^* \Omega_u^a) \varepsilon^{\bar{\mu}\bar{\nu}\bar{\rho}\bar{\sigma}} (\bar{u}_{cs} \gamma^{\bar{\sigma}} u_r^b) \right] \\
& + \frac{i}{3} \mathcal{C}_{uu}^{sttr} \left[ (\Omega_{u,a}^* D_{\bar{\nu}} \Omega_u^c) (\Omega_{u,b}^* D_{\bar{\mu}} \Omega_u^a) (D^{\bar{\mu}} \bar{u}_{cs} \gamma^{\bar{\nu}} u_r^b) - (D_{\bar{\mu}} \Omega_{u,a}^* \Omega_u^c) (D_{\bar{\nu}} \Omega_{u,b}^* \Omega_u^a) (\bar{u}_{cs} \gamma^{\bar{\nu}} D^{\bar{\mu}} u_r^b) \right] \\
& + \frac{i}{3} \mathcal{C}_{uu}^{sttr} \left[ (\Omega_{u,a}^* D_{\bar{\mu}} \Omega_u^c) (\Omega_{u,b}^* D_{\bar{\nu}} \Omega_u^a) (\bar{u}_{cs} \gamma^{\bar{\mu}} D^{\bar{\nu}} u_r^b) - (D_{\bar{\mu}} \Omega_{u,a}^* \Omega_u^c) (D_{\bar{\nu}} \Omega_{u,b}^* \Omega_u^a) (D^{\bar{\mu}} \bar{u}_{cs} \gamma^{\bar{\nu}} u_r^b) \right] \\
& - \frac{i}{3} y_u^{tv} \bar{y}_u^{tu} \mathcal{C}_{uu}^{srvu} (\Omega_q^\dagger \overleftrightarrow{D}_{\bar{\mu}} \Omega_q) (H^\dagger H) (\bar{u}_s \gamma^{\bar{\mu}} u_r) - \frac{i}{3} y_u^{tv} \bar{y}_u^{tu} \mathcal{C}_{uu}^{suvr} (\Omega_{q,a}^* \overleftrightarrow{D}_{\bar{\mu}} \Omega_q^b) (H^\dagger H) (\bar{u}_{bs} \gamma^{\bar{\mu}} u_r^a) \\
& + \frac{i}{3} y_u^{tv} \bar{y}_u^{tu} \mathcal{C}_{uu}^{srvu} (\Omega_{q,j}^* \overleftrightarrow{D}_{\bar{\mu}} \Omega_q^i) H_i^\dagger H^j (\bar{u}_s \gamma^{\bar{\mu}} u_r) + \frac{i}{3} y_u^{tv} \bar{y}_u^{tu} \mathcal{C}_{uu}^{suvr} (\Omega_{q,a,j}^* \overleftrightarrow{D}_{\bar{\mu}} \Omega_q^{bi}) H_i^\dagger H^j (\bar{u}_{bs} \gamma^{\bar{\mu}} u_r^a) \\
& + \frac{4i}{9} g_Y \mathcal{C}_{uu}^{srtt} \left[ 2(\Omega_u^\dagger D_{\bar{\sigma}} \Omega_u) \tilde{B}^{\bar{\rho}\bar{\sigma}} (\bar{u}_s \gamma^{\bar{\rho}} u_r) + 2(D_{\bar{\mu}} \Omega_u^\dagger \Omega_u) \tilde{B}^{\bar{\mu}\bar{\sigma}} (\bar{u}_s \gamma^{\bar{\sigma}} u_r) \right] \\
& + \frac{4i}{9} g_Y \mathcal{C}_{uu}^{sttr} \left[ 2(\Omega_{u,a}^* D_{\bar{\rho}} \Omega_u^b) \tilde{B}^{\bar{\rho}\bar{\sigma}} (\bar{u}_{bs} \gamma^{\bar{\sigma}} u_r^a) - 2(D_{\bar{\mu}} \Omega_{u,a}^* \Omega_u^b) \tilde{B}^{\bar{\mu}\bar{\sigma}} (\bar{u}_{bs} \gamma^{\bar{\sigma}} u_r^a) \right] \\
& - \frac{2i}{3} g_s \mathcal{C}_{uu}^{srtt} \left[ 2T_b^{Aa} (\Omega_{u,a}^* D_{\bar{\rho}} \Omega_u^b) \tilde{G}^{\bar{\rho}\bar{\sigma}A} (\bar{u}_s \gamma^{\bar{\sigma}} u_r) - 2T_b^{Aa} (D_{\bar{\mu}} \Omega_{u,a}^* \Omega_u^b) \tilde{G}^{\bar{\mu}\bar{\sigma}A} (\bar{u}_s \gamma^{\bar{\sigma}} u_r) \right] \\
& + \frac{2i}{3} \mathcal{C}_{uu}^{srtt} \left[ (\Omega_u^\dagger D_{\bar{\nu}} \Omega_u) (D^{\bar{\mu}} \bar{u}_s \gamma^{\bar{\nu}} D^{\bar{\mu}} u_r) - (D_{\bar{\mu}} \Omega_u^\dagger \Omega_u) (D^{\bar{\nu}} \bar{u}_s \gamma^{\bar{\mu}} D^{\bar{\nu}} u_r) \right]
\end{aligned}$$

$$\begin{aligned}
& + \frac{2i}{3} \mathcal{C}_{uu}^{srtt} \left[ (\Omega_u^\dagger D_{\bar{\nu}} \Omega_u) (D^{\bar{\mu}} D^{\bar{\mu}} \bar{u}_s \gamma^{\bar{\nu}} u_r) - (D_{\bar{\mu}} \Omega_u^\dagger \Omega_u) (\bar{u}_s \gamma^{\bar{\mu}} D^{\bar{\nu}} D^{\bar{\nu}} u_r) \right] \\
& + \frac{2i}{3} \mathcal{C}_{uu}^{sttr} \left[ (\Omega_{u,a}^* D_{\bar{\nu}} \Omega_u^b) (D^{\bar{\mu}} \bar{u}_{bs} \gamma^{\bar{\nu}} D^{\bar{\mu}} u_r^a) - (D_{\bar{\mu}} \Omega_{u,a}^* \Omega_u^b) (D^{\bar{\nu}} \bar{u}_{bs} \gamma^{\bar{\mu}} D^{\bar{\nu}} u_r^a) \right] \\
& + \frac{2i}{3} \mathcal{C}_{uu}^{sttr} \left[ (\Omega_{u,a}^* D_{\bar{\nu}} \Omega_u^b) (D^{\bar{\mu}} D^{\bar{\mu}} \bar{u}_{bs} \gamma^{\bar{\nu}} u_r^a) - (D_{\bar{\mu}} \Omega_{u,a}^* \Omega_u^b) (\bar{u}_{bs} \gamma^{\bar{\mu}} D^{\bar{\nu}} D^{\bar{\nu}} u_r^a) \right] \\
& - \frac{2i}{3} \mathcal{C}_{uu}^{sttr} \left[ (\Omega_{u,a}^* D_{\bar{\mu}} \Omega_u^c) (D_{\bar{\mu}} \Omega_{u,b}^* D_{\bar{\nu}} \Omega_u^a) (\bar{u}_{cs} \gamma^{\bar{\nu}} u_r^b) - (D_{\bar{\mu}} \Omega_{u,a}^* D_{\bar{\nu}} \Omega_u^c) (D_{\bar{\nu}} \Omega_{u,b}^* \Omega_u^a) (\bar{u}_{cs} \gamma^{\bar{\mu}} u_r^b) \right] \\
& + \frac{2i}{3} g_s \mathcal{C}_{uu}^{sttr} \left[ 2T_b^{Aa} (\Omega_{u,a}^* D_{\bar{\rho}} \Omega_u^c) \tilde{G}^{\bar{\rho}\bar{\sigma}A} (\bar{u}_{cs} \gamma^{\bar{\sigma}} u_r^b) - 2T_c^{Ab} (D_{\bar{\mu}} \Omega_{u,a}^* \Omega_u^c) \tilde{G}^{\bar{\mu}\bar{\sigma}A} (\bar{u}_{bs} \gamma^{\bar{\sigma}} u_r^a) \right] \\
& + \frac{4i}{3} y_u^{tv} \bar{y}_u^{tu} \mathcal{C}_{uu}^{srvu} (\Omega_u^\dagger \overset{\leftrightarrow}{D}_{\bar{\mu}} \Omega_u) (H^\dagger H) (\bar{u}_s \gamma^{\bar{\mu}} u_r) + \frac{4i}{3} y_u^{tv} \bar{y}_u^{tu} \mathcal{C}_{uu}^{suwr} (\Omega_{u,a}^* \overset{\leftrightarrow}{D}_{\bar{\mu}} \Omega_u^b) (H^\dagger H) (\bar{u}_{bs} \gamma^{\bar{\mu}} u_r^a) \\
& - 2g_s \mathcal{C}_{uu}^{sttr} \left[ T_b^{Aa} (\Omega_{u,a}^* D_{\bar{\nu}} \Omega_u^c) G^{\bar{\mu}\bar{\nu}A} (\bar{u}_{cs} \gamma^{\bar{\mu}} u_r^b) - T_c^{Ab} (D_{\bar{\mu}} \Omega_{u,a}^* \Omega_u^c) G^{\bar{\mu}\bar{\nu}A} (\bar{u}_{bs} \gamma^{\bar{\nu}} u_r^a) \right], \tag{3.41}
\end{aligned}$$

$$\begin{aligned}
\Gamma_\Omega^{(1)} [\mathcal{O}_{dd}] = & -\frac{2i}{9} g_Y \mathcal{C}_{dd}^{srtt} \left[ 2(\Omega_d^\dagger D_{\bar{\sigma}} \Omega_d) \tilde{B}^{\bar{\rho}\bar{\sigma}} (\bar{d}_s \gamma^{\bar{\rho}} d_r) + 2(D_{\bar{\mu}} \Omega_d^\dagger \Omega_d) \tilde{B}^{\bar{\mu}\bar{\sigma}} (\bar{d}_s \gamma^{\bar{\sigma}} d_r) \right] \\
& - \frac{2i}{9} g_Y \mathcal{C}_{dd}^{sttr} \left[ 2(\Omega_{d,a}^* D_{\bar{\rho}} \Omega_d^b) \tilde{B}^{\bar{\rho}\bar{\sigma}} (\bar{d}_{bs} \gamma^{\bar{\sigma}} d_r^a) - 2(D_{\bar{\mu}} \Omega_{d,a}^* \Omega_d^b) \tilde{B}^{\bar{\mu}\bar{\sigma}} (\bar{d}_{bs} \gamma^{\bar{\sigma}} d_r^a) \right] \\
& + \frac{i}{3} \mathcal{C}_{dd}^{srtt} \left[ (\Omega_d^\dagger D_2 D_{\bar{\mu}} \Omega_d) (\bar{d}_s \gamma^{\bar{\mu}} d_r) - (D_2 D_{\bar{\nu}} \Omega_d^\dagger \Omega_d) (\bar{d}_s \gamma^{\bar{\nu}} d_r) \right] \\
& - \frac{1}{3} \mathcal{C}_{dd}^{srtt} \left[ (D_{\bar{\mu}} \Omega_{d,a}^* D_{\bar{\rho}} \Omega_d^b) (\Omega_{d,b}^* D_{\bar{\sigma}} \Omega_d^a) \varepsilon^{\bar{\mu}\bar{\nu}\bar{\rho}\bar{\sigma}} (\bar{d}_s \gamma^{\bar{\nu}} d_r) - (D_{\bar{\mu}} \Omega_{d,a}^* \Omega_d^b) (D_{\bar{\nu}} \Omega_{d,b}^* D_{\bar{\rho}} \Omega_d^a) \varepsilon^{\bar{\mu}\bar{\nu}\bar{\rho}\bar{\sigma}} (\bar{d}_s \gamma^{\bar{\sigma}} d_r) \right] \\
& + \frac{i}{3} \mathcal{C}_{dd}^{sttr} \left[ (\Omega_{d,a}^* D_2 D_{\bar{\mu}} \Omega_d^b) (\bar{d}_{bs} \gamma^{\bar{\mu}} d_r^a) - (D_2 D_{\bar{\nu}} \Omega_{d,a}^* \Omega_d^b) (\bar{d}_{bs} \gamma^{\bar{\nu}} d_r^a) \right] \\
& - \frac{i}{3} \mathcal{C}_{dd}^{sttr} \left[ (D_{\bar{\mu}} D_{\bar{\nu}} \Omega_{d,a}^* \Omega_d^c) (\Omega_{d,b}^* D_{\bar{\mu}} \Omega_d^a) (\bar{d}_{cs} \gamma^{\bar{\nu}} d_r^b) - (D_{\bar{\mu}} \Omega_{d,a}^* \Omega_d^c) (\Omega_{d,b}^* D_{\bar{\nu}} D_{\bar{\mu}} \Omega_d^a) (\bar{d}_{cs} \gamma^{\bar{\nu}} d_r^b) \right] \\
& + \frac{i}{3} \mathcal{C}_{dd}^{sttr} \left[ (\Omega_{d,a}^* D_{\bar{\nu}} \Omega_d^c) (D_{\bar{\mu}} \Omega_{d,b}^* D_{\bar{\nu}} \Omega_d^a) (\bar{d}_{cs} \gamma^{\bar{\mu}} d_r^b) - (D_{\bar{\mu}} \Omega_{d,a}^* D_{\bar{\nu}} \Omega_d^c) (D_{\bar{\mu}} \Omega_{d,b}^* \Omega_d^a) (\bar{d}_{cs} \gamma^{\bar{\nu}} d_r^b) \right] \\
& - \frac{1}{3} \mathcal{C}_{dd}^{sttr} \left[ (\Omega_{d,a}^* D_{\bar{\nu}} \Omega_d^c) (D_{\bar{\mu}} \Omega_{d,b}^* D_{\bar{\rho}} \Omega_d^a) \varepsilon^{\bar{\mu}\bar{\nu}\bar{\rho}\bar{\sigma}} (\bar{d}_{cs} \gamma^{\bar{\sigma}} d_r^b) - (D_{\bar{\mu}} \Omega_{d,a}^* D_{\bar{\rho}} \Omega_d^c) (D_{\bar{\nu}} \Omega_{d,b}^* \Omega_d^a) \varepsilon^{\bar{\mu}\bar{\nu}\bar{\rho}\bar{\sigma}} (\bar{d}_{cs} \gamma^{\bar{\sigma}} d_r^b) \right] \\
& + \frac{i}{3} \mathcal{C}_{dd}^{sttr} \left[ (\Omega_{d,a}^* D_{\bar{\nu}} \Omega_d^c) (\Omega_{d,b}^* D_{\bar{\mu}} \Omega_d^a) (D^{\bar{\mu}} \bar{d}_{cs} \gamma^{\bar{\nu}} d_r^b) - (D_{\bar{\mu}} \Omega_{d,a}^* \Omega_d^c) (D_{\bar{\nu}} \Omega_{d,b}^* \Omega_d^a) (\bar{d}_{cs} \gamma^{\bar{\nu}} D^{\bar{\mu}} d_r^b) \right] \\
& + \frac{i}{3} \mathcal{C}_{dd}^{sttr} \left[ (\Omega_{d,a}^* D_{\bar{\mu}} \Omega_d^c) (\Omega_{d,b}^* D_{\bar{\nu}} \Omega_d^a) (\bar{d}_{cs} \gamma^{\bar{\mu}} D^{\bar{\nu}} d_r^b) - (D_{\bar{\mu}} \Omega_{d,a}^* \Omega_d^c) (D_{\bar{\nu}} \Omega_{d,b}^* \Omega_d^a) (D^{\bar{\mu}} \bar{d}_{cs} \gamma^{\bar{\nu}} d_r^b) \right] \\
& - \frac{i}{3} y_d^{tv} \bar{y}_d^{tu} \mathcal{C}_{dd}^{srvu} (\Omega_{q,j}^* \overset{\leftrightarrow}{D}_{\bar{\mu}} \Omega_q^i) H_i^\dagger H^j (\bar{d}_s \gamma^{\bar{\mu}} d_r) - \frac{i}{3} y_d^{tv} \bar{y}_d^{tu} \mathcal{C}_{dd}^{suwr} (\Omega_{q,aj}^* \overset{\leftrightarrow}{D}_{\bar{\mu}} \Omega_q^{bi}) H_i^\dagger H^j (\bar{d}_{bs} \gamma^{\bar{\mu}} d_r^a) \\
& - \frac{2i}{3} g_s \mathcal{C}_{dd}^{srtt} \left[ 2T_b^{Aa} (\Omega_{d,a}^* D_{\bar{\rho}} \Omega_d^b) \tilde{G}^{\bar{\rho}\bar{\sigma}A} (\bar{d}_s \gamma^{\bar{\sigma}} d_r) - 2T_b^{Aa} (D_{\bar{\mu}} \Omega_{d,a}^* \Omega_d^b) \tilde{G}^{\bar{\mu}\bar{\sigma}A} (\bar{d}_s \gamma^{\bar{\sigma}} d_r) \right] \\
& + \frac{2i}{3} \mathcal{C}_{dd}^{srtt} \left[ (\Omega_d^\dagger D_{\bar{\nu}} \Omega_d) (D^{\bar{\mu}} \bar{d}_s \gamma^{\bar{\nu}} D^{\bar{\mu}} d_r) - (D_{\bar{\mu}} \Omega_d^\dagger \Omega_d) (D^{\bar{\nu}} \bar{d}_s \gamma^{\bar{\mu}} D^{\bar{\nu}} d_r) \right] \\
& + \frac{2i}{3} \mathcal{C}_{dd}^{srtt} \left[ (\Omega_d^\dagger D_{\bar{\nu}} \Omega_d) (D^{\bar{\mu}} D^{\bar{\mu}} \bar{d}_s \gamma^{\bar{\nu}} d_r) - (D_{\bar{\mu}} \Omega_d^\dagger \Omega_d) (\bar{d}_s \gamma^{\bar{\mu}} D^{\bar{\nu}} D^{\bar{\nu}} d_r) \right] \\
& + \frac{2i}{3} \mathcal{C}_{dd}^{sttr} \left[ (\Omega_{d,a}^* D_{\bar{\nu}} \Omega_d^b) (D^{\bar{\mu}} \bar{d}_{bs} \gamma^{\bar{\nu}} D^{\bar{\mu}} d_r^a) - (D_{\bar{\mu}} \Omega_{d,a}^* \Omega_d^b) (D^{\bar{\nu}} \bar{d}_{bs} \gamma^{\bar{\mu}} D^{\bar{\nu}} d_r^a) \right] \\
& + \frac{2i}{3} \mathcal{C}_{dd}^{sttr} \left[ (\Omega_{d,a}^* D_{\bar{\nu}} \Omega_d^b) (D^{\bar{\mu}} D^{\bar{\mu}} \bar{d}_{bs} \gamma^{\bar{\nu}} d_r^a) - (D_{\bar{\mu}} \Omega_{d,a}^* \Omega_d^b) (\bar{d}_{bs} \gamma^{\bar{\mu}} D^{\bar{\nu}} D^{\bar{\nu}} d_r^a) \right]
\end{aligned}$$

$$\begin{aligned}
& -\frac{2i}{3}\mathcal{C}_{dd}^{sttr}\left[(\Omega_{d,a}^*D_{\bar{\mu}}\Omega_d^c)(D_{\bar{\mu}}\Omega_{d,b}^*D_{\bar{\nu}}\Omega_d^a)(\bar{d}_{cs}\gamma^{\bar{\mu}}d_r^b) - (D_{\bar{\mu}}\Omega_{d,a}^*D_{\bar{\nu}}\Omega_d^c)(D_{\bar{\nu}}\Omega_{d,b}^*\Omega_d^a)(\bar{d}_{cs}\gamma^{\bar{\mu}}d_r^b)\right] \\
& +\frac{2i}{3}g_s\mathcal{C}_{dd}^{sttr}\left[2T_b^{Aa}(\Omega_{d,a}^*D_{\bar{\rho}}\Omega_d^c)\tilde{G}^{\bar{\rho}\bar{\sigma}A}(\bar{d}_{cs}\gamma^{\bar{\sigma}}d_r^b) - 2T_c^{Ab}(D_{\bar{\mu}}\Omega_{d,a}^*\Omega_d^c)\tilde{G}^{\bar{\mu}\bar{\sigma}A}(\bar{d}_{bs}\gamma^{\bar{\sigma}}d_r^a)\right] \\
& +\frac{4i}{3}y_d^{tv}\bar{y}_d^{tu}\mathcal{C}_{dd}^{srvu}(\Omega_d^\dagger\overset{\leftrightarrow}{D}_{\bar{\mu}}\Omega_d)(H^\dagger H)(\bar{d}_s\gamma^{\bar{\mu}}d_r) + \frac{4i}{3}y_d^{tv}\bar{y}_d^{tu}\mathcal{C}_{dd}^{suwr}(\Omega_{d,a}^*\overset{\leftrightarrow}{D}_{\bar{\mu}}\Omega_d^b)(H^\dagger H)(\bar{d}_{bs}\gamma^{\bar{\mu}}d_r^a) \\
& -2g_s\mathcal{C}_{dd}^{sttr}\left[T_b^{Aa}(\Omega_{d,a}^*D_{\bar{\nu}}\Omega_d^c)G^{\bar{\mu}\bar{\nu}A}(\bar{d}_{cs}\gamma^{\bar{\mu}}d_r^b) - T_c^{Ab}(D_{\bar{\mu}}\Omega_{d,a}^*\Omega_d^c)G^{\bar{\mu}\bar{\nu}A}(\bar{d}_{bs}\gamma^{\bar{\nu}}d_r^a)\right], \tag{3.42}
\end{aligned}$$

$$\begin{aligned}
\Gamma_\Omega^{(1)}[\mathcal{O}_{qq}^{(1)}] &= \frac{i}{36}g_Y(\mathcal{C}_{qq}^{(1)})^{sttr}\left[2(\Omega_{q,a}^*D_{\bar{\rho}}\Omega_q^b)\tilde{B}^{\bar{\rho}\bar{\sigma}}(\bar{q}_{bs}\gamma^{\bar{\sigma}}q_r^a) - 2(D_{\bar{\mu}}\Omega_{q,a}^*\Omega_q^b)\tilde{B}^{\bar{\mu}\bar{\sigma}}(\bar{q}_{bs}\gamma^{\bar{\sigma}}q_r^a)\right] \\
& -\frac{i}{18}g_Y(\mathcal{C}_{qq}^{(1)})^{srtt}\left[2(\Omega_{q,i}^*D_{\bar{\sigma}}\Omega_q^j)\tilde{B}^{\bar{\rho}\bar{\sigma}}(\bar{q}_{js}\gamma^{\bar{\rho}}q_r^i) + 2(D_{\bar{\mu}}\Omega_{q,i}^*\Omega_q^j)\tilde{B}^{\bar{\mu}\bar{\sigma}}(\bar{q}_{js}\gamma^{\bar{\sigma}}q_r^i)\right] \\
& -\frac{i}{12}g_Y(\mathcal{C}_{qq}^{(1)})^{srtt}\left[2(\Omega_q^\dagger D_{\bar{\sigma}}\Omega_q)\tilde{B}^{\bar{\rho}\bar{\sigma}}(\bar{q}_s\gamma^{\bar{\rho}}q_r) + 2(D_{\bar{\mu}}\Omega_q^\dagger\Omega_q)\tilde{B}^{\bar{\mu}\bar{\sigma}}(\bar{q}_s\gamma^{\bar{\sigma}}q_r)\right] \\
& +\frac{i}{6}g_L(\mathcal{C}_{qq}^{(1)})^{sttr}\left[2(\Omega_{q,a}^*D_{\bar{\rho}}\Omega_q^c)\tilde{W}^{\bar{\rho}\bar{\sigma}I}(\bar{q}_{bs}t^I\gamma^{\bar{\sigma}}q_r^a) - 2(D_{\bar{\mu}}\Omega_{q,a}^*\Omega_q^c)\tilde{W}^{\bar{\mu}\bar{\sigma}I}(\bar{q}_{bs}t^I\gamma^{\bar{\sigma}}q_r^a)\right] \\
& -\frac{i}{6}g_s(\mathcal{C}_{qq}^{(1)})^{sttr}\left[2T_c^{Ab}(D_{\bar{\mu}}\Omega_{q,a}^*\Omega_q^c)\tilde{G}^{\bar{\mu}\bar{\sigma}A}(\bar{q}_{bs}\gamma^{\bar{\sigma}}q_r^a) + 2T_b^{Aa}(\Omega_{q,a}^*D_{\bar{\sigma}}\Omega_q^c)\tilde{G}^{\bar{\rho}\bar{\sigma}A}(\bar{q}_{cs}\gamma^{\bar{\rho}}q_r^b)\right] \\
& -\frac{i}{6}g_Y(\mathcal{C}_{qq}^{(1)})^{sttr}\left[2(\Omega_{q,ai}^*D_{\bar{\rho}}\Omega_q^{bj})\tilde{B}^{\bar{\rho}\bar{\sigma}}(\bar{q}_{bjs}\gamma^{\bar{\sigma}}q_r^{ai}) - 2(D_{\bar{\mu}}\Omega_{q,ai}^*\Omega_q^{bj})\tilde{B}^{\bar{\mu}\bar{\sigma}}(\bar{q}_{bjs}\gamma^{\bar{\sigma}}q_r^{ai})\right] \\
& +\frac{i}{3}(\mathcal{C}_{qq}^{(1)})^{srtt}\left[(\Omega_q^\dagger D_2D_{\bar{\mu}}\Omega_q)(\bar{q}_s\gamma^{\bar{\mu}}q_r) - (D_2D_{\bar{\nu}}\Omega_q^\dagger\Omega_q)(\bar{q}_s\gamma^{\bar{\nu}}q_r)\right] \\
& +\frac{1}{3}(\mathcal{C}_{qq}^{(1)})^{srtt}\left[(D_{\bar{\mu}}\Omega_{q,a}^*D_{\bar{\rho}}\Omega_q^b)(\Omega_{q,b}^*D_{\bar{\sigma}}\Omega_q^a)\varepsilon^{\bar{\mu}\bar{\nu}\bar{\rho}\bar{\sigma}}(\bar{q}_s\gamma^{\bar{\nu}}q_r) - (D_{\bar{\mu}}\Omega_{q,a}^*\Omega_q^b)(D_{\bar{\nu}}\Omega_{q,b}^*D_{\bar{\rho}}\Omega_q^a)\varepsilon^{\bar{\mu}\bar{\nu}\bar{\rho}\bar{\sigma}}(\bar{q}_s\gamma^{\bar{\sigma}}q_r)\right] \\
& +\frac{i}{3}g_s(\mathcal{C}_{qq}^{(1)})^{srtt}\left[2T_b^{Aa}(\Omega_{q,ai}^*D_{\bar{\rho}}\Omega_q^{bj})\tilde{G}^{\bar{\rho}\bar{\sigma}A}(\bar{q}_{js}\gamma^{\bar{\sigma}}q_r^i) - 2T_b^{Aa}(D_{\bar{\mu}}\Omega_{q,ai}^*\Omega_q^{bj})\tilde{G}^{\bar{\mu}\bar{\sigma}A}(\bar{q}_{js}\gamma^{\bar{\sigma}}q_r^i)\right] \\
& +\frac{1}{3}g_s(\mathcal{C}_{qq}^{(1)})^{sttr}\left[T_b^{Aa}(\Omega_{q,a}^*D_{\bar{\nu}}\Omega_q^c)G^{\bar{\mu}\bar{\nu}A}(\bar{q}_{cs}\gamma^{\bar{\mu}}q_r^b) - T_c^{Ab}(D_{\bar{\mu}}\Omega_{q,a}^*\Omega_q^c)G^{\bar{\mu}\bar{\nu}A}(\bar{q}_{bs}\gamma^{\bar{\nu}}q_r^a)\right] \\
& +\frac{i}{3}(\mathcal{C}_{qq}^{(1)})^{sttr}\left[(D_{\bar{\mu}}D_{\bar{\nu}}\Omega_{q,a}^*\Omega_q^c)(\Omega_{q,b}^*D_{\bar{\mu}}\Omega_q^a)(\bar{q}_{cs}\gamma^{\bar{\nu}}q_r^b) - (D_{\bar{\mu}}\Omega_{q,a}^*\Omega_q^c)(\Omega_{q,b}^*D_{\bar{\mu}}D_{\bar{\nu}}\Omega_q^a)(\bar{q}_{cs}\gamma^{\bar{\nu}}q_r^b)\right] \\
& -\frac{i}{3}(\mathcal{C}_{qq}^{(1)})^{sttr}\left[(\Omega_{q,a}^*D_{\bar{\nu}}\Omega_q^c)(D_{\bar{\mu}}\Omega_{q,b}^*D_{\bar{\nu}}\Omega_q^a)(\bar{q}_{cs}\gamma^{\bar{\mu}}q_r^b) - (D_{\bar{\mu}}\Omega_{q,a}^*D_{\bar{\nu}}\Omega_q^c)(D_{\bar{\mu}}\Omega_{q,b}^*\Omega_q^a)(\bar{q}_{cs}\gamma^{\bar{\nu}}q_r^b)\right] \\
& -\frac{i}{3}(\mathcal{C}_{qq}^{(1)})^{sttr}\left[(D_{\bar{\mu}}D_{\bar{\nu}}\Omega_{q,ai}^*\Omega_q^{cj})(\Omega_{q,bj}^*D_{\bar{\mu}}\Omega_q^{ai})(\bar{q}_{cs}\gamma^{\bar{\nu}}q_r^b) - (D_{\bar{\mu}}\Omega_{q,ai}^*\Omega_q^{cj})(\Omega_{q,bj}^*D_{\bar{\mu}}D_{\bar{\nu}}\Omega_q^{ai})(\bar{q}_{cs}\gamma^{\bar{\nu}}q_r^b)\right] \\
& +\frac{i}{3}(\mathcal{C}_{qq}^{(1)})^{sttr}\left[(\Omega_{q,ai}^*D_{\bar{\nu}}\Omega_q^{cj})(D_{\bar{\mu}}\Omega_{q,bj}^*D_{\bar{\nu}}\Omega_q^{ai})(\bar{q}_{cs}\gamma^{\bar{\mu}}q_r^b) - (D_{\bar{\mu}}\Omega_{q,ai}^*D_{\bar{\nu}}\Omega_q^{cj})(D_{\bar{\mu}}\Omega_{q,bj}^*\Omega_q^{ai})(\bar{q}_{cs}\gamma^{\bar{\nu}}q_r^b)\right] \\
& +\frac{1}{3}(\mathcal{C}_{qq}^{(1)})^{sttr}\left[(\Omega_{q,ai}^*D_{\bar{\nu}}\Omega_q^{cj})(D_{\bar{\mu}}\Omega_{q,bj}^*D_{\bar{\rho}}\Omega_q^{ai})\varepsilon^{\bar{\mu}\bar{\nu}\bar{\rho}\bar{\sigma}}(\bar{q}_{cs}\gamma^{\bar{\sigma}}q_r^b) - (D_{\bar{\mu}}\Omega_{q,ai}^*D_{\bar{\rho}}\Omega_q^{cj})(D_{\bar{\nu}}\Omega_{q,bj}^*\Omega_q^{ai})\varepsilon^{\bar{\mu}\bar{\nu}\bar{\rho}\bar{\sigma}}(\bar{q}_{cs}\gamma^{\bar{\sigma}}q_r^b)\right] \\
& -\frac{1}{3}(\mathcal{C}_{qq}^{(1)})^{sttr}\left[(\Omega_{q,a}^*D_{\bar{\nu}}\Omega_q^c)(D_{\bar{\mu}}\Omega_{q,b}^*D_{\bar{\rho}}\Omega_q^a)\varepsilon^{\bar{\mu}\bar{\nu}\bar{\rho}\bar{\sigma}}(\bar{q}_{cs}\gamma^{\bar{\sigma}}q_r^b) - (D_{\bar{\mu}}\Omega_{q,a}^*D_{\bar{\rho}}\Omega_q^c)(D_{\bar{\nu}}\Omega_{q,b}^*\Omega_q^a)\varepsilon^{\bar{\mu}\bar{\nu}\bar{\rho}\bar{\sigma}}(\bar{q}_{cs}\gamma^{\bar{\sigma}}q_r^b)\right] \\
& -\frac{i}{3}(\mathcal{C}_{qq}^{(1)})^{sttr}\left[(\Omega_{q,a}^*D_{\bar{\nu}}\Omega_q^c)(\Omega_{q,b}^*D_{\bar{\mu}}\Omega_q^a)(D_{\bar{\mu}}\bar{q}_{cs}\gamma^{\bar{\nu}}q_r^b) - (D_{\bar{\mu}}\Omega_{q,a}^*\Omega_q^c)(D_{\bar{\nu}}\Omega_{q,b}^*\Omega_q^a)(\bar{q}_{cs}\gamma^{\bar{\nu}}D_{\bar{\mu}}q_r^b)\right] \\
& -\frac{i}{3}(\mathcal{C}_{qq}^{(1)})^{sttr}\left[(\Omega_{q,a}^*D_{\bar{\mu}}\Omega_q^c)(\Omega_{q,b}^*D_{\bar{\nu}}\Omega_q^a)(\bar{q}_{cs}\gamma^{\bar{\mu}}D_{\bar{\nu}}q_r^b) - (D_{\bar{\mu}}\Omega_{q,a}^*\Omega_q^c)(D_{\bar{\nu}}\Omega_{q,b}^*\Omega_q^a)(D_{\bar{\mu}}\bar{q}_{cs}\gamma^{\bar{\nu}}q_r^b)\right] \\
& +\frac{i}{3}(\mathcal{C}_{qq}^{(1)})^{sttr}\left[(\Omega_{q,ai}^*D_{\bar{\nu}}\Omega_q^{cj})(\Omega_{q,bj}^*D_{\bar{\mu}}\Omega_q^{ai})(D_{\bar{\mu}}\bar{q}_{cs}\gamma^{\bar{\nu}}q_r^b) - (D_{\bar{\mu}}\Omega_{q,ai}^*\Omega_q^{cj})(D_{\bar{\nu}}\Omega_{q,bj}^*\Omega_q^{ai})(\bar{q}_{cs}\gamma^{\bar{\nu}}D_{\bar{\mu}}q_r^b)\right]
\end{aligned}$$

$$\begin{aligned}
& + \frac{i}{3} (\mathcal{C}_{qq}^{(1)})^{sttr} \left[ (\Omega_{q,ai}^* D_{\bar{\mu}} \Omega_q^{cj}) (\Omega_{q,bj}^* D_{\bar{\nu}} \Omega_q^{ai}) (\bar{q}_{cs} \gamma^{\bar{\mu}} D^{\bar{\nu}} q_r^b) - (D_{\bar{\mu}} \Omega_{q,ai}^* \Omega_q^{cj}) (D_{\bar{\nu}} \Omega_{q,bj}^* \Omega_q^{ai}) (D^{\bar{\mu}} \bar{q}_{cs} \gamma^{\bar{\nu}} q_r^b) \right] \\
& + \frac{i}{3} (\mathcal{C}_{qq}^{(1)})^{sttr} \left[ (\Omega_{q,ai}^* D_2 D_{\bar{\mu}} \Omega_q^{bj}) (\bar{q}_{bjs} \gamma^{\bar{\mu}} q_r^{ai}) - (D_2 D_{\bar{\nu}} \Omega_{q,ai}^* \Omega_q^{bj}) (\bar{q}_{bjs} \gamma^{\bar{\nu}} q_r^{ai}) \right] \\
& + \frac{i}{3} (\mathcal{C}_{qq}^{(1)})^{sttr} \left[ (D_{\bar{\mu}} D_{\bar{\nu}} \Omega_{q,ai}^* \Omega_q^{cj}) (\Omega_{q,bj}^* D_{\bar{\mu}} \Omega_q^{ak}) (\bar{q}_{cks} \gamma^{\bar{\nu}} q_r^{bi}) - (D_{\bar{\mu}} \Omega_{q,ai}^* \Omega_q^{cj}) (\Omega_{q,bj}^* D_{\bar{\nu}} \Omega_q^{ak}) (\bar{q}_{cks} \gamma^{\bar{\nu}} q_r^{bi}) \right] \\
& - \frac{i}{3} (\mathcal{C}_{qq}^{(1)})^{sttr} \left[ (\Omega_{q,ai}^* D_{\bar{\nu}} \Omega_q^{cj}) (D_{\bar{\mu}} \Omega_{q,bj}^* D_{\bar{\nu}} \Omega_q^{ak}) (\bar{q}_{cks} \gamma^{\bar{\mu}} q_r^{bi}) - (D_{\bar{\mu}} \Omega_{q,ai}^* D_{\bar{\nu}} \Omega_q^{cj}) (D_{\bar{\mu}} \Omega_{q,bj}^* \Omega_q^{ak}) (\bar{q}_{cks} \gamma^{\bar{\nu}} q_r^{bi}) \right] \\
& - \frac{1}{3} (\mathcal{C}_{qq}^{(1)})^{sttr} \left[ (\Omega_{q,ai}^* D_{\bar{\nu}} \Omega_q^{cj}) (D_{\bar{\mu}} \Omega_{q,bj}^* D_{\bar{\rho}} \Omega_q^{ak}) \varepsilon^{\bar{\mu}\bar{\nu}\bar{\rho}\bar{\sigma}} (\bar{q}_{cks} \gamma^{\bar{\sigma}} q_r^{bi}) - (D_{\bar{\mu}} \Omega_{q,ai}^* D_{\bar{\rho}} \Omega_q^{cj}) (D_{\bar{\nu}} \Omega_{q,bj}^* \Omega_q^{ak}) \varepsilon^{\bar{\mu}\bar{\nu}\bar{\rho}\bar{\sigma}} (\bar{q}_{cks} \gamma^{\bar{\sigma}} q_r^{bi}) \right] \\
& + \frac{i}{3} (\mathcal{C}_{qq}^{(1)})^{sttr} \left[ (\Omega_{q,b}^* D_{\bar{\mu}} \Omega_q^a) (\Omega_{q,ai}^* D_{\bar{\nu}} \Omega_q^{ck}) (D^{\bar{\mu}} \bar{q}_{cks} \gamma^{\bar{\nu}} q_r^{bi}) - (D_{\bar{\mu}} \Omega_{q,a}^* \Omega_q^c) (D_{\bar{\nu}} \Omega_{q,bj}^* \Omega_q^{ak}) (\bar{q}_{cks} \gamma^{\bar{\nu}} D^{\bar{\mu}} q_r^{bj}) \right] \\
& + \frac{i}{3} (\mathcal{C}_{qq}^{(1)})^{sttr} \left[ (\Omega_{q,a}^* D_{\bar{\mu}} \Omega_q^c) (\Omega_{q,bj}^* D_{\bar{\nu}} \Omega_q^{ak}) (\bar{q}_{cks} \gamma^{\bar{\mu}} D^{\bar{\nu}} q_r^{bj}) - (D_{\bar{\nu}} \Omega_{q,b}^* \Omega_q^a) (D_{\bar{\mu}} \Omega_{q,ai}^* \Omega_q^{ck}) (D^{\bar{\mu}} \bar{q}_{cks} \gamma^{\bar{\nu}} q_r^{bi}) \right] \\
& - \frac{i}{3} (\mathcal{C}_{qq}^{(1)})^{sttr} \left[ (\Omega_{q,ai}^* D_{\bar{\nu}} \Omega_q^{cj}) (\Omega_{q,bj}^* D_{\bar{\mu}} \Omega_q^{ak}) (D^{\bar{\mu}} \bar{q}_{cks} \gamma^{\bar{\nu}} q_r^{bi}) - (D_{\bar{\mu}} \Omega_{q,ai}^* \Omega_q^{cj}) (D_{\bar{\nu}} \Omega_{q,bj}^* \Omega_q^{ak}) (\bar{q}_{cks} \gamma^{\bar{\nu}} D^{\bar{\mu}} q_r^{bi}) \right] \\
& - \frac{i}{3} (\mathcal{C}_{qq}^{(1)})^{sttr} \left[ (\Omega_{q,ai}^* D_{\bar{\mu}} \Omega_q^{cj}) (\Omega_{q,bj}^* D_{\bar{\nu}} \Omega_q^{ak}) (\bar{q}_{cks} \gamma^{\bar{\mu}} D^{\bar{\nu}} q_r^{bi}) - (D_{\bar{\mu}} \Omega_{q,ai}^* \Omega_q^{cj}) (D_{\bar{\nu}} \Omega_{q,bj}^* \Omega_q^{ak}) (D^{\bar{\mu}} \bar{q}_{cks} \gamma^{\bar{\nu}} q_r^{bi}) \right] \\
& + \frac{i}{3} (\mathcal{C}_{qq}^{(1)})^{sttr} \left[ (\Omega_{q,a}^* D_{\bar{\nu}} \Omega_q^c) (\Omega_{q,bj}^* D_{\bar{\mu}} \Omega_q^{ak}) (D^{\bar{\mu}} \bar{q}_{cks} \gamma^{\bar{\nu}} q_r^{bj}) - (D_{\bar{\nu}} \Omega_{q,b}^* \Omega_q^a) (D_{\bar{\mu}} \Omega_{q,ai}^* \Omega_q^{ck}) (\bar{q}_{cks} \gamma^{\bar{\nu}} D^{\bar{\mu}} q_r^{bi}) \right] \\
& + \frac{i}{3} (\mathcal{C}_{qq}^{(1)})^{sttr} \left[ (\Omega_{q,b}^* D_{\bar{\nu}} \Omega_q^a) (\Omega_{q,ai}^* D_{\bar{\mu}} \Omega_q^{ck}) (\bar{q}_{cks} \gamma^{\bar{\mu}} D^{\bar{\nu}} q_r^{bi}) - (D_{\bar{\mu}} \Omega_{q,a}^* \Omega_q^c) (D_{\bar{\nu}} \Omega_{q,bj}^* \Omega_q^{ak}) (D^{\bar{\mu}} \bar{q}_{cks} \gamma^{\bar{\nu}} q_r^{bj}) \right] \\
& - \frac{1}{3} (\mathcal{C}_{qq}^{(1)})^{sttr} \left[ (D_{\bar{\nu}} \Omega_{q,b}^* \Omega_q^a) (D_{\bar{\mu}} \Omega_{q,ai}^* \Omega_q^{ck}) \varepsilon^{\bar{\mu}\bar{\nu}\bar{\rho}\bar{\sigma}} (\bar{q}_{cks} \gamma^{\bar{\sigma}} D^{\bar{\rho}} q_r^{bi}) + (\Omega_{q,a}^* D_{\bar{\mu}} \Omega_q^c) (\Omega_{q,bj}^* D_{\bar{\rho}} \Omega_q^{ak}) \varepsilon^{\bar{\mu}\bar{\nu}\bar{\rho}\bar{\sigma}} (D^{\bar{\nu}} \bar{q}_{cks} \gamma^{\bar{\sigma}} q_r^{bj}) \right] \\
& - \frac{1}{3} (\mathcal{C}_{qq}^{(1)})^{sttr} \left[ (\Omega_{q,a}^* D_{\bar{\mu}} \Omega_q^c) (\Omega_{q,bj}^* D_{\bar{\rho}} \Omega_q^{ak}) \varepsilon^{\bar{\mu}\bar{\nu}\bar{\rho}\bar{\sigma}} (\bar{q}_{cks} \gamma^{\bar{\sigma}} D^{\bar{\nu}} q_r^{bj}) + (D_{\bar{\nu}} \Omega_{q,b}^* \Omega_q^a) (D_{\bar{\mu}} \Omega_{q,ai}^* \Omega_q^{ck}) \varepsilon^{\bar{\mu}\bar{\nu}\bar{\rho}\bar{\sigma}} (D^{\bar{\rho}} \bar{q}_{cks} \gamma^{\bar{\sigma}} q_r^{bi}) \right] \\
& - \frac{i}{3} y_d^{vu} \bar{y}_d^{tu} (\mathcal{C}_{qq}^{(1)})^{srtv} (\Omega_d^{\dagger} \bar{D}_{\bar{\mu}} \Omega_d) (H^{\dagger} H) (\bar{q}_s \gamma^{\bar{\mu}} q_r) - \frac{i}{3} y_d^{vu} \bar{y}_d^{tu} (\mathcal{C}_{qq}^{(1)})^{svtr} (\Omega_{d,a}^* \bar{D}_{\bar{\mu}} \Omega_d^b) (\bar{q}_{bs} H \gamma^{\bar{\mu}} H^{\dagger} q_r^a) \\
& - \frac{i}{3} y_u^{vu} \bar{y}_u^{tu} (\mathcal{C}_{qq}^{(1)})^{srtv} (\Omega_u^{\dagger} \bar{D}_{\bar{\mu}} \Omega_u) (H^{\dagger} H) (\bar{q}_s \gamma^{\bar{\mu}} q_r) - \frac{i}{3} y_u^{vu} \bar{y}_u^{tu} (\mathcal{C}_{qq}^{(1)})^{svtr} (\Omega_{u,a}^* \bar{D}_{\bar{\mu}} \Omega_u^b) (H^{\dagger} H) (\bar{q}_{bs} \gamma^{\bar{\mu}} q_r^a) \\
& + \frac{i}{3} y_u^{vu} \bar{y}_u^{tu} (\mathcal{C}_{qq}^{(1)})^{svtr} (\Omega_{u,a}^* \bar{D}_{\bar{\mu}} \Omega_u^b) (\bar{q}_{bs} H \gamma^{\bar{\mu}} H^{\dagger} q_r^a) \\
& - \frac{i}{2} g_s (\mathcal{C}_{qq}^{(1)})^{srtt} \left[ 2T_b^{Aa} (\Omega_{q,a}^* D_{\bar{\sigma}} \Omega_q^b) \tilde{G}^{\bar{\rho}\bar{\sigma}A} (\bar{q}_s \gamma^{\bar{\rho}} q_r) + 2T_b^{Aa} (D_{\bar{\mu}} \Omega_{q,a}^* \Omega_q^b) \tilde{G}^{\bar{\mu}\bar{\sigma}A} (\bar{q}_s \gamma^{\bar{\sigma}} q_r) \right] \\
& + \frac{2i}{3} (\mathcal{C}_{qq}^{(1)})^{srtt} \left[ (\Omega_q^{\dagger} D_{\bar{\nu}} \Omega_q) (D^{\bar{\mu}} \bar{q}_s \gamma^{\bar{\nu}} D^{\bar{\mu}} q_r) - (D_{\bar{\mu}} \Omega_q^{\dagger} \Omega_q) (D^{\bar{\nu}} \bar{q}_s \gamma^{\bar{\mu}} D^{\bar{\nu}} q_r) \right] \\
& + \frac{2i}{3} (\mathcal{C}_{qq}^{(1)})^{srtt} \left[ (D_q^{\dagger} D_{\bar{\nu}} \Omega_q) (D^{\bar{\mu}} D^{\bar{\mu}} \bar{q}_s \gamma^{\bar{\nu}} q_r) - (D_{\bar{\mu}} \Omega_q^{\dagger} \Omega_q) (\bar{q}_s \gamma^{\bar{\mu}} D^{\bar{\nu}} D^{\bar{\nu}} q_r) \right] \\
& + \frac{2}{3} (\mathcal{C}_{qq}^{(1)})^{srtt} \left[ (D_{\bar{\mu}} \Omega_{q,ai}^* D_{\bar{\rho}} \Omega_q^{bk}) (\Omega_{q,bj}^* D_{\bar{\sigma}} \Omega_q^{ai}) \varepsilon^{\bar{\mu}\bar{\nu}\bar{\rho}\bar{\sigma}} (\bar{q}_{ks} \gamma^{\bar{\nu}} q_r^j) - (D_{\bar{\mu}} \Omega_{q,ai}^* \Omega_q^{bk}) (D_{\bar{\nu}} \Omega_{q,bj}^* D_{\bar{\rho}} \Omega_q^{ai}) \varepsilon^{\bar{\mu}\bar{\nu}\bar{\rho}\bar{\sigma}} (\bar{q}_{ks} \gamma^{\bar{\sigma}} q_r^j) \right] \\
& + \frac{2}{3} (\mathcal{C}_{qq}^{(1)})^{srtt} \left[ (D_{\bar{\mu}} \Omega_{q,a}^* \Omega_q^b) (D_{\bar{\nu}} \Omega_{q,bj}^* \Omega_q^{ak}) \varepsilon^{\bar{\mu}\bar{\nu}\bar{\rho}\bar{\sigma}} (\bar{q}_{ks} \gamma^{\bar{\rho}} D^{\bar{\sigma}} q_r^j) + (\Omega_{q,b}^* D_{\bar{\sigma}} \Omega_q^a) (\Omega_{q,ai}^* D_{\bar{\nu}} \Omega_q^{bk}) \varepsilon^{\bar{\mu}\bar{\nu}\bar{\rho}\bar{\sigma}} (D^{\bar{\rho}} \bar{q}_{ks} \gamma^{\bar{\mu}} q_r^j) \right] \\
& - \frac{2}{3} (\mathcal{C}_{qq}^{(1)})^{srtt} \left[ (D_{\bar{\mu}} \Omega_{q,a}^* D_{\bar{\rho}} \Omega_q^b) (\Omega_{q,bj}^* D_{\bar{\sigma}} \Omega_q^{ak}) \varepsilon^{\bar{\mu}\bar{\nu}\bar{\rho}\bar{\sigma}} (\bar{q}_{ks} \gamma^{\bar{\nu}} q_r^j) - (D_{\bar{\nu}} \Omega_{q,b}^* D_{\bar{\rho}} \Omega_q^a) (D_{\bar{\mu}} \Omega_{q,ai}^* \Omega_q^{bk}) \varepsilon^{\bar{\mu}\bar{\nu}\bar{\rho}\bar{\sigma}} (\bar{q}_{ks} \gamma^{\bar{\sigma}} q_r^j) \right] \\
& + \frac{2i}{3} (\mathcal{C}_{qq}^{(1)})^{sttr} \left[ (\Omega_{q,a}^* D_{\bar{\mu}} \Omega_q^c) (D_{\bar{\mu}} \Omega_{q,b}^* D_{\bar{\nu}} \Omega_q^a) (\bar{q}_{cs} \gamma^{\bar{\nu}} q_r^b) - (D_{\bar{\mu}} \Omega_{q,a}^* D_{\bar{\nu}} \Omega_q^c) (D_{\bar{\nu}} \Omega_{q,b}^* \Omega_q^a) (\bar{q}_{cs} \gamma^{\bar{\mu}} q_r^b) \right]
\end{aligned}$$

$$\begin{aligned}
& -\frac{2i}{3}(\mathcal{C}_{qq}^{(1)})^{sttr} \left[ (\Omega_{q,ai}^* D_{\bar{\mu}} \Omega_q^{cj}) (D_{\bar{\mu}} \Omega_{q,bj}^* D_{\bar{\nu}} \Omega_q^{ai}) (\bar{q}_{cs} \gamma^{\bar{\nu}} q_r^b) - (D_{\bar{\mu}} \Omega_{q,ai}^* D_{\bar{\nu}} \Omega_q^{cj}) (D_{\bar{\nu}} \Omega_{q,bj}^* \Omega_q^{ai}) (\bar{q}_{cs} \gamma^{\bar{\mu}} q_r^b) \right] \\
& + \frac{2i}{3}(\mathcal{C}_{qq}^{(1)})^{sttr} \left[ (\Omega_{q,ai}^* D_{\bar{\nu}} \Omega_q^{bj}) (D_{\bar{\mu}} \bar{q}_{bjs} \gamma^{\bar{\nu}} D_{\bar{\mu}} q_r^{ai}) - (D_{\bar{\mu}} \Omega_{q,ai}^* \Omega_q^{bj}) (D_{\bar{\nu}} \bar{q}_{bjs} \gamma^{\bar{\mu}} D_{\bar{\nu}} q_r^{ai}) \right] \\
& + \frac{2i}{3}(\mathcal{C}_{qq}^{(1)})^{sttr} \left[ (\Omega_{q,ai}^* D_{\bar{\nu}} \Omega_q^{bj}) (D_{\bar{\mu}} D_{\bar{\mu}} \bar{q}_{bjs} \gamma^{\bar{\nu}} q_r^{ai}) - (D_{\bar{\mu}} \Omega_{q,ai}^* \Omega_q^{bj}) (\bar{q}_{bjs} \gamma^{\bar{\mu}} D_{\bar{\nu}} D_{\bar{\nu}} q_r^{ai}) \right] \\
& - \frac{2i}{3}g_L(\mathcal{C}_{qq}^{(1)})^{sttr} \left[ 2t_j^{Ii} (\Omega_{q,ai}^* D_{\bar{\rho}} \Omega_q^{bk}) \widetilde{W}^{\bar{\rho}\bar{\sigma}I} (\bar{q}_{bks} \gamma^{\bar{\sigma}} q_r^{aj}) - 2t_k^{Ij} (D_{\bar{\mu}} \Omega_{q,ai}^* \Omega_q^{bk}) \widetilde{W}^{\bar{\mu}\bar{\sigma}I} (\bar{q}_{bjs} \gamma^{\bar{\sigma}} q_r^{ai}) \right] \\
& - \frac{2i}{3}(\mathcal{C}_{qq}^{(1)})^{sttr} \left[ (D_{\bar{\mu}} \Omega_{q,b}^* D_{\bar{\nu}} \Omega_q^a) (\Omega_{q,ai}^* D_{\bar{\mu}} \Omega_q^{ck}) (\bar{q}_{cks} \gamma^{\bar{\nu}} q_r^{bi}) - (D_{\bar{\mu}} \Omega_{q,a}^* D_{\bar{\nu}} \Omega_q^c) (D_{\bar{\nu}} \Omega_{q,bj}^* \Omega_q^{ak}) (\bar{q}_{cks} \gamma^{\bar{\mu}} q_r^{bj}) \right] \\
& + \frac{2i}{3}(\mathcal{C}_{qq}^{(1)})^{sttr} \left[ (\Omega_{q,ai}^* D_{\bar{\mu}} \Omega_q^{cj}) (D_{\bar{\mu}} \Omega_{q,bj}^* D_{\bar{\nu}} \Omega_q^{ak}) (\bar{q}_{cks} \gamma^{\bar{\nu}} q_r^{bi}) - (D_{\bar{\mu}} \Omega_{q,ai}^* D_{\bar{\nu}} \Omega_q^{cj}) (D_{\bar{\nu}} \Omega_{q,bj}^* \Omega_q^{ak}) (\bar{q}_{cks} \gamma^{\bar{\mu}} q_r^{bi}) \right] \\
& - \frac{2i}{3}(\mathcal{C}_{qq}^{(1)})^{sttr} \left[ (\Omega_{q,b}^* D_{\bar{\nu}} \Omega_q^a) (D_{\bar{\mu}} D_{\bar{\nu}} \Omega_{q,ai}^* \Omega_q^{ck}) (\bar{q}_{cks} \gamma^{\bar{\mu}} q_r^{bi}) - (D_{\bar{\mu}} \Omega_{q,a}^* \Omega_q^c) (\Omega_{q,bj}^* D_{\bar{\nu}} D_{\bar{\mu}} \Omega_q^{ak}) (\bar{q}_{cks} \gamma^{\bar{\nu}} q_r^{bj}) \right] \\
& + \frac{2i}{3}(\mathcal{C}_{qq}^{(1)})^{sttr} \left[ (D_{\bar{\mu}} \Omega_{q,b}^* D_{\bar{\nu}} \Omega_q^a) (\Omega_{q,ai}^* D_{\bar{\nu}} \Omega_q^{ck}) (\bar{q}_{cks} \gamma^{\bar{\mu}} q_r^{bi}) - (D_{\bar{\mu}} \Omega_{q,a}^* D_{\bar{\nu}} \Omega_q^c) (D_{\bar{\mu}} \Omega_{q,bj}^* \Omega_q^{ak}) (\bar{q}_{cks} \gamma^{\bar{\nu}} q_r^{bj}) \right] \\
& - \frac{2i}{3}(\mathcal{C}_{qq}^{(1)})^{sttr} \left[ (\Omega_{q,a}^* D_{\bar{\mu}} \Omega_q^c) (D_{\bar{\mu}} \Omega_{q,bj}^* D_{\bar{\nu}} \Omega_q^{ak}) (\bar{q}_{cks} \gamma^{\bar{\nu}} q_r^{bj}) - (D_{\bar{\nu}} \Omega_{q,b}^* \Omega_q^a) (D_{\bar{\mu}} \Omega_{q,ai}^* D_{\bar{\nu}} \Omega_q^{ck}) (\bar{q}_{cks} \gamma^{\bar{\mu}} q_r^{bi}) \right] \\
& + \frac{2}{3}(\mathcal{C}_{qq}^{(1)})^{sttr} \left[ (\Omega_{q,a}^* D_{\bar{\nu}} \Omega_q^c) (D_{\bar{\mu}} \Omega_{q,bj}^* D_{\bar{\rho}} \Omega_q^{ak}) \varepsilon^{\bar{\mu}\bar{\nu}\bar{\rho}\bar{\sigma}} (\bar{q}_{cks} \gamma^{\bar{\sigma}} q_r^{bj}) - (D_{\bar{\nu}} \Omega_{q,b}^* \Omega_q^a) (D_{\bar{\mu}} \Omega_{q,ai}^* D_{\bar{\rho}} \Omega_q^{ck}) \varepsilon^{\bar{\mu}\bar{\nu}\bar{\rho}\bar{\sigma}} (\bar{q}_{cks} \gamma^{\bar{\sigma}} q_r^{bi}) \right] \\
& + \frac{5i}{6}g_L(\mathcal{C}_{qq}^{(1)})^{srtt} \left[ 2(\Omega_q^\dagger D_{\bar{\sigma}} \Omega_q) \widetilde{W}^{\bar{\rho}\bar{\sigma}I} (\bar{q}_s t^I \gamma^{\bar{\rho}} q_r) + 2(D_{\bar{\mu}} \Omega_q^\dagger \Omega_q) \widetilde{W}^{\bar{\mu}\bar{\sigma}I} (\bar{q}_s t^I \gamma^{\bar{\sigma}} q_r) \right] \\
& - ig_s(\mathcal{C}_{qq}^{(1)})^{sttr} \left[ 2T_b^{Aa} (\Omega_{q,ai}^* D_{\bar{\rho}} \Omega_q^{cj}) \widetilde{G}^{\bar{\rho}\bar{\sigma}A} (\bar{q}_{cjs} \gamma^{\bar{\sigma}} q_r^{bi}) - 2T_c^{Ab} (D_{\bar{\mu}} \Omega_{q,ai}^* \Omega_q^{cj}) \widetilde{G}^{\bar{\mu}\bar{\sigma}A} (\bar{q}_{bjs} \gamma^{\bar{\sigma}} q_r^{ai}) \right] \\
& - \frac{4i}{3}g_L(\mathcal{C}_{qq}^{(1)})^{srtt} \left[ 2t_k^{Ij} (D_{\bar{\mu}} \Omega_{q,i}^* \Omega_q^k) \widetilde{W}^{\bar{\mu}\bar{\sigma}I} (\bar{q}_{js} \gamma^{\bar{\sigma}} q_r^i) + 2t_j^{Ii} (\Omega_{q,i}^* D_{\bar{\sigma}} \Omega_q^k) \widetilde{W}^{\bar{\rho}\bar{\sigma}I} (\bar{q}_{ks} \gamma^{\bar{\rho}} q_r^j) \right] \\
& + \frac{4i}{3}(\mathcal{C}_{qq}^{(1)})^{svtr} \left[ y_d^{vu} \bar{y}_d^{tu} + y_u^{vu} \bar{y}_u^{tu} \right] \left[ (\Omega_{q,aj}^* D_{\bar{\mu}} \Omega_q^{bi}) H_i^\dagger (\bar{q}_{bs} H \gamma^{\bar{\mu}} q_r^{aj}) - (D_{\bar{\mu}} \Omega_{q,aj}^* \Omega_q^{bk}) H^j (\bar{q}_{bks} \gamma^{\bar{\mu}} H^\dagger q_r^a) \right] \\
& + \frac{4i}{3}y_u^{vu} \bar{y}_u^{tu} (\mathcal{C}_{qq}^{(1)})^{srtv} (\Omega_q^\dagger \overleftrightarrow{D}_{\bar{\mu}} \Omega_q) (H^\dagger H) (\bar{q}_s \gamma^{\bar{\mu}} q_r) + \frac{4i}{3}y_u^{vu} \bar{y}_u^{tu} (\mathcal{C}_{qq}^{(1)})^{svtr} (\Omega_{q,a}^* \overleftrightarrow{D}_{\bar{\mu}} \Omega_q^b) (H^\dagger H) (\bar{q}_{bs} \gamma^{\bar{\mu}} q_r^a) \\
& - \frac{4i}{3}y_u^{vu} \bar{y}_u^{tu} (\mathcal{C}_{qq}^{(1)})^{svtr} (\Omega_{q,a}^* \overleftrightarrow{D}_{\bar{\mu}} \Omega_q^b) (\bar{q}_{bs} H \gamma^{\bar{\mu}} H^\dagger q_r^a) \\
& + \frac{4i}{3}(\mathcal{C}_{qq}^{(1)})^{srtv} \left[ y_d^{vu} \bar{y}_d^{tu} - y_u^{vu} \bar{y}_u^{tu} \right] (\Omega_{q,j}^* \overleftrightarrow{D}_{\bar{\mu}} \Omega_q^i) H_i^\dagger H^j (\bar{q}_s \gamma^{\bar{\mu}} q_r) \\
& - \frac{4i}{3}y_u^{vu} \bar{y}_u^{tu} (\mathcal{C}_{qq}^{(1)})^{svtr} (\Omega_{q,aj}^* \overleftrightarrow{D}_{\bar{\mu}} \Omega_q^{bi}) H_i^\dagger H^j (\bar{q}_{bs} \gamma^{\bar{\mu}} q_r^a) \\
& + 2g_L(\mathcal{C}_{qq}^{(1)})^{sttr} \left[ t_k^{Ij} (D_{\bar{\mu}} \Omega_{q,ai}^* \Omega_q^{bk}) W^{\bar{\mu}\bar{\nu}I} (\bar{q}_{bjs} \gamma^{\bar{\nu}} q_r^{ai}) + t_j^{Ii} (\Omega_{q,ai}^* D_{\bar{\mu}} \Omega_q^{bk}) W^{\bar{\mu}\bar{\nu}I} (\bar{q}_{bks} \gamma^{\bar{\nu}} q_r^{aj}) \right] \\
& - \frac{4}{3}g_s(\mathcal{C}_{qq}^{(1)})^{sttr} \left[ T_b^{Aa} (\Omega_{q,ai}^* D_{\bar{\nu}} \Omega_q^{cj}) G^{\bar{\mu}\bar{\nu}A} (\bar{q}_{cjs} \gamma^{\bar{\mu}} q_r^{bi}) - T_c^{Ab} (D_{\bar{\mu}} \Omega_{q,ai}^* \Omega_q^{cj}) G^{\bar{\mu}\bar{\nu}A} (\bar{q}_{bjs} \gamma^{\bar{\nu}} q_r^{ai}) \right], \quad (3.43)
\end{aligned}$$

$$\begin{aligned}
\Gamma_\Omega^{(1)} [\mathcal{O}_{qq}^{(3)}] &= \frac{i}{12}g_Y(\mathcal{C}_{qq}^{(3)})^{srtt} \left[ 2(\Omega_q^\dagger D_{\bar{\sigma}} \Omega_q) \widetilde{B}^{\bar{\rho}\bar{\sigma}} (\bar{q}_s \gamma^{\bar{\rho}} q_r) + 2(D_{\bar{\mu}} \Omega_q^\dagger \Omega_q) \widetilde{B}^{\bar{\mu}\bar{\sigma}} (\bar{q}_s \gamma^{\bar{\sigma}} q_r) \right] \\
& - \frac{i}{6}g_Y(\mathcal{C}_{qq}^{(3)})^{srtt} \left[ 2(\Omega_{q,i}^* D_{\bar{\sigma}} \Omega_q^j) \widetilde{B}^{\bar{\rho}\bar{\sigma}} (\bar{q}_{js} \gamma^{\bar{\rho}} q_r^i) + 2(D_{\bar{\mu}} \Omega_{q,i}^* \Omega_q^j) \widetilde{B}^{\bar{\mu}\bar{\sigma}} (\bar{q}_{js} \gamma^{\bar{\sigma}} q_r^i) \right] \\
& + \frac{i}{6}g_Y(\mathcal{C}_{qq}^{(3)})^{sttr} \left[ 2(\Omega_{q,ai}^* D_{\bar{\rho}} \Omega_q^{bj}) \widetilde{B}^{\bar{\rho}\bar{\sigma}} (\bar{q}_{bjs} \gamma^{\bar{\sigma}} q_r^{ai}) - 2(D_{\bar{\mu}} \Omega_{q,ai}^* \Omega_q^{bj}) \widetilde{B}^{\bar{\mu}\bar{\sigma}} (\bar{q}_{bjs} \gamma^{\bar{\sigma}} q_r^{ai}) \right]
\end{aligned}$$

[illegible]

$$\begin{aligned}
& + \frac{1}{3}(\mathcal{C}_{qq}^{(3)})^{sttr} \left[ (D_{\bar{\nu}}\Omega_{q,b}^*\Omega_q^a)(D_{\bar{\mu}}\Omega_{q,ai}^*\Omega_q^{ck})\varepsilon^{\bar{\mu}\bar{\nu}\bar{\rho}\bar{\sigma}}(\bar{q}_{cks}\gamma^{\bar{\sigma}}D^{\bar{\rho}}q_r^{bi}) + (\Omega_{q,a}^*D_{\bar{\mu}}\Omega_q^c)(\Omega_{q,bj}^*D_{\bar{\rho}}\Omega_q^{ak})\varepsilon^{\bar{\mu}\bar{\nu}\bar{\rho}\bar{\sigma}}(D^{\bar{\nu}}\bar{q}_{cks}\gamma^{\bar{\sigma}}q_r^{bj}) \right] \\
& + \frac{1}{3}(\mathcal{C}_{qq}^{(3)})^{sttr} \left[ (\Omega_{q,a}^*D_{\bar{\mu}}\Omega_q^c)(\Omega_{q,bj}^*D_{\bar{\rho}}\Omega_q^{ak})\varepsilon^{\bar{\mu}\bar{\nu}\bar{\rho}\bar{\sigma}}(\bar{q}_{cks}\gamma^{\bar{\sigma}}D^{\bar{\rho}}q_r^{bj}) + (D_{\bar{\nu}}\Omega_{q,b}^*\Omega_q^a)(D_{\bar{\mu}}\Omega_{q,ai}^*\Omega_q^{ck})\varepsilon^{\bar{\mu}\bar{\nu}\bar{\rho}\bar{\sigma}}(D^{\bar{\rho}}\bar{q}_{cks}\gamma^{\bar{\sigma}}q_r^{bi}) \right] \\
& + \frac{i}{3}y_d^{vu}\bar{y}_d^{tu}(\mathcal{C}_{qq}^{(3)})^{srtv}(\Omega_d^\dagger\bar{D}_{\bar{\mu}}\Omega_d)(H^\dagger H)(\bar{q}_s\gamma^{\bar{\mu}}q_r) + \frac{i}{3}y_d^{vu}\bar{y}_d^{tu}(\mathcal{C}_{qq}^{(3)})^{svtr}(\Omega_{d,a}^*\bar{D}_{\bar{\mu}}\Omega_d^b)(\bar{q}_{bs}H\gamma^{\bar{\mu}}H^\dagger q_r^a) \\
& - \frac{i}{3}y_u^{vu}\bar{y}_u^{tu}(\mathcal{C}_{qq}^{(3)})^{srtv}(\Omega_u^\dagger\bar{D}_{\bar{\mu}}\Omega_u)(H^\dagger H)(\bar{q}_s\gamma^{\bar{\mu}}q_r) - \frac{i}{3}y_u^{vu}\bar{y}_u^{tu}(\mathcal{C}_{qq}^{(3)})^{svtr}(\Omega_{u,a}^*\bar{D}_{\bar{\mu}}\Omega_u^b)(H^\dagger H)(\bar{q}_{bs}\gamma^{\bar{\mu}}q_r^a) \\
& - \frac{i}{3}y_u^{vu}\bar{y}_u^{tu}(\mathcal{C}_{qq}^{(3)})^{svtr}(\Omega_{u,a}^*\bar{D}_{\bar{\mu}}\Omega_u^b)(\bar{q}_{bs}H\gamma^{\bar{\mu}}H^\dagger q_r^a) \\
& + \frac{i}{2}g_s(\mathcal{C}_{qq}^{(3)})^{srtt} \left[ 2T_b^{Aa}(\Omega_{q,a}^*D_{\bar{\sigma}}\Omega_q^b)\tilde{G}^{\bar{\rho}\bar{\sigma}A}(\bar{q}_s\gamma^{\bar{\rho}}q_r) + 2T_b^{Aa}(D_{\bar{\mu}}\Omega_{q,a}^*\Omega_q^b)\tilde{G}^{\bar{\mu}\bar{\sigma}A}(\bar{q}_s\gamma^{\bar{\sigma}}q_r) \right] \\
& - \frac{2i}{3}(\mathcal{C}_{qq}^{(3)})^{srtt} \left[ (D_q^\dagger D_{\bar{\nu}}\Omega_q)(D^{\bar{\mu}}\bar{q}_s\gamma^{\bar{\nu}}D^{\bar{\mu}}q_r) - (D_{\bar{\mu}}\Omega_q^\dagger\Omega_q)(D^{\bar{\nu}}\bar{q}_s\gamma^{\bar{\mu}}D^{\bar{\nu}}q_r) \right] \\
& - \frac{2i}{3}(\mathcal{C}_{qq}^{(3)})^{srtt} \left[ (D_q^\dagger D_{\bar{\nu}}\Omega_q)(D^{\bar{\mu}}D^{\bar{\mu}}\bar{q}_s\gamma^{\bar{\nu}}q_r) - (D_{\bar{\mu}}\Omega_q^\dagger\Omega_q)(\bar{q}_s\gamma^{\bar{\mu}}D^{\bar{\nu}}D^{\bar{\nu}}q_r) \right] \\
& + \frac{2i}{3}(\mathcal{C}_{qq}^{(3)})^{srtt} \left[ (\Omega_{q,i}^*D_2D_{\bar{\mu}}\Omega_q^j)(\bar{q}_{js}\gamma^{\bar{\mu}}q_r^i) - (D_2D_{\bar{\nu}}\Omega_{q,i}^*\Omega_q^j)(\bar{q}_{js}\gamma^{\bar{\nu}}q_r^i) \right] \\
& + \frac{2i}{3}(\mathcal{C}_{qq}^{(3)})^{sttr} \left[ (\Omega_{q,a}^*D_2D_{\bar{\mu}}\Omega_q^b)(\bar{q}_{bs}\gamma^{\bar{\mu}}q_r^a) - (D_2D_{\bar{\nu}}\Omega_{q,a}^*\Omega_q^b)(\bar{q}_{bs}\gamma^{\bar{\nu}}q_r^a) \right] \\
& - \frac{2i}{3}(\mathcal{C}_{qq}^{(3)})^{srtt} \left[ (D_{\bar{\mu}}\Omega_{q,ai}^*D_{\bar{\nu}}\Omega_q^{bj})(\Omega_{q,bj}^*D_{\bar{\mu}}\Omega_q^{ak})(\bar{q}_{ks}\gamma^{\bar{\nu}}q_r^i) - (D_{\bar{\mu}}\Omega_{q,ai}^*\Omega_q^{bj})(D_{\bar{\nu}}\Omega_{q,bj}^*D_{\bar{\mu}}\Omega_q^{ak})(\bar{q}_{ks}\gamma^{\bar{\nu}}q_r^i) \right] \\
& + \frac{2i}{3}(\mathcal{C}_{qq}^{(3)})^{srtt} \left[ (\Omega_{q,ai}^*D_{\bar{\mu}}\Omega_q^{bk})(D_{\bar{\mu}}D_{\bar{\nu}}\Omega_{q,bj}^*\Omega_q^{ai})(\bar{q}_{ks}\gamma^{\bar{\nu}}q_r^j) - (\Omega_{q,ai}^*D_{\bar{\mu}}D_{\bar{\nu}}\Omega_q^{bk})(D_{\bar{\mu}}\Omega_{q,bj}^*\Omega_q^{ai})(\bar{q}_{ks}\gamma^{\bar{\nu}}q_r^j) \right] \\
& + \frac{2}{3}(\mathcal{C}_{qq}^{(3)})^{srtt} \left[ (D_{\bar{\mu}}\Omega_{q,a}^*D_{\bar{\rho}}\Omega_q^b)(\Omega_{q,bj}^*D_{\bar{\sigma}}\Omega_q^{ak})\varepsilon^{\bar{\mu}\bar{\nu}\bar{\rho}\bar{\sigma}}(\bar{q}_{ks}\gamma^{\bar{\nu}}q_r^j) - (D_{\bar{\nu}}\Omega_{q,b}^*D_{\bar{\rho}}\Omega_q^a)(D_{\bar{\mu}}\Omega_{q,ai}^*\Omega_q^{bk})\varepsilon^{\bar{\mu}\bar{\nu}\bar{\rho}\bar{\sigma}}(\bar{q}_{ks}\gamma^{\bar{\sigma}}q_r^i) \right] \\
& - \frac{2i}{3}(\mathcal{C}_{qq}^{(3)})^{srtt} \left[ (\Omega_{q,ai}^*D_{\bar{\mu}}\Omega_q^{bk})(\Omega_{q,bj}^*D_{\bar{\nu}}\Omega_q^{ai})(D^{\bar{\mu}}\bar{q}_{ks}\gamma^{\bar{\nu}}q_r^j) - (D_{\bar{\mu}}\Omega_{q,ai}^*\Omega_q^{bk})(D_{\bar{\nu}}\Omega_{q,bj}^*\Omega_q^{ai})(\bar{q}_{ks}\gamma^{\bar{\mu}}D^{\bar{\nu}}q_r^j) \right] \\
& - \frac{2i}{3}(\mathcal{C}_{qq}^{(3)})^{srtt} \left[ (\Omega_{q,ai}^*D_{\bar{\nu}}\Omega_q^{bk})(\Omega_{q,bj}^*D_{\bar{\mu}}\Omega_q^{ai})(\bar{q}_{ks}\gamma^{\bar{\mu}}D^{\bar{\nu}}q_r^j) - (D_{\bar{\mu}}\Omega_{q,ai}^*\Omega_q^{bk})(D_{\bar{\nu}}\Omega_{q,bj}^*\Omega_q^{ai})(D^{\bar{\nu}}\bar{q}_{ks}\gamma^{\bar{\mu}}q_r^j) \right] \\
& - \frac{2}{3}(\mathcal{C}_{qq}^{(3)})^{srtt} \left[ (D_{\bar{\mu}}\Omega_{q,a}^*\Omega_q^b)(D_{\bar{\nu}}\Omega_{q,bj}^*\Omega_q^{ak})\varepsilon^{\bar{\mu}\bar{\nu}\bar{\rho}\bar{\sigma}}(\bar{q}_{ks}\gamma^{\bar{\rho}}D^{\bar{\sigma}}q_r^j) + (\Omega_{q,b}^*D_{\bar{\sigma}}\Omega_q^a)(\Omega_{q,ai}^*D_{\bar{\nu}}\Omega_q^{bk})\varepsilon^{\bar{\mu}\bar{\nu}\bar{\rho}\bar{\sigma}}(D^{\bar{\rho}}\bar{q}_{ks}\gamma^{\bar{\mu}}q_r^i) \right] \\
& - \frac{2i}{3}(\mathcal{C}_{qq}^{(3)})^{sttr} \left[ (\Omega_{q,a}^*D_{\bar{\mu}}\Omega_q^c)(D_{\bar{\mu}}\Omega_{q,b}^*D_{\bar{\nu}}\Omega_q^a)(\bar{q}_{cs}\gamma^{\bar{\nu}}q_r^b) - (D_{\bar{\mu}}\Omega_{q,a}^*D_{\bar{\nu}}\Omega_q^c)(D_{\bar{\nu}}\Omega_{q,b}^*\Omega_q^a)(\bar{q}_{cs}\gamma^{\bar{\mu}}q_r^b) \right] \\
& - \frac{2i}{3}(\mathcal{C}_{qq}^{(3)})^{sttr} \left[ (\Omega_{q,ai}^*D_{\bar{\mu}}\Omega_q^{cj})(D_{\bar{\mu}}\Omega_{q,bj}^*D_{\bar{\nu}}\Omega_q^{ai})(\bar{q}_{cs}\gamma^{\bar{\nu}}q_r^b) - (D_{\bar{\mu}}\Omega_{q,ai}^*D_{\bar{\nu}}\Omega_q^{cj})(D_{\bar{\nu}}\Omega_{q,bj}^*\Omega_q^{ai})(\bar{q}_{cs}\gamma^{\bar{\mu}}q_r^b) \right] \\
& - \frac{2i}{3}(\mathcal{C}_{qq}^{(3)})^{sttr} \left[ (\Omega_{q,ai}^*D_{\bar{\nu}}\Omega_q^{bj})(D^{\bar{\mu}}\bar{q}_{bjs}\gamma^{\bar{\nu}}D^{\bar{\mu}}q_r^{ai}) - (D_{\bar{\mu}}\Omega_{q,ai}^*\Omega_q^{bj})(D^{\bar{\nu}}\bar{q}_{bjs}\gamma^{\bar{\mu}}D^{\bar{\nu}}q_r^{ai}) \right] \\
& - \frac{2i}{3}(\mathcal{C}_{qq}^{(3)})^{sttr} \left[ (\Omega_{q,ai}^*D_{\bar{\nu}}\Omega_q^{bj})(D^{\bar{\mu}}D^{\bar{\mu}}\bar{q}_{bjs}\gamma^{\bar{\nu}}q_r^{ai}) - (D_{\bar{\mu}}\Omega_{q,ai}^*\Omega_q^{bj})(\bar{q}_{bjs}\gamma^{\bar{\mu}}D^{\bar{\nu}}D^{\bar{\nu}}q_r^{ai}) \right] \\
& + \frac{2i}{3}(\mathcal{C}_{qq}^{(3)})^{sttr} \left[ (D_{\bar{\mu}}\Omega_{q,b}^*D_{\bar{\nu}}\Omega_q^a)(\Omega_{q,ai}^*D_{\bar{\mu}}\Omega_q^{ck})(\bar{q}_{cks}\gamma^{\bar{\nu}}q_r^{bi}) - (D_{\bar{\mu}}\Omega_{q,a}^*D_{\bar{\nu}}\Omega_q^c)(D_{\bar{\nu}}\Omega_{q,bj}^*\Omega_q^{ak})(\bar{q}_{cks}\gamma^{\bar{\mu}}q_r^{bj}) \right] \\
& - \frac{2i}{3}(\mathcal{C}_{qq}^{(3)})^{sttr} \left[ (\Omega_{q,ai}^*D_{\bar{\mu}}\Omega_q^{cj})(D_{\bar{\mu}}\Omega_{q,bj}^*D_{\bar{\nu}}\Omega_q^{ak})(\bar{q}_{cks}\gamma^{\bar{\nu}}q_r^{bi}) - (D_{\bar{\mu}}\Omega_{q,ai}^*D_{\bar{\nu}}\Omega_q^{cj})(D_{\bar{\nu}}\Omega_{q,bj}^*\Omega_q^{ak})(\bar{q}_{cks}\gamma^{\bar{\mu}}q_r^{bi}) \right] \\
& + \frac{2i}{3}(\mathcal{C}_{qq}^{(3)})^{sttr} \left[ (\Omega_{q,b}^*D_{\bar{\nu}}\Omega_q^a)(D_{\bar{\mu}}D_{\bar{\nu}}\Omega_{q,ai}^*\Omega_q^{ck})(\bar{q}_{cks}\gamma^{\bar{\mu}}q_r^{bi}) - (D_{\bar{\mu}}\Omega_{q,a}^*\Omega_q^c)(\Omega_{q,bj}^*D_{\bar{\nu}}D_{\bar{\mu}}\Omega_q^{ak})(\bar{q}_{cks}\gamma^{\bar{\nu}}q_r^{bj}) \right]
\end{aligned}$$

$$\begin{aligned}
& -\frac{2i}{3}(\mathcal{C}_{qq}^{(3)})^{sttr} \left[ (D_{\bar{\mu}}\Omega_{q,b}^* D_{\bar{\nu}}\Omega_q^a)(\Omega_{q,ai}^* D_{\bar{\nu}}\Omega_q^{ck})(\bar{q}_{cks}\gamma^{\bar{\mu}} q_r^{bi}) - (D_{\bar{\mu}}\Omega_{q,a}^* D_{\bar{\nu}}\Omega_q^c)(D_{\bar{\mu}}\Omega_{q,bj}^* \Omega_q^{ak})(\bar{q}_{cks}\gamma^{\bar{\nu}} q_r^{bj}) \right] \\
& + \frac{2i}{3}(\mathcal{C}_{qq}^{(3)})^{sttr} \left[ (\Omega_{q,a}^* D_{\bar{\mu}}\Omega_q^c)(D_{\bar{\mu}}\Omega_{q,bj}^* D_{\bar{\nu}}\Omega_q^{ak})(\bar{q}_{cks}\gamma^{\bar{\nu}} q_r^{bj}) - (D_{\bar{\nu}}\Omega_{q,b}^* \Omega_q^a)(D_{\bar{\mu}}\Omega_{q,ai}^* D_{\bar{\nu}}\Omega_q^{ck})(\bar{q}_{cks}\gamma^{\bar{\mu}} q_r^{bi}) \right] \\
& - \frac{2}{3}(\mathcal{C}_{qq}^{(3)})^{sttr} \left[ (\Omega_{q,a}^* D_{\bar{\nu}}\Omega_q^c)(D_{\bar{\mu}}\Omega_{q,bj}^* D_{\bar{\rho}}\Omega_q^{ak})\varepsilon^{\bar{\mu}\bar{\nu}\bar{\rho}\bar{\sigma}}(\bar{q}_{cks}\gamma^{\bar{\sigma}} q_r^{bj}) - (D_{\bar{\nu}}\Omega_{q,b}^* \Omega_q^a)(D_{\bar{\mu}}\Omega_{q,ai}^* D_{\bar{\rho}}\Omega_q^{ck})\varepsilon^{\bar{\mu}\bar{\nu}\bar{\rho}\bar{\sigma}}(\bar{q}_{cks}\gamma^{\bar{\sigma}} q_r^{bi}) \right] \\
& - \frac{2i}{3}y_d^{vu}\bar{y}_d^{tu}(\mathcal{C}_{qq}^{(3)})^{srtv}(\Omega_d^\dagger \overleftrightarrow{D}_{\bar{\mu}}\Omega_d)(\bar{q}_s H\gamma^{\bar{\mu}} H^\dagger q_r) - \frac{2i}{3}y_d^{vu}\bar{y}_d^{tu}(\mathcal{C}_{qq}^{(3)})^{svtr}(\Omega_{d,a}^* \overleftrightarrow{D}_{\bar{\mu}}\Omega_d^b)(H^\dagger H)(\bar{q}_{bs}\gamma^{\bar{\mu}} q_r^a) \\
& + \frac{2i}{3}y_u^{vu}\bar{y}_u^{tu}(\mathcal{C}_{qq}^{(3)})^{srtv}(\Omega_u^\dagger \overleftrightarrow{D}_{\bar{\mu}}\Omega_u)(\bar{q}_s H\gamma^{\bar{\mu}} H^\dagger q_r) \\
& - \frac{5i}{6}g_L(\mathcal{C}_{qq}^{(3)})^{srtt} \left[ 2(\Omega_q^\dagger D_{\bar{\sigma}}\Omega_q)\widetilde{W}^{\bar{\rho}\bar{\sigma}I}(\bar{q}_s t^I \gamma^{\bar{\rho}} q_r) + 2(D_{\bar{\mu}}\Omega_q^\dagger \Omega_q)\widetilde{W}^{\bar{\mu}\bar{\sigma}I}(\bar{q}_s t^I \gamma^{\bar{\sigma}} q_r) \right] \\
& + ig_s(\mathcal{C}_{qq}^{(3)})^{srtt} \left[ 2T_b^{Aa}(\Omega_{q,ai}^* D_{\bar{\rho}}\Omega_q^{bj})\widetilde{G}^{\bar{\rho}\bar{\sigma}A}(\bar{q}_{js}\gamma^{\bar{\sigma}} q_r^i) - 2T_b^{Aa}(D_{\bar{\mu}}\Omega_{q,ai}^* \Omega_q^{bj})\widetilde{G}^{\bar{\mu}\bar{\sigma}A}(\bar{q}_{js}\gamma^{\bar{\sigma}} q_r^i) \right] \\
& + ig_s(\mathcal{C}_{qq}^{(3)})^{sttr} \left[ 2T_b^{Aa}(\Omega_{q,ai}^* D_{\bar{\rho}}\Omega_q^{cj})\widetilde{G}^{\bar{\rho}\bar{\sigma}A}(\bar{q}_{cjs}\gamma^{\bar{\sigma}} q_r^{bi}) - 2T_c^{Ab}(D_{\bar{\mu}}\Omega_{q,ai}^* \Omega_q^{cj})\widetilde{G}^{\bar{\mu}\bar{\sigma}A}(\bar{q}_{bj}s\gamma^{\bar{\sigma}} q_r^{ai}) \right] \\
& + \frac{7i}{6}g_L(\mathcal{C}_{qq}^{(3)})^{sttr} \left[ 2(\Omega_{q,a}^* D_{\bar{\rho}}\Omega_q^b)\widetilde{W}^{\bar{\rho}\bar{\sigma}I}(\bar{q}_{bs}t^I \gamma^{\bar{\sigma}} q_r^a) - 2(D_{\bar{\mu}}\Omega_{q,a}^* \Omega_q^b)\widetilde{W}^{\bar{\mu}\bar{\sigma}I}(\bar{q}_{bs}t^I \gamma^{\bar{\sigma}} q_r^a) \right] \\
& + \frac{4i}{3}(\mathcal{C}_{qq}^{(3)})^{srtt} \left[ (\Omega_{q,i}^* D_{\bar{\nu}}\Omega_q^j)(D_{\bar{\mu}}\bar{q}_{js}\gamma^{\bar{\nu}} D_{\bar{\mu}} q_r^i) - (D_{\bar{\mu}}\Omega_{q,i}^* \Omega_q^j)(D_{\bar{\nu}}\bar{q}_{js}\gamma^{\bar{\mu}} D_{\bar{\nu}} q_r^i) \right] \\
& + \frac{4i}{3}(\mathcal{C}_{qq}^{(3)})^{srtt} \left[ (\Omega_{q,i}^* D_{\bar{\nu}}\Omega_q^j)(D_{\bar{\mu}}D_{\bar{\nu}}\bar{q}_{js}\gamma^{\bar{\nu}} q_r^i) - (D_{\bar{\mu}}\Omega_{q,i}^* \Omega_q^j)(\bar{q}_{js}\gamma^{\bar{\mu}} D_{\bar{\nu}} D_{\bar{\nu}} q_r^i) \right] \\
& + \frac{4i}{3}(\mathcal{C}_{qq}^{(3)})^{sttr} \left[ (\Omega_{q,a}^* D_{\bar{\nu}}\Omega_q^b)(D_{\bar{\mu}}\bar{q}_{bs}\gamma^{\bar{\nu}} D_{\bar{\mu}} q_r^a) - (D_{\bar{\mu}}\Omega_{q,a}^* \Omega_q^b)(D_{\bar{\nu}}\bar{q}_{bs}\gamma^{\bar{\mu}} D_{\bar{\nu}} q_r^a) \right] \\
& + \frac{4i}{3}(\mathcal{C}_{qq}^{(3)})^{sttr} \left[ (\Omega_{q,a}^* D_{\bar{\nu}}\Omega_q^b)(D_{\bar{\mu}}D_{\bar{\nu}}\bar{q}_{bs}\gamma^{\bar{\nu}} q_r^a) - (D_{\bar{\mu}}\Omega_{q,a}^* \Omega_q^b)(\bar{q}_{bs}\gamma^{\bar{\mu}} D_{\bar{\nu}} D_{\bar{\nu}} q_r^a) \right] \\
& + \frac{4i}{3}(\mathcal{C}_{qq}^{(3)})^{srtt} \left[ (D_{\bar{\mu}}\Omega_{q,ai}^* D_{\bar{\nu}}\Omega_q^{bk})(\Omega_{q,bj}^* D_{\bar{\mu}}\Omega_q^{ai})(\bar{q}_{ks}\gamma^{\bar{\nu}} q_r^j) - (D_{\bar{\mu}}\Omega_{q,ai}^* \Omega_q^{bk})(D_{\bar{\nu}}\Omega_{q,bj}^* D_{\bar{\mu}}\Omega_q^{ai})(\bar{q}_{ks}\gamma^{\bar{\nu}} q_r^j) \right] \\
& - \frac{4i}{3}(\mathcal{C}_{qq}^{(3)})^{svtr} \left[ y_d^{vu}\bar{y}_d^{tu} + y_u^{vu}\bar{y}_u^{tu} \right] \left[ (\Omega_{q,aj}^* D_{\bar{\mu}}\Omega_q^{bi})H_i^\dagger(\bar{q}_{bs}H\gamma^{\bar{\mu}} q_r^{aj}) - (D_{\bar{\mu}}\Omega_{q,aj}^* \Omega_q^{bk})H^j(\bar{q}_{bks}\gamma^{\bar{\mu}} H^\dagger q_r^a) \right] \\
& + \frac{4}{3}g_s(\mathcal{C}_{qq}^{(3)})^{sttr} \left[ T_b^{Aa}(\Omega_{q,ai}^* D_{\bar{\nu}}\Omega_q^{cj})G^{\bar{\mu}\bar{\nu}A}(\bar{q}_{cjs}\gamma^{\bar{\mu}} q_r^{bi}) - T_c^{Ab}(D_{\bar{\mu}}\Omega_{q,ai}^* \Omega_q^{cj})G^{\bar{\mu}\bar{\nu}A}(\bar{q}_{bj}s\gamma^{\bar{\nu}} q_r^{ai}) \right] \\
& + \frac{4i}{3}y_u^{vu}\bar{y}_u^{tu}(\mathcal{C}_{qq}^{(3)})^{srtv}(\Omega_q^\dagger \overleftrightarrow{D}_{\bar{\mu}}\Omega_q)(H^\dagger H)(\bar{q}_s\gamma^{\bar{\mu}} q_r) + \frac{4i}{3}y_u^{vu}\bar{y}_u^{tu}(\mathcal{C}_{qq}^{(3)})^{svtr}(\Omega_{q,a}^* \overleftrightarrow{D}_{\bar{\mu}}\Omega_q^b)(H^\dagger H)(\bar{q}_{bs}\gamma^{\bar{\mu}} q_r^a) \\
& + \frac{4i}{3}y_u^{vu}\bar{y}_u^{tu}(\mathcal{C}_{qq}^{(3)})^{svtr}(\Omega_{q,a}^* \overleftrightarrow{D}_{\bar{\mu}}\Omega_q^b)(\bar{q}_{bs}H\gamma^{\bar{\mu}} H^\dagger q_r^a) \\
& - \frac{4i}{3}(\mathcal{C}_{qq}^{(3)})^{srtv} \left[ y_d^{vu}\bar{y}_d^{tu} + y_u^{vu}\bar{y}_u^{tu} \right] (\Omega_{q,j}^* \overleftrightarrow{D}_{\bar{\mu}}\Omega_q^i)H_i^\dagger H^j(\bar{q}_s\gamma^{\bar{\mu}} q_r) \\
& + \frac{4i}{3}(\mathcal{C}_{qq}^{(3)})^{svtr} \left[ 2y_d^{vu}\bar{y}_d^{tu} - y_u^{vu}\bar{y}_u^{tu} \right] (\Omega_{q,aj}^* \overleftrightarrow{D}_{\bar{\mu}}\Omega_q^{bi})H_i^\dagger H^j(\bar{q}_{bs}\gamma^{\bar{\mu}} q_r^a) \\
& + \frac{3i}{2}g_s(\mathcal{C}_{qq}^{(3)})^{sttr} \left[ 2T_c^{Ab}(D_{\bar{\mu}}\Omega_{q,a}^* \Omega_q^c)\widetilde{G}^{\bar{\mu}\bar{\sigma}A}(\bar{q}_{bs}\gamma^{\bar{\sigma}} q_r^a) + 2T_b^{Aa}(\Omega_{q,a}^* D_{\bar{\sigma}}\Omega_q^c)\widetilde{G}^{\bar{\rho}\bar{\sigma}A}(\bar{q}_{cs}\gamma^{\bar{\rho}} q_r^b) \right] \\
& - 2g_L(\mathcal{C}_{qq}^{(3)})^{sttr} \left[ t_k^{Ij}(D_{\bar{\mu}}\Omega_{q,ai}^* \Omega_q^{bk})W^{\bar{\mu}\bar{\nu}I}(\bar{q}_{bj}s\gamma^{\bar{\nu}} q_r^{ai}) + t_j^{Ii}(\Omega_{q,ai}^* D_{\bar{\mu}}\Omega_q^{bk})W^{\bar{\mu}\bar{\nu}I}(\bar{q}_{bks}\gamma^{\bar{\nu}} q_r^{aj}) \right] \\
& - 2ig_L(\mathcal{C}_{qq}^{(3)})^{sttr} \left[ 2t_j^{Ii}(\Omega_{q,ai}^* D_{\bar{\rho}}\Omega_q^{bk})\widetilde{W}^{\bar{\rho}\bar{\sigma}I}(\bar{q}_{bks}\gamma^{\bar{\sigma}} q_r^{aj}) - 2t_k^{Ij}(D_{\bar{\mu}}\Omega_{q,ai}^* \Omega_q^{bk})\widetilde{W}^{\bar{\mu}\bar{\sigma}I}(\bar{q}_{bj}s\gamma^{\bar{\sigma}} q_r^{ai}) \right] \\
& + \frac{8i}{3}(\mathcal{C}_{qq}^{(3)})^{srtv} \left[ y_d^{vu}\bar{y}_d^{tu} + y_u^{vu}\bar{y}_u^{tu} \right] \left[ (\Omega_{q,j}^* D_{\bar{\mu}}\Omega_q^i)H_i^\dagger(\bar{q}_s H\gamma^{\bar{\mu}} q_r^j) - (D_{\bar{\mu}}\Omega_{q,j}^* \Omega_q^k)H^j(\bar{q}_{ks}\gamma^{\bar{\mu}} H^\dagger q_r) \right]
\end{aligned}$$

$$\begin{aligned}
& -\frac{8i}{3}y_u^{vu}\bar{y}_u^{tu}(\mathcal{C}_{qq}^{(3)})^{srtv}(\Omega_q^\dagger\overset{\leftrightarrow}{D}_{\bar{\mu}}\Omega_q)(\bar{q}_sH\gamma^{\bar{\mu}}H^\dagger q_r) \\
& -4g_L(\mathcal{C}_{qq}^{(3)})^{srtt}\left[t_j^{Ii}(\Omega_{q,i}^*D_{\bar{\nu}}\Omega_q^k)W^{\bar{\mu}\bar{\nu}I}(\bar{q}_{ks}\gamma^{\bar{\mu}}q_r^j)-t_k^{Ij}(D_{\bar{\mu}}\Omega_{q,i}^*\Omega_q^k)W^{\bar{\mu}\bar{\nu}I}(\bar{q}_{js}\gamma^{\bar{\nu}}q_r^i)\right] \\
& -\frac{13}{3}g_s(\mathcal{C}_{qq}^{(3)})^{sttr}\left[T_b^{Aa}(\Omega_{q,a}^*D_{\bar{\nu}}\Omega_q^c)G^{\bar{\mu}\bar{\nu}A}(\bar{q}_{cs}\gamma^{\bar{\mu}}q_r^b)-T_c^{Ab}(D_{\bar{\mu}}\Omega_{q,a}^*\Omega_q^c)G^{\bar{\mu}\bar{\nu}A}(\bar{q}_{bs}\gamma^{\bar{\nu}}q_r^a)\right], \tag{3.44}
\end{aligned}$$

$$\begin{aligned}
\Gamma_\Omega^{(1)}[\mathcal{O}_{eu}] &= \frac{i}{6}\mathcal{C}_{eu}^{srtt}\left[(\Omega_u^\dagger D_2 D_{\bar{\mu}}\Omega_u)(\bar{e}_s\gamma^{\bar{\mu}}e_r)-(D_2 D_{\bar{\nu}}\Omega_u^\dagger\Omega_u)(\bar{e}_s\gamma^{\bar{\nu}}e_r)\right] \\
& -\frac{1}{6}\mathcal{C}_{eu}^{srtt}\left[(D_{\bar{\mu}}\Omega_{u,a}^*D_{\bar{\rho}}\Omega_u^b)(\Omega_{u,b}^*D_{\bar{\sigma}}\Omega_u^a)\varepsilon^{\bar{\mu}\bar{\nu}\bar{\rho}\bar{\sigma}}(\bar{e}_s\gamma^{\bar{\nu}}e_r)-(D_{\bar{\mu}}\Omega_{u,a}^*\Omega_u^b)(D_{\bar{\nu}}\Omega_{u,b}^*D_{\bar{\rho}}\Omega_u^a)\varepsilon^{\bar{\mu}\bar{\nu}\bar{\rho}\bar{\sigma}}(\bar{e}_s\gamma^{\bar{\sigma}}e_r)\right] \\
& +\frac{i}{6}\mathcal{C}_{eu}^{ttsr}\left[(\Omega_e^\dagger D_2 D_{\bar{\mu}}\Omega_e)(\bar{u}_s\gamma^{\bar{\mu}}u_r)-(D_2 D_{\bar{\nu}}\Omega_e^\dagger\Omega_e)(\bar{u}_s\gamma^{\bar{\nu}}u_r)\right] \\
& -\frac{1}{6}\mathcal{C}_{eu}^{ttsr}\left[(\Omega_e^\dagger D_{\bar{\sigma}}\Omega_e)(D_{\bar{\mu}}\Omega_e^\dagger D_{\bar{\rho}}\Omega_e)\varepsilon^{\bar{\mu}\bar{\nu}\bar{\rho}\bar{\sigma}}(\bar{u}_s\gamma^{\bar{\nu}}u_r)+(D_{\bar{\mu}}\Omega_e^\dagger D_{\bar{\rho}}\Omega_e)(D_{\bar{\nu}}\Omega_e^\dagger\Omega_e)\varepsilon^{\bar{\mu}\bar{\nu}\bar{\rho}\bar{\sigma}}(\bar{u}_s\gamma^{\bar{\sigma}}u_r)\right] \\
& -\frac{i}{6}y_e^{tv}\bar{y}_e^{tu}\mathcal{C}_{eu}^{vvsr}(\Omega_{\ell,j}^*\overset{\leftrightarrow}{D}_{\bar{\mu}}\Omega_\ell^i)H_i^\dagger H^j(\bar{u}_s\gamma^{\bar{\mu}}u_r)-\frac{i}{6}y_u^{tv}\bar{y}_u^{tu}\mathcal{C}_{eu}^{srvu}(\Omega_q^\dagger\overset{\leftrightarrow}{D}_{\bar{\mu}}\Omega_q)(H^\dagger H)(\bar{e}_s\gamma^{\bar{\mu}}e_r) \\
& +\frac{i}{6}y_u^{tv}\bar{y}_u^{tu}\mathcal{C}_{eu}^{srvu}(\Omega_{q,j}^*\overset{\leftrightarrow}{D}_{\bar{\mu}}\Omega_q^i)H_i^\dagger H^j(\bar{e}_s\gamma^{\bar{\mu}}e_r) \\
& +\frac{2i}{9}g_Y\mathcal{C}_{eu}^{srtt}\left[2(\Omega_u^\dagger D_{\bar{\sigma}}\Omega_u)\tilde{B}^{\bar{\rho}\bar{\sigma}}(\bar{e}_s\gamma^{\bar{\rho}}e_r)+2(D_{\bar{\mu}}\Omega_u^\dagger\Omega_u)\tilde{B}^{\bar{\mu}\bar{\sigma}}(\bar{e}_s\gamma^{\bar{\sigma}}e_r)\right] \\
& +\frac{i}{3}g_s\mathcal{C}_{eu}^{srtt}\left[2T_b^{Aa}(\Omega_{u,a}^*D_{\bar{\sigma}}\Omega_u^b)\tilde{G}^{\bar{\rho}\bar{\sigma}A}(\bar{e}_s\gamma^{\bar{\rho}}e_r)+2T_b^{Aa}(D_{\bar{\mu}}\Omega_{u,a}^*\Omega_u^b)\tilde{G}^{\bar{\mu}\bar{\sigma}A}(\bar{e}_s\gamma^{\bar{\sigma}}e_r)\right] \\
& +\frac{i}{3}\mathcal{C}_{eu}^{srtt}\left[(\Omega_u^\dagger D_{\bar{\nu}}\Omega_u)(D^{\bar{\mu}}\bar{e}_s\gamma^{\bar{\nu}}D^{\bar{\mu}}e_r)-(D_{\bar{\mu}}\Omega_u^\dagger\Omega_u)(D^{\bar{\nu}}\bar{e}_s\gamma^{\bar{\mu}}D^{\bar{\nu}}e_r)\right] \\
& +\frac{i}{3}\mathcal{C}_{eu}^{srtt}\left[(\Omega_u^\dagger D_{\bar{\nu}}\Omega_u)(D^{\bar{\mu}}D^{\bar{\mu}}\bar{e}_s\gamma^{\bar{\nu}}e_r)-(D_{\bar{\mu}}\Omega_u^\dagger\Omega_u)(\bar{e}_s\gamma^{\bar{\mu}}D^{\bar{\nu}}D^{\bar{\nu}}e_r)\right] \\
& -\frac{i}{3}g_Y\mathcal{C}_{eu}^{ttsr}\left[2(\Omega_e^\dagger D_{\bar{\sigma}}\Omega_e)\tilde{B}^{\bar{\rho}\bar{\sigma}}(\bar{u}_s\gamma^{\bar{\rho}}u_r)+2(D_{\bar{\mu}}\Omega_e^\dagger\Omega_e)\tilde{B}^{\bar{\mu}\bar{\sigma}}(\bar{u}_s\gamma^{\bar{\sigma}}u_r)\right] \\
& +\frac{i}{3}\mathcal{C}_{eu}^{ttsr}\left[(\Omega_e^\dagger D_{\bar{\nu}}\Omega_e)(D^{\bar{\mu}}\bar{u}_s\gamma^{\bar{\nu}}D^{\bar{\mu}}u_r)-(D_{\bar{\mu}}\Omega_e^\dagger\Omega_e)(D^{\bar{\nu}}\bar{u}_s\gamma^{\bar{\mu}}D^{\bar{\nu}}u_r)\right] \\
& +\frac{i}{3}\mathcal{C}_{eu}^{ttsr}\left[(\Omega_e^\dagger D_{\bar{\nu}}\Omega_e)(D^{\bar{\mu}}D^{\bar{\mu}}\bar{u}_s\gamma^{\bar{\nu}}u_r)-(D_{\bar{\mu}}\Omega_e^\dagger\Omega_e)(\bar{u}_s\gamma^{\bar{\mu}}D^{\bar{\nu}}D^{\bar{\nu}}u_r)\right] \\
& +\frac{2i}{3}y_e^{tv}\bar{y}_e^{tu}\mathcal{C}_{eu}^{vvsr}(\Omega_e^\dagger\overset{\leftrightarrow}{D}_{\bar{\mu}}\Omega_e)(H^\dagger H)(\bar{u}_s\gamma^{\bar{\mu}}u_r)+\frac{2i}{3}y_u^{tv}\bar{y}_u^{tu}\mathcal{C}_{eu}^{srvu}(\Omega_u^\dagger\overset{\leftrightarrow}{D}_{\bar{\mu}}\Omega_u)(H^\dagger H)(\bar{e}_s\gamma^{\bar{\mu}}e_r), \tag{3.45}
\end{aligned}$$

$$\begin{aligned}
\Gamma_\Omega^{(1)}[\mathcal{O}_{ed}] &= -\frac{i}{9}g_Y\mathcal{C}_{ed}^{srtt}\left[2(\Omega_d^\dagger D_{\bar{\sigma}}\Omega_d)\tilde{B}^{\bar{\rho}\bar{\sigma}}(\bar{e}_s\gamma^{\bar{\rho}}e_r)+2(D_{\bar{\mu}}\Omega_d^\dagger\Omega_d)\tilde{B}^{\bar{\mu}\bar{\sigma}}(\bar{e}_s\gamma^{\bar{\sigma}}e_r)\right] \\
& +\frac{i}{6}\mathcal{C}_{ed}^{ttsr}\left[(\Omega_e^\dagger D_2 D_{\bar{\mu}}\Omega_e)(\bar{d}_s\gamma^{\bar{\mu}}d_r)-(D_2 D_{\bar{\nu}}\Omega_e^\dagger\Omega_e)(\bar{d}_s\gamma^{\bar{\nu}}d_r)\right] \\
& -\frac{1}{6}\mathcal{C}_{ed}^{ttsr}\left[(\Omega_e^\dagger D_{\bar{\sigma}}\Omega_e)(D_{\bar{\mu}}\Omega_e^\dagger D_{\bar{\rho}}\Omega_e)\varepsilon^{\bar{\mu}\bar{\nu}\bar{\rho}\bar{\sigma}}(\bar{d}_s\gamma^{\bar{\nu}}d_r)+(D_{\bar{\mu}}\Omega_e^\dagger D_{\bar{\rho}}\Omega_e)(D_{\bar{\nu}}\Omega_e^\dagger\Omega_e)\varepsilon^{\bar{\mu}\bar{\nu}\bar{\rho}\bar{\sigma}}(\bar{d}_s\gamma^{\bar{\sigma}}d_r)\right] \\
& +\frac{i}{6}\mathcal{C}_{ed}^{srtt}\left[(\Omega_d^\dagger D_2 D_{\bar{\mu}}\Omega_d)(\bar{e}_s\gamma^{\bar{\mu}}e_r)-(D_2 D_{\bar{\nu}}\Omega_d^\dagger\Omega_d)(\bar{e}_s\gamma^{\bar{\nu}}e_r)\right] \\
& -\frac{1}{6}\mathcal{C}_{ed}^{srtt}\left[(D_{\bar{\mu}}\Omega_{d,a}^*D_{\bar{\rho}}\Omega_d^b)(\Omega_{d,b}^*D_{\bar{\sigma}}\Omega_d^a)\varepsilon^{\bar{\mu}\bar{\nu}\bar{\rho}\bar{\sigma}}(\bar{e}_s\gamma^{\bar{\nu}}e_r)-(D_{\bar{\mu}}\Omega_{d,a}^*\Omega_d^b)(D_{\bar{\nu}}\Omega_{d,b}^*D_{\bar{\rho}}\Omega_d^a)\varepsilon^{\bar{\mu}\bar{\nu}\bar{\rho}\bar{\sigma}}(\bar{e}_s\gamma^{\bar{\sigma}}e_r)\right] \\
& -\frac{i}{6}y_e^{tv}\bar{y}_e^{tu}\mathcal{C}_{ed}^{vvsr}(\Omega_{\ell,j}^*\overset{\leftrightarrow}{D}_{\bar{\mu}}\Omega_\ell^i)H_i^\dagger H^j(\bar{d}_s\gamma^{\bar{\mu}}d_r)-\frac{i}{6}y_d^{tv}\bar{y}_d^{tu}\mathcal{C}_{ed}^{srvu}(\Omega_{q,j}^*\overset{\leftrightarrow}{D}_{\bar{\mu}}\Omega_q^i)H_i^\dagger H^j(\bar{e}_s\gamma^{\bar{\mu}}e_r)
\end{aligned}$$

$$\begin{aligned}
& -\frac{i}{3}g_Y\mathcal{C}_{ed}^{ttsr}\left[2(\Omega_e^\dagger D_{\bar{\sigma}}\Omega_e)\tilde{B}^{\bar{\rho}\bar{\sigma}}(\bar{d}_s\gamma^{\bar{\rho}}d_r)+2(D_{\bar{\mu}}\Omega_e^\dagger\Omega_e)\tilde{B}^{\bar{\mu}\bar{\sigma}}(\bar{d}_s\gamma^{\bar{\sigma}}d_r)\right] \\
& +\frac{i}{3}\mathcal{C}_{ed}^{ttsr}\left[(\Omega_e^\dagger D_{\bar{\nu}}\Omega_e)(D^{\bar{\mu}}\bar{d}_s\gamma^{\bar{\nu}}D^{\bar{\mu}}d_r)-(D_{\bar{\mu}}\Omega_e^\dagger\Omega_e)(D^{\bar{\nu}}\bar{d}_s\gamma^{\bar{\mu}}D^{\bar{\nu}}d_r)\right] \\
& +\frac{i}{3}\mathcal{C}_{ed}^{ttsr}\left[(\Omega_e^\dagger D_{\bar{\nu}}\Omega_e)(D^{\bar{\mu}}D^{\bar{\mu}}\bar{d}_s\gamma^{\bar{\nu}}d_r)-(D_{\bar{\mu}}\Omega_e^\dagger\Omega_e)(\bar{d}_s\gamma^{\bar{\mu}}D^{\bar{\nu}}D^{\bar{\nu}}d_r)\right] \\
& +\frac{i}{3}g_s\mathcal{C}_{ed}^{srtt}\left[2T_b^{Aa}(\Omega_{d,a}^*D_{\bar{\sigma}}\Omega_d^b)\tilde{G}^{\bar{\rho}\bar{\sigma}A}(\bar{e}_s\gamma^{\bar{\rho}}e_r)+2T_b^{Aa}(D_{\bar{\mu}}\Omega_{d,a}^*\Omega_d^b)\tilde{G}^{\bar{\mu}\bar{\sigma}A}(\bar{e}_s\gamma^{\bar{\sigma}}e_r)\right] \\
& +\frac{i}{3}\mathcal{C}_{ed}^{srtt}\left[(\Omega_d^\dagger D_{\bar{\nu}}\Omega_d)(D^{\bar{\mu}}\bar{e}_s\gamma^{\bar{\nu}}D^{\bar{\mu}}e_r)-(D_{\bar{\mu}}\Omega_d^\dagger\Omega_d)(D^{\bar{\nu}}\bar{e}_s\gamma^{\bar{\mu}}D^{\bar{\nu}}e_r)\right] \\
& +\frac{i}{3}\mathcal{C}_{ed}^{srtt}\left[(\Omega_d^\dagger D_{\bar{\nu}}\Omega_d)(D^{\bar{\mu}}D^{\bar{\mu}}\bar{e}_s\gamma^{\bar{\nu}}e_r)-(D_{\bar{\mu}}\Omega_d^\dagger\Omega_d)(\bar{e}_s\gamma^{\bar{\mu}}D^{\bar{\nu}}D^{\bar{\nu}}e_r)\right] \\
& +\frac{2i}{3}y_d^{tv}\bar{y}_d^{tu}\mathcal{C}_{ed}^{srrv}(\Omega_d^\dagger\overset{\leftrightarrow}{D}_{\bar{\mu}}\Omega_d)(H^\dagger H)(\bar{e}_s\gamma^{\bar{\mu}}e_r)+\frac{2i}{3}y_e^{tv}\bar{y}_e^{tu}\mathcal{C}_{ed}^{vsur}(\Omega_e^\dagger\overset{\leftrightarrow}{D}_{\bar{\mu}}\Omega_e)(H^\dagger H)(\bar{d}_s\gamma^{\bar{\mu}}d_r), \tag{3.46}
\end{aligned}$$

$$\begin{aligned}
\Gamma_\Omega^{(1)}[\mathcal{O}_{qe}] &= -\frac{i}{18}g_Y\mathcal{C}_{qe}^{ttsr}\left[2(\Omega_q^\dagger D_{\bar{\sigma}}\Omega_q)\tilde{B}^{\bar{\rho}\bar{\sigma}}(\bar{e}_s\gamma^{\bar{\rho}}e_r)+2(D_{\bar{\mu}}\Omega_q^\dagger\Omega_q)\tilde{B}^{\bar{\mu}\bar{\sigma}}(\bar{e}_s\gamma^{\bar{\sigma}}e_r)\right] \\
& +\frac{i}{6}\mathcal{C}_{qe}^{ttsr}\left[(\Omega_q^\dagger D_2D_{\bar{\mu}}\Omega_q)(\bar{e}_s\gamma^{\bar{\mu}}e_r)-(D_2D_{\bar{\nu}}\Omega_q^\dagger\Omega_q)(\bar{e}_s\gamma^{\bar{\nu}}e_r)\right] \\
& +\frac{1}{6}\mathcal{C}_{qe}^{ttsr}\left[(D_{\bar{\mu}}\Omega_{q,ai}^*D_{\bar{\rho}}\Omega_q^{bj})(\Omega_{q,bj}^*D_{\bar{\sigma}}\Omega_q^{ai})\varepsilon^{\bar{\mu}\bar{\nu}\bar{\rho}\bar{\sigma}}(\bar{e}_s\gamma^{\bar{\nu}}e_r)-(D_{\bar{\mu}}\Omega_{q,ai}^*\Omega_q^{bj})(D_{\bar{\nu}}\Omega_{q,bj}^*D_{\bar{\rho}}\Omega_q^{ai})\varepsilon^{\bar{\mu}\bar{\nu}\bar{\rho}\bar{\sigma}}(\bar{e}_s\gamma^{\bar{\sigma}}e_r)\right] \\
& +\frac{i}{6}\mathcal{C}_{qe}^{srtt}\left[(\Omega_e^\dagger D_2D_{\bar{\mu}}\Omega_e)(\bar{q}_s\gamma^{\bar{\mu}}q_r)-(D_2D_{\bar{\nu}}\Omega_e^\dagger\Omega_e)(\bar{q}_s\gamma^{\bar{\nu}}q_r)\right] \\
& -\frac{1}{6}\mathcal{C}_{qe}^{srtt}\left[(\Omega_e^\dagger D_{\bar{\sigma}}\Omega_e)(D_{\bar{\mu}}\Omega_e^\dagger D_{\bar{\rho}}\Omega_e)\varepsilon^{\bar{\mu}\bar{\nu}\bar{\rho}\bar{\sigma}}(\bar{q}_s\gamma^{\bar{\nu}}q_r)+(D_{\bar{\mu}}\Omega_e^\dagger D_{\bar{\rho}}\Omega_e)(D_{\bar{\nu}}\Omega_e^\dagger\Omega_e)\varepsilon^{\bar{\mu}\bar{\nu}\bar{\rho}\bar{\sigma}}(\bar{q}_s\gamma^{\bar{\sigma}}q_r)\right] \\
& -\frac{i}{6}y_d^{vu}\bar{y}_d^{tu}\mathcal{C}_{qe}^{tvsr}(\Omega_d^\dagger\overset{\leftrightarrow}{D}_{\bar{\mu}}\Omega_d)(H^\dagger H)(\bar{e}_s\gamma^{\bar{\mu}}e_r)-\frac{i}{6}y_e^{tv}\bar{y}_e^{tu}\mathcal{C}_{qe}^{srrv}(\Omega_{\ell,j}^*\overset{\leftrightarrow}{D}_{\bar{\mu}}\Omega_\ell^i)H_i^\dagger H^j(\bar{q}_s\gamma^{\bar{\mu}}q_r) \\
& -\frac{i}{6}y_u^{vu}\bar{y}_u^{tu}\mathcal{C}_{qe}^{tvsr}(\Omega_u^\dagger\overset{\leftrightarrow}{D}_{\bar{\mu}}\Omega_u)(H^\dagger H)(\bar{e}_s\gamma^{\bar{\mu}}e_r) \\
& -\frac{i}{3}g_s\mathcal{C}_{qe}^{ttsr}\left[2T_b^{Aa}(\Omega_{q,a}^*D_{\bar{\sigma}}\Omega_q^b)\tilde{G}^{\bar{\rho}\bar{\sigma}A}(\bar{e}_s\gamma^{\bar{\rho}}e_r)+2T_b^{Aa}(D_{\bar{\mu}}\Omega_{q,a}^*\Omega_q^b)\tilde{G}^{\bar{\mu}\bar{\sigma}A}(\bar{e}_s\gamma^{\bar{\sigma}}e_r)\right] \\
& -\frac{i}{3}g_L\mathcal{C}_{qe}^{ttsr}\left[2t_j^{Li}(\Omega_{q,i}^*D_{\bar{\sigma}}\Omega_q^j)\widetilde{W}^{\bar{\rho}\bar{\sigma}I}(\bar{e}_s\gamma^{\bar{\rho}}e_r)+2t_j^{Li}(D_{\bar{\mu}}\Omega_{q,i}^*\Omega_q^j)\widetilde{W}^{\bar{\mu}\bar{\sigma}I}(\bar{e}_s\gamma^{\bar{\sigma}}e_r)\right] \\
& +\frac{i}{3}\mathcal{C}_{qe}^{ttsr}\left[(\Omega_q^\dagger D_{\bar{\nu}}\Omega_q)(D^{\bar{\mu}}\bar{e}_s\gamma^{\bar{\nu}}D^{\bar{\mu}}e_r)-(D_{\bar{\mu}}\Omega_q^\dagger\Omega_q)(D^{\bar{\nu}}\bar{e}_s\gamma^{\bar{\mu}}D^{\bar{\nu}}e_r)\right] \\
& +\frac{i}{3}\mathcal{C}_{qe}^{ttsr}\left[(\Omega_q^\dagger D_{\bar{\nu}}\Omega_q)(D^{\bar{\mu}}D^{\bar{\mu}}\bar{e}_s\gamma^{\bar{\nu}}e_r)-(D_{\bar{\mu}}\Omega_q^\dagger\Omega_q)(\bar{e}_s\gamma^{\bar{\mu}}D^{\bar{\nu}}D^{\bar{\nu}}e_r)\right] \\
& -\frac{i}{3}g_Y\mathcal{C}_{qe}^{srtt}\left[2(\Omega_e^\dagger D_{\bar{\sigma}}\Omega_e)\tilde{B}^{\bar{\rho}\bar{\sigma}}(\bar{q}_s\gamma^{\bar{\rho}}q_r)+2(D_{\bar{\mu}}\Omega_e^\dagger\Omega_e)\tilde{B}^{\bar{\mu}\bar{\sigma}}(\bar{q}_s\gamma^{\bar{\sigma}}q_r)\right] \\
& +\frac{i}{3}\mathcal{C}_{qe}^{srtt}\left[(\Omega_e^\dagger D_{\bar{\nu}}\Omega_e)(D^{\bar{\mu}}\bar{q}_s\gamma^{\bar{\nu}}D^{\bar{\mu}}q_r)-(D_{\bar{\mu}}\Omega_e^\dagger\Omega_e)(D^{\bar{\nu}}\bar{q}_s\gamma^{\bar{\mu}}D^{\bar{\nu}}q_r)\right] \\
& +\frac{i}{3}\mathcal{C}_{qe}^{srtt}\left[(\Omega_e^\dagger D_{\bar{\nu}}\Omega_e)(D^{\bar{\mu}}D^{\bar{\mu}}\bar{q}_s\gamma^{\bar{\nu}}q_r)-(D_{\bar{\mu}}\Omega_e^\dagger\Omega_e)(\bar{q}_s\gamma^{\bar{\mu}}D^{\bar{\nu}}D^{\bar{\nu}}q_r)\right] \\
& +\frac{2i}{3}y_e^{tv}\bar{y}_e^{tu}\mathcal{C}_{qe}^{srrv}(\Omega_e^\dagger\overset{\leftrightarrow}{D}_{\bar{\mu}}\Omega_e)(H^\dagger H)(\bar{q}_s\gamma^{\bar{\mu}}q_r)+\frac{2i}{3}y_u^{vu}\bar{y}_u^{tu}\mathcal{C}_{qe}^{tvsr}(\Omega_q^\dagger\overset{\leftrightarrow}{D}_{\bar{\mu}}\Omega_q)(H^\dagger H)(\bar{e}_s\gamma^{\bar{\mu}}e_r) \\
& +\frac{2i}{3}\mathcal{C}_{qe}^{tvsr}\left[y_d^{vu}\bar{y}_d^{tu}-y_u^{vu}\bar{y}_u^{tu}\right](\Omega_{q,j}^*\overset{\leftrightarrow}{D}_{\bar{\mu}}\Omega_q^i)H_i^\dagger H^j(\bar{e}_s\gamma^{\bar{\mu}}e_r), \tag{3.47}
\end{aligned}$$

$$\begin{aligned}
\Gamma_{\Omega}^{(1)} [\mathcal{O}_{\ell u}] = & \frac{i}{6} \mathcal{C}_{\ell u}^{srtt} \left[ (\Omega_u^\dagger D_2 D_{\bar{\mu}} \Omega_u) (\bar{\ell}_s \gamma^{\bar{\mu}} \ell_r) - (D_2 D_{\bar{\nu}} \Omega_u^\dagger \Omega_u) (\bar{\ell}_s \gamma^{\bar{\nu}} \ell_r) \right] \\
& + \frac{1}{6} \mathcal{C}_{\ell u}^{ttsr} \left[ (D_{\bar{\mu}} \Omega_{\ell, i}^* D_{\bar{\rho}} \Omega_{\ell}^j) (\Omega_{\ell, j}^* D_{\bar{\sigma}} \Omega_{\ell}^i) \varepsilon^{\bar{\mu}\bar{\nu}\bar{\rho}\bar{\sigma}} (\bar{u}_s \gamma^{\bar{\nu}} u_r) - (D_{\bar{\mu}} \Omega_{\ell, i}^* \Omega_{\ell}^j) (D_{\bar{\nu}} \Omega_{\ell, j}^* D_{\bar{\rho}} \Omega_{\ell}^i) \varepsilon^{\bar{\mu}\bar{\nu}\bar{\rho}\bar{\sigma}} (\bar{u}_s \gamma^{\bar{\sigma}} u_r) \right] \\
& - \frac{1}{6} \mathcal{C}_{\ell u}^{srtt} \left[ (D_{\bar{\mu}} \Omega_{u, a}^* D_{\bar{\rho}} \Omega_u^b) (\Omega_{u, b}^* D_{\bar{\sigma}} \Omega_u^a) \varepsilon^{\bar{\mu}\bar{\nu}\bar{\rho}\bar{\sigma}} (\bar{\ell}_s \gamma^{\bar{\nu}} \ell_r) - (D_{\bar{\mu}} \Omega_{u, a}^* \Omega_u^b) (D_{\bar{\nu}} \Omega_{u, b}^* D_{\bar{\rho}} \Omega_u^a) \varepsilon^{\bar{\mu}\bar{\nu}\bar{\rho}\bar{\sigma}} (\bar{\ell}_s \gamma^{\bar{\sigma}} \ell_r) \right] \\
& + \frac{i}{6} \mathcal{C}_{\ell u}^{ttsr} \left[ (\Omega_{\ell}^\dagger D_2 D_{\bar{\mu}} \Omega_{\ell}) (\bar{u}_s \gamma^{\bar{\mu}} u_r) - (D_2 D_{\bar{\nu}} \Omega_{\ell}^\dagger \Omega_{\ell}) (\bar{u}_s \gamma^{\bar{\nu}} u_r) \right] \\
& + \frac{i}{6} g_Y \mathcal{C}_{\ell u}^{ttsr} \left[ 2(\Omega_{\ell}^\dagger D_{\bar{\sigma}} \Omega_{\ell}) \tilde{B}^{\bar{\rho}\bar{\sigma}} (\bar{u}_s \gamma^{\bar{\rho}} u_r) + 2(D_{\bar{\mu}} \Omega_{\ell}^\dagger \Omega_{\ell}) \tilde{B}^{\bar{\mu}\bar{\sigma}} (\bar{u}_s \gamma^{\bar{\sigma}} u_r) \right] \\
& - \frac{i}{6} y_e^{vu} \bar{y}_e^{tu} \mathcal{C}_{\ell u}^{tvsr} (\Omega_e^\dagger \overleftrightarrow{D}_{\bar{\mu}} \Omega_e) (H^\dagger H) (\bar{u}_s \gamma^{\bar{\mu}} u_r) - \frac{i}{6} y_u^{tv} \bar{y}_u^{tu} \mathcal{C}_{\ell u}^{srvu} (\Omega_q^\dagger \overleftrightarrow{D}_{\bar{\mu}} \Omega_q) (H^\dagger H) (\bar{\ell}_s \gamma^{\bar{\mu}} \ell_r) \\
& + \frac{i}{6} y_u^{tv} \bar{y}_u^{tu} \mathcal{C}_{\ell u}^{srvu} (\Omega_{q, j}^* \overleftrightarrow{D}_{\bar{\mu}} \Omega_q^i) H_i^\dagger H^j (\bar{\ell}_s \gamma^{\bar{\mu}} \ell_r) \\
& + \frac{2i}{9} g_Y \mathcal{C}_{\ell u}^{srtt} \left[ 2(\Omega_u^\dagger D_{\bar{\sigma}} \Omega_u) \tilde{B}^{\bar{\rho}\bar{\sigma}} (\bar{\ell}_s \gamma^{\bar{\rho}} \ell_r) + 2(D_{\bar{\mu}} \Omega_u^\dagger \Omega_u) \tilde{B}^{\bar{\mu}\bar{\sigma}} (\bar{\ell}_s \gamma^{\bar{\sigma}} \ell_r) \right] \\
& + \frac{i}{3} g_s \mathcal{C}_{\ell u}^{srtt} \left[ 2T_b^{Aa} (\Omega_{u, a}^* D_{\bar{\sigma}} \Omega_u^b) \tilde{G}^{\bar{\rho}\bar{\sigma} A} (\bar{\ell}_s \gamma^{\bar{\rho}} \ell_r) + 2T_b^{Aa} (D_{\bar{\mu}} \Omega_{u, a}^* \Omega_u^b) \tilde{G}^{\bar{\mu}\bar{\sigma} A} (\bar{\ell}_s \gamma^{\bar{\sigma}} \ell_r) \right] \\
& + \frac{i}{3} \mathcal{C}_{\ell u}^{srtt} \left[ (\Omega_u^\dagger D_{\bar{\nu}} \Omega_u) (D^{\bar{\mu}} \bar{\ell}_s \gamma^{\bar{\nu}} D^{\bar{\mu}} \ell_r) - (D_{\bar{\mu}} \Omega_u^\dagger \Omega_u) (D^{\bar{\nu}} \bar{\ell}_s \gamma^{\bar{\mu}} D^{\bar{\nu}} \ell_r) \right] \\
& + \frac{i}{3} \mathcal{C}_{\ell u}^{srtt} \left[ (\Omega_u^\dagger D_{\bar{\nu}} \Omega_u) (D^{\bar{\mu}} D^{\bar{\mu}} \bar{\ell}_s \gamma^{\bar{\nu}} \ell_r) - (D_{\bar{\mu}} \Omega_u^\dagger \Omega_u) (\bar{\ell}_s \gamma^{\bar{\mu}} D^{\bar{\nu}} D^{\bar{\nu}} \ell_r) \right] \\
& - \frac{i}{3} g_L \mathcal{C}_{\ell u}^{ttsr} \left[ 2t_j^{Ii} (\Omega_{\ell, i}^* D_{\bar{\sigma}} \Omega_{\ell}^j) \widetilde{W}^{\bar{\rho}\bar{\sigma} I} (\bar{u}_s \gamma^{\bar{\rho}} u_r) + 2t_j^{Ii} (D_{\bar{\mu}} \Omega_{\ell, i}^* \Omega_{\ell}^j) \widetilde{W}^{\bar{\mu}\bar{\sigma} I} (\bar{u}_s \gamma^{\bar{\sigma}} u_r) \right] \\
& + \frac{i}{3} \mathcal{C}_{\ell u}^{ttsr} \left[ (\Omega_{\ell}^\dagger D_{\bar{\nu}} \Omega_{\ell}) (D^{\bar{\mu}} \bar{u}_s \gamma^{\bar{\nu}} D^{\bar{\mu}} u_r) - (D_{\bar{\mu}} \Omega_{\ell}^\dagger \Omega_{\ell}) (D^{\bar{\nu}} \bar{u}_s \gamma^{\bar{\mu}} D^{\bar{\nu}} u_r) \right] \\
& + \frac{i}{3} \mathcal{C}_{\ell u}^{ttsr} \left[ (\Omega_{\ell}^\dagger D_{\bar{\nu}} \Omega_{\ell}) (D^{\bar{\mu}} D^{\bar{\mu}} \bar{u}_s \gamma^{\bar{\nu}} u_r) - (D_{\bar{\mu}} \Omega_{\ell}^\dagger \Omega_{\ell}) (\bar{u}_s \gamma^{\bar{\mu}} D^{\bar{\nu}} D^{\bar{\nu}} u_r) \right] \\
& + \frac{2i}{3} y_e^{vu} \bar{y}_e^{tu} \mathcal{C}_{\ell u}^{tvsr} (\Omega_{\ell, j}^* \overleftrightarrow{D}_{\bar{\mu}} \Omega_{\ell}^i) H_i^\dagger H^j (\bar{u}_s \gamma^{\bar{\mu}} u_r) + \frac{2i}{3} y_u^{tv} \bar{y}_u^{tu} \mathcal{C}_{\ell u}^{srvu} (\Omega_u^\dagger \overleftrightarrow{D}_{\bar{\mu}} \Omega_u) (H^\dagger H) (\bar{\ell}_s \gamma^{\bar{\mu}} \ell_r), \quad (3.48)
\end{aligned}$$

$$\begin{aligned}
\Gamma_{\Omega}^{(1)} [\mathcal{O}_{\ell d}] = & -\frac{i}{9} g_Y \mathcal{C}_{\ell d}^{srtt} \left[ 2(\Omega_d^\dagger D_{\bar{\sigma}} \Omega_d) \tilde{B}^{\bar{\rho}\bar{\sigma}} (\bar{\ell}_s \gamma^{\bar{\rho}} \ell_r) + 2(D_{\bar{\mu}} \Omega_d^\dagger \Omega_d) \tilde{B}^{\bar{\mu}\bar{\sigma}} (\bar{\ell}_s \gamma^{\bar{\sigma}} \ell_r) \right] \\
& + \frac{i}{6} \mathcal{C}_{\ell d}^{ttsr} \left[ (\Omega_{\ell}^\dagger D_2 D_{\bar{\mu}} \Omega_{\ell}) (\bar{d}_s \gamma^{\bar{\mu}} d_r) - (D_2 D_{\bar{\nu}} \Omega_{\ell}^\dagger \Omega_{\ell}) (\bar{d}_s \gamma^{\bar{\nu}} d_r) \right] \\
& + \frac{i}{6} g_Y \mathcal{C}_{\ell d}^{ttsr} \left[ 2(\Omega_{\ell}^\dagger D_{\bar{\sigma}} \Omega_{\ell}) \tilde{B}^{\bar{\rho}\bar{\sigma}} (\bar{d}_s \gamma^{\bar{\rho}} d_r) + 2(D_{\bar{\mu}} \Omega_{\ell}^\dagger \Omega_{\ell}) \tilde{B}^{\bar{\mu}\bar{\sigma}} (\bar{d}_s \gamma^{\bar{\sigma}} d_r) \right] \\
& + \frac{1}{6} \mathcal{C}_{\ell d}^{ttsr} \left[ (D_{\bar{\mu}} \Omega_{\ell, i}^* D_{\bar{\rho}} \Omega_{\ell}^j) (\Omega_{\ell, j}^* D_{\bar{\sigma}} \Omega_{\ell}^i) \varepsilon^{\bar{\mu}\bar{\nu}\bar{\rho}\bar{\sigma}} (\bar{d}_s \gamma^{\bar{\nu}} d_r) - (D_{\bar{\mu}} \Omega_{\ell, i}^* \Omega_{\ell}^j) (D_{\bar{\nu}} \Omega_{\ell, j}^* D_{\bar{\rho}} \Omega_{\ell}^i) \varepsilon^{\bar{\mu}\bar{\nu}\bar{\rho}\bar{\sigma}} (\bar{d}_s \gamma^{\bar{\sigma}} d_r) \right] \\
& + \frac{i}{6} \mathcal{C}_{\ell d}^{srtt} \left[ (\Omega_d^\dagger D_2 D_{\bar{\mu}} \Omega_d) (\bar{\ell}_s \gamma^{\bar{\mu}} \ell_r) - (D_2 D_{\bar{\nu}} \Omega_d^\dagger \Omega_d) (\bar{\ell}_s \gamma^{\bar{\nu}} \ell_r) \right] \\
& - \frac{1}{6} \mathcal{C}_{\ell d}^{srtt} \left[ (D_{\bar{\mu}} \Omega_{d, a}^* D_{\bar{\rho}} \Omega_d^b) (\Omega_{d, b}^* D_{\bar{\sigma}} \Omega_d^a) \varepsilon^{\bar{\mu}\bar{\nu}\bar{\rho}\bar{\sigma}} (\bar{\ell}_s \gamma^{\bar{\nu}} \ell_r) - (D_{\bar{\mu}} \Omega_{d, a}^* \Omega_d^b) (D_{\bar{\nu}} \Omega_{d, b}^* D_{\bar{\rho}} \Omega_d^a) \varepsilon^{\bar{\mu}\bar{\nu}\bar{\rho}\bar{\sigma}} (\bar{\ell}_s \gamma^{\bar{\sigma}} \ell_r) \right] \\
& - \frac{i}{6} y_e^{vu} \bar{y}_e^{tu} \mathcal{C}_{\ell d}^{tvsr} (\Omega_e^\dagger \overleftrightarrow{D}_{\bar{\mu}} \Omega_e) (H^\dagger H) (\bar{d}_s \gamma^{\bar{\mu}} d_r) - \frac{i}{6} y_d^{tv} \bar{y}_d^{tu} \mathcal{C}_{\ell d}^{srvu} (\Omega_{q, j}^* \overleftrightarrow{D}_{\bar{\mu}} \Omega_q^i) H_i^\dagger H^j (\bar{\ell}_s \gamma^{\bar{\mu}} \ell_r) \\
& - \frac{i}{3} g_L \mathcal{C}_{\ell d}^{ttsr} \left[ 2t_j^{Ii} (\Omega_{\ell, i}^* D_{\bar{\sigma}} \Omega_{\ell}^j) \widetilde{W}^{\bar{\rho}\bar{\sigma} I} (\bar{d}_s \gamma^{\bar{\rho}} d_r) + 2t_j^{Ii} (D_{\bar{\mu}} \Omega_{\ell, i}^* \Omega_{\ell}^j) \widetilde{W}^{\bar{\mu}\bar{\sigma} I} (\bar{d}_s \gamma^{\bar{\sigma}} d_r) \right]
\end{aligned}$$

$$\begin{aligned}
& + \frac{i}{3} \mathcal{C}_{\ell d}^{ttsr} \left[ (\Omega_\ell^\dagger D_{\bar{\nu}} \Omega_\ell) (D^{\bar{\mu}} \bar{d}_s \gamma^{\bar{\nu}} D^{\bar{\mu}} d_r) - (D_{\bar{\mu}} \Omega_\ell^\dagger \Omega_\ell) (D^{\bar{\nu}} \bar{d}_s \gamma^{\bar{\mu}} D^{\bar{\nu}} d_r) \right] \\
& + \frac{i}{3} \mathcal{C}_{\ell d}^{ttsr} \left[ (\Omega_\ell^\dagger D_{\bar{\nu}} \Omega_\ell) (D^{\bar{\mu}} D^{\bar{\mu}} \bar{d}_s \gamma^{\bar{\nu}} d_r) - (D_{\bar{\mu}} \Omega_\ell^\dagger \Omega_\ell) (\bar{d}_s \gamma^{\bar{\mu}} D^{\bar{\nu}} D^{\bar{\nu}} d_r) \right] \\
& + \frac{i}{3} g_s \mathcal{C}_{\ell d}^{srtt} \left[ 2T_b^{Aa} (\Omega_{d,a}^* D_{\bar{\sigma}} \Omega_d^b) \tilde{G}^{\bar{\rho}\bar{\sigma}A} (\bar{\ell}_s \gamma^{\bar{\rho}} \ell_r) + 2T_b^{Aa} (D_{\bar{\mu}} \Omega_{d,a}^* \Omega_d^b) \tilde{G}^{\bar{\mu}\bar{\sigma}A} (\bar{\ell}_s \gamma^{\bar{\sigma}} \ell_r) \right] \\
& + \frac{i}{3} \mathcal{C}_{\ell d}^{srtt} \left[ (\Omega_d^\dagger D_{\bar{\nu}} \Omega_d) (D^{\bar{\mu}} \bar{\ell}_s \gamma^{\bar{\nu}} D^{\bar{\mu}} \ell_r) - (D_{\bar{\mu}} \Omega_d^\dagger \Omega_d) (D^{\bar{\nu}} \bar{\ell}_s \gamma^{\bar{\mu}} D^{\bar{\nu}} \ell_r) \right] \\
& + \frac{i}{3} \mathcal{C}_{\ell d}^{srtt} \left[ (\Omega_d^\dagger D_{\bar{\nu}} \Omega_d) (D^{\bar{\mu}} D^{\bar{\mu}} \bar{\ell}_s \gamma^{\bar{\nu}} \ell_r) - (D_{\bar{\mu}} \Omega_d^\dagger \Omega_d) (\bar{\ell}_s \gamma^{\bar{\mu}} D^{\bar{\nu}} D^{\bar{\nu}} \ell_r) \right] \\
& + \frac{2i}{3} y_d^{tv} \bar{y}_d^{tu} \mathcal{C}_{\ell d}^{srtv} (\Omega_d^\dagger \bar{D}_{\bar{\mu}} \Omega_d) (H^\dagger H) (\bar{\ell}_s \gamma^{\bar{\mu}} \ell_r) + \frac{2i}{3} y_e^{vu} \bar{y}_e^{tu} \mathcal{C}_{\ell d}^{tvsr} (\Omega_{\ell,j}^* \bar{D}_{\bar{\mu}} \Omega_\ell^i) H_i^\dagger H^j (\bar{d}_s \gamma^{\bar{\mu}} d_r), \quad (3.49)
\end{aligned}$$

$$\begin{aligned}
\Gamma_\Omega^{(1)} [\mathcal{O}_{\ell q}^{(1)}] = & -\frac{i}{36} g_Y (\mathcal{C}_{\ell q}^{(1)})^{srtt} \left[ 2(\Omega_{q,i}^* D_{\bar{\sigma}} \Omega_q^j) \tilde{B}^{\bar{\rho}\bar{\sigma}} (\bar{\ell}_{js} \gamma^{\bar{\rho}} \ell_r^i) + 2(D_{\bar{\mu}} \Omega_{q,i}^* \Omega_q^j) \tilde{B}^{\bar{\mu}\bar{\sigma}} (\bar{\ell}_{js} \gamma^{\bar{\sigma}} \ell_r^i) \right] \\
& - \frac{i}{24} g_Y (\mathcal{C}_{\ell q}^{(1)})^{srtt} \left[ 2(\Omega_q^\dagger D_{\bar{\sigma}} \Omega_q) \tilde{B}^{\bar{\rho}\bar{\sigma}} (\bar{\ell}_s \gamma^{\bar{\rho}} \ell_r) + 2(D_{\bar{\mu}} \Omega_q^\dagger \Omega_q) \tilde{B}^{\bar{\mu}\bar{\sigma}} (\bar{\ell}_s \gamma^{\bar{\sigma}} \ell_r) \right] \\
& + \frac{i}{12} g_Y (\mathcal{C}_{\ell q}^{(1)})^{ttsr} \left[ 2(\Omega_{\ell,i}^* D_{\bar{\sigma}} \Omega_\ell^j) \tilde{B}^{\bar{\rho}\bar{\sigma}} (\bar{q}_{js} \gamma^{\bar{\rho}} q_r^i) + 2(D_{\bar{\mu}} \Omega_{\ell,i}^* \Omega_\ell^j) \tilde{B}^{\bar{\mu}\bar{\sigma}} (\bar{q}_{js} \gamma^{\bar{\sigma}} q_r^i) \right] \\
& + \frac{i}{8} g_Y (\mathcal{C}_{\ell q}^{(1)})^{ttsr} \left[ 2(\Omega_\ell^\dagger D_{\bar{\sigma}} \Omega_\ell) \tilde{B}^{\bar{\rho}\bar{\sigma}} (\bar{q}_s \gamma^{\bar{\rho}} q_r) + 2(D_{\bar{\mu}} \Omega_\ell^\dagger \Omega_\ell) \tilde{B}^{\bar{\mu}\bar{\sigma}} (\bar{q}_s \gamma^{\bar{\sigma}} q_r) \right] \\
& + \frac{i}{6} (\mathcal{C}_{\ell q}^{(1)})^{srtt} \left[ (\Omega_q^\dagger D_2 D_{\bar{\mu}} \Omega_q) (\bar{\ell}_s \gamma^{\bar{\mu}} \ell_r) - (D_2 D_{\bar{\nu}} \Omega_q^\dagger \Omega_q) (\bar{\ell}_s \gamma^{\bar{\nu}} \ell_r) \right] \\
& + \frac{1}{6} (\mathcal{C}_{\ell q}^{(1)})^{srtt} \left[ (D_{\bar{\mu}} \Omega_{q,a}^* D_{\bar{\rho}} \Omega_q^b) (\Omega_{q,b}^* D_{\bar{\sigma}} \Omega_q^a) \varepsilon^{\bar{\mu}\bar{\nu}\bar{\rho}\bar{\sigma}} (\bar{\ell}_s \gamma^{\bar{\nu}} \ell_r) - (D_{\bar{\mu}} \Omega_{q,a}^* \Omega_q^b) (D_{\bar{\nu}} \Omega_{q,b}^* D_{\bar{\rho}} \Omega_q^a) \varepsilon^{\bar{\mu}\bar{\nu}\bar{\rho}\bar{\sigma}} (\bar{\ell}_s \gamma^{\bar{\sigma}} \ell_r) \right] \\
& - \frac{i}{6} g_s (\mathcal{C}_{\ell q}^{(1)})^{srtt} \left[ 2T_b^{Aa} (\Omega_{q,ai}^* D_{\bar{\sigma}} \Omega_q^{bj}) \tilde{G}^{\bar{\rho}\bar{\sigma}A} (\bar{\ell}_{js} \gamma^{\bar{\rho}} \ell_r^i) + 2T_b^{Aa} (D_{\bar{\mu}} \Omega_{q,ai}^* \Omega_q^{bj}) \tilde{G}^{\bar{\mu}\bar{\sigma}A} (\bar{\ell}_{js} \gamma^{\bar{\sigma}} \ell_r^i) \right] \\
& + \frac{i}{6} (\mathcal{C}_{\ell q}^{(1)})^{ttsr} \left[ (\Omega_\ell^\dagger D_2 D_{\bar{\mu}} \Omega_\ell) (\bar{q}_s \gamma^{\bar{\mu}} q_r) - (D_2 D_{\bar{\nu}} \Omega_\ell^\dagger \Omega_\ell) (\bar{q}_s \gamma^{\bar{\nu}} q_r) \right] \\
& + \frac{1}{6} (\mathcal{C}_{\ell q}^{(1)})^{ttsr} \left[ (\Omega_\ell^\dagger D_{\bar{\sigma}} \Omega_\ell) (D_{\bar{\mu}} \Omega_\ell^\dagger D_{\bar{\rho}} \Omega_\ell) \varepsilon^{\bar{\mu}\bar{\nu}\bar{\rho}\bar{\sigma}} (\bar{q}_s \gamma^{\bar{\nu}} q_r) - (D_{\bar{\mu}} \Omega_\ell^\dagger \Omega_\ell) (D_{\bar{\nu}} \Omega_\ell^\dagger D_{\bar{\rho}} \Omega_\ell) \varepsilon^{\bar{\mu}\bar{\nu}\bar{\rho}\bar{\sigma}} (\bar{q}_s \gamma^{\bar{\sigma}} q_r) \right] \\
& - \frac{i}{6} y_d^{vu} \bar{y}_d^{tu} (\mathcal{C}_{\ell q}^{(1)})^{srtv} (\Omega_d^\dagger \bar{D}_{\bar{\mu}} \Omega_d) (H^\dagger H) (\bar{\ell}_s \gamma^{\bar{\mu}} \ell_r) - \frac{i}{6} y_e^{vu} \bar{y}_e^{tu} (\mathcal{C}_{\ell q}^{(1)})^{tvsr} (\Omega_\ell^\dagger \bar{D}_{\bar{\mu}} \Omega_\ell) (H^\dagger H) (\bar{q}_s \gamma^{\bar{\mu}} q_r) \\
& - \frac{i}{6} y_u^{vu} \bar{y}_u^{tu} (\mathcal{C}_{\ell q}^{(1)})^{srtv} (\Omega_u^\dagger \bar{D}_{\bar{\mu}} \Omega_u) (H^\dagger H) (\bar{\ell}_s \gamma^{\bar{\mu}} \ell_r) \\
& - \frac{i}{4} g_s (\mathcal{C}_{\ell q}^{(1)})^{srtt} \left[ 2T_b^{Aa} (\Omega_{q,a}^* D_{\bar{\sigma}} \Omega_q^b) \tilde{G}^{\bar{\rho}\bar{\sigma}A} (\bar{\ell}_s \gamma^{\bar{\rho}} \ell_r) + 2T_b^{Aa} (D_{\bar{\mu}} \Omega_{q,a}^* \Omega_q^b) \tilde{G}^{\bar{\mu}\bar{\sigma}A} (\bar{\ell}_s \gamma^{\bar{\sigma}} \ell_r) \right] \\
& + \frac{i}{3} (\mathcal{C}_{\ell q}^{(1)})^{srtt} \left[ (\Omega_q^\dagger D_{\bar{\nu}} \Omega_q) (D^{\bar{\mu}} \bar{\ell}_s \gamma^{\bar{\nu}} D^{\bar{\mu}} \ell_r) - (D_{\bar{\mu}} \Omega_q^\dagger \Omega_q) (D^{\bar{\nu}} \bar{\ell}_s \gamma^{\bar{\mu}} D^{\bar{\nu}} \ell_r) \right] \\
& + \frac{i}{3} (\mathcal{C}_{\ell q}^{(1)})^{srtt} \left[ (\Omega_q^\dagger D_{\bar{\nu}} \Omega_q) (D^{\bar{\mu}} D^{\bar{\mu}} \bar{\ell}_s \gamma^{\bar{\nu}} \ell_r) - (D_{\bar{\mu}} \Omega_q^\dagger \Omega_q) (\bar{\ell}_s \gamma^{\bar{\mu}} D^{\bar{\nu}} D^{\bar{\nu}} \ell_r) \right] \\
& + \frac{1}{3} (\mathcal{C}_{\ell q}^{(1)})^{srtt} \left[ (D_{\bar{\mu}} \Omega_{q,ai}^* D_{\bar{\rho}} \Omega_q^{bk}) (\Omega_{q,bj}^* D_{\bar{\sigma}} \Omega_q^{ai}) \varepsilon^{\bar{\mu}\bar{\nu}\bar{\rho}\bar{\sigma}} (\bar{\ell}_{ks} \gamma^{\bar{\nu}} \ell_r^j) - (D_{\bar{\mu}} \Omega_{q,ai}^* \Omega_q^{bk}) (D_{\bar{\nu}} \Omega_{q,bj}^* D_{\bar{\rho}} \Omega_q^{ai}) \varepsilon^{\bar{\mu}\bar{\nu}\bar{\rho}\bar{\sigma}} (\bar{\ell}_{ks} \gamma^{\bar{\sigma}} \ell_r^j) \right] \\
& + \frac{1}{3} (\mathcal{C}_{\ell q}^{(1)})^{srtt} \left[ (D_{\bar{\mu}} \Omega_{q,a}^* \Omega_q^b) (D_{\bar{\nu}} \Omega_{q,bj}^* \Omega_q^{ak}) \varepsilon^{\bar{\mu}\bar{\nu}\bar{\rho}\bar{\sigma}} (\bar{\ell}_{ks} \gamma^{\bar{\rho}} D^{\bar{\sigma}} \ell_r^j) + (\Omega_{q,b}^* D_{\bar{\sigma}} \Omega_q^a) (\Omega_{q,ai}^* D_{\bar{\nu}} \Omega_q^{bk}) \varepsilon^{\bar{\mu}\bar{\nu}\bar{\rho}\bar{\sigma}} (D^{\bar{\rho}} \bar{\ell}_{ks} \gamma^{\bar{\mu}} \ell_r^i) \right] \\
& - \frac{1}{3} (\mathcal{C}_{\ell q}^{(1)})^{srtt} \left[ (D_{\bar{\mu}} \Omega_{q,a}^* D_{\bar{\rho}} \Omega_q^b) (\Omega_{q,bj}^* D_{\bar{\sigma}} \Omega_q^{ak}) \varepsilon^{\bar{\mu}\bar{\nu}\bar{\rho}\bar{\sigma}} (\bar{\ell}_{ks} \gamma^{\bar{\nu}} \ell_r^j) - (D_{\bar{\nu}} \Omega_{q,b}^* D_{\bar{\rho}} \Omega_q^a) (D_{\bar{\mu}} \Omega_{q,ai}^* \Omega_q^{bk}) \varepsilon^{\bar{\mu}\bar{\nu}\bar{\rho}\bar{\sigma}} (\bar{\ell}_{ks} \gamma^{\bar{\sigma}} \ell_r^i) \right]
\end{aligned}$$

$$\begin{aligned}
& + \frac{i}{3}(\mathcal{C}_{\ell q}^{(1)})^{ttsr} \left[ (\Omega_\ell^\dagger D_{\bar{\nu}} \Omega_\ell) (D^{\bar{\mu}} \bar{q}_s \gamma^{\bar{\nu}} D^{\bar{\mu}} q_r) - (D_{\bar{\mu}} \Omega_\ell^\dagger \Omega_\ell) (D^{\bar{\nu}} \bar{q}_s \gamma^{\bar{\mu}} D^{\bar{\nu}} q_r) \right] \\
& + \frac{i}{3}(\mathcal{C}_{\ell q}^{(1)})^{ttsr} \left[ (\Omega_\ell^\dagger D_{\bar{\nu}} \Omega_\ell) (D^{\bar{\mu}} D^{\bar{\mu}} \bar{q}_s \gamma^{\bar{\nu}} q_r) - (D_{\bar{\mu}} \Omega_\ell^\dagger \Omega_\ell) (\bar{q}_s \gamma^{\bar{\mu}} D^{\bar{\nu}} D^{\bar{\nu}} q_r) \right] \\
& + \frac{1}{3}(\mathcal{C}_{\ell q}^{(1)})^{ttsr} \left[ (D_{\bar{\mu}} \Omega_{\ell,i}^* D_{\bar{\rho}} \Omega_\ell^k) (\Omega_{\ell,j}^* D_{\bar{\sigma}} \Omega_\ell^i) \varepsilon^{\bar{\mu}\bar{\nu}\bar{\rho}\bar{\sigma}} (\bar{q}_{ks} \gamma^{\bar{\nu}} q_r^j) - (D_{\bar{\mu}} \Omega_{\ell,i}^* \Omega_\ell^k) (D_{\bar{\nu}} \Omega_{\ell,j}^* D_{\bar{\rho}} \Omega_\ell^i) \varepsilon^{\bar{\mu}\bar{\nu}\bar{\rho}\bar{\sigma}} (\bar{q}_{ks} \gamma^{\bar{\sigma}} q_r^j) \right] \\
& + \frac{1}{3}(\mathcal{C}_{\ell q}^{(1)})^{ttsr} \left[ (D_{\bar{\mu}} \Omega_\ell^\dagger \Omega_\ell) (D_{\bar{\nu}} \Omega_{\ell,j}^* \Omega_\ell^k) \varepsilon^{\bar{\mu}\bar{\nu}\bar{\rho}\bar{\sigma}} (\bar{q}_{ks} \gamma^{\bar{\rho}} D^{\bar{\sigma}} q_r^j) + (\Omega_\ell^\dagger D_{\bar{\sigma}} \Omega_\ell) (\Omega_{\ell,j}^* D_{\bar{\nu}} \Omega_\ell^k) \varepsilon^{\bar{\mu}\bar{\nu}\bar{\rho}\bar{\sigma}} (D^{\bar{\rho}} \bar{q}_{ks} \gamma^{\bar{\mu}} q_r^j) \right] \\
& - \frac{1}{3}(\mathcal{C}_{\ell q}^{(1)})^{ttsr} \left[ (D_{\bar{\mu}} \Omega_\ell^\dagger D_{\bar{\rho}} \Omega_\ell) (\Omega_{\ell,j}^* D_{\bar{\sigma}} \Omega_\ell^k) \varepsilon^{\bar{\mu}\bar{\nu}\bar{\rho}\bar{\sigma}} (\bar{q}_{ks} \gamma^{\bar{\nu}} q_r^j) + (D_{\bar{\mu}} \Omega_\ell^\dagger D_{\bar{\rho}} \Omega_\ell) (D_{\bar{\nu}} \Omega_{\ell,j}^* \Omega_\ell^k) \varepsilon^{\bar{\mu}\bar{\nu}\bar{\rho}\bar{\sigma}} (\bar{q}_{ks} \gamma^{\bar{\sigma}} q_r^j) \right] \\
& + \frac{5i}{12} g_L (\mathcal{C}_{\ell q}^{(1)})^{srtt} \left[ 2(\Omega_q^\dagger D_{\bar{\sigma}} \Omega_q) \widetilde{W}^{\bar{\rho}\bar{\sigma}} I (\bar{\ell}_s t^I \gamma^{\bar{\rho}} \ell_r) + 2(D_{\bar{\mu}} \Omega_q^\dagger \Omega_q) \widetilde{W}^{\bar{\mu}\bar{\sigma}} I (\bar{\ell}_s t^I \gamma^{\bar{\sigma}} \ell_r) \right] \\
& + \frac{5i}{12} g_L (\mathcal{C}_{\ell q}^{(1)})^{ttsr} \left[ 2(\Omega_\ell^\dagger D_{\bar{\sigma}} \Omega_\ell) \widetilde{W}^{\bar{\rho}\bar{\sigma}} I (\bar{q}_s t^I \gamma^{\bar{\rho}} q_r) + 2(D_{\bar{\mu}} \Omega_\ell^\dagger \Omega_\ell) \widetilde{W}^{\bar{\mu}\bar{\sigma}} I (\bar{q}_s t^I \gamma^{\bar{\sigma}} q_r) \right] \\
& - \frac{2i}{3} g_L (\mathcal{C}_{\ell q}^{(1)})^{srtt} \left[ 2t_k^{Ij} (D_{\bar{\mu}} \Omega_{q,i}^* \Omega_q^k) \widetilde{W}^{\bar{\mu}\bar{\sigma}} I (\bar{\ell}_{js} \gamma^{\bar{\sigma}} \ell_r^i) + 2t_j^{Ii} (\Omega_{q,i}^* D_{\bar{\sigma}} \Omega_q^k) \widetilde{W}^{\bar{\rho}\bar{\sigma}} I (\bar{\ell}_{ks} \gamma^{\bar{\rho}} \ell_r^j) \right] \\
& - \frac{2i}{3} g_L (\mathcal{C}_{\ell q}^{(1)})^{ttsr} \left[ 2t_k^{Ij} (D_{\bar{\mu}} \Omega_{\ell,i}^* \Omega_\ell^k) \widetilde{W}^{\bar{\mu}\bar{\sigma}} I (\bar{q}_{js} \gamma^{\bar{\sigma}} q_r^i) + 2t_j^{Ii} (\Omega_{\ell,i}^* D_{\bar{\sigma}} \Omega_\ell^k) \widetilde{W}^{\bar{\rho}\bar{\sigma}} I (\bar{q}_{ks} \gamma^{\bar{\rho}} q_r^j) \right] \\
& + \frac{2i}{3} y_e^{vu} \bar{y}_e^{tu} (\mathcal{C}_{\ell q}^{(1)})^{tvsr} (\Omega_{\ell,j}^* \overset{\leftrightarrow}{D}_{\bar{\mu}} \Omega_\ell^i) H_i^\dagger H^j (\bar{q}_s \gamma^{\bar{\mu}} q_r) + \frac{2i}{3} y_u^{vu} \bar{y}_u^{tu} (\mathcal{C}_{\ell q}^{(1)})^{srtv} (\Omega_q^\dagger \overset{\leftrightarrow}{D}_{\bar{\mu}} \Omega_q) (H^\dagger H) (\bar{\ell}_s \gamma^{\bar{\mu}} \ell_r) \\
& + \frac{2i}{3} (\mathcal{C}_{\ell q}^{(1)})^{srtv} \left[ y_d^{vu} \bar{y}_d^{tu} - y_u^{vu} \bar{y}_u^{tu} \right] (\Omega_{q,j}^* \overset{\leftrightarrow}{D}_{\bar{\mu}} \Omega_q^i) H_i^\dagger H^j (\bar{\ell}_s \gamma^{\bar{\mu}} \ell_r), \tag{3.50}
\end{aligned}$$

$$\begin{aligned}
\Gamma_\Omega^{(1)} [\mathcal{O}_{\ell q}^{(3)}] &= \frac{i}{24} g_Y (\mathcal{C}_{\ell q}^{(3)})^{srtt} \left[ 2(\Omega_q^\dagger D_{\bar{\sigma}} \Omega_q) \widetilde{B}^{\bar{\rho}\bar{\sigma}} (\bar{\ell}_s \gamma^{\bar{\rho}} \ell_r) + 2(D_{\bar{\mu}} \Omega_q^\dagger \Omega_q) \widetilde{B}^{\bar{\mu}\bar{\sigma}} (\bar{\ell}_s \gamma^{\bar{\sigma}} \ell_r) \right] \\
& - \frac{i}{12} g_Y (\mathcal{C}_{\ell q}^{(3)})^{srtt} \left[ 2(\Omega_{q,i}^* D_{\bar{\sigma}} \Omega_q^j) \widetilde{B}^{\bar{\rho}\bar{\sigma}} (\bar{\ell}_{js} \gamma^{\bar{\rho}} \ell_r^i) + 2(D_{\bar{\mu}} \Omega_{q,i}^* \Omega_q^j) \widetilde{B}^{\bar{\mu}\bar{\sigma}} (\bar{\ell}_{js} \gamma^{\bar{\sigma}} \ell_r^i) \right] \\
& - \frac{i}{8} g_Y (\mathcal{C}_{\ell q}^{(3)})^{ttsr} \left[ 2(\Omega_\ell^\dagger D_{\bar{\sigma}} \Omega_\ell) \widetilde{B}^{\bar{\rho}\bar{\sigma}} (\bar{q}_s \gamma^{\bar{\rho}} q_r) + 2(D_{\bar{\mu}} \Omega_\ell^\dagger \Omega_\ell) \widetilde{B}^{\bar{\mu}\bar{\sigma}} (\bar{q}_s \gamma^{\bar{\sigma}} q_r) \right] \\
& - \frac{i}{6} (\mathcal{C}_{\ell q}^{(3)})^{srtt} \left[ (\Omega_q^\dagger D_2 D_{\bar{\mu}} \Omega_q) (\bar{\ell}_s \gamma^{\bar{\mu}} \ell_r) - (D_2 D_{\bar{\nu}} \Omega_q^\dagger \Omega_q) (\bar{\ell}_s \gamma^{\bar{\nu}} \ell_r) \right] \\
& - \frac{1}{6} (\mathcal{C}_{\ell q}^{(3)})^{srtt} \left[ (D_{\bar{\mu}} \Omega_{q,a}^* D_{\bar{\rho}} \Omega_q^b) (\Omega_{q,b}^* D_{\bar{\sigma}} \Omega_q^a) \varepsilon^{\bar{\mu}\bar{\nu}\bar{\rho}\bar{\sigma}} (\bar{\ell}_s \gamma^{\bar{\nu}} \ell_r) - (D_{\bar{\mu}} \Omega_{q,a}^* \Omega_q^b) (D_{\bar{\nu}} \Omega_{q,b}^* D_{\bar{\rho}} \Omega_q^a) \varepsilon^{\bar{\mu}\bar{\nu}\bar{\rho}\bar{\sigma}} (\bar{\ell}_s \gamma^{\bar{\sigma}} \ell_r) \right] \\
& - \frac{i}{6} (\mathcal{C}_{\ell q}^{(3)})^{ttsr} \left[ (\Omega_\ell^\dagger D_2 D_{\bar{\mu}} \Omega_\ell) (\bar{q}_s \gamma^{\bar{\mu}} q_r) - (D_2 D_{\bar{\nu}} \Omega_\ell^\dagger \Omega_\ell) (\bar{q}_s \gamma^{\bar{\nu}} q_r) \right] \\
& - \frac{1}{6} (\mathcal{C}_{\ell q}^{(3)})^{ttsr} \left[ (\Omega_\ell^\dagger D_{\bar{\sigma}} \Omega_\ell) (D_{\bar{\mu}} \Omega_\ell^\dagger D_{\bar{\rho}} \Omega_\ell) \varepsilon^{\bar{\mu}\bar{\nu}\bar{\rho}\bar{\sigma}} (\bar{q}_s \gamma^{\bar{\nu}} q_r) - (D_{\bar{\mu}} \Omega_\ell^\dagger \Omega_\ell) (D_{\bar{\nu}} \Omega_\ell^\dagger D_{\bar{\rho}} \Omega_\ell) \varepsilon^{\bar{\mu}\bar{\nu}\bar{\rho}\bar{\sigma}} (\bar{q}_s \gamma^{\bar{\sigma}} q_r) \right] \\
& + \frac{i}{6} y_d^{vu} \bar{y}_d^{tu} (\mathcal{C}_{\ell q}^{(3)})^{srtv} (\Omega_d^\dagger \overset{\leftrightarrow}{D}_{\bar{\mu}} \Omega_d) (H^\dagger H) (\bar{\ell}_s \gamma^{\bar{\mu}} \ell_r) + \frac{i}{6} y_e^{vu} \bar{y}_e^{tu} (\mathcal{C}_{\ell q}^{(3)})^{tvsr} (\Omega_e^\dagger \overset{\leftrightarrow}{D}_{\bar{\mu}} \Omega_e) (H^\dagger H) (\bar{q}_s \gamma^{\bar{\mu}} q_r) \\
& - \frac{i}{6} y_u^{vu} \bar{y}_u^{tu} (\mathcal{C}_{\ell q}^{(3)})^{srtv} (\Omega_u^\dagger \overset{\leftrightarrow}{D}_{\bar{\mu}} \Omega_u) (H^\dagger H) (\bar{\ell}_s \gamma^{\bar{\mu}} \ell_r) \\
& + \frac{i}{4} g_s (\mathcal{C}_{\ell q}^{(3)})^{srtt} \left[ 2T_b^{Aa} (\Omega_{q,a}^* D_{\bar{\sigma}} \Omega_q^b) \widetilde{G}^{\bar{\rho}\bar{\sigma} A} (\bar{\ell}_s \gamma^{\bar{\rho}} \ell_r) + 2T_b^{Aa} (D_{\bar{\mu}} \Omega_{q,a}^* \Omega_q^b) \widetilde{G}^{\bar{\mu}\bar{\sigma} A} (\bar{\ell}_s \gamma^{\bar{\sigma}} \ell_r) \right] \\
& + \frac{i}{4} g_Y (\mathcal{C}_{\ell q}^{(3)})^{ttsr} \left[ 2(\Omega_{\ell,i}^* D_{\bar{\sigma}} \Omega_\ell^j) \widetilde{B}^{\bar{\rho}\bar{\sigma}} (\bar{q}_{js} \gamma^{\bar{\rho}} q_r^i) + 2(D_{\bar{\mu}} \Omega_{\ell,i}^* \Omega_\ell^j) \widetilde{B}^{\bar{\mu}\bar{\sigma}} (\bar{q}_{js} \gamma^{\bar{\sigma}} q_r^i) \right] \\
& - \frac{i}{3} (\mathcal{C}_{\ell q}^{(3)})^{srtt} \left[ (\Omega_q^\dagger D_{\bar{\nu}} \Omega_q) (D^{\bar{\mu}} \bar{\ell}_s \gamma^{\bar{\nu}} D^{\bar{\mu}} \ell_r) - (D_{\bar{\mu}} \Omega_q^\dagger \Omega_q) (D^{\bar{\nu}} \bar{\ell}_s \gamma^{\bar{\mu}} D^{\bar{\nu}} \ell_r) \right]
\end{aligned}$$

$$\begin{aligned}
& -\frac{i}{3}(\mathcal{C}_{\ell q}^{(3)})^{srtt} \left[ (\Omega_q^\dagger D_{\bar{\nu}} \Omega_q) (D^{\bar{\mu}} D^{\bar{\mu}} \bar{\ell}_s \gamma^{\bar{\nu}} \ell_r) - (D_{\bar{\mu}} \Omega_q^\dagger \Omega_q) (\bar{\ell}_s \gamma^{\bar{\mu}} D^{\bar{\nu}} D^{\bar{\nu}} \ell_r) \right] \\
& + \frac{i}{3}(\mathcal{C}_{\ell q}^{(3)})^{srtt} \left[ (\Omega_{q,i}^* D_2 D_{\bar{\mu}} \Omega_q^j) (\bar{\ell}_{js} \gamma^{\bar{\mu}} \ell_r^i) - (D_2 D_{\bar{\nu}} \Omega_{q,i}^* \Omega_q^j) (\bar{\ell}_{js} \gamma^{\bar{\nu}} \ell_r^i) \right] \\
& - \frac{i}{3}(\mathcal{C}_{\ell q}^{(3)})^{srtt} \left[ (D_{\bar{\mu}} \Omega_{q,ai}^* D_{\bar{\nu}} \Omega_q^{bj}) (\Omega_{q,bj}^* D_{\bar{\mu}} \Omega_q^{ak}) (\bar{\ell}_{ks} \gamma^{\bar{\nu}} \ell_r^i) - (D_{\bar{\mu}} \Omega_{q,ai}^* \Omega_q^{bj}) (D_{\bar{\nu}} \Omega_{q,bj}^* D_{\bar{\mu}} \Omega_q^{ak}) (\bar{\ell}_{ks} \gamma^{\bar{\nu}} \ell_r^i) \right] \\
& + \frac{i}{3}(\mathcal{C}_{\ell q}^{(3)})^{srtt} \left[ (\Omega_{q,ai}^* D_{\bar{\mu}} \Omega_q^{bk}) (D_{\bar{\mu}} D_{\bar{\nu}} \Omega_{q,bj}^* \Omega_q^{ai}) (\bar{\ell}_{ks} \gamma^{\bar{\nu}} \ell_r^j) - (\Omega_{q,ai}^* D_{\bar{\mu}} D_{\bar{\nu}} \Omega_q^{bk}) (D_{\bar{\mu}} \Omega_{q,bj}^* \Omega_q^{ai}) (\bar{\ell}_{ks} \gamma^{\bar{\nu}} \ell_r^j) \right] \\
& + \frac{1}{3}(\mathcal{C}_{\ell q}^{(3)})^{srtt} \left[ (D_{\bar{\mu}} \Omega_{q,a}^* D_{\bar{\rho}} \Omega_q^b) (\Omega_{q,bj}^* D_{\bar{\sigma}} \Omega_q^{ak}) \varepsilon^{\bar{\mu}\bar{\nu}\bar{\rho}\bar{\sigma}} (\bar{\ell}_{ks} \gamma^{\bar{\nu}} \ell_r^j) - (D_{\bar{\nu}} \Omega_{q,b}^* D_{\bar{\rho}} \Omega_q^a) (D_{\bar{\mu}} \Omega_{q,ai}^* \Omega_q^{bk}) \varepsilon^{\bar{\mu}\bar{\nu}\bar{\rho}\bar{\sigma}} (\bar{\ell}_{ks} \gamma^{\bar{\sigma}} \ell_r^i) \right] \\
& - \frac{i}{3}(\mathcal{C}_{\ell q}^{(3)})^{srtt} \left[ (\Omega_{q,ai}^* D_{\bar{\mu}} \Omega_q^{bk}) (\Omega_{q,bj}^* D_{\bar{\nu}} \Omega_q^{ai}) (D^{\bar{\mu}} \bar{\ell}_{ks} \gamma^{\bar{\nu}} \ell_r^j) - (D_{\bar{\mu}} \Omega_{q,ai}^* \Omega_q^{bk}) (D_{\bar{\nu}} \Omega_{q,bj}^* \Omega_q^{ai}) (\bar{\ell}_{ks} \gamma^{\bar{\mu}} D^{\bar{\nu}} \ell_r^j) \right] \\
& - \frac{i}{3}(\mathcal{C}_{\ell q}^{(3)})^{srtt} \left[ (\Omega_{q,ai}^* D_{\bar{\nu}} \Omega_q^{bk}) (\Omega_{q,bj}^* D_{\bar{\mu}} \Omega_q^{ai}) (\bar{\ell}_{ks} \gamma^{\bar{\mu}} D^{\bar{\nu}} \ell_r^j) - (D_{\bar{\mu}} \Omega_{q,ai}^* \Omega_q^{bk}) (D_{\bar{\nu}} \Omega_{q,bj}^* \Omega_q^{ai}) (D^{\bar{\nu}} \bar{\ell}_{ks} \gamma^{\bar{\mu}} \ell_r^j) \right] \\
& - \frac{1}{3}(\mathcal{C}_{\ell q}^{(3)})^{srtt} \left[ (D_{\bar{\mu}} \Omega_{q,a}^* \Omega_q^b) (D_{\bar{\nu}} \Omega_{q,bj}^* \Omega_q^{ak}) \varepsilon^{\bar{\mu}\bar{\nu}\bar{\rho}\bar{\sigma}} (\bar{\ell}_{ks} \gamma^{\bar{\rho}} D^{\bar{\sigma}} \ell_r^j) + (\Omega_{q,b}^* D_{\bar{\sigma}} \Omega_q^a) (\Omega_{q,ai}^* D_{\bar{\nu}} \Omega_q^{bk}) \varepsilon^{\bar{\mu}\bar{\nu}\bar{\rho}\bar{\sigma}} (D^{\bar{\rho}} \bar{\ell}_{ks} \gamma^{\bar{\mu}} \ell_r^i) \right] \\
& - \frac{i}{3}(\mathcal{C}_{\ell q}^{(3)})^{ttsr} \left[ (\Omega_\ell^\dagger D_{\bar{\nu}} \Omega_\ell) (D^{\bar{\mu}} \bar{q}_s \gamma^{\bar{\nu}} D^{\bar{\mu}} q_r) - (D_{\bar{\mu}} \Omega_\ell^\dagger \Omega_\ell) (D^{\bar{\nu}} \bar{q}_s \gamma^{\bar{\mu}} D^{\bar{\nu}} q_r) \right] \\
& - \frac{i}{3}(\mathcal{C}_{\ell q}^{(3)})^{ttsr} \left[ (\Omega_\ell^\dagger D_{\bar{\nu}} \Omega_\ell) (D^{\bar{\mu}} D^{\bar{\mu}} \bar{q}_s \gamma^{\bar{\nu}} q_r) - (D_{\bar{\mu}} \Omega_\ell^\dagger \Omega_\ell) (\bar{q}_s \gamma^{\bar{\mu}} D^{\bar{\nu}} D^{\bar{\nu}} q_r) \right] \\
& + \frac{i}{3}(\mathcal{C}_{\ell q}^{(3)})^{ttsr} \left[ (\Omega_{\ell,i}^* D_2 D_{\bar{\mu}} \Omega_\ell^j) (\bar{q}_{js} \gamma^{\bar{\mu}} q_r^i) - (D_2 D_{\bar{\nu}} \Omega_{\ell,i}^* \Omega_\ell^j) (\bar{q}_{js} \gamma^{\bar{\nu}} q_r^i) \right] \\
& - \frac{i}{3}(\mathcal{C}_{\ell q}^{(3)})^{ttsr} \left[ (D_{\bar{\mu}} D_{\bar{\nu}} \Omega_{\ell,i}^* \Omega_\ell^k) (\Omega_{\ell,j}^* D_{\bar{\mu}} \Omega_\ell^i) (\bar{q}_{ks} \gamma^{\bar{\nu}} q_r^j) - (D_{\bar{\mu}} \Omega_{\ell,i}^* \Omega_\ell^k) (\Omega_{\ell,j}^* D_{\bar{\mu}} D_{\bar{\nu}} \Omega_\ell^i) (\bar{q}_{ks} \gamma^{\bar{\nu}} q_r^j) \right] \\
& + \frac{i}{3}(\mathcal{C}_{\ell q}^{(3)})^{ttsr} \left[ (D_{\bar{\mu}} \Omega_{\ell,i}^* D_{\bar{\nu}} \Omega_\ell^k) (\Omega_{\ell,j}^* D_{\bar{\mu}} \Omega_\ell^i) (\bar{q}_{ks} \gamma^{\bar{\nu}} q_r^j) - (D_{\bar{\mu}} \Omega_{\ell,i}^* \Omega_\ell^k) (D_{\bar{\nu}} \Omega_{\ell,j}^* D_{\bar{\mu}} \Omega_\ell^i) (\bar{q}_{ks} \gamma^{\bar{\nu}} q_r^j) \right] \\
& + \frac{1}{3}(\mathcal{C}_{\ell q}^{(3)})^{ttsr} \left[ (D_{\bar{\mu}} \Omega_\ell^\dagger D_{\bar{\rho}} \Omega_\ell) (\Omega_{\ell,j}^* D_{\bar{\sigma}} \Omega_\ell^k) \varepsilon^{\bar{\mu}\bar{\nu}\bar{\rho}\bar{\sigma}} (\bar{q}_{ks} \gamma^{\bar{\nu}} q_r^j) + (D_{\bar{\mu}} \Omega_\ell^\dagger D_{\bar{\rho}} \Omega_\ell) (D_{\bar{\nu}} \Omega_{\ell,j}^* \Omega_\ell^k) \varepsilon^{\bar{\mu}\bar{\nu}\bar{\rho}\bar{\sigma}} (\bar{q}_{ks} \gamma^{\bar{\sigma}} q_r^j) \right] \\
& + \frac{i}{3}(\mathcal{C}_{\ell q}^{(3)})^{ttsr} \left[ (\Omega_{\ell,i}^* D_{\bar{\nu}} \Omega_\ell^k) (\Omega_{\ell,j}^* D_{\bar{\mu}} \Omega_\ell^i) (D^{\bar{\mu}} \bar{q}_{ks} \gamma^{\bar{\nu}} q_r^j) - (D_{\bar{\mu}} \Omega_{\ell,i}^* \Omega_\ell^k) (D_{\bar{\nu}} \Omega_{\ell,j}^* \Omega_\ell^i) (\bar{q}_{ks} \gamma^{\bar{\nu}} D^{\bar{\mu}} q_r^j) \right] \\
& + \frac{i}{3}(\mathcal{C}_{\ell q}^{(3)})^{ttsr} \left[ (\Omega_{\ell,i}^* D_{\bar{\mu}} \Omega_\ell^k) (\Omega_{\ell,j}^* D_{\bar{\nu}} \Omega_\ell^i) (\bar{q}_{ks} \gamma^{\bar{\mu}} D^{\bar{\nu}} q_r^j) - (D_{\bar{\mu}} \Omega_{\ell,i}^* \Omega_\ell^k) (D_{\bar{\nu}} \Omega_{\ell,j}^* \Omega_\ell^i) (D^{\bar{\mu}} \bar{q}_{ks} \gamma^{\bar{\nu}} q_r^j) \right] \\
& - \frac{1}{3}(\mathcal{C}_{\ell q}^{(3)})^{ttsr} \left[ (D_{\bar{\mu}} \Omega_\ell^\dagger \Omega_\ell) (D_{\bar{\nu}} \Omega_{\ell,j}^* \Omega_\ell^k) \varepsilon^{\bar{\mu}\bar{\nu}\bar{\rho}\bar{\sigma}} (\bar{q}_{ks} \gamma^{\bar{\rho}} D^{\bar{\sigma}} q_r^j) + (\Omega_\ell^\dagger D_{\bar{\sigma}} \Omega_\ell) (\Omega_{\ell,j}^* D_{\bar{\nu}} \Omega_\ell^k) \varepsilon^{\bar{\mu}\bar{\nu}\bar{\rho}\bar{\sigma}} (D^{\bar{\rho}} \bar{q}_{ks} \gamma^{\bar{\mu}} q_r^j) \right] \\
& - \frac{i}{3} y_d^{vu} \bar{y}_d^{tu} (\mathcal{C}_{\ell q}^{(3)})^{srtv} (\Omega_d^\dagger \bar{D}_{\bar{\mu}} \Omega_d) (\bar{\ell}_s H \gamma^{\bar{\mu}} H^\dagger \ell_r) - \frac{i}{3} y_e^{vu} \bar{y}_e^{tu} (\mathcal{C}_{\ell q}^{(3)})^{tvsr} (\Omega_e^\dagger \bar{D}_{\bar{\mu}} \Omega_e) (\bar{q}_s H \gamma^{\bar{\mu}} H^\dagger q_r) \\
& + \frac{i}{3} y_u^{vu} \bar{y}_u^{tu} (\mathcal{C}_{\ell q}^{(3)})^{srtv} (\Omega_u^\dagger \bar{D}_{\bar{\mu}} \Omega_u) (\bar{\ell}_s H \gamma^{\bar{\mu}} H^\dagger \ell_r) \\
& - \frac{5i}{12} g_L (\mathcal{C}_{\ell q}^{(3)})^{srtt} \left[ 2(\Omega_q^\dagger D_{\bar{\sigma}} \Omega_q) \widetilde{W}^{\bar{\rho}\bar{\sigma}I} (\bar{\ell}_s t^I \gamma^{\bar{\rho}} \ell_r) + 2(D_{\bar{\mu}} \Omega_q^\dagger \Omega_q) \widetilde{W}^{\bar{\mu}\bar{\sigma}I} (\bar{\ell}_s t^I \gamma^{\bar{\sigma}} \ell_r) \right] \\
& - \frac{5i}{12} g_L (\mathcal{C}_{\ell q}^{(3)})^{ttsr} \left[ 2(\Omega_\ell^\dagger D_{\bar{\sigma}} \Omega_\ell) \widetilde{W}^{\bar{\rho}\bar{\sigma}I} (\bar{q}_s t^I \gamma^{\bar{\rho}} q_r) + 2(D_{\bar{\mu}} \Omega_\ell^\dagger \Omega_\ell) \widetilde{W}^{\bar{\mu}\bar{\sigma}I} (\bar{q}_s t^I \gamma^{\bar{\sigma}} q_r) \right] \\
& - \frac{i}{2} g_s (\mathcal{C}_{\ell q}^{(3)})^{srtt} \left[ 2T_b^{Aa} (\Omega_{q,ai}^* D_{\bar{\sigma}} \Omega_q^{bj}) \widetilde{G}^{\bar{\rho}\bar{\sigma}A} (\bar{\ell}_{js} \gamma^{\bar{\rho}} \ell_r^i) + 2T_b^{Aa} (D_{\bar{\mu}} \Omega_{q,ai}^* \Omega_q^{bj}) \widetilde{G}^{\bar{\mu}\bar{\sigma}A} (\bar{\ell}_{js} \gamma^{\bar{\sigma}} \ell_r^i) \right] \\
& + \frac{2i}{3} (\mathcal{C}_{\ell q}^{(3)})^{srtt} \left[ (\Omega_{q,i}^* D_{\bar{\nu}} \Omega_q^j) (D^{\bar{\mu}} \bar{\ell}_{js} \gamma^{\bar{\nu}} D^{\bar{\mu}} \ell_r^i) - (D_{\bar{\mu}} \Omega_{q,i}^* \Omega_q^j) (D^{\bar{\nu}} \bar{\ell}_{js} \gamma^{\bar{\mu}} D^{\bar{\nu}} \ell_r^i) \right]
\end{aligned}$$

$$\begin{aligned}
& + \frac{2i}{3}(\mathcal{C}_{\ell q}^{(3)})^{srtt} \left[ (\Omega_{q,i}^* D_{\bar{\nu}} \Omega_q^j) (D^{\bar{\mu}} D^{\bar{\mu}} \bar{\ell}_{js} \gamma^{\bar{\nu}} \ell_r^i) - (D_{\bar{\mu}} \Omega_{q,i}^* \Omega_q^j) (\bar{\ell}_{js} \gamma^{\bar{\mu}} D^{\bar{\nu}} D^{\bar{\nu}} \ell_r^i) \right] \\
& + \frac{2i}{3}(\mathcal{C}_{\ell q}^{(3)})^{srtt} \left[ (D_{\bar{\mu}} \Omega_{q,ai}^* D_{\bar{\nu}} \Omega_q^{bk}) (\Omega_{q,bj}^* D_{\bar{\mu}} \Omega_q^{ai}) (\bar{\ell}_{ks} \gamma^{\bar{\nu}} \ell_r^j) - (D_{\bar{\mu}} \Omega_{q,ai}^* \Omega_q^{bk}) (D_{\bar{\nu}} \Omega_{q,bj}^* D_{\bar{\mu}} \Omega_q^{ai}) (\bar{\ell}_{ks} \gamma^{\bar{\nu}} \ell_r^j) \right] \\
& + \frac{2i}{3}(\mathcal{C}_{\ell q}^{(3)})^{ttsr} \left[ (\Omega_{\ell,i}^* D_{\bar{\nu}} \Omega_{\ell}^j) (D^{\bar{\mu}} \bar{q}_{js} \gamma^{\bar{\nu}} D^{\bar{\mu}} q_r^i) - (D_{\bar{\mu}} \Omega_{\ell,i}^* \Omega_{\ell}^j) (D^{\bar{\nu}} \bar{q}_{js} \gamma^{\bar{\mu}} D^{\bar{\nu}} q_r^i) \right] \\
& + \frac{2i}{3}(\mathcal{C}_{\ell q}^{(3)})^{ttsr} \left[ (\Omega_{\ell,i}^* D_{\bar{\nu}} \Omega_{\ell}^j) (D^{\bar{\mu}} D^{\bar{\mu}} \bar{q}_{js} \gamma^{\bar{\nu}} q_r^i) - (D_{\bar{\mu}} \Omega_{\ell,i}^* \Omega_{\ell}^j) (\bar{q}_{js} \gamma^{\bar{\mu}} D^{\bar{\nu}} D^{\bar{\nu}} q_r^i) \right] \\
& - \frac{2i}{3}(\mathcal{C}_{\ell q}^{(3)})^{ttsr} \left[ (\Omega_{\ell,i}^* D_{\bar{\mu}} \Omega_{\ell}^k) (D_{\bar{\mu}} \Omega_{\ell,j}^* D_{\bar{\nu}} \Omega_{\ell}^i) (\bar{q}_{ks} \gamma^{\bar{\nu}} q_r^j) - (D_{\bar{\mu}} \Omega_{\ell,i}^* D_{\bar{\nu}} \Omega_{\ell}^k) (D_{\bar{\nu}} \Omega_{\ell,j}^* \Omega_{\ell}^i) (\bar{q}_{ks} \gamma^{\bar{\mu}} q_r^j) \right] \\
& - \frac{2i}{3} y_e^{vu} \bar{y}_e^{tu} (\mathcal{C}_{\ell q}^{(3)})^{tvsr} (\Omega_{\ell,j}^* \overset{\leftrightarrow}{D}_{\bar{\mu}} \Omega_{\ell}^i) H_i^{\dagger} H^j (\bar{q}_s \gamma^{\bar{\mu}} q_r) - \frac{2i}{3} y_u^{vu} \bar{y}_u^{tu} (\mathcal{C}_{\ell q}^{(3)})^{srtv} (\Omega_q^{\dagger} \overset{\leftrightarrow}{D}_{\bar{\mu}} \Omega_q) (H^{\dagger} H) (\bar{\ell}_s \gamma^{\bar{\mu}} \ell_r) \\
& - \frac{2i}{3} (\mathcal{C}_{\ell q}^{(3)})^{srtv} \left[ y_d^{vu} \bar{y}_d^{tu} - y_u^{vu} \bar{y}_u^{tu} \right] (\Omega_{q,j}^* \overset{\leftrightarrow}{D}_{\bar{\mu}} \Omega_q^i) H_i^{\dagger} H^j (\bar{\ell}_s \gamma^{\bar{\mu}} \ell_r) \\
& + \frac{4i}{3} (\mathcal{C}_{\ell q}^{(3)})^{srtv} \left[ y_d^{vu} \bar{y}_d^{tu} - y_u^{vu} \bar{y}_u^{tu} \right] \left[ (\Omega_{q,j}^* D_{\bar{\mu}} \Omega_q^i) H_i^{\dagger} (\bar{\ell}_s H \gamma^{\bar{\mu}} \ell_r^j) - (D_{\bar{\mu}} \Omega_{q,j}^* \Omega_q^k) H^j (\bar{\ell}_{ks} \gamma^{\bar{\mu}} H^{\dagger} \ell_r) \right] \\
& + \frac{4i}{3} y_e^{vu} \bar{y}_e^{tu} (\mathcal{C}_{\ell q}^{(3)})^{tvsr} \left[ (\Omega_{\ell,j}^* D_{\bar{\mu}} \Omega_{\ell}^i) H_i^{\dagger} (\bar{q}_s H \gamma^{\bar{\mu}} q_r^j) - (D_{\bar{\mu}} \Omega_{\ell,j}^* \Omega_{\ell}^k) H^j (\bar{q}_{ks} \gamma^{\bar{\mu}} H^{\dagger} q_r) \right] \\
& + \frac{4i}{3} y_u^{vu} \bar{y}_u^{tu} (\mathcal{C}_{\ell q}^{(3)})^{srtv} (\Omega_{q,j}^* \overset{\leftrightarrow}{D}_{\bar{\mu}} \Omega_q^k) (H^{\dagger} H) (\bar{\ell}_{ks} \gamma^{\bar{\mu}} \ell_r^j) \\
& - 2g_L (\mathcal{C}_{\ell q}^{(3)})^{srtt} \left[ t_j^{Ii} (\Omega_{q,i}^* D_{\bar{\nu}} \Omega_q^k) W^{\bar{\mu}\bar{\nu}I} (\bar{\ell}_{ks} \gamma^{\bar{\mu}} \ell_r^j) - t_k^{Ij} (D_{\bar{\mu}} \Omega_{q,i}^* \Omega_q^k) W^{\bar{\mu}\bar{\nu}I} (\bar{\ell}_{js} \gamma^{\bar{\nu}} \ell_r^i) \right] \\
& - 2g_L (\mathcal{C}_{\ell q}^{(3)})^{ttsr} \left[ t_j^{Ii} (\Omega_{\ell,i}^* D_{\bar{\nu}} \Omega_{\ell}^k) W^{\bar{\mu}\bar{\nu}I} (\bar{q}_{ks} \gamma^{\bar{\mu}} q_r^j) - t_k^{Ij} (D_{\bar{\mu}} \Omega_{\ell,i}^* \Omega_{\ell}^k) W^{\bar{\mu}\bar{\nu}I} (\bar{q}_{js} \gamma^{\bar{\nu}} q_r^i) \right], \tag{3.51}
\end{aligned}$$

$$\begin{aligned}
\Gamma_{ud}^{(1)} [\mathcal{O}_{ud}^{(1)}] &= -\frac{i}{9} g_Y (\mathcal{C}_{ud}^{(1)})^{srtt} \left[ 2(\Omega_d^{\dagger} D_{\bar{\sigma}} \Omega_d) \tilde{B}^{\bar{\rho}\bar{\sigma}} (\bar{u}_s \gamma^{\bar{\rho}} u_r) + 2(D_{\bar{\mu}} \Omega_d^{\dagger} \Omega_d) \tilde{B}^{\bar{\mu}\bar{\sigma}} (\bar{u}_s \gamma^{\bar{\sigma}} u_r) \right] \\
&+ \frac{i}{6} (\mathcal{C}_{ud}^{(1)})^{ttsr} \left[ (\Omega_u^{\dagger} D_2 D_{\bar{\mu}} \Omega_u) (\bar{d}_s \gamma^{\bar{\mu}} d_r) - (D_2 D_{\bar{\nu}} \Omega_u^{\dagger} \Omega_u) (\bar{d}_s \gamma^{\bar{\nu}} d_r) \right] \\
&- \frac{1}{6} (\mathcal{C}_{ud}^{(1)})^{ttsr} \left[ (D_{\bar{\mu}} \Omega_{u,a}^* D_{\bar{\rho}} \Omega_u^b) (\Omega_{u,b}^* D_{\bar{\sigma}} \Omega_u^a) \varepsilon^{\bar{\mu}\bar{\nu}\bar{\rho}\bar{\sigma}} (\bar{d}_s \gamma^{\bar{\nu}} d_r) - (D_{\bar{\mu}} \Omega_{u,a}^* \Omega_u^b) (D_{\bar{\nu}} \Omega_{u,b}^* D_{\bar{\rho}} \Omega_u^a) \varepsilon^{\bar{\mu}\bar{\nu}\bar{\rho}\bar{\sigma}} (\bar{d}_s \gamma^{\bar{\sigma}} d_r) \right] \\
&+ \frac{i}{6} (\mathcal{C}_{ud}^{(1)})^{srtt} \left[ (\Omega_d^{\dagger} D_2 D_{\bar{\mu}} \Omega_d) (\bar{u}_s \gamma^{\bar{\mu}} u_r) - (D_2 D_{\bar{\nu}} \Omega_d^{\dagger} \Omega_d) (\bar{u}_s \gamma^{\bar{\nu}} u_r) \right] \\
&- \frac{1}{6} (\mathcal{C}_{ud}^{(1)})^{srtt} \left[ (D_{\bar{\mu}} \Omega_{d,a}^* D_{\bar{\rho}} \Omega_d^b) (\Omega_{d,b}^* D_{\bar{\sigma}} \Omega_d^a) \varepsilon^{\bar{\mu}\bar{\nu}\bar{\rho}\bar{\sigma}} (\bar{u}_s \gamma^{\bar{\nu}} u_r) - (D_{\bar{\mu}} \Omega_{d,a}^* \Omega_d^b) (D_{\bar{\nu}} \Omega_{d,b}^* D_{\bar{\rho}} \Omega_d^a) \varepsilon^{\bar{\mu}\bar{\nu}\bar{\rho}\bar{\sigma}} (\bar{u}_s \gamma^{\bar{\sigma}} u_r) \right] \\
&- \frac{i}{6} y_u^{tv} \bar{y}_u^{tu} (\mathcal{C}_{ud}^{(1)})^{vusr} (\Omega_q^{\dagger} \overset{\leftrightarrow}{D}_{\bar{\mu}} \Omega_q) (H^{\dagger} H) (\bar{d}_s \gamma^{\bar{\mu}} d_r) + \frac{i}{6} y_u^{tv} \bar{y}_u^{tu} (\mathcal{C}_{ud}^{(1)})^{vusr} (\Omega_{q,j}^* \overset{\leftrightarrow}{D}_{\bar{\mu}} \Omega_q^i) H_i^{\dagger} H^j (\bar{d}_s \gamma^{\bar{\mu}} d_r) \\
&- \frac{i}{6} y_d^{tv} \bar{y}_d^{tu} (\mathcal{C}_{ud}^{(1)})^{srvu} (\Omega_{q,j}^* \overset{\leftrightarrow}{D}_{\bar{\mu}} \Omega_q^i) H_i^{\dagger} H^j (\bar{u}_s \gamma^{\bar{\mu}} u_r) \\
&+ \frac{2i}{9} g_Y (\mathcal{C}_{ud}^{(1)})^{ttsr} \left[ 2(\Omega_u^{\dagger} D_{\bar{\sigma}} \Omega_u) \tilde{B}^{\bar{\rho}\bar{\sigma}} (\bar{d}_s \gamma^{\bar{\rho}} d_r) + 2(D_{\bar{\mu}} \Omega_u^{\dagger} \Omega_u) \tilde{B}^{\bar{\mu}\bar{\sigma}} (\bar{d}_s \gamma^{\bar{\sigma}} d_r) \right] \\
&+ \frac{i}{3} g_s (\mathcal{C}_{ud}^{(1)})^{ttsr} \left[ 2T_b^{Aa} (\Omega_{u,a}^* D_{\bar{\sigma}} \Omega_u^b) \tilde{G}^{\bar{\rho}\bar{\sigma}A} (\bar{d}_s \gamma^{\bar{\rho}} d_r) + 2T_b^{Aa} (D_{\bar{\mu}} \Omega_{u,a}^* \Omega_u^b) \tilde{G}^{\bar{\mu}\bar{\sigma}A} (\bar{d}_s \gamma^{\bar{\sigma}} d_r) \right] \\
&+ \frac{i}{3} (\mathcal{C}_{ud}^{(1)})^{ttsr} \left[ (\Omega_u^{\dagger} D_{\bar{\nu}} \Omega_u) (D^{\bar{\mu}} \bar{d}_s \gamma^{\bar{\nu}} D^{\bar{\mu}} d_r) - (D_{\bar{\mu}} \Omega_u^{\dagger} \Omega_u) (D^{\bar{\nu}} \bar{d}_s \gamma^{\bar{\mu}} D^{\bar{\nu}} d_r) \right] \\
&+ \frac{i}{3} (\mathcal{C}_{ud}^{(1)})^{ttsr} \left[ (\Omega_u^{\dagger} D_{\bar{\nu}} \Omega_u) (D^{\bar{\mu}} D^{\bar{\mu}} \bar{d}_s \gamma^{\bar{\nu}} d_r) - (D_{\bar{\mu}} \Omega_u^{\dagger} \Omega_u) (\bar{d}_s \gamma^{\bar{\mu}} D^{\bar{\nu}} D^{\bar{\nu}} d_r) \right]
\end{aligned}$$

$$\begin{aligned}
& + \frac{i}{3} y_u^{rt} \bar{y}_d^{rs} (\mathcal{C}_{ud}^{(1)})^{tuv s} (D_{\bar{\mu}} \Omega_{q,ak}^* \Omega_q^{bj}) H_j^\dagger \tilde{H}_k (\bar{d}_{bv} \gamma^{\bar{\mu}} u_u^a) \\
& + \frac{i}{3} g_s (\mathcal{C}_{ud}^{(1)})^{srtt} \left[ 2T_b^{Aa} (\Omega_{d,a}^* D_{\bar{\sigma}} \Omega_d^b) \tilde{G}^{\bar{\rho}\bar{\sigma} A} (\bar{u}_s \gamma^{\bar{\rho}} u_r) + 2T_b^{Aa} (D_{\bar{\mu}} \Omega_{d,a}^* \Omega_d^b) \tilde{G}^{\bar{\mu}\bar{\sigma} A} (\bar{u}_s \gamma^{\bar{\sigma}} u_r) \right] \\
& + \frac{i}{3} (\mathcal{C}_{ud}^{(1)})^{srtt} \left[ (\Omega_d^\dagger D_{\bar{\nu}} \Omega_d) (D^{\bar{\mu}} \bar{u}_s \gamma^{\bar{\nu}} D^{\bar{\mu}} u_r) - (D_{\bar{\mu}} \Omega_d^\dagger \Omega_d) (D^{\bar{\nu}} \bar{u}_s \gamma^{\bar{\mu}} D^{\bar{\nu}} u_r) \right] \\
& + \frac{i}{3} (\mathcal{C}_{ud}^{(1)})^{srtt} \left[ (\Omega_d^\dagger D_{\bar{\nu}} \Omega_d) (D^{\bar{\mu}} D^{\bar{\mu}} \bar{u}_s \gamma^{\bar{\nu}} u_r) - (D_{\bar{\mu}} \Omega_d^\dagger \Omega_d) (\bar{u}_s \gamma^{\bar{\mu}} D^{\bar{\nu}} D^{\bar{\nu}} u_r) \right] \\
& - \frac{i}{3} y_d^{ru} \bar{y}_u^{rs} (\mathcal{C}_{ud}^{(1)})^{tsuv} (\Omega_{q,ai}^* D_{\bar{\mu}} \Omega_q^{bj}) \tilde{H}^{\dagger j} H^i (\bar{u}_{bt} \gamma^{\bar{\mu}} d_v^a) + \frac{2i}{3} y_d^{tv} \bar{y}_d^{tu} (\mathcal{C}_{ud}^{(1)})^{srvu} (\Omega_d^\dagger \overleftrightarrow{D}_{\bar{\mu}} \Omega_d) (H^\dagger H) (\bar{u}_s \gamma^{\bar{\mu}} u_r) \\
& + \frac{2i}{3} y_u^{tv} \bar{y}_u^{tu} (\mathcal{C}_{ud}^{(1)})^{vusr} (\Omega_u^\dagger \overleftrightarrow{D}_{\bar{\mu}} \Omega_u) (H^\dagger H) (\bar{d}_s \gamma^{\bar{\mu}} d_r), \tag{3.52}
\end{aligned}$$

$$\begin{aligned}
\Gamma_\Omega^{(1)} [\mathcal{O}_{ud}^{(8)}] &= \frac{i}{54} g_Y (\mathcal{C}_{ud}^{(8)})^{srtt} \left[ 2(\Omega_d^\dagger D_{\bar{\sigma}} \Omega_d) \tilde{B}^{\bar{\rho}\bar{\sigma}} (\bar{u}_s \gamma^{\bar{\rho}} u_r) + 2(D_{\bar{\mu}} \Omega_d^\dagger \Omega_d) \tilde{B}^{\bar{\mu}\bar{\sigma}} (\bar{u}_s \gamma^{\bar{\sigma}} u_r) \right] \\
& - \frac{i}{36} (\mathcal{C}_{ud}^{(8)})^{ttsr} \left[ (\Omega_u^\dagger D_2 D_{\bar{\mu}} \Omega_u) (\bar{d}_s \gamma^{\bar{\mu}} d_r) - (D_2 D_{\bar{\nu}} \Omega_u^\dagger \Omega_u) (\bar{d}_s \gamma^{\bar{\nu}} d_r) \right] \\
& + \frac{1}{36} (\mathcal{C}_{ud}^{(8)})^{ttsr} \left[ (D_{\bar{\mu}} \Omega_{u,a}^* D_{\bar{\rho}} \Omega_u^b) (\Omega_{u,b}^* D_{\bar{\sigma}} \Omega_u^a) \varepsilon^{\bar{\mu}\bar{\nu}\bar{\rho}\bar{\sigma}} (\bar{d}_s \gamma^{\bar{\nu}} d_r) - (D_{\bar{\mu}} \Omega_{u,a}^* \Omega_u^b) (D_{\bar{\nu}} \Omega_{u,b}^* D_{\bar{\rho}} \Omega_u^a) \varepsilon^{\bar{\mu}\bar{\nu}\bar{\rho}\bar{\sigma}} (\bar{d}_s \gamma^{\bar{\sigma}} d_r) \right] \\
& - \frac{i}{36} (\mathcal{C}_{ud}^{(8)})^{srtt} \left[ (\Omega_d^\dagger D_2 D_{\bar{\mu}} \Omega_d) (\bar{u}_s \gamma^{\bar{\mu}} u_r) - (D_2 D_{\bar{\nu}} \Omega_d^\dagger \Omega_d) (\bar{u}_s \gamma^{\bar{\nu}} u_r) \right] \\
& + \frac{1}{36} (\mathcal{C}_{ud}^{(8)})^{srtt} \left[ (D_{\bar{\mu}} \Omega_{d,a}^* D_{\bar{\rho}} \Omega_d^b) (\Omega_{d,b}^* D_{\bar{\sigma}} \Omega_d^a) \varepsilon^{\bar{\mu}\bar{\nu}\bar{\rho}\bar{\sigma}} (\bar{u}_s \gamma^{\bar{\nu}} u_r) - (D_{\bar{\mu}} \Omega_{d,a}^* \Omega_d^b) (D_{\bar{\nu}} \Omega_{d,b}^* D_{\bar{\rho}} \Omega_d^a) \varepsilon^{\bar{\mu}\bar{\nu}\bar{\rho}\bar{\sigma}} (\bar{u}_s \gamma^{\bar{\sigma}} u_r) \right] \\
& + \frac{i}{36} y_u^{tv} \bar{y}_u^{tu} (\mathcal{C}_{ud}^{(8)})^{vusr} (\Omega_q^\dagger \overleftrightarrow{D}_{\bar{\mu}} \Omega_q) (H^\dagger H) (\bar{d}_s \gamma^{\bar{\mu}} d_r) - \frac{i}{36} y_u^{tv} \bar{y}_u^{tu} (\mathcal{C}_{ud}^{(8)})^{vusr} (\Omega_{q,j}^* \overleftrightarrow{D}_{\bar{\mu}} \Omega_q^i) H_i^\dagger H^j (\bar{d}_s \gamma^{\bar{\mu}} d_r) \\
& + \frac{i}{36} y_d^{tv} \bar{y}_d^{tu} (\mathcal{C}_{ud}^{(8)})^{srvu} (\Omega_{q,j}^* \overleftrightarrow{D}_{\bar{\mu}} \Omega_q^i) H_i^\dagger H^j (\bar{u}_s \gamma^{\bar{\mu}} u_r) \\
& - \frac{i}{27} g_Y (\mathcal{C}_{ud}^{(8)})^{ttsr} \left[ 2(\Omega_u^\dagger D_{\bar{\sigma}} \Omega_u) \tilde{B}^{\bar{\rho}\bar{\sigma}} (\bar{d}_s \gamma^{\bar{\rho}} d_r) + 2(D_{\bar{\mu}} \Omega_u^\dagger \Omega_u) \tilde{B}^{\bar{\mu}\bar{\sigma}} (\bar{d}_s \gamma^{\bar{\sigma}} d_r) \right] \\
& - \frac{i}{18} g_s (\mathcal{C}_{ud}^{(8)})^{ttsr} \left[ 2T_b^{Aa} (\Omega_{u,a}^* D_{\bar{\sigma}} \Omega_u^b) \tilde{G}^{\bar{\rho}\bar{\sigma} A} (\bar{d}_s \gamma^{\bar{\rho}} d_r) + 2T_b^{Aa} (D_{\bar{\mu}} \Omega_{u,a}^* \Omega_u^b) \tilde{G}^{\bar{\mu}\bar{\sigma} A} (\bar{d}_s \gamma^{\bar{\sigma}} d_r) \right] \\
& - \frac{i}{18} (\mathcal{C}_{ud}^{(8)})^{ttsr} \left[ (\Omega_u^\dagger D_{\bar{\nu}} \Omega_u) (D^{\bar{\mu}} \bar{d}_s \gamma^{\bar{\nu}} D^{\bar{\mu}} d_r) - (D_{\bar{\mu}} \Omega_u^\dagger \Omega_u) (D^{\bar{\nu}} \bar{d}_s \gamma^{\bar{\mu}} D^{\bar{\nu}} d_r) \right] \\
& - \frac{i}{18} (\mathcal{C}_{ud}^{(8)})^{ttsr} \left[ (\Omega_u^\dagger D_{\bar{\nu}} \Omega_u) (D^{\bar{\mu}} D^{\bar{\mu}} \bar{d}_s \gamma^{\bar{\nu}} d_r) - (D_{\bar{\mu}} \Omega_u^\dagger \Omega_u) (\bar{d}_s \gamma^{\bar{\mu}} D^{\bar{\nu}} D^{\bar{\nu}} d_r) \right] \\
& - \frac{i}{18} y_u^{rt} \bar{y}_d^{rs} (\mathcal{C}_{ud}^{(8)})^{tuv s} (D_{\bar{\mu}} \Omega_{q,ak}^* \Omega_q^{bj}) H_j^\dagger \tilde{H}_k (\bar{d}_{bv} \gamma^{\bar{\mu}} u_u^a) \\
& - \frac{i}{18} g_s (\mathcal{C}_{ud}^{(8)})^{srtt} \left[ 2T_b^{Aa} (\Omega_{d,a}^* D_{\bar{\sigma}} \Omega_d^b) \tilde{G}^{\bar{\rho}\bar{\sigma} A} (\bar{u}_s \gamma^{\bar{\rho}} u_r) + 2T_b^{Aa} (D_{\bar{\mu}} \Omega_{d,a}^* \Omega_d^b) \tilde{G}^{\bar{\mu}\bar{\sigma} A} (\bar{u}_s \gamma^{\bar{\sigma}} u_r) \right] \\
& - \frac{i}{18} (\mathcal{C}_{ud}^{(8)})^{srtt} \left[ (\Omega_d^\dagger D_{\bar{\nu}} \Omega_d) (D^{\bar{\mu}} \bar{u}_s \gamma^{\bar{\nu}} D^{\bar{\mu}} u_r) - (D_{\bar{\mu}} \Omega_d^\dagger \Omega_d) (D^{\bar{\nu}} \bar{u}_s \gamma^{\bar{\mu}} D^{\bar{\nu}} u_r) \right] \\
& - \frac{i}{18} (\mathcal{C}_{ud}^{(8)})^{srtt} \left[ (\Omega_d^\dagger D_{\bar{\nu}} \Omega_d) (D^{\bar{\mu}} D^{\bar{\mu}} \bar{u}_s \gamma^{\bar{\nu}} u_r) - (D_{\bar{\mu}} \Omega_d^\dagger \Omega_d) (\bar{u}_s \gamma^{\bar{\mu}} D^{\bar{\nu}} D^{\bar{\nu}} u_r) \right] \\
& - \frac{i}{18} g_Y (\mathcal{C}_{ud}^{(8)})^{srtt} \left[ 2(\Omega_{d,a}^* D_{\bar{\sigma}} \Omega_d^b) \tilde{B}^{\bar{\rho}\bar{\sigma}} (\bar{u}_{bs} \gamma^{\bar{\rho}} u_r^a) + 2(D_{\bar{\mu}} \Omega_{d,a}^* \Omega_d^b) \tilde{B}^{\bar{\mu}\bar{\sigma}} (\bar{u}_{bs} \gamma^{\bar{\sigma}} u_r^a) \right] \\
& + \frac{i}{18} y_d^{ru} \bar{y}_u^{rs} (\mathcal{C}_{ud}^{(8)})^{tsuv} (\Omega_{q,ai}^* D_{\bar{\mu}} \Omega_q^{bj}) \tilde{H}^{\dagger j} H^i (\bar{u}_{bt} \gamma^{\bar{\mu}} d_v^a)
\end{aligned}$$

$$\begin{aligned}
& + \frac{i}{12}(\mathcal{C}_{ud}^{(8)})^{ttsr} \left[ (\Omega_{u,a}^* D_2 D_{\bar{\mu}} \Omega_u^b) (\bar{d}_{bs} \gamma^{\bar{\mu}} d_r^a) - (D_2 D_{\bar{\nu}} \Omega_{u,a}^* \Omega_u^b) (\bar{d}_{bs} \gamma^{\bar{\nu}} d_r^a) \right] \\
& - \frac{i}{12}(\mathcal{C}_{ud}^{(8)})^{ttsr} \left[ (D_{\bar{\mu}} D_{\bar{\nu}} \Omega_{u,a}^* \Omega_u^c) (\Omega_{u,b}^* D_{\bar{\mu}} \Omega_u^a) (\bar{d}_{cs} \gamma^{\bar{\nu}} d_r^b) - (D_{\bar{\mu}} \Omega_{u,a}^* \Omega_u^c) (\Omega_{u,b}^* D_{\bar{\mu}} D_{\bar{\nu}} \Omega_u^a) (\bar{d}_{cs} \gamma^{\bar{\nu}} d_r^b) \right] \\
& + \frac{i}{12}(\mathcal{C}_{ud}^{(8)})^{ttsr} \left[ (\Omega_{u,a}^* D_{\bar{\nu}} \Omega_u^c) (D_{\bar{\mu}} \Omega_{u,b}^* D_{\bar{\nu}} \Omega_u^a) (\bar{d}_{cs} \gamma^{\bar{\mu}} d_r^b) - (D_{\bar{\mu}} \Omega_{u,a}^* D_{\bar{\nu}} \Omega_u^c) (D_{\bar{\mu}} \Omega_{u,b}^* \Omega_u^a) (\bar{d}_{cs} \gamma^{\bar{\nu}} d_r^b) \right] \\
& + \frac{1}{12}(\mathcal{C}_{ud}^{(8)})^{ttsr} \left[ (\Omega_{u,a}^* D_{\bar{\rho}} \Omega_u^c) (D_{\bar{\mu}} \Omega_{u,b}^* D_{\bar{\sigma}} \Omega_u^a) \varepsilon^{\bar{\mu}\bar{\nu}\bar{\rho}\bar{\sigma}} (\bar{d}_{cs} \gamma^{\bar{\nu}} d_r^b) - (D_{\bar{\mu}} \Omega_{u,a}^* D_{\bar{\rho}} \Omega_u^c) (D_{\bar{\nu}} \Omega_{u,b}^* \Omega_u^a) \varepsilon^{\bar{\mu}\bar{\nu}\bar{\rho}\bar{\sigma}} (\bar{d}_{cs} \gamma^{\bar{\sigma}} d_r^b) \right] \\
& + \frac{i}{12}(\mathcal{C}_{ud}^{(8)})^{ttsr} \left[ (\Omega_{u,a}^* D_{\bar{\nu}} \Omega_u^c) (\Omega_{u,b}^* D_{\bar{\mu}} \Omega_u^a) (D^{\bar{\mu}} \bar{d}_{cs} \gamma^{\bar{\nu}} d_r^b) - (D_{\bar{\mu}} \Omega_{u,a}^* \Omega_u^c) (D_{\bar{\nu}} \Omega_{u,b}^* \Omega_u^a) (\bar{d}_{cs} \gamma^{\bar{\nu}} D^{\bar{\mu}} d_r^b) \right] \\
& + \frac{i}{12}(\mathcal{C}_{ud}^{(8)})^{ttsr} \left[ (\Omega_{u,a}^* D_{\bar{\mu}} \Omega_u^c) (\Omega_{u,b}^* D_{\bar{\nu}} \Omega_u^a) (\bar{d}_{cs} \gamma^{\bar{\mu}} D^{\bar{\nu}} d_r^b) - (D_{\bar{\mu}} \Omega_{u,a}^* \Omega_u^c) (D_{\bar{\nu}} \Omega_{u,b}^* \Omega_u^a) (D^{\bar{\mu}} \bar{d}_{cs} \gamma^{\bar{\nu}} d_r^b) \right] \\
& + \frac{i}{12}(\mathcal{C}_{ud}^{(8)})^{srtt} \left[ (\Omega_{d,a}^* D_2 D_{\bar{\mu}} \Omega_d^b) (\bar{u}_{bs} \gamma^{\bar{\mu}} u_r^a) - (D_2 D_{\bar{\nu}} \Omega_{d,a}^* \Omega_d^b) (\bar{u}_{bs} \gamma^{\bar{\nu}} u_r^a) \right] \\
& - \frac{i}{12}(\mathcal{C}_{ud}^{(8)})^{srtt} \left[ (D_{\bar{\mu}} D_{\bar{\nu}} \Omega_{d,a}^* \Omega_d^c) (\Omega_{d,b}^* D_{\bar{\mu}} \Omega_d^a) (\bar{u}_{cs} \gamma^{\bar{\nu}} u_r^b) - (D_{\bar{\mu}} \Omega_{d,a}^* \Omega_d^c) (\Omega_{d,b}^* D_{\bar{\mu}} D_{\bar{\nu}} \Omega_d^a) (\bar{u}_{cs} \gamma^{\bar{\nu}} u_r^b) \right] \\
& + \frac{i}{12}(\mathcal{C}_{ud}^{(8)})^{srtt} \left[ (\Omega_{d,a}^* D_{\bar{\nu}} \Omega_d^c) (D_{\bar{\mu}} \Omega_{d,b}^* D_{\bar{\nu}} \Omega_d^a) (\bar{u}_{cs} \gamma^{\bar{\mu}} u_r^b) - (D_{\bar{\mu}} \Omega_{d,a}^* D_{\bar{\nu}} \Omega_d^c) (D_{\bar{\mu}} \Omega_{d,b}^* \Omega_d^a) (\bar{u}_{cs} \gamma^{\bar{\nu}} u_r^b) \right] \\
& + \frac{1}{12}(\mathcal{C}_{ud}^{(8)})^{srtt} \left[ (\Omega_{d,a}^* D_{\bar{\rho}} \Omega_d^c) (D_{\bar{\mu}} \Omega_{d,b}^* D_{\bar{\sigma}} \Omega_d^a) \varepsilon^{\bar{\mu}\bar{\nu}\bar{\rho}\bar{\sigma}} (\bar{u}_{cs} \gamma^{\bar{\nu}} u_r^b) - (D_{\bar{\mu}} \Omega_{d,a}^* D_{\bar{\rho}} \Omega_d^c) (D_{\bar{\nu}} \Omega_{d,b}^* \Omega_d^a) \varepsilon^{\bar{\mu}\bar{\nu}\bar{\rho}\bar{\sigma}} (\bar{u}_{cs} \gamma^{\bar{\sigma}} u_r^b) \right] \\
& + \frac{i}{12}(\mathcal{C}_{ud}^{(8)})^{srtt} \left[ (\Omega_{d,a}^* D_{\bar{\nu}} \Omega_d^c) (\Omega_{d,b}^* D_{\bar{\mu}} \Omega_d^a) (D^{\bar{\mu}} \bar{u}_{cs} \gamma^{\bar{\nu}} u_r^b) - (D_{\bar{\mu}} \Omega_{d,a}^* \Omega_d^c) (D_{\bar{\nu}} \Omega_{d,b}^* \Omega_d^a) (\bar{u}_{cs} \gamma^{\bar{\nu}} D^{\bar{\mu}} u_r^b) \right] \\
& + \frac{i}{12}(\mathcal{C}_{ud}^{(8)})^{srtt} \left[ (\Omega_{d,a}^* D_{\bar{\mu}} \Omega_d^c) (\Omega_{d,b}^* D_{\bar{\nu}} \Omega_d^a) (\bar{u}_{cs} \gamma^{\bar{\mu}} D^{\bar{\nu}} u_r^b) - (D_{\bar{\mu}} \Omega_{d,a}^* \Omega_d^c) (D_{\bar{\nu}} \Omega_{d,b}^* \Omega_d^a) (D^{\bar{\mu}} \bar{u}_{cs} \gamma^{\bar{\nu}} u_r^b) \right] \\
& - \frac{i}{12} y_u^{tv} \bar{y}_u^{tu} (\mathcal{C}_{ud}^{(8)})^{vusr} (\Omega_{q,a}^* \overleftrightarrow{D}_{\bar{\mu}} \Omega_q^b) (H^\dagger H) (\bar{d}_{bs} \gamma^{\bar{\mu}} d_r^a) + \frac{i}{12} y_u^{tv} \bar{y}_u^{tu} (\mathcal{C}_{ud}^{(8)})^{vusr} (\Omega_{q,a,j}^* \overleftrightarrow{D}_{\bar{\mu}} \Omega_q^{bi}) H_i^\dagger H^j (\bar{d}_{bs} \gamma^{\bar{\mu}} d_r^a) \\
& - \frac{i}{12} y_d^{tv} \bar{y}_d^{tu} (\mathcal{C}_{ud}^{(8)})^{srvu} (\Omega_{q,a,j}^* \overleftrightarrow{D}_{\bar{\mu}} \Omega_q^{bi}) H_i^\dagger H^j (\bar{u}_{bs} \gamma^{\bar{\mu}} u_r^a) \\
& + \frac{i}{9} g_Y (\mathcal{C}_{ud}^{(8)})^{ttsr} \left[ 2(\Omega_{u,a}^* D_{\bar{\sigma}} \Omega_u^b) \tilde{B}^{\bar{\rho}\bar{\sigma}} (\bar{d}_{bs} \gamma^{\bar{\rho}} d_r^a) + 2(D_{\bar{\mu}} \Omega_{u,a}^* \Omega_u^b) \tilde{B}^{\bar{\mu}\bar{\sigma}} (\bar{d}_{bs} \gamma^{\bar{\sigma}} d_r^a) \right] \\
& - \frac{i}{9} y_d^{tv} \bar{y}_d^{tu} (\mathcal{C}_{ud}^{(8)})^{srvu} (\Omega_d^\dagger \overleftrightarrow{D}_{\bar{\mu}} \Omega_d) (H^\dagger H) (\bar{u}_s \gamma^{\bar{\mu}} u_r) - \frac{i}{9} y_u^{tv} \bar{y}_u^{tu} (\mathcal{C}_{ud}^{(8)})^{vusr} (\Omega_u^\dagger \overleftrightarrow{D}_{\bar{\mu}} \Omega_u) (H^\dagger H) (\bar{d}_s \gamma^{\bar{\mu}} d_r) \\
& + \frac{i}{6} y_u^{rt} \bar{y}_u^{rs} (\mathcal{C}_{ud}^{(8)})^{tuv s} (D_{\bar{\mu}} \Omega_{q,k}^* \Omega_q^j) H_j^\dagger \tilde{H}_k (\bar{d}_v \gamma^{\bar{\mu}} u_u) \\
& + \frac{i}{6} (\mathcal{C}_{ud}^{(8)})^{ttsr} \left[ (\Omega_{u,a}^* D_{\bar{\nu}} \Omega_u^b) (D^{\bar{\mu}} \bar{d}_{bs} \gamma^{\bar{\nu}} D^{\bar{\mu}} d_r^a) - (D_{\bar{\mu}} \Omega_{u,a}^* \Omega_u^b) (D^{\bar{\nu}} \bar{d}_{bs} \gamma^{\bar{\mu}} D^{\bar{\nu}} d_r^a) \right] \\
& + \frac{i}{6} (\mathcal{C}_{ud}^{(8)})^{ttsr} \left[ (\Omega_{u,a}^* D_{\bar{\nu}} \Omega_u^b) (D^{\bar{\mu}} D^{\bar{\mu}} \bar{d}_{bs} \gamma^{\bar{\nu}} d_r^a) - (D_{\bar{\mu}} \Omega_{u,a}^* \Omega_u^b) (\bar{d}_{bs} \gamma^{\bar{\mu}} D^{\bar{\nu}} D^{\bar{\nu}} d_r^a) \right] \\
& - \frac{i}{6} (\mathcal{C}_{ud}^{(8)})^{ttsr} \left[ (\Omega_{u,a}^* D_{\bar{\mu}} \Omega_u^c) (D_{\bar{\mu}} \Omega_{u,b}^* D_{\bar{\nu}} \Omega_u^a) (\bar{d}_{cs} \gamma^{\bar{\nu}} d_r^b) - (D_{\bar{\mu}} \Omega_{u,a}^* D_{\bar{\nu}} \Omega_u^c) (D_{\bar{\nu}} \Omega_{u,b}^* \Omega_u^a) (\bar{d}_{cs} \gamma^{\bar{\mu}} d_r^b) \right] \\
& - \frac{i}{6} g_s (\mathcal{C}_{ud}^{(8)})^{ttsr} \left[ 2T_b^{Aa} (\Omega_{u,a}^* D_{\bar{\rho}} \Omega_u^c) \tilde{G}^{\bar{\rho}\bar{\sigma} A} (\bar{d}_{cs} \gamma^{\bar{\sigma}} d_r^b) - 2T_c^{Ab} (D_{\bar{\mu}} \Omega_{u,a}^* \Omega_u^c) \tilde{G}^{\bar{\mu}\bar{\sigma} A} (\bar{d}_{bs} \gamma^{\bar{\sigma}} d_r^a) \right] \\
& - \frac{i}{6} y_d^{ru} \bar{y}_u^{rs} (\mathcal{C}_{ud}^{(8)})^{tsuv} (\Omega_{q,i}^* D_{\bar{\mu}} \Omega_q^j) \tilde{H}^{\dagger j} H^i (\bar{u}_t \gamma^{\bar{\mu}} d_v) \\
& + \frac{i}{6} (\mathcal{C}_{ud}^{(8)})^{srtt} \left[ (\Omega_{d,a}^* D_{\bar{\nu}} \Omega_d^b) (D^{\bar{\mu}} \bar{u}_{bs} \gamma^{\bar{\nu}} D^{\bar{\mu}} u_r^a) - (D_{\bar{\mu}} \Omega_{d,a}^* \Omega_d^b) (D^{\bar{\nu}} \bar{u}_{bs} \gamma^{\bar{\mu}} D^{\bar{\nu}} u_r^a) \right]
\end{aligned}$$

$$\begin{aligned}
& + \frac{i}{6} (\mathcal{C}_{ud}^{(8)})^{srtt} \left[ (\Omega_{d,a}^* D_{\bar{\nu}} \Omega_d^b) (D^{\bar{\mu}} D^{\bar{\mu}} \bar{u}_{bs} \gamma^{\bar{\nu}} u_r^a) - (D_{\bar{\mu}} \Omega_{d,a}^* \Omega_d^b) (\bar{u}_{bs} \gamma^{\bar{\mu}} D^{\bar{\nu}} D^{\bar{\nu}} u_r^a) \right] \\
& - \frac{i}{6} (\mathcal{C}_{ud}^{(8)})^{srtt} \left[ (\Omega_{d,a}^* D_{\bar{\mu}} \Omega_d^c) (D_{\bar{\mu}} \Omega_{d,b}^* D_{\bar{\nu}} \Omega_d^a) (\bar{u}_{cs} \gamma^{\bar{\nu}} u_r^b) - (D_{\bar{\mu}} \Omega_{d,a}^* D_{\bar{\nu}} \Omega_d^c) (D_{\bar{\nu}} \Omega_{d,b}^* \Omega_d^a) (\bar{u}_{cs} \gamma^{\bar{\mu}} u_r^b) \right] \\
& - \frac{i}{6} (\mathcal{C}_{ud}^{(8)})^{srtt} \left[ 2T_b^{Aa} (\Omega_{d,a}^* D_{\bar{\rho}} \Omega_d^c) \tilde{G}^{\bar{\rho}\bar{\sigma}A} (\bar{u}_{cs} \gamma^{\bar{\sigma}} u_r^b) - 2T_c^{Ab} (D_{\bar{\mu}} \Omega_{d,a}^* \Omega_d^c) \tilde{G}^{\bar{\mu}\bar{\sigma}A} (\bar{u}_{bs} \gamma^{\bar{\sigma}} u_r^a) \right] \\
& + \frac{i}{3} y_d^{tv} \bar{y}_d^{tu} (\mathcal{C}_{ud}^{(8)})^{srvu} (\Omega_{d,a}^* \overset{\leftrightarrow}{D}_{\bar{\mu}} \Omega_d^b) (H^\dagger H) (\bar{u}_{bs} \gamma^{\bar{\mu}} u_r^a) + \frac{i}{3} y_u^{tv} \bar{y}_u^{tu} (\mathcal{C}_{ud}^{(8)})^{vusr} (\Omega_{u,a}^* \overset{\leftrightarrow}{D}_{\bar{\mu}} \Omega_u^b) (H^\dagger H) (\bar{d}_{bs} \gamma^{\bar{\mu}} d_r^a) \\
& - \frac{1}{2} g_s (\mathcal{C}_{ud}^{(8)})^{ttsr} \left[ T_b^{Aa} (\Omega_{u,a}^* D_{\bar{\nu}} \Omega_u^c) G^{\bar{\mu}\bar{\nu}A} (\bar{d}_{cs} \gamma^{\bar{\mu}} d_r^b) - T_c^{Ab} (D_{\bar{\mu}} \Omega_{u,a}^* \Omega_u^c) G^{\bar{\mu}\bar{\nu}A} (\bar{d}_{bs} \gamma^{\bar{\nu}} d_r^a) \right] \\
& - \frac{1}{2} g_s (\mathcal{C}_{ud}^{(8)})^{srtt} \left[ T_b^{Aa} (\Omega_{d,a}^* D_{\bar{\nu}} \Omega_d^c) G^{\bar{\mu}\bar{\nu}A} (\bar{u}_{cs} \gamma^{\bar{\mu}} u_r^b) - T_c^{Ab} (D_{\bar{\mu}} \Omega_{d,a}^* \Omega_d^c) G^{\bar{\mu}\bar{\nu}A} (\bar{u}_{bs} \gamma^{\bar{\nu}} u_r^a) \right], \tag{3.53}
\end{aligned}$$

$$\begin{aligned}
\Gamma_\Omega^{(1)} [\mathcal{O}_{qu}^{(1)}] = & -\frac{i}{18} g_Y (\mathcal{C}_{qu}^{(1)})^{ttsr} \left[ 2(\Omega_q^\dagger D_{\bar{\sigma}} \Omega_q) \tilde{B}^{\bar{\rho}\bar{\sigma}} (\bar{u}_s \gamma^{\bar{\rho}} u_r) + 2(D_{\bar{\mu}} \Omega_q^\dagger \Omega_q) \tilde{B}^{\bar{\mu}\bar{\sigma}} (\bar{u}_s \gamma^{\bar{\sigma}} u_r) \right] \\
& + \frac{i}{6} (\mathcal{C}_{qu}^{(1)})^{srtt} \left[ (\Omega_u^\dagger D_2 D_{\bar{\mu}} \Omega_u) (\bar{q}_s \gamma^{\bar{\mu}} q_r) - (D_2 D_{\bar{\nu}} \Omega_u^\dagger \Omega_u) (\bar{q}_s \gamma^{\bar{\nu}} q_r) \right] \\
& + \frac{1}{6} (\mathcal{C}_{qu}^{(1)})^{ttsr} \left[ (D_{\bar{\mu}} \Omega_{q,ai}^* D_{\bar{\rho}} \Omega_q^{bj}) (\Omega_{q,bj}^* D_{\bar{\sigma}} \Omega_q^{ai}) \varepsilon^{\bar{\mu}\bar{\nu}\bar{\rho}\bar{\sigma}} (\bar{u}_s \gamma^{\bar{\nu}} u_r) - (D_{\bar{\mu}} \Omega_{q,ai}^* \Omega_q^{bj}) (D_{\bar{\nu}} \Omega_{q,bj}^* D_{\bar{\rho}} \Omega_q^{ai}) \varepsilon^{\bar{\mu}\bar{\nu}\bar{\rho}\bar{\sigma}} (\bar{u}_s \gamma^{\bar{\sigma}} u_r) \right] \\
& - \frac{1}{6} (\mathcal{C}_{qu}^{(1)})^{srtt} \left[ (D_{\bar{\mu}} \Omega_{u,a}^* D_{\bar{\rho}} \Omega_u^b) (\Omega_{u,b}^* D_{\bar{\sigma}} \Omega_u^a) \varepsilon^{\bar{\mu}\bar{\nu}\bar{\rho}\bar{\sigma}} (\bar{q}_s \gamma^{\bar{\nu}} q_r) - (D_{\bar{\mu}} \Omega_{u,a}^* \Omega_u^b) (D_{\bar{\nu}} \Omega_{u,b}^* D_{\bar{\rho}} \Omega_u^a) \varepsilon^{\bar{\mu}\bar{\nu}\bar{\rho}\bar{\sigma}} (\bar{q}_s \gamma^{\bar{\sigma}} q_r) \right] \\
& + \frac{i}{6} (\mathcal{C}_{qu}^{(1)})^{ttsr} \left[ (\Omega_q^\dagger D_2 D_{\bar{\mu}} \Omega_q) (\bar{u}_s \gamma^{\bar{\mu}} u_r) - (D_2 D_{\bar{\nu}} \Omega_q^\dagger \Omega_q) (\bar{u}_s \gamma^{\bar{\nu}} u_r) \right] \\
& - \frac{i}{6} y_d^{vu} \bar{y}_d^{tu} (\mathcal{C}_{qu}^{(1)})^{tv sr} (\Omega_d^\dagger \overset{\leftrightarrow}{D}_{\bar{\mu}} \Omega_d) (H^\dagger H) (\bar{u}_s \gamma^{\bar{\mu}} u_r) - \frac{i}{6} y_u^{tv} \bar{y}_u^{tu} (\mathcal{C}_{qu}^{(1)})^{srvu} (\Omega_q^\dagger \overset{\leftrightarrow}{D}_{\bar{\mu}} \Omega_q) (H^\dagger H) (\bar{q}_s \gamma^{\bar{\mu}} q_r) \\
& + \frac{i}{6} y_u^{tv} \bar{y}_u^{tu} (\mathcal{C}_{qu}^{(1)})^{srvu} (\Omega_{q,j}^* \overset{\leftrightarrow}{D}_{\bar{\mu}} \Omega_q^i) H_i^\dagger H^j (\bar{q}_s \gamma^{\bar{\mu}} q_r) - \frac{i}{6} y_u^{vu} \bar{y}_u^{tu} (\mathcal{C}_{qu}^{(1)})^{tv sr} (\Omega_u^\dagger \overset{\leftrightarrow}{D}_{\bar{\mu}} \Omega_u) (H^\dagger H) (\bar{u}_s \gamma^{\bar{\mu}} u_r) \\
& + \frac{2i}{9} g_Y (\mathcal{C}_{qu}^{(1)})^{srtt} \left[ 2(\Omega_u^\dagger D_{\bar{\sigma}} \Omega_u) \tilde{B}^{\bar{\rho}\bar{\sigma}} (\bar{q}_s \gamma^{\bar{\rho}} q_r) + 2(D_{\bar{\mu}} \Omega_u^\dagger \Omega_u) \tilde{B}^{\bar{\mu}\bar{\sigma}} (\bar{q}_s \gamma^{\bar{\sigma}} q_r) \right] \\
& + \frac{i}{3} g_s (\mathcal{C}_{qu}^{(1)})^{srtt} \left[ 2T_b^{Aa} (\Omega_{u,a}^* D_{\bar{\sigma}} \Omega_u^b) \tilde{G}^{\bar{\rho}\bar{\sigma}A} (\bar{q}_s \gamma^{\bar{\rho}} q_r) + 2T_b^{Aa} (D_{\bar{\mu}} \Omega_{u,a}^* \Omega_u^b) \tilde{G}^{\bar{\mu}\bar{\sigma}A} (\bar{q}_s \gamma^{\bar{\sigma}} q_r) \right] \\
& + \frac{i}{3} (\mathcal{C}_{qu}^{(1)})^{srtt} \left[ (\Omega_u^\dagger D_{\bar{\nu}} \Omega_u) (D^{\bar{\mu}} \bar{q}_s \gamma^{\bar{\nu}} D^{\bar{\mu}} q_r) - (D_{\bar{\mu}} \Omega_u^\dagger \Omega_u) (D^{\bar{\nu}} \bar{q}_s \gamma^{\bar{\mu}} D^{\bar{\nu}} q_r) \right] \\
& + \frac{i}{3} (\mathcal{C}_{qu}^{(1)})^{srtt} \left[ (\Omega_u^\dagger D_{\bar{\nu}} \Omega_u) (D^{\bar{\mu}} D^{\bar{\mu}} \bar{q}_s \gamma^{\bar{\nu}} q_r) - (D_{\bar{\mu}} \Omega_u^\dagger \Omega_u) (\bar{q}_s \gamma^{\bar{\mu}} D^{\bar{\nu}} D^{\bar{\nu}} q_r) \right] \\
& - \frac{i}{3} g_s (\mathcal{C}_{qu}^{(1)})^{ttsr} \left[ 2T_b^{Aa} (\Omega_{q,a}^* D_{\bar{\sigma}} \Omega_q^b) \tilde{G}^{\bar{\rho}\bar{\sigma}A} (\bar{u}_s \gamma^{\bar{\rho}} u_r) + 2T_b^{Aa} (D_{\bar{\mu}} \Omega_{q,a}^* \Omega_q^b) \tilde{G}^{\bar{\mu}\bar{\sigma}A} (\bar{u}_s \gamma^{\bar{\sigma}} u_r) \right] \\
& - \frac{i}{3} g_L (\mathcal{C}_{qu}^{(1)})^{ttsr} \left[ 2t_j^{Ii} (\Omega_{q,i}^* D_{\bar{\sigma}} \Omega_q^j) \tilde{W}^{\bar{\rho}\bar{\sigma}I} (\bar{u}_s \gamma^{\bar{\rho}} u_r) + 2t_j^{Ii} (D_{\bar{\mu}} \Omega_{q,i}^* \Omega_q^j) \tilde{W}^{\bar{\mu}\bar{\sigma}I} (\bar{u}_s \gamma^{\bar{\sigma}} u_r) \right] \\
& + \frac{i}{3} (\mathcal{C}_{qu}^{(1)})^{ttsr} \left[ (\Omega_q^\dagger D_{\bar{\nu}} \Omega_q) (D^{\bar{\mu}} \bar{u}_s \gamma^{\bar{\nu}} D^{\bar{\mu}} u_r) - (D_{\bar{\mu}} \Omega_q^\dagger \Omega_q) (D^{\bar{\nu}} \bar{u}_s \gamma^{\bar{\mu}} D^{\bar{\nu}} u_r) \right] \\
& + \frac{i}{3} (\mathcal{C}_{qu}^{(1)})^{ttsr} \left[ (\Omega_q^\dagger D_{\bar{\nu}} \Omega_q) (D^{\bar{\mu}} D^{\bar{\mu}} \bar{u}_s \gamma^{\bar{\nu}} u_r) - (D_{\bar{\mu}} \Omega_q^\dagger \Omega_q) (\bar{u}_s \gamma^{\bar{\mu}} D^{\bar{\nu}} D^{\bar{\nu}} u_r) \right] \\
& + \frac{2}{3} y_u^{st} (\mathcal{C}_{qu}^{(1)})^{rstu} (D_{\bar{\mu}} \Omega_{u,a}^* D_{\bar{\mu}} \Omega_u^b) (\bar{q}_{br} \tilde{H} u_u^a) + \frac{2}{3} y_u^{st} (\mathcal{C}_{qu}^{(1)})^{rstu} (D_{\bar{\mu}} \Omega_{q,a}^* \Omega_q^b) (\bar{q}_{br} \tilde{H} D^{\bar{\mu}} u_u^a) \\
& + \frac{2}{3} y_u^{st} (\mathcal{C}_{qu}^{(1)})^{rstu} (D_{\bar{\mu}} \Omega_{u,a}^* \Omega_u^b) (\bar{q}_{br} \tilde{H} D^{\bar{\mu}} u_u^a) + \frac{2}{3} y_u^{st} (\mathcal{C}_{qu}^{(1)})^{rstu} (D_{\bar{\mu}} \Omega_{q,a}^* \Omega_q^b) (D^{\bar{\mu}} \bar{q}_{br} \tilde{H} u_u^a)
\end{aligned}$$

$$\begin{aligned}
& + \frac{2}{3} y_u^{st} (\mathcal{C}_{qu}^{(1)})^{rstu} (D_{\bar{\mu}} \Omega_{u,a}^* \Omega_u^b) (D_{\bar{\mu}} \bar{q}_{br} \tilde{H} u_u^a) + \frac{2}{3} y_u^{st} (\mathcal{C}_{qu}^{(1)})^{rstu} (D_{\bar{\mu}} \Omega_{q,a}^* \Omega_q^c) (D_{\bar{\mu}} \Omega_{u,b}^* \Omega_u^a) (\bar{q}_{cr} \tilde{H} u_u^b) \\
& + \frac{2}{3} y_u^{st} (\mathcal{C}_{qu}^{(1)})^{rstu} \varepsilon^{kj} (D_{\bar{\mu}} \Omega_{q,aj}^* \Omega_q^{bi}) H_i^\dagger (\bar{q}_{bkr} D_{\bar{\mu}} u_u^a) + \frac{2}{3} y_u^{st} (\mathcal{C}_{qu}^{(1)})^{rstu} \varepsilon^{kj} (D_{\bar{\mu}} \Omega_{q,aj}^* \Omega_q^{bi}) H_i^\dagger (D_{\bar{\mu}} \bar{q}_{bkr} u_u^a) \\
& + \frac{2}{3} y_u^{st} (\mathcal{C}_{qu}^{(1)})^{rstu} \varepsilon^{kj} (D_{\bar{\mu}} \Omega_{q,aj}^* \Omega_q^{ci}) (D_{\bar{\mu}} \Omega_{u,b}^* \Omega_u^a) H_i^\dagger (\bar{q}_{ckr} u_u^b) + \frac{2}{3} \bar{y}_u^{rs} (\mathcal{C}_{qu}^{(1)})^{rtus} \bar{\varepsilon}_{jk} (\Omega_{q,ai}^* D_{\bar{\mu}} \Omega_q^{bk}) H^i (\bar{u}_{bu} D_{\bar{\mu}} q_t^{aj}) \\
& + \frac{2}{3} \bar{y}_u^{rs} (\mathcal{C}_{qu}^{(1)})^{rtus} (D_{\bar{\mu}} \Omega_{u,a}^* D_{\bar{\mu}} \Omega_u^b) (\bar{u}_{bu} \tilde{H}^\dagger q_t^a) + \frac{2}{3} \bar{y}_u^{rs} (\mathcal{C}_{qu}^{(1)})^{rtus} (\Omega_{q,a}^* D_{\bar{\mu}} \Omega_q^b) (\bar{u}_{bu} \tilde{H}^\dagger D_{\bar{\mu}} q_t^a) \\
& + \frac{2}{3} \bar{y}_u^{rs} (\mathcal{C}_{qu}^{(1)})^{rtus} (\Omega_{u,a}^* D_{\bar{\mu}} \Omega_u^b) (\bar{u}_{bu} \tilde{H}^\dagger D_{\bar{\mu}} q_t^a) + \frac{2}{3} \bar{y}_u^{rs} (\mathcal{C}_{qu}^{(1)})^{rtus} \bar{\varepsilon}_{jk} (\Omega_{q,ai}^* D_{\bar{\mu}} \Omega_q^{bk}) H^i (D_{\bar{\mu}} \bar{u}_{bu} q_t^{aj}) \\
& + \frac{2}{3} \bar{y}_u^{rs} (\mathcal{C}_{qu}^{(1)})^{rtus} (\Omega_{q,a}^* D_{\bar{\mu}} \Omega_q^b) (D_{\bar{\mu}} \bar{u}_{bu} \tilde{H}^\dagger q_t^a) + \frac{2}{3} \bar{y}_u^{rs} (\mathcal{C}_{qu}^{(1)})^{rtus} (\Omega_{u,a}^* D_{\bar{\mu}} \Omega_u^b) (D_{\bar{\mu}} \bar{u}_{bu} \tilde{H}^\dagger q_t^a) \\
& + \frac{2}{3} \bar{y}_u^{rs} (\mathcal{C}_{qu}^{(1)})^{rtus} \bar{\varepsilon}_{jk} (\Omega_{q,ai}^* D_{\bar{\mu}} \Omega_q^{bk}) (\Omega_{u,b}^* D_{\bar{\mu}} \Omega_u^c) H^i (\bar{u}_{cu} q_t^{aj}) + \frac{2}{3} \bar{y}_u^{rs} (\mathcal{C}_{qu}^{(1)})^{rtus} (\Omega_{q,a}^* D_{\bar{\mu}} \Omega_q^b) (\Omega_{u,b}^* D_{\bar{\mu}} \Omega_u^c) (\bar{u}_{cu} \tilde{H}^\dagger q_t^a) \\
& - \frac{2}{3} y_u^{st} (\mathcal{C}_{qu}^{(1)})^{rstu} (D_{\bar{\mu}} \Omega_{q,a}^* D_{\bar{\mu}} \Omega_q^b) (\bar{q}_{br} \tilde{H} u_u^a) - \frac{2}{3} y_u^{st} (\mathcal{C}_{qu}^{(1)})^{rstu} (D_{\bar{\mu}} \Omega_{q,a}^* \Omega_q^b) (\bar{q}_{br} D_{\bar{\mu}} \tilde{H} u_u^a) \\
& - \frac{2}{3} y_u^{st} (\mathcal{C}_{qu}^{(1)})^{rstu} (D_{\bar{\mu}} \Omega_{u,a}^* \Omega_u^b) (\bar{q}_{br} D_{\bar{\mu}} \tilde{H} u_u^a) - \frac{2}{3} y_u^{st} (\mathcal{C}_{qu}^{(1)})^{rstu} \varepsilon^{kj} (D_{\bar{\mu}} \Omega_{q,aj}^* \Omega_q^{bi}) D_{\bar{\mu}} H_i^\dagger (\bar{q}_{bkr} u_u^a) \\
& - \frac{2}{3} y_u^{st} (\mathcal{C}_{qu}^{(1)})^{rstu} \varepsilon^{kj} (D_{\bar{\mu}} \Omega_{q,aj}^* D_{\bar{\mu}} \Omega_q^{bi}) H_i^\dagger (\bar{q}_{bkr} u_u^a) - \frac{2}{3} \bar{y}_u^{rs} (\mathcal{C}_{qu}^{(1)})^{rtus} \bar{\varepsilon}_{jk} (D_{\bar{\mu}} \Omega_{q,ai}^* D_{\bar{\mu}} \Omega_q^{bk}) H^i (\bar{u}_{bu} q_t^{aj}) \\
& - \frac{2}{3} \bar{y}_u^{rs} (\mathcal{C}_{qu}^{(1)})^{rtus} \bar{\varepsilon}_{jk} (\Omega_{q,ai}^* D_{\bar{\mu}} \Omega_q^{bk}) D_{\bar{\mu}} H^i (\bar{u}_{bu} q_t^{aj}) - \frac{2}{3} \bar{y}_u^{rs} (\mathcal{C}_{qu}^{(1)})^{rtus} (D_{\bar{\mu}} \Omega_{q,a}^* D_{\bar{\mu}} \Omega_q^b) (\bar{u}_{bu} \tilde{H}^\dagger q_t^a) \\
& - \frac{2}{3} \bar{y}_u^{rs} (\mathcal{C}_{qu}^{(1)})^{rtus} (\Omega_{q,a}^* D_{\bar{\mu}} \Omega_q^b) (\bar{u}_{bu} D_{\bar{\mu}} \tilde{H}^\dagger q_t^a) - \frac{2}{3} \bar{y}_u^{rs} (\mathcal{C}_{qu}^{(1)})^{rtus} (\Omega_{u,a}^* D_{\bar{\mu}} \Omega_u^b) (\bar{u}_{bu} D_{\bar{\mu}} \tilde{H}^\dagger q_t^a) \\
& + \frac{2i}{3} y_u^{vu} \bar{y}_u^{tu} (\mathcal{C}_{qu}^{(1)})^{tvsr} (\Omega_q^\dagger \overset{\leftrightarrow}{D}_{\bar{\mu}} \Omega_q) (H^\dagger H) (\bar{u}_s \gamma^{\bar{\mu}} u_r) \\
& + \frac{2i}{3} (\mathcal{C}_{qu}^{(1)})^{tvsr} \left[ y_d^{vu} \bar{y}_d^{tu} - y_u^{vu} \bar{y}_u^{tu} \right] (\Omega_{q,j}^* \overset{\leftrightarrow}{D}_{\bar{\mu}} \Omega_q^i) H_i^\dagger H^j (\bar{u}_s \gamma^{\bar{\mu}} u_r) \\
& + \frac{2i}{3} y_u^{tv} \bar{y}_u^{tu} (\mathcal{C}_{qu}^{(1)})^{srvu} (\Omega_u^\dagger \overset{\leftrightarrow}{D}_{\bar{\mu}} \Omega_u) (H^\dagger H) (\bar{q}_s \gamma^{\bar{\mu}} q_r), \tag{3.54}
\end{aligned}$$

$$\begin{aligned}
\Gamma_\Omega^{(1)} [\mathcal{O}_{qu}^{(8)}] &= \frac{i}{108} g_Y (\mathcal{C}_{qu}^{(8)})^{ttsr} \left[ 2(\Omega_q^\dagger D_{\bar{\sigma}} \Omega_q) \tilde{B}^{\bar{\rho}\bar{\sigma}} (\bar{u}_s \gamma^{\bar{\rho}} u_r) + 2(D_{\bar{\mu}} \Omega_q^\dagger \Omega_q) \tilde{B}^{\bar{\mu}\bar{\sigma}} (\bar{u}_s \gamma^{\bar{\sigma}} u_r) \right] \\
& - \frac{i}{36} (\mathcal{C}_{qu}^{(8)})^{srtt} \left[ (\Omega_u^\dagger D_2 D_{\bar{\mu}} \Omega_u) (\bar{q}_s \gamma^{\bar{\mu}} q_r) - (D_2 D_{\bar{\nu}} \Omega_u^\dagger \Omega_u) (\bar{q}_s \gamma^{\bar{\nu}} q_r) \right] \\
& + \frac{1}{36} (\mathcal{C}_{qu}^{(8)})^{srtt} \left[ (D_{\bar{\mu}} \Omega_{u,a}^* D_{\bar{\rho}} \Omega_u^b) (\Omega_{u,b}^* D_{\bar{\sigma}} \Omega_u^a) \varepsilon^{\bar{\mu}\bar{\nu}\bar{\rho}\bar{\sigma}} (\bar{q}_s \gamma^{\bar{\nu}} q_r) - (D_{\bar{\mu}} \Omega_{u,a}^* \Omega_u^b) (D_{\bar{\nu}} \Omega_{u,b}^* D_{\bar{\rho}} \Omega_u^a) \varepsilon^{\bar{\mu}\bar{\nu}\bar{\rho}\bar{\sigma}} (\bar{q}_s \gamma^{\bar{\sigma}} q_r) \right] \\
& - \frac{i}{36} (\mathcal{C}_{qu}^{(8)})^{ttsr} \left[ (\Omega_q^\dagger D_2 D_{\bar{\mu}} \Omega_q) (\bar{u}_s \gamma^{\bar{\mu}} u_r) - (D_2 D_{\bar{\nu}} \Omega_q^\dagger \Omega_q) (\bar{u}_s \gamma^{\bar{\nu}} u_r) \right] \\
& - \frac{1}{36} (\mathcal{C}_{qu}^{(8)})^{ttsr} \left[ (D_{\bar{\mu}} \Omega_{q,ai}^* D_{\bar{\rho}} \Omega_q^{bj}) (\Omega_{q,bj}^* D_{\bar{\sigma}} \Omega_q^{ai}) \varepsilon^{\bar{\mu}\bar{\nu}\bar{\rho}\bar{\sigma}} (\bar{u}_s \gamma^{\bar{\nu}} u_r) - (D_{\bar{\mu}} \Omega_{q,ai}^* \Omega_q^{bj}) (D_{\bar{\nu}} \Omega_{q,bj}^* D_{\bar{\rho}} \Omega_q^{ai}) \varepsilon^{\bar{\mu}\bar{\nu}\bar{\rho}\bar{\sigma}} (\bar{u}_s \gamma^{\bar{\sigma}} u_r) \right] \\
& + \frac{i}{36} g_Y (\mathcal{C}_{qu}^{(8)})^{ttsr} \left[ 2(\Omega_{q,a}^* D_{\bar{\rho}} \Omega_q^b) \tilde{B}^{\bar{\rho}\bar{\sigma}} (\bar{u}_{bs} \gamma^{\bar{\sigma}} u_r^a) - 2(D_{\bar{\mu}} \Omega_{q,a}^* \Omega_q^b) \tilde{B}^{\bar{\mu}\bar{\sigma}} (\bar{u}_{bs} \gamma^{\bar{\sigma}} u_r^a) \right] \\
& + \frac{i}{36} y_d^{vu} \bar{y}_d^{tu} (\mathcal{C}_{qu}^{(8)})^{tvsr} (\Omega_d^\dagger \overset{\leftrightarrow}{D}_{\bar{\mu}} \Omega_d) (H^\dagger H) (\bar{u}_s \gamma^{\bar{\mu}} u_r) + \frac{i}{36} y_u^{tv} \bar{y}_u^{tu} (\mathcal{C}_{qu}^{(8)})^{srvu} (\Omega_q^\dagger \overset{\leftrightarrow}{D}_{\bar{\mu}} \Omega_q) (H^\dagger H) (\bar{q}_s \gamma^{\bar{\mu}} q_r) \\
& - \frac{i}{36} y_u^{tv} \bar{y}_u^{tu} (\mathcal{C}_{qu}^{(8)})^{srvu} (\Omega_{q,j}^* \overset{\leftrightarrow}{D}_{\bar{\mu}} \Omega_q^i) H_i^\dagger H^j (\bar{q}_s \gamma^{\bar{\mu}} q_r) + \frac{i}{36} y_u^{vu} \bar{y}_u^{tu} (\mathcal{C}_{qu}^{(8)})^{tvsr} (\Omega_u^\dagger \overset{\leftrightarrow}{D}_{\bar{\mu}} \Omega_u) (H^\dagger H) (\bar{u}_s \gamma^{\bar{\mu}} u_r)
\end{aligned}$$

$$\begin{aligned}
& -\frac{i}{27}g_Y(\mathcal{C}_{qu}^{(8)})^{srtt}\left[2(\Omega_u^\dagger D_{\bar{\sigma}}\Omega_u)\tilde{B}^{\bar{\rho}\bar{\sigma}}(\bar{q}_s\gamma^{\bar{\rho}}q_r)+2(D_{\bar{\mu}}\Omega_u^\dagger\Omega_u)\tilde{B}^{\bar{\mu}\bar{\sigma}}(\bar{q}_s\gamma^{\bar{\sigma}}q_r)\right] \\
& -\frac{i}{18}g_s(\mathcal{C}_{qu}^{(8)})^{srtt}\left[2T_b^{Aa}(\Omega_{u,a}^*D_{\bar{\sigma}}\Omega_u^b)\tilde{G}^{\bar{\rho}\bar{\sigma}A}(\bar{q}_s\gamma^{\bar{\rho}}q_r)+2T_b^{Aa}(D_{\bar{\mu}}\Omega_{u,a}^*\Omega_u^b)\tilde{G}^{\bar{\mu}\bar{\sigma}A}(\bar{q}_s\gamma^{\bar{\sigma}}q_r)\right] \\
& -\frac{i}{18}(\mathcal{C}_{qu}^{(8)})^{srtt}\left[(\Omega_u^\dagger D_{\bar{\nu}}\Omega_u)(D^{\bar{\mu}}\bar{q}_s\gamma^{\bar{\nu}}D^{\bar{\mu}}q_r)-(D_{\bar{\mu}}\Omega_u^\dagger\Omega_u)(D^{\bar{\nu}}\bar{q}_s\gamma^{\bar{\mu}}D^{\bar{\nu}}q_r)\right] \\
& -\frac{i}{18}(\mathcal{C}_{qu}^{(8)})^{srtt}\left[(\Omega_u^\dagger D_{\bar{\nu}}\Omega_u)(D^{\bar{\mu}}D^{\bar{\mu}}\bar{q}_s\gamma^{\bar{\nu}}q_r)-(D_{\bar{\mu}}\Omega_u^\dagger\Omega_u)(\bar{q}_s\gamma^{\bar{\mu}}D^{\bar{\nu}}D^{\bar{\nu}}q_r)\right] \\
& +\frac{i}{18}g_s(\mathcal{C}_{qu}^{(8)})^{ttsr}\left[2T_b^{Aa}(\Omega_{q,a}^*D_{\bar{\sigma}}\Omega_q^b)\tilde{G}^{\bar{\rho}\bar{\sigma}A}(\bar{u}_s\gamma^{\bar{\rho}}u_r)+2T_b^{Aa}(D_{\bar{\mu}}\Omega_{q,a}^*\Omega_q^b)\tilde{G}^{\bar{\mu}\bar{\sigma}A}(\bar{u}_s\gamma^{\bar{\sigma}}u_r)\right] \\
& +\frac{i}{18}g_L(\mathcal{C}_{qu}^{(8)})^{ttsr}\left[2t_j^{Ii}(\Omega_{q,i}^*D_{\bar{\sigma}}\Omega_q^j)\tilde{W}^{\bar{\rho}\bar{\sigma}I}(\bar{u}_s\gamma^{\bar{\rho}}u_r)+2t_j^{Ii}(D_{\bar{\mu}}\Omega_{q,i}^*\Omega_q^j)\tilde{W}^{\bar{\mu}\bar{\sigma}I}(\bar{u}_s\gamma^{\bar{\sigma}}u_r)\right] \\
& -\frac{i}{18}(\mathcal{C}_{qu}^{(8)})^{ttsr}\left[(\Omega_q^\dagger D_{\bar{\nu}}\Omega_q)(D^{\bar{\mu}}\bar{u}_s\gamma^{\bar{\nu}}D^{\bar{\mu}}u_r)-(D_{\bar{\mu}}\Omega_q^\dagger\Omega_q)(D^{\bar{\nu}}\bar{u}_s\gamma^{\bar{\mu}}D^{\bar{\nu}}u_r)\right] \\
& -\frac{i}{18}(\mathcal{C}_{qu}^{(8)})^{ttsr}\left[(\Omega_q^\dagger D_{\bar{\nu}}\Omega_q)(D^{\bar{\mu}}D^{\bar{\mu}}\bar{u}_s\gamma^{\bar{\nu}}u_r)-(D_{\bar{\mu}}\Omega_q^\dagger\Omega_q)(\bar{u}_s\gamma^{\bar{\mu}}D^{\bar{\nu}}D^{\bar{\nu}}u_r)\right] \\
& +\frac{i}{12}(\mathcal{C}_{qu}^{(8)})^{srtt}\left[(\Omega_{u,a}^*D_2D_{\bar{\mu}}\Omega_u^b)(\bar{q}_{bs}\gamma^{\bar{\mu}}q_r^a)-(D_2D_{\bar{\nu}}\Omega_{u,a}^*\Omega_u^b)(\bar{q}_{bs}\gamma^{\bar{\nu}}q_r^a)\right] \\
& -\frac{i}{12}(\mathcal{C}_{qu}^{(8)})^{srtt}\left[(D_{\bar{\mu}}D_{\bar{\nu}}\Omega_{u,a}^*\Omega_u^c)(\Omega_{u,b}^*D_{\bar{\mu}}\Omega_u^a)(\bar{q}_{cs}\gamma^{\bar{\nu}}q_r^b)-(D_{\bar{\mu}}\Omega_{u,a}^*\Omega_u^c)(\Omega_{u,b}^*D_{\bar{\mu}}D_{\bar{\nu}}\Omega_u^a)(\bar{q}_{cs}\gamma^{\bar{\nu}}q_r^b)\right] \\
& +\frac{i}{12}(\mathcal{C}_{qu}^{(8)})^{srtt}\left[(\Omega_{u,a}^*D_{\bar{\nu}}\Omega_u^c)(D_{\bar{\mu}}\Omega_{u,b}^*D_{\bar{\nu}}\Omega_u^a)(\bar{q}_{cs}\gamma^{\bar{\mu}}q_r^b)-(D_{\bar{\mu}}\Omega_{u,a}^*D_{\bar{\nu}}\Omega_u^c)(D_{\bar{\mu}}\Omega_{u,b}^*\Omega_u^a)(\bar{q}_{cs}\gamma^{\bar{\nu}}q_r^b)\right] \\
& +\frac{1}{12}(\mathcal{C}_{qu}^{(8)})^{srtt}\left[(\Omega_{u,a}^*D_{\bar{\rho}}\Omega_u^c)(D_{\bar{\mu}}\Omega_{u,b}^*D_{\bar{\sigma}}\Omega_u^a)\varepsilon^{\bar{\mu}\bar{\nu}\bar{\rho}\bar{\sigma}}(\bar{q}_{cs}\gamma^{\bar{\nu}}q_r^b)-(D_{\bar{\mu}}\Omega_{u,a}^*D_{\bar{\rho}}\Omega_u^c)(D_{\bar{\nu}}\Omega_{u,b}^*\Omega_u^a)\varepsilon^{\bar{\mu}\bar{\nu}\bar{\rho}\bar{\sigma}}(\bar{q}_{cs}\gamma^{\bar{\sigma}}q_r^b)\right] \\
& +\frac{i}{12}(\mathcal{C}_{qu}^{(8)})^{srtt}\left[(\Omega_{u,a}^*D_{\bar{\nu}}\Omega_u^c)(\Omega_{u,b}^*D_{\bar{\mu}}\Omega_u^a)(D^{\bar{\mu}}\bar{q}_{cs}\gamma^{\bar{\nu}}q_r^b)-(D_{\bar{\mu}}\Omega_{u,a}^*\Omega_u^c)(D_{\bar{\nu}}\Omega_{u,b}^*\Omega_u^a)(\bar{q}_{cs}\gamma^{\bar{\nu}}D^{\bar{\mu}}q_r^b)\right] \\
& +\frac{i}{12}(\mathcal{C}_{qu}^{(8)})^{srtt}\left[(\Omega_{u,a}^*D_{\bar{\mu}}\Omega_u^c)(\Omega_{u,b}^*D_{\bar{\nu}}\Omega_u^a)(\bar{q}_{cs}\gamma^{\bar{\mu}}D^{\bar{\nu}}q_r^b)-(D_{\bar{\mu}}\Omega_{u,a}^*\Omega_u^c)(D_{\bar{\nu}}\Omega_{u,b}^*\Omega_u^a)(D^{\bar{\mu}}\bar{q}_{cs}\gamma^{\bar{\nu}}q_r^b)\right] \\
& +\frac{i}{12}(\mathcal{C}_{qu}^{(8)})^{ttsr}\left[(\Omega_{q,a}^*D_2D_{\bar{\mu}}\Omega_q^b)(\bar{u}_{bs}\gamma^{\bar{\mu}}u_r^a)-(D_2D_{\bar{\nu}}\Omega_{q,a}^*\Omega_q^b)(\bar{u}_{bs}\gamma^{\bar{\nu}}u_r^a)\right] \\
& -\frac{i}{12}(\mathcal{C}_{qu}^{(8)})^{ttsr}\left[(D_{\bar{\mu}}D_{\bar{\nu}}\Omega_{q,ai}^*\Omega_q^{cj})(\Omega_{q,bj}^*D_{\bar{\mu}}\Omega_q^{ai})(\bar{u}_{cs}\gamma^{\bar{\nu}}u_r^b)-(D_{\bar{\mu}}\Omega_{q,ai}^*\Omega_q^{cj})(\Omega_{q,bj}^*D_{\bar{\mu}}D_{\bar{\nu}}\Omega_q^{ai})(\bar{u}_{cs}\gamma^{\bar{\nu}}u_r^b)\right] \\
& +\frac{i}{12}(\mathcal{C}_{qu}^{(8)})^{ttsr}\left[(\Omega_{q,ai}^*D_{\bar{\nu}}\Omega_q^{cj})(D_{\bar{\mu}}\Omega_{q,bj}^*D_{\bar{\nu}}\Omega_q^{ai})(\bar{u}_{cs}\gamma^{\bar{\mu}}u_r^b)-(D_{\bar{\mu}}\Omega_{q,ai}^*D_{\bar{\nu}}\Omega_q^{cj})(D_{\bar{\mu}}\Omega_{q,bj}^*\Omega_q^{ai})(\bar{u}_{cs}\gamma^{\bar{\nu}}u_r^b)\right] \\
& +\frac{1}{9}y_u^{st}(\mathcal{C}_{qu}^{(8)})^{rstu}(D_{\bar{\mu}}\Omega_{q,a}^*D_{\bar{\mu}}\Omega_q^b)(\bar{q}_{br}\tilde{H}u_u^a)+\frac{1}{9}y_u^{st}(\mathcal{C}_{qu}^{(8)})^{rstu}(D_{\bar{\mu}}\Omega_{q,a}^*\Omega_q^b)(\bar{q}_{br}D_{\bar{\mu}}\tilde{H}u_u^a) \\
& +\frac{1}{9}y_u^{st}(\mathcal{C}_{qu}^{(8)})^{rstu}(D_{\bar{\mu}}\Omega_{u,a}^*\Omega_u^b)(\bar{q}_{br}D_{\bar{\mu}}\tilde{H}u_u^a)+\frac{1}{9}y_u^{st}(\mathcal{C}_{qu}^{(8)})^{rstu}\varepsilon^{kj}(D_{\bar{\mu}}\Omega_{q,aj}^*\Omega_q^{bi})D^{\bar{\mu}}H_i^\dagger(\bar{q}_{bkr}u_u^a) \\
& +\frac{1}{9}y_u^{st}(\mathcal{C}_{qu}^{(8)})^{rstu}\varepsilon^{kj}(D_{\bar{\mu}}\Omega_{q,aj}^*D_{\bar{\mu}}\Omega_q^{bi})H_i^\dagger(\bar{q}_{bkr}u_u^a)+\frac{1}{9}\bar{y}_u^{rs}(\mathcal{C}_{qu}^{(8)})^{rtus}\bar{\varepsilon}_{jk}(D_{\bar{\mu}}\Omega_{q,ai}^*D_{\bar{\mu}}\Omega_q^{bk})H^i(\bar{u}_{bu}q_t^{aj}) \\
& +\frac{1}{9}\bar{y}_u^{rs}(\mathcal{C}_{qu}^{(8)})^{rtus}\bar{\varepsilon}_{jk}(\Omega_{q,ai}^*D_{\bar{\mu}}\Omega_q^{bk})D^{\bar{\mu}}H^i(\bar{u}_{bu}q_t^{aj})+\frac{1}{9}\bar{y}_u^{rs}(\mathcal{C}_{qu}^{(8)})^{rtus}(D_{\bar{\mu}}\Omega_{q,a}^*D_{\bar{\mu}}\Omega_q^b)(\bar{u}_{bu}\tilde{H}^\dagger q_t^a) \\
& +\frac{1}{9}\bar{y}_u^{rs}(\mathcal{C}_{qu}^{(8)})^{rtus}(\Omega_{q,a}^*D_{\bar{\mu}}\Omega_q^b)(\bar{u}_{bu}D_{\bar{\mu}}\tilde{H}^\dagger q_t^a)+\frac{1}{9}\bar{y}_u^{rs}(\mathcal{C}_{qu}^{(8)})^{rtus}(\Omega_{u,a}^*D_{\bar{\mu}}\Omega_u^b)(\bar{u}_{bu}D_{\bar{\mu}}\tilde{H}^\dagger q_t^a) \\
& +\frac{1}{3}y_u^{st}(\mathcal{C}_{qu}^{(8)})^{rstu}(D_{\bar{\mu}}\Omega_u^\dagger D_{\bar{\mu}}\Omega_u)(\bar{q}_r\tilde{H}u_u)+\frac{1}{3}y_u^{st}(\mathcal{C}_{qu}^{(8)})^{rstu}(D_{\bar{\mu}}\Omega_{q,a}^*\Omega_q^b)(D_{\bar{\mu}}\Omega_{u,b}^*\Omega_u^a)(\bar{q}_r\tilde{H}u_u)
\end{aligned}$$

$$\begin{aligned}
& + \frac{1}{3} y_u^{st} (\mathcal{C}_{qu}^{(8)})^{rstu} (D_{\bar{\mu}} \Omega_q^\dagger \Omega_q) (\bar{q}_r \tilde{H} D^{\bar{\mu}} u_u) + \frac{1}{3} y_u^{st} (\mathcal{C}_{qu}^{(8)})^{rstu} (D_{\bar{\mu}} \Omega_u^\dagger \Omega_u) (\bar{q}_r \tilde{H} D^{\bar{\mu}} u_u) \\
& + \frac{1}{3} y_u^{st} (\mathcal{C}_{qu}^{(8)})^{rstu} (D_{\bar{\mu}} \Omega_q^\dagger \Omega_q) (D^{\bar{\mu}} \bar{q}_r \tilde{H} u_u) + \frac{1}{3} y_u^{st} (\mathcal{C}_{qu}^{(8)})^{rstu} (D_{\bar{\mu}} \Omega_u^\dagger \Omega_u) (D^{\bar{\mu}} \bar{q}_r \tilde{H} u_u) \\
& + \frac{1}{3} \bar{y}_u^{rs} (\mathcal{C}_{qu}^{(8)})^{rtus} \bar{\varepsilon}_{jk} (\Omega_{q,ai}^* D_{\bar{\mu}} \Omega_q^{bk}) (\Omega_{u,b}^* D_{\bar{\mu}} \Omega_u^a) H^i (\bar{u}_u q_t^j) + \frac{1}{3} \bar{y}_u^{rs} (\mathcal{C}_{qu}^{(8)})^{rtus} \bar{\varepsilon}_{jk} (\Omega_{q,i}^* D_{\bar{\mu}} \Omega_q^k) H^i (\bar{u}_u D^{\bar{\mu}} q_t^j) \\
& + \frac{1}{3} \bar{y}_u^{rs} (\mathcal{C}_{qu}^{(8)})^{rtus} (D_{\bar{\mu}} \Omega_u^\dagger D_{\bar{\mu}} \Omega_u) (\bar{u}_u \tilde{H}^\dagger q_t) + \frac{1}{3} \bar{y}_u^{rs} (\mathcal{C}_{qu}^{(8)})^{rtus} (\Omega_{q,a}^* D_{\bar{\mu}} \Omega_q^b) (\Omega_{u,b}^* D_{\bar{\mu}} \Omega_u^a) (\bar{u}_u \tilde{H}^\dagger q_t) \\
& + \frac{1}{3} \bar{y}_u^{rs} (\mathcal{C}_{qu}^{(8)})^{rtus} (\Omega_q^\dagger D_{\bar{\mu}} \Omega_q) (\bar{u}_u \tilde{H}^\dagger D^{\bar{\mu}} q_t) + \frac{1}{3} \bar{y}_u^{rs} (\mathcal{C}_{qu}^{(8)})^{rtus} (\Omega_u^\dagger D_{\bar{\mu}} \Omega_u) (\bar{u}_u \tilde{H}^\dagger D^{\bar{\mu}} q_t) \\
& + \frac{1}{3} \bar{y}_u^{rs} (\mathcal{C}_{qu}^{(8)})^{rtus} \bar{\varepsilon}_{jk} (\Omega_{q,i}^* D_{\bar{\mu}} \Omega_q^k) H^i (D^{\bar{\mu}} \bar{u}_u q_t^j) + \frac{1}{3} \bar{y}_u^{rs} (\mathcal{C}_{qu}^{(8)})^{rtus} (\Omega_q^\dagger D_{\bar{\mu}} \Omega_q) (D^{\bar{\mu}} \bar{u}_u \tilde{H}^\dagger q_t) \\
& + \frac{1}{3} \bar{y}_u^{rs} (\mathcal{C}_{qu}^{(8)})^{rtus} (\Omega_u^\dagger D_{\bar{\mu}} \Omega_u) (D^{\bar{\mu}} \bar{u}_u \tilde{H}^\dagger q_t) \\
& - \frac{1}{12} (\mathcal{C}_{qu}^{(8)})^{ttsr} \left[ (\Omega_{q,ai}^* D_{\bar{\rho}} \Omega_q^{cj}) (D_{\bar{\mu}} \Omega_{q,bj}^* D_{\bar{\sigma}} \Omega_q^{ai}) \varepsilon^{\bar{\mu}\bar{\nu}\bar{\rho}\bar{\sigma}} (\bar{u}_{cs} \gamma^{\bar{\nu}} u_r^b) - (D_{\bar{\mu}} \Omega_{q,ai}^* D_{\bar{\rho}} \Omega_q^{cj}) (D_{\bar{\nu}} \Omega_{q,bj}^* \Omega_q^{ai}) \varepsilon^{\bar{\mu}\bar{\nu}\bar{\rho}\bar{\sigma}} (\bar{u}_{cs} \gamma^{\bar{\sigma}} u_r^b) \right] \\
& + \frac{i}{12} (\mathcal{C}_{qu}^{(8)})^{ttsr} \left[ (\Omega_{q,ai}^* D_{\bar{\nu}} \Omega_q^{cj}) (\Omega_{q,bj}^* D_{\bar{\mu}} \Omega_q^{ai}) (D^{\bar{\mu}} \bar{u}_{cs} \gamma^{\bar{\nu}} u_r^b) - (D_{\bar{\mu}} \Omega_{q,ai}^* \Omega_q^{cj}) (D_{\bar{\nu}} \Omega_{q,bj}^* \Omega_q^{ai}) (\bar{u}_{cs} \gamma^{\bar{\nu}} D^{\bar{\mu}} u_r^b) \right] \\
& + \frac{i}{12} (\mathcal{C}_{qu}^{(8)})^{ttsr} \left[ (\Omega_{q,ai}^* D_{\bar{\mu}} \Omega_q^{cj}) (\Omega_{q,bj}^* D_{\bar{\nu}} \Omega_q^{ai}) (\bar{u}_{cs} \gamma^{\bar{\mu}} D^{\bar{\nu}} u_r^b) - (D_{\bar{\mu}} \Omega_{q,ai}^* \Omega_q^{cj}) (D_{\bar{\nu}} \Omega_{q,bj}^* \Omega_q^{ai}) (D^{\bar{\mu}} \bar{u}_{cs} \gamma^{\bar{\nu}} u_r^b) \right] \\
& - \frac{i}{12} \bar{y}_d^{vu} \bar{y}_d^{tu} (\mathcal{C}_{qu}^{(8)})^{tvsr} (\Omega_{d,a}^* \overleftrightarrow{D}_{\bar{\mu}} \Omega_d^b) (H^\dagger H) (\bar{u}_{bs} \gamma^{\bar{\mu}} u_r^a) - \frac{i}{12} y_u^{tv} \bar{y}_u^{tu} (\mathcal{C}_{qu}^{(8)})^{srvu} (\Omega_{q,a}^* \overleftrightarrow{D}_{\bar{\mu}} \Omega_q^b) (H^\dagger H) (\bar{q}_{bs} \gamma^{\bar{\mu}} q_r^a) \\
& + \frac{i}{12} y_u^{tv} \bar{y}_u^{tu} (\mathcal{C}_{qu}^{(8)})^{srvu} (\Omega_{q,aj}^* \overleftrightarrow{D}_{\bar{\mu}} \Omega_q^{bi}) H_i^\dagger H^j (\bar{q}_{bs} \gamma^{\bar{\mu}} q_r^a) - \frac{i}{12} y_u^{vu} \bar{y}_u^{tu} (\mathcal{C}_{qu}^{(8)})^{tvsr} (\Omega_{u,a}^* \overleftrightarrow{D}_{\bar{\mu}} \Omega_u^b) (H^\dagger H) (\bar{u}_{bs} \gamma^{\bar{\mu}} u_r^a) \\
& - \frac{1}{9} y_u^{st} (\mathcal{C}_{qu}^{(8)})^{rstu} (D_{\bar{\mu}} \Omega_{u,a}^* D_{\bar{\mu}} \Omega_u^b) (\bar{q}_{br} \tilde{H} u_u^a) - \frac{1}{9} y_u^{st} (\mathcal{C}_{qu}^{(8)})^{rstu} (D_{\bar{\mu}} \Omega_{q,a}^* \Omega_q^b) (\bar{q}_{br} \tilde{H} D^{\bar{\mu}} u_u^a) \\
& - \frac{1}{9} y_u^{st} (\mathcal{C}_{qu}^{(8)})^{rstu} (D_{\bar{\mu}} \Omega_{u,a}^* \Omega_u^b) (\bar{q}_{br} \tilde{H} D^{\bar{\mu}} u_u^a) - \frac{1}{9} y_u^{st} (\mathcal{C}_{qu}^{(8)})^{rstu} (D_{\bar{\mu}} \Omega_{q,a}^* \Omega_q^b) (D^{\bar{\mu}} \bar{q}_{br} \tilde{H} u_u^a) \\
& - \frac{1}{9} y_u^{st} (\mathcal{C}_{qu}^{(8)})^{rstu} (D_{\bar{\mu}} \Omega_{u,a}^* \Omega_u^b) (D^{\bar{\mu}} \bar{q}_{br} \tilde{H} u_u^a) \\
& - \frac{i}{9} g_Y (\mathcal{C}_{qu}^{(8)})^{srtt} \left[ 2 (\Omega_{u,a}^* D_{\bar{\rho}} \Omega_u^b) \tilde{B}^{\bar{\rho}\bar{\sigma}} (\bar{q}_{bs} \gamma^{\bar{\sigma}} q_r^a) - 2 (D_{\bar{\mu}} \Omega_{u,a}^* \Omega_u^b) \tilde{B}^{\bar{\mu}\bar{\sigma}} (\bar{q}_{bs} \gamma^{\bar{\sigma}} q_r^a) \right] \\
& - \frac{1}{9} y_u^{st} (\mathcal{C}_{qu}^{(8)})^{rstu} \varepsilon^{kj} (D_{\bar{\mu}} \Omega_{q,aj}^* \Omega_q^{bi}) H_i^\dagger (\bar{q}_{bkr} D^{\bar{\mu}} u_u^a) - \frac{1}{9} y_u^{st} (\mathcal{C}_{qu}^{(8)})^{rstu} \varepsilon^{kj} (D_{\bar{\mu}} \Omega_{q,aj}^* \Omega_q^{bi}) H_i^\dagger (D^{\bar{\mu}} \bar{q}_{bkr} u_u^a) \\
& - \frac{1}{9} y_u^{st} (\mathcal{C}_{qu}^{(8)})^{rstu} \varepsilon^{kj} (D_{\bar{\mu}} \Omega_{q,aj}^* \Omega_q^{ci}) (D_{\bar{\mu}} \Omega_{u,b}^* \Omega_u^a) H_i^\dagger (\bar{q}_{ckr} u_u^b) - \frac{1}{9} \bar{y}_u^{rs} (\mathcal{C}_{qu}^{(8)})^{rtus} \bar{\varepsilon}_{jk} (\Omega_{q,ai}^* D_{\bar{\mu}} \Omega_q^{bk}) H^i (\bar{u}_{bu} D^{\bar{\mu}} q_t^{aj}) \\
& - \frac{1}{9} \bar{y}_u^{rs} (\mathcal{C}_{qu}^{(8)})^{rtus} (D_{\bar{\mu}} \Omega_{u,a}^* D_{\bar{\mu}} \Omega_u^b) (\bar{u}_{bu} \tilde{H}^\dagger q_t^a) - \frac{1}{9} \bar{y}_u^{rs} (\mathcal{C}_{qu}^{(8)})^{rtus} (\Omega_{q,a}^* D_{\bar{\mu}} \Omega_q^b) (\bar{u}_{bu} \tilde{H}^\dagger D^{\bar{\mu}} q_t^a) \\
& - \frac{1}{9} \bar{y}_u^{rs} (\mathcal{C}_{qu}^{(8)})^{rtus} (\Omega_{u,a}^* D_{\bar{\mu}} \Omega_u^b) (\bar{u}_{bu} \tilde{H}^\dagger D^{\bar{\mu}} q_t^a) - \frac{1}{9} \bar{y}_u^{rs} (\mathcal{C}_{qu}^{(8)})^{rtus} \bar{\varepsilon}_{jk} (\Omega_{q,ai}^* D_{\bar{\mu}} \Omega_q^{bk}) H^i (D^{\bar{\mu}} \bar{u}_{bu} q_t^{aj}) \\
& - \frac{1}{9} \bar{y}_u^{rs} (\mathcal{C}_{qu}^{(8)})^{rtus} (\Omega_{q,a}^* D_{\bar{\mu}} \Omega_q^b) (D^{\bar{\mu}} \bar{u}_{bu} \tilde{H}^\dagger q_t^a) - \frac{1}{9} \bar{y}_u^{rs} (\mathcal{C}_{qu}^{(8)})^{rtus} (\Omega_{u,a}^* D_{\bar{\mu}} \Omega_u^b) (D^{\bar{\mu}} \bar{u}_{bu} \tilde{H}^\dagger q_t^a) \\
& - \frac{1}{9} \bar{y}_u^{rs} (\mathcal{C}_{qu}^{(8)})^{rtus} \bar{\varepsilon}_{jk} (\Omega_{q,ai}^* D_{\bar{\mu}} \Omega_q^{bk}) (\Omega_{u,b}^* D_{\bar{\mu}} \Omega_u^c) H^i (\bar{u}_{cu} q_t^{aj}) - \frac{1}{9} \bar{y}_u^{rs} (\mathcal{C}_{qu}^{(8)})^{rtus} (\Omega_{q,a}^* D_{\bar{\mu}} \Omega_q^b) (\Omega_{u,b}^* D_{\bar{\mu}} \Omega_u^c) (\bar{u}_{cu} \tilde{H}^\dagger q_t^a) \\
& - \frac{i}{9} \bar{y}_u^{vu} \bar{y}_u^{tu} (\mathcal{C}_{qu}^{(8)})^{tvsr} (\Omega_q^\dagger \overleftrightarrow{D}_{\bar{\mu}} \Omega_q) (H^\dagger H) (\bar{u}_s \gamma^{\bar{\mu}} u_r)
\end{aligned}$$

$$\begin{aligned}
& -\frac{i}{9}(\mathcal{C}_{qu}^{(8)})^{tvsr} \left[ y_d^{vu} \bar{y}_d^{tu} - y_u^{vu} \bar{y}_u^{tu} \right] (\Omega_{q,j}^* \overset{\leftrightarrow}{D}_{\bar{\mu}} \Omega_q^i) H_i^\dagger H^j (\bar{u}_s \gamma^{\bar{\mu}} u_r) \\
& -\frac{i}{9} y_u^{tv} \bar{y}_u^{tu} (\mathcal{C}_{qu}^{(8)})^{srvu} (\Omega_u^\dagger \overset{\leftrightarrow}{D}_{\bar{\mu}} \Omega_u) (H^\dagger H) (\bar{q}_s \gamma^{\bar{\mu}} q_r) \\
& +\frac{i}{6} (\mathcal{C}_{qu}^{(8)})^{srtt} \left[ (\Omega_{u,a}^* D_{\bar{\nu}} \Omega_u^b) (D_{\bar{\mu}} \bar{q}_{bs} \gamma^{\bar{\nu}} D_{\bar{\mu}} q_r^a) - (D_{\bar{\mu}} \Omega_{u,a}^* \Omega_u^b) (D_{\bar{\nu}} \bar{q}_{bs} \gamma^{\bar{\mu}} D_{\bar{\nu}} q_r^a) \right] \\
& +\frac{i}{6} (\mathcal{C}_{qu}^{(8)})^{srtt} \left[ (\Omega_{u,a}^* D_{\bar{\nu}} \Omega_u^b) (D_{\bar{\mu}} D_{\bar{\mu}} \bar{q}_{bs} \gamma^{\bar{\nu}} q_r^a) - (D_{\bar{\mu}} \Omega_{u,a}^* \Omega_u^b) (\bar{q}_{bs} \gamma^{\bar{\mu}} D_{\bar{\nu}} D_{\bar{\nu}} q_r^a) \right] \\
& -\frac{i}{6} (\mathcal{C}_{qu}^{(8)})^{srtt} \left[ (\Omega_{u,a}^* D_{\bar{\mu}} \Omega_u^c) (D_{\bar{\mu}} \Omega_{u,b}^* D_{\bar{\nu}} \Omega_u^a) (\bar{q}_{cs} \gamma^{\bar{\nu}} q_r^b) - (D_{\bar{\mu}} \Omega_{u,a}^* D_{\bar{\nu}} \Omega_u^c) (D_{\bar{\nu}} \Omega_{u,b}^* \Omega_u^a) (\bar{q}_{cs} \gamma^{\bar{\mu}} q_r^b) \right] \\
& -\frac{i}{6} g_s (\mathcal{C}_{qu}^{(8)})^{srtt} \left[ 2T_b^{Aa} (\Omega_{u,a}^* D_{\bar{\rho}} \Omega_u^c) \tilde{G}^{\bar{\rho}\bar{\sigma}A} (\bar{q}_{cs} \gamma^{\bar{\sigma}} q_r^b) - 2T_c^{Ab} (D_{\bar{\mu}} \Omega_{u,a}^* \Omega_u^c) \tilde{G}^{\bar{\mu}\bar{\sigma}A} (\bar{q}_{bs} \gamma^{\bar{\sigma}} q_r^a) \right] \\
& +\frac{i}{6} g_L (\mathcal{C}_{qu}^{(8)})^{ttsr} \left[ 2t_j^{Ii} (\Omega_{q,ai}^* D_{\bar{\rho}} \Omega_q^{bj}) \tilde{W}^{\bar{\rho}\bar{\sigma}I} (\bar{u}_{bs} \gamma^{\bar{\sigma}} u_r^a) - 2t_j^{Ii} (D_{\bar{\mu}} \Omega_{q,ai}^* \Omega_q^{bj}) \tilde{W}^{\bar{\mu}\bar{\sigma}I} (\bar{u}_{bs} \gamma^{\bar{\sigma}} u_r^a) \right] \\
& +\frac{i}{6} (\mathcal{C}_{qu}^{(8)})^{ttsr} \left[ (\Omega_{q,a}^* D_{\bar{\nu}} \Omega_q^b) (D_{\bar{\mu}} \bar{u}_{bs} \gamma^{\bar{\nu}} D_{\bar{\mu}} u_r^a) - (D_{\bar{\mu}} \Omega_{q,a}^* \Omega_q^b) (D_{\bar{\nu}} \bar{u}_{bs} \gamma^{\bar{\mu}} D_{\bar{\nu}} u_r^a) \right] \\
& +\frac{i}{6} (\mathcal{C}_{qu}^{(8)})^{ttsr} \left[ (\Omega_{q,a}^* D_{\bar{\nu}} \Omega_q^b) (D_{\bar{\mu}} D_{\bar{\mu}} \bar{u}_{bs} \gamma^{\bar{\nu}} u_r^a) - (D_{\bar{\mu}} \Omega_{q,a}^* \Omega_q^b) (\bar{u}_{bs} \gamma^{\bar{\mu}} D_{\bar{\nu}} D_{\bar{\nu}} u_r^a) \right] \\
& -\frac{i}{6} (\mathcal{C}_{qu}^{(8)})^{ttsr} \left[ (\Omega_{q,ai}^* D_{\bar{\mu}} \Omega_q^{cj}) (D_{\bar{\mu}} \Omega_{q,bj}^* D_{\bar{\nu}} \Omega_q^{ai}) (\bar{u}_{cs} \gamma^{\bar{\nu}} u_r^b) - (D_{\bar{\mu}} \Omega_{q,ai}^* D_{\bar{\nu}} \Omega_q^{cj}) (D_{\bar{\nu}} \Omega_{q,bj}^* \Omega_q^{ai}) (\bar{u}_{cs} \gamma^{\bar{\mu}} u_r^b) \right] \\
& +\frac{i}{6} g_s (\mathcal{C}_{qu}^{(8)})^{ttsr} \left[ 2T_b^{Aa} (\Omega_{q,a}^* D_{\bar{\rho}} \Omega_q^c) \tilde{G}^{\bar{\rho}\bar{\sigma}A} (\bar{u}_{cs} \gamma^{\bar{\sigma}} u_r^b) - 2T_c^{Ab} (D_{\bar{\mu}} \Omega_{q,a}^* \Omega_q^c) \tilde{G}^{\bar{\mu}\bar{\sigma}A} (\bar{u}_{bs} \gamma^{\bar{\sigma}} u_r^a) \right] \\
& +\frac{1}{3} y_u^{st} (\mathcal{C}_{qu}^{(8)})^{rstu} \varepsilon^{kj} (D_{\bar{\mu}} \Omega_{q,aj}^* \Omega_q^{bi}) (D_{\bar{\mu}} \Omega_{u,b}^* \Omega_u^a) H_i^\dagger (\bar{q}_{kr} u_u) + \frac{1}{3} y_u^{st} (\mathcal{C}_{qu}^{(8)})^{rstu} \varepsilon^{kj} (D_{\bar{\mu}} \Omega_{q,j}^* \Omega_q^i) H_i^\dagger (\bar{q}_{kr} D_{\bar{\mu}} u_u) \\
& +\frac{1}{3} y_u^{st} (\mathcal{C}_{qu}^{(8)})^{rstu} \varepsilon^{kj} (D_{\bar{\mu}} \Omega_{q,j}^* \Omega_q^i) H_i^\dagger (D_{\bar{\mu}} \bar{q}_{kr} u_u) - \frac{1}{9} y_u^{st} (\mathcal{C}_{qu}^{(8)})^{rstu} (D_{\bar{\mu}} \Omega_{q,a}^* \Omega_q^c) (D_{\bar{\mu}} \Omega_{u,b}^* \Omega_u^a) (\bar{q}_{cr} \tilde{H} u_u^b) \\
& -\frac{1}{3} y_u^{st} (\mathcal{C}_{qu}^{(8)})^{rstu} (D_{\bar{\mu}} \Omega_q^\dagger D_{\bar{\mu}} \Omega_q) (\bar{q}_r \tilde{H} u_u) - \frac{1}{3} y_u^{st} (\mathcal{C}_{qu}^{(8)})^{rstu} (D_{\bar{\mu}} \Omega_q^\dagger \Omega_q) (\bar{q}_r D_{\bar{\mu}} \tilde{H} u_u) \\
& -\frac{1}{3} y_u^{st} (\mathcal{C}_{qu}^{(8)})^{rstu} (D_{\bar{\mu}} \Omega_u^\dagger \Omega_u) (\bar{q}_r D_{\bar{\mu}} \tilde{H} u_u) - \frac{1}{3} y_u^{st} (\mathcal{C}_{qu}^{(8)})^{rstu} \varepsilon^{kj} (D_{\bar{\mu}} \Omega_{q,j}^* \Omega_q^i) D_{\bar{\mu}} H_i^\dagger (\bar{q}_{kr} u_u) \\
& -\frac{1}{3} y_u^{st} (\mathcal{C}_{qu}^{(8)})^{rstu} \varepsilon^{kj} (D_{\bar{\mu}} \Omega_{q,j}^* D_{\bar{\mu}} \Omega_q^i) H_i^\dagger (\bar{q}_{kr} u_u) - \frac{1}{3} \bar{y}_u^{rs} (\mathcal{C}_{qu}^{(8)})^{rtus} \bar{\varepsilon}_{jk} (D_{\bar{\mu}} \Omega_{q,i}^* D_{\bar{\mu}} \Omega_q^k) H^i (\bar{u}_u q_t^j) \\
& -\frac{1}{3} \bar{y}_u^{rs} (\mathcal{C}_{qu}^{(8)})^{rtus} \bar{\varepsilon}_{jk} (\Omega_{q,i}^* D_{\bar{\mu}} \Omega_q^k) D_{\bar{\mu}} H^i (\bar{u}_u q_t^j) - \frac{1}{3} \bar{y}_u^{rs} (\mathcal{C}_{qu}^{(8)})^{rtus} (D_{\bar{\mu}} \Omega_q^\dagger D_{\bar{\mu}} \Omega_q) (\bar{u}_u \tilde{H}^\dagger q_t) \\
& -\frac{1}{3} \bar{y}_u^{rs} (\mathcal{C}_{qu}^{(8)})^{rtus} (\Omega_q^\dagger D_{\bar{\mu}} \Omega_q) (\bar{u}_u D_{\bar{\mu}} \tilde{H}^\dagger q_t) - \frac{1}{3} \bar{y}_u^{rs} (\mathcal{C}_{qu}^{(8)})^{rtus} (\Omega_u^\dagger D_{\bar{\mu}} \Omega_u) (\bar{u}_u D_{\bar{\mu}} \tilde{H}^\dagger q_t) \\
& +\frac{i}{3} y_u^{vu} \bar{y}_u^{tu} (\mathcal{C}_{qu}^{(8)})^{tvsr} (\Omega_{q,a}^* \overset{\leftrightarrow}{D}_{\bar{\mu}} \Omega_q^b) (H^\dagger H) (\bar{u}_{bs} \gamma^{\bar{\mu}} u_r^a) \\
& +\frac{i}{3} (\mathcal{C}_{qu}^{(8)})^{tvsr} \left[ y_d^{vu} \bar{y}_d^{tu} - y_u^{vu} \bar{y}_u^{tu} \right] (\Omega_{q,aj}^* \overset{\leftrightarrow}{D}_{\bar{\mu}} \Omega_q^{bi}) H_i^\dagger H^j (\bar{u}_{bs} \gamma^{\bar{\mu}} u_r^a) \\
& +\frac{i}{3} y_u^{tv} \bar{y}_u^{tu} (\mathcal{C}_{qu}^{(8)})^{srvu} (\Omega_{u,a}^* \overset{\leftrightarrow}{D}_{\bar{\mu}} \Omega_u^b) (H^\dagger H) (\bar{q}_{bs} \gamma^{\bar{\mu}} q_r^a) \\
& -\frac{1}{2} g_s (\mathcal{C}_{qu}^{(8)})^{srtt} \left[ T_b^{Aa} (\Omega_{u,a}^* D_{\bar{\nu}} \Omega_u^c) G^{\bar{\mu}\bar{\nu}A} (\bar{q}_{cs} \gamma^{\bar{\mu}} q_r^b) - T_c^{Ab} (D_{\bar{\mu}} \Omega_{u,a}^* \Omega_u^c) G^{\bar{\mu}\bar{\nu}A} (\bar{q}_{bs} \gamma^{\bar{\nu}} q_r^a) \right] \\
& -\frac{1}{2} g_s (\mathcal{C}_{qu}^{(8)})^{ttsr} \left[ T_b^{Aa} (\Omega_{q,a}^* D_{\bar{\nu}} \Omega_q^c) G^{\bar{\mu}\bar{\nu}A} (\bar{u}_{cs} \gamma^{\bar{\mu}} u_r^b) - T_c^{Ab} (D_{\bar{\mu}} \Omega_{q,a}^* \Omega_q^c) G^{\bar{\mu}\bar{\nu}A} (\bar{u}_{bs} \gamma^{\bar{\nu}} u_r^a) \right], \tag{3.55}
\end{aligned}$$

$$\begin{aligned}
\Gamma_{\Omega}^{(1)} [\mathcal{O}_{qd}^{(1)}] = & -\frac{i}{18} g_Y (\mathcal{C}_{qd}^{(1)})^{ttsr} \left[ 2(\Omega_q^\dagger D_{\bar{\sigma}} \Omega_q) \tilde{B}^{\bar{\rho}\bar{\sigma}} (\bar{d}_s \gamma^{\bar{\rho}} d_r) + 2(D_{\bar{\mu}} \Omega_q^\dagger \Omega_q) \tilde{B}^{\bar{\mu}\bar{\sigma}} (\bar{d}_s \gamma^{\bar{\sigma}} d_r) \right] \\
& -\frac{i}{9} g_Y (\mathcal{C}_{qd}^{(1)})^{srtt} \left[ 2(\Omega_d^\dagger D_{\bar{\sigma}} \Omega_d) \tilde{B}^{\bar{\rho}\bar{\sigma}} (\bar{q}_s \gamma^{\bar{\rho}} q_r) + 2(D_{\bar{\mu}} \Omega_d^\dagger \Omega_d) \tilde{B}^{\bar{\mu}\bar{\sigma}} (\bar{q}_s \gamma^{\bar{\sigma}} q_r) \right] \\
& +\frac{i}{6} (\mathcal{C}_{qd}^{(1)})^{ttsr} \left[ (\Omega_q^\dagger D_2 D_{\bar{\mu}} \Omega_q) (\bar{d}_s \gamma^{\bar{\mu}} d_r) - (D_2 D_{\bar{\nu}} \Omega_q^\dagger \Omega_q) (\bar{d}_s \gamma^{\bar{\nu}} d_r) \right] \\
& +\frac{1}{6} (\mathcal{C}_{qd}^{(1)})^{ttsr} \left[ (D_{\bar{\mu}} \Omega_{q,ai}^* D_{\bar{\rho}} \Omega_q^{bj}) (\Omega_{q,bj}^* D_{\bar{\sigma}} \Omega_q^{ai}) \varepsilon^{\bar{\mu}\bar{\nu}\bar{\rho}\bar{\sigma}} (\bar{d}_s \gamma^{\bar{\nu}} d_r) - (D_{\bar{\mu}} \Omega_{q,ai}^* \Omega_q^{bj}) (D_{\bar{\nu}} \Omega_{q,bj}^* D_{\bar{\rho}} \Omega_q^{ai}) \varepsilon^{\bar{\mu}\bar{\nu}\bar{\rho}\bar{\sigma}} (\bar{d}_s \gamma^{\bar{\sigma}} d_r) \right] \\
& +\frac{i}{6} (\mathcal{C}_{qd}^{(1)})^{srtt} \left[ (\Omega_d^\dagger D_2 D_{\bar{\mu}} \Omega_d) (\bar{q}_s \gamma^{\bar{\mu}} q_r) - (D_2 D_{\bar{\nu}} \Omega_d^\dagger \Omega_d) (\bar{q}_s \gamma^{\bar{\nu}} q_r) \right] \\
& -\frac{1}{6} (\mathcal{C}_{qd}^{(1)})^{srtt} \left[ (D_{\bar{\mu}} \Omega_{d,a}^* D_{\bar{\rho}} \Omega_d^b) (\Omega_{d,b}^* D_{\bar{\sigma}} \Omega_d^a) \varepsilon^{\bar{\mu}\bar{\nu}\bar{\rho}\bar{\sigma}} (\bar{q}_s \gamma^{\bar{\nu}} q_r) - (D_{\bar{\mu}} \Omega_{d,a}^* \Omega_d^b) (D_{\bar{\nu}} \Omega_{d,b}^* D_{\bar{\rho}} \Omega_d^a) \varepsilon^{\bar{\mu}\bar{\nu}\bar{\rho}\bar{\sigma}} (\bar{q}_s \gamma^{\bar{\sigma}} q_r) \right] \\
& -\frac{i}{6} y_d^{vu} \bar{y}_d^{tu} (\mathcal{C}_{qd}^{(1)})^{tv sr} (\Omega_d^\dagger \overset{\leftrightarrow}{D}_{\bar{\mu}} \Omega_d) (H^\dagger H) (\bar{d}_s \gamma^{\bar{\mu}} d_r) - \frac{i}{6} y_d^{tv} \bar{y}_d^{tu} (\mathcal{C}_{qd}^{(1)})^{sr vu} (\Omega_{q,j}^* \overset{\leftrightarrow}{D}_{\bar{\mu}} \Omega_q^i) H_i^\dagger H^j (\bar{q}_s \gamma^{\bar{\mu}} q_r) \\
& -\frac{i}{6} y_u^{vu} \bar{y}_u^{tu} (\mathcal{C}_{qd}^{(1)})^{tv sr} (\Omega_u^\dagger \overset{\leftrightarrow}{D}_{\bar{\mu}} \Omega_u) (H^\dagger H) (\bar{d}_s \gamma^{\bar{\mu}} d_r) \\
& -\frac{i}{3} g_s (\mathcal{C}_{qd}^{(1)})^{ttsr} \left[ 2T_b^{Aa} (\Omega_{q,a}^* D_{\bar{\sigma}} \Omega_q^b) \tilde{G}^{\bar{\rho}\bar{\sigma} A} (\bar{d}_s \gamma^{\bar{\rho}} d_r) + 2T_b^{Aa} (D_{\bar{\mu}} \Omega_{q,a}^* \Omega_q^b) \tilde{G}^{\bar{\mu}\bar{\sigma} A} (\bar{d}_s \gamma^{\bar{\sigma}} d_r) \right] \\
& -\frac{i}{3} g_L (\mathcal{C}_{qd}^{(1)})^{ttsr} \left[ 2t_j^{Ii} (\Omega_{q,i}^* D_{\bar{\sigma}} \Omega_q^j) \tilde{W}^{\bar{\rho}\bar{\sigma} I} (\bar{d}_s \gamma^{\bar{\rho}} d_r) + 2t_j^{Ii} (D_{\bar{\mu}} \Omega_{q,i}^* \Omega_q^j) \tilde{W}^{\bar{\mu}\bar{\sigma} I} (\bar{d}_s \gamma^{\bar{\sigma}} d_r) \right] \\
& +\frac{i}{3} (\mathcal{C}_{qd}^{(1)})^{ttsr} \left[ (\Omega_q^\dagger D_{\bar{\nu}} \Omega_q) (D^{\bar{\mu}} \bar{d}_s \gamma^{\bar{\nu}} D^{\bar{\mu}} d_r) - (D_{\bar{\mu}} \Omega_q^\dagger \Omega_q) (D^{\bar{\nu}} \bar{d}_s \gamma^{\bar{\mu}} D^{\bar{\nu}} d_r) \right] \\
& +\frac{i}{3} (\mathcal{C}_{qd}^{(1)})^{ttsr} \left[ (\Omega_q^\dagger D_{\bar{\nu}} \Omega_q) (D^{\bar{\mu}} D^{\bar{\mu}} \bar{d}_s \gamma^{\bar{\nu}} d_r) - (D_{\bar{\mu}} \Omega_q^\dagger \Omega_q) (\bar{d}_s \gamma^{\bar{\mu}} D^{\bar{\nu}} D^{\bar{\nu}} d_r) \right] \\
& +\frac{i}{3} g_s (\mathcal{C}_{qd}^{(1)})^{srtt} \left[ 2T_b^{Aa} (\Omega_{d,a}^* D_{\bar{\sigma}} \Omega_d^b) \tilde{G}^{\bar{\rho}\bar{\sigma} A} (\bar{q}_s \gamma^{\bar{\rho}} q_r) + 2T_b^{Aa} (D_{\bar{\mu}} \Omega_{d,a}^* \Omega_d^b) \tilde{G}^{\bar{\mu}\bar{\sigma} A} (\bar{q}_s \gamma^{\bar{\sigma}} q_r) \right] \\
& +\frac{i}{3} (\mathcal{C}_{qd}^{(1)})^{srtt} \left[ (\Omega_d^\dagger D_{\bar{\nu}} \Omega_d) (D^{\bar{\mu}} \bar{q}_s \gamma^{\bar{\nu}} D^{\bar{\mu}} q_r) - (D_{\bar{\mu}} \Omega_d^\dagger \Omega_d) (D^{\bar{\nu}} \bar{q}_s \gamma^{\bar{\mu}} D^{\bar{\nu}} q_r) \right] \\
& +\frac{i}{3} (\mathcal{C}_{qd}^{(1)})^{srtt} \left[ (\Omega_d^\dagger D_{\bar{\nu}} \Omega_d) (D^{\bar{\mu}} D^{\bar{\mu}} \bar{q}_s \gamma^{\bar{\nu}} q_r) - (D_{\bar{\mu}} \Omega_d^\dagger \Omega_d) (\bar{q}_s \gamma^{\bar{\mu}} D^{\bar{\nu}} D^{\bar{\nu}} q_r) \right] \\
& +\frac{2}{3} \bar{y}_d^{tu} (\mathcal{C}_{qd}^{(1)})^{tr su} (D_{\bar{\mu}} \Omega_{q,aj}^* D_{\bar{\mu}} \Omega_q^{bi}) H_i^\dagger (\bar{d}_{bs} q_r^{aj}) + \frac{2}{3} \bar{y}_d^{tu} (\mathcal{C}_{qd}^{(1)})^{tr su} (D_{\bar{\mu}} \Omega_{q,aj}^* \Omega_q^{bi}) H_i^\dagger (\bar{d}_{bs} D^{\bar{\mu}} q_r^{aj}) \\
& +\frac{2}{3} \bar{y}_d^{tu} (\mathcal{C}_{qd}^{(1)})^{tr su} (D_{\bar{\mu}} \Omega_{d,a}^* D_{\bar{\mu}} \Omega_d^b) (\bar{d}_{bs} H^\dagger q_r^a) + \frac{2}{3} \bar{y}_d^{tu} (\mathcal{C}_{qd}^{(1)})^{tr su} (D_{\bar{\mu}} \Omega_{d,a}^* \Omega_d^b) (\bar{d}_{bs} D_{\bar{\mu}} H^\dagger q_r^a) \\
& +\frac{2}{3} \bar{y}_d^{tu} (\mathcal{C}_{qd}^{(1)})^{tr su} (D_{\bar{\mu}} \Omega_{q,aj}^* \Omega_q^{bi}) H_i^\dagger (D^{\bar{\mu}} \bar{d}_{bs} q_r^{aj}) + \frac{2}{3} y_d^{tu} (\mathcal{C}_{qd}^{(1)})^{stur} (D_{\bar{\mu}} \Omega_{d,a}^* D_{\bar{\mu}} \Omega_d^b) (\bar{q}_{bs} H d_r^a) \\
& +\frac{2}{3} y_d^{tu} (\mathcal{C}_{qd}^{(1)})^{stur} (\Omega_{d,a}^* D_{\bar{\mu}} \Omega_d^b) (\bar{q}_{bs} D_{\bar{\mu}} H d_r^a) + \frac{2}{3} y_d^{tu} (\mathcal{C}_{qd}^{(1)})^{stur} (D_{\bar{\mu}} \Omega_{q,ai}^* D_{\bar{\mu}} \Omega_q^{bj}) H^i (\bar{q}_{bj} d_r^a) \\
& +\frac{2}{3} y_d^{tu} (\mathcal{C}_{qd}^{(1)})^{stur} (\Omega_{q,ai}^* D_{\bar{\mu}} \Omega_q^{bj}) H^i (\bar{q}_{bj} s D^{\bar{\mu}} d_r^a) + \frac{2}{3} y_d^{tu} (\mathcal{C}_{qd}^{(1)})^{stur} (\Omega_{q,ai}^* D_{\bar{\mu}} \Omega_q^{bj}) H^i (D^{\bar{\mu}} \bar{q}_{bj} s d_r^a) \\
& -\frac{2}{3} \bar{y}_d^{tu} (\mathcal{C}_{qd}^{(1)})^{tr su} (D_{\bar{\mu}} \Omega_{q,aj}^* \Omega_q^{bi}) D^{\bar{\mu}} H_i^\dagger (\bar{d}_{bs} q_r^{aj}) - \frac{2}{3} \bar{y}_d^{tu} (\mathcal{C}_{qd}^{(1)})^{tr su} (D_{\bar{\mu}} \Omega_{d,a}^* \Omega_d^b) (\bar{d}_{bs} H^\dagger D^{\bar{\mu}} q_r^a) \\
& -\frac{2}{3} \bar{y}_d^{tu} (\mathcal{C}_{qd}^{(1)})^{tr su} (D_{\bar{\mu}} \Omega_{d,a}^* \Omega_d^b) (D^{\bar{\mu}} \bar{d}_{bs} H^\dagger q_r^a) - \frac{2}{3} \bar{y}_d^{tu} (\mathcal{C}_{qd}^{(1)})^{tr su} (D_{\bar{\mu}} \Omega_{d,a}^* \Omega_d^c) (D_{\bar{\mu}} \Omega_{q,bj}^* \Omega_q^{ai}) H_i^\dagger (\bar{d}_{cs} q_r^{bj}) \\
& -\frac{2}{3} y_d^{tu} (\mathcal{C}_{qd}^{(1)})^{stur} (\Omega_{d,a}^* D_{\bar{\mu}} \Omega_d^b) (\bar{q}_{bs} H D^{\bar{\mu}} d_r^a) - \frac{2}{3} y_d^{tu} (\mathcal{C}_{qd}^{(1)})^{stur} (\Omega_{d,a}^* D_{\bar{\mu}} \Omega_d^b) (D^{\bar{\mu}} \bar{q}_{bs} H d_r^a)
\end{aligned}$$

$$\begin{aligned}
& -\frac{2}{3}y_d^{tu}(\mathcal{C}_{qd}^{(1)})^{stur}(\Omega_{q,ai}^*D_{\bar{\mu}}\Omega_q^{bj})D^{\bar{\mu}}H^i(\bar{q}_{bjs}d_r^a) - \frac{2}{3}y_d^{tu}(\mathcal{C}_{qd}^{(1)})^{stur}(\Omega_{d,a}^*D_{\bar{\mu}}\Omega_d^b)(\Omega_{q,bi}^*D_{\bar{\mu}}\Omega_q^{cj})H^i(\bar{q}_{cjs}d_r^a) \\
& + \frac{2i}{3}y_d^{tv}\bar{y}_d^{tu}(\mathcal{C}_{qd}^{(1)})^{srvu}(\Omega_d^{\dagger}\overset{\leftrightarrow}{D}_{\bar{\mu}}\Omega_d)(H^{\dagger}H)(\bar{q}_s\gamma^{\bar{\mu}}q_r) + \frac{2i}{3}y_u^{vu}\bar{y}_u^{tu}(\mathcal{C}_{qd}^{(1)})^{tvsr}(\Omega_q^{\dagger}\overset{\leftrightarrow}{D}_{\bar{\mu}}\Omega_q)(H^{\dagger}H)(\bar{d}_s\gamma^{\bar{\mu}}d_r) \\
& + \frac{2i}{3}(\mathcal{C}_{qd}^{(1)})^{tvsr}\left[y_d^{vu}\bar{y}_d^{tu} - y_u^{vu}\bar{y}_u^{tu}\right](\Omega_{q,j}^*\overset{\leftrightarrow}{D}_{\bar{\mu}}\Omega_q^i)H_i^{\dagger}H^j(\bar{d}_s\gamma^{\bar{\mu}}d_r), \tag{3.56}
\end{aligned}$$

$$\begin{aligned}
\Gamma_{\Omega}^{(1)}[\mathcal{O}_{qd}^{(8)}] &= \frac{i}{108}g_Y(\mathcal{C}_{qd}^{(8)})^{ttsr}\left[2(\Omega_q^{\dagger}D_{\bar{\sigma}}\Omega_q)\tilde{B}^{\bar{\rho}\bar{\sigma}}(\bar{d}_s\gamma^{\bar{\rho}}d_r) + 2(D_{\bar{\mu}}\Omega_q^{\dagger}\Omega_q)\tilde{B}^{\bar{\mu}\bar{\sigma}}(\bar{d}_s\gamma^{\bar{\sigma}}d_r)\right] \\
& + \frac{i}{54}g_Y(\mathcal{C}_{qd}^{(8)})^{srtt}\left[2(\Omega_d^{\dagger}D_{\bar{\sigma}}\Omega_d)\tilde{B}^{\bar{\rho}\bar{\sigma}}(\bar{q}_s\gamma^{\bar{\rho}}q_r) + 2(D_{\bar{\mu}}\Omega_d^{\dagger}\Omega_d)\tilde{B}^{\bar{\mu}\bar{\sigma}}(\bar{q}_s\gamma^{\bar{\sigma}}q_r)\right] \\
& - \frac{i}{36}(\mathcal{C}_{qd}^{(8)})^{ttsr}\left[(\Omega_q^{\dagger}D_2D_{\bar{\mu}}\Omega_q)(\bar{d}_s\gamma^{\bar{\mu}}d_r) - (D_2D_{\bar{\nu}}\Omega_q^{\dagger}\Omega_q)(\bar{d}_s\gamma^{\bar{\nu}}d_r)\right] \\
& - \frac{1}{36}(\mathcal{C}_{qd}^{(8)})^{ttsr}\left[(D_{\bar{\mu}}\Omega_{q,ai}^*D_{\bar{\rho}}\Omega_q^{bj})(\Omega_{q,bj}^*D_{\bar{\sigma}}\Omega_q^{ai})\varepsilon^{\bar{\mu}\bar{\nu}\bar{\rho}\bar{\sigma}}(\bar{d}_s\gamma^{\bar{\nu}}d_r) - (D_{\bar{\mu}}\Omega_{q,ai}^*\Omega_q^{bj})(D_{\bar{\nu}}\Omega_{q,bj}^*D_{\bar{\rho}}\Omega_q^{ai})\varepsilon^{\bar{\mu}\bar{\nu}\bar{\rho}\bar{\sigma}}(\bar{d}_s\gamma^{\bar{\sigma}}d_r)\right] \\
& + \frac{i}{36}g_Y(\mathcal{C}_{qd}^{(8)})^{ttsr}\left[2(\Omega_{q,a}^*D_{\bar{\rho}}\Omega_q^b)\tilde{B}^{\bar{\rho}\bar{\sigma}}(\bar{d}_{bs}\gamma^{\bar{\sigma}}d_r^a) - 2(D_{\bar{\mu}}\Omega_{q,a}^*\Omega_q^b)\tilde{B}^{\bar{\mu}\bar{\sigma}}(\bar{d}_{bs}\gamma^{\bar{\sigma}}d_r^a)\right] \\
& - \frac{i}{36}(\mathcal{C}_{qd}^{(8)})^{srtt}\left[(\Omega_d^{\dagger}D_2D_{\bar{\mu}}\Omega_d)(\bar{q}_s\gamma^{\bar{\mu}}q_r) - (D_2D_{\bar{\nu}}\Omega_d^{\dagger}\Omega_d)(\bar{q}_s\gamma^{\bar{\nu}}q_r)\right] \\
& + \frac{1}{36}(\mathcal{C}_{qd}^{(8)})^{srtt}\left[(D_{\bar{\mu}}\Omega_{d,a}^*D_{\bar{\rho}}\Omega_d^b)(\Omega_{d,b}^*D_{\bar{\sigma}}\Omega_d^a)\varepsilon^{\bar{\mu}\bar{\nu}\bar{\rho}\bar{\sigma}}(\bar{q}_s\gamma^{\bar{\nu}}q_r) - (D_{\bar{\mu}}\Omega_{d,a}^*\Omega_d^b)(D_{\bar{\nu}}\Omega_{d,b}^*D_{\bar{\rho}}\Omega_d^a)\varepsilon^{\bar{\mu}\bar{\nu}\bar{\rho}\bar{\sigma}}(\bar{q}_s\gamma^{\bar{\sigma}}q_r)\right] \\
& + \frac{i}{36}y_d^{vu}\bar{y}_d^{tu}(\mathcal{C}_{qd}^{(8)})^{tvsr}(\Omega_d^{\dagger}\overset{\leftrightarrow}{D}_{\bar{\mu}}\Omega_d)(H^{\dagger}H)(\bar{d}_s\gamma^{\bar{\mu}}d_r) + \frac{i}{36}y_d^{tv}\bar{y}_d^{tu}(\mathcal{C}_{qd}^{(8)})^{srvu}(\Omega_{q,j}^*\overset{\leftrightarrow}{D}_{\bar{\mu}}\Omega_q^i)H_i^{\dagger}H^j(\bar{q}_s\gamma^{\bar{\mu}}q_r) \\
& + \frac{i}{36}y_u^{vu}\bar{y}_u^{tu}(\mathcal{C}_{qd}^{(8)})^{tvsr}(\Omega_u^{\dagger}\overset{\leftrightarrow}{D}_{\bar{\mu}}\Omega_u)(H^{\dagger}H)(\bar{d}_s\gamma^{\bar{\mu}}d_r) \\
& + \frac{i}{18}g_s(\mathcal{C}_{qd}^{(8)})^{ttsr}\left[2T_b^{Aa}(\Omega_{q,a}^*D_{\bar{\sigma}}\Omega_q^b)\tilde{G}^{\bar{\rho}\bar{\sigma}A}(\bar{d}_s\gamma^{\bar{\rho}}d_r) + 2T_b^{Aa}(D_{\bar{\mu}}\Omega_{q,a}^*\Omega_q^b)\tilde{G}^{\bar{\mu}\bar{\sigma}A}(\bar{d}_s\gamma^{\bar{\sigma}}d_r)\right] \\
& + \frac{i}{18}g_L(\mathcal{C}_{qd}^{(8)})^{ttsr}\left[2t_j^{Li}(\Omega_{q,i}^*D_{\bar{\sigma}}\Omega_q^j)\tilde{W}^{\bar{\rho}\bar{\sigma}I}(\bar{d}_s\gamma^{\bar{\rho}}d_r) + 2t_j^{Li}(D_{\bar{\mu}}\Omega_{q,i}^*\Omega_q^j)\tilde{W}^{\bar{\mu}\bar{\sigma}I}(\bar{d}_s\gamma^{\bar{\sigma}}d_r)\right] \\
& - \frac{i}{18}(\mathcal{C}_{qd}^{(8)})^{ttsr}\left[(\Omega_q^{\dagger}D_{\bar{\nu}}\Omega_q)(D^{\bar{\mu}}\bar{d}_s\gamma^{\bar{\nu}}D^{\bar{\mu}}d_r) - (D_{\bar{\mu}}\Omega_q^{\dagger}\Omega_q)(D^{\bar{\nu}}\bar{d}_s\gamma^{\bar{\mu}}D^{\bar{\nu}}d_r)\right] \\
& - \frac{i}{18}(\mathcal{C}_{qd}^{(8)})^{ttsr}\left[(\Omega_q^{\dagger}D_{\bar{\nu}}\Omega_q)(D^{\bar{\mu}}D^{\bar{\mu}}\bar{d}_s\gamma^{\bar{\nu}}d_r) - (D_{\bar{\mu}}\Omega_q^{\dagger}\Omega_q)(\bar{d}_s\gamma^{\bar{\mu}}D^{\bar{\nu}}D^{\bar{\nu}}d_r)\right] \\
& - \frac{i}{18}g_s(\mathcal{C}_{qd}^{(8)})^{srtt}\left[2T_b^{Aa}(\Omega_{d,a}^*D_{\bar{\sigma}}\Omega_d^b)\tilde{G}^{\bar{\rho}\bar{\sigma}A}(\bar{q}_s\gamma^{\bar{\rho}}q_r) + 2T_b^{Aa}(D_{\bar{\mu}}\Omega_{d,a}^*\Omega_d^b)\tilde{G}^{\bar{\mu}\bar{\sigma}A}(\bar{q}_s\gamma^{\bar{\sigma}}q_r)\right] \\
& - \frac{i}{18}(\mathcal{C}_{qd}^{(8)})^{srtt}\left[(\Omega_d^{\dagger}D_{\bar{\nu}}\Omega_d)(D^{\bar{\mu}}\bar{q}_s\gamma^{\bar{\nu}}D^{\bar{\mu}}q_r) - (D_{\bar{\mu}}\Omega_d^{\dagger}\Omega_d)(D^{\bar{\nu}}\bar{q}_s\gamma^{\bar{\mu}}D^{\bar{\nu}}q_r)\right] \\
& - \frac{i}{18}(\mathcal{C}_{qd}^{(8)})^{srtt}\left[(\Omega_d^{\dagger}D_{\bar{\nu}}\Omega_d)(D^{\bar{\mu}}D^{\bar{\mu}}\bar{q}_s\gamma^{\bar{\nu}}q_r) - (D_{\bar{\mu}}\Omega_d^{\dagger}\Omega_d)(\bar{q}_s\gamma^{\bar{\mu}}D^{\bar{\nu}}D^{\bar{\nu}}q_r)\right] \\
& + \frac{i}{18}g_Y(\mathcal{C}_{qd}^{(8)})^{srtt}\left[2(\Omega_{d,a}^*D_{\bar{\rho}}\Omega_d^b)\tilde{B}^{\bar{\rho}\bar{\sigma}}(\bar{q}_{bs}\gamma^{\bar{\sigma}}q_r^a) - 2(D_{\bar{\mu}}\Omega_{d,a}^*\Omega_d^b)\tilde{B}^{\bar{\mu}\bar{\sigma}}(\bar{q}_{bs}\gamma^{\bar{\sigma}}q_r^a)\right] \\
& + \frac{i}{12}(\mathcal{C}_{qd}^{(8)})^{ttsr}\left[(\Omega_{q,a}^*D_2D_{\bar{\mu}}\Omega_q^b)(\bar{d}_{bs}\gamma^{\bar{\mu}}d_r^a) - (D_2D_{\bar{\nu}}\Omega_{q,a}^*\Omega_q^b)(\bar{d}_{bs}\gamma^{\bar{\nu}}d_r^a)\right] \\
& - \frac{i}{12}(\mathcal{C}_{qd}^{(8)})^{ttsr}\left[(D_{\bar{\mu}}D_{\bar{\nu}}\Omega_{q,ai}^*\Omega_q^{cj})(\Omega_{q,bj}^*D_{\bar{\mu}}\Omega_q^{ai})(\bar{d}_{cs}\gamma^{\bar{\nu}}d_r^b) - (D_{\bar{\mu}}\Omega_{q,ai}^*\Omega_q^{cj})(\Omega_{q,bj}^*D_{\bar{\mu}}D_{\bar{\nu}}\Omega_q^{ai})(\bar{d}_{cs}\gamma^{\bar{\nu}}d_r^b)\right] \\
& + \frac{i}{12}(\mathcal{C}_{qd}^{(8)})^{ttsr}\left[(\Omega_{q,ai}^*D_{\bar{\nu}}\Omega_q^{cj})(D_{\bar{\mu}}\Omega_{q,bj}^*D_{\bar{\nu}}\Omega_q^{ai})(\bar{d}_{cs}\gamma^{\bar{\mu}}d_r^b) - (D_{\bar{\mu}}\Omega_{q,ai}^*D_{\bar{\nu}}\Omega_q^{cj})(D_{\bar{\mu}}\Omega_{q,bj}^*\Omega_q^{ai})(\bar{d}_{cs}\gamma^{\bar{\nu}}d_r^b)\right]
\end{aligned}$$

$$\begin{aligned}
& + \frac{i}{12}(\mathcal{C}_{qd}^{(8)})^{srtt} \left[ (\Omega_{d,a}^* D_2 D_{\bar{\mu}} \Omega_d^b) (\bar{q}_{bs} \gamma^{\bar{\mu}} q_r^a) - (D_2 D_{\bar{\nu}} \Omega_{d,a}^* \Omega_d^b) (\bar{q}_{bs} \gamma^{\bar{\nu}} q_r^a) \right] \\
& - \frac{i}{12}(\mathcal{C}_{qd}^{(8)})^{srtt} \left[ (D_{\bar{\mu}} D_{\bar{\nu}} \Omega_{d,a}^* \Omega_d^c) (\Omega_{d,b}^* D_{\bar{\mu}} \Omega_d^a) (\bar{q}_{cs} \gamma^{\bar{\nu}} q_r^b) - (D_{\bar{\mu}} \Omega_{d,a}^* \Omega_d^c) (\Omega_{d,b}^* D_{\bar{\mu}} D_{\bar{\nu}} \Omega_d^a) (\bar{q}_{cs} \gamma^{\bar{\nu}} q_r^b) \right] \\
& + \frac{i}{12}(\mathcal{C}_{qd}^{(8)})^{srtt} \left[ (\Omega_{d,a}^* D_{\bar{\nu}} \Omega_d^c) (D_{\bar{\mu}} \Omega_{d,b}^* D_{\bar{\nu}} \Omega_d^a) (\bar{q}_{cs} \gamma^{\bar{\mu}} q_r^b) - (D_{\bar{\mu}} \Omega_{d,a}^* D_{\bar{\nu}} \Omega_d^c) (D_{\bar{\mu}} \Omega_{d,b}^* \Omega_d^a) (\bar{q}_{cs} \gamma^{\bar{\nu}} q_r^b) \right] \\
& + \frac{1}{12}(\mathcal{C}_{qd}^{(8)})^{srtt} \left[ (\Omega_{d,a}^* D_{\bar{\rho}} \Omega_d^c) (D_{\bar{\mu}} \Omega_{d,b}^* D_{\bar{\sigma}} \Omega_d^a) \varepsilon^{\bar{\mu}\bar{\nu}\bar{\rho}\bar{\sigma}} (\bar{q}_{cs} \gamma^{\bar{\nu}} q_r^b) - (D_{\bar{\mu}} \Omega_{d,a}^* D_{\bar{\rho}} \Omega_d^c) (D_{\bar{\nu}} \Omega_{d,b}^* \Omega_d^a) \varepsilon^{\bar{\mu}\bar{\nu}\bar{\rho}\bar{\sigma}} (\bar{q}_{cs} \gamma^{\bar{\sigma}} q_r^b) \right] \\
& + \frac{i}{12}(\mathcal{C}_{qd}^{(8)})^{srtt} \left[ (\Omega_{d,a}^* D_{\bar{\nu}} \Omega_d^c) (\Omega_{d,b}^* D_{\bar{\mu}} \Omega_d^a) (D_{\bar{\mu}} \bar{q}_{cs} \gamma^{\bar{\nu}} q_r^b) - (D_{\bar{\mu}} \Omega_{d,a}^* \Omega_d^c) (D_{\bar{\nu}} \Omega_{d,b}^* \Omega_d^a) (\bar{q}_{cs} \gamma^{\bar{\nu}} D_{\bar{\mu}} q_r^b) \right] \\
& + \frac{i}{12}(\mathcal{C}_{qd}^{(8)})^{srtt} \left[ (\Omega_{d,a}^* D_{\bar{\mu}} \Omega_d^c) (\Omega_{d,b}^* D_{\bar{\nu}} \Omega_d^a) (\bar{q}_{cs} \gamma^{\bar{\mu}} D_{\bar{\nu}} q_r^b) - (D_{\bar{\mu}} \Omega_{d,a}^* \Omega_d^c) (D_{\bar{\nu}} \Omega_{d,b}^* \Omega_d^a) (D_{\bar{\mu}} \bar{q}_{cs} \gamma^{\bar{\nu}} q_r^b) \right] \\
& - \frac{i}{12} y_d^{vu} \bar{y}_d^{tu} (\mathcal{C}_{qd}^{(8)})^{tvsr} (\Omega_{d,a}^* \overleftrightarrow{D}_{\bar{\mu}} \Omega_d^b) (H^\dagger H) (\bar{d}_{bs} \gamma^{\bar{\mu}} d_r^a) - \frac{i}{12} y_d^{tv} \bar{y}_d^{tu} (\mathcal{C}_{qd}^{(8)})^{srvu} (\Omega_{q,aj}^* \overleftrightarrow{D}_{\bar{\mu}} \Omega_q^{bi}) H_i^\dagger H^j (\bar{q}_{bs} \gamma^{\bar{\mu}} q_r^a) \\
& - \frac{i}{12} y_u^{vu} \bar{y}_u^{tu} (\mathcal{C}_{qd}^{(8)})^{tvsr} (\Omega_{u,a}^* \overleftrightarrow{D}_{\bar{\mu}} \Omega_u^b) (H^\dagger H) (\bar{d}_{bs} \gamma^{\bar{\mu}} d_r^a) + \frac{1}{9} \bar{y}_d^{tu} (\mathcal{C}_{qd}^{(8)})^{trsu} (D_{\bar{\mu}} \Omega_{q,aj}^* \Omega_q^{bi}) D_{\bar{\mu}} H_i^\dagger (\bar{d}_{bs} q_r^{aj}) \\
& + \frac{1}{9} \bar{y}_d^{tu} (\mathcal{C}_{qd}^{(8)})^{trsu} (D_{\bar{\mu}} \Omega_{d,a}^* \Omega_d^b) (\bar{d}_{bs} H^\dagger D_{\bar{\mu}} q_r^a) + \frac{1}{9} \bar{y}_d^{tu} (\mathcal{C}_{qd}^{(8)})^{trsu} (D_{\bar{\mu}} \Omega_{d,a}^* \Omega_d^b) (D_{\bar{\mu}} \bar{d}_{bs} H^\dagger q_r^a) \\
& + \frac{1}{9} \bar{y}_d^{tu} (\mathcal{C}_{qd}^{(8)})^{trsu} (D_{\bar{\mu}} \Omega_{d,a}^* \Omega_d^c) (D_{\bar{\mu}} \Omega_{q,bj}^* \Omega_q^{ai}) H_i^\dagger (\bar{d}_{cs} q_r^{bj}) + \frac{1}{9} \bar{y}_d^{tu} (\mathcal{C}_{qd}^{(8)})^{stur} (\Omega_{d,a}^* D_{\bar{\mu}} \Omega_d^b) (\bar{q}_{bs} H D_{\bar{\mu}} d_r^a) \\
& + \frac{1}{9} \bar{y}_d^{tu} (\mathcal{C}_{qd}^{(8)})^{stur} (\Omega_{d,a}^* D_{\bar{\mu}} \Omega_d^b) (D_{\bar{\mu}} \bar{q}_{bs} H d_r^a) + \frac{1}{9} \bar{y}_d^{tu} (\mathcal{C}_{qd}^{(8)})^{stur} (\Omega_{q,ai}^* D_{\bar{\mu}} \Omega_q^{bj}) D_{\bar{\mu}} H^i (\bar{q}_{bj} s d_r^a) \\
& + \frac{1}{9} \bar{y}_d^{tu} (\mathcal{C}_{qd}^{(8)})^{stur} (\Omega_{d,a}^* D_{\bar{\mu}} \Omega_d^b) (\Omega_{q,bi}^* D_{\bar{\mu}} \Omega_q^{cj}) H^i (\bar{q}_{cj} s d_r^a) + \frac{1}{3} \bar{y}_d^{tu} (\mathcal{C}_{qd}^{(8)})^{trsu} (D_{\bar{\mu}} \Omega_{q,j}^* D_{\bar{\mu}} \Omega_q^i) H_i^\dagger (\bar{d}_s q_r^j) \\
& + \frac{1}{3} \bar{y}_d^{tu} (\mathcal{C}_{qd}^{(8)})^{trsu} (D_{\bar{\mu}} \Omega_{q,j}^* \Omega_q^i) H_i^\dagger (\bar{d}_s D_{\bar{\mu}} q_r^j) + \frac{1}{3} \bar{y}_d^{tu} (\mathcal{C}_{qd}^{(8)})^{trsu} (D_{\bar{\mu}} \Omega_d^\dagger D_{\bar{\mu}} \Omega_d) (\bar{d}_s H^\dagger q_r) \\
& + \frac{1}{3} \bar{y}_d^{tu} (\mathcal{C}_{qd}^{(8)})^{trsu} (D_{\bar{\mu}} \Omega_d^\dagger \Omega_d) (\bar{d}_s D_{\bar{\mu}} H^\dagger q_r) + \frac{1}{3} \bar{y}_d^{tu} (\mathcal{C}_{qd}^{(8)})^{trsu} (D_{\bar{\mu}} \Omega_{q,j}^* \Omega_q^i) H_i^\dagger (D_{\bar{\mu}} \bar{d}_s q_r^j) \\
& + \frac{1}{3} \bar{y}_d^{tu} (\mathcal{C}_{qd}^{(8)})^{stur} (\Omega_d^\dagger D_{\bar{\mu}} \Omega_d) (\bar{q}_s D_{\bar{\mu}} H d_r) + \frac{1}{3} \bar{y}_d^{tu} (\mathcal{C}_{qd}^{(8)})^{stur} (D_{\bar{\mu}} \Omega_{q,i}^* D_{\bar{\mu}} \Omega_q^j) H^i (\bar{q}_{js} d_r) + \frac{1}{3} \bar{y}_d^{tu} (\mathcal{C}_{qd}^{(8)})^{stur} (\Omega_{q,i}^* D_{\bar{\mu}} \Omega_q^j) H^i (\bar{q}_{js} L) \\
& + \frac{1}{3} \bar{y}_d^{tu} (\mathcal{C}_{qd}^{(8)})^{stur} (\Omega_{q,i}^* D_{\bar{\mu}} \Omega_q^j) H^i (D_{\bar{\mu}} \bar{q}_{js} d_r) \\
& - \frac{1}{12} (\mathcal{C}_{qd}^{(8)})^{ttsr} \left[ (\Omega_{q,ai}^* D_{\bar{\rho}} \Omega_q^{cj}) (D_{\bar{\mu}} \Omega_{q,bj}^* D_{\bar{\sigma}} \Omega_q^{ai}) \varepsilon^{\bar{\mu}\bar{\nu}\bar{\rho}\bar{\sigma}} (\bar{d}_{cs} \gamma^{\bar{\nu}} d_r^b) - (D_{\bar{\mu}} \Omega_{q,ai}^* D_{\bar{\rho}} \Omega_q^{cj}) (D_{\bar{\nu}} \Omega_{q,bj}^* \Omega_q^{ai}) \varepsilon^{\bar{\mu}\bar{\nu}\bar{\rho}\bar{\sigma}} (\bar{d}_{cs} \gamma^{\bar{\sigma}} d_r^b) \right] \\
& + \frac{i}{12} (\mathcal{C}_{qd}^{(8)})^{ttsr} \left[ (\Omega_{q,ai}^* D_{\bar{\nu}} \Omega_q^{cj}) (\Omega_{q,bj}^* D_{\bar{\mu}} \Omega_q^{ai}) (D_{\bar{\mu}} \bar{d}_{cs} \gamma^{\bar{\nu}} d_r^b) - (D_{\bar{\mu}} \Omega_{q,ai}^* \Omega_q^{cj}) (D_{\bar{\nu}} \Omega_{q,bj}^* \Omega_q^{ai}) (\bar{d}_{cs} \gamma^{\bar{\nu}} D_{\bar{\mu}} d_r^b) \right] \\
& + \frac{i}{12} (\mathcal{C}_{qd}^{(8)})^{ttsr} \left[ (\Omega_{q,ai}^* D_{\bar{\mu}} \Omega_q^{cj}) (\Omega_{q,bj}^* D_{\bar{\nu}} \Omega_q^{ai}) (\bar{d}_{cs} \gamma^{\bar{\mu}} D_{\bar{\nu}} d_r^b) - (D_{\bar{\mu}} \Omega_{q,ai}^* \Omega_q^{cj}) (D_{\bar{\nu}} \Omega_{q,bj}^* \Omega_q^{ai}) (D_{\bar{\mu}} \bar{d}_{cs} \gamma^{\bar{\nu}} d_r^b) \right] \\
& - \frac{1}{9} \bar{y}_d^{tu} (\mathcal{C}_{qd}^{(8)})^{trsu} (D_{\bar{\mu}} \Omega_{q,aj}^* D_{\bar{\mu}} \Omega_q^{bi}) H_i^\dagger (\bar{d}_{bs} q_r^{aj}) - \frac{1}{9} \bar{y}_d^{tu} (\mathcal{C}_{qd}^{(8)})^{trsu} (D_{\bar{\mu}} \Omega_{q,aj}^* \Omega_q^{bi}) H_i^\dagger (\bar{d}_{bs} D_{\bar{\mu}} q_r^{aj}) \\
& - \frac{1}{9} \bar{y}_d^{tu} (\mathcal{C}_{qd}^{(8)})^{trsu} (D_{\bar{\mu}} \Omega_{d,a}^* D_{\bar{\mu}} \Omega_d^b) (\bar{d}_{bs} H^\dagger q_r^a) - \frac{1}{9} \bar{y}_d^{tu} (\mathcal{C}_{qd}^{(8)})^{trsu} (D_{\bar{\mu}} \Omega_{d,a}^* \Omega_d^b) (\bar{d}_{bs} D_{\bar{\mu}} H^\dagger q_r^a) \\
& - \frac{1}{9} \bar{y}_d^{tu} (\mathcal{C}_{qd}^{(8)})^{trsu} (D_{\bar{\mu}} \Omega_{q,aj}^* \Omega_q^{bi}) H_i^\dagger (D_{\bar{\mu}} \bar{d}_{bs} q_r^{aj}) - \frac{1}{9} \bar{y}_d^{tu} (\mathcal{C}_{qd}^{(8)})^{stur} (D_{\bar{\mu}} \Omega_{d,a}^* D_{\bar{\mu}} \Omega_d^b) (\bar{q}_{bs} H d_r^a) \\
& - \frac{1}{9} \bar{y}_d^{tu} (\mathcal{C}_{qd}^{(8)})^{stur} (\Omega_{d,a}^* D_{\bar{\mu}} \Omega_d^b) (\bar{q}_{bs} D_{\bar{\mu}} H d_r^a) - \frac{1}{9} \bar{y}_d^{tu} (\mathcal{C}_{qd}^{(8)})^{stur} (D_{\bar{\mu}} \Omega_{q,ai}^* D_{\bar{\mu}} \Omega_q^{bj}) H^i (\bar{q}_{bj} s d_r^a)
\end{aligned}$$

$$\begin{aligned}
& -\frac{1}{9}y_d^{tu}(\mathcal{C}_{qd}^{(8)})^{stur}(\Omega_{q,ai}^*D_{\bar{\mu}}\Omega_q^{bj})H^i(\bar{q}_{bjs}D^{\bar{\mu}}d_r^a) - \frac{1}{9}y_d^{tu}(\mathcal{C}_{qd}^{(8)})^{stur}(\Omega_{q,ai}^*D_{\bar{\mu}}\Omega_q^{bj})H^i(D^{\bar{\mu}}\bar{q}_{bjs}d_r^a) \\
& -\frac{i}{9}y_d^{tv}\bar{y}_d^{tu}(\mathcal{C}_{qd}^{(8)})^{srvu}(\Omega_d^{\dagger}\overset{\leftrightarrow}{D}_{\bar{\mu}}\Omega_d)(H^{\dagger}H)(\bar{q}_s\gamma^{\bar{\mu}}q_r) - \frac{i}{9}y_u^{vu}\bar{y}_u^{tu}(\mathcal{C}_{qd}^{(8)})^{tvsr}(\Omega_q^{\dagger}\overset{\leftrightarrow}{D}_{\bar{\mu}}\Omega_q)(H^{\dagger}H)(\bar{d}_s\gamma^{\bar{\mu}}d_r) \\
& -\frac{i}{9}(\mathcal{C}_{qd}^{(8)})^{tvsr}\left[y_d^{vu}\bar{y}_d^{tu} - y_u^{vu}\bar{y}_u^{tu}\right](\Omega_{q,j}^*\overset{\leftrightarrow}{D}_{\bar{\mu}}\Omega_q^i)H_i^{\dagger}H^j(\bar{d}_s\gamma^{\bar{\mu}}d_r) \\
& +\frac{i}{6}g_L(\mathcal{C}_{qd}^{(8)})^{ttsr}\left[2t_j^{Ii}(\Omega_{q,ai}^*D_{\bar{\rho}}\Omega_q^{bj})\widetilde{W}^{\bar{\rho}\bar{\sigma}I}(\bar{d}_{bs}\gamma^{\bar{\sigma}}d_r^a) - 2t_j^{Ii}(D_{\bar{\mu}}\Omega_{q,ai}^*\Omega_q^{bj})\widetilde{W}^{\bar{\mu}\bar{\sigma}I}(\bar{d}_{bs}\gamma^{\bar{\sigma}}d_r^a)\right] \\
& +\frac{i}{6}(\mathcal{C}_{qd}^{(8)})^{ttsr}\left[(\Omega_{q,a}^*D_{\bar{\nu}}\Omega_q^b)(D^{\bar{\mu}}\bar{d}_{bs}\gamma^{\bar{\nu}}D^{\bar{\mu}}d_r^a) - (D_{\bar{\mu}}\Omega_{q,a}^*\Omega_q^b)(D^{\bar{\nu}}\bar{d}_{bs}\gamma^{\bar{\mu}}D^{\bar{\nu}}d_r^a)\right] \\
& +\frac{i}{6}(\mathcal{C}_{qd}^{(8)})^{ttsr}\left[(\Omega_{q,a}^*D_{\bar{\nu}}\Omega_q^b)(D^{\bar{\mu}}D^{\bar{\mu}}\bar{d}_{bs}\gamma^{\bar{\nu}}d_r^a) - (D_{\bar{\mu}}\Omega_{q,a}^*\Omega_q^b)(\bar{d}_{bs}\gamma^{\bar{\mu}}D^{\bar{\nu}}D^{\bar{\nu}}d_r^a)\right] \\
& -\frac{i}{6}(\mathcal{C}_{qd}^{(8)})^{ttsr}\left[(\Omega_{q,ai}^*D_{\bar{\mu}}\Omega_q^{cj})(D_{\bar{\mu}}\Omega_{q,bj}^*D_{\bar{\nu}}\Omega_q^{ai})(\bar{d}_{cs}\gamma^{\bar{\nu}}d_r^b) - (D_{\bar{\mu}}\Omega_{q,ai}^*D_{\bar{\nu}}\Omega_q^{cj})(D_{\bar{\nu}}\Omega_{q,bj}^*\Omega_q^{ai})(\bar{d}_{cs}\gamma^{\bar{\mu}}d_r^b)\right] \\
& +\frac{i}{6}g_s(\mathcal{C}_{qd}^{(8)})^{ttsr}\left[2T_b^{Aa}(\Omega_{q,a}^*D_{\bar{\rho}}\Omega_q^c)\widetilde{G}^{\bar{\rho}\bar{\sigma}A}(\bar{d}_{cs}\gamma^{\bar{\sigma}}d_r^b) - 2T_c^{Ab}(D_{\bar{\mu}}\Omega_{q,a}^*\Omega_q^c)\widetilde{G}^{\bar{\mu}\bar{\sigma}A}(\bar{d}_{bs}\gamma^{\bar{\sigma}}d_r^a)\right] \\
& +\frac{i}{6}(\mathcal{C}_{qd}^{(8)})^{srtt}\left[(\Omega_{d,a}^*D_{\bar{\nu}}\Omega_d^b)(D^{\bar{\mu}}\bar{q}_{bs}\gamma^{\bar{\nu}}D^{\bar{\mu}}q_r^a) - (D_{\bar{\mu}}\Omega_{d,a}^*\Omega_d^b)(D^{\bar{\nu}}\bar{q}_{bs}\gamma^{\bar{\mu}}D^{\bar{\nu}}q_r^a)\right] \\
& +\frac{i}{6}(\mathcal{C}_{qd}^{(8)})^{srtt}\left[(\Omega_{d,a}^*D_{\bar{\nu}}\Omega_d^b)(D^{\bar{\mu}}D^{\bar{\mu}}\bar{q}_{bs}\gamma^{\bar{\nu}}q_r^a) - (D_{\bar{\mu}}\Omega_{d,a}^*\Omega_d^b)(\bar{q}_{bs}\gamma^{\bar{\mu}}D^{\bar{\nu}}D^{\bar{\nu}}q_r^a)\right] \\
& -\frac{i}{6}(\mathcal{C}_{qd}^{(8)})^{srtt}\left[(\Omega_{d,a}^*D_{\bar{\mu}}\Omega_d^c)(D_{\bar{\mu}}\Omega_{d,b}^*D_{\bar{\nu}}\Omega_d^a)(\bar{q}_{cs}\gamma^{\bar{\nu}}q_r^b) - (D_{\bar{\mu}}\Omega_{d,a}^*D_{\bar{\nu}}\Omega_d^c)(D_{\bar{\nu}}\Omega_{d,b}^*\Omega_d^a)(\bar{q}_{cs}\gamma^{\bar{\mu}}q_r^b)\right] \\
& -\frac{i}{6}g_s(\mathcal{C}_{qd}^{(8)})^{srtt}\left[2T_b^{Aa}(\Omega_{d,a}^*D_{\bar{\rho}}\Omega_d^c)\widetilde{G}^{\bar{\rho}\bar{\sigma}A}(\bar{q}_{cs}\gamma^{\bar{\sigma}}q_r^b) - 2T_c^{Ab}(D_{\bar{\mu}}\Omega_{d,a}^*\Omega_d^c)\widetilde{G}^{\bar{\mu}\bar{\sigma}A}(\bar{q}_{bs}\gamma^{\bar{\sigma}}q_r^a)\right] \\
& +\frac{1}{3}y_d^{tu}(\mathcal{C}_{qd}^{(8)})^{stur}(D_{\bar{\mu}}\Omega_d^{\dagger}D_{\bar{\mu}}\Omega_d)(\bar{q}_sHd_r) - \frac{1}{3}\bar{y}_d^{tu}(\mathcal{C}_{qd}^{(8)})^{trsu}(D_{\bar{\mu}}\Omega_{q,j}^*\Omega_q^i)D^{\bar{\mu}}H_i^{\dagger}(\bar{d}_sq_r^j) \\
& -\frac{1}{3}\bar{y}_d^{tu}(\mathcal{C}_{qd}^{(8)})^{trsu}(D_{\bar{\mu}}\Omega_{d,a}^*\Omega_d^b)(D_{\bar{\mu}}\Omega_{q,bj}^*\Omega_q^{ai})H_i^{\dagger}(\bar{d}_sq_r^j) - \frac{1}{3}\bar{y}_d^{tu}(\mathcal{C}_{qd}^{(8)})^{trsu}(D_{\bar{\mu}}\Omega_d^{\dagger}\Omega_d)(\bar{d}_sH^{\dagger}D^{\bar{\mu}}q_r) \\
& -\frac{1}{3}\bar{y}_d^{tu}(\mathcal{C}_{qd}^{(8)})^{trsu}(D_{\bar{\mu}}\Omega_d^{\dagger}\Omega_d)(D^{\bar{\mu}}\bar{d}_sH^{\dagger}q_r) - \frac{1}{3}y_d^{tu}(\mathcal{C}_{qd}^{(8)})^{stur}(\Omega_d^{\dagger}D_{\bar{\mu}}\Omega_d)(\bar{q}_sHD^{\bar{\mu}}d_r) \\
& -\frac{1}{3}y_d^{tu}(\mathcal{C}_{qd}^{(8)})^{stur}(\Omega_d^{\dagger}D_{\bar{\mu}}\Omega_d)(D^{\bar{\mu}}\bar{q}_sHd_r) - \frac{1}{3}y_d^{tu}(\mathcal{C}_{qd}^{(8)})^{stur}(\Omega_{d,a}^*D_{\bar{\mu}}\Omega_d^b)(\Omega_{q,bi}^*D_{\bar{\mu}}\Omega_q^{aj})H^i(\bar{q}_{js}d_r) \\
& -\frac{1}{3}y_d^{tu}(\mathcal{C}_{qd}^{(8)})^{stur}(\Omega_{q,i}^*D_{\bar{\mu}}\Omega_q^j)D^{\bar{\mu}}H^i(\bar{q}_{js}d_r) + \frac{i}{3}y_d^{tv}\bar{y}_d^{tu}(\mathcal{C}_{qd}^{(8)})^{srvu}(\Omega_{d,a}^*\overset{\leftrightarrow}{D}_{\bar{\mu}}\Omega_d^b)(H^{\dagger}H)(\bar{q}_{bs}\gamma^{\bar{\mu}}q_r^a) \\
& +\frac{i}{3}y_u^{vu}\bar{y}_u^{tu}(\mathcal{C}_{qd}^{(8)})^{tvsr}(\Omega_{q,a}^*\overset{\leftrightarrow}{D}_{\bar{\mu}}\Omega_q^b)(H^{\dagger}H)(\bar{d}_{bs}\gamma^{\bar{\mu}}d_r^a) \\
& +\frac{i}{3}(\mathcal{C}_{qd}^{(8)})^{tvsr}\left[y_d^{vu}\bar{y}_d^{tu} - y_u^{vu}\bar{y}_u^{tu}\right](\Omega_{q,aj}^*\overset{\leftrightarrow}{D}_{\bar{\mu}}\Omega_q^{bi})H_i^{\dagger}H^j(\bar{d}_{bs}\gamma^{\bar{\mu}}d_r^a) \\
& -\frac{1}{2}g_s(\mathcal{C}_{qd}^{(8)})^{ttsr}\left[T_b^{Aa}(\Omega_{q,a}^*D_{\bar{\nu}}\Omega_q^c)G^{\bar{\mu}\bar{\nu}A}(\bar{d}_{cs}\gamma^{\bar{\mu}}d_r^b) - T_c^{Ab}(D_{\bar{\mu}}\Omega_{q,a}^*\Omega_q^c)G^{\bar{\mu}\bar{\nu}A}(\bar{d}_{bs}\gamma^{\bar{\nu}}d_r^a)\right] \\
& -\frac{1}{2}g_s(\mathcal{C}_{qd}^{(8)})^{srtt}\left[T_b^{Aa}(\Omega_{d,a}^*D_{\bar{\nu}}\Omega_d^c)G^{\bar{\mu}\bar{\nu}A}(\bar{q}_{cs}\gamma^{\bar{\mu}}q_r^b) - T_c^{Ab}(D_{\bar{\mu}}\Omega_{d,a}^*\Omega_d^c)G^{\bar{\mu}\bar{\nu}A}(\bar{q}_{bs}\gamma^{\bar{\nu}}q_r^a)\right], \tag{3.57}
\end{aligned}$$

$$\begin{aligned}
\Gamma_{\Omega}^{(1)}[\mathcal{O}_{\ell edq}] &= \frac{1}{3}\bar{y}_e^{tu}\mathcal{C}_{\ell edq}^{tusr}(D_{\bar{\mu}}\Omega_{\ell,j}^*\Omega_{\ell}^i)D^{\bar{\mu}}H_i^{\dagger}(\bar{d}_sq_r^j) + \frac{1}{3}\bar{y}_e^{tu}\mathcal{C}_{\ell edq}^{tusr}(D_{\bar{\mu}}\Omega_e^{\dagger}\Omega_e)(D_{\bar{\mu}}\Omega_{\ell,j}^*\Omega_{\ell}^i)H_i^{\dagger}(\bar{d}_sq_r^j) \\
& +\frac{1}{3}\bar{y}_e^{tu}\mathcal{C}_{\ell edq}^{tusr}(D_{\bar{\mu}}\Omega_e^{\dagger}\Omega_e)(\bar{d}_sH^{\dagger}D^{\bar{\mu}}q_r) + \frac{1}{3}\bar{y}_e^{tu}\mathcal{C}_{\ell edq}^{tusr}(D_{\bar{\mu}}\Omega_e^{\dagger}\Omega_e)(D^{\bar{\mu}}\bar{d}_sH^{\dagger}q_r)
\end{aligned}$$

$$\begin{aligned}
& + \frac{1}{3} \bar{y}_d^{ut} \bar{\mathcal{C}}_{ledq}^{rstu} (D_{\bar{\mu}} \Omega_{q,j}^* \Omega_q^i) D^{\bar{\mu}} H_i^\dagger (\bar{e}_s \ell_r^j) + \frac{1}{3} \bar{y}_d^{ut} \bar{\mathcal{C}}_{ledq}^{rstu} (D_{\bar{\mu}} \Omega_{d,a}^* \Omega_d^b) (D_{\bar{\mu}} \Omega_{q,bj}^* \Omega_q^{ai}) H_i^\dagger (\bar{e}_s \ell_r^j) \\
& + \frac{1}{3} \bar{y}_d^{ut} \bar{\mathcal{C}}_{ledq}^{rstu} (D_{\bar{\mu}} \Omega_d^\dagger \Omega_d) (\bar{e}_s H^\dagger D^{\bar{\mu}} \ell_r) + \frac{1}{3} \bar{y}_d^{ut} \bar{\mathcal{C}}_{ledq}^{rstu} (D_{\bar{\mu}} \Omega_d^\dagger \Omega_d) (D^{\bar{\mu}} \bar{e}_s H^\dagger \ell_r) \\
& + \frac{1}{3} \bar{y}_d^{ut} \mathcal{C}_{ledq}^{srtu} (\Omega_d^\dagger D_{\bar{\mu}} \Omega_d) (\bar{\ell}_s H D^{\bar{\mu}} e_r) + \frac{1}{3} \bar{y}_d^{ut} \mathcal{C}_{ledq}^{srtu} (\Omega_d^\dagger D_{\bar{\mu}} \Omega_d) (D^{\bar{\mu}} \bar{\ell}_s H e_r) \\
& + \frac{1}{3} \bar{y}_d^{ut} \mathcal{C}_{ledq}^{srtu} (\Omega_{d,a}^* D_{\bar{\mu}} \Omega_d^b) (\Omega_{q,bi}^* D_{\bar{\mu}} \Omega_q^{aj}) H^i (\bar{\ell}_{js} e_r) + \frac{1}{3} \bar{y}_d^{ut} \mathcal{C}_{ledq}^{srtu} (\Omega_{q,i}^* D_{\bar{\mu}} \Omega_q^j) D^{\bar{\mu}} H^i (\bar{\ell}_{js} e_r) \\
& + \frac{1}{3} \bar{y}_e^{tu} \bar{\mathcal{C}}_{ledq}^{turs} (\Omega_e^\dagger D_{\bar{\mu}} \Omega_e) (\bar{q}_s H D^{\bar{\mu}} d_r) + \frac{1}{3} \bar{y}_e^{tu} \bar{\mathcal{C}}_{ledq}^{turs} (\Omega_e^\dagger D_{\bar{\mu}} \Omega_e) (D^{\bar{\mu}} \bar{q}_s H d_r) \\
& + \frac{1}{3} \bar{y}_e^{tu} \bar{\mathcal{C}}_{ledq}^{turs} (\Omega_e^\dagger D_{\bar{\mu}} \Omega_e) (\Omega_{\ell,i}^* D_{\bar{\mu}} \Omega_\ell^j) H^i (\bar{q}_{js} d_r) + \frac{1}{3} \bar{y}_e^{tu} \bar{\mathcal{C}}_{ledq}^{turs} (\Omega_{\ell,i}^* D_{\bar{\mu}} \Omega_\ell^j) D^{\bar{\mu}} H^i (\bar{q}_{js} d_r) \\
& - \frac{1}{3} \bar{y}_e^{tu} \mathcal{C}_{ledq}^{tusr} (D_{\bar{\mu}} \Omega_{\ell,j}^* D_{\bar{\mu}} \Omega_\ell^i) H_i^\dagger (\bar{d}_s q_r^j) - \frac{1}{3} \bar{y}_e^{tu} \mathcal{C}_{ledq}^{tusr} (D_{\bar{\mu}} \Omega_{\ell,j}^* \Omega_\ell^i) H_i^\dagger (\bar{d}_s D^{\bar{\mu}} q_r^j) \\
& - \frac{1}{3} \bar{y}_e^{tu} \mathcal{C}_{ledq}^{tusr} (D_{\bar{\mu}} \Omega_e^\dagger D_{\bar{\mu}} \Omega_e) (\bar{d}_s H^\dagger q_r) - \frac{1}{3} \bar{y}_e^{tu} \mathcal{C}_{ledq}^{tusr} (D_{\bar{\mu}} \Omega_e^\dagger \Omega_e) (\bar{d}_s D_{\bar{\mu}} H^\dagger q_r) \\
& - \frac{1}{3} \bar{y}_e^{tu} \mathcal{C}_{ledq}^{tusr} (D_{\bar{\mu}} \Omega_{\ell,j}^* \Omega_\ell^i) H_i^\dagger (D^{\bar{\mu}} \bar{d}_s q_r^j) - \frac{1}{3} \bar{y}_d^{ut} \bar{\mathcal{C}}_{ledq}^{rstu} (D_{\bar{\mu}} \Omega_{q,j}^* D_{\bar{\mu}} \Omega_q^i) H_i^\dagger (\bar{e}_s \ell_r^j) \\
& - \frac{1}{3} \bar{y}_d^{ut} \bar{\mathcal{C}}_{ledq}^{rstu} (D_{\bar{\mu}} \Omega_{q,j}^* \Omega_q^i) H_i^\dagger (\bar{e}_s D^{\bar{\mu}} \ell_r^j) - \frac{1}{3} \bar{y}_d^{ut} \bar{\mathcal{C}}_{ledq}^{rstu} (D_{\bar{\mu}} \Omega_d^\dagger D_{\bar{\mu}} \Omega_d) (\bar{e}_s H^\dagger \ell_r) \\
& - \frac{1}{3} \bar{y}_d^{ut} \bar{\mathcal{C}}_{ledq}^{rstu} (D_{\bar{\mu}} \Omega_d^\dagger \Omega_d) (\bar{e}_s D_{\bar{\mu}} H^\dagger \ell_r) - \frac{1}{3} \bar{y}_d^{ut} \bar{\mathcal{C}}_{ledq}^{rstu} (D_{\bar{\mu}} \Omega_{q,j}^* \Omega_q^i) H_i^\dagger (D^{\bar{\mu}} \bar{e}_s \ell_r^j) \\
& - \frac{1}{3} \bar{y}_d^{ut} \mathcal{C}_{ledq}^{srtu} (D_{\bar{\mu}} \Omega_d^\dagger D_{\bar{\mu}} \Omega_d) (\bar{\ell}_s H e_r) - \frac{1}{3} \bar{y}_d^{ut} \mathcal{C}_{ledq}^{srtu} (\Omega_d^\dagger D_{\bar{\mu}} \Omega_d) (\bar{\ell}_s D_{\bar{\mu}} H e_r) - \frac{1}{3} \bar{y}_d^{ut} \mathcal{C}_{ledq}^{srtu} (D_{\bar{\mu}} \Omega_{q,i}^* D_{\bar{\mu}} \Omega_q^j) H^i (\bar{\ell}_{js} e_r) \\
& - \frac{1}{3} \bar{y}_d^{ut} \mathcal{C}_{ledq}^{srtu} (\Omega_{q,i}^* D_{\bar{\mu}} \Omega_q^j) H^i (\bar{\ell}_{js} D^{\bar{\mu}} e_r) - \frac{1}{3} \bar{y}_d^{ut} \mathcal{C}_{ledq}^{srtu} (\Omega_{q,i}^* D_{\bar{\mu}} \Omega_q^j) H^i (D^{\bar{\mu}} \bar{\ell}_{js} e_r) \\
& - \frac{1}{3} \bar{y}_e^{tu} \bar{\mathcal{C}}_{ledq}^{turs} (D_{\bar{\mu}} \Omega_e^\dagger D_{\bar{\mu}} \Omega_e) (\bar{q}_s H d_r) - \frac{1}{3} \bar{y}_e^{tu} \bar{\mathcal{C}}_{ledq}^{turs} (\Omega_e^\dagger D_{\bar{\mu}} \Omega_e) (\bar{q}_s D_{\bar{\mu}} H d_r) \\
& - \frac{1}{3} \bar{y}_e^{tu} \bar{\mathcal{C}}_{ledq}^{turs} (D_{\bar{\mu}} \Omega_{\ell,i}^* D_{\bar{\mu}} \Omega_\ell^j) H^i (\bar{q}_{js} d_r) - \frac{1}{3} \bar{y}_e^{tu} \bar{\mathcal{C}}_{ledq}^{turs} (\Omega_{\ell,i}^* D_{\bar{\mu}} \Omega_\ell^j) H^i (\bar{q}_{js} D^{\bar{\mu}} d_r) \\
& - \frac{1}{3} \bar{y}_e^{tu} \bar{\mathcal{C}}_{ledq}^{turs} (\Omega_{\ell,i}^* D_{\bar{\mu}} \Omega_\ell^j) H^i (D^{\bar{\mu}} \bar{q}_{js} d_r), \tag{3.58}
\end{aligned}$$

$$\begin{aligned}
\Gamma_\Omega^{(1)} [\mathcal{O}_{lequ}^{(1)}] &= \frac{1}{3} y_u^{tu} (\bar{\mathcal{C}}_{lequ}^{(1)})^{rstu} (D_{\bar{\mu}} \Omega_{q,aj}^* \Omega_q^{bi}) (D_{\bar{\mu}} \Omega_{u,b}^* \Omega_u^a) H_i^\dagger (\bar{e}_s \ell_r^j) + \frac{1}{3} y_u^{tu} (\bar{\mathcal{C}}_{lequ}^{(1)})^{rstu} (D_{\bar{\mu}} \Omega_{q,j}^* \Omega_q^i) H_i^\dagger (\bar{e}_s D^{\bar{\mu}} \ell_r^j) \\
& + \frac{1}{3} y_u^{tu} (\bar{\mathcal{C}}_{lequ}^{(1)})^{rstu} (D_{\bar{\mu}} \Omega_q^\dagger D_{\bar{\mu}} \Omega_q) (\bar{e}_s H^\dagger \ell_r) + \frac{1}{3} y_u^{tu} (\bar{\mathcal{C}}_{lequ}^{(1)})^{rstu} (D_{\bar{\mu}} \Omega_u^\dagger D_{\bar{\mu}} \Omega_u) (\bar{e}_s H^\dagger \ell_r) \\
& + \frac{1}{3} y_u^{tu} (\bar{\mathcal{C}}_{lequ}^{(1)})^{rstu} (D_{\bar{\mu}} \Omega_u^\dagger \Omega_u) (\bar{e}_s H^\dagger D^{\bar{\mu}} \ell_r) + \frac{1}{3} y_u^{tu} (\bar{\mathcal{C}}_{lequ}^{(1)})^{rstu} (D_{\bar{\mu}} \Omega_q^\dagger \Omega_q) (\bar{e}_s D_{\bar{\mu}} H^\dagger \ell_r) \\
& + \frac{1}{3} y_u^{tu} (\bar{\mathcal{C}}_{lequ}^{(1)})^{rstu} (D_{\bar{\mu}} \Omega_{q,j}^* \Omega_q^i) H_i^\dagger (D^{\bar{\mu}} \bar{e}_s \ell_r^j) + \frac{1}{3} y_u^{tu} (\bar{\mathcal{C}}_{lequ}^{(1)})^{rstu} (D_{\bar{\mu}} \Omega_u^\dagger \Omega_u) (D^{\bar{\mu}} \bar{e}_s H^\dagger \ell_r) \\
& + \frac{1}{3} \bar{y}_u^{tu} (\mathcal{C}_{lequ}^{(1)})^{srtu} (D_{\bar{\mu}} \Omega_q^\dagger D_{\bar{\mu}} \Omega_q) (\bar{\ell}_s H e_r) + \frac{1}{3} \bar{y}_u^{tu} (\mathcal{C}_{lequ}^{(1)})^{srtu} (D_{\bar{\mu}} \Omega_u^\dagger D_{\bar{\mu}} \Omega_u) (\bar{\ell}_s H e_r) \\
& + \frac{1}{3} \bar{y}_u^{tu} (\mathcal{C}_{lequ}^{(1)})^{srtu} (\Omega_u^\dagger D_{\bar{\mu}} \Omega_u) (\bar{\ell}_s H D^{\bar{\mu}} e_r) + \frac{1}{3} \bar{y}_u^{tu} (\mathcal{C}_{lequ}^{(1)})^{srtu} (\Omega_q^\dagger D_{\bar{\mu}} \Omega_q) (\bar{\ell}_s D_{\bar{\mu}} H e_r) \\
& + \frac{1}{3} \bar{y}_u^{tu} (\mathcal{C}_{lequ}^{(1)})^{srtu} (\Omega_u^\dagger D_{\bar{\mu}} \Omega_u) (D^{\bar{\mu}} \bar{\ell}_s H e_r) + \frac{1}{3} \bar{y}_u^{tu} (\mathcal{C}_{lequ}^{(1)})^{srtu} (\Omega_{q,ai}^* D_{\bar{\mu}} \Omega_q^{bj}) (\Omega_{u,b}^* D_{\bar{\mu}} \Omega_u^a) H^i (\bar{\ell}_{js} e_r)
\end{aligned}$$

$$\begin{aligned}
& + \frac{1}{3} \bar{y}_u^{tu} (\mathcal{C}_{lequ}^{(1)})^{srtu} (\Omega_{q,i}^* D_{\bar{\mu}} \Omega_q^j) H^i (\bar{\ell}_{js} D^{\bar{\mu}} e_r) + \frac{1}{3} \bar{y}_u^{tu} (\mathcal{C}_{lequ}^{(1)})^{srtu} (\Omega_{q,i}^* D_{\bar{\mu}} \Omega_q^j) H^i (D^{\bar{\mu}} \bar{\ell}_{js} e_r) \\
& + \frac{1}{3} \bar{y}_e^{rs} (\mathcal{C}_{lequ}^{(1)})^{rstu} (D_{\bar{\mu}} \Omega_e^\dagger \Omega_e) (D_{\bar{\mu}} \Omega_\ell^\dagger \Omega_\ell) (\bar{q}_t \tilde{H} u_u) + \frac{1}{3} \bar{y}_e^{rs} (\mathcal{C}_{lequ}^{(1)})^{rstu} (D_{\bar{\mu}} \Omega_e^\dagger \Omega_e) (\bar{q}_t \tilde{H} D^{\bar{\mu}} u_u) \\
& + \frac{1}{3} \bar{y}_e^{rs} (\mathcal{C}_{lequ}^{(1)})^{rstu} (D_{\bar{\mu}} \Omega_\ell^\dagger \Omega_\ell) (\bar{q}_t D_{\bar{\mu}} \tilde{H} u_u) + \frac{1}{3} \bar{y}_e^{rs} (\mathcal{C}_{lequ}^{(1)})^{rstu} (D_{\bar{\mu}} \Omega_e^\dagger \Omega_e) (D^{\bar{\mu}} \bar{q}_t \tilde{H} u_u) \\
& + \frac{1}{3} \bar{y}_e^{rs} (\mathcal{C}_{lequ}^{(1)})^{rstu} (D_{\bar{\mu}} \Omega_{\ell,j}^* D_{\bar{\mu}} \Omega_\ell^k) \tilde{H}_j (\bar{q}_{kt} u_u) + \frac{1}{3} \bar{y}_e^{rs} (\mathcal{C}_{lequ}^{(1)})^{rstu} (D_{\bar{\mu}} \Omega_{\ell,j}^* \Omega_\ell^k) \tilde{H}_j (\bar{q}_{kt} D^{\bar{\mu}} u_u) \\
& + \frac{1}{3} \bar{y}_e^{rs} (\mathcal{C}_{lequ}^{(1)})^{rstu} (D_{\bar{\mu}} \Omega_{\ell,j}^* \Omega_\ell^k) \tilde{H}_j (D^{\bar{\mu}} \bar{q}_{kt} u_u) + \frac{1}{3} \bar{y}_e^{rs} (\mathcal{C}_{lequ}^{(1)})^{rstu} (D_{\bar{\mu}} \Omega_{\ell,i}^* D_{\bar{\mu}} \Omega_\ell^k) \tilde{H}^{\dagger k} (\bar{u}_u q_t^i) \\
& + \frac{1}{3} \bar{y}_e^{rs} (\mathcal{C}_{lequ}^{(1)})^{rstu} (\Omega_{\ell,i}^* D_{\bar{\mu}} \Omega_\ell^k) \tilde{H}^{\dagger k} (\bar{u}_u D^{\bar{\mu}} q_t^i) + \frac{1}{3} \bar{y}_e^{rs} (\mathcal{C}_{lequ}^{(1)})^{rstu} (\Omega_e^\dagger D_{\bar{\mu}} \Omega_e) (\Omega_\ell^\dagger D_{\bar{\mu}} \Omega_\ell) (\bar{u}_u \tilde{H}^{\dagger} q_t) \\
& + \frac{1}{3} \bar{y}_e^{rs} (\mathcal{C}_{lequ}^{(1)})^{rstu} (\Omega_e^\dagger D_{\bar{\mu}} \Omega_e) (\bar{u}_u \tilde{H}^{\dagger} D^{\bar{\mu}} q_t) + \frac{1}{3} \bar{y}_e^{rs} (\mathcal{C}_{lequ}^{(1)})^{rstu} (\Omega_\ell^\dagger D_{\bar{\mu}} \Omega_\ell) (\bar{u}_u D_{\bar{\mu}} \tilde{H}^{\dagger} q_t) \\
& + \frac{1}{3} \bar{y}_e^{rs} (\mathcal{C}_{lequ}^{(1)})^{rstu} (\Omega_{\ell,i}^* D_{\bar{\mu}} \Omega_\ell^k) \tilde{H}^{\dagger k} (D^{\bar{\mu}} \bar{u}_u q_t^i) + \frac{1}{3} \bar{y}_e^{rs} (\mathcal{C}_{lequ}^{(1)})^{rstu} (\Omega_e^\dagger D_{\bar{\mu}} \Omega_e) (D^{\bar{\mu}} \bar{u}_u \tilde{H}^{\dagger} q_t) \\
& - \frac{1}{3} \bar{y}_u^{tu} (\mathcal{C}_{lequ}^{(1)})^{rstu} (D_{\bar{\mu}} \Omega_{q,j}^* \Omega_q^i) D^{\bar{\mu}} H_i^\dagger (\bar{e}_s \ell_r^j) - \frac{1}{3} \bar{y}_u^{tu} (\mathcal{C}_{lequ}^{(1)})^{rstu} (D_{\bar{\mu}} \Omega_{q,j}^* D_{\bar{\mu}} \Omega_q^i) H_i^\dagger (\bar{e}_s \ell_r^j) \\
& - \frac{1}{3} \bar{y}_u^{tu} (\mathcal{C}_{lequ}^{(1)})^{rstu} (D_{\bar{\mu}} \Omega_{q,a}^* \Omega_q^b) (D_{\bar{\mu}} \Omega_{u,b}^* \Omega_u^a) (\bar{e}_s H^\dagger \ell_r) - \frac{1}{3} \bar{y}_u^{tu} (\mathcal{C}_{lequ}^{(1)})^{rstu} (D_{\bar{\mu}} \Omega_q^\dagger \Omega_q) (\bar{e}_s H^\dagger D^{\bar{\mu}} \ell_r) \\
& - \frac{1}{3} \bar{y}_u^{tu} (\mathcal{C}_{lequ}^{(1)})^{rstu} (D_{\bar{\mu}} \Omega_u^\dagger \Omega_u) (\bar{e}_s D_{\bar{\mu}} H^\dagger \ell_r) - \frac{1}{3} \bar{y}_u^{tu} (\mathcal{C}_{lequ}^{(1)})^{rstu} (D_{\bar{\mu}} \Omega_q^\dagger \Omega_q) (D^{\bar{\mu}} \bar{e}_s H^\dagger \ell_r) \\
& - \frac{1}{3} \bar{y}_u^{tu} (\mathcal{C}_{lequ}^{(1)})^{srtu} (\Omega_{q,a}^* D_{\bar{\mu}} \Omega_q^b) (\Omega_{u,b}^* D_{\bar{\mu}} \Omega_u^a) (\bar{\ell}_s H e_r) - \frac{1}{3} \bar{y}_u^{tu} (\mathcal{C}_{lequ}^{(1)})^{srtu} (\Omega_q^\dagger D_{\bar{\mu}} \Omega_q) (\bar{\ell}_s H D^{\bar{\mu}} e_r) \\
& - \frac{1}{3} \bar{y}_u^{tu} (\mathcal{C}_{lequ}^{(1)})^{srtu} (\Omega_u^\dagger D_{\bar{\mu}} \Omega_u) (\bar{\ell}_s D_{\bar{\mu}} H e_r) - \frac{1}{3} \bar{y}_u^{tu} (\mathcal{C}_{lequ}^{(1)})^{srtu} (\Omega_q^\dagger D_{\bar{\mu}} \Omega_q) (D^{\bar{\mu}} \bar{\ell}_s H e_r) \\
& - \frac{1}{3} \bar{y}_u^{tu} (\mathcal{C}_{lequ}^{(1)})^{srtu} (D_{\bar{\mu}} \Omega_{q,i}^* D_{\bar{\mu}} \Omega_q^j) H^i (\bar{\ell}_{js} e_r) - \frac{1}{3} \bar{y}_u^{tu} (\mathcal{C}_{lequ}^{(1)})^{srtu} (\Omega_{q,i}^* D_{\bar{\mu}} \Omega_q^j) D^{\bar{\mu}} H^i (\bar{\ell}_{js} e_r) \\
& - \frac{1}{3} \bar{y}_e^{rs} (\mathcal{C}_{lequ}^{(1)})^{rstu} (D_{\bar{\mu}} \Omega_e^\dagger D_{\bar{\mu}} \Omega_e) (\bar{q}_t \tilde{H} u_u) - \frac{1}{3} \bar{y}_e^{rs} (\mathcal{C}_{lequ}^{(1)})^{rstu} (D_{\bar{\mu}} \Omega_\ell^\dagger D_{\bar{\mu}} \Omega_\ell) (\bar{q}_t \tilde{H} u_u) \\
& - \frac{1}{3} \bar{y}_e^{rs} (\mathcal{C}_{lequ}^{(1)})^{rstu} (D_{\bar{\mu}} \Omega_\ell^\dagger \Omega_\ell) (\bar{q}_t \tilde{H} D^{\bar{\mu}} u_u) - \frac{1}{3} \bar{y}_e^{rs} (\mathcal{C}_{lequ}^{(1)})^{rstu} (D_{\bar{\mu}} \Omega_e^\dagger \Omega_e) (\bar{q}_t D_{\bar{\mu}} \tilde{H} u_u) \\
& - \frac{1}{3} \bar{y}_e^{rs} (\mathcal{C}_{lequ}^{(1)})^{rstu} (D_{\bar{\mu}} \Omega_\ell^\dagger \Omega_\ell) (D^{\bar{\mu}} \bar{q}_t \tilde{H} u_u) - \frac{1}{3} \bar{y}_e^{rs} (\mathcal{C}_{lequ}^{(1)})^{rstu} (D_{\bar{\mu}} \Omega_e^\dagger \Omega_e) (D_{\bar{\mu}} \Omega_{\ell,j}^* \Omega_\ell^k) \tilde{H}_j (\bar{q}_{kt} u_u) \\
& - \frac{1}{3} \bar{y}_e^{rs} (\mathcal{C}_{lequ}^{(1)})^{rstu} (D_{\bar{\mu}} \Omega_{\ell,j}^* \Omega_\ell^k) D^{\bar{\mu}} \tilde{H}_j (\bar{q}_{kt} u_u) - \frac{1}{3} \bar{y}_e^{rs} (\mathcal{C}_{lequ}^{(1)})^{rstu} (\Omega_{\ell,i}^* D_{\bar{\mu}} \Omega_\ell^k) D^{\bar{\mu}} \tilde{H}^{\dagger k} (\bar{u}_u q_t^i) \\
& - \frac{1}{3} \bar{y}_e^{rs} (\mathcal{C}_{lequ}^{(1)})^{rstu} (\Omega_e^\dagger D_{\bar{\mu}} \Omega_e) (\Omega_{\ell,i}^* D_{\bar{\mu}} \Omega_\ell^k) \tilde{H}^{\dagger k} (\bar{u}_u q_t^i) - \frac{1}{3} \bar{y}_e^{rs} (\mathcal{C}_{lequ}^{(1)})^{rstu} (D_{\bar{\mu}} \Omega_e^\dagger D_{\bar{\mu}} \Omega_e) (\bar{u}_u \tilde{H}^{\dagger} q_t) \\
& - \frac{1}{3} \bar{y}_e^{rs} (\mathcal{C}_{lequ}^{(1)})^{rstu} (D_{\bar{\mu}} \Omega_\ell^\dagger D_{\bar{\mu}} \Omega_\ell) (\bar{u}_u \tilde{H}^{\dagger} q_t) - \frac{1}{3} \bar{y}_e^{rs} (\mathcal{C}_{lequ}^{(1)})^{rstu} (\Omega_\ell^\dagger D_{\bar{\mu}} \Omega_\ell) (\bar{u}_u \tilde{H}^{\dagger} D^{\bar{\mu}} q_t) \\
& - \frac{1}{3} \bar{y}_e^{rs} (\mathcal{C}_{lequ}^{(1)})^{rstu} (\Omega_e^\dagger D_{\bar{\mu}} \Omega_e) (\bar{u}_u D_{\bar{\mu}} \tilde{H}^{\dagger} q_t) - \frac{1}{3} \bar{y}_e^{rs} (\mathcal{C}_{lequ}^{(1)})^{rstu} (\Omega_\ell^\dagger D_{\bar{\mu}} \Omega_\ell) (D^{\bar{\mu}} \bar{u}_u \tilde{H}^{\dagger} q_t), \tag{3.59}
\end{aligned}$$

$$\begin{aligned}
\Gamma_\Omega^{(1)} [\mathcal{O}_{lequ}^{(3)}] &= \frac{4i}{3} \bar{y}_u^{tu} (\mathcal{C}_{lequ}^{(3)})^{rstu} (D_{\bar{\mu}} \Omega_{q,a,j}^* \Omega_q^{bi}) (D_{\bar{\nu}} \Omega_{u,b}^* \Omega_u^a) H_i^\dagger (\bar{e}_s \sigma^{\bar{\mu}\bar{\nu}} \ell_r^j) \\
&- \frac{4i}{3} \bar{y}_u^{tu} (\mathcal{C}_{lequ}^{(3)})^{rstu} (D_{\bar{\mu}} \Omega_{q,a}^* \Omega_q^b) (D_{\bar{\nu}} \Omega_{u,b}^* \Omega_u^a) (\bar{e}_s \sigma^{\bar{\mu}\bar{\nu}} H^\dagger \ell_r)
\end{aligned}$$

$$\begin{aligned}
& + \frac{4i}{3} \bar{y}_u^{tu} (\mathcal{C}_{lequ}^{(3)})^{srtu} (\Omega_{q,a}^* D_{\bar{\mu}} \Omega_q^b) (\Omega_{u,b}^* D_{\bar{\nu}} \Omega_u^a) (\bar{\ell}_s H \sigma^{\bar{\mu}\bar{\nu}} e_r) \\
& - \frac{4i}{3} \bar{y}_u^{tu} (\mathcal{C}_{lequ}^{(3)})^{srtu} (\Omega_{q,ai}^* D_{\bar{\mu}} \Omega_q^{bj}) (\Omega_{u,b}^* D_{\bar{\nu}} \Omega_u^a) H^i (\bar{\ell}_{js} \sigma^{\bar{\mu}\bar{\nu}} e_r) \\
& + \frac{4i}{3} \bar{y}_e^{rs} (\mathcal{C}_{lequ}^{(3)})^{rstu} (D_{\bar{\mu}} \Omega_e^\dagger \Omega_e) (D_{\bar{\nu}} \Omega_\ell^\dagger \Omega_\ell) (\bar{q}_t \tilde{H} \sigma^{\bar{\mu}\bar{\nu}} u_u) \\
& - \frac{4i}{3} \bar{y}_e^{rs} (\mathcal{C}_{lequ}^{(3)})^{rstu} (D_{\bar{\mu}} \Omega_e^\dagger \Omega_e) (D_{\bar{\nu}} \Omega_{\ell,j}^* \Omega_\ell^k) \tilde{H}_j (\bar{q}_{kt} \sigma^{\bar{\mu}\bar{\nu}} u_u) \\
& + \frac{4i}{3} \bar{y}_e^{rs} (\bar{\mathcal{C}}_{lequ}^{(3)})^{rstu} (\Omega_e^\dagger D_{\bar{\mu}} \Omega_e) (\Omega_{\ell,i}^* D_{\bar{\nu}} \Omega_\ell^k) \tilde{H}^{\dagger k} (\bar{u}_u \sigma^{\bar{\mu}\bar{\nu}} q_t^i) \\
& - \frac{4i}{3} \bar{y}_e^{rs} (\bar{\mathcal{C}}_{lequ}^{(3)})^{rstu} (\Omega_e^\dagger D_{\bar{\mu}} \Omega_e) (\Omega_\ell^\dagger D_{\bar{\nu}} \Omega_\ell) (\bar{u}_u \sigma^{\bar{\mu}\bar{\nu}} \tilde{H}^\dagger q_t) \\
& + \frac{8i}{3} \bar{y}_u^{tu} (\bar{\mathcal{C}}_{lequ}^{(3)})^{rstu} (D_{\bar{\nu}} \Omega_{q,j}^* \Omega_q^i) D_{\bar{\mu}} H_i^\dagger (\bar{e}_s \sigma^{\bar{\mu}\bar{\nu}} \ell_r^j) - \frac{8i}{3} \bar{y}_u^{tu} (\bar{\mathcal{C}}_{lequ}^{(3)})^{rstu} (D_{\bar{\nu}} \Omega_q^\dagger \Omega_q) (\bar{e}_s \sigma^{\bar{\mu}\bar{\nu}} D_{\bar{\mu}} H^\dagger \ell_r) \\
& - \frac{8i}{3} \bar{y}_u^{tu} (\bar{\mathcal{C}}_{lequ}^{(3)})^{rstu} (D_{\bar{\nu}} \Omega_u^\dagger \Omega_u) (\bar{e}_s \sigma^{\bar{\mu}\bar{\nu}} D_{\bar{\mu}} H^\dagger \ell_r) + \frac{8i}{3} \bar{y}_u^{tu} (\mathcal{C}_{lequ}^{(3)})^{srtu} (\Omega_q^\dagger D_{\bar{\nu}} \Omega_q) (\bar{\ell}_s D_{\bar{\mu}} H \sigma^{\bar{\mu}\bar{\nu}} e_r) \\
& + \frac{8i}{3} \bar{y}_u^{tu} (\mathcal{C}_{lequ}^{(3)})^{srtu} (\Omega_u^\dagger D_{\bar{\nu}} \Omega_u) (\bar{\ell}_s D_{\bar{\mu}} H \sigma^{\bar{\mu}\bar{\nu}} e_r) - \frac{8i}{3} \bar{y}_u^{tu} (\mathcal{C}_{lequ}^{(3)})^{srtu} (\Omega_{q,i}^* D_{\bar{\nu}} \Omega_q^j) D_{\bar{\mu}} H^i (\bar{\ell}_{js} \sigma^{\bar{\mu}\bar{\nu}} e_r) \\
& + \frac{8i}{3} \bar{y}_e^{rs} (\mathcal{C}_{lequ}^{(3)})^{rstu} (D_{\bar{\nu}} \Omega_e^\dagger \Omega_e) (\bar{q}_t D_{\bar{\mu}} \tilde{H} \sigma^{\bar{\mu}\bar{\nu}} u_u) + \frac{8i}{3} \bar{y}_e^{rs} (\mathcal{C}_{lequ}^{(3)})^{rstu} (D_{\bar{\nu}} \Omega_\ell^\dagger \Omega_\ell) (\bar{q}_t D_{\bar{\mu}} \tilde{H} \sigma^{\bar{\mu}\bar{\nu}} u_u) \\
& - \frac{8i}{3} \bar{y}_e^{rs} (\mathcal{C}_{lequ}^{(3)})^{rstu} (D_{\bar{\nu}} \Omega_{\ell,j}^* \Omega_\ell^k) D_{\bar{\mu}} \tilde{H}_j (\bar{q}_{kt} \sigma^{\bar{\mu}\bar{\nu}} u_u) + \frac{8i}{3} \bar{y}_e^{rs} (\bar{\mathcal{C}}_{lequ}^{(3)})^{rstu} (\Omega_{\ell,i}^* D_{\bar{\nu}} \Omega_\ell^k) D_{\bar{\mu}} \tilde{H}^{\dagger k} (\bar{u}_u \sigma^{\bar{\mu}\bar{\nu}} q_t^i) \\
& - \frac{8i}{3} \bar{y}_e^{rs} (\bar{\mathcal{C}}_{lequ}^{(3)})^{rstu} (\Omega_e^\dagger D_{\bar{\nu}} \Omega_e) (\bar{u}_u \sigma^{\bar{\mu}\bar{\nu}} D_{\bar{\mu}} \tilde{H}^\dagger q_t) - \frac{8i}{3} \bar{y}_e^{rs} (\bar{\mathcal{C}}_{lequ}^{(3)})^{rstu} (\Omega_\ell^\dagger D_{\bar{\nu}} \Omega_\ell) (\bar{u}_u \sigma^{\bar{\mu}\bar{\nu}} D_{\bar{\mu}} \tilde{H}^\dagger q_t), \quad (3.60)
\end{aligned}$$

$$\begin{aligned}
\Gamma_\Omega^{(1)} [\mathcal{O}_{quqd}^{(1)}] &= \frac{1}{6} y_u^{ut} (\bar{\mathcal{C}}_{quqd}^{(1)})^{rtus} (D_{\bar{\mu}} \Omega_{q,aj}^* \Omega_q^{bi}) D_{\bar{\mu}} H_i^\dagger (\bar{d}_{bs} q_r^{aj}) + \frac{1}{6} y_u^{ut} (\bar{\mathcal{C}}_{quqd}^{(1)})^{rtus} (D_{\bar{\mu}} \Omega_{q,aj}^* D_{\bar{\mu}} \Omega_q^{bi}) H_i^\dagger (\bar{d}_{bs} q_r^{aj}) \\
& + \frac{1}{6} y_u^{ut} (\bar{\mathcal{C}}_{quqd}^{(1)})^{rtus} (D_{\bar{\mu}} \Omega_{q,a}^* \Omega_q^b) (\bar{d}_{bs} H^\dagger D_{\bar{\mu}} q_r^a) + \frac{1}{6} y_u^{ut} (\bar{\mathcal{C}}_{quqd}^{(1)})^{rtus} (D_{\bar{\mu}} \Omega_{u,a}^* \Omega_u^b) (\bar{d}_{bs} D_{\bar{\mu}} H^\dagger q_r^a) \\
& + \frac{1}{6} y_u^{ut} (\bar{\mathcal{C}}_{quqd}^{(1)})^{rtus} (D_{\bar{\mu}} \Omega_{q,a}^* \Omega_q^b) (D_{\bar{\mu}} \bar{d}_{bs} H^\dagger q_r^a) + \frac{1}{6} y_u^{ut} (\bar{\mathcal{C}}_{quqd}^{(1)})^{rtus} (D_{\bar{\mu}} \Omega_{q,a}^* \Omega_q^c) (D_{\bar{\mu}} \Omega_{u,b}^* \Omega_u^a) (\bar{d}_{cs} H^\dagger q_r^b) \\
& + \frac{1}{6} \bar{y}_u^{tu} (\mathcal{C}_{quqd}^{(1)})^{sutr} (\Omega_{q,a}^* D_{\bar{\mu}} \Omega_q^b) (\bar{q}_{bs} H D_{\bar{\mu}} d_r^a) + \frac{1}{6} \bar{y}_u^{tu} (\mathcal{C}_{quqd}^{(1)})^{sutr} (\Omega_{u,a}^* D_{\bar{\mu}} \Omega_u^b) (\bar{q}_{bs} D_{\bar{\mu}} H d_r^a) \\
& + \frac{1}{6} \bar{y}_u^{tu} (\mathcal{C}_{quqd}^{(1)})^{sutr} (\Omega_{q,a}^* D_{\bar{\mu}} \Omega_q^b) (D_{\bar{\mu}} \bar{q}_{bs} H d_r^a) + \frac{1}{6} \bar{y}_d^{rs} (\mathcal{C}_{quqd}^{(1)})^{rtus} (D_{\bar{\mu}} \Omega_{d,a}^* \Omega_d^b) (\bar{q}_{bu} \tilde{H} D_{\bar{\mu}} u_t^a) \\
& + \frac{1}{6} \bar{y}_d^{rs} (\mathcal{C}_{quqd}^{(1)})^{rtus} (D_{\bar{\mu}} \Omega_{d,a}^* \Omega_d^b) (\bar{q}_{bu} D_{\bar{\mu}} \tilde{H} u_t^a) + \frac{1}{6} \bar{y}_d^{rs} (\mathcal{C}_{quqd}^{(1)})^{rtus} (D_{\bar{\mu}} \Omega_{d,a}^* \Omega_d^b) (D_{\bar{\mu}} \bar{q}_{bu} \tilde{H} u_t^a) \\
& + \frac{1}{6} \bar{y}_u^{tu} (\mathcal{C}_{quqd}^{(1)})^{sutr} (\Omega_{q,a}^* D_{\bar{\mu}} \Omega_q^b) (\Omega_{u,b}^* D_{\bar{\mu}} \Omega_u^c) (\bar{q}_{cs} H d_r^a) + \frac{1}{6} y_d^{ru} (\bar{\mathcal{C}}_{quqd}^{(1)})^{rstu} \bar{\varepsilon}_{jk} (\Omega_{q,ai}^* D_{\bar{\mu}} \Omega_q^{bk}) D_{\bar{\mu}} H^i (\bar{u}_{bs} q_t^{aj}) \\
& + \frac{1}{6} y_d^{ru} (\bar{\mathcal{C}}_{quqd}^{(1)})^{rstu} (\Omega_{d,a}^* D_{\bar{\mu}} \Omega_d^b) (\bar{u}_{bs} \tilde{H}^\dagger D_{\bar{\mu}} q_t^a) + \frac{1}{6} y_d^{ru} (\bar{\mathcal{C}}_{quqd}^{(1)})^{rstu} (\Omega_{d,a}^* D_{\bar{\mu}} \Omega_d^b) (\bar{u}_{bs} D_{\bar{\mu}} \tilde{H}^\dagger q_t^a) \\
& + \frac{1}{6} y_d^{ru} (\bar{\mathcal{C}}_{quqd}^{(1)})^{rstu} (\Omega_{d,a}^* D_{\bar{\mu}} \Omega_d^b) (D_{\bar{\mu}} \bar{u}_{bs} \tilde{H}^\dagger q_t^a) + \frac{1}{6} y_d^{ru} (\bar{\mathcal{C}}_{quqd}^{(1)})^{rstu} (\Omega_{d,a}^* D_{\bar{\mu}} \Omega_d^b) (\Omega_{q,bi}^* D_{\bar{\mu}} \Omega_q^{ck}) \tilde{H}^{\dagger k} (\bar{u}_{cs} q_t^{ai}) \\
& + \frac{1}{3} \bar{y}_u^{tu} (\bar{\mathcal{C}}_{quqd}^{(1)})^{turs} (D_{\bar{\mu}} \Omega_{q,j}^* \Omega_q^i) D_{\bar{\mu}} H_i^\dagger (\bar{d}_s q_r^j) + \frac{1}{3} \bar{y}_u^{tu} (\bar{\mathcal{C}}_{quqd}^{(1)})^{turs} (D_{\bar{\mu}} \Omega_{q,j}^* D_{\bar{\mu}} \Omega_q^i) H_i^\dagger (\bar{d}_s q_r^j) \\
& + \frac{1}{3} \bar{y}_u^{tu} (\bar{\mathcal{C}}_{quqd}^{(1)})^{turs} (D_{\bar{\mu}} \Omega_{q,a}^* \Omega_q^b) (D_{\bar{\mu}} \Omega_{u,b}^* \Omega_u^a) (\bar{d}_s H^\dagger q_r) + \frac{1}{3} \bar{y}_u^{tu} (\bar{\mathcal{C}}_{quqd}^{(1)})^{turs} (D_{\bar{\mu}} \Omega_q^\dagger \Omega_q) (\bar{d}_s H^\dagger D_{\bar{\mu}} q_r)
\end{aligned}$$

$$\begin{aligned}
& + \frac{1}{3} \bar{y}_u^{tu} (\bar{\mathcal{C}}_{quqd}^{(1)})^{turs} (D_{\bar{\mu}} \Omega_u^\dagger \Omega_u) (\bar{d}_s D_{\bar{\mu}} H^\dagger q_r) + \frac{1}{3} \bar{y}_u^{tu} (\bar{\mathcal{C}}_{quqd}^{(1)})^{turs} (D_{\bar{\mu}} \Omega_q^\dagger \Omega_q) (D^{\bar{\mu}} \bar{d}_s H^\dagger q_r) \\
& + \frac{1}{3} \bar{y}_u^{tu} (\mathcal{C}_{quqd}^{(1)})^{tusr} (\Omega_{q,a}^* D_{\bar{\mu}} \Omega_q^b) (\Omega_{u,b}^* D_{\bar{\mu}} \Omega_u^a) (\bar{q}_s H d_r) + \frac{1}{3} \bar{y}_u^{tu} (\mathcal{C}_{quqd}^{(1)})^{tusr} (\Omega_q^\dagger D_{\bar{\mu}} \Omega_q) (\bar{q}_s H D^{\bar{\mu}} d_r) \\
& + \frac{1}{3} \bar{y}_u^{tu} (\mathcal{C}_{quqd}^{(1)})^{tusr} (\Omega_u^\dagger D_{\bar{\mu}} \Omega_u) (\bar{q}_s D_{\bar{\mu}} H d_r) + \frac{1}{3} \bar{y}_u^{tu} (\mathcal{C}_{quqd}^{(1)})^{tusr} (\Omega_q^\dagger D_{\bar{\mu}} \Omega_q) (D^{\bar{\mu}} \bar{q}_s H d_r) \\
& + \frac{1}{3} \bar{y}_d^{rs} (\mathcal{C}_{quqd}^{(1)})^{turs} (D_{\bar{\mu}} \Omega_d^\dagger \Omega_d) (\bar{q}_t \tilde{H} D^{\bar{\mu}} u_u) + \frac{1}{3} \bar{y}_d^{rs} (\mathcal{C}_{quqd}^{(1)})^{turs} (D_{\bar{\mu}} \Omega_d^\dagger \Omega_d) (D^{\bar{\mu}} \bar{q}_t \tilde{H} u_u) \\
& + \frac{1}{3} \bar{y}_u^{tu} (\mathcal{C}_{quqd}^{(1)})^{tusr} (D_{\bar{\mu}} \Omega_{q,i}^* D_{\bar{\mu}} \Omega_q^j) H^i (\bar{q}_{js} d_r) + \frac{1}{3} \bar{y}_u^{tu} (\mathcal{C}_{quqd}^{(1)})^{tusr} (\Omega_{q,i}^* D_{\bar{\mu}} \Omega_q^j) D^{\bar{\mu}} H^i (\bar{q}_{js} d_r) \\
& + \frac{1}{3} \bar{y}_d^{tu} (\bar{\mathcal{C}}_{quqd}^{(1)})^{rstu} \bar{\varepsilon}_{jk} (\Omega_{q,i}^* D_{\bar{\mu}} \Omega_q^k) D^{\bar{\mu}} H^i (\bar{u}_s q_r^j) + \frac{1}{3} \bar{y}_d^{tu} (\bar{\mathcal{C}}_{quqd}^{(1)})^{rstu} (\Omega_d^\dagger D_{\bar{\mu}} \Omega_d) (\bar{u}_s \tilde{H}^\dagger D^{\bar{\mu}} q_r) \\
& + \frac{1}{3} \bar{y}_d^{tu} (\bar{\mathcal{C}}_{quqd}^{(1)})^{rstu} (\Omega_d^\dagger D_{\bar{\mu}} \Omega_d) (D^{\bar{\mu}} \bar{u}_s \tilde{H}^\dagger q_r) - \frac{1}{6} \bar{y}_u^{ut} (\bar{\mathcal{C}}_{quqd}^{(1)})^{rtus} (D_{\bar{\mu}} \Omega_{q,aj}^* \Omega_q^{bi}) H_i^\dagger (\bar{d}_{bs} D^{\bar{\mu}} q_r^{aj}) \\
& - \frac{1}{6} \bar{y}_u^{ut} (\bar{\mathcal{C}}_{quqd}^{(1)})^{rtus} (D_{\bar{\mu}} \Omega_{q,a}^* D_{\bar{\mu}} \Omega_q^b) (\bar{d}_{bs} H^\dagger q_r^a) - \frac{1}{6} \bar{y}_u^{ut} (\bar{\mathcal{C}}_{quqd}^{(1)})^{rtus} (D_{\bar{\mu}} \Omega_{u,a}^* D_{\bar{\mu}} \Omega_u^b) (\bar{d}_{bs} H^\dagger q_r^a) \\
& - \frac{1}{6} \bar{y}_u^{ut} (\bar{\mathcal{C}}_{quqd}^{(1)})^{rtus} (D_{\bar{\mu}} \Omega_{u,a}^* \Omega_u^b) (\bar{d}_{bs} H^\dagger D^{\bar{\mu}} q_r^a) - \frac{1}{6} \bar{y}_u^{ut} (\bar{\mathcal{C}}_{quqd}^{(1)})^{rtus} (D_{\bar{\mu}} \Omega_{q,a}^* \Omega_q^b) (\bar{d}_{bs} D_{\bar{\mu}} H^\dagger q_r^a) \\
& - \frac{1}{6} \bar{y}_u^{ut} (\bar{\mathcal{C}}_{quqd}^{(1)})^{rtus} (D_{\bar{\mu}} \Omega_{q,aj}^* \Omega_q^{bi}) H_i^\dagger (D^{\bar{\mu}} \bar{d}_{bs} q_r^{aj}) - \frac{1}{6} \bar{y}_u^{ut} (\bar{\mathcal{C}}_{quqd}^{(1)})^{rtus} (D_{\bar{\mu}} \Omega_{u,a}^* \Omega_u^b) (D^{\bar{\mu}} \bar{d}_{bs} H^\dagger q_r^a) \\
& - \frac{1}{6} \bar{y}_u^{ut} (\bar{\mathcal{C}}_{quqd}^{(1)})^{rtus} (D_{\bar{\mu}} \Omega_{q,aj}^* \Omega_q^{ci}) (D_{\bar{\mu}} \Omega_{u,b}^* \Omega_u^a) H_i^\dagger (\bar{d}_{cs} q_r^{bj}) - \frac{i}{6} \bar{y}_u^{ut} (\bar{\mathcal{C}}_{quqd}^{(1)})^{rtus} (D_{\bar{\mu}} \Omega_{q,aj}^* \Omega_q^{ci}) (D_{\bar{\nu}} \Omega_{u,b}^* \Omega_u^a) H_i^\dagger (\bar{d}_{cs} \sigma^{\bar{\mu}\bar{\nu}} q_r^{bj}) \\
& + \frac{i}{6} \bar{y}_u^{ut} (\bar{\mathcal{C}}_{quqd}^{(1)})^{rtus} (D_{\bar{\mu}} \Omega_{q,a}^* \Omega_q^c) (D_{\bar{\nu}} \Omega_{u,b}^* \Omega_u^a) (\bar{d}_{cs} \sigma^{\bar{\mu}\bar{\nu}} H^\dagger q_r^b) - \frac{1}{6} \bar{y}_u^{tu} (\mathcal{C}_{quqd}^{(1)})^{sutr} (D_{\bar{\mu}} \Omega_{q,a}^* D_{\bar{\mu}} \Omega_q^b) (\bar{q}_{bs} H d_r^a) \\
& - \frac{1}{6} \bar{y}_u^{tu} (\mathcal{C}_{quqd}^{(1)})^{sutr} (D_{\bar{\mu}} \Omega_{u,a}^* D_{\bar{\mu}} \Omega_u^b) (\bar{q}_{bs} H d_r^a) - \frac{1}{6} \bar{y}_u^{tu} (\mathcal{C}_{quqd}^{(1)})^{sutr} (\Omega_{u,a}^* D_{\bar{\mu}} \Omega_u^b) (\bar{q}_{bs} H D^{\bar{\mu}} d_r^a) \\
& - \frac{1}{6} \bar{y}_u^{tu} (\mathcal{C}_{quqd}^{(1)})^{sutr} (\Omega_{q,a}^* D_{\bar{\mu}} \Omega_q^b) (\bar{q}_{bs} D_{\bar{\mu}} H d_r^a) - \frac{1}{6} \bar{y}_u^{tu} (\mathcal{C}_{quqd}^{(1)})^{sutr} (\Omega_{u,a}^* D_{\bar{\mu}} \Omega_u^b) (D^{\bar{\mu}} \bar{q}_{bs} H d_r^a) \\
& - \frac{1}{6} \bar{y}_d^{rs} (\mathcal{C}_{quqd}^{(1)})^{rtus} (D_{\bar{\mu}} \Omega_{d,a}^* D_{\bar{\mu}} \Omega_d^b) (\bar{q}_{bu} \tilde{H} u_t^a) - \frac{i}{6} \bar{y}_u^{tu} (\mathcal{C}_{quqd}^{(1)})^{sutr} (\Omega_{q,a}^* D_{\bar{\mu}} \Omega_q^b) (\Omega_{u,b}^* D_{\bar{\nu}} \Omega_u^c) (\bar{q}_{cs} H \sigma^{\bar{\mu}\bar{\nu}} d_r^a) \\
& + \frac{1}{6} \bar{y}_d^{rs} (\mathcal{C}_{quqd}^{(1)})^{rtus} \varepsilon^{kj} (D_{\bar{\mu}} \Omega_{q,aj}^* \Omega_q^{bi}) D^{\bar{\mu}} H_i^\dagger (\bar{q}_{bku} u_t^a) - \frac{1}{6} \bar{y}_d^{rs} (\mathcal{C}_{quqd}^{(1)})^{rtus} (D_{\bar{\mu}} \Omega_{d,a}^* \Omega_d^c) (D_{\bar{\mu}} \Omega_{q,b}^* \Omega_q^a) (\bar{q}_{cu} \tilde{H} u_t^b) \\
& - \frac{i}{6} \bar{y}_d^{rs} (\mathcal{C}_{quqd}^{(1)})^{rtus} (D_{\bar{\mu}} \Omega_{d,a}^* \Omega_d^c) (D_{\bar{\nu}} \Omega_{q,b}^* \Omega_q^a) (\bar{q}_{cu} \tilde{H} \sigma^{\bar{\mu}\bar{\nu}} u_t^b) + \frac{1}{6} \bar{y}_u^{tu} (\mathcal{C}_{quqd}^{(1)})^{sutr} (D_{\bar{\mu}} \Omega_{q,ai}^* D_{\bar{\mu}} \Omega_q^{bj}) H^i (\bar{q}_{bjs} d_r^a) \\
& + \frac{1}{6} \bar{y}_u^{tu} (\mathcal{C}_{quqd}^{(1)})^{sutr} (\Omega_{q,ai}^* D_{\bar{\mu}} \Omega_q^{bj}) D^{\bar{\mu}} H^i (\bar{q}_{bjs} d_r^a) - \frac{1}{6} \bar{y}_u^{tu} (\mathcal{C}_{quqd}^{(1)})^{sutr} (\Omega_{q,ai}^* D_{\bar{\mu}} \Omega_q^{bj}) H^i (\bar{q}_{bjs} D^{\bar{\mu}} d_r^a) \\
& - \frac{1}{6} \bar{y}_u^{tu} (\mathcal{C}_{quqd}^{(1)})^{sutr} (\Omega_{q,ai}^* D_{\bar{\mu}} \Omega_q^{bj}) H^i (D^{\bar{\mu}} \bar{q}_{bjs} d_r^a) - \frac{1}{6} \bar{y}_d^{rs} (\mathcal{C}_{quqd}^{(1)})^{rtus} \varepsilon^{kj} (D_{\bar{\mu}} \Omega_{q,aj}^* D_{\bar{\mu}} \Omega_q^{bi}) H_i^\dagger (\bar{q}_{bku} u_t^a) \\
& - \frac{1}{6} \bar{y}_d^{rs} (\mathcal{C}_{quqd}^{(1)})^{rtus} \varepsilon^{kj} (D_{\bar{\mu}} \Omega_{q,aj}^* \Omega_q^{bi}) H_i^\dagger (\bar{q}_{bku} D^{\bar{\mu}} u_t^a) - \frac{1}{6} \bar{y}_d^{rs} (\mathcal{C}_{quqd}^{(1)})^{rtus} \varepsilon^{kj} (D_{\bar{\mu}} \Omega_{q,aj}^* \Omega_q^{bi}) H_i^\dagger (D^{\bar{\mu}} \bar{q}_{bku} u_t^a) \\
& - \frac{1}{6} \bar{y}_u^{tu} (\mathcal{C}_{quqd}^{(1)})^{sutr} (\Omega_{q,ai}^* D_{\bar{\mu}} \Omega_q^{bj}) (\Omega_{u,b}^* D_{\bar{\mu}} \Omega_u^c) H^i (\bar{q}_{cjs} d_r^a) + \frac{i}{6} \bar{y}_u^{tu} (\mathcal{C}_{quqd}^{(1)})^{sutr} (\Omega_{q,ai}^* D_{\bar{\mu}} \Omega_q^{bj}) (\Omega_{u,b}^* D_{\bar{\nu}} \Omega_u^c) H^i (\bar{q}_{cjs} \sigma^{\bar{\mu}\bar{\nu}} d_r^a) \\
& + \frac{1}{6} \bar{y}_d^{rs} (\mathcal{C}_{quqd}^{(1)})^{rtus} (D_{\bar{\mu}} \Omega_{d,a}^* \Omega_d^c) (D_{\bar{\mu}} \Omega_{q,bj}^* \Omega_q^{ak}) \tilde{H}_j (\bar{q}_{cku} u_t^b) + \frac{i}{6} \bar{y}_d^{rs} (\mathcal{C}_{quqd}^{(1)})^{rtus} (D_{\bar{\mu}} \Omega_{d,a}^* \Omega_d^c) (D_{\bar{\nu}} \Omega_{q,bj}^* \Omega_q^{ak}) \tilde{H}_j (\bar{q}_{cku} \sigma^{\bar{\mu}\bar{\nu}} u_t^b) \\
& - \frac{1}{3} \bar{y}_u^{tu} (\bar{\mathcal{C}}_{quqd}^{(1)})^{turs} (D_{\bar{\mu}} \Omega_{q,aj}^* \Omega_q^{bi}) (D_{\bar{\mu}} \Omega_{u,b}^* \Omega_u^a) H_i^\dagger (\bar{d}_s q_r^j) - \frac{1}{3} \bar{y}_u^{tu} (\bar{\mathcal{C}}_{quqd}^{(1)})^{turs} (D_{\bar{\mu}} \Omega_{q,j}^* \Omega_q^i) H_i^\dagger (\bar{d}_s D^{\bar{\mu}} q_r^j)
\end{aligned}$$

$$\begin{aligned}
& -\frac{1}{3}y_u^{tu}(\bar{\mathcal{C}}_{quqd}^{(1)})^{turs}(D_{\bar{\mu}}\Omega_q^\dagger D_{\bar{\mu}}\Omega_q)(\bar{d}_s H^\dagger q_r) - \frac{1}{3}y_u^{tu}(\bar{\mathcal{C}}_{quqd}^{(1)})^{turs}(D_{\bar{\mu}}\Omega_u^\dagger D_{\bar{\mu}}\Omega_u)(\bar{d}_s H^\dagger q_r) \\
& -\frac{1}{3}y_u^{tu}(\bar{\mathcal{C}}_{quqd}^{(1)})^{turs}(D_{\bar{\mu}}\Omega_u^\dagger \Omega_u)(\bar{d}_s H^\dagger D_{\bar{\mu}}q_r) - \frac{1}{3}y_u^{tu}(\bar{\mathcal{C}}_{quqd}^{(1)})^{turs}(D_{\bar{\mu}}\Omega_q^\dagger \Omega_q)(\bar{d}_s D_{\bar{\mu}} H^\dagger q_r) \\
& -\frac{1}{3}y_u^{tu}(\bar{\mathcal{C}}_{quqd}^{(1)})^{turs}(D_{\bar{\mu}}\Omega_{q,j}^* \Omega_q^i)H_i^\dagger(D^{\bar{\mu}}\bar{d}_s q_r^j) - \frac{1}{3}y_u^{tu}(\bar{\mathcal{C}}_{quqd}^{(1)})^{turs}(D_{\bar{\mu}}\Omega_u^\dagger \Omega_u)(D^{\bar{\mu}}\bar{d}_s H^\dagger q_r) \\
& -\frac{i}{3}y_u^{ut}(\bar{\mathcal{C}}_{quqd}^{(1)})^{rtus}(D_{\bar{\nu}}\Omega_{q,a}^* \Omega_q^{bi})D^{\bar{\mu}}H_i^\dagger(\bar{d}_{bs}\sigma^{\bar{\mu}\bar{\nu}}q_r^{aj}) + \frac{i}{3}y_u^{ut}(\bar{\mathcal{C}}_{quqd}^{(1)})^{rtus}(D_{\bar{\nu}}\Omega_{q,a}^* \Omega_q^b)(\bar{d}_{bs}\sigma^{\bar{\mu}\bar{\nu}}D_{\bar{\mu}}H^\dagger q_r^a) \\
& +\frac{i}{3}y_u^{ut}(\bar{\mathcal{C}}_{quqd}^{(1)})^{rtus}(D_{\bar{\nu}}\Omega_{u,a}^* \Omega_u^b)(\bar{d}_{bs}\sigma^{\bar{\mu}\bar{\nu}}D_{\bar{\mu}}H^\dagger q_r^a) - \frac{1}{3}\bar{y}_u^{tu}(\mathcal{C}_{quqd}^{(1)})^{tusr}(D_{\bar{\mu}}\Omega_q^\dagger D_{\bar{\mu}}\Omega_q)(\bar{q}_s H d_r) \\
& -\frac{1}{3}\bar{y}_u^{tu}(\mathcal{C}_{quqd}^{(1)})^{tusr}(D_{\bar{\mu}}\Omega_u^\dagger D_{\bar{\mu}}\Omega_u)(\bar{q}_s H d_r) - \frac{1}{3}\bar{y}_u^{tu}(\mathcal{C}_{quqd}^{(1)})^{tusr}(\Omega_u^\dagger D_{\bar{\mu}}\Omega_u)(\bar{q}_s H D^{\bar{\mu}}d_r) \\
& -\frac{1}{3}\bar{y}_u^{tu}(\mathcal{C}_{quqd}^{(1)})^{tusr}(\Omega_q^\dagger D_{\bar{\mu}}\Omega_q)(\bar{q}_s D_{\bar{\mu}} H d_r) - \frac{1}{3}\bar{y}_u^{tu}(\mathcal{C}_{quqd}^{(1)})^{tusr}(\Omega_u^\dagger D_{\bar{\mu}}\Omega_u)(D^{\bar{\mu}}\bar{q}_s H d_r) \\
& -\frac{1}{3}\bar{y}_d^{rs}(\mathcal{C}_{quqd}^{(1)})^{turs}(D_{\bar{\mu}}\Omega_d^\dagger D_{\bar{\mu}}\Omega_d)(\bar{q}_t \tilde{H} u_u) - \frac{1}{3}\bar{y}_d^{rs}(\mathcal{C}_{quqd}^{(1)})^{turs}(D_{\bar{\mu}}\Omega_{d,a}^* \Omega_d^b)(D_{\bar{\mu}}\Omega_{q,b}^* \Omega_q^a)(\bar{q}_t \tilde{H} u_u) \\
& -\frac{1}{3}\bar{y}_d^{rs}(\mathcal{C}_{quqd}^{(1)})^{turs}(D_{\bar{\mu}}\Omega_d^\dagger \Omega_d)(\bar{q}_t D_{\bar{\mu}} \tilde{H} u_u) - \frac{1}{3}\bar{y}_u^{tu}(\mathcal{C}_{quqd}^{(1)})^{tusr}(\Omega_{q,ai}^* D_{\bar{\mu}}\Omega_q^{bj})(\Omega_{u,b}^* D_{\bar{\mu}}\Omega_u^a)H^i(\bar{q}_{js} d_r) \\
& -\frac{1}{3}\bar{y}_u^{tu}(\mathcal{C}_{quqd}^{(1)})^{tusr}(\Omega_{q,i}^* D_{\bar{\mu}}\Omega_q^j)H^i(\bar{q}_{js} D^{\bar{\mu}}d_r) - \frac{1}{3}\bar{y}_u^{tu}(\mathcal{C}_{quqd}^{(1)})^{tusr}(\Omega_{q,i}^* D_{\bar{\mu}}\Omega_q^j)H^i(D^{\bar{\mu}}\bar{q}_{js} d_r) \\
& -\frac{i}{3}\bar{y}_u^{tu}(\mathcal{C}_{quqd}^{(1)})^{sutr}(\Omega_{q,a}^* D_{\bar{\nu}}\Omega_q^b)(\bar{q}_{bs} D_{\bar{\mu}} H \sigma^{\bar{\mu}\bar{\nu}} d_r^a) - \frac{i}{3}\bar{y}_u^{tu}(\mathcal{C}_{quqd}^{(1)})^{sutr}(\Omega_{u,a}^* D_{\bar{\nu}}\Omega_u^b)(\bar{q}_{bs} D_{\bar{\mu}} H \sigma^{\bar{\mu}\bar{\nu}} d_r^a) \\
& -\frac{i}{3}\bar{y}_d^{rs}(\mathcal{C}_{quqd}^{(1)})^{rtus}(D_{\bar{\nu}}\Omega_{d,a}^* \Omega_d^b)(\bar{q}_{bu} D_{\bar{\mu}} \tilde{H} \sigma^{\bar{\mu}\bar{\nu}} u_t^a) + \frac{1}{3}\bar{y}_d^{rs}(\mathcal{C}_{quqd}^{(1)})^{turs}\varepsilon^{kj}(D_{\bar{\mu}}\Omega_{q,j}^* \Omega_q^i)D^{\bar{\mu}}H_i^\dagger(\bar{q}_{kt} u_u) \\
& +\frac{1}{3}\bar{y}_d^{rs}(\mathcal{C}_{quqd}^{(1)})^{turs}(D_{\bar{\mu}}\Omega_{d,a}^* \Omega_d^b)(D_{\bar{\mu}}\Omega_{q,bj}^* \Omega_q^{ak})\tilde{H}_j(\bar{q}_{kt} u_u) + \frac{1}{3}y_d^{tu}(\bar{\mathcal{C}}_{quqd}^{(1)})^{rstu}(\Omega_{d,a}^* D_{\bar{\mu}}\Omega_d^b)(\Omega_{q,bi}^* D_{\bar{\mu}}\Omega_q^{ak})\tilde{H}^{\dagger k}(\bar{u}_s q_r^i) \\
& -\frac{1}{6}y_d^{ru}(\bar{\mathcal{C}}_{quqd}^{(1)})^{rstu}\bar{\varepsilon}_{jk}(D_{\bar{\mu}}\Omega_{q,ai}^* D_{\bar{\mu}}\Omega_q^{bk})H^i(\bar{u}_{bs} q_t^{aj}) - \frac{1}{6}y_d^{ru}(\bar{\mathcal{C}}_{quqd}^{(1)})^{rstu}\bar{\varepsilon}_{jk}(D_{\bar{\mu}}\Omega_{q,ai}^* D_{\bar{\mu}}\Omega_q^{bk})H^i(\bar{u}_{bs} D^{\bar{\mu}}q_t^{aj}) \\
& -\frac{1}{6}y_d^{ru}(\bar{\mathcal{C}}_{quqd}^{(1)})^{rstu}(D_{\bar{\mu}}\Omega_{d,a}^* D_{\bar{\mu}}\Omega_d^b)(\bar{u}_{bs} \tilde{H}^\dagger q_t^a) - \frac{1}{6}y_d^{ru}(\bar{\mathcal{C}}_{quqd}^{(1)})^{rstu}\bar{\varepsilon}_{jk}(\Omega_{q,ai}^* D_{\bar{\mu}}\Omega_q^{bk})H^i(D^{\bar{\mu}}\bar{u}_{bs} q_t^{aj}) \\
& -\frac{1}{6}y_d^{ru}(\bar{\mathcal{C}}_{quqd}^{(1)})^{rstu}(\Omega_{d,a}^* D_{\bar{\mu}}\Omega_d^b)(\Omega_{q,b}^* D_{\bar{\mu}}\Omega_q^c)(\bar{u}_{cs} \tilde{H}^\dagger q_t^a) \\
& -\frac{i}{6}y_d^{ru}(\bar{\mathcal{C}}_{quqd}^{(1)})^{rstu}(\Omega_{d,a}^* D_{\bar{\mu}}\Omega_d^b)(\Omega_{q,bi}^* D_{\bar{\nu}}\Omega_q^{ck})\tilde{H}^{\dagger k}(\bar{u}_{cs}\sigma^{\bar{\mu}\bar{\nu}}q_t^{ai}) \\
& +\frac{i}{6}y_d^{ru}(\bar{\mathcal{C}}_{quqd}^{(1)})^{rstu}(\Omega_{d,a}^* D_{\bar{\mu}}\Omega_d^b)(\Omega_{q,b}^* D_{\bar{\nu}}\Omega_q^c)(\bar{u}_{cs}\sigma^{\bar{\mu}\bar{\nu}}\tilde{H}^\dagger q_t^a) - \frac{1}{3}\bar{y}_d^{rs}(\mathcal{C}_{quqd}^{(1)})^{turs}\varepsilon^{kj}(D_{\bar{\mu}}\Omega_{q,j}^* D_{\bar{\mu}}\Omega_q^i)H_i^\dagger(\bar{q}_{kt} u_u) \\
& -\frac{1}{3}\bar{y}_d^{rs}(\mathcal{C}_{quqd}^{(1)})^{turs}\varepsilon^{kj}(D_{\bar{\mu}}\Omega_{q,j}^* \Omega_q^i)H_i^\dagger(\bar{q}_{kt} D^{\bar{\mu}}u_u) - \frac{1}{3}\bar{y}_d^{rs}(\mathcal{C}_{quqd}^{(1)})^{turs}\varepsilon^{kj}(D_{\bar{\mu}}\Omega_{q,j}^* \Omega_q^i)H_i^\dagger(D^{\bar{\mu}}\bar{q}_{kt} u_u) \\
& +\frac{i}{3}\bar{y}_u^{tu}(\mathcal{C}_{quqd}^{(1)})^{sutr}(\Omega_{q,ai}^* D_{\bar{\nu}}\Omega_q^{bj})D^{\bar{\mu}}H^i(\bar{q}_{bj} \sigma^{\bar{\mu}\bar{\nu}} d_r^a) + \frac{i}{3}\bar{y}_d^{rs}(\mathcal{C}_{quqd}^{(1)})^{rtus}\varepsilon^{kj}(D_{\bar{\nu}}\Omega_{q,aj}^* \Omega_q^{bi})D^{\bar{\mu}}H_i^\dagger(\bar{q}_{bku} \sigma^{\bar{\mu}\bar{\nu}} u_t^a) \\
& -\frac{1}{3}y_d^{tu}(\bar{\mathcal{C}}_{quqd}^{(1)})^{rstu}\bar{\varepsilon}_{jk}(D_{\bar{\mu}}\Omega_{q,i}^* D_{\bar{\mu}}\Omega_q^k)H^i(\bar{u}_s q_r^j) - \frac{1}{3}y_d^{tu}(\bar{\mathcal{C}}_{quqd}^{(1)})^{rstu}\bar{\varepsilon}_{jk}(\Omega_{q,i}^* D_{\bar{\mu}}\Omega_q^k)H^i(\bar{u}_s D^{\bar{\mu}}q_r^j) \\
& -\frac{1}{3}y_d^{tu}(\bar{\mathcal{C}}_{quqd}^{(1)})^{rstu}(D_{\bar{\mu}}\Omega_d^\dagger D_{\bar{\mu}}\Omega_d)(\bar{u}_s \tilde{H}^\dagger q_r) - \frac{1}{3}y_d^{tu}(\bar{\mathcal{C}}_{quqd}^{(1)})^{rstu}(\Omega_{d,a}^* D_{\bar{\mu}}\Omega_d^b)(\Omega_{q,b}^* D_{\bar{\mu}}\Omega_q^a)(\bar{u}_s \tilde{H}^\dagger q_r) \\
& -\frac{1}{3}y_d^{tu}(\bar{\mathcal{C}}_{quqd}^{(1)})^{rstu}(\Omega_d^\dagger D_{\bar{\mu}}\Omega_d)(\bar{u}_s D_{\bar{\mu}} \tilde{H}^\dagger q_r) - \frac{1}{3}y_d^{tu}(\bar{\mathcal{C}}_{quqd}^{(1)})^{rstu}\bar{\varepsilon}_{jk}(\Omega_{q,i}^* D_{\bar{\mu}}\Omega_q^k)H^i(D^{\bar{\mu}}\bar{u}_s q_r^j)
\end{aligned}$$

$$-\frac{i}{3}y_d^{ru}(\bar{\mathcal{C}}_{quqd}^{(1)})^{rstu}\bar{\varepsilon}_{jk}(\Omega_{q,ai}^*D_{\bar{\nu}}\Omega_q^{bk})D^{\bar{\mu}}H^i(\bar{u}_{bs}\sigma^{\bar{\mu}\bar{\nu}}q_t^{aj})+\frac{i}{3}y_d^{ru}(\bar{\mathcal{C}}_{quqd}^{(1)})^{rstu}(\Omega_{d,a}^*D_{\bar{\nu}}\Omega_d^b)(\bar{u}_{bs}\sigma^{\bar{\mu}\bar{\nu}}D_{\bar{\mu}}\tilde{H}^\dagger q_t^a), \quad (3.61)$$

$$\begin{aligned} \Gamma_\Omega^{(1)}[\mathcal{O}_{quqd}^{(8)}] = & \frac{1}{36}\left[2y_u^{tu}(\bar{\mathcal{C}}_{quqd}^{(8)})^{turs}-3y_u^{ut}(\bar{\mathcal{C}}_{quqd}^{(8)})^{rtus}\right](D_{\bar{\mu}}\Omega_{q,a}^*\Omega_q^{bi})(D_{\bar{\mu}}\Omega_{u,b}^*\Omega_u^a)H_i^\dagger(\bar{d}_sq_r^j) \\ & +\frac{1}{36}\left[3y_u^{ut}(\bar{\mathcal{C}}_{quqd}^{(8)})^{rtus}-2y_u^{tu}(\bar{\mathcal{C}}_{quqd}^{(8)})^{turs}\right](D_{\bar{\mu}}\Omega_{q,j}^*\Omega_q^i)D^{\bar{\mu}}H_i^\dagger(\bar{d}_sq_r^j) \\ & +\frac{1}{36}\left[3y_u^{ut}(\bar{\mathcal{C}}_{quqd}^{(8)})^{rtus}-2y_u^{tu}(\bar{\mathcal{C}}_{quqd}^{(8)})^{turs}\right](D_{\bar{\mu}}\Omega_{q,j}^*D_{\bar{\mu}}\Omega_q^i)H_i^\dagger(\bar{d}_sq_r^j) \\ & +\frac{1}{36}\left[2y_u^{tu}(\bar{\mathcal{C}}_{quqd}^{(8)})^{turs}-3y_u^{ut}(\bar{\mathcal{C}}_{quqd}^{(8)})^{rtus}\right](D_{\bar{\mu}}\Omega_{q,j}^*\Omega_q^i)H_i^\dagger(\bar{d}_sD^{\bar{\mu}}q_r^j) \\ & +\frac{1}{36}\left[2y_u^{tu}(\bar{\mathcal{C}}_{quqd}^{(8)})^{turs}-3y_u^{ut}(\bar{\mathcal{C}}_{quqd}^{(8)})^{rtus}\right](D_{\bar{\mu}}\Omega_q^\dagger D_{\bar{\mu}}\Omega_q)(\bar{d}_sH^\dagger q_r) \\ & +\frac{1}{36}\left[2y_u^{tu}(\bar{\mathcal{C}}_{quqd}^{(8)})^{turs}-3y_u^{ut}(\bar{\mathcal{C}}_{quqd}^{(8)})^{rtus}\right](D_{\bar{\mu}}\Omega_u^\dagger D_{\bar{\mu}}\Omega_u)(\bar{d}_sH^\dagger q_r) \\ & +\frac{1}{36}\left[3y_u^{ut}(\bar{\mathcal{C}}_{quqd}^{(8)})^{rtus}-2y_u^{tu}(\bar{\mathcal{C}}_{quqd}^{(8)})^{turs}\right](D_{\bar{\mu}}\Omega_{q,a}^*\Omega_q^b)(D_{\bar{\mu}}\Omega_{u,b}^*\Omega_u^a)(\bar{d}_sH^\dagger q_r) \\ & +\frac{1}{36}\left[2y_u^{tu}(\bar{\mathcal{C}}_{quqd}^{(8)})^{turs}-3y_u^{ut}(\bar{\mathcal{C}}_{quqd}^{(8)})^{rtus}\right](D_{\bar{\mu}}\Omega_u^\dagger\Omega_u)(\bar{d}_sH^\dagger D^{\bar{\mu}}q_r) \\ & +\frac{1}{36}\left[3y_u^{ut}(\bar{\mathcal{C}}_{quqd}^{(8)})^{rtus}-2y_u^{tu}(\bar{\mathcal{C}}_{quqd}^{(8)})^{turs}\right](D_{\bar{\mu}}\Omega_q^\dagger\Omega_q)(\bar{d}_sH^\dagger D^{\bar{\mu}}q_r) \\ & +\frac{1}{36}\left[2y_u^{tu}(\bar{\mathcal{C}}_{quqd}^{(8)})^{turs}-3y_u^{ut}(\bar{\mathcal{C}}_{quqd}^{(8)})^{rtus}\right](D_{\bar{\mu}}\Omega_q^\dagger\Omega_q)(\bar{d}_sD_{\bar{\mu}}H^\dagger q_r) \\ & +\frac{1}{36}\left[3y_u^{ut}(\bar{\mathcal{C}}_{quqd}^{(8)})^{rtus}-2y_u^{tu}(\bar{\mathcal{C}}_{quqd}^{(8)})^{turs}\right](D_{\bar{\mu}}\Omega_u^\dagger\Omega_u)(\bar{d}_sD_{\bar{\mu}}H^\dagger q_r) \\ & +\frac{1}{36}\left[2y_u^{tu}(\bar{\mathcal{C}}_{quqd}^{(8)})^{turs}-3y_u^{ut}(\bar{\mathcal{C}}_{quqd}^{(8)})^{rtus}\right](D_{\bar{\mu}}\Omega_{q,j}^*\Omega_q^i)H_i^\dagger(D^{\bar{\mu}}\bar{d}_sq_r^j) \\ & +\frac{1}{36}\left[2y_u^{tu}(\bar{\mathcal{C}}_{quqd}^{(8)})^{turs}-3y_u^{ut}(\bar{\mathcal{C}}_{quqd}^{(8)})^{rtus}\right](D_{\bar{\mu}}\Omega_u^\dagger\Omega_u)(D^{\bar{\mu}}\bar{d}_sH^\dagger q_r) \\ & +\frac{1}{36}\left[3y_u^{ut}(\bar{\mathcal{C}}_{quqd}^{(8)})^{rtus}-2y_u^{tu}(\bar{\mathcal{C}}_{quqd}^{(8)})^{turs}\right](D_{\bar{\mu}}\Omega_q^\dagger\Omega_q)(D^{\bar{\mu}}\bar{d}_sH^\dagger q_r) \\ & +\frac{1}{36}\left[6y_u^{tu}(\bar{\mathcal{C}}_{quqd}^{(8)})^{turs}-y_u^{ut}(\bar{\mathcal{C}}_{quqd}^{(8)})^{rtus}\right](D_{\bar{\mu}}\Omega_{q,aj}^*\Omega_q^{bi})D^{\bar{\mu}}H_i^\dagger(\bar{d}_{bs}q_r^{aj}) \\ & +\frac{1}{36}\left[6y_u^{tu}(\bar{\mathcal{C}}_{quqd}^{(8)})^{turs}-y_u^{ut}(\bar{\mathcal{C}}_{quqd}^{(8)})^{rtus}\right](D_{\bar{\mu}}\Omega_{q,aj}^*D_{\bar{\mu}}\Omega_q^{bi})H_i^\dagger(\bar{d}_{bs}q_r^{aj}) \\ & +\frac{1}{36}\left[y_u^{ut}(\bar{\mathcal{C}}_{quqd}^{(8)})^{rtus}-6y_u^{tu}(\bar{\mathcal{C}}_{quqd}^{(8)})^{turs}\right](D_{\bar{\mu}}\Omega_{q,aj}^*\Omega_q^{bi})H_i^\dagger(\bar{d}_{bs}D^{\bar{\mu}}q_r^{aj}) \\ & +\frac{1}{36}\left[y_u^{ut}(\bar{\mathcal{C}}_{quqd}^{(8)})^{rtus}-6y_u^{tu}(\bar{\mathcal{C}}_{quqd}^{(8)})^{turs}\right](D_{\bar{\mu}}\Omega_{q,a}^*D_{\bar{\mu}}\Omega_q^b)(\bar{d}_{bs}H^\dagger q_r^a) \\ & +\frac{1}{36}\left[y_u^{ut}(\bar{\mathcal{C}}_{quqd}^{(8)})^{rtus}-6y_u^{tu}(\bar{\mathcal{C}}_{quqd}^{(8)})^{turs}\right](D_{\bar{\mu}}\Omega_{u,a}^*D_{\bar{\mu}}\Omega_u^b)(\bar{d}_{bs}H^\dagger q_r^a) \\ & +\frac{1}{36}\left[6y_u^{tu}(\bar{\mathcal{C}}_{quqd}^{(8)})^{turs}-y_u^{ut}(\bar{\mathcal{C}}_{quqd}^{(8)})^{rtus}\right](D_{\bar{\mu}}\Omega_{q,a}^*\Omega_q^b)(\bar{d}_{bs}H^\dagger D^{\bar{\mu}}q_r^a) \\ & +\frac{1}{36}\left[y_u^{ut}(\bar{\mathcal{C}}_{quqd}^{(8)})^{rtus}-6y_u^{tu}(\bar{\mathcal{C}}_{quqd}^{(8)})^{turs}\right](D_{\bar{\mu}}\Omega_{u,a}^*\Omega_u^b)(\bar{d}_{bs}H^\dagger D^{\bar{\mu}}q_r^a) \\ & +\frac{1}{36}\left[6y_u^{tu}(\bar{\mathcal{C}}_{quqd}^{(8)})^{turs}-y_u^{ut}(\bar{\mathcal{C}}_{quqd}^{(8)})^{rtus}\right](D_{\bar{\mu}}\Omega_{u,a}^*\Omega_u^b)(\bar{d}_{bs}D_{\bar{\mu}}H^\dagger q_r^a) \end{aligned}$$

$$\begin{aligned}
& + \frac{1}{36} \left[ y_u^{ut} (\bar{\mathcal{C}}_{quqd}^{(8)})^{rtus} - 6y_u^{tu} (\bar{\mathcal{C}}_{quqd}^{(8)})^{turs} \right] (D_{\bar{\mu}} \Omega_{q,a}^* \Omega_q^b) (\bar{d}_{bs} D_{\bar{\mu}} H^\dagger q_r^a) \\
& + \frac{1}{36} \left[ y_u^{ut} (\bar{\mathcal{C}}_{quqd}^{(8)})^{rtus} - 6y_u^{tu} (\bar{\mathcal{C}}_{quqd}^{(8)})^{turs} \right] (D_{\bar{\mu}} \Omega_{q,aj}^* \Omega_q^{bi}) H_i^\dagger (D^{\bar{\mu}} \bar{d}_{bs} q_r^{aj}) \\
& + \frac{1}{36} \left[ 6y_u^{tu} (\bar{\mathcal{C}}_{quqd}^{(8)})^{turs} - y_u^{ut} (\bar{\mathcal{C}}_{quqd}^{(8)})^{rtus} \right] (D_{\bar{\mu}} \Omega_{q,a}^* \Omega_q^b) (D^{\bar{\mu}} \bar{d}_{bs} H^\dagger q_r^a) \\
& + \frac{1}{36} \left[ y_u^{ut} (\bar{\mathcal{C}}_{quqd}^{(8)})^{rtus} - 6y_u^{tu} (\bar{\mathcal{C}}_{quqd}^{(8)})^{turs} \right] (D_{\bar{\mu}} \Omega_{u,a}^* \Omega_u^b) (D^{\bar{\mu}} \bar{d}_{bs} H^\dagger q_r^a) \\
& + \frac{1}{36} \left[ y_u^{ut} (\bar{\mathcal{C}}_{quqd}^{(8)})^{rtus} - 6y_u^{tu} (\bar{\mathcal{C}}_{quqd}^{(8)})^{turs} \right] (D_{\bar{\mu}} \Omega_{q,aj}^* \Omega_q^{ci}) (D_{\bar{\mu}} \Omega_{u,b}^* \Omega_u^a) H_i^\dagger (\bar{d}_{cs} q_r^{bj}) \\
& + \frac{1}{36} \left[ 6y_u^{tu} (\bar{\mathcal{C}}_{quqd}^{(8)})^{turs} - y_u^{ut} (\bar{\mathcal{C}}_{quqd}^{(8)})^{rtus} \right] (D_{\bar{\mu}} \Omega_{q,a}^* \Omega_q^c) (D_{\bar{\mu}} \Omega_{u,b}^* \Omega_u^a) (\bar{d}_{cs} H^\dagger q_r^b) \\
& + \frac{i}{36} y_u^{ut} (\bar{\mathcal{C}}_{quqd}^{(8)})^{rtus} (D_{\bar{\mu}} \Omega_{q,aj}^* \Omega_q^{ci}) (D_{\bar{\nu}} \Omega_{u,b}^* \Omega_u^a) H_i^\dagger (\bar{d}_{cs} \sigma^{\bar{\mu}\bar{\nu}} q_r^{bj}) \\
& - \frac{i}{36} y_u^{ut} (\bar{\mathcal{C}}_{quqd}^{(8)})^{rtus} (D_{\bar{\mu}} \Omega_{q,a}^* \Omega_q^c) (D_{\bar{\nu}} \Omega_{u,b}^* \Omega_u^a) (\bar{d}_{cs} \sigma^{\bar{\mu}\bar{\nu}} H^\dagger q_r^b) \\
& + \frac{1}{36} \bar{y}_u^{tu} \left[ 3(\mathcal{C}_{quqd}^{(8)})^{sutr} - 2(\mathcal{C}_{quqd}^{(8)})^{tusr} \right] (\Omega_{q,a}^* D_{\bar{\mu}} \Omega_q^b) (\Omega_{u,b}^* D_{\bar{\mu}} \Omega_u^a) (\bar{q}_s H d_r) \\
& + \frac{1}{36} \bar{y}_u^{tu} \left[ 2(\mathcal{C}_{quqd}^{(8)})^{tusr} - 3(\mathcal{C}_{quqd}^{(8)})^{sutr} \right] (D_{\bar{\mu}} \Omega_q^\dagger D_{\bar{\mu}} \Omega_q) (\bar{q}_s H d_r) \\
& + \frac{1}{36} \bar{y}_u^{tu} \left[ 2(\mathcal{C}_{quqd}^{(8)})^{tusr} - 3(\mathcal{C}_{quqd}^{(8)})^{sutr} \right] (D_{\bar{\mu}} \Omega_u^\dagger D_{\bar{\mu}} \Omega_u) (\bar{q}_s H d_r) \\
& + \frac{1}{36} \bar{y}_u^{tu} \left[ 3(\mathcal{C}_{quqd}^{(8)})^{sutr} - 2(\mathcal{C}_{quqd}^{(8)})^{tusr} \right] (\Omega_q^\dagger D_{\bar{\mu}} \Omega_q) (\bar{q}_s H D^{\bar{\mu}} d_r) \\
& + \frac{1}{36} \bar{y}_u^{tu} \left[ 2(\mathcal{C}_{quqd}^{(8)})^{tusr} - 3(\mathcal{C}_{quqd}^{(8)})^{sutr} \right] (\Omega_u^\dagger D_{\bar{\mu}} \Omega_u) (\bar{q}_s H D^{\bar{\mu}} d_r) \\
& + \frac{1}{36} \bar{y}_u^{tu} \left[ 3(\mathcal{C}_{quqd}^{(8)})^{sutr} - 2(\mathcal{C}_{quqd}^{(8)})^{tusr} \right] (\Omega_u^\dagger D_{\bar{\mu}} \Omega_u) (\bar{q}_s D_{\bar{\mu}} H d_r) \\
& + \frac{1}{36} \bar{y}_u^{tu} \left[ 2(\mathcal{C}_{quqd}^{(8)})^{tusr} - 3(\mathcal{C}_{quqd}^{(8)})^{sutr} \right] (\Omega_q^\dagger D_{\bar{\mu}} \Omega_q) (\bar{q}_s D_{\bar{\mu}} H d_r) \\
& + \frac{1}{36} \bar{y}_u^{tu} \left[ 3(\mathcal{C}_{quqd}^{(8)})^{sutr} - 2(\mathcal{C}_{quqd}^{(8)})^{tusr} \right] (\Omega_q^\dagger D_{\bar{\mu}} \Omega_q) (D^{\bar{\mu}} \bar{q}_s H d_r) \\
& + \frac{1}{36} \bar{y}_u^{tu} \left[ 2(\mathcal{C}_{quqd}^{(8)})^{tusr} - 3(\mathcal{C}_{quqd}^{(8)})^{sutr} \right] (\Omega_u^\dagger D_{\bar{\mu}} \Omega_u) (D^{\bar{\mu}} \bar{q}_s H d_r) \\
& + \frac{1}{36} \bar{y}_u^{tu} \left[ 3(\mathcal{C}_{quqd}^{(8)})^{sutr} - 2(\mathcal{C}_{quqd}^{(8)})^{tusr} \right] (D_{\bar{\mu}} \Omega_{q,i}^* D_{\bar{\mu}} \Omega_q^j) H^i (\bar{q}_{js} d_r) \\
& + \frac{1}{36} \bar{y}_u^{tu} \left[ 2(\mathcal{C}_{quqd}^{(8)})^{tusr} - 3(\mathcal{C}_{quqd}^{(8)})^{sutr} \right] (\Omega_{q,ai}^* D_{\bar{\mu}} \Omega_q^{bj}) (\Omega_{u,b}^* D_{\bar{\mu}} \Omega_u^a) H^i (\bar{q}_{js} d_r) \\
& + \frac{1}{36} \bar{y}_u^{tu} \left[ 3(\mathcal{C}_{quqd}^{(8)})^{sutr} - 2(\mathcal{C}_{quqd}^{(8)})^{tusr} \right] (\Omega_{q,i}^* D_{\bar{\mu}} \Omega_q^j) D^{\bar{\mu}} H^i (\bar{q}_{js} d_r) \\
& + \frac{1}{36} \bar{y}_u^{tu} \left[ 2(\mathcal{C}_{quqd}^{(8)})^{tusr} - 3(\mathcal{C}_{quqd}^{(8)})^{sutr} \right] (\Omega_{q,i}^* D_{\bar{\mu}} \Omega_q^j) H^i (\bar{q}_{js} D^{\bar{\mu}} d_r) \\
& + \frac{1}{36} \bar{y}_u^{tu} \left[ 2(\mathcal{C}_{quqd}^{(8)})^{tusr} - 3(\mathcal{C}_{quqd}^{(8)})^{sutr} \right] (\Omega_{q,i}^* D_{\bar{\mu}} \Omega_q^j) H^i (D^{\bar{\mu}} \bar{q}_{js} d_r) \\
& + \frac{1}{36} \bar{y}_u^{tu} \left[ (\mathcal{C}_{quqd}^{(8)})^{sutr} - 6(\mathcal{C}_{quqd}^{(8)})^{tusr} \right] (D_{\bar{\mu}} \Omega_{q,a}^* D_{\bar{\mu}} \Omega_q^b) (\bar{q}_{bs} H d_r^a)
\end{aligned}$$

$$\begin{aligned}
& + \frac{1}{36} \bar{y}_u^{tu} \left[ (\mathcal{C}_{quqd}^{(8)})^{sutr} - 6(\mathcal{C}_{quqd}^{(8)})^{tusr} \right] (D_{\bar{\mu}} \Omega_{u,a}^* D_{\bar{\mu}} \Omega_u^b) (\bar{q}_{bs} H d_r^a) \\
& + \frac{1}{36} \bar{y}_u^{tu} \left[ (\mathcal{C}_{quqd}^{(8)})^{sutr} - 6(\mathcal{C}_{quqd}^{(8)})^{tusr} \right] (\Omega_{u,a}^* D_{\bar{\mu}} \Omega_u^b) (\bar{q}_{bs} H D^{\bar{\mu}} d_r^a) \\
& + \frac{1}{36} \bar{y}_u^{tu} \left[ (\mathcal{C}_{quqd}^{(8)})^{sutr} - 6(\mathcal{C}_{quqd}^{(8)})^{tusr} \right] (\Omega_{q,a}^* D_{\bar{\mu}} \Omega_q^b) (\bar{q}_{bs} D_{\bar{\mu}} H d_r^a) \\
& + \frac{1}{36} \bar{y}_u^{tu} \left[ (\mathcal{C}_{quqd}^{(8)})^{sutr} - 6(\mathcal{C}_{quqd}^{(8)})^{tusr} \right] (\Omega_{u,a}^* D_{\bar{\mu}} \Omega_u^b) (D^{\bar{\mu}} \bar{q}_{bs} H d_r^a) \\
& + \frac{1}{36} \bar{y}_d^{rs} (\mathcal{C}_{quqd}^{(8)})^{rtus} (D_{\bar{\mu}} \Omega_{d,a}^* D_{\bar{\mu}} \Omega_d^b) (\bar{q}_{bu} \tilde{H} u_t^a) + \frac{1}{36} \bar{y}_u^{tu} \left[ (\mathcal{C}_{quqd}^{(8)})^{sutr} - 6(\mathcal{C}_{quqd}^{(8)})^{tusr} \right] (\Omega_{q,ai}^* D_{\bar{\mu}} \Omega_q^{bj}) H^i (\bar{q}_{bjs} D^{\bar{\mu}} d_r^a) \\
& + \frac{1}{36} \bar{y}_u^{tu} \left[ (\mathcal{C}_{quqd}^{(8)})^{sutr} - 6(\mathcal{C}_{quqd}^{(8)})^{tusr} \right] (\Omega_{q,ai}^* D_{\bar{\mu}} \Omega_q^{bj}) H^i (D^{\bar{\mu}} \bar{q}_{bjs} d_r^a) + \frac{1}{36} \bar{y}_d^{rs} (\mathcal{C}_{quqd}^{(8)})^{rtus} \varepsilon^{kj} (D_{\bar{\mu}} \Omega_{q,aj}^* D_{\bar{\mu}} \Omega_q^{bi}) H_i^\dagger (\bar{q}_{bku} u_t^a) \\
& + \frac{1}{36} \bar{y}_d^{rs} (\mathcal{C}_{quqd}^{(8)})^{rtus} \varepsilon^{kj} (D_{\bar{\mu}} \Omega_{q,aj}^* \Omega_q^{bi}) H_i^\dagger (\bar{q}_{bku} D^{\bar{\mu}} u_t^a) + \frac{1}{36} \bar{y}_d^{rs} (\mathcal{C}_{quqd}^{(8)})^{rtus} \varepsilon^{kj} (D_{\bar{\mu}} \Omega_{q,aj}^* \Omega_q^{bi}) H_i^\dagger (D^{\bar{\mu}} \bar{q}_{bku} u_t^a) \\
& + \frac{1}{36} \bar{y}_u^{tu} \left[ (\mathcal{C}_{quqd}^{(8)})^{sutr} - 6(\mathcal{C}_{quqd}^{(8)})^{tusr} \right] (\Omega_{q,ai}^* D_{\bar{\mu}} \Omega_q^{bj}) (\Omega_{u,b}^* D_{\bar{\mu}} \Omega_u^c) H^i (\bar{q}_{cjs} d_r^a) \\
& + \frac{1}{36} \bar{y}_d^{ru} (\bar{\mathcal{C}}_{quqd}^{(8)})^{rstu} \bar{\varepsilon}_{jk} (D_{\bar{\mu}} \Omega_{q,ai}^* D_{\bar{\mu}} \Omega_q^{bk}) H^i (\bar{u}_{bs} q_t^{aj}) \\
& + \frac{1}{36} \bar{y}_d^{ru} (\bar{\mathcal{C}}_{quqd}^{(8)})^{rstu} \bar{\varepsilon}_{jk} (\Omega_{q,ai}^* D_{\bar{\mu}} \Omega_q^{bk}) H^i (\bar{u}_{bs} D^{\bar{\mu}} q_t^{aj}) + \frac{1}{36} \bar{y}_d^{ru} (\bar{\mathcal{C}}_{quqd}^{(8)})^{rstu} (D_{\bar{\mu}} \Omega_{d,a}^* D_{\bar{\mu}} \Omega_d^b) (\bar{u}_{bs} \tilde{H}^\dagger q_t^a) \\
& + \frac{1}{36} \bar{y}_d^{ru} (\bar{\mathcal{C}}_{quqd}^{(8)})^{rstu} \bar{\varepsilon}_{jk} (\Omega_{q,ai}^* D_{\bar{\mu}} \Omega_q^{bk}) H^i (D^{\bar{\mu}} \bar{u}_{bs} q_t^{aj}) + \frac{1}{36} \bar{y}_d^{ru} (\bar{\mathcal{C}}_{quqd}^{(8)})^{rstu} (\Omega_{d,a}^* D_{\bar{\mu}} \Omega_d^b) (\Omega_{q,b}^* D_{\bar{\mu}} \Omega_q^c) (\bar{u}_{cs} \tilde{H}^\dagger q_t^a) \\
& + \frac{i}{36} \bar{y}_d^{ru} (\bar{\mathcal{C}}_{quqd}^{(8)})^{rstu} (\Omega_{d,a}^* D_{\bar{\mu}} \Omega_d^b) (\Omega_{q,bi}^* D_{\bar{\nu}} \Omega_q^{ck}) \tilde{H}^{\dagger k} (\bar{u}_{cs} \sigma^{\bar{\mu}\bar{\nu}} q_t^{ai}) \\
& - \frac{i}{36} \bar{y}_d^{ru} (\bar{\mathcal{C}}_{quqd}^{(8)})^{rstu} (\Omega_{d,a}^* D_{\bar{\mu}} \Omega_d^b) (\Omega_{q,b}^* D_{\bar{\nu}} \Omega_q^c) (\bar{u}_{cs} \sigma^{\bar{\mu}\bar{\nu}} \tilde{H}^\dagger q_t^a) + \frac{i}{18} \bar{y}_u^{ut} (\bar{\mathcal{C}}_{quqd}^{(8)})^{rtus} (D_{\bar{\nu}} \Omega_{q,aj}^* \Omega_q^{bi}) D^{\bar{\mu}} H_i^\dagger (\bar{d}_{bs} \sigma^{\bar{\mu}\bar{\nu}} q_r^{aj}) \\
& - \frac{i}{18} \bar{y}_u^{ut} (\bar{\mathcal{C}}_{quqd}^{(8)})^{rtus} (D_{\bar{\nu}} \Omega_{q,a}^* \Omega_q^b) (\bar{d}_{bs} \sigma^{\bar{\mu}\bar{\nu}} D_{\bar{\mu}} H^\dagger q_r^a) - \frac{i}{18} \bar{y}_u^{ut} (\bar{\mathcal{C}}_{quqd}^{(8)})^{rtus} (D_{\bar{\nu}} \Omega_{u,a}^* \Omega_u^b) (\bar{d}_{bs} \sigma^{\bar{\mu}\bar{\nu}} D_{\bar{\mu}} H^\dagger q_r^a) \\
& + \frac{1}{18} \bar{y}_d^{rs} (\mathcal{C}_{quqd}^{(8)})^{turs} (D_{\bar{\mu}} \Omega_d^\dagger D_{\bar{\mu}} \Omega_d) (\bar{q}_t \tilde{H} u_u) + \frac{1}{18} \bar{y}_d^{rs} (\mathcal{C}_{quqd}^{(8)})^{turs} (D_{\bar{\mu}} \Omega_{d,a}^* \Omega_d^b) (D_{\bar{\mu}} \Omega_{q,b}^* \Omega_q^a) (\bar{q}_t \tilde{H} u_u) \\
& + \frac{1}{18} \bar{y}_d^{rs} (\mathcal{C}_{quqd}^{(8)})^{turs} (D_{\bar{\mu}} \Omega_d^\dagger \Omega_d) (\bar{q}_t D_{\bar{\mu}} \tilde{H} u_u) + \frac{1}{18} \bar{y}_d^{rs} (\mathcal{C}_{quqd}^{(8)})^{turs} \varepsilon^{kj} (D_{\bar{\mu}} \Omega_{q,j}^* \Omega_q^i) H_i^\dagger (\bar{q}_{kt} D^{\bar{\mu}} u_u) \\
& + \frac{1}{18} \bar{y}_d^{rs} (\mathcal{C}_{quqd}^{(8)})^{turs} \varepsilon^{kj} (D_{\bar{\mu}} \Omega_{q,j}^* \Omega_q^i) H_i^\dagger (D^{\bar{\mu}} \bar{q}_{kt} u_u) + \frac{1}{18} \bar{y}_d^{tu} (\bar{\mathcal{C}}_{quqd}^{(8)})^{rstu} (D_{\bar{\mu}} \Omega_d^\dagger D_{\bar{\mu}} \Omega_d) (\bar{u}_s \tilde{H}^\dagger q_r) \\
& + \frac{1}{18} \bar{y}_d^{tu} (\bar{\mathcal{C}}_{quqd}^{(8)})^{rstu} (\Omega_{d,a}^* D_{\bar{\mu}} \Omega_d^b) (\Omega_{q,b}^* D_{\bar{\mu}} \Omega_q^a) (\bar{u}_s \tilde{H}^\dagger q_r) + \frac{1}{18} \bar{y}_d^{tu} (\bar{\mathcal{C}}_{quqd}^{(8)})^{rstu} (\Omega_d^\dagger D_{\bar{\mu}} \Omega_d) (\bar{u}_s D_{\bar{\mu}} \tilde{H}^\dagger q_r) \\
& + \frac{1}{18} \bar{y}_d^{tu} (\bar{\mathcal{C}}_{quqd}^{(8)})^{rstu} \bar{\varepsilon}_{jk} (\Omega_{q,i}^* D_{\bar{\mu}} \Omega_q^k) H^i (D^{\bar{\mu}} \bar{u}_s q_r^j) - \frac{i}{18} \bar{y}_d^{ru} (\bar{\mathcal{C}}_{quqd}^{(8)})^{rstu} (\Omega_{d,a}^* D_{\bar{\nu}} \Omega_d^b) (\bar{u}_{bs} \sigma^{\bar{\mu}\bar{\nu}} D_{\bar{\mu}} \tilde{H}^\dagger q_t^a) \\
& - \frac{i}{12} \bar{y}_u^{ut} (\bar{\mathcal{C}}_{quqd}^{(8)})^{rtus} (D_{\bar{\mu}} \Omega_{q,aj}^* \Omega_q^{bi}) (D_{\bar{\nu}} \Omega_{u,b}^* \Omega_u^a) H_i^\dagger (\bar{d}_s \sigma^{\bar{\mu}\bar{\nu}} q_r^j) \\
& + \frac{i}{12} \bar{y}_u^{ut} (\bar{\mathcal{C}}_{quqd}^{(8)})^{rtus} (D_{\bar{\mu}} \Omega_{q,a}^* \Omega_q^b) (D_{\bar{\nu}} \Omega_{u,b}^* \Omega_u^a) (\bar{d}_s \sigma^{\bar{\mu}\bar{\nu}} H^\dagger q_r) + \frac{1}{12} \bar{y}_d^{rs} (\mathcal{C}_{quqd}^{(8)})^{rtus} (D_{\bar{\mu}} \Omega_d^\dagger \Omega_d) (\bar{q}_u \tilde{H} D^{\bar{\mu}} u_t) \\
& + \frac{1}{12} \bar{y}_d^{rs} (\mathcal{C}_{quqd}^{(8)})^{rtus} (D_{\bar{\mu}} \Omega_d^\dagger \Omega_d) (D^{\bar{\mu}} \bar{q}_u \tilde{H} u_t) + \frac{1}{12} \bar{y}_d^{rs} (\mathcal{C}_{quqd}^{(8)})^{rtus} \varepsilon^{kj} (D_{\bar{\mu}} \Omega_{q,j}^* \Omega_q^i) D^{\bar{\mu}} H_i^\dagger (\bar{q}_{ku} u_t) \\
& + \frac{1}{12} \bar{y}_d^{rs} (\mathcal{C}_{quqd}^{(8)})^{rtus} (D_{\bar{\mu}} \Omega_{d,a}^* \Omega_d^b) (D_{\bar{\mu}} \Omega_{q,bj}^* \Omega_q^{ak}) \tilde{H}_j (\bar{q}_{ku} u_t) + \frac{1}{12} \bar{y}_d^{ru} (\bar{\mathcal{C}}_{quqd}^{(8)})^{rstu} \bar{\varepsilon}_{jk} (\Omega_{q,i}^* D_{\bar{\mu}} \Omega_q^k) D^{\bar{\mu}} H^i (\bar{u}_s q_t^j)
\end{aligned}$$

$$\begin{aligned}
& + \frac{1}{12} y_d^{ru} (\bar{\mathcal{C}}_{quqd}^{(8)})^{rstu} (\Omega_d^\dagger D_{\bar{\mu}} \Omega_d) (\bar{u}_s \tilde{H}^\dagger D^{\bar{\mu}} q_t) + \frac{1}{12} y_d^{ru} (\bar{\mathcal{C}}_{quqd}^{(8)})^{rstu} (\Omega_d^\dagger D_{\bar{\mu}} \Omega_d) (D^{\bar{\mu}} \bar{u}_s \tilde{H}^\dagger q_t) \\
& - \frac{i}{6} y_u^{ut} (\bar{\mathcal{C}}_{quqd}^{(8)})^{rtus} (D_{\bar{\nu}} \Omega_{q,j}^* \Omega_q^i) D^{\bar{\mu}} H_i^\dagger (\bar{d}_s \sigma^{\bar{\mu}\bar{\nu}} q_r^j) + \frac{i}{6} y_u^{ut} (\bar{\mathcal{C}}_{quqd}^{(8)})^{rtus} (D_{\bar{\nu}} \Omega_q^\dagger \Omega_q) (\bar{d}_s \sigma^{\bar{\mu}\bar{\nu}} D_{\bar{\mu}} H^\dagger q_r) \\
& + \frac{i}{6} y_u^{ut} (\bar{\mathcal{C}}_{quqd}^{(8)})^{rtus} (D_{\bar{\nu}} \Omega_u^\dagger \Omega_u) (\bar{d}_s \sigma^{\bar{\mu}\bar{\nu}} D_{\bar{\mu}} H^\dagger q_r) + \frac{1}{6} \bar{y}_d^{rs} (\mathcal{C}_{quqd}^{(8)})^{turs} (D_{\bar{\mu}} \Omega_{d,a}^* \Omega_d^b) (\bar{q}_{bt} \tilde{H} D^{\bar{\mu}} u_u^a) \\
& + \frac{1}{6} \bar{y}_d^{rs} (\mathcal{C}_{quqd}^{(8)})^{turs} (D_{\bar{\mu}} \Omega_{d,a}^* \Omega_d^b) (\bar{q}_{bt} D_{\bar{\mu}} \tilde{H} u_u^a) + \frac{1}{6} \bar{y}_d^{rs} (\mathcal{C}_{quqd}^{(8)})^{turs} (D_{\bar{\mu}} \Omega_{d,a}^* \Omega_d^b) (D^{\bar{\mu}} \bar{q}_{bt} \tilde{H} u_u^a) \\
& + \frac{1}{6} y_d^{tu} (\bar{\mathcal{C}}_{quqd}^{(8)})^{rstu} \bar{\varepsilon}_{jk} (\Omega_{q,ai}^* D_{\bar{\mu}} \Omega_q^{bk}) D^{\bar{\mu}} H^i (\bar{u}_{bs} q_r^{aj}) + \frac{1}{6} y_d^{tu} (\bar{\mathcal{C}}_{quqd}^{(8)})^{rstu} (\Omega_{d,a}^* D_{\bar{\mu}} \Omega_d^b) (\bar{u}_{bs} \tilde{H}^\dagger D^{\bar{\mu}} q_r^a) \\
& + \frac{1}{6} y_d^{tu} (\bar{\mathcal{C}}_{quqd}^{(8)})^{rstu} (\Omega_{d,a}^* D_{\bar{\mu}} \Omega_d^b) (\bar{u}_{bs} D_{\bar{\mu}} \tilde{H}^\dagger q_r^a) + \frac{1}{6} y_d^{tu} (\bar{\mathcal{C}}_{quqd}^{(8)})^{rstu} (\Omega_{d,a}^* D_{\bar{\mu}} \Omega_d^b) (D^{\bar{\mu}} \bar{u}_{bs} \tilde{H}^\dagger q_r^a) \\
& + \frac{1}{6} y_d^{tu} (\bar{\mathcal{C}}_{quqd}^{(8)})^{rstu} (\Omega_{d,a}^* D_{\bar{\mu}} \Omega_d^b) (\Omega_{q,bi}^* D_{\bar{\mu}} \Omega_q^{ck}) \tilde{H}^{\dagger k} (\bar{u}_{cs} q_r^{ai}) \\
& - \frac{1}{36} \bar{y}_u^{tu} \left[ (\mathcal{C}_{quqd}^{(8)})^{sutr} - 6(\mathcal{C}_{quqd}^{(8)})^{tusr} \right] (\Omega_{q,a}^* D_{\bar{\mu}} \Omega_q^b) (\bar{q}_{bs} H D^{\bar{\mu}} d_r^a) \\
& - \frac{1}{36} \bar{y}_u^{tu} \left[ (\mathcal{C}_{quqd}^{(8)})^{sutr} - 6(\mathcal{C}_{quqd}^{(8)})^{tusr} \right] (\Omega_{u,a}^* D_{\bar{\mu}} \Omega_u^b) (\bar{q}_{bs} D_{\bar{\mu}} H d_r^a) \\
& - \frac{1}{36} \bar{y}_u^{tu} \left[ (\mathcal{C}_{quqd}^{(8)})^{sutr} - 6(\mathcal{C}_{quqd}^{(8)})^{tusr} \right] (\Omega_{q,a}^* D_{\bar{\mu}} \Omega_q^b) (D^{\bar{\mu}} \bar{q}_{bs} H d_r^a) \\
& - \frac{1}{36} \bar{y}_d^{rs} (\mathcal{C}_{quqd}^{(8)})^{rtus} (D_{\bar{\mu}} \Omega_{d,a}^* \Omega_d^b) (\bar{q}_{bu} \tilde{H} D^{\bar{\mu}} u_t^a) - \frac{1}{36} \bar{y}_d^{rs} (\mathcal{C}_{quqd}^{(8)})^{rtus} (D_{\bar{\mu}} \Omega_{d,a}^* \Omega_d^b) (\bar{q}_{bu} D_{\bar{\mu}} \tilde{H} u_t^a) \\
& - \frac{1}{36} \bar{y}_d^{rs} (\mathcal{C}_{quqd}^{(8)})^{rtus} (D_{\bar{\mu}} \Omega_{d,a}^* \Omega_d^b) (D^{\bar{\mu}} \bar{q}_{bu} \tilde{H} u_t^a) - \frac{1}{36} \bar{y}_u^{tu} \left[ (\mathcal{C}_{quqd}^{(8)})^{sutr} - 6(\mathcal{C}_{quqd}^{(8)})^{tusr} \right] (\Omega_{q,a}^* D_{\bar{\mu}} \Omega_q^b) (\Omega_{u,b}^* D_{\bar{\mu}} \Omega_u^c) (\bar{q}_{cs} H d_r^a) \\
& + \frac{i}{36} \bar{y}_u^{tu} (\mathcal{C}_{quqd}^{(8)})^{sutr} (\Omega_{q,a}^* D_{\bar{\mu}} \Omega_q^b) (\Omega_{u,b}^* D_{\bar{\nu}} \Omega_u^c) (\bar{q}_{cs} H \sigma^{\bar{\mu}\bar{\nu}} d_r^a) + \frac{1}{36} \bar{y}_d^{rs} (\mathcal{C}_{quqd}^{(8)})^{rtus} (D_{\bar{\mu}} \Omega_{d,a}^* \Omega_d^b) (D_{\bar{\mu}} \Omega_{q,b}^* \Omega_q^a) (\bar{q}_{cu} \tilde{H} u_t^b) \\
& + \frac{i}{36} \bar{y}_d^{rs} (\mathcal{C}_{quqd}^{(8)})^{rtus} (D_{\bar{\mu}} \Omega_{d,a}^* \Omega_d^c) (D_{\bar{\nu}} \Omega_{q,b}^* \Omega_q^a) (\bar{q}_{cu} \tilde{H} \sigma^{\bar{\mu}\bar{\nu}} u_t^b) \\
& - \frac{1}{36} \bar{y}_u^{tu} \left[ (\mathcal{C}_{quqd}^{(8)})^{sutr} - 6(\mathcal{C}_{quqd}^{(8)})^{tusr} \right] (D_{\bar{\mu}} \Omega_{q,ai}^* D_{\bar{\mu}} \Omega_q^{bj}) H^i (\bar{q}_{bjs} d_r^a) \\
& - \frac{1}{36} \bar{y}_u^{tu} \left[ (\mathcal{C}_{quqd}^{(8)})^{sutr} - 6(\mathcal{C}_{quqd}^{(8)})^{tusr} \right] (\Omega_{q,ai}^* D_{\bar{\mu}} \Omega_q^{bj}) D^{\bar{\mu}} H^i (\bar{q}_{bjs} d_r^a) \\
& - \frac{1}{36} \bar{y}_d^{rs} (\mathcal{C}_{quqd}^{(8)})^{rtus} \varepsilon^{kj} (D_{\bar{\mu}} \Omega_{q,aj}^* \Omega_q^{bi}) D^{\bar{\mu}} H_i^\dagger (\bar{q}_{bku} u_t^a) \\
& - \frac{i}{36} \bar{y}_u^{tu} (\mathcal{C}_{quqd}^{(8)})^{sutr} (\Omega_{q,ai}^* D_{\bar{\mu}} \Omega_q^{bj}) (\Omega_{u,b}^* D_{\bar{\nu}} \Omega_u^c) H^i (\bar{q}_{cjs} \sigma^{\bar{\mu}\bar{\nu}} d_r^a) - \frac{1}{36} y_d^{ru} (\bar{\mathcal{C}}_{quqd}^{(8)})^{rstu} \bar{\varepsilon}_{jk} (\Omega_{q,ai}^* D_{\bar{\mu}} \Omega_q^{bk}) D^{\bar{\mu}} H^i (\bar{u}_{bs} q_t^{aj}) \\
& - \frac{1}{36} y_d^{ru} (\bar{\mathcal{C}}_{quqd}^{(8)})^{rstu} (\Omega_{d,a}^* D_{\bar{\mu}} \Omega_d^b) (\bar{u}_{bs} \tilde{H}^\dagger D^{\bar{\mu}} q_t^a) - \frac{1}{36} y_d^{ru} (\bar{\mathcal{C}}_{quqd}^{(8)})^{rstu} (\Omega_{d,a}^* D_{\bar{\mu}} \Omega_d^b) (\bar{u}_{bs} D_{\bar{\mu}} \tilde{H}^\dagger q_t^a) \\
& - \frac{1}{36} y_d^{ru} (\bar{\mathcal{C}}_{quqd}^{(8)})^{rstu} (\Omega_{d,a}^* D_{\bar{\mu}} \Omega_d^b) (D^{\bar{\mu}} \bar{u}_{bs} \tilde{H}^\dagger q_t^a) - \frac{1}{36} y_d^{ru} (\bar{\mathcal{C}}_{quqd}^{(8)})^{rstu} (\Omega_{d,a}^* D_{\bar{\mu}} \Omega_d^b) (\Omega_{q,bi}^* D_{\bar{\mu}} \Omega_q^{ck}) \tilde{H}^{\dagger k} (\bar{u}_{cs} q_t^{ai}) \\
& - \frac{1}{18} \bar{y}_d^{rs} (\mathcal{C}_{quqd}^{(8)})^{turs} (D_{\bar{\mu}} \Omega_d^\dagger \Omega_d) (\bar{q}_t \tilde{H} D^{\bar{\mu}} u_u) - \frac{1}{18} \bar{y}_d^{rs} (\mathcal{C}_{quqd}^{(8)})^{turs} (D_{\bar{\mu}} \Omega_d^\dagger \Omega_d) (D^{\bar{\mu}} \bar{q}_t \tilde{H} u_u) \\
& + \frac{i}{18} \bar{y}_u^{tu} (\mathcal{C}_{quqd}^{(8)})^{sutr} (\Omega_{q,a}^* D_{\bar{\nu}} \Omega_u^b) (\bar{q}_{bs} D_{\bar{\mu}} H \sigma^{\bar{\mu}\bar{\nu}} d_r^a) + \frac{i}{18} \bar{y}_u^{tu} (\mathcal{C}_{quqd}^{(8)})^{sutr} (\Omega_{u,a}^* D_{\bar{\nu}} \Omega_u^b) (\bar{q}_{bs} D_{\bar{\mu}} H \sigma^{\bar{\mu}\bar{\nu}} d_r^a) \\
& + \frac{i}{18} \bar{y}_d^{rs} (\mathcal{C}_{quqd}^{(8)})^{rtus} (D_{\bar{\nu}} \Omega_{d,a}^* \Omega_d^b) (\bar{q}_{bu} D_{\bar{\mu}} \tilde{H} \sigma^{\bar{\mu}\bar{\nu}} u_t^a) + \frac{1}{18} \bar{y}_d^{rs} (\mathcal{C}_{quqd}^{(8)})^{turs} \varepsilon^{kj} (D_{\bar{\mu}} \Omega_{q,j}^* D_{\bar{\mu}} \Omega_q^i) H_i^\dagger (\bar{q}_{kt} u_u)
\end{aligned}$$

$$\begin{aligned}
& -\frac{1}{18}\bar{y}_d^{rs}(\mathcal{C}_{quqd}^{(8)})^{turs}\varepsilon^{kj}(D_{\bar{\mu}}\Omega_{q,j}^*\Omega_q^i)D^{\bar{\mu}}H_i^\dagger(\bar{q}_{kt}u_u) -\frac{1}{18}\bar{y}_d^{rs}(\mathcal{C}_{quqd}^{(8)})^{turs}(D_{\bar{\mu}}\Omega_{d,a}^*\Omega_d^b)(D_{\bar{\mu}}\Omega_{q,bj}^*\Omega_q^{ak})\tilde{H}_j(\bar{q}_{kt}u_u) \\
& -\frac{i}{18}\bar{y}_u^{tu}(\mathcal{C}_{quqd}^{(8)})^{sutr}(\Omega_{q,ai}^*D_{\bar{\nu}}\Omega_q^{bj})D^{\bar{\mu}}H^i(\bar{q}_{bjs}\sigma^{\bar{\mu}\bar{\nu}}d_r^a) -\frac{i}{18}\bar{y}_d^{rs}(\mathcal{C}_{quqd}^{(8)})^{rtus}\varepsilon^{kj}(D_{\bar{\nu}}\Omega_{q,aj}^*\Omega_q^{bi})D^{\bar{\mu}}H_i^\dagger(\bar{q}_{bku}\sigma^{\bar{\mu}\bar{\nu}}u_t^a) \\
& -\frac{i}{12}\bar{y}_u^{tu}(\mathcal{C}_{quqd}^{(8)})^{sutr}(\Omega_{q,a}^*D_{\bar{\mu}}\Omega_q^b)(\Omega_{u,b}^*D_{\bar{\nu}}\Omega_u^a)(\bar{q}_sH\sigma^{\bar{\mu}\bar{\nu}}d_r) +\frac{1}{6}\bar{y}_d^{rs}(\mathcal{C}_{quqd}^{(8)})^{turs}\varepsilon^{kj}(D_{\bar{\mu}}\Omega_{q,aj}^*\Omega_q^{bi})D^{\bar{\mu}}H_i^\dagger(\bar{q}_{bkt}u_u^a) \\
& +\frac{1}{6}\bar{y}_d^{rs}(\mathcal{C}_{quqd}^{(8)})^{turs}(D_{\bar{\mu}}\Omega_{d,a}^*\Omega_d^c)(D_{\bar{\mu}}\Omega_{q,bj}^*\Omega_q^{ak})\tilde{H}_j(\bar{q}_{ckt}u_u^b) -\frac{1}{36}\bar{y}_d^{rs}(\mathcal{C}_{quqd}^{(8)})^{rtus}(D_{\bar{\mu}}\Omega_{d,a}^*\Omega_d^c)(D_{\bar{\mu}}\Omega_{q,bj}^*\Omega_q^{ak})\tilde{H}_j(\bar{q}_{cku}u_t^b) \\
& -\frac{i}{36}\bar{y}_d^{rs}(\mathcal{C}_{quqd}^{(8)})^{rtus}(D_{\bar{\mu}}\Omega_{d,a}^*\Omega_d^c)(D_{\bar{\nu}}\Omega_{q,bj}^*\Omega_q^{ak})\tilde{H}_j(\bar{q}_{cku}\sigma^{\bar{\mu}\bar{\nu}}u_t^b) +\frac{1}{18}y_d^{tu}(\bar{\mathcal{C}}_{quqd}^{(8)})^{rstu}\bar{\varepsilon}_{jk}(D_{\bar{\mu}}\Omega_{q,i}^*D_{\bar{\mu}}\Omega_q^k)H^i(\bar{u}_sq_r^j) \\
& +\frac{1}{18}y_d^{tu}(\bar{\mathcal{C}}_{quqd}^{(8)})^{rstu}\bar{\varepsilon}_{jk}(\Omega_{q,i}^*D_{\bar{\mu}}\Omega_q^k)H^i(\bar{u}_sD^{\bar{\mu}}q_r^j) +\frac{1}{12}y_d^{ru}(\bar{\mathcal{C}}_{quqd}^{(8)})^{rstu}(\Omega_{d,a}^*D_{\bar{\mu}}\Omega_d^b)(\Omega_{q,bi}^*D_{\bar{\mu}}\Omega_q^{ak})\tilde{H}^{\dagger k}(\bar{u}_sq_t^i) \\
& -\frac{1}{18}y_d^{tu}(\bar{\mathcal{C}}_{quqd}^{(8)})^{rstu}(\Omega_{d,a}^*D_{\bar{\mu}}\Omega_d^b)(\Omega_{q,bi}^*D_{\bar{\mu}}\Omega_q^{ak})\tilde{H}^{\dagger k}(\bar{u}_sq_r^i) -\frac{1}{18}y_d^{tu}(\bar{\mathcal{C}}_{quqd}^{(8)})^{rstu}\bar{\varepsilon}_{jk}(\Omega_{q,i}^*D_{\bar{\mu}}\Omega_q^k)D^{\bar{\mu}}H^i(\bar{u}_sq_r^j) \\
& -\frac{1}{18}y_d^{tu}(\bar{\mathcal{C}}_{quqd}^{(8)})^{rstu}(\Omega_d^\dagger D_{\bar{\mu}}\Omega_d)(\bar{u}_s\tilde{H}^\dagger D^{\bar{\mu}}q_r) -\frac{1}{18}y_d^{tu}(\bar{\mathcal{C}}_{quqd}^{(8)})^{rstu}(\Omega_d^\dagger D_{\bar{\mu}}\Omega_d)(D^{\bar{\mu}}\bar{u}_s\tilde{H}^\dagger q_r) \\
& +\frac{i}{18}y_d^{ru}(\bar{\mathcal{C}}_{quqd}^{(8)})^{rstu}\bar{\varepsilon}_{jk}(\Omega_{q,ai}^*D_{\bar{\nu}}\Omega_q^{bk})D^{\bar{\mu}}H^i(\bar{u}_{bs}\sigma^{\bar{\mu}\bar{\nu}}q_t^a) -\frac{1}{12}\bar{y}_d^{rs}(\mathcal{C}_{quqd}^{(8)})^{rtus}(D_{\bar{\mu}}\Omega_d^\dagger D_{\bar{\mu}}\Omega_d)(\bar{q}_u\tilde{H}u_t) \\
& -\frac{1}{12}\bar{y}_d^{rs}(\mathcal{C}_{quqd}^{(8)})^{rtus}(D_{\bar{\mu}}\Omega_{d,a}^*\Omega_d^b)(D_{\bar{\mu}}\Omega_{q,b}^*\Omega_q^a)(\bar{q}_u\tilde{H}u_t) -\frac{1}{12}\bar{y}_d^{rs}(\mathcal{C}_{quqd}^{(8)})^{rtus}(D_{\bar{\mu}}\Omega_d^\dagger \Omega_d)(\bar{q}_u D_{\bar{\mu}}\tilde{H}u_t) \\
& -\frac{i}{12}\bar{y}_d^{rs}(\mathcal{C}_{quqd}^{(8)})^{rtus}(D_{\bar{\mu}}\Omega_{d,a}^*\Omega_d^b)(D_{\bar{\nu}}\Omega_{q,b}^*\Omega_q^a)(\bar{q}_u\tilde{H}\sigma^{\bar{\mu}\bar{\nu}}u_t) +\frac{i}{12}\bar{y}_u^{tu}(\mathcal{C}_{quqd}^{(8)})^{sutr}(\Omega_{q,ai}^*D_{\bar{\mu}}\Omega_q^{bj})(\Omega_{u,b}^*D_{\bar{\nu}}\Omega_u^a)H^i(\bar{q}_{js}\sigma^{\bar{\mu}\bar{\nu}}d_r) \\
& -\frac{1}{12}\bar{y}_d^{rs}(\mathcal{C}_{quqd}^{(8)})^{rtus}\varepsilon^{kj}(D_{\bar{\mu}}\Omega_{q,j}^*D_{\bar{\mu}}\Omega_q^i)H_i^\dagger(\bar{q}_{ku}u_t) -\frac{1}{12}\bar{y}_d^{rs}(\mathcal{C}_{quqd}^{(8)})^{rtus}\varepsilon^{kj}(D_{\bar{\mu}}\Omega_{q,j}^*\Omega_q^i)H_i^\dagger(\bar{q}_{ku}D^{\bar{\mu}}u_t) \\
& +\frac{i}{12}\bar{y}_d^{rs}(\mathcal{C}_{quqd}^{(8)})^{rtus}(D_{\bar{\mu}}\Omega_{d,a}^*\Omega_d^b)(D_{\bar{\nu}}\Omega_{q,bj}^*\Omega_q^{ak})\tilde{H}_j(\bar{q}_{ku}\sigma^{\bar{\mu}\bar{\nu}}u_t) -\frac{1}{12}\bar{y}_d^{rs}(\mathcal{C}_{quqd}^{(8)})^{rtus}\varepsilon^{kj}(D_{\bar{\mu}}\Omega_{q,j}^*\Omega_q^i)H_i^\dagger(D^{\bar{\mu}}\bar{q}_{ku}u_t) \\
& -\frac{1}{12}y_d^{ru}(\bar{\mathcal{C}}_{quqd}^{(8)})^{rstu}\bar{\varepsilon}_{jk}(D_{\bar{\mu}}\Omega_{q,i}^*D_{\bar{\mu}}\Omega_q^k)H^i(\bar{u}_sq_t^j) -\frac{1}{12}y_d^{ru}(\bar{\mathcal{C}}_{quqd}^{(8)})^{rstu}\bar{\varepsilon}_{jk}(\Omega_{q,i}^*D_{\bar{\mu}}\Omega_q^k)H^i(\bar{u}_sD^{\bar{\mu}}q_t^j) \\
& -\frac{1}{12}y_d^{ru}(\bar{\mathcal{C}}_{quqd}^{(8)})^{rstu}(D_{\bar{\mu}}\Omega_d^\dagger D_{\bar{\mu}}\Omega_d)(\bar{u}_s\tilde{H}^\dagger q_t) -\frac{1}{12}y_d^{ru}(\bar{\mathcal{C}}_{quqd}^{(8)})^{rstu}(\Omega_{d,a}^*D_{\bar{\mu}}\Omega_d^b)(\Omega_{q,b}^*D_{\bar{\mu}}\Omega_q^a)(\bar{u}_s\tilde{H}^\dagger q_t) \\
& -\frac{1}{12}y_d^{ru}(\bar{\mathcal{C}}_{quqd}^{(8)})^{rstu}(\Omega_d^\dagger D_{\bar{\mu}}\Omega_d)(\bar{u}_sD_{\bar{\mu}}\tilde{H}^\dagger q_t) -\frac{i}{12}y_d^{ru}(\bar{\mathcal{C}}_{quqd}^{(8)})^{rstu}(\Omega_{d,a}^*D_{\bar{\mu}}\Omega_d^b)(\Omega_{q,bi}^*D_{\bar{\nu}}\Omega_q^{ak})\tilde{H}^{\dagger k}(\bar{u}_s\sigma^{\bar{\mu}\bar{\nu}}q_t^i) \\
& +\frac{i}{12}y_d^{ru}(\bar{\mathcal{C}}_{quqd}^{(8)})^{rstu}(\Omega_{d,a}^*D_{\bar{\mu}}\Omega_d^b)(\Omega_{q,b}^*D_{\bar{\nu}}\Omega_q^a)(\bar{u}_s\sigma^{\bar{\mu}\bar{\nu}}\tilde{H}^\dagger q_t) -\frac{1}{12}y_d^{ru}(\bar{\mathcal{C}}_{quqd}^{(8)})^{rstu}\bar{\varepsilon}_{jk}(\Omega_{q,i}^*D_{\bar{\mu}}\Omega_q^k)H^i(D^{\bar{\mu}}\bar{u}_sq_t^j) \\
& -\frac{i}{6}\bar{y}_u^{tu}(\mathcal{C}_{quqd}^{(8)})^{sutr}(\Omega_q^\dagger D_{\bar{\nu}}\Omega_q)(\bar{q}_sD_{\bar{\mu}}H\sigma^{\bar{\mu}\bar{\nu}}d_r) -\frac{i}{6}\bar{y}_u^{tu}(\mathcal{C}_{quqd}^{(8)})^{sutr}(\Omega_u^\dagger D_{\bar{\nu}}\Omega_u)(\bar{q}_sD_{\bar{\mu}}H\sigma^{\bar{\mu}\bar{\nu}}d_r) \\
& -\frac{i}{6}\bar{y}_d^{rs}(\mathcal{C}_{quqd}^{(8)})^{rtus}(D_{\bar{\nu}}\Omega_d^\dagger \Omega_d)(\bar{q}_u D_{\bar{\mu}}\tilde{H}\sigma^{\bar{\mu}\bar{\nu}}u_t) +\frac{i}{6}\bar{y}_u^{tu}(\mathcal{C}_{quqd}^{(8)})^{sutr}(\Omega_{q,i}^*D_{\bar{\nu}}\Omega_q^j)D^{\bar{\mu}}H^i(\bar{q}_{js}\sigma^{\bar{\mu}\bar{\nu}}d_r) \\
& -\frac{1}{6}\bar{y}_d^{rs}(\mathcal{C}_{quqd}^{(8)})^{turs}(D_{\bar{\mu}}\Omega_{d,a}^*D_{\bar{\mu}}\Omega_d^b)(\bar{q}_{bt}\tilde{H}u_u^a) +\frac{i}{6}\bar{y}_d^{rs}(\mathcal{C}_{quqd}^{(8)})^{rtus}\varepsilon^{kj}(D_{\bar{\nu}}\Omega_{q,j}^*\Omega_q^i)D^{\bar{\mu}}H_i^\dagger(\bar{q}_{ku}\sigma^{\bar{\mu}\bar{\nu}}u_t) \\
& -\frac{1}{6}\bar{y}_d^{rs}(\mathcal{C}_{quqd}^{(8)})^{turs}(D_{\bar{\mu}}\Omega_{d,a}^*\Omega_d^c)(D_{\bar{\mu}}\Omega_{q,b}^*\Omega_q^a)(\bar{q}_{ct}\tilde{H}u_u^b) -\frac{1}{6}\bar{y}_d^{rs}(\mathcal{C}_{quqd}^{(8)})^{turs}\varepsilon^{kj}(D_{\bar{\mu}}\Omega_{q,aj}^*D_{\bar{\mu}}\Omega_q^{bi})H_i^\dagger(\bar{q}_{bkt}u_u^a) \\
& -\frac{1}{6}\bar{y}_d^{rs}(\mathcal{C}_{quqd}^{(8)})^{turs}\varepsilon^{kj}(D_{\bar{\mu}}\Omega_{q,aj}^*\Omega_q^{bi})H_i^\dagger(\bar{q}_{bkt}D^{\bar{\mu}}u_u^a) -\frac{1}{6}\bar{y}_d^{rs}(\mathcal{C}_{quqd}^{(8)})^{turs}\varepsilon^{kj}(D_{\bar{\mu}}\Omega_{q,aj}^*\Omega_q^{bi})H_i^\dagger(D^{\bar{\mu}}\bar{q}_{bkt}u_u^a) \\
& -\frac{i}{6}y_d^{ru}(\bar{\mathcal{C}}_{quqd}^{(8)})^{rstu}\bar{\varepsilon}_{jk}(\Omega_{q,i}^*D_{\bar{\nu}}\Omega_q^k)D^{\bar{\mu}}H^i(\bar{u}_s\sigma^{\bar{\mu}\bar{\nu}}q_t^j) +\frac{i}{6}y_d^{ru}(\bar{\mathcal{C}}_{quqd}^{(8)})^{rstu}(\Omega_d^\dagger D_{\bar{\nu}}\Omega_d)(\bar{u}_s\sigma^{\bar{\mu}\bar{\nu}}D_{\bar{\mu}}\tilde{H}^\dagger q_t)
\end{aligned}$$

$$\begin{aligned}
& -\frac{1}{6}y_d^{tu}(\bar{C}_{quqd}^{(8)})^{rstu}\bar{\varepsilon}_{jk}(D_{\bar{\mu}}\Omega_{q,ai}^*D_{\bar{\mu}}\Omega_q^{bk})H^i(\bar{u}_{bs}q_r^{aj}) - \frac{1}{6}y_d^{tu}(\bar{C}_{quqd}^{(8)})^{rstu}\bar{\varepsilon}_{jk}(\Omega_{q,ai}^*D_{\bar{\mu}}\Omega_q^{bk})H^i(\bar{u}_{bs}D^{\bar{\mu}}q_r^{aj}) \\
& -\frac{1}{6}y_d^{tu}(\bar{C}_{quqd}^{(8)})^{rstu}(D_{\bar{\mu}}\Omega_{d,a}^*D_{\bar{\mu}}\Omega_d^b)(\bar{u}_{bs}\tilde{H}^\dagger q_r^a) - \frac{1}{6}y_d^{tu}(\bar{C}_{quqd}^{(8)})^{rstu}\bar{\varepsilon}_{jk}(\Omega_{q,ai}^*D_{\bar{\mu}}\Omega_q^{bk})H^i(D^{\bar{\mu}}\bar{u}_{bs}q_r^{aj}) \\
& -\frac{1}{6}y_d^{tu}(\bar{C}_{quqd}^{(8)})^{rstu}(\Omega_{d,a}^*D_{\bar{\mu}}\Omega_d^b)(\Omega_{q,b}^*D_{\bar{\mu}}\Omega_q^c)(\bar{u}_{cs}\tilde{H}^\dagger q_r^a). \tag{3.62}
\end{aligned}$$

## References

- [1] B. Grzadkowski, M. Iskrzynski, M. Misiak and J. Rosiek, *Dimension-Six Terms in the Standard Model Lagrangian*, *JHEP* **10** (2010), 085 [1008.4884].
